# Supplementary material for: Estimating $T_{\rm eff}$, radius and luminosity of M-dwarfs using high resolution optical and NIR spectral features
Source: arXiv:2107.14023 source file (2021-07-29)
Supplement: Supplementary file 1 [file table4_online_supplimentary.pdf]

**Table 4 : Linear test functions using simple functional forms of the selected EWs and EW ratios (x = $EW_{Ca[0.854\mu m]}$ ; y = $EW_{Ca[0.866\mu m]}$ ; z = $EW_{Mg[1.574\mu m]}$) and associated RMSE, MAD and $R^2{}_{ap}$ values of the stellar parameters.**

| Functional form | $T_{eff}$ (K) | | | Radius ($R_\odot$) | | | log (L/$L_\odot$) | | |
|---|---|---|---|---|---|---|---|---|---|
| | RMSE | MAD | $R^2_{ap}$ | RMSE | MAD | $R^2_{ap}$ | RMSE | MAD | $R^2_{ap}$ |
| Single line EW, single component functions result ( x ; y ; z) | | | | | | | | | |
| a+bx | 147.15 | 111.90 | 0.737 | 0.0816 | 0.0617 | 0.6715 | 0.2525 | 0.1744 | 0.730 |
| a+b$x^2$ | 123.94 | 98.73 | 0.813 | 0.0760 | 0.0533 | 0.7147 | 0.2483 | 0.1790 | 0.739 |
| a+b$\sqrt{x}$ | 180.84 | 134.72 | 0.602 | 0.0926 | 0.0739 | 0.5762 | 0.2900 | 0.2108 | 0.644 |
| a+b/x | 271.46 | 207.10 | 0.103 | 0.1292 | 0.1060 | 0.1753 | 0.4343 | 0.3433 | 0.201 |
| a+b/$x^2$ | 283.83 | 213.59 | 0.020 | 0.1356 | 0.1092 | 0.0926 | 0.4607 | 0.3606 | 0.101 |
| a+b/$\sqrt{x}$ | 253.33 | 194.31 | 0.219 | 0.1210 | 0.0990 | 0.2770 | 0.4006 | 0.3138 | 0.320 |
| a+by | 172.40 | 140.07 | 0.638 | 0.0958 | 0.0710 | 0.5470 | 0.3108 | 0.2158 | 0.591 |
| a+b$y^2$ | 162.79 | 133.16 | 0.678 | 0.0944 | 0.0674 | 0.5597 | 0.3156 | 0.2206 | 0.578 |
| a+b$\sqrt{y}$ | 183.85 | 144.62 | 0.589 | 0.0989 | 0.0765 | 0.5169 | 0.3176 | 0.2251 | 0.573 |
| a+b/y | 228.76 | 172.91 | 0.363 | 0.1146 | 0.0922 | 0.3513 | 0.3697 | 0.2822 | 0.421 |
| a+b/$y^2$ | 248.05 | 188.15 | 0.251 | 0.1223 | 0.0977 | 0.2613 | 0.3990 | 0.3032 | 0.326 |
| a+b/$\sqrt{y}$ | 214.62 | 162.25 | 0.440 | 0.1093 | 0.0868 | 0.4103 | 0.3505 | 0.2651 | 0.480 |
| a+bz | 137.18 | 108.68 | 0.771 | 0.0764 | 0.0549 | 0.7116 | 0.2819 | 0.2162 | 0.663 |
| a+b$z^2$ | 153.91 | 121.54 | 0.712 | 0.0821 | 0.0627 | 0.6669 | 0.3083 | 0.2445 | 0.597 |
| a+b$\sqrt{z}$ | 134.10 | 107.82 | 0.781 | 0.0772 | 0.0514 | 0.7057 | 0.2766 | 0.1962 | 0.676 |
| a+b/z | 179.29 | 124.76 | 0.609 | 0.1024 | 0.0745 | 0.4822 | 0.3406 | 0.2332 | 0.508 |
| a+b/$z^2$ | 224.39 | 167.83 | 0.387 | 0.1219 | 0.0971 | 0.2660 | 0.4070 | 0.3074 | 0.298 |
| a+b/$\sqrt{z}$ | 156.22 | 111.48 | 0.703 | 0.0913 | 0.0631 | 0.5883 | 0.3072 | 0.2026 | 0.600 |
| Single line EW, double component functions result ( x ; y ; z) | | | | | | | | | |
| a+bx+c$x^2$ | 126.75 | 98.000 | 0.805 | 0.0778 | 0.0530 | 0.7013 | 0.2491 | 0.1706 | 0.737 |
| a+bx+c$\sqrt{x}$ | 119.51 | 89.460 | 0.826 | 0.0778 | 0.0527 | 0.7010 | 0.2453 | 0.1637 | 0.745 |
| a+bx+c/x | 114.40 | 81.570 | 0.841 | 0.0794 | 0.0548 | 0.6887 | 0.2436 | 0.1571 | 0.749 |
| a+bx+c/$x^2$ | 116.07 | 86.100 | 0.836 | 0.0804 | 0.0559 | 0.6812 | 0.2447 | 0.1581 | 0.746 |
| a+bx+c/$\sqrt{x}$ | 114.75 | 82.410 | 0.840 | 0.0788 | 0.0539 | 0.6937 | 0.2435 | 0.1563 | 0.749 |
| a+by+c$y^2$ | 166.72 | 132.76 | 0.662 | 0.0965 | 0.0663 | 0.5399 | 0.3176 | 0.2147 | 0.573 |
| a+by+c$\sqrt{y}$ | 168.04 | 133.95 | 0.656 | 0.0969 | 0.0668 | 0.5360 | 0.3179 | 0.2156 | 0.572 |
| a+by+c/y | 168.52 | 134.39 | 0.654 | 0.0972 | 0.0671 | 0.5339 | 0.3180 | 0.2159 | 0.572 |
| a+by+c/$y^2$ | 168.40 | 134.09 | 0.655 | 0.0972 | 0.0673 | 0.5333 | 0.3179 | 0.2158 | 0.572 |
| a+by+c/$\sqrt{y}$ | 168.46 | 134.38 | 0.655 | 0.0971 | 0.0670 | 0.5344 | 0.3180 | 0.2158 | 0.572 |
| a+bz+c$z^2$ | 138.66 | 109.38 | 0.766 | 0.0780 | 0.0529 | 0.6993 | 0.2827 | 0.1949 | 0.661 |
| a+bz+c$\sqrt{z}$ | 137.36 | 107.80 | 0.770 | 0.0782 | 0.0538 | 0.6980 | 0.2835 | 0.1955 | 0.660 |
| a+bz+c/z | 138.17 | 107.38 | 0.768 | 0.0783 | 0.0552 | 0.6974 | 0.2870 | 0.2068 | 0.651 |
| a+bz+c/$z^2$ | 139.50 | 108.38 | 0.763 | 0.0780 | 0.0555 | 0.6994 | 0.2887 | 0.2143 | 0.647 |
| a+bz+c/$\sqrt{z}$ | 137.62 | 107.27 | 0.770 | 0.0783 | 0.0548 | 0.6972 | 0.2857 | 0.2021 | 0.654 |
| a+b$x^2$+c$\sqrt{x}$ | 126.23 | 96.98 | 0.806 | 0.0061 | 0.0778 | 0.3966 | 0.2505 | 0.1738 | 0.734 |
| a+b$x^2$+c/x | 122.01 | 91.34 | 0.819 | 0.0061 | 0.0779 | 0.3966 | 0.2539 | 0.1796 | 0.727 |
| a+b$x^2$+c/$x^2$ | 119.87 | 88.26 | 0.825 | 0.0061 | 0.0779 | 0.3966 | 0.2543 | 0.1794 | 0.726 |
| a+b$x^2$+c/$\sqrt{x}$ | 123.64 | 93.61 | 0.814 | 0.0061 | 0.0779 | 0.3966 | 0.2531 | 0.1788 | 0.728 |
| a+b$y^2$+c$\sqrt{y}$ | 166.76 | 132.86 | 0.662 | 0.0093 | 0.0965 | 0.3966 | 0.3172 | 0.2139 | 0.574 |
| a+b$y^2$+c/y | 166.78 | 132.92 | 0.662 | 0.0093 | 0.0964 | 0.3966 | 0.3171 | 0.2125 | 0.574 |
| a+b$y^2$+c/$y^2$ | 166.75 | 132.81 | 0.662 | 0.0093 | 0.0964 | 0.3966 | 0.3176 | 0.2124 | 0.573 |
| a+b$y^2$+c/$\sqrt{y}$ | 166.78 | 132.94 | 0.662 | 0.0093 | 0.0964 | 0.3966 | 0.3170 | 0.2128 | 0.574 |
| a+b$z^2$+c$\sqrt{z}$ | 137.22 | 107.44 | 0.771 | 0.0062 | 0.0785 | 0.3966 | 0.2834 | 0.1943 | 0.660 |
| a+b$z^2$+c/z | 139.60 | 106.24 | 0.763 | 0.0066 | 0.0810 | 0.3966 | 0.2947 | 0.2114 | 0.632 |
| a+b$z^2$+c/$z^2$ | 145.30 | 112.08 | 0.743 | 0.0068 | 0.0827 | 0.3966 | 0.3046 | 0.2273 | 0.607 |
| a+b$z^2$+c/$\sqrt{z}$ | 137.60 | 104.82 | 0.770 | 0.0064 | 0.0800 | 0.3966 | 0.2897 | 0.2033 | 0.644 |
| a+b$\sqrt{x}$+c/x | 120.64 | 90.05 | 0.823 | 0.0836 | 0.0602 | 0.6553 | 0.2499 | 0.1668 | 0.735 |
| a+b$\sqrt{x}$+c/$x^2$ | 129.39 | 97.68 | 0.796 | 0.0863 | 0.0635 | 0.6322 | 0.2574 | 0.1751 | 0.719 |
| a+b$\sqrt{x}$+c/$\sqrt{x}$ | 116.41 | 85.01 | 0.835 | 0.0816 | 0.0577 | 0.6713 | 0.2458 | 0.1610 | 0.744 |
| a+b$\sqrt{y}$+c/y | 169.41 | 134.91 | 0.651 | 0.0976 | 0.0680 | 0.5297 | 0.3184 | 0.2169 | 0.570 |
| a+b$\sqrt{y}$+c/$y^2$ | 169.36 | 134.40 | 0.651 | 0.0978 | 0.0684 | 0.5282 | 0.3182 | 0.2167 | 0.571 |
| a+b$\sqrt{y}$+c/$\sqrt{y}$ | 169.25 | 134.94 | 0.651 | 0.0975 | 0.0677 | 0.5308 | 0.3184 | 0.2168 | 0.570 |
| a+b$\sqrt{z}$+c/z | 137.24 | 107.90 | 0.771 | 0.0770 | 0.0533 | 0.7074 | 0.2825 | 0.2019 | 0.662 |
| a+b$\sqrt{z}$+c/$z^2$ | 136.73 | 107.52 | 0.773 | 0.0760 | 0.0522 | 0.7145 | 0.2802 | 0.2033 | 0.667 |
| a+b$\sqrt{z}$+c/$\sqrt{z}$ | 137.34 | 107.91 | 0.771 | 0.0774 | 0.0537 | 0.7042 | 0.2831 | 0.2001 | 0.660 |
| a+b/x+c/$x^2$ | 211.92 | 154.88 | 0.454 | 0.1152 | 0.0902 | 0.3442 | 0.3611 | 0.2662 | 0.447 |
| a+b/x+c/$\sqrt{x}$ | 162.04 | 120.58 | 0.681 | 0.0990 | 0.0771 | 0.5159 | 0.2979 | 0.2164 | 0.624 |
| a+b/y+c/$y^2$ | 172.29 | 132.72 | 0.639 | 0.0997 | 0.0713 | 0.5094 | 0.3196 | 0.2147 | 0.567 |
| a+b/y+c/$\sqrt{y}$ | 170.99 | 134.97 | 0.644 | 0.0985 | 0.0695 | 0.5212 | 0.3191 | 0.2175 | 0.569 |
| a+b/z+c/$z^2$ | 131.68 | 99.58 | 0.789 | 0.0740 | 0.0439 | 0.7297 | 0.2588 | 0.1701 | 0.716 |
| a+b/z+c/$\sqrt{z}$ | 135.08 | 106.17 | 0.778 | 0.0750 | 0.0488 | 0.7226 | 0.2725 | 0.1892 | 0.685 |
| a+b/$x^2$+c/$\sqrt{x}$ | 186.22 | 135.79 | 0.578 | 0.1065 | 0.0835 | 0.4400 | 0.3266 | 0.2387 | 0.548 |
| a+b/$y^2$+c/$\sqrt{y}$ | 171.34 | 133.72 | 0.643 | 0.0990 | 0.0704 | 0.5162 | 0.3191 | 0.2161 | 0.569 |
| a+b/$z^2$+c/$\sqrt{z}$ | 132.66 | 102.98 | 0.786 | 0.0739 | 0.0462 | 0.7302 | 0.2647 | 0.1801 | 0.703 |
| Different double line EWs, double component functions result ( (x,y) ; (x,z) ; (y,z) ) | | | | | | | | | |
| a+bx+cy | 150.66 | 112.24 | 0.724 | 0.0826 | 0.0618 | 0.6629 | 0.2541 | 0.1745 | 0.726 |
| a+bx+c$y^2$ | 147.09 | 112.92 | 0.737 | 0.0835 | 0.0616 | 0.6555 | 0.2585 | 0.1748 | 0.717 |
| a+bx+c$\sqrt{y}$ | 146.58 | 113.81 | 0.739 | 0.0805 | 0.0593 | 0.6799 | 0.2491 | 0.1724 | 0.737 |
| a+bx+c/y | 129.87 | 102.80 | 0.795 | 0.0776 | 0.0525 | 0.7030 | 0.2452 | 0.1679 | 0.745 |
| a+bx+c/$y^2$ | 127.22 | 97.68 | 0.803 | 0.0778 | 0.0515 | 0.7013 | 0.2457 | 0.1661 | 0.744 |
| a+bx+c/$\sqrt{y}$ | 133.02 | 107.47 | 0.785 | 0.0777 | 0.0532 | 0.7022 | 0.2449 | 0.1694 | 0.746 |
| a+b$x^2$+cy | 126.53 | 100.01 | 0.805 | 0.0775 | 0.0544 | 0.7037 | 0.2543 | 0.1803 | 0.726 |
| a+b$x^2$+c$y^2$ | 126.63 | 100.88 | 0.805 | 0.0767 | 0.0545 | 0.7093 | 0.2500 | 0.1814 | 0.735 |
| a+b$x^2$+c$\sqrt{y}$ | 126.55 | 99.33 | 0.805 | 0.0777 | 0.0542 | 0.7016 | 0.2543 | 0.1781 | 0.726 |
| a+b$x^2$+c/y | 126.53 | 97.98 | 0.805 | 0.0779 | 0.0531 | 0.7005 | 0.2522 | 0.1751 | 0.730 |
| a+b$x^2$+c/$y^2$ | 126.40 | 97.39 | 0.806 | 0.0779 | 0.0529 | 0.7007 | 0.2519 | 0.1751 | 0.731 |
| a+b$x^2$+c/$\sqrt{y}$ | 126.56 | 98.33 | 0.805 | 0.0779 | 0.0534 | 0.7005 | 0.2527 | 0.1757 | 0.729 |
| a+b$\sqrt{x}$+cy | 173.94 | 133.91 | 0.632 | 0.0937 | 0.0725 | 0.5669 | 0.2946 | 0.2081 | 0.632 |
| a+b$\sqrt{x}$+c$y^2$ | 160.70 | 127.55 | 0.686 | 0.0902 | 0.0674 | 0.5979 | 0.2868 | 0.1962 | 0.652 |
| a+b$\sqrt{x}$+c$\sqrt{y}$ | 182.86 | 136.71 | 0.593 | 0.0949 | 0.0739 | 0.5550 | 0.2971 | 0.2104 | 0.626 |
| a+b$\sqrt{x}$+c/y | 155.73 | 120.64 | 0.705 | 0.0823 | 0.0605 | 0.6657 | 0.2612 | 0.1848 | 0.711 |

(continued on next page)

**Table 4 – continued from previous page**

| Functional form | $T_{eff}$ (K) | | | Radius ($R_\odot$) | | | log (L/$L_\odot$) | | |
|---|---|---|---|---|---|---|---|---|---|
| | RMSE | MAD | $R^2_{ap}$ | RMSE | MAD | $R^2_{ap}$ | RMSE | MAD | $R^2_{ap}$ |
| $a+b\sqrt{x}+c/y^2$ | 142.12 | 107.88 | 0.754 | 0.0800 | 0.0559 | 0.6843 | 0.2537 | 0.1731 | 0.727 |
| $a+b\sqrt{x}+c/\sqrt{y}$ | 170.31 | 127.55 | 0.647 | 0.0865 | 0.0663 | 0.6306 | 0.2730 | 0.1992 | 0.684 |
| $a+b/x+cy$ | 164.88 | 126.33 | 0.669 | 0.0978 | 0.0689 | 0.5273 | 0.3178 | 0.2130 | 0.572 |
| $a+b/x+cy^2$ | 165.15 | 128.85 | 0.668 | 0.0963 | 0.0668 | 0.5421 | 0.3204 | 0.2177 | 0.565 |
| $a+b/x+c\sqrt{y}$ | 168.54 | 129.59 | 0.654 | 0.1000 | 0.0727 | 0.5064 | 0.3204 | 0.2161 | 0.565 |
| $a+b/x+c/y$ | 211.34 | 155.65 | 0.457 | 0.1152 | 0.0885 | 0.3453 | 0.3656 | 0.2677 | 0.434 |
| $a+b/x+c/y^2$ | 243.99 | 176.13 | 0.276 | 0.1249 | 0.0975 | 0.2292 | 0.4043 | 0.2995 | 0.307 |
| $a+b/x+c/\sqrt{y}$ | 192.43 | 145.98 | 0.549 | 0.1090 | 0.0831 | 0.4133 | 0.3445 | 0.2436 | 0.497 |
| $a+b/x^2+cy$ | 162.48 | 122.95 | 0.679 | 0.0977 | 0.0691 | 0.5282 | 0.3168 | 0.2096 | 0.575 |
| $a+b/x^2+cy^2$ | 163.09 | 124.83 | 0.676 | 0.0966 | 0.0667 | 0.5396 | 0.3225 | 0.2179 | 0.559 |
| $a+b/x^2+c\sqrt{y}$ | 167.27 | 130.26 | 0.660 | 0.1000 | 0.0734 | 0.5061 | 0.3192 | 0.2162 | 0.568 |
| $a+b/x^2+c/y$ | 210.24 | 155.47 | 0.462 | 0.1150 | 0.0887 | 0.3474 | 0.3641 | 0.2682 | 0.438 |
| $a+b/x^2+c/y^2$ | 238.36 | 172.43 | 0.309 | 0.1241 | 0.0968 | 0.2396 | 0.3993 | 0.2959 | 0.324 |
| $a+b/x^2+c/\sqrt{y}$ | 192.94 | 144.82 | 0.547 | 0.1092 | 0.0836 | 0.4112 | 0.3441 | 0.2459 | 0.498 |
| $a+b/\sqrt{x}+cy$ | 169.07 | 132.43 | 0.652 | 0.0981 | 0.0699 | 0.5250 | 0.3185 | 0.2158 | 0.570 |
| $a+b/\sqrt{x}+cy^2$ | 166.54 | 132.05 | 0.663 | 0.0957 | 0.0669 | 0.5474 | 0.3164 | 0.2160 | 0.576 |
| $a+b/\sqrt{x}+c\sqrt{y}$ | 173.93 | 134.03 | 0.632 | 0.1006 | 0.0734 | 0.5004 | 0.3234 | 0.2202 | 0.557 |
| $a+b/\sqrt{x}+c/y$ | 223.77 | 165.58 | 0.391 | 0.1171 | 0.0914 | 0.3228 | 0.3756 | 0.2797 | 0.402 |
| $a+b/\sqrt{x}+c/y^2$ | 254.15 | 187.74 | 0.214 | 0.1238 | 0.0983 | 0.2430 | 0.4068 | 0.3074 | 0.299 |
| $a+b/\sqrt{x}+c/\sqrt{y}$ | 201.68 | 152.66 | 0.505 | 0.1106 | 0.0843 | 0.3958 | 0.3522 | 0.2531 | 0.474 |
| $a+bx+cz$ | 114.20 | 85.69 | 0.841 | 0.0685 | 0.0408 | 0.7686 | 0.2296 | 0.1391 | 0.777 |
| $a+bx+cz^2$ | 115.88 | 83.86 | 0.837 | 0.0683 | 0.0439 | 0.7696 | 0.2315 | 0.1504 | 0.773 |
| $a+bx+c\sqrt{z}$ | 115.25 | 87.25 | 0.838 | 0.0703 | 0.0438 | 0.7562 | 0.2309 | 0.1352 | 0.774 |
| $a+bx+c/z$ | 133.76 | 97.55 | 0.782 | 0.0804 | 0.0581 | 0.6807 | 0.2483 | 0.1634 | 0.739 |
| $a+bx+c/z^2$ | 141.94 | 104.45 | 0.755 | 0.0828 | 0.0610 | 0.6613 | 0.2551 | 0.1738 | 0.724 |
| $a+bx+c/\sqrt{z}$ | 126.80 | 92.73 | 0.804 | 0.0775 | 0.0541 | 0.7032 | 0.2421 | 0.1515 | 0.752 |
| $a+bx^2+cz$ | 112.02 | 87.68 | 0.847 | 0.0702 | 0.0467 | 0.7566 | 0.2430 | 0.1702 | 0.750 |
| $a+bx^2+cz^2$ | 114.33 | 87.11 | 0.841 | 0.0709 | 0.0504 | 0.7521 | 0.2465 | 0.1762 | 0.743 |
| $a+bx^2+c\sqrt{z}$ | 111.42 | 89.01 | 0.849 | 0.0711 | 0.0460 | 0.7504 | 0.2420 | 0.1645 | 0.752 |
| $a+bx^2+c/z$ | 117.94 | 93.72 | 0.831 | 0.0766 | 0.0528 | 0.7105 | 0.2486 | 0.1723 | 0.738 |
| $a+bx^2+c/z^2$ | 121.57 | 96.28 | 0.820 | 0.0776 | 0.0535 | 0.7023 | 0.2523 | 0.1784 | 0.730 |
| $a+bx^2+c/\sqrt{z}$ | 115.21 | 92.14 | 0.839 | 0.0752 | 0.0510 | 0.7210 | 0.2457 | 0.1667 | 0.744 |
| $a+b\sqrt{x}+cz$ | 120.74 | 91.88 | 0.823 | 0.0689 | 0.0411 | 0.7654 | 0.2339 | 0.1393 | 0.768 |
| $a+b\sqrt{x}+cz^2$ | 125.03 | 93.17 | 0.810 | 0.0693 | 0.0435 | 0.7630 | 0.2384 | 0.1515 | 0.759 |
| $a+b\sqrt{x}+c\sqrt{z}$ | 121.47 | 92.62 | 0.820 | 0.0710 | 0.0438 | 0.7510 | 0.2355 | 0.1351 | 0.765 |
| $a+b\sqrt{x}+c/z$ | 150.27 | 106.39 | 0.725 | 0.0861 | 0.0645 | 0.6335 | 0.2673 | 0.1766 | 0.697 |
| $a+b\sqrt{x}+c/z^2$ | 166.80 | 118.94 | 0.661 | 0.0917 | 0.0713 | 0.5845 | 0.2841 | 0.1987 | 0.658 |
| $a+b\sqrt{x}+c/\sqrt{z}$ | 138.20 | 97.70 | 0.768 | 0.0810 | 0.0572 | 0.6757 | 0.2545 | 0.1581 | 0.726 |
| $a+b/x+cz$ | 136.88 | 106.68 | 0.772 | 0.0722 | 0.0470 | 0.7426 | 0.2618 | 0.1788 | 0.710 |
| $a+b/x+cz^2$ | 151.53 | 117.04 | 0.721 | 0.0763 | 0.0535 | 0.7125 | 0.2827 | 0.2019 | 0.661 |
| $a+b/x+c\sqrt{z}$ | 134.34 | 105.79 | 0.780 | 0.0735 | 0.0448 | 0.7335 | 0.2582 | 0.1628 | 0.717 |
| $a+b/x+c/z$ | 176.81 | 121.08 | 0.620 | 0.0966 | 0.0674 | 0.5390 | 0.3147 | 0.2006 | 0.580 |
| $a+b/x+c/z^2$ | 216.44 | 159.08 | 0.430 | 0.1127 | 0.0861 | 0.3724 | 0.3690 | 0.2693 | 0.423 |
| $a+b/x+c/\sqrt{z}$ | 155.59 | 106.23 | 0.705 | 0.0869 | 0.0573 | 0.6273 | 0.2862 | 0.1748 | 0.653 |
| $a+b/x^2+cz$ | 139.34 | 107.04 | 0.764 | 0.0734 | 0.0487 | 0.7343 | 0.2701 | 0.1878 | 0.691 |
| $a+b/x^2+cz^2$ | 155.68 | 118.62 | 0.705 | 0.0785 | 0.0556 | 0.6958 | 0.2948 | 0.2127 | 0.632 |
| $a+b/x^2+c\sqrt{z}$ | 136.24 | 106.09 | 0.774 | 0.0742 | 0.0460 | 0.7281 | 0.2648 | 0.1701 | 0.703 |
| $a+b/x^2+c/z$ | 179.57 | 120.69 | 0.608 | 0.0978 | 0.0676 | 0.5282 | 0.3221 | 0.2046 | 0.560 |
| $a+b/x^2+c/z^2$ | 222.13 | 160.16 | 0.400 | 0.1155 | 0.0883 | 0.3410 | 0.3823 | 0.2765 | 0.381 |
| $a+b/x^2+c/\sqrt{z}$ | 157.54 | 106.90 | 0.698 | 0.0875 | 0.0571 | 0.6218 | 0.2919 | 0.1785 | 0.639 |
| $a+b/\sqrt{x}+cz$ | 133.55 | 104.57 | 0.783 | 0.0712 | 0.0449 | 0.7497 | 0.2538 | 0.1678 | 0.727 |
| $a+b/\sqrt{x}+cz^2$ | 145.86 | 112.45 | 0.741 | 0.0742 | 0.0508 | 0.7281 | 0.2702 | 0.1887 | 0.691 |
| $a+b/\sqrt{x}+c\sqrt{z}$ | 131.84 | 104.03 | 0.789 | 0.0728 | 0.0437 | 0.7380 | 0.2520 | 0.1550 | 0.731 |
| $a+b/\sqrt{x}+c/z$ | 172.73 | 120.13 | 0.637 | 0.0949 | 0.0681 | 0.5550 | 0.3056 | 0.1945 | 0.604 |
| $a+b/\sqrt{x}+c/z^2$ | 208.03 | 154.40 | 0.473 | 0.1088 | 0.0828 | 0.4151 | 0.3517 | 0.2556 | 0.476 |
| $a+b/\sqrt{x}+c/\sqrt{z}$ | 152.87 | 104.71 | 0.716 | 0.0860 | 0.0580 | 0.6351 | 0.2797 | 0.1695 | 0.669 |
| $a+by+cz$ | 124.14 | 98.57 | 0.812 | 0.0740 | 0.0457 | 0.7297 | 0.2606 | 0.1715 | 0.712 |
| $a+by+cz^2$ | 130.82 | 102.12 | 0.792 | 0.0762 | 0.0512 | 0.7133 | 0.2708 | 0.1842 | 0.689 |
| $a+by+c\sqrt{z}$ | 123.66 | 95.45 | 0.814 | 0.0753 | 0.0453 | 0.7198 | 0.2594 | 0.1600 | 0.715 |
| $a+by+c/z$ | 149.00 | 109.05 | 0.730 | 0.0903 | 0.0643 | 0.5974 | 0.2907 | 0.1852 | 0.642 |
| $a+by+c/z^2$ | 163.67 | 126.27 | 0.674 | 0.0959 | 0.0701 | 0.5464 | 0.3084 | 0.2072 | 0.597 |
| $a+by+c/\sqrt{z}$ | 138.12 | 98.51 | 0.768 | 0.0851 | 0.0579 | 0.6424 | 0.2771 | 0.1680 | 0.675 |
| $a+by^2+cz$ | 126.34 | 99.15 | 0.806 | 0.0759 | 0.0496 | 0.7159 | 0.2727 | 0.1959 | 0.685 |
| $a+by^2+cz^2$ | 134.86 | 102.53 | 0.779 | 0.0792 | 0.0565 | 0.6906 | 0.2868 | 0.2120 | 0.652 |
| $a+by^2+c\sqrt{z}$ | 124.36 | 96.11 | 0.812 | 0.0766 | 0.0466 | 0.7100 | 0.2692 | 0.1798 | 0.693 |
| $a+by^2+c/z$ | 142.89 | 108.78 | 0.752 | 0.0897 | 0.0622 | 0.6027 | 0.2958 | 0.1958 | 0.629 |
| $a+by^2+c/z^2$ | 155.04 | 123.73 | 0.708 | 0.0946 | 0.0670 | 0.5578 | 0.3128 | 0.2164 | 0.585 |
| $a+by^2+c/\sqrt{z}$ | 134.38 | 99.00 | 0.780 | 0.0852 | 0.0560 | 0.6418 | 0.2835 | 0.1792 | 0.660 |
| $a+b\sqrt{y}+cz$ | 124.10 | 98.47 | 0.813 | 0.0731 | 0.0440 | 0.7361 | 0.2552 | 0.1607 | 0.724 |
| $a+b\sqrt{y}+cz^2$ | 130.54 | 102.69 | 0.793 | 0.0750 | 0.0483 | 0.7226 | 0.2645 | 0.1730 | 0.703 |
| $a+b\sqrt{y}+c\sqrt{z}$ | 124.14 | 95.23 | 0.812 | 0.0747 | 0.0452 | 0.7242 | 0.2550 | 0.1501 | 0.725 |
| $a+b\sqrt{y}+c/z$ | 154.22 | 108.51 | 0.711 | 0.0915 | 0.0664 | 0.5867 | 0.2916 | 0.1840 | 0.640 |
| $a+b\sqrt{y}+c/z^2$ | 172.12 | 128.40 | 0.640 | 0.0982 | 0.0736 | 0.5238 | 0.3126 | 0.2136 | 0.586 |
| $a+b\sqrt{y}+c/\sqrt{z}$ | 141.26 | 97.46 | 0.757 | 0.0855 | 0.0590 | 0.6389 | 0.2759 | 0.1646 | 0.678 |
| $a+b/y+cz$ | 127.22 | 99.45 | 0.803 | 0.0719 | 0.0443 | 0.7447 | 0.2498 | 0.1540 | 0.736 |
| $a+b/y+cz^2$ | 135.63 | 106.24 | 0.776 | 0.0739 | 0.0472 | 0.7307 | 0.2609 | 0.1710 | 0.712 |
| $a+b/y+c\sqrt{z}$ | 127.39 | 98.31 | 0.803 | 0.0740 | 0.0454 | 0.7295 | 0.2507 | 0.1439 | 0.734 |
| $a+b/y+c/z$ | 168.77 | 114.54 | 0.653 | 0.0962 | 0.0709 | 0.5433 | 0.3054 | 0.1950 | 0.605 |
| $a+b/y+c/z^2$ | 199.34 | 144.76 | 0.517 | 0.1082 | 0.0829 | 0.4221 | 0.3440 | 0.2475 | 0.499 |
| $a+b/y+c/\sqrt{z}$ | 149.85 | 98.81 | 0.727 | 0.0875 | 0.0609 | 0.6216 | 0.2809 | 0.1675 | 0.666 |
| $a+b/y^2+cz$ | 129.39 | 100.70 | 0.796 | 0.0719 | 0.0454 | 0.7445 | 0.2514 | 0.1569 | 0.732 |
| $a+b/y^2+cz^2$ | 139.49 | 108.43 | 0.763 | 0.0744 | 0.0485 | 0.7269 | 0.2650 | 0.1759 | 0.702 |
| $a+b/y^2+c\sqrt{z}$ | 129.10 | 100.82 | 0.797 | 0.0740 | 0.0461 | 0.7294 | 0.2519 | 0.1477 | 0.731 |
| $a+b/y^2+c/z$ | 173.23 | 116.24 | 0.635 | 0.0979 | 0.0719 | 0.5269 | 0.3126 | 0.2015 | 0.586 |
| $a+b/y^2+c/z^2$ | 208.82 | 150.38 | 0.469 | 0.1122 | 0.0866 | 0.3782 | 0.3595 | 0.2585 | 0.453 |
| $a+b/y^2+c/\sqrt{z}$ | 152.52 | 100.65 | 0.717 | 0.0883 | 0.0615 | 0.6147 | 0.2847 | 0.1727 | 0.657 |
| $a+b/\sqrt{y}+cz$ | 125.95 | 98.96 | 0.807 | 0.0721 | 0.0437 | 0.7435 | 0.2499 | 0.1532 | 0.735 |
| $a+b/\sqrt{y}+cz^2$ | 133.45 | 104.95 | 0.783 | 0.0738 | 0.0466 | 0.7309 | 0.2599 | 0.1686 | 0.714 |
| $a+b/\sqrt{y}+c\sqrt{z}$ | 126.27 | 96.27 | 0.806 | 0.0741 | 0.0451 | 0.7289 | 0.2508 | 0.1417 | 0.733 |
| $a+b/\sqrt{y}+c/z$ | 164.92 | 112.87 | 0.669 | 0.0948 | 0.0699 | 0.5564 | 0.3004 | 0.1915 | 0.618 |
| $a+b/\sqrt{y}+c/z^2$ | 191.61 | 139.43 | 0.553 | 0.1051 | 0.0802 | 0.4548 | 0.3330 | 0.2374 | 0.530 |
| $a+b/\sqrt{y}+c/\sqrt{z}$ | 147.59 | 97.64 | 0.735 | 0.0869 | 0.0605 | 0.6270 | 0.2786 | 0.1643 | 0.671 |

Single EW ratio, single component functions result ( x/y ; x/z ; y/z)

(continued on next page)

**Table 4 – continued from previous page**

| Functional form | $T_{eff}$ (K) | | | Radius ($R_\odot$) | | | log (L/$L_\odot$) | | |
|---|---|---|---|---|---|---|---|---|---|
| | RMSE | MAD | $R^2_{ap}$ | RMSE | MAD | $R^2_{ap}$ | RMSE | MAD | $R^2_{ap}$ |
| a+bx/y | 248.36 | 191.47 | 0.250 | 0.1192 | 0.0952 | 0.2990 | 0.3896 | 0.3092 | 0.357 |
| a+b$x^2$/y | 250.06 | 198.53 | 0.239 | 0.1338 | 0.1059 | 0.1166 | 0.4500 | 0.3518 | 0.142 |
| a+b$\sqrt{x}$/y | 182.75 | 138.25 | 0.594 | 0.0924 | 0.0748 | 0.5789 | 0.2868 | 0.2141 | 0.652 |
| a+b/xy | 136.06 | 110.84 | 0.775 | 0.0824 | 0.0572 | 0.6649 | 0.2720 | 0.1920 | 0.687 |
| a+b/$x^2$y | 147.79 | 116.37 | 0.734 | 0.0889 | 0.0669 | 0.6097 | 0.3045 | 0.2294 | 0.607 |
| a+b/$\sqrt{x}$y | 135.44 | 108.25 | 0.777 | 0.0801 | 0.0571 | 0.6829 | 0.2562 | 0.1749 | 0.722 |
| a+bx/$y^2$ | 154.18 | 125.15 | 0.711 | 0.0830 | 0.0652 | 0.6597 | 0.2564 | 0.1901 | 0.721 |
| a+b$x^2$/$y^2$ | 248.88 | 190.62 | 0.246 | 0.1216 | 0.0972 | 0.2696 | 0.3979 | 0.3141 | 0.329 |
| a+b$\sqrt{x}$/$y^2$ | 129.60 | 109.07 | 0.796 | 0.0759 | 0.0549 | 0.7156 | 0.2388 | 0.1735 | 0.758 |
| a+b/x$y^2$ | 136.78 | 111.12 | 0.772 | 0.0835 | 0.0637 | 0.6561 | 0.2862 | 0.2188 | 0.653 |
| a+b/$x^2y^2$ | 153.28 | 122.46 | 0.714 | 0.0911 | 0.0715 | 0.5904 | 0.3178 | 0.2425 | 0.572 |
| a+b/$\sqrt{x}y^2$ | 128.62 | 104.41 | 0.799 | 0.0793 | 0.0588 | 0.6893 | 0.2670 | 0.2014 | 0.698 |
| a+bx/$\sqrt{y}$ | 250.51 | 200.15 | 0.236 | 0.1342 | 0.1062 | 0.1110 | 0.4526 | 0.3537 | 0.132 |
| a+b$x^2$/$\sqrt{y}$ | 220.59 | 166.97 | 0.408 | 0.1166 | 0.0934 | 0.3292 | 0.3729 | 0.2841 | 0.411 |
| a+b$\sqrt{x}$/$\sqrt{y}$ | 253.12 | 194.02 | 0.220 | 0.1203 | 0.0965 | 0.2851 | 0.3960 | 0.3108 | 0.336 |
| a+b/x$\sqrt{y}$ | 148.22 | 120.78 | 0.733 | 0.0862 | 0.0614 | 0.6330 | 0.2798 | 0.1909 | 0.668 |
| a+b/$x^2\sqrt{y}$ | 151.12 | 120.18 | 0.722 | 0.0901 | 0.0659 | 0.5995 | 0.3044 | 0.2219 | 0.607 |
| a+b/$\sqrt{x}\sqrt{y}$ | 156.03 | 122.25 | 0.704 | 0.0866 | 0.0665 | 0.6295 | 0.2740 | 0.1879 | 0.682 |
| a+bxy | 274.77 | 209.71 | 0.081 | 0.1312 | 0.1072 | 0.1504 | 0.4414 | 0.3493 | 0.175 |
| a+b$x^2$y | 276.96 | 211.14 | 0.067 | 0.1323 | 0.1078 | 0.1352 | 0.4459 | 0.3528 | 0.157 |
| a+b$\sqrt{x}$y | 273.19 | 208.53 | 0.092 | 0.1303 | 0.1067 | 0.1619 | 0.4381 | 0.3466 | 0.187 |
| a+by/x | 275.01 | 207.75 | 0.080 | 0.1302 | 0.1060 | 0.1635 | 0.4391 | 0.3442 | 0.183 |
| a+by/$x^2$ | 253.02 | 204.42 | 0.221 | 0.1358 | 0.1076 | 0.0898 | 0.4611 | 0.3585 | 0.099 |
| a+by/$\sqrt{x}$ | 270.65 | 206.02 | 0.109 | 0.1285 | 0.1054 | 0.1849 | 0.4319 | 0.3406 | 0.209 |
| a+bx$y^2$ | 284.33 | 213.75 | 0.016 | 0.1359 | 0.1093 | 0.0884 | 0.4619 | 0.3612 | 0.096 |
| a+b$x^2y^2$ | 284.65 | 213.82 | 0.014 | 0.1361 | 0.1093 | 0.0858 | 0.4626 | 0.3616 | 0.093 |
| a+b$\sqrt{x}y^2$ | 284.11 | 213.69 | 0.018 | 0.1357 | 0.1092 | 0.0902 | 0.4613 | 0.3610 | 0.098 |
| a+b$y^2$/x | 283.08 | 213.22 | 0.025 | 0.1351 | 0.1090 | 0.0994 | 0.4588 | 0.3594 | 0.108 |
| a+b$y^2$/$x^2$ | 282.93 | 212.54 | 0.026 | 0.1347 | 0.1087 | 0.1040 | 0.4578 | 0.3578 | 0.112 |
| a+b$y^2$/$\sqrt{x}$ | 283.48 | 213.45 | 0.022 | 0.1353 | 0.1091 | 0.0956 | 0.4598 | 0.3601 | 0.104 |
| a+bx$\sqrt{y}$ | 260.42 | 199.44 | 0.175 | 0.1252 | 0.1021 | 0.2260 | 0.4153 | 0.3256 | 0.269 |
| a+b$x^2\sqrt{y}$ | 266.91 | 204.39 | 0.133 | 0.1284 | 0.1045 | 0.1865 | 0.4275 | 0.3365 | 0.226 |
| a+b$\sqrt{x}\sqrt{y}$ | 256.03 | 196.50 | 0.202 | 0.1229 | 0.1004 | 0.2540 | 0.4069 | 0.3192 | 0.298 |
| a+b$\sqrt{y}$/x | 252.04 | 203.20 | 0.227 | 0.1352 | 0.1068 | 0.0973 | 0.4583 | 0.3571 | 0.110 |
| a+b$\sqrt{y}$/$x^2$ | 186.54 | 152.14 | 0.577 | 0.1048 | 0.0773 | 0.4581 | 0.3494 | 0.2488 | 0.483 |
| a+b$\sqrt{y}$/$\sqrt{x}$ | 268.35 | 203.05 | 0.124 | 0.1267 | 0.1028 | 0.2068 | 0.4247 | 0.3318 | 0.236 |
| a+bx/z | 285.48 | 209.99 | 0.008 | 0.1429 | 0.1121 | -0.0083 | 0.4929 | 0.3826 | -0.029 |
| a+b$x^2$/z | 269.23 | 199.39 | 0.118 | 0.1374 | 0.1098 | 0.0672 | 0.4726 | 0.3696 | 0.054 |
| a+b$\sqrt{x}$/z | 272.64 | 210.85 | 0.096 | 0.1357 | 0.1126 | 0.0907 | 0.4457 | 0.3628 | 0.158 |
| a+b/xz | 125.35 | 95.96 | 0.809 | 0.0716 | 0.0527 | 0.7471 | 0.2643 | 0.2083 | 0.704 |
| a+b/$x^2$z | 153.03 | 116.66 | 0.715 | 0.0833 | 0.0664 | 0.6577 | 0.3115 | 0.2508 | 0.589 |
| a+b/$\sqrt{x}$z | 114.30 | 90.66 | 0.841 | 0.0679 | 0.0444 | 0.7723 | 0.2359 | 0.1609 | 0.764 |
| a+bx/$z^2$ | 282.41 | 218.56 | 0.030 | 0.1411 | 0.1190 | 0.0170 | 0.4687 | 0.3894 | 0.069 |
| a+b$x^2$/$z^2$ | 283.50 | 210.00 | 0.022 | 0.1422 | 0.1133 | 0.0017 | 0.4897 | 0.3840 | -0.016 |
| a+b$\sqrt{x}$/$z^2$ | 189.55 | 156.02 | 0.563 | 0.1028 | 0.0830 | 0.4785 | 0.3198 | 0.2538 | 0.567 |
| a+b/x$z^2$ | 134.83 | 103.81 | 0.779 | 0.0778 | 0.0612 | 0.7013 | 0.2865 | 0.2346 | 0.652 |
| a+b/$x^2z^2$ | 160.27 | 127.19 | 0.687 | 0.0884 | 0.0722 | 0.6141 | 0.3269 | 0.2649 | 0.547 |
| a+b/$\sqrt{x}z^2$ | 121.07 | 95.87 | 0.822 | 0.0733 | 0.0553 | 0.7350 | 0.2611 | 0.2033 | 0.711 |
| a+bx/$\sqrt{z}$ | 250.92 | 182.11 | 0.234 | 0.1302 | 0.1005 | 0.1626 | 0.4519 | 0.3449 | 0.135 |
| a+b$x^2$/$\sqrt{z}$ | 253.67 | 188.13 | 0.217 | 0.1323 | 0.1061 | 0.1362 | 0.4518 | 0.3500 | 0.135 |
| a+b$\sqrt{x}$/$\sqrt{z}$ | 289.79 | 219.62 | -0.022 | 0.1448 | 0.1145 | -0.0352 | 0.4968 | 0.3962 | -0.046 |
| a+b/x$\sqrt{z}$ | 126.32 | 99.86 | 0.806 | 0.0707 | 0.0493 | 0.7533 | 0.2608 | 0.1982 | 0.712 |
| a+b/$x^2\sqrt{z}$ | 151.71 | 117.91 | 0.720 | 0.0816 | 0.0640 | 0.6711 | 0.3065 | 0.2442 | 0.602 |
| a+b/$\sqrt{x}\sqrt{z}$ | 119.17 | 92.30 | 0.827 | 0.0679 | 0.0417 | 0.7721 | 0.2346 | 0.1491 | 0.767 |
| a+bxz | 252.77 | 193.46 | 0.223 | 0.1217 | 0.0983 | 0.2693 | 0.4012 | 0.3103 | 0.318 |
| a+b$x^2$z | 237.09 | 177.41 | 0.316 | 0.1187 | 0.0934 | 0.3045 | 0.3835 | 0.2830 | 0.377 |
| a+b$\sqrt{x}$z | 262.06 | 199.70 | 0.164 | 0.1250 | 0.1023 | 0.2286 | 0.4166 | 0.3263 | 0.265 |
| a+bz/x | 290.14 | 219.23 | -0.024 | 0.1407 | 0.1140 | 0.0224 | 0.4774 | 0.3764 | 0.034 |
| a+bz/$x^2$ | 271.93 | 206.64 | 0.100 | 0.1403 | 0.1079 | 0.0277 | 0.4837 | 0.3762 | 0.009 |
| a+bz/$\sqrt{x}$ | 281.05 | 213.14 | 0.039 | 0.1345 | 0.1092 | 0.1069 | 0.4546 | 0.3584 | 0.125 |
| a+bx$z^2$ | 280.69 | 212.69 | 0.041 | 0.1340 | 0.1087 | 0.1139 | 0.4536 | 0.3572 | 0.128 |
| a+b$x^2z^2$ | 275.33 | 210.11 | 0.078 | 0.1316 | 0.1073 | 0.1444 | 0.4428 | 0.3499 | 0.169 |
| a+b$\sqrt{x}z^2$ | 282.46 | 213.27 | 0.029 | 0.1348 | 0.1090 | 0.1023 | 0.4575 | 0.3592 | 0.113 |
| a+b$z^2$/x | 285.90 | 213.87 | 0.005 | 0.1368 | 0.1094 | 0.0759 | 0.4657 | 0.3625 | 0.081 |
| a+b$z^2$/$x^2$ | 288.01 | 214.21 | -0.009 | 0.1383 | 0.1101 | 0.0555 | 0.4712 | 0.3647 | 0.059 |
| a+b$z^2$/$\sqrt{x}$ | 284.94 | 213.78 | 0.012 | 0.1362 | 0.1093 | 0.0841 | 0.4633 | 0.3616 | 0.090 |
| a+bx$\sqrt{z}$ | 200.22 | 144.48 | 0.512 | 0.1028 | 0.0811 | 0.4782 | 0.3255 | 0.2401 | 0.551 |
| a+b$x^2\sqrt{z}$ | 207.12 | 154.84 | 0.478 | 0.1126 | 0.0914 | 0.3741 | 0.3597 | 0.2733 | 0.452 |
| a+b$\sqrt{x}\sqrt{z}$ | 216.96 | 160.46 | 0.427 | 0.1061 | 0.0823 | 0.4439 | 0.3422 | 0.2455 | 0.504 |
| a+b$\sqrt{z}$/x | 253.44 | 182.32 | 0.218 | 0.1328 | 0.0993 | 0.1298 | 0.4618 | 0.3426 | 0.096 |
| a+b$\sqrt{z}$/$x^2$ | 171.97 | 135.99 | 0.640 | 0.0932 | 0.0686 | 0.5713 | 0.3428 | 0.2633 | 0.502 |
| a+b$\sqrt{z}$/$\sqrt{x}$ | 292.51 | 224.65 | -0.041 | 0.1435 | 0.1177 | -0.0165 | 0.4862 | 0.3908 | -0.002 |
| a+by/z | 264.92 | 193.59 | 0.146 | 0.1339 | 0.1054 | 0.1146 | 0.4656 | 0.3620 | 0.081 |
| a+b$y^2$/z | 256.04 | 188.75 | 0.202 | 0.1323 | 0.1052 | 0.1357 | 0.4536 | 0.3525 | 0.128 |
| a+b$\sqrt{y}$/z | 291.92 | 226.81 | 0.037 | 0.1451 | 0.1196 | -0.0401 | 0.4915 | 0.4003 | -0.023 |
| a+b/yz | 134.03 | 107.30 | 0.781 | 0.0771 | 0.0568 | 0.7068 | 0.2831 | 0.2229 | 0.660 |
| a+b/$y^2$z | 157.33 | 123.41 | 0.699 | 0.0859 | 0.0679 | 0.6360 | 0.3198 | 0.2551 | 0.567 |
| a+b/$\sqrt{y}$z | 128.10 | 100.75 | 0.800 | 0.0764 | 0.0501 | 0.7115 | 0.2678 | 0.1853 | 0.696 |
| a+by/$z^2$ | 293.44 | 226.69 | 0.048 | 0.1456 | 0.1173 | -0.0468 | 0.4969 | 0.4019 | -0.046 |
| a+b$y^2$/$z^2$ | 272.38 | 199.93 | 0.097 | 0.1375 | 0.1089 | 0.0662 | 0.4745 | 0.3720 | 0.046 |
| a+b$\sqrt{y}$/$z^2$ | 243.40 | 203.04 | 0.279 | 0.1271 | 0.1060 | 0.2024 | 0.4184 | 0.3351 | 0.258 |
| a+b/y$z^2$ | 146.08 | 112.46 | 0.740 | 0.0843 | 0.0635 | 0.6489 | 0.3076 | 0.2420 | 0.599 |
| a+b/$y^2z^2$ | 165.55 | 129.60 | 0.667 | 0.0915 | 0.0729 | 0.5868 | 0.3367 | 0.2662 | 0.520 |
| a+b/$\sqrt{y}z^2$ | 141.07 | 104.68 | 0.758 | 0.0839 | 0.0606 | 0.6523 | 0.2968 | 0.2153 | 0.627 |
| a+by/$\sqrt{z}$ | 224.06 | 161.44 | 0.389 | 0.1186 | 0.0907 | 0.3059 | 0.4102 | 0.3063 | 0.287 |
| a+b$y^2$/$\sqrt{z}$ | 242.17 | 179.57 | 0.286 | 0.1278 | 0.1021 | 0.1939 | 0.4342 | 0.3332 | 0.201 |
| a+b$\sqrt{y}$/$\sqrt{z}$ | 263.06 | 191.71 | 0.158 | 0.1331 | 0.1046 | 0.1258 | 0.4640 | 0.3573 | 0.088 |
| a+b/y$\sqrt{z}$ | 131.16 | 107.00 | 0.791 | 0.0746 | 0.0535 | 0.7251 | 0.2750 | 0.2122 | 0.680 |
| a+b/$y^2\sqrt{z}$ | 154.44 | 122.52 | 0.710 | 0.0834 | 0.0651 | 0.6563 | 0.3124 | 0.2479 | 0.587 |
| a+b/$\sqrt{y}\sqrt{z}$ | 122.99 | 99.45 | 0.816 | 0.0731 | 0.0447 | 0.7361 | 0.2564 | 0.1738 | 0.722 |
| a+byz | 198.20 | 145.83 | 0.522 | 0.1077 | 0.0850 | 0.4272 | 0.3380 | 0.2495 | 0.516 |
| a+b$y^2$z | 213.51 | 160.15 | 0.445 | 0.1178 | 0.0970 | 0.3145 | 0.3769 | 0.2947 | 0.398 |
| a+b$\sqrt{y}$z | 202.72 | 150.12 | 0.500 | 0.1064 | 0.0825 | 0.4413 | 0.3352 | 0.2436 | 0.524 |
| a+bz/y | 270.66 | 197.16 | 0.109 | 0.1372 | 0.1049 | 0.0700 | 0.4766 | 0.3586 | 0.038 |

(continued on next page)

**Table 4 – continued from previous page**

| Functional form | $T_{eff}$ (K) | | | Radius ($R_\odot$) | | | log (L/$L_\odot$) | | |
|---|---|---|---|---|---|---|---|---|---|
| | RMSE | MAD | $R^2_{ap}$ | RMSE | MAD | $R^2_{ap}$ | RMSE | MAD | $R^2_{ap}$ |
| $a+bz/y^2$ | 176.53 | 136.92 | 0.621 | 0.0926 | 0.0701 | 0.5769 | 0.3404 | 0.2573 | 0.509 |
| $a+bz/\sqrt{y}$ | 281.51 | 215.64 | 0.036 | 0.1384 | 0.1142 | 0.0542 | 0.4631 | 0.3707 | 0.091 |
| $a+byz^2$ | 235.70 | 176.11 | 0.324 | 0.1210 | 0.0972 | 0.2766 | 0.3886 | 0.2909 | 0.360 |
| $a+by^2z^2$ | 236.48 | 173.81 | 0.320 | 0.1248 | 0.1016 | 0.2305 | 0.4016 | 0.3079 | 0.317 |
| $a+b\sqrt{y}z^2$ | 239.65 | 177.59 | 0.301 | 0.1206 | 0.0964 | 0.2821 | 0.3892 | 0.2944 | 0.358 |
| $a+bz^2/y$ | 278.76 | 213.93 | 0.055 | 0.1355 | 0.1093 | 0.0939 | 0.4539 | 0.3591 | 0.127 |
| $a+bz^2/y^2$ | 280.79 | 211.05 | 0.041 | 0.1421 | 0.1103 | 0.0033 | 0.4894 | 0.3816 | -0.015 |
| $a+bz^2/\sqrt{y}$ | 261.39 | 201.52 | 0.169 | 0.1272 | 0.1029 | 0.2015 | 0.4204 | 0.3314 | 0.251 |
| $a+by\sqrt{z}$ | 173.34 | 125.97 | 0.634 | 0.0997 | 0.0782 | 0.5096 | 0.3145 | 0.2220 | 0.581 |
| $a+by^2\sqrt{z}$ | 211.26 | 155.45 | 0.457 | 0.1175 | 0.0943 | 0.3185 | 0.3821 | 0.2846 | 0.381 |
| $a+b\sqrt{y}\sqrt{z}$ | 165.31 | 120.07 | 0.668 | 0.0930 | 0.0703 | 0.5728 | 0.2905 | 0.1950 | 0.643 |
| $a+b\sqrt{z}/y$ | 176.78 | 140.02 | 0.620 | 0.0945 | 0.0708 | 0.5590 | 0.3427 | 0.2540 | 0.502 |
| $a+b\sqrt{z}/y^2$ | 158.71 | 123.59 | 0.694 | 0.0837 | 0.0637 | 0.6537 | 0.3132 | 0.2477 | 0.584 |
| $a+b\sqrt{z}/\sqrt{y}$ | 266.28 | 191.11 | 0.137 | 0.1349 | 0.1043 | 0.1008 | 0.4702 | 0.3548 | 0.063 |
| Single line EW, single EW ratio, double component functions result ( (x, x/y) ; (x, x/z) ; (x, y/z) ) | | | | | | | | | |
| $a+bx+cx/y$ | 140.03 | 110.91 | 0.761 | 0.0828 | 0.0599 | 0.6618 | 0.2577 | 0.1710 | 0.719 |
| $a+bx+cx/y^2$ | 145.97 | 112.45 | 0.741 | 0.0836 | 0.0617 | 0.6550 | 0.2586 | 0.1745 | 0.717 |
| $a+bx+cx/\sqrt{y}$ | 139.10 | 110.69 | 0.765 | 0.0824 | 0.0589 | 0.6649 | 0.2575 | 0.1701 | 0.719 |
| $a+bx+cxy$ | 137.84 | 108.70 | 0.769 | 0.0818 | 0.0573 | 0.6700 | 0.2573 | 0.1698 | 0.720 |
| $a+bx+cxy^2$ | 137.05 | 106.74 | 0.771 | 0.0815 | 0.0574 | 0.6720 | 0.2571 | 0.1698 | 0.720 |
| $a+bx+cx\sqrt{y}$ | 138.21 | 109.51 | 0.768 | 0.0819 | 0.0576 | 0.6687 | 0.2573 | 0.1697 | 0.719 |
| $a+bx+cx^2/y$ | 149.50 | 113.79 | 0.728 | 0.0825 | 0.0619 | 0.6636 | 0.2536 | 0.1752 | 0.727 |
| $a+bx+cx^2/y^2$ | 147.98 | 113.15 | 0.734 | 0.0834 | 0.0615 | 0.6562 | 0.2588 | 0.1745 | 0.716 |
| $a+bx+cx^2/\sqrt{y}$ | 131.27 | 109.86 | 0.790 | 0.0776 | 0.0545 | 0.7029 | 0.2446 | 0.1724 | 0.746 |
| $a+bx+cx^2y$ | 131.94 | 102.36 | 0.788 | 0.0797 | 0.0559 | 0.6865 | 0.2541 | 0.1709 | 0.727 |
| $a+bx+cx^2y^2$ | 133.63 | 102.32 | 0.783 | 0.0803 | 0.0570 | 0.6817 | 0.2552 | 0.1714 | 0.724 |
| $a+bx+cx^2\sqrt{y}$ | 129.91 | 101.02 | 0.795 | 0.0790 | 0.0549 | 0.6918 | 0.2525 | 0.1709 | 0.730 |
| $a+bx+c\sqrt{x}/y$ | 145.69 | 112.15 | 0.742 | 0.0836 | 0.0617 | 0.6550 | 0.2587 | 0.1744 | 0.716 |
| $a+bx+c\sqrt{x}/y^2$ | 147.87 | 112.31 | 0.734 | 0.0805 | 0.0576 | 0.6799 | 0.2548 | 0.1716 | 0.725 |
| $a+bx+c\sqrt{x}/\sqrt{y}$ | 132.90 | 104.82 | 0.785 | 0.0821 | 0.0584 | 0.6671 | 0.2556 | 0.1679 | 0.723 |
| $a+bx+c\sqrt{x}y$ | 147.35 | 113.09 | 0.736 | 0.0835 | 0.0616 | 0.6556 | 0.2586 | 0.1748 | 0.717 |
| $a+bx+c\sqrt{x}y^2$ | 141.34 | 110.18 | 0.757 | 0.0826 | 0.0593 | 0.6630 | 0.2584 | 0.1726 | 0.717 |
| $a+bx+c\sqrt{x}\sqrt{y}$ | 150.01 | 113.03 | 0.726 | 0.0824 | 0.0618 | 0.6649 | 0.2529 | 0.1745 | 0.729 |
| $a+bx+c/xy$ | 114.24 | 80.71 | 0.841 | 0.0792 | 0.0546 | 0.6901 | 0.2431 | 0.1565 | 0.750 |
| $a+bx+c/xy^2$ | 114.25 | 80.57 | 0.841 | 0.0793 | 0.0546 | 0.6898 | 0.2431 | 0.1563 | 0.750 |
| $a+bx+c/x\sqrt{y}$ | 114.25 | 80.99 | 0.841 | 0.0793 | 0.0546 | 0.6898 | 0.2432 | 0.1567 | 0.749 |
| $a+bx+cy/x$ | 118.52 | 86.29 | 0.829 | 0.0808 | 0.0559 | 0.6773 | 0.2481 | 0.1604 | 0.739 |
| $a+bx+cy^2/x$ | 145.07 | 110.98 | 0.744 | 0.0836 | 0.0617 | 0.6551 | 0.2587 | 0.1744 | 0.716 |
| $a+bx+c\sqrt{y}/x$ | 115.14 | 82.71 | 0.839 | 0.0798 | 0.0552 | 0.6855 | 0.2447 | 0.1575 | 0.746 |
| $a+bx+c/x^2y$ | 116.07 | 86.08 | 0.836 | 0.0804 | 0.0559 | 0.6811 | 0.2447 | 0.1581 | 0.746 |
| $a+bx+c/x^2y^2$ | 116.14 | 86.17 | 0.836 | 0.0804 | 0.0559 | 0.6809 | 0.2447 | 0.1581 | 0.746 |
| $a+bx+c/x^2\sqrt{y}$ | 116.06 | 86.07 | 0.836 | 0.0804 | 0.0559 | 0.6812 | 0.2447 | 0.1581 | 0.746 |
| $a+bx+cy/x^2$ | 116.32 | 86.36 | 0.835 | 0.0804 | 0.0559 | 0.6806 | 0.2450 | 0.1582 | 0.746 |
| $a+bx+cy^2/x^2$ | 117.61 | 86.93 | 0.832 | 0.0808 | 0.0562 | 0.6775 | 0.2464 | 0.1589 | 0.743 |
| $a+bx+c\sqrt{y}/x^2$ | 116.14 | 86.19 | 0.836 | 0.0804 | 0.0559 | 0.6811 | 0.2448 | 0.1581 | 0.746 |
| $a+bx+c/\sqrt{x}y$ | 115.99 | 86.07 | 0.836 | 0.0782 | 0.0528 | 0.6980 | 0.2427 | 0.1566 | 0.751 |
| $a+bx+c/\sqrt{x}y^2$ | 116.28 | 85.97 | 0.835 | 0.0783 | 0.0527 | 0.6973 | 0.2429 | 0.1566 | 0.750 |
| $a+bx+c/\sqrt{x}\sqrt{y}$ | 115.41 | 85.20 | 0.838 | 0.0783 | 0.0531 | 0.6975 | 0.2426 | 0.1558 | 0.751 |
| $a+bx+cy/\sqrt{x}$ | 145.24 | 111.41 | 0.743 | 0.0836 | 0.0617 | 0.6550 | 0.2588 | 0.1744 | 0.716 |
| $a+bx+cy^2/\sqrt{x}$ | 150.09 | 112.94 | 0.726 | 0.0833 | 0.0615 | 0.6570 | 0.2566 | 0.1752 | 0.721 |
| $a+bx+c\sqrt{y}/\sqrt{x}$ | 120.87 | 90.29 | 0.822 | 0.0810 | 0.0561 | 0.6757 | 0.2499 | 0.1620 | 0.735 |
| $a+bx+cx/z$ | 128.86 | 100.45 | 0.798 | 0.0768 | 0.0516 | 0.7090 | 0.2455 | 0.1587 | 0.745 |
| $a+bx+cx/z^2$ | 139.88 | 105.86 | 0.762 | 0.0814 | 0.0589 | 0.6731 | 0.2538 | 0.1703 | 0.727 |
| $a+bx+cx/\sqrt{z}$ | 122.69 | 97.30 | 0.817 | 0.0735 | 0.0461 | 0.7332 | 0.2403 | 0.1515 | 0.755 |
| $a+bx+cxz$ | 116.87 | 87.71 | 0.834 | 0.0693 | 0.0454 | 0.7630 | 0.2349 | 0.1540 | 0.766 |
| $a+bx+cxz^2$ | 117.71 | 88.07 | 0.831 | 0.0701 | 0.0480 | 0.7576 | 0.2363 | 0.1587 | 0.763 |
| $a+bx+cx\sqrt{z}$ | 117.04 | 90.64 | 0.833 | 0.0696 | 0.0442 | 0.7609 | 0.2351 | 0.1506 | 0.766 |
| $a+bx+cx^2/z$ | 134.31 | 102.07 | 0.781 | 0.0761 | 0.0507 | 0.7143 | 0.2470 | 0.1567 | 0.742 |
| $a+bx+cx^2/z^2$ | 140.82 | 106.68 | 0.759 | 0.0809 | 0.0581 | 0.6771 | 0.2542 | 0.1697 | 0.726 |
| $a+bx+cx^2/\sqrt{z}$ | 143.67 | 100.64 | 0.749 | 0.0774 | 0.0531 | 0.7045 | 0.2495 | 0.1542 | 0.736 |
| $a+bx+cx^2z$ | 118.76 | 91.11 | 0.828 | 0.0718 | 0.0495 | 0.7457 | 0.2402 | 0.1603 | 0.756 |
| $a+bx+cx^2z^2$ | 119.48 | 90.41 | 0.826 | 0.0722 | 0.0508 | 0.7426 | 0.2404 | 0.1623 | 0.755 |
| $a+bx+cx^2\sqrt{z}$ | 119.06 | 92.44 | 0.828 | 0.0726 | 0.0496 | 0.7394 | 0.2415 | 0.1616 | 0.753 |
| $a+bx+c\sqrt{x}/z$ | 127.41 | 97.95 | 0.803 | 0.0777 | 0.0534 | 0.7017 | 0.2450 | 0.1577 | 0.746 |
| $a+bx+c\sqrt{x}/z^2$ | 139.54 | 105.22 | 0.763 | 0.0818 | 0.0597 | 0.6695 | 0.2538 | 0.1706 | 0.727 |
| $a+bx+c\sqrt{x}/\sqrt{z}$ | 118.76 | 93.62 | 0.828 | 0.0745 | 0.0479 | 0.7259 | 0.2392 | 0.1497 | 0.758 |
| $a+bx+c\sqrt{x}z$ | 117.44 | 87.07 | 0.832 | 0.0685 | 0.0425 | 0.7680 | 0.2327 | 0.1479 | 0.771 |
| $a+bx+c\sqrt{x}z^2$ | 117.24 | 86.38 | 0.833 | 0.0691 | 0.0460 | 0.7641 | 0.2341 | 0.1553 | 0.768 |
| $a+bx+c\sqrt{x}\sqrt{z}$ | 121.69 | 90.90 | 0.820 | 0.0696 | 0.0421 | 0.7608 | 0.2341 | 0.1427 | 0.768 |
| $a+bx+c/xz$ | 120.09 | 91.20 | 0.825 | 0.0789 | 0.0532 | 0.6926 | 0.2454 | 0.1590 | 0.745 |
| $a+bx+c/xz^2$ | 136.53 | 105.76 | 0.773 | 0.0793 | 0.0545 | 0.6894 | 0.2509 | 0.1712 | 0.733 |
| $a+bx+c/x\sqrt{z}$ | 116.27 | 84.68 | 0.836 | 0.0792 | 0.0540 | 0.6901 | 0.2443 | 0.1567 | 0.747 |
| $a+bx+cz/x$ | 109.47 | 80.25 | 0.854 | 0.0783 | 0.0545 | 0.6972 | 0.2397 | 0.1554 | 0.756 |
| *** $a+bx+cz^2/x$** | **99.00** | **70.97** | **0.881** | 0.0732 | 0.0496 | 0.7355 | 0.2297 | 0.1441 | 0.776 |
| $a+bx+c\sqrt{z}/x$ | 112.63 | 81.63 | 0.846 | 0.0792 | 0.0550 | 0.6903 | 0.2423 | 0.1569 | 0.751 |
| $a+bx+c/x^2z$ | 115.06 | 83.88 | 0.839 | 0.0799 | 0.0553 | 0.6848 | 0.2440 | 0.1574 | 0.748 |
| $a+bx+c/x^2z^2$ | 114.71 | 81.78 | 0.840 | 0.0791 | 0.0542 | 0.6907 | 0.2432 | 0.1557 | 0.749 |
| $a+bx+c/x^2\sqrt{z}$ | 115.58 | 85.18 | 0.837 | 0.0802 | 0.0556 | 0.6827 | 0.2444 | 0.1578 | 0.747 |
| $a+bx+cz/x^2$ | 116.67 | 87.10 | 0.834 | 0.0806 | 0.0561 | 0.6796 | 0.2450 | 0.1582 | 0.746 |
| $a+bx+cz^2/x^2$ | 116.18 | 87.07 | 0.836 | 0.0805 | 0.0561 | 0.6804 | 0.2446 | 0.1582 | 0.747 |
| $a+bx+c\sqrt{z}/x^2$ | 116.46 | 86.72 | 0.835 | 0.0805 | 0.0560 | 0.6802 | 0.2449 | 0.1582 | 0.746 |
| $a+bx+c/\sqrt{x}z$ | 146.08 | 112.86 | 0.740 | 0.0823 | 0.0599 | 0.6659 | 0.2571 | 0.1751 | 0.720 |
| $a+bx+c/\sqrt{x}z^2$ | 150.51 | 110.22 | 0.724 | 0.0833 | 0.0616 | 0.6571 | 0.2588 | 0.1742 | 0.716 |
| $a+bx+c/\sqrt{x}\sqrt{z}$ | 130.78 | 101.66 | 0.792 | 0.0807 | 0.0564 | 0.6784 | 0.2514 | 0.1689 | 0.732 |
| $a+bx+cz/\sqrt{x}$ | 101.60 | 74.17 | 0.874 | 0.0721 | 0.0477 | 0.7430 | 0.2291 | 0.1391 | 0.778 |
| $a+bx+cz^2/\sqrt{x}$ | 108.03 | 79.08 | 0.858 | 0.0680 | 0.0434 | 0.7718 | 0.2271 | 0.1413 | 0.781 |
| $a+bx+c\sqrt{z}/\sqrt{x}$ | 105.69 | 75.91 | 0.864 | 0.0759 | 0.0519 | 0.7152 | 0.2358 | 0.1508 | 0.764 |
| $a+bx+cy/z$ | 128.28 | 101.01 | 0.800 | 0.0760 | 0.0525 | 0.7151 | 0.2413 | 0.1563 | 0.753 |
| $a+bx+cy/z^2$ | 139.08 | 104.78 | 0.765 | 0.0812 | 0.0588 | 0.6744 | 0.2526 | 0.1694 | 0.730 |
| $a+bx+cy/\sqrt{z}$ | 126.44 | 102.81 | 0.805 | 0.0728 | 0.0498 | 0.7384 | 0.2341 | 0.1543 | 0.768 |
| $a+bx+cyz$ | 119.71 | 89.75 | 0.826 | 0.0719 | 0.0465 | 0.7451 | 0.2403 | 0.1511 | 0.755 |
| $a+bx+cyz^2$ | 118.51 | 88.64 | 0.829 | 0.0709 | 0.0481 | 0.7515 | 0.2380 | 0.1568 | 0.760 |
| $a+bx+cy\sqrt{z}$ | 125.98 | 95.04 | 0.807 | 0.0755 | 0.0489 | 0.7184 | 0.2472 | 0.1547 | 0.741 |

(continued on next page)

**Table 4 – continued from previous page**

| Functional form | $T_{eff}$ (K) | | | Radius ($R_{\odot}$) | | | log (L/$L_{\odot}$) | | |
|---|---|---|---|---|---|---|---|---|---|
| | RMSE | MAD | $R^2_{ap}$ | RMSE | MAD | $R^2_{ap}$ | RMSE | MAD | $R^2_{ap}$ |
| $a+bx+cy^2/z$ | 131.78 | 104.03 | 0.789 | 0.0740 | 0.0514 | 0.7297 | 0.2377 | 0.1569 | 0.760 |
| $a+bx+cy^2/z^2$ | 138.11 | 105.16 | 0.768 | 0.0798 | 0.0571 | 0.6852 | 0.2505 | 0.1672 | 0.734 |
| $a+bx+cy^2/\sqrt{z}$ | 141.51 | 109.15 | 0.756 | 0.0756 | 0.0555 | 0.7178 | 0.2384 | 0.1650 | 0.759 |
| $a+bx+cy^2z$ | 123.36 | 93.72 | 0.815 | 0.0747 | 0.0502 | 0.7242 | 0.2462 | 0.1585 | 0.743 |
| $a+bx+cy^2z^2$ | 120.65 | 90.73 | 0.823 | 0.0732 | 0.0506 | 0.7355 | 0.2425 | 0.1593 | 0.751 |
| $a+bx+cy^2\sqrt{z}$ | 129.63 | 98.38 | 0.796 | 0.0780 | 0.0532 | 0.6994 | 0.2522 | 0.1636 | 0.731 |
| $a+bx+c\sqrt{y}/z$ | 128.86 | 98.91 | 0.798 | 0.0777 | 0.0545 | 0.7020 | 0.2438 | 0.1564 | 0.748 |
| $a+bx+c\sqrt{y}/z^2$ | 139.99 | 104.77 | 0.762 | 0.0820 | 0.0599 | 0.6684 | 0.2536 | 0.1711 | 0.728 |
| $a+bx+c\sqrt{y}/\sqrt{z}$ | 122.23 | 97.18 | 0.818 | 0.0738 | 0.0495 | 0.7314 | 0.2357 | 0.1494 | 0.765 |
| $a+bx+c\sqrt{y}z$ | 117.21 | 86.82 | 0.833 | 0.0700 | 0.0436 | 0.7581 | 0.2354 | 0.1465 | 0.765 |
| $a+bx+c\sqrt{y}z^2$ | 117.30 | 86.65 | 0.833 | 0.0696 | 0.0462 | 0.7606 | 0.2350 | 0.1544 | 0.766 |
| $a+bx+c\sqrt{y}\sqrt{z}$ | 121.59 | 91.49 | 0.820 | 0.0729 | 0.0451 | 0.7374 | 0.2406 | 0.1436 | 0.755 |
| $a+bx+c/yz$ | 150.69 | 112.64 | 0.724 | 0.0827 | 0.0602 | 0.6625 | 0.2586 | 0.1744 | 0.717 |
| $a+bx+c/yz^2$ | 149.65 | 109.99 | 0.728 | 0.0833 | 0.0614 | 0.6572 | 0.2587 | 0.1743 | 0.717 |
| $a+bx+c/y\sqrt{z}$ | 146.61 | 112.70 | 0.738 | 0.0812 | 0.0579 | 0.6745 | 0.2560 | 0.1745 | 0.722 |
| $a+bx+cz/y$ | 107.25 | 83.46 | 0.860 | 0.0703 | 0.0483 | 0.7558 | 0.2248 | 0.1402 | 0.786 |
| *** $a+bx+cz^2/y$** | 110.50 | 84.24 | 0.851 | **0.0669** | **0.0425** | **0.7791** | 0.2235 | 0.1398 | 0.788 |
| $a+bx+c\sqrt{z}/y$ | 112.66 | 91.21 | 0.846 | 0.0736 | 0.0495 | 0.7328 | 0.2320 | 0.1520 | 0.772 |
| $a+bx+c/y^2z$ | 144.37 | 110.06 | 0.746 | 0.0800 | 0.0562 | 0.6838 | 0.2543 | 0.1716 | 0.726 |
| $a+bx+c/y^2z^2$ | 150.12 | 112.78 | 0.726 | 0.0817 | 0.0587 | 0.6708 | 0.2577 | 0.1747 | 0.719 |
| $a+bx+c/y^2\sqrt{z}$ | 137.15 | 105.31 | 0.771 | 0.0789 | 0.0538 | 0.6928 | 0.2506 | 0.1698 | 0.734 |
| $a+bx+cz/y^2$ | 110.14 | 83.80 | 0.852 | 0.0757 | 0.0516 | 0.7167 | 0.2353 | 0.1531 | 0.765 |
| $a+bx+cz^2/y^2$ | 102.65 | 76.54 | 0.872 | 0.0712 | 0.0494 | 0.7500 | 0.2242 | 0.1421 | 0.787 |
| $a+bx+c\sqrt{z}/y^2$ | 117.46 | 89.99 | 0.832 | 0.0769 | 0.0512 | 0.7084 | 0.2405 | 0.1586 | 0.755 |
| $a+bx+c/\sqrt{y}z$ | 145.78 | 104.31 | 0.741 | 0.0834 | 0.0610 | 0.6567 | 0.2562 | 0.1742 | 0.722 |
| $a+bx+c/\sqrt{y}z^2$ | 145.73 | 106.37 | 0.742 | 0.0835 | 0.0613 | 0.6555 | 0.2571 | 0.1756 | 0.720 |
| $a+bx+c/\sqrt{y}\sqrt{z}$ | 149.23 | 107.59 | 0.729 | 0.0836 | 0.0616 | 0.6552 | 0.2578 | 0.1737 | 0.718 |
| $a+bx+cz/\sqrt{y}$ | 110.50 | 85.12 | 0.851 | 0.0683 | 0.0445 | 0.7695 | 0.2249 | 0.1360 | 0.786 |
| $a+bx+cz^2/\sqrt{y}$ | 113.86 | 84.83 | 0.842 | 0.0672 | 0.0414 | 0.7768 | 0.2275 | 0.1444 | 0.781 |
| $a+bx+c\sqrt{z}/\sqrt{y}$ | 111.25 | 88.01 | 0.849 | 0.0708 | 0.0481 | 0.7528 | 0.2270 | 0.1407 | 0.782 |
| $a+bx^2+cx/y$ | 126.51 | 97.91 | 0.805 | 0.0774 | 0.0530 | 0.7043 | 0.2485 | 0.1767 | 0.738 |
| $a+bx^2+cx/y^2$ | 124.79 | 97.45 | 0.811 | 0.0777 | 0.0537 | 0.7020 | 0.2544 | 0.1793 | 0.726 |
| $a+bx^2+cx/\sqrt{y}$ | 126.75 | 97.68 | 0.805 | 0.0775 | 0.0531 | 0.7034 | 0.2472 | 0.1709 | 0.741 |
| $a+bx^2+cxy$ | 126.72 | 100.78 | 0.805 | 0.0770 | 0.0546 | 0.7070 | 0.2512 | 0.1821 | 0.733 |
| $a+bx^2+cxy^2$ | 126.94 | 99.81 | 0.804 | 0.0768 | 0.0534 | 0.7085 | 0.2450 | 0.1761 | 0.746 |
| $a+bx^2+cx\sqrt{y}$ | 126.63 | 99.69 | 0.805 | 0.0778 | 0.0541 | 0.7014 | 0.2542 | 0.1780 | 0.726 |
| $a+bx^2+cx^2/y$ | 126.97 | 99.43 | 0.804 | 0.0772 | 0.0532 | 0.7056 | 0.2454 | 0.1749 | 0.745 |
| $a+bx^2+cx^2/y^2$ | 127.00 | 98.53 | 0.804 | 0.0773 | 0.0532 | 0.7046 | 0.2479 | 0.1783 | 0.740 |
| $a+bx^2+cx^2/\sqrt{y}$ | 126.95 | 99.52 | 0.804 | 0.0772 | 0.0532 | 0.7059 | 0.2447 | 0.1735 | 0.746 |
| $a+bx^2+cx^2y$ | 126.98 | 99.20 | 0.804 | 0.0772 | 0.0529 | 0.7057 | 0.2443 | 0.1709 | 0.747 |
| $a+bx^2+cx^2y^2$ | 127.00 | 98.72 | 0.804 | 0.0773 | 0.0527 | 0.7051 | 0.2449 | 0.1701 | 0.746 |
| $a+bx^2+cx^2\sqrt{y}$ | 126.97 | 99.37 | 0.804 | 0.0772 | 0.0530 | 0.7059 | 0.2442 | 0.1716 | 0.747 |
| $a+bx^2+c\sqrt{x}/y$ | 125.20 | 97.51 | 0.809 | 0.0775 | 0.0538 | 0.7033 | 0.2540 | 0.1800 | 0.727 |
| $a+bx^2+c\sqrt{x}/y^2$ | 126.62 | 98.04 | 0.805 | 0.0779 | 0.0532 | 0.7005 | 0.2516 | 0.1708 | 0.732 |
| $a+bx^2+c\sqrt{x}/\sqrt{y}$ | 125.66 | 97.03 | 0.808 | 0.0775 | 0.0531 | 0.7035 | 0.2498 | 0.1763 | 0.736 |
| $a+bx^2+c\sqrt{x}y$ | 126.51 | 100.44 | 0.805 | 0.0774 | 0.0546 | 0.7042 | 0.2540 | 0.1806 | 0.727 |
| $a+bx^2+c\sqrt{x}y^2$ | 126.80 | 100.59 | 0.804 | 0.0767 | 0.0536 | 0.7097 | 0.2473 | 0.1791 | 0.741 |
| $a+bx^2+c\sqrt{x}\sqrt{y}$ | 126.41 | 98.98 | 0.806 | 0.0778 | 0.0539 | 0.7008 | 0.2536 | 0.1772 | 0.727 |
| $a+bx^2+c/xy$ | 122.07 | 91.26 | 0.819 | 0.0779 | 0.0531 | 0.7006 | 0.2539 | 0.1795 | 0.727 |
| $a+bx^2+c/xy^2$ | 121.95 | 91.01 | 0.819 | 0.0779 | 0.0531 | 0.7006 | 0.2539 | 0.1796 | 0.727 |
| $a+bx^2+c/x\sqrt{y}$ | 122.08 | 91.35 | 0.819 | 0.0779 | 0.0531 | 0.7006 | 0.2539 | 0.1796 | 0.727 |
| $a+bx^2+cy/x$ | 121.67 | 91.17 | 0.820 | 0.0778 | 0.0534 | 0.7012 | 0.2536 | 0.1800 | 0.728 |
| $a+bx^2+cy^2/x$ | 126.12 | 97.44 | 0.806 | 0.0768 | 0.0543 | 0.7087 | 0.2511 | 0.1800 | 0.733 |
| $a+bx^2+c\sqrt{y}/x$ | 121.83 | 91.14 | 0.819 | 0.0779 | 0.0532 | 0.7007 | 0.2538 | 0.1797 | 0.727 |
| $a+bx^2+c/x^2y$ | 119.80 | 88.14 | 0.825 | 0.0779 | 0.0531 | 0.7006 | 0.2544 | 0.1794 | 0.726 |
| $a+bx^2+c/x^2y^2$ | 119.74 | 88.03 | 0.826 | 0.0779 | 0.0531 | 0.7006 | 0.2544 | 0.1793 | 0.726 |
| $a+bx^2+c/x^2\sqrt{y}$ | 119.84 | 88.20 | 0.825 | 0.0779 | 0.0531 | 0.7006 | 0.2544 | 0.1794 | 0.726 |
| $a+bx^2+cy/x^2$ | 119.91 | 88.36 | 0.825 | 0.0779 | 0.0532 | 0.7006 | 0.2543 | 0.1795 | 0.726 |
| $a+bx^2+cy^2/x^2$ | 119.97 | 88.40 | 0.825 | 0.0779 | 0.0533 | 0.7007 | 0.2543 | 0.1797 | 0.726 |
| $a+bx^2+c\sqrt{y}/x^2$ | 119.89 | 88.31 | 0.825 | 0.0779 | 0.0531 | 0.7006 | 0.2543 | 0.1794 | 0.726 |
| $a+bx^2+c/\sqrt{x}y$ | 124.16 | 93.97 | 0.812 | 0.0779 | 0.0530 | 0.7006 | 0.2531 | 0.1785 | 0.728 |
| $a+bx^2+c/\sqrt{x}y^2$ | 124.09 | 93.69 | 0.813 | 0.0779 | 0.0530 | 0.7007 | 0.2532 | 0.1786 | 0.728 |
| $a+bx^2+c/\sqrt{x}\sqrt{y}$ | 124.03 | 93.97 | 0.813 | 0.0779 | 0.0530 | 0.7006 | 0.2532 | 0.1785 | 0.728 |
| $a+bx^2+cy/\sqrt{x}$ | 125.87 | 97.46 | 0.807 | 0.0771 | 0.0542 | 0.7067 | 0.2523 | 0.1799 | 0.730 |
| $a+bx^2+cy^2/\sqrt{x}$ | 126.76 | 100.29 | 0.804 | 0.0768 | 0.0545 | 0.7090 | 0.2514 | 0.1808 | 0.732 |
| $a+bx^2+c\sqrt{y}/\sqrt{x}$ | 122.95 | 93.24 | 0.816 | 0.0777 | 0.0534 | 0.7017 | 0.2527 | 0.1795 | 0.729 |
| $a+bx^2+cx/z$ | 122.56 | 97.10 | 0.817 | 0.0770 | 0.0544 | 0.7075 | 0.2543 | 0.1800 | 0.726 |
| $a+bx^2+cx/z^2$ | 124.35 | 97.63 | 0.812 | 0.0777 | 0.0540 | 0.7018 | 0.2544 | 0.1796 | 0.726 |
| $a+bx^2+cx/\sqrt{z}$ | 122.77 | 95.98 | 0.817 | 0.0769 | 0.0548 | 0.7082 | 0.2544 | 0.1790 | 0.726 |
| $a+bx^2+cxz$ | 116.65 | 89.71 | 0.834 | 0.0712 | 0.0500 | 0.7497 | 0.2478 | 0.1750 | 0.740 |
| $a+bx^2+cxz^2$ | 117.64 | 91.58 | 0.832 | 0.0729 | 0.0534 | 0.7372 | 0.2508 | 0.1772 | 0.733 |
| $a+bx^2+cx\sqrt{z}$ | 116.32 | 91.18 | 0.835 | 0.0694 | 0.0435 | 0.7620 | 0.2407 | 0.1614 | 0.755 |
| $a+bx^2+cx^2/z$ | 122.94 | 97.70 | 0.816 | 0.0762 | 0.0543 | 0.7132 | 0.2542 | 0.1797 | 0.726 |
| $a+bx^2+cx^2/z^2$ | 125.00 | 97.84 | 0.810 | 0.0776 | 0.0542 | 0.7026 | 0.2544 | 0.1789 | 0.726 |
| $a+bx^2+cx^2/\sqrt{z}$ | 121.94 | 96.63 | 0.819 | 0.0753 | 0.0539 | 0.7201 | 0.2540 | 0.1795 | 0.727 |
| $a+bx^2+cx^2z$ | 120.64 | 95.39 | 0.823 | 0.0746 | 0.0543 | 0.7250 | 0.2535 | 0.1785 | 0.728 |
| $a+bx^2+cx^2z^2$ | 120.17 | 95.27 | 0.824 | 0.0750 | 0.0549 | 0.7222 | 0.2535 | 0.1783 | 0.728 |
| $a+bx^2+cx^2\sqrt{z}$ | 120.93 | 95.04 | 0.822 | 0.0746 | 0.0539 | 0.7255 | 0.2536 | 0.1787 | 0.728 |
| $a+bx^2+c\sqrt{x}/z$ | 120.61 | 95.98 | 0.823 | 0.0770 | 0.0540 | 0.7075 | 0.2537 | 0.1805 | 0.727 |
| $a+bx^2+c\sqrt{x}/z^2$ | 123.22 | 97.28 | 0.815 | 0.0777 | 0.0539 | 0.7019 | 0.2541 | 0.1803 | 0.726 |
| $a+bx^2+c\sqrt{x}/\sqrt{z}$ | 120.60 | 94.86 | 0.823 | 0.0768 | 0.0545 | 0.7086 | 0.2542 | 0.1804 | 0.726 |
| $a+bx^2+c\sqrt{x}z$ | 115.06 | 89.38 | 0.839 | 0.0699 | 0.0469 | 0.7591 | 0.2439 | 0.1708 | 0.748 |
| $a+bx^2+c\sqrt{x}z^2$ | 116.22 | 89.12 | 0.836 | 0.0718 | 0.0519 | 0.7456 | 0.2487 | 0.1769 | 0.738 |
| $a+bx^2+c\sqrt{x}\sqrt{z}$ | 117.23 | 91.76 | 0.833 | 0.0695 | 0.0423 | 0.7616 | 0.2367 | 0.1522 | 0.763 |
| $a+bx^2+c/xz$ | 125.19 | 95.49 | 0.809 | 0.0778 | 0.0532 | 0.7012 | 0.2522 | 0.1776 | 0.730 |
| $a+bx^2+c/xz^2$ | 126.99 | 98.65 | 0.804 | 0.0778 | 0.0532 | 0.7013 | 0.2502 | 0.1732 | 0.735 |
| $a+bx^2+c/x\sqrt{z}$ | 123.64 | 93.51 | 0.814 | 0.0778 | 0.0532 | 0.7009 | 0.2532 | 0.1790 | 0.728 |
| $a+bx^2+cz/x$ | 118.06 | 86.64 | 0.830 | 0.0778 | 0.0538 | 0.7010 | 0.2544 | 0.1795 | 0.726 |
| $a+bx^2+cz^2/x$ | 111.33 | 83.64 | 0.849 | 0.0763 | 0.0537 | 0.7124 | 0.2523 | 0.1806 | 0.730 |
| $a+bx^2+c\sqrt{z}/x$ | 120.24 | 89.04 | 0.824 | 0.0779 | 0.0533 | 0.7005 | 0.2543 | 0.1794 | 0.726 |

(continued on next page)

**Table 4 – continued from previous page**

| Functional form | $T_{eff}$ (K) | | | Radius ($R_\odot$) | | | log ($L/L_\odot$) | | |
|---|---|---|---|---|---|---|---|---|---|
| | RMSE | MAD | $R^2_{ap}$ | RMSE | MAD | $R^2_{ap}$ | RMSE | MAD | $R^2_{ap}$ |
| $a+bx^2+c/x^2z$ | 120.84 | 89.61 | 0.822 | 0.0779 | 0.0531 | 0.7006 | 0.2542 | 0.1796 | 0.726 |
| $a+bx^2+c/x^2z^2$ | 122.43 | 91.73 | 0.818 | 0.0779 | 0.0531 | 0.7006 | 0.2538 | 0.1795 | 0.727 |
| $a+bx^2+c/x^2\sqrt{z}$ | 120.29 | 88.85 | 0.824 | 0.0779 | 0.0531 | 0.7006 | 0.2543 | 0.1795 | 0.726 |
| $a+bx^2+cz/x^2$ | 119.22 | 87.36 | 0.827 | 0.0779 | 0.0531 | 0.7005 | 0.2544 | 0.1791 | 0.726 |
| $a+bx^2+cz^2/x^2$ | 118.54 | 86.62 | 0.829 | 0.0779 | 0.0533 | 0.7005 | 0.2544 | 0.1789 | 0.726 |
| $a+bx^2+c\sqrt{z}/x^2$ | 119.52 | 87.77 | 0.826 | 0.0779 | 0.0531 | 0.7005 | 0.2544 | 0.1793 | 0.726 |
| $a+bx^2+c/\sqrt{x}z$ | 126.70 | 98.43 | 0.805 | 0.0774 | 0.0537 | 0.7045 | 0.2469 | 0.1675 | 0.742 |
| $a+bx^2+c/\sqrt{x}z^2$ | 123.91 | 95.37 | 0.813 | 0.0776 | 0.0534 | 0.7024 | 0.2485 | 0.1685 | 0.738 |
| $a+bx^2+c/\sqrt{x}\sqrt{z}$ | 126.68 | 97.91 | 0.805 | 0.0775 | 0.0535 | 0.7033 | 0.2495 | 0.1731 | 0.736 |
| $a+bx^2+cz/\sqrt{x}$ | 111.96 | 85.49 | 0.847 | 0.0758 | 0.0533 | 0.7165 | 0.2518 | 0.1798 | 0.731 |
| $a+bx^2+cz^2/\sqrt{x}$ | 110.37 | 82.59 | 0.852 | 0.0716 | 0.0505 | 0.7470 | 0.2463 | 0.1766 | 0.743 |
| $a+bx^2+c\sqrt{z}/\sqrt{x}$ | 117.95 | 87.73 | 0.831 | 0.0776 | 0.0542 | 0.7028 | 0.2544 | 0.1801 | 0.726 |
| $a+bx^2+cy/z$ | 121.00 | 96.42 | 0.822 | 0.0762 | 0.0539 | 0.7135 | 0.2527 | 0.1803 | 0.729 |
| $a+bx^2+cy/z^2$ | 123.45 | 97.65 | 0.815 | 0.0776 | 0.0541 | 0.7029 | 0.2540 | 0.1804 | 0.727 |
| $a+bx^2+cy/\sqrt{z}$ | 121.41 | 96.09 | 0.821 | 0.0755 | 0.0545 | 0.7184 | 0.2525 | 0.1805 | 0.730 |
| $a+bx^2+cyz$ | 117.97 | 91.41 | 0.831 | 0.0734 | 0.0511 | 0.7341 | 0.2510 | 0.1746 | 0.733 |
| $a+bx^2+cyz^2$ | 117.61 | 91.51 | 0.832 | 0.0734 | 0.0533 | 0.7339 | 0.2513 | 0.1766 | 0.732 |
| $a+bx^2+cy\sqrt{z}$ | 120.97 | 94.68 | 0.822 | 0.0752 | 0.0501 | 0.7206 | 0.2520 | 0.1732 | 0.731 |
| $a+bx^2+cy^2/z$ | 121.75 | 97.40 | 0.820 | 0.0750 | 0.0541 | 0.7219 | 0.2516 | 0.1791 | 0.732 |
| $a+bx^2+cy^2/z^2$ | 123.94 | 98.02 | 0.813 | 0.0773 | 0.0543 | 0.7052 | 0.2540 | 0.1805 | 0.727 |
| $a+bx^2+cy^2/\sqrt{z}$ | 122.48 | 98.26 | 0.817 | 0.0743 | 0.0547 | 0.7278 | 0.2495 | 0.1808 | 0.736 |
| $a+bx^2+cy^2z$ | 121.73 | 95.68 | 0.820 | 0.0761 | 0.0535 | 0.7142 | 0.2543 | 0.1789 | 0.726 |
| $a+bx^2+cy^2z^2$ | 119.82 | 94.48 | 0.825 | 0.0753 | 0.0544 | 0.7202 | 0.2536 | 0.1781 | 0.727 |
| $a+bx^2+cy^2\sqrt{z}$ | 124.58 | 97.16 | 0.811 | 0.0775 | 0.0535 | 0.7038 | 0.2542 | 0.1790 | 0.726 |
| $a+bx^2+c\sqrt{y}/z$ | 119.52 | 95.48 | 0.826 | 0.0764 | 0.0534 | 0.7118 | 0.2518 | 0.1790 | 0.731 |
| $a+bx^2+c\sqrt{y}/z^2$ | 122.68 | 97.25 | 0.817 | 0.0776 | 0.0538 | 0.7025 | 0.2535 | 0.1802 | 0.728 |
| $a+bx^2+c\sqrt{y}/\sqrt{z}$ | 119.06 | 94.60 | 0.828 | 0.0755 | 0.0535 | 0.7184 | 0.2517 | 0.1796 | 0.731 |
| $a+bx^2+c\sqrt{y}z$ | 115.08 | 89.43 | 0.839 | 0.0715 | 0.0487 | 0.7478 | 0.2470 | 0.1724 | 0.742 |
| $a+bx^2+c\sqrt{y}z^2$ | 116.11 | 89.21 | 0.836 | 0.0722 | 0.0521 | 0.7429 | 0.2492 | 0.1764 | 0.737 |
| $a+bx^2+c\sqrt{y}\sqrt{z}$ | 116.70 | 92.20 | 0.834 | 0.0727 | 0.0465 | 0.7389 | 0.2460 | 0.1644 | 0.744 |
| $a+bx^2+c/yz$ | 124.55 | 95.21 | 0.811 | 0.0776 | 0.0534 | 0.7028 | 0.2467 | 0.1642 | 0.742 |
| $a+bx^2+c/yz^2$ | 122.07 | 92.97 | 0.819 | 0.0777 | 0.0535 | 0.7017 | 0.2485 | 0.1673 | 0.738 |
| $a+bx^2+c/y\sqrt{z}$ | 126.49 | 98.10 | 0.805 | 0.0777 | 0.0533 | 0.7022 | 0.2481 | 0.1661 | 0.739 |
| $a+bx^2+cz/y$ | 113.98 | 88.76 | 0.842 | 0.0748 | 0.0533 | 0.7240 | 0.2501 | 0.1782 | 0.735 |
| $a+bx^2+cz^2/y$ | 110.25 | 85.88 | 0.852 | 0.0701 | 0.0490 | 0.7570 | 0.2426 | 0.1738 | 0.751 |
| $a+bx^2+c\sqrt{z}/y$ | 121.41 | 92.02 | 0.821 | 0.0773 | 0.0546 | 0.7052 | 0.2544 | 0.1803 | 0.726 |
| $a+bx^2+c/y^2z$ | 126.64 | 98.59 | 0.805 | 0.0778 | 0.0531 | 0.7011 | 0.2492 | 0.1681 | 0.737 |
| $a+bx^2+c/y^2z^2$ | 124.78 | 96.24 | 0.811 | 0.0778 | 0.0532 | 0.7010 | 0.2488 | 0.1673 | 0.738 |
| $a+bx^2+c/y^2\sqrt{z}$ | 127.00 | 98.70 | 0.804 | 0.0778 | 0.0530 | 0.7010 | 0.2503 | 0.1712 | 0.735 |
| $a+bx^2+cz/y^2$ | 121.45 | 91.30 | 0.821 | 0.0777 | 0.0541 | 0.7017 | 0.2544 | 0.1788 | 0.726 |
| $a+bx^2+cz^2/y^2$ | 112.44 | 86.39 | 0.846 | 0.0754 | 0.0535 | 0.7195 | 0.2506 | 0.1791 | 0.734 |
| $a+bx^2+c\sqrt{z}/y^2$ | 124.56 | 94.57 | 0.811 | 0.0779 | 0.0534 | 0.7005 | 0.2535 | 0.1782 | 0.728 |
| $a+bx^2+c/\sqrt{y}z$ | 120.74 | 92.60 | 0.823 | 0.0771 | 0.0534 | 0.7063 | 0.2456 | 0.1606 | 0.744 |
| $a+bx^2+c/\sqrt{y}z^2$ | 121.00 | 94.50 | 0.822 | 0.0777 | 0.0536 | 0.7021 | 0.2501 | 0.1733 | 0.735 |
| $a+bx^2+c/\sqrt{y}\sqrt{z}$ | 123.39 | 92.90 | 0.815 | 0.0770 | 0.0531 | 0.7073 | 0.2446 | 0.1589 | 0.747 |
| $a+bx^2+cz/\sqrt{y}$ | 110.70 | 88.01 | 0.851 | 0.0714 | 0.0491 | 0.7485 | 0.2439 | 0.1711 | 0.748 |
| $a+bx^2+cz^2/\sqrt{y}$ | 112.28 | 86.06 | 0.847 | 0.0699 | 0.0487 | 0.7585 | 0.2437 | 0.1749 | 0.748 |
| $a+bx^2+c\sqrt{z}/\sqrt{y}$ | 115.35 | 90.64 | 0.838 | 0.0747 | 0.0533 | 0.7241 | 0.2503 | 0.1784 | 0.735 |
| $a+b\sqrt{x}+cx/y$ | 174.94 | 134.14 | 0.628 | 0.0936 | 0.0726 | 0.5672 | 0.2941 | 0.2079 | 0.634 |
| $a+b\sqrt{x}+cx/y^2$ | 173.97 | 134.19 | 0.632 | 0.0942 | 0.0735 | 0.5619 | 0.2933 | 0.2101 | 0.635 |
| $a+b\sqrt{x}+cx/\sqrt{y}$ | 184.69 | 134.50 | 0.585 | 0.0941 | 0.0735 | 0.5627 | 0.2925 | 0.2100 | 0.638 |
| $a+b\sqrt{x}+cxy$ | 139.41 | 110.84 | 0.764 | 0.0835 | 0.0581 | 0.6559 | 0.2681 | 0.1796 | 0.695 |
| $a+b\sqrt{x}+cxy^2$ | 143.64 | 112.41 | 0.749 | 0.0844 | 0.0599 | 0.6479 | 0.2722 | 0.1844 | 0.686 |
| $a+b\sqrt{x}+cx\sqrt{y}$ | 133.26 | 105.43 | 0.784 | 0.0820 | 0.0562 | 0.6683 | 0.2623 | 0.1746 | 0.709 |
| $a+b\sqrt{x}+cx^2/y$ | 157.83 | 125.58 | 0.697 | 0.0851 | 0.0653 | 0.6428 | 0.2623 | 0.1891 | 0.709 |
| $a+b\sqrt{x}+cx^2/y^2$ | 184.09 | 136.97 | 0.588 | 0.0949 | 0.0738 | 0.5556 | 0.2971 | 0.2106 | 0.626 |
| $a+b\sqrt{x}+cx^2/\sqrt{y}$ | 128.07 | 106.28 | 0.800 | 0.0774 | 0.0539 | 0.7043 | 0.2447 | 0.1736 | 0.746 |
| $a+b\sqrt{x}+cx^2y$ | 135.29 | 106.28 | 0.777 | 0.0810 | 0.0572 | 0.6764 | 0.2626 | 0.1806 | 0.708 |
| $a+b\sqrt{x}+cx^2y^2$ | 140.39 | 109.13 | 0.760 | 0.0827 | 0.0597 | 0.6624 | 0.2682 | 0.1857 | 0.695 |
| $a+b\sqrt{x}+cx^2\sqrt{y}$ | 131.12 | 102.94 | 0.791 | 0.0796 | 0.0554 | 0.6874 | 0.2577 | 0.1776 | 0.719 |
| $a+b\sqrt{x}+c\sqrt{x}/y$ | 173.08 | 133.89 | 0.636 | 0.0941 | 0.0734 | 0.5626 | 0.2934 | 0.2097 | 0.635 |
| $a+b\sqrt{x}+c\sqrt{x}/y^2$ | 184.67 | 134.45 | 0.585 | 0.0925 | 0.0699 | 0.5778 | 0.2935 | 0.2093 | 0.635 |
| $a+b\sqrt{x}+c\sqrt{x}/\sqrt{y}$ | 162.84 | 128.30 | 0.677 | 0.0918 | 0.0704 | 0.5839 | 0.2873 | 0.2006 | 0.650 |
| $a+b\sqrt{x}+c\sqrt{x}y$ | 151.68 | 121.14 | 0.720 | 0.0877 | 0.0637 | 0.6201 | 0.2793 | 0.1867 | 0.669 |
| $a+b\sqrt{x}+c\sqrt{x}y^2$ | 149.55 | 118.19 | 0.728 | 0.0867 | 0.0618 | 0.6289 | 0.2778 | 0.1862 | 0.673 |
| $a+b\sqrt{x}+c\sqrt{x}\sqrt{y}$ | 153.55 | 122.48 | 0.713 | 0.0886 | 0.0652 | 0.6126 | 0.2807 | 0.1886 | 0.666 |
| $a+b\sqrt{x}+c/xy$ | 118.85 | 87.72 | 0.828 | 0.0828 | 0.0593 | 0.6612 | 0.2476 | 0.1643 | 0.740 |
| $a+b\sqrt{x}+c/xy^2$ | 118.86 | 87.21 | 0.828 | 0.0829 | 0.0592 | 0.6610 | 0.2476 | 0.1642 | 0.740 |
| $a+b\sqrt{x}+c/x\sqrt{y}$ | 119.33 | 88.57 | 0.827 | 0.0830 | 0.0595 | 0.6596 | 0.2482 | 0.1651 | 0.739 |
| $a+b\sqrt{x}+cy/x$ | 133.60 | 101.36 | 0.783 | 0.0875 | 0.0643 | 0.6220 | 0.2647 | 0.1780 | 0.703 |
| $a+b\sqrt{x}+cy^2/x$ | 171.11 | 132.02 | 0.644 | 0.0940 | 0.0731 | 0.5635 | 0.2940 | 0.2093 | 0.634 |
| $a+b\sqrt{x}+c\sqrt{y}/x$ | 124.08 | 93.14 | 0.813 | 0.0848 | 0.0618 | 0.6450 | 0.2541 | 0.1701 | 0.726 |
| $a+b\sqrt{x}+c/x^2y$ | 129.37 | 97.62 | 0.796 | 0.0863 | 0.0635 | 0.6322 | 0.2574 | 0.1751 | 0.719 |
| $a+b\sqrt{x}+c/x^2y^2$ | 129.61 | 97.77 | 0.796 | 0.0864 | 0.0635 | 0.6316 | 0.2576 | 0.1752 | 0.719 |
| $a+b\sqrt{x}+c/x^2\sqrt{y}$ | 129.33 | 97.61 | 0.797 | 0.0863 | 0.0635 | 0.6323 | 0.2573 | 0.1750 | 0.719 |
| $a+b\sqrt{x}+cy/x^2$ | 130.18 | 98.30 | 0.794 | 0.0865 | 0.0637 | 0.6302 | 0.2583 | 0.1757 | 0.717 |
| $a+b\sqrt{x}+cy^2/x^2$ | 133.42 | 100.39 | 0.783 | 0.0875 | 0.0646 | 0.6218 | 0.2624 | 0.1778 | 0.708 |
| $a+b\sqrt{x}+c\sqrt{y}/x^2$ | 129.63 | 97.89 | 0.796 | 0.0864 | 0.0635 | 0.6316 | 0.2577 | 0.1753 | 0.719 |
| $a+b\sqrt{x}+c/\sqrt{x}y$ | 115.68 | 84.80 | 0.837 | 0.0795 | 0.0547 | 0.6878 | 0.2411 | 0.1520 | 0.754 |
| $a+b\sqrt{x}+c/\sqrt{x}y^2$ | 116.19 | 84.01 | 0.836 | 0.0796 | 0.0544 | 0.6868 | 0.2417 | 0.1513 | 0.753 |
| $a+b\sqrt{x}+c/\sqrt{x}\sqrt{y}$ | 115.18 | 82.69 | 0.839 | 0.0799 | 0.0555 | 0.6849 | 0.2414 | 0.1545 | 0.753 |
| $a+b\sqrt{x}+cy/\sqrt{x}$ | 171.64 | 132.77 | 0.642 | 0.0940 | 0.0731 | 0.5634 | 0.2937 | 0.2093 | 0.634 |
| $a+b\sqrt{x}+cy^2/\sqrt{x}$ | 173.49 | 133.58 | 0.634 | 0.0937 | 0.0724 | 0.5667 | 0.2948 | 0.2082 | 0.632 |
| $a+b\sqrt{x}+c\sqrt{y}/\sqrt{x}$ | 137.81 | 107.56 | 0.769 | 0.0881 | 0.0652 | 0.6168 | 0.2692 | 0.1818 | 0.693 |
| $a+b\sqrt{x}+cx/z$ | 149.98 | 109.62 | 0.726 | 0.0819 | 0.0574 | 0.6686 | 0.2646 | 0.1694 | 0.703 |
| $a+b\sqrt{x}+cx/z^2$ | 165.39 | 120.16 | 0.667 | 0.0895 | 0.0682 | 0.6049 | 0.2816 | 0.1917 | 0.664 |
| $a+b\sqrt{x}+cx/\sqrt{z}$ | 149.86 | 107.77 | 0.727 | 0.0789 | 0.0526 | 0.6925 | 0.2613 | 0.1621 | 0.711 |
| $a+b\sqrt{x}+cxz$ | 120.64 | 89.02 | 0.823 | 0.0693 | 0.0453 | 0.7631 | 0.2380 | 0.1556 | 0.760 |
| $a+b\sqrt{x}+cxz^2$ | 125.96 | 93.68 | 0.807 | 0.0710 | 0.0481 | 0.7514 | 0.2434 | 0.1623 | 0.749 |
| $a+b\sqrt{x}+cx\sqrt{z}$ | 117.01 | 90.59 | 0.833 | 0.0696 | 0.0442 | 0.7611 | 0.2360 | 0.1512 | 0.764 |
| $a+b\sqrt{x}+cx^2/z$ | 168.86 | 115.98 | 0.653 | 0.0859 | 0.0605 | 0.6357 | 0.2802 | 0.1791 | 0.667 |

(continued on next page)

**Table 4 – continued from previous page**

| Functional form | $T_{eff}$ (K) | | | Radius ($R_\odot$) | | | log (L/$L_\odot$) | | |
|---|---|---|---|---|---|---|---|---|---|
| | RMSE | MAD | $R^2_{ap}$ | RMSE | MAD | $R^2_{ap}$ | RMSE | MAD | $R^2_{ap}$ |
| $a+b\sqrt{x}+cx^2/z^2$ | 168.64 | 121.70 | 0.654 | 0.0894 | 0.0674 | 0.6056 | 0.2840 | 0.1923 | 0.658 |
| $a+b\sqrt{x}+cx^2/\sqrt{z}$ | 183.28 | 139.46 | 0.591 | 0.0949 | 0.0736 | 0.5553 | 0.2966 | 0.2144 | 0.627 |
| $a+b\sqrt{x}+cx^2z$ | 122.85 | 92.77 | 0.816 | 0.0718 | 0.0501 | 0.7455 | 0.2440 | 0.1662 | 0.748 |
| $a+b\sqrt{x}+cx^2z^2$ | 127.92 | 96.08 | 0.801 | 0.0734 | 0.0516 | 0.7343 | 0.2487 | 0.1704 | 0.738 |
| $a+b\sqrt{x}+cx^2\sqrt{z}$ | 120.49 | 93.45 | 0.823 | 0.0724 | 0.0497 | 0.7415 | 0.2431 | 0.1638 | 0.750 |
| $a+b\sqrt{x}+c\sqrt{x}/z$ | 144.61 | 105.63 | 0.746 | 0.0823 | 0.0587 | 0.6652 | 0.2611 | 0.1661 | 0.711 |
| $a+b\sqrt{x}+c\sqrt{x}/z^2$ | 164.13 | 118.61 | 0.672 | 0.0900 | 0.0692 | 0.6005 | 0.2810 | 0.1921 | 0.665 |
| $a+b\sqrt{x}+c\sqrt{x}/\sqrt{z}$ | 133.18 | 98.87 | 0.784 | 0.0770 | 0.0514 | 0.7076 | 0.2491 | 0.1504 | 0.737 |
| $a+b\sqrt{x}+c\sqrt{x}z$ | 122.12 | 91.21 | 0.819 | 0.0688 | 0.0420 | 0.7664 | 0.2366 | 0.1478 | 0.763 |
| $a+b\sqrt{x}+c\sqrt{x}z^2$ | 125.87 | 92.48 | 0.807 | 0.0700 | 0.0459 | 0.7578 | 0.2411 | 0.1580 | 0.754 |
| $a+b\sqrt{x}+c\sqrt{x}\sqrt{z}$ | 121.88 | 93.45 | 0.819 | 0.0696 | 0.0415 | 0.7608 | 0.2365 | 0.1421 | 0.763 |
| $a+b\sqrt{x}+c/xz$ | 124.22 | 94.20 | 0.812 | 0.0813 | 0.0572 | 0.6738 | 0.2486 | 0.1613 | 0.738 |
| $a+b\sqrt{x}+c/xz^2$ | 164.43 | 122.81 | 0.671 | 0.0858 | 0.0647 | 0.6368 | 0.2739 | 0.1996 | 0.682 |
| $a+b\sqrt{x}+c/x\sqrt{z}$ | 119.84 | 88.52 | 0.825 | 0.0825 | 0.0593 | 0.6637 | 0.2483 | 0.1641 | 0.739 |
| $a+b\sqrt{x}+cz/x$ | 116.22 | 86.25 | 0.836 | 0.0818 | 0.0581 | 0.6695 | 0.2450 | 0.1611 | 0.746 |
| $a+b\sqrt{x}+cz^2/x$ | 101.74 | 72.82 | 0.874 | 0.0734 | 0.0494 | 0.7338 | 0.2284 | 0.1392 | 0.779 |
| $a+b\sqrt{x}+c\sqrt{z}/x$ | 120.32 | 89.37 | 0.824 | 0.0835 | 0.0598 | 0.6560 | 0.2493 | 0.1666 | 0.737 |
| $a+b\sqrt{x}+c/x^2z$ | 124.62 | 93.88 | 0.811 | 0.0849 | 0.0620 | 0.6440 | 0.2532 | 0.1710 | 0.728 |
| $a+b\sqrt{x}+c/x^2z^2$ | 118.41 | 86.57 | 0.829 | 0.0824 | 0.0589 | 0.6646 | 0.2467 | 0.1621 | 0.742 |
| $a+b\sqrt{x}+c/x^2\sqrt{z}$ | 127.29 | 96.15 | 0.803 | 0.0857 | 0.0629 | 0.6372 | 0.2556 | 0.1735 | 0.723 |
| $a+b\sqrt{x}+cz/x^2$ | 131.87 | 99.21 | 0.788 | 0.0869 | 0.0640 | 0.6268 | 0.2594 | 0.1766 | 0.715 |
| $a+b\sqrt{x}+cz^2/x^2$ | 131.63 | 98.80 | 0.789 | 0.0868 | 0.0639 | 0.6279 | 0.2591 | 0.1760 | 0.716 |
| $a+b\sqrt{x}+c\sqrt{z}/x^2$ | 130.91 | 98.67 | 0.791 | 0.0867 | 0.0638 | 0.6288 | 0.2587 | 0.1761 | 0.716 |
| $a+b\sqrt{x}+c/\sqrt{x}z$ | 184.84 | 136.69 | 0.584 | 0.0944 | 0.0740 | 0.5599 | 0.2965 | 0.2121 | 0.628 |
| $a+b\sqrt{x}+c/\sqrt{x}z^2$ | 181.78 | 127.45 | 0.598 | 0.0949 | 0.0738 | 0.5553 | 0.2958 | 0.2073 | 0.629 |
| $a+b\sqrt{x}+c/\sqrt{x}\sqrt{z}$ | 157.49 | 121.72 | 0.698 | 0.0889 | 0.0685 | 0.6097 | 0.2756 | 0.2003 | 0.678 |
| $a+b\sqrt{x}+cz/\sqrt{x}$ | 104.87 | 75.52 | 0.866 | 0.0719 | 0.0476 | 0.7449 | 0.2277 | 0.1327 | 0.780 |
| $a+b\sqrt{x}+cz^2/\sqrt{x}$ | 116.31 | 87.12 | 0.835 | 0.0684 | 0.0415 | 0.7688 | 0.2313 | 0.1405 | 0.773 |
| $a+b\sqrt{x}+c\sqrt{z}/\sqrt{x}$ | 106.93 | 78.17 | 0.861 | 0.0768 | 0.0534 | 0.7088 | 0.2344 | 0.1469 | 0.767 |
| $a+b\sqrt{x}+cy/z$ | 147.72 | 111.55 | 0.735 | 0.0805 | 0.0582 | 0.6796 | 0.2575 | 0.1683 | 0.719 |
| $a+b\sqrt{x}+cy/z^2$ | 163.43 | 118.67 | 0.675 | 0.0890 | 0.0679 | 0.6092 | 0.2788 | 0.1894 | 0.671 |
| $a+b\sqrt{x}+cy/\sqrt{z}$ | 152.60 | 115.42 | 0.717 | 0.0783 | 0.0572 | 0.6973 | 0.2531 | 0.1764 | 0.729 |
| $a+b\sqrt{x}+cyz$ | 125.25 | 93.37 | 0.809 | 0.0725 | 0.0462 | 0.7404 | 0.2466 | 0.1526 | 0.742 |
| $a+b\sqrt{x}+cyz^2$ | 127.68 | 95.50 | 0.802 | 0.0722 | 0.0481 | 0.7424 | 0.2466 | 0.1606 | 0.742 |
| $a+b\sqrt{x}+cy\sqrt{z}$ | 129.54 | 97.76 | 0.796 | 0.0764 | 0.0483 | 0.7115 | 0.2546 | 0.1528 | 0.725 |
| $a+b\sqrt{x}+cy^2/z$ | 160.47 | 118.12 | 0.687 | 0.0812 | 0.0593 | 0.6748 | 0.2622 | 0.1807 | 0.709 |
| $a+b\sqrt{x}+cy^2/z^2$ | 163.21 | 118.47 | 0.676 | 0.0872 | 0.0649 | 0.6243 | 0.2760 | 0.1867 | 0.677 |
| $a+b\sqrt{x}+cy^2/\sqrt{z}$ | 182.73 | 130.73 | 0.594 | 0.0903 | 0.0684 | 0.5972 | 0.2852 | 0.1969 | 0.655 |
| $a+b\sqrt{x}+cy^2z$ | 130.21 | 96.62 | 0.794 | 0.0760 | 0.0510 | 0.7146 | 0.2554 | 0.1611 | 0.724 |
| $a+b\sqrt{x}+cy^2z^2$ | 130.55 | 97.25 | 0.793 | 0.0750 | 0.0517 | 0.7221 | 0.2531 | 0.1672 | 0.729 |
| $a+b\sqrt{x}+cy^2\sqrt{z}$ | 135.74 | 101.36 | 0.776 | 0.0798 | 0.0536 | 0.6853 | 0.2635 | 0.1665 | 0.706 |
| $a+b\sqrt{x}+c\sqrt{y}/z$ | 145.90 | 107.41 | 0.741 | 0.0823 | 0.0599 | 0.6652 | 0.2598 | 0.1662 | 0.714 |
| $a+b\sqrt{x}+c\sqrt{y}/z^2$ | 164.30 | 118.48 | 0.672 | 0.0901 | 0.0695 | 0.5990 | 0.2807 | 0.1925 | 0.666 |
| $a+b\sqrt{x}+c\sqrt{y}/\sqrt{z}$ | 138.48 | 106.84 | 0.767 | 0.0768 | 0.0543 | 0.7088 | 0.2468 | 0.1605 | 0.742 |
| $a+b\sqrt{x}+c\sqrt{y}z$ | 122.68 | 93.03 | 0.817 | 0.0705 | 0.0429 | 0.7547 | 0.2405 | 0.1454 | 0.755 |
| $a+b\sqrt{x}+c\sqrt{y}z^2$ | 126.33 | 94.32 | 0.806 | 0.0707 | 0.0459 | 0.7530 | 0.2428 | 0.1565 | 0.750 |
| $a+b\sqrt{x}+c\sqrt{y}\sqrt{z}$ | 124.71 | 94.98 | 0.811 | 0.0735 | 0.0445 | 0.7331 | 0.2460 | 0.1445 | 0.744 |
| $a+b\sqrt{x}+c/yz$ | 183.69 | 131.65 | 0.589 | 0.0948 | 0.0736 | 0.5559 | 0.2969 | 0.2107 | 0.627 |
| $a+b\sqrt{x}+c/yz^2$ | 180.43 | 129.27 | 0.604 | 0.0949 | 0.0739 | 0.5551 | 0.2955 | 0.2088 | 0.630 |
| $a+b\sqrt{x}+c/y\sqrt{z}$ | 184.80 | 135.88 | 0.585 | 0.0933 | 0.0715 | 0.5701 | 0.2951 | 0.2128 | 0.631 |
| $a+b\sqrt{x}+cz/y$ | 116.10 | 90.56 | 0.836 | 0.0704 | 0.0495 | 0.7555 | 0.2247 | 0.1417 | 0.786 |
| $a+b\sqrt{x}+cz^2/y$ | 120.62 | 92.01 | 0.823 | 0.0677 | 0.0434 | 0.7740 | 0.2284 | 0.1431 | 0.779 |
| $a+b\sqrt{x}+c\sqrt{z}/y$ | 121.25 | 98.71 | 0.821 | 0.0734 | 0.0517 | 0.7339 | 0.2297 | 0.1500 | 0.777 |
| $a+b\sqrt{x}+c/y^2z$ | 178.37 | 131.65 | 0.613 | 0.0892 | 0.0680 | 0.6071 | 0.2867 | 0.2073 | 0.652 |
| $a+b\sqrt{x}+c/y^2z^2$ | 185.11 | 135.41 | 0.583 | 0.0929 | 0.0713 | 0.5735 | 0.2955 | 0.2110 | 0.630 |
| $a+b\sqrt{x}+c/y^2\sqrt{z}$ | 165.29 | 121.48 | 0.668 | 0.0850 | 0.0632 | 0.6429 | 0.2736 | 0.1951 | 0.683 |
| $a+b\sqrt{x}+cz/y^2$ | 110.55 | 83.34 | 0.851 | 0.0756 | 0.0539 | 0.7182 | 0.2294 | 0.1476 | 0.777 |
| $a+b\sqrt{x}+cz^2/y^2$ | 109.31 | 81.30 | 0.855 | 0.0711 | 0.0512 | 0.7504 | 0.2221 | 0.1424 | 0.791 |
| $a+b\sqrt{x}+c\sqrt{z}/y^2$ | 120.14 | 94.63 | 0.824 | 0.0768 | 0.0513 | 0.7086 | 0.2371 | 0.1562 | 0.762 |
| $a+b\sqrt{x}+c/\sqrt{y}z$ | 166.72 | 119.62 | 0.662 | 0.0922 | 0.0711 | 0.5801 | 0.2840 | 0.1971 | 0.658 |
| $a+b\sqrt{x}+c/\sqrt{y}z^2$ | 172.57 | 123.60 | 0.638 | 0.0937 | 0.0722 | 0.5661 | 0.2897 | 0.2050 | 0.644 |
| $a+b\sqrt{x}+c/\sqrt{y}\sqrt{z}$ | 168.08 | 118.68 | 0.656 | 0.0922 | 0.0704 | 0.5805 | 0.2851 | 0.1954 | 0.656 |
| $a+b\sqrt{x}+cz/\sqrt{y}$ | 119.20 | 92.91 | 0.827 | 0.0688 | 0.0445 | 0.7661 | 0.2282 | 0.1371 | 0.779 |
| $a+b\sqrt{x}+cz^2/\sqrt{y}$ | 123.45 | 92.56 | 0.815 | 0.0681 | 0.0421 | 0.7707 | 0.2337 | 0.1465 | 0.769 |
| $a+b\sqrt{x}+c\sqrt{z}/\sqrt{y}$ | 122.03 | 95.82 | 0.819 | 0.0714 | 0.0493 | 0.7482 | 0.2296 | 0.1462 | 0.777 |
| $a+b/x+cx/y$ | 252.82 | 188.55 | 0.222 | 0.1221 | 0.0950 | 0.2642 | 0.3988 | 0.3096 | 0.326 |
| $a+b/x+cx/y^2$ | 233.53 | 175.99 | 0.336 | 0.1203 | 0.0900 | 0.2851 | 0.3960 | 0.2909 | 0.336 |
| $a+b/x+cx/\sqrt{y}$ | 142.16 | 108.57 | 0.754 | 0.0864 | 0.0665 | 0.6311 | 0.2587 | 0.1830 | 0.716 |
| $a+b/x+cxy$ | 134.60 | 102.73 | 0.780 | 0.0844 | 0.0573 | 0.6484 | 0.2780 | 0.1920 | 0.673 |
| $a+b/x+cxy^2$ | 151.44 | 116.49 | 0.721 | 0.0891 | 0.0638 | 0.6084 | 0.3014 | 0.2118 | 0.615 |
| $a+b/x+cx\sqrt{y}$ | 123.09 | 92.29 | 0.816 | 0.0815 | 0.0555 | 0.6722 | 0.2611 | 0.1731 | 0.711 |
| $a+b/x+cx^2/y$ | 142.81 | 112.97 | 0.752 | 0.0839 | 0.0618 | 0.6522 | 0.2588 | 0.1817 | 0.716 |
| $a+b/x+cx^2/y^2$ | 254.70 | 191.63 | 0.211 | 0.1230 | 0.0964 | 0.2525 | 0.4029 | 0.3132 | 0.312 |
| $a+b/x+cx^2/\sqrt{y}$ | 120.69 | 95.88 | 0.823 | 0.0774 | 0.0540 | 0.7043 | 0.2440 | 0.1725 | 0.748 |
| $a+b/x+cx^2y$ | 140.16 | 111.10 | 0.761 | 0.0836 | 0.0609 | 0.6550 | 0.2831 | 0.2018 | 0.660 |
| $a+b/x+cx^2y^2$ | 155.37 | 123.86 | 0.706 | 0.0888 | 0.0662 | 0.6105 | 0.3050 | 0.2152 | 0.606 |
| $a+b/x+cx^2\sqrt{y}$ | 130.80 | 102.71 | 0.792 | 0.0806 | 0.0574 | 0.6794 | 0.2690 | 0.1920 | 0.693 |
| $a+b/x+c\sqrt{x}/y$ | 232.83 | 176.68 | 0.340 | 0.1203 | 0.0895 | 0.2857 | 0.3969 | 0.2917 | 0.333 |
| $a+b/x+c\sqrt{x}/y^2$ | 224.31 | 163.13 | 0.388 | 0.1189 | 0.0918 | 0.3016 | 0.3812 | 0.2809 | 0.384 |
| $a+b/x+c\sqrt{x}/\sqrt{y}$ | 255.19 | 189.44 | 0.208 | 0.1226 | 0.0953 | 0.2578 | 0.4017 | 0.3106 | 0.316 |
| $a+b/x+c\sqrt{x}y$ | 140.24 | 107.78 | 0.761 | 0.0881 | 0.0597 | 0.6169 | 0.2863 | 0.1898 | 0.653 |
| $a+b/x+c\sqrt{x}y^2$ | 154.36 | 117.97 | 0.710 | 0.0913 | 0.0640 | 0.5887 | 0.3060 | 0.2112 | 0.603 |
| $a+b/x+c\sqrt{x}\sqrt{y}$ | 129.51 | 96.87 | 0.796 | 0.0858 | 0.0604 | 0.6367 | 0.2705 | 0.1725 | 0.690 |
| $a+b/x+c/xy$ | 200.66 | 133.60 | 0.510 | 0.0991 | 0.0722 | 0.5147 | 0.3303 | 0.2252 | 0.538 |
| $a+b/x+c/xy^2$ | 166.34 | 117.02 | 0.663 | 0.0900 | 0.0632 | 0.5998 | 0.2885 | 0.1884 | 0.647 |
| $a+b/x+c/x\sqrt{y}$ | 224.74 | 149.27 | 0.385 | 0.1071 | 0.0806 | 0.4338 | 0.3614 | 0.2526 | 0.446 |
| $a+b/x+cy/x$ | 274.99 | 206.30 | 0.080 | 0.1324 | 0.1059 | 0.1349 | 0.4441 | 0.3428 | 0.164 |
| $a+b/x+cy^2/x$ | 232.56 | 179.39 | 0.342 | 0.1208 | 0.0908 | 0.2794 | 0.4018 | 0.2937 | 0.316 |
| $a+b/x+c\sqrt{y}/x$ | 274.75 | 199.12 | 0.082 | 0.1286 | 0.1005 | 0.1833 | 0.4351 | 0.3247 | 0.198 |
| $a+b/x+c/x^2y$ | 209.07 | 152.81 | 0.468 | 0.1144 | 0.0897 | 0.3541 | 0.3573 | 0.2631 | 0.459 |
| $a+b/x+c/x^2y^2$ | 208.96 | 152.74 | 0.469 | 0.1143 | 0.0897 | 0.3544 | 0.3571 | 0.2630 | 0.460 |
| $a+b/x+c/x^2\sqrt{y}$ | 209.98 | 153.46 | 0.464 | 0.1146 | 0.0898 | 0.3510 | 0.3585 | 0.2640 | 0.455 |
| $a+b/x+cy/x^2$ | 221.01 | 161.14 | 0.406 | 0.1182 | 0.0922 | 0.3107 | 0.3738 | 0.2761 | 0.408 |

(continued on next page)

**Table 4 – continued from previous page**

| Functional form | $T_{eff}$ (K) | | | Radius ($R_\odot$) | | | log (L/$L_\odot$) | | |
|---|---|---|---|---|---|---|---|---|---|
| | RMSE | MAD | $R^2_{ap}$ | RMSE | MAD | $R^2_{ap}$ | RMSE | MAD | $R^2_{ap}$ |
| $a+b/x+cy^2/x^2$ | 237.83 | 172.82 | 0.312 | 0.1237 | 0.0961 | 0.2450 | 0.3992 | 0.2953 | 0.325 |
| $a+b/x+c\sqrt{y}/x^2$ | 215.42 | 157.37 | 0.435 | 0.1164 | 0.0908 | 0.3316 | 0.3659 | 0.2700 | 0.433 |
| $a+b/x+c/\sqrt{x}y$ | 242.39 | 175.28 | 0.285 | 0.1246 | 0.0972 | 0.2337 | 0.4028 | 0.2985 | 0.313 |
| $a+b/x+c/\sqrt{x}y^2$ | 269.61 | 198.07 | 0.116 | 0.1315 | 0.1041 | 0.1461 | 0.4361 | 0.3305 | 0.194 |
| $a+b/x+c/\sqrt{x}\sqrt{y}$ | 212.44 | 156.37 | 0.451 | 0.1156 | 0.0898 | 0.3397 | 0.3653 | 0.2701 | 0.435 |
| $a+b/x+cy/\sqrt{x}$ | 232.35 | 178.24 | 0.343 | 0.1205 | 0.0903 | 0.2827 | 0.3999 | 0.2930 | 0.323 |
| $a+b/x+cy^2/\sqrt{x}$ | 190.77 | 150.45 | 0.557 | 0.1062 | 0.0760 | 0.4433 | 0.3523 | 0.2441 | 0.474 |
| $a+b/x+c\sqrt{y}/\sqrt{x}$ | 274.33 | 200.80 | 0.084 | 0.1293 | 0.1001 | 0.1745 | 0.4329 | 0.3250 | 0.206 |
| $a+b/x+cx/z$ | 246.39 | 174.66 | 0.261 | 0.1162 | 0.0888 | 0.3333 | 0.4033 | 0.3018 | 0.311 |
| $a+b/x+cx/z^2$ | 244.35 | 177.94 | 0.274 | 0.1194 | 0.0941 | 0.2963 | 0.4039 | 0.3018 | 0.309 |
| $a+b/x+cx/\sqrt{z}$ | 276.04 | 209.13 | 0.073 | 0.1324 | 0.1060 | 0.1341 | 0.4423 | 0.3471 | 0.171 |
| $a+b/x+cxz$ | 128.35 | 96.12 | 0.800 | 0.0711 | 0.0486 | 0.7503 | 0.2585 | 0.1848 | 0.717 |
| $a+b/x+cxz^2$ | 151.60 | 114.01 | 0.720 | 0.0782 | 0.0576 | 0.6982 | 0.2884 | 0.2088 | 0.648 |
| $a+b/x+cx\sqrt{z}$ | 112.56 | 85.97 | 0.846 | 0.0696 | 0.0444 | 0.7610 | 0.2408 | 0.1596 | 0.754 |
| $a+b/x+cx^2/z$ | 277.59 | 208.44 | 0.062 | 0.1324 | 0.1054 | 0.1350 | 0.4440 | 0.3456 | 0.165 |
| $a+b/x+cx^2/z^2$ | 259.16 | 188.40 | 0.183 | 0.1241 | 0.0974 | 0.2399 | 0.4230 | 0.3203 | 0.242 |
| $a+b/x+cx^2/\sqrt{z}$ | 187.63 | 144.54 | 0.572 | 0.1053 | 0.0827 | 0.4526 | 0.3275 | 0.2514 | 0.546 |
| $a+b/x+cx^2z$ | 136.36 | 104.67 | 0.774 | 0.0752 | 0.0548 | 0.7208 | 0.2724 | 0.2017 | 0.686 |
| $a+b/x+cx^2z^2$ | 157.08 | 121.39 | 0.700 | 0.0821 | 0.0625 | 0.6670 | 0.2995 | 0.2229 | 0.620 |
| $a+b/x+cx^2\sqrt{z}$ | 124.05 | 95.81 | 0.813 | 0.0733 | 0.0523 | 0.7346 | 0.2575 | 0.1850 | 0.719 |
| $a+b/x+c\sqrt{x}/z$ | 210.55 | 147.66 | 0.461 | 0.1040 | 0.0750 | 0.4655 | 0.3565 | 0.2518 | 0.462 |
| $a+b/x+c\sqrt{x}/z^2$ | 232.13 | 170.27 | 0.344 | 0.1161 | 0.0908 | 0.3350 | 0.3884 | 0.2877 | 0.361 |
| $a+b/x+c\sqrt{x}/\sqrt{z}$ | 235.61 | 164.14 | 0.325 | 0.1100 | 0.0827 | 0.4024 | 0.3868 | 0.2868 | 0.366 |
| $a+b/x+c\sqrt{x}z$ | 129.43 | 99.89 | 0.796 | 0.0706 | 0.0457 | 0.7537 | 0.2567 | 0.1770 | 0.721 |
| $a+b/x+c\sqrt{x}z^2$ | 150.79 | 115.65 | 0.723 | 0.0769 | 0.0554 | 0.7080 | 0.2847 | 0.2031 | 0.657 |
| $a+b/x+c\sqrt{x}\sqrt{z}$ | 114.74 | 87.91 | 0.840 | 0.0695 | 0.0408 | 0.7613 | 0.2403 | 0.1490 | 0.755 |
| $a+b/x+c/xz$ | 219.12 | 153.60 | 0.416 | 0.1167 | 0.0887 | 0.3271 | 0.3707 | 0.2667 | 0.418 |
| $a+b/x+c/xz^2$ | 231.66 | 163.91 | 0.347 | 0.1212 | 0.0924 | 0.2750 | 0.3886 | 0.2828 | 0.360 |
| $a+b/x+c/x\sqrt{z}$ | 207.98 | 145.20 | 0.474 | 0.1126 | 0.0854 | 0.3743 | 0.3552 | 0.2531 | 0.465 |
| $a+b/x+cz/x$ | 148.34 | 104.60 | 0.732 | 0.0866 | 0.0597 | 0.6300 | 0.2760 | 0.1831 | 0.677 |
| $a+b/x+cz^2/x$ | 138.66 | 100.59 | 0.766 | 0.0753 | 0.0520 | 0.7198 | 0.2638 | 0.1766 | 0.705 |
| $a+b/x+c\sqrt{z}/x$ | 170.22 | 116.33 | 0.647 | 0.0971 | 0.0704 | 0.5346 | 0.3043 | 0.2054 | 0.608 |
| $a+b/x+c/x^2z$ | 182.86 | 134.63 | 0.593 | 0.1060 | 0.0841 | 0.4452 | 0.3231 | 0.2415 | 0.558 |
| $a+b/x+c/x^2z^2$ | 239.34 | 164.09 | 0.303 | 0.1134 | 0.0885 | 0.3656 | 0.3850 | 0.2827 | 0.372 |
| $a+b/x+c/x^2\sqrt{z}$ | 202.82 | 148.29 | 0.500 | 0.1124 | 0.0886 | 0.3759 | 0.3493 | 0.2571 | 0.483 |
| $a+b/x+cz/x^2$ | 217.41 | 158.31 | 0.425 | 0.1168 | 0.0911 | 0.3266 | 0.3681 | 0.2706 | 0.426 |
| $a+b/x+cz^2/x^2$ | 210.76 | 152.26 | 0.460 | 0.1142 | 0.0889 | 0.3560 | 0.3593 | 0.2617 | 0.453 |
| $a+b/x+c\sqrt{z}/x^2$ | 216.17 | 157.63 | 0.431 | 0.1165 | 0.0909 | 0.3298 | 0.3666 | 0.2698 | 0.431 |
| $a+b/x+c/\sqrt{x}z$ | 179.42 | 128.36 | 0.608 | 0.1023 | 0.0777 | 0.4828 | 0.3196 | 0.2221 | 0.567 |
| $a+b/x+c/\sqrt{x}z^2$ | 212.06 | 153.70 | 0.453 | 0.1139 | 0.0881 | 0.3591 | 0.3640 | 0.2651 | 0.439 |
| $a+b/x+c/\sqrt{x}\sqrt{z}$ | 157.87 | 111.86 | 0.697 | 0.0948 | 0.0713 | 0.5564 | 0.2916 | 0.1951 | 0.640 |
| $a+b/x+cz/\sqrt{x}$ | 145.32 | 114.31 | 0.743 | 0.0756 | 0.0496 | 0.7178 | 0.2690 | 0.1818 | 0.693 |
| $a+b/x+cz^2/\sqrt{x}$ | 151.07 | 116.20 | 0.722 | 0.0759 | 0.0543 | 0.7154 | 0.2794 | 0.2020 | 0.669 |
| $a+b/x+c\sqrt{z}/\sqrt{x}$ | 172.99 | 132.18 | 0.636 | 0.0854 | 0.0594 | 0.6397 | 0.3015 | 0.2075 | 0.615 |
| $a+b/x+cy/z$ | 226.40 | 162.97 | 0.376 | 0.1073 | 0.0797 | 0.4316 | 0.3709 | 0.2743 | 0.417 |
| $a+b/x+cy/z^2$ | 233.84 | 170.45 | 0.335 | 0.1156 | 0.0900 | 0.3407 | 0.3887 | 0.2871 | 0.360 |
| $a+b/x+cy/\sqrt{z}$ | 272.93 | 200.12 | 0.094 | 0.1263 | 0.0956 | 0.2123 | 0.4331 | 0.3271 | 0.205 |
| $a+b/x+cyz$ | 136.75 | 107.46 | 0.772 | 0.0758 | 0.0502 | 0.7162 | 0.2741 | 0.1930 | 0.682 |
| $a+b/x+cyz^2$ | 155.36 | 119.69 | 0.706 | 0.0804 | 0.0583 | 0.6808 | 0.2953 | 0.2108 | 0.630 |
| $a+b/x+cy\sqrt{z}$ | 130.02 | 99.64 | 0.794 | 0.0778 | 0.0481 | 0.7010 | 0.2703 | 0.1724 | 0.690 |
| $a+b/x+cy^2/z$ | 270.82 | 197.85 | 0.108 | 0.1254 | 0.0956 | 0.2238 | 0.4302 | 0.3236 | 0.216 |
| $a+b/x+cy^2/z^2$ | 245.84 | 177.77 | 0.265 | 0.1180 | 0.0912 | 0.3121 | 0.4019 | 0.3008 | 0.316 |
| $a+b/x+cy^2/\sqrt{z}$ | 249.23 | 202.62 | 0.244 | 0.1269 | 0.1024 | 0.2043 | 0.4182 | 0.3308 | 0.259 |
| $a+b/x+cy^2z$ | 147.59 | 112.72 | 0.735 | 0.0817 | 0.0565 | 0.6708 | 0.2930 | 0.2049 | 0.636 |
| $a+b/x+cy^2z^2$ | 162.18 | 123.70 | 0.680 | 0.0851 | 0.0629 | 0.6424 | 0.3089 | 0.2232 | 0.596 |
| $a+b/x+cy^2\sqrt{z}$ | 144.52 | 104.92 | 0.746 | 0.0838 | 0.0562 | 0.6530 | 0.2925 | 0.1909 | 0.638 |
| $a+b/x+c\sqrt{y}/z$ | 198.26 | 141.24 | 0.522 | 0.0996 | 0.0712 | 0.5102 | 0.3376 | 0.2341 | 0.517 |
| $a+b/x+c\sqrt{y}/z^2$ | 225.51 | 165.97 | 0.381 | 0.1140 | 0.0884 | 0.3584 | 0.3792 | 0.2789 | 0.391 |
| $a+b/x+c\sqrt{y}/\sqrt{z}$ | 215.38 | 156.84 | 0.436 | 0.1011 | 0.0769 | 0.4956 | 0.3530 | 0.2611 | 0.472 |
| $a+b/x+c\sqrt{y}z$ | 133.72 | 107.19 | 0.782 | 0.0732 | 0.0469 | 0.7354 | 0.2654 | 0.1828 | 0.702 |
| $a+b/x+c\sqrt{y}z^2$ | 152.74 | 118.99 | 0.716 | 0.0781 | 0.0560 | 0.6985 | 0.2886 | 0.2047 | 0.647 |
| $a+b/x+c\sqrt{y}\sqrt{z}$ | 124.83 | 98.55 | 0.810 | 0.0744 | 0.0428 | 0.7267 | 0.2585 | 0.1622 | 0.717 |
| $a+b/x+c/yz$ | 198.87 | 140.85 | 0.519 | 0.1103 | 0.0843 | 0.3994 | 0.3463 | 0.2487 | 0.492 |
| $a+b/x+c/yz^2$ | 217.94 | 157.43 | 0.422 | 0.1166 | 0.0901 | 0.3282 | 0.3720 | 0.2731 | 0.414 |
| $a+b/x+c/y\sqrt{z}$ | 192.17 | 131.75 | 0.551 | 0.1082 | 0.0811 | 0.4223 | 0.3384 | 0.2368 | 0.515 |
| $a+b/x+cz/y$ | 189.16 | 147.29 | 0.565 | 0.0872 | 0.0702 | 0.6242 | 0.3110 | 0.2386 | 0.590 |
| $a+b/x+cz^2/y$ | 157.88 | 119.70 | 0.697 | 0.0762 | 0.0570 | 0.7135 | 0.2796 | 0.2024 | 0.669 |
| $a+b/x+c\sqrt{z}/y$ | 274.93 | 201.28 | 0.080 | 0.1274 | 0.0966 | 0.1990 | 0.4360 | 0.3294 | 0.194 |
| $a+b/x+c/y^2z$ | 239.67 | 172.86 | 0.301 | 0.1236 | 0.0961 | 0.2455 | 0.3979 | 0.2916 | 0.329 |
| $a+b/x+c/y^2z^2$ | 241.97 | 174.22 | 0.288 | 0.1244 | 0.0964 | 0.2355 | 0.4014 | 0.2927 | 0.317 |
| $a+b/x+c/y^2\sqrt{z}$ | 239.58 | 172.51 | 0.302 | 0.1235 | 0.0963 | 0.2463 | 0.3979 | 0.2921 | 0.329 |
| $a+b/x+cz/y^2$ | 271.22 | 194.42 | 0.105 | 0.1249 | 0.0941 | 0.2294 | 0.4289 | 0.3188 | 0.220 |
| $a+b/x+cz^2/y^2$ | 179.01 | 140.86 | 0.610 | 0.0840 | 0.0674 | 0.6515 | 0.2966 | 0.2314 | 0.627 |
| $a+b/x+c\sqrt{z}/y^2$ | 262.76 | 194.32 | 0.160 | 0.1303 | 0.1026 | 0.1617 | 0.4293 | 0.3270 | 0.219 |
| $a+b/x+c/\sqrt{y}z$ | 177.09 | 123.03 | 0.618 | 0.1011 | 0.0760 | 0.4954 | 0.3183 | 0.2156 | 0.571 |
| $a+b/x+c/\sqrt{y}z^2$ | 211.89 | 151.15 | 0.454 | 0.1133 | 0.0871 | 0.3661 | 0.3643 | 0.2614 | 0.438 |
| $a+b/x+c/\sqrt{y}\sqrt{z}$ | 159.05 | 110.17 | 0.692 | 0.0951 | 0.0708 | 0.5533 | 0.2969 | 0.1935 | 0.627 |
| $a+b/x+cz/\sqrt{y}$ | 153.19 | 121.52 | 0.714 | 0.0755 | 0.0552 | 0.7184 | 0.2725 | 0.1940 | 0.685 |
| $a+b/x+cz^2/\sqrt{y}$ | 152.84 | 115.20 | 0.716 | 0.0754 | 0.0539 | 0.7192 | 0.2791 | 0.1999 | 0.670 |
| $a+b/x+c\sqrt{z}/\sqrt{y}$ | 196.26 | 149.03 | 0.531 | 0.0906 | 0.0715 | 0.5946 | 0.3221 | 0.2427 | 0.561 |
| $a+b/x^2+cx/y$ | 245.28 | 179.09 | 0.268 | 0.1211 | 0.0929 | 0.2758 | 0.3928 | 0.3016 | 0.346 |
| $a+b/x^2+cx/y^2$ | 240.12 | 180.83 | 0.298 | 0.1234 | 0.0920 | 0.2480 | 0.4104 | 0.3038 | 0.286 |
| $a+b/x^2+cx/\sqrt{y}$ | 143.79 | 109.49 | 0.748 | 0.0879 | 0.0680 | 0.6186 | 0.2617 | 0.1887 | 0.710 |
| $a+b/x^2+cxy$ | 132.29 | 99.31 | 0.787 | 0.0844 | 0.0572 | 0.6482 | 0.2786 | 0.1923 | 0.671 |
| $a+b/x^2+cxy^2$ | 150.93 | 114.21 | 0.723 | 0.0898 | 0.0641 | 0.6020 | 0.3064 | 0.2162 | 0.602 |
| $a+b/x^2+cx\sqrt{y}$ | 121.32 | 89.03 | 0.821 | 0.0816 | 0.0557 | 0.6716 | 0.2605 | 0.1707 | 0.713 |
| $a+b/x^2+cx^2/y$ | 140.73 | 108.49 | 0.759 | 0.0841 | 0.0623 | 0.6512 | 0.2580 | 0.1785 | 0.718 |
| $a+b/x^2+cx^2/y^2$ | 254.21 | 187.87 | 0.214 | 0.1244 | 0.0965 | 0.2365 | 0.4074 | 0.3154 | 0.297 |
| $a+b/x^2+cx^2/\sqrt{y}$ | 118.80 | 92.79 | 0.828 | 0.0775 | 0.0540 | 0.7037 | 0.2435 | 0.1708 | 0.749 |
| $a+b/x^2+cx^2y$ | 139.59 | 109.22 | 0.763 | 0.0842 | 0.0614 | 0.6499 | 0.2877 | 0.2059 | 0.649 |
| $a+b/x^2+cx^2y^2$ | 156.93 | 123.32 | 0.700 | 0.0903 | 0.0672 | 0.5977 | 0.3135 | 0.2215 | 0.584 |
| $a+b/x^2+cx^2\sqrt{y}$ | 129.22 | 100.14 | 0.797 | 0.0808 | 0.0576 | 0.6776 | 0.2714 | 0.1945 | 0.688 |
| $a+b/x^2+c\sqrt{x}/y$ | 239.97 | 181.68 | 0.299 | 0.1236 | 0.0922 | 0.2457 | 0.4124 | 0.3049 | 0.279 |

(continued on next page)

**Table 4 – continued from previous page**

| Functional form | $T_{eff}$ (K) | | | Radius ($R_\odot$) | | | log (L/$L_\odot$) | | |
|---|---|---|---|---|---|---|---|---|---|
| | RMSE | MAD | $R^2_{ap}$ | RMSE | MAD | $R^2_{ap}$ | RMSE | MAD | $R^2_{ap}$ |
| a+b/$x^2$+c$\sqrt{x}/y^2$ | 223.47 | 163.02 | 0.392 | 0.1191 | 0.0921 | 0.2992 | 0.3818 | 0.2813 | 0.382 |
| a+b/$x^2$+c$\sqrt{x}/\sqrt{y}$ | 241.64 | 174.63 | 0.290 | 0.1198 | 0.0912 | 0.2918 | 0.3868 | 0.2946 | 0.366 |
| a+b/$x^2$+c$\sqrt{x}$y | 137.89 | 104.00 | 0.769 | 0.0880 | 0.0599 | 0.6172 | 0.2856 | 0.1876 | 0.654 |
| a+b/$x^2$+c$\sqrt{x}y^2$ | 152.91 | 114.56 | 0.716 | 0.0917 | 0.0641 | 0.5848 | 0.3093 | 0.2137 | 0.595 |
| a+b/$x^2$+c$\sqrt{x}\sqrt{y}$ | 129.72 | 99.74 | 0.795 | 0.0863 | 0.0613 | 0.6324 | 0.2703 | 0.1741 | 0.691 |
| a+b/$x^2$+c/xy | 244.91 | 175.94 | 0.270 | 0.1262 | 0.0981 | 0.2133 | 0.4077 | 0.3000 | 0.296 |
| a+b/$x^2$+c/x$y^2$ | 259.01 | 181.85 | 0.184 | 0.1307 | 0.1001 | 0.1571 | 0.4274 | 0.3106 | 0.226 |
| a+b/$x^2$+c/x$\sqrt{y}$ | 231.75 | 168.73 | 0.347 | 0.1220 | 0.0954 | 0.2657 | 0.3893 | 0.2887 | 0.358 |
| a+b/$x^2$+cy/x | 241.74 | 176.55 | 0.289 | 0.1187 | 0.0894 | 0.3048 | 0.3844 | 0.2877 | 0.374 |
| a+b/$x^2$+c$y^2$/x | 241.37 | 185.21 | 0.291 | 0.1249 | 0.0937 | 0.2298 | 0.4206 | 0.3075 | 0.251 |
| a+b/$x^2$+c$\sqrt{y}$/x | 187.99 | 137.01 | 0.570 | 0.1060 | 0.0826 | 0.4455 | 0.3227 | 0.2333 | 0.559 |
| a+b/$x^2$+c/$x^2$y | 144.12 | 97.29 | 0.747 | 0.0913 | 0.0674 | 0.5882 | 0.2646 | 0.1728 | 0.703 |
| a+b/$x^2$+c/$x^2y^2$ | 165.01 | 114.74 | 0.669 | 0.0996 | 0.0778 | 0.5100 | 0.2940 | 0.2128 | 0.634 |
| a+b/$x^2$+c/$x^2\sqrt{y}$ | 142.55 | 99.90 | 0.753 | 0.0889 | 0.0620 | 0.6099 | 0.2604 | 0.1592 | 0.713 |
| a+b/$x^2$+cy/$x^2$ | 220.85 | 153.73 | 0.407 | 0.1082 | 0.0844 | 0.4223 | 0.3590 | 0.2619 | 0.454 |
| a+b/$x^2$+c$y^2$/$x^2$ | 285.66 | 200.90 | 0.007 | 0.1345 | 0.1016 | 0.1068 | 0.4580 | 0.3339 | 0.111 |
| a+b/$x^2$+c$\sqrt{y}$/$x^2$ | 182.06 | 131.47 | 0.597 | 0.0962 | 0.0736 | 0.5428 | 0.3068 | 0.2197 | 0.601 |
| a+b/$x^2$+c/$\sqrt{x}$y | 229.55 | 167.34 | 0.359 | 0.1213 | 0.0949 | 0.2738 | 0.3871 | 0.2877 | 0.365 |
| a+b/$x^2$+c/$\sqrt{x}y^2$ | 250.30 | 178.33 | 0.238 | 0.1279 | 0.0990 | 0.1920 | 0.4152 | 0.3039 | 0.269 |
| a+b/$x^2$+c/$\sqrt{x}\sqrt{y}$ | 211.48 | 155.56 | 0.456 | 0.1153 | 0.0898 | 0.3434 | 0.3627 | 0.2687 | 0.442 |
| a+b/$x^2$+cy/$\sqrt{x}$ | 240.62 | 183.96 | 0.296 | 0.1244 | 0.0931 | 0.2363 | 0.4176 | 0.3067 | 0.261 |
| a+b/$x^2$+c$y^2$/$\sqrt{x}$ | 189.42 | 146.91 | 0.563 | 0.1068 | 0.0760 | 0.4373 | 0.3558 | 0.2437 | 0.464 |
| a+b/$x^2$+c$\sqrt{y}/\sqrt{x}$ | 238.48 | 172.35 | 0.308 | 0.1182 | 0.0889 | 0.3102 | 0.3806 | 0.2852 | 0.386 |
| a+b/$x^2$+cx/z | 268.70 | 185.60 | 0.122 | 0.1268 | 0.0963 | 0.2061 | 0.4436 | 0.3269 | 0.166 |
| a+b/$x^2$+cx/$z^2$ | 259.24 | 183.52 | 0.182 | 0.1263 | 0.0981 | 0.2123 | 0.4331 | 0.3206 | 0.205 |
| a+b/$x^2$+cx/$\sqrt{z}$ | 279.35 | 210.48 | 0.051 | 0.1372 | 0.1093 | 0.0710 | 0.4546 | 0.3592 | 0.125 |
| a+b/$x^2$+cxz | 128.16 | 95.06 | 0.800 | 0.0718 | 0.0495 | 0.7454 | 0.2639 | 0.1912 | 0.705 |
| a+b/$x^2$+cx$z^2$ | 155.44 | 115.13 | 0.706 | 0.0804 | 0.0595 | 0.6806 | 0.3005 | 0.2191 | 0.617 |
| a+b/$x^2$+cx$\sqrt{z}$ | 109.94 | 82.93 | 0.853 | 0.0696 | 0.0443 | 0.7609 | 0.2415 | 0.1605 | 0.753 |
| a+b/$x^2$+c$x^2$/z | 286.62 | 214.24 | 0.000 | 0.1385 | 0.1101 | 0.0525 | 0.4647 | 0.3639 | 0.085 |
| a+b/$x^2$+c$x^2$/$z^2$ | 275.23 | 193.95 | 0.078 | 0.1319 | 0.1016 | 0.1415 | 0.4544 | 0.3387 | 0.125 |
| a+b/$x^2$+c$x^2$/$\sqrt{z}$ | 185.01 | 139.56 | 0.584 | 0.1052 | 0.0823 | 0.4532 | 0.3267 | 0.2475 | 0.548 |
| a+b/$x^2$+c$x^2$z | 138.01 | 104.53 | 0.768 | 0.0765 | 0.0560 | 0.7107 | 0.2809 | 0.2104 | 0.666 |
| a+b/$x^2$+c$x^2z^2$ | 161.96 | 123.64 | 0.681 | 0.0848 | 0.0645 | 0.6448 | 0.3133 | 0.2315 | 0.584 |
| a+b/$x^2$+c$x^2\sqrt{z}$ | 123.39 | 94.23 | 0.815 | 0.0738 | 0.0528 | 0.7309 | 0.2619 | 0.1898 | 0.709 |
| a+b/$x^2$+c$\sqrt{x}$/z | 227.93 | 155.03 | 0.368 | 0.1113 | 0.0799 | 0.3883 | 0.3878 | 0.2745 | 0.363 |
| a+b/$x^2$+c$\sqrt{x}/z^2$ | 244.28 | 173.91 | 0.274 | 0.1216 | 0.0944 | 0.2700 | 0.4128 | 0.3022 | 0.278 |
| a+b/$x^2$+c$\sqrt{x}/\sqrt{z}$ | 265.79 | 181.32 | 0.141 | 0.1241 | 0.0932 | 0.2394 | 0.4381 | 0.3210 | 0.187 |
| a+b/$x^2$+c$\sqrt{x}$z | 128.92 | 98.73 | 0.798 | 0.0712 | 0.0464 | 0.7498 | 0.2615 | 0.1830 | 0.710 |
| a+b/$x^2$+c$\sqrt{x}z^2$ | 154.31 | 116.73 | 0.710 | 0.0790 | 0.0573 | 0.6919 | 0.2963 | 0.2137 | 0.628 |
| a+b/$x^2$+c$\sqrt{x}\sqrt{z}$ | 111.80 | 84.23 | 0.848 | 0.0695 | 0.0408 | 0.7614 | 0.2403 | 0.1488 | 0.755 |
| a+b/$x^2$+c/xz | 214.29 | 154.10 | 0.441 | 0.1158 | 0.0887 | 0.3385 | 0.3650 | 0.2611 | 0.436 |
| a+b/$x^2$+c/x$z^2$ | 227.76 | 161.43 | 0.369 | 0.1207 | 0.0921 | 0.2812 | 0.3855 | 0.2805 | 0.370 |
| a+b/$x^2$+c/x$\sqrt{z}$ | 207.84 | 150.11 | 0.474 | 0.1135 | 0.0873 | 0.3644 | 0.3555 | 0.2557 | 0.465 |
| a+b/$x^2$+cz/x | 222.24 | 159.18 | 0.399 | 0.1018 | 0.0757 | 0.4885 | 0.3724 | 0.2685 | 0.412 |
| a+b/$x^2$+c$z^2$/x | 164.45 | 122.23 | 0.671 | 0.0805 | 0.0593 | 0.6799 | 0.2990 | 0.2171 | 0.621 |
| a+b/$x^2$+c$\sqrt{z}$/x | 273.03 | 202.47 | 0.093 | 0.1359 | 0.1071 | 0.0882 | 0.4475 | 0.3454 | 0.152 |
| a+b/$x^2$+c/$x^2$z | 254.98 | 180.36 | 0.209 | 0.1293 | 0.0993 | 0.1740 | 0.4215 | 0.3068 | 0.247 |
| a+b/$x^2$+c/$x^2z^2$ | 256.44 | 180.97 | 0.200 | 0.1299 | 0.0995 | 0.1668 | 0.4240 | 0.3077 | 0.238 |
| a+b/$x^2$+c/$x^2\sqrt{z}$ | 253.55 | 179.64 | 0.218 | 0.1288 | 0.0990 | 0.1807 | 0.4193 | 0.3056 | 0.255 |
| a+b/$x^2$+cz/$x^2$ | 241.08 | 172.43 | 0.293 | 0.1241 | 0.0962 | 0.2393 | 0.4010 | 0.2949 | 0.319 |
| a+b/$x^2$+c$z^2$/$x^2$ | 212.90 | 149.64 | 0.449 | 0.1128 | 0.0862 | 0.3714 | 0.3615 | 0.2629 | 0.446 |
| a+b/$x^2$+c$\sqrt{z}/x^2$ | 247.44 | 176.33 | 0.255 | 0.1265 | 0.0978 | 0.2094 | 0.4102 | 0.3007 | 0.287 |
| a+b/$x^2$+c/$\sqrt{x}$z | 179.80 | 129.33 | 0.607 | 0.1028 | 0.0780 | 0.4787 | 0.3199 | 0.2238 | 0.566 |
| a+b/$x^2$+c/$\sqrt{x}z^2$ | 211.54 | 152.45 | 0.456 | 0.1144 | 0.0883 | 0.3544 | 0.3659 | 0.2643 | 0.433 |
| a+b/$x^2$+c/$\sqrt{x}\sqrt{z}$ | 165.51 | 115.75 | 0.667 | 0.0978 | 0.0735 | 0.5282 | 0.2998 | 0.2037 | 0.619 |
| a+b/$x^2$+cz/$\sqrt{x}$ | 169.45 | 127.34 | 0.651 | 0.0821 | 0.0576 | 0.6675 | 0.3041 | 0.2117 | 0.608 |
| a+b/$x^2$+c$z^2$/$\sqrt{x}$ | 160.17 | 120.78 | 0.688 | 0.0792 | 0.0576 | 0.6900 | 0.2970 | 0.2172 | 0.626 |
| a+b/$x^2$+c$\sqrt{z}/\sqrt{x}$ | 253.63 | 168.96 | 0.217 | 0.1162 | 0.0854 | 0.3335 | 0.4182 | 0.2985 | 0.259 |
| a+b/$x^2$+cy/z | 245.84 | 168.26 | 0.265 | 0.1162 | 0.0862 | 0.3334 | 0.4071 | 0.2986 | 0.298 |
| a+b/$x^2$+cy/$z^2$ | 246.86 | 174.54 | 0.259 | 0.1216 | 0.0936 | 0.2703 | 0.4147 | 0.3034 | 0.271 |
| a+b/$x^2$+cy/$\sqrt{z}$ | 290.34 | 210.77 | -0.026 | 0.1369 | 0.1044 | 0.0744 | 0.4702 | 0.3543 | 0.063 |
| a+b/$x^2$+cyz | 137.34 | 107.17 | 0.771 | 0.0767 | 0.0515 | 0.7092 | 0.2807 | 0.2012 | 0.666 |
| a+b/$x^2$+cy$z^2$ | 159.53 | 121.19 | 0.690 | 0.0828 | 0.0605 | 0.6617 | 0.3080 | 0.2219 | 0.598 |
| a+b/$x^2$+cy$\sqrt{z}$ | 128.31 | 97.17 | 0.800 | 0.0780 | 0.0485 | 0.6997 | 0.2725 | 0.1766 | 0.685 |
| a+b/$x^2$+c$y^2$/z | 288.31 | 207.77 | -0.011 | 0.1353 | 0.1023 | 0.0965 | 0.4664 | 0.3485 | 0.078 |
| a+b/$x^2$+c$y^2$/$z^2$ | 261.94 | 183.51 | 0.165 | 0.1257 | 0.0954 | 0.2201 | 0.4334 | 0.3213 | 0.204 |
| a+b/$x^2$+c$y^2$/$\sqrt{z}$ | 248.80 | 201.93 | 0.247 | 0.1290 | 0.1036 | 0.1785 | 0.4257 | 0.3314 | 0.232 |
| a+b/$x^2$+c$y^2$z | 149.47 | 113.20 | 0.728 | 0.0832 | 0.0579 | 0.6585 | 0.3021 | 0.2149 | 0.613 |
| a+b/$x^2$+c$y^2z^2$ | 167.24 | 125.67 | 0.660 | 0.0879 | 0.0651 | 0.6186 | 0.3230 | 0.2317 | 0.558 |
| a+b/$x^2$+c$y^2\sqrt{z}$ | 144.17 | 103.47 | 0.747 | 0.0846 | 0.0571 | 0.6468 | 0.2978 | 0.1978 | 0.624 |
| a+b/$x^2$+c$\sqrt{y}$/z | 210.16 | 145.39 | 0.463 | 0.1046 | 0.0741 | 0.4603 | 0.3606 | 0.2500 | 0.449 |
| a+b/$x^2$+c$\sqrt{y}/z^2$ | 235.43 | 168.10 | 0.326 | 0.1186 | 0.0915 | 0.3056 | 0.4000 | 0.2904 | 0.322 |
| a+b/$x^2$+c$\sqrt{y}/\sqrt{z}$ | 237.22 | 163.87 | 0.315 | 0.1109 | 0.0832 | 0.3931 | 0.3926 | 0.2846 | 0.347 |
| a+b/$x^2$+c$\sqrt{y}$z | 134.40 | 107.01 | 0.780 | 0.0740 | 0.0482 | 0.7294 | 0.2717 | 0.1904 | 0.687 |
| a+b/$x^2$+c$\sqrt{y}z^2$ | 156.67 | 120.42 | 0.701 | 0.0804 | 0.0580 | 0.6812 | 0.3006 | 0.2157 | 0.617 |
| a+b/$x^2$+c$\sqrt{y}\sqrt{z}$ | 123.38 | 96.31 | 0.815 | 0.0745 | 0.0431 | 0.7259 | 0.2605 | 0.1652 | 0.712 |
| a+b/$x^2$+c/yz | 198.87 | 140.62 | 0.519 | 0.1103 | 0.0842 | 0.3996 | 0.3463 | 0.2488 | 0.492 |
| a+b/$x^2$+c/y$z^2$ | 218.42 | 157.57 | 0.420 | 0.1173 | 0.0909 | 0.3207 | 0.3749 | 0.2748 | 0.405 |
| a+b/$x^2$+c/y$\sqrt{z}$ | 193.27 | 133.67 | 0.546 | 0.1084 | 0.0810 | 0.4201 | 0.3390 | 0.2368 | 0.513 |
| a+b/$x^2$+cz/y | 219.31 | 157.99 | 0.415 | 0.0996 | 0.0785 | 0.5102 | 0.3614 | 0.2656 | 0.446 |
| a+b/$x^2$+c$z^2$/y | 166.87 | 123.44 | 0.661 | 0.0797 | 0.0600 | 0.6867 | 0.2976 | 0.2150 | 0.625 |
| a+b/$x^2$+c$\sqrt{z}$/y | 288.36 | 215.49 | -0.012 | 0.1389 | 0.1092 | 0.0472 | 0.4701 | 0.3621 | 0.063 |
| a+b/$x^2$+c/$y^2$z | 238.07 | 171.41 | 0.310 | 0.1239 | 0.0962 | 0.2418 | 0.3982 | 0.2912 | 0.328 |
| a+b/$x^2$+c/$y^2z^2$ | 242.31 | 173.36 | 0.286 | 0.1255 | 0.0967 | 0.2224 | 0.4049 | 0.2933 | 0.305 |
| a+b/$x^2$+c/$y^2\sqrt{z}$ | 236.55 | 170.37 | 0.319 | 0.1234 | 0.0961 | 0.2484 | 0.3961 | 0.2907 | 0.335 |
| a+b/$x^2$+cz/$y^2$ | 284.18 | 213.22 | 0.017 | 0.1385 | 0.1096 | 0.0535 | 0.4651 | 0.3592 | 0.084 |
| a+b/$x^2$+c$z^2$/$y^2$ | 214.12 | 157.00 | 0.442 | 0.0970 | 0.0781 | 0.5356 | 0.3524 | 0.2653 | 0.474 |
| a+b/$x^2$+c$\sqrt{z}/y^2$ | 251.17 | 182.93 | 0.232 | 0.1288 | 0.0996 | 0.1815 | 0.4188 | 0.3131 | 0.257 |

(continued on next page)

**Table 4 – continued from previous page**

| Functional form | $T_{eff}$ (K) | | | Radius ($R_\odot$) | | | log (L/$L_\odot$) | | |
|---|---|---|---|---|---|---|---|---|---|
| | RMSE | MAD | $R^2_{ap}$ | RMSE | MAD | $R^2_{ap}$ | RMSE | MAD | $R^2_{ap}$ |
| $a+b/x^2+c/\sqrt{y}z$ | 176.94 | 123.47 | 0.619 | 0.1010 | 0.0756 | 0.4962 | 0.3188 | 0.2151 | 0.569 |
| $a+b/x^2+c/\sqrt{y}z^2$ | 213.86 | 150.95 | 0.444 | 0.1145 | 0.0870 | 0.3521 | 0.3705 | 0.2635 | 0.418 |
| $a+b/x^2+c/\sqrt{y}\sqrt{z}$ | 160.03 | 110.53 | 0.688 | 0.0953 | 0.0707 | 0.5520 | 0.2971 | 0.1937 | 0.626 |
| $a+b/x^2+cz/\sqrt{y}$ | 162.65 | 125.19 | 0.678 | 0.0788 | 0.0584 | 0.6931 | 0.2906 | 0.2062 | 0.642 |
| $a+b/x^2+cz^2/\sqrt{y}$ | 158.26 | 117.00 | 0.695 | 0.0779 | 0.0562 | 0.7005 | 0.2926 | 0.2116 | 0.637 |
| $a+b/x^2+c\sqrt{z}/\sqrt{y}$ | 223.63 | 159.09 | 0.392 | 0.1022 | 0.0790 | 0.4838 | 0.3691 | 0.2664 | 0.423 |
| $a+b/\sqrt{x}+cx/y$ | 252.80 | 189.73 | 0.222 | 0.1206 | 0.0946 | 0.2818 | 0.3945 | 0.3005 | 0.341 |
| $a+b/\sqrt{x}+cx/y^2$ | 223.28 | 167.78 | 0.393 | 0.1155 | 0.0882 | 0.3410 | 0.3756 | 0.2717 | 0.402 |
| $a+b/\sqrt{x}+cx/\sqrt{y}$ | 147.04 | 112.65 | 0.737 | 0.0863 | 0.0657 | 0.6319 | 0.2609 | 0.1823 | 0.712 |
| $a+b/\sqrt{x}+cxy$ | 136.56 | 105.80 | 0.773 | 0.0843 | 0.0575 | 0.6489 | 0.2768 | 0.1901 | 0.675 |
| $a+b/\sqrt{x}+cxy^2$ | 150.82 | 117.09 | 0.723 | 0.0882 | 0.0631 | 0.6161 | 0.2954 | 0.2059 | 0.630 |
| $a+b/\sqrt{x}+cx\sqrt{y}$ | 125.42 | 95.72 | 0.809 | 0.0815 | 0.0553 | 0.6721 | 0.2618 | 0.1744 | 0.710 |
| $a+b/\sqrt{x}+cx^2/y$ | 146.21 | 117.48 | 0.740 | 0.0841 | 0.0615 | 0.6512 | 0.2601 | 0.1851 | 0.713 |
| $a+b/\sqrt{x}+cx^2/y^2$ | 248.93 | 188.11 | 0.246 | 0.1195 | 0.0942 | 0.2950 | 0.3893 | 0.2984 | 0.358 |
| $a+b/\sqrt{x}+cx^2/\sqrt{y}$ | 122.68 | 98.63 | 0.817 | 0.0774 | 0.0540 | 0.7046 | 0.2443 | 0.1735 | 0.747 |
| $a+b/\sqrt{x}+cx^2y$ | 139.75 | 111.45 | 0.762 | 0.0830 | 0.0602 | 0.6601 | 0.2782 | 0.1963 | 0.672 |
| $a+b/\sqrt{x}+cx^2y^2$ | 152.54 | 122.15 | 0.717 | 0.0873 | 0.0650 | 0.6236 | 0.2959 | 0.2084 | 0.629 |
| $a+b/\sqrt{x}+cx^2\sqrt{y}$ | 131.58 | 104.06 | 0.789 | 0.0803 | 0.0570 | 0.6813 | 0.2664 | 0.1892 | 0.699 |
| $a+b/\sqrt{x}+c\sqrt{x}/y$ | 222.20 | 168.17 | 0.399 | 0.1153 | 0.0877 | 0.3431 | 0.3758 | 0.2714 | 0.402 |
| $a+b/\sqrt{x}+c\sqrt{x}/y^2$ | 225.98 | 166.61 | 0.379 | 0.1176 | 0.0921 | 0.3176 | 0.3771 | 0.2816 | 0.397 |
| $a+b/\sqrt{x}+c\sqrt{x}/\sqrt{y}$ | 257.38 | 190.67 | 0.194 | 0.1223 | 0.0953 | 0.2616 | 0.4025 | 0.3034 | 0.314 |
| $a+b/\sqrt{x}+c\sqrt{x}y$ | 143.31 | 112.07 | 0.750 | 0.0882 | 0.0601 | 0.6159 | 0.2867 | 0.1908 | 0.652 |
| $a+b/\sqrt{x}+c\sqrt{x}y^2$ | 154.86 | 120.20 | 0.708 | 0.0906 | 0.0636 | 0.5945 | 0.3014 | 0.2066 | 0.615 |
| $a+b/\sqrt{x}+c\sqrt{x}\sqrt{y}$ | 132.05 | 100.61 | 0.788 | 0.0858 | 0.0597 | 0.6369 | 0.2722 | 0.1737 | 0.686 |
| $a+b/\sqrt{x}+c/xy$ | 138.85 | 101.90 | 0.765 | 0.0912 | 0.0694 | 0.5896 | 0.2684 | 0.1883 | 0.695 |
| $a+b/\sqrt{x}+c/xy^2$ | 136.28 | 98.86 | 0.774 | 0.0904 | 0.0685 | 0.5967 | 0.2654 | 0.1847 | 0.701 |
| $a+b/\sqrt{x}+c/x\sqrt{y}$ | 145.82 | 108.17 | 0.741 | 0.0935 | 0.0720 | 0.5679 | 0.2770 | 0.1969 | 0.675 |
| $a+b/\sqrt{x}+cy/x$ | 219.87 | 163.40 | 0.412 | 0.1164 | 0.0900 | 0.3310 | 0.3737 | 0.2760 | 0.408 |
| $a+b/\sqrt{x}+cy^2/x$ | 220.61 | 169.97 | 0.408 | 0.1154 | 0.0868 | 0.3427 | 0.3784 | 0.2745 | 0.393 |
| $a+b/\sqrt{x}+c\sqrt{y}/x$ | 191.49 | 141.75 | 0.554 | 0.1084 | 0.0840 | 0.4199 | 0.3368 | 0.2441 | 0.519 |
| $a+b/\sqrt{x}+c/x^2y$ | 185.15 | 135.03 | 0.583 | 0.1062 | 0.0833 | 0.4433 | 0.3252 | 0.2379 | 0.552 |
| $a+b/\sqrt{x}+c/x^2y^2$ | 185.43 | 135.16 | 0.582 | 0.1063 | 0.0833 | 0.4423 | 0.3255 | 0.2381 | 0.551 |
| $a+b/\sqrt{x}+c/x^2\sqrt{y}$ | 185.43 | 135.23 | 0.582 | 0.1063 | 0.0833 | 0.4424 | 0.3256 | 0.2381 | 0.551 |
| $a+b/\sqrt{x}+cy/x^2$ | 190.63 | 138.83 | 0.558 | 0.1079 | 0.0844 | 0.4255 | 0.3324 | 0.2424 | 0.532 |
| $a+b/\sqrt{x}+cy^2/x^2$ | 201.26 | 147.37 | 0.507 | 0.1113 | 0.0864 | 0.3880 | 0.3480 | 0.2539 | 0.487 |
| $a+b/\sqrt{x}+c\sqrt{y}/x^2$ | 187.83 | 136.90 | 0.571 | 0.1070 | 0.0838 | 0.4348 | 0.3287 | 0.2400 | 0.542 |
| $a+b/\sqrt{x}+c/\sqrt{x}y$ | 231.07 | 160.24 | 0.350 | 0.1080 | 0.0839 | 0.4240 | 0.3633 | 0.2633 | 0.441 |
| $a+b/\sqrt{x}+c/\sqrt{x}y^2$ | 197.59 | 129.82 | 0.525 | 0.0965 | 0.0709 | 0.5402 | 0.3212 | 0.2247 | 0.563 |
| $a+b/\sqrt{x}+c/\sqrt{x}\sqrt{y}$ | 251.20 | 180.68 | 0.232 | 0.1170 | 0.0923 | 0.3245 | 0.3922 | 0.2891 | 0.348 |
| $a+b/\sqrt{x}+cy/\sqrt{x}$ | 220.86 | 169.09 | 0.407 | 0.1153 | 0.0869 | 0.3439 | 0.3773 | 0.2729 | 0.397 |
| $a+b/\sqrt{x}+cy^2/\sqrt{x}$ | 191.04 | 152.52 | 0.556 | 0.1050 | 0.0761 | 0.4561 | 0.3456 | 0.2419 | 0.494 |
| $a+b/\sqrt{x}+c\sqrt{y}/\sqrt{x}$ | 244.41 | 182.03 | 0.273 | 0.1219 | 0.0949 | 0.2666 | 0.4004 | 0.3029 | 0.321 |
| $a+b/\sqrt{x}+cx/z$ | 220.13 | 158.37 | 0.410 | 0.1053 | 0.0782 | 0.4522 | 0.3603 | 0.2630 | 0.450 |
| $a+b/\sqrt{x}+cx/z^2$ | 226.02 | 167.08 | 0.378 | 0.1117 | 0.0873 | 0.3840 | 0.3716 | 0.2750 | 0.415 |
| $a+b/\sqrt{x}+cx/\sqrt{z}$ | 258.37 | 191.17 | 0.188 | 0.1213 | 0.0934 | 0.2731 | 0.4084 | 0.3088 | 0.293 |
| $a+b/\sqrt{x}+cxz$ | 127.34 | 95.37 | 0.803 | 0.0705 | 0.0474 | 0.7546 | 0.2528 | 0.1769 | 0.729 |
| $a+b/\sqrt{x}+cxz^2$ | 146.07 | 109.94 | 0.740 | 0.0760 | 0.0551 | 0.7148 | 0.2757 | 0.1971 | 0.678 |
| $a+b/\sqrt{x}+cx\sqrt{z}$ | 114.46 | 88.10 | 0.841 | 0.0696 | 0.0444 | 0.7611 | 0.2397 | 0.1575 | 0.757 |
| $a+b/\sqrt{x}+cx^2/z$ | 259.00 | 192.20 | 0.184 | 0.1225 | 0.0948 | 0.2594 | 0.4098 | 0.3100 | 0.289 |
| $a+b/\sqrt{x}+cx^2/z^2$ | 238.30 | 174.35 | 0.309 | 0.1151 | 0.0900 | 0.3461 | 0.3865 | 0.2875 | 0.367 |
| $a+b/\sqrt{x}+cx^2/\sqrt{z}$ | 191.13 | 150.72 | 0.556 | 0.1052 | 0.0836 | 0.4534 | 0.3276 | 0.2548 | 0.545 |
| $a+b/\sqrt{x}+cx^2z$ | 133.49 | 102.93 | 0.783 | 0.0740 | 0.0533 | 0.7295 | 0.2640 | 0.1920 | 0.705 |
| $a+b/\sqrt{x}+cx^2z^2$ | 150.45 | 115.98 | 0.725 | 0.0795 | 0.0596 | 0.6881 | 0.2851 | 0.2113 | 0.656 |
| $a+b/\sqrt{x}+cx^2\sqrt{z}$ | 123.73 | 95.96 | 0.814 | 0.0729 | 0.0516 | 0.7376 | 0.2531 | 0.1796 | 0.729 |
| $a+b/\sqrt{x}+c\sqrt{x}/z$ | 192.62 | 136.46 | 0.549 | 0.0974 | 0.0700 | 0.5311 | 0.3271 | 0.2230 | 0.547 |
| $a+b/\sqrt{x}+c\sqrt{x}/z^2$ | 217.15 | 161.87 | 0.426 | 0.1098 | 0.0850 | 0.4048 | 0.3613 | 0.2666 | 0.447 |
| $a+b/\sqrt{x}+c\sqrt{x}/\sqrt{z}$ | 202.68 | 143.38 | 0.500 | 0.0971 | 0.0693 | 0.5347 | 0.3360 | 0.2391 | 0.522 |
| $a+b/\sqrt{x}+c\sqrt{x}z$ | 128.75 | 99.21 | 0.798 | 0.0701 | 0.0448 | 0.7574 | 0.2514 | 0.1691 | 0.732 |
| $a+b/\sqrt{x}+c\sqrt{x}z^2$ | 145.60 | 111.36 | 0.742 | 0.0749 | 0.0529 | 0.7232 | 0.2726 | 0.1915 | 0.685 |
| $a+b/\sqrt{x}+c\sqrt{x}\sqrt{z}$ | 117.30 | 90.79 | 0.833 | 0.0696 | 0.0409 | 0.7612 | 0.2399 | 0.1477 | 0.756 |
| $a+b/\sqrt{x}+c/xz$ | 259.00 | 193.49 | 0.184 | 0.1240 | 0.0992 | 0.2413 | 0.4103 | 0.3119 | 0.287 |
| $a+b/\sqrt{x}+c/xz^2$ | 241.31 | 172.33 | 0.292 | 0.1213 | 0.0937 | 0.2738 | 0.3928 | 0.2831 | 0.346 |
| $a+b/\sqrt{x}+c/x\sqrt{z}$ | 178.23 | 131.34 | 0.614 | 0.1002 | 0.0791 | 0.5038 | 0.3114 | 0.2310 | 0.589 |
| $a+b/\sqrt{x}+cz/x$ | 144.07 | 97.15 | 0.747 | 0.0898 | 0.0652 | 0.6022 | 0.2742 | 0.1778 | 0.681 |
| $a+b/\sqrt{x}+cz^2/x$ | 124.17 | 88.76 | 0.812 | 0.0746 | 0.0490 | 0.7254 | 0.2475 | 0.1583 | 0.740 |
| $a+b/\sqrt{x}+c\sqrt{z}/x$ | 159.18 | 112.24 | 0.692 | 0.0968 | 0.0732 | 0.5373 | 0.2933 | 0.1976 | 0.635 |
| $a+b/\sqrt{x}+c/x^2z$ | 169.72 | 125.88 | 0.650 | 0.1015 | 0.0796 | 0.4916 | 0.3066 | 0.2254 | 0.602 |
| $a+b/\sqrt{x}+c/x^2z^2$ | 132.36 | 96.83 | 0.787 | 0.0878 | 0.0657 | 0.6192 | 0.2586 | 0.1796 | 0.717 |
| $a+b/\sqrt{x}+c/x^2\sqrt{z}$ | 179.93 | 132.07 | 0.606 | 0.1046 | 0.0821 | 0.4596 | 0.3190 | 0.2341 | 0.569 |
| $a+b/\sqrt{x}+cz/x^2$ | 191.79 | 138.75 | 0.552 | 0.1081 | 0.0845 | 0.4235 | 0.3332 | 0.2417 | 0.530 |
| $a+b/\sqrt{x}+cz^2/x^2$ | 189.19 | 136.33 | 0.565 | 0.1070 | 0.0835 | 0.4349 | 0.3299 | 0.2375 | 0.539 |
| $a+b/\sqrt{x}+c\sqrt{z}/x^2$ | 189.97 | 137.81 | 0.561 | 0.1076 | 0.0842 | 0.4286 | 0.3311 | 0.2411 | 0.536 |
| $a+b/\sqrt{x}+c/\sqrt{x}z$ | 186.78 | 134.57 | 0.576 | 0.1035 | 0.0779 | 0.4716 | 0.3252 | 0.2279 | 0.552 |
| $a+b/\sqrt{x}+c/\sqrt{x}z^2$ | 211.96 | 155.59 | 0.453 | 0.1124 | 0.0875 | 0.3762 | 0.3581 | 0.2637 | 0.457 |
| $a+b/\sqrt{x}+c/\sqrt{x}\sqrt{z}$ | 168.38 | 116.75 | 0.655 | 0.0961 | 0.0708 | 0.5443 | 0.3011 | 0.1963 | 0.616 |
| $a+b/\sqrt{x}+cz/\sqrt{x}$ | 129.36 | 99.86 | 0.796 | 0.0733 | 0.0471 | 0.7344 | 0.2493 | 0.1530 | 0.737 |
| $a+b/\sqrt{x}+cz^2/\sqrt{x}$ | 141.72 | 109.14 | 0.756 | 0.0733 | 0.0503 | 0.7349 | 0.2637 | 0.1848 | 0.705 |
| $a+b/\sqrt{x}+c\sqrt{z}/\sqrt{x}$ | 133.78 | 98.50 | 0.782 | 0.0786 | 0.0519 | 0.6946 | 0.2560 | 0.1563 | 0.722 |
| $a+b/\sqrt{x}+cy/z$ | 205.12 | 151.14 | 0.488 | 0.0989 | 0.0727 | 0.5175 | 0.3353 | 0.2427 | 0.524 |
| $a+b/\sqrt{x}+cy/z^2$ | 217.91 | 161.90 | 0.422 | 0.1089 | 0.0840 | 0.4142 | 0.3601 | 0.2638 | 0.450 |
| $a+b/\sqrt{x}+cy/\sqrt{z}$ | 244.87 | 176.18 | 0.270 | 0.1123 | 0.0863 | 0.3768 | 0.3823 | 0.2880 | 0.381 |
| $a+b/\sqrt{x}+cyz$ | 134.93 | 105.63 | 0.778 | 0.0749 | 0.0488 | 0.7229 | 0.2670 | 0.1825 | 0.698 |
| $a+b/\sqrt{x}+cyz^2$ | 149.44 | 115.44 | 0.728 | 0.0780 | 0.0555 | 0.6993 | 0.2819 | 0.1985 | 0.663 |
| $a+b/\sqrt{x}+cy\sqrt{z}$ | 131.01 | 100.80 | 0.791 | 0.0776 | 0.0477 | 0.7027 | 0.2673 | 0.1661 | 0.697 |
| $a+b/\sqrt{x}+cy^2/z$ | 245.48 | 175.96 | 0.267 | 0.1132 | 0.0864 | 0.3675 | 0.3844 | 0.2890 | 0.374 |
| $a+b/\sqrt{x}+cy^2/z^2$ | 226.12 | 165.05 | 0.378 | 0.1097 | 0.0842 | 0.4054 | 0.3674 | 0.2695 | 0.428 |
| $a+b/\sqrt{x}+cy^2/\sqrt{z}$ | 245.01 | 198.27 | 0.270 | 0.1224 | 0.0977 | 0.2607 | 0.4011 | 0.3163 | 0.318 |
| $a+b/\sqrt{x}+cy^2z$ | 144.26 | 110.43 | 0.747 | 0.0801 | 0.0548 | 0.6830 | 0.2833 | 0.1920 | 0.660 |
| $a+b/\sqrt{x}+cy^2z^2$ | 155.21 | 119.21 | 0.707 | 0.0822 | 0.0597 | 0.6660 | 0.2937 | 0.2105 | 0.635 |
| $a+b/\sqrt{x}+cy^2\sqrt{z}$ | 143.65 | 104.98 | 0.749 | 0.0830 | 0.0553 | 0.6600 | 0.2861 | 0.1838 | 0.653 |
| $a+b/\sqrt{x}+c\sqrt{y}/z$ | 185.41 | 133.28 | 0.582 | 0.0949 | 0.0678 | 0.5553 | 0.3154 | 0.2128 | 0.578 |
| $a+b/\sqrt{x}+c\sqrt{y}/z^2$ | 212.83 | 158.90 | 0.449 | 0.1086 | 0.0833 | 0.4176 | 0.3556 | 0.2606 | 0.464 |
| $a+b/\sqrt{x}+c\sqrt{y}/\sqrt{z}$ | 192.97 | 144.22 | 0.547 | 0.0926 | 0.0691 | 0.5769 | 0.3167 | 0.2299 | 0.575 |

(continued on next page)

**Table 4 – continued from previous page**

| Functional form | $T_{eff}$ (K) | | | Radius ($R_{\odot}$) | | | log (L/$L_{\odot}$) | | |
|---|---|---|---|---|---|---|---|---|---|
| | RMSE | MAD | $R^2_{ap}$ | RMSE | MAD | $R^2_{ap}$ | RMSE | MAD | $R^2_{ap}$ |
| $a+b/\sqrt{x}+c\sqrt{y}z$ | 131.96 | 105.40 | 0.788 | 0.0724 | 0.0454 | 0.7409 | 0.2588 | 0.1734 | 0.716 |
| $a+b/\sqrt{x}+c\sqrt{y}z^2$ | 147.15 | 114.55 | 0.737 | 0.0760 | 0.0533 | 0.7150 | 0.2759 | 0.1923 | 0.678 |
| $a+b/\sqrt{x}+c\sqrt{y}\sqrt{z}$ | 125.72 | 99.62 | 0.808 | 0.0743 | 0.0431 | 0.7277 | 0.2561 | 0.1576 | 0.722 |
| $a+b/\sqrt{x}+c/yz$ | 201.16 | 142.82 | 0.508 | 0.1099 | 0.0835 | 0.4032 | 0.3455 | 0.2481 | 0.494 |
| $a+b/\sqrt{x}+c/yz^2$ | 215.70 | 157.42 | 0.434 | 0.1144 | 0.0887 | 0.3538 | 0.3636 | 0.2685 | 0.440 |
| $a+b/\sqrt{x}+c/y\sqrt{z}$ | 196.93 | 134.05 | 0.528 | 0.1087 | 0.0809 | 0.4166 | 0.3413 | 0.2382 | 0.507 |
| $a+b/\sqrt{x}+cz/y$ | 163.28 | 130.83 | 0.676 | 0.0792 | 0.0606 | 0.6906 | 0.2733 | 0.2074 | 0.684 |
| $a+b/\sqrt{x}+cz^2/y$ | 148.31 | 113.19 | 0.732 | 0.0733 | 0.0533 | 0.7348 | 0.2632 | 0.1873 | 0.706 |
| $a+b/\sqrt{x}+c\sqrt{z}/y$ | 228.38 | 164.52 | 0.365 | 0.1041 | 0.0826 | 0.4652 | 0.3552 | 0.2721 | 0.465 |
| $a+b/\sqrt{x}+c/y^2z$ | 241.49 | 176.14 | 0.290 | 0.1215 | 0.0952 | 0.2713 | 0.3927 | 0.2903 | 0.347 |
| $a+b/\sqrt{x}+c/y^2z^2$ | 239.03 | 174.84 | 0.305 | 0.1210 | 0.0947 | 0.2769 | 0.3903 | 0.2880 | 0.355 |
| $a+b/\sqrt{x}+c/y^2\sqrt{z}$ | 245.34 | 177.52 | 0.268 | 0.1223 | 0.0955 | 0.2615 | 0.3971 | 0.2926 | 0.332 |
| $a+b/\sqrt{x}+cz/y^2$ | 189.59 | 138.97 | 0.563 | 0.0901 | 0.0712 | 0.5993 | 0.3013 | 0.2341 | 0.615 |
| $a+b/\sqrt{x}+cz^2/y^2$ | 152.32 | 119.90 | 0.718 | 0.0772 | 0.0586 | 0.7056 | 0.2608 | 0.1955 | 0.712 |
| $a+b/\sqrt{x}+c\sqrt{z}/y^2$ | 254.26 | 183.65 | 0.213 | 0.1180 | 0.0919 | 0.3120 | 0.3975 | 0.2914 | 0.331 |
| $a+b/\sqrt{x}+c/\sqrt{y}z$ | 177.56 | 125.10 | 0.616 | 0.1006 | 0.0754 | 0.5002 | 0.3158 | 0.2163 | 0.577 |
| $a+b/\sqrt{x}+c/\sqrt{y}z^2$ | 207.53 | 151.16 | 0.476 | 0.1106 | 0.0859 | 0.3955 | 0.3530 | 0.2573 | 0.472 |
| $a+b/\sqrt{x}+c/\sqrt{y}\sqrt{z}$ | 160.81 | 110.19 | 0.685 | 0.0952 | 0.0707 | 0.5527 | 0.2973 | 0.1927 | 0.625 |
| $a+b/\sqrt{x}+cz/\sqrt{y}$ | 143.91 | 115.54 | 0.748 | 0.0731 | 0.0515 | 0.7363 | 0.2575 | 0.1796 | 0.719 |
| $a+b/\sqrt{x}+cz^2/\sqrt{y}$ | 146.16 | 110.78 | 0.740 | 0.0732 | 0.0509 | 0.7357 | 0.2658 | 0.1863 | 0.701 |
| $a+b/\sqrt{x}+c\sqrt{z}/\sqrt{y}$ | 171.39 | 135.59 | 0.643 | 0.0822 | 0.0626 | 0.6662 | 0.2845 | 0.2120 | 0.657 |
| Single line EW, single EW ratio, double component functions result ( (y, x/y) ; (y, x/z) ; (y, y/z) ) | | | | | | | | | |
| $a+by+cx/y$ | 173.69 | 133.40 | 0.633 | 0.0937 | 0.0723 | 0.5661 | 0.2957 | 0.2080 | 0.629 |
| $a+by+cx/y^2$ | 176.09 | 139.17 | 0.623 | 0.0948 | 0.0714 | 0.5559 | 0.3086 | 0.2168 | 0.596 |
| $a+by+cx/\sqrt{y}$ | 167.86 | 127.16 | 0.657 | 0.0905 | 0.0695 | 0.5957 | 0.2812 | 0.1966 | 0.665 |
| $a+by+cxy$ | 132.86 | 102.71 | 0.785 | 0.0822 | 0.0596 | 0.6667 | 0.2759 | 0.1985 | 0.677 |
| $a+by+cxy^2$ | 150.99 | 116.67 | 0.723 | 0.0906 | 0.0646 | 0.5948 | 0.3041 | 0.2073 | 0.608 |
| $a+by+cx\sqrt{y}$ | 127.82 | 101.00 | 0.801 | 0.0764 | 0.0520 | 0.7116 | 0.2463 | 0.1721 | 0.743 |
| $a+by+cx^2/y$ | 147.09 | 112.44 | 0.737 | 0.0826 | 0.0619 | 0.6630 | 0.2539 | 0.1757 | 0.727 |
| $a+by+cx^2/y^2$ | 166.69 | 126.03 | 0.662 | 0.0911 | 0.0696 | 0.5902 | 0.2831 | 0.1975 | 0.660 |
| $a+by+cx^2/\sqrt{y}$ | 132.58 | 107.64 | 0.786 | 0.0778 | 0.0549 | 0.7015 | 0.2447 | 0.1734 | 0.746 |
| $a+by+cx^2y$ | 139.64 | 110.53 | 0.763 | 0.0852 | 0.0623 | 0.6412 | 0.2879 | 0.2052 | 0.649 |
| $a+by+cx^2y^2$ | 150.23 | 118.49 | 0.725 | 0.0900 | 0.0645 | 0.5996 | 0.3027 | 0.2069 | 0.612 |
| $a+by+cx^2\sqrt{y}$ | 131.72 | 104.44 | 0.789 | 0.0812 | 0.0591 | 0.6741 | 0.2730 | 0.1979 | 0.684 |
| $a+by+c\sqrt{x}/y$ | 176.02 | 138.97 | 0.623 | 0.0945 | 0.0712 | 0.5593 | 0.3065 | 0.2161 | 0.602 |
| $a+by+c\sqrt{x}/y^2$ | 173.82 | 139.97 | 0.632 | 0.0963 | 0.0685 | 0.5422 | 0.3175 | 0.2182 | 0.573 |
| $a+by+c\sqrt{x}/\sqrt{y}$ | 176.21 | 138.59 | 0.622 | 0.0955 | 0.0732 | 0.5500 | 0.3044 | 0.2133 | 0.607 |
| $a+by+c\sqrt{x}y$ | 130.31 | 98.40 | 0.793 | 0.0796 | 0.0566 | 0.6872 | 0.2649 | 0.1875 | 0.703 |
| $a+by+c\sqrt{x}y^2$ | 154.75 | 119.32 | 0.709 | 0.0922 | 0.0653 | 0.5799 | 0.3083 | 0.2076 | 0.597 |
| $a+by+c\sqrt{x}\sqrt{y}$ | 155.40 | 114.99 | 0.706 | 0.0837 | 0.0621 | 0.6543 | 0.2586 | 0.1772 | 0.717 |
| $a+by+c/xy$ | 163.16 | 124.38 | 0.676 | 0.0976 | 0.0688 | 0.5294 | 0.3171 | 0.2116 | 0.574 |
| $a+by+c/xy^2$ | 162.66 | 123.72 | 0.678 | 0.0976 | 0.0688 | 0.5300 | 0.3169 | 0.2112 | 0.574 |
| $a+by+c/x\sqrt{y}$ | 163.74 | 125.06 | 0.674 | 0.0977 | 0.0688 | 0.5287 | 0.3174 | 0.2121 | 0.573 |
| $a+by+cy/x$ | 171.02 | 133.45 | 0.644 | 0.0981 | 0.0714 | 0.5246 | 0.3183 | 0.2173 | 0.571 |
| $a+by+cy^2/x$ | 175.97 | 138.76 | 0.623 | 0.0937 | 0.0713 | 0.5667 | 0.3009 | 0.2126 | 0.616 |
| $a+by+c\sqrt{y}/x$ | 167.09 | 128.84 | 0.660 | 0.0980 | 0.0698 | 0.5253 | 0.3183 | 0.2146 | 0.571 |
| $a+by+c/x^2y$ | 162.27 | 122.79 | 0.680 | 0.0977 | 0.0691 | 0.5284 | 0.3167 | 0.2093 | 0.575 |
| $a+by+c/x^2y^2$ | 162.21 | 122.83 | 0.680 | 0.0977 | 0.0691 | 0.5284 | 0.3167 | 0.2092 | 0.575 |
| $a+by+c/x^2\sqrt{y}$ | 162.34 | 122.80 | 0.679 | 0.0977 | 0.0691 | 0.5284 | 0.3167 | 0.2094 | 0.575 |
| $a+by+cy/x^2$ | 163.24 | 123.85 | 0.676 | 0.0978 | 0.0691 | 0.5275 | 0.3171 | 0.2103 | 0.574 |
| $a+by+cy^2/x^2$ | 165.86 | 126.83 | 0.665 | 0.0980 | 0.0700 | 0.5253 | 0.3180 | 0.2129 | 0.572 |
| $a+by+c\sqrt{y}/x^2$ | 162.74 | 123.26 | 0.678 | 0.0978 | 0.0691 | 0.5280 | 0.3169 | 0.2098 | 0.574 |
| $a+by+c/\sqrt{x}y$ | 165.24 | 128.52 | 0.668 | 0.0976 | 0.0684 | 0.5299 | 0.3177 | 0.2139 | 0.572 |
| $a+by+c/\sqrt{x}y^2$ | 164.38 | 127.53 | 0.671 | 0.0974 | 0.0685 | 0.5313 | 0.3174 | 0.2133 | 0.573 |
| $a+by+c/\sqrt{x}\sqrt{y}$ | 166.40 | 129.70 | 0.663 | 0.0978 | 0.0686 | 0.5280 | 0.3181 | 0.2146 | 0.571 |
| $a+by+cy/\sqrt{x}$ | 175.96 | 138.76 | 0.623 | 0.0939 | 0.0710 | 0.5648 | 0.3026 | 0.2139 | 0.612 |
| $a+by+cy^2/\sqrt{x}$ | 174.60 | 135.31 | 0.629 | 0.0937 | 0.0728 | 0.5666 | 0.2935 | 0.2080 | 0.635 |
| $a+by+c\sqrt{y}/\sqrt{x}$ | 174.25 | 137.87 | 0.631 | 0.0978 | 0.0725 | 0.5276 | 0.3166 | 0.2183 | 0.575 |
| $a+by+cx/z$ | 159.53 | 124.71 | 0.690 | 0.0928 | 0.0643 | 0.5744 | 0.3089 | 0.2042 | 0.596 |
| $a+by+cx/z^2$ | 165.84 | 132.27 | 0.665 | 0.0956 | 0.0680 | 0.5485 | 0.3125 | 0.2140 | 0.586 |
| $a+by+cx/\sqrt{z}$ | 167.68 | 129.29 | 0.658 | 0.0956 | 0.0662 | 0.5483 | 0.3167 | 0.2121 | 0.575 |
| $a+by+cxz$ | 123.01 | 94.16 | 0.816 | 0.0725 | 0.0492 | 0.7403 | 0.2592 | 0.1818 | 0.715 |
| $a+by+cxz^2$ | 132.62 | 102.22 | 0.786 | 0.0780 | 0.0540 | 0.6996 | 0.2762 | 0.1891 | 0.677 |
| $a+by+cx\sqrt{z}$ | 117.05 | 90.76 | 0.833 | 0.0689 | 0.0457 | 0.7654 | 0.2417 | 0.1607 | 0.752 |
| $a+by+cx^2/z$ | 171.00 | 131.08 | 0.644 | 0.0958 | 0.0661 | 0.5466 | 0.3171 | 0.2129 | 0.574 |
| $a+by+cx^2/z^2$ | 168.59 | 133.73 | 0.654 | 0.0959 | 0.0678 | 0.5460 | 0.3149 | 0.2151 | 0.580 |
| $a+by+cx^2/\sqrt{z}$ | 173.85 | 139.73 | 0.632 | 0.0972 | 0.0741 | 0.5338 | 0.3075 | 0.2247 | 0.599 |
| $a+by+cx^2z$ | 127.88 | 98.90 | 0.801 | 0.0770 | 0.0555 | 0.7073 | 0.2716 | 0.1907 | 0.687 |
| $a+by+cx^2z^2$ | 135.97 | 104.72 | 0.775 | 0.0811 | 0.0571 | 0.6751 | 0.2835 | 0.1896 | 0.659 |
| $a+by+cx^2\sqrt{z}$ | 122.41 | 96.39 | 0.818 | 0.0749 | 0.0544 | 0.7232 | 0.2617 | 0.1875 | 0.710 |
| $a+by+c\sqrt{x}/z$ | 152.69 | 118.23 | 0.716 | 0.0915 | 0.0636 | 0.5870 | 0.3020 | 0.2002 | 0.614 |
| $a+by+c\sqrt{x}/z^2$ | 164.03 | 129.99 | 0.673 | 0.0956 | 0.0685 | 0.5492 | 0.3106 | 0.2116 | 0.591 |
| $a+by+c\sqrt{x}/\sqrt{z}$ | 153.75 | 117.90 | 0.712 | 0.0919 | 0.0636 | 0.5833 | 0.3064 | 0.2023 | 0.602 |
| $a+by+c\sqrt{x}z$ | 123.55 | 95.65 | 0.814 | 0.0716 | 0.0462 | 0.7467 | 0.2559 | 0.1751 | 0.722 |
| $a+by+c\sqrt{x}z^2$ | 131.69 | 101.58 | 0.789 | 0.0767 | 0.0527 | 0.7093 | 0.2729 | 0.1873 | 0.685 |
| $a+by+c\sqrt{x}\sqrt{z}$ | 122.11 | 92.14 | 0.819 | 0.0690 | 0.0425 | 0.7649 | 0.2404 | 0.1491 | 0.755 |
| $a+by+c/xz$ | 169.79 | 135.05 | 0.649 | 0.0980 | 0.0696 | 0.5255 | 0.3185 | 0.2158 | 0.570 |
| $a+by+c/xz^2$ | 174.82 | 141.47 | 0.628 | 0.0981 | 0.0700 | 0.5252 | 0.3181 | 0.2151 | 0.571 |
| $a+by+c/x\sqrt{z}$ | 167.35 | 130.78 | 0.659 | 0.0980 | 0.0694 | 0.5260 | 0.3183 | 0.2149 | 0.571 |
| $a+by+cz/x$ | 156.73 | 116.90 | 0.701 | 0.0966 | 0.0693 | 0.5393 | 0.3138 | 0.2086 | 0.583 |
| $a+by+cz^2/x$ | 138.46 | 98.11 | 0.767 | 0.0903 | 0.0639 | 0.5975 | 0.2979 | 0.1893 | 0.624 |
| $a+by+c\sqrt{z}/x$ | 161.70 | 120.99 | 0.682 | 0.0975 | 0.0690 | 0.5307 | 0.3165 | 0.2094 | 0.575 |
| $a+by+c/x^2z$ | 162.68 | 122.84 | 0.678 | 0.0977 | 0.0690 | 0.5287 | 0.3169 | 0.2104 | 0.574 |
| $a+by+c/x^2z^2$ | 163.36 | 125.11 | 0.675 | 0.0976 | 0.0688 | 0.5298 | 0.3171 | 0.2118 | 0.574 |
| $a+by+c/x^2\sqrt{z}$ | 162.56 | 122.59 | 0.678 | 0.0977 | 0.0691 | 0.5284 | 0.3169 | 0.2100 | 0.575 |
| $a+by+cz/x^2$ | 162.22 | 123.38 | 0.680 | 0.0977 | 0.0692 | 0.5282 | 0.3166 | 0.2088 | 0.575 |
| $a+by+cz^2/x^2$ | 161.32 | 123.17 | 0.683 | 0.0976 | 0.0693 | 0.5293 | 0.3161 | 0.2089 | 0.577 |
| $a+by+c\sqrt{z}/x^2$ | 162.38 | 123.19 | 0.679 | 0.0978 | 0.0691 | 0.5282 | 0.3167 | 0.2092 | 0.575 |
| $a+by+c/\sqrt{x}z$ | 175.63 | 135.06 | 0.625 | 0.0967 | 0.0722 | 0.5387 | 0.3076 | 0.2120 | 0.599 |
| $a+by+c/\sqrt{x}z^2$ | 172.36 | 129.51 | 0.639 | 0.0974 | 0.0721 | 0.5314 | 0.3109 | 0.2139 | 0.590 |
| $a+by+c/\sqrt{x}\sqrt{z}$ | 176.31 | 141.08 | 0.622 | 0.0975 | 0.0722 | 0.5310 | 0.3134 | 0.2106 | 0.584 |
| $a+by+cz/\sqrt{x}$ | 134.68 | 98.33 | 0.779 | 0.0877 | 0.0604 | 0.6204 | 0.2920 | 0.1838 | 0.639 |
| $a+by+cz^2/\sqrt{x}$ | 127.92 | 98.85 | 0.801 | 0.0785 | 0.0505 | 0.6961 | 0.2738 | 0.1803 | 0.682 |

(continued on next page)

**Table 4 – continued from previous page**

| Functional form | $T_{eff}$ (K) | | | Radius ($R_\odot$) | | | log (L/$L_\odot$) | | |
|---|---|---|---|---|---|---|---|---|---|
| | RMSE | MAD | $R^2_{ap}$ | RMSE | MAD | $R^2_{ap}$ | RMSE | MAD | $R^2_{ap}$ |
| $a+by+c\sqrt{z}/\sqrt{x}$ | 152.47 | 113.24 | 0.717 | 0.0949 | 0.0682 | 0.5551 | 0.3105 | 0.2070 | 0.591 |
| a+by+cy/z | 143.75 | 109.19 | 0.749 | 0.0865 | 0.0571 | 0.6307 | 0.2884 | 0.1847 | 0.648 |
| $a+by+cy/z^2$ | 160.89 | 127.27 | 0.685 | 0.0941 | 0.0672 | 0.5630 | 0.3066 | 0.2077 | 0.602 |
| $a+by+cy/\sqrt{z}$ | 135.35 | 103.00 | 0.777 | 0.0818 | 0.0525 | 0.6693 | 0.2792 | 0.1723 | 0.670 |
| a+by+cyz | 132.51 | 102.09 | 0.786 | 0.0780 | 0.0530 | 0.6993 | 0.2768 | 0.1860 | 0.675 |
| $a+by+cyz^2$ | 137.31 | 105.30 | 0.771 | 0.0805 | 0.0549 | 0.6801 | 0.2833 | 0.1871 | 0.660 |
| $a+by+cy\sqrt{z}$ | 130.66 | 101.53 | 0.792 | 0.0776 | 0.0514 | 0.7025 | 0.2743 | 0.1814 | 0.681 |
| $a+by+cy^2/z$ | 140.23 | 106.22 | 0.761 | 0.0820 | 0.0516 | 0.6679 | 0.2793 | 0.1671 | 0.669 |
| $a+by+cy^2/z^2$ | 158.09 | 124.30 | 0.696 | 0.0921 | 0.0642 | 0.5812 | 0.3030 | 0.2025 | 0.611 |
| $a+by+cy^2/\sqrt{z}$ | 136.88 | 101.85 | 0.772 | 0.0760 | 0.0455 | 0.7151 | 0.2622 | 0.1567 | 0.709 |
| $a+by+cy^2z$ | 141.38 | 104.29 | 0.757 | 0.0838 | 0.0580 | 0.6531 | 0.2921 | 0.1892 | 0.639 |
| $a+by+cy^2z^2$ | 142.53 | 108.44 | 0.753 | 0.0843 | 0.0578 | 0.6493 | 0.2926 | 0.1880 | 0.637 |
| $a+by+cy^2\sqrt{z}$ | 143.98 | 104.77 | 0.748 | 0.0858 | 0.0594 | 0.6365 | 0.2966 | 0.1912 | 0.627 |
| $a+by+c\sqrt{y}/z$ | 145.29 | 109.60 | 0.743 | 0.0882 | 0.0600 | 0.6161 | 0.2900 | 0.1866 | 0.644 |
| $a+by+c\sqrt{y}/z^2$ | 162.00 | 127.29 | 0.681 | 0.0949 | 0.0685 | 0.5552 | 0.3076 | 0.2081 | 0.599 |
| $a+by+c\sqrt{y}/\sqrt{z}$ | 135.96 | 101.93 | 0.775 | 0.0837 | 0.0543 | 0.6542 | 0.2811 | 0.1774 | 0.665 |
| $a+by+c\sqrt{y}z$ | 127.99 | 100.50 | 0.801 | 0.0753 | 0.0494 | 0.7203 | 0.2675 | 0.1807 | 0.697 |
| $a+by+c\sqrt{y}z^2$ | 134.21 | 103.12 | 0.781 | 0.0783 | 0.0534 | 0.6973 | 0.2774 | 0.1869 | 0.674 |
| $a+by+c\sqrt{y}\sqrt{z}$ | 126.01 | 99.67 | 0.807 | 0.0746 | 0.0451 | 0.7252 | 0.2622 | 0.1688 | 0.709 |
| a+by+c/yz | 174.59 | 133.84 | 0.629 | 0.0978 | 0.0715 | 0.5280 | 0.3117 | 0.2135 | 0.588 |
| $a+by+c/yz^2$ | 172.51 | 131.17 | 0.638 | 0.0979 | 0.0713 | 0.5263 | 0.3137 | 0.2151 | 0.583 |
| $a+by+c/y\sqrt{z}$ | 176.65 | 139.72 | 0.620 | 0.0981 | 0.0716 | 0.5252 | 0.3147 | 0.2140 | 0.580 |
| a+by+cz/y | 123.23 | 90.55 | 0.815 | 0.0814 | 0.0532 | 0.6728 | 0.2740 | 0.1718 | 0.682 |
| $a+by+cz^2/y$ | 122.75 | 95.46 | 0.817 | 0.0746 | 0.0468 | 0.7253 | 0.2611 | 0.1732 | 0.711 |
| $a+by+c\sqrt{z}/y$ | 141.05 | 106.86 | 0.758 | 0.0900 | 0.0622 | 0.6005 | 0.2987 | 0.1990 | 0.622 |
| $a+by+c/y^2z$ | 175.77 | 141.51 | 0.624 | 0.0978 | 0.0690 | 0.5273 | 0.3183 | 0.2145 | 0.571 |
| $a+by+c/y^2z^2$ | 176.61 | 139.29 | 0.621 | 0.0980 | 0.0697 | 0.5260 | 0.3178 | 0.2143 | 0.572 |
| $a+by+c/y^2\sqrt{z}$ | 173.32 | 139.93 | 0.634 | 0.0976 | 0.0681 | 0.5292 | 0.3185 | 0.2159 | 0.570 |
| $a+by+cz/y^2$ | 150.06 | 113.42 | 0.726 | 0.0942 | 0.0671 | 0.5620 | 0.3086 | 0.2085 | 0.596 |
| $a+by+cz^2/y^2$ | 125.31 | 90.29 | 0.809 | 0.0845 | 0.0574 | 0.6478 | 0.2806 | 0.1771 | 0.666 |
| $a+by+c\sqrt{z}/y^2$ | 160.66 | 122.99 | 0.686 | 0.0963 | 0.0677 | 0.5425 | 0.3152 | 0.2113 | 0.579 |
| $a+by+c/\sqrt{y}z$ | 161.97 | 121.42 | 0.681 | 0.0945 | 0.0693 | 0.5592 | 0.2983 | 0.1984 | 0.623 |
| $a+by+c/\sqrt{y}z^2$ | 167.31 | 128.67 | 0.659 | 0.0970 | 0.0714 | 0.5353 | 0.3103 | 0.2117 | 0.592 |
| $a+by+c/\sqrt{y}\sqrt{z}$ | 164.32 | 119.53 | 0.671 | 0.0934 | 0.0689 | 0.5691 | 0.2933 | 0.1941 | 0.636 |
| $a+by+cz/\sqrt{y}$ | 120.97 | 93.74 | 0.822 | 0.0755 | 0.0458 | 0.7183 | 0.2607 | 0.1657 | 0.712 |
| $a+by+cz^2/\sqrt{y}$ | 127.06 | 99.77 | 0.804 | 0.0747 | 0.0484 | 0.7247 | 0.2647 | 0.1790 | 0.703 |
| $a+by+c\sqrt{z}/\sqrt{y}$ | 125.11 | 91.02 | 0.810 | 0.0810 | 0.0521 | 0.6761 | 0.2735 | 0.1707 | 0.683 |
| $a+by^2+cx/y$ | 156.38 | 121.58 | 0.702 | 0.0877 | 0.0649 | 0.6203 | 0.2794 | 0.1933 | 0.669 |
| $a+by^2+cx/y^2$ | 164.53 | 130.77 | 0.671 | 0.0920 | 0.0679 | 0.5820 | 0.3115 | 0.2179 | 0.589 |
| $a+by^2+cx/\sqrt{y}$ | 152.91 | 118.11 | 0.716 | 0.0863 | 0.0643 | 0.6320 | 0.2706 | 0.1847 | 0.690 |
| $a+by^2+cxy$ | 126.33 | 98.64 | 0.806 | 0.0757 | 0.0525 | 0.7171 | 0.2465 | 0.1733 | 0.743 |
| $a+by^2+cxy^2$ | 150.64 | 115.94 | 0.724 | 0.0907 | 0.0679 | 0.5934 | 0.3120 | 0.2290 | 0.588 |
| $a+by^2+cx\sqrt{y}$ | 136.54 | 104.15 | 0.773 | 0.0786 | 0.0561 | 0.6948 | 0.2430 | 0.1639 | 0.750 |
| $a+by^2+cx^2/y$ | 136.61 | 104.27 | 0.773 | 0.0804 | 0.0574 | 0.6811 | 0.2497 | 0.1691 | 0.736 |
| $a+by^2+cx^2/y^2$ | 146.55 | 112.39 | 0.739 | 0.0848 | 0.0613 | 0.6448 | 0.2662 | 0.1784 | 0.700 |
| $a+by^2+cx^2/\sqrt{y}$ | 130.44 | 102.62 | 0.793 | 0.0777 | 0.0547 | 0.7016 | 0.2447 | 0.1738 | 0.746 |
| $a+by^2+cx^2y$ | 139.83 | 111.24 | 0.762 | 0.0850 | 0.0644 | 0.6429 | 0.2931 | 0.2195 | 0.636 |
| $a+by^2+cx^2y^2$ | 154.35 | 119.61 | 0.710 | 0.0924 | 0.0688 | 0.5785 | 0.3165 | 0.2287 | 0.576 |
| $a+by^2+cx^2\sqrt{y}$ | 130.28 | 103.06 | 0.793 | 0.0796 | 0.0591 | 0.6869 | 0.2699 | 0.2004 | 0.691 |
| $a+by^2+c\sqrt{x}/y$ | 163.57 | 129.72 | 0.674 | 0.0908 | 0.0672 | 0.5933 | 0.3068 | 0.2167 | 0.601 |
| $a+by^2+c\sqrt{x}/y^2$ | 166.66 | 133.17 | 0.662 | 0.0967 | 0.0671 | 0.5379 | 0.3194 | 0.2103 | 0.568 |
| $a+by^2+c\sqrt{x}/\sqrt{y}$ | 161.60 | 128.28 | 0.682 | 0.0899 | 0.0662 | 0.6007 | 0.2902 | 0.2011 | 0.643 |
| $a+by^2+c\sqrt{x}y$ | 148.18 | 114.16 | 0.733 | 0.0833 | 0.0619 | 0.6570 | 0.2570 | 0.1741 | 0.720 |
| $a+by^2+c\sqrt{x}y^2$ | 147.94 | 113.09 | 0.734 | 0.0895 | 0.0671 | 0.6048 | 0.3079 | 0.2276 | 0.598 |
| $a+by^2+c\sqrt{x}\sqrt{y}$ | 157.79 | 124.33 | 0.697 | 0.0888 | 0.0668 | 0.6111 | 0.2786 | 0.1919 | 0.671 |
| $a+by^2+c/xy$ | 164.68 | 127.89 | 0.670 | 0.0965 | 0.0667 | 0.5406 | 0.3211 | 0.2173 | 0.563 |
| $a+by^2+c/xy^2$ | 164.46 | 127.45 | 0.671 | 0.0965 | 0.0666 | 0.5402 | 0.3214 | 0.2172 | 0.562 |
| $a+by^2+c/x\sqrt{y}$ | 164.86 | 128.25 | 0.669 | 0.0964 | 0.0667 | 0.5411 | 0.3209 | 0.2175 | 0.564 |
| $a+by^2+cy/x$ | 166.47 | 131.84 | 0.663 | 0.0953 | 0.0677 | 0.5519 | 0.3165 | 0.2172 | 0.576 |
| $a+by^2+cy^2/x$ | 160.78 | 127.12 | 0.685 | 0.0870 | 0.0646 | 0.6262 | 0.2907 | 0.2057 | 0.642 |
| $a+by^2+c\sqrt{y}/x$ | 165.67 | 129.93 | 0.666 | 0.0960 | 0.0670 | 0.5446 | 0.3193 | 0.2178 | 0.568 |
| $a+by^2+c/x^2y$ | 162.96 | 124.59 | 0.677 | 0.0966 | 0.0667 | 0.5394 | 0.3226 | 0.2178 | 0.559 |
| $a+by^2+c/x^2y^2$ | 162.89 | 124.46 | 0.677 | 0.0966 | 0.0667 | 0.5394 | 0.3226 | 0.2178 | 0.559 |
| $a+by^2+c/x^2\sqrt{y}$ | 163.01 | 124.69 | 0.677 | 0.0966 | 0.0667 | 0.5395 | 0.3225 | 0.2178 | 0.559 |
| $a+by^2+cy/x^2$ | 163.40 | 125.41 | 0.675 | 0.0965 | 0.0669 | 0.5401 | 0.3223 | 0.2180 | 0.560 |
| $a+by^2+cy^2/x^2$ | 164.36 | 127.25 | 0.671 | 0.0963 | 0.0672 | 0.5424 | 0.3214 | 0.2185 | 0.562 |
| $a+by^2+c\sqrt{y}/x^2$ | 163.20 | 125.04 | 0.676 | 0.0965 | 0.0668 | 0.5397 | 0.3224 | 0.2179 | 0.560 |
| $a+by^2+c/\sqrt{x}y$ | 166.00 | 130.74 | 0.665 | 0.0963 | 0.0664 | 0.5420 | 0.3191 | 0.2163 | 0.568 |
| $a+by^2+c/\sqrt{x}y^2$ | 165.78 | 130.23 | 0.666 | 0.0964 | 0.0664 | 0.5411 | 0.3198 | 0.2162 | 0.567 |
| $a+by^2+c/\sqrt{x}\sqrt{y}$ | 166.20 | 131.19 | 0.664 | 0.0962 | 0.0665 | 0.5434 | 0.3183 | 0.2163 | 0.571 |
| $a+by^2+cy/\sqrt{x}$ | 161.61 | 127.66 | 0.682 | 0.0882 | 0.0656 | 0.6161 | 0.2960 | 0.2094 | 0.629 |
| $a+by^2+cy^2/\sqrt{x}$ | 142.62 | 107.17 | 0.753 | 0.0830 | 0.0608 | 0.6595 | 0.2850 | 0.2026 | 0.656 |
| $a+by^2+c\sqrt{y}/\sqrt{x}$ | 166.75 | 133.40 | 0.662 | 0.0941 | 0.0679 | 0.5631 | 0.3106 | 0.2131 | 0.591 |
| $a+by^2+cx/z$ | 160.45 | 124.45 | 0.687 | 0.0951 | 0.0682 | 0.5537 | 0.3221 | 0.2220 | 0.561 |
| $a+by^2+cx/z^2$ | 161.41 | 129.03 | 0.683 | 0.0958 | 0.0685 | 0.5473 | 0.3215 | 0.2233 | 0.562 |
| $a+by^2+cx/\sqrt{z}$ | 165.81 | 128.42 | 0.665 | 0.0967 | 0.0679 | 0.5385 | 0.3220 | 0.2174 | 0.561 |
| $a+by^2+cxz$ | 125.22 | 96.26 | 0.809 | 0.0733 | 0.0524 | 0.7346 | 0.2681 | 0.2024 | 0.696 |
| $a+by^2+cxz^2$ | 137.81 | 105.19 | 0.769 | 0.0812 | 0.0592 | 0.6742 | 0.2930 | 0.2166 | 0.636 |
| $a+by^2+cx\sqrt{z}$ | 117.07 | 90.83 | 0.833 | 0.0679 | 0.0459 | 0.7722 | 0.2395 | 0.1638 | 0.757 |
| $a+by^2+cx^2/z$ | 165.78 | 128.16 | 0.666 | 0.0964 | 0.0680 | 0.5412 | 0.3230 | 0.2193 | 0.558 |
| $a+by^2+cx^2/z^2$ | 163.68 | 129.77 | 0.674 | 0.0961 | 0.0684 | 0.5445 | 0.3230 | 0.2221 | 0.558 |
| $a+by^2+cx^2/\sqrt{z}$ | 163.26 | 133.71 | 0.676 | 0.0950 | 0.0675 | 0.5543 | 0.3049 | 0.2188 | 0.606 |
| $a+by^2+cx^2z$ | 132.49 | 101.80 | 0.786 | 0.0791 | 0.0588 | 0.6908 | 0.2855 | 0.2156 | 0.655 |
| $a+by^2+cx^2z^2$ | 142.24 | 108.96 | 0.754 | 0.0848 | 0.0622 | 0.6446 | 0.3017 | 0.2159 | 0.614 |
| $a+by^2+cx^2\sqrt{z}$ | 123.88 | 96.61 | 0.813 | 0.0748 | 0.0554 | 0.7239 | 0.2675 | 0.2028 | 0.697 |
| $a+by^2+c\sqrt{x}/z$ | 153.95 | 118.88 | 0.712 | 0.0935 | 0.0667 | 0.5683 | 0.3167 | 0.2195 | 0.575 |
| $a+by^2+c\sqrt{x}/z^2$ | 158.88 | 127.34 | 0.693 | 0.0954 | 0.0682 | 0.5508 | 0.3191 | 0.2225 | 0.568 |
| $a+by^2+c\sqrt{x}/\sqrt{z}$ | 158.85 | 120.31 | 0.693 | 0.0951 | 0.0683 | 0.5535 | 0.3221 | 0.2220 | 0.560 |
| $a+by^2+c\sqrt{x}z$ | 124.80 | 96.76 | 0.810 | 0.0723 | 0.0488 | 0.7416 | 0.2637 | 0.1938 | 0.705 |
| $a+by^2+c\sqrt{x}z^2$ | 136.12 | 104.07 | 0.775 | 0.0797 | 0.0579 | 0.6863 | 0.2889 | 0.2149 | 0.646 |
| $a+by^2+c\sqrt{x}\sqrt{z}$ | 121.70 | 90.47 | 0.820 | 0.0689 | 0.0435 | 0.7655 | 0.2397 | 0.1490 | 0.757 |

(continued on next page)

**Table 4 – continued from previous page**

| Functional form | $T_{eff}$ (K) | | | Radius ($R_{\odot}$) | | | log (L/$L_{\odot}$) | | |
|---|---|---|---|---|---|---|---|---|---|
| | RMSE | MAD | $R^2_{ap}$ | RMSE | MAD | $R^2_{ap}$ | RMSE | MAD | $R^2_{ap}$ |
| $a+by^2+c/xz$ | 166.74 | 132.82 | 0.662 | 0.0957 | 0.0667 | 0.5476 | 0.3156 | 0.2150 | 0.578 |
| $a+by^2+c/xz^2$ | 166.03 | 132.24 | 0.665 | 0.0955 | 0.0673 | 0.5494 | 0.3118 | 0.2091 | 0.588 |
| $a+by^2+c/x\sqrt{z}$ | 166.20 | 131.29 | 0.664 | 0.0960 | 0.0668 | 0.5451 | 0.3181 | 0.2169 | 0.571 |
| $a+by^2+cz/x$ | 160.70 | 120.97 | 0.686 | 0.0968 | 0.0675 | 0.5377 | 0.3233 | 0.2195 | 0.557 |
| $a+by^2+cz^2/x$ | 148.57 | 109.02 | 0.731 | 0.0940 | 0.0663 | 0.5638 | 0.3180 | 0.2189 | 0.572 |
| $a+by^2+c\sqrt{z}/x$ | 163.49 | 125.24 | 0.675 | 0.0966 | 0.0665 | 0.5391 | 0.3222 | 0.2178 | 0.560 |
| $a+by^2+c/x^2z$ | 163.80 | 126.20 | 0.674 | 0.0965 | 0.0668 | 0.5400 | 0.3220 | 0.2178 | 0.561 |
| $a+by^2+c/x^2z^2$ | 164.86 | 128.33 | 0.669 | 0.0965 | 0.0667 | 0.5407 | 0.3210 | 0.2173 | 0.563 |
| $a+by^2+c/x^2\sqrt{z}$ | 163.41 | 125.44 | 0.675 | 0.0965 | 0.0668 | 0.5398 | 0.3223 | 0.2179 | 0.560 |
| $a+by^2+cz/x^2$ | 162.54 | 123.79 | 0.679 | 0.0966 | 0.0667 | 0.5391 | 0.3228 | 0.2177 | 0.559 |
| $a+by^2+cz^2/x^2$ | 161.85 | 122.73 | 0.681 | 0.0967 | 0.0669 | 0.5385 | 0.3231 | 0.2177 | 0.558 |
| $a+by^2+c\sqrt{z}/x^2$ | 162.81 | 124.30 | 0.678 | 0.0966 | 0.0667 | 0.5394 | 0.3226 | 0.2178 | 0.559 |
| $a+by^2+c/\sqrt{x}z$ | 160.97 | 124.41 | 0.685 | 0.0923 | 0.0676 | 0.5793 | 0.2961 | 0.1992 | 0.628 |
| $a+by^2+c/\sqrt{x}z^2$ | 157.73 | 123.04 | 0.697 | 0.0943 | 0.0679 | 0.5611 | 0.3047 | 0.2027 | 0.607 |
| $a+by^2+c/\sqrt{x}\sqrt{z}$ | 165.18 | 131.44 | 0.668 | 0.0932 | 0.0673 | 0.5711 | 0.3028 | 0.2035 | 0.611 |
| $a+by^2+cz/\sqrt{x}$ | 145.20 | 107.65 | 0.743 | 0.0921 | 0.0645 | 0.5808 | 0.3140 | 0.2168 | 0.582 |
| $a+by^2+cz^2/\sqrt{x}$ | 134.46 | 100.41 | 0.780 | 0.0826 | 0.0571 | 0.6632 | 0.2936 | 0.2095 | 0.635 |
| $a+by^2+c\sqrt{z}/\sqrt{x}$ | 159.44 | 119.02 | 0.691 | 0.0965 | 0.0681 | 0.5399 | 0.3234 | 0.2212 | 0.557 |
| $a+by^2+cy/z$ | 147.40 | 111.28 | 0.736 | 0.0900 | 0.0632 | 0.5998 | 0.3083 | 0.2140 | 0.597 |
| $a+by^2+cy/z^2$ | 156.84 | 125.21 | 0.701 | 0.0944 | 0.0675 | 0.5598 | 0.3168 | 0.2205 | 0.575 |
| $a+by^2+cy/\sqrt{z}$ | 147.06 | 108.01 | 0.737 | 0.0894 | 0.0639 | 0.6056 | 0.3101 | 0.2173 | 0.592 |
| $a+by^2+cyz$ | 135.10 | 104.44 | 0.778 | 0.0790 | 0.0566 | 0.6922 | 0.2869 | 0.2116 | 0.651 |
| $a+by^2+cyz^2$ | 142.46 | 107.89 | 0.753 | 0.0838 | 0.0604 | 0.6536 | 0.3000 | 0.2146 | 0.619 |
| $a+by^2+cy\sqrt{z}$ | 129.11 | 102.20 | 0.797 | 0.0747 | 0.0490 | 0.7248 | 0.2702 | 0.1920 | 0.691 |
| $a+by^2+cy^2/z$ | 146.10 | 109.44 | 0.740 | 0.0878 | 0.0615 | 0.6194 | 0.3059 | 0.2097 | 0.604 |
| $a+by^2+cy^2/z^2$ | 156.12 | 123.09 | 0.703 | 0.0935 | 0.0665 | 0.5686 | 0.3161 | 0.2195 | 0.577 |
| $a+by^2+cy^2/\sqrt{z}$ | 143.30 | 107.37 | 0.750 | 0.0855 | 0.0598 | 0.6386 | 0.3028 | 0.2083 | 0.611 |
| $a+by^2+cy^2z$ | 145.71 | 107.03 | 0.742 | 0.0860 | 0.0620 | 0.6352 | 0.3061 | 0.2143 | 0.603 |
| $a+by^2+cy^2z^2$ | 148.35 | 109.93 | 0.732 | 0.0879 | 0.0635 | 0.6187 | 0.3098 | 0.2152 | 0.593 |
| $a+by^2+cy^2\sqrt{z}$ | 144.19 | 105.88 | 0.747 | 0.0851 | 0.0611 | 0.6423 | 0.3041 | 0.2135 | 0.608 |
| $a+by^2+c\sqrt{y}/z$ | 145.30 | 110.78 | 0.743 | 0.0900 | 0.0624 | 0.5999 | 0.3046 | 0.2082 | 0.607 |
| $a+by^2+c\sqrt{y}/z^2$ | 156.17 | 125.02 | 0.703 | 0.0946 | 0.0675 | 0.5583 | 0.3156 | 0.2192 | 0.578 |
| $a+by^2+c\sqrt{y}/\sqrt{z}$ | 142.83 | 105.41 | 0.752 | 0.0884 | 0.0620 | 0.6141 | 0.3046 | 0.2115 | 0.607 |
| $a+by^2+c\sqrt{y}z$ | 130.10 | 102.08 | 0.794 | 0.0763 | 0.0527 | 0.7126 | 0.2771 | 0.2033 | 0.675 |
| $a+by^2+c\sqrt{y}z^2$ | 138.81 | 105.60 | 0.766 | 0.0814 | 0.0587 | 0.6731 | 0.2936 | 0.2146 | 0.635 |
| $a+by^2+c\sqrt{y}\sqrt{z}$ | 126.00 | 99.75 | 0.807 | 0.0737 | 0.0453 | 0.7316 | 0.2619 | 0.1754 | 0.709 |
| $a+by^2+c/yz$ | 159.41 | 121.74 | 0.691 | 0.0942 | 0.0672 | 0.5615 | 0.3021 | 0.2029 | 0.613 |
| $a+by^2+c/yz^2$ | 157.77 | 122.67 | 0.697 | 0.0953 | 0.0683 | 0.5514 | 0.3089 | 0.2103 | 0.596 |
| $a+by^2+c/y\sqrt{z}$ | 163.42 | 128.66 | 0.675 | 0.0946 | 0.0672 | 0.5583 | 0.3048 | 0.2046 | 0.606 |
| $a+by^2+cz/y$ | 136.59 | 102.71 | 0.773 | 0.0878 | 0.0614 | 0.6196 | 0.3030 | 0.2110 | 0.611 |
| $a+by^2+cz^2/y$ | 127.57 | 97.56 | 0.802 | 0.0784 | 0.0533 | 0.6963 | 0.2806 | 0.2041 | 0.666 |
| $a+by^2+c\sqrt{z}/y$ | 156.50 | 115.85 | 0.702 | 0.0953 | 0.0687 | 0.5516 | 0.3221 | 0.2238 | 0.561 |
| $a+by^2+c/y^2z$ | 165.33 | 131.46 | 0.667 | 0.0960 | 0.0664 | 0.5451 | 0.3128 | 0.2063 | 0.586 |
| $a+by^2+c/y^2z^2$ | 163.01 | 127.27 | 0.677 | 0.0961 | 0.0672 | 0.5438 | 0.3131 | 0.2079 | 0.585 |
| $a+by^2+c/y^2\sqrt{z}$ | 166.45 | 133.10 | 0.663 | 0.0961 | 0.0661 | 0.5442 | 0.3144 | 0.2072 | 0.581 |
| $a+by^2+cz/y^2$ | 160.37 | 119.34 | 0.687 | 0.0965 | 0.0683 | 0.5397 | 0.3234 | 0.2207 | 0.557 |
| $a+by^2+cz^2/y^2$ | 138.94 | 102.32 | 0.765 | 0.0901 | 0.0631 | 0.5987 | 0.3081 | 0.2149 | 0.598 |
| $a+by^2+c\sqrt{z}/y^2$ | 165.17 | 128.77 | 0.668 | 0.0967 | 0.0669 | 0.5382 | 0.3214 | 0.2157 | 0.562 |
| $a+by^2+c/\sqrt{y}z$ | 149.50 | 115.56 | 0.728 | 0.0915 | 0.0662 | 0.5864 | 0.2929 | 0.1938 | 0.637 |
| $a+by^2+c/\sqrt{y}z^2$ | 155.06 | 121.84 | 0.707 | 0.0948 | 0.0681 | 0.5561 | 0.3095 | 0.2106 | 0.594 |
| $a+by^2+c/\sqrt{y}\sqrt{z}$ | 152.24 | 115.61 | 0.718 | 0.0903 | 0.0646 | 0.5974 | 0.2865 | 0.1868 | 0.652 |
| $a+by^2+cz/\sqrt{y}$ | 126.07 | 95.40 | 0.807 | 0.0793 | 0.0516 | 0.6892 | 0.2804 | 0.1964 | 0.667 |
| $a+by^2+cz^2/\sqrt{y}$ | 130.85 | 101.32 | 0.792 | 0.0778 | 0.0542 | 0.7011 | 0.2813 | 0.2077 | 0.665 |
| $a+by^2+c\sqrt{z}/\sqrt{y}$ | 137.14 | 103.25 | 0.771 | 0.0872 | 0.0610 | 0.6245 | 0.3018 | 0.2096 | 0.614 |
| $a+b\sqrt{y}+cx/y$ | 187.18 | 141.26 | 0.574 | 0.0985 | 0.0769 | 0.5209 | 0.3106 | 0.2238 | 0.591 |
| $a+b\sqrt{y}+cx/y^2$ | 188.34 | 144.82 | 0.568 | 0.0999 | 0.0770 | 0.5070 | 0.3210 | 0.2274 | 0.564 |
| $a+b\sqrt{y}+cx/\sqrt{y}$ | 177.91 | 130.68 | 0.615 | 0.0930 | 0.0719 | 0.5728 | 0.2884 | 0.2040 | 0.648 |
| $a+b\sqrt{y}+cxy$ | 135.74 | 105.00 | 0.776 | 0.0837 | 0.0594 | 0.6544 | 0.2786 | 0.1937 | 0.671 |
| $a+b\sqrt{y}+cxy^2$ | 150.30 | 116.48 | 0.725 | 0.0900 | 0.0632 | 0.6002 | 0.2999 | 0.2017 | 0.619 |
| $a+b\sqrt{y}+cx\sqrt{y}$ | 126.84 | 96.83 | 0.804 | 0.0778 | 0.0538 | 0.7008 | 0.2541 | 0.1779 | 0.726 |
| $a+b\sqrt{y}+cx^2/y$ | 152.96 | 117.76 | 0.715 | 0.0839 | 0.0640 | 0.6524 | 0.2573 | 0.1824 | 0.720 |
| $a+b\sqrt{y}+cx^2/y^2$ | 181.72 | 135.19 | 0.598 | 0.0962 | 0.0745 | 0.5435 | 0.2992 | 0.2144 | 0.621 |
| $a+b\sqrt{y}+cx^2/\sqrt{y}$ | 132.77 | 109.44 | 0.786 | 0.0777 | 0.0547 | 0.7021 | 0.2447 | 0.1731 | 0.746 |
| $a+b\sqrt{y}+cx^2y$ | 138.90 | 110.22 | 0.765 | 0.0847 | 0.0607 | 0.6460 | 0.2833 | 0.1958 | 0.660 |
| $a+b\sqrt{y}+cx^2y^2$ | 148.76 | 117.91 | 0.731 | 0.0890 | 0.0630 | 0.6087 | 0.2973 | 0.2016 | 0.625 |
| $a+b\sqrt{y}+cx^2\sqrt{y}$ | 131.79 | 104.38 | 0.789 | 0.0812 | 0.0582 | 0.6741 | 0.2706 | 0.1903 | 0.690 |
| $a+b\sqrt{y}+c\sqrt{x}/y$ | 188.31 | 144.91 | 0.569 | 0.0999 | 0.0771 | 0.5073 | 0.3203 | 0.2271 | 0.565 |
| $a+b\sqrt{y}+c\sqrt{x}/y^2$ | 183.23 | 145.50 | 0.592 | 0.0972 | 0.0720 | 0.5331 | 0.3199 | 0.2244 | 0.566 |
| $a+b\sqrt{y}+c\sqrt{x}/\sqrt{y}$ | 188.39 | 144.65 | 0.568 | 0.0999 | 0.0777 | 0.5069 | 0.3178 | 0.2270 | 0.572 |
| $a+b\sqrt{y}+c\sqrt{x}y$ | 137.85 | 106.01 | 0.769 | 0.0844 | 0.0594 | 0.6480 | 0.2807 | 0.1937 | 0.666 |
| $a+b\sqrt{y}+c\sqrt{x}y^2$ | 154.84 | 120.40 | 0.708 | 0.0920 | 0.0640 | 0.5824 | 0.3053 | 0.2045 | 0.605 |
| $a+b\sqrt{y}+c\sqrt{x}\sqrt{y}$ | 138.01 | 107.05 | 0.768 | 0.0779 | 0.0540 | 0.7002 | 0.2484 | 0.1710 | 0.739 |
| $a+b\sqrt{y}+c/xy$ | 165.62 | 126.85 | 0.666 | 0.0994 | 0.0724 | 0.5118 | 0.3185 | 0.2143 | 0.570 |
| $a+b\sqrt{y}+c/xy^2$ | 164.90 | 126.34 | 0.669 | 0.0993 | 0.0724 | 0.5130 | 0.3180 | 0.2144 | 0.572 |
| $a+b\sqrt{y}+c/x\sqrt{y}$ | 166.60 | 127.55 | 0.662 | 0.0996 | 0.0725 | 0.5099 | 0.3192 | 0.2142 | 0.568 |
| $a+b\sqrt{y}+cy/x$ | 178.24 | 139.22 | 0.613 | 0.1012 | 0.0756 | 0.4939 | 0.3249 | 0.2235 | 0.553 |
| $a+b\sqrt{y}+cy^2/x$ | 188.16 | 145.18 | 0.569 | 0.0998 | 0.0774 | 0.5077 | 0.3187 | 0.2256 | 0.570 |
| $a+b\sqrt{y}+c\sqrt{y}/x$ | 172.20 | 133.49 | 0.639 | 0.1006 | 0.0736 | 0.5006 | 0.3224 | 0.2194 | 0.559 |
| $a+b\sqrt{y}+c/x^2y$ | 167.01 | 130.14 | 0.661 | 0.1000 | 0.0734 | 0.5065 | 0.3190 | 0.2163 | 0.569 |
| $a+b\sqrt{y}+c/x^2y^2$ | 166.99 | 130.16 | 0.661 | 0.1000 | 0.0734 | 0.5065 | 0.3189 | 0.2163 | 0.569 |
| $a+b\sqrt{y}+c/x^2\sqrt{y}$ | 167.09 | 130.18 | 0.660 | 0.1000 | 0.0734 | 0.5064 | 0.3190 | 0.2162 | 0.569 |
| $a+b\sqrt{y}+cy/x^2$ | 168.35 | 130.72 | 0.655 | 0.1002 | 0.0734 | 0.5045 | 0.3199 | 0.2165 | 0.566 |
| $a+b\sqrt{y}+cy^2/x^2$ | 172.00 | 134.13 | 0.640 | 0.1007 | 0.0742 | 0.4993 | 0.3221 | 0.2195 | 0.560 |
| $a+b\sqrt{y}+c\sqrt{y}/x^2$ | 167.64 | 130.43 | 0.658 | 0.1001 | 0.0734 | 0.5056 | 0.3194 | 0.2162 | 0.568 |
| $a+b\sqrt{y}+c/\sqrt{x}y$ | 166.38 | 126.58 | 0.663 | 0.0990 | 0.0714 | 0.5158 | 0.3189 | 0.2130 | 0.569 |
| $a+b\sqrt{y}+c/\sqrt{x}y^2$ | 164.87 | 125.16 | 0.669 | 0.0986 | 0.0711 | 0.5195 | 0.3176 | 0.2116 | 0.573 |
| $a+b\sqrt{y}+c/\sqrt{x}\sqrt{y}$ | 168.71 | 128.51 | 0.654 | 0.0996 | 0.0717 | 0.5103 | 0.3205 | 0.2151 | 0.565 |
| $a+b\sqrt{y}+cy/\sqrt{x}$ | 188.22 | 145.10 | 0.569 | 0.0999 | 0.0773 | 0.5077 | 0.3192 | 0.2262 | 0.568 |
| $a+b\sqrt{y}+cy^2/\sqrt{x}$ | 185.91 | 146.59 | 0.579 | 0.1014 | 0.0768 | 0.4928 | 0.3239 | 0.2282 | 0.555 |
| $a+b\sqrt{y}+c\sqrt{y}/\sqrt{x}$ | 182.85 | 142.53 | 0.593 | 0.1014 | 0.0767 | 0.4928 | 0.3254 | 0.2253 | 0.551 |
| $a+b\sqrt{y}+cx/z$ | 163.09 | 124.09 | 0.676 | 0.0929 | 0.0635 | 0.5736 | 0.3069 | 0.2002 | 0.601 |

(continued on next page)

**Table 4 – continued from previous page**

| Functional form | $T_{eff}$ (K) | | | Radius ($R_\odot$) | | | log (L/$L_\odot$) | | |
|---|---|---|---|---|---|---|---|---|---|
| | RMSE | MAD | $R^2_{ap}$ | RMSE | MAD | $R^2_{ap}$ | RMSE | MAD | $R^2_{ap}$ |
| $a+b\sqrt{y}+cx/z^2$ | 172.84 | 133.60 | 0.637 | 0.0973 | 0.0714 | 0.5326 | 0.3147 | 0.2143 | 0.580 |
| $a+b\sqrt{y}+cx/\sqrt{z}$ | 173.38 | 129.63 | 0.634 | 0.0964 | 0.0666 | 0.5411 | 0.3183 | 0.2095 | 0.571 |
| $a+b\sqrt{y}+cxz$ | 122.40 | 93.11 | 0.818 | 0.0718 | 0.0476 | 0.7451 | 0.2542 | 0.1715 | 0.726 |
| $a+b\sqrt{y}+cxz^2$ | 131.67 | 101.62 | 0.789 | 0.0766 | 0.0513 | 0.7102 | 0.2695 | 0.1803 | 0.692 |
| $a+b\sqrt{y}+cx\sqrt{z}$ | 117.05 | 90.73 | 0.833 | 0.0693 | 0.0453 | 0.7627 | 0.2411 | 0.1586 | 0.754 |
| $a+b\sqrt{y}+cx^2/z$ | 180.17 | 132.35 | 0.605 | 0.0977 | 0.0684 | 0.5288 | 0.3213 | 0.2131 | 0.563 |
| $a+b\sqrt{y}+cx^2/z^2$ | 176.31 | 135.50 | 0.622 | 0.0977 | 0.0710 | 0.5291 | 0.3178 | 0.2157 | 0.572 |
| $a+b\sqrt{y}+cx^2/\sqrt{z}$ | 182.53 | 145.75 | 0.595 | 0.0997 | 0.0791 | 0.5096 | 0.3123 | 0.2355 | 0.587 |
| $a+b\sqrt{y}+cx^2z$ | 126.34 | 97.61 | 0.806 | 0.0758 | 0.0534 | 0.7165 | 0.2649 | 0.1802 | 0.703 |
| $a+b\sqrt{y}+cx^2z^2$ | 134.66 | 104.02 | 0.779 | 0.0796 | 0.0545 | 0.6870 | 0.2766 | 0.1834 | 0.676 |
| $a+b\sqrt{y}+cx^2\sqrt{z}$ | 121.60 | 95.64 | 0.820 | 0.0744 | 0.0530 | 0.7269 | 0.2571 | 0.1772 | 0.720 |
| $a+b\sqrt{y}+c\sqrt{x}/z$ | 155.48 | 116.67 | 0.706 | 0.0915 | 0.0635 | 0.5864 | 0.2989 | 0.1912 | 0.621 |
| $a+b\sqrt{y}+c\sqrt{x}/z^2$ | 171.17 | 130.86 | 0.644 | 0.0974 | 0.0720 | 0.5319 | 0.3130 | 0.2123 | 0.585 |
| $a+b\sqrt{y}+c\sqrt{x}/\sqrt{z}$ | 153.99 | 115.19 | 0.711 | 0.0910 | 0.0628 | 0.5915 | 0.3012 | 0.1913 | 0.616 |
| $a+b\sqrt{y}+c\sqrt{x}z$ | 123.49 | 95.47 | 0.814 | 0.0711 | 0.0445 | 0.7503 | 0.2518 | 0.1660 | 0.731 |
| $a+b\sqrt{y}+c\sqrt{x}z^2$ | 131.13 | 101.71 | 0.791 | 0.0755 | 0.0500 | 0.7189 | 0.2665 | 0.1780 | 0.699 |
| $a+b\sqrt{y}+c\sqrt{x}\sqrt{z}$ | 122.05 | 92.94 | 0.819 | 0.0692 | 0.0418 | 0.7638 | 0.2401 | 0.1479 | 0.756 |
| $a+b\sqrt{y}+c/xz$ | 173.85 | 136.65 | 0.632 | 0.1003 | 0.0729 | 0.5038 | 0.3229 | 0.2203 | 0.558 |
| $a+b\sqrt{y}+c/xz^2$ | 182.69 | 148.15 | 0.594 | 0.1003 | 0.0735 | 0.5028 | 0.3246 | 0.2239 | 0.553 |
| $a+b\sqrt{y}+c/x\sqrt{z}$ | 171.08 | 132.06 | 0.644 | 0.1002 | 0.0728 | 0.5042 | 0.3218 | 0.2186 | 0.561 |
| $a+b\sqrt{y}+cz/x$ | 158.69 | 122.11 | 0.694 | 0.0979 | 0.0713 | 0.5271 | 0.3129 | 0.2134 | 0.585 |
| $a+b\sqrt{y}+cz^2/x$ | 135.85 | 97.57 | 0.775 | 0.0892 | 0.0634 | 0.6073 | 0.2903 | 0.1873 | 0.643 |
| $a+b\sqrt{y}+c\sqrt{z}/x$ | 164.92 | 127.02 | 0.669 | 0.0994 | 0.0724 | 0.5125 | 0.3179 | 0.2148 | 0.572 |
| $a+b\sqrt{y}+c/x^2z$ | 166.42 | 129.05 | 0.663 | 0.0998 | 0.0731 | 0.5085 | 0.3188 | 0.2156 | 0.569 |
| $a+b\sqrt{y}+c/x^2z^2$ | 165.47 | 126.23 | 0.667 | 0.0993 | 0.0723 | 0.5131 | 0.3182 | 0.2139 | 0.571 |
| $a+b\sqrt{y}+c/x^2\sqrt{z}$ | 166.90 | 129.79 | 0.661 | 0.0999 | 0.0733 | 0.5071 | 0.3190 | 0.2160 | 0.569 |
| $a+b\sqrt{y}+cz/x^2$ | 167.54 | 130.63 | 0.658 | 0.1001 | 0.0735 | 0.5055 | 0.3192 | 0.2165 | 0.568 |
| $a+b\sqrt{y}+cz^2/x^2$ | 166.63 | 130.13 | 0.662 | 0.0999 | 0.0735 | 0.5072 | 0.3185 | 0.2164 | 0.570 |
| $a+b\sqrt{y}+c\sqrt{z}/x^2$ | 167.50 | 130.53 | 0.659 | 0.1001 | 0.0734 | 0.5056 | 0.3192 | 0.2164 | 0.568 |
| $a+b\sqrt{y}+c/\sqrt{x}z$ | 187.52 | 138.73 | 0.572 | 0.1002 | 0.0753 | 0.5045 | 0.3175 | 0.2216 | 0.573 |
| $a+b\sqrt{y}+c/\sqrt{x}z^2$ | 183.83 | 134.54 | 0.589 | 0.1008 | 0.0757 | 0.4987 | 0.3196 | 0.2243 | 0.567 |
| $a+b\sqrt{y}+c/\sqrt{x}\sqrt{z}$ | 187.07 | 147.52 | 0.574 | 0.1011 | 0.0768 | 0.4954 | 0.3235 | 0.2237 | 0.557 |
| $a+b\sqrt{y}+cz/\sqrt{x}$ | 131.36 | 94.92 | 0.790 | 0.0860 | 0.0593 | 0.6350 | 0.2828 | 0.1764 | 0.661 |
| $a+b\sqrt{y}+cz^2/\sqrt{x}$ | 126.63 | 98.53 | 0.805 | 0.0768 | 0.0494 | 0.7090 | 0.2659 | 0.1689 | 0.700 |
| $a+b\sqrt{y}+c\sqrt{z}/\sqrt{x}$ | 151.26 | 112.46 | 0.722 | 0.0949 | 0.0692 | 0.5550 | 0.3063 | 0.2062 | 0.603 |
| $a+b\sqrt{y}+cy/z$ | 146.53 | 107.80 | 0.739 | 0.0860 | 0.0570 | 0.6348 | 0.2831 | 0.1730 | 0.661 |
| $a+b\sqrt{y}+cy/z^2$ | 167.60 | 127.72 | 0.658 | 0.0956 | 0.0703 | 0.5489 | 0.3079 | 0.2069 | 0.598 |
| $a+b\sqrt{y}+cy/\sqrt{z}$ | 136.62 | 99.84 | 0.773 | 0.0797 | 0.0497 | 0.6865 | 0.2680 | 0.1531 | 0.696 |
| $a+b\sqrt{y}+cyz$ | 131.54 | 101.23 | 0.789 | 0.0772 | 0.0510 | 0.7055 | 0.2714 | 0.1744 | 0.688 |
| $a+b\sqrt{y}+cyz^2$ | 136.31 | 105.01 | 0.774 | 0.0791 | 0.0522 | 0.6911 | 0.2769 | 0.1791 | 0.675 |
| $a+b\sqrt{y}+cy\sqrt{z}$ | 131.08 | 101.29 | 0.791 | 0.0782 | 0.0510 | 0.6980 | 0.2727 | 0.1700 | 0.685 |
| $a+b\sqrt{y}+cy^2/z$ | 145.91 | 104.32 | 0.741 | 0.0816 | 0.0518 | 0.6711 | 0.2736 | 0.1597 | 0.683 |
| $a+b\sqrt{y}+cy^2/z^2$ | 164.31 | 124.29 | 0.672 | 0.0931 | 0.0669 | 0.5717 | 0.3028 | 0.2006 | 0.612 |
| $a+b\sqrt{y}+cy^2/\sqrt{z}$ | 160.14 | 106.26 | 0.688 | 0.0822 | 0.0565 | 0.6664 | 0.2717 | 0.1701 | 0.687 |
| $a+b\sqrt{y}+cy^2z$ | 139.82 | 103.99 | 0.762 | 0.0826 | 0.0557 | 0.6628 | 0.2860 | 0.1792 | 0.653 |
| $a+b\sqrt{y}+cy^2z^2$ | 141.30 | 108.50 | 0.757 | 0.0829 | 0.0551 | 0.6610 | 0.2863 | 0.1813 | 0.653 |
| $a+b\sqrt{y}+cy^2\sqrt{z}$ | 143.20 | 104.76 | 0.751 | 0.0853 | 0.0575 | 0.6411 | 0.2920 | 0.1821 | 0.639 |
| $a+b\sqrt{y}+c\sqrt{y}/z$ | 148.82 | 107.66 | 0.731 | 0.0884 | 0.0612 | 0.6143 | 0.2869 | 0.1759 | 0.651 |
| $a+b\sqrt{y}+c\sqrt{y}/z^2$ | 169.36 | 127.80 | 0.651 | 0.0968 | 0.0719 | 0.5376 | 0.3100 | 0.2096 | 0.593 |
| $a+b\sqrt{y}+c\sqrt{y}/\sqrt{z}$ | 136.75 | 99.47 | 0.772 | 0.0824 | 0.0532 | 0.6647 | 0.2730 | 0.1618 | 0.684 |
| $a+b\sqrt{y}+c\sqrt{y}z$ | 127.42 | 100.38 | 0.802 | 0.0745 | 0.0475 | 0.7257 | 0.2626 | 0.1692 | 0.708 |
| $a+b\sqrt{y}+c\sqrt{y}z^2$ | 133.50 | 103.74 | 0.783 | 0.0770 | 0.0507 | 0.7074 | 0.2709 | 0.1774 | 0.689 |
| $a+b\sqrt{y}+c\sqrt{y}\sqrt{z}$ | 126.02 | 99.53 | 0.807 | 0.0749 | 0.0450 | 0.7233 | 0.2607 | 0.1608 | 0.712 |
| $a+b\sqrt{y}+c/yz$ | 186.29 | 139.17 | 0.578 | 0.1012 | 0.0762 | 0.4946 | 0.3211 | 0.2225 | 0.563 |
| $a+b\sqrt{y}+c/yz^2$ | 184.24 | 137.18 | 0.587 | 0.1013 | 0.0761 | 0.4938 | 0.3222 | 0.2234 | 0.560 |
| $a+b\sqrt{y}+c/y\sqrt{z}$ | 188.35 | 145.63 | 0.568 | 0.1014 | 0.0765 | 0.4928 | 0.3241 | 0.2243 | 0.555 |
| $a+b\sqrt{y}+cz/y$ | 119.91 | 85.39 | 0.825 | 0.0789 | 0.0512 | 0.6925 | 0.2615 | 0.1556 | 0.710 |
| $a+b\sqrt{y}+cz^2/y$ | 123.11 | 94.99 | 0.816 | 0.0732 | 0.0459 | 0.7352 | 0.2539 | 0.1636 | 0.727 |
| $a+b\sqrt{y}+c\sqrt{z}/y$ | 132.24 | 97.74 | 0.787 | 0.0867 | 0.0601 | 0.6286 | 0.2839 | 0.1817 | 0.658 |
| $a+b\sqrt{y}+c/y^2z$ | 184.85 | 148.48 | 0.584 | 0.0997 | 0.0723 | 0.5093 | 0.3243 | 0.2250 | 0.554 |
| $a+b\sqrt{y}+c/y^2z^2$ | 188.27 | 146.08 | 0.569 | 0.1005 | 0.0741 | 0.5014 | 0.3253 | 0.2244 | 0.551 |
| $a+b\sqrt{y}+c/y^2\sqrt{z}$ | 179.06 | 145.01 | 0.610 | 0.0989 | 0.0705 | 0.5169 | 0.3224 | 0.2230 | 0.560 |
| $a+b\sqrt{y}+cz/y^2$ | 144.78 | 107.79 | 0.745 | 0.0932 | 0.0677 | 0.5715 | 0.3004 | 0.2025 | 0.618 |
| $a+b\sqrt{y}+cz^2/y^2$ | 121.97 | 88.25 | 0.819 | 0.0824 | 0.0559 | 0.6646 | 0.2691 | 0.1674 | 0.693 |
| $a+b\sqrt{y}+c\sqrt{z}/y^2$ | 157.42 | 118.20 | 0.699 | 0.0960 | 0.0690 | 0.5447 | 0.3112 | 0.2088 | 0.590 |
| $a+b\sqrt{y}+c/\sqrt{y}z$ | 169.46 | 122.64 | 0.651 | 0.0969 | 0.0724 | 0.5365 | 0.3039 | 0.2051 | 0.609 |
| $a+b\sqrt{y}+c/\sqrt{y}z^2$ | 177.34 | 132.72 | 0.617 | 0.1000 | 0.0751 | 0.5066 | 0.3168 | 0.2200 | 0.575 |
| $a+b\sqrt{y}+c/\sqrt{y}\sqrt{z}$ | 169.08 | 119.71 | 0.652 | 0.0950 | 0.0707 | 0.5546 | 0.2968 | 0.1958 | 0.627 |
| $a+b\sqrt{y}+cz/\sqrt{y}$ | 120.93 | 93.13 | 0.822 | 0.0741 | 0.0452 | 0.7286 | 0.2529 | 0.1529 | 0.729 |
| $a+b\sqrt{y}+cz^2/\sqrt{y}$ | 127.25 | 99.31 | 0.803 | 0.0735 | 0.0459 | 0.7336 | 0.2583 | 0.1665 | 0.717 |
| $a+b\sqrt{y}+c\sqrt{z}/\sqrt{y}$ | 122.64 | 89.01 | 0.817 | 0.0786 | 0.0506 | 0.6948 | 0.2616 | 0.1530 | 0.710 |
| $a+b/y+cx/y$ | 232.66 | 170.66 | 0.341 | 0.1147 | 0.0892 | 0.3506 | 0.3674 | 0.2659 | 0.428 |
| $a+b/y+cx/y^2$ | 221.90 | 166.55 | 0.401 | 0.1163 | 0.0894 | 0.3324 | 0.3742 | 0.2756 | 0.407 |
| $a+b/y+cx/\sqrt{y}$ | 181.65 | 136.94 | 0.599 | 0.0918 | 0.0717 | 0.5839 | 0.2868 | 0.2155 | 0.652 |
| $a+b/y+cxy$ | 138.23 | 108.16 | 0.768 | 0.0844 | 0.0574 | 0.6481 | 0.2770 | 0.1876 | 0.675 |
| $a+b/y+cxy^2$ | 149.23 | 116.21 | 0.729 | 0.0889 | 0.0612 | 0.6102 | 0.2941 | 0.1978 | 0.633 |
| $a+b/y+cx\sqrt{y}$ | 129.99 | 100.39 | 0.794 | 0.0806 | 0.0549 | 0.6792 | 0.2615 | 0.1769 | 0.710 |
| $a+b/y+cx^2/y$ | 157.01 | 125.55 | 0.700 | 0.0849 | 0.0640 | 0.6442 | 0.2627 | 0.1901 | 0.707 |
| $a+b/y+cx^2/y^2$ | 228.14 | 167.20 | 0.367 | 0.1131 | 0.0888 | 0.3686 | 0.3595 | 0.2627 | 0.452 |
| $a+b/y+cx^2/\sqrt{y}$ | 130.36 | 108.03 | 0.793 | 0.0774 | 0.0538 | 0.7039 | 0.2447 | 0.1732 | 0.746 |
| $a+b/y+cx^2y$ | 137.75 | 109.74 | 0.769 | 0.0834 | 0.0583 | 0.6568 | 0.2758 | 0.1883 | 0.678 |
| $a+b/y+cx^2y^2$ | 147.68 | 117.63 | 0.735 | 0.0876 | 0.0616 | 0.6212 | 0.2912 | 0.1969 | 0.641 |
| $a+b/y+cx^2\sqrt{y}$ | 131.54 | 104.12 | 0.789 | 0.0806 | 0.0561 | 0.6791 | 0.2648 | 0.1822 | 0.703 |
| $a+b/y+c\sqrt{x}/y$ | 220.79 | 165.92 | 0.407 | 0.1161 | 0.0891 | 0.3343 | 0.3739 | 0.2748 | 0.408 |
| $a+b/y+c\sqrt{x}/y^2$ | 226.03 | 166.93 | 0.378 | 0.1173 | 0.0918 | 0.3209 | 0.3764 | 0.2810 | 0.400 |
| $a+b/y+c\sqrt{x}/\sqrt{y}$ | 234.37 | 172.88 | 0.332 | 0.1161 | 0.0908 | 0.3349 | 0.3737 | 0.2746 | 0.408 |
| $a+b/y+c\sqrt{x}y$ | 145.06 | 114.57 | 0.744 | 0.0875 | 0.0591 | 0.6222 | 0.2865 | 0.1917 | 0.652 |
| $a+b/y+c\sqrt{x}y^2$ | 154.56 | 121.10 | 0.709 | 0.0913 | 0.0622 | 0.5883 | 0.3014 | 0.2012 | 0.615 |
| $a+b/y+c\sqrt{x}\sqrt{y}$ | 135.69 | 104.33 | 0.776 | 0.0826 | 0.0558 | 0.6629 | 0.2681 | 0.1804 | 0.696 |
| $a+b/y+c/xy$ | 203.64 | 151.96 | 0.495 | 0.1135 | 0.0876 | 0.3636 | 0.3585 | 0.2638 | 0.455 |
| $a+b/y+c/xy^2$ | 201.04 | 150.36 | 0.508 | 0.1129 | 0.0874 | 0.3702 | 0.3560 | 0.2619 | 0.463 |
| $a+b/y+c/x\sqrt{y}$ | 206.67 | 153.58 | 0.480 | 0.1142 | 0.0879 | 0.3562 | 0.3614 | 0.2657 | 0.447 |
| $a+b/y+cy/x$ | 222.70 | 164.89 | 0.397 | 0.1170 | 0.0912 | 0.3238 | 0.3753 | 0.2791 | 0.403 |

(continued on next page)

**Table 4 – continued from previous page**

| Functional form | $T_{eff}$ (K) | | | Radius ($R_\odot$) | | | log (L/$L_\odot$) | | |
|---|---|---|---|---|---|---|---|---|---|
| | RMSE | MAD | $R^2_{ap}$ | RMSE | MAD | $R^2_{ap}$ | RMSE | MAD | $R^2_{ap}$ |
| a+b/y+c$y^2$/x | 218.23 | 163.53 | 0.421 | 0.1158 | 0.0885 | 0.3380 | 0.3736 | 0.2734 | 0.409 |
| a+b/y+c$\sqrt{y}$/x | 217.34 | 160.23 | 0.425 | 0.1163 | 0.0898 | 0.3327 | 0.3709 | 0.2739 | 0.417 |
| a+b/y+c/$x^2$y | 209.70 | 155.24 | 0.465 | 0.1149 | 0.0886 | 0.3486 | 0.3635 | 0.2680 | 0.440 |
| a+b/y+c/$x^2y^2$ | 209.66 | 155.22 | 0.465 | 0.1149 | 0.0886 | 0.3487 | 0.3635 | 0.2680 | 0.440 |
| a+b/y+c/$x^2\sqrt{y}$ | 209.88 | 155.31 | 0.464 | 0.1149 | 0.0887 | 0.3482 | 0.3637 | 0.2680 | 0.439 |
| a+b/y+cy/$x^2$ | 212.03 | 156.15 | 0.453 | 0.1153 | 0.0888 | 0.3434 | 0.3658 | 0.2687 | 0.433 |
| a+b/y+c$y^2$/$x^2$ | 216.15 | 159.18 | 0.432 | 0.1161 | 0.0897 | 0.3344 | 0.3698 | 0.2727 | 0.421 |
| a+b/y+c$\sqrt{y}$/$x^2$ | 210.91 | 155.73 | 0.459 | 0.1151 | 0.0887 | 0.3459 | 0.3647 | 0.2684 | 0.436 |
| a+b/y+c/$\sqrt{x}$y | 200.24 | 151.18 | 0.512 | 0.1126 | 0.0870 | 0.3739 | 0.3559 | 0.2598 | 0.463 |
| a+b/y+c/$\sqrt{x}y^2$ | 189.61 | 146.19 | 0.563 | 0.1099 | 0.0852 | 0.4042 | 0.3453 | 0.2491 | 0.495 |
| a+b/y+c/$\sqrt{x}\sqrt{y}$ | 211.62 | 155.43 | 0.455 | 0.1151 | 0.0882 | 0.3455 | 0.3662 | 0.2670 | 0.432 |
| a+b/y+cy/$\sqrt{x}$ | 218.94 | 164.34 | 0.417 | 0.1159 | 0.0886 | 0.3371 | 0.3736 | 0.2737 | 0.409 |
| a+b/y+c$y^2$/$\sqrt{x}$ | 190.86 | 152.12 | 0.557 | 0.1059 | 0.0759 | 0.4460 | 0.3462 | 0.2362 | 0.492 |
| a+b/y+c$\sqrt{y}$/$\sqrt{x}$ | 228.18 | 168.65 | 0.367 | 0.1174 | 0.0920 | 0.3191 | 0.3783 | 0.2821 | 0.394 |
| a+b/y+cx/z | 189.87 | 134.23 | 0.561 | 0.0998 | 0.0701 | 0.5077 | 0.3296 | 0.2137 | 0.540 |
| a+b/y+cx/$z^2$ | 203.65 | 147.43 | 0.495 | 0.1073 | 0.0814 | 0.4312 | 0.3469 | 0.2438 | 0.490 |
| a+b/y+cx/$\sqrt{z}$ | 220.82 | 149.94 | 0.407 | 0.1109 | 0.0817 | 0.3929 | 0.3658 | 0.2520 | 0.433 |
| a+b/y+cxz | 123.03 | 92.52 | 0.816 | 0.0705 | 0.0451 | 0.7545 | 0.2475 | 0.1648 | 0.741 |
| a+b/y+cx$z^2$ | 135.42 | 103.56 | 0.777 | 0.0752 | 0.0506 | 0.7205 | 0.2650 | 0.1777 | 0.702 |
| a+b/y+cx$\sqrt{z}$ | 116.97 | 90.65 | 0.834 | 0.0696 | 0.0442 | 0.7609 | 0.2383 | 0.1531 | 0.759 |
| a+b/y+c$x^2$/z | 228.75 | 160.17 | 0.363 | 0.1139 | 0.0847 | 0.3597 | 0.3735 | 0.2596 | 0.409 |
| a+b/y+c$x^2$/$z^2$ | 211.71 | 151.31 | 0.455 | 0.1090 | 0.0826 | 0.4129 | 0.3558 | 0.2483 | 0.464 |
| a+b/y+c$x^2$/$\sqrt{z}$ | 194.22 | 155.99 | 0.541 | 0.1049 | 0.0843 | 0.4562 | 0.3260 | 0.2527 | 0.550 |
| a+b/y+c$x^2$z | 126.32 | 98.05 | 0.806 | 0.0738 | 0.0503 | 0.7311 | 0.2566 | 0.1753 | 0.721 |
| a+b/y+c$x^2z^2$ | 138.49 | 107.41 | 0.767 | 0.0784 | 0.0542 | 0.6964 | 0.2730 | 0.1872 | 0.684 |
| a+b/y+c$x^2\sqrt{z}$ | 120.87 | 94.73 | 0.822 | 0.0730 | 0.0500 | 0.7368 | 0.2490 | 0.1688 | 0.737 |
| a+b/y+c$\sqrt{x}$/z | 174.31 | 119.69 | 0.630 | 0.0963 | 0.0681 | 0.5423 | 0.3124 | 0.1957 | 0.586 |
| a+b/y+c$\sqrt{x}$/$z^2$ | 200.01 | 144.72 | 0.513 | 0.1071 | 0.0815 | 0.4338 | 0.3435 | 0.2434 | 0.500 |
| a+b/y+c$\sqrt{x}$/$\sqrt{z}$ | 172.81 | 121.83 | 0.637 | 0.0946 | 0.0640 | 0.5583 | 0.3121 | 0.1962 | 0.587 |
| a+b/y+c$\sqrt{x}$z | 125.06 | 95.98 | 0.810 | 0.0702 | 0.0425 | 0.7569 | 0.2467 | 0.1581 | 0.742 |
| a+b/y+c$\sqrt{x}z^2$ | 135.42 | 105.03 | 0.777 | 0.0742 | 0.0489 | 0.7280 | 0.2625 | 0.1736 | 0.708 |
| a+b/y+c$\sqrt{x}\sqrt{z}$ | 121.33 | 93.30 | 0.821 | 0.0695 | 0.0411 | 0.7616 | 0.2391 | 0.1448 | 0.758 |
| a+b/y+c/xz | 217.69 | 164.66 | 0.423 | 0.1160 | 0.0897 | 0.3355 | 0.3709 | 0.2758 | 0.417 |
| a+b/y+c/x$z^2$ | 233.59 | 174.42 | 0.336 | 0.1170 | 0.0913 | 0.3238 | 0.3782 | 0.2824 | 0.394 |
| a+b/y+c/x$\sqrt{z}$ | 214.75 | 159.81 | 0.439 | 0.1158 | 0.0890 | 0.3380 | 0.3689 | 0.2724 | 0.424 |
| a+b/y+cz/x | 192.04 | 139.39 | 0.551 | 0.1099 | 0.0845 | 0.4040 | 0.3460 | 0.2483 | 0.493 |
| a+b/y+c$z^2$/x | 146.23 | 108.83 | 0.740 | 0.0916 | 0.0636 | 0.5856 | 0.2930 | 0.1880 | 0.636 |
| a+b/y+c$\sqrt{z}$/x | 204.76 | 149.79 | 0.490 | 0.1136 | 0.0875 | 0.3633 | 0.3592 | 0.2625 | 0.453 |
| a+b/y+c/$x^2$z | 207.22 | 154.18 | 0.478 | 0.1143 | 0.0882 | 0.3545 | 0.3615 | 0.2666 | 0.446 |
| a+b/y+c/$x^2z^2$ | 200.44 | 150.55 | 0.511 | 0.1127 | 0.0875 | 0.3726 | 0.3554 | 0.2613 | 0.465 |
| a+b/y+c/$x^2\sqrt{z}$ | 209.05 | 155.01 | 0.468 | 0.1147 | 0.0885 | 0.3501 | 0.3631 | 0.2676 | 0.441 |
| a+b/y+cz/$x^2$ | 211.18 | 155.56 | 0.457 | 0.1151 | 0.0888 | 0.3455 | 0.3648 | 0.2685 | 0.436 |
| a+b/y+c$z^2$/$x^2$ | 209.66 | 154.23 | 0.465 | 0.1147 | 0.0887 | 0.3499 | 0.3633 | 0.2675 | 0.441 |
| a+b/y+c$\sqrt{z}$/$x^2$ | 210.95 | 155.64 | 0.459 | 0.1151 | 0.0888 | 0.3459 | 0.3646 | 0.2684 | 0.437 |
| a+b/y+c/$\sqrt{x}$z | 198.34 | 146.34 | 0.521 | 0.1033 | 0.0773 | 0.4735 | 0.3280 | 0.2286 | 0.544 |
| a+b/y+c/$\sqrt{x}z^2$ | 210.45 | 155.11 | 0.461 | 0.1123 | 0.0869 | 0.3773 | 0.3559 | 0.2619 | 0.463 |
| a+b/y+c/$\sqrt{x}\sqrt{z}$ | 220.62 | 157.09 | 0.408 | 0.1058 | 0.0793 | 0.4477 | 0.3451 | 0.2446 | 0.495 |
| a+b/y+cz/$\sqrt{x}$ | 136.20 | 101.56 | 0.774 | 0.0856 | 0.0576 | 0.6379 | 0.2772 | 0.1761 | 0.675 |
| a+b/y+c$z^2$/$\sqrt{x}$ | 131.58 | 100.95 | 0.789 | 0.0752 | 0.0501 | 0.7207 | 0.2601 | 0.1689 | 0.713 |
| a+b/y+c$\sqrt{z}$/$\sqrt{x}$ | 170.99 | 120.77 | 0.644 | 0.1020 | 0.0753 | 0.4861 | 0.3225 | 0.2170 | 0.559 |
| a+b/y+cy/z | 172.96 | 120.48 | 0.636 | 0.0921 | 0.0634 | 0.5807 | 0.3006 | 0.1918 | 0.617 |
| a+b/y+cy/$z^2$ | 196.97 | 144.03 | 0.528 | 0.1050 | 0.0794 | 0.4560 | 0.3373 | 0.2369 | 0.518 |
| a+b/y+cy/$\sqrt{z}$ | 190.22 | 136.15 | 0.560 | 0.0942 | 0.0689 | 0.5618 | 0.3104 | 0.2198 | 0.592 |
| a+b/y+cyz | 131.12 | 101.40 | 0.791 | 0.0756 | 0.0469 | 0.7181 | 0.2640 | 0.1691 | 0.705 |
| a+b/y+cy$z^2$ | 139.54 | 108.39 | 0.763 | 0.0777 | 0.0510 | 0.7022 | 0.2726 | 0.1792 | 0.685 |
| a+b/y+cy$\sqrt{z}$ | 131.26 | 100.67 | 0.790 | 0.0781 | 0.0483 | 0.6986 | 0.2679 | 0.1596 | 0.696 |
| a+b/y+c$y^2$/z | 199.68 | 142.06 | 0.515 | 0.0980 | 0.0714 | 0.5255 | 0.3233 | 0.2300 | 0.557 |
| a+b/y+c$y^2$/$z^2$ | 197.23 | 144.31 | 0.527 | 0.1030 | 0.0769 | 0.4762 | 0.3338 | 0.2297 | 0.528 |
| a+b/y+c$y^2$/$\sqrt{z}$ | 233.48 | 177.38 | 0.337 | 0.1173 | 0.0920 | 0.3209 | 0.3786 | 0.2801 | 0.393 |
| a+b/y+c$y^2$z | 138.95 | 105.39 | 0.765 | 0.0807 | 0.0520 | 0.6788 | 0.2788 | 0.1771 | 0.671 |
| a+b/y+c$y^2z^2$ | 144.56 | 111.44 | 0.746 | 0.0817 | 0.0545 | 0.6706 | 0.2834 | 0.1867 | 0.660 |
| a+b/y+c$y^2\sqrt{z}$ | 141.93 | 104.42 | 0.755 | 0.0838 | 0.0538 | 0.6529 | 0.2852 | 0.1757 | 0.655 |
| a+b/y+c$\sqrt{y}$/z | 168.19 | 115.19 | 0.656 | 0.0932 | 0.0657 | 0.5711 | 0.3002 | 0.1863 | 0.618 |
| a+b/y+c$\sqrt{y}$/$z^2$ | 197.54 | 143.57 | 0.525 | 0.1063 | 0.0809 | 0.4421 | 0.3398 | 0.2414 | 0.511 |
| a+b/y+c$\sqrt{y}$/$\sqrt{z}$ | 159.56 | 113.86 | 0.690 | 0.0865 | 0.0578 | 0.6307 | 0.2830 | 0.1762 | 0.661 |
| a+b/y+c$\sqrt{y}$z | 127.99 | 101.25 | 0.801 | 0.0731 | 0.0441 | 0.7362 | 0.2559 | 0.1617 | 0.723 |
| a+b/y+c$\sqrt{y}z^2$ | 137.34 | 107.73 | 0.771 | 0.0756 | 0.0493 | 0.7176 | 0.2667 | 0.1745 | 0.699 |
| a+b/y+c$\sqrt{y}\sqrt{z}$ | 126.02 | 99.35 | 0.807 | 0.0748 | 0.0440 | 0.7240 | 0.2567 | 0.1524 | 0.721 |
| a+b/y+c/yz | 200.09 | 143.37 | 0.513 | 0.1104 | 0.0848 | 0.3986 | 0.3463 | 0.2497 | 0.492 |
| a+b/y+c/y$z^2$ | 214.36 | 155.12 | 0.441 | 0.1147 | 0.0873 | 0.3507 | 0.3636 | 0.2640 | 0.440 |
| a+b/y+c/y$\sqrt{z}$ | 186.95 | 132.44 | 0.575 | 0.1056 | 0.0805 | 0.4499 | 0.3295 | 0.2331 | 0.540 |
| a+b/y+cz/y | 136.62 | 105.86 | 0.773 | 0.0800 | 0.0570 | 0.6836 | 0.2596 | 0.1731 | 0.714 |
| a+b/y+c$z^2$/y | 133.95 | 99.88 | 0.782 | 0.0733 | 0.0500 | 0.7345 | 0.2531 | 0.1620 | 0.729 |
| a+b/y+c$\sqrt{z}$/y | 150.13 | 109.25 | 0.726 | 0.0886 | 0.0643 | 0.6121 | 0.2795 | 0.1869 | 0.669 |
| a+b/y+c/$y^2$z | 234.40 | 173.32 | 0.332 | 0.1163 | 0.0900 | 0.3324 | 0.3780 | 0.2812 | 0.395 |
| a+b/y+c/$y^2z^2$ | 232.62 | 170.24 | 0.342 | 0.1173 | 0.0916 | 0.3210 | 0.3787 | 0.2825 | 0.392 |
| a+b/y+c/$y^2\sqrt{z}$ | 226.90 | 174.34 | 0.374 | 0.1122 | 0.0888 | 0.3781 | 0.3679 | 0.2764 | 0.426 |
| a+b/y+cz/$y^2$ | 160.83 | 110.38 | 0.685 | 0.0990 | 0.0740 | 0.5156 | 0.3071 | 0.2044 | 0.600 |
| a+b/y+c$z^2$/$y^2$ | 140.99 | 105.91 | 0.758 | 0.0853 | 0.0596 | 0.6406 | 0.2718 | 0.1809 | 0.687 |
| a+b/y+c$\sqrt{z}$/$y^2$ | 160.28 | 117.99 | 0.687 | 0.1003 | 0.0751 | 0.5028 | 0.3117 | 0.2180 | 0.588 |
| a+b/y+c/$\sqrt{y}$z | 177.48 | 124.53 | 0.617 | 0.1017 | 0.0776 | 0.4894 | 0.3191 | 0.2203 | 0.568 |
| a+b/y+c/$\sqrt{y}z^2$ | 204.30 | 149.86 | 0.492 | 0.1111 | 0.0853 | 0.3911 | 0.3516 | 0.2558 | 0.476 |
| a+b/y+c/$\sqrt{y}\sqrt{z}$ | 155.60 | 103.09 | 0.705 | 0.0931 | 0.0689 | 0.5716 | 0.2929 | 0.1880 | 0.637 |
| a+b/y+cz/$\sqrt{y}$ | 130.28 | 102.25 | 0.793 | 0.0738 | 0.0497 | 0.7309 | 0.2497 | 0.1536 | 0.736 |
| a+b/y+c$z^2$/$\sqrt{y}$ | 134.56 | 102.07 | 0.780 | 0.0728 | 0.0478 | 0.7381 | 0.2559 | 0.1675 | 0.722 |
| a+b/y+c$\sqrt{z}$/$\sqrt{y}$ | 140.14 | 107.17 | 0.761 | 0.0799 | 0.0558 | 0.6846 | 0.2611 | 0.1678 | 0.711 |
| a+b/$y^2$+cx/y | 248.12 | 184.82 | 0.251 | 0.1201 | 0.0924 | 0.2883 | 0.3889 | 0.2917 | 0.359 |
| a+b/$y^2$+cx/$y^2$ | 231.80 | 170.94 | 0.346 | 0.1215 | 0.0935 | 0.2709 | 0.3938 | 0.2870 | 0.343 |
| a+b/$y^2$+cx/$\sqrt{y}$ | 168.54 | 132.05 | 0.654 | 0.0877 | 0.0671 | 0.6206 | 0.2742 | 0.2034 | 0.681 |
| a+b/$y^2$+cxy | 138.42 | 108.65 | 0.767 | 0.0844 | 0.0570 | 0.6482 | 0.2765 | 0.1872 | 0.676 |
| a+b/$y^2$+cx$y^2$ | 149.31 | 116.43 | 0.729 | 0.0887 | 0.0614 | 0.6118 | 0.2940 | 0.1983 | 0.634 |
| a+b/$y^2$+cx$\sqrt{y}$ | 130.56 | 101.17 | 0.793 | 0.0810 | 0.0545 | 0.6758 | 0.2620 | 0.1760 | 0.709 |
| a+b/$y^2$+c$x^2$/y | 153.63 | 124.51 | 0.713 | 0.0842 | 0.0616 | 0.6496 | 0.2620 | 0.1896 | 0.709 |

(continued on next page)

**Table 4 – continued from previous page**

| Functional form | $T_{eff}$ (K) | | | Radius ($R_{\odot}$) | | | log (L/$L_{\odot}$) | | |
|---|---|---|---|---|---|---|---|---|---|
| | RMSE | MAD | $R^2_{ap}$ | RMSE | MAD | $R^2_{ap}$ | RMSE | MAD | $R^2_{ap}$ |
| $a+b/y^2+cx^2/y^2$ | 243.81 | 183.39 | 0.277 | 0.1193 | 0.0920 | 0.2978 | 0.3837 | 0.2872 | 0.376 |
| $a+b/y^2+cx^2/\sqrt{y}$ | 128.97 | 106.07 | 0.798 | 0.0774 | 0.0535 | 0.7044 | 0.2447 | 0.1736 | 0.746 |
| $a+b/y^2+cx^2y$ | 137.88 | 110.19 | 0.769 | 0.0831 | 0.0584 | 0.6587 | 0.2753 | 0.1880 | 0.679 |
| $a+b/y^2+cx^2y^2$ | 148.51 | 118.81 | 0.732 | 0.0876 | 0.0624 | 0.6213 | 0.2923 | 0.1984 | 0.638 |
| $a+b/y^2+cx^2\sqrt{y}$ | 131.56 | 104.23 | 0.789 | 0.0804 | 0.0559 | 0.6805 | 0.2641 | 0.1821 | 0.704 |
| $a+b/y^2+c\sqrt{x}/y$ | 230.42 | 170.29 | 0.354 | 0.1212 | 0.0931 | 0.2744 | 0.3932 | 0.2861 | 0.345 |
| $a+b/y^2+c\sqrt{x}/y^2$ | 219.43 | 164.78 | 0.414 | 0.1194 | 0.0935 | 0.2960 | 0.3819 | 0.2852 | 0.382 |
| $a+b/y^2+c\sqrt{x}/\sqrt{y}$ | 251.93 | 187.39 | 0.228 | 0.1216 | 0.0936 | 0.2694 | 0.3964 | 0.2966 | 0.334 |
| $a+b/y^2+c\sqrt{x}y$ | 145.74 | 115.47 | 0.742 | 0.0878 | 0.0589 | 0.6198 | 0.2866 | 0.1912 | 0.652 |
| $a+b/y^2+c\sqrt{x}y^2$ | 154.57 | 121.07 | 0.709 | 0.0912 | 0.0623 | 0.5894 | 0.3013 | 0.2013 | 0.615 |
| $a+b/y^2+c\sqrt{x}\sqrt{y}$ | 137.33 | 107.01 | 0.771 | 0.0838 | 0.0561 | 0.6533 | 0.2706 | 0.1806 | 0.690 |
| $a+b/y^2+c/xy$ | 236.83 | 172.16 | 0.318 | 0.1238 | 0.0969 | 0.2430 | 0.3980 | 0.2960 | 0.329 |
| $a+b/y^2+c/xy^2$ | 233.28 | 171.18 | 0.338 | 0.1231 | 0.0969 | 0.2512 | 0.3947 | 0.2956 | 0.340 |
| $a+b/y^2+c/x\sqrt{y}$ | 240.04 | 172.93 | 0.299 | 0.1244 | 0.0968 | 0.2362 | 0.4009 | 0.2963 | 0.319 |
| $a+b/y^2+cy/x$ | 248.70 | 179.31 | 0.247 | 0.1253 | 0.0978 | 0.2244 | 0.4080 | 0.3017 | 0.295 |
| $a+b/y^2+cy^2/x$ | 227.48 | 167.70 | 0.370 | 0.1208 | 0.0919 | 0.2800 | 0.3928 | 0.2844 | 0.346 |
| $a+b/y^2+c\sqrt{y}/x$ | 247.58 | 178.59 | 0.254 | 0.1253 | 0.0978 | 0.2250 | 0.4070 | 0.3015 | 0.298 |
| $a+b/y^2+c/x^2y$ | 237.70 | 172.31 | 0.313 | 0.1240 | 0.0969 | 0.2410 | 0.3987 | 0.2960 | 0.326 |
| $a+b/y^2+c/x^2y^2$ | 237.53 | 172.27 | 0.314 | 0.1240 | 0.0969 | 0.2413 | 0.3985 | 0.2960 | 0.327 |
| $a+b/y^2+c/x^2\sqrt{y}$ | 237.94 | 172.35 | 0.311 | 0.1240 | 0.0969 | 0.2405 | 0.3989 | 0.2960 | 0.326 |
| $a+b/y^2+cy/x^2$ | 240.02 | 172.92 | 0.299 | 0.1244 | 0.0968 | 0.2361 | 0.4009 | 0.2962 | 0.319 |
| $a+b/y^2+cy^2/x^2$ | 242.78 | 175.24 | 0.283 | 0.1248 | 0.0973 | 0.2306 | 0.4037 | 0.2989 | 0.310 |
| $a+b/y^2+c\sqrt{y}/x^2$ | 239.02 | 172.54 | 0.305 | 0.1242 | 0.0968 | 0.2382 | 0.3999 | 0.2958 | 0.322 |
| $a+b/y^2+c/\sqrt{x}y$ | 244.66 | 176.69 | 0.272 | 0.1250 | 0.0976 | 0.2284 | 0.4047 | 0.2999 | 0.306 |
| $a+b/y^2+c/\sqrt{x}y^2$ | 228.83 | 169.38 | 0.363 | 0.1222 | 0.0966 | 0.2628 | 0.3905 | 0.2942 | 0.354 |
| $a+b/y^2+c/\sqrt{x}\sqrt{y}$ | 252.12 | 181.63 | 0.227 | 0.1251 | 0.0975 | 0.2267 | 0.4088 | 0.3025 | 0.292 |
| $a+b/y^2+cy/\sqrt{x}$ | 228.24 | 168.62 | 0.366 | 0.1208 | 0.0923 | 0.2789 | 0.3927 | 0.2848 | 0.346 |
| $a+b/y^2+cy^2/\sqrt{x}$ | 191.11 | 152.24 | 0.556 | 0.1064 | 0.0756 | 0.4411 | 0.3494 | 0.2376 | 0.483 |
| $a+b/y^2+c\sqrt{y}/\sqrt{x}$ | 252.55 | 183.60 | 0.224 | 0.1250 | 0.0975 | 0.2281 | 0.4087 | 0.3046 | 0.292 |
| $a+b/y^2+cx/z$ | 207.56 | 147.50 | 0.476 | 0.1057 | 0.0757 | 0.4478 | 0.3524 | 0.2435 | 0.474 |
| $a+b/y^2+cx/z^2$ | 218.62 | 160.17 | 0.419 | 0.1129 | 0.0857 | 0.3710 | 0.3683 | 0.2624 | 0.425 |
| $a+b/y^2+cx/\sqrt{z}$ | 249.92 | 181.36 | 0.240 | 0.1224 | 0.0912 | 0.2600 | 0.4046 | 0.2933 | 0.306 |
| $a+b/y^2+cxz$ | 124.09 | 93.08 | 0.813 | 0.0704 | 0.0455 | 0.7556 | 0.2480 | 0.1666 | 0.739 |
| $a+b/y^2+cxz^2$ | 139.06 | 105.76 | 0.765 | 0.0757 | 0.0519 | 0.7168 | 0.2691 | 0.1821 | 0.693 |
| $a+b/y^2+cx\sqrt{z}$ | 116.85 | 90.55 | 0.834 | 0.0696 | 0.0442 | 0.7610 | 0.2380 | 0.1527 | 0.760 |
| $a+b/y^2+cx^2/z$ | 252.26 | 185.00 | 0.226 | 0.1235 | 0.0926 | 0.2465 | 0.4070 | 0.2974 | 0.298 |
| $a+b/y^2+cx^2/z^2$ | 229.51 | 166.92 | 0.359 | 0.1157 | 0.0874 | 0.3393 | 0.3813 | 0.2735 | 0.384 |
| $a+b/y^2+cx^2/\sqrt{z}$ | 192.92 | 154.01 | 0.547 | 0.1053 | 0.0831 | 0.4525 | 0.3276 | 0.2541 | 0.545 |
| $a+b/y^2+cx^2z$ | 127.94 | 99.49 | 0.801 | 0.0737 | 0.0507 | 0.7318 | 0.2578 | 0.1785 | 0.718 |
| $a+b/y^2+cx^2z^2$ | 142.69 | 110.65 | 0.752 | 0.0792 | 0.0562 | 0.6905 | 0.2781 | 0.1964 | 0.672 |
| $a+b/y^2+cx^2\sqrt{z}$ | 121.30 | 94.85 | 0.821 | 0.0728 | 0.0499 | 0.7386 | 0.2486 | 0.1693 | 0.738 |
| $a+b/y^2+c\sqrt{x}/z$ | 185.48 | 127.13 | 0.581 | 0.0998 | 0.0704 | 0.5082 | 0.3265 | 0.2113 | 0.548 |
| $a+b/y^2+c\sqrt{x}/z^2$ | 212.90 | 155.75 | 0.449 | 0.1120 | 0.0852 | 0.3808 | 0.3624 | 0.2580 | 0.443 |
| $a+b/y^2+c\sqrt{x}/\sqrt{z}$ | 190.20 | 132.41 | 0.560 | 0.0998 | 0.0701 | 0.5086 | 0.3325 | 0.2213 | 0.532 |
| $a+b/y^2+c\sqrt{x}z$ | 126.17 | 96.63 | 0.806 | 0.0701 | 0.0431 | 0.7575 | 0.2475 | 0.1595 | 0.741 |
| $a+b/y^2+c\sqrt{x}z^2$ | 139.01 | 107.48 | 0.765 | 0.0747 | 0.0499 | 0.7245 | 0.2664 | 0.1771 | 0.699 |
| $a+b/y^2+c\sqrt{x}\sqrt{z}$ | 120.85 | 93.01 | 0.822 | 0.0695 | 0.0411 | 0.7613 | 0.2391 | 0.1450 | 0.758 |
| $a+b/y^2+c/xz$ | 253.83 | 186.81 | 0.216 | 0.1245 | 0.0977 | 0.2343 | 0.4081 | 0.3046 | 0.294 |
| $a+b/y^2+c/xz^2$ | 237.31 | 172.75 | 0.315 | 0.1208 | 0.0929 | 0.2795 | 0.3896 | 0.2849 | 0.357 |
| $a+b/y^2+c/x\sqrt{z}$ | 249.71 | 180.56 | 0.241 | 0.1253 | 0.0977 | 0.2244 | 0.4081 | 0.3023 | 0.294 |
| $a+b/y^2+cz/x$ | 218.54 | 158.02 | 0.419 | 0.1188 | 0.0939 | 0.3031 | 0.3788 | 0.2796 | 0.392 |
| $a+b/y^2+cz^2/x$ | 158.30 | 114.39 | 0.695 | 0.0951 | 0.0670 | 0.5532 | 0.3064 | 0.2022 | 0.602 |
| $a+b/y^2+c\sqrt{z}/x$ | 235.01 | 169.59 | 0.328 | 0.1233 | 0.0968 | 0.2496 | 0.3962 | 0.2934 | 0.335 |
| $a+b/y^2+c/x^2z$ | 236.99 | 172.32 | 0.317 | 0.1239 | 0.0969 | 0.2425 | 0.3981 | 0.2962 | 0.328 |
| $a+b/y^2+c/x^2z^2$ | 233.27 | 171.50 | 0.338 | 0.1231 | 0.0969 | 0.2516 | 0.3946 | 0.2960 | 0.340 |
| $a+b/y^2+c/x^2\sqrt{z}$ | 237.85 | 172.39 | 0.312 | 0.1240 | 0.0969 | 0.2406 | 0.3989 | 0.2960 | 0.326 |
| $a+b/y^2+cz/x^2$ | 238.40 | 172.30 | 0.309 | 0.1241 | 0.0968 | 0.2397 | 0.3993 | 0.2957 | 0.324 |
| $a+b/y^2+cz^2/x^2$ | 236.30 | 171.35 | 0.321 | 0.1236 | 0.0970 | 0.2452 | 0.3973 | 0.2952 | 0.331 |
| $a+b/y^2+c\sqrt{z}/x^2$ | 238.55 | 172.42 | 0.308 | 0.1241 | 0.0968 | 0.2392 | 0.3995 | 0.2958 | 0.324 |
| $a+b/y^2+c/\sqrt{x}z$ | 180.22 | 130.78 | 0.605 | 0.0983 | 0.0707 | 0.5230 | 0.3125 | 0.2019 | 0.586 |
| $a+b/y^2+c/\sqrt{x}z^2$ | 212.16 | 154.12 | 0.452 | 0.1147 | 0.0899 | 0.3508 | 0.3650 | 0.2674 | 0.436 |
| $a+b/y^2+c/\sqrt{x}\sqrt{z}$ | 194.70 | 139.76 | 0.539 | 0.0942 | 0.0722 | 0.5622 | 0.3119 | 0.2215 | 0.588 |
| $a+b/y^2+cz/\sqrt{x}$ | 144.39 | 108.33 | 0.746 | 0.0874 | 0.0606 | 0.6224 | 0.2849 | 0.1883 | 0.656 |
| $a+b/y^2+cz^2/\sqrt{x}$ | 136.57 | 103.24 | 0.773 | 0.0759 | 0.0525 | 0.7159 | 0.2648 | 0.1737 | 0.703 |
| $a+b/y^2+c\sqrt{z}/\sqrt{x}$ | 193.28 | 133.85 | 0.545 | 0.1094 | 0.0818 | 0.4092 | 0.3490 | 0.2463 | 0.484 |
| $a+b/y^2+cy/z$ | 190.00 | 137.07 | 0.561 | 0.0977 | 0.0668 | 0.5287 | 0.3219 | 0.2184 | 0.561 |
| $a+b/y^2+cy/z^2$ | 210.90 | 155.50 | 0.459 | 0.1101 | 0.0832 | 0.4015 | 0.3570 | 0.2519 | 0.460 |
| $a+b/y^2+cy/\sqrt{z}$ | 225.94 | 161.77 | 0.379 | 0.1086 | 0.0818 | 0.4180 | 0.3606 | 0.2652 | 0.449 |
| $a+b/y^2+cyz$ | 131.87 | 102.55 | 0.788 | 0.0753 | 0.0468 | 0.7202 | 0.2642 | 0.1716 | 0.704 |
| $a+b/y^2+cyz^2$ | 142.95 | 111.31 | 0.751 | 0.0781 | 0.0523 | 0.6987 | 0.2765 | 0.1841 | 0.676 |
| $a+b/y^2+cy\sqrt{z}$ | 131.26 | 100.65 | 0.790 | 0.0780 | 0.0476 | 0.6999 | 0.2671 | 0.1603 | 0.698 |
| $a+b/y^2+cy^2/z$ | 229.93 | 164.16 | 0.357 | 0.1104 | 0.0820 | 0.3983 | 0.3671 | 0.2688 | 0.429 |
| $a+b/y^2+cy^2/z^2$ | 214.72 | 157.70 | 0.439 | 0.1093 | 0.0814 | 0.4101 | 0.3580 | 0.2530 | 0.457 |
| $a+b/y^2+cy^2/\sqrt{z}$ | 244.30 | 194.60 | 0.274 | 0.1242 | 0.0970 | 0.2388 | 0.4033 | 0.3082 | 0.311 |
| $a+b/y^2+cy^2z$ | 140.03 | 107.09 | 0.761 | 0.0805 | 0.0523 | 0.6802 | 0.2798 | 0.1813 | 0.668 |
| $a+b/y^2+cy^2z^2$ | 148.35 | 114.43 | 0.732 | 0.0824 | 0.0564 | 0.6651 | 0.2883 | 0.1963 | 0.648 |
| $a+b/y^2+cy^2\sqrt{z}$ | 142.00 | 104.24 | 0.755 | 0.0835 | 0.0535 | 0.6554 | 0.2849 | 0.1758 | 0.656 |
| $a+b/y^2+c\sqrt{y}/z$ | 178.30 | 124.16 | 0.613 | 0.0964 | 0.0673 | 0.5412 | 0.3130 | 0.2011 | 0.585 |
| $a+b/y^2+c\sqrt{y}/z^2$ | 209.44 | 153.48 | 0.466 | 0.1109 | 0.0842 | 0.3930 | 0.3575 | 0.2545 | 0.459 |
| $a+b/y^2+c\sqrt{y}/\sqrt{z}$ | 176.48 | 130.62 | 0.621 | 0.0916 | 0.0638 | 0.5858 | 0.3028 | 0.2041 | 0.611 |
| $a+b/y^2+c\sqrt{y}z$ | 128.97 | 102.39 | 0.798 | 0.0729 | 0.0442 | 0.7378 | 0.2563 | 0.1636 | 0.722 |
| $a+b/y^2+c\sqrt{y}z^2$ | 140.81 | 110.52 | 0.759 | 0.0760 | 0.0504 | 0.7144 | 0.2705 | 0.1783 | 0.690 |
| $a+b/y^2+c\sqrt{y}\sqrt{z}$ | 126.03 | 99.43 | 0.807 | 0.0746 | 0.0438 | 0.7250 | 0.2561 | 0.1528 | 0.722 |
| $a+b/y^2+c/yz$ | 190.21 | 138.50 | 0.560 | 0.1093 | 0.0855 | 0.4097 | 0.3427 | 0.2511 | 0.502 |
| $a+b/y^2+c/yz^2$ | 218.48 | 157.98 | 0.419 | 0.1184 | 0.0928 | 0.3082 | 0.3765 | 0.2793 | 0.399 |
| $a+b/y^2+c/y\sqrt{z}$ | 163.26 | 114.92 | 0.676 | 0.0999 | 0.0767 | 0.5069 | 0.3109 | 0.2143 | 0.591 |
| $a+b/y^2+cz/y$ | 154.50 | 117.16 | 0.710 | 0.0847 | 0.0654 | 0.6457 | 0.2777 | 0.2015 | 0.673 |
| $a+b/y^2+cz^2/y$ | 141.14 | 106.41 | 0.758 | 0.0748 | 0.0535 | 0.7239 | 0.2605 | 0.1697 | 0.712 |
| $a+b/y^2+c\sqrt{z}/y$ | 200.27 | 143.40 | 0.512 | 0.1042 | 0.0799 | 0.4638 | 0.3355 | 0.2528 | 0.523 |

(continued on next page)

**Table 4 – continued from previous page**

| Functional form | $T_{eff}$ (K) | | | Radius ($R_\odot$) | | | log ($L/L_\odot$) | | |
|---|---|---|---|---|---|---|---|---|---|
| | RMSE | MAD | $R^2_{ap}$ | RMSE | MAD | $R^2_{ap}$ | RMSE | MAD | $R^2_{ap}$ |
| $a+b/y^2+c/y^2z$ | 238.60 | 171.15 | 0.307 | 0.1239 | 0.0963 | 0.2419 | 0.3982 | 0.2911 | 0.328 |
| $a+b/y^2+c/y^2z^2$ | 241.97 | 174.26 | 0.288 | 0.1246 | 0.0969 | 0.2334 | 0.4020 | 0.2943 | 0.315 |
| $a+b/y^2+c/y^2\sqrt{z}$ | 235.08 | 168.89 | 0.328 | 0.1230 | 0.0962 | 0.2524 | 0.3941 | 0.2894 | 0.342 |
| $a+b/y^2+cz/y^2$ | 202.33 | 144.04 | 0.502 | 0.1116 | 0.0843 | 0.3847 | 0.3523 | 0.2524 | 0.474 |
| $a+b/y^2+cz^2/y^2$ | 160.76 | 121.53 | 0.686 | 0.0908 | 0.0684 | 0.5927 | 0.2926 | 0.2120 | 0.637 |
| $a+b/y^2+c\sqrt{z}/y^2$ | 218.78 | 155.92 | 0.418 | 0.1179 | 0.0920 | 0.3131 | 0.3740 | 0.2737 | 0.407 |
| $a+b/y^2+c/\sqrt{y}z$ | 175.98 | 121.24 | 0.623 | 0.1021 | 0.0782 | 0.4854 | 0.3215 | 0.2227 | 0.562 |
| $a+b/y^2+c/\sqrt{y}z^2$ | 210.88 | 152.22 | 0.459 | 0.1146 | 0.0900 | 0.3512 | 0.3651 | 0.2676 | 0.435 |
| $a+b/y^2+c/\sqrt{y}\sqrt{z}$ | 150.47 | 100.05 | 0.725 | 0.0922 | 0.0680 | 0.5799 | 0.2905 | 0.1852 | 0.642 |
| $a+b/y^2+cz/\sqrt{y}$ | 136.85 | 107.82 | 0.772 | 0.0750 | 0.0534 | 0.7224 | 0.2558 | 0.1652 | 0.723 |
| $a+b/y^2+cz^2/\sqrt{y}$ | 139.43 | 105.33 | 0.763 | 0.0736 | 0.0496 | 0.7324 | 0.2610 | 0.1721 | 0.711 |
| $a+b/y^2+c\sqrt{z}/\sqrt{y}$ | 157.43 | 119.37 | 0.698 | 0.0845 | 0.0638 | 0.6474 | 0.2790 | 0.1961 | 0.670 |
| $a+b/\sqrt{y}+cx/y$ | 219.12 | 160.56 | 0.416 | 0.1099 | 0.0866 | 0.4040 | 0.3496 | 0.2546 | 0.482 |
| $a+b/\sqrt{y}+cx/y^2$ | 213.22 | 161.38 | 0.447 | 0.1118 | 0.0862 | 0.3826 | 0.3584 | 0.2630 | 0.456 |
| $a+b/\sqrt{y}+cx/\sqrt{y}$ | 186.76 | 138.80 | 0.576 | 0.0940 | 0.0743 | 0.5639 | 0.2925 | 0.2164 | 0.637 |
| $a+b/\sqrt{y}+cxy$ | 137.89 | 107.44 | 0.769 | 0.0844 | 0.0579 | 0.6485 | 0.2776 | 0.1885 | 0.673 |
| $a+b/\sqrt{y}+cxy^2$ | 149.38 | 116.19 | 0.728 | 0.0891 | 0.0615 | 0.6081 | 0.2950 | 0.1982 | 0.631 |
| $a+b/\sqrt{y}+cx\sqrt{y}$ | 129.20 | 99.24 | 0.797 | 0.0801 | 0.0550 | 0.6830 | 0.2606 | 0.1776 | 0.712 |
| $a+b/\sqrt{y}+cx^2/y$ | 157.98 | 125.27 | 0.696 | 0.0851 | 0.0652 | 0.6427 | 0.2622 | 0.1886 | 0.709 |
| $a+b/\sqrt{y}+cx^2/y^2$ | 214.81 | 153.67 | 0.439 | 0.1080 | 0.0849 | 0.4237 | 0.3406 | 0.2468 | 0.508 |
| $a+b/\sqrt{y}+cx^2/\sqrt{y}$ | 131.27 | 109.09 | 0.790 | 0.0775 | 0.0540 | 0.7034 | 0.2447 | 0.1730 | 0.746 |
| $a+b/\sqrt{y}+cx^2y$ | 137.91 | 109.72 | 0.769 | 0.0837 | 0.0587 | 0.6544 | 0.2771 | 0.1895 | 0.675 |
| $a+b/\sqrt{y}+cx^2y^2$ | 147.58 | 117.45 | 0.735 | 0.0878 | 0.0614 | 0.6192 | 0.2918 | 0.1974 | 0.639 |
| $a+b/\sqrt{y}+cx^2\sqrt{y}$ | 131.59 | 104.13 | 0.789 | 0.0808 | 0.0565 | 0.6777 | 0.2660 | 0.1837 | 0.700 |
| $a+b/\sqrt{y}+c\sqrt{x}/y$ | 212.44 | 160.90 | 0.451 | 0.1118 | 0.0861 | 0.3833 | 0.3584 | 0.2627 | 0.456 |
| $a+b/\sqrt{y}+c\sqrt{x}/y^2$ | 219.80 | 161.80 | 0.412 | 0.1107 | 0.0852 | 0.3945 | 0.3579 | 0.2614 | 0.457 |
| $a+b/\sqrt{y}+c\sqrt{x}/\sqrt{y}$ | 219.85 | 162.34 | 0.412 | 0.1111 | 0.0873 | 0.3905 | 0.3554 | 0.2617 | 0.465 |
| $a+b/\sqrt{y}+c\sqrt{x}y$ | 144.05 | 113.26 | 0.748 | 0.0871 | 0.0592 | 0.6254 | 0.2861 | 0.1922 | 0.653 |
| $a+b/\sqrt{y}+c\sqrt{x}y^2$ | 154.62 | 121.04 | 0.709 | 0.0915 | 0.0624 | 0.5870 | 0.3020 | 0.2017 | 0.613 |
| $a+b/\sqrt{y}+c\sqrt{x}\sqrt{y}$ | 133.87 | 102.01 | 0.782 | 0.0813 | 0.0556 | 0.6734 | 0.2646 | 0.1794 | 0.703 |
| $a+b/\sqrt{y}+c/xy$ | 185.97 | 143.53 | 0.579 | 0.1076 | 0.0826 | 0.4284 | 0.3388 | 0.2404 | 0.514 |
| $a+b/\sqrt{y}+c/xy^2$ | 184.19 | 142.55 | 0.587 | 0.1072 | 0.0823 | 0.4327 | 0.3371 | 0.2397 | 0.519 |
| $a+b/\sqrt{y}+c/x\sqrt{y}$ | 188.33 | 144.56 | 0.568 | 0.1081 | 0.0828 | 0.4228 | 0.3409 | 0.2413 | 0.508 |
| $a+b/\sqrt{y}+cy/x$ | 205.91 | 155.55 | 0.484 | 0.1114 | 0.0855 | 0.3877 | 0.3552 | 0.2584 | 0.465 |
| $a+b/\sqrt{y}+cy^2/x$ | 210.49 | 159.27 | 0.461 | 0.1116 | 0.0859 | 0.3847 | 0.3583 | 0.2619 | 0.456 |
| $a+b/\sqrt{y}+c\sqrt{y}/x$ | 198.62 | 149.19 | 0.520 | 0.1102 | 0.0838 | 0.4003 | 0.3497 | 0.2500 | 0.482 |
| $a+b/\sqrt{y}+c/x^2y$ | 192.50 | 144.63 | 0.549 | 0.1091 | 0.0835 | 0.4121 | 0.3437 | 0.2456 | 0.499 |
| $a+b/\sqrt{y}+c/x^2y^2$ | 192.51 | 144.57 | 0.549 | 0.1091 | 0.0836 | 0.4120 | 0.3437 | 0.2457 | 0.499 |
| $a+b/\sqrt{y}+c/x^2\sqrt{y}$ | 192.63 | 144.69 | 0.549 | 0.1091 | 0.0835 | 0.4118 | 0.3439 | 0.2457 | 0.499 |
| $a+b/\sqrt{y}+cy/x^2$ | 194.62 | 145.35 | 0.539 | 0.1095 | 0.0836 | 0.4076 | 0.3457 | 0.2466 | 0.494 |
| $a+b/\sqrt{y}+cy^2/x^2$ | 199.16 | 148.46 | 0.517 | 0.1104 | 0.0842 | 0.3982 | 0.3498 | 0.2513 | 0.482 |
| $a+b/\sqrt{y}+c\sqrt{y}/x^2$ | 193.54 | 145.02 | 0.544 | 0.1093 | 0.0836 | 0.4099 | 0.3447 | 0.2461 | 0.497 |
| $a+b/\sqrt{y}+c/\sqrt{x}y$ | 181.29 | 141.43 | 0.600 | 0.1061 | 0.0809 | 0.4441 | 0.3352 | 0.2373 | 0.524 |
| $a+b/\sqrt{y}+c/\sqrt{x}y^2$ | 175.44 | 137.11 | 0.626 | 0.1045 | 0.0795 | 0.4611 | 0.3293 | 0.2333 | 0.541 |
| $a+b/\sqrt{y}+c/\sqrt{x}\sqrt{y}$ | 189.30 | 145.38 | 0.564 | 0.1081 | 0.0822 | 0.4230 | 0.3424 | 0.2405 | 0.503 |
| $a+b/\sqrt{y}+cy/\sqrt{x}$ | 211.05 | 159.61 | 0.458 | 0.1117 | 0.0859 | 0.3843 | 0.3583 | 0.2621 | 0.456 |
| $a+b/\sqrt{y}+cy^2/\sqrt{x}$ | 190.44 | 151.72 | 0.559 | 0.1054 | 0.0764 | 0.4519 | 0.3430 | 0.2350 | 0.502 |
| $a+b/\sqrt{y}+c\sqrt{y}/\sqrt{x}$ | 211.70 | 159.96 | 0.455 | 0.1119 | 0.0864 | 0.3820 | 0.3583 | 0.2631 | 0.456 |
| $a+b/\sqrt{y}+cx/z$ | 179.50 | 127.55 | 0.608 | 0.0967 | 0.0670 | 0.5381 | 0.3182 | 0.2024 | 0.571 |
| $a+b/\sqrt{y}+cx/z^2$ | 193.46 | 139.15 | 0.545 | 0.1037 | 0.0780 | 0.4687 | 0.3341 | 0.2328 | 0.527 |
| $a+b/\sqrt{y}+cx/\sqrt{z}$ | 201.72 | 139.94 | 0.505 | 0.1042 | 0.0736 | 0.4636 | 0.3435 | 0.2315 | 0.500 |
| $a+b/\sqrt{y}+cxz$ | 122.55 | 92.41 | 0.817 | 0.0708 | 0.0454 | 0.7527 | 0.2483 | 0.1651 | 0.739 |
| $a+b/\sqrt{y}+cxz^2$ | 133.52 | 102.48 | 0.783 | 0.0753 | 0.0498 | 0.7203 | 0.2642 | 0.1766 | 0.704 |
| $a+b/\sqrt{y}+cx\sqrt{z}$ | 117.01 | 90.68 | 0.833 | 0.0696 | 0.0446 | 0.7609 | 0.2390 | 0.1542 | 0.758 |
| $a+b/\sqrt{y}+cx^2/z$ | 211.95 | 143.78 | 0.453 | 0.1076 | 0.0788 | 0.4284 | 0.3523 | 0.2403 | 0.474 |
| $a+b/\sqrt{y}+cx^2/z^2$ | 199.77 | 142.37 | 0.514 | 0.1049 | 0.0783 | 0.4571 | 0.3406 | 0.2364 | 0.508 |
| $a+b/\sqrt{y}+cx^2/\sqrt{z}$ | 193.49 | 155.57 | 0.544 | 0.1041 | 0.0844 | 0.4649 | 0.3233 | 0.2506 | 0.557 |
| $a+b/\sqrt{y}+cx^2z$ | 125.75 | 97.47 | 0.808 | 0.0741 | 0.0506 | 0.7287 | 0.2574 | 0.1747 | 0.719 |
| $a+b/\sqrt{y}+cx^2z^2$ | 136.39 | 105.73 | 0.774 | 0.0783 | 0.0529 | 0.6971 | 0.2717 | 0.1836 | 0.687 |
| $a+b/\sqrt{y}+cx^2\sqrt{z}$ | 120.84 | 94.83 | 0.822 | 0.0733 | 0.0506 | 0.7345 | 0.2504 | 0.1699 | 0.734 |
| $a+b/\sqrt{y}+c\sqrt{x}/z$ | 167.39 | 117.05 | 0.659 | 0.0943 | 0.0665 | 0.5613 | 0.3053 | 0.1893 | 0.605 |
| $a+b/\sqrt{y}+c\sqrt{x}/z^2$ | 190.83 | 136.97 | 0.557 | 0.1038 | 0.0786 | 0.4685 | 0.3317 | 0.2327 | 0.534 |
| $a+b/\sqrt{y}+c\sqrt{x}/\sqrt{z}$ | 164.05 | 115.14 | 0.673 | 0.0923 | 0.0629 | 0.5790 | 0.3039 | 0.1842 | 0.609 |
| $a+b/\sqrt{y}+c\sqrt{x}z$ | 124.42 | 95.68 | 0.812 | 0.0703 | 0.0426 | 0.7557 | 0.2471 | 0.1588 | 0.741 |
| $a+b/\sqrt{y}+c\sqrt{x}z^2$ | 133.46 | 103.82 | 0.783 | 0.0742 | 0.0482 | 0.7279 | 0.2616 | 0.1729 | 0.710 |
| $a+b/\sqrt{y}+c\sqrt{x}\sqrt{z}$ | 121.58 | 93.39 | 0.820 | 0.0694 | 0.0411 | 0.7621 | 0.2393 | 0.1452 | 0.757 |
| $a+b/\sqrt{y}+c/xz$ | 196.40 | 153.16 | 0.531 | 0.1092 | 0.0833 | 0.4112 | 0.3477 | 0.2486 | 0.488 |
| $a+b/\sqrt{y}+c/xz^2$ | 213.27 | 165.62 | 0.447 | 0.1098 | 0.0854 | 0.4044 | 0.3546 | 0.2560 | 0.467 |
| $a+b/\sqrt{y}+c/x\sqrt{z}$ | 194.58 | 148.81 | 0.539 | 0.1094 | 0.0834 | 0.4096 | 0.3466 | 0.2453 | 0.491 |
| $a+b/\sqrt{y}+cz/x$ | 177.33 | 133.47 | 0.617 | 0.1048 | 0.0795 | 0.4574 | 0.3295 | 0.2300 | 0.540 |
| $a+b/\sqrt{y}+cz^2/x$ | 140.24 | 104.62 | 0.761 | 0.0900 | 0.0627 | 0.6004 | 0.2879 | 0.1831 | 0.649 |
| $a+b/\sqrt{y}+c\sqrt{z}/x$ | 187.46 | 141.78 | 0.572 | 0.1078 | 0.0822 | 0.4265 | 0.3396 | 0.2392 | 0.511 |
| $a+b/\sqrt{y}+c/x^2z$ | 189.87 | 144.60 | 0.561 | 0.1085 | 0.0833 | 0.4183 | 0.3418 | 0.2435 | 0.505 |
| $a+b/\sqrt{y}+c/x^2z^2$ | 183.83 | 143.02 | 0.589 | 0.1070 | 0.0823 | 0.4348 | 0.3367 | 0.2402 | 0.520 |
| $a+b/\sqrt{y}+c/x^2\sqrt{z}$ | 191.69 | 144.79 | 0.553 | 0.1089 | 0.0835 | 0.4140 | 0.3432 | 0.2449 | 0.501 |
| $a+b/\sqrt{y}+cz/x^2$ | 194.06 | 144.56 | 0.542 | 0.1094 | 0.0836 | 0.4089 | 0.3449 | 0.2466 | 0.496 |
| $a+b/\sqrt{y}+cz^2/x^2$ | 192.88 | 143.57 | 0.547 | 0.1091 | 0.0835 | 0.4122 | 0.3437 | 0.2458 | 0.499 |
| $a+b/\sqrt{y}+c\sqrt{z}/x^2$ | 193.72 | 144.74 | 0.543 | 0.1094 | 0.0836 | 0.4095 | 0.3447 | 0.2464 | 0.497 |
| $a+b/\sqrt{y}+c/\sqrt{x}z$ | 205.06 | 144.98 | 0.488 | 0.1053 | 0.0810 | 0.4525 | 0.3335 | 0.2399 | 0.529 |
| $a+b/\sqrt{y}+c/\sqrt{x}z^2$ | 205.51 | 150.08 | 0.486 | 0.1094 | 0.0841 | 0.4093 | 0.3459 | 0.2524 | 0.493 |
| $a+b/\sqrt{y}+c/\sqrt{x}\sqrt{z}$ | 219.03 | 159.03 | 0.416 | 0.1087 | 0.0826 | 0.4162 | 0.3499 | 0.2456 | 0.481 |
| $a+b/\sqrt{y}+cz/\sqrt{x}$ | 132.48 | 99.23 | 0.786 | 0.0850 | 0.0574 | 0.6432 | 0.2753 | 0.1722 | 0.679 |
| $a+b/\sqrt{y}+cz^2/\sqrt{x}$ | 129.00 | 99.78 | 0.798 | 0.0752 | 0.0489 | 0.7208 | 0.2593 | 0.1659 | 0.715 |
| $a+b/\sqrt{y}+c\sqrt{z}/\sqrt{x}$ | 160.49 | 117.22 | 0.687 | 0.0985 | 0.0719 | 0.5210 | 0.3117 | 0.2122 | 0.588 |
| $a+b/\sqrt{y}+cy/z$ | 162.68 | 111.91 | 0.678 | 0.0892 | 0.0611 | 0.6072 | 0.2902 | 0.1762 | 0.643 |
| $a+b/\sqrt{y}+cy/z^2$ | 187.35 | 134.82 | 0.573 | 0.1016 | 0.0769 | 0.4902 | 0.3253 | 0.2252 | 0.552 |
| $a+b/\sqrt{y}+cy/\sqrt{z}$ | 167.47 | 119.29 | 0.659 | 0.0863 | 0.0595 | 0.6321 | 0.2843 | 0.1850 | 0.658 |
| $a+b/\sqrt{y}+cyz$ | 130.93 | 100.86 | 0.791 | 0.0759 | 0.0477 | 0.7154 | 0.2650 | 0.1687 | 0.702 |
| $a+b/\sqrt{y}+cyz^2$ | 137.82 | 106.63 | 0.769 | 0.0777 | 0.0501 | 0.7018 | 0.2718 | 0.1776 | 0.687 |
| $a+b/\sqrt{y}+cy\sqrt{z}$ | 131.27 | 100.78 | 0.790 | 0.0783 | 0.0490 | 0.6977 | 0.2689 | 0.1605 | 0.694 |
| $a+b/\sqrt{y}+cy^2/z$ | 179.44 | 124.36 | 0.608 | 0.0906 | 0.0631 | 0.5944 | 0.2985 | 0.2016 | 0.623 |
| $a+b/\sqrt{y}+cy^2/z^2$ | 185.75 | 133.92 | 0.580 | 0.0992 | 0.0739 | 0.5145 | 0.3202 | 0.2160 | 0.566 |
| $a+b/\sqrt{y}+cy^2/\sqrt{z}$ | 219.15 | 157.39 | 0.416 | 0.1092 | 0.0836 | 0.4107 | 0.3515 | 0.2497 | 0.477 |

(continued on next page)

**Table 4 – continued from previous page**

| Functional form | $T_{eff}$ (K) | | | Radius ($R_\odot$) | | | log (L/$L_\odot$) | | |
|---|---|---|---|---|---|---|---|---|---|
| | RMSE | MAD | $R^2_{ap}$ | RMSE | MAD | $R^2_{ap}$ | RMSE | MAD | $R^2_{ap}$ |
| $a+b/\sqrt{y}+cy^2z$ | 138.72 | 104.65 | 0.766 | 0.0810 | 0.0524 | 0.6759 | 0.2795 | 0.1756 | 0.669 |
| $a+b/\sqrt{y}+cy^2z^2$ | 142.71 | 109.98 | 0.752 | 0.0816 | 0.0536 | 0.6711 | 0.2821 | 0.1827 | 0.663 |
| $a+b/\sqrt{y}+cy^2\sqrt{z}$ | 142.12 | 104.59 | 0.754 | 0.0842 | 0.0546 | 0.6502 | 0.2863 | 0.1767 | 0.653 |
| $a+b/\sqrt{y}+c\sqrt{y}/z$ | 161.49 | 110.84 | 0.683 | 0.0913 | 0.0645 | 0.5888 | 0.2933 | 0.1797 | 0.635 |
| $a+b/\sqrt{y}+c\sqrt{y}/z^2$ | 188.80 | 135.76 | 0.566 | 0.1031 | 0.0785 | 0.4752 | 0.3284 | 0.2305 | 0.543 |
| $a+b/\sqrt{y}+c\sqrt{y}/\sqrt{z}$ | 149.89 | 103.90 | 0.727 | 0.0840 | 0.0559 | 0.6514 | 0.2745 | 0.1620 | 0.681 |
| $a+b/\sqrt{y}+c\sqrt{y}z$ | 127.56 | 100.84 | 0.802 | 0.0734 | 0.0445 | 0.7341 | 0.2567 | 0.1617 | 0.721 |
| $a+b/\sqrt{y}+c\sqrt{y}z^2$ | 135.49 | 106.30 | 0.777 | 0.0757 | 0.0485 | 0.7173 | 0.2659 | 0.1735 | 0.700 |
| $a+b/\sqrt{y}+c\sqrt{y}\sqrt{z}$ | 126.02 | 99.36 | 0.807 | 0.0749 | 0.0442 | 0.7234 | 0.2575 | 0.1529 | 0.719 |
| $a+b/\sqrt{y}+c/yz$ | 203.08 | 145.71 | 0.498 | 0.1093 | 0.0824 | 0.4107 | 0.3436 | 0.2454 | 0.500 |
| $a+b/\sqrt{y}+c/yz^2$ | 207.85 | 148.79 | 0.474 | 0.1109 | 0.0846 | 0.3930 | 0.3511 | 0.2543 | 0.478 |
| $a+b/\sqrt{y}+c/y\sqrt{z}$ | 205.78 | 147.66 | 0.485 | 0.1090 | 0.0821 | 0.4137 | 0.3428 | 0.2434 | 0.502 |
| $a+b/\sqrt{y}+cz/y$ | 127.48 | 97.67 | 0.802 | 0.0782 | 0.0520 | 0.6978 | 0.2538 | 0.1580 | 0.727 |
| $a+b/\sqrt{y}+cz^2/y$ | 129.60 | 97.20 | 0.796 | 0.0727 | 0.0475 | 0.7387 | 0.2504 | 0.1596 | 0.734 |
| $a+b/\sqrt{y}+c\sqrt{z}/y$ | 131.68 | 94.34 | 0.789 | 0.0843 | 0.0587 | 0.6490 | 0.2667 | 0.1638 | 0.699 |
| $a+b/\sqrt{y}+c/y^2z$ | 216.80 | 164.81 | 0.428 | 0.1087 | 0.0847 | 0.4162 | 0.3543 | 0.2590 | 0.468 |
| $a+b/\sqrt{y}+c/y^2z^2$ | 219.87 | 161.35 | 0.412 | 0.1110 | 0.0858 | 0.3913 | 0.3587 | 0.2630 | 0.455 |
| $a+b/\sqrt{y}+c/y^2\sqrt{z}$ | 203.08 | 162.24 | 0.498 | 0.1047 | 0.0798 | 0.4588 | 0.3424 | 0.2501 | 0.503 |
| $a+b/\sqrt{y}+cz/y^2$ | 146.72 | 106.34 | 0.738 | 0.0947 | 0.0694 | 0.5569 | 0.2952 | 0.2023 | 0.631 |
| $a+b/\sqrt{y}+cz^2/y^2$ | 130.73 | 97.34 | 0.792 | 0.0829 | 0.0554 | 0.6606 | 0.2642 | 0.1657 | 0.704 |
| $a+b/\sqrt{y}+c\sqrt{z}/y^2$ | 152.84 | 115.46 | 0.716 | 0.0970 | 0.0718 | 0.5358 | 0.3050 | 0.2128 | 0.606 |
| $a+b/\sqrt{y}+c/\sqrt{y}z$ | 177.40 | 127.00 | 0.617 | 0.1009 | 0.0766 | 0.4973 | 0.3160 | 0.2156 | 0.577 |
| $a+b/\sqrt{y}+c/\sqrt{y}z^2$ | 197.65 | 145.32 | 0.525 | 0.1079 | 0.0824 | 0.4253 | 0.3406 | 0.2464 | 0.508 |
| $a+b/\sqrt{y}+c/\sqrt{y}\sqrt{z}$ | 161.23 | 111.39 | 0.684 | 0.0942 | 0.0699 | 0.5620 | 0.2952 | 0.1906 | 0.631 |
| $a+b/\sqrt{y}+cz/\sqrt{y}$ | 126.39 | 98.17 | 0.806 | 0.0734 | 0.0469 | 0.7339 | 0.2479 | 0.1482 | 0.740 |
| $a+b/\sqrt{y}+cz^2/\sqrt{y}$ | 131.64 | 100.97 | 0.789 | 0.0726 | 0.0465 | 0.7396 | 0.2544 | 0.1655 | 0.726 |
| $a+b/\sqrt{y}+c\sqrt{z}/\sqrt{y}$ | 131.13 | 99.29 | 0.791 | 0.0781 | 0.0516 | 0.6987 | 0.2551 | 0.1536 | 0.724 |
| Single line EW, single EW ratio, double component functions result ( (z, x/y) ; (z, x/z) ; (z, y/z) ) | | | | | | | | | |
| $a+bz+cx/y$ | 130.58 | 101.53 | 0.793 | 0.0700 | 0.0478 | 0.7582 | 0.2453 | 0.1741 | 0.745 |
| $a+bz+cx/y^2$ | 136.03 | 111.46 | 0.775 | 0.0783 | 0.0549 | 0.6973 | 0.2881 | 0.2161 | 0.648 |
| $a+bz+cx/\sqrt{y}$ | 119.92 | 92.24 | 0.825 | 0.0678 | 0.0433 | 0.7728 | 0.2281 | 0.1463 | 0.780 |
| $a+bz+cxy$ | 117.54 | 90.31 | 0.832 | 0.0728 | 0.0475 | 0.7381 | 0.2565 | 0.1779 | 0.721 |
| $a+bz+cxy^2$ | 124.91 | 94.57 | 0.810 | 0.0758 | 0.0513 | 0.7161 | 0.2751 | 0.2057 | 0.679 |
| $a+bz+cx\sqrt{y}$ | 114.22 | 87.13 | 0.841 | 0.0706 | 0.0439 | 0.7542 | 0.2422 | 0.1558 | 0.751 |
| $a+bz+cx^2/y$ | 115.51 | 89.91 | 0.838 | 0.0680 | 0.0451 | 0.7717 | 0.2278 | 0.1559 | 0.780 |
| $a+bz+cx^2/y^2$ | 130.54 | 101.99 | 0.793 | 0.0717 | 0.0513 | 0.7462 | 0.2516 | 0.1840 | 0.732 |
| $a+bz+cx^2/\sqrt{y}$ | 111.03 | 87.75 | 0.850 | 0.0683 | 0.0442 | 0.7698 | 0.2302 | 0.1562 | 0.775 |
| $a+bz+cx^2y$ | 121.15 | 90.50 | 0.821 | 0.0744 | 0.0508 | 0.7265 | 0.2688 | 0.2003 | 0.694 |
| $a+bz+cx^2y^2$ | 127.67 | 94.88 | 0.802 | 0.0765 | 0.0531 | 0.7109 | 0.2806 | 0.2138 | 0.666 |
| $a+bz+cx^2\sqrt{y}$ | 116.42 | 89.52 | 0.835 | 0.0725 | 0.0493 | 0.7401 | 0.2576 | 0.1891 | 0.719 |
| $a+bz+c\sqrt{x}/y$ | 136.89 | 111.84 | 0.772 | 0.0782 | 0.0550 | 0.6979 | 0.2887 | 0.2165 | 0.647 |
| $a+bz+c\sqrt{x}/y^2$ | 123.57 | 94.86 | 0.814 | 0.0739 | 0.0478 | 0.7300 | 0.2558 | 0.1665 | 0.723 |
| $a+bz+c\sqrt{x}/\sqrt{y}$ | 132.02 | 102.39 | 0.788 | 0.0698 | 0.0474 | 0.7596 | 0.2464 | 0.1730 | 0.743 |
| $a+bz+c\sqrt{x}y$ | 119.33 | 91.93 | 0.827 | 0.0727 | 0.0454 | 0.7389 | 0.2543 | 0.1670 | 0.726 |
| $a+bz+c\sqrt{x}y^2$ | 124.70 | 95.44 | 0.811 | 0.0756 | 0.0502 | 0.7175 | 0.2728 | 0.1999 | 0.685 |
| $a+bz+c\sqrt{x}\sqrt{y}$ | 118.18 | 90.29 | 0.830 | 0.0707 | 0.0417 | 0.7530 | 0.2425 | 0.1470 | 0.751 |
| $a+bz+c/xy$ | 137.16 | 106.86 | 0.771 | 0.0724 | 0.0472 | 0.7410 | 0.2629 | 0.1800 | 0.707 |
| $a+bz+c/xy^2$ | 137.47 | 106.98 | 0.770 | 0.0726 | 0.0474 | 0.7400 | 0.2639 | 0.1811 | 0.705 |
| $a+bz+c/x\sqrt{y}$ | 137.00 | 106.78 | 0.772 | 0.0723 | 0.0471 | 0.7417 | 0.2624 | 0.1795 | 0.708 |
| $a+bz+cy/x$ | 137.63 | 106.54 | 0.770 | 0.0718 | 0.0476 | 0.7456 | 0.2618 | 0.1776 | 0.710 |
| $a+bz+cy^2/x$ | 138.82 | 111.82 | 0.766 | 0.0775 | 0.0561 | 0.7033 | 0.2879 | 0.2132 | 0.649 |
| $a+bz+c\sqrt{y}/x$ | 136.94 | 106.59 | 0.772 | 0.0720 | 0.0471 | 0.7440 | 0.2613 | 0.1782 | 0.711 |
| $a+bz+c/x^2y$ | 139.41 | 107.02 | 0.764 | 0.0734 | 0.0487 | 0.7339 | 0.2704 | 0.1881 | 0.690 |
| $a+bz+c/x^2y^2$ | 139.47 | 107.00 | 0.763 | 0.0735 | 0.0488 | 0.7336 | 0.2707 | 0.1884 | 0.689 |
| $a+bz+c/x^2\sqrt{y}$ | 139.38 | 107.03 | 0.764 | 0.0734 | 0.0487 | 0.7341 | 0.2703 | 0.1880 | 0.690 |
| $a+bz+cy/x^2$ | 139.27 | 107.04 | 0.764 | 0.0733 | 0.0486 | 0.7350 | 0.2697 | 0.1874 | 0.692 |
| $a+bz+cy^2/x^2$ | 139.28 | 106.92 | 0.764 | 0.0730 | 0.0487 | 0.7366 | 0.2691 | 0.1864 | 0.693 |
| $a+bz+c\sqrt{y}/x^2$ | 139.31 | 107.05 | 0.764 | 0.0733 | 0.0486 | 0.7346 | 0.2699 | 0.1876 | 0.691 |
| $a+bz+c/\sqrt{x}y$ | 133.84 | 104.91 | 0.782 | 0.0718 | 0.0451 | 0.7457 | 0.2559 | 0.1697 | 0.723 |
| $a+bz+c/\sqrt{x}y^2$ | 134.62 | 105.44 | 0.780 | 0.0720 | 0.0456 | 0.7440 | 0.2576 | 0.1717 | 0.719 |
| $a+bz+c/\sqrt{x}\sqrt{y}$ | 133.48 | 104.63 | 0.783 | 0.0716 | 0.0449 | 0.7472 | 0.2548 | 0.1686 | 0.725 |
| $a+bz+cy/\sqrt{x}$ | 138.29 | 111.98 | 0.767 | 0.0778 | 0.0557 | 0.7011 | 0.2885 | 0.2149 | 0.647 |
| $a+bz+cy^2/\sqrt{x}$ | 130.29 | 103.65 | 0.793 | 0.0770 | 0.0509 | 0.7075 | 0.2783 | 0.1997 | 0.672 |
| $a+bz+c\sqrt{y}/\sqrt{x}$ | 136.08 | 105.56 | 0.775 | 0.0709 | 0.0474 | 0.7515 | 0.2564 | 0.1737 | 0.721 |
| $a+bz+cx/z$ | 124.47 | 98.52 | 0.811 | 0.0695 | 0.0436 | 0.7617 | 0.2458 | 0.1715 | 0.744 |
| $a+bz+cx/z^2$ | 136.79 | 103.51 | 0.772 | 0.0743 | 0.0509 | 0.7274 | 0.2752 | 0.2084 | 0.679 |
| $a+bz+cx/\sqrt{z}$ | 115.45 | 87.11 | 0.838 | 0.0677 | 0.0398 | 0.7739 | 0.2280 | 0.1345 | 0.780 |
| $a+bz+cxz$ | 128.40 | 95.90 | 0.799 | 0.0733 | 0.0529 | 0.7346 | 0.2703 | 0.2080 | 0.690 |
| $a+bz+cxz^2$ | 140.46 | 108.33 | 0.760 | 0.0783 | 0.0550 | 0.6974 | 0.2881 | 0.2123 | 0.648 |
| $a+bz+cx\sqrt{z}$ | 116.86 | 89.75 | 0.834 | 0.0694 | 0.0442 | 0.7620 | 0.2407 | 0.1607 | 0.755 |
| $a+bz+cx^2/z$ | 110.27 | 83.66 | 0.852 | 0.0675 | 0.0404 | 0.7751 | 0.2267 | 0.1420 | 0.782 |
| $a+bz+cx^2/z^2$ | 130.45 | 101.69 | 0.793 | 0.0722 | 0.0480 | 0.7426 | 0.2623 | 0.1995 | 0.709 |
| $a+bz+cx^2/\sqrt{z}$ | 107.43 | 81.10 | 0.860 | 0.0682 | 0.0427 | 0.7702 | 0.2280 | 0.1434 | 0.780 |
| $a+bz+cx^2z$ | 133.03 | 97.49 | 0.785 | 0.0765 | 0.0551 | 0.7112 | 0.2837 | 0.2183 | 0.659 |
| $a+bz+cx^2z^2$ | 139.78 | 107.93 | 0.762 | 0.0783 | 0.0548 | 0.6975 | 0.2885 | 0.2147 | 0.647 |
| $a+bz+cx^2\sqrt{z}$ | 121.70 | 90.38 | 0.820 | 0.0732 | 0.0515 | 0.7357 | 0.2653 | 0.2019 | 0.702 |
| $a+bz+c\sqrt{x}/z$ | 134.89 | 104.24 | 0.779 | 0.0725 | 0.0485 | 0.7403 | 0.2675 | 0.1999 | 0.697 |
| $a+bz+c\sqrt{x}/z^2$ | 139.78 | 106.80 | 0.762 | 0.0759 | 0.0531 | 0.7158 | 0.2833 | 0.2155 | 0.660 |
| $a+bz+c\sqrt{x}/\sqrt{z}$ | 125.53 | 97.37 | 0.808 | 0.0690 | 0.0415 | 0.7652 | 0.2428 | 0.1613 | 0.750 |
| $a+bz+c\sqrt{x}z$ | 128.04 | 96.68 | 0.801 | 0.0710 | 0.0482 | 0.7511 | 0.2590 | 0.1873 | 0.716 |
| $a+bz+c\sqrt{x}z^2$ | 140.50 | 109.17 | 0.760 | 0.0783 | 0.0549 | 0.6972 | 0.2874 | 0.2084 | 0.650 |
| $a+bz+c\sqrt{x}\sqrt{z}$ | 121.53 | 93.71 | 0.820 | 0.0695 | 0.0408 | 0.7613 | 0.2384 | 0.1441 | 0.759 |
| $a+bz+c/xz$ | 133.65 | 104.66 | 0.783 | 0.0720 | 0.0451 | 0.7442 | 0.2554 | 0.1661 | 0.724 |
| $a+bz+c/xz^2$ | 129.76 | 101.00 | 0.795 | 0.0732 | 0.0469 | 0.7358 | 0.2546 | 0.1539 | 0.725 |
| $a+bz+c/x\sqrt{z}$ | 135.48 | 105.96 | 0.777 | 0.0720 | 0.0462 | 0.7442 | 0.2585 | 0.1731 | 0.717 |
| $a+bz+cz/x$ | 138.31 | 107.05 | 0.767 | 0.0727 | 0.0479 | 0.7391 | 0.2666 | 0.1848 | 0.699 |
| $a+bz+cz^2/x$ | 138.00 | 107.10 | 0.768 | 0.0727 | 0.0467 | 0.7389 | 0.2660 | 0.1793 | 0.700 |
| $a+bz+c\sqrt{z}/x$ | 137.81 | 106.97 | 0.769 | 0.0725 | 0.0476 | 0.7407 | 0.2647 | 0.1828 | 0.703 |
| $a+bz+c/x^2z$ | 138.62 | 107.17 | 0.766 | 0.0730 | 0.0482 | 0.7370 | 0.2673 | 0.1850 | 0.697 |
| $a+bz+c/x^2z^2$ | 137.16 | 106.86 | 0.771 | 0.0726 | 0.0473 | 0.7401 | 0.2631 | 0.1795 | 0.707 |
| $a+bz+c/x^2\sqrt{z}$ | 139.05 | 107.13 | 0.765 | 0.0732 | 0.0485 | 0.7355 | 0.2689 | 0.1866 | 0.694 |
| $a+bz+cz/x^2$ | 139.70 | 106.85 | 0.763 | 0.0736 | 0.0489 | 0.7325 | 0.2718 | 0.1893 | 0.687 |
| $a+bz+cz^2/x^2$ | 139.84 | 106.73 | 0.762 | 0.0737 | 0.0489 | 0.7315 | 0.2727 | 0.1898 | 0.685 |

(continued on next page)

**Table 4 – continued from previous page**

| Functional form | $T_{eff}$ (K) | | | Radius ($R_\odot$) | | | log (L/$L_\odot$) | | |
|---|---|---|---|---|---|---|---|---|---|
| | RMSE | MAD | $R^2_{ap}$ | RMSE | MAD | $R^2_{ap}$ | RMSE | MAD | $R^2_{ap}$ |
| $a+bz+c\sqrt{z}/x^2$ | 139.55 | 106.94 | 0.763 | 0.0735 | 0.0488 | 0.7333 | 0.2711 | 0.1887 | 0.689 |
| $a+bz+c/\sqrt{x}z$ | 128.53 | 100.23 | 0.799 | 0.0731 | 0.0458 | 0.7362 | 0.2521 | 0.1488 | 0.731 |
| $a+bz+c/\sqrt{x}z^2$ | 130.30 | 98.48 | 0.793 | 0.0767 | 0.0504 | 0.7096 | 0.2696 | 0.1717 | 0.692 |
| $a+bz+c/\sqrt{x}\sqrt{z}$ | 130.66 | 102.38 | 0.792 | 0.0716 | 0.0436 | 0.7466 | 0.2500 | 0.1555 | 0.735 |
| $a+bz+cz/\sqrt{x}$ | 136.16 | 106.04 | 0.774 | 0.0717 | 0.0465 | 0.7462 | 0.2613 | 0.1791 | 0.711 |
| $a+bz+cz^2/\sqrt{x}$ | 133.69 | 105.43 | 0.783 | 0.0735 | 0.0457 | 0.7334 | 0.2601 | 0.1601 | 0.713 |
| $a+bz+c\sqrt{z}/\sqrt{x}$ | 135.63 | 105.78 | 0.776 | 0.0715 | 0.0463 | 0.7478 | 0.2592 | 0.1777 | 0.715 |
| $a+bz+cy/z$ | 132.00 | 105.23 | 0.788 | 0.0735 | 0.0483 | 0.7333 | 0.2675 | 0.1965 | 0.697 |
| $a+bz+cy/z^2$ | 139.02 | 106.17 | 0.765 | 0.0758 | 0.0529 | 0.7165 | 0.2820 | 0.2150 | 0.663 |
| $a+bz+cy/\sqrt{z}$ | 125.06 | 98.26 | 0.810 | 0.0729 | 0.0449 | 0.7379 | 0.2575 | 0.1721 | 0.719 |
| $a+bz+cyz$ | 135.52 | 106.84 | 0.777 | 0.0773 | 0.0541 | 0.7048 | 0.2856 | 0.2157 | 0.654 |
| $a+bz+cyz^2$ | 140.56 | 108.65 | 0.760 | 0.0783 | 0.0545 | 0.6975 | 0.2866 | 0.2069 | 0.652 |
| $a+bz+cy\sqrt{z}$ | 127.57 | 101.31 | 0.802 | 0.0754 | 0.0492 | 0.7196 | 0.2711 | 0.1932 | 0.689 |
| $a+bz+cy^2/z$ | 124.85 | 98.45 | 0.810 | 0.0736 | 0.0460 | 0.7328 | 0.2612 | 0.1808 | 0.711 |
| $a+bz+cy^2/z^2$ | 134.87 | 104.59 | 0.779 | 0.0745 | 0.0503 | 0.7257 | 0.2739 | 0.2070 | 0.682 |
| $a+bz+cy^2/\sqrt{z}$ | 123.63 | 97.02 | 0.814 | 0.0746 | 0.0471 | 0.7255 | 0.2642 | 0.1814 | 0.704 |
| $a+bz+cy^2z$ | 137.00 | 107.79 | 0.772 | 0.0781 | 0.0540 | 0.6992 | 0.2884 | 0.2162 | 0.648 |
| $a+bz+cy^2z^2$ | 140.27 | 108.98 | 0.761 | 0.0783 | 0.0547 | 0.6974 | 0.2873 | 0.2100 | 0.650 |
| $a+bz+cy^2\sqrt{z}$ | 131.51 | 103.19 | 0.790 | 0.0771 | 0.0529 | 0.7063 | 0.2827 | 0.2121 | 0.661 |
| $a+bz+c\sqrt{y}/z$ | 138.69 | 106.08 | 0.766 | 0.0755 | 0.0527 | 0.7185 | 0.2812 | 0.2149 | 0.665 |
| $a+bz+c\sqrt{y}/z^2$ | 140.47 | 108.22 | 0.760 | 0.0769 | 0.0546 | 0.7083 | 0.2868 | 0.2186 | 0.651 |
| $a+bz+c\sqrt{y}/\sqrt{z}$ | 130.86 | 104.51 | 0.792 | 0.0730 | 0.0471 | 0.7371 | 0.2642 | 0.1887 | 0.704 |
| $a+bz+c\sqrt{y}z$ | 134.32 | 107.20 | 0.781 | 0.0764 | 0.0534 | 0.7114 | 0.2817 | 0.2126 | 0.664 |
| $a+bz+c\sqrt{y}z^2$ | 140.33 | 109.49 | 0.760 | 0.0782 | 0.0542 | 0.6978 | 0.2857 | 0.2033 | 0.654 |
| $a+bz+c\sqrt{y}\sqrt{z}$ | 125.77 | 100.16 | 0.808 | 0.0744 | 0.0456 | 0.7270 | 0.2626 | 0.1712 | 0.708 |
| $a+bz+c/yz$ | 124.63 | 94.24 | 0.811 | 0.0746 | 0.0482 | 0.7253 | 0.2561 | 0.1589 | 0.722 |
| $a+bz+c/yz^2$ | 128.49 | 96.17 | 0.799 | 0.0771 | 0.0511 | 0.7064 | 0.2715 | 0.1762 | 0.688 |
| $a+bz+c/y\sqrt{z}$ | 124.87 | 95.52 | 0.810 | 0.0730 | 0.0463 | 0.7369 | 0.2501 | 0.1509 | 0.735 |
| $a+bz+cz/y$ | 132.57 | 105.79 | 0.786 | 0.0727 | 0.0453 | 0.7390 | 0.2625 | 0.1785 | 0.708 |
| $a+bz+cz^2/y$ | 131.05 | 103.97 | 0.791 | 0.0749 | 0.0468 | 0.7229 | 0.2680 | 0.1751 | 0.696 |
| $a+bz+c\sqrt{z}/y$ | 130.49 | 103.57 | 0.793 | 0.0719 | 0.0434 | 0.7447 | 0.2556 | 0.1697 | 0.723 |
| $a+bz+c/y^2z$ | 125.60 | 95.40 | 0.808 | 0.0734 | 0.0483 | 0.7339 | 0.2531 | 0.1599 | 0.729 |
| $a+bz+c/y^2z^2$ | 125.14 | 92.38 | 0.809 | 0.0753 | 0.0503 | 0.7198 | 0.2614 | 0.1712 | 0.710 |
| $a+bz+c/y^2\sqrt{z}$ | 127.14 | 97.80 | 0.803 | 0.0725 | 0.0468 | 0.7403 | 0.2510 | 0.1540 | 0.733 |
| $a+bz+cz/y^2$ | 133.80 | 105.48 | 0.782 | 0.0720 | 0.0450 | 0.7439 | 0.2584 | 0.1746 | 0.717 |
| $a+bz+cz^2/y^2$ | 135.27 | 107.18 | 0.777 | 0.0731 | 0.0461 | 0.7365 | 0.2655 | 0.1801 | 0.701 |
| $a+bz+c\sqrt{z}/y^2$ | 131.80 | 103.41 | 0.789 | 0.0718 | 0.0443 | 0.7456 | 0.2542 | 0.1664 | 0.726 |
| $a+bz+c/\sqrt{y}z$ | 127.86 | 96.09 | 0.801 | 0.0765 | 0.0493 | 0.7109 | 0.2669 | 0.1672 | 0.698 |
| $a+bz+c/\sqrt{y}z^2$ | 134.29 | 103.25 | 0.781 | 0.0782 | 0.0539 | 0.6981 | 0.2823 | 0.1958 | 0.662 |
| $a+bz+c/\sqrt{y}\sqrt{z}$ | 124.69 | 94.93 | 0.811 | 0.0743 | 0.0465 | 0.7275 | 0.2545 | 0.1520 | 0.726 |
| $a+bz+cz/\sqrt{y}$ | 132.45 | 106.55 | 0.787 | 0.0737 | 0.0482 | 0.7315 | 0.2681 | 0.1896 | 0.695 |
| $a+bz+cz^2/\sqrt{y}$ | 133.28 | 101.38 | 0.784 | 0.0769 | 0.0492 | 0.7080 | 0.2744 | 0.1765 | 0.681 |
| $a+bz+c\sqrt{z}/\sqrt{y}$ | 131.30 | 104.90 | 0.790 | 0.0726 | 0.0455 | 0.7398 | 0.2616 | 0.1788 | 0.710 |
| $a+bz^2+cx/y$ | 140.06 | 106.86 | 0.761 | 0.0716 | 0.0516 | 0.7471 | 0.2564 | 0.1871 | 0.721 |
| $a+bz^2+cx/y^2$ | 149.59 | 121.45 | 0.728 | 0.0840 | 0.0626 | 0.6517 | 0.3126 | 0.2430 | 0.586 |
| $a+bz^2+cx/\sqrt{y}$ | 123.21 | 93.38 | 0.815 | 0.0676 | 0.0440 | 0.7743 | 0.2307 | 0.1555 | 0.774 |
| $a+bz^2+cxy$ | 122.12 | 92.97 | 0.819 | 0.0745 | 0.0521 | 0.7258 | 0.2637 | 0.1868 | 0.705 |
| $a+bz^2+cxy^2$ | 133.79 | 99.52 | 0.782 | 0.0795 | 0.0581 | 0.6883 | 0.2900 | 0.2219 | 0.644 |
| $a+bz^2+cx\sqrt{y}$ | 116.88 | 88.44 | 0.834 | 0.0712 | 0.0477 | 0.7495 | 0.2462 | 0.1641 | 0.743 |
| $a+bz^2+cx^2/y$ | 116.41 | 90.24 | 0.835 | 0.0673 | 0.0461 | 0.7760 | 0.2283 | 0.1655 | 0.779 |
| $a+bz^2+cx^2/y^2$ | 139.20 | 106.43 | 0.764 | 0.0732 | 0.0544 | 0.7353 | 0.2621 | 0.1956 | 0.709 |
| $a+bz^2+cx^2/\sqrt{y}$ | 111.79 | 87.94 | 0.848 | 0.0680 | 0.0467 | 0.7714 | 0.2314 | 0.1633 | 0.773 |
| $a+bz^2+cx^2y$ | 128.18 | 97.34 | 0.800 | 0.0773 | 0.0565 | 0.7050 | 0.2802 | 0.2140 | 0.667 |
| $a+bz^2+cx^2y^2$ | 139.24 | 104.58 | 0.764 | 0.0811 | 0.0610 | 0.6752 | 0.2998 | 0.2359 | 0.619 |
| $a+bz^2+cx^2\sqrt{y}$ | 120.95 | 92.98 | 0.822 | 0.0743 | 0.0541 | 0.7274 | 0.2646 | 0.1989 | 0.703 |
| $a+bz^2+c\sqrt{x}/y$ | 151.05 | 122.47 | 0.722 | 0.0841 | 0.0627 | 0.6505 | 0.3142 | 0.2444 | 0.582 |
| $a+bz^2+c\sqrt{x}/y^2$ | 129.88 | 100.03 | 0.795 | 0.0759 | 0.0512 | 0.7154 | 0.2658 | 0.1785 | 0.701 |
| $a+bz^2+c\sqrt{x}/\sqrt{y}$ | 142.82 | 107.89 | 0.752 | 0.0719 | 0.0513 | 0.7450 | 0.2597 | 0.1864 | 0.714 |
| $a+bz^2+c\sqrt{x}y$ | 124.12 | 94.01 | 0.813 | 0.0743 | 0.0502 | 0.7274 | 0.2616 | 0.1766 | 0.710 |
| $a+bz^2+c\sqrt{x}y^2$ | 132.91 | 99.80 | 0.785 | 0.0789 | 0.0569 | 0.6923 | 0.2864 | 0.2148 | 0.652 |
| $a+bz^2+c\sqrt{x}\sqrt{y}$ | 121.88 | 92.15 | 0.819 | 0.0715 | 0.0452 | 0.7475 | 0.2475 | 0.1596 | 0.740 |
| $a+bz^2+c/xy$ | 152.10 | 117.69 | 0.719 | 0.0767 | 0.0538 | 0.7095 | 0.2845 | 0.2036 | 0.657 |
| $a+bz^2+c/xy^2$ | 152.66 | 118.05 | 0.716 | 0.0770 | 0.0541 | 0.7074 | 0.2860 | 0.2049 | 0.653 |
| $a+bz^2+c/x\sqrt{y}$ | 151.79 | 117.41 | 0.720 | 0.0765 | 0.0536 | 0.7109 | 0.2836 | 0.2028 | 0.659 |
| $a+bz^2+cy/x$ | 152.70 | 116.30 | 0.716 | 0.0760 | 0.0539 | 0.7146 | 0.2834 | 0.2027 | 0.660 |
| $a+bz^2+cy^2/x$ | 154.56 | 123.97 | 0.709 | 0.0839 | 0.0628 | 0.6526 | 0.3159 | 0.2441 | 0.577 |
| $a+bz^2+c\sqrt{y}/x$ | 151.58 | 116.61 | 0.720 | 0.0761 | 0.0535 | 0.7143 | 0.2821 | 0.2011 | 0.663 |
| $a+bz^2+c/x^2y$ | 155.80 | 118.64 | 0.705 | 0.0786 | 0.0556 | 0.6951 | 0.2953 | 0.2130 | 0.631 |
| $a+bz^2+c/x^2y^2$ | 155.90 | 118.63 | 0.704 | 0.0787 | 0.0557 | 0.6945 | 0.2956 | 0.2133 | 0.630 |
| $a+bz^2+c/x^2\sqrt{y}$ | 155.75 | 118.64 | 0.705 | 0.0785 | 0.0556 | 0.6954 | 0.2951 | 0.2129 | 0.631 |
| $a+bz^2+cy/x^2$ | 155.54 | 118.54 | 0.706 | 0.0783 | 0.0555 | 0.6970 | 0.2942 | 0.2121 | 0.633 |
| $a+bz^2+cy^2/x^2$ | 155.53 | 118.23 | 0.706 | 0.0781 | 0.0554 | 0.6989 | 0.2935 | 0.2110 | 0.635 |
| $a+bz^2+c\sqrt{y}/x^2$ | 155.61 | 118.60 | 0.705 | 0.0784 | 0.0555 | 0.6963 | 0.2945 | 0.2125 | 0.632 |
| $a+bz^2+c/\sqrt{x}y$ | 146.58 | 113.94 | 0.739 | 0.0750 | 0.0512 | 0.7221 | 0.2733 | 0.1908 | 0.683 |
| $a+bz^2+c/\sqrt{x}y^2$ | 148.02 | 115.28 | 0.733 | 0.0756 | 0.0518 | 0.7180 | 0.2764 | 0.1937 | 0.676 |
| $a+bz^2+c/\sqrt{x}\sqrt{y}$ | 145.88 | 113.15 | 0.741 | 0.0747 | 0.0508 | 0.7248 | 0.2716 | 0.1892 | 0.688 |
| $a+bz^2+cy/\sqrt{x}$ | 153.56 | 123.59 | 0.713 | 0.0841 | 0.0628 | 0.6510 | 0.3158 | 0.2449 | 0.577 |
| $a+bz^2+cy^2/\sqrt{x}$ | 140.58 | 109.19 | 0.760 | 0.0810 | 0.0586 | 0.6763 | 0.2955 | 0.2210 | 0.630 |
| $a+bz^2+c\sqrt{y}/\sqrt{x}$ | 150.01 | 113.34 | 0.726 | 0.0745 | 0.0527 | 0.7258 | 0.2755 | 0.1961 | 0.678 |
| $a+bz^2+cx/z$ | 150.26 | 121.35 | 0.725 | 0.0793 | 0.0598 | 0.6894 | 0.2918 | 0.2283 | 0.639 |
| $a+bz^2+cx/z^2$ | 157.70 | 121.64 | 0.697 | 0.0838 | 0.0620 | 0.6535 | 0.3146 | 0.2419 | 0.581 |
| $a+bz^2+cx/\sqrt{z}$ | 129.51 | 101.52 | 0.796 | 0.0717 | 0.0485 | 0.7460 | 0.2501 | 0.1806 | 0.735 |
| $a+bz^2+cxz$ | 123.20 | 95.02 | 0.815 | 0.0721 | 0.0498 | 0.7437 | 0.2567 | 0.1800 | 0.721 |
| $a+bz^2+cxz^2$ | 156.22 | 118.49 | 0.703 | 0.0841 | 0.0628 | 0.6506 | 0.3158 | 0.2438 | 0.577 |
| $a+bz^2+cx\sqrt{z}$ | 117.02 | 89.85 | 0.833 | 0.0694 | 0.0449 | 0.7623 | 0.2399 | 0.1554 | 0.756 |
| $a+bz^2+cx^2/z$ | 128.41 | 99.84 | 0.799 | 0.0730 | 0.0520 | 0.7367 | 0.2556 | 0.1889 | 0.723 |
| $a+bz^2+cx^2/z^2$ | 155.51 | 123.97 | 0.706 | 0.0822 | 0.0621 | 0.6663 | 0.3066 | 0.2439 | 0.602 |
| $a+bz^2+cx^2/\sqrt{z}$ | 112.82 | 86.89 | 0.845 | 0.0695 | 0.0477 | 0.7615 | 0.2364 | 0.1653 | 0.763 |
| $a+bz^2+cx^2z$ | 138.13 | 104.22 | 0.768 | 0.0794 | 0.0611 | 0.6888 | 0.2936 | 0.2345 | 0.635 |
| $a+bz^2+cx^2z^2$ | 156.90 | 119.91 | 0.700 | 0.0841 | 0.0630 | 0.6506 | 0.3157 | 0.2466 | 0.578 |
| $a+bz^2+cx^2\sqrt{z}$ | 123.90 | 94.53 | 0.813 | 0.0744 | 0.0547 | 0.7267 | 0.2675 | 0.2029 | 0.697 |

(continued on next page)

**Table 4 – continued from previous page**

| Functional form | $T_{eff}$ (K) | | | Radius ($R_\odot$) | | | log (L/$L_\odot$) | | |
|---|---|---|---|---|---|---|---|---|---|
| | RMSE | MAD | $R^2_{ap}$ | RMSE | MAD | $R^2_{ap}$ | RMSE | MAD | $R^2_{ap}$ |
| $a+bz^2+c\sqrt{x}/z$ | 157.68 | 122.12 | 0.698 | 0.0833 | 0.0621 | 0.6575 | 0.3128 | 0.2415 | 0.586 |
| $a+bz^2+c\sqrt{x}/z^2$ | 155.70 | 121.55 | 0.705 | 0.0842 | 0.0627 | 0.6502 | 0.3157 | 0.2443 | 0.578 |
| $a+bz^2+c\sqrt{x}/\sqrt{z}$ | 148.06 | 119.91 | 0.733 | 0.0774 | 0.0567 | 0.7046 | 0.2831 | 0.2112 | 0.660 |
| $a+bz^2+c\sqrt{x}z$ | 123.93 | 96.71 | 0.813 | 0.0703 | 0.0428 | 0.7557 | 0.2471 | 0.1532 | 0.741 |
| $a+bz^2+c\sqrt{x}z^2$ | 155.21 | 116.17 | 0.707 | 0.0836 | 0.0640 | 0.6546 | 0.3140 | 0.2448 | 0.582 |
| $a+bz^2+c\sqrt{x}\sqrt{z}$ | 121.45 | 92.96 | 0.821 | 0.0693 | 0.0410 | 0.7630 | 0.2390 | 0.1420 | 0.758 |
| $a+bz^2+c/xz$ | 144.70 | 110.77 | 0.745 | 0.0744 | 0.0509 | 0.7269 | 0.2693 | 0.1870 | 0.693 |
| $a+bz^2+c/xz^2$ | 135.88 | 102.44 | 0.775 | 0.0741 | 0.0495 | 0.7288 | 0.2615 | 0.1727 | 0.710 |
| $a+bz^2+c/x\sqrt{z}$ | 148.58 | 114.53 | 0.731 | 0.0753 | 0.0522 | 0.7203 | 0.2761 | 0.1947 | 0.677 |
| $a+bz^2+cz/x$ | 154.87 | 118.83 | 0.708 | 0.0781 | 0.0552 | 0.6987 | 0.2927 | 0.2104 | 0.637 |
| $a+bz^2+cz^2/x$ | 155.44 | 118.48 | 0.706 | 0.0787 | 0.0561 | 0.6941 | 0.2959 | 0.2119 | 0.629 |
| $a+bz^2+c\sqrt{z}/x$ | 153.59 | 118.34 | 0.713 | 0.0773 | 0.0545 | 0.7050 | 0.2884 | 0.2071 | 0.648 |
| $a+bz^2+c/x^2z$ | 154.45 | 118.51 | 0.710 | 0.0778 | 0.0550 | 0.7014 | 0.2907 | 0.2095 | 0.642 |
| $a+bz^2+c/x^2z^2$ | 151.97 | 117.50 | 0.719 | 0.0767 | 0.0538 | 0.7093 | 0.2844 | 0.2032 | 0.657 |
| $a+bz^2+c/x^2\sqrt{z}$ | 155.17 | 118.62 | 0.707 | 0.0782 | 0.0553 | 0.6983 | 0.2930 | 0.2114 | 0.636 |
| $a+bz^2+cz/x^2$ | 156.29 | 118.51 | 0.703 | 0.0790 | 0.0559 | 0.6922 | 0.2972 | 0.2143 | 0.626 |
| $a+bz^2+cz^2/x^2$ | 156.58 | 118.36 | 0.702 | 0.0792 | 0.0560 | 0.6901 | 0.2986 | 0.2150 | 0.622 |
| $a+bz^2+c\sqrt{z}/x^2$ | 156.04 | 118.58 | 0.704 | 0.0787 | 0.0557 | 0.6938 | 0.2962 | 0.2136 | 0.628 |
| $a+bz^2+c/\sqrt{x}z$ | 130.33 | 98.10 | 0.793 | 0.0726 | 0.0474 | 0.7400 | 0.2524 | 0.1609 | 0.730 |
| $a+bz^2+c/\sqrt{x}z^2$ | 129.15 | 95.12 | 0.797 | 0.0769 | 0.0528 | 0.7083 | 0.2700 | 0.1792 | 0.691 |
| $a+bz^2+c/\sqrt{x}\sqrt{z}$ | 137.30 | 103.74 | 0.771 | 0.0724 | 0.0479 | 0.7415 | 0.2564 | 0.1721 | 0.721 |
| $a+bz^2+cz/\sqrt{x}$ | 155.78 | 119.95 | 0.705 | 0.0796 | 0.0571 | 0.6870 | 0.2989 | 0.2142 | 0.622 |
| $a+bz^2+cz^2/\sqrt{x}$ | 154.12 | 117.57 | 0.711 | 0.0791 | 0.0580 | 0.6908 | 0.2971 | 0.2173 | 0.626 |
| $a+bz^2+c\sqrt{z}/\sqrt{x}$ | 152.50 | 118.88 | 0.717 | 0.0771 | 0.0543 | 0.7061 | 0.2868 | 0.2042 | 0.651 |
| $a+bz^2+cy/z$ | 156.56 | 124.10 | 0.702 | 0.0831 | 0.0616 | 0.6592 | 0.3106 | 0.2423 | 0.591 |
| $a+bz^2+cy/z^2$ | 156.65 | 121.56 | 0.701 | 0.0842 | 0.0627 | 0.6503 | 0.3159 | 0.2444 | 0.577 |
| $a+bz^2+cy/\sqrt{z}$ | 144.40 | 118.03 | 0.746 | 0.0792 | 0.0563 | 0.6903 | 0.2883 | 0.2143 | 0.648 |
| $a+bz^2+cyz$ | 135.94 | 106.00 | 0.775 | 0.0790 | 0.0567 | 0.6921 | 0.2879 | 0.2137 | 0.649 |
| $a+bz^2+cyz^2$ | 157.66 | 121.81 | 0.698 | 0.0837 | 0.0626 | 0.6543 | 0.3140 | 0.2450 | 0.582 |
| $a+bz^2+cy\sqrt{z}$ | 130.01 | 101.21 | 0.794 | 0.0766 | 0.0521 | 0.7101 | 0.2742 | 0.1902 | 0.681 |
| $a+bz^2+cy^2/z$ | 146.49 | 119.20 | 0.739 | 0.0806 | 0.0584 | 0.6790 | 0.2952 | 0.2263 | 0.631 |
| $a+bz^2+cy^2/z^2$ | 157.51 | 123.30 | 0.698 | 0.0837 | 0.0619 | 0.6543 | 0.3137 | 0.2423 | 0.583 |
| $a+bz^2+cy^2/\sqrt{z}$ | 136.72 | 108.78 | 0.773 | 0.0789 | 0.0554 | 0.6926 | 0.2848 | 0.2067 | 0.656 |
| $a+bz^2+cy^2z$ | 147.98 | 111.23 | 0.734 | 0.0831 | 0.0629 | 0.6586 | 0.3098 | 0.2433 | 0.593 |
| $a+bz^2+cy^2z^2$ | 157.68 | 121.74 | 0.697 | 0.0834 | 0.0626 | 0.6569 | 0.3128 | 0.2450 | 0.585 |
| $a+bz^2+cy^2\sqrt{z}$ | 139.50 | 106.23 | 0.763 | 0.0809 | 0.0598 | 0.6771 | 0.2970 | 0.2280 | 0.626 |
| $a+bz^2+c\sqrt{y}/z$ | 156.09 | 120.60 | 0.704 | 0.0842 | 0.0626 | 0.6503 | 0.3156 | 0.2439 | 0.578 |
| $a+bz^2+c\sqrt{y}/z^2$ | 153.17 | 118.82 | 0.715 | 0.0839 | 0.0624 | 0.6521 | 0.3135 | 0.2409 | 0.583 |
| $a+bz^2+c\sqrt{y}/\sqrt{z}$ | 155.64 | 123.26 | 0.705 | 0.0825 | 0.0611 | 0.6637 | 0.3079 | 0.2394 | 0.598 |
| $a+bz^2+c\sqrt{y}z$ | 129.07 | 102.36 | 0.797 | 0.0756 | 0.0489 | 0.7180 | 0.2700 | 0.1779 | 0.691 |
| $a+bz^2+c\sqrt{y}z^2$ | 157.59 | 121.87 | 0.698 | 0.0839 | 0.0627 | 0.6523 | 0.3149 | 0.2452 | 0.580 |
| $a+bz^2+c\sqrt{y}\sqrt{z}$ | 125.92 | 100.02 | 0.807 | 0.0744 | 0.0468 | 0.7265 | 0.2621 | 0.1652 | 0.709 |
| $a+bz^2+c/yz$ | 124.23 | 91.27 | 0.812 | 0.0744 | 0.0508 | 0.7264 | 0.2564 | 0.1679 | 0.721 |
| $a+bz^2+c/yz^2$ | 127.42 | 91.68 | 0.802 | 0.0781 | 0.0545 | 0.6992 | 0.2742 | 0.1853 | 0.681 |
| $a+bz^2+c/y\sqrt{z}$ | 127.63 | 95.65 | 0.802 | 0.0733 | 0.0483 | 0.7348 | 0.2534 | 0.1611 | 0.728 |
| $a+bz^2+cz/y$ | 153.44 | 121.73 | 0.714 | 0.0804 | 0.0585 | 0.6805 | 0.2994 | 0.2199 | 0.620 |
| $a+bz^2+cz^2/y$ | 155.93 | 119.48 | 0.704 | 0.0832 | 0.0631 | 0.6584 | 0.3119 | 0.2410 | 0.588 |
| $a+bz^2+c\sqrt{z}/y$ | 145.94 | 116.87 | 0.741 | 0.0768 | 0.0517 | 0.7090 | 0.2798 | 0.1958 | 0.668 |
| $a+bz^2+c/y^2z$ | 131.39 | 97.12 | 0.790 | 0.0748 | 0.0514 | 0.7236 | 0.2613 | 0.1719 | 0.711 |
| $a+bz^2+c/y^2z^2$ | 129.00 | 93.01 | 0.798 | 0.0769 | 0.0544 | 0.7080 | 0.2689 | 0.1862 | 0.694 |
| $a+bz^2+c/y^2\sqrt{z}$ | 134.83 | 102.69 | 0.779 | 0.0743 | 0.0496 | 0.7277 | 0.2612 | 0.1689 | 0.711 |
| $a+bz^2+cz/y^2$ | 148.86 | 117.60 | 0.730 | 0.0766 | 0.0526 | 0.7103 | 0.2813 | 0.1985 | 0.665 |
| $a+bz^2+cz^2/y^2$ | 153.78 | 119.98 | 0.712 | 0.0797 | 0.0577 | 0.6867 | 0.2974 | 0.2155 | 0.625 |
| $a+bz^2+c\sqrt{z}/y^2$ | 144.48 | 113.55 | 0.746 | 0.0752 | 0.0502 | 0.7207 | 0.2723 | 0.1875 | 0.686 |
| $a+bz^2+c/\sqrt{y}z$ | 124.32 | 91.93 | 0.812 | 0.0760 | 0.0511 | 0.7145 | 0.2646 | 0.1698 | 0.703 |
| $a+bz^2+c/\sqrt{y}z^2$ | 134.24 | 101.00 | 0.781 | 0.0803 | 0.0570 | 0.6818 | 0.2882 | 0.2029 | 0.648 |
| $a+bz^2+c/\sqrt{y}\sqrt{z}$ | 122.81 | 93.09 | 0.816 | 0.0735 | 0.0480 | 0.7335 | 0.2524 | 0.1569 | 0.730 |
| $a+bz^2+cz/\sqrt{y}$ | 157.65 | 121.44 | 0.698 | 0.0841 | 0.0629 | 0.6508 | 0.3158 | 0.2442 | 0.577 |
| $a+bz^2+cz^2/\sqrt{y}$ | 156.90 | 121.24 | 0.700 | 0.0841 | 0.0630 | 0.6512 | 0.3155 | 0.2440 | 0.578 |
| $a+bz^2+c\sqrt{z}/\sqrt{y}$ | 153.82 | 122.67 | 0.712 | 0.0811 | 0.0591 | 0.6754 | 0.3017 | 0.2265 | 0.614 |
| $a+b\sqrt{z}+cx/y$ | 129.90 | 103.27 | 0.795 | 0.0721 | 0.0488 | 0.7431 | 0.2456 | 0.1697 | 0.744 |
| $a+b\sqrt{z}+cx/y^2$ | 134.40 | 106.81 | 0.780 | 0.0790 | 0.0525 | 0.6918 | 0.2833 | 0.1958 | 0.660 |
| $a+b\sqrt{z}+cx/\sqrt{y}$ | 121.04 | 94.21 | 0.822 | 0.0701 | 0.0461 | 0.7570 | 0.2305 | 0.1459 | 0.775 |
| $a+b\sqrt{z}+cxy$ | 116.33 | 90.30 | 0.835 | 0.0737 | 0.0458 | 0.7321 | 0.2544 | 0.1692 | 0.726 |
| $a+b\sqrt{z}+cxy^2$ | 121.63 | 91.79 | 0.820 | 0.0761 | 0.0482 | 0.7139 | 0.2702 | 0.1901 | 0.691 |
| $a+b\sqrt{z}+cx\sqrt{y}$ | 114.22 | 87.76 | 0.841 | 0.0718 | 0.0439 | 0.7453 | 0.2419 | 0.1493 | 0.752 |
| $a+b\sqrt{z}+cx^2/y$ | 116.93 | 91.58 | 0.834 | 0.0701 | 0.0480 | 0.7576 | 0.2298 | 0.1548 | 0.776 |
| $a+b\sqrt{z}+cx^2/y^2$ | 130.25 | 103.52 | 0.794 | 0.0739 | 0.0520 | 0.7304 | 0.2524 | 0.1826 | 0.730 |
| $a+b\sqrt{z}+cx^2/\sqrt{y}$ | 111.67 | 89.39 | 0.848 | 0.0697 | 0.0458 | 0.7600 | 0.2307 | 0.1543 | 0.774 |
| $a+b\sqrt{z}+cx^2y$ | 118.12 | 90.62 | 0.830 | 0.0746 | 0.0492 | 0.7249 | 0.2643 | 0.1886 | 0.704 |
| $a+b\sqrt{z}+cx^2y^2$ | 122.97 | 91.51 | 0.816 | 0.0765 | 0.0495 | 0.7113 | 0.2742 | 0.1968 | 0.681 |
| $a+b\sqrt{z}+cx^2\sqrt{y}$ | 114.55 | 89.71 | 0.840 | 0.0730 | 0.0480 | 0.7366 | 0.2548 | 0.1811 | 0.725 |
| $a+b\sqrt{z}+c\sqrt{x}/y$ | 134.94 | 107.12 | 0.778 | 0.0789 | 0.0532 | 0.6929 | 0.2835 | 0.1963 | 0.660 |
| $a+b\sqrt{z}+c\sqrt{x}/y^2$ | 125.14 | 92.86 | 0.809 | 0.0761 | 0.0479 | 0.7140 | 0.2578 | 0.1589 | 0.718 |
| $a+b\sqrt{z}+c\sqrt{x}/\sqrt{y}$ | 130.81 | 103.86 | 0.792 | 0.0718 | 0.0474 | 0.7458 | 0.2458 | 0.1677 | 0.744 |
| $a+b\sqrt{z}+c\sqrt{x}y$ | 118.77 | 90.53 | 0.828 | 0.0739 | 0.0444 | 0.7305 | 0.2530 | 0.1569 | 0.729 |
| $a+b\sqrt{z}+c\sqrt{x}y^2$ | 122.15 | 92.81 | 0.818 | 0.0762 | 0.0471 | 0.7134 | 0.2687 | 0.1846 | 0.694 |
| $a+b\sqrt{z}+c\sqrt{x}\sqrt{y}$ | 118.56 | 89.20 | 0.829 | 0.0723 | 0.0440 | 0.7416 | 0.2428 | 0.1395 | 0.750 |
| $a+b\sqrt{z}+c/xy$ | 134.58 | 105.95 | 0.780 | 0.0737 | 0.0448 | 0.7319 | 0.2592 | 0.1637 | 0.715 |
| $a+b\sqrt{z}+c/xy^2$ | 134.82 | 106.07 | 0.779 | 0.0738 | 0.0450 | 0.7312 | 0.2600 | 0.1645 | 0.714 |
| $a+b\sqrt{z}+c/x\sqrt{y}$ | 134.45 | 105.87 | 0.780 | 0.0736 | 0.0448 | 0.7325 | 0.2588 | 0.1633 | 0.716 |
| $a+b\sqrt{z}+cy/x$ | 134.87 | 105.92 | 0.779 | 0.0729 | 0.0465 | 0.7374 | 0.2576 | 0.1648 | 0.719 |
| $a+b\sqrt{z}+cy^2/x$ | 136.10 | 107.18 | 0.775 | 0.0782 | 0.0548 | 0.6980 | 0.2820 | 0.1965 | 0.663 |
| $a+b\sqrt{z}+c\sqrt{y}/x$ | 134.36 | 105.77 | 0.780 | 0.0732 | 0.0451 | 0.7351 | 0.2576 | 0.1627 | 0.719 |
| $a+b\sqrt{z}+c/x^2y$ | 136.30 | 106.08 | 0.774 | 0.0742 | 0.0460 | 0.7278 | 0.2651 | 0.1704 | 0.702 |
| $a+b\sqrt{z}+c/x^2y^2$ | 136.34 | 106.06 | 0.774 | 0.0743 | 0.0460 | 0.7276 | 0.2653 | 0.1706 | 0.702 |
| $a+b\sqrt{z}+c/x^2\sqrt{y}$ | 136.27 | 106.08 | 0.774 | 0.0742 | 0.0460 | 0.7279 | 0.2650 | 0.1703 | 0.703 |
| $a+b\sqrt{z}+cy/x^2$ | 136.18 | 106.09 | 0.774 | 0.0741 | 0.0460 | 0.7287 | 0.2644 | 0.1698 | 0.704 |
| $a+b\sqrt{z}+cy^2/x^2$ | 136.17 | 106.05 | 0.774 | 0.0739 | 0.0463 | 0.7305 | 0.2637 | 0.1692 | 0.705 |
| $a+b\sqrt{z}+c\sqrt{y}/x^2$ | 136.21 | 106.09 | 0.774 | 0.0742 | 0.0460 | 0.7284 | 0.2646 | 0.1700 | 0.703 |

(continued on next page)

**Table 4 – continued from previous page**

| Functional form | $T_{eff}$ (K) | | | Radius ($R_{\odot}$) | | | log (L/$L_{\odot}$) | | |
|---|---|---|---|---|---|---|---|---|---|
| | RMSE | MAD | $R^2_{ap}$ | RMSE | MAD | $R^2_{ap}$ | RMSE | MAD | $R^2_{ap}$ |
| $a+b\sqrt{z}+c/\sqrt{x}y$ | 132.16 | 104.23 | 0.787 | 0.0734 | 0.0441 | 0.7337 | 0.2541 | 0.1560 | 0.726 |
| $a+b\sqrt{z}+c/\sqrt{x}y^2$ | 132.75 | 104.78 | 0.786 | 0.0736 | 0.0445 | 0.7324 | 0.2555 | 0.1575 | 0.723 |
| $a+b\sqrt{z}+c/\sqrt{x}\sqrt{y}$ | 131.86 | 103.96 | 0.788 | 0.0732 | 0.0439 | 0.7352 | 0.2532 | 0.1552 | 0.728 |
| $a+b\sqrt{z}+cy/\sqrt{x}$ | 135.79 | 107.27 | 0.776 | 0.0785 | 0.0543 | 0.6961 | 0.2827 | 0.1961 | 0.661 |
| $a+b\sqrt{z}+cy^2/\sqrt{x}$ | 128.46 | 99.95 | 0.799 | 0.0779 | 0.0480 | 0.7004 | 0.2747 | 0.1844 | 0.680 |
| $a+b\sqrt{z}+c\sqrt{y}/\sqrt{x}$ | 133.70 | 105.58 | 0.783 | 0.0723 | 0.0467 | 0.7416 | 0.2532 | 0.1653 | 0.728 |
| $a+b\sqrt{z}+cx/z$ | 115.47 | 86.83 | 0.838 | 0.0683 | 0.0399 | 0.7695 | 0.2286 | 0.1340 | 0.778 |
| $a+b\sqrt{z}+cx/z^2$ | 125.74 | 96.29 | 0.808 | 0.0708 | 0.0444 | 0.7525 | 0.2536 | 0.1794 | 0.728 |
| $a+b\sqrt{z}+cx/\sqrt{z}$ | 114.05 | 83.64 | 0.842 | 0.0694 | 0.0432 | 0.7619 | 0.2256 | 0.1290 | 0.784 |
| $a+b\sqrt{z}+cxz$ | 126.94 | 96.44 | 0.804 | 0.0732 | 0.0517 | 0.7354 | 0.2695 | 0.2032 | 0.692 |
| $a+b\sqrt{z}+cxz^2$ | 134.97 | 103.97 | 0.778 | 0.0777 | 0.0530 | 0.7020 | 0.2829 | 0.2002 | 0.661 |
| $a+b\sqrt{z}+cx\sqrt{z}$ | 116.45 | 89.68 | 0.835 | 0.0695 | 0.0441 | 0.7613 | 0.2414 | 0.1619 | 0.753 |
| $a+b\sqrt{z}+cx^2/z$ | 106.82 | 78.16 | 0.861 | 0.0686 | 0.0427 | 0.7674 | 0.2208 | 0.1235 | 0.793 |
| $a+b\sqrt{z}+cx^2/z^2$ | 118.48 | 91.14 | 0.829 | 0.0694 | 0.0418 | 0.7622 | 0.2405 | 0.1638 | 0.755 |
| $a+b\sqrt{z}+cx^2/\sqrt{z}$ | 108.20 | 82.79 | 0.858 | 0.0702 | 0.0442 | 0.7568 | 0.2285 | 0.1378 | 0.779 |
| $a+b\sqrt{z}+cx^2z$ | 127.86 | 94.78 | 0.801 | 0.0756 | 0.0528 | 0.7178 | 0.2765 | 0.2039 | 0.676 |
| $a+b\sqrt{z}+cx^2z^2$ | 133.40 | 102.02 | 0.783 | 0.0778 | 0.0529 | 0.7012 | 0.2827 | 0.1994 | 0.661 |
| $a+b\sqrt{z}+cx^2\sqrt{z}$ | 119.20 | 89.93 | 0.827 | 0.0729 | 0.0501 | 0.7374 | 0.2620 | 0.1951 | 0.709 |
| $a+b\sqrt{z}+c\sqrt{x}/z$ | 123.52 | 95.28 | 0.814 | 0.0690 | 0.0415 | 0.7649 | 0.2432 | 0.1607 | 0.749 |
| $a+b\sqrt{z}+c\sqrt{x}/z^2$ | 130.73 | 99.84 | 0.792 | 0.0722 | 0.0467 | 0.7426 | 0.2640 | 0.1908 | 0.705 |
| $a+b\sqrt{z}+c\sqrt{x}/\sqrt{z}$ | 120.00 | 90.94 | 0.825 | 0.0692 | 0.0416 | 0.7636 | 0.2319 | 0.1326 | 0.772 |
| $a+b\sqrt{z}+c\sqrt{x}z$ | 129.11 | 99.90 | 0.797 | 0.0722 | 0.0502 | 0.7424 | 0.2672 | 0.1990 | 0.698 |
| $a+b\sqrt{z}+c\sqrt{x}z^2$ | 136.06 | 105.43 | 0.775 | 0.0778 | 0.0533 | 0.7011 | 0.2832 | 0.1995 | 0.660 |
| $a+b\sqrt{z}+c\sqrt{x}\sqrt{z}$ | 121.43 | 93.83 | 0.821 | 0.0696 | 0.0419 | 0.7607 | 0.2387 | 0.1488 | 0.759 |
| $a+b\sqrt{z}+c/xz$ | 132.66 | 104.47 | 0.786 | 0.0740 | 0.0449 | 0.7295 | 0.2554 | 0.1562 | 0.724 |
| $a+b\sqrt{z}+c/xz^2$ | 131.23 | 101.98 | 0.790 | 0.0759 | 0.0480 | 0.7159 | 0.2585 | 0.1527 | 0.717 |
| $a+b\sqrt{z}+c/x\sqrt{z}$ | 133.58 | 105.27 | 0.783 | 0.0736 | 0.0443 | 0.7325 | 0.2565 | 0.1597 | 0.721 |
| $a+b\sqrt{z}+cz/x$ | 135.25 | 106.02 | 0.777 | 0.0737 | 0.0454 | 0.7321 | 0.2613 | 0.1658 | 0.711 |
| $a+b\sqrt{z}+cz^2/x$ | 135.60 | 105.82 | 0.776 | 0.0747 | 0.0458 | 0.7244 | 0.2632 | 0.1621 | 0.707 |
| $a+b\sqrt{z}+c\sqrt{z}/x$ | 134.90 | 106.00 | 0.779 | 0.0735 | 0.0452 | 0.7332 | 0.2599 | 0.1651 | 0.714 |
| $a+b\sqrt{z}+c/x^2z$ | 135.70 | 106.20 | 0.776 | 0.0740 | 0.0456 | 0.7295 | 0.2627 | 0.1678 | 0.708 |
| $a+b\sqrt{z}+c/x^2z^2$ | 134.69 | 105.97 | 0.779 | 0.0739 | 0.0449 | 0.7303 | 0.2598 | 0.1635 | 0.714 |
| $a+b\sqrt{z}+c/x^2\sqrt{z}$ | 136.02 | 106.16 | 0.775 | 0.0741 | 0.0458 | 0.7288 | 0.2639 | 0.1691 | 0.705 |
| $a+b\sqrt{z}+cz/x^2$ | 136.51 | 105.93 | 0.773 | 0.0744 | 0.0461 | 0.7270 | 0.2661 | 0.1713 | 0.700 |
| $a+b\sqrt{z}+cz^2/x^2$ | 136.64 | 105.82 | 0.773 | 0.0745 | 0.0462 | 0.7263 | 0.2669 | 0.1716 | 0.698 |
| $a+b\sqrt{z}+c\sqrt{z}/x^2$ | 136.40 | 106.01 | 0.774 | 0.0743 | 0.0461 | 0.7275 | 0.2656 | 0.1709 | 0.701 |
| $a+b\sqrt{z}+c/\sqrt{x}z$ | 131.10 | 101.67 | 0.791 | 0.0760 | 0.0475 | 0.7147 | 0.2576 | 0.1507 | 0.719 |
| $a+b\sqrt{z}+c/\sqrt{x}z^2$ | 134.23 | 101.83 | 0.781 | 0.0789 | 0.0507 | 0.6923 | 0.2753 | 0.1741 | 0.679 |
| $a+b\sqrt{z}+c/\sqrt{x}\sqrt{z}$ | 131.06 | 102.99 | 0.791 | 0.0740 | 0.0451 | 0.7294 | 0.2523 | 0.1506 | 0.730 |
| $a+b\sqrt{z}+cz/\sqrt{x}$ | 133.22 | 104.87 | 0.784 | 0.0733 | 0.0444 | 0.7344 | 0.2561 | 0.1572 | 0.722 |
| $a+b\sqrt{z}+cz^2/\sqrt{x}$ | 136.49 | 105.89 | 0.773 | 0.0786 | 0.0500 | 0.6951 | 0.2744 | 0.1742 | 0.681 |
| $a+b\sqrt{z}+c\sqrt{z}/\sqrt{x}$ | 132.65 | 104.61 | 0.786 | 0.0726 | 0.0442 | 0.7398 | 0.2540 | 0.1579 | 0.727 |
| $a+b\sqrt{z}+cy/z$ | 122.07 | 94.24 | 0.819 | 0.0718 | 0.0433 | 0.7452 | 0.2496 | 0.1636 | 0.736 |
| $a+b\sqrt{z}+cy/z^2$ | 129.15 | 98.80 | 0.797 | 0.0724 | 0.0464 | 0.7410 | 0.2626 | 0.1896 | 0.708 |
| $a+b\sqrt{z}+cy/\sqrt{z}$ | 121.56 | 93.44 | 0.820 | 0.0738 | 0.0447 | 0.7311 | 0.2515 | 0.1512 | 0.732 |
| $a+b\sqrt{z}+cyz$ | 131.61 | 102.70 | 0.789 | 0.0768 | 0.0514 | 0.7087 | 0.2796 | 0.2012 | 0.669 |
| $a+b\sqrt{z}+cyz^2$ | 135.62 | 105.05 | 0.776 | 0.0783 | 0.0529 | 0.6976 | 0.2834 | 0.1976 | 0.660 |
| $a+b\sqrt{z}+cy\sqrt{z}$ | 125.90 | 99.75 | 0.807 | 0.0756 | 0.0464 | 0.7174 | 0.2687 | 0.1859 | 0.694 |
| $a+b\sqrt{z}+cy^2/z$ | 119.90 | 91.31 | 0.825 | 0.0741 | 0.0451 | 0.7290 | 0.2532 | 0.1570 | 0.728 |
| $a+b\sqrt{z}+cy^2/z^2$ | 123.91 | 95.48 | 0.813 | 0.0720 | 0.0449 | 0.7439 | 0.2545 | 0.1763 | 0.726 |
| $a+b\sqrt{z}+cy^2/\sqrt{z}$ | 122.06 | 93.15 | 0.819 | 0.0758 | 0.0459 | 0.7163 | 0.2611 | 0.1640 | 0.711 |
| $a+b\sqrt{z}+cy^2z$ | 131.47 | 102.78 | 0.790 | 0.0777 | 0.0514 | 0.7016 | 0.2816 | 0.1995 | 0.664 |
| $a+b\sqrt{z}+cy^2z^2$ | 134.37 | 104.26 | 0.780 | 0.0784 | 0.0525 | 0.6968 | 0.2833 | 0.1976 | 0.660 |
| $a+b\sqrt{z}+cy^2\sqrt{z}$ | 127.64 | 99.25 | 0.802 | 0.0771 | 0.0489 | 0.7062 | 0.2769 | 0.1959 | 0.675 |
| $a+b\sqrt{z}+c\sqrt{y}/z$ | 127.73 | 99.31 | 0.802 | 0.0718 | 0.0453 | 0.7457 | 0.2590 | 0.1858 | 0.716 |
| $a+b\sqrt{z}+c\sqrt{y}/z^2$ | 132.98 | 103.02 | 0.785 | 0.0736 | 0.0491 | 0.7325 | 0.2706 | 0.1989 | 0.690 |
| $a+b\sqrt{z}+c\sqrt{y}/\sqrt{z}$ | 122.67 | 95.66 | 0.817 | 0.0722 | 0.0429 | 0.7429 | 0.2491 | 0.1567 | 0.737 |
| $a+b\sqrt{z}+c\sqrt{y}z$ | 132.71 | 103.31 | 0.786 | 0.0762 | 0.0517 | 0.7131 | 0.2790 | 0.2034 | 0.670 |
| $a+b\sqrt{z}+c\sqrt{y}z^2$ | 136.41 | 105.70 | 0.774 | 0.0783 | 0.0532 | 0.6976 | 0.2834 | 0.1971 | 0.660 |
| $a+b\sqrt{z}+c\sqrt{y}\sqrt{z}$ | 125.50 | 99.67 | 0.808 | 0.0747 | 0.0446 | 0.7246 | 0.2627 | 0.1739 | 0.708 |
| $a+b\sqrt{z}+c/yz$ | 128.77 | 97.04 | 0.798 | 0.0774 | 0.0492 | 0.7044 | 0.2622 | 0.1611 | 0.709 |
| $a+b\sqrt{z}+c/yz^2$ | 132.95 | 101.20 | 0.785 | 0.0791 | 0.0509 | 0.6914 | 0.2764 | 0.1765 | 0.676 |
| $a+b\sqrt{z}+c/y\sqrt{z}$ | 127.43 | 97.46 | 0.802 | 0.0757 | 0.0477 | 0.7174 | 0.2545 | 0.1523 | 0.726 |
| $a+b\sqrt{z}+cz/y$ | 129.40 | 100.47 | 0.796 | 0.0740 | 0.0433 | 0.7295 | 0.2567 | 0.1543 | 0.721 |
| $a+b\sqrt{z}+cz^2/y$ | 134.52 | 100.51 | 0.780 | 0.0786 | 0.0495 | 0.6948 | 0.2749 | 0.1715 | 0.680 |
| $a+b\sqrt{z}+c\sqrt{z}/y$ | 128.32 | 99.30 | 0.800 | 0.0733 | 0.0436 | 0.7345 | 0.2521 | 0.1497 | 0.731 |
| $a+b\sqrt{z}+c/y^2z$ | 127.61 | 97.32 | 0.802 | 0.0760 | 0.0490 | 0.7151 | 0.2566 | 0.1591 | 0.721 |
| $a+b\sqrt{z}+c/y^2z^2$ | 128.41 | 95.33 | 0.799 | 0.0777 | 0.0501 | 0.7015 | 0.2656 | 0.1683 | 0.701 |
| $a+b\sqrt{z}+c/y^2\sqrt{z}$ | 128.08 | 99.06 | 0.800 | 0.0749 | 0.0477 | 0.7229 | 0.2533 | 0.1527 | 0.728 |
| $a+b\sqrt{z}+cz/y^2$ | 131.49 | 103.05 | 0.790 | 0.0734 | 0.0435 | 0.7341 | 0.2549 | 0.1550 | 0.725 |
| $a+b\sqrt{z}+cz^2/y^2$ | 132.79 | 102.72 | 0.785 | 0.0747 | 0.0444 | 0.7247 | 0.2615 | 0.1577 | 0.710 |
| $a+b\sqrt{z}+c\sqrt{z}/y^2$ | 130.35 | 102.18 | 0.793 | 0.0735 | 0.0446 | 0.7333 | 0.2526 | 0.1510 | 0.730 |
| $a+b\sqrt{z}+c/\sqrt{y}z$ | 132.57 | 99.90 | 0.786 | 0.0789 | 0.0502 | 0.6930 | 0.2730 | 0.1705 | 0.684 |
| $a+b\sqrt{z}+c/\sqrt{y}z^2$ | 136.71 | 106.34 | 0.773 | 0.0786 | 0.0525 | 0.6952 | 0.2830 | 0.1916 | 0.661 |
| $a+b\sqrt{z}+c/\sqrt{y}\sqrt{z}$ | 128.60 | 97.28 | 0.799 | 0.0770 | 0.0481 | 0.7071 | 0.2601 | 0.1545 | 0.713 |
| $a+b\sqrt{z}+cz/\sqrt{y}$ | 129.31 | 98.45 | 0.797 | 0.0760 | 0.0453 | 0.7148 | 0.2620 | 0.1552 | 0.709 |
| $a+b\sqrt{z}+cz^2/\sqrt{y}$ | 137.15 | 106.92 | 0.771 | 0.0790 | 0.0523 | 0.6918 | 0.2820 | 0.1869 | 0.663 |
| $a+b\sqrt{z}+c\sqrt{z}/\sqrt{y}$ | 127.03 | 99.15 | 0.804 | 0.0734 | 0.0431 | 0.7337 | 0.2535 | 0.1529 | 0.728 |
| $a+b/z+cx/y$ | 170.89 | 124.22 | 0.645 | 0.0943 | 0.0707 | 0.5606 | 0.2998 | 0.2117 | 0.619 |
| $a+b/z+cx/y^2$ | 179.52 | 124.53 | 0.608 | 0.1048 | 0.0742 | 0.4573 | 0.3479 | 0.2277 | 0.487 |
| $a+b/z+cx/\sqrt{y}$ | 150.49 | 110.73 | 0.724 | 0.0855 | 0.0659 | 0.6393 | 0.2629 | 0.1851 | 0.707 |
| $a+b/z+cxy$ | 126.40 | 99.16 | 0.806 | 0.0817 | 0.0561 | 0.6707 | 0.2671 | 0.1792 | 0.698 |
| $a+b/z+cxy^2$ | 131.17 | 99.95 | 0.791 | 0.0856 | 0.0606 | 0.6386 | 0.2878 | 0.1997 | 0.649 |
| $a+b/z+cx\sqrt{y}$ | 126.64 | 95.93 | 0.805 | 0.0799 | 0.0549 | 0.6846 | 0.2544 | 0.1616 | 0.726 |
| $a+b/z+cx^2/y$ | 137.71 | 108.27 | 0.769 | 0.0811 | 0.0618 | 0.6752 | 0.2497 | 0.1733 | 0.736 |
| $a+b/z+cx^2/y^2$ | 172.49 | 124.34 | 0.638 | 0.0968 | 0.0745 | 0.5373 | 0.3092 | 0.2284 | 0.595 |
| $a+b/z+cx^2/\sqrt{y}$ | 122.55 | 99.84 | 0.817 | 0.0764 | 0.0536 | 0.7118 | 0.2397 | 0.1640 | 0.757 |
| $a+b/z+cx^2y$ | 123.97 | 97.46 | 0.813 | 0.0817 | 0.0594 | 0.6704 | 0.2756 | 0.1971 | 0.678 |
| $a+b/z+cx^2y^2$ | 130.62 | 100.63 | 0.792 | 0.0857 | 0.0632 | 0.6372 | 0.2924 | 0.2041 | 0.638 |
| $a+b/z+cx^2\sqrt{y}$ | 120.04 | 95.35 | 0.825 | 0.0790 | 0.0562 | 0.6916 | 0.2630 | 0.1879 | 0.707 |
| $a+b/z+c\sqrt{x}/y$ | 179.64 | 124.73 | 0.607 | 0.1049 | 0.0743 | 0.4569 | 0.3484 | 0.2293 | 0.486 |
| $a+b/z+c\sqrt{x}/y^2$ | 169.11 | 113.62 | 0.652 | 0.0995 | 0.0748 | 0.5113 | 0.3168 | 0.2123 | 0.575 |
| $a+b/z+c\sqrt{x}/\sqrt{y}$ | 171.61 | 123.88 | 0.642 | 0.0939 | 0.0690 | 0.5649 | 0.2995 | 0.2095 | 0.620 |
| $a+b/z+c\sqrt{x}y$ | 134.94 | 103.63 | 0.778 | 0.0844 | 0.0587 | 0.6483 | 0.2719 | 0.1732 | 0.687 |

(continued on next page)

**Table 4 – continued from previous page**

| Functional form | $T_{eff}$ (K) | | | Radius ($R_{\odot}$) | | | log (L/$L_{\odot}$) | | |
|---|---|---|---|---|---|---|---|---|---|
| | RMSE | MAD | $R^2_{ap}$ | RMSE | MAD | $R^2_{ap}$ | RMSE | MAD | $R^2_{ap}$ |
| $a+b/z+c\sqrt{x}y^2$ | 134.85 | 103.99 | 0.779 | 0.0867 | 0.0592 | 0.6285 | 0.2888 | 0.1957 | 0.647 |
| $a+b/z+c\sqrt{x}\sqrt{y}$ | 139.37 | 100.19 | 0.764 | 0.0842 | 0.0606 | 0.6503 | 0.2649 | 0.1710 | 0.703 |
| $a+b/z+c/xy$ | 177.69 | 120.86 | 0.616 | 0.0973 | 0.0676 | 0.5324 | 0.3174 | 0.2015 | 0.573 |
| $a+b/z+c/xy^2$ | 178.19 | 120.80 | 0.614 | 0.0976 | 0.0676 | 0.5295 | 0.3187 | 0.2022 | 0.570 |
| $a+b/z+c/x\sqrt{y}$ | 177.30 | 120.92 | 0.618 | 0.0970 | 0.0676 | 0.5350 | 0.3162 | 0.2010 | 0.576 |
| $a+b/z+cy/x$ | 176.89 | 122.44 | 0.619 | 0.0957 | 0.0670 | 0.5474 | 0.3126 | 0.2036 | 0.586 |
| $a+b/z+cy^2/x$ | 179.78 | 124.78 | 0.607 | 0.1049 | 0.0745 | 0.4563 | 0.3490 | 0.2326 | 0.484 |
| $a+b/z+c\sqrt{y}/x$ | 176.38 | 121.49 | 0.622 | 0.0961 | 0.0671 | 0.5443 | 0.3130 | 0.2006 | 0.585 |
| $a+b/z+c/x^2y$ | 179.70 | 120.63 | 0.607 | 0.0978 | 0.0676 | 0.5273 | 0.3225 | 0.2048 | 0.559 |
| $a+b/z+c/x^2y^2$ | 179.78 | 120.59 | 0.607 | 0.0979 | 0.0676 | 0.5269 | 0.3228 | 0.2049 | 0.559 |
| $a+b/z+c/x^2\sqrt{y}$ | 179.64 | 120.66 | 0.607 | 0.0978 | 0.0676 | 0.5277 | 0.3224 | 0.2047 | 0.560 |
| $a+b/z+cy/x^2$ | 179.33 | 120.84 | 0.609 | 0.0975 | 0.0676 | 0.5303 | 0.3213 | 0.2045 | 0.563 |
| $a+b/z+cy^2/x^2$ | 179.08 | 121.22 | 0.610 | 0.0971 | 0.0676 | 0.5345 | 0.3199 | 0.2046 | 0.566 |
| $a+b/z+c\sqrt{y}/x^2$ | 179.47 | 120.75 | 0.608 | 0.0977 | 0.0676 | 0.5290 | 0.3218 | 0.2045 | 0.561 |
| $a+b/z+c/\sqrt{x}y$ | 174.93 | 119.69 | 0.628 | 0.0968 | 0.0687 | 0.5376 | 0.3120 | 0.1952 | 0.588 |
| $a+b/z+c/\sqrt{x}y^2$ | 176.37 | 119.98 | 0.622 | 0.0976 | 0.0694 | 0.5298 | 0.3155 | 0.1973 | 0.578 |
| $a+b/z+c/\sqrt{x}\sqrt{y}$ | 173.79 | 119.60 | 0.633 | 0.0960 | 0.0684 | 0.5449 | 0.3091 | 0.1943 | 0.595 |
| $a+b/z+cy/\sqrt{x}$ | 179.78 | 124.85 | 0.607 | 0.1049 | 0.0744 | 0.4564 | 0.3489 | 0.2318 | 0.484 |
| $a+b/z+cy^2/\sqrt{x}$ | 156.08 | 113.52 | 0.704 | 0.0955 | 0.0674 | 0.5496 | 0.3142 | 0.2063 | 0.582 |
| $a+b/z+c\sqrt{y}/\sqrt{x}$ | 175.16 | 123.12 | 0.627 | 0.0949 | 0.0671 | 0.5557 | 0.3075 | 0.2051 | 0.599 |
| $a+b/z+cx/z$ | 162.85 | 115.59 | 0.677 | 0.0968 | 0.0747 | 0.5373 | 0.2969 | 0.2084 | 0.627 |
| $a+b/z+cx/z^2$ | 140.08 | 94.90 | 0.761 | 0.0864 | 0.0620 | 0.6313 | 0.2605 | 0.1664 | 0.713 |
| $a+b/z+cx/\sqrt{z}$ | 160.37 | 114.64 | 0.687 | 0.0950 | 0.0729 | 0.5547 | 0.2911 | 0.1990 | 0.641 |
| $a+b/z+cxz$ | 122.86 | 92.37 | 0.816 | 0.0731 | 0.0517 | 0.7358 | 0.2664 | 0.1954 | 0.699 |
| $a+b/z+cxz^2$ | 133.27 | 100.11 | 0.784 | 0.0802 | 0.0586 | 0.6821 | 0.2907 | 0.2085 | 0.642 |
| $a+b/z+cx\sqrt{z}$ | 115.70 | 90.80 | 0.837 | 0.0695 | 0.0449 | 0.7618 | 0.2417 | 0.1604 | 0.753 |
| $a+b/z+cx^2/z$ | 152.63 | 109.54 | 0.717 | 0.0942 | 0.0733 | 0.5620 | 0.2842 | 0.2014 | 0.658 |
| $a+b/z+cx^2/z^2$ | 141.49 | 96.13 | 0.756 | 0.0892 | 0.0667 | 0.6071 | 0.2650 | 0.1791 | 0.702 |
| $a+b/z+cx^2/\sqrt{z}$ | 139.29 | 102.06 | 0.764 | 0.0878 | 0.0654 | 0.6195 | 0.2667 | 0.1853 | 0.699 |
| $a+b/z+cx^2z$ | 124.03 | 92.56 | 0.813 | 0.0773 | 0.0567 | 0.7049 | 0.2778 | 0.2069 | 0.673 |
| $a+b/z+cx^2z^2$ | 132.45 | 98.89 | 0.787 | 0.0823 | 0.0612 | 0.6656 | 0.2948 | 0.2136 | 0.632 |
| $a+b/z+cx^2\sqrt{z}$ | 117.03 | 91.72 | 0.833 | 0.0744 | 0.0538 | 0.7266 | 0.2616 | 0.1910 | 0.710 |
| $a+b/z+c\sqrt{x}/z$ | 167.34 | 117.46 | 0.659 | 0.0976 | 0.0743 | 0.5299 | 0.3030 | 0.2080 | 0.611 |
| $a+b/z+c\sqrt{x}/z^2$ | 134.13 | 92.15 | 0.781 | 0.0813 | 0.0553 | 0.6737 | 0.2488 | 0.1489 | 0.738 |
| $a+b/z+c\sqrt{x}/\sqrt{z}$ | 171.79 | 117.81 | 0.641 | 0.0991 | 0.0750 | 0.5147 | 0.3109 | 0.2108 | 0.590 |
| $a+b/z+c\sqrt{x}z$ | 126.26 | 97.44 | 0.806 | 0.0724 | 0.0494 | 0.7410 | 0.2656 | 0.1906 | 0.701 |
| $a+b/z+c\sqrt{x}z^2$ | 135.24 | 102.63 | 0.777 | 0.0798 | 0.0572 | 0.6857 | 0.2903 | 0.2068 | 0.643 |
| $a+b/z+c\sqrt{x}\sqrt{z}$ | 121.64 | 92.45 | 0.820 | 0.0689 | 0.0417 | 0.7659 | 0.2398 | 0.1528 | 0.756 |
| $a+b/z+c/xz$ | 176.35 | 120.34 | 0.622 | 0.0976 | 0.0694 | 0.5299 | 0.3149 | 0.1978 | 0.580 |
| $a+b/z+c/xz^2$ | 178.59 | 119.06 | 0.612 | 0.1010 | 0.0742 | 0.4968 | 0.3250 | 0.2125 | 0.552 |
| $a+b/z+c/x\sqrt{z}$ | 176.27 | 120.78 | 0.622 | 0.0968 | 0.0680 | 0.5378 | 0.3137 | 0.1990 | 0.583 |
| $a+b/z+cz/x$ | 180.13 | 120.87 | 0.605 | 0.0990 | 0.0691 | 0.5156 | 0.3244 | 0.2048 | 0.554 |
| $a+b/z+cz^2/x$ | 183.01 | 123.74 | 0.593 | 0.1049 | 0.0747 | 0.4572 | 0.3468 | 0.2299 | 0.490 |
| $a+b/z+c\sqrt{z}/x$ | 178.03 | 121.25 | 0.614 | 0.0973 | 0.0674 | 0.5326 | 0.3181 | 0.2026 | 0.571 |
| $a+b/z+c/x^2z$ | 179.07 | 120.83 | 0.610 | 0.0977 | 0.0673 | 0.5285 | 0.3207 | 0.2040 | 0.564 |
| $a+b/z+c/x^2z^2$ | 178.42 | 120.75 | 0.613 | 0.0979 | 0.0682 | 0.5264 | 0.3195 | 0.2024 | 0.568 |
| $a+b/z+c/x^2\sqrt{z}$ | 179.34 | 120.77 | 0.609 | 0.0977 | 0.0675 | 0.5285 | 0.3214 | 0.2044 | 0.562 |
| $a+b/z+cz/x^2$ | 179.97 | 120.52 | 0.606 | 0.0979 | 0.0678 | 0.5266 | 0.3234 | 0.2050 | 0.557 |
| $a+b/z+cz^2/x^2$ | 180.49 | 120.30 | 0.604 | 0.0984 | 0.0682 | 0.5223 | 0.3251 | 0.2054 | 0.552 |
| $a+b/z+c\sqrt{z}/x^2$ | 179.77 | 120.61 | 0.607 | 0.0978 | 0.0677 | 0.5276 | 0.3228 | 0.2048 | 0.559 |
| $a+b/z+c/\sqrt{x}z$ | 174.02 | 118.71 | 0.632 | 0.0977 | 0.0714 | 0.5284 | 0.3114 | 0.1993 | 0.589 |
| $a+b/z+c/\sqrt{x}z^2$ | 183.46 | 124.90 | 0.591 | 0.1049 | 0.0745 | 0.4570 | 0.3445 | 0.2280 | 0.497 |
| $a+b/z+c/\sqrt{x}\sqrt{z}$ | 171.20 | 118.71 | 0.643 | 0.0947 | 0.0683 | 0.5571 | 0.3027 | 0.1922 | 0.612 |
| $a+b/z+cz/\sqrt{x}$ | 183.14 | 123.95 | 0.592 | 0.1049 | 0.0746 | 0.4563 | 0.3471 | 0.2304 | 0.489 |
| $a+b/z+cz^2/\sqrt{x}$ | 153.39 | 115.96 | 0.714 | 0.0899 | 0.0615 | 0.6007 | 0.3190 | 0.2141 | 0.569 |
| $a+b/z+c\sqrt{z}/\sqrt{x}$ | 179.28 | 121.31 | 0.609 | 0.0996 | 0.0709 | 0.5102 | 0.3229 | 0.2048 | 0.558 |
| $a+b/z+cy/z$ | 172.00 | 114.18 | 0.640 | 0.1013 | 0.0763 | 0.4929 | 0.3222 | 0.2194 | 0.560 |
| $a+b/z+cy/z^2$ | 142.60 | 96.81 | 0.753 | 0.0876 | 0.0621 | 0.6208 | 0.2701 | 0.1687 | 0.691 |
| $a+b/z+cy/\sqrt{z}$ | 171.74 | 113.58 | 0.641 | 0.1011 | 0.0760 | 0.4954 | 0.3231 | 0.2161 | 0.558 |
| $a+b/z+cyz$ | 129.56 | 99.69 | 0.796 | 0.0782 | 0.0538 | 0.6981 | 0.2818 | 0.2014 | 0.664 |
| $a+b/z+cyz^2$ | 135.83 | 104.39 | 0.776 | 0.0821 | 0.0588 | 0.6673 | 0.2959 | 0.2086 | 0.629 |
| $a+b/z+cy\sqrt{z}$ | 127.69 | 97.29 | 0.802 | 0.0782 | 0.0494 | 0.6981 | 0.2719 | 0.1773 | 0.687 |
| $a+b/z+cy^2/z$ | 170.16 | 114.12 | 0.648 | 0.1015 | 0.0762 | 0.4918 | 0.3241 | 0.2182 | 0.555 |
| $a+b/z+cy^2/z^2$ | 153.59 | 103.68 | 0.713 | 0.0943 | 0.0705 | 0.5606 | 0.2923 | 0.1949 | 0.638 |
| $a+b/z+cy^2/\sqrt{z}$ | 163.00 | 115.90 | 0.677 | 0.0987 | 0.0738 | 0.5191 | 0.3167 | 0.2129 | 0.575 |
| $a+b/z+cy^2z$ | 131.67 | 99.36 | 0.789 | 0.0824 | 0.0568 | 0.6649 | 0.2924 | 0.2041 | 0.638 |
| $a+b/z+cy^2z^2$ | 135.57 | 101.95 | 0.776 | 0.0844 | 0.0604 | 0.6487 | 0.3006 | 0.2092 | 0.617 |
| $a+b/z+cy^2\sqrt{z}$ | 131.51 | 98.31 | 0.790 | 0.0832 | 0.0561 | 0.6581 | 0.2885 | 0.1892 | 0.647 |
| $a+b/z+c\sqrt{y}/z$ | 172.80 | 115.33 | 0.637 | 0.1013 | 0.0761 | 0.4937 | 0.3218 | 0.2190 | 0.561 |
| $a+b/z+c\sqrt{y}/z^2$ | 131.23 | 92.57 | 0.790 | 0.0801 | 0.0522 | 0.6834 | 0.2503 | 0.1502 | 0.735 |
| $a+b/z+c\sqrt{y}/\sqrt{z}$ | 178.36 | 119.41 | 0.613 | 0.1034 | 0.0761 | 0.4720 | 0.3335 | 0.2219 | 0.529 |
| $a+b/z+c\sqrt{y}z$ | 130.45 | 101.40 | 0.793 | 0.0764 | 0.0527 | 0.7118 | 0.2784 | 0.1989 | 0.672 |
| $a+b/z+c\sqrt{y}z^2$ | 136.91 | 105.44 | 0.772 | 0.0812 | 0.0576 | 0.6748 | 0.2942 | 0.2088 | 0.633 |
| $a+b/z+c\sqrt{y}\sqrt{z}$ | 125.70 | 98.56 | 0.808 | 0.0745 | 0.0454 | 0.7262 | 0.2627 | 0.1746 | 0.708 |
| $a+b/z+c/yz$ | 174.62 | 117.24 | 0.629 | 0.1011 | 0.0757 | 0.4952 | 0.3223 | 0.2187 | 0.560 |
| $a+b/z+c/yz^2$ | 183.36 | 124.87 | 0.591 | 0.1049 | 0.0746 | 0.4566 | 0.3470 | 0.2289 | 0.490 |
| $a+b/z+c/y\sqrt{z}$ | 169.68 | 115.35 | 0.650 | 0.0976 | 0.0728 | 0.5294 | 0.3090 | 0.2039 | 0.596 |
| $a+b/z+cz/y$ | 183.61 | 124.66 | 0.590 | 0.1048 | 0.0748 | 0.4575 | 0.3452 | 0.2275 | 0.495 |
| $a+b/z+cz^2/y$ | 158.28 | 123.71 | 0.695 | 0.0900 | 0.0647 | 0.5997 | 0.3194 | 0.2208 | 0.568 |
| $a+b/z+c\sqrt{z}/y$ | 174.85 | 118.27 | 0.628 | 0.0993 | 0.0732 | 0.5131 | 0.3190 | 0.2041 | 0.569 |
| $a+b/z+c/y^2z$ | 175.36 | 117.71 | 0.626 | 0.1011 | 0.0754 | 0.4957 | 0.3231 | 0.2180 | 0.558 |
| $a+b/z+c/y^2z^2$ | 179.31 | 120.90 | 0.609 | 0.1039 | 0.0759 | 0.4670 | 0.3368 | 0.2271 | 0.519 |
| $a+b/z+c/y^2\sqrt{z}$ | 173.83 | 116.50 | 0.632 | 0.0993 | 0.0738 | 0.5132 | 0.3165 | 0.2099 | 0.575 |
| $a+b/z+cz/y^2$ | 176.37 | 119.43 | 0.622 | 0.0985 | 0.0710 | 0.5208 | 0.3184 | 0.1987 | 0.571 |
| $a+b/z+cz^2/y^2$ | 183.71 | 124.77 | 0.589 | 0.1047 | 0.0748 | 0.4590 | 0.3451 | 0.2273 | 0.496 |
| $a+b/z+c\sqrt{z}/y^2$ | 173.96 | 117.62 | 0.632 | 0.0974 | 0.0707 | 0.5312 | 0.3128 | 0.1974 | 0.586 |
| $a+b/z+c/\sqrt{y}z$ | 174.11 | 116.66 | 0.631 | 0.1012 | 0.0759 | 0.4948 | 0.3220 | 0.2189 | 0.561 |
| $a+b/z+c/\sqrt{y}z^2$ | 178.65 | 122.82 | 0.612 | 0.0996 | 0.0686 | 0.5104 | 0.3429 | 0.2287 | 0.502 |
| $a+b/z+c/\sqrt{y}\sqrt{z}$ | 162.56 | 112.02 | 0.678 | 0.0942 | 0.0698 | 0.5616 | 0.2961 | 0.1904 | 0.628 |
| $a+b/z+cz/\sqrt{y}$ | 166.69 | 127.90 | 0.662 | 0.0943 | 0.0672 | 0.5610 | 0.3307 | 0.2234 | 0.537 |
| $a+b/z+cz^2/\sqrt{y}$ | 145.61 | 112.18 | 0.742 | 0.0830 | 0.0597 | 0.6595 | 0.3009 | 0.2123 | 0.616 |
| $a+b/z+c\sqrt{z}/\sqrt{y}$ | 183.18 | 124.23 | 0.592 | 0.1047 | 0.0748 | 0.4583 | 0.3438 | 0.2264 | 0.499 |
| $a+b/z^2+cx/y$ | 204.45 | 155.49 | 0.491 | 0.1075 | 0.0810 | 0.4294 | 0.3428 | 0.2531 | 0.502 |

(continued on next page)

**Table 4 – continued from previous page**

| Functional form | $T_{eff}$ (K) | | | Radius ($R_\odot$) | | | log (L/$L_\odot$) | | |
|---|---|---|---|---|---|---|---|---|---|
| | RMSE | MAD | $R^2_{ap}$ | RMSE | MAD | $R^2_{ap}$ | RMSE | MAD | $R^2_{ap}$ |
| $a+b/z^2+cx/y^2$ | 217.86 | 158.72 | 0.423 | 0.1228 | 0.0939 | 0.2549 | 0.4078 | 0.2957 | 0.295 |
| $a+b/z^2+cx/\sqrt{y}$ | 167.25 | 125.06 | 0.660 | 0.0911 | 0.0718 | 0.5903 | 0.2795 | 0.2034 | 0.669 |
| $a+b/z^2+cxy$ | 132.41 | 106.32 | 0.787 | 0.0838 | 0.0579 | 0.6534 | 0.2745 | 0.1891 | 0.681 |
| $a+b/z^2+cxy^2$ | 140.01 | 108.57 | 0.762 | 0.0892 | 0.0658 | 0.6068 | 0.3015 | 0.2197 | 0.615 |
| $a+b/z^2+cx\sqrt{y}$ | 132.41 | 102.59 | 0.787 | 0.0817 | 0.0573 | 0.6705 | 0.2599 | 0.1725 | 0.714 |
| $a+b/z^2+cx^2/y$ | 147.11 | 113.66 | 0.737 | 0.0839 | 0.0645 | 0.6523 | 0.2575 | 0.1832 | 0.719 |
| $a+b/z^2+cx^2/y^2$ | 206.65 | 153.47 | 0.480 | 0.1105 | 0.0855 | 0.3976 | 0.3536 | 0.2699 | 0.470 |
| $a+b/z^2+cx^2/\sqrt{y}$ | 126.97 | 103.44 | 0.804 | 0.0775 | 0.0551 | 0.7032 | 0.2430 | 0.1710 | 0.750 |
| $a+b/z^2+cx^2y$ | 130.41 | 103.23 | 0.793 | 0.0843 | 0.0633 | 0.6494 | 0.2854 | 0.2116 | 0.655 |
| $a+b/z^2+cx^2y^2$ | 141.04 | 110.19 | 0.758 | 0.0902 | 0.0697 | 0.5982 | 0.3094 | 0.2283 | 0.594 |
| $a+b/z^2+cx^2\sqrt{y}$ | 124.70 | 98.53 | 0.811 | 0.0807 | 0.0587 | 0.6785 | 0.2692 | 0.1975 | 0.693 |
| $a+b/z^2+c\sqrt{x}/y$ | 218.06 | 159.20 | 0.421 | 0.1230 | 0.0942 | 0.2526 | 0.4091 | 0.2973 | 0.291 |
| $a+b/z^2+c\sqrt{x}/y^2$ | 198.82 | 141.96 | 0.519 | 0.1119 | 0.0882 | 0.3819 | 0.3554 | 0.2619 | 0.465 |
| $a+b/z^2+c\sqrt{x}/\sqrt{y}$ | 206.18 | 156.94 | 0.483 | 0.1075 | 0.0813 | 0.4299 | 0.3442 | 0.2523 | 0.498 |
| $a+b/z^2+c\sqrt{x}y$ | 143.50 | 113.16 | 0.749 | 0.0874 | 0.0620 | 0.6229 | 0.2816 | 0.1855 | 0.664 |
| $a+b/z^2+c\sqrt{x}y^2$ | 144.28 | 114.31 | 0.747 | 0.0906 | 0.0649 | 0.5949 | 0.3026 | 0.2146 | 0.612 |
| $a+b/z^2+c\sqrt{x}\sqrt{y}$ | 149.73 | 112.33 | 0.727 | 0.0876 | 0.0658 | 0.6214 | 0.2751 | 0.1873 | 0.679 |
| $a+b/z^2+c/xy$ | 218.32 | 159.51 | 0.420 | 0.1140 | 0.0867 | 0.3585 | 0.3735 | 0.2717 | 0.409 |
| $a+b/z^2+c/xy^2$ | 219.39 | 159.73 | 0.414 | 0.1146 | 0.0870 | 0.3515 | 0.3760 | 0.2729 | 0.401 |
| $a+b/z^2+c/x\sqrt{y}$ | 217.48 | 159.32 | 0.425 | 0.1135 | 0.0864 | 0.3644 | 0.3715 | 0.2707 | 0.415 |
| $a+b/z^2+cy/x$ | 216.84 | 159.32 | 0.428 | 0.1120 | 0.0856 | 0.3803 | 0.3675 | 0.2674 | 0.428 |
| $a+b/z^2+cy^2/x$ | 218.65 | 161.01 | 0.418 | 0.1235 | 0.0950 | 0.2463 | 0.4122 | 0.3003 | 0.280 |
| $a+b/z^2+c\sqrt{y}/x$ | 215.59 | 158.91 | 0.434 | 0.1120 | 0.0857 | 0.3812 | 0.3664 | 0.2679 | 0.431 |
| $a+b/z^2+c/x^2y$ | 222.40 | 160.13 | 0.398 | 0.1157 | 0.0884 | 0.3389 | 0.3830 | 0.2768 | 0.378 |
| $a+b/z^2+c/x^2y^2$ | 222.57 | 160.11 | 0.397 | 0.1158 | 0.0884 | 0.3379 | 0.3835 | 0.2769 | 0.377 |
| $a+b/z^2+c/x^2\sqrt{y}$ | 222.28 | 160.15 | 0.399 | 0.1156 | 0.0884 | 0.3398 | 0.3827 | 0.2767 | 0.379 |
| $a+b/z^2+cy/x^2$ | 221.64 | 160.19 | 0.402 | 0.1152 | 0.0882 | 0.3451 | 0.3810 | 0.2760 | 0.385 |
| $a+b/z^2+cy^2/x^2$ | 221.18 | 160.23 | 0.405 | 0.1146 | 0.0879 | 0.3515 | 0.3791 | 0.2749 | 0.391 |
| $a+b/z^2+c\sqrt{y}/x^2$ | 221.91 | 160.18 | 0.401 | 0.1154 | 0.0883 | 0.3427 | 0.3817 | 0.2763 | 0.383 |
| $a+b/z^2+c/\sqrt{x}y$ | 212.51 | 156.20 | 0.451 | 0.1119 | 0.0851 | 0.3821 | 0.3623 | 0.2616 | 0.444 |
| $a+b/z^2+c/\sqrt{x}y^2$ | 215.64 | 157.56 | 0.434 | 0.1136 | 0.0858 | 0.3633 | 0.3689 | 0.2656 | 0.423 |
| $a+b/z^2+c/\sqrt{x}\sqrt{y}$ | 210.13 | 155.13 | 0.463 | 0.1105 | 0.0842 | 0.3976 | 0.3572 | 0.2585 | 0.460 |
| $a+b/z^2+cy/\sqrt{x}$ | 218.48 | 160.34 | 0.419 | 0.1234 | 0.0947 | 0.2482 | 0.4113 | 0.2996 | 0.283 |
| $a+b/z^2+cy^2/\sqrt{x}$ | 174.75 | 135.47 | 0.628 | 0.1034 | 0.0760 | 0.4716 | 0.3410 | 0.2411 | 0.507 |
| $a+b/z^2+c\sqrt{y}/\sqrt{x}$ | 213.40 | 158.74 | 0.446 | 0.1102 | 0.0833 | 0.4000 | 0.3590 | 0.2593 | 0.454 |
| $a+b/z^2+cx/z$ | 219.98 | 161.60 | 0.411 | 0.1216 | 0.0957 | 0.2700 | 0.3892 | 0.2964 | 0.358 |
| $a+b/z^2+cx/z^2$ | 204.82 | 151.88 | 0.490 | 0.1161 | 0.0932 | 0.3341 | 0.3636 | 0.2816 | 0.440 |
| $a+b/z^2+cx/\sqrt{z}$ | 201.06 | 150.22 | 0.508 | 0.1125 | 0.0894 | 0.3753 | 0.3502 | 0.2581 | 0.480 |
| $a+b/z^2+cxz$ | 124.21 | 93.12 | 0.812 | 0.0733 | 0.0525 | 0.7346 | 0.2688 | 0.2020 | 0.694 |
| $a+b/z^2+cxz^2$ | 139.79 | 104.69 | 0.762 | 0.0826 | 0.0632 | 0.6629 | 0.3026 | 0.2277 | 0.612 |
| $a+b/z^2+cx\sqrt{z}$ | 116.12 | 91.26 | 0.836 | 0.0692 | 0.0446 | 0.7633 | 0.2417 | 0.1611 | 0.752 |
| $a+b/z^2+cx^2/z$ | 196.10 | 145.37 | 0.532 | 0.1130 | 0.0914 | 0.3696 | 0.3485 | 0.2682 | 0.486 |
| $a+b/z^2+cx^2/z^2$ | 199.36 | 150.21 | 0.516 | 0.1150 | 0.0928 | 0.3467 | 0.3554 | 0.2759 | 0.465 |
| $a+b/z^2+cx^2/\sqrt{z}$ | 159.43 | 121.15 | 0.691 | 0.0962 | 0.0742 | 0.5429 | 0.2921 | 0.2121 | 0.639 |
| $a+b/z^2+cx^2z$ | 127.92 | 96.72 | 0.801 | 0.0787 | 0.0596 | 0.6943 | 0.2851 | 0.2204 | 0.656 |
| $a+b/z^2+cx^2z^2$ | 141.55 | 107.09 | 0.756 | 0.0861 | 0.0674 | 0.6343 | 0.3112 | 0.2369 | 0.590 |
| $a+b/z^2+cx^2\sqrt{z}$ | 119.04 | 93.58 | 0.828 | 0.0749 | 0.0551 | 0.7227 | 0.2649 | 0.1981 | 0.703 |
| $a+b/z^2+c\sqrt{x}/z$ | 229.56 | 168.92 | 0.359 | 0.1249 | 0.0975 | 0.2298 | 0.4124 | 0.3122 | 0.279 |
| $a+b/z^2+c\sqrt{x}/z^2$ | 207.31 | 152.55 | 0.477 | 0.1163 | 0.0933 | 0.3317 | 0.3666 | 0.2820 | 0.430 |
| $a+b/z^2+c\sqrt{x}/\sqrt{z}$ | 224.33 | 164.75 | 0.388 | 0.1223 | 0.0959 | 0.2611 | 0.3957 | 0.2997 | 0.337 |
| $a+b/z^2+c\sqrt{x}z$ | 127.17 | 97.99 | 0.803 | 0.0723 | 0.0496 | 0.7416 | 0.2667 | 0.1952 | 0.699 |
| $a+b/z^2+c\sqrt{x}z^2$ | 140.97 | 107.61 | 0.758 | 0.0817 | 0.0612 | 0.6705 | 0.3005 | 0.2236 | 0.617 |
| $a+b/z^2+c\sqrt{x}\sqrt{z}$ | 121.92 | 92.41 | 0.819 | 0.0685 | 0.0408 | 0.7684 | 0.2394 | 0.1530 | 0.757 |
| $a+b/z^2+c/xz$ | 212.93 | 156.51 | 0.448 | 0.1119 | 0.0850 | 0.3823 | 0.3622 | 0.2614 | 0.444 |
| $a+b/z^2+c/xz^2$ | 213.92 | 154.09 | 0.443 | 0.1146 | 0.0890 | 0.3515 | 0.3685 | 0.2641 | 0.425 |
| $a+b/z^2+c/x\sqrt{z}$ | 214.17 | 157.76 | 0.442 | 0.1118 | 0.0848 | 0.3826 | 0.3641 | 0.2648 | 0.438 |
| $a+b/z^2+cz/x$ | 224.90 | 161.97 | 0.385 | 0.1184 | 0.0914 | 0.3075 | 0.3904 | 0.2849 | 0.354 |
| $a+b/z^2+cz^2/x$ | 224.94 | 159.37 | 0.384 | 0.1244 | 0.0947 | 0.2363 | 0.4167 | 0.3060 | 0.264 |
| $a+b/z^2+c\sqrt{z}/x$ | 219.96 | 160.34 | 0.411 | 0.1148 | 0.0877 | 0.3490 | 0.3773 | 0.2752 | 0.397 |
| $a+b/z^2+c/x^2z$ | 221.01 | 160.16 | 0.406 | 0.1151 | 0.0879 | 0.3458 | 0.3795 | 0.2754 | 0.390 |
| $a+b/z^2+c/x^2z^2$ | 219.49 | 159.69 | 0.414 | 0.1148 | 0.0870 | 0.3494 | 0.3763 | 0.2729 | 0.400 |
| $a+b/z^2+c/x^2\sqrt{z}$ | 221.62 | 160.19 | 0.402 | 0.1153 | 0.0881 | 0.3434 | 0.3810 | 0.2760 | 0.385 |
| $a+b/z^2+cz/x^2$ | 223.02 | 160.06 | 0.395 | 0.1160 | 0.0886 | 0.3354 | 0.3847 | 0.2773 | 0.373 |
| $a+b/z^2+cz^2/x^2$ | 224.20 | 160.12 | 0.388 | 0.1169 | 0.0893 | 0.3252 | 0.3880 | 0.2789 | 0.362 |
| $a+b/z^2+c\sqrt{z}/x^2$ | 222.58 | 160.11 | 0.397 | 0.1158 | 0.0885 | 0.3384 | 0.3835 | 0.2769 | 0.377 |
| $a+b/z^2+c/\sqrt{x}z$ | 196.88 | 142.89 | 0.528 | 0.1047 | 0.0803 | 0.4589 | 0.3315 | 0.2376 | 0.534 |
| $a+b/z^2+c/\sqrt{x}z^2$ | 211.45 | 151.45 | 0.456 | 0.1154 | 0.0914 | 0.3429 | 0.3678 | 0.2736 | 0.427 |
| $a+b/z^2+c/\sqrt{x}\sqrt{z}$ | 198.37 | 145.69 | 0.521 | 0.1041 | 0.0797 | 0.4650 | 0.3327 | 0.2347 | 0.531 |
| $a+b/z^2+cz/\sqrt{x}$ | 221.77 | 156.15 | 0.402 | 0.1229 | 0.0913 | 0.2548 | 0.4146 | 0.3015 | 0.272 |
| $a+b/z^2+cz^2/\sqrt{x}$ | 163.16 | 123.64 | 0.676 | 0.0934 | 0.0660 | 0.5690 | 0.3368 | 0.2372 | 0.519 |
| $a+b/z^2+c\sqrt{z}/\sqrt{x}$ | 225.49 | 163.62 | 0.381 | 0.1200 | 0.0935 | 0.2888 | 0.3931 | 0.2913 | 0.345 |
| $a+b/z^2+cy/z$ | 229.18 | 168.67 | 0.361 | 0.1249 | 0.0973 | 0.2294 | 0.4137 | 0.3117 | 0.275 |
| $a+b/z^2+cy/z^2$ | 215.87 | 156.23 | 0.433 | 0.1208 | 0.0957 | 0.2799 | 0.3878 | 0.2945 | 0.363 |
| $a+b/z^2+cy/\sqrt{z}$ | 219.89 | 161.33 | 0.412 | 0.1217 | 0.0953 | 0.2683 | 0.3951 | 0.2992 | 0.339 |
| $a+b/z^2+cyz$ | 132.29 | 102.70 | 0.787 | 0.0788 | 0.0560 | 0.6932 | 0.2867 | 0.2131 | 0.652 |
| $a+b/z^2+cyz^2$ | 143.34 | 110.47 | 0.750 | 0.0849 | 0.0640 | 0.6438 | 0.3095 | 0.2299 | 0.594 |
| $a+b/z^2+cy\sqrt{z}$ | 129.64 | 99.46 | 0.796 | 0.0783 | 0.0502 | 0.6974 | 0.2741 | 0.1831 | 0.682 |
| $a+b/z^2+cy^2/z$ | 220.64 | 162.93 | 0.408 | 0.1228 | 0.0963 | 0.2557 | 0.3995 | 0.3036 | 0.324 |
| $a+b/z^2+cy^2/z^2$ | 217.14 | 156.29 | 0.426 | 0.1217 | 0.0956 | 0.2690 | 0.3919 | 0.2951 | 0.349 |
| $a+b/z^2+cy^2/\sqrt{z}$ | 197.59 | 148.86 | 0.525 | 0.1137 | 0.0888 | 0.3617 | 0.3658 | 0.2709 | 0.433 |
| $a+b/z^2+cy^2z$ | 137.87 | 104.67 | 0.769 | 0.0848 | 0.0611 | 0.6450 | 0.3038 | 0.2225 | 0.609 |
| $a+b/z^2+cy^2z^2$ | 145.90 | 111.41 | 0.741 | 0.0887 | 0.0675 | 0.6115 | 0.3192 | 0.2353 | 0.568 |
| $a+b/z^2+cy^2\sqrt{z}$ | 137.15 | 102.48 | 0.771 | 0.0853 | 0.0596 | 0.6411 | 0.2979 | 0.2033 | 0.624 |
| $a+b/z^2+c\sqrt{y}/z$ | 225.47 | 159.55 | 0.381 | 0.1212 | 0.0899 | 0.2745 | 0.4133 | 0.3019 | 0.276 |
| $a+b/z^2+c\sqrt{y}/z^2$ | 215.51 | 156.60 | 0.435 | 0.1204 | 0.0957 | 0.2842 | 0.3865 | 0.2938 | 0.367 |
| $a+b/z^2+c\sqrt{y}/\sqrt{z}$ | 229.89 | 167.25 | 0.357 | 0.1247 | 0.0956 | 0.2325 | 0.4166 | 0.3093 | 0.265 |
| $a+b/z^2+c\sqrt{y}z$ | 131.96 | 103.48 | 0.788 | 0.0764 | 0.0538 | 0.7116 | 0.2808 | 0.2072 | 0.666 |
| $a+b/z^2+c\sqrt{y}z^2$ | 143.27 | 111.27 | 0.750 | 0.0833 | 0.0621 | 0.6571 | 0.3056 | 0.2257 | 0.604 |
| $a+b/z^2+c\sqrt{y}\sqrt{z}$ | 125.99 | 99.25 | 0.807 | 0.0739 | 0.0449 | 0.7307 | 0.2620 | 0.1767 | 0.709 |

(continued on next page)

**Table 4 – continued from previous page**

| Functional form | $T_{eff}$ (K) | | | Radius ($R_{\odot}$) | | | log (L/$L_{\odot}$) | | |
|---|---|---|---|---|---|---|---|---|---|
| | RMSE | MAD | $R^2_{ap}$ | RMSE | MAD | $R^2_{ap}$ | RMSE | MAD | $R^2_{ap}$ |
| a+b/$z^2$+c/yz | 197.38 | 143.85 | 0.526 | 0.1096 | 0.0856 | 0.4066 | 0.3449 | 0.2511 | 0.496 |
| a+b/$z^2$+c/y$z^2$ | 215.48 | 157.01 | 0.435 | 0.1198 | 0.0954 | 0.2909 | 0.3853 | 0.2919 | 0.371 |
| a+b/$z^2$+c/y$\sqrt{z}$ | 193.77 | 141.84 | 0.543 | 0.1065 | 0.0813 | 0.4403 | 0.3352 | 0.2387 | 0.524 |
| a+b/$z^2$+cz/y | 227.62 | 161.78 | 0.370 | 0.1240 | 0.0937 | 0.2402 | 0.4167 | 0.3062 | 0.264 |
| a+b/$z^2$+c$z^2$/y | 168.63 | 131.40 | 0.654 | 0.0932 | 0.0686 | 0.5708 | 0.3362 | 0.2400 | 0.521 |
| a+b/$z^2$+c$\sqrt{z}$/y | 218.29 | 158.12 | 0.420 | 0.1179 | 0.0915 | 0.3133 | 0.3822 | 0.2798 | 0.381 |
| a+b/$z^2$+c/$y^2$z | 209.81 | 149.92 | 0.464 | 0.1152 | 0.0914 | 0.3449 | 0.3676 | 0.2737 | 0.427 |
| a+b/$z^2$+c/$y^2z^2$ | 215.84 | 156.91 | 0.433 | 0.1197 | 0.0953 | 0.2922 | 0.3856 | 0.2910 | 0.370 |
| a+b/$z^2$+c/$y^2\sqrt{z}$ | 208.28 | 149.91 | 0.472 | 0.1132 | 0.0887 | 0.3675 | 0.3611 | 0.2632 | 0.447 |
| a+b/$z^2$+cz/$y^2$ | 218.64 | 159.56 | 0.418 | 0.1164 | 0.0886 | 0.3310 | 0.3788 | 0.2735 | 0.392 |
| a+b/$z^2$+c$z^2$/$y^2$ | 228.41 | 162.72 | 0.365 | 0.1247 | 0.0958 | 0.2317 | 0.4170 | 0.3079 | 0.263 |
| a+b/$z^2$+c$\sqrt{z}$/$y^2$ | 212.11 | 154.91 | 0.453 | 0.1131 | 0.0863 | 0.3688 | 0.3648 | 0.2602 | 0.436 |
| a+b/$z^2$+c/$\sqrt{y}$z | 173.46 | 123.47 | 0.634 | 0.0982 | 0.0726 | 0.5239 | 0.3035 | 0.1984 | 0.610 |
| a+b/$z^2$+c/$\sqrt{y}z^2$ | 215.37 | 156.96 | 0.436 | 0.1200 | 0.0955 | 0.2895 | 0.3854 | 0.2925 | 0.371 |
| a+b/$z^2$+c/$\sqrt{y}\sqrt{z}$ | 169.37 | 120.21 | 0.651 | 0.0946 | 0.0699 | 0.5577 | 0.2946 | 0.1933 | 0.632 |
| a+b/$z^2$+cz/$\sqrt{y}$ | 176.51 | 136.29 | 0.621 | 0.0967 | 0.0707 | 0.5384 | 0.3467 | 0.2455 | 0.491 |
| a+b/$z^2$+c$z^2$/$\sqrt{y}$ | 151.82 | 115.64 | 0.720 | 0.0847 | 0.0625 | 0.6455 | 0.3112 | 0.2303 | 0.590 |
| a+b/$z^2$+c$\sqrt{z}$/$\sqrt{y}$ | 228.05 | 162.45 | 0.367 | 0.1239 | 0.0934 | 0.2416 | 0.4167 | 0.3063 | 0.264 |
| a+b/$\sqrt{z}$+cx/y | 151.50 | 108.92 | 0.721 | 0.0856 | 0.0626 | 0.6384 | 0.2748 | 0.1873 | 0.680 |
| a+b/$\sqrt{z}$+cx/$y^2$ | 157.56 | 108.84 | 0.698 | 0.0935 | 0.0632 | 0.5680 | 0.3147 | 0.2020 | 0.580 |
| a+b/$\sqrt{z}$+cx/$\sqrt{y}$ | 138.26 | 102.91 | 0.767 | 0.0804 | 0.0595 | 0.6812 | 0.2501 | 0.1686 | 0.735 |
| a+b/$\sqrt{z}$+cxy | 121.96 | 94.77 | 0.819 | 0.0793 | 0.0528 | 0.6896 | 0.2614 | 0.1717 | 0.710 |
| a+b/$\sqrt{z}$+cx$y^2$ | 125.84 | 96.25 | 0.807 | 0.0823 | 0.0558 | 0.6655 | 0.2788 | 0.1845 | 0.671 |
| a+b/$\sqrt{z}$+cx$\sqrt{y}$ | 121.84 | 91.84 | 0.819 | 0.0777 | 0.0520 | 0.7019 | 0.2495 | 0.1534 | 0.736 |
| a+b/$\sqrt{z}$+c$x^2$/y | 129.87 | 103.11 | 0.795 | 0.0779 | 0.0580 | 0.7003 | 0.2427 | 0.1643 | 0.750 |
| a+b/$\sqrt{z}$+c$x^2$/$y^2$ | 152.63 | 108.47 | 0.717 | 0.0877 | 0.0656 | 0.6201 | 0.2831 | 0.2023 | 0.660 |
| a+b/$\sqrt{z}$+c$x^2$/$\sqrt{y}$ | 118.67 | 96.57 | 0.829 | 0.0748 | 0.0517 | 0.7240 | 0.2366 | 0.1577 | 0.763 |
| a+b/$\sqrt{z}$+c$x^2$y | 120.28 | 94.74 | 0.824 | 0.0794 | 0.0555 | 0.6890 | 0.2694 | 0.1865 | 0.693 |
| a+b/$\sqrt{z}$+c$x^2y^2$ | 125.24 | 95.97 | 0.809 | 0.0823 | 0.0576 | 0.6658 | 0.2823 | 0.1904 | 0.662 |
| a+b/$\sqrt{z}$+c$x^2\sqrt{y}$ | 117.09 | 93.18 | 0.833 | 0.0773 | 0.0534 | 0.7053 | 0.2587 | 0.1805 | 0.716 |
| a+b/$\sqrt{z}$+c$\sqrt{x}$/y | 157.74 | 109.00 | 0.697 | 0.0935 | 0.0635 | 0.5683 | 0.3148 | 0.2024 | 0.580 |
| a+b/$\sqrt{z}$+c$\sqrt{x}$/$y^2$ | 149.75 | 97.88 | 0.727 | 0.0903 | 0.0637 | 0.5974 | 0.2909 | 0.1819 | 0.641 |
| a+b/$\sqrt{z}$+c$\sqrt{x}$/$\sqrt{y}$ | 152.02 | 108.54 | 0.719 | 0.0850 | 0.0606 | 0.6429 | 0.2742 | 0.1853 | 0.682 |
| a+b/$\sqrt{z}$+c$\sqrt{x}$y | 128.25 | 96.08 | 0.800 | 0.0811 | 0.0541 | 0.6749 | 0.2640 | 0.1635 | 0.705 |
| a+b/$\sqrt{z}$+c$\sqrt{x}y^2$ | 128.59 | 97.11 | 0.799 | 0.0832 | 0.0545 | 0.6584 | 0.2791 | 0.1803 | 0.670 |
| a+b/$\sqrt{z}$+c$\sqrt{x}\sqrt{y}$ | 131.06 | 93.50 | 0.791 | 0.0805 | 0.0546 | 0.6802 | 0.2562 | 0.1551 | 0.722 |
| a+b/$\sqrt{z}$+c/xy | 156.10 | 106.17 | 0.704 | 0.0873 | 0.0574 | 0.6235 | 0.2879 | 0.1750 | 0.649 |
| a+b/$\sqrt{z}$+c/x$y^2$ | 156.41 | 106.25 | 0.702 | 0.0875 | 0.0575 | 0.6220 | 0.2888 | 0.1755 | 0.647 |
| a+b/$\sqrt{z}$+c/x$\sqrt{y}$ | 155.87 | 106.15 | 0.704 | 0.0872 | 0.0574 | 0.6249 | 0.2872 | 0.1748 | 0.651 |
| a+b/$\sqrt{z}$+cy/x | 155.76 | 107.62 | 0.705 | 0.0861 | 0.0578 | 0.6343 | 0.2843 | 0.1798 | 0.658 |
| a+b/$\sqrt{z}$+c$y^2$/x | 158.03 | 109.11 | 0.696 | 0.0933 | 0.0638 | 0.5698 | 0.3143 | 0.2049 | 0.581 |
| a+b/$\sqrt{z}$+c$\sqrt{y}$/x | 155.38 | 106.58 | 0.706 | 0.0865 | 0.0573 | 0.6309 | 0.2849 | 0.1753 | 0.656 |
| a+b/$\sqrt{z}$+c/$x^2$y | 157.62 | 106.90 | 0.698 | 0.0876 | 0.0571 | 0.6213 | 0.2922 | 0.1785 | 0.638 |
| a+b/$\sqrt{z}$+c/$x^2y^2$ | 157.67 | 106.91 | 0.698 | 0.0876 | 0.0571 | 0.6211 | 0.2924 | 0.1786 | 0.638 |
| a+b/$\sqrt{z}$+c/$x^2\sqrt{y}$ | 157.58 | 106.90 | 0.698 | 0.0876 | 0.0571 | 0.6215 | 0.2921 | 0.1785 | 0.639 |
| a+b/$\sqrt{z}$+cy/$x^2$ | 157.40 | 106.92 | 0.699 | 0.0874 | 0.0571 | 0.6231 | 0.2913 | 0.1784 | 0.640 |
| a+b/$\sqrt{z}$+c$y^2$/$x^2$ | 157.27 | 107.02 | 0.699 | 0.0870 | 0.0575 | 0.6262 | 0.2902 | 0.1789 | 0.643 |
| a+b/$\sqrt{z}$+c$\sqrt{y}$/$x^2$ | 157.48 | 106.90 | 0.698 | 0.0875 | 0.0571 | 0.6223 | 0.2917 | 0.1784 | 0.640 |
| a+b/$\sqrt{z}$+c/$\sqrt{x}$y | 154.08 | 104.39 | 0.711 | 0.0872 | 0.0588 | 0.6245 | 0.2840 | 0.1692 | 0.658 |
| a+b/$\sqrt{z}$+c/$\sqrt{x}y^2$ | 154.95 | 104.90 | 0.708 | 0.0877 | 0.0592 | 0.6205 | 0.2862 | 0.1706 | 0.653 |
| a+b/$\sqrt{z}$+c/$\sqrt{x}\sqrt{y}$ | 153.43 | 104.21 | 0.714 | 0.0867 | 0.0583 | 0.6286 | 0.2822 | 0.1686 | 0.663 |
| a+b/$\sqrt{z}$+cy/$\sqrt{x}$ | 157.97 | 109.13 | 0.696 | 0.0934 | 0.0638 | 0.5693 | 0.3146 | 0.2040 | 0.581 |
| a+b/$\sqrt{z}$+c$y^2$/$\sqrt{x}$ | 143.38 | 100.09 | 0.750 | 0.0889 | 0.0595 | 0.6097 | 0.2957 | 0.1842 | 0.630 |
| a+b/$\sqrt{z}$+c$\sqrt{y}$/$\sqrt{x}$ | 154.55 | 107.95 | 0.709 | 0.0855 | 0.0586 | 0.6392 | 0.2802 | 0.1810 | 0.667 |
| a+b/$\sqrt{z}$+cx/z | 134.75 | 94.67 | 0.779 | 0.0831 | 0.0598 | 0.6587 | 0.2532 | 0.1609 | 0.728 |
| a+b/$\sqrt{z}$+cx/$z^2$ | 121.69 | 86.88 | 0.820 | 0.0755 | 0.0492 | 0.7188 | 0.2360 | 0.1359 | 0.764 |
| a+b/$\sqrt{z}$+cx/$\sqrt{z}$ | 138.20 | 97.05 | 0.768 | 0.0844 | 0.0610 | 0.6482 | 0.2593 | 0.1660 | 0.715 |
| a+b/$\sqrt{z}$+cxz | 123.11 | 93.07 | 0.816 | 0.0730 | 0.0512 | 0.7365 | 0.2659 | 0.1936 | 0.700 |
| a+b/$\sqrt{z}$+cx$z^2$ | 131.63 | 99.20 | 0.789 | 0.0790 | 0.0560 | 0.6919 | 0.2855 | 0.1992 | 0.655 |
| a+b/$\sqrt{z}$+cx$\sqrt{z}$ | 115.69 | 90.45 | 0.837 | 0.0695 | 0.0448 | 0.7612 | 0.2417 | 0.1604 | 0.752 |
| a+b/$\sqrt{z}$+c$x^2$/z | 129.66 | 90.40 | 0.795 | 0.0833 | 0.0611 | 0.6576 | 0.2513 | 0.1661 | 0.732 |
| a+b/$\sqrt{z}$+c$x^2$/$z^2$ | 120.33 | 82.25 | 0.824 | 0.0777 | 0.0532 | 0.7021 | 0.2352 | 0.1373 | 0.766 |
| a+b/$\sqrt{z}$+c$x^2$/$\sqrt{z}$ | 125.92 | 90.43 | 0.807 | 0.0813 | 0.0585 | 0.6735 | 0.2500 | 0.1636 | 0.735 |
| a+b/$\sqrt{z}$+c$x^2$z | 123.33 | 92.16 | 0.815 | 0.0765 | 0.0547 | 0.7113 | 0.2747 | 0.2009 | 0.680 |
| a+b/$\sqrt{z}$+c$x^2z^2$ | 129.85 | 96.34 | 0.795 | 0.0803 | 0.0576 | 0.6819 | 0.2873 | 0.2022 | 0.650 |
| a+b/$\sqrt{z}$+c$x^2\sqrt{z}$ | 116.64 | 90.96 | 0.834 | 0.0739 | 0.0525 | 0.7303 | 0.2601 | 0.1877 | 0.713 |
| a+b/$\sqrt{z}$+c$\sqrt{x}$/z | 135.33 | 95.72 | 0.777 | 0.0812 | 0.0566 | 0.6746 | 0.2507 | 0.1546 | 0.734 |
| a+b/$\sqrt{z}$+c$\sqrt{x}$/$z^2$ | 121.77 | 89.30 | 0.820 | 0.0726 | 0.0439 | 0.7398 | 0.2361 | 0.1407 | 0.764 |
| a+b/$\sqrt{z}$+c$\sqrt{x}$/$\sqrt{z}$ | 144.58 | 98.67 | 0.746 | 0.0858 | 0.0611 | 0.6364 | 0.2678 | 0.1693 | 0.696 |
| a+b/$\sqrt{z}$+c$\sqrt{x}$z | 126.46 | 97.84 | 0.805 | 0.0724 | 0.0494 | 0.7410 | 0.2655 | 0.1898 | 0.701 |
| a+b/$\sqrt{z}$+c$\sqrt{x}z^2$ | 133.71 | 101.14 | 0.782 | 0.0788 | 0.0552 | 0.6933 | 0.2858 | 0.2002 | 0.654 |
| a+b/$\sqrt{z}$+c$\sqrt{x}\sqrt{z}$ | 121.50 | 92.74 | 0.820 | 0.0691 | 0.0421 | 0.7643 | 0.2398 | 0.1529 | 0.756 |
| a+b/$\sqrt{z}$+c/xz | 155.41 | 104.80 | 0.706 | 0.0881 | 0.0597 | 0.6166 | 0.2872 | 0.1715 | 0.651 |
| a+b/$\sqrt{z}$+c/x$z^2$ | 156.89 | 102.69 | 0.701 | 0.0911 | 0.0635 | 0.5905 | 0.2962 | 0.1837 | 0.628 |
| a+b/$\sqrt{z}$+c/x$\sqrt{z}$ | 155.34 | 105.69 | 0.706 | 0.0872 | 0.0580 | 0.6241 | 0.2859 | 0.1733 | 0.654 |
| a+b/$\sqrt{z}$+cz/x | 157.24 | 106.01 | 0.699 | 0.0880 | 0.0576 | 0.6177 | 0.2914 | 0.1770 | 0.640 |
| a+b/$\sqrt{z}$+c$z^2$/x | 160.08 | 111.46 | 0.688 | 0.0927 | 0.0627 | 0.5761 | 0.3076 | 0.1926 | 0.599 |
| a+b/$\sqrt{z}$+c$\sqrt{z}$/x | 156.19 | 106.37 | 0.703 | 0.0871 | 0.0570 | 0.6257 | 0.2879 | 0.1760 | 0.649 |
| a+b/$\sqrt{z}$+c/$x^2$z | 157.14 | 106.65 | 0.700 | 0.0875 | 0.0568 | 0.6216 | 0.2907 | 0.1775 | 0.642 |
| a+b/$\sqrt{z}$+c/$x^2z^2$ | 156.56 | 106.09 | 0.702 | 0.0878 | 0.0581 | 0.6194 | 0.2895 | 0.1755 | 0.645 |
| a+b/$\sqrt{z}$+c/$x^2\sqrt{z}$ | 157.36 | 106.81 | 0.699 | 0.0875 | 0.0569 | 0.6219 | 0.2913 | 0.1781 | 0.640 |
| a+b/$\sqrt{z}$+cz/$x^2$ | 157.81 | 106.93 | 0.697 | 0.0876 | 0.0572 | 0.6211 | 0.2929 | 0.1789 | 0.636 |
| a+b/$\sqrt{z}$+c$z^2$/$x^2$ | 158.10 | 106.77 | 0.696 | 0.0879 | 0.0574 | 0.6189 | 0.2941 | 0.1791 | 0.634 |
| a+b/$\sqrt{z}$+c$\sqrt{z}$/$x^2$ | 157.68 | 106.93 | 0.697 | 0.0875 | 0.0572 | 0.6216 | 0.2924 | 0.1787 | 0.638 |
| a+b/$\sqrt{z}$+c/$\sqrt{x}$z | 155.63 | 102.27 | 0.705 | 0.0900 | 0.0627 | 0.5997 | 0.2908 | 0.1775 | 0.642 |
| a+b/$\sqrt{z}$+c/$\sqrt{x}z^2$ | 160.06 | 112.17 | 0.688 | 0.0934 | 0.0627 | 0.5696 | 0.3137 | 0.2011 | 0.583 |
| a+b/$\sqrt{z}$+c/$\sqrt{x}\sqrt{z}$ | 153.11 | 103.62 | 0.715 | 0.0871 | 0.0593 | 0.6257 | 0.2813 | 0.1685 | 0.665 |
| a+b/$\sqrt{z}$+cz/$\sqrt{x}$ | 159.87 | 109.28 | 0.689 | 0.0926 | 0.0627 | 0.5770 | 0.3054 | 0.1901 | 0.605 |
| a+b/$\sqrt{z}$+c$z^2$/$\sqrt{x}$ | 147.67 | 113.20 | 0.735 | 0.0871 | 0.0583 | 0.6254 | 0.3064 | 0.2022 | 0.602 |
| a+b/$\sqrt{z}$+c$\sqrt{z}$/$\sqrt{x}$ | 155.62 | 104.82 | 0.705 | 0.0879 | 0.0588 | 0.6183 | 0.2874 | 0.1739 | 0.650 |
| a+b/$\sqrt{z}$+cy/z | 141.34 | 96.46 | 0.757 | 0.0868 | 0.0614 | 0.6277 | 0.2747 | 0.1706 | 0.680 |
| a+b/$\sqrt{z}$+cy/$z^2$ | 123.83 | 91.22 | 0.813 | 0.0762 | 0.0480 | 0.7135 | 0.2445 | 0.1479 | 0.747 |
| a+b/$\sqrt{z}$+cy/$\sqrt{z}$ | 146.56 | 97.29 | 0.739 | 0.0892 | 0.0630 | 0.6068 | 0.2862 | 0.1767 | 0.653 |

(continued on next page)

| Functional form | $T_{eff}$ (K) | | | Radius ($R_\odot$) | | | log (L/$L_\odot$) | | |
|---|---|---|---|---|---|---|---|---|---|
| | RMSE | MAD | $R^2_{ap}$ | RMSE | MAD | $R^2_{ap}$ | RMSE | MAD | $R^2_{ap}$ |
| $a+b/\sqrt{z}+cyz$ | 128.86 | 99.46 | 0.798 | 0.0777 | 0.0524 | 0.7021 | 0.2792 | 0.1959 | 0.670 |
| $a+b/\sqrt{z}+cyz^2$ | 133.54 | 102.59 | 0.783 | 0.0805 | 0.0558 | 0.6801 | 0.2893 | 0.2001 | 0.645 |
| $a+b/\sqrt{z}+cy\sqrt{z}$ | 126.48 | 96.35 | 0.805 | 0.0777 | 0.0482 | 0.7017 | 0.2701 | 0.1753 | 0.691 |
| $a+b/\sqrt{z}+cy^2/z$ | 144.07 | 96.15 | 0.747 | 0.0893 | 0.0630 | 0.6060 | 0.2861 | 0.1797 | 0.653 |
| $a+b/\sqrt{z}+cy^2/z^2$ | 128.82 | 90.58 | 0.798 | 0.0814 | 0.0549 | 0.6726 | 0.2561 | 0.1532 | 0.722 |
| $a+b/\sqrt{z}+cy^2/\sqrt{z}$ | 143.37 | 98.28 | 0.750 | 0.0892 | 0.0621 | 0.6075 | 0.2893 | 0.1819 | 0.645 |
| $a+b/\sqrt{z}+cy^2z$ | 129.41 | 97.91 | 0.796 | 0.0807 | 0.0535 | 0.6785 | 0.2861 | 0.1955 | 0.653 |
| $a+b/\sqrt{z}+cy^2z^2$ | 132.20 | 100.24 | 0.787 | 0.0819 | 0.0563 | 0.6689 | 0.2915 | 0.1976 | 0.640 |
| $a+b/\sqrt{z}+cy^2\sqrt{z}$ | 128.50 | 96.11 | 0.799 | 0.0813 | 0.0530 | 0.6737 | 0.2823 | 0.1835 | 0.662 |
| $a+b/\sqrt{z}+c\sqrt{y}/z$ | 135.58 | 95.58 | 0.776 | 0.0828 | 0.0569 | 0.6616 | 0.2612 | 0.1557 | 0.711 |
| $a+b/\sqrt{z}+c\sqrt{y}/z^2$ | 122.62 | 90.53 | 0.817 | 0.0727 | 0.0437 | 0.7392 | 0.2429 | 0.1488 | 0.750 |
| $a+b/\sqrt{z}+c\sqrt{y}/\sqrt{z}$ | 148.18 | 97.31 | 0.733 | 0.0893 | 0.0631 | 0.6061 | 0.2857 | 0.1761 | 0.654 |
| $a+b/\sqrt{z}+c\sqrt{y}z$ | 130.22 | 101.05 | 0.794 | 0.0763 | 0.0520 | 0.7126 | 0.2772 | 0.1961 | 0.674 |
| $a+b/\sqrt{z}+c\sqrt{y}z^2$ | 134.96 | 103.43 | 0.778 | 0.0799 | 0.0556 | 0.6845 | 0.2887 | 0.2012 | 0.647 |
| $a+b/\sqrt{z}+c\sqrt{y}\sqrt{z}$ | 125.51 | 98.38 | 0.808 | 0.0748 | 0.0452 | 0.7241 | 0.2627 | 0.1734 | 0.708 |
| $a+b/\sqrt{z}+c/yz$ | 155.48 | 99.64 | 0.706 | 0.0922 | 0.0645 | 0.5806 | 0.2987 | 0.1897 | 0.622 |
| $a+b/\sqrt{z}+c/yz^2$ | 160.06 | 110.83 | 0.688 | 0.0931 | 0.0626 | 0.5723 | 0.3143 | 0.2016 | 0.581 |
| $a+b/\sqrt{z}+c/y\sqrt{z}$ | 151.76 | 98.28 | 0.720 | 0.0896 | 0.0631 | 0.6039 | 0.2871 | 0.1785 | 0.651 |
| $a+b/\sqrt{z}+cz/y$ | 158.06 | 102.25 | 0.696 | 0.0923 | 0.0632 | 0.5792 | 0.3032 | 0.1853 | 0.610 |
| $a+b/\sqrt{z}+cz^2/y$ | 151.32 | 118.68 | 0.721 | 0.0873 | 0.0610 | 0.6238 | 0.3068 | 0.2058 | 0.601 |
| $a+b/\sqrt{z}+c\sqrt{z}/y$ | 151.88 | 99.80 | 0.719 | 0.0883 | 0.0609 | 0.6151 | 0.2857 | 0.1667 | 0.654 |
| $a+b/\sqrt{z}+c/y^2z$ | 154.02 | 98.87 | 0.711 | 0.0911 | 0.0643 | 0.5903 | 0.2941 | 0.1886 | 0.633 |
| $a+b/\sqrt{z}+c/y^2z^2$ | 156.74 | 103.09 | 0.701 | 0.0931 | 0.0642 | 0.5720 | 0.3053 | 0.1965 | 0.605 |
| $a+b/\sqrt{z}+c/y^2\sqrt{z}$ | 152.98 | 99.27 | 0.715 | 0.0896 | 0.0631 | 0.6032 | 0.2885 | 0.1809 | 0.647 |
| $a+b/\sqrt{z}+cz/y^2$ | 154.04 | 102.36 | 0.711 | 0.0879 | 0.0595 | 0.6187 | 0.2866 | 0.1676 | 0.652 |
| $a+b/\sqrt{z}+cz^2/y^2$ | 159.24 | 105.88 | 0.691 | 0.0923 | 0.0626 | 0.5791 | 0.3051 | 0.1883 | 0.605 |
| $a+b/\sqrt{z}+c\sqrt{z}/y^2$ | 152.83 | 101.79 | 0.716 | 0.0876 | 0.0600 | 0.6211 | 0.2838 | 0.1674 | 0.659 |
| $a+b/\sqrt{z}+c/\sqrt{y}z$ | 158.47 | 104.36 | 0.694 | 0.0934 | 0.0634 | 0.5691 | 0.3074 | 0.1916 | 0.600 |
| $a+b/\sqrt{z}+c/\sqrt{y}z^2$ | 154.91 | 116.31 | 0.708 | 0.0871 | 0.0577 | 0.6253 | 0.3071 | 0.2008 | 0.600 |
| $a+b/\sqrt{z}+c/\sqrt{y}\sqrt{z}$ | 150.83 | 97.96 | 0.723 | 0.0895 | 0.0630 | 0.6045 | 0.2864 | 0.1768 | 0.652 |
| $a+b/\sqrt{z}+cz/\sqrt{y}$ | 157.00 | 118.94 | 0.700 | 0.0908 | 0.0625 | 0.5933 | 0.3133 | 0.2039 | 0.584 |
| $a+b/\sqrt{z}+cz^2/\sqrt{y}$ | 142.63 | 110.99 | 0.752 | 0.0819 | 0.0576 | 0.6688 | 0.2949 | 0.2036 | 0.632 |
| $a+b/\sqrt{z}+c\sqrt{z}/\sqrt{y}$ | 156.42 | 99.58 | 0.702 | 0.0919 | 0.0634 | 0.5828 | 0.3001 | 0.1818 | 0.618 |
| Single EW ratio, double component functions result (x/y) | | | | | | | | | |
| $a+bx/y+cx/y^2$ | 181.69 | 138.02 | 0.598 | 0.1000 | 0.0777 | 0.5066 | 0.3053 | 0.2218 | 0.605 |
| $a+bx/y+cx/\sqrt{y}$ | 144.09 | 113.64 | 0.747 | 0.0849 | 0.0630 | 0.6444 | 0.2609 | 0.1770 | 0.711 |
| $a+bx/y+cxy$ | 137.97 | 108.11 | 0.768 | 0.0811 | 0.0574 | 0.6750 | 0.2588 | 0.1777 | 0.716 |
| $a+bx/y+cxy^2$ | 139.41 | 106.29 | 0.764 | 0.0813 | 0.0593 | 0.6737 | 0.2639 | 0.1877 | 0.705 |
| $a+bx/y+cx\sqrt{y}$ | 138.32 | 109.67 | 0.767 | 0.0816 | 0.0577 | 0.6710 | 0.2574 | 0.1722 | 0.719 |
| $a+bx/y+cx^2/y$ | 121.11 | 93.38 | 0.822 | 0.0789 | 0.0564 | 0.6928 | 0.2457 | 0.1726 | 0.744 |
| $a+bx/y+cx^2/y^2$ | 253.93 | 191.00 | 0.215 | 0.1220 | 0.0953 | 0.2648 | 0.3992 | 0.3089 | 0.325 |
| $a+bx/y+cx^2/\sqrt{y}$ | 122.41 | 95.18 | 0.818 | 0.0772 | 0.0531 | 0.7058 | 0.2444 | 0.1730 | 0.747 |
| $a+bx/y+cx^2y$ | 133.92 | 106.06 | 0.782 | 0.0790 | 0.0571 | 0.6921 | 0.2583 | 0.1838 | 0.717 |
| $a+bx/y+cx^2y^2$ | 140.16 | 113.51 | 0.761 | 0.0810 | 0.0610 | 0.6757 | 0.2677 | 0.1935 | 0.696 |
| $a+bx/y+cx^2\sqrt{y}$ | 130.42 | 101.65 | 0.793 | 0.0781 | 0.0551 | 0.6990 | 0.2534 | 0.1798 | 0.728 |
| $a+bx/y+c\sqrt{x}/y$ | 177.55 | 136.79 | 0.616 | 0.0989 | 0.0766 | 0.5171 | 0.3023 | 0.2200 | 0.613 |
| $a+bx/y+c\sqrt{x}/y^2$ | 219.54 | 162.20 | 0.414 | 0.1122 | 0.0878 | 0.3788 | 0.3530 | 0.2598 | 0.472 |
| $a+bx/y+c\sqrt{x}/\sqrt{y}$ | 250.67 | 186.84 | 0.235 | 0.1220 | 0.0948 | 0.2656 | 0.3977 | 0.3090 | 0.330 |
| $a+bx/y+c\sqrt{x}y$ | 151.13 | 118.38 | 0.722 | 0.0858 | 0.0633 | 0.6367 | 0.2711 | 0.1848 | 0.689 |
| $a+bx/y+c\sqrt{x}y^2$ | 144.60 | 111.28 | 0.746 | 0.0834 | 0.0599 | 0.6568 | 0.2678 | 0.1874 | 0.696 |
| $a+bx/y+c\sqrt{x}\sqrt{y}$ | 159.04 | 124.08 | 0.692 | 0.0885 | 0.0671 | 0.6130 | 0.2780 | 0.1902 | 0.673 |
| $a+bx/y+c/xy$ | 251.47 | 186.94 | 0.231 | 0.1219 | 0.0948 | 0.2664 | 0.3979 | 0.3091 | 0.329 |
| $a+bx/y+c/xy^2$ | 250.06 | 185.42 | 0.239 | 0.1217 | 0.0944 | 0.2692 | 0.3967 | 0.3081 | 0.333 |
| $a+bx/y+c/x\sqrt{y}$ | 252.25 | 187.70 | 0.226 | 0.1220 | 0.0949 | 0.2650 | 0.3984 | 0.3094 | 0.327 |
| $a+bx/y+cy/x$ | 246.27 | 180.96 | 0.262 | 0.1214 | 0.0935 | 0.2727 | 0.3940 | 0.3036 | 0.342 |
| $a+bx/y+cy^2/x$ | 170.03 | 133.11 | 0.648 | 0.0976 | 0.0750 | 0.5294 | 0.3017 | 0.2170 | 0.614 |
| $a+bx/y+c\sqrt{y}/x$ | 252.58 | 188.28 | 0.224 | 0.1221 | 0.0950 | 0.2642 | 0.3987 | 0.3094 | 0.326 |
| $a+bx/y+c/x^2y$ | 244.81 | 178.46 | 0.271 | 0.1210 | 0.0928 | 0.2769 | 0.3923 | 0.3010 | 0.348 |
| $a+bx/y+c/x^2y^2$ | 244.50 | 178.04 | 0.273 | 0.1210 | 0.0927 | 0.2775 | 0.3920 | 0.3006 | 0.349 |
| $a+bx/y+c/x^2\sqrt{y}$ | 245.02 | 178.74 | 0.270 | 0.1211 | 0.0929 | 0.2764 | 0.3925 | 0.3013 | 0.347 |
| $a+bx/y+cy/x^2$ | 245.80 | 179.76 | 0.265 | 0.1212 | 0.0931 | 0.2745 | 0.3933 | 0.3023 | 0.345 |
| $a+bx/y+cy^2/x^2$ | 244.25 | 177.85 | 0.274 | 0.1210 | 0.0927 | 0.2766 | 0.3921 | 0.3003 | 0.349 |
| $a+bx/y+c\sqrt{y}/x^2$ | 245.57 | 179.47 | 0.266 | 0.1212 | 0.0930 | 0.2751 | 0.3931 | 0.3020 | 0.345 |
| $a+bx/y+c/\sqrt{x}y$ | 254.20 | 191.45 | 0.214 | 0.1217 | 0.0952 | 0.2690 | 0.3977 | 0.3054 | 0.330 |
| $a+bx/y+c/\sqrt{x}y^2$ | 254.29 | 190.75 | 0.213 | 0.1221 | 0.0952 | 0.2640 | 0.3992 | 0.3089 | 0.325 |
| $a+bx/y+c/\sqrt{x}\sqrt{y}$ | 253.24 | 190.30 | 0.220 | 0.1211 | 0.0948 | 0.2764 | 0.3956 | 0.3021 | 0.337 |
| $a+bx/y+cy/\sqrt{x}$ | 171.62 | 134.36 | 0.642 | 0.0977 | 0.0752 | 0.5285 | 0.3006 | 0.2176 | 0.617 |
| $a+bx/y+cy^2/\sqrt{x}$ | 172.95 | 133.79 | 0.636 | 0.0941 | 0.0723 | 0.5631 | 0.2980 | 0.2088 | 0.624 |
| $a+bx/y+c\sqrt{y}/\sqrt{x}$ | 247.64 | 182.93 | 0.254 | 0.1216 | 0.0940 | 0.2702 | 0.3953 | 0.3056 | 0.338 |
| $a+bx/y^2+cx/\sqrt{y}$ | 161.78 | 125.17 | 0.682 | 0.0906 | 0.0698 | 0.5949 | 0.2753 | 0.1950 | 0.679 |
| $a+bx/y^2+cxy$ | 139.27 | 110.11 | 0.764 | 0.0820 | 0.0598 | 0.6680 | 0.2733 | 0.1949 | 0.684 |
| $a+bx/y^2+cxy^2$ | 151.24 | 116.34 | 0.722 | 0.0890 | 0.0667 | 0.6091 | 0.3084 | 0.2244 | 0.597 |
| $a+bx/y^2+cx\sqrt{y}$ | 138.61 | 109.05 | 0.766 | 0.0809 | 0.0566 | 0.6770 | 0.2598 | 0.1793 | 0.714 |
| $a+bx/y^2+cx^2/y$ | 133.05 | 106.01 | 0.785 | 0.0817 | 0.0603 | 0.6706 | 0.2464 | 0.1696 | 0.743 |
| $a+bx/y^2+cx^2/y^2$ | 170.62 | 128.44 | 0.646 | 0.0993 | 0.0778 | 0.5133 | 0.2991 | 0.2188 | 0.621 |
| $a+bx/y^2+cx^2/\sqrt{y}$ | 124.32 | 94.18 | 0.812 | 0.0776 | 0.0544 | 0.7027 | 0.2430 | 0.1655 | 0.750 |
| $a+bx/y^2+cx^2y$ | 139.89 | 110.63 | 0.762 | 0.0847 | 0.0638 | 0.6461 | 0.2924 | 0.2165 | 0.638 |
| $a+bx/y^2+cx^2y^2$ | 156.53 | 121.98 | 0.702 | 0.0929 | 0.0719 | 0.5741 | 0.3256 | 0.2419 | 0.551 |
| $a+bx/y^2+cx^2\sqrt{y}$ | 131.22 | 103.94 | 0.791 | 0.0806 | 0.0586 | 0.6795 | 0.2729 | 0.1991 | 0.685 |
| $a+bx/y^2+c\sqrt{x}/y$ | 256.18 | 198.10 | 0.201 | 0.1365 | 0.1053 | 0.0799 | 0.4549 | 0.3475 | 0.123 |
| $a+bx/y^2+c\sqrt{x}/y^2$ | 224.34 | 165.34 | 0.388 | 0.1194 | 0.0933 | 0.2964 | 0.3814 | 0.2821 | 0.384 |
| $a+bx/y^2+c\sqrt{x}/\sqrt{y}$ | 192.61 | 147.04 | 0.549 | 0.1028 | 0.0808 | 0.4777 | 0.3200 | 0.2347 | 0.566 |
| $a+bx/y^2+c\sqrt{x}y$ | 151.57 | 119.86 | 0.721 | 0.0854 | 0.0611 | 0.6395 | 0.2791 | 0.1941 | 0.670 |
| $a+bx/y^2+c\sqrt{x}y^2$ | 153.77 | 118.44 | 0.712 | 0.0888 | 0.0657 | 0.6105 | 0.3045 | 0.2157 | 0.607 |
| $a+bx/y^2+c\sqrt{x}\sqrt{y}$ | 159.30 | 122.76 | 0.691 | 0.0880 | 0.0659 | 0.6180 | 0.2787 | 0.1908 | 0.671 |
| $a+bx/y^2+c/xy$ | 237.03 | 177.34 | 0.316 | 0.1223 | 0.0910 | 0.2613 | 0.4033 | 0.2953 | 0.311 |
| $a+bx/y^2+c/xy^2$ | 238.49 | 177.95 | 0.308 | 0.1231 | 0.0913 | 0.2517 | 0.4065 | 0.2973 | 0.300 |
| $a+bx/y^2+c/x\sqrt{y}$ | 235.66 | 176.82 | 0.324 | 0.1215 | 0.0906 | 0.2707 | 0.4004 | 0.2936 | 0.321 |
| $a+bx/y^2+cy/x$ | 225.79 | 172.16 | 0.380 | 0.1158 | 0.0874 | 0.3375 | 0.3794 | 0.2802 | 0.390 |
| $a+bx/y^2+cy^2/x$ | 256.23 | 198.64 | 0.201 | 0.1366 | 0.1056 | 0.0784 | 0.4559 | 0.3497 | 0.119 |
| $a+bx/y^2+c\sqrt{y}/x$ | 230.32 | 174.59 | 0.355 | 0.1185 | 0.0889 | 0.3067 | 0.3893 | 0.2867 | 0.358 |
| $a+bx/y^2+c/x^2y$ | 240.59 | 180.98 | 0.296 | 0.1237 | 0.0922 | 0.2448 | 0.4114 | 0.3044 | 0.283 |

(continued on next page)

**Table 4 – continued from previous page**

| Functional form | $T_{eff}$ (K) | | | Radius ($R_{\odot}$) | | | log (L/$L_{\odot}$) | | |
|---|---|---|---|---|---|---|---|---|---|
| | RMSE | MAD | $R^2_{ap}$ | RMSE | MAD | $R^2_{ap}$ | RMSE | MAD | $R^2_{ap}$ |
| $a+bx/y^2+c/x^2y^2$ | 240.79 | 181.08 | 0.295 | 0.1238 | 0.0923 | 0.2435 | 0.4119 | 0.3047 | 0.281 |
| $a+bx/y^2+c/x^2\sqrt{y}$ | 240.41 | 180.91 | 0.297 | 0.1236 | 0.0921 | 0.2460 | 0.4110 | 0.3041 | 0.284 |
| $a+bx/y^2+cy/x^2$ | 238.98 | 180.52 | 0.305 | 0.1227 | 0.0916 | 0.2562 | 0.4079 | 0.3024 | 0.295 |
| $a+bx/y^2+cy^2/x^2$ | 236.08 | 179.64 | 0.322 | 0.1210 | 0.0907 | 0.2775 | 0.4013 | 0.2991 | 0.318 |
| $a+bx/y^2+c\sqrt{y}/x^2$ | 239.68 | 180.71 | 0.301 | 0.1232 | 0.0918 | 0.2511 | 0.4094 | 0.3032 | 0.290 |
| $a+bx/y^2+c/\sqrt{x}y$ | 232.13 | 172.10 | 0.344 | 0.1204 | 0.0912 | 0.2844 | 0.3932 | 0.2841 | 0.345 |
| $a+bx/y^2+c/\sqrt{x}y^2$ | 236.03 | 173.84 | 0.322 | 0.1225 | 0.0924 | 0.2588 | 0.4014 | 0.2889 | 0.317 |
| $a+bx/y^2+c/\sqrt{x}\sqrt{y}$ | 228.52 | 170.45 | 0.365 | 0.1184 | 0.0901 | 0.3078 | 0.3860 | 0.2793 | 0.369 |
| $a+bx/y^2+cy/\sqrt{x}$ | 256.24 | 198.52 | 0.201 | 0.1366 | 0.1055 | 0.0789 | 0.4556 | 0.3490 | 0.121 |
| $a+bx/y^2+cy^2/\sqrt{x}$ | 187.09 | 150.81 | 0.574 | 0.1013 | 0.0761 | 0.4931 | 0.3415 | 0.2361 | 0.506 |
| $a+bx/y^2+c\sqrt{y}/\sqrt{x}$ | 216.71 | 163.75 | 0.429 | 0.1118 | 0.0856 | 0.3832 | 0.3615 | 0.2625 | 0.446 |
| $a+bx/\sqrt{y}+cxy$ | 137.80 | 108.28 | 0.769 | 0.0815 | 0.0574 | 0.6724 | 0.2574 | 0.1724 | 0.719 |
| $a+bx/\sqrt{y}+cxy^2$ | 137.36 | 105.32 | 0.770 | 0.0811 | 0.0582 | 0.6750 | 0.2580 | 0.1766 | 0.718 |
| $a+bx/\sqrt{y}+cx\sqrt{y}$ | 138.27 | 109.61 | 0.767 | 0.0818 | 0.0577 | 0.6695 | 0.2573 | 0.1703 | 0.720 |
| $a+bx/\sqrt{y}+cx^2/y$ | 148.21 | 120.43 | 0.733 | 0.0837 | 0.0603 | 0.6541 | 0.2608 | 0.1881 | 0.712 |
| $a+bx/\sqrt{y}+cx^2/y^2$ | 171.85 | 128.45 | 0.641 | 0.0901 | 0.0695 | 0.5995 | 0.2806 | 0.1958 | 0.666 |
| $a+bx/\sqrt{y}+cx^2/\sqrt{y}$ | 124.72 | 100.16 | 0.811 | 0.0772 | 0.0535 | 0.7059 | 0.2447 | 0.1737 | 0.746 |
| $a+bx/\sqrt{y}+cx^2y$ | 131.88 | 102.75 | 0.788 | 0.0788 | 0.0560 | 0.6933 | 0.2524 | 0.1735 | 0.730 |
| $a+bx/\sqrt{y}+cx^2y^2$ | 134.68 | 106.05 | 0.779 | 0.0797 | 0.0582 | 0.6861 | 0.2556 | 0.1778 | 0.723 |
| $a+bx/\sqrt{y}+cx^2\sqrt{y}$ | 129.72 | 100.46 | 0.795 | 0.0782 | 0.0547 | 0.6979 | 0.2501 | 0.1722 | 0.735 |
| $a+bx/\sqrt{y}+c\sqrt{x}/y$ | 160.04 | 124.48 | 0.688 | 0.0903 | 0.0693 | 0.5973 | 0.2750 | 0.1942 | 0.680 |
| $a+bx/\sqrt{y}+c\sqrt{x}/y^2$ | 186.58 | 136.37 | 0.576 | 0.0945 | 0.0744 | 0.5591 | 0.2938 | 0.2144 | 0.634 |
| $a+bx/\sqrt{y}+c\sqrt{x}/\sqrt{y}$ | 127.00 | 97.74 | 0.804 | 0.0829 | 0.0583 | 0.6609 | 0.2505 | 0.1650 | 0.734 |
| $a+bx/\sqrt{y}+c\sqrt{x}y$ | 150.36 | 116.82 | 0.725 | 0.0854 | 0.0633 | 0.6399 | 0.2674 | 0.1816 | 0.697 |
| $a+bx/\sqrt{y}+c\sqrt{x}y^2$ | 142.87 | 110.70 | 0.752 | 0.0831 | 0.0594 | 0.6589 | 0.2625 | 0.1769 | 0.708 |
| $a+bx/\sqrt{y}+c\sqrt{x}\sqrt{y}$ | 159.88 | 122.31 | 0.689 | 0.0880 | 0.0670 | 0.6175 | 0.2742 | 0.1894 | 0.681 |
| $a+bx/\sqrt{y}+c/xy$ | 141.18 | 107.23 | 0.757 | 0.0860 | 0.0658 | 0.6348 | 0.2575 | 0.1807 | 0.719 |
| $a+bx/\sqrt{y}+c/xy^2$ | 140.15 | 106.64 | 0.761 | 0.0858 | 0.0657 | 0.6363 | 0.2567 | 0.1800 | 0.721 |
| $a+bx/\sqrt{y}+c/x\sqrt{y}$ | 141.85 | 107.87 | 0.755 | 0.0862 | 0.0661 | 0.6332 | 0.2582 | 0.1816 | 0.718 |
| $a+bx/\sqrt{y}+cy/x$ | 135.54 | 106.58 | 0.776 | 0.0866 | 0.0665 | 0.6301 | 0.2572 | 0.1850 | 0.720 |
| $a+bx/\sqrt{y}+cy^2/x$ | 156.52 | 122.27 | 0.702 | 0.0900 | 0.0685 | 0.6001 | 0.2759 | 0.1934 | 0.677 |
| $a+bx/\sqrt{y}+c\sqrt{y}/x$ | 140.82 | 108.47 | 0.759 | 0.0866 | 0.0668 | 0.6295 | 0.2586 | 0.1847 | 0.717 |
| $a+bx/\sqrt{y}+c/x^2y$ | 143.70 | 109.37 | 0.749 | 0.0879 | 0.0680 | 0.6186 | 0.2616 | 0.1886 | 0.710 |
| $a+bx/\sqrt{y}+c/x^2y^2$ | 143.76 | 109.33 | 0.749 | 0.0879 | 0.0680 | 0.6183 | 0.2617 | 0.1888 | 0.710 |
| $a+bx/\sqrt{y}+c/x^2\sqrt{y}$ | 143.72 | 109.42 | 0.749 | 0.0879 | 0.0680 | 0.6187 | 0.2617 | 0.1886 | 0.710 |
| $a+bx/\sqrt{y}+cy/x^2$ | 143.96 | 109.53 | 0.748 | 0.0880 | 0.0681 | 0.6178 | 0.2620 | 0.1891 | 0.709 |
| $a+bx/\sqrt{y}+cy^2/x^2$ | 142.95 | 109.61 | 0.751 | 0.0881 | 0.0681 | 0.6166 | 0.2622 | 0.1899 | 0.709 |
| $a+bx/\sqrt{y}+c\sqrt{y}/x^2$ | 143.89 | 109.55 | 0.748 | 0.0879 | 0.0680 | 0.6183 | 0.2618 | 0.1889 | 0.710 |
| $a+bx/\sqrt{y}+c/\sqrt{x}y$ | 148.72 | 118.08 | 0.731 | 0.0856 | 0.0637 | 0.6378 | 0.2607 | 0.1800 | 0.712 |
| $a+bx/\sqrt{y}+c/\sqrt{x}y^2$ | 144.74 | 115.80 | 0.745 | 0.0847 | 0.0626 | 0.6454 | 0.2574 | 0.1754 | 0.719 |
| $a+bx/\sqrt{y}+c/\sqrt{x}\sqrt{y}$ | 150.25 | 117.80 | 0.725 | 0.0862 | 0.0646 | 0.6327 | 0.2622 | 0.1817 | 0.709 |
| $a+bx/\sqrt{y}+cy/\sqrt{x}$ | 157.39 | 123.01 | 0.699 | 0.0900 | 0.0687 | 0.5998 | 0.2754 | 0.1933 | 0.679 |
| $a+bx/\sqrt{y}+cy^2/\sqrt{x}$ | 163.93 | 125.16 | 0.673 | 0.0898 | 0.0686 | 0.6015 | 0.2795 | 0.1947 | 0.669 |
| $a+bx/\sqrt{y}+c\sqrt{y}/\sqrt{x}$ | 129.17 | 102.35 | 0.797 | 0.0851 | 0.0644 | 0.6422 | 0.2530 | 0.1791 | 0.729 |
| $a+bxy+cxy^2$ | 138.73 | 110.67 | 0.766 | 0.0828 | 0.0575 | 0.6615 | 0.2616 | 0.1714 | 0.710 |
| $a+bxy+cx\sqrt{y}$ | 137.99 | 109.21 | 0.768 | 0.0820 | 0.0575 | 0.6678 | 0.2578 | 0.1698 | 0.718 |
| $a+bxy+cx^2/y$ | 131.48 | 100.83 | 0.790 | 0.0787 | 0.0547 | 0.6945 | 0.2464 | 0.1697 | 0.743 |
| $a+bxy+cx^2/y^2$ | 134.11 | 103.23 | 0.781 | 0.0799 | 0.0560 | 0.6849 | 0.2523 | 0.1717 | 0.730 |
| $a+bxy+cx^2/\sqrt{y}$ | 129.22 | 100.57 | 0.797 | 0.0776 | 0.0542 | 0.7028 | 0.2447 | 0.1734 | 0.746 |
| $a+bxy+cx^2y$ | 137.50 | 107.93 | 0.770 | 0.0841 | 0.0592 | 0.6509 | 0.2784 | 0.1900 | 0.672 |
| $a+bxy+cx^2y^2$ | 139.28 | 110.14 | 0.764 | 0.0843 | 0.0567 | 0.6488 | 0.2735 | 0.1809 | 0.683 |
| $a+bxy+cx^2\sqrt{y}$ | 131.68 | 104.63 | 0.789 | 0.0812 | 0.0594 | 0.6748 | 0.2734 | 0.1997 | 0.683 |
| $a+bxy+c\sqrt{x}/y$ | 139.07 | 109.62 | 0.765 | 0.0813 | 0.0594 | 0.6734 | 0.2707 | 0.1941 | 0.689 |
| $a+bxy+c\sqrt{x}/y^2$ | 139.41 | 110.72 | 0.764 | 0.0843 | 0.0581 | 0.6489 | 0.2774 | 0.1859 | 0.674 |
| $a+bxy+c\sqrt{x}/\sqrt{y}$ | 139.25 | 110.49 | 0.764 | 0.0821 | 0.0577 | 0.6673 | 0.2643 | 0.1827 | 0.704 |
| $a+bxy+c\sqrt{x}y$ | 134.86 | 105.25 | 0.779 | 0.0834 | 0.0597 | 0.6567 | 0.2784 | 0.1951 | 0.672 |
| $a+bxy+c\sqrt{x}y^2$ | 132.65 | 102.24 | 0.786 | 0.0779 | 0.0538 | 0.7001 | 0.2419 | 0.1625 | 0.752 |
| $a+bxy+c\sqrt{x}\sqrt{y}$ | 138.96 | 109.63 | 0.765 | 0.0843 | 0.0571 | 0.6489 | 0.2741 | 0.1836 | 0.682 |
| $a+bxy+c/xy$ | 134.34 | 102.25 | 0.780 | 0.0844 | 0.0572 | 0.6482 | 0.2782 | 0.1920 | 0.672 |
| $a+bxy+c/xy^2$ | 134.17 | 102.00 | 0.781 | 0.0844 | 0.0572 | 0.6482 | 0.2782 | 0.1920 | 0.672 |
| $a+bxy+c/x\sqrt{y}$ | 134.43 | 102.41 | 0.780 | 0.0844 | 0.0572 | 0.6483 | 0.2781 | 0.1920 | 0.672 |
| $a+bxy+cy/x$ | 136.23 | 105.70 | 0.774 | 0.0841 | 0.0581 | 0.6510 | 0.2766 | 0.1916 | 0.676 |
| $a+bxy+cy^2/x$ | 138.26 | 108.50 | 0.767 | 0.0792 | 0.0575 | 0.6900 | 0.2614 | 0.1870 | 0.711 |
| $a+bxy+c\sqrt{y}/x$ | 135.03 | 103.53 | 0.778 | 0.0843 | 0.0576 | 0.6488 | 0.2777 | 0.1919 | 0.673 |
| $a+bxy+c/x^2y$ | 132.19 | 99.16 | 0.787 | 0.0844 | 0.0572 | 0.6482 | 0.2786 | 0.1922 | 0.671 |
| $a+bxy+c/x^2y^2$ | 132.12 | 99.05 | 0.788 | 0.0844 | 0.0572 | 0.6482 | 0.2786 | 0.1922 | 0.671 |
| $a+bxy+c/x^2\sqrt{y}$ | 132.24 | 99.22 | 0.787 | 0.0844 | 0.0572 | 0.6482 | 0.2786 | 0.1923 | 0.671 |
| $a+bxy+cy/x^2$ | 132.52 | 99.68 | 0.786 | 0.0844 | 0.0573 | 0.6482 | 0.2785 | 0.1924 | 0.671 |
| $a+bxy+cy^2/x^2$ | 133.35 | 101.09 | 0.784 | 0.0844 | 0.0576 | 0.6487 | 0.2783 | 0.1927 | 0.672 |
| $a+bxy+c\sqrt{y}/x^2$ | 132.38 | 99.44 | 0.787 | 0.0844 | 0.0572 | 0.6482 | 0.2786 | 0.1923 | 0.671 |
| $a+bxy+c/\sqrt{x}y$ | 136.28 | 105.17 | 0.774 | 0.0844 | 0.0572 | 0.6483 | 0.2774 | 0.1903 | 0.674 |
| $a+bxy+c/\sqrt{x}y^2$ | 136.20 | 105.06 | 0.774 | 0.0844 | 0.0572 | 0.6483 | 0.2775 | 0.1905 | 0.674 |
| $a+bxy+c/\sqrt{x}\sqrt{y}$ | 136.31 | 105.25 | 0.774 | 0.0844 | 0.0572 | 0.6484 | 0.2773 | 0.1903 | 0.674 |
| $a+bxy+cy/\sqrt{x}$ | 138.54 | 108.77 | 0.766 | 0.0799 | 0.0581 | 0.6847 | 0.2645 | 0.1901 | 0.703 |
| $a+bxy+cy^2/\sqrt{x}$ | 128.98 | 99.66 | 0.798 | 0.0769 | 0.0539 | 0.7078 | 0.2554 | 0.1820 | 0.724 |
| $a+bxy+c\sqrt{y}/\sqrt{x}$ | 137.99 | 108.57 | 0.768 | 0.0837 | 0.0582 | 0.6542 | 0.2741 | 0.1890 | 0.682 |
| $a+bxy^2+cx\sqrt{y}$ | 137.63 | 108.69 | 0.770 | 0.0821 | 0.0572 | 0.6673 | 0.2586 | 0.1700 | 0.717 |
| $a+bxy^2+cx^2/y$ | 128.22 | 98.51 | 0.800 | 0.0781 | 0.0546 | 0.6991 | 0.2467 | 0.1739 | 0.742 |
| $a+bxy^2+cx^2/y^2$ | 132.07 | 100.94 | 0.788 | 0.0798 | 0.0565 | 0.6857 | 0.2568 | 0.1827 | 0.721 |
| $a+bxy^2+cx^2/\sqrt{y}$ | 127.37 | 98.75 | 0.803 | 0.0774 | 0.0538 | 0.7041 | 0.2447 | 0.1735 | 0.746 |
| $a+bxy^2+cx^2y$ | 135.76 | 108.84 | 0.776 | 0.0814 | 0.0617 | 0.6725 | 0.2799 | 0.2132 | 0.668 |
| $a+bxy^2+cx^2y^2$ | 151.40 | 116.22 | 0.721 | 0.0911 | 0.0662 | 0.5906 | 0.3088 | 0.2194 | 0.596 |
| $a+bxy^2+cx^2\sqrt{y}$ | 127.87 | 101.12 | 0.801 | 0.0770 | 0.0558 | 0.7076 | 0.2520 | 0.1892 | 0.731 |
| $a+bxy^2+c\sqrt{x}/y$ | 150.78 | 116.33 | 0.723 | 0.0880 | 0.0658 | 0.6177 | 0.3055 | 0.2197 | 0.605 |
| $a+bxy^2+c\sqrt{x}/y^2$ | 147.24 | 114.59 | 0.736 | 0.0898 | 0.0630 | 0.6015 | 0.2974 | 0.1979 | 0.625 |
| $a+bxy^2+c\sqrt{x}/\sqrt{y}$ | 144.05 | 109.94 | 0.748 | 0.0829 | 0.0611 | 0.6603 | 0.2723 | 0.1946 | 0.686 |
| $a+bxy^2+c\sqrt{x}y$ | 147.14 | 116.12 | 0.737 | 0.0878 | 0.0596 | 0.6191 | 0.2866 | 0.1902 | 0.652 |
| $a+bxy^2+c\sqrt{x}y^2$ | 151.22 | 116.37 | 0.722 | 0.0910 | 0.0675 | 0.5908 | 0.3113 | 0.2256 | 0.589 |
| $a+bxy^2+c\sqrt{x}\sqrt{y}$ | 145.02 | 114.56 | 0.744 | 0.0861 | 0.0598 | 0.6340 | 0.2782 | 0.1831 | 0.672 |
| $a+bxy^2+c/xy$ | 151.44 | 116.30 | 0.721 | 0.0893 | 0.0637 | 0.6065 | 0.3024 | 0.2123 | 0.613 |
| $a+bxy^2+c/xy^2$ | 151.43 | 116.13 | 0.721 | 0.0894 | 0.0637 | 0.6058 | 0.3029 | 0.2127 | 0.611 |
| $a+bxy^2+c/x\sqrt{y}$ | 151.44 | 116.39 | 0.721 | 0.0892 | 0.0637 | 0.6072 | 0.3020 | 0.2120 | 0.614 |

(continued on next page)

**Table 4 – continued from previous page**

| Functional form | $T_{eff}$ (K) | | | Radius ($R_\odot$) | | | log ($L/L_\odot$) | | |
|---|---|---|---|---|---|---|---|---|---|
| | RMSE | MAD | $R^2_{ap}$ | RMSE | MAD | $R^2_{ap}$ | RMSE | MAD | $R^2_{ap}$ |
| $a+bxy^2+cy/x$ | 151.31 | 116.86 | 0.721 | 0.0880 | 0.0641 | 0.6178 | 0.2980 | 0.2107 | 0.624 |
| $a+bxy^2+cy^2/x$ | 148.28 | 115.01 | 0.732 | 0.0843 | 0.0630 | 0.6494 | 0.2922 | 0.2068 | 0.638 |
| $a+bxy^2+c\sqrt{y}/x$ | 151.42 | 116.64 | 0.721 | 0.0887 | 0.0638 | 0.6111 | 0.3003 | 0.2115 | 0.618 |
| $a+bxy^2+c/x^2y$ | 150.88 | 114.09 | 0.723 | 0.0898 | 0.0641 | 0.6016 | 0.3066 | 0.2163 | 0.602 |
| $a+bxy^2+c/x^2y^2$ | 150.84 | 114.00 | 0.723 | 0.0898 | 0.0641 | 0.6015 | 0.3067 | 0.2164 | 0.601 |
| $a+bxy^2+c/x^2\sqrt{y}$ | 150.90 | 114.15 | 0.723 | 0.0898 | 0.0641 | 0.6018 | 0.3065 | 0.2163 | 0.602 |
| $a+bxy^2+cy/x^2$ | 151.00 | 114.40 | 0.723 | 0.0897 | 0.0641 | 0.6027 | 0.3060 | 0.2161 | 0.603 |
| $a+bxy^2+cy^2/x^2$ | 151.17 | 114.98 | 0.722 | 0.0894 | 0.0643 | 0.6056 | 0.3049 | 0.2159 | 0.606 |
| $a+bxy^2+c\sqrt{y}/x^2$ | 150.96 | 114.29 | 0.723 | 0.0898 | 0.0641 | 0.6022 | 0.3063 | 0.2162 | 0.603 |
| $a+bxy^2+c/\sqrt{x}y$ | 151.00 | 117.18 | 0.723 | 0.0888 | 0.0629 | 0.6108 | 0.2978 | 0.2066 | 0.624 |
| $a+bxy^2+c/\sqrt{x}y^2$ | 151.12 | 117.17 | 0.722 | 0.0889 | 0.0630 | 0.6095 | 0.2988 | 0.2073 | 0.622 |
| $a+bxy^2+c/\sqrt{x}\sqrt{y}$ | 150.94 | 117.16 | 0.723 | 0.0886 | 0.0630 | 0.6122 | 0.2970 | 0.2063 | 0.626 |
| $a+bxy^2+cy/\sqrt{x}$ | 149.23 | 115.61 | 0.729 | 0.0856 | 0.0639 | 0.6385 | 0.2971 | 0.2104 | 0.626 |
| $a+bxy^2+cy^2/\sqrt{x}$ | 149.06 | 114.53 | 0.730 | 0.0894 | 0.0680 | 0.6053 | 0.3101 | 0.2308 | 0.593 |
| $a+bxy^2+c\sqrt{y}/\sqrt{x}$ | 150.35 | 116.68 | 0.725 | 0.0867 | 0.0635 | 0.6292 | 0.2913 | 0.2056 | 0.640 |
| $a+bx\sqrt{y}+cx^2/y$ | 136.42 | 103.69 | 0.774 | 0.0797 | 0.0563 | 0.6867 | 0.2475 | 0.1665 | 0.740 |
| $a+bx\sqrt{y}+cx^2/y^2$ | 138.45 | 106.95 | 0.767 | 0.0809 | 0.0573 | 0.6765 | 0.2530 | 0.1669 | 0.729 |
| $a+bx\sqrt{y}+cx^2/\sqrt{y}$ | 131.68 | 104.89 | 0.789 | 0.0777 | 0.0547 | 0.7016 | 0.2446 | 0.1727 | 0.746 |
| $a+bx\sqrt{y}+cx^2y$ | 133.85 | 104.91 | 0.782 | 0.0815 | 0.0560 | 0.6723 | 0.2625 | 0.1743 | 0.708 |
| $a+bx\sqrt{y}+cx^2y^2$ | 135.43 | 106.03 | 0.777 | 0.0819 | 0.0567 | 0.6688 | 0.2618 | 0.1718 | 0.710 |
| $a+bx\sqrt{y}+cx^2\sqrt{y}$ | 131.04 | 102.38 | 0.791 | 0.0805 | 0.0554 | 0.6803 | 0.2620 | 0.1771 | 0.709 |
| $a+bx\sqrt{y}+c\sqrt{x}/y$ | 138.66 | 108.95 | 0.766 | 0.0806 | 0.0565 | 0.6790 | 0.2586 | 0.1785 | 0.717 |
| $a+bx\sqrt{y}+c\sqrt{x}/y^2$ | 136.99 | 106.00 | 0.772 | 0.0806 | 0.0565 | 0.6790 | 0.2621 | 0.1775 | 0.709 |
| $a+bx\sqrt{y}+c\sqrt{x}/\sqrt{y}$ | 136.46 | 109.10 | 0.773 | 0.0820 | 0.0574 | 0.6684 | 0.2601 | 0.1749 | 0.713 |
| $a+bx\sqrt{y}+c\sqrt{x}y$ | 131.44 | 103.92 | 0.790 | 0.0769 | 0.0537 | 0.7081 | 0.2414 | 0.1689 | 0.753 |
| $a+bx\sqrt{y}+c\sqrt{x}y^2$ | 138.79 | 108.35 | 0.766 | 0.0813 | 0.0579 | 0.6738 | 0.2525 | 0.1668 | 0.730 |
| $a+bx\sqrt{y}+c\sqrt{x}\sqrt{y}$ | 126.58 | 96.92 | 0.805 | 0.0796 | 0.0551 | 0.6871 | 0.2595 | 0.1777 | 0.715 |
| $a+bx\sqrt{y}+c/xy$ | 122.79 | 91.89 | 0.817 | 0.0814 | 0.0555 | 0.6729 | 0.2609 | 0.1730 | 0.712 |
| $a+bx\sqrt{y}+c/xy^2$ | 122.68 | 91.67 | 0.817 | 0.0814 | 0.0555 | 0.6729 | 0.2609 | 0.1729 | 0.712 |
| $a+bx\sqrt{y}+c/x\sqrt{y}$ | 122.87 | 92.02 | 0.816 | 0.0814 | 0.0555 | 0.6728 | 0.2610 | 0.1731 | 0.711 |
| $a+bx\sqrt{y}+cy/x$ | 126.47 | 96.65 | 0.805 | 0.0820 | 0.0564 | 0.6682 | 0.2623 | 0.1737 | 0.708 |
| $a+bx\sqrt{y}+cy^2/x$ | 138.75 | 108.64 | 0.766 | 0.0798 | 0.0561 | 0.6852 | 0.2542 | 0.1744 | 0.726 |
| $a+bx\sqrt{y}+c\sqrt{y}/x$ | 123.86 | 93.11 | 0.813 | 0.0816 | 0.0555 | 0.6709 | 0.2615 | 0.1731 | 0.710 |
| $a+bx\sqrt{y}+c/x^2y$ | 121.24 | 88.89 | 0.821 | 0.0816 | 0.0557 | 0.6716 | 0.2604 | 0.1706 | 0.713 |
| $a+bx\sqrt{y}+c/x^2y^2$ | 121.20 | 88.80 | 0.821 | 0.0816 | 0.0557 | 0.6716 | 0.2604 | 0.1706 | 0.713 |
| $a+bx\sqrt{y}+c/x^2\sqrt{y}$ | 121.27 | 88.95 | 0.821 | 0.0816 | 0.0557 | 0.6716 | 0.2605 | 0.1707 | 0.713 |
| $a+bx\sqrt{y}+cy/x^2$ | 121.60 | 89.38 | 0.820 | 0.0816 | 0.0557 | 0.6713 | 0.2606 | 0.1709 | 0.712 |
| $a+bx\sqrt{y}+cy^2/x^2$ | 122.91 | 91.08 | 0.816 | 0.0818 | 0.0559 | 0.6698 | 0.2612 | 0.1715 | 0.711 |
| $a+bx\sqrt{y}+c\sqrt{y}/x^2$ | 121.41 | 89.15 | 0.821 | 0.0816 | 0.0557 | 0.6715 | 0.2605 | 0.1708 | 0.712 |
| $a+bx\sqrt{y}+c/\sqrt{x}y$ | 125.25 | 95.43 | 0.809 | 0.0812 | 0.0552 | 0.6743 | 0.2614 | 0.1748 | 0.711 |
| $a+bx\sqrt{y}+c/\sqrt{x}y^2$ | 125.39 | 95.45 | 0.809 | 0.0812 | 0.0551 | 0.6741 | 0.2614 | 0.1747 | 0.711 |
| $a+bx\sqrt{y}+c/\sqrt{x}\sqrt{y}$ | 125.09 | 95.32 | 0.810 | 0.0813 | 0.0553 | 0.6740 | 0.2614 | 0.1747 | 0.710 |
| $a+bx\sqrt{y}+cy/\sqrt{x}$ | 138.73 | 108.73 | 0.766 | 0.0801 | 0.0561 | 0.6832 | 0.2557 | 0.1760 | 0.723 |
| $a+bx\sqrt{y}+cy^2/\sqrt{x}$ | 134.34 | 102.70 | 0.780 | 0.0770 | 0.0537 | 0.7072 | 0.2419 | 0.1663 | 0.752 |
| $a+bx\sqrt{y}+c\sqrt{y}/\sqrt{x}$ | 129.58 | 101.14 | 0.796 | 0.0821 | 0.0568 | 0.6673 | 0.2625 | 0.1751 | 0.708 |
| $a+bx^2/y+cx^2/y^2$ | 125.48 | 97.53 | 0.808 | 0.0772 | 0.0525 | 0.7054 | 0.2416 | 0.1654 | 0.753 |
| $a+bx^2/y+cx^2/\sqrt{y}$ | 126.78 | 98.87 | 0.804 | 0.0772 | 0.0530 | 0.7061 | 0.2447 | 0.1735 | 0.746 |
| $a+bx^2/y+cx^2y$ | 127.18 | 99.97 | 0.803 | 0.0774 | 0.0541 | 0.7042 | 0.2466 | 0.1768 | 0.742 |
| $a+bx^2/y+cx^2y^2$ | 127.40 | 101.86 | 0.803 | 0.0777 | 0.0550 | 0.7023 | 0.2476 | 0.1778 | 0.740 |
| $a+bx^2/y+cx^2\sqrt{y}$ | 127.09 | 99.77 | 0.803 | 0.0773 | 0.0536 | 0.7050 | 0.2460 | 0.1760 | 0.744 |
| $a+bx^2/y+c\sqrt{x}/y$ | 132.01 | 105.03 | 0.788 | 0.0816 | 0.0600 | 0.6709 | 0.2471 | 0.1700 | 0.741 |
| $a+bx^2/y+c\sqrt{x}/y^2$ | 156.66 | 121.53 | 0.701 | 0.0850 | 0.0654 | 0.6429 | 0.2607 | 0.1890 | 0.712 |
| $a+bx^2/y+c\sqrt{x}/\sqrt{y}$ | 124.29 | 97.96 | 0.812 | 0.0805 | 0.0588 | 0.6799 | 0.2495 | 0.1748 | 0.736 |
| $a+bx^2/y+c\sqrt{x}y$ | 139.56 | 106.24 | 0.763 | 0.0806 | 0.0582 | 0.6789 | 0.2496 | 0.1683 | 0.736 |
| $a+bx^2/y+c\sqrt{x}y^2$ | 131.22 | 100.35 | 0.790 | 0.0789 | 0.0552 | 0.6924 | 0.2475 | 0.1714 | 0.741 |
| $a+bx^2/y+c\sqrt{x}\sqrt{y}$ | 149.03 | 113.83 | 0.730 | 0.0827 | 0.0620 | 0.6627 | 0.2541 | 0.1759 | 0.726 |
| $a+bx^2/y+c/xy$ | 142.71 | 113.15 | 0.752 | 0.0839 | 0.0616 | 0.6527 | 0.2587 | 0.1816 | 0.716 |
| $a+bx^2/y+c/xy^2$ | 142.18 | 112.60 | 0.754 | 0.0838 | 0.0616 | 0.6532 | 0.2584 | 0.1811 | 0.717 |
| $a+bx^2/y+c/x\sqrt{y}$ | 142.93 | 113.32 | 0.751 | 0.0839 | 0.0617 | 0.6524 | 0.2588 | 0.1818 | 0.716 |
| $a+bx^2/y+cy/x$ | 136.46 | 105.63 | 0.773 | 0.0835 | 0.0618 | 0.6557 | 0.2565 | 0.1781 | 0.721 |
| $a+bx^2/y+cy^2/x$ | 130.61 | 102.67 | 0.792 | 0.0819 | 0.0599 | 0.6688 | 0.2503 | 0.1724 | 0.735 |
| $a+bx^2/y+c\sqrt{y}/x$ | 141.53 | 111.00 | 0.756 | 0.0839 | 0.0619 | 0.6526 | 0.2584 | 0.1806 | 0.717 |
| $a+bx^2/y+c/x^2y$ | 140.66 | 108.37 | 0.759 | 0.0840 | 0.0623 | 0.6512 | 0.2580 | 0.1784 | 0.718 |
| $a+bx^2/y+c/x^2y^2$ | 140.60 | 108.22 | 0.759 | 0.0841 | 0.0623 | 0.6512 | 0.2580 | 0.1783 | 0.718 |
| $a+bx^2/y+c/x^2\sqrt{y}$ | 140.70 | 108.44 | 0.759 | 0.0841 | 0.0623 | 0.6512 | 0.2580 | 0.1785 | 0.718 |
| $a+bx^2/y+cy/x^2$ | 140.66 | 108.29 | 0.759 | 0.0841 | 0.0623 | 0.6511 | 0.2580 | 0.1785 | 0.718 |
| $a+bx^2/y+cy^2/x^2$ | 139.28 | 106.78 | 0.764 | 0.0840 | 0.0624 | 0.6517 | 0.2576 | 0.1788 | 0.719 |
| $a+bx^2/y+c\sqrt{y}/x^2$ | 140.75 | 108.48 | 0.759 | 0.0841 | 0.0623 | 0.6511 | 0.2580 | 0.1785 | 0.718 |
| $a+bx^2/y+c/\sqrt{x}y$ | 147.33 | 119.27 | 0.736 | 0.0840 | 0.0611 | 0.6518 | 0.2603 | 0.1859 | 0.713 |
| $a+bx^2/y+c/\sqrt{x}y^2$ | 145.85 | 117.91 | 0.741 | 0.0838 | 0.0607 | 0.6536 | 0.2596 | 0.1849 | 0.714 |
| $a+bx^2/y+c/\sqrt{x}\sqrt{y}$ | 147.75 | 119.45 | 0.734 | 0.0841 | 0.0615 | 0.6508 | 0.2605 | 0.1862 | 0.712 |
| $a+bx^2/y+cy/\sqrt{x}$ | 130.81 | 103.36 | 0.792 | 0.0818 | 0.0599 | 0.6699 | 0.2491 | 0.1713 | 0.737 |
| $a+bx^2/y+cy^2/\sqrt{x}$ | 141.12 | 108.28 | 0.758 | 0.0818 | 0.0603 | 0.6694 | 0.2523 | 0.1722 | 0.730 |
| $a+bx^2/y+c\sqrt{y}/\sqrt{x}$ | 133.53 | 104.75 | 0.783 | 0.0829 | 0.0612 | 0.6603 | 0.2552 | 0.1783 | 0.724 |
| $a+bx^2/y^2+cx^2/\sqrt{y}$ | 125.97 | 97.90 | 0.807 | 0.0771 | 0.0528 | 0.7065 | 0.2444 | 0.1727 | 0.747 |
| $a+bx^2/y^2+cx^2y$ | 130.14 | 102.91 | 0.794 | 0.0786 | 0.0560 | 0.6951 | 0.2559 | 0.1860 | 0.723 |
| $a+bx^2/y^2+cx^2y^2$ | 134.46 | 108.92 | 0.780 | 0.0805 | 0.0589 | 0.6799 | 0.2648 | 0.1948 | 0.703 |
| $a+bx^2/y^2+cx^2\sqrt{y}$ | 128.41 | 99.94 | 0.799 | 0.0779 | 0.0546 | 0.7007 | 0.2517 | 0.1827 | 0.731 |
| $a+bx^2/y^2+c\sqrt{x}/y$ | 165.68 | 126.78 | 0.666 | 0.0981 | 0.0765 | 0.5244 | 0.2960 | 0.2163 | 0.629 |
| $a+bx^2/y^2+c\sqrt{x}/y^2$ | 214.51 | 159.16 | 0.440 | 0.1111 | 0.0875 | 0.3908 | 0.3465 | 0.2562 | 0.491 |
| $a+bx^2/y^2+c\sqrt{x}/\sqrt{y}$ | 254.68 | 191.33 | 0.211 | 0.1227 | 0.0959 | 0.2561 | 0.4020 | 0.3121 | 0.315 |
| $a+bx^2/y^2+c\sqrt{x}y$ | 146.94 | 112.73 | 0.737 | 0.0840 | 0.0613 | 0.6514 | 0.2622 | 0.1756 | 0.709 |
| $a+bx^2/y^2+c\sqrt{x}y^2$ | 136.22 | 104.10 | 0.774 | 0.0812 | 0.0577 | 0.6742 | 0.2579 | 0.1785 | 0.718 |
| $a+bx^2/y^2+c\sqrt{x}\sqrt{y}$ | 159.43 | 121.01 | 0.691 | 0.0876 | 0.0664 | 0.6212 | 0.2721 | 0.1875 | 0.686 |
| $a+bx^2/y^2+c/xy$ | 254.98 | 191.12 | 0.209 | 0.1236 | 0.0963 | 0.2458 | 0.4046 | 0.3143 | 0.306 |
| $a+bx^2/y^2+c/xy^2$ | 255.02 | 190.39 | 0.209 | 0.1239 | 0.0962 | 0.2420 | 0.4057 | 0.3149 | 0.303 |
| $a+bx^2/y^2+c/x\sqrt{y}$ | 254.87 | 191.45 | 0.210 | 0.1233 | 0.0963 | 0.2490 | 0.4037 | 0.3137 | 0.309 |
| $a+bx^2/y^2+cy/x$ | 254.70 | 189.17 | 0.211 | 0.1241 | 0.0965 | 0.2400 | 0.4067 | 0.3158 | 0.299 |
| $a+bx^2/y^2+cy^2/x$ | 157.54 | 123.85 | 0.698 | 0.0972 | 0.0752 | 0.5340 | 0.2969 | 0.2160 | 0.627 |
| $a+bx^2/y^2+c\sqrt{y}/x$ | 254.76 | 191.55 | 0.210 | 0.1230 | 0.0965 | 0.2530 | 0.4030 | 0.3136 | 0.312 |

(continued on next page)

**Table 4 – continued from previous page**

| Functional form | $T_{eff}$ (K) | | | Radius ($R_\odot$) | | | log (L/$L_\odot$) | | |
|---|---|---|---|---|---|---|---|---|---|
| | RMSE | MAD | $R^2_{ap}$ | RMSE | MAD | $R^2_{ap}$ | RMSE | MAD | $R^2_{ap}$ |
| $a+bx^2/y^2+c/x^2y$ | 254.08 | 187.57 | 0.215 | 0.1244 | 0.0965 | 0.2360 | 0.4075 | 0.3153 | 0.296 |
| $a+bx^2/y^2+c/x^2y^2$ | 253.99 | 187.36 | 0.215 | 0.1244 | 0.0964 | 0.2357 | 0.4076 | 0.3152 | 0.296 |
| $a+bx^2/y^2+c/x^2\sqrt{y}$ | 254.14 | 187.70 | 0.214 | 0.1244 | 0.0965 | 0.2362 | 0.4075 | 0.3153 | 0.296 |
| $a+bx^2/y^2+cy/x^2$ | 254.34 | 188.19 | 0.213 | 0.1243 | 0.0965 | 0.2372 | 0.4073 | 0.3156 | 0.297 |
| $a+bx^2/y^2+cy^2/x^2$ | 254.00 | 187.44 | 0.215 | 0.1244 | 0.0965 | 0.2363 | 0.4075 | 0.3153 | 0.296 |
| $a+bx^2/y^2+c\sqrt{y}/x^2$ | 254.28 | 188.04 | 0.213 | 0.1243 | 0.0965 | 0.2368 | 0.4074 | 0.3155 | 0.297 |
| $a+bx^2/y^2+c/\sqrt{x}y$ | 251.40 | 190.29 | 0.231 | 0.1213 | 0.0949 | 0.2735 | 0.3949 | 0.3038 | 0.339 |
| $a+bx^2/y^2+c/\sqrt{x}y^2$ | 253.71 | 191.61 | 0.217 | 0.1228 | 0.0956 | 0.2559 | 0.4004 | 0.3088 | 0.321 |
| $a+bx^2/y^2+c/\sqrt{x}\sqrt{y}$ | 249.53 | 188.73 | 0.242 | 0.1202 | 0.0943 | 0.2871 | 0.3909 | 0.2998 | 0.353 |
| $a+bx^2/y^2+cy/\sqrt{x}$ | 159.02 | 124.60 | 0.692 | 0.0971 | 0.0752 | 0.5346 | 0.2949 | 0.2150 | 0.631 |
| $a+bx^2/y^2+cy^2/\sqrt{x}$ | 160.44 | 121.98 | 0.687 | 0.0905 | 0.0681 | 0.5957 | 0.2818 | 0.1953 | 0.664 |
| $a+bx^2/y^2+c\sqrt{y}/\sqrt{x}$ | 254.96 | 189.98 | 0.209 | 0.1238 | 0.0965 | 0.2437 | 0.4057 | 0.3154 | 0.302 |
| $a+bx^2/\sqrt{y}+cx^2y$ | 126.81 | 99.59 | 0.804 | 0.0772 | 0.0533 | 0.7058 | 0.2447 | 0.1734 | 0.746 |
| $a+bx^2/\sqrt{y}+cx^2y^2$ | 126.53 | 99.38 | 0.805 | 0.0772 | 0.0536 | 0.7057 | 0.2447 | 0.1734 | 0.746 |
| $a+bx^2/\sqrt{y}+cx^2\sqrt{y}$ | 126.91 | 99.61 | 0.804 | 0.0772 | 0.0533 | 0.7058 | 0.2447 | 0.1735 | 0.746 |
| $a+bx^2/\sqrt{y}+c\sqrt{x}/y$ | 124.44 | 93.93 | 0.812 | 0.0776 | 0.0545 | 0.7023 | 0.2436 | 0.1678 | 0.749 |
| $a+bx^2/\sqrt{y}+c\sqrt{x}/y^2$ | 132.74 | 108.59 | 0.786 | 0.0777 | 0.0544 | 0.7022 | 0.2439 | 0.1682 | 0.748 |
| $a+bx^2/\sqrt{y}+c\sqrt{x}/\sqrt{y}$ | 120.56 | 93.14 | 0.823 | 0.0773 | 0.0535 | 0.7053 | 0.2444 | 0.1729 | 0.747 |
| $a+bx^2/\sqrt{y}+c\sqrt{x}y$ | 131.75 | 105.16 | 0.789 | 0.0778 | 0.0548 | 0.7014 | 0.2447 | 0.1733 | 0.746 |
| $a+bx^2/\sqrt{y}+c\sqrt{x}y^2$ | 128.71 | 99.97 | 0.798 | 0.0776 | 0.0542 | 0.7027 | 0.2447 | 0.1736 | 0.746 |
| $a+bx^2/\sqrt{y}+c\sqrt{x}\sqrt{y}$ | 132.73 | 109.64 | 0.786 | 0.0777 | 0.0548 | 0.7018 | 0.2447 | 0.1730 | 0.746 |
| $a+bx^2/\sqrt{y}+c/xy$ | 120.91 | 96.21 | 0.822 | 0.0774 | 0.0540 | 0.7043 | 0.2440 | 0.1726 | 0.748 |
| $a+bx^2/\sqrt{y}+c/xy^2$ | 120.73 | 95.94 | 0.823 | 0.0774 | 0.0540 | 0.7044 | 0.2439 | 0.1725 | 0.748 |
| $a+bx^2/\sqrt{y}+c/x\sqrt{y}$ | 120.90 | 96.20 | 0.822 | 0.0774 | 0.0540 | 0.7043 | 0.2440 | 0.1726 | 0.748 |
| $a+bx^2/\sqrt{y}+cy/x$ | 118.40 | 91.96 | 0.829 | 0.0774 | 0.0540 | 0.7039 | 0.2439 | 0.1717 | 0.748 |
| $a+bx^2/\sqrt{y}+cy^2/x$ | 125.12 | 95.55 | 0.810 | 0.0778 | 0.0548 | 0.7015 | 0.2446 | 0.1727 | 0.746 |
| $a+bx^2/\sqrt{y}+c\sqrt{y}/x$ | 120.00 | 94.79 | 0.825 | 0.0774 | 0.0541 | 0.7042 | 0.2439 | 0.1723 | 0.748 |
| $a+bx^2/\sqrt{y}+c/x^2y$ | 118.76 | 92.72 | 0.828 | 0.0775 | 0.0540 | 0.7037 | 0.2435 | 0.1708 | 0.749 |
| $a+bx^2/\sqrt{y}+c/x^2y^2$ | 118.71 | 92.63 | 0.829 | 0.0775 | 0.0540 | 0.7037 | 0.2435 | 0.1707 | 0.749 |
| $a+bx^2/\sqrt{y}+c/x^2\sqrt{y}$ | 118.78 | 92.77 | 0.828 | 0.0775 | 0.0540 | 0.7037 | 0.2435 | 0.1708 | 0.749 |
| $a+bx^2/\sqrt{y}+cy/x^2$ | 118.75 | 92.69 | 0.828 | 0.0775 | 0.0540 | 0.7037 | 0.2435 | 0.1709 | 0.749 |
| $a+bx^2/\sqrt{y}+cy^2/x^2$ | 118.28 | 91.95 | 0.830 | 0.0775 | 0.0540 | 0.7035 | 0.2436 | 0.1708 | 0.749 |
| $a+bx^2/\sqrt{y}+c\sqrt{y}/x^2$ | 118.80 | 92.78 | 0.828 | 0.0775 | 0.0540 | 0.7037 | 0.2435 | 0.1709 | 0.749 |
| $a+bx^2/\sqrt{y}+c/\sqrt{x}y$ | 124.07 | 100.42 | 0.813 | 0.0773 | 0.0538 | 0.7046 | 0.2444 | 0.1738 | 0.747 |
| $a+bx^2/\sqrt{y}+c/\sqrt{x}y^2$ | 123.76 | 99.86 | 0.814 | 0.0773 | 0.0537 | 0.7047 | 0.2444 | 0.1737 | 0.747 |
| $a+bx^2/\sqrt{y}+c/\sqrt{x}\sqrt{y}$ | 123.87 | 100.20 | 0.813 | 0.0773 | 0.0538 | 0.7046 | 0.2444 | 0.1738 | 0.747 |
| $a+bx^2/\sqrt{y}+cy/\sqrt{x}$ | 124.86 | 94.95 | 0.810 | 0.0777 | 0.0547 | 0.7017 | 0.2444 | 0.1715 | 0.747 |
| $a+bx^2/\sqrt{y}+cy^2/\sqrt{x}$ | 131.14 | 104.08 | 0.791 | 0.0778 | 0.0549 | 0.7014 | 0.2447 | 0.1739 | 0.746 |
| $a+bx^2/\sqrt{y}+c\sqrt{y}/\sqrt{x}$ | 118.64 | 91.94 | 0.829 | 0.0774 | 0.0540 | 0.7042 | 0.2441 | 0.1722 | 0.748 |
| $a+bx^2y+cx^2y^2$ | 130.52 | 102.69 | 0.793 | 0.0785 | 0.0519 | 0.6955 | 0.2517 | 0.1710 | 0.732 |
| $a+bx^2y+cx^2\sqrt{y}$ | 127.56 | 98.80 | 0.802 | 0.0774 | 0.0524 | 0.7043 | 0.2450 | 0.1690 | 0.746 |
| $a+bx^2y+c\sqrt{x}/y$ | 140.12 | 110.97 | 0.761 | 0.0841 | 0.0632 | 0.6508 | 0.2910 | 0.2135 | 0.641 |
| $a+bx^2y+c\sqrt{x}/y^2$ | 134.93 | 106.74 | 0.778 | 0.0841 | 0.0597 | 0.6505 | 0.2779 | 0.1878 | 0.673 |
| $a+bx^2y+c\sqrt{x}/\sqrt{y}$ | 136.47 | 108.18 | 0.773 | 0.0798 | 0.0585 | 0.6854 | 0.2633 | 0.1889 | 0.706 |
| $a+bx^2y+c\sqrt{x}y$ | 138.53 | 109.42 | 0.767 | 0.0845 | 0.0603 | 0.6472 | 0.2819 | 0.1942 | 0.663 |
| $a+bx^2y+c\sqrt{x}y^2$ | 139.22 | 111.23 | 0.764 | 0.0844 | 0.0642 | 0.6482 | 0.2918 | 0.2194 | 0.639 |
| $a+bx^2y+c\sqrt{x}\sqrt{y}$ | 136.50 | 107.57 | 0.773 | 0.0828 | 0.0573 | 0.6617 | 0.2709 | 0.1839 | 0.689 |
| $a+bx^2y+c/xy$ | 140.15 | 111.02 | 0.761 | 0.0837 | 0.0609 | 0.6539 | 0.2837 | 0.2021 | 0.659 |
| $a+bx^2y+c/xy^2$ | 140.14 | 110.91 | 0.761 | 0.0838 | 0.0609 | 0.6534 | 0.2842 | 0.2025 | 0.658 |
| $a+bx^2y+c/x\sqrt{y}$ | 140.16 | 111.07 | 0.761 | 0.0837 | 0.0609 | 0.6543 | 0.2835 | 0.2020 | 0.660 |
| $a+bx^2y+cy/x$ | 140.16 | 111.19 | 0.761 | 0.0830 | 0.0613 | 0.6603 | 0.2814 | 0.2014 | 0.664 |
| $a+bx^2y+cy^2/x$ | 139.74 | 111.35 | 0.762 | 0.0818 | 0.0602 | 0.6700 | 0.2829 | 0.2044 | 0.661 |
| $a+bx^2y+c\sqrt{y}/x$ | 140.16 | 111.13 | 0.761 | 0.0834 | 0.0610 | 0.6564 | 0.2826 | 0.2015 | 0.662 |
| $a+bx^2y+c/x^2y$ | 139.54 | 109.12 | 0.763 | 0.0842 | 0.0614 | 0.6496 | 0.2879 | 0.2060 | 0.649 |
| $a+bx^2y+c/x^2y^2$ | 139.51 | 109.03 | 0.763 | 0.0843 | 0.0614 | 0.6495 | 0.2880 | 0.2061 | 0.649 |
| $a+bx^2y+c/x^2\sqrt{y}$ | 139.56 | 109.17 | 0.763 | 0.0842 | 0.0614 | 0.6497 | 0.2878 | 0.2059 | 0.649 |
| $a+bx^2y+cy/x^2$ | 139.63 | 109.36 | 0.763 | 0.0842 | 0.0614 | 0.6503 | 0.2875 | 0.2058 | 0.650 |
| $a+bx^2y+cy^2/x^2$ | 139.73 | 109.61 | 0.762 | 0.0839 | 0.0615 | 0.6521 | 0.2867 | 0.2055 | 0.652 |
| $a+bx^2y+c\sqrt{y}/x^2$ | 139.61 | 109.28 | 0.763 | 0.0842 | 0.0614 | 0.6500 | 0.2876 | 0.2058 | 0.650 |
| $a+bx^2y+c/\sqrt{x}y$ | 139.75 | 111.53 | 0.762 | 0.0833 | 0.0600 | 0.6574 | 0.2794 | 0.1966 | 0.669 |
| $a+bx^2y+c/\sqrt{x}y^2$ | 139.83 | 111.59 | 0.762 | 0.0834 | 0.0601 | 0.6567 | 0.2801 | 0.1973 | 0.668 |
| $a+bx^2y+c/\sqrt{x}\sqrt{y}$ | 139.73 | 111.49 | 0.762 | 0.0832 | 0.0600 | 0.6580 | 0.2790 | 0.1965 | 0.670 |
| $a+bx^2y+cy/\sqrt{x}$ | 140.01 | 111.31 | 0.762 | 0.0826 | 0.0614 | 0.6631 | 0.2861 | 0.2079 | 0.653 |
| $a+bx^2y+cy^2/\sqrt{x}$ | 139.76 | 111.02 | 0.762 | 0.0847 | 0.0642 | 0.6455 | 0.2927 | 0.2193 | 0.637 |
| $a+bx^2y+c\sqrt{y}/\sqrt{x}$ | 139.80 | 111.45 | 0.762 | 0.0821 | 0.0607 | 0.6675 | 0.2764 | 0.1988 | 0.676 |
| $a+bx^2y^2+cx^2\sqrt{y}$ | 128.46 | 99.95 | 0.799 | 0.0778 | 0.0518 | 0.7014 | 0.2475 | 0.1700 | 0.740 |
| $a+bx^2y^2+c\sqrt{x}/y$ | 156.94 | 121.91 | 0.700 | 0.0924 | 0.0716 | 0.5787 | 0.3247 | 0.2399 | 0.553 |
| $a+bx^2y^2+c\sqrt{x}/y^2$ | 144.07 | 113.75 | 0.747 | 0.0891 | 0.0641 | 0.6079 | 0.2954 | 0.1980 | 0.630 |
| $a+bx^2y^2+c\sqrt{x}/\sqrt{y}$ | 144.81 | 116.39 | 0.745 | 0.0824 | 0.0630 | 0.6647 | 0.2749 | 0.2003 | 0.680 |
| $a+bx^2y^2+c\sqrt{x}y$ | 144.51 | 113.10 | 0.746 | 0.0869 | 0.0599 | 0.6269 | 0.2863 | 0.1927 | 0.653 |
| $a+bx^2y^2+c\sqrt{x}y^2$ | 152.65 | 118.04 | 0.716 | 0.0916 | 0.0673 | 0.5854 | 0.3119 | 0.2227 | 0.588 |
| $a+bx^2y^2+c\sqrt{x}\sqrt{y}$ | 141.53 | 110.79 | 0.756 | 0.0847 | 0.0591 | 0.6461 | 0.2755 | 0.1848 | 0.678 |
| $a+bx^2y^2+c/xy$ | 155.60 | 124.00 | 0.705 | 0.0891 | 0.0663 | 0.6079 | 0.3063 | 0.2158 | 0.602 |
| $a+bx^2y^2+c/xy^2$ | 155.81 | 124.06 | 0.705 | 0.0893 | 0.0664 | 0.6064 | 0.3073 | 0.2165 | 0.600 |
| $a+bx^2y^2+c/x\sqrt{y}$ | 155.48 | 123.94 | 0.706 | 0.0890 | 0.0662 | 0.6089 | 0.3057 | 0.2155 | 0.604 |
| $a+bx^2y^2+cy/x$ | 155.22 | 123.74 | 0.707 | 0.0879 | 0.0667 | 0.6185 | 0.3028 | 0.2155 | 0.612 |
| $a+bx^2y^2+cy^2/x$ | 156.54 | 123.11 | 0.702 | 0.0898 | 0.0689 | 0.6017 | 0.3172 | 0.2314 | 0.574 |
| $a+bx^2y^2+c\sqrt{y}/x$ | 155.27 | 123.78 | 0.707 | 0.0885 | 0.0664 | 0.6133 | 0.3041 | 0.2147 | 0.608 |
| $a+bx^2y^2+c/x^2y$ | 156.96 | 123.25 | 0.700 | 0.0903 | 0.0672 | 0.5971 | 0.3138 | 0.2217 | 0.583 |
| $a+bx^2y^2+c/x^2y^2$ | 156.97 | 123.19 | 0.700 | 0.0904 | 0.0672 | 0.5967 | 0.3141 | 0.2218 | 0.582 |
| $a+bx^2y^2+c/x^2\sqrt{y}$ | 156.94 | 123.28 | 0.700 | 0.0903 | 0.0672 | 0.5974 | 0.3137 | 0.2216 | 0.583 |
| $a+bx^2y^2+cy/x^2$ | 156.89 | 123.39 | 0.701 | 0.0901 | 0.0672 | 0.5987 | 0.3130 | 0.2213 | 0.585 |
| $a+bx^2y^2+cy^2/x^2$ | 156.81 | 123.51 | 0.701 | 0.0898 | 0.0673 | 0.6019 | 0.3119 | 0.2207 | 0.588 |
| $a+bx^2y^2+c\sqrt{y}/x^2$ | 156.91 | 123.36 | 0.700 | 0.0902 | 0.0672 | 0.5981 | 0.3133 | 0.2214 | 0.584 |
| $a+bx^2y^2+c/\sqrt{x}y$ | 152.89 | 122.61 | 0.716 | 0.0880 | 0.0648 | 0.6173 | 0.2986 | 0.2082 | 0.622 |
| $a+bx^2y^2+c/\sqrt{x}y^2$ | 153.41 | 123.12 | 0.714 | 0.0883 | 0.0651 | 0.6147 | 0.3003 | 0.2092 | 0.618 |
| $a+bx^2y^2+c/\sqrt{x}\sqrt{y}$ | 152.67 | 122.33 | 0.716 | 0.0878 | 0.0648 | 0.6194 | 0.2975 | 0.2078 | 0.625 |
| $a+bx^2y^2+cy/\sqrt{x}$ | 156.92 | 122.89 | 0.700 | 0.0908 | 0.0701 | 0.5929 | 0.3204 | 0.2343 | 0.565 |
| $a+bx^2y^2+cy^2/\sqrt{x}$ | 156.28 | 121.26 | 0.703 | 0.0933 | 0.0710 | 0.5705 | 0.3232 | 0.2388 | 0.557 |

(continued on next page)

**Table 4 – continued from previous page**

| Functional form | $T_{eff}$ (K) | | | Radius ($R_\odot$) | | | log ($L/L_\odot$) | | |
|---|---|---|---|---|---|---|---|---|---|
| | RMSE | MAD | $R^2_{ap}$ | RMSE | MAD | $R^2_{ap}$ | RMSE | MAD | $R^2_{ap}$ |
| $a+bx^2y^2+c\sqrt{y}/\sqrt{x}$ | 153.02 | 122.53 | 0.715 | 0.0863 | 0.0661 | 0.6324 | 0.2948 | 0.2123 | 0.632 |
| $a+bx^2\sqrt{y}+c\sqrt{x}/y$ | 131.53 | 104.19 | 0.790 | 0.0802 | 0.0581 | 0.6828 | 0.2717 | 0.1979 | 0.687 |
| $a+bx^2\sqrt{y}+c\sqrt{x}/y^2$ | 129.69 | 101.87 | 0.795 | 0.0809 | 0.0570 | 0.6767 | 0.2654 | 0.1801 | 0.702 |
| $a+bx^2\sqrt{y}+c\sqrt{x}/\sqrt{y}$ | 131.39 | 103.54 | 0.790 | 0.0786 | 0.0561 | 0.6953 | 0.2567 | 0.1837 | 0.721 |
| $a+bx^2\sqrt{y}+c\sqrt{x}y$ | 131.78 | 104.50 | 0.789 | 0.0813 | 0.0589 | 0.6738 | 0.2722 | 0.1949 | 0.686 |
| $a+bx^2\sqrt{y}+c\sqrt{x}y^2$ | 129.22 | 101.61 | 0.797 | 0.0784 | 0.0581 | 0.6963 | 0.2637 | 0.1971 | 0.705 |
| $a+bx^2\sqrt{y}+c\sqrt{x}\sqrt{y}$ | 131.53 | 103.63 | 0.790 | 0.0807 | 0.0562 | 0.6782 | 0.2649 | 0.1820 | 0.703 |
| $a+bx^2\sqrt{y}+c/xy$ | 130.76 | 102.56 | 0.792 | 0.0806 | 0.0573 | 0.6790 | 0.2693 | 0.1922 | 0.693 |
| $a+bx^2\sqrt{y}+c/xy^2$ | 130.67 | 102.38 | 0.792 | 0.0807 | 0.0573 | 0.6788 | 0.2695 | 0.1924 | 0.692 |
| $a+bx^2\sqrt{y}+c/x\sqrt{y}$ | 130.79 | 102.64 | 0.792 | 0.0806 | 0.0573 | 0.6791 | 0.2692 | 0.1921 | 0.693 |
| $a+bx^2\sqrt{y}+cy/x$ | 130.85 | 102.93 | 0.792 | 0.0802 | 0.0577 | 0.6824 | 0.2679 | 0.1928 | 0.696 |
| $a+bx^2\sqrt{y}+cy^2/x$ | 131.77 | 104.41 | 0.789 | 0.0785 | 0.0567 | 0.6959 | 0.2654 | 0.1908 | 0.702 |
| $a+bx^2\sqrt{y}+c\sqrt{y}/x$ | 130.79 | 102.77 | 0.792 | 0.0805 | 0.0575 | 0.6801 | 0.2687 | 0.1922 | 0.694 |
| $a+bx^2\sqrt{y}+c/x^2y$ | 129.15 | 100.02 | 0.797 | 0.0808 | 0.0575 | 0.6775 | 0.2715 | 0.1945 | 0.688 |
| $a+bx^2\sqrt{y}+c/x^2y^2$ | 129.09 | 99.92 | 0.797 | 0.0808 | 0.0575 | 0.6774 | 0.2716 | 0.1945 | 0.688 |
| $a+bx^2\sqrt{y}+c/x^2\sqrt{y}$ | 129.19 | 100.08 | 0.797 | 0.0808 | 0.0575 | 0.6775 | 0.2715 | 0.1945 | 0.688 |
| $a+bx^2\sqrt{y}+cy/x^2$ | 129.29 | 100.30 | 0.797 | 0.0808 | 0.0576 | 0.6778 | 0.2713 | 0.1944 | 0.688 |
| $a+bx^2\sqrt{y}+cy^2/x^2$ | 129.44 | 100.62 | 0.796 | 0.0807 | 0.0577 | 0.6787 | 0.2709 | 0.1943 | 0.689 |
| $a+bx^2\sqrt{y}+c\sqrt{y}/x^2$ | 129.25 | 100.21 | 0.797 | 0.0808 | 0.0576 | 0.6776 | 0.2714 | 0.1944 | 0.688 |
| $a+bx^2\sqrt{y}+c/\sqrt{x}y$ | 131.64 | 104.07 | 0.789 | 0.0805 | 0.0568 | 0.6801 | 0.2668 | 0.1886 | 0.698 |
| $a+bx^2\sqrt{y}+c/\sqrt{x}y^2$ | 131.60 | 103.97 | 0.789 | 0.0805 | 0.0569 | 0.6800 | 0.2671 | 0.1890 | 0.698 |
| $a+bx^2\sqrt{y}+c/\sqrt{x}\sqrt{y}$ | 131.63 | 104.08 | 0.789 | 0.0805 | 0.0569 | 0.6803 | 0.2667 | 0.1887 | 0.699 |
| $a+bx^2\sqrt{y}+cy/\sqrt{x}$ | 131.79 | 104.40 | 0.789 | 0.0791 | 0.0571 | 0.6912 | 0.2678 | 0.1927 | 0.696 |
| $a+bx^2\sqrt{y}+cy^2/\sqrt{x}$ | 130.80 | 103.45 | 0.792 | 0.0797 | 0.0591 | 0.6860 | 0.2707 | 0.2005 | 0.690 |
| $a+bx^2\sqrt{y}+c\sqrt{y}/\sqrt{x}$ | 131.53 | 104.03 | 0.790 | 0.0798 | 0.0575 | 0.6859 | 0.2650 | 0.1910 | 0.702 |
| $a+b\sqrt{x}/y + c\sqrt{x}/y^2$ | 223.61 | 165.18 | 0.392 | 0.1194 | 0.0934 | 0.2958 | 0.3817 | 0.2829 | 0.383 |
| $a+b\sqrt{x}/y + c\sqrt{x}/\sqrt{y}$ | 189.32 | 144.85 | 0.564 | 0.1020 | 0.0799 | 0.4865 | 0.3179 | 0.2333 | 0.572 |
| $a+b\sqrt{x}/y + c\sqrt{x}y$ | 151.42 | 119.58 | 0.721 | 0.0849 | 0.0609 | 0.6437 | 0.2767 | 0.1928 | 0.676 |
| $a+b\sqrt{x}/y + c\sqrt{x}y^2$ | 152.95 | 117.50 | 0.715 | 0.0876 | 0.0654 | 0.6208 | 0.3005 | 0.2144 | 0.617 |
| $a+b\sqrt{x}/y + c\sqrt{x}\sqrt{y}$ | 159.27 | 122.90 | 0.691 | 0.0879 | 0.0660 | 0.6187 | 0.2781 | 0.1910 | 0.672 |
| $a+b\sqrt{x}/y+c/xy$ | 236.36 | 178.10 | 0.320 | 0.1223 | 0.0906 | 0.2620 | 0.4042 | 0.2962 | 0.308 |
| $a+b\sqrt{x}/y+c/xy^2$ | 237.84 | 178.76 | 0.312 | 0.1231 | 0.0910 | 0.2523 | 0.4074 | 0.2983 | 0.297 |
| $a+b\sqrt{x}/y+c/x\sqrt{y}$ | 234.97 | 177.55 | 0.328 | 0.1215 | 0.0902 | 0.2714 | 0.4013 | 0.2944 | 0.318 |
| $a+b\sqrt{x}/y+cy/x$ | 224.86 | 172.81 | 0.385 | 0.1157 | 0.0867 | 0.3386 | 0.3804 | 0.2808 | 0.387 |
| $a+b\sqrt{x}/y+cy^2/x$ | 256.63 | 199.33 | 0.199 | 0.1367 | 0.1059 | 0.0770 | 0.4566 | 0.3510 | 0.117 |
| $a+b\sqrt{x}/y+c\sqrt{y}/x$ | 229.58 | 175.24 | 0.359 | 0.1184 | 0.0884 | 0.3074 | 0.3902 | 0.2874 | 0.355 |
| $a+b\sqrt{x}/y+c/x^2y$ | 240.44 | 181.84 | 0.297 | 0.1239 | 0.0924 | 0.2425 | 0.4134 | 0.3055 | 0.276 |
| $a+b\sqrt{x}/y+c/x^2y^2$ | 240.66 | 181.94 | 0.295 | 0.1240 | 0.0925 | 0.2411 | 0.4140 | 0.3058 | 0.274 |
| $a+b\sqrt{x}/y+c/x^2\sqrt{y}$ | 240.25 | 181.77 | 0.298 | 0.1238 | 0.0923 | 0.2437 | 0.4130 | 0.3052 | 0.277 |
| $a+b\sqrt{x}/y+cy/x^2$ | 238.80 | 181.35 | 0.306 | 0.1229 | 0.0919 | 0.2540 | 0.4099 | 0.3035 | 0.288 |
| $a+b\sqrt{x}/y+cy^2/x^2$ | 235.84 | 180.46 | 0.323 | 0.1211 | 0.0909 | 0.2755 | 0.4034 | 0.3001 | 0.311 |
| $a+b\sqrt{x}/y+c\sqrt{y}/x^2$ | 239.52 | 181.55 | 0.302 | 0.1233 | 0.0921 | 0.2488 | 0.4114 | 0.3044 | 0.283 |
| $a+b\sqrt{x}/y+c/\sqrt{x}y$ | 231.06 | 172.59 | 0.350 | 0.1202 | 0.0908 | 0.2869 | 0.3933 | 0.2832 | 0.345 |
| $a+b\sqrt{x}/y+c/\sqrt{x}y^2$ | 234.98 | 174.45 | 0.328 | 0.1223 | 0.0918 | 0.2613 | 0.4015 | 0.2885 | 0.317 |
| $a+b\sqrt{x}/y+c/\sqrt{x}\sqrt{y}$ | 227.47 | 170.88 | 0.370 | 0.1182 | 0.0896 | 0.3100 | 0.3861 | 0.2785 | 0.368 |
| $a+b\sqrt{x}/y+cy/\sqrt{x}$ | 256.56 | 199.01 | 0.199 | 0.1367 | 0.1058 | 0.0778 | 0.4561 | 0.3502 | 0.118 |
| $a+b\sqrt{x}/y+cy^2/\sqrt{x}$ | 185.88 | 149.81 | 0.580 | 0.0999 | 0.0757 | 0.5073 | 0.3357 | 0.2335 | 0.522 |
| $a+b\sqrt{x}/y+c\sqrt{y}/\sqrt{x}$ | 215.17 | 163.92 | 0.437 | 0.1114 | 0.0848 | 0.3868 | 0.3616 | 0.2610 | 0.446 |
| $a+b\sqrt{x}/y^2+c\sqrt{x}/\sqrt{y}$ | 222.75 | 165.08 | 0.396 | 0.1136 | 0.0894 | 0.3629 | 0.3600 | 0.2679 | 0.451 |
| $a+b\sqrt{x}/y^2+c\sqrt{x}y$ | 150.05 | 119.63 | 0.726 | 0.0870 | 0.0604 | 0.6259 | 0.2864 | 0.1928 | 0.652 |
| $a+b\sqrt{x}/y^2+c\sqrt{x}y^2$ | 153.60 | 120.81 | 0.713 | 0.0919 | 0.0641 | 0.5826 | 0.3041 | 0.2009 | 0.608 |
| $a+b\sqrt{x}/y^2+c\sqrt{x}\sqrt{y}$ | 154.32 | 118.70 | 0.710 | 0.0844 | 0.0606 | 0.6481 | 0.2747 | 0.1881 | 0.680 |
| $a+b\sqrt{x}/y^2+c/xy$ | 222.63 | 163.22 | 0.397 | 0.1193 | 0.0927 | 0.2973 | 0.3820 | 0.2827 | 0.382 |
| $a+b\sqrt{x}/y^2+c/xy^2$ | 221.87 | 163.36 | 0.401 | 0.1194 | 0.0930 | 0.2964 | 0.3821 | 0.2838 | 0.381 |
| $a+b\sqrt{x}/y^2+c/x\sqrt{y}$ | 223.36 | 162.95 | 0.393 | 0.1192 | 0.0923 | 0.2987 | 0.3818 | 0.2814 | 0.382 |
| $a+b\sqrt{x}/y^2+cy/x$ | 225.84 | 166.24 | 0.379 | 0.1178 | 0.0923 | 0.3148 | 0.3777 | 0.2820 | 0.396 |
| $a+b\sqrt{x}/y^2+cy^2/x$ | 221.40 | 164.03 | 0.404 | 0.1194 | 0.0933 | 0.2959 | 0.3821 | 0.2840 | 0.382 |
| $a+b\sqrt{x}/y^2+c\sqrt{y}/x$ | 225.27 | 164.93 | 0.383 | 0.1185 | 0.0921 | 0.3072 | 0.3799 | 0.2818 | 0.389 |
| $a+b\sqrt{x}/y^2+c/x^2y$ | 223.31 | 163.11 | 0.393 | 0.1192 | 0.0922 | 0.2988 | 0.3819 | 0.2816 | 0.382 |
| $a+b\sqrt{x}/y^2+c/x^2y^2$ | 223.28 | 163.13 | 0.393 | 0.1192 | 0.0922 | 0.2987 | 0.3819 | 0.2817 | 0.382 |
| $a+b\sqrt{x}/y^2+c/x^2\sqrt{y}$ | 223.37 | 163.08 | 0.393 | 0.1192 | 0.0921 | 0.2989 | 0.3818 | 0.2815 | 0.382 |
| $a+b\sqrt{x}/y^2+cy/x^2$ | 223.93 | 162.71 | 0.390 | 0.1190 | 0.0917 | 0.3005 | 0.3815 | 0.2802 | 0.383 |
| $a+b\sqrt{x}/y^2+cy^2/x^2$ | 224.81 | 164.09 | 0.385 | 0.1187 | 0.0920 | 0.3046 | 0.3806 | 0.2814 | 0.386 |
| $a+b\sqrt{x}/y^2+c\sqrt{y}/x^2$ | 223.65 | 162.91 | 0.391 | 0.1191 | 0.0920 | 0.2996 | 0.3817 | 0.2809 | 0.383 |
| $a+b\sqrt{x}/y^2+c/\sqrt{x}y$ | 223.24 | 162.85 | 0.394 | 0.1192 | 0.0925 | 0.2981 | 0.3818 | 0.2816 | 0.382 |
| $a+b\sqrt{x}/y^2+c/\sqrt{x}y^2$ | 220.57 | 163.97 | 0.408 | 0.1194 | 0.0934 | 0.2956 | 0.3820 | 0.2849 | 0.382 |
| $a+b\sqrt{x}/y^2+c/\sqrt{x}\sqrt{y}$ | 224.95 | 164.29 | 0.384 | 0.1187 | 0.0920 | 0.3044 | 0.3805 | 0.2816 | 0.387 |
| $a+b\sqrt{x}/y^2+cy/\sqrt{x}$ | 222.10 | 164.49 | 0.400 | 0.1194 | 0.0933 | 0.2957 | 0.3820 | 0.2838 | 0.382 |
| $a+b\sqrt{x}/y^2+cy^2/\sqrt{x}$ | 190.57 | 150.91 | 0.558 | 0.1070 | 0.0771 | 0.4343 | 0.3510 | 0.2380 | 0.478 |
| $a+b\sqrt{x}/y^2+c\sqrt{y}/\sqrt{x}$ | 226.00 | 167.13 | 0.379 | 0.1168 | 0.0921 | 0.3264 | 0.3738 | 0.2805 | 0.408 |
| $a+b\sqrt{x}/\sqrt{y}+c\sqrt{x}y$ | 151.87 | 120.90 | 0.719 | 0.0869 | 0.0636 | 0.6274 | 0.2772 | 0.1882 | 0.675 |
| $a+b\sqrt{x}/\sqrt{y}+c\sqrt{x}y^2$ | 149.31 | 116.60 | 0.729 | 0.0853 | 0.0612 | 0.6411 | 0.2772 | 0.1947 | 0.674 |
| $a+b\sqrt{x}/\sqrt{y}+c\sqrt{x}\sqrt{y}$ | 155.80 | 123.38 | 0.705 | 0.0888 | 0.0666 | 0.6110 | 0.2803 | 0.1898 | 0.667 |
| $a+b\sqrt{x}/\sqrt{y}+c/xy$ | 252.59 | 186.85 | 0.224 | 0.1218 | 0.0948 | 0.2669 | 0.3986 | 0.3092 | 0.327 |
| $a+b\sqrt{x}/\sqrt{y}+c/xy^2$ | 249.97 | 184.40 | 0.240 | 0.1211 | 0.0941 | 0.2754 | 0.3955 | 0.3069 | 0.337 |
| $a+b\sqrt{x}/\sqrt{y}+c/x\sqrt{y}$ | 254.06 | 188.11 | 0.215 | 0.1223 | 0.0951 | 0.2619 | 0.4003 | 0.3101 | 0.321 |
| $a+b\sqrt{x}/\sqrt{y}+cy/x$ | 242.30 | 176.34 | 0.286 | 0.1201 | 0.0918 | 0.2872 | 0.3881 | 0.2967 | 0.362 |
| $a+b\sqrt{x}/\sqrt{y}+cy^2/x$ | 183.56 | 141.70 | 0.590 | 0.1011 | 0.0789 | 0.4958 | 0.3185 | 0.2311 | 0.570 |
| $a+b\sqrt{x}/\sqrt{y}+c\sqrt{y}/x$ | 254.67 | 189.07 | 0.211 | 0.1226 | 0.0952 | 0.2577 | 0.4013 | 0.3101 | 0.318 |
| $a+b\sqrt{x}/\sqrt{y}+c/x^2y$ | 240.87 | 173.72 | 0.294 | 0.1196 | 0.0910 | 0.2941 | 0.3859 | 0.2936 | 0.369 |
| $a+b\sqrt{x}/\sqrt{y}+c/x^2y^2$ | 240.39 | 173.12 | 0.297 | 0.1195 | 0.0908 | 0.2953 | 0.3853 | 0.2929 | 0.371 |
| $a+b\sqrt{x}/\sqrt{y}+c/x^2\sqrt{y}$ | 241.22 | 174.13 | 0.292 | 0.1197 | 0.0911 | 0.2931 | 0.3863 | 0.2941 | 0.368 |
| $a+b\sqrt{x}/\sqrt{y}+cy/x^2$ | 242.47 | 175.60 | 0.285 | 0.1200 | 0.0915 | 0.2887 | 0.3878 | 0.2956 | 0.363 |
| $a+b\sqrt{x}/\sqrt{y}+cy^2/x^2$ | 239.82 | 172.57 | 0.300 | 0.1196 | 0.0907 | 0.2936 | 0.3852 | 0.2919 | 0.371 |
| $a+b\sqrt{x}/\sqrt{y}+c\sqrt{y}/x^2$ | 242.11 | 175.18 | 0.287 | 0.1199 | 0.0914 | 0.2902 | 0.3873 | 0.2952 | 0.364 |
| $a+b\sqrt{x}/\sqrt{y}+c/\sqrt{x}y$ | 259.23 | 193.61 | 0.182 | 0.1232 | 0.0963 | 0.2501 | 0.4054 | 0.3090 | 0.304 |
| $a+b\sqrt{x}/\sqrt{y}+c/\sqrt{x}y^2$ | 258.67 | 193.22 | 0.186 | 0.1231 | 0.0963 | 0.2521 | 0.4051 | 0.3114 | 0.305 |
| $a+b\sqrt{x}/\sqrt{y}+c/\sqrt{x}\sqrt{y}$ | 258.15 | 191.53 | 0.189 | 0.1228 | 0.0956 | 0.2557 | 0.4037 | 0.3055 | 0.309 |
| $a+b\sqrt{x}/\sqrt{y}+cy/\sqrt{x}$ | 184.73 | 142.31 | 0.585 | 0.1011 | 0.0790 | 0.4955 | 0.3173 | 0.2315 | 0.574 |
| $a+b\sqrt{x}/\sqrt{y}+cy^2/\sqrt{x}$ | 180.29 | 141.63 | 0.605 | 0.0970 | 0.0742 | 0.5357 | 0.3116 | 0.2216 | 0.589 |
| $a+b\sqrt{x}/\sqrt{y}+c\sqrt{y}/\sqrt{x}$ | 244.07 | 178.84 | 0.275 | 0.1205 | 0.0925 | 0.2826 | 0.3902 | 0.2998 | 0.355 |

(continued on next page)

**Table 4 – continued from previous page**

| Functional form | $T_{eff}$ (K) | | | Radius ($R_\odot$) | | | log (L/$L_\odot$) | | |
|---|---|---|---|---|---|---|---|---|---|
| | RMSE | MAD | $R^2_{ap}$ | RMSE | MAD | $R^2_{ap}$ | RMSE | MAD | $R^2_{ap}$ |
| $a+b\sqrt{x}y+c\sqrt{x}y^2$ | 150.78 | 120.22 | 0.723 | 0.0883 | 0.0620 | 0.6149 | 0.2830 | 0.1882 | 0.661 |
| $a+b\sqrt{x}y+c\sqrt{x}\sqrt{y}$ | 151.47 | 121.07 | 0.721 | 0.0880 | 0.0632 | 0.6173 | 0.2806 | 0.1864 | 0.666 |
| $a+b\sqrt{x}y+c/xy$ | 139.45 | 106.83 | 0.763 | 0.0880 | 0.0596 | 0.6179 | 0.2861 | 0.1894 | 0.653 |
| $a+b\sqrt{x}y+c/xy^2$ | 139.21 | 106.49 | 0.764 | 0.0880 | 0.0596 | 0.6180 | 0.2860 | 0.1893 | 0.653 |
| $a+b\sqrt{x}y+c/x\sqrt{y}$ | 139.70 | 107.14 | 0.763 | 0.0880 | 0.0596 | 0.6176 | 0.2861 | 0.1895 | 0.653 |
| $a+b\sqrt{x}y+cy/x$ | 144.68 | 113.02 | 0.745 | 0.0883 | 0.0616 | 0.6147 | 0.2866 | 0.1912 | 0.652 |
| $a+b\sqrt{x}y+cy^2/x$ | 151.07 | 119.13 | 0.722 | 0.0836 | 0.0603 | 0.6551 | 0.2693 | 0.1865 | 0.693 |
| $a+b\sqrt{x}y+c\sqrt{y}/x$ | 141.55 | 109.33 | 0.756 | 0.0882 | 0.0603 | 0.6157 | 0.2866 | 0.1902 | 0.652 |
| $a+b\sqrt{x}y+c/x^2y$ | 137.75 | 103.80 | 0.769 | 0.0880 | 0.0599 | 0.6173 | 0.2856 | 0.1875 | 0.654 |
| $a+b\sqrt{x}y+c/x^2y^2$ | 137.69 | 103.69 | 0.769 | 0.0880 | 0.0600 | 0.6173 | 0.2856 | 0.1874 | 0.655 |
| $a+b\sqrt{x}y+c/x^2\sqrt{y}$ | 137.80 | 103.88 | 0.769 | 0.0880 | 0.0599 | 0.6173 | 0.2856 | 0.1875 | 0.654 |
| $a+b\sqrt{x}y+cy/x^2$ | 138.35 | 104.58 | 0.767 | 0.0881 | 0.0599 | 0.6169 | 0.2858 | 0.1879 | 0.654 |
| $a+b\sqrt{x}y+cy^2/x^2$ | 140.20 | 106.83 | 0.761 | 0.0882 | 0.0606 | 0.6155 | 0.2863 | 0.1891 | 0.653 |
| $a+b\sqrt{x}y+c\sqrt{y}/x^2$ | 138.05 | 104.20 | 0.768 | 0.0881 | 0.0599 | 0.6171 | 0.2857 | 0.1877 | 0.654 |
| $a+b\sqrt{x}y+c/\sqrt{x}y$ | 141.79 | 110.34 | 0.755 | 0.0879 | 0.0593 | 0.6184 | 0.2864 | 0.1907 | 0.652 |
| $a+b\sqrt{x}y+c/\sqrt{x}y^2$ | 141.62 | 110.13 | 0.756 | 0.0879 | 0.0592 | 0.6186 | 0.2863 | 0.1906 | 0.653 |
| $a+b\sqrt{x}y+c/\sqrt{x}\sqrt{y}$ | 142.07 | 110.67 | 0.754 | 0.0880 | 0.0593 | 0.6177 | 0.2865 | 0.1907 | 0.652 |
| $a+b\sqrt{x}y+cy/\sqrt{x}$ | 151.16 | 119.19 | 0.722 | 0.0840 | 0.0605 | 0.6518 | 0.2716 | 0.1887 | 0.687 |
| $a+b\sqrt{x}y+cy^2/\sqrt{x}$ | 139.17 | 105.94 | 0.764 | 0.0776 | 0.0537 | 0.7024 | 0.2446 | 0.1664 | 0.747 |
| $a+b\sqrt{x}y+c\sqrt{y}/\sqrt{x}$ | 147.85 | 117.17 | 0.734 | 0.0882 | 0.0622 | 0.6159 | 0.2855 | 0.1905 | 0.655 |
| $a+b\sqrt{x}y^2+c\sqrt{x}\sqrt{y}$ | 150.14 | 119.32 | 0.726 | 0.0876 | 0.0620 | 0.6208 | 0.2804 | 0.1854 | 0.667 |
| $a+b\sqrt{x}y^2+c/xy$ | 154.18 | 117.45 | 0.711 | 0.0914 | 0.0639 | 0.5871 | 0.3069 | 0.2114 | 0.601 |
| $a+b\sqrt{x}y^2+c/xy^2$ | 154.07 | 117.15 | 0.711 | 0.0915 | 0.0639 | 0.5866 | 0.3073 | 0.2116 | 0.600 |
| $a+b\sqrt{x}y^2+c/x\sqrt{y}$ | 154.26 | 117.65 | 0.710 | 0.0914 | 0.0640 | 0.5877 | 0.3066 | 0.2113 | 0.602 |
| $a+b\sqrt{x}y^2+cy/x$ | 154.81 | 119.67 | 0.708 | 0.0902 | 0.0645 | 0.5982 | 0.3023 | 0.2104 | 0.613 |
| $a+b\sqrt{x}y^2+cy^2/x$ | 149.94 | 114.92 | 0.726 | 0.0837 | 0.0629 | 0.6544 | 0.2850 | 0.2045 | 0.656 |
| $a+b\sqrt{x}y^2+c\sqrt{y}/x$ | 154.54 | 118.55 | 0.709 | 0.0910 | 0.0642 | 0.5913 | 0.3050 | 0.2110 | 0.606 |
| $a+b\sqrt{x}y^2+c/x^2y$ | 152.82 | 114.39 | 0.716 | 0.0917 | 0.0641 | 0.5846 | 0.3094 | 0.2137 | 0.594 |
| $a+b\sqrt{x}y^2+c/x^2y^2$ | 152.76 | 114.27 | 0.716 | 0.0917 | 0.0641 | 0.5845 | 0.3095 | 0.2137 | 0.594 |
| $a+b\sqrt{x}y^2+c/x^2\sqrt{y}$ | 152.86 | 114.46 | 0.716 | 0.0917 | 0.0641 | 0.5847 | 0.3094 | 0.2137 | 0.594 |
| $a+b\sqrt{x}y^2+cy/x^2$ | 153.08 | 114.94 | 0.715 | 0.0916 | 0.0642 | 0.5854 | 0.3090 | 0.2136 | 0.595 |
| $a+b\sqrt{x}y^2+cy^2/x^2$ | 153.58 | 116.13 | 0.713 | 0.0913 | 0.0645 | 0.5880 | 0.3080 | 0.2136 | 0.598 |
| $a+b\sqrt{x}y^2+c\sqrt{y}/x^2$ | 152.97 | 114.71 | 0.715 | 0.0917 | 0.0642 | 0.5850 | 0.3092 | 0.2136 | 0.595 |
| $a+b\sqrt{x}y^2+c/\sqrt{x}y$ | 154.81 | 119.67 | 0.708 | 0.0912 | 0.0634 | 0.5894 | 0.3038 | 0.2073 | 0.609 |
| $a+b\sqrt{x}y^2+c/\sqrt{x}y^2$ | 154.77 | 119.42 | 0.709 | 0.0913 | 0.0634 | 0.5885 | 0.3046 | 0.2079 | 0.607 |
| $a+b\sqrt{x}y^2+c/\sqrt{x}\sqrt{y}$ | 154.84 | 119.85 | 0.708 | 0.0910 | 0.0635 | 0.5907 | 0.3031 | 0.2070 | 0.611 |
| $a+b\sqrt{x}y^2+cy/\sqrt{x}$ | 150.94 | 115.55 | 0.723 | 0.0850 | 0.0639 | 0.6434 | 0.2904 | 0.2091 | 0.643 |
| $a+b\sqrt{x}y^2+cy^2/\sqrt{x}$ | 144.87 | 110.36 | 0.745 | 0.0866 | 0.0653 | 0.6295 | 0.2996 | 0.2213 | 0.620 |
| $a+b\sqrt{x}y^2+c\sqrt{y}/\sqrt{x}$ | 154.59 | 120.79 | 0.709 | 0.0890 | 0.0640 | 0.6088 | 0.2963 | 0.2053 | 0.628 |
| $a+b\sqrt{x}\sqrt{y}+c/xy$ | 128.22 | 94.63 | 0.800 | 0.0854 | 0.0601 | 0.6397 | 0.2694 | 0.1715 | 0.693 |
| $a+b\sqrt{x}\sqrt{y}+c/xy^2$ | 128.08 | 94.35 | 0.800 | 0.0854 | 0.0601 | 0.6398 | 0.2692 | 0.1714 | 0.693 |
| $a+b\sqrt{x}\sqrt{y}+c/x\sqrt{y}$ | 128.55 | 95.29 | 0.799 | 0.0855 | 0.0602 | 0.6389 | 0.2697 | 0.1717 | 0.692 |
| $a+b\sqrt{x}\sqrt{y}+cy/x$ | 138.63 | 108.00 | 0.766 | 0.0876 | 0.0629 | 0.6212 | 0.2765 | 0.1810 | 0.676 |
| $a+b\sqrt{x}\sqrt{y}+cy^2/x$ | 159.14 | 123.14 | 0.692 | 0.0877 | 0.0664 | 0.6205 | 0.2762 | 0.1902 | 0.677 |
| $a+b\sqrt{x}\sqrt{y}+c\sqrt{y}/x$ | 132.10 | 100.46 | 0.788 | 0.0864 | 0.0609 | 0.6316 | 0.2724 | 0.1751 | 0.686 |
| $a+b\sqrt{x}\sqrt{y}+c/x^2y$ | 129.61 | 99.65 | 0.796 | 0.0863 | 0.0613 | 0.6325 | 0.2701 | 0.1741 | 0.691 |
| $a+b\sqrt{x}\sqrt{y}+c/x^2y^2$ | 129.64 | 99.71 | 0.796 | 0.0863 | 0.0614 | 0.6324 | 0.2701 | 0.1741 | 0.691 |
| $a+b\sqrt{x}\sqrt{y}+c/x^2\sqrt{y}$ | 129.64 | 99.66 | 0.796 | 0.0863 | 0.0613 | 0.6325 | 0.2702 | 0.1741 | 0.691 |
| $a+b\sqrt{x}\sqrt{y}+cy/x^2$ | 130.40 | 100.33 | 0.793 | 0.0864 | 0.0614 | 0.6313 | 0.2708 | 0.1741 | 0.689 |
| $a+b\sqrt{x}\sqrt{y}+cy^2/x^2$ | 133.41 | 103.43 | 0.783 | 0.0870 | 0.0620 | 0.6264 | 0.2730 | 0.1768 | 0.684 |
| $a+b\sqrt{x}\sqrt{y}+c\sqrt{y}/x^2$ | 129.94 | 99.94 | 0.795 | 0.0863 | 0.0614 | 0.6321 | 0.2704 | 0.1741 | 0.690 |
| $a+b\sqrt{x}\sqrt{y}+c/\sqrt{x}y$ | 129.23 | 98.05 | 0.797 | 0.0846 | 0.0582 | 0.6467 | 0.2692 | 0.1727 | 0.693 |
| $a+b\sqrt{x}\sqrt{y}+c/\sqrt{x}y^2$ | 129.52 | 98.28 | 0.796 | 0.0846 | 0.0582 | 0.6465 | 0.2691 | 0.1726 | 0.693 |
| $a+b\sqrt{x}\sqrt{y}+c/\sqrt{x}\sqrt{y}$ | 129.47 | 98.24 | 0.796 | 0.0848 | 0.0586 | 0.6447 | 0.2698 | 0.1725 | 0.692 |
| $a+b\sqrt{x}\sqrt{y}+cy/\sqrt{x}$ | 159.18 | 123.09 | 0.692 | 0.0877 | 0.0663 | 0.6199 | 0.2768 | 0.1906 | 0.675 |
| $a+b\sqrt{x}\sqrt{y}+cy^2/\sqrt{x}$ | 159.53 | 121.10 | 0.690 | 0.0865 | 0.0656 | 0.6309 | 0.2677 | 0.1841 | 0.696 |
| $a+b\sqrt{x}\sqrt{y}+c\sqrt{y}/\sqrt{x}$ | 143.77 | 112.22 | 0.749 | 0.0881 | 0.0640 | 0.6168 | 0.2788 | 0.1836 | 0.671 |
| $a+b/xy+c/xy^2$ | 142.24 | 102.77 | 0.754 | 0.0901 | 0.0652 | 0.5988 | 0.2708 | 0.1745 | 0.689 |
| $a+b/xy+c/x\sqrt{y}$ | 167.63 | 115.55 | 0.658 | 0.0906 | 0.0639 | 0.5944 | 0.2925 | 0.1935 | 0.638 |
| $a+b/xy+cy/x$ | 281.46 | 209.05 | 0.036 | 0.1333 | 0.1055 | 0.1225 | 0.4499 | 0.3443 | 0.142 |
| $a+b/xy+cy^2/x$ | 236.13 | 180.90 | 0.322 | 0.1228 | 0.0919 | 0.2557 | 0.4090 | 0.2984 | 0.291 |
| $a+b/xy+c\sqrt{y}/x$ | 250.70 | 168.45 | 0.235 | 0.1172 | 0.0903 | 0.3218 | 0.3972 | 0.2866 | 0.332 |
| $a+b/xy+c/x^2y$ | 241.66 | 174.59 | 0.289 | 0.1253 | 0.0977 | 0.2250 | 0.4034 | 0.2980 | 0.311 |
| $a+b/xy+c/x^2y^2$ | 240.75 | 174.20 | 0.295 | 0.1250 | 0.0976 | 0.2283 | 0.4022 | 0.2975 | 0.315 |
| $a+b/xy+c/x^2\sqrt{y}$ | 242.86 | 175.10 | 0.282 | 0.1256 | 0.0979 | 0.2207 | 0.4050 | 0.2988 | 0.305 |
| $a+b/xy+cy/x^2$ | 252.59 | 179.56 | 0.224 | 0.1285 | 0.0992 | 0.1850 | 0.4182 | 0.3056 | 0.259 |
| $a+b/xy+cy^2/x^2$ | 262.49 | 186.20 | 0.162 | 0.1314 | 0.1013 | 0.1479 | 0.4329 | 0.3193 | 0.206 |
| $a+b/xy+c\sqrt{y}/x^2$ | 248.10 | 177.20 | 0.251 | 0.1272 | 0.0985 | 0.2016 | 0.4120 | 0.3019 | 0.281 |
| $a+b/xy+c/\sqrt{x}y$ | 216.88 | 160.63 | 0.428 | 0.1178 | 0.0925 | 0.3146 | 0.3726 | 0.2788 | 0.412 |
| $a+b/xy+c/\sqrt{x}y^2$ | 254.51 | 180.51 | 0.212 | 0.1289 | 0.0995 | 0.1796 | 0.4201 | 0.3067 | 0.252 |
| $a+b/xy+c/\sqrt{x}\sqrt{y}$ | 183.66 | 138.44 | 0.590 | 0.1072 | 0.0842 | 0.4322 | 0.3304 | 0.2440 | 0.537 |
| $a+b/xy+cy/\sqrt{x}$ | 235.92 | 179.70 | 0.323 | 0.1225 | 0.0914 | 0.2591 | 0.4071 | 0.2977 | 0.298 |
| $a+b/xy+cy^2/\sqrt{x}$ | 190.36 | 149.39 | 0.559 | 0.1066 | 0.0758 | 0.4394 | 0.3538 | 0.2435 | 0.469 |
| $a+b/xy+c\sqrt{y}/\sqrt{x}$ | 270.67 | 196.49 | 0.109 | 0.1275 | 0.0986 | 0.1979 | 0.4264 | 0.3210 | 0.230 |
| $a+b/xy^2+c/x\sqrt{y}$ | 143.83 | 106.23 | 0.748 | 0.0873 | 0.0622 | 0.6233 | 0.2681 | 0.1771 | 0.695 |
| $a+b/xy^2+cy/x$ | 281.26 | 205.02 | 0.038 | 0.1323 | 0.1027 | 0.1356 | 0.4476 | 0.3364 | 0.151 |
| $a+b/xy^2+cy^2/x$ | 237.72 | 181.70 | 0.312 | 0.1236 | 0.0924 | 0.2454 | 0.4124 | 0.3006 | 0.279 |
| $a+b/xy^2+c\sqrt{y}/x$ | 224.31 | 150.78 | 0.388 | 0.1072 | 0.0814 | 0.4330 | 0.3594 | 0.2533 | 0.453 |
| $a+b/xy^2+c/x^2y$ | 255.71 | 180.64 | 0.204 | 0.1297 | 0.0998 | 0.1689 | 0.4230 | 0.3082 | 0.242 |
| $a+b/xy^2+c/x^2y^2$ | 254.50 | 180.39 | 0.212 | 0.1294 | 0.0998 | 0.1732 | 0.4214 | 0.3076 | 0.248 |
| $a+b/xy^2+c/x^2\sqrt{y}$ | 257.00 | 180.89 | 0.196 | 0.1301 | 0.0998 | 0.1643 | 0.4247 | 0.3089 | 0.236 |
| $a+b/xy^2+cy/x^2$ | 265.73 | 187.99 | 0.141 | 0.1325 | 0.1018 | 0.1332 | 0.4364 | 0.3202 | 0.193 |
| $a+b/xy^2+cy^2/x^2$ | 272.51 | 198.11 | 0.096 | 0.1343 | 0.1051 | 0.1093 | 0.4465 | 0.3368 | 0.155 |
| $a+b/xy^2+c\sqrt{y}/x^2$ | 261.94 | 183.32 | 0.165 | 0.1315 | 0.1003 | 0.1467 | 0.4313 | 0.3130 | 0.212 |
| $a+b/xy^2+c/\sqrt{x}y$ | 206.66 | 153.62 | 0.480 | 0.1149 | 0.0903 | 0.3480 | 0.3602 | 0.2692 | 0.450 |
| $a+b/xy^2+c/\sqrt{x}y^2$ | 243.29 | 176.33 | 0.280 | 0.1262 | 0.0988 | 0.2140 | 0.4070 | 0.3022 | 0.298 |
| $a+b/xy^2+c/\sqrt{x}\sqrt{y}$ | 176.27 | 133.40 | 0.622 | 0.1050 | 0.0823 | 0.4556 | 0.3214 | 0.2372 | 0.562 |
| $a+b/xy^2+cy/\sqrt{x}$ | 237.47 | 180.47 | 0.314 | 0.1233 | 0.0919 | 0.2490 | 0.4104 | 0.2999 | 0.286 |
| $a+b/xy^2+cy^2/\sqrt{x}$ | 190.16 | 148.90 | 0.560 | 0.1067 | 0.0757 | 0.4382 | 0.3544 | 0.2433 | 0.468 |
| $a+b/xy^2+c\sqrt{y}/\sqrt{x}$ | 265.70 | 191.23 | 0.141 | 0.1254 | 0.0974 | 0.2239 | 0.4184 | 0.3174 | 0.258 |
| $a+b/x\sqrt{y}+cy/x$ | 279.56 | 209.34 | 0.049 | 0.1333 | 0.1063 | 0.1231 | 0.4487 | 0.3458 | 0.147 |

(continued on next page)

**Table 4 – continued from previous page**

| Functional form | $T_{eff}$ (K) RMSE | MAD | $R^2_{ap}$ | Radius ($R_\odot$) RMSE | MAD | $R^2_{ap}$ | log (L/$L_\odot$) RMSE | MAD | $R^2_{ap}$ |
|---|---|---|---|---|---|---|---|---|---|
| $a+b/x\sqrt{y}+cy^2/x$ | 234.71 | 180.28 | 0.330 | 0.1220 | 0.0915 | 0.2651 | 0.4061 | 0.2965 | 0.301 |
| $a+b/x\sqrt{y}+c\sqrt{y}/x$ | 264.29 | 182.85 | 0.150 | 0.1231 | 0.0947 | 0.2516 | 0.4176 | 0.3042 | 0.261 |
| $a+b/x\sqrt{y}+c/x^2y$ | 228.61 | 166.95 | 0.364 | 0.1210 | 0.0948 | 0.2770 | 0.3851 | 0.2861 | 0.372 |
| $a+b/x\sqrt{y}+c/x^2y^2$ | 228.00 | 166.61 | 0.368 | 0.1208 | 0.0947 | 0.2791 | 0.3843 | 0.2856 | 0.374 |
| $a+b/x\sqrt{y}+c/x^2\sqrt{y}$ | 229.71 | 167.58 | 0.358 | 0.1213 | 0.0950 | 0.2730 | 0.3866 | 0.2870 | 0.367 |
| $a+b/x\sqrt{y}+cy/x^2$ | 240.19 | 173.09 | 0.298 | 0.1245 | 0.0969 | 0.2344 | 0.4009 | 0.2956 | 0.319 |
| $a+b/x\sqrt{y}+cy^2/x^2$ | 253.00 | 180.26 | 0.221 | 0.1285 | 0.0989 | 0.1851 | 0.4200 | 0.3069 | 0.252 |
| $a+b/x\sqrt{y}+c\sqrt{y}/x^2$ | 235.15 | 170.52 | 0.327 | 0.1230 | 0.0960 | 0.2532 | 0.3939 | 0.2914 | 0.342 |
| $a+b/x\sqrt{y}+c/\sqrt{x}y$ | 228.09 | 166.86 | 0.367 | 0.1209 | 0.0946 | 0.2783 | 0.3859 | 0.2871 | 0.369 |
| $a+b/x\sqrt{y}+c/\sqrt{x}y^2$ | 262.76 | 186.88 | 0.160 | 0.1306 | 0.1010 | 0.1577 | 0.4293 | 0.3157 | 0.219 |
| $a+b/x\sqrt{y}+c/\sqrt{x}\sqrt{y}$ | 194.61 | 145.04 | 0.539 | 0.1105 | 0.0866 | 0.3973 | 0.3436 | 0.2528 | 0.500 |
| $a+b/x\sqrt{y}+cy/\sqrt{x}$ | 234.51 | 179.11 | 0.331 | 0.1217 | 0.0910 | 0.2684 | 0.4042 | 0.2959 | 0.308 |
| $a+b/x\sqrt{y}+cy^2/\sqrt{x}$ | 190.53 | 149.81 | 0.558 | 0.1064 | 0.0759 | 0.4407 | 0.3533 | 0.2438 | 0.471 |
| $a+b/x\sqrt{y}+c\sqrt{y}/\sqrt{x}$ | 272.91 | 198.59 | 0.094 | 0.1285 | 0.0993 | 0.1845 | 0.4302 | 0.3233 | 0.216 |
| $a+by/x+cy^2/x$ | 224.60 | 175.89 | 0.386 | 0.1165 | 0.0885 | 0.3302 | 0.3869 | 0.2825 | 0.366 |
| $a+by/x+c\sqrt{y}/x$ | 266.66 | 199.65 | 0.135 | 0.1301 | 0.1036 | 0.1638 | 0.4350 | 0.3345 | 0.198 |
| $a+by/x+c/x^2y$ | 238.25 | 174.46 | 0.309 | 0.1175 | 0.0883 | 0.3183 | 0.3794 | 0.2848 | 0.390 |
| $a+by/x+c/x^2y^2$ | 235.97 | 172.68 | 0.323 | 0.1168 | 0.0876 | 0.3259 | 0.3762 | 0.2819 | 0.400 |
| $a+by/x+c/x^2\sqrt{y}$ | 239.84 | 175.47 | 0.300 | 0.1180 | 0.0888 | 0.3124 | 0.3817 | 0.2863 | 0.383 |
| $a+by/x+cy/x^2$ | 245.11 | 177.82 | 0.269 | 0.1201 | 0.0903 | 0.2884 | 0.3895 | 0.2909 | 0.357 |
| $a+by/x+cy^2/x^2$ | 230.87 | 159.18 | 0.351 | 0.1170 | 0.0875 | 0.3239 | 0.3720 | 0.2704 | 0.414 |
| $a+by/x+c\sqrt{y}/x^2$ | 243.75 | 177.57 | 0.277 | 0.1194 | 0.0899 | 0.2960 | 0.3874 | 0.2895 | 0.364 |
| $a+by/x+c/\sqrt{x}y$ | 256.18 | 186.15 | 0.202 | 0.1275 | 0.0995 | 0.1968 | 0.4195 | 0.3143 | 0.254 |
| $a+by/x+c/\sqrt{x}y^2$ | 270.63 | 200.32 | 0.109 | 0.1315 | 0.1046 | 0.1459 | 0.4376 | 0.3347 | 0.189 |
| $a+by/x+c/\sqrt{x}\sqrt{y}$ | 242.39 | 175.35 | 0.285 | 0.1234 | 0.0957 | 0.2483 | 0.4022 | 0.2964 | 0.315 |
| $a+by/x+cy/\sqrt{x}$ | 224.28 | 174.68 | 0.388 | 0.1161 | 0.0875 | 0.3348 | 0.3843 | 0.2820 | 0.374 |
| $a+by/x+cy^2/\sqrt{x}$ | 191.08 | 152.56 | 0.556 | 0.1045 | 0.0768 | 0.4607 | 0.3463 | 0.2438 | 0.492 |
| $a+by/x+c\sqrt{y}/\sqrt{x}$ | 235.86 | 167.50 | 0.323 | 0.1183 | 0.0887 | 0.3093 | 0.3788 | 0.2832 | 0.392 |
| $a+by^2/x+c\sqrt{y}/x$ | 229.32 | 178.02 | 0.360 | 0.1190 | 0.0897 | 0.3005 | 0.3956 | 0.2893 | 0.337 |
| $a+by^2/x+c/x^2y$ | 241.88 | 185.40 | 0.288 | 0.1252 | 0.0938 | 0.2263 | 0.4217 | 0.3081 | 0.247 |
| $a+by^2/x+c/x^2y^2$ | 242.15 | 185.52 | 0.287 | 0.1253 | 0.0939 | 0.2246 | 0.4223 | 0.3084 | 0.244 |
| $a+by^2/x+c/x^2\sqrt{y}$ | 241.68 | 185.32 | 0.289 | 0.1251 | 0.0938 | 0.2277 | 0.4212 | 0.3079 | 0.248 |
| $a+by^2/x+cy/x^2$ | 240.17 | 184.87 | 0.298 | 0.1242 | 0.0934 | 0.2382 | 0.4181 | 0.3061 | 0.259 |
| $a+by^2/x+cy^2/x^2$ | 237.19 | 183.98 | 0.316 | 0.1225 | 0.0924 | 0.2592 | 0.4120 | 0.3026 | 0.281 |
| $a+by^2/x+c\sqrt{y}/x^2$ | 240.90 | 185.07 | 0.294 | 0.1246 | 0.0936 | 0.2330 | 0.4196 | 0.3070 | 0.254 |
| $a+by^2/x+c/\sqrt{x}y$ | 229.41 | 174.19 | 0.360 | 0.1201 | 0.0899 | 0.2874 | 0.3954 | 0.2856 | 0.338 |
| $a+by^2/x+c/\sqrt{x}y^2$ | 233.43 | 176.31 | 0.337 | 0.1223 | 0.0910 | 0.2616 | 0.4037 | 0.2906 | 0.309 |
| $a+by^2/x+c/\sqrt{x}\sqrt{y}$ | 225.82 | 172.46 | 0.380 | 0.1182 | 0.0887 | 0.3104 | 0.3882 | 0.2812 | 0.361 |
| $a+by^2/x+cy/\sqrt{x}$ | 257.37 | 200.70 | 0.194 | 0.1370 | 0.1064 | 0.0737 | 0.4581 | 0.3533 | 0.111 |
| $a+by^2/x+cy^2/\sqrt{x}$ | 183.05 | 146.98 | 0.592 | 0.0961 | 0.0737 | 0.5439 | 0.3181 | 0.2260 | 0.571 |
| $a+by^2/x+c\sqrt{y}/\sqrt{x}$ | 213.45 | 166.58 | 0.446 | 0.1117 | 0.0847 | 0.3843 | 0.3664 | 0.2651 | 0.431 |
| $a+b\sqrt{y}/x+c/x^2y$ | 185.78 | 135.46 | 0.580 | 0.1053 | 0.0821 | 0.4526 | 0.3198 | 0.2315 | 0.567 |
| $a+b\sqrt{y}/x+c/x^2y^2$ | 186.15 | 135.67 | 0.578 | 0.1055 | 0.0823 | 0.4507 | 0.3204 | 0.2319 | 0.565 |
| $a+b\sqrt{y}/x+c/x^2\sqrt{y}$ | 186.41 | 135.92 | 0.577 | 0.1055 | 0.0822 | 0.4508 | 0.3206 | 0.2320 | 0.564 |
| $a+b\sqrt{y}/x+cy/x^2$ | 195.90 | 142.13 | 0.533 | 0.1088 | 0.0849 | 0.4158 | 0.3343 | 0.2417 | 0.526 |
| $a+b\sqrt{y}/x+cy^2/x^2$ | 213.40 | 155.85 | 0.446 | 0.1155 | 0.0897 | 0.3416 | 0.3638 | 0.2674 | 0.439 |
| $a+b\sqrt{y}/x+c\sqrt{y}/x^2$ | 190.99 | 138.97 | 0.556 | 0.1070 | 0.0834 | 0.4348 | 0.3270 | 0.2359 | 0.547 |
| $a+b\sqrt{y}/x+c/\sqrt{x}y$ | 253.81 | 181.13 | 0.216 | 0.1271 | 0.0983 | 0.2022 | 0.4160 | 0.3064 | 0.267 |
| $a+b\sqrt{y}/x+c/\sqrt{x}y^2$ | 272.34 | 202.61 | 0.098 | 0.1313 | 0.1050 | 0.1482 | 0.4380 | 0.3360 | 0.187 |
| $a+b\sqrt{y}/x+c/\sqrt{x}\sqrt{y}$ | 232.18 | 170.07 | 0.344 | 0.1210 | 0.0944 | 0.2773 | 0.3893 | 0.2897 | 0.358 |
| $a+b\sqrt{y}/x+cy/\sqrt{x}$ | 229.09 | 176.88 | 0.361 | 0.1187 | 0.0892 | 0.3041 | 0.3935 | 0.2887 | 0.344 |
| $a+b\sqrt{y}/x+cy^2/\sqrt{x}$ | 191.05 | 151.40 | 0.556 | 0.1057 | 0.0763 | 0.4486 | 0.3504 | 0.2444 | 0.480 |
| $a+b\sqrt{y}/x+c\sqrt{y}/\sqrt{x}$ | 274.40 | 201.23 | 0.084 | 0.1295 | 0.1006 | 0.1723 | 0.4331 | 0.3255 | 0.205 |
| $a+b/x^2y+c/x^2y^2$ | 206.15 | 150.52 | 0.483 | 0.1138 | 0.0895 | 0.3607 | 0.3521 | 0.2596 | 0.475 |
| $a+b/x^2y+c/x^2\sqrt{y}$ | 158.71 | 108.62 | 0.694 | 0.0975 | 0.0757 | 0.5302 | 0.2862 | 0.2048 | 0.653 |
| $a+b/x^2y+cy/x^2$ | 182.86 | 134.62 | 0.593 | 0.0965 | 0.0748 | 0.5399 | 0.3058 | 0.2241 | 0.604 |
| $a+b/x^2y+cy^2/x^2$ | 279.58 | 190.59 | 0.049 | 0.1315 | 0.0980 | 0.1461 | 0.4469 | 0.3188 | 0.154 |
| $a+b/x^2y+c\sqrt{y}/x^2$ | 147.87 | 105.84 | 0.734 | 0.0891 | 0.0619 | 0.6079 | 0.2644 | 0.1728 | 0.704 |
| $a+b/x^2y+c/\sqrt{x}y$ | 228.13 | 166.64 | 0.367 | 0.1209 | 0.0947 | 0.2783 | 0.3854 | 0.2868 | 0.371 |
| $a+b/x^2y+c/\sqrt{x}y^2$ | 248.83 | 178.02 | 0.247 | 0.1276 | 0.0990 | 0.1965 | 0.4135 | 0.3036 | 0.276 |
| $a+b/x^2y+c/\sqrt{x}\sqrt{y}$ | 210.16 | 154.70 | 0.463 | 0.1149 | 0.0897 | 0.3476 | 0.3611 | 0.2675 | 0.448 |
| $a+b/x^2y+cy/\sqrt{x}$ | 241.12 | 184.14 | 0.293 | 0.1246 | 0.0932 | 0.2329 | 0.4187 | 0.3074 | 0.257 |
| $a+b/x^2y+cy^2/\sqrt{x}$ | 189.31 | 146.65 | 0.564 | 0.1068 | 0.0759 | 0.4369 | 0.3559 | 0.2435 | 0.463 |
| $a+b/x^2y+c\sqrt{y}/\sqrt{x}$ | 236.47 | 170.99 | 0.320 | 0.1176 | 0.0883 | 0.3174 | 0.3779 | 0.2826 | 0.395 |
| $a+b/x^2y^2+c/x^2\sqrt{y}$ | 187.66 | 135.53 | 0.572 | 0.1076 | 0.0848 | 0.4285 | 0.3261 | 0.2408 | 0.549 |
| $a+b/x^2y^2+cy/x^2$ | 160.12 | 117.07 | 0.688 | 0.0915 | 0.0676 | 0.5868 | 0.2757 | 0.1960 | 0.678 |
| $a+b/x^2y^2+cy^2/x^2$ | 273.52 | 184.22 | 0.090 | 0.1288 | 0.0961 | 0.1805 | 0.4362 | 0.3114 | 0.194 |
| $a+b/x^2y^2+c\sqrt{y}/x^2$ | 146.95 | 99.41 | 0.737 | 0.0918 | 0.0686 | 0.5836 | 0.2660 | 0.1781 | 0.700 |
| $a+b/x^2y^2+c/\sqrt{x}y$ | 227.85 | 166.49 | 0.368 | 0.1208 | 0.0947 | 0.2792 | 0.3850 | 0.2866 | 0.372 |
| $a+b/x^2y^2+c/\sqrt{x}y^2$ | 248.35 | 177.91 | 0.250 | 0.1274 | 0.0990 | 0.1980 | 0.4129 | 0.3035 | 0.278 |
| $a+b/x^2y^2+c/\sqrt{x}\sqrt{y}$ | 210.09 | 154.63 | 0.463 | 0.1149 | 0.0897 | 0.3478 | 0.3610 | 0.2675 | 0.448 |
| $a+b/x^2y^2+cy/\sqrt{x}$ | 241.38 | 184.27 | 0.291 | 0.1248 | 0.0933 | 0.2314 | 0.4193 | 0.3077 | 0.255 |
| $a+b/x^2y^2+cy^2/\sqrt{x}$ | 189.25 | 146.52 | 0.564 | 0.1068 | 0.0759 | 0.4367 | 0.3560 | 0.2435 | 0.463 |
| $a+b/x^2y^2+c\sqrt{y}/\sqrt{x}$ | 235.22 | 169.87 | 0.327 | 0.1172 | 0.0879 | 0.3213 | 0.3762 | 0.2808 | 0.400 |
| $a+b/x^2\sqrt{y}+cy/x^2$ | 200.35 | 144.27 | 0.512 | 0.1015 | 0.0792 | 0.4908 | 0.3300 | 0.2416 | 0.539 |
| $a+b/x^2\sqrt{y}+cy^2/x^2$ | 282.67 | 195.46 | 0.028 | 0.1330 | 0.0997 | 0.1270 | 0.4524 | 0.3257 | 0.133 |
| $a+b/x^2\sqrt{y}+c\sqrt{y}/x^2$ | 160.40 | 116.11 | 0.687 | 0.0910 | 0.0668 | 0.5908 | 0.2792 | 0.1932 | 0.670 |
| $a+b/x^2\sqrt{y}+c/\sqrt{x}y$ | 228.62 | 166.89 | 0.364 | 0.1210 | 0.0948 | 0.2767 | 0.3860 | 0.2871 | 0.369 |
| $a+b/x^2\sqrt{y}+c/\sqrt{x}y^2$ | 249.39 | 178.15 | 0.243 | 0.1277 | 0.0990 | 0.1948 | 0.4141 | 0.3037 | 0.273 |
| $a+b/x^2\sqrt{y}+c/\sqrt{x}\sqrt{y}$ | 210.58 | 154.98 | 0.460 | 0.1151 | 0.0897 | 0.3463 | 0.3616 | 0.2679 | 0.446 |
| $a+b/x^2\sqrt{y}+cy/\sqrt{x}$ | 240.92 | 184.06 | 0.294 | 0.1245 | 0.0932 | 0.2343 | 0.4182 | 0.3071 | 0.259 |
| $a+b/x^2\sqrt{y}+cy^2/\sqrt{x}$ | 189.35 | 146.75 | 0.564 | 0.1068 | 0.0760 | 0.4370 | 0.3559 | 0.2436 | 0.463 |
| $a+b/x^2\sqrt{y}+c\sqrt{y}/\sqrt{x}$ | 237.37 | 171.64 | 0.314 | 0.1178 | 0.0886 | 0.3143 | 0.3791 | 0.2838 | 0.391 |
| $a+by/x^2+cy^2/x^2$ | 289.78 | 211.05 | -0.022 | 0.1373 | 0.1065 | 0.0693 | 0.4673 | 0.3507 | 0.075 |
| $a+by/x^2+c\sqrt{y}/x^2$ | 242.97 | 167.10 | 0.282 | 0.1161 | 0.0892 | 0.3347 | 0.3910 | 0.2813 | 0.352 |
| $a+by/x^2+c/\sqrt{x}y$ | 233.47 | 169.13 | 0.337 | 0.1223 | 0.0953 | 0.2610 | 0.3920 | 0.2899 | 0.349 |
| $a+by/x^2+c/\sqrt{x}y^2$ | 253.65 | 180.04 | 0.217 | 0.1287 | 0.0994 | 0.1816 | 0.4193 | 0.3062 | 0.255 |
| $a+by/x^2+c/\sqrt{x}\sqrt{y}$ | 215.75 | 158.20 | 0.434 | 0.1165 | 0.0907 | 0.3295 | 0.3681 | 0.2724 | 0.426 |
| $a+by/x^2+cy/\sqrt{x}$ | 239.43 | 183.62 | 0.303 | 0.1237 | 0.0927 | 0.2447 | 0.4151 | 0.3054 | 0.270 |
| $a+by/x^2+cy^2/\sqrt{x}$ | 189.71 | 147.53 | 0.562 | 0.1066 | 0.0761 | 0.4385 | 0.3553 | 0.2440 | 0.465 |

(continued on next page)

**Table 4 – continued from previous page**

| Functional form | $T_{eff}$ (K) RMSE | MAD | $R^2_{ap}$ | Radius ($R_\odot$) RMSE | MAD | $R^2_{ap}$ | log (L/$L_\odot$) RMSE | MAD | $R^2_{ap}$ |
|---|---|---|---|---|---|---|---|---|---|
| $a+by/x^2+c\sqrt{y}/\sqrt{x}$ | 240.56 | 172.98 | 0.296 | 0.1190 | 0.0895 | 0.3005 | 0.3837 | 0.2874 | 0.376 |
| $a+by^2/x^2+c\sqrt{y}/x^2$ | 288.23 | 206.05 | -0.011 | 0.1360 | 0.1039 | 0.0866 | 0.4632 | 0.3421 | 0.091 |
| $a+by^2/x^2+c/\sqrt{x}y$ | 240.33 | 174.12 | 0.297 | 0.1242 | 0.0967 | 0.2380 | 0.4013 | 0.2972 | 0.318 |
| $a+by^2/x^2+c/\sqrt{x}y^2$ | 258.15 | 182.08 | 0.189 | 0.1299 | 0.0997 | 0.1674 | 0.4254 | 0.3096 | 0.233 |
| $a+by^2/x^2+c/\sqrt{x}\sqrt{y}$ | 224.55 | 164.57 | 0.387 | 0.1191 | 0.0927 | 0.2995 | 0.3802 | 0.2821 | 0.387 |
| $a+by^2/x^2+cy/\sqrt{x}$ | 236.42 | 182.72 | 0.320 | 0.1219 | 0.0918 | 0.2660 | 0.4088 | 0.3019 | 0.292 |
| $a+by^2/x^2+cy^2/\sqrt{x}$ | 190.43 | 149.27 | 0.559 | 0.1062 | 0.0765 | 0.4433 | 0.3537 | 0.2446 | 0.470 |
| $a+by^2/x^2+c\sqrt{y}/\sqrt{x}$ | 233.03 | 162.78 | 0.339 | 0.1176 | 0.0879 | 0.3174 | 0.3750 | 0.2757 | 0.404 |
| $a+b\sqrt{y}/x^2+c/\sqrt{x}y$ | 231.10 | 168.07 | 0.350 | 0.1217 | 0.0951 | 0.2688 | 0.3890 | 0.2886 | 0.359 |
| $a+b\sqrt{y}/x^2+c/\sqrt{x}y^2$ | 251.70 | 178.95 | 0.229 | 0.1283 | 0.0991 | 0.1877 | 0.4169 | 0.3047 | 0.263 |
| $a+b\sqrt{y}/x^2+c/\sqrt{x}\sqrt{y}$ | 213.10 | 156.58 | 0.447 | 0.1158 | 0.0902 | 0.3382 | 0.3648 | 0.2701 | 0.436 |
| $a+b\sqrt{y}/x^2+cy/\sqrt{x}$ | 240.16 | 183.82 | 0.298 | 0.1241 | 0.0929 | 0.2395 | 0.4166 | 0.3062 | 0.265 |
| $a+b\sqrt{y}/x^2+cy^2/\sqrt{x}$ | 189.53 | 147.14 | 0.563 | 0.1067 | 0.0760 | 0.4377 | 0.3556 | 0.2438 | 0.464 |
| $a+b\sqrt{y}/x^2+c\sqrt{y}/\sqrt{x}$ | 239.69 | 172.98 | 0.301 | 0.1186 | 0.0893 | 0.3052 | 0.3823 | 0.2866 | 0.381 |
| $a+b/\sqrt{x}y+c/\sqrt{x}y^2$ | 154.95 | 118.91 | 0.708 | 0.0906 | 0.0656 | 0.5943 | 0.2862 | 0.1931 | 0.653 |
| $a+b/\sqrt{x}y+c/\sqrt{x}\sqrt{y}$ | 184.05 | 122.06 | 0.588 | 0.0930 | 0.0681 | 0.5728 | 0.3085 | 0.2144 | 0.597 |
| $a+b/\sqrt{x}y+cy/\sqrt{x}$ | 229.70 | 173.24 | 0.358 | 0.1201 | 0.0901 | 0.2883 | 0.3944 | 0.2841 | 0.341 |
| $a+b/\sqrt{x}y+cy^2/\sqrt{x}$ | 191.05 | 151.54 | 0.556 | 0.1062 | 0.0754 | 0.4430 | 0.3508 | 0.2424 | 0.479 |
| $a+b/\sqrt{x}y+c\sqrt{y}/\sqrt{x}$ | 265.52 | 198.56 | 0.142 | 0.1282 | 0.1023 | 0.1885 | 0.4255 | 0.3257 | 0.233 |
| $a+b/\sqrt{x}y^2+c/\sqrt{x}\sqrt{y}$ | 161.30 | 116.53 | 0.683 | 0.0892 | 0.0653 | 0.6072 | 0.2874 | 0.1962 | 0.650 |
| $a+b/\sqrt{x}y^2+cy/\sqrt{x}$ | 233.67 | 175.27 | 0.336 | 0.1222 | 0.0912 | 0.2627 | 0.4027 | 0.2895 | 0.313 |
| $a+b/\sqrt{x}y^2+cy^2/\sqrt{x}$ | 190.86 | 150.94 | 0.557 | 0.1065 | 0.0753 | 0.4398 | 0.3524 | 0.2423 | 0.474 |
| $a+b/\sqrt{x}y^2+c\sqrt{y}/\sqrt{x}$ | 273.26 | 203.79 | 0.091 | 0.1298 | 0.1031 | 0.1677 | 0.4341 | 0.3331 | 0.202 |
| $a+b/\sqrt{x}\sqrt{y}+cy/\sqrt{x}$ | 226.11 | 171.56 | 0.378 | 0.1181 | 0.0889 | 0.3112 | 0.3873 | 0.2796 | 0.365 |
| $a+b/\sqrt{x}\sqrt{y}+cy^2/\sqrt{x}$ | 191.13 | 152.00 | 0.556 | 0.1058 | 0.0756 | 0.4470 | 0.3491 | 0.2424 | 0.484 |
| $a+b/\sqrt{x}\sqrt{y}+c\sqrt{y}/\sqrt{x}$ | 256.93 | 192.11 | 0.197 | 0.1258 | 0.0997 | 0.2189 | 0.4154 | 0.3173 | 0.269 |
| $a+by/\sqrt{x}+cy^2/\sqrt{x}$ | 183.77 | 147.78 | 0.589 | 0.0972 | 0.0745 | 0.5337 | 0.3235 | 0.2287 | 0.557 |
| $a+by/\sqrt{x}+c\sqrt{y}/\sqrt{x}$ | 213.53 | 165.50 | 0.445 | 0.1114 | 0.0844 | 0.3872 | 0.3642 | 0.2631 | 0.438 |
| $a+by^2/\sqrt{x}+c\sqrt{y}/\sqrt{x}$ | 189.85 | 152.44 | 0.561 | 0.1027 | 0.0765 | 0.4792 | 0.3380 | 0.2388 | 0.516 |
| Single EW ratio, double component functions result (x/z) | | | | | | | | | |
| $a+bx/z+cx/z^2$ | 261.95 | 196.47 | 0.165 | 0.1363 | 0.1111 | 0.0824 | 0.4528 | 0.3618 | 0.131 |
| $a+bx/z+cx/\sqrt{z}$ | 163.69 | 122.60 | 0.674 | 0.0935 | 0.0679 | 0.5687 | 0.2941 | 0.2067 | 0.634 |
| $a+bx/z+cxz$ | 124.97 | 95.65 | 0.810 | 0.0709 | 0.0482 | 0.7519 | 0.2542 | 0.1862 | 0.726 |
| $a+bx/z+cxz^2$ | 153.04 | 117.63 | 0.715 | 0.0827 | 0.0656 | 0.6623 | 0.3041 | 0.2433 | 0.608 |
| $a+bx/z+cx\sqrt{z}$ | 117.06 | 90.26 | 0.833 | 0.0693 | 0.0444 | 0.7628 | 0.2358 | 0.1555 | 0.764 |
| $a+bx/z+cx^2/z$ | 163.47 | 116.58 | 0.675 | 0.1007 | 0.0763 | 0.4996 | 0.3160 | 0.2390 | 0.577 |
| $a+bx/z+cx^2/z^2$ | 290.31 | 210.64 | -0.025 | 0.1456 | 0.1139 | -0.0470 | 0.4993 | 0.3872 | -0.056 |
| $a+bx/z+cx^2/\sqrt{z}$ | 139.46 | 106.46 | 0.763 | 0.0872 | 0.0633 | 0.6246 | 0.2759 | 0.1983 | 0.677 |
| $a+bx/z+cx^2z$ | 135.86 | 107.88 | 0.775 | 0.0781 | 0.0592 | 0.6991 | 0.2816 | 0.2219 | 0.664 |
| $a+bx/z+cx^2z^2$ | 162.20 | 127.42 | 0.680 | 0.0891 | 0.0726 | 0.6078 | 0.3250 | 0.2647 | 0.552 |
| $a+bx/z+cx^2\sqrt{z}$ | 123.61 | 96.96 | 0.814 | 0.0745 | 0.0540 | 0.7257 | 0.2603 | 0.1906 | 0.713 |
| $a+bx/z+c\sqrt{x}/z$ | 152.31 | 106.32 | 0.718 | 0.0973 | 0.0759 | 0.5326 | 0.2929 | 0.2121 | 0.636 |
| $a+bx/z+c\sqrt{x}/z^2$ | 240.18 | 183.02 | 0.298 | 0.1292 | 0.1043 | 0.1755 | 0.4201 | 0.3313 | 0.252 |
| $a+bx/z+c\sqrt{x}/\sqrt{z}$ | 281.94 | 201.36 | 0.033 | 0.1392 | 0.1098 | 0.0439 | 0.4773 | 0.3644 | 0.035 |
| $a+bx/z+c\sqrt{x}z$ | 124.54 | 96.14 | 0.811 | 0.0691 | 0.0432 | 0.7645 | 0.2462 | 0.1742 | 0.743 |
| $a+bx/z+c\sqrt{x}z^2$ | 150.52 | 118.76 | 0.724 | 0.0802 | 0.0623 | 0.6821 | 0.2957 | 0.2340 | 0.630 |
| $a+bx/z+c\sqrt{x}\sqrt{z}$ | 121.97 | 90.99 | 0.819 | 0.0692 | 0.0429 | 0.7635 | 0.2332 | 0.1411 | 0.770 |
| $a+bx/z+c/xz$ | 224.64 | 163.85 | 0.386 | 0.1091 | 0.0817 | 0.4123 | 0.3698 | 0.2738 | 0.421 |
| $a+bx/z+c/xz^2$ | 215.41 | 155.94 | 0.435 | 0.1110 | 0.0812 | 0.3916 | 0.3657 | 0.2575 | 0.433 |
| $a+bx/z+c/x\sqrt{z}$ | 234.60 | 168.71 | 0.330 | 0.1117 | 0.0848 | 0.3841 | 0.3839 | 0.2867 | 0.376 |
| $a+bx/z+cz/x$ | 275.94 | 188.61 | 0.074 | 0.1317 | 0.0993 | 0.1430 | 0.4590 | 0.3352 | 0.107 |
| $a+bx/z+cz^2/x$ | 278.39 | 208.53 | 0.057 | 0.1438 | 0.1077 | -0.0208 | 0.4953 | 0.3788 | -0.039 |
| $a+bx/z+c\sqrt{z}/x$ | 259.92 | 181.53 | 0.178 | 0.1227 | 0.0936 | 0.2571 | 0.4277 | 0.3181 | 0.225 |
| $a+bx/z+c/x^2z$ | 262.31 | 183.33 | 0.163 | 0.1237 | 0.0948 | 0.2442 | 0.4317 | 0.3220 | 0.210 |
| $a+bx/z+c/x^2z^2$ | 251.80 | 179.33 | 0.229 | 0.1194 | 0.0919 | 0.2966 | 0.4137 | 0.3123 | 0.275 |
| $a+bx/z+c/x^2\sqrt{z}$ | 265.91 | 184.69 | 0.140 | 0.1254 | 0.0957 | 0.2234 | 0.4383 | 0.3248 | 0.186 |
| $a+bx/z+cz/x^2$ | 272.79 | 186.76 | 0.095 | 0.1290 | 0.0973 | 0.1783 | 0.4516 | 0.3296 | 0.136 |
| $a+bx/z+cz^2/x^2$ | 276.51 | 187.73 | 0.070 | 0.1313 | 0.0982 | 0.1493 | 0.4593 | 0.3324 | 0.106 |
| $a+bx/z+c\sqrt{z}/x^2$ | 270.92 | 186.25 | 0.107 | 0.1280 | 0.0968 | 0.1914 | 0.4479 | 0.3284 | 0.150 |
| $a+bx/z+c/\sqrt{x}z$ | 190.60 | 135.29 | 0.558 | 0.1004 | 0.0721 | 0.5026 | 0.3242 | 0.2189 | 0.555 |
| $a+bx/z+c/\sqrt{x}z^2$ | 210.08 | 147.32 | 0.463 | 0.1148 | 0.0899 | 0.3492 | 0.3686 | 0.2731 | 0.424 |
| $a+bx/z+c/\sqrt{x}\sqrt{z}$ | 195.34 | 140.31 | 0.536 | 0.0979 | 0.0693 | 0.5265 | 0.3244 | 0.2237 | 0.554 |
| $a+bx/z+cz/\sqrt{x}$ | 247.35 | 180.04 | 0.256 | 0.1325 | 0.0978 | 0.1335 | 0.4551 | 0.3407 | 0.123 |
| $a+bx/z+cz^2/\sqrt{x}$ | 158.33 | 131.49 | 0.695 | 0.0862 | 0.0656 | 0.6330 | 0.3112 | 0.2500 | 0.590 |
| $a+bx/z+c\sqrt{z}/\sqrt{x}$ | 276.51 | 190.05 | 0.070 | 0.1331 | 0.1016 | 0.1255 | 0.4614 | 0.3406 | 0.098 |
| $a+bx/z^2+cx/\sqrt{z}$ | 208.92 | 162.50 | 0.469 | 0.1133 | 0.0878 | 0.3660 | 0.3583 | 0.2713 | 0.456 |
| $a+bx/z^2+cxz$ | 128.29 | 95.32 | 0.800 | 0.0724 | 0.0510 | 0.7412 | 0.2670 | 0.2030 | 0.698 |
| $a+bx/z^2+cxz^2$ | 156.25 | 115.42 | 0.703 | 0.0853 | 0.0662 | 0.6408 | 0.3190 | 0.2502 | 0.569 |
| $a+bx/z^2+cx\sqrt{z}$ | 117.10 | 90.37 | 0.833 | 0.0689 | 0.0438 | 0.7653 | 0.2380 | 0.1582 | 0.760 |
| $a+bx/z^2+cx^2/z$ | 204.73 | 155.88 | 0.490 | 0.1156 | 0.0932 | 0.3407 | 0.3625 | 0.2876 | 0.443 |
| $a+bx/z^2+cx^2/z^2$ | 203.32 | 147.31 | 0.497 | 0.1189 | 0.0944 | 0.3019 | 0.3687 | 0.2835 | 0.424 |
| $a+bx/z^2+cx^2/\sqrt{z}$ | 158.91 | 123.57 | 0.693 | 0.0948 | 0.0706 | 0.5559 | 0.2939 | 0.2143 | 0.634 |
| $a+bx/z^2+cx^2z$ | 138.06 | 103.69 | 0.768 | 0.0795 | 0.0606 | 0.6878 | 0.2927 | 0.2325 | 0.637 |
| $a+bx/z^2+cx^2z^2$ | 162.62 | 123.95 | 0.678 | 0.0905 | 0.0724 | 0.5953 | 0.3349 | 0.2654 | 0.525 |
| $a+bx/z^2+cx^2\sqrt{z}$ | 124.03 | 96.10 | 0.813 | 0.0748 | 0.0544 | 0.7237 | 0.2659 | 0.1997 | 0.700 |
| $a+bx/z^2+c\sqrt{x}/z$ | 237.41 | 163.01 | 0.314 | 0.1243 | 0.0881 | 0.2374 | 0.4379 | 0.3088 | 0.188 |
| $a+bx/z^2+c\sqrt{x}/z^2$ | 199.94 | 151.73 | 0.514 | 0.1167 | 0.0939 | 0.3280 | 0.3611 | 0.2796 | 0.448 |
| $a+bx/z^2+c\sqrt{x}/\sqrt{z}$ | 266.20 | 196.04 | 0.138 | 0.1364 | 0.1107 | 0.0815 | 0.4573 | 0.3577 | 0.114 |
| $a+bx/z^2+c\sqrt{x}z$ | 128.75 | 98.34 | 0.798 | 0.0707 | 0.0470 | 0.7531 | 0.2607 | 0.1907 | 0.712 |
| $a+bx/z^2+c\sqrt{x}z^2$ | 155.23 | 117.35 | 0.707 | 0.0835 | 0.0635 | 0.6558 | 0.3135 | 0.2429 | 0.584 |
| $a+bx/z^2+c\sqrt{x}\sqrt{z}$ | 121.90 | 91.10 | 0.819 | 0.0685 | 0.0412 | 0.7684 | 0.2343 | 0.1460 | 0.767 |
| $a+bx/z^2+c/xz$ | 230.13 | 170.49 | 0.356 | 0.1146 | 0.0891 | 0.3514 | 0.3800 | 0.2818 | 0.388 |
| $a+bx/z^2+c/xz^2$ | 223.50 | 164.38 | 0.392 | 0.1157 | 0.0878 | 0.3389 | 0.3763 | 0.2698 | 0.400 |
| $a+bx/z^2+c/x\sqrt{z}$ | 236.60 | 173.96 | 0.319 | 0.1163 | 0.0914 | 0.3319 | 0.3900 | 0.2908 | 0.356 |
| $a+bx/z^2+cz/x$ | 264.61 | 185.26 | 0.148 | 0.1305 | 0.1016 | 0.1590 | 0.4458 | 0.3270 | 0.158 |
| $a+bx/z^2+cz^2/x$ | 268.39 | 194.12 | 0.124 | 0.1396 | 0.1059 | 0.0380 | 0.4818 | 0.3653 | 0.016 |
| $a+bx/z^2+c\sqrt{z}/x$ | 253.56 | 182.38 | 0.218 | 0.1240 | 0.0973 | 0.2414 | 0.4220 | 0.3141 | 0.245 |
| $a+bx/z^2+c/x^2z$ | 255.15 | 183.11 | 0.208 | 0.1244 | 0.0973 | 0.2354 | 0.4248 | 0.3172 | 0.235 |
| $a+bx/z^2+c/x^2z^2$ | 248.65 | 181.41 | 0.248 | 0.1219 | 0.0958 | 0.2658 | 0.4128 | 0.3103 | 0.278 |
| $a+bx/z^2+c/x^2\sqrt{z}$ | 257.44 | 183.40 | 0.194 | 0.1255 | 0.0978 | 0.2229 | 0.4293 | 0.3192 | 0.219 |

(continued on next page)

**Table 4 – continued from previous page**

| Functional form | $T_{eff}$ (K) | | | Radius ($R_\odot$) | | | log (L/$L_\odot$) | | |
|---|---|---|---|---|---|---|---|---|---|
| | RMSE | MAD | $R^2_{ap}$ | RMSE | MAD | $R^2_{ap}$ | RMSE | MAD | $R^2_{ap}$ |
| $a+bx/z^2+cz/x^2$ | 261.97 | 183.60 | 0.165 | 0.1277 | 0.0985 | 0.1943 | 0.4390 | 0.3227 | 0.183 |
| $a+bx/z^2+cz^2/x^2$ | 264.63 | 183.76 | 0.148 | 0.1294 | 0.0992 | 0.1732 | 0.4450 | 0.3248 | 0.161 |
| $a+bx/z^2+c\sqrt{z}/x^2$ | 260.70 | 183.57 | 0.173 | 0.1271 | 0.0983 | 0.2030 | 0.4362 | 0.3217 | 0.194 |
| $a+bx/z^2+c/\sqrt{x}z$ | 198.53 | 144.84 | 0.520 | 0.1041 | 0.0792 | 0.4653 | 0.3315 | 0.2357 | 0.534 |
| $a+bx/z^2+c/\sqrt{x}z^2$ | 212.14 | 153.91 | 0.452 | 0.1154 | 0.0914 | 0.3429 | 0.3669 | 0.2745 | 0.430 |
| $a+bx/z^2+c/\sqrt{x}\sqrt{z}$ | 204.70 | 150.68 | 0.490 | 0.1037 | 0.0778 | 0.4688 | 0.3368 | 0.2388 | 0.519 |
| $a+bx/z^2+cz/\sqrt{x}$ | 257.63 | 182.07 | 0.192 | 0.1353 | 0.1006 | 0.0967 | 0.4703 | 0.3472 | 0.063 |
| $a+bx/z^2+cz^2/\sqrt{x}$ | 176.07 | 136.41 | 0.623 | 0.0948 | 0.0679 | 0.5564 | 0.3493 | 0.2619 | 0.483 |
| $a+bx/z^2+c\sqrt{z}/\sqrt{x}$ | 265.20 | 187.70 | 0.144 | 0.1322 | 0.1046 | 0.1374 | 0.4487 | 0.3328 | 0.147 |
| $a+bx/\sqrt{z}+cxz$ | 120.00 | 90.69 | 0.825 | 0.0696 | 0.0462 | 0.7606 | 0.2409 | 0.1678 | 0.754 |
| $a+bx/\sqrt{z}+cxz^2$ | 134.76 | 104.73 | 0.779 | 0.0757 | 0.0556 | 0.7174 | 0.2647 | 0.2020 | 0.703 |
| $a+bx/\sqrt{z}+cx\sqrt{z}$ | 117.03 | 90.38 | 0.833 | 0.0695 | 0.0444 | 0.7615 | 0.2349 | 0.1532 | 0.766 |
| $a+bx/\sqrt{z}+cx^2/z$ | 267.86 | 201.76 | 0.127 | 0.1306 | 0.0999 | 0.1577 | 0.4324 | 0.3279 | 0.208 |
| $a+bx/\sqrt{z}+cx^2/z^2$ | 219.28 | 169.95 | 0.415 | 0.1153 | 0.0898 | 0.3439 | 0.3703 | 0.2815 | 0.419 |
| $a+bx/\sqrt{z}+cx^2/\sqrt{z}$ | 144.80 | 101.95 | 0.745 | 0.0901 | 0.0661 | 0.5992 | 0.2878 | 0.2123 | 0.649 |
| $a+bx/\sqrt{z}+cx^2z$ | 127.74 | 101.64 | 0.801 | 0.0751 | 0.0551 | 0.7213 | 0.2602 | 0.1947 | 0.713 |
| $a+bx/\sqrt{z}+cx^2z^2$ | 143.06 | 115.73 | 0.751 | 0.0813 | 0.0626 | 0.6733 | 0.2827 | 0.2183 | 0.661 |
| $a+bx/\sqrt{z}+cx^2\sqrt{z}$ | 121.95 | 96.88 | 0.819 | 0.0740 | 0.0527 | 0.7297 | 0.2524 | 0.1779 | 0.730 |
| $a+bx/\sqrt{z}+c\sqrt{x}/z$ | 154.65 | 111.47 | 0.709 | 0.0933 | 0.0704 | 0.5706 | 0.2866 | 0.1959 | 0.652 |
| $a+bx/\sqrt{z}+c\sqrt{x}/z^2$ | 203.35 | 155.83 | 0.497 | 0.1125 | 0.0879 | 0.3751 | 0.3524 | 0.2601 | 0.474 |
| $a+bx/\sqrt{z}+c\sqrt{x}/\sqrt{z}$ | 124.99 | 86.66 | 0.810 | 0.0854 | 0.0618 | 0.6397 | 0.2590 | 0.1785 | 0.716 |
| $a+bx/\sqrt{z}+c\sqrt{x}z$ | 119.92 | 88.93 | 0.825 | 0.0683 | 0.0424 | 0.7699 | 0.2349 | 0.1521 | 0.766 |
| $a+bx/\sqrt{z}+c\sqrt{x}z^2$ | 132.20 | 101.88 | 0.787 | 0.0734 | 0.0521 | 0.7341 | 0.2571 | 0.1916 | 0.720 |
| $a+bx/\sqrt{z}+c\sqrt{x}\sqrt{z}$ | 121.97 | 90.85 | 0.819 | 0.0695 | 0.0427 | 0.7614 | 0.2334 | 0.1406 | 0.769 |
| $a+bx/\sqrt{z}+c/xz$ | 258.34 | 191.99 | 0.188 | 0.1232 | 0.0939 | 0.2511 | 0.4104 | 0.3088 | 0.286 |
| $a+bx/\sqrt{z}+c/xz^2$ | 240.79 | 170.88 | 0.295 | 0.1206 | 0.0919 | 0.2822 | 0.3921 | 0.2826 | 0.348 |
| $a+bx/\sqrt{z}+c/x\sqrt{z}$ | 268.48 | 200.43 | 0.123 | 0.1275 | 0.1004 | 0.1969 | 0.4268 | 0.3266 | 0.228 |
| $a+bx/\sqrt{z}+cz/x$ | 273.03 | 209.43 | 0.093 | 0.1390 | 0.1131 | 0.0458 | 0.4547 | 0.3652 | 0.124 |
| $a+bx/\sqrt{z}+cz^2/x$ | 178.35 | 132.62 | 0.613 | 0.1089 | 0.0891 | 0.4146 | 0.3436 | 0.2721 | 0.500 |
| $a+bx/\sqrt{z}+c\sqrt{z}/x$ | 279.38 | 210.89 | 0.050 | 0.1369 | 0.1091 | 0.0742 | 0.4540 | 0.3587 | 0.127 |
| $a+bx/\sqrt{z}+c/x^2z$ | 279.28 | 211.31 | 0.051 | 0.1363 | 0.1090 | 0.0822 | 0.4526 | 0.3579 | 0.132 |
| $a+bx/\sqrt{z}+c/x^2z^2$ | 278.08 | 210.80 | 0.059 | 0.1347 | 0.1077 | 0.1037 | 0.4482 | 0.3528 | 0.149 |
| $a+bx/\sqrt{z}+c/x^2\sqrt{z}$ | 279.38 | 210.94 | 0.050 | 0.1368 | 0.1092 | 0.0757 | 0.4538 | 0.3588 | 0.128 |
| $a+bx/\sqrt{z}+cz/x^2$ | 279.12 | 209.37 | 0.052 | 0.1377 | 0.1094 | 0.0634 | 0.4556 | 0.3592 | 0.120 |
| $a+bx/\sqrt{z}+cz^2/x^2$ | 278.37 | 208.89 | 0.057 | 0.1384 | 0.1102 | 0.0546 | 0.4565 | 0.3606 | 0.117 |
| $a+bx/\sqrt{z}+c\sqrt{z}/x^2$ | 279.26 | 209.97 | 0.051 | 0.1375 | 0.1093 | 0.0671 | 0.4551 | 0.3593 | 0.122 |
| $a+bx/\sqrt{z}+c/\sqrt{x}z$ | 200.64 | 142.90 | 0.510 | 0.1035 | 0.0776 | 0.4711 | 0.3318 | 0.2339 | 0.534 |
| $a+bx/\sqrt{z}+c/\sqrt{x}z^2$ | 211.55 | 156.27 | 0.456 | 0.1146 | 0.0904 | 0.3511 | 0.3608 | 0.2679 | 0.448 |
| $a+bx/\sqrt{z}+c/\sqrt{x}\sqrt{z}$ | 214.35 | 152.83 | 0.441 | 0.1037 | 0.0759 | 0.4686 | 0.3429 | 0.2444 | 0.502 |
| $a+bx/\sqrt{z}+cz/\sqrt{x}$ | 133.00 | 97.27 | 0.785 | 0.0910 | 0.0689 | 0.5916 | 0.2817 | 0.2080 | 0.664 |
| $a+bx/\sqrt{z}+cz^2/\sqrt{x}$ | 119.78 | 92.85 | 0.825 | 0.0720 | 0.0494 | 0.7443 | 0.2433 | 0.1657 | 0.749 |
| $a+bx/\sqrt{z}+c\sqrt{z}/\sqrt{x}$ | 252.78 | 195.52 | 0.223 | 0.1350 | 0.1116 | 0.0997 | 0.4350 | 0.3547 | 0.198 |
| $a+bxz+cxz^2$ | 121.72 | 95.42 | 0.820 | 0.0704 | 0.0441 | 0.7553 | 0.2466 | 0.1563 | 0.742 |
| $a+bxz+cx\sqrt{z}$ | 117.11 | 90.75 | 0.833 | 0.0696 | 0.0447 | 0.7610 | 0.2369 | 0.1491 | 0.762 |
| $a+bxz+cx^2/z$ | 117.98 | 90.46 | 0.831 | 0.0699 | 0.0472 | 0.7590 | 0.2420 | 0.1732 | 0.752 |
| $a+bxz+cx^2/z^2$ | 126.30 | 96.29 | 0.806 | 0.0715 | 0.0499 | 0.7474 | 0.2605 | 0.1995 | 0.713 |
| $a+bxz+cx^2/\sqrt{z}$ | 115.03 | 88.97 | 0.839 | 0.0700 | 0.0481 | 0.7579 | 0.2395 | 0.1631 | 0.757 |
| $a+bxz+cx^2z$ | 127.64 | 97.62 | 0.802 | 0.0712 | 0.0461 | 0.7494 | 0.2600 | 0.1863 | 0.714 |
| $a+bxz+cx^2z^2$ | 124.29 | 96.60 | 0.812 | 0.0700 | 0.0414 | 0.7583 | 0.2482 | 0.1546 | 0.739 |
| $a+bxz+cx^2\sqrt{z}$ | 123.54 | 93.50 | 0.814 | 0.0732 | 0.0524 | 0.7358 | 0.2664 | 0.2034 | 0.699 |
| $a+bxz+c\sqrt{x}/z$ | 128.28 | 95.52 | 0.800 | 0.0722 | 0.0509 | 0.7424 | 0.2654 | 0.1990 | 0.701 |
| $a+bxz+c\sqrt{x}/z^2$ | 128.16 | 96.14 | 0.800 | 0.0730 | 0.0522 | 0.7371 | 0.2702 | 0.2081 | 0.691 |
| $a+bxz+c\sqrt{x}/\sqrt{z}$ | 125.61 | 95.20 | 0.808 | 0.0707 | 0.0476 | 0.7530 | 0.2528 | 0.1824 | 0.729 |
| $a+bxz+c\sqrt{x}z$ | 128.36 | 96.44 | 0.800 | 0.0724 | 0.0489 | 0.7411 | 0.2670 | 0.1956 | 0.698 |
| $a+bxz+c\sqrt{x}z^2$ | 121.31 | 95.36 | 0.821 | 0.0712 | 0.0471 | 0.7495 | 0.2505 | 0.1673 | 0.734 |
| $a+bxz+c\sqrt{x}\sqrt{z}$ | 120.64 | 92.14 | 0.823 | 0.0693 | 0.0416 | 0.7627 | 0.2390 | 0.1414 | 0.758 |
| $a+bxz+c/xz$ | 126.76 | 95.15 | 0.805 | 0.0705 | 0.0470 | 0.7549 | 0.2516 | 0.1736 | 0.732 |
| $a+bxz+c/xz^2$ | 122.56 | 91.84 | 0.817 | 0.0704 | 0.0453 | 0.7552 | 0.2466 | 0.1617 | 0.742 |
| $a+bxz+c/x\sqrt{z}$ | 127.87 | 95.94 | 0.801 | 0.0708 | 0.0478 | 0.7528 | 0.2552 | 0.1799 | 0.724 |
| $a+bxz+cz/x$ | 128.38 | 95.63 | 0.799 | 0.0717 | 0.0495 | 0.7461 | 0.2627 | 0.1905 | 0.707 |
| $a+bxz+cz^2/x$ | 128.43 | 95.80 | 0.799 | 0.0720 | 0.0496 | 0.7444 | 0.2633 | 0.1918 | 0.706 |
| $a+bxz+c\sqrt{z}/x$ | 128.45 | 95.92 | 0.799 | 0.0714 | 0.0491 | 0.7480 | 0.2610 | 0.1883 | 0.711 |
| $a+bxz+c/x^2z$ | 128.40 | 95.68 | 0.799 | 0.0716 | 0.0492 | 0.7472 | 0.2620 | 0.1891 | 0.709 |
| $a+bxz+c/x^2z^2$ | 128.35 | 96.16 | 0.800 | 0.0712 | 0.0486 | 0.7497 | 0.2588 | 0.1851 | 0.716 |
| $a+bxz+c/x^2\sqrt{z}$ | 128.29 | 95.36 | 0.800 | 0.0717 | 0.0493 | 0.7462 | 0.2631 | 0.1904 | 0.707 |
| $a+bxz+cz/x^2$ | 127.92 | 94.57 | 0.801 | 0.0720 | 0.0496 | 0.7443 | 0.2650 | 0.1923 | 0.702 |
| $a+bxz+cz^2/x^2$ | 127.77 | 94.29 | 0.801 | 0.0721 | 0.0497 | 0.7437 | 0.2656 | 0.1928 | 0.701 |
| $a+bxz+c\sqrt{z}/x^2$ | 128.03 | 94.79 | 0.801 | 0.0719 | 0.0495 | 0.7448 | 0.2645 | 0.1918 | 0.703 |
| $a+bxz+c/\sqrt{x}z$ | 120.93 | 91.05 | 0.822 | 0.0701 | 0.0440 | 0.7574 | 0.2432 | 0.1532 | 0.749 |
| $a+bxz+c/\sqrt{x}z^2$ | 117.77 | 89.06 | 0.831 | 0.0717 | 0.0482 | 0.7459 | 0.2520 | 0.1649 | 0.731 |
| $a+bxz+c/\sqrt{x}\sqrt{z}$ | 124.60 | 93.18 | 0.811 | 0.0699 | 0.0453 | 0.7586 | 0.2458 | 0.1628 | 0.744 |
| $a+bxz+cz/\sqrt{x}$ | 128.43 | 96.03 | 0.799 | 0.0719 | 0.0498 | 0.7445 | 0.2627 | 0.1923 | 0.708 |
| $a+bxz+cz^2/\sqrt{x}$ | 127.12 | 95.85 | 0.803 | 0.0721 | 0.0502 | 0.7433 | 0.2602 | 0.1872 | 0.713 |
| $a+bxz+c\sqrt{z}/\sqrt{x}$ | 128.33 | 96.07 | 0.800 | 0.0713 | 0.0491 | 0.7487 | 0.2594 | 0.1877 | 0.715 |
| $a+bxz^2+cx\sqrt{z}$ | 117.07 | 90.12 | 0.833 | 0.0696 | 0.0449 | 0.7611 | 0.2381 | 0.1491 | 0.760 |
| $a+bxz^2+cx^2/z$ | 135.47 | 104.36 | 0.777 | 0.0774 | 0.0596 | 0.7039 | 0.2726 | 0.2126 | 0.685 |
| $a+bxz^2+cx^2/z^2$ | 156.10 | 118.17 | 0.704 | 0.0845 | 0.0664 | 0.6478 | 0.3141 | 0.2529 | 0.582 |
| $a+bxz^2+cx^2/\sqrt{z}$ | 119.36 | 93.86 | 0.827 | 0.0731 | 0.0543 | 0.7359 | 0.2489 | 0.1829 | 0.737 |
| $a+bxz^2+cx^2z$ | 134.78 | 102.89 | 0.779 | 0.0793 | 0.0601 | 0.6894 | 0.2869 | 0.2196 | 0.651 |
| $a+bxz^2+cx^2z^2$ | 154.94 | 118.02 | 0.708 | 0.0816 | 0.0621 | 0.6716 | 0.3069 | 0.2438 | 0.601 |
| $a+bxz^2+cx^2\sqrt{z}$ | 123.79 | 96.99 | 0.814 | 0.0751 | 0.0554 | 0.7218 | 0.2644 | 0.1941 | 0.704 |
| $a+bxz^2+c\sqrt{x}/z$ | 156.45 | 115.43 | 0.702 | 0.0852 | 0.0661 | 0.6414 | 0.3186 | 0.2491 | 0.570 |
| $a+bxz^2+c\sqrt{x}/z^2$ | 152.61 | 114.72 | 0.717 | 0.0851 | 0.0663 | 0.6426 | 0.3176 | 0.2496 | 0.573 |
| $a+bxz^2+c\sqrt{x}/\sqrt{z}$ | 151.35 | 117.20 | 0.721 | 0.0812 | 0.0634 | 0.6746 | 0.2969 | 0.2309 | 0.626 |
| $a+bxz^2+c\sqrt{x}z$ | 127.14 | 100.45 | 0.803 | 0.0708 | 0.0427 | 0.7525 | 0.2515 | 0.1560 | 0.732 |
| $a+bxz^2+c\sqrt{x}z^2$ | 155.40 | 118.24 | 0.706 | 0.0825 | 0.0622 | 0.6638 | 0.3102 | 0.2439 | 0.592 |
| $a+bxz^2+c\sqrt{x}\sqrt{z}$ | 120.83 | 91.85 | 0.822 | 0.0693 | 0.0418 | 0.7629 | 0.2392 | 0.1417 | 0.758 |
| $a+bxz^2+c/xz$ | 144.15 | 107.74 | 0.747 | 0.0757 | 0.0544 | 0.7171 | 0.2732 | 0.1935 | 0.684 |
| $a+bxz^2+c/xz^2$ | 133.86 | 96.97 | 0.782 | 0.0748 | 0.0518 | 0.7241 | 0.2629 | 0.1785 | 0.707 |
| $a+bxz^2+c/x\sqrt{z}$ | 148.43 | 111.59 | 0.732 | 0.0769 | 0.0561 | 0.7081 | 0.2809 | 0.2014 | 0.666 |
| $a+bxz^2+cz/x$ | 155.10 | 115.46 | 0.707 | 0.0805 | 0.0598 | 0.6799 | 0.3001 | 0.2192 | 0.619 |
| $a+bxz^2+cz^2/x$ | 156.06 | 115.05 | 0.704 | 0.0821 | 0.0621 | 0.6674 | 0.3065 | 0.2266 | 0.602 |

(continued on next page)

**Table 4 – continued from previous page**

| Functional form | $T_{eff}$ (K) | | | Radius ($R_{\odot}$) | | | log (L/$L_{\odot}$) | | |
|---|---|---|---|---|---|---|---|---|---|
| | RMSE | MAD | $R^2_{ap}$ | RMSE | MAD | $R^2_{ap}$ | RMSE | MAD | $R^2_{ap}$ |
| $a+bxz^2+c\sqrt{z}/x$ | 153.76 | 115.17 | 0.712 | 0.0794 | 0.0588 | 0.6885 | 0.2948 | 0.2145 | 0.632 |
| $a+bxz^2+c/x^2z$ | 154.32 | 115.16 | 0.710 | 0.0797 | 0.0590 | 0.6866 | 0.2964 | 0.2157 | 0.628 |
| $a+bxz^2+c/x^2z^2$ | 151.91 | 114.35 | 0.719 | 0.0785 | 0.0578 | 0.6954 | 0.2898 | 0.2097 | 0.644 |
| $a+bxz^2+c/x^2\sqrt{z}$ | 154.99 | 115.20 | 0.708 | 0.0801 | 0.0593 | 0.6833 | 0.2987 | 0.2177 | 0.622 |
| $a+bxz^2+cz/x^2$ | 155.97 | 114.92 | 0.704 | 0.0809 | 0.0599 | 0.6767 | 0.3030 | 0.2209 | 0.611 |
| $a+bxz^2+cz^2/x^2$ | 156.23 | 114.72 | 0.703 | 0.0812 | 0.0601 | 0.6742 | 0.3045 | 0.2220 | 0.607 |
| $a+bxz^2+c\sqrt{z}/x^2$ | 155.76 | 115.03 | 0.705 | 0.0807 | 0.0597 | 0.6785 | 0.3019 | 0.2202 | 0.614 |
| $a+bxz^2+c/\sqrt{x}z$ | 126.97 | 92.89 | 0.804 | 0.0725 | 0.0487 | 0.7401 | 0.2514 | 0.1640 | 0.732 |
| $a+bxz^2+c/\sqrt{x}z^2$ | 123.56 | 89.78 | 0.814 | 0.0764 | 0.0542 | 0.7119 | 0.2669 | 0.1799 | 0.698 |
| $a+bxz^2+c/\sqrt{x}\sqrt{z}$ | 135.78 | 99.35 | 0.776 | 0.0731 | 0.0505 | 0.7363 | 0.2581 | 0.1769 | 0.718 |
| $a+bxz^2+cz/\sqrt{x}$ | 156.49 | 115.28 | 0.702 | 0.0832 | 0.0639 | 0.6578 | 0.3105 | 0.2346 | 0.592 |
| $a+bxz^2+cz^2/\sqrt{x}$ | 156.74 | 116.22 | 0.701 | 0.0850 | 0.0668 | 0.6433 | 0.3173 | 0.2490 | 0.573 |
| $a+bxz^2+c\sqrt{z}/\sqrt{x}$ | 153.56 | 115.92 | 0.713 | 0.0801 | 0.0598 | 0.6836 | 0.2961 | 0.2194 | 0.628 |
| $a+bx\sqrt{z}+cx^2/z$ | 116.24 | 88.96 | 0.836 | 0.0694 | 0.0444 | 0.7621 | 0.2336 | 0.1524 | 0.769 |
| $a+bx\sqrt{z}+cx^2/z^2$ | 116.63 | 88.85 | 0.835 | 0.0689 | 0.0438 | 0.7658 | 0.2351 | 0.1544 | 0.766 |
| $a+bx\sqrt{z}+cx^2/\sqrt{z}$ | 116.24 | 90.02 | 0.836 | 0.0696 | 0.0443 | 0.7609 | 0.2357 | 0.1546 | 0.765 |
| $a+bx\sqrt{z}+cx^2z$ | 117.09 | 90.50 | 0.833 | 0.0695 | 0.0435 | 0.7613 | 0.2355 | 0.1411 | 0.765 |
| $a+bx\sqrt{z}+cx^2z^2$ | 116.99 | 89.87 | 0.833 | 0.0696 | 0.0441 | 0.7609 | 0.2372 | 0.1448 | 0.762 |
| $a+bx\sqrt{z}+cx^2\sqrt{z}$ | 116.97 | 90.75 | 0.834 | 0.0693 | 0.0423 | 0.7630 | 0.2367 | 0.1426 | 0.763 |
| $a+bx\sqrt{z}+c\sqrt{x}/z$ | 116.95 | 91.10 | 0.834 | 0.0693 | 0.0447 | 0.7626 | 0.2388 | 0.1601 | 0.758 |
| $a+bx\sqrt{z}+c\sqrt{x}/z^2$ | 116.99 | 91.23 | 0.833 | 0.0690 | 0.0442 | 0.7646 | 0.2400 | 0.1609 | 0.756 |
| $a+bx\sqrt{z}+c\sqrt{x}/\sqrt{z}$ | 117.00 | 90.84 | 0.833 | 0.0695 | 0.0445 | 0.7616 | 0.2373 | 0.1573 | 0.761 |
| $a+bx\sqrt{z}+c\sqrt{x}z$ | 117.09 | 90.91 | 0.833 | 0.0694 | 0.0445 | 0.7619 | 0.2393 | 0.1566 | 0.757 |
| $a+bx\sqrt{z}+c\sqrt{x}z^2$ | 117.08 | 90.20 | 0.833 | 0.0695 | 0.0450 | 0.7616 | 0.2389 | 0.1519 | 0.758 |
| $a+bx\sqrt{z}+c\sqrt{x}\sqrt{z}$ | 116.66 | 90.65 | 0.834 | 0.0693 | 0.0423 | 0.7627 | 0.2400 | 0.1525 | 0.756 |
| $a+bx\sqrt{z}+c/xz$ | 115.19 | 88.72 | 0.839 | 0.0696 | 0.0443 | 0.7610 | 0.2394 | 0.1560 | 0.757 |
| $a+bx\sqrt{z}+c/xz^2$ | 117.05 | 90.58 | 0.833 | 0.0696 | 0.0442 | 0.7609 | 0.2379 | 0.1511 | 0.760 |
| $a+bx\sqrt{z}+c/x\sqrt{z}$ | 113.81 | 87.30 | 0.842 | 0.0696 | 0.0443 | 0.7610 | 0.2402 | 0.1582 | 0.756 |
| $a+bx\sqrt{z}+cz/x$ | 111.11 | 84.02 | 0.850 | 0.0696 | 0.0443 | 0.7609 | 0.2414 | 0.1606 | 0.753 |
| $a+bx\sqrt{z}+cz^2/x$ | 111.79 | 83.74 | 0.848 | 0.0696 | 0.0446 | 0.7611 | 0.2415 | 0.1605 | 0.753 |
| $a+bx\sqrt{z}+c\sqrt{z}/x$ | 111.62 | 84.86 | 0.848 | 0.0696 | 0.0444 | 0.7609 | 0.2412 | 0.1603 | 0.754 |
| $a+bx\sqrt{z}+c/x^2z$ | 111.02 | 84.16 | 0.850 | 0.0696 | 0.0444 | 0.7609 | 0.2413 | 0.1603 | 0.753 |
| $a+bx\sqrt{z}+c/x^2z^2$ | 112.75 | 86.11 | 0.845 | 0.0696 | 0.0443 | 0.7610 | 0.2408 | 0.1595 | 0.754 |
| $a+bx\sqrt{z}+c/x^2\sqrt{z}$ | 110.41 | 83.47 | 0.852 | 0.0696 | 0.0443 | 0.7609 | 0.2415 | 0.1604 | 0.753 |
| $a+bx\sqrt{z}+cz/x^2$ | 109.31 | 82.18 | 0.855 | 0.0696 | 0.0443 | 0.7609 | 0.2416 | 0.1604 | 0.753 |
| $a+bx\sqrt{z}+cz^2/x^2$ | 108.99 | 81.70 | 0.855 | 0.0696 | 0.0443 | 0.7609 | 0.2417 | 0.1603 | 0.753 |
| $a+bx\sqrt{z}+c\sqrt{z}/x^2$ | 109.58 | 82.51 | 0.854 | 0.0696 | 0.0443 | 0.7609 | 0.2416 | 0.1604 | 0.753 |
| $a+bx\sqrt{z}+c/\sqrt{x}z$ | 117.11 | 90.63 | 0.833 | 0.0696 | 0.0441 | 0.7609 | 0.2373 | 0.1480 | 0.761 |
| $a+bx\sqrt{z}+c/\sqrt{x}z^2$ | 116.09 | 90.38 | 0.836 | 0.0695 | 0.0448 | 0.7612 | 0.2392 | 0.1496 | 0.758 |
| $a+bx\sqrt{z}+c/\sqrt{x}\sqrt{z}$ | 116.22 | 89.74 | 0.836 | 0.0696 | 0.0442 | 0.7611 | 0.2382 | 0.1524 | 0.760 |
| $a+bx\sqrt{z}+cz/\sqrt{x}$ | 113.61 | 86.58 | 0.843 | 0.0696 | 0.0445 | 0.7610 | 0.2411 | 0.1609 | 0.754 |
| $a+bx\sqrt{z}+cz^2/\sqrt{x}$ | 115.92 | 87.89 | 0.837 | 0.0694 | 0.0448 | 0.7622 | 0.2408 | 0.1591 | 0.754 |
| $a+bx\sqrt{z}+c\sqrt{z}/\sqrt{x}$ | 113.38 | 86.73 | 0.844 | 0.0696 | 0.0443 | 0.7609 | 0.2407 | 0.1602 | 0.754 |
| $a+bx^2/z+cx^2/z^2$ | 210.77 | 165.14 | 0.459 | 0.1163 | 0.0939 | 0.3325 | 0.3690 | 0.2907 | 0.423 |
| $a+bx^2/z+cx^2/\sqrt{z}$ | 136.44 | 107.75 | 0.774 | 0.0832 | 0.0594 | 0.6581 | 0.2690 | 0.1896 | 0.693 |
| $a+bx^2/z+cx^2z$ | 128.39 | 103.40 | 0.799 | 0.0764 | 0.0578 | 0.7116 | 0.2667 | 0.2059 | 0.699 |
| $a+bx^2/z+cx^2z^2$ | 145.87 | 116.37 | 0.741 | 0.0839 | 0.0670 | 0.6524 | 0.2939 | 0.2352 | 0.634 |
| $a+bx^2/z+cx^2\sqrt{z}$ | 121.92 | 97.40 | 0.819 | 0.0745 | 0.0539 | 0.7261 | 0.2559 | 0.1845 | 0.723 |
| $a+bx^2/z+c\sqrt{x}/z$ | 151.92 | 107.60 | 0.719 | 0.0972 | 0.0719 | 0.5338 | 0.2978 | 0.2187 | 0.624 |
| $a+bx^2/z+c\sqrt{x}/z^2$ | 199.10 | 148.65 | 0.518 | 0.1143 | 0.0908 | 0.3549 | 0.3552 | 0.2767 | 0.466 |
| $a+bx^2/z+c\sqrt{x}/\sqrt{z}$ | 195.64 | 145.32 | 0.534 | 0.1153 | 0.0876 | 0.3440 | 0.3711 | 0.2841 | 0.416 |
| $a+bx^2/z+c\sqrt{x}z$ | 116.29 | 86.60 | 0.835 | 0.0679 | 0.0420 | 0.7722 | 0.2331 | 0.1578 | 0.770 |
| $a+bx^2/z+c\sqrt{x}z^2$ | 131.74 | 101.13 | 0.789 | 0.0748 | 0.0554 | 0.7241 | 0.2630 | 0.1992 | 0.707 |
| $a+bx^2/z+c\sqrt{x}\sqrt{z}$ | 120.39 | 88.50 | 0.824 | 0.0692 | 0.0430 | 0.7636 | 0.2296 | 0.1389 | 0.777 |
| $a+bx^2/z+c/xz$ | 258.83 | 192.65 | 0.185 | 0.1239 | 0.0954 | 0.2418 | 0.4111 | 0.3094 | 0.284 |
| $a+bx^2/z+c/xz^2$ | 242.53 | 174.74 | 0.284 | 0.1212 | 0.0923 | 0.2749 | 0.3929 | 0.2830 | 0.346 |
| $a+bx^2/z+c/x\sqrt{z}$ | 268.52 | 199.95 | 0.123 | 0.1277 | 0.1005 | 0.1951 | 0.4268 | 0.3270 | 0.228 |
| $a+bx^2/z+cz/x$ | 289.37 | 219.00 | -0.019 | 0.1431 | 0.1154 | -0.0107 | 0.4773 | 0.3812 | 0.035 |
| $a+bx^2/z+cz^2/x$ | 227.74 | 166.66 | 0.369 | 0.1276 | 0.1011 | 0.1962 | 0.4183 | 0.3267 | 0.259 |
| $a+bx^2/z+c\sqrt{z}/x$ | 285.44 | 214.00 | 0.009 | 0.1377 | 0.1095 | 0.0632 | 0.4618 | 0.3618 | 0.096 |
| $a+bx^2/z+c/x^2z$ | 284.75 | 213.68 | 0.013 | 0.1371 | 0.1093 | 0.0716 | 0.4598 | 0.3604 | 0.104 |
| $a+bx^2/z+c/x^2z^2$ | 280.90 | 211.17 | 0.040 | 0.1349 | 0.1073 | 0.1016 | 0.4515 | 0.3523 | 0.136 |
| $a+bx^2/z+c/x^2\sqrt{z}$ | 285.84 | 214.08 | 0.006 | 0.1379 | 0.1098 | 0.0610 | 0.4626 | 0.3625 | 0.093 |
| $a+bx^2/z+cz/x^2$ | 287.70 | 214.18 | -0.007 | 0.1395 | 0.1105 | 0.0385 | 0.4679 | 0.3658 | 0.072 |
| $a+bx^2/z+cz^2/x^2$ | 288.68 | 214.62 | -0.014 | 0.1408 | 0.1114 | 0.0213 | 0.4715 | 0.3690 | 0.058 |
| $a+bx^2/z+c\sqrt{z}/x^2$ | 287.21 | 214.26 | -0.004 | 0.1390 | 0.1103 | 0.0454 | 0.4664 | 0.3650 | 0.078 |
| $a+bx^2/z+c/\sqrt{x}z$ | 204.59 | 144.65 | 0.491 | 0.1049 | 0.0801 | 0.4568 | 0.3335 | 0.2404 | 0.529 |
| $a+bx^2/z+c/\sqrt{x}z^2$ | 209.72 | 156.19 | 0.465 | 0.1144 | 0.0905 | 0.3543 | 0.3574 | 0.2683 | 0.459 |
| $a+bx^2/z+c/\sqrt{x}\sqrt{z}$ | 220.29 | 154.96 | 0.410 | 0.1069 | 0.0792 | 0.4359 | 0.3494 | 0.2448 | 0.483 |
| $a+bx^2/z+cz/\sqrt{x}$ | 182.82 | 124.04 | 0.593 | 0.1105 | 0.0820 | 0.3975 | 0.3582 | 0.2640 | 0.456 |
| $a+bx^2/z+cz^2/\sqrt{x}$ | 124.83 | 92.08 | 0.810 | 0.0765 | 0.0530 | 0.7114 | 0.2605 | 0.1900 | 0.712 |
| $a+bx^2/z+c\sqrt{z}/\sqrt{x}$ | 286.01 | 220.30 | 0.005 | 0.1446 | 0.1189 | -0.0321 | 0.4801 | 0.3898 | 0.024 |
| $a+bx^2/z^2+cx^2/\sqrt{z}$ | 158.58 | 124.18 | 0.694 | 0.0936 | 0.0692 | 0.5676 | 0.2929 | 0.2143 | 0.636 |
| $a+bx^2/z^2+cx^2z$ | 137.38 | 106.83 | 0.770 | 0.0789 | 0.0598 | 0.6928 | 0.2880 | 0.2315 | 0.649 |
| $a+bx^2/z^2+cx^2z^2$ | 164.11 | 128.13 | 0.672 | 0.0903 | 0.0727 | 0.5975 | 0.3325 | 0.2687 | 0.532 |
| $a+bx^2/z^2+cx^2\sqrt{z}$ | 123.72 | 96.72 | 0.814 | 0.0746 | 0.0539 | 0.7255 | 0.2627 | 0.1971 | 0.708 |
| $a+bx^2/z^2+c\sqrt{x}/z$ | 188.22 | 120.08 | 0.569 | 0.1087 | 0.0689 | 0.4167 | 0.3656 | 0.2330 | 0.434 |
| $a+bx^2/z^2+c\sqrt{x}/z^2$ | 196.62 | 144.95 | 0.530 | 0.1163 | 0.0933 | 0.3316 | 0.3571 | 0.2752 | 0.460 |
| $a+bx^2/z^2+c\sqrt{x}/\sqrt{z}$ | 288.83 | 209.43 | -0.015 | 0.1444 | 0.1144 | -0.0300 | 0.4932 | 0.3825 | -0.031 |
| $a+bx^2/z^2+c\sqrt{x}z$ | 125.83 | 98.28 | 0.807 | 0.0696 | 0.0455 | 0.7606 | 0.2527 | 0.1861 | 0.729 |
| $a+bx^2/z^2+c\sqrt{x}z^2$ | 154.23 | 119.52 | 0.711 | 0.0823 | 0.0637 | 0.6652 | 0.3072 | 0.2454 | 0.600 |
| $a+bx^2/z^2+c\sqrt{x}\sqrt{z}$ | 121.02 | 88.23 | 0.822 | 0.0684 | 0.0416 | 0.7691 | 0.2308 | 0.1387 | 0.774 |
| $a+bx^2/z^2+c/xz$ | 241.42 | 178.67 | 0.291 | 0.1177 | 0.0917 | 0.3160 | 0.3931 | 0.2955 | 0.345 |
| $a+bx^2/z^2+c/xz^2$ | 231.03 | 169.25 | 0.351 | 0.1175 | 0.0895 | 0.3179 | 0.3838 | 0.2758 | 0.376 |
| $a+bx^2/z^2+c/x\sqrt{z}$ | 249.75 | 183.60 | 0.241 | 0.1202 | 0.0944 | 0.2865 | 0.4062 | 0.3076 | 0.301 |
| $a+bx^2/z^2+cz/x$ | 281.49 | 196.36 | 0.036 | 0.1366 | 0.1051 | 0.0791 | 0.4693 | 0.3474 | 0.067 |
| $a+bx^2/z^2+cz^2/x$ | 277.30 | 200.14 | 0.064 | 0.1430 | 0.1069 | -0.0094 | 0.4943 | 0.3702 | -0.035 |
| $a+bx^2/z^2+c\sqrt{z}/x$ | 269.71 | 192.82 | 0.115 | 0.1294 | 0.1007 | 0.1730 | 0.4437 | 0.3336 | 0.166 |
| $a+bx^2/z^2+c/x^2z$ | 270.92 | 193.48 | 0.107 | 0.1298 | 0.1008 | 0.1684 | 0.4456 | 0.3357 | 0.159 |
| $a+bx^2/z^2+c/x^2z^2$ | 263.80 | 191.90 | 0.153 | 0.1268 | 0.0992 | 0.2055 | 0.4325 | 0.3290 | 0.207 |

(continued on next page)

**Table 4 – continued from previous page**

| Functional form | $T_{eff}$ (K) RMSE | $T_{eff}$ (K) MAD | $T_{eff}$ (K) $R^2_{ap}$ | Radius ($R_\odot$) RMSE | Radius ($R_\odot$) MAD | Radius ($R_\odot$) $R^2_{ap}$ | log (L/$L_\odot$) RMSE | log (L/$L_\odot$) MAD | log (L/$L_\odot$) $R^2_{ap}$ |
|---|---|---|---|---|---|---|---|---|---|
| $a+bx^2/z^2+c/x^2\sqrt{z}$ | 273.34 | 193.81 | 0.091 | 0.1309 | 0.1013 | 0.1538 | 0.4505 | 0.3375 | 0.140 |
| $a+bx^2/z^2+cz/x^2$ | 278.05 | 194.01 | 0.059 | 0.1334 | 0.1021 | 0.1212 | 0.4605 | 0.3404 | 0.101 |
| $a+bx^2/z^2+cz^2/x^2$ | 280.77 | 194.07 | 0.041 | 0.1352 | 0.1027 | 0.0979 | 0.4667 | 0.3421 | 0.077 |
| $a+bx^2/z^2+c\sqrt{z}/x^2$ | 276.75 | 193.99 | 0.068 | 0.1327 | 0.1019 | 0.1310 | 0.4576 | 0.3396 | 0.113 |
| $a+bx^2/z^2+c/\sqrt{x}z$ | 201.48 | 145.95 | 0.506 | 0.1045 | 0.0797 | 0.4612 | 0.3329 | 0.2380 | 0.530 |
| $a+bx^2/z^2+c/\sqrt{x}z^2$ | 212.10 | 155.59 | 0.453 | 0.1152 | 0.0915 | 0.3444 | 0.3645 | 0.2744 | 0.437 |
| $a+bx^2/z^2+c/\sqrt{x}\sqrt{z}$ | 211.04 | 153.43 | 0.458 | 0.1049 | 0.0785 | 0.4562 | 0.3426 | 0.2426 | 0.503 |
| $a+bx^2/z^2+cz/\sqrt{x}$ | 259.12 | 184.98 | 0.183 | 0.1359 | 0.0987 | 0.0880 | 0.4722 | 0.3433 | 0.055 |
| $a+bx^2/z^2+cz^2/\sqrt{x}$ | 171.63 | 139.69 | 0.642 | 0.0925 | 0.0683 | 0.5771 | 0.3387 | 0.2667 | 0.514 |
| $a+bx^2/z^2+c\sqrt{z}/\sqrt{x}$ | 283.17 | 200.15 | 0.024 | 0.1387 | 0.1085 | 0.0503 | 0.4746 | 0.3566 | 0.046 |
| $a+bx^2/\sqrt{z}+cx^2z$ | 122.23 | 98.12 | 0.818 | 0.0751 | 0.0550 | 0.7217 | 0.2555 | 0.1830 | 0.723 |
| $a+bx^2/\sqrt{z}+cx^2z^2$ | 126.26 | 103.60 | 0.806 | 0.0777 | 0.0599 | 0.7022 | 0.2618 | 0.1955 | 0.710 |
| $a+bx^2/\sqrt{z}+cx^2\sqrt{z}$ | 121.03 | 96.19 | 0.822 | 0.0745 | 0.0540 | 0.7259 | 0.2535 | 0.1766 | 0.728 |
| $a+bx^2/\sqrt{z}+c\sqrt{x}/z$ | 136.83 | 102.45 | 0.772 | 0.0875 | 0.0631 | 0.6216 | 0.2727 | 0.1932 | 0.685 |
| $a+bx^2/\sqrt{z}+c\sqrt{x}/z^2$ | 157.88 | 121.83 | 0.697 | 0.0953 | 0.0720 | 0.5520 | 0.2927 | 0.2120 | 0.637 |
| $a+bx^2/\sqrt{z}+c\sqrt{x}/\sqrt{z}$ | 133.75 | 97.38 | 0.782 | 0.0872 | 0.0623 | 0.6243 | 0.2755 | 0.2000 | 0.678 |
| $a+bx^2/\sqrt{z}+c\sqrt{x}z$ | 113.38 | 86.88 | 0.844 | 0.0684 | 0.0440 | 0.7689 | 0.2327 | 0.1537 | 0.771 |
| $a+bx^2/\sqrt{z}+c\sqrt{x}z^2$ | 116.45 | 90.65 | 0.835 | 0.0711 | 0.0509 | 0.7505 | 0.2425 | 0.1751 | 0.751 |
| $a+bx^2/\sqrt{z}+c\sqrt{x}\sqrt{z}$ | 119.59 | 89.82 | 0.826 | 0.0695 | 0.0427 | 0.7618 | 0.2317 | 0.1440 | 0.773 |
| $a+bx^2/\sqrt{z}+c/xz$ | 192.86 | 153.72 | 0.547 | 0.1051 | 0.0839 | 0.4546 | 0.3270 | 0.2549 | 0.547 |
| $a+bx^2/\sqrt{z}+c/xz^2$ | 193.95 | 155.48 | 0.542 | 0.1046 | 0.0842 | 0.4597 | 0.3235 | 0.2505 | 0.557 |
| $a+bx^2/\sqrt{z}+c/x\sqrt{z}$ | 190.67 | 149.87 | 0.558 | 0.1053 | 0.0834 | 0.4529 | 0.3277 | 0.2544 | 0.545 |
| $a+bx^2/\sqrt{z}+cz/x$ | 174.15 | 130.63 | 0.631 | 0.1036 | 0.0821 | 0.4698 | 0.3204 | 0.2438 | 0.565 |
| $a+bx^2/\sqrt{z}+cz^2/x$ | 131.28 | 98.93 | 0.790 | 0.0905 | 0.0685 | 0.5954 | 0.2810 | 0.2084 | 0.665 |
| $a+bx^2/\sqrt{z}+c\sqrt{z}/x$ | 182.91 | 137.68 | 0.593 | 0.1050 | 0.0825 | 0.4557 | 0.3257 | 0.2466 | 0.550 |
| $a+bx^2/\sqrt{z}+c/x^2z$ | 185.69 | 140.96 | 0.580 | 0.1052 | 0.0823 | 0.4532 | 0.3269 | 0.2487 | 0.547 |
| $a+bx^2/\sqrt{z}+c/x^2z^2$ | 187.03 | 143.57 | 0.574 | 0.1052 | 0.0822 | 0.4531 | 0.3272 | 0.2504 | 0.546 |
| $a+bx^2/\sqrt{z}+c/x^2\sqrt{z}$ | 185.31 | 140.17 | 0.582 | 0.1052 | 0.0823 | 0.4532 | 0.3268 | 0.2481 | 0.548 |
| $a+bx^2/\sqrt{z}+cz/x^2$ | 184.36 | 138.42 | 0.586 | 0.1052 | 0.0824 | 0.4535 | 0.3264 | 0.2465 | 0.549 |
| $a+bx^2/\sqrt{z}+cz^2/x^2$ | 182.84 | 137.39 | 0.593 | 0.1051 | 0.0827 | 0.4547 | 0.3257 | 0.2463 | 0.551 |
| $a+bx^2/\sqrt{z}+c\sqrt{z}/x^2$ | 184.72 | 138.98 | 0.585 | 0.1052 | 0.0823 | 0.4533 | 0.3266 | 0.2470 | 0.548 |
| $a+bx^2/\sqrt{z}+c/\sqrt{x}z$ | 183.96 | 140.24 | 0.588 | 0.0990 | 0.0779 | 0.5164 | 0.3030 | 0.2249 | 0.611 |
| $a+bx^2/\sqrt{z}+c/\sqrt{x}z^2$ | 176.33 | 135.73 | 0.622 | 0.1000 | 0.0774 | 0.5060 | 0.3031 | 0.2264 | 0.611 |
| $a+bx^2/\sqrt{z}+c/\sqrt{x}\sqrt{z}$ | 192.18 | 152.56 | 0.551 | 0.1015 | 0.0813 | 0.4917 | 0.3147 | 0.2389 | 0.580 |
| $a+bx^2/\sqrt{z}+cz/\sqrt{x}$ | 118.95 | 87.45 | 0.828 | 0.0849 | 0.0596 | 0.6444 | 0.2655 | 0.1857 | 0.701 |
| $a+bx^2/\sqrt{z}+cz^2/\sqrt{x}$ | 104.25 | 77.52 | 0.868 | 0.0705 | 0.0482 | 0.7545 | 0.2343 | 0.1619 | 0.767 |
| $a+bx^2/\sqrt{z}+c\sqrt{z}/\sqrt{x}$ | 160.76 | 119.16 | 0.686 | 0.1000 | 0.0774 | 0.5065 | 0.3094 | 0.2334 | 0.595 |
| $a+bx^2z+cx^2z^2$ | 127.05 | 100.89 | 0.804 | 0.0747 | 0.0525 | 0.7244 | 0.2628 | 0.1908 | 0.707 |
| $a+bx^2z+cx^2\sqrt{z}$ | 121.80 | 96.34 | 0.820 | 0.0746 | 0.0536 | 0.7252 | 0.2556 | 0.1812 | 0.723 |
| $a+bx^2z+c\sqrt{x}/z$ | 138.06 | 103.33 | 0.768 | 0.0795 | 0.0607 | 0.6880 | 0.2922 | 0.2312 | 0.638 |
| $a+bx^2z+c\sqrt{x}/z^2$ | 136.19 | 103.75 | 0.774 | 0.0797 | 0.0612 | 0.6864 | 0.2934 | 0.2345 | 0.635 |
| $a+bx^2z+c\sqrt{x}/\sqrt{z}$ | 135.49 | 107.54 | 0.777 | 0.0774 | 0.0579 | 0.7043 | 0.2777 | 0.2114 | 0.673 |
| $a+bx^2z+c\sqrt{x}z$ | 129.06 | 98.16 | 0.797 | 0.0722 | 0.0477 | 0.7424 | 0.2653 | 0.1926 | 0.702 |
| $a+bx^2z+c\sqrt{x}z^2$ | 137.41 | 104.26 | 0.770 | 0.0797 | 0.0614 | 0.6866 | 0.2927 | 0.2323 | 0.637 |
| $a+bx^2z+c\sqrt{x}\sqrt{z}$ | 119.51 | 91.23 | 0.826 | 0.0694 | 0.0421 | 0.7624 | 0.2396 | 0.1435 | 0.757 |
| $a+bx^2z+c/xz$ | 131.81 | 101.08 | 0.789 | 0.0736 | 0.0526 | 0.7325 | 0.2611 | 0.1883 | 0.711 |
| $a+bx^2z+c/xz^2$ | 124.30 | 93.76 | 0.812 | 0.0731 | 0.0506 | 0.7359 | 0.2534 | 0.1742 | 0.728 |
| $a+bx^2z+c/x\sqrt{z}$ | 134.55 | 103.53 | 0.780 | 0.0744 | 0.0538 | 0.7270 | 0.2669 | 0.1955 | 0.698 |
| $a+bx^2z+cz/x$ | 137.94 | 104.82 | 0.769 | 0.0768 | 0.0562 | 0.7086 | 0.2810 | 0.2102 | 0.665 |
| $a+bx^2z+cz^2/x$ | 138.15 | 103.94 | 0.768 | 0.0783 | 0.0585 | 0.6976 | 0.2862 | 0.2164 | 0.653 |
| $a+bx^2z+c\sqrt{z}/x$ | 137.41 | 105.05 | 0.770 | 0.0760 | 0.0556 | 0.7146 | 0.2771 | 0.2068 | 0.675 |
| $a+bx^2z+c/x^2z$ | 137.58 | 104.90 | 0.770 | 0.0760 | 0.0556 | 0.7145 | 0.2779 | 0.2077 | 0.673 |
| $a+bx^2z+c/x^2z^2$ | 136.34 | 104.77 | 0.774 | 0.0753 | 0.0549 | 0.7199 | 0.2729 | 0.2023 | 0.684 |
| $a+bx^2z+c/x^2\sqrt{z}$ | 137.86 | 104.73 | 0.769 | 0.0763 | 0.0559 | 0.7124 | 0.2796 | 0.2092 | 0.669 |
| $a+bx^2z+cz/x^2$ | 138.13 | 104.13 | 0.768 | 0.0769 | 0.0563 | 0.7083 | 0.2827 | 0.2118 | 0.661 |
| $a+bx^2z+cz^2/x^2$ | 138.16 | 103.82 | 0.768 | 0.0771 | 0.0564 | 0.7064 | 0.2839 | 0.2125 | 0.659 |
| $a+bx^2z+c\sqrt{z}/x^2$ | 138.09 | 104.32 | 0.768 | 0.0767 | 0.0562 | 0.7094 | 0.2819 | 0.2112 | 0.663 |
| $a+bx^2z+c/\sqrt{x}z$ | 120.36 | 90.58 | 0.824 | 0.0719 | 0.0487 | 0.7450 | 0.2461 | 0.1622 | 0.743 |
| $a+bx^2z+c/\sqrt{x}z^2$ | 116.60 | 87.99 | 0.835 | 0.0747 | 0.0530 | 0.7245 | 0.2584 | 0.1764 | 0.717 |
| $a+bx^2z+c/\sqrt{x}\sqrt{z}$ | 126.89 | 95.00 | 0.804 | 0.0721 | 0.0501 | 0.7434 | 0.2510 | 0.1735 | 0.733 |
| $a+bx^2z+cz/\sqrt{x}$ | 138.16 | 103.77 | 0.768 | 0.0787 | 0.0595 | 0.6938 | 0.2879 | 0.2206 | 0.649 |
| $a+bx^2z+cz^2/\sqrt{x}$ | 138.15 | 103.51 | 0.768 | 0.0797 | 0.0612 | 0.6864 | 0.2926 | 0.2317 | 0.637 |
| $a+bx^2z+c\sqrt{z}/\sqrt{x}$ | 137.31 | 105.69 | 0.771 | 0.0767 | 0.0560 | 0.7096 | 0.2783 | 0.2071 | 0.672 |
| $a+bx^2z^2+cx^2\sqrt{z}$ | 122.64 | 97.16 | 0.817 | 0.0745 | 0.0533 | 0.7256 | 0.2571 | 0.1838 | 0.720 |
| $a+bx^2z^2+c\sqrt{x}/z$ | 162.60 | 123.74 | 0.678 | 0.0905 | 0.0722 | 0.5952 | 0.3349 | 0.2652 | 0.525 |
| $a+bx^2z^2+c\sqrt{x}/z^2$ | 157.37 | 120.77 | 0.699 | 0.0897 | 0.0719 | 0.6025 | 0.3309 | 0.2625 | 0.536 |
| $a+bx^2z^2+c\sqrt{x}/\sqrt{z}$ | 160.47 | 126.86 | 0.687 | 0.0877 | 0.0710 | 0.6204 | 0.3180 | 0.2548 | 0.572 |
| $a+bx^2z^2+c\sqrt{x}z$ | 128.88 | 100.83 | 0.798 | 0.0712 | 0.0441 | 0.7496 | 0.2564 | 0.1704 | 0.721 |
| $a+bx^2z^2+c\sqrt{x}z^2$ | 155.33 | 118.34 | 0.706 | 0.0821 | 0.0623 | 0.6671 | 0.3087 | 0.2443 | 0.596 |
| $a+bx^2z^2+c\sqrt{x}\sqrt{z}$ | 120.00 | 90.44 | 0.825 | 0.0694 | 0.0421 | 0.7624 | 0.2394 | 0.1423 | 0.757 |
| $a+bx^2z^2+c/xz$ | 147.82 | 112.82 | 0.734 | 0.0789 | 0.0583 | 0.6926 | 0.2815 | 0.2058 | 0.664 |
| $a+bx^2z^2+c/xz^2$ | 135.87 | 99.87 | 0.775 | 0.0776 | 0.0556 | 0.7028 | 0.2696 | 0.1893 | 0.692 |
| $a+bx^2z^2+c/x\sqrt{z}$ | 153.04 | 117.91 | 0.715 | 0.0804 | 0.0603 | 0.6805 | 0.2906 | 0.2141 | 0.642 |
| $a+bx^2z^2+cz/x$ | 162.02 | 124.28 | 0.681 | 0.0854 | 0.0653 | 0.6396 | 0.3146 | 0.2351 | 0.581 |
| $a+bx^2z^2+cz^2/x$ | 163.94 | 125.86 | 0.673 | 0.0884 | 0.0694 | 0.6138 | 0.3261 | 0.2490 | 0.550 |
| $a+bx^2z^2+c\sqrt{z}/x$ | 160.01 | 123.42 | 0.689 | 0.0838 | 0.0642 | 0.6532 | 0.3075 | 0.2300 | 0.599 |
| $a+bx^2z^2+c/x^2z$ | 160.48 | 123.33 | 0.687 | 0.0839 | 0.0639 | 0.6524 | 0.3087 | 0.2288 | 0.596 |
| $a+bx^2z^2+c/x^2z^2$ | 157.48 | 121.89 | 0.698 | 0.0826 | 0.0626 | 0.6634 | 0.3012 | 0.2231 | 0.615 |
| $a+bx^2z^2+c/x^2\sqrt{z}$ | 161.35 | 123.56 | 0.683 | 0.0844 | 0.0642 | 0.6482 | 0.3113 | 0.2304 | 0.589 |
| $a+bx^2z^2+cz/x^2$ | 162.72 | 123.62 | 0.678 | 0.0854 | 0.0648 | 0.6398 | 0.3162 | 0.2328 | 0.576 |
| $a+bx^2z^2+cz^2/x^2$ | 163.13 | 123.53 | 0.676 | 0.0859 | 0.0650 | 0.6360 | 0.3182 | 0.2339 | 0.571 |
| $a+bx^2z^2+c\sqrt{z}/x^2$ | 162.40 | 123.65 | 0.679 | 0.0851 | 0.0647 | 0.6421 | 0.3149 | 0.2322 | 0.580 |
| $a+bx^2z^2+c/\sqrt{x}z$ | 126.61 | 92.70 | 0.805 | 0.0743 | 0.0518 | 0.7276 | 0.2543 | 0.1720 | 0.726 |
| $a+bx^2z^2+c/\sqrt{x}z^2$ | 123.11 | 90.27 | 0.816 | 0.0787 | 0.0577 | 0.6941 | 0.2715 | 0.1889 | 0.688 |
| $a+bx^2z^2+c/\sqrt{x}\sqrt{z}$ | 137.21 | 101.68 | 0.771 | 0.0753 | 0.0536 | 0.7203 | 0.2628 | 0.1860 | 0.707 |
| $a+bx^2z^2+cz/\sqrt{x}$ | 164.23 | 127.19 | 0.672 | 0.0897 | 0.0716 | 0.6023 | 0.3308 | 0.2582 | 0.536 |
| $a+bx^2z^2+cz^2/\sqrt{x}$ | 162.03 | 122.00 | 0.681 | 0.0897 | 0.0699 | 0.6026 | 0.3332 | 0.2613 | 0.530 |
| $a+bx^2z^2+c\sqrt{z}/\sqrt{x}$ | 160.83 | 125.05 | 0.685 | 0.0854 | 0.0658 | 0.6397 | 0.3123 | 0.2375 | 0.587 |
| $a+bx^2\sqrt{z}+c\sqrt{x}/z$ | 123.86 | 95.86 | 0.813 | 0.0749 | 0.0549 | 0.7228 | 0.2659 | 0.1992 | 0.700 |

(continued on next page)

**Table 4 – continued from previous page**

| Functional form | $T_{eff}$ (K) | | | Radius ($R_\odot$) | | | log (L/$L_\odot$) | | |
|---|---|---|---|---|---|---|---|---|---|
| | RMSE | MAD | $R^2_{ap}$ | RMSE | MAD | $R^2_{ap}$ | RMSE | MAD | $R^2_{ap}$ |
| $a+bx^2\sqrt{z}+c\sqrt{x}/z^2$ | 123.16 | 96.22 | 0.815 | 0.0750 | 0.0550 | 0.7222 | 0.2674 | 0.2031 | 0.697 |
| $a+bx^2\sqrt{z}+c\sqrt{x}/\sqrt{z}$ | 123.81 | 96.39 | 0.813 | 0.0744 | 0.0538 | 0.7265 | 0.2594 | 0.1848 | 0.715 |
| $a+bx^2\sqrt{z}+c\sqrt{x}z$ | 122.26 | 91.24 | 0.818 | 0.0719 | 0.0497 | 0.7447 | 0.2626 | 0.1982 | 0.708 |
| $a+bx^2\sqrt{z}+c\sqrt{x}z^2$ | 124.05 | 96.09 | 0.813 | 0.0748 | 0.0551 | 0.7239 | 0.2668 | 0.2003 | 0.698 |
| $a+bx^2\sqrt{z}+c\sqrt{x}\sqrt{z}$ | 117.71 | 91.02 | 0.831 | 0.0694 | 0.0422 | 0.7622 | 0.2404 | 0.1483 | 0.755 |
| $a+bx^2\sqrt{z}+c/xz$ | 123.13 | 95.75 | 0.816 | 0.0726 | 0.0511 | 0.7394 | 0.2510 | 0.1763 | 0.733 |
| $a+bx^2\sqrt{z}+c/xz^2$ | 119.54 | 93.06 | 0.826 | 0.0725 | 0.0497 | 0.7402 | 0.2461 | 0.1661 | 0.743 |
| $a+bx^2\sqrt{z}+c/x\sqrt{z}$ | 123.89 | 96.07 | 0.813 | 0.0729 | 0.0517 | 0.7373 | 0.2544 | 0.1810 | 0.726 |
| $a+bx^2\sqrt{z}+cz/x$ | 123.45 | 94.26 | 0.815 | 0.0741 | 0.0529 | 0.7289 | 0.2621 | 0.1899 | 0.709 |
| $a+bx^2\sqrt{z}+cz^2/x$ | 122.70 | 92.32 | 0.817 | 0.0749 | 0.0547 | 0.7232 | 0.2651 | 0.1943 | 0.702 |
| $a+bx^2\sqrt{z}+c\sqrt{z}/x$ | 123.85 | 95.17 | 0.813 | 0.0737 | 0.0526 | 0.7318 | 0.2601 | 0.1880 | 0.713 |
| $a+bx^2\sqrt{z}+c/x^2z$ | 123.80 | 95.03 | 0.814 | 0.0736 | 0.0526 | 0.7324 | 0.2603 | 0.1882 | 0.713 |
| $a+bx^2\sqrt{z}+c/x^2z^2$ | 124.06 | 95.87 | 0.813 | 0.0733 | 0.0522 | 0.7346 | 0.2575 | 0.1849 | 0.719 |
| $a+bx^2\sqrt{z}+c/x^2\sqrt{z}$ | 123.59 | 94.61 | 0.814 | 0.0737 | 0.0527 | 0.7316 | 0.2612 | 0.1891 | 0.711 |
| $a+bx^2\sqrt{z}+cz/x^2$ | 123.04 | 93.62 | 0.816 | 0.0740 | 0.0529 | 0.7299 | 0.2629 | 0.1905 | 0.707 |
| $a+bx^2\sqrt{z}+cz^2/x^2$ | 122.78 | 93.14 | 0.817 | 0.0741 | 0.0529 | 0.7290 | 0.2635 | 0.1909 | 0.706 |
| $a+bx^2\sqrt{z}+c\sqrt{z}/x^2$ | 123.20 | 93.90 | 0.815 | 0.0739 | 0.0528 | 0.7304 | 0.2625 | 0.1902 | 0.708 |
| $a+bx^2\sqrt{z}+c/\sqrt{x}z$ | 117.84 | 92.05 | 0.831 | 0.0720 | 0.0487 | 0.7443 | 0.2422 | 0.1577 | 0.751 |
| $a+bx^2\sqrt{z}+c/\sqrt{x}z^2$ | 114.18 | 90.51 | 0.841 | 0.0734 | 0.0519 | 0.7336 | 0.2498 | 0.1679 | 0.736 |
| $a+bx^2\sqrt{z}+c/\sqrt{x}\sqrt{z}$ | 121.40 | 94.10 | 0.821 | 0.0720 | 0.0496 | 0.7441 | 0.2454 | 0.1670 | 0.745 |
| $a+bx^2\sqrt{z}+cz/\sqrt{x}$ | 123.02 | 92.89 | 0.816 | 0.0750 | 0.0550 | 0.7225 | 0.2654 | 0.1959 | 0.702 |
| $a+bx^2\sqrt{z}+cz^2/\sqrt{x}$ | 123.19 | 92.77 | 0.815 | 0.0748 | 0.0549 | 0.7240 | 0.2674 | 0.2021 | 0.697 |
| $a+bx^2\sqrt{z}+c\sqrt{z}/\sqrt{x}$ | 123.90 | 95.25 | 0.813 | 0.0742 | 0.0531 | 0.7285 | 0.2608 | 0.1884 | 0.712 |
| $a+b\sqrt{x}/z+c\sqrt{x}/z^2$ | 256.85 | 183.13 | 0.197 | 0.1334 | 0.1005 | 0.1209 | 0.4616 | 0.3464 | 0.097 |
| $a+b\sqrt{x}/z+c\sqrt{x}/\sqrt{z}$ | 193.80 | 139.34 | 0.543 | 0.1066 | 0.0804 | 0.4387 | 0.3420 | 0.2357 | 0.504 |
| $a+b\sqrt{x}/z+c\sqrt{x}z$ | 128.74 | 98.55 | 0.798 | 0.0705 | 0.0466 | 0.7548 | 0.2585 | 0.1852 | 0.717 |
| $a+b\sqrt{x}/z+c\sqrt{x}z^2$ | 155.38 | 117.20 | 0.706 | 0.0833 | 0.0634 | 0.6575 | 0.3126 | 0.2415 | 0.586 |
| $a+b\sqrt{x}/z+c\sqrt{x}\sqrt{z}$ | 122.05 | 92.84 | 0.819 | 0.0692 | 0.0425 | 0.7638 | 0.2362 | 0.1471 | 0.764 |
| $a+b\sqrt{x}/z+c/xz$ | 198.62 | 140.98 | 0.520 | 0.1015 | 0.0717 | 0.4914 | 0.3388 | 0.2342 | 0.514 |
| $a+b\sqrt{x}/z+c/xz^2$ | 197.15 | 136.79 | 0.527 | 0.1058 | 0.0772 | 0.4476 | 0.3456 | 0.2311 | 0.494 |
| $a+b\sqrt{x}/z+c/x\sqrt{z}$ | 203.67 | 144.12 | 0.495 | 0.1020 | 0.0730 | 0.4866 | 0.3453 | 0.2423 | 0.495 |
| $a+b\sqrt{x}/z+cz/x$ | 230.98 | 156.81 | 0.351 | 0.1140 | 0.0820 | 0.3580 | 0.3949 | 0.2772 | 0.339 |
| $a+b\sqrt{x}/z+cz^2/x$ | 256.93 | 181.97 | 0.197 | 0.1333 | 0.1003 | 0.1233 | 0.4616 | 0.3458 | 0.097 |
| $a+b\sqrt{x}/z+c\sqrt{z}/x$ | 219.28 | 151.87 | 0.415 | 0.1078 | 0.0778 | 0.4261 | 0.3722 | 0.2632 | 0.413 |
| $a+b\sqrt{x}/z+c/x^2z$ | 222.64 | 153.59 | 0.397 | 0.1091 | 0.0786 | 0.4120 | 0.3781 | 0.2693 | 0.394 |
| $a+b\sqrt{x}/z+c/x^2z^2$ | 214.72 | 150.88 | 0.439 | 0.1065 | 0.0767 | 0.4402 | 0.3647 | 0.2601 | 0.436 |
| $a+b\sqrt{x}/z+c/x^2\sqrt{z}$ | 225.57 | 154.40 | 0.381 | 0.1103 | 0.0793 | 0.3993 | 0.3834 | 0.2722 | 0.377 |
| $a+b\sqrt{x}/z+cz/x^2$ | 231.46 | 155.86 | 0.348 | 0.1130 | 0.0807 | 0.3698 | 0.3948 | 0.2778 | 0.340 |
| $a+b\sqrt{x}/z+cz^2/x^2$ | 234.64 | 156.69 | 0.330 | 0.1147 | 0.0816 | 0.3500 | 0.4012 | 0.2808 | 0.318 |
| $a+b\sqrt{x}/z+c\sqrt{z}/x^2$ | 229.84 | 155.49 | 0.357 | 0.1122 | 0.0803 | 0.3787 | 0.3915 | 0.2763 | 0.350 |
| $a+b\sqrt{x}/z+c/\sqrt{x}z$ | 181.69 | 127.05 | 0.598 | 0.0985 | 0.0703 | 0.5209 | 0.3170 | 0.2066 | 0.574 |
| $a+b\sqrt{x}/z+c/\sqrt{x}z^2$ | 204.06 | 142.76 | 0.493 | 0.1130 | 0.0864 | 0.3692 | 0.3659 | 0.2637 | 0.433 |
| $a+b\sqrt{x}/z+c/\sqrt{x}\sqrt{z}$ | 180.82 | 127.87 | 0.602 | 0.0948 | 0.0663 | 0.5565 | 0.3102 | 0.2031 | 0.592 |
| $a+b\sqrt{x}/z+cz/\sqrt{x}$ | 253.50 | 179.32 | 0.218 | 0.1329 | 0.0996 | 0.1282 | 0.4622 | 0.3416 | 0.095 |
| $a+b\sqrt{x}/z+cz^2/\sqrt{x}$ | 175.05 | 139.47 | 0.627 | 0.0936 | 0.0695 | 0.5672 | 0.3455 | 0.2673 | 0.494 |
| $a+b\sqrt{x}/z+c\sqrt{z}/\sqrt{x}$ | 226.30 | 156.12 | 0.377 | 0.1133 | 0.0823 | 0.3658 | 0.3876 | 0.2702 | 0.363 |
| $a+b\sqrt{x}/z^2+c\sqrt{x}/\sqrt{z}$ | 247.13 | 184.25 | 0.257 | 0.1301 | 0.1052 | 0.1639 | 0.4289 | 0.3347 | 0.221 |
| $a+b\sqrt{x}/z^2+c\sqrt{x}z$ | 129.44 | 99.89 | 0.796 | 0.0715 | 0.0485 | 0.7478 | 0.2652 | 0.1974 | 0.702 |
| $a+b\sqrt{x}/z^2+c\sqrt{x}z^2$ | 152.37 | 116.99 | 0.718 | 0.0836 | 0.0640 | 0.6552 | 0.3133 | 0.2434 | 0.584 |
| $a+b\sqrt{x}/z^2+c\sqrt{x}\sqrt{z}$ | 122.11 | 92.25 | 0.819 | 0.0685 | 0.0408 | 0.7683 | 0.2366 | 0.1503 | 0.763 |
| $a+b\sqrt{x}/z^2+c/xz$ | 222.06 | 165.13 | 0.400 | 0.1129 | 0.0868 | 0.3704 | 0.3711 | 0.2734 | 0.416 |
| $a+b\sqrt{x}/z^2+c/xz^2$ | 218.90 | 160.44 | 0.417 | 0.1150 | 0.0878 | 0.3475 | 0.3721 | 0.2659 | 0.413 |
| $a+b\sqrt{x}/z^2+c/x\sqrt{z}$ | 226.43 | 167.62 | 0.376 | 0.1139 | 0.0886 | 0.3599 | 0.3779 | 0.2798 | 0.395 |
| $a+b\sqrt{x}/z^2+cz/x$ | 248.74 | 176.19 | 0.247 | 0.1253 | 0.0978 | 0.2244 | 0.4236 | 0.3091 | 0.240 |
| $a+b\sqrt{x}/z^2+cz^2/x$ | 255.20 | 183.46 | 0.208 | 0.1349 | 0.1030 | 0.1012 | 0.4624 | 0.3478 | 0.094 |
| $a+b\sqrt{x}/z^2+c\sqrt{z}/x$ | 239.41 | 173.72 | 0.303 | 0.1197 | 0.0936 | 0.2925 | 0.4031 | 0.2975 | 0.312 |
| $a+b\sqrt{x}/z^2+c/x^2z$ | 241.05 | 173.73 | 0.293 | 0.1202 | 0.0937 | 0.2867 | 0.4061 | 0.2991 | 0.301 |
| $a+b\sqrt{x}/z^2+c/x^2z^2$ | 236.14 | 172.63 | 0.322 | 0.1185 | 0.0924 | 0.3070 | 0.3968 | 0.2939 | 0.333 |
| $a+b\sqrt{x}/z^2+c/x^2\sqrt{z}$ | 242.84 | 173.88 | 0.283 | 0.1209 | 0.0942 | 0.2778 | 0.4097 | 0.3009 | 0.289 |
| $a+b\sqrt{x}/z^2+cz/x^2$ | 246.51 | 173.92 | 0.261 | 0.1227 | 0.0949 | 0.2561 | 0.4177 | 0.3041 | 0.261 |
| $a+b\sqrt{x}/z^2+cz^2/x^2$ | 248.81 | 174.10 | 0.247 | 0.1242 | 0.0956 | 0.2385 | 0.4231 | 0.3061 | 0.242 |
| $a+b\sqrt{x}/z^2+c\sqrt{z}/x^2$ | 245.46 | 173.91 | 0.267 | 0.1222 | 0.0947 | 0.2630 | 0.4154 | 0.3032 | 0.269 |
| $a+b\sqrt{x}/z^2+c/\sqrt{x}z$ | 197.01 | 143.69 | 0.528 | 0.1041 | 0.0793 | 0.4649 | 0.3309 | 0.2354 | 0.536 |
| $a+b\sqrt{x}/z^2+c/\sqrt{x}z^2$ | 211.86 | 152.74 | 0.454 | 0.1154 | 0.0914 | 0.3428 | 0.3675 | 0.2742 | 0.428 |
| $a+b\sqrt{x}/z^2+c/\sqrt{x}\sqrt{z}$ | 200.80 | 148.26 | 0.509 | 0.1034 | 0.0781 | 0.4722 | 0.3336 | 0.2358 | 0.528 |
| $a+b\sqrt{x}/z^2+cz/\sqrt{x}$ | 248.88 | 176.08 | 0.246 | 0.1323 | 0.0988 | 0.1358 | 0.4569 | 0.3394 | 0.115 |
| $a+b\sqrt{x}/z^2+cz^2/\sqrt{x}$ | 175.06 | 134.98 | 0.627 | 0.0955 | 0.0686 | 0.5499 | 0.3511 | 0.2624 | 0.478 |
| $a+b\sqrt{x}/z^2+c\sqrt{z}/\sqrt{x}$ | 248.95 | 179.11 | 0.246 | 0.1269 | 0.1005 | 0.2050 | 0.4256 | 0.3175 | 0.232 |
| $a+b\sqrt{x}/\sqrt{z}+c\sqrt{x}z$ | 125.79 | 95.29 | 0.807 | 0.0692 | 0.0441 | 0.7636 | 0.2462 | 0.1689 | 0.743 |
| $a+b\sqrt{x}/\sqrt{z}+c\sqrt{x}z^2$ | 148.88 | 117.62 | 0.730 | 0.0787 | 0.0597 | 0.6943 | 0.2885 | 0.2199 | 0.647 |
| $a+b\sqrt{x}/\sqrt{z}+c\sqrt{x}\sqrt{z}$ | 121.97 | 93.23 | 0.819 | 0.0695 | 0.0426 | 0.7614 | 0.2360 | 0.1436 | 0.764 |
| $a+b\sqrt{x}/\sqrt{z}+c/xz$ | 209.31 | 150.04 | 0.467 | 0.1023 | 0.0733 | 0.4831 | 0.3491 | 0.2530 | 0.484 |
| $a+b\sqrt{x}/\sqrt{z}+c/xz^2$ | 203.56 | 141.81 | 0.496 | 0.1073 | 0.0789 | 0.4318 | 0.3530 | 0.2453 | 0.472 |
| $a+b\sqrt{x}/\sqrt{z}+c/x\sqrt{z}$ | 220.83 | 156.21 | 0.407 | 0.1047 | 0.0774 | 0.4584 | 0.3640 | 0.2685 | 0.439 |
| $a+b\sqrt{x}/\sqrt{z}+cz/x$ | 274.72 | 185.99 | 0.082 | 0.1298 | 0.0968 | 0.1683 | 0.4556 | 0.3303 | 0.120 |
| $a+b\sqrt{x}/\sqrt{z}+cz^2/x$ | 267.95 | 206.34 | 0.126 | 0.1411 | 0.1089 | 0.0174 | 0.4795 | 0.3728 | 0.026 |
| $a+b\sqrt{x}/\sqrt{z}+c\sqrt{z}/x$ | 253.15 | 174.35 | 0.220 | 0.1180 | 0.0890 | 0.3122 | 0.4164 | 0.3077 | 0.265 |
| $a+b\sqrt{x}/\sqrt{z}+c/x^2z$ | 256.87 | 177.45 | 0.197 | 0.1198 | 0.0909 | 0.2914 | 0.4225 | 0.3138 | 0.244 |
| $a+b\sqrt{x}/\sqrt{z}+c/x^2z^2$ | 242.16 | 169.45 | 0.287 | 0.1137 | 0.0866 | 0.3614 | 0.3987 | 0.2997 | 0.326 |
| $a+b\sqrt{x}/\sqrt{z}+c/x^2\sqrt{z}$ | 261.91 | 179.73 | 0.165 | 0.1222 | 0.0922 | 0.2629 | 0.4312 | 0.3180 | 0.212 |
| $a+b\sqrt{x}/\sqrt{z}+cz/x^2$ | 271.37 | 183.41 | 0.104 | 0.1271 | 0.0947 | 0.2025 | 0.4484 | 0.3250 | 0.148 |
| $a+b\sqrt{x}/\sqrt{z}+cz^2/x^2$ | 276.27 | 185.19 | 0.071 | 0.1300 | 0.0962 | 0.1658 | 0.4578 | 0.3287 | 0.112 |
| $a+b\sqrt{x}/\sqrt{z}+c\sqrt{z}/x^2$ | 268.83 | 182.48 | 0.121 | 0.1257 | 0.0940 | 0.2198 | 0.4437 | 0.3232 | 0.166 |
| $a+b\sqrt{x}/\sqrt{z}+c/\sqrt{x}z$ | 180.60 | 125.22 | 0.603 | 0.0974 | 0.0683 | 0.5319 | 0.3152 | 0.2054 | 0.579 |
| $a+b\sqrt{x}/\sqrt{z}+c/\sqrt{x}z^2$ | 207.28 | 145.08 | 0.477 | 0.1143 | 0.0892 | 0.3547 | 0.3681 | 0.2705 | 0.426 |
| $a+b\sqrt{x}/\sqrt{z}+c/\sqrt{x}\sqrt{z}$ | 180.57 | 128.96 | 0.603 | 0.0924 | 0.0617 | 0.5784 | 0.3075 | 0.2051 | 0.599 |
| $a+b\sqrt{x}/\sqrt{z}+cz/\sqrt{x}$ | 206.53 | 142.28 | 0.481 | 0.1170 | 0.0852 | 0.3238 | 0.3916 | 0.2851 | 0.350 |
| $a+b\sqrt{x}/\sqrt{z}+cz^2/\sqrt{x}$ | 148.47 | 119.90 | 0.732 | 0.0802 | 0.0601 | 0.6820 | 0.2879 | 0.2245 | 0.649 |
| $a+b\sqrt{x}/\sqrt{z}+c\sqrt{z}/\sqrt{x}$ | 274.38 | 187.01 | 0.084 | 0.1305 | 0.0981 | 0.1592 | 0.4562 | 0.3322 | 0.118 |
| $a+b\sqrt{x}z+c\sqrt{x}z^2$ | 125.23 | 98.69 | 0.809 | 0.0706 | 0.0420 | 0.7542 | 0.2485 | 0.1511 | 0.738 |
| $a+b\sqrt{x}z+c\sqrt{x}\sqrt{z}$ | 121.66 | 93.23 | 0.820 | 0.0694 | 0.0410 | 0.7622 | 0.2381 | 0.1409 | 0.760 |

(continued on next page)

**Table 4 – continued from previous page**

| Functional form | $T_{eff}$ (K) | | | Radius ($R_\odot$) | | | log (L/$L_\odot$) | | |
|---|---|---|---|---|---|---|---|---|---|
| | RMSE | MAD | $R^2_{ap}$ | RMSE | MAD | $R^2_{ap}$ | RMSE | MAD | $R^2_{ap}$ |
| $a+b\sqrt{x}z+c/xz$ | 128.49 | 99.09 | 0.799 | 0.0703 | 0.0446 | 0.7563 | 0.2512 | 0.1662 | 0.733 |
| $a+b\sqrt{x}z+c/xz^2$ | 125.41 | 96.35 | 0.809 | 0.0704 | 0.0436 | 0.7553 | 0.2475 | 0.1547 | 0.740 |
| $a+b\sqrt{x}z+c/x\sqrt{z}$ | 129.20 | 99.79 | 0.797 | 0.0704 | 0.0452 | 0.7551 | 0.2541 | 0.1723 | 0.727 |
| $a+b\sqrt{x}z+cz/x$ | 129.31 | 99.53 | 0.797 | 0.0710 | 0.0463 | 0.7513 | 0.2598 | 0.1822 | 0.714 |
| $a+b\sqrt{x}z+cz^2/x$ | 129.42 | 99.81 | 0.796 | 0.0709 | 0.0464 | 0.7515 | 0.2592 | 0.1816 | 0.715 |
| $a+b\sqrt{x}z+c\sqrt{z}/x$ | 129.40 | 99.71 | 0.796 | 0.0708 | 0.0460 | 0.7523 | 0.2586 | 0.1803 | 0.717 |
| $a+b\sqrt{x}z+c/x^2z$ | 129.26 | 99.36 | 0.797 | 0.0710 | 0.0461 | 0.7510 | 0.2599 | 0.1811 | 0.714 |
| $a+b\sqrt{x}z+c/x^2z^2$ | 129.44 | 99.89 | 0.796 | 0.0707 | 0.0457 | 0.7529 | 0.2571 | 0.1772 | 0.720 |
| $a+b\sqrt{x}z+c/x^2\sqrt{z}$ | 129.09 | 99.03 | 0.797 | 0.0711 | 0.0463 | 0.7503 | 0.2608 | 0.1822 | 0.712 |
| $a+b\sqrt{x}z+cz/x^2$ | 128.64 | 98.26 | 0.799 | 0.0713 | 0.0465 | 0.7490 | 0.2624 | 0.1839 | 0.708 |
| $a+b\sqrt{x}z+cz^2/x^2$ | 128.50 | 98.04 | 0.799 | 0.0714 | 0.0465 | 0.7485 | 0.2628 | 0.1843 | 0.707 |
| $a+b\sqrt{x}z+c\sqrt{z}/x^2$ | 128.77 | 98.47 | 0.798 | 0.0713 | 0.0464 | 0.7493 | 0.2620 | 0.1835 | 0.709 |
| $a+b\sqrt{x}z+c/\sqrt{x}z$ | 124.30 | 95.59 | 0.812 | 0.0703 | 0.0430 | 0.7560 | 0.2452 | 0.1495 | 0.745 |
| $a+b\sqrt{x}z+c/\sqrt{x}z^2$ | 122.03 | 93.63 | 0.819 | 0.0717 | 0.0465 | 0.7463 | 0.2536 | 0.1607 | 0.727 |
| $a+b\sqrt{x}z+c/\sqrt{x}\sqrt{z}$ | 126.93 | 97.64 | 0.804 | 0.0699 | 0.0434 | 0.7585 | 0.2465 | 0.1568 | 0.743 |
| $a+b\sqrt{x}z+cz/\sqrt{x}$ | 129.38 | 99.77 | 0.796 | 0.0707 | 0.0466 | 0.7534 | 0.2575 | 0.1821 | 0.719 |
| $a+b\sqrt{x}z+cz^2/\sqrt{x}$ | 127.54 | 97.19 | 0.802 | 0.0704 | 0.0446 | 0.7555 | 0.2516 | 0.1707 | 0.732 |
| $a+b\sqrt{x}z+c\sqrt{z}/\sqrt{x}$ | 129.34 | 99.79 | 0.796 | 0.0705 | 0.0460 | 0.7548 | 0.2559 | 0.1787 | 0.722 |
| $a+b\sqrt{x}z^2+c\sqrt{x}\sqrt{z}$ | 121.27 | 92.52 | 0.821 | 0.0693 | 0.0414 | 0.7630 | 0.2390 | 0.1415 | 0.758 |
| $a+b\sqrt{x}z^2+c/xz$ | 144.06 | 109.64 | 0.747 | 0.0747 | 0.0522 | 0.7241 | 0.2707 | 0.1876 | 0.689 |
| $a+b\sqrt{x}z^2+c/xz^2$ | 134.64 | 99.99 | 0.779 | 0.0740 | 0.0497 | 0.7294 | 0.2614 | 0.1728 | 0.710 |
| $a+b\sqrt{x}z^2+c/x\sqrt{z}$ | 147.95 | 113.43 | 0.734 | 0.0758 | 0.0539 | 0.7165 | 0.2779 | 0.1959 | 0.673 |
| $a+b\sqrt{x}z^2+cz/x$ | 153.82 | 116.86 | 0.712 | 0.0789 | 0.0574 | 0.6930 | 0.2950 | 0.2137 | 0.631 |
| $a+b\sqrt{x}z^2+cz^2/x$ | 154.43 | 116.27 | 0.710 | 0.0798 | 0.0585 | 0.6856 | 0.2993 | 0.2187 | 0.620 |
| $a+b\sqrt{x}z^2+c\sqrt{z}/x$ | 152.68 | 116.65 | 0.716 | 0.0780 | 0.0565 | 0.6999 | 0.2905 | 0.2093 | 0.642 |
| $a+b\sqrt{x}z^2+c/x^2z$ | 153.30 | 116.79 | 0.714 | 0.0783 | 0.0567 | 0.6974 | 0.2924 | 0.2104 | 0.638 |
| $a+b\sqrt{x}z^2+c/x^2z^2$ | 151.10 | 116.05 | 0.722 | 0.0773 | 0.0556 | 0.7053 | 0.2862 | 0.2040 | 0.653 |
| $a+b\sqrt{x}z^2+c/x^2\sqrt{z}$ | 153.90 | 116.81 | 0.712 | 0.0787 | 0.0570 | 0.6943 | 0.2946 | 0.2123 | 0.632 |
| $a+b\sqrt{x}z^2+cz/x^2$ | 154.77 | 116.50 | 0.709 | 0.0794 | 0.0576 | 0.6884 | 0.2986 | 0.2154 | 0.622 |
| $a+b\sqrt{x}z^2+cz^2/x^2$ | 154.98 | 116.29 | 0.708 | 0.0797 | 0.0578 | 0.6863 | 0.2999 | 0.2165 | 0.619 |
| $a+b\sqrt{x}z^2+c\sqrt{z}/x^2$ | 154.58 | 116.62 | 0.709 | 0.0792 | 0.0575 | 0.6900 | 0.2976 | 0.2147 | 0.625 |
| $a+b\sqrt{x}z^2+c/\sqrt{x}z$ | 128.59 | 96.07 | 0.799 | 0.0722 | 0.0471 | 0.7424 | 0.2514 | 0.1612 | 0.732 |
| $a+b\sqrt{x}z^2+c/\sqrt{x}z^2$ | 125.66 | 93.04 | 0.808 | 0.0759 | 0.0522 | 0.7152 | 0.2667 | 0.1762 | 0.699 |
| $a+b\sqrt{x}z^2+c/\sqrt{x}\sqrt{z}$ | 136.50 | 101.86 | 0.773 | 0.0725 | 0.0485 | 0.7404 | 0.2570 | 0.1724 | 0.720 |
| $a+b\sqrt{x}z^2+cz/\sqrt{x}$ | 154.77 | 116.88 | 0.709 | 0.0808 | 0.0603 | 0.6778 | 0.3026 | 0.2234 | 0.612 |
| $a+b\sqrt{x}z^2+cz^2/\sqrt{x}$ | 154.33 | 114.93 | 0.710 | 0.0817 | 0.0628 | 0.6703 | 0.3061 | 0.2345 | 0.603 |
| $a+b\sqrt{x}z^2+c\sqrt{z}/\sqrt{x}$ | 152.09 | 116.94 | 0.719 | 0.0782 | 0.0569 | 0.6983 | 0.2903 | 0.2109 | 0.643 |
| $a+b\sqrt{x}\sqrt{z}+c/xz$ | 117.63 | 90.71 3 | 0.832 | 0.0695 | 0.0407 | 0.7617 | 0.2400 | 0.1473 | 0.756 |
| $a+b\sqrt{x}\sqrt{z}+c/xz^2$ | 120.97 | 92.83 3 | 0.822 | 0.0693 | 0.0409 | 0.7625 | 0.2395 | 0.1447 | 0.757 |
| $a+b\sqrt{x}\sqrt{z}+c/x\sqrt{z}$ | 115.98 | 89.19 3 | 0.836 | 0.0695 | 0.0407 | 0.7614 | 0.2402 | 0.1485 | 0.756 |
| $a+b\sqrt{x}\sqrt{z}+cz/x$ | 113.80 | 86.99 3 | 0.842 | 0.0695 | 0.0409 | 0.7613 | 0.2404 | 0.1491 | 0.755 |
| $a+b\sqrt{x}\sqrt{z}+cz^2/x$ | 115.12 | 89.08 3 | 0.839 | 0.0695 | 0.0407 | 0.7618 | 0.2403 | 0.1491 | 0.755 |
| $a+b\sqrt{x}\sqrt{z}+c\sqrt{z}/x$ | 114.01 | 87.14 3 | 0.842 | 0.0695 | 0.0409 | 0.7612 | 0.2404 | 0.1491 | 0.755 |
| $a+b\sqrt{x}\sqrt{z}+c/x^2z$ | 112.84 | 85.54 3 | 0.845 | 0.0695 | 0.0408 | 0.7614 | 0.2404 | 0.1491 | 0.755 |
| $a+b\sqrt{x}\sqrt{z}+c/x^2z^2$ | 114.71 | 87.67 3 | 0.840 | 0.0695 | 0.0406 | 0.7615 | 0.2403 | 0.1490 | 0.755 |
| $a+b\sqrt{x}\sqrt{z}+c/x^2\sqrt{z}$ | 112.24 | 84.80 3 | 0.847 | 0.0695 | 0.0408 | 0.7614 | 0.2403 | 0.1490 | 0.755 |
| $a+b\sqrt{x}\sqrt{z}+cz/x^2$ | 111.25 | 83.52 3 | 0.849 | 0.0695 | 0.0409 | 0.7614 | 0.2402 | 0.1486 | 0.755 |
| $a+b\sqrt{x}\sqrt{z}+cz^2/x^2$ | 111.05 | 83.27 3 | 0.850 | 0.0695 | 0.0409 | 0.7614 | 0.2402 | 0.1484 | 0.756 |
| $a+b\sqrt{x}\sqrt{z}+c\sqrt{z}/x^2$ | 111.48 | 83.81 3 | 0.849 | 0.0695 | 0.0409 | 0.7614 | 0.2403 | 0.1487 | 0.755 |
| $a+b\sqrt{x}\sqrt{z}+c/\sqrt{x}z$ | 121.15 | 92.82 3 | 0.821 | 0.0692 | 0.0411 | 0.7632 | 0.2394 | 0.1437 | 0.757 |
| $a+b\sqrt{x}\sqrt{z}+c/\sqrt{x}z^2$ | 122.07 | 92.06 3 | 0.819 | 0.0688 | 0.0413 | 0.7660 | 0.2401 | 0.1456 | 0.756 |
| $a+b\sqrt{x}\sqrt{z}+c/\sqrt{x}\sqrt{z}$ | 119.08 | 91.98 3 | 0.827 | 0.0694 | 0.0408 | 0.7619 | 0.2396 | 0.1457 | 0.757 |
| $a+b\sqrt{x}\sqrt{z}+cz/\sqrt{x}$ | 117.63 | 91.53 3 | 0.832 | 0.0695 | 0.0409 | 0.7612 | 0.2400 | 0.1488 | 0.756 |
| $a+b\sqrt{x}\sqrt{z}+cz^2/\sqrt{x}$ | 120.12 | 92.98 3 | 0.824 | 0.0693 | 0.0406 | 0.7626 | 0.2396 | 0.1455 | 0.757 |
| $a+b\sqrt{x}\sqrt{z}+c\sqrt{z}/\sqrt{x}$ | 116.91 | 90.64 3 | 0.834 | 0.0696 | 0.0411 | 0.7610 | 0.2401 | 0.1488 | 0.756 |
| $a+b/xz+c/xz^2$ | 236.06 | 167.91 | 0.322 | 0.1216 | 0.0932 | 0.2700 | 0.3917 | 0.2849 | 0.350 |
| $a+b/xz+c/x\sqrt{z}$ | 226.93 | 161.14 | 0.373 | 0.1191 | 0.0907 | 0.2995 | 0.3802 | 0.2758 | 0.387 |
| $a+b/xz+cz/x$ | 183.97 | 127.54 | 0.588 | 0.1043 | 0.0787 | 0.4631 | 0.3275 | 0.2320 | 0.545 |
| $a+b/xz+cz^2/x$ | 138.02 | 98.66 | 0.768 | 0.0820 | 0.0580 | 0.6677 | 0.2691 | 0.1790 | 0.693 |
| $a+b/xz+c\sqrt{z}/x$ | 205.65 | 144.62 | 0.485 | 0.1123 | 0.0859 | 0.3777 | 0.3542 | 0.2543 | 0.468 |
| $a+b/xz+c/x^2z$ | 206.63 | 147.87 | 0.481 | 0.1136 | 0.0866 | 0.3632 | 0.3560 | 0.2566 | 0.463 |
| $a+b/xz+c/x^2z^2$ | 182.78 | 131.97 | 0.594 | 0.1061 | 0.0818 | 0.4441 | 0.3267 | 0.2351 | 0.548 |
| $a+b/xz+c/x^2\sqrt{z}$ | 211.43 | 151.87 | 0.456 | 0.1149 | 0.0879 | 0.3476 | 0.3616 | 0.2595 | 0.446 |
| $a+b/xz+cz/x^2$ | 216.41 | 155.63 | 0.430 | 0.1163 | 0.0892 | 0.3323 | 0.3674 | 0.2632 | 0.428 |
| $a+b/xz+cz^2/x^2$ | 213.41 | 153.17 | 0.446 | 0.1153 | 0.0885 | 0.3439 | 0.3637 | 0.2601 | 0.439 |
| $a+b/xz+c\sqrt{z}/x^2$ | 215.88 | 155.28 | 0.433 | 0.1162 | 0.0891 | 0.3336 | 0.3668 | 0.2627 | 0.430 |
| $a+b/xz+c/\sqrt{x}z$ | 170.37 | 120.45 | 0.647 | 0.0996 | 0.0759 | 0.5097 | 0.3112 | 0.2119 | 0.590 |
| $a+b/xz+c/\sqrt{x}z^2$ | 212.10 | 153.84 | 0.453 | 0.1140 | 0.0881 | 0.3584 | 0.3637 | 0.2655 | 0.440 |
| $a+b/xz+c/\sqrt{x}\sqrt{z}$ | 125.28 | 83.15 | 0.809 | 0.0816 | 0.0581 | 0.6716 | 0.2528 | 0.1530 | 0.729 |
| $a+b/xz+cz/\sqrt{x}$ | 139.56 | 101.65 | 0.763 | 0.0796 | 0.0548 | 0.6870 | 0.2668 | 0.1690 | 0.698 |
| $a+b/xz+cz^2/\sqrt{x}$ | 141.51 | 107.95 | 0.756 | 0.0744 | 0.0509 | 0.7267 | 0.2654 | 0.1826 | 0.702 |
| $a+b/xz+c\sqrt{z}/\sqrt{x}$ | 168.59 | 117.34 | 0.654 | 0.0943 | 0.0669 | 0.5611 | 0.3050 | 0.2073 | 0.606 |
| $a+b/xz^2+c/x\sqrt{z}$ | 234.53 | 166.42 | 0.331 | 0.1215 | 0.0928 | 0.2712 | 0.3907 | 0.2845 | 0.353 |
| $a+b/xz^2+cz/x$ | 214.06 | 154.61 | 0.442 | 0.1172 | 0.0921 | 0.3219 | 0.3725 | 0.2765 | 0.412 |
| $a+b/xz^2+cz^2/x$ | 161.44 | 116.75 | 0.683 | 0.0976 | 0.0724 | 0.5300 | 0.3125 | 0.2229 | 0.586 |
| $a+b/xz^2+c\sqrt{z}/x$ | 225.91 | 160.77 | 0.379 | 0.1202 | 0.0926 | 0.2872 | 0.3839 | 0.2809 | 0.376 |
| $a+b/xz^2+c/x^2z$ | 226.15 | 160.91 | 0.378 | 0.1204 | 0.0924 | 0.2843 | 0.3842 | 0.2812 | 0.375 |
| $a+b/xz^2+c/x^2z^2$ | 222.16 | 160.89 | 0.400 | 0.1196 | 0.0929 | 0.2934 | 0.3807 | 0.2820 | 0.386 |
| $a+b/xz^2+c/x^2\sqrt{z}$ | 227.14 | 160.94 | 0.372 | 0.1206 | 0.0923 | 0.2823 | 0.3850 | 0.2808 | 0.372 |
| $a+b/xz^2+cz/x^2$ | 228.06 | 161.76 | 0.367 | 0.1207 | 0.0921 | 0.2808 | 0.3856 | 0.2802 | 0.370 |
| $a+b/xz^2+cz^2/x^2$ | 226.45 | 161.03 | 0.376 | 0.1204 | 0.0923 | 0.2844 | 0.3843 | 0.2803 | 0.374 |
| $a+b/xz^2+c\sqrt{z}/x^2$ | 228.07 | 161.69 | 0.367 | 0.1207 | 0.0921 | 0.2806 | 0.3857 | 0.2803 | 0.370 |
| $a+b/xz^2+c/\sqrt{x}z$ | 148.41 | 101.08 | 0.732 | 0.0845 | 0.0569 | 0.6476 | 0.2720 | 0.1618 | 0.687 |
| $a+b/xz^2+c/\sqrt{x}z^2$ | 210.84 | 151.24 | 0.459 | 0.1152 | 0.0909 | 0.3445 | 0.3676 | 0.2712 | 0.428 |
| $a+b/xz^2+c/\sqrt{x}\sqrt{z}$ | 207.99 | 145.27 | 0.474 | 0.0957 | 0.0717 | 0.5478 | 0.3215 | 0.2197 | 0.562 |
| $a+b/xz^2+cz/\sqrt{x}$ | 154.19 | 112.31 | 0.711 | 0.0926 | 0.0670 | 0.5770 | 0.3002 | 0.2078 | 0.618 |
| $a+b/xz^2+cz^2/\sqrt{x}$ | 134.38 | 98.08 | 0.780 | 0.0767 | 0.0545 | 0.7099 | 0.2647 | 0.1746 | 0.703 |
| $a+b/xz^2+c\sqrt{z}/\sqrt{x}$ | 200.41 | 145.36 | 0.511 | 0.1119 | 0.0880 | 0.3813 | 0.3572 | 0.2657 | 0.460 |
| $a+b/x\sqrt{z}+cz/x$ | 165.40 | 114.69 | 0.667 | 0.0956 | 0.0694 | 0.5489 | 0.3004 | 0.2037 | 0.618 |
| $a+b/x\sqrt{z}+cz^2/x$ | 135.46 | 96.27 | 0.777 | 0.0773 | 0.0533 | 0.7049 | 0.2616 | 0.1713 | 0.710 |
| $a+b/x\sqrt{z}+c\sqrt{z}/x$ | 189.80 | 131.00 | 0.562 | 0.1057 | 0.0793 | 0.4483 | 0.3316 | 0.2325 | 0.534 |

(continued on next page)

**Table 4 – continued from previous page**

| Functional form | $T_{eff}$ (K) | | | Radius ($R_\odot$) | | | log (L/$L_\odot$) | | |
|---|---|---|---|---|---|---|---|---|---|
| | RMSE | MAD | $R^2_{ap}$ | RMSE | MAD | $R^2_{ap}$ | RMSE | MAD | $R^2_{ap}$ |
| $a+b/x\sqrt{z}+c/x^2z$ | 191.98 | 137.83 | 0.552 | 0.1085 | 0.0831 | 0.4186 | 0.3355 | 0.2363 | 0.523 |
| $a+b/x\sqrt{z}+c/x^2z^2$ | 132.33 | 86.19 | 0.787 | 0.0873 | 0.0643 | 0.6241 | 0.2576 | 0.1686 | 0.719 |
| $a+b/x\sqrt{z}+c/x^2\sqrt{z}$ | 202.22 | 145.72 | 0.502 | 0.1117 | 0.0857 | 0.3836 | 0.3485 | 0.2492 | 0.486 |
| $a+b/x\sqrt{z}+cz/x^2$ | 212.01 | 153.09 | 0.453 | 0.1146 | 0.0884 | 0.3512 | 0.3606 | 0.2600 | 0.449 |
| $a+b/x\sqrt{z}+cz^2/x^2$ | 208.03 | 149.36 | 0.473 | 0.1131 | 0.0871 | 0.3681 | 0.3555 | 0.2549 | 0.464 |
| $a+b/x\sqrt{z}+c\sqrt{z}/x^2$ | 210.87 | 152.37 | 0.459 | 0.1143 | 0.0881 | 0.3544 | 0.3592 | 0.2590 | 0.453 |
| $a+b/x\sqrt{z}+c/\sqrt{x}z$ | 177.13 | 126.52 | 0.618 | 0.1017 | 0.0774 | 0.4889 | 0.3177 | 0.2200 | 0.572 |
| $a+b/x\sqrt{z}+c/\sqrt{x}z^2$ | 212.15 | 154.09 | 0.452 | 0.1138 | 0.0881 | 0.3610 | 0.3633 | 0.2652 | 0.441 |
| $a+b/x\sqrt{z}+c/\sqrt{x}\sqrt{z}$ | 147.08 | 103.74 | 0.737 | 0.0912 | 0.0683 | 0.5891 | 0.2800 | 0.1859 | 0.668 |
| $a+b/x\sqrt{z}+cz/\sqrt{x}$ | 140.54 | 108.62 | 0.760 | 0.0765 | 0.0506 | 0.7114 | 0.2641 | 0.1693 | 0.704 |
| $a+b/x\sqrt{z}+cz^2/\sqrt{x}$ | 146.47 | 112.30 | 0.739 | 0.0749 | 0.0526 | 0.7232 | 0.2718 | 0.1925 | 0.687 |
| $a+b/x\sqrt{z}+c\sqrt{z}/\sqrt{x}$ | 162.33 | 116.68 | 0.679 | 0.0868 | 0.0590 | 0.6280 | 0.2911 | 0.1885 | 0.641 |
| $a+bz/x+cz^2/x$ | 153.06 | 118.86 | 0.715 | 0.0775 | 0.0555 | 0.7035 | 0.2846 | 0.2079 | 0.657 |
| $a+bz/x+c\sqrt{z}/x$ | 137.93 | 99.17 | 0.769 | 0.0792 | 0.0543 | 0.6901 | 0.2614 | 0.1681 | 0.710 |
| $a+bz/x+c/x^2z$ | 181.07 | 131.63 | 0.601 | 0.0905 | 0.0641 | 0.5954 | 0.3160 | 0.2226 | 0.577 |
| $a+bz/x+c/x^2z^2$ | 195.30 | 134.37 | 0.536 | 0.1050 | 0.0778 | 0.4552 | 0.3416 | 0.2451 | 0.506 |
| $a+bz/x+c/x^2\sqrt{z}$ | 198.12 | 148.02 | 0.522 | 0.0933 | 0.0690 | 0.5702 | 0.3381 | 0.2477 | 0.516 |
| $a+bz/x+cz/x^2$ | 260.19 | 168.54 | 0.176 | 0.1191 | 0.0852 | 0.2997 | 0.4294 | 0.2985 | 0.219 |
| $a+bz/x+cz^2/x^2$ | 285.13 | 194.28 | 0.011 | 0.1330 | 0.0949 | 0.1272 | 0.4683 | 0.3311 | 0.071 |
| $a+bz/x+c\sqrt{z}/x^2$ | 243.66 | 165.69 | 0.278 | 0.1111 | 0.0807 | 0.3909 | 0.4042 | 0.2821 | 0.308 |
| $a+bz/x+c/\sqrt{x}z$ | 171.96 | 122.07 | 0.640 | 0.1002 | 0.0764 | 0.5041 | 0.3127 | 0.2154 | 0.586 |
| $a+bz/x+c/\sqrt{x}z^2$ | 209.59 | 152.99 | 0.466 | 0.1153 | 0.0908 | 0.3441 | 0.3682 | 0.2713 | 0.426 |
| $a+bz/x+c/\sqrt{x}\sqrt{z}$ | 152.36 | 105.50 | 0.718 | 0.0922 | 0.0684 | 0.5805 | 0.2849 | 0.1881 | 0.656 |
| $a+bz/x+cz/\sqrt{x}$ | 159.43 | 121.89 | 0.691 | 0.0785 | 0.0545 | 0.6959 | 0.2897 | 0.2027 | 0.644 |
| $a+bz/x+cz^2/\sqrt{x}$ | 157.73 | 120.66 | 0.697 | 0.0783 | 0.0566 | 0.6970 | 0.2929 | 0.2143 | 0.637 |
| $a+bz/x+c\sqrt{z}/\sqrt{x}$ | 277.71 | 183.61 | 0.062 | 0.1294 | 0.0945 | 0.1733 | 0.4577 | 0.3255 | 0.112 |
| $a+bz^2/x+c\sqrt{z}/x$ | 145.27 | 110.45 | 0.743 | 0.0757 | 0.0522 | 0.7173 | 0.2726 | 0.1938 | 0.685 |
| $a+bz^2/x+c/x^2z$ | 154.83 | 116.00 | 0.708 | 0.0785 | 0.0557 | 0.6955 | 0.2855 | 0.2033 | 0.655 |
| $a+bz^2/x+c/x^2z^2$ | 147.77 | 104.61 | 0.734 | 0.0799 | 0.0564 | 0.6848 | 0.2784 | 0.1825 | 0.672 |
| $a+bz^2/x+c/x^2\sqrt{z}$ | 159.76 | 119.70 | 0.689 | 0.0794 | 0.0578 | 0.6891 | 0.2922 | 0.2113 | 0.638 |
| $a+bz^2/x+cz/x^2$ | 171.97 | 125.86 | 0.640 | 0.0829 | 0.0612 | 0.6610 | 0.3104 | 0.2246 | 0.592 |
| $a+bz^2/x+cz^2/x^2$ | 176.88 | 127.95 | 0.619 | 0.0846 | 0.0622 | 0.6464 | 0.3182 | 0.2282 | 0.571 |
| $a+bz^2/x+c\sqrt{z}/x^2$ | 168.54 | 124.32 | 0.654 | 0.0817 | 0.0604 | 0.6701 | 0.3051 | 0.2215 | 0.605 |
| $a+bz^2/x+c/\sqrt{x}z$ | 142.24 | 102.46 | 0.754 | 0.0888 | 0.0646 | 0.6104 | 0.2820 | 0.1882 | 0.663 |
| $a+bz^2/x+c/\sqrt{x}z^2$ | 184.84 | 129.66 | 0.584 | 0.1096 | 0.0841 | 0.4073 | 0.3538 | 0.2542 | 0.470 |
| $a+bz^2/x+c/\sqrt{x}\sqrt{z}$ | 127.67 | 92.46 | 0.802 | 0.0797 | 0.0546 | 0.6867 | 0.2559 | 0.1645 | 0.722 |
| $a+bz^2/x+cz/\sqrt{x}$ | 215.75 | 157.33 | 0.434 | 0.1078 | 0.0772 | 0.4266 | 0.3841 | 0.2682 | 0.375 |
| $a+bz^2/x+cz^2/\sqrt{x}$ | 159.53 | 120.61 | 0.690 | 0.0791 | 0.0567 | 0.6907 | 0.2976 | 0.2166 | 0.625 |
| $a+bz^2/x+c\sqrt{z}/\sqrt{x}$ | 143.37 | 109.23 | 0.750 | 0.0812 | 0.0599 | 0.6746 | 0.2774 | 0.2037 | 0.674 |
| $a+b\sqrt{z}/x+c/x^2z$ | 286.92 | 210.79 | -0.002 | 0.1355 | 0.1051 | 0.0937 | 0.4635 | 0.3542 | 0.090 |
| $a+b\sqrt{z}/x+c/x^2z^2$ | 254.71 | 177.51 | 0.211 | 0.1276 | 0.0954 | 0.1958 | 0.4209 | 0.3023 | 0.250 |
| $a+b\sqrt{z}/x+c/x^2\sqrt{z}$ | 281.31 | 211.58 | 0.037 | 0.1375 | 0.1092 | 0.0664 | 0.4583 | 0.3579 | 0.110 |
| $a+b\sqrt{z}/x+cz/x^2$ | 262.91 | 189.23 | 0.159 | 0.1331 | 0.1027 | 0.1256 | 0.4336 | 0.3245 | 0.203 |
| $a+b\sqrt{z}/x+cz^2/x^2$ | 246.29 | 180.90 | 0.262 | 0.1277 | 0.1001 | 0.1952 | 0.4108 | 0.3121 | 0.285 |
| $a+b\sqrt{z}/x+c\sqrt{z}/x^2$ | 267.73 | 195.62 | 0.128 | 0.1345 | 0.1049 | 0.1069 | 0.4402 | 0.3346 | 0.179 |
| $a+b\sqrt{z}/x+c/\sqrt{x}z$ | 177.98 | 127.15 | 0.615 | 0.1020 | 0.0775 | 0.4868 | 0.3182 | 0.2210 | 0.571 |
| $a+b\sqrt{z}/x+c/\sqrt{x}z^2$ | 211.58 | 152.12 | 0.455 | 0.1145 | 0.0888 | 0.3526 | 0.3659 | 0.2651 | 0.433 |
| $a+b\sqrt{z}/x+c/\sqrt{x}\sqrt{z}$ | 159.00 | 111.77 | 0.692 | 0.0949 | 0.0711 | 0.5554 | 0.2924 | 0.1947 | 0.638 |
| $a+b\sqrt{z}/x+cz/\sqrt{x}$ | 151.95 | 118.49 | 0.719 | 0.0764 | 0.0523 | 0.7115 | 0.2782 | 0.1942 | 0.672 |
| $a+b\sqrt{z}/x+cz^2/\sqrt{x}$ | 154.87 | 118.88 | 0.708 | 0.0772 | 0.0556 | 0.7060 | 0.2867 | 0.2092 | 0.652 |
| $a+b\sqrt{z}/x+c\sqrt{z}/\sqrt{x}$ | 206.38 | 148.64 | 0.482 | 0.0955 | 0.0698 | 0.5499 | 0.3476 | 0.2455 | 0.488 |
| $a+b/x^2z+c/x^2z^2$ | 257.23 | 181.34 | 0.195 | 0.1302 | 0.0996 | 0.1636 | 0.4251 | 0.3081 | 0.234 |
| $a+b/x^2z+c/x^2\sqrt{z}$ | 256.05 | 180.91 | 0.202 | 0.1297 | 0.0995 | 0.1692 | 0.4231 | 0.3076 | 0.242 |
| $a+b/x^2z+cz/x^2$ | 250.03 | 177.81 | 0.239 | 0.1276 | 0.0985 | 0.1960 | 0.4144 | 0.3034 | 0.272 |
| $a+b/x^2z+cz^2/x^2$ | 234.54 | 168.27 | 0.331 | 0.1219 | 0.0949 | 0.2662 | 0.3930 | 0.2904 | 0.346 |
| $a+b/x^2z+c\sqrt{z}/x^2$ | 253.17 | 179.40 | 0.220 | 0.1287 | 0.0990 | 0.1820 | 0.4189 | 0.3054 | 0.257 |
| $a+b/x^2z+c/\sqrt{x}z$ | 176.86 | 127.37 | 0.619 | 0.1020 | 0.0778 | 0.4858 | 0.3175 | 0.2217 | 0.573 |
| $a+b/x^2z+c/\sqrt{x}z^2$ | 211.42 | 152.53 | 0.456 | 0.1145 | 0.0887 | 0.3528 | 0.3662 | 0.2653 | 0.432 |
| $a+b/x^2z+c/\sqrt{x}\sqrt{z}$ | 157.69 | 111.47 | 0.697 | 0.0954 | 0.0719 | 0.5507 | 0.2915 | 0.1976 | 0.640 |
| $a+b/x^2z+cz/\sqrt{x}$ | 160.52 | 123.72 | 0.687 | 0.0795 | 0.0551 | 0.6876 | 0.2907 | 0.2022 | 0.642 |
| $a+b/x^2z+cz^2/\sqrt{x}$ | 157.14 | 119.49 | 0.700 | 0.0781 | 0.0567 | 0.6988 | 0.2909 | 0.2123 | 0.641 |
| $a+b/x^2z+c\sqrt{z}/\sqrt{x}$ | 226.00 | 162.37 | 0.379 | 0.1042 | 0.0778 | 0.4644 | 0.3763 | 0.2740 | 0.400 |
| $a+b/x^2z^2+c/x^2\sqrt{z}$ | 256.95 | 181.23 | 0.197 | 0.1301 | 0.0996 | 0.1648 | 0.4247 | 0.3080 | 0.236 |
| $a+b/x^2z^2+cz/x^2$ | 253.98 | 179.79 | 0.215 | 0.1291 | 0.0993 | 0.1768 | 0.4206 | 0.3063 | 0.250 |
| $a+b/x^2z^2+cz^2/x^2$ | 245.88 | 176.04 | 0.264 | 0.1265 | 0.0983 | 0.2102 | 0.4100 | 0.3021 | 0.288 |
| $a+b/x^2z^2+c\sqrt{z}/x^2$ | 255.56 | 180.43 | 0.205 | 0.1296 | 0.0994 | 0.1704 | 0.4227 | 0.3070 | 0.243 |
| $a+b/x^2z^2+c/\sqrt{x}z$ | 171.19 | 122.81 | 0.643 | 0.1004 | 0.0769 | 0.5020 | 0.3122 | 0.2157 | 0.587 |
| $a+b/x^2z^2+c/\sqrt{x}z^2$ | 211.11 | 152.60 | 0.458 | 0.1148 | 0.0895 | 0.3498 | 0.3667 | 0.2673 | 0.430 |
| $a+b/x^2z^2+c/\sqrt{x}\sqrt{z}$ | 142.58 | 100.12 | 0.753 | 0.0901 | 0.0676 | 0.5989 | 0.2745 | 0.1829 | 0.681 |
| $a+b/x^2z^2+cz/\sqrt{x}$ | 150.59 | 116.42 | 0.724 | 0.0785 | 0.0520 | 0.6956 | 0.2783 | 0.1853 | 0.672 |
| $a+b/x^2z^2+cz^2/\sqrt{x}$ | 152.30 | 116.85 | 0.718 | 0.0768 | 0.0549 | 0.7087 | 0.2825 | 0.2033 | 0.662 |
| $a+b/x^2z^2+c\sqrt{z}/\sqrt{x}$ | 193.68 | 141.12 | 0.544 | 0.0957 | 0.0672 | 0.5477 | 0.3336 | 0.2386 | 0.529 |
| $a+b/x^2\sqrt{z}+cz/x^2$ | 246.49 | 175.84 | 0.261 | 0.1262 | 0.0977 | 0.2132 | 0.4091 | 0.3002 | 0.291 |
| $a+b/x^2\sqrt{z}+cz^2/x^2$ | 225.36 | 160.86 | 0.382 | 0.1181 | 0.0915 | 0.3111 | 0.3795 | 0.2794 | 0.390 |
| $a+b/x^2\sqrt{z}+c\sqrt{z}/x^2$ | 250.94 | 178.27 | 0.234 | 0.1279 | 0.0986 | 0.1927 | 0.4155 | 0.3037 | 0.269 |
| $a+b/x^2\sqrt{z}+c/\sqrt{x}z$ | 178.58 | 128.58 | 0.612 | 0.1025 | 0.0780 | 0.4815 | 0.3190 | 0.2230 | 0.569 |
| $a+b/x^2\sqrt{z}+c/\sqrt{x}z^2$ | 211.49 | 152.48 | 0.456 | 0.1144 | 0.0884 | 0.3538 | 0.3660 | 0.2647 | 0.432 |
| $a+b/x^2\sqrt{z}+c/\sqrt{x}\sqrt{z}$ | 162.29 | 114.12 | 0.680 | 0.0968 | 0.0729 | 0.5373 | 0.2964 | 0.2014 | 0.628 |
| $a+b/x^2\sqrt{z}+cz/\sqrt{x}$ | 165.31 | 125.86 | 0.668 | 0.0808 | 0.0566 | 0.6778 | 0.2978 | 0.2078 | 0.624 |
| $a+b/x^2\sqrt{z}+cz^2/\sqrt{x}$ | 158.84 | 120.22 | 0.693 | 0.0787 | 0.0573 | 0.6941 | 0.2943 | 0.2151 | 0.633 |
| $a+b/x^2\sqrt{z}+c\sqrt{z}/\sqrt{x}$ | 241.62 | 166.65 | 0.290 | 0.1106 | 0.0816 | 0.3958 | 0.3996 | 0.2863 | 0.323 |
| $a+bz/x^2+cz^2/x^2$ | 179.34 | 127.17 | 0.609 | 0.0974 | 0.0689 | 0.5317 | 0.3147 | 0.2183 | 0.580 |
| $a+bz/x^2+c\sqrt{z}/x^2$ | 232.74 | 166.39 | 0.341 | 0.1208 | 0.0936 | 0.2795 | 0.3888 | 0.2859 | 0.359 |
| $a+bz/x^2+c/\sqrt{x}z$ | 181.02 | 129.93 | 0.601 | 0.1030 | 0.0781 | 0.4760 | 0.3209 | 0.2245 | 0.564 |
| $a+bz/x^2+c/\sqrt{x}z^2$ | 211.53 | 152.50 | 0.456 | 0.1143 | 0.0882 | 0.3545 | 0.3660 | 0.2643 | 0.432 |
| $a+bz/x^2+c/\sqrt{x}\sqrt{z}$ | 168.96 | 117.22 | 0.653 | 0.0987 | 0.0740 | 0.5189 | 0.3033 | 0.2057 | 0.610 |
| $a+bz/x^2+cz/\sqrt{x}$ | 175.69 | 128.99 | 0.624 | 0.0843 | 0.0590 | 0.6494 | 0.3141 | 0.2167 | 0.582 |
| $a+bz/x^2+cz^2/\sqrt{x}$ | 161.96 | 121.44 | 0.681 | 0.0800 | 0.0581 | 0.6839 | 0.3009 | 0.2198 | 0.616 |
| $a+bz/x^2+c\sqrt{z}/\sqrt{x}$ | 269.49 | 176.52 | 0.116 | 0.1243 | 0.0905 | 0.2372 | 0.4436 | 0.3140 | 0.166 |
| $a+bz^2/x^2+c\sqrt{z}/x^2$ | 197.00 | 137.84 | 0.528 | 0.1058 | 0.0781 | 0.4475 | 0.3389 | 0.2393 | 0.513 |

(continued on next page)

**Table 4 – continued from previous page**

| Functional form | $T_{eff}$ (K) | | | Radius ($R_\odot$) | | | log (L/$L_\odot$) | | |
|---|---|---|---|---|---|---|---|---|---|
| | RMSE | MAD | $R^2_{ap}$ | RMSE | MAD | $R^2_{ap}$ | RMSE | MAD | $R^2_{ap}$ |
| $a+bz^2/x^2+c/\sqrt{x}z$ | 180.30 | 129.25 | 0.604 | 0.1028 | 0.0780 | 0.4779 | 0.3202 | 0.2240 | 0.565 |
| $a+bz^2/x^2+c/\sqrt{x}z^2$ | 211.26 | 152.89 | 0.457 | 0.1145 | 0.0887 | 0.3521 | 0.3666 | 0.2658 | 0.431 |
| $a+bz^2/x^2+c/\sqrt{x}\sqrt{z}$ | 168.48 | 116.36 | 0.655 | 0.0985 | 0.0738 | 0.5213 | 0.3027 | 0.2047 | 0.612 |
| $a+bz^2/x^2+cz/\sqrt{x}$ | 179.83 | 129.87 | 0.607 | 0.0859 | 0.0597 | 0.6354 | 0.3210 | 0.2190 | 0.563 |
| $a+bz^2/x^2+cz^2/\sqrt{x}$ | 162.90 | 121.72 | 0.677 | 0.0805 | 0.0583 | 0.6803 | 0.3032 | 0.2210 | 0.611 |
| $a+bz^2/x^2+c\sqrt{z}/\sqrt{x}$ | 281.39 | 188.40 | 0.037 | 0.1311 | 0.0945 | 0.1513 | 0.4633 | 0.3253 | 0.091 |
| $a+b\sqrt{z}/x^2+c/\sqrt{x}z$ | 180.60 | 129.76 | 0.603 | 0.1029 | 0.0781 | 0.4769 | 0.3206 | 0.2243 | 0.565 |
| $a+b\sqrt{z}/x^2+c/\sqrt{x}z^2$ | 211.56 | 152.45 | 0.455 | 0.1143 | 0.0882 | 0.3546 | 0.3659 | 0.2642 | 0.433 |
| $a+b\sqrt{z}/x^2+c/\sqrt{x}\sqrt{z}$ | 167.68 | 116.72 | 0.658 | 0.0984 | 0.0739 | 0.5222 | 0.3020 | 0.2051 | 0.614 |
| $a+b\sqrt{z}/x^2+cz/\sqrt{x}$ | 172.89 | 128.33 | 0.636 | 0.0832 | 0.0584 | 0.6579 | 0.3096 | 0.2147 | 0.594 |
| $a+b\sqrt{z}/x^2+cz^2/\sqrt{x}$ | 161.18 | 121.17 | 0.684 | 0.0797 | 0.0579 | 0.6867 | 0.2992 | 0.2187 | 0.621 |
| $a+b\sqrt{z}/x^2+c\sqrt{z}/\sqrt{x}$ | 262.58 | 172.77 | 0.161 | 0.1206 | 0.0883 | 0.2813 | 0.4324 | 0.3073 | 0.208 |
| $a+b/\sqrt{x}z+c/\sqrt{x}z^2$ | 204.27 | 147.96 | 0.492 | 0.1045 | 0.0790 | 0.4610 | 0.3322 | 0.2351 | 0.532 |
| $a+b/\sqrt{x}z+c/\sqrt{x}\sqrt{z}$ | 197.00 | 145.51 | 0.528 | 0.1052 | 0.0810 | 0.4533 | 0.3321 | 0.2395 | 0.533 |
| $a+b/\sqrt{x}z+cz/\sqrt{x}$ | 143.35 | 102.47 | 0.750 | 0.0872 | 0.0617 | 0.6247 | 0.2805 | 0.1822 | 0.667 |
| $a+b/\sqrt{x}z+cz^2/\sqrt{x}$ | 128.65 | 95.97 | 0.799 | 0.0749 | 0.0510 | 0.7231 | 0.2552 | 0.1601 | 0.724 |
| $a+b/\sqrt{x}z+c\sqrt{z}/\sqrt{x}$ | 167.06 | 114.87 | 0.660 | 0.0974 | 0.0731 | 0.5315 | 0.3070 | 0.2046 | 0.601 |
| $a+b/\sqrt{x}z^2+c/\sqrt{x}\sqrt{z}$ | 208.12 | 152.53 | 0.473 | 0.1077 | 0.0830 | 0.4276 | 0.3430 | 0.2486 | 0.502 |
| $a+b/\sqrt{x}z^2+cz/\sqrt{x}$ | 180.54 | 124.03 | 0.603 | 0.1068 | 0.0793 | 0.4364 | 0.3480 | 0.2434 | 0.487 |
| $a+b/\sqrt{x}z^2+cz^2/\sqrt{x}$ | 137.19 | 99.55 | 0.771 | 0.0838 | 0.0579 | 0.6531 | 0.2884 | 0.1871 | 0.648 |
| $a+b/\sqrt{x}z^2+c\sqrt{z}/\sqrt{x}$ | 207.51 | 150.86 | 0.476 | 0.1153 | 0.0915 | 0.3436 | 0.3686 | 0.2734 | 0.424 |
| $a+b/\sqrt{x}\sqrt{z}+cz/\sqrt{x}$ | 132.04 | 96.63 | 0.788 | 0.0787 | 0.0524 | 0.6945 | 0.2575 | 0.1587 | 0.719 |
| $a+b/\sqrt{x}\sqrt{z}+cz^2/\sqrt{x}$ | 132.81 | 100.55 | 0.785 | 0.0726 | 0.0484 | 0.7400 | 0.2527 | 0.1656 | 0.729 |
| $a+b/\sqrt{x}\sqrt{z}+c\sqrt{z}/\sqrt{x}$ | 147.32 | 101.63 | 0.736 | 0.0873 | 0.0618 | 0.6236 | 0.2769 | 0.1755 | 0.675 |
| $a+bz/\sqrt{x}+cz^2/\sqrt{x}$ | 161.05 | 126.42 | 0.684 | 0.0812 | 0.0595 | 0.6743 | 0.3040 | 0.2243 | 0.609 |
| $a+bz/\sqrt{x}+c\sqrt{z}/\sqrt{x}$ | 133.92 | 103.52 | 0.782 | 0.0718 | 0.0468 | 0.7453 | 0.2549 | 0.1727 | 0.725 |
| $a+bz^2/\sqrt{x}+c\sqrt{z}/\sqrt{x}$ | 152.01 | 119.88 | 0.719 | 0.0766 | 0.0542 | 0.7102 | 0.2830 | 0.2055 | 0.661 |
| Single EW ratio, double component functions result (y/z) | | | | | | | | | |
| $a+by/z+cy/z^2$ | 262.06 | 189.85 | 0.164 | 0.1355 | 0.1041 | 0.0932 | 0.4639 | 0.3518 | 0.088 |
| $a+by/z+cy/\sqrt{z}$ | 180.49 | 133.66 | 0.604 | 0.1034 | 0.0771 | 0.4720 | 0.3392 | 0.2377 | 0.513 |
| $a+by/z+cyz$ | 137.19 | 106.91 | 0.771 | 0.0787 | 0.0560 | 0.6939 | 0.2877 | 0.2178 | 0.649 |
| $a+by/z+cyz^2$ | 161.22 | 123.32 | 0.684 | 0.0879 | 0.0676 | 0.6182 | 0.3269 | 0.2534 | 0.547 |
| $a+by/z+cy\sqrt{z}$ | 130.49 | 101.38 | 0.793 | 0.0782 | 0.0503 | 0.6981 | 0.2744 | 0.1840 | 0.681 |
| $a+by/z+cy^2/z$ | 182.40 | 144.92 | 0.595 | 0.1085 | 0.0826 | 0.4191 | 0.3574 | 0.2708 | 0.459 |
| $a+by/z+cy^2/z^2$ | 266.85 | 186.47 | 0.134 | 0.1342 | 0.1013 | 0.1111 | 0.4707 | 0.3448 | 0.061 |
| $a+by/z+cy^2/\sqrt{z}$ | 167.58 | 131.13 | 0.658 | 0.1004 | 0.0747 | 0.5018 | 0.3345 | 0.2458 | 0.526 |
| $a+by/z+cy^2z$ | 149.28 | 112.92 | 0.729 | 0.0863 | 0.0638 | 0.6319 | 0.3151 | 0.2414 | 0.579 |
| $a+by/z+cy^2z^2$ | 168.97 | 126.59 | 0.653 | 0.0936 | 0.0732 | 0.5674 | 0.3449 | 0.2664 | 0.496 |
| $a+by/z+cy^2\sqrt{z}$ | 142.17 | 105.48 | 0.754 | 0.0853 | 0.0608 | 0.6407 | 0.3036 | 0.2175 | 0.609 |
| $a+by/z+c\sqrt{y}/z$ | 171.49 | 117.02 | 0.642 | 0.1024 | 0.0769 | 0.4819 | 0.3273 | 0.2214 | 0.546 |
| $a+by/z+c\sqrt{y}/z^2$ | 246.40 | 182.27 | 0.261 | 0.1309 | 0.1029 | 0.1546 | 0.4405 | 0.3357 | 0.178 |
| $a+by/z+c\sqrt{y}/\sqrt{z}$ | 269.00 | 190.08 | 0.120 | 0.1360 | 0.1037 | 0.0863 | 0.4752 | 0.3545 | 0.043 |
| $a+by/z+c\sqrt{y}z$ | 132.70 | 105.89 | 0.786 | 0.0752 | 0.0515 | 0.7205 | 0.2744 | 0.2028 | 0.681 |
| $a+by/z+c\sqrt{y}z^2$ | 158.04 | 123.57 | 0.696 | 0.0852 | 0.0643 | 0.6420 | 0.3178 | 0.2463 | 0.572 |
| $a+by/z+c\sqrt{y}\sqrt{z}$ | 125.95 | 99.06 | 0.807 | 0.0748 | 0.0444 | 0.7241 | 0.2598 | 0.1657 | 0.714 |
| $a+by/z+c/yz$ | 180.35 | 124.19 | 0.604 | 0.1019 | 0.0755 | 0.4876 | 0.3257 | 0.2244 | 0.550 |
| $a+by/z+c/yz^2$ | 207.54 | 147.53 | 0.476 | 0.1160 | 0.0880 | 0.3352 | 0.3777 | 0.2757 | 0.396 |
| $a+by/z+c/y\sqrt{z}$ | 171.19 | 118.56 | 0.643 | 0.0951 | 0.0679 | 0.5535 | 0.3047 | 0.1977 | 0.607 |
| $a+by/z+cz/y$ | 271.26 | 193.37 | 0.105 | 0.1372 | 0.1054 | 0.0703 | 0.4769 | 0.3633 | 0.036 |
| $a+by/z+cz^2/y$ | 173.43 | 139.06 | 0.634 | 0.0902 | 0.0673 | 0.5981 | 0.3313 | 0.2602 | 0.535 |
| $a+by/z+c\sqrt{z}/y$ | 203.53 | 147.22 | 0.496 | 0.1027 | 0.0732 | 0.4791 | 0.3458 | 0.2405 | 0.493 |
| $a+by/z+c/y^2z$ | 190.00 | 132.50 | 0.561 | 0.1038 | 0.0759 | 0.4681 | 0.3360 | 0.2418 | 0.522 |
| $a+by/z+c/y^2z^2$ | 203.15 | 147.32 | 0.498 | 0.1130 | 0.0844 | 0.3694 | 0.3683 | 0.2751 | 0.425 |
| $a+by/z+c/y^2\sqrt{z}$ | 187.38 | 131.42 | 0.573 | 0.0998 | 0.0708 | 0.5085 | 0.3245 | 0.2225 | 0.554 |
| $a+by/z+cz/y^2$ | 216.74 | 156.46 | 0.428 | 0.1055 | 0.0765 | 0.4501 | 0.3607 | 0.2636 | 0.449 |
| $a+by/z+cz^2/y^2$ | 271.21 | 193.13 | 0.105 | 0.1364 | 0.1056 | 0.0819 | 0.4732 | 0.3629 | 0.051 |
| $a+by/z+c\sqrt{z}/y^2$ | 199.29 | 144.85 | 0.517 | 0.0990 | 0.0690 | 0.5157 | 0.3326 | 0.2361 | 0.531 |
| $a+by/z+c/\sqrt{y}z$ | 175.38 | 118.89 | 0.626 | 0.1012 | 0.0758 | 0.4940 | 0.3221 | 0.2198 | 0.560 |
| $a+by/z+c/\sqrt{y}z^2$ | 215.52 | 155.23 | 0.435 | 0.1196 | 0.0905 | 0.2933 | 0.3915 | 0.2842 | 0.351 |
| $a+by/z+c/\sqrt{y}\sqrt{z}$ | 159.35 | 108.13 | 0.691 | 0.0918 | 0.0660 | 0.5835 | 0.2920 | 0.1829 | 0.639 |
| $a+by/z+cz/\sqrt{y}$ | 155.14 | 125.30 | 0.707 | 0.0840 | 0.0607 | 0.6517 | 0.3038 | 0.2368 | 0.609 |
| $a+by/z+cz^2/\sqrt{y}$ | 159.12 | 126.53 | 0.692 | 0.0832 | 0.0624 | 0.6580 | 0.3102 | 0.2468 | 0.592 |
| $a+by/z+c\sqrt{z}/\sqrt{y}$ | 270.69 | 192.58 | 0.108 | 0.1371 | 0.1051 | 0.0723 | 0.4771 | 0.3612 | 0.036 |
| $a+by/z^2+cy/\sqrt{z}$ | 232.22 | 176.50 | 0.344 | 0.1254 | 0.1003 | 0.2235 | 0.4131 | 0.3243 | 0.277 |
| $a+by/z^2+cyz$ | 137.11 | 107.39 | 0.771 | 0.0788 | 0.0567 | 0.6932 | 0.2898 | 0.2230 | 0.644 |
| $a+by/z^2+cyz^2$ | 157.91 | 121.13 | 0.697 | 0.0877 | 0.0679 | 0.6203 | 0.3262 | 0.2539 | 0.549 |
| $a+by/z^2+cy\sqrt{z}$ | 130.99 | 101.12 | 0.791 | 0.0782 | 0.0498 | 0.6977 | 0.2740 | 0.1845 | 0.682 |
| $a+by/z^2+cy^2/z$ | 235.84 | 183.12 | 0.323 | 0.1283 | 0.1035 | 0.1874 | 0.4245 | 0.3359 | 0.236 |
| $a+by/z^2+cy^2/z^2$ | 228.28 | 170.23 | 0.366 | 0.1268 | 0.1012 | 0.2062 | 0.4140 | 0.3182 | 0.274 |
| $a+by/z^2+cy^2/\sqrt{z}$ | 199.64 | 159.08 | 0.515 | 0.1137 | 0.0901 | 0.3620 | 0.3721 | 0.2847 | 0.413 |
| $a+by/z^2+cy^2z$ | 147.41 | 112.18 | 0.736 | 0.0863 | 0.0635 | 0.6327 | 0.3145 | 0.2416 | 0.581 |
| $a+by/z^2+cy^2z^2$ | 163.65 | 124.12 | 0.674 | 0.0927 | 0.0727 | 0.5758 | 0.3409 | 0.2634 | 0.508 |
| $a+by/z^2+cy^2\sqrt{z}$ | 142.36 | 105.61 | 0.753 | 0.0858 | 0.0607 | 0.6363 | 0.3036 | 0.2155 | 0.609 |
| $a+by/z^2+c\sqrt{y}/z$ | 181.66 | 137.71 | 0.598 | 0.0964 | 0.0652 | 0.5412 | 0.3445 | 0.2393 | 0.497 |
| $a+by/z^2+c\sqrt{y}/z^2$ | 217.45 | 156.56 | 0.425 | 0.1219 | 0.0960 | 0.2667 | 0.3918 | 0.2958 | 0.349 |
| $a+by/z^2+c\sqrt{y}/\sqrt{z}$ | 262.00 | 187.25 | 0.165 | 0.1349 | 0.1029 | 0.1020 | 0.4648 | 0.3526 | 0.085 |
| $a+by/z^2+c\sqrt{y}z$ | 134.33 | 106.99 | 0.780 | 0.0756 | 0.0531 | 0.7176 | 0.2796 | 0.2121 | 0.669 |
| $a+by/z^2+c\sqrt{y}z^2$ | 156.16 | 121.29 | 0.703 | 0.0854 | 0.0652 | 0.6397 | 0.3196 | 0.2472 | 0.567 |
| $a+by/z^2+c\sqrt{y}\sqrt{z}$ | 125.74 | 98.94 | 0.808 | 0.0739 | 0.0437 | 0.7307 | 0.2588 | 0.1708 | 0.716 |
| $a+by/z^2+c/yz$ | 193.96 | 140.56 | 0.542 | 0.1080 | 0.0839 | 0.4241 | 0.3413 | 0.2468 | 0.506 |
| $a+by/z^2+c/yz^2$ | 215.62 | 157.19 | 0.434 | 0.1197 | 0.0951 | 0.2924 | 0.3853 | 0.2915 | 0.371 |
| $a+by/z^2+c/y\sqrt{z}$ | 189.24 | 137.04 | 0.564 | 0.1037 | 0.0782 | 0.4685 | 0.3284 | 0.2297 | 0.543 |
| $a+by/z^2+cz/y$ | 260.63 | 185.70 | 0.174 | 0.1349 | 0.1024 | 0.1016 | 0.4645 | 0.3519 | 0.086 |
| $a+by/z^2+cz^2/y$ | 180.71 | 137.49 | 0.603 | 0.0947 | 0.0696 | 0.5576 | 0.3486 | 0.2577 | 0.485 |
| $a+by/z^2+c\sqrt{z}/y$ | 230.16 | 172.03 | 0.355 | 0.1193 | 0.0924 | 0.2970 | 0.3943 | 0.2942 | 0.341 |
| $a+by/z^2+c/y^2z$ | 208.65 | 149.15 | 0.470 | 0.1132 | 0.0886 | 0.3672 | 0.3632 | 0.2647 | 0.441 |
| $a+by/z^2+c/y^2z^2$ | 216.93 | 157.17 | 0.427 | 0.1195 | 0.0947 | 0.2947 | 0.3862 | 0.2898 | 0.368 |
| $a+by/z^2+c/y^2\sqrt{z}$ | 207.78 | 149.75 | 0.475 | 0.1108 | 0.0848 | 0.3938 | 0.3563 | 0.2520 | 0.462 |
| $a+by/z^2+cz/y^2$ | 233.28 | 173.45 | 0.338 | 0.1183 | 0.0919 | 0.3088 | 0.3942 | 0.2930 | 0.342 |
| $a+by/z^2+cz^2/y^2$ | 261.80 | 187.17 | 0.166 | 0.1356 | 0.1046 | 0.0928 | 0.4646 | 0.3525 | 0.085 |

(continued on next page)

**Table 4 – continued from previous page**

| Functional form | $T_{eff}$ (K) | | | Radius ($R_\odot$) | | | log ($L/L_\odot$) | | |
|---|---|---|---|---|---|---|---|---|---|
| | RMSE | MAD | $R^2_{ap}$ | RMSE | MAD | $R^2_{ap}$ | RMSE | MAD | $R^2_{ap}$ |
| $a+by/z^2+c\sqrt{z}/y^2$ | 219.09 | 163.57 | 0.416 | 0.1122 | 0.0855 | 0.3783 | 0.3687 | 0.2692 | 0.424 |
| $a+by/z^2+c/\sqrt{y}z$ | 177.25 | 126.77 | 0.618 | 0.1017 | 0.0780 | 0.4897 | 0.3170 | 0.2206 | 0.574 |
| $a+by/z^2+c/\sqrt{y}z^2$ | 215.38 | 156.85 | 0.436 | 0.1201 | 0.0954 | 0.2882 | 0.3858 | 0.2929 | 0.369 |
| $a+by/z^2+c/\sqrt{y}\sqrt{z}$ | 167.79 | 118.89 | 0.657 | 0.0952 | 0.0704 | 0.5524 | 0.2976 | 0.1952 | 0.625 |
| $a+by/z^2+cz/\sqrt{y}$ | 179.12 | 137.40 | 0.610 | 0.0942 | 0.0676 | 0.5622 | 0.3449 | 0.2513 | 0.496 |
| $a+by/z^2+cz^2/\sqrt{y}$ | 162.25 | 123.81 | 0.680 | 0.0857 | 0.0634 | 0.6375 | 0.3208 | 0.2479 | 0.564 |
| $a+by/z^2+c\sqrt{z}/\sqrt{y}$ | 260.48 | 185.25 | 0.174 | 0.1345 | 0.1024 | 0.1065 | 0.4642 | 0.3515 | 0.087 |
| $a+by/\sqrt{z}+cyz$ | 135.42 | 105.04 | 0.777 | 0.0784 | 0.0546 | 0.6962 | 0.2826 | 0.2035 | 0.662 |
| $a+by/\sqrt{z}+cyz^2$ | 154.27 | 121.60 | 0.710 | 0.0856 | 0.0637 | 0.6383 | 0.3112 | 0.2368 | 0.590 |
| $a+by/\sqrt{z}+cy\sqrt{z}$ | 130.46 | 101.54 | 0.793 | 0.0779 | 0.0508 | 0.7007 | 0.2744 | 0.1833 | 0.681 |
| $a+by/\sqrt{z}+cy^2/z$ | 260.02 | 192.39 | 0.177 | 0.1251 | 0.0951 | 0.2270 | 0.4235 | 0.3202 | 0.240 |
| $a+by/\sqrt{z}+cy^2/z^2$ | 238.07 | 182.97 | 0.310 | 0.1260 | 0.1009 | 0.2156 | 0.4185 | 0.3287 | 0.258 |
| $a+by/\sqrt{z}+cy^2/\sqrt{z}$ | 169.83 | 136.44 | 0.649 | 0.1025 | 0.0776 | 0.4812 | 0.3467 | 0.2604 | 0.491 |
| $a+by/\sqrt{z}+cy^2z$ | 148.84 | 114.06 | 0.730 | 0.0862 | 0.0626 | 0.6330 | 0.3103 | 0.2262 | 0.592 |
| $a+by/\sqrt{z}+cy^2z^2$ | 164.94 | 127.00 | 0.669 | 0.0922 | 0.0706 | 0.5803 | 0.3327 | 0.2542 | 0.531 |
| $a+by/\sqrt{z}+cy^2\sqrt{z}$ | 143.75 | 105.84 | 0.749 | 0.0856 | 0.0613 | 0.6385 | 0.3040 | 0.2132 | 0.608 |
| $a+by/\sqrt{z}+c\sqrt{y}/z$ | 174.56 | 123.72 | 0.629 | 0.1023 | 0.0756 | 0.4828 | 0.3315 | 0.2273 | 0.534 |
| $a+by/\sqrt{z}+c\sqrt{y}/z^2$ | 226.53 | 169.99 | 0.376 | 0.1238 | 0.0984 | 0.2428 | 0.4053 | 0.3146 | 0.304 |
| $a+by/\sqrt{z}+c\sqrt{y}/\sqrt{z}$ | 146.03 | 104.31 | 0.741 | 0.0914 | 0.0630 | 0.5875 | 0.2981 | 0.1988 | 0.624 |
| $a+by/\sqrt{z}+c\sqrt{y}z$ | 129.75 | 102.92 | 0.795 | 0.0750 | 0.0496 | 0.7222 | 0.2687 | 0.1881 | 0.694 |
| $a+by/\sqrt{z}+c\sqrt{y}z^2$ | 149.07 | 119.79 | 0.730 | 0.0822 | 0.0603 | 0.6663 | 0.2996 | 0.2266 | 0.620 |
| $a+by/\sqrt{z}+c\sqrt{y}\sqrt{z}$ | 126.02 | 99.26 | 0.807 | 0.0749 | 0.0448 | 0.7230 | 0.2608 | 0.1643 | 0.712 |
| $a+by/\sqrt{z}+c/yz$ | 189.77 | 136.47 | 0.562 | 0.1050 | 0.0789 | 0.4560 | 0.3336 | 0.2390 | 0.528 |
| $a+by/\sqrt{z}+c/yz^2$ | 217.17 | 159.35 | 0.426 | 0.1202 | 0.0956 | 0.2869 | 0.3859 | 0.2931 | 0.369 |
| $a+by/\sqrt{z}+c/y\sqrt{z}$ | 180.86 | 130.99 | 0.602 | 0.0969 | 0.0697 | 0.5364 | 0.3101 | 0.2146 | 0.593 |
| $a+by/\sqrt{z}+cz/y$ | 179.16 | 122.61 | 0.609 | 0.1078 | 0.0755 | 0.4263 | 0.3584 | 0.2476 | 0.456 |
| $a+by/\sqrt{z}+cz^2/y$ | 138.96 | 108.00 | 0.765 | 0.0784 | 0.0538 | 0.6969 | 0.2776 | 0.2074 | 0.674 |
| $a+by/\sqrt{z}+c\sqrt{z}/y$ | 270.70 | 200.93 | 0.108 | 0.1267 | 0.0976 | 0.2071 | 0.4329 | 0.3290 | 0.206 |
| $a+by/\sqrt{z}+c/y^2z$ | 219.85 | 155.03 | 0.412 | 0.1143 | 0.0879 | 0.3554 | 0.3697 | 0.2777 | 0.421 |
| $a+by/\sqrt{z}+c/y^2z^2$ | 232.05 | 166.91 | 0.345 | 0.1242 | 0.0961 | 0.2388 | 0.4020 | 0.3081 | 0.315 |
| $a+by/\sqrt{z}+c/y^2\sqrt{z}$ | 218.66 | 154.82 | 0.418 | 0.1098 | 0.0832 | 0.4050 | 0.3582 | 0.2634 | 0.456 |
| $a+by/\sqrt{z}+cz/y^2$ | 276.00 | 204.75 | 0.073 | 0.1289 | 0.0988 | 0.1801 | 0.4413 | 0.3345 | 0.175 |
| $a+by/\sqrt{z}+cz^2/y^2$ | 241.05 | 179.79 | 0.293 | 0.1322 | 0.1007 | 0.1373 | 0.4426 | 0.3334 | 0.170 |
| $a+by/\sqrt{z}+c\sqrt{z}/y^2$ | 244.94 | 177.08 | 0.270 | 0.1140 | 0.0873 | 0.3587 | 0.3864 | 0.2929 | 0.367 |
| $a+by/\sqrt{z}+c/\sqrt{y}z$ | 176.55 | 121.94 | 0.621 | 0.1016 | 0.0767 | 0.4898 | 0.3223 | 0.2215 | 0.560 |
| $a+by/\sqrt{z}+c/\sqrt{y}z^2$ | 215.58 | 155.60 | 0.435 | 0.1201 | 0.0953 | 0.2876 | 0.3868 | 0.2918 | 0.366 |
| $a+by/\sqrt{z}+c/\sqrt{y}\sqrt{z}$ | 159.57 | 110.41 | 0.690 | 0.0912 | 0.0646 | 0.5897 | 0.2902 | 0.1831 | 0.643 |
| $a+by/\sqrt{z}+cz/\sqrt{y}$ | 121.77 | 90.85 | 0.820 | 0.0748 | 0.0465 | 0.7238 | 0.2568 | 0.1683 | 0.721 |
| $a+by/\sqrt{z}+cz^2/\sqrt{y}$ | 140.62 | 114.38 | 0.759 | 0.0773 | 0.0536 | 0.7051 | 0.2792 | 0.2073 | 0.670 |
| $a+by/\sqrt{z}+c\sqrt{z}/\sqrt{y}$ | 145.67 | 101.55 | 0.742 | 0.0944 | 0.0618 | 0.5596 | 0.3116 | 0.2006 | 0.589 |
| $a+byz+cyz^2$ | 131.80 | 103.45 | 0.789 | 0.0772 | 0.0501 | 0.7054 | 0.2737 | 0.1757 | 0.682 |
| $a+byz+cy\sqrt{z}$ | 130.97 | 101.20 | 0.791 | 0.0777 | 0.0520 | 0.7017 | 0.2740 | 0.1768 | 0.682 |
| $a+byz+cy^2/z$ | 135.64 | 105.15 | 0.776 | 0.0787 | 0.0554 | 0.6941 | 0.2849 | 0.2099 | 0.656 |
| $a+byz+cy^2/z^2$ | 137.21 | 106.82 | 0.771 | 0.0786 | 0.0561 | 0.6946 | 0.2880 | 0.2197 | 0.649 |
| $a+byz+cy^2/\sqrt{z}$ | 134.69 | 103.79 | 0.779 | 0.0788 | 0.0555 | 0.6933 | 0.2845 | 0.2065 | 0.657 |
| $a+byz+cy^2z$ | 134.06 | 108.01 | 0.781 | 0.0742 | 0.0500 | 0.7281 | 0.2705 | 0.1987 | 0.690 |
| $a+byz+cy^2z^2$ | 132.36 | 106.53 | 0.787 | 0.0756 | 0.0464 | 0.7175 | 0.2686 | 0.1728 | 0.694 |
| $a+byz+cy^2\sqrt{z}$ | 137.09 | 106.33 | 0.771 | 0.0783 | 0.0573 | 0.6972 | 0.2900 | 0.2233 | 0.644 |
| $a+byz+c\sqrt{y}/z$ | 136.62 | 106.85 | 0.773 | 0.0790 | 0.0568 | 0.6921 | 0.2901 | 0.2229 | 0.643 |
| $a+byz+c\sqrt{y}/z^2$ | 135.85 | 106.36 | 0.775 | 0.0790 | 0.0569 | 0.6922 | 0.2899 | 0.2219 | 0.644 |
| $a+byz+c\sqrt{y}/\sqrt{z}$ | 137.21 | 107.00 | 0.771 | 0.0788 | 0.0560 | 0.6937 | 0.2874 | 0.2163 | 0.650 |
| $a+byz+c\sqrt{y}z$ | 134.33 | 106.83 | 0.780 | 0.0756 | 0.0520 | 0.7174 | 0.2784 | 0.2082 | 0.671 |
| $a+byz+c\sqrt{y}z^2$ | 133.51 | 104.18 | 0.783 | 0.0785 | 0.0538 | 0.6960 | 0.2814 | 0.1942 | 0.664 |
| $a+byz+c\sqrt{y}\sqrt{z}$ | 126.02 | 99.31 | 0.807 | 0.0749 | 0.0447 | 0.7229 | 0.2584 | 0.1516 | 0.717 |
| $a+byz+c/yz$ | 122.39 | 92.70 | 0.818 | 0.0754 | 0.0481 | 0.7196 | 0.2580 | 0.1583 | 0.718 |
| $a+byz+c/yz^2$ | 122.47 | 92.33 | 0.818 | 0.0771 | 0.0505 | 0.7068 | 0.2689 | 0.1753 | 0.694 |
| $a+byz+c/y\sqrt{z}$ | 125.68 | 95.83 | 0.808 | 0.0749 | 0.0468 | 0.7229 | 0.2571 | 0.1547 | 0.720 |
| $a+byz+cz/y$ | 137.32 | 107.30 | 0.771 | 0.0787 | 0.0554 | 0.6944 | 0.2866 | 0.2120 | 0.652 |
| $a+byz+cz^2/y$ | 137.34 | 107.34 | 0.771 | 0.0789 | 0.0572 | 0.6929 | 0.2899 | 0.2217 | 0.644 |
| $a+byz+c\sqrt{z}/y$ | 135.83 | 106.13 | 0.776 | 0.0773 | 0.0515 | 0.7051 | 0.2770 | 0.1915 | 0.675 |
| $a+byz+c/y^2z$ | 126.00 | 95.55 | 0.807 | 0.0753 | 0.0485 | 0.7202 | 0.2600 | 0.1621 | 0.713 |
| $a+byz+c/y^2z^2$ | 122.88 | 91.51 | 0.816 | 0.0762 | 0.0504 | 0.7133 | 0.2638 | 0.1735 | 0.705 |
| $a+byz+c/y^2\sqrt{z}$ | 128.77 | 98.95 | 0.798 | 0.0751 | 0.0474 | 0.7216 | 0.2608 | 0.1628 | 0.712 |
| $a+byz+cz/y^2$ | 136.41 | 107.06 | 0.774 | 0.0768 | 0.0503 | 0.7089 | 0.2761 | 0.1928 | 0.677 |
| $a+byz+cz^2/y^2$ | 137.34 | 107.27 | 0.771 | 0.0785 | 0.0549 | 0.6956 | 0.2862 | 0.2101 | 0.653 |
| $a+byz+c\sqrt{z}/y^2$ | 134.59 | 105.46 | 0.780 | 0.0759 | 0.0485 | 0.7157 | 0.2697 | 0.1827 | 0.692 |
| $a+byz+c/\sqrt{y}z$ | 122.02 | 93.23 | 0.819 | 0.0762 | 0.0481 | 0.7133 | 0.2636 | 0.1637 | 0.705 |
| $a+byz+c/\sqrt{y}z^2$ | 126.46 | 96.61 | 0.805 | 0.0781 | 0.0533 | 0.6991 | 0.2780 | 0.1932 | 0.673 |
| $a+byz+c/\sqrt{y}\sqrt{z}$ | 122.77 | 94.15 | 0.817 | 0.0750 | 0.0464 | 0.7222 | 0.2562 | 0.1506 | 0.722 |
| $a+byz+cz/\sqrt{y}$ | 136.94 | 107.15 | 0.772 | 0.0788 | 0.0569 | 0.6933 | 0.2901 | 0.2230 | 0.644 |
| $a+byz+cz^2/\sqrt{y}$ | 137.17 | 106.75 | 0.771 | 0.0788 | 0.0573 | 0.6932 | 0.2898 | 0.2211 | 0.644 |
| $a+byz+c\sqrt{z}/\sqrt{y}$ | 137.28 | 107.23 | 0.771 | 0.0787 | 0.0557 | 0.6940 | 0.2868 | 0.2133 | 0.651 |
| $a+byz^2+cy\sqrt{z}$ | 131.02 | 100.93 | 0.791 | 0.0780 | 0.0519 | 0.6998 | 0.2737 | 0.1738 | 0.683 |
| $a+byz^2+cy^2/z$ | 156.20 | 121.77 | 0.703 | 0.0867 | 0.0654 | 0.6289 | 0.3172 | 0.2468 | 0.574 |
| $a+byz^2+cy^2/z^2$ | 161.05 | 121.87 | 0.684 | 0.0880 | 0.0678 | 0.6178 | 0.3275 | 0.2546 | 0.546 |
| $a+byz^2+cy^2/\sqrt{z}$ | 147.34 | 115.30 | 0.736 | 0.0848 | 0.0611 | 0.6450 | 0.3051 | 0.2222 | 0.606 |
| $a+byz^2+cy^2z$ | 149.37 | 111.81 | 0.729 | 0.0862 | 0.0645 | 0.6333 | 0.3149 | 0.2393 | 0.580 |
| $a+byz^2+cy^2z^2$ | 157.51 | 122.01 | 0.698 | 0.0820 | 0.0627 | 0.6683 | 0.3081 | 0.2452 | 0.598 |
| $a+byz^2+cy^2\sqrt{z}$ | 143.38 | 106.81 | 0.750 | 0.0842 | 0.0612 | 0.6501 | 0.3035 | 0.2211 | 0.610 |
| $a+byz^2+c\sqrt{y}/z$ | 155.92 | 119.83 | 0.704 | 0.0871 | 0.0670 | 0.6252 | 0.3240 | 0.2504 | 0.555 |
| $a+byz^2+c\sqrt{y}/z^2$ | 152.89 | 118.13 | 0.716 | 0.0869 | 0.0669 | 0.6274 | 0.3214 | 0.2472 | 0.562 |
| $a+byz^2+c\sqrt{y}/\sqrt{z}$ | 161.18 | 123.63 | 0.684 | 0.0879 | 0.0674 | 0.6189 | 0.3262 | 0.2528 | 0.549 |
| $a+byz^2+c\sqrt{y}z$ | 130.66 | 104.77 | 0.792 | 0.0746 | 0.0459 | 0.7251 | 0.2657 | 0.1729 | 0.701 |
| $a+byz^2+c\sqrt{y}z^2$ | 157.17 | 121.27 | 0.699 | 0.0827 | 0.0622 | 0.6626 | 0.3104 | 0.2437 | 0.592 |
| $a+byz^2+c\sqrt{y}\sqrt{z}$ | 125.93 | 99.79 | 0.807 | 0.0748 | 0.0458 | 0.7236 | 0.2606 | 0.1578 | 0.712 |
| $a+byz^2+c/yz$ | 123.14 | 90.04 | 0.815 | 0.0763 | 0.0524 | 0.7123 | 0.2607 | 0.1685 | 0.712 |
| $a+byz^2+c/yz^2$ | 125.18 | 89.90 | 0.809 | 0.0799 | 0.0571 | 0.6845 | 0.2780 | 0.1893 | 0.672 |
| $a+byz^2+c/y\sqrt{z}$ | 128.45 | 94.83 | 0.799 | 0.0758 | 0.0503 | 0.7167 | 0.2599 | 0.1642 | 0.714 |
| $a+byz^2+cz/y$ | 160.61 | 121.62 | 0.686 | 0.0871 | 0.0663 | 0.6257 | 0.3221 | 0.2450 | 0.560 |
| $a+byz^2+cz^2/y$ | 160.36 | 124.28 | 0.687 | 0.0873 | 0.0662 | 0.6236 | 0.3262 | 0.2519 | 0.549 |
| $a+byz^2+c\sqrt{z}/y$ | 153.06 | 120.31 | 0.715 | 0.0826 | 0.0590 | 0.6632 | 0.2992 | 0.2145 | 0.621 |
| $a+byz^2+c/y^2z$ | 132.87 | 99.02 | 0.785 | 0.0778 | 0.0541 | 0.7015 | 0.2696 | 0.1761 | 0.692 |

(continued on next page)

**Table 4 – continued from previous page**

| Functional form | $T_{eff}$ (K) | | | Radius ($R_\odot$) | | | log (L/$L_\odot$) | | |
|---|---|---|---|---|---|---|---|---|---|
| | RMSE | MAD | $R^2_{ap}$ | RMSE | MAD | $R^2_{ap}$ | RMSE | MAD | $R^2_{ap}$ |
| $a+byz^2+c/y^2z^2$ | 129.29 | 92.62 | 0.797 | 0.0796 | 0.0576 | 0.6875 | 0.2760 | 0.1917 | 0.677 |
| $a+byz^2+c/y^2\sqrt{z}$ | 137.22 | 105.01 | 0.771 | 0.0775 | 0.0524 | 0.7033 | 0.2709 | 0.1751 | 0.689 |
| $a+byz^2+cz/y^2$ | 154.47 | 119.99 | 0.710 | 0.0818 | 0.0583 | 0.6696 | 0.2981 | 0.2131 | 0.623 |
| $a+byz^2+cz^2/y^2$ | 160.43 | 120.75 | 0.687 | 0.0863 | 0.0654 | 0.6319 | 0.3196 | 0.2397 | 0.567 |
| $a+byz^2+c\sqrt{z}/y^2$ | 149.07 | 116.68 | 0.730 | 0.0796 | 0.0553 | 0.6870 | 0.2862 | 0.1993 | 0.653 |
| $a+byz^2+c/\sqrt{y}z$ | 121.07 | 90.07 | 0.822 | 0.0771 | 0.0518 | 0.7063 | 0.2659 | 0.1691 | 0.701 |
| $a+byz^2+c/\sqrt{y}z^2$ | 131.37 | 98.53 | 0.790 | 0.0820 | 0.0593 | 0.6676 | 0.2915 | 0.2042 | 0.640 |
| $a+byz^2+c/\sqrt{y}\sqrt{z}$ | 121.32 | 91.39 | 0.821 | 0.0749 | 0.0486 | 0.7232 | 0.2551 | 0.1570 | 0.724 |
| $a+byz^2+cz/\sqrt{y}$ | 157.50 | 121.58 | 0.698 | 0.0866 | 0.0651 | 0.6296 | 0.3233 | 0.2478 | 0.557 |
| $a+byz^2+cz^2/\sqrt{y}$ | 158.77 | 123.03 | 0.693 | 0.0854 | 0.0633 | 0.6403 | 0.3198 | 0.2469 | 0.567 |
| $a+byz^2+c\sqrt{z}/\sqrt{y}$ | 160.81 | 122.50 | 0.685 | 0.0874 | 0.0668 | 0.6227 | 0.3236 | 0.2486 | 0.556 |
| $a+by\sqrt{z}+cy^2/z$ | 130.66 | 101.74 | 0.792 | 0.0777 | 0.0504 | 0.7018 | 0.2745 | 0.1851 | 0.681 |
| $a+by\sqrt{z}+cy^2/z^2$ | 131.17 | 101.19 | 0.791 | 0.0783 | 0.0500 | 0.6971 | 0.2738 | 0.1826 | 0.682 |
| $a+by\sqrt{z}+cy^2/\sqrt{z}$ | 130.22 | 101.75 | 0.794 | 0.0767 | 0.0503 | 0.7093 | 0.2741 | 0.1894 | 0.682 |
| $a+by\sqrt{z}+cy^2z$ | 131.15 | 100.33 | 0.791 | 0.0781 | 0.0480 | 0.6987 | 0.2670 | 0.1563 | 0.698 |
| $a+by\sqrt{z}+cy^2z^2$ | 131.21 | 100.84 | 0.791 | 0.0783 | 0.0504 | 0.6971 | 0.2715 | 0.1641 | 0.688 |
| $a+by\sqrt{z}+cy^2\sqrt{z}$ | 129.10 | 99.75 | 0.797 | 0.0749 | 0.0441 | 0.7234 | 0.2556 | 0.1526 | 0.723 |
| $a+by\sqrt{z}+c\sqrt{y}/z$ | 129.72 | 100.55 | 0.795 | 0.0783 | 0.0501 | 0.6976 | 0.2744 | 0.1856 | 0.681 |
| $a+by\sqrt{z}+c\sqrt{y}/z^2$ | 130.60 | 100.76 | 0.792 | 0.0782 | 0.0500 | 0.6978 | 0.2744 | 0.1855 | 0.681 |
| $a+by\sqrt{z}+c\sqrt{y}/\sqrt{z}$ | 129.85 | 101.03 | 0.795 | 0.0780 | 0.0504 | 0.6995 | 0.2745 | 0.1851 | 0.681 |
| $a+by\sqrt{z}+c\sqrt{y}z$ | 129.38 | 101.56 | 0.796 | 0.0760 | 0.0513 | 0.7151 | 0.2734 | 0.1931 | 0.683 |
| $a+by\sqrt{z}+c\sqrt{y}z^2$ | 130.69 | 100.88 | 0.792 | 0.0774 | 0.0522 | 0.7040 | 0.2744 | 0.1826 | 0.681 |
| $a+by\sqrt{z}+c\sqrt{y}\sqrt{z}$ | 125.74 | 99.53 | 0.808 | 0.0739 | 0.0436 | 0.7302 | 0.2589 | 0.1693 | 0.716 |
| $a+by\sqrt{z}+c/yz$ | 128.30 | 95.85 | 0.800 | 0.0780 | 0.0483 | 0.6998 | 0.2634 | 0.1488 | 0.706 |
| $a+by\sqrt{z}+c/yz^2$ | 127.24 | 95.19 | 0.803 | 0.0783 | 0.0494 | 0.6975 | 0.2682 | 0.1609 | 0.695 |
| $a+by\sqrt{z}+c/y\sqrt{z}$ | 130.04 | 98.12 | 0.794 | 0.0779 | 0.0479 | 0.7004 | 0.2635 | 0.1487 | 0.706 |
| $a+by\sqrt{z}+cz/y$ | 127.63 | 99.05 | 0.802 | 0.0777 | 0.0508 | 0.7016 | 0.2744 | 0.1875 | 0.681 |
| $a+by\sqrt{z}+cz^2/y$ | 127.49 | 101.18 | 0.802 | 0.0760 | 0.0504 | 0.7148 | 0.2725 | 0.1940 | 0.685 |
| $a+by\sqrt{z}+c\sqrt{z}/y$ | 130.02 | 100.51 | 0.794 | 0.0783 | 0.0504 | 0.6971 | 0.2732 | 0.1745 | 0.684 |
| $a+by\sqrt{z}+c/y^2z$ | 129.77 | 97.53 | 0.795 | 0.0779 | 0.0482 | 0.7002 | 0.2644 | 0.1512 | 0.704 |
| $a+by\sqrt{z}+c/y^2z^2$ | 127.84 | 94.70 | 0.801 | 0.0781 | 0.0488 | 0.6988 | 0.2656 | 0.1562 | 0.701 |
| $a+by\sqrt{z}+c/y^2\sqrt{z}$ | 130.76 | 99.29 | 0.792 | 0.0779 | 0.0479 | 0.7004 | 0.2651 | 0.1542 | 0.702 |
| $a+by\sqrt{z}+cz/y^2$ | 129.76 | 99.81 | 0.795 | 0.0783 | 0.0495 | 0.6974 | 0.2724 | 0.1729 | 0.686 |
| $a+by\sqrt{z}+cz^2/y^2$ | 126.61 | 97.52 | 0.805 | 0.0779 | 0.0509 | 0.7002 | 0.2744 | 0.1871 | 0.681 |
| $a+by\sqrt{z}+c\sqrt{z}/y^2$ | 130.93 | 100.85 | 0.791 | 0.0781 | 0.0483 | 0.6987 | 0.2698 | 0.1671 | 0.692 |
| $a+by\sqrt{z}+c/\sqrt{y}z$ | 126.93 | 94.92 | 0.804 | 0.0780 | 0.0483 | 0.6992 | 0.2653 | 0.1539 | 0.702 |
| $a+by\sqrt{z}+c/\sqrt{y}z^2$ | 128.11 | 97.11 | 0.800 | 0.0783 | 0.0501 | 0.6971 | 0.2718 | 0.1729 | 0.687 |
| $a+by\sqrt{z}+c/\sqrt{y}\sqrt{z}$ | 128.36 | 96.17 | 0.800 | 0.0778 | 0.0479 | 0.7013 | 0.2618 | 0.1467 | 0.710 |
| $a+by\sqrt{z}+cz/\sqrt{y}$ | 126.86 | 100.12 | 0.804 | 0.0764 | 0.0494 | 0.7119 | 0.2724 | 0.1920 | 0.686 |
| $a+by\sqrt{z}+cz^2/\sqrt{y}$ | 128.89 | 101.81 | 0.798 | 0.0760 | 0.0513 | 0.7151 | 0.2731 | 0.1939 | 0.684 |
| $a+by\sqrt{z}+c\sqrt{z}/\sqrt{y}$ | 128.32 | 99.69 | 0.800 | 0.0777 | 0.0507 | 0.7016 | 0.2744 | 0.1871 | 0.681 |
| $a+by^2/z+cy^2/z^2$ | 242.91 | 190.42 | 0.282 | 0.1301 | 0.1055 | 0.1647 | 0.4337 | 0.3461 | 0.203 |
| $a+by^2/z+cy^2/\sqrt{z}$ | 162.34 | 125.42 | 0.679 | 0.0959 | 0.0686 | 0.5458 | 0.3253 | 0.2299 | 0.552 |
| $a+by^2/z+cy^2z$ | 149.30 | 113.86 | 0.729 | 0.0864 | 0.0634 | 0.6314 | 0.3130 | 0.2335 | 0.585 |
| $a+by^2/z+cy^2z^2$ | 166.91 | 128.42 | 0.661 | 0.0932 | 0.0719 | 0.5714 | 0.3385 | 0.2632 | 0.515 |
| $a+by^2/z+cy^2\sqrt{z}$ | 143.40 | 106.44 | 0.750 | 0.0851 | 0.0608 | 0.6424 | 0.3040 | 0.2170 | 0.608 |
| $a+by^2/z+c\sqrt{y}/z$ | 173.66 | 129.43 | 0.633 | 0.1044 | 0.0778 | 0.4616 | 0.3388 | 0.2433 | 0.514 |
| $a+by^2/z+c\sqrt{y}/z^2$ | 228.70 | 174.23 | 0.364 | 0.1259 | 0.1006 | 0.2180 | 0.4134 | 0.3228 | 0.276 |
| $a+by^2/z+c\sqrt{y}/\sqrt{z}$ | 159.13 | 124.62 | 0.692 | 0.1010 | 0.0728 | 0.4967 | 0.3338 | 0.2403 | 0.528 |
| $a+by^2/z+c\sqrt{y}z$ | 129.69 | 102.79 | 0.795 | 0.0754 | 0.0506 | 0.7196 | 0.2712 | 0.1945 | 0.688 |
| $a+by^2/z+c\sqrt{y}z^2$ | 150.99 | 120.50 | 0.723 | 0.0834 | 0.0622 | 0.6564 | 0.3058 | 0.2373 | 0.604 |
| $a+by^2/z+c\sqrt{y}\sqrt{z}$ | 125.91 | 98.68 | 0.807 | 0.0749 | 0.0447 | 0.7230 | 0.2610 | 0.1663 | 0.711 |
| $a+by^2/z+c/yz$ | 192.32 | 139.53 | 0.550 | 0.1051 | 0.0787 | 0.4545 | 0.3349 | 0.2399 | 0.525 |
| $a+by^2/z+c/yz^2$ | 217.14 | 159.03 | 0.426 | 0.1198 | 0.0947 | 0.2919 | 0.3855 | 0.2913 | 0.370 |
| $a+by^2/z+c/y\sqrt{z}$ | 186.63 | 135.69 | 0.576 | 0.0983 | 0.0699 | 0.5226 | 0.3156 | 0.2191 | 0.578 |
| $a+by^2/z+cz/y$ | 230.11 | 164.99 | 0.356 | 0.1272 | 0.0915 | 0.2017 | 0.4319 | 0.3163 | 0.209 |
| $a+by^2/z+cz^2/y$ | 145.90 | 114.72 | 0.741 | 0.0824 | 0.0575 | 0.6650 | 0.2938 | 0.2274 | 0.634 |
| $a+by^2/z+c\sqrt{z}/y$ | 267.47 | 197.26 | 0.130 | 0.1258 | 0.0971 | 0.2185 | 0.4291 | 0.3275 | 0.220 |
| $a+by^2/z+c/y^2z$ | 221.72 | 156.75 | 0.402 | 0.1140 | 0.0870 | 0.3582 | 0.3703 | 0.2759 | 0.419 |
| $a+by^2/z+c/y^2z^2$ | 231.02 | 165.85 | 0.351 | 0.1228 | 0.0954 | 0.2554 | 0.3989 | 0.3067 | 0.326 |
| $a+by^2/z+c/y^2\sqrt{z}$ | 222.29 | 156.08 | 0.399 | 0.1107 | 0.0822 | 0.3951 | 0.3624 | 0.2645 | 0.444 |
| $a+by^2/z+cz/y^2$ | 272.74 | 201.35 | 0.095 | 0.1276 | 0.0984 | 0.1965 | 0.4367 | 0.3318 | 0.192 |
| $a+by^2/z+cz^2/y^2$ | 272.19 | 206.43 | 0.099 | 0.1426 | 0.1092 | -0.0041 | 0.4853 | 0.3668 | 0.002 |
| $a+by^2/z+c\sqrt{z}/y^2$ | 246.55 | 177.84 | 0.260 | 0.1154 | 0.0877 | 0.3430 | 0.3904 | 0.2967 | 0.354 |
| $a+by^2/z+c/\sqrt{y}z$ | 177.13 | 123.59 | 0.618 | 0.1016 | 0.0765 | 0.4899 | 0.3223 | 0.2219 | 0.560 |
| $a+by^2/z+c/\sqrt{y}z^2$ | 215.64 | 155.72 | 0.434 | 0.1203 | 0.0949 | 0.2852 | 0.3883 | 0.2920 | 0.361 |
| $a+by^2/z+c/\sqrt{y}\sqrt{z}$ | 162.67 | 113.48 | 0.678 | 0.0917 | 0.0650 | 0.5844 | 0.2920 | 0.1837 | 0.639 |
| $a+by^2/z+cz/\sqrt{y}$ | 127.07 | 96.30 | 0.804 | 0.0785 | 0.0481 | 0.6955 | 0.2720 | 0.1865 | 0.686 |
| $a+by^2/z+cz^2/\sqrt{y}$ | 143.57 | 116.21 | 0.749 | 0.0793 | 0.0566 | 0.6895 | 0.2882 | 0.2224 | 0.648 |
| $a+by^2/z+c\sqrt{z}/\sqrt{y}$ | 198.87 | 135.71 | 0.519 | 0.1155 | 0.0800 | 0.3414 | 0.3908 | 0.2786 | 0.353 |
| $a+by^2/z^2+cy^2/\sqrt{z}$ | 197.12 | 159.09 | 0.527 | 0.1117 | 0.0883 | 0.3841 | 0.3688 | 0.2813 | 0.424 |
| $a+by^2/z^2+cy^2z$ | 149.37 | 112.70 | 0.729 | 0.0864 | 0.0636 | 0.6314 | 0.3151 | 0.2416 | 0.579 |
| $a+by^2/z^2+cy^2z^2$ | 168.59 | 125.76 | 0.654 | 0.0936 | 0.0734 | 0.5676 | 0.3448 | 0.2666 | 0.496 |
| $a+by^2/z^2+cy^2\sqrt{z}$ | 143.48 | 105.85 | 0.750 | 0.0858 | 0.0609 | 0.6363 | 0.3041 | 0.2157 | 0.608 |
| $a+by^2/z^2+c\sqrt{y}/z$ | 134.59 | 97.74 | 0.780 | 0.0867 | 0.0571 | 0.6286 | 0.2810 | 0.1697 | 0.665 |
| $a+by^2/z^2+c\sqrt{y}/z^2$ | 221.65 | 162.64 | 0.402 | 0.1240 | 0.0972 | 0.2408 | 0.4016 | 0.3022 | 0.317 |
| $a+by^2/z^2+c\sqrt{y}/\sqrt{z}$ | 268.26 | 188.39 | 0.124 | 0.1353 | 0.1025 | 0.0955 | 0.4738 | 0.3494 | 0.049 |
| $a+by^2/z^2+c\sqrt{y}z$ | 133.09 | 105.67 | 0.785 | 0.0752 | 0.0519 | 0.7205 | 0.2759 | 0.2066 | 0.677 |
| $a+by^2/z^2+c\sqrt{y}z^2$ | 158.25 | 122.46 | 0.695 | 0.0854 | 0.0646 | 0.6402 | 0.3192 | 0.2466 | 0.568 |
| $a+by^2/z^2+c\sqrt{y}\sqrt{z}$ | 125.46 | 98.10 | 0.808 | 0.0743 | 0.0441 | 0.7276 | 0.2581 | 0.1664 | 0.718 |
| $a+by^2/z^2+c/yz$ | 192.96 | 139.64 | 0.547 | 0.1070 | 0.0824 | 0.4351 | 0.3393 | 0.2430 | 0.512 |
| $a+by^2/z^2+c/yz^2$ | 215.87 | 157.58 | 0.433 | 0.1195 | 0.0947 | 0.2943 | 0.3852 | 0.2910 | 0.371 |
| $a+by^2/z^2+c/y\sqrt{z}$ | 187.97 | 135.48 | 0.570 | 0.1021 | 0.0758 | 0.4855 | 0.3249 | 0.2238 | 0.553 |
| $a+by^2/z^2+cz/y$ | 274.13 | 195.03 | 0.086 | 0.1393 | 0.1061 | 0.0424 | 0.4833 | 0.3650 | 0.010 |
| $a+by^2/z^2+cz^2/y$ | 178.69 | 139.11 | 0.612 | 0.0929 | 0.0684 | 0.5734 | 0.3420 | 0.2594 | 0.505 |
| $a+by^2/z^2+c\sqrt{z}/y$ | 238.90 | 179.05 | 0.306 | 0.1202 | 0.0932 | 0.2871 | 0.4019 | 0.3003 | 0.315 |
| $a+by^2/z^2+c/y^2z$ | 210.21 | 149.50 | 0.462 | 0.1124 | 0.0866 | 0.3765 | 0.3625 | 0.2617 | 0.443 |
| $a+by^2/z^2+c/y^2z^2$ | 219.09 | 157.85 | 0.416 | 0.1195 | 0.0939 | 0.2947 | 0.3875 | 0.2920 | 0.364 |
| $a+by^2/z^2+c/y^2\sqrt{z}$ | 209.94 | 150.88 | 0.464 | 0.1098 | 0.0822 | 0.4049 | 0.3556 | 0.2500 | 0.464 |
| $a+by^2/z^2+cz/y^2$ | 244.12 | 180.12 | 0.275 | 0.1201 | 0.0934 | 0.2883 | 0.4052 | 0.3017 | 0.304 |

(continued on next page)

**Table 4 – continued from previous page**

| Functional form | $T_{eff}$ (K) RMSE | MAD | $R^2_{ap}$ | Radius ($R_\odot$) RMSE | MAD | $R^2_{ap}$ | log ($L/L_\odot$) RMSE | MAD | $R^2_{ap}$ |
|---|---|---|---|---|---|---|---|---|---|
| $a+by^2/z^2+cz^2/y^2$ | 277.62 | 198.38 | 0.062 | 0.1408 | 0.1082 | 0.0213 | 0.4862 | 0.3717 | -0.002 |
| $a+by^2/z^2+c\sqrt{z}/y^2$ | 225.79 | 167.37 | 0.380 | 0.1123 | 0.0856 | 0.3776 | 0.3734 | 0.2733 | 0.409 |
| $a+by^2/z^2+c/\sqrt{y}z$ | 177.59 | 126.31 | 0.616 | 0.1021 | 0.0783 | 0.4854 | 0.3199 | 0.2238 | 0.566 |
| $a+by^2/z^2+c/\sqrt{y}z^2$ | 215.43 | 156.58 | 0.435 | 0.1202 | 0.0952 | 0.2865 | 0.3866 | 0.2932 | 0.367 |
| $a+by^2/z^2+c/\sqrt{y}\sqrt{z}$ | 166.65 | 117.62 | 0.662 | 0.0946 | 0.0698 | 0.5579 | 0.2973 | 0.1926 | 0.626 |
| $a+by^2/z^2+cz/\sqrt{y}$ | 169.01 | 134.24 | 0.652 | 0.0900 | 0.0649 | 0.6005 | 0.3274 | 0.2460 | 0.546 |
| $a+by^2/z^2+cz^2/\sqrt{y}$ | 161.61 | 125.77 | 0.682 | 0.0846 | 0.0625 | 0.6465 | 0.3162 | 0.2477 | 0.576 |
| $a+by^2/z^2+c\sqrt{z}/\sqrt{y}$ | 272.04 | 192.86 | 0.100 | 0.1380 | 0.1050 | 0.0594 | 0.4804 | 0.3599 | 0.022 |
| $a+by^2/\sqrt{z}+cy^2z$ | 147.63 | 111.67 | 0.735 | 0.0863 | 0.0628 | 0.6326 | 0.3096 | 0.2234 | 0.594 |
| $a+by^2/\sqrt{z}+cy^2z^2$ | 157.26 | 121.15 | 0.699 | 0.0908 | 0.0668 | 0.5933 | 0.3233 | 0.2356 | 0.557 |
| $a+by^2/\sqrt{z}+cy^2\sqrt{z}$ | 143.81 | 106.36 | 0.748 | 0.0850 | 0.0609 | 0.6436 | 0.3041 | 0.2160 | 0.608 |
| $a+by^2/\sqrt{z}+c\sqrt{y}/z$ | 164.59 | 125.64 | 0.670 | 0.0997 | 0.0733 | 0.5090 | 0.3274 | 0.2360 | 0.546 |
| $a+by^2/\sqrt{z}+c\sqrt{y}/z^2$ | 198.72 | 154.91 | 0.520 | 0.1138 | 0.0894 | 0.3607 | 0.3699 | 0.2796 | 0.420 |
| $a+by^2/\sqrt{z}+c\sqrt{y}/\sqrt{z}$ | 153.75 | 119.59 | 0.712 | 0.0957 | 0.0691 | 0.5474 | 0.3205 | 0.2301 | 0.565 |
| $a+by^2/\sqrt{z}+c\sqrt{y}z$ | 128.84 | 101.12 | 0.798 | 0.0758 | 0.0511 | 0.7163 | 0.2723 | 0.1939 | 0.686 |
| $a+by^2/\sqrt{z}+c\sqrt{y}z^2$ | 142.05 | 111.47 | 0.755 | 0.0817 | 0.0586 | 0.6705 | 0.2949 | 0.2149 | 0.632 |
| $a+by^2/\sqrt{z}+c\sqrt{y}\sqrt{z}$ | 126.02 | 99.27 | 0.807 | 0.0745 | 0.0450 | 0.7258 | 0.2625 | 0.1713 | 0.708 |
| $a+by^2/\sqrt{z}+c/yz$ | 202.39 | 145.03 | 0.502 | 0.1103 | 0.0848 | 0.3991 | 0.3459 | 0.2483 | 0.493 |
| $a+by^2/\sqrt{z}+c/yz^2$ | 210.05 | 156.13 | 0.463 | 0.1175 | 0.0927 | 0.3184 | 0.3718 | 0.2841 | 0.414 |
| $a+by^2/\sqrt{z}+c/y\sqrt{z}$ | 207.73 | 150.11 | 0.475 | 0.1086 | 0.0816 | 0.4172 | 0.3427 | 0.2426 | 0.502 |
| $a+by^2/\sqrt{z}+cz/y$ | 150.57 | 110.98 | 0.724 | 0.0979 | 0.0689 | 0.5266 | 0.3274 | 0.2303 | 0.546 |
| $a+by^2/\sqrt{z}+cz^2/y$ | 126.97 | 95.99 | 0.804 | 0.0780 | 0.0507 | 0.6999 | 0.2746 | 0.1908 | 0.681 |
| $a+by^2/\sqrt{z}+c\sqrt{z}/y$ | 235.22 | 201.34 | 0.327 | 0.1287 | 0.1055 | 0.1818 | 0.4248 | 0.3391 | 0.235 |
| $a+by^2/\sqrt{z}+c/y^2z$ | 234.85 | 179.91 | 0.329 | 0.1226 | 0.0959 | 0.2583 | 0.3925 | 0.2958 | 0.347 |
| $a+by^2/\sqrt{z}+c/y^2z^2$ | 231.99 | 179.17 | 0.345 | 0.1242 | 0.0989 | 0.2386 | 0.3972 | 0.3055 | 0.332 |
| $a+by^2/\sqrt{z}+c/y^2\sqrt{z}$ | 238.72 | 184.76 | 0.307 | 0.1226 | 0.0959 | 0.2582 | 0.3946 | 0.2991 | 0.340 |
| $a+by^2/\sqrt{z}+cz/y^2$ | 245.57 | 203.91 | 0.266 | 0.1302 | 0.1058 | 0.1627 | 0.4287 | 0.3341 | 0.221 |
| $a+by^2/\sqrt{z}+cz^2/y^2$ | 174.11 | 136.81 | 0.631 | 0.1086 | 0.0808 | 0.4182 | 0.3592 | 0.2658 | 0.453 |
| $a+by^2/\sqrt{z}+c\sqrt{z}/y^2$ | 249.06 | 201.88 | 0.245 | 0.1275 | 0.1008 | 0.1973 | 0.4179 | 0.3272 | 0.260 |
| $a+by^2/\sqrt{z}+c/\sqrt{y}z$ | 175.71 | 126.53 | 0.624 | 0.1018 | 0.0785 | 0.4887 | 0.3192 | 0.2213 | 0.568 |
| $a+by^2/\sqrt{z}+c/\sqrt{y}z^2$ | 200.15 | 150.07 | 0.513 | 0.1146 | 0.0905 | 0.3520 | 0.3644 | 0.2741 | 0.437 |
| $a+by^2/\sqrt{z}+c/\sqrt{y}\sqrt{z}$ | 169.02 | 119.54 | 0.652 | 0.0946 | 0.0689 | 0.5585 | 0.2966 | 0.1899 | 0.627 |
| $a+by^2/\sqrt{z}+cz/\sqrt{y}$ | 121.09 | 89.50 | 0.822 | 0.0782 | 0.0484 | 0.6981 | 0.2701 | 0.1769 | 0.691 |
| $a+by^2/\sqrt{z}+cz^2/\sqrt{y}$ | 131.42 | 104.09 | 0.790 | 0.0771 | 0.0519 | 0.7064 | 0.2764 | 0.1972 | 0.676 |
| $a+by^2/\sqrt{z}+c\sqrt{z}/\sqrt{y}$ | 144.44 | 109.77 | 0.746 | 0.0944 | 0.0662 | 0.5599 | 0.3169 | 0.2242 | 0.575 |
| $a+by^2z+cy^2z^2$ | 144.04 | 107.53 | 0.748 | 0.0846 | 0.0593 | 0.6464 | 0.3006 | 0.2044 | 0.617 |
| $a+by^2z+cy^2\sqrt{z}$ | 144.49 | 104.98 | 0.746 | 0.0856 | 0.0614 | 0.6383 | 0.3036 | 0.2099 | 0.609 |
| $a+by^2z+c\sqrt{y}/z$ | 145.03 | 111.54 | 0.744 | 0.0855 | 0.0627 | 0.6387 | 0.3121 | 0.2395 | 0.587 |
| $a+by^2z+c\sqrt{y}/z^2$ | 144.24 | 110.13 | 0.747 | 0.0858 | 0.0629 | 0.6361 | 0.3117 | 0.2368 | 0.588 |
| $a+by^2z+c\sqrt{y}/\sqrt{z}$ | 149.27 | 113.03 | 0.729 | 0.0863 | 0.0638 | 0.6320 | 0.3151 | 0.2411 | 0.579 |
| $a+by^2z+c\sqrt{y}z$ | 134.26 | 106.91 | 0.781 | 0.0751 | 0.0516 | 0.7216 | 0.2754 | 0.2047 | 0.679 |
| $a+by^2z+c\sqrt{y}z^2$ | 149.44 | 112.04 | 0.728 | 0.0847 | 0.0645 | 0.6458 | 0.3137 | 0.2454 | 0.583 |
| $a+by^2z+c\sqrt{y}\sqrt{z}$ | 126.02 | 99.49 | 0.807 | 0.0748 | 0.0440 | 0.7240 | 0.2572 | 0.1526 | 0.720 |
| $a+by^2z+c/yz$ | 124.75 | 90.77 | 0.811 | 0.0790 | 0.0531 | 0.6915 | 0.2664 | 0.1643 | 0.699 |
| $a+by^2z+c/yz^2$ | 125.11 | 90.40 | 0.810 | 0.0816 | 0.0562 | 0.6711 | 0.2800 | 0.1831 | 0.668 |
| $a+by^2z+c/y\sqrt{z}$ | 129.75 | 94.69 | 0.795 | 0.0788 | 0.0515 | 0.6935 | 0.2666 | 0.1613 | 0.699 |
| $a+by^2z+cz/y$ | 149.30 | 113.33 | 0.729 | 0.0864 | 0.0636 | 0.6314 | 0.3146 | 0.2379 | 0.581 |
| $a+by^2z+cz^2/y$ | 146.26 | 111.49 | 0.740 | 0.0838 | 0.0629 | 0.6532 | 0.3105 | 0.2437 | 0.592 |
| $a+by^2z+c\sqrt{z}/y$ | 147.83 | 113.67 | 0.734 | 0.0845 | 0.0585 | 0.6476 | 0.3011 | 0.2054 | 0.616 |
| $a+by^2z+c/y^2z$ | 131.66 | 96.73 | 0.789 | 0.0800 | 0.0537 | 0.6839 | 0.2732 | 0.1708 | 0.684 |
| $a+by^2z+c/y^2z^2$ | 127.87 | 90.93 | 0.801 | 0.0812 | 0.0562 | 0.6745 | 0.2776 | 0.1845 | 0.674 |
| $a+by^2z+c/y^2\sqrt{z}$ | 135.44 | 101.78 | 0.777 | 0.0799 | 0.0523 | 0.6846 | 0.2747 | 0.1712 | 0.680 |
| $a+by^2z+cz/y^2$ | 147.94 | 113.51 | 0.734 | 0.0835 | 0.0569 | 0.6555 | 0.2984 | 0.2057 | 0.623 |
| $a+by^2z+cz^2/y^2$ | 149.33 | 113.48 | 0.729 | 0.0863 | 0.0631 | 0.6319 | 0.3138 | 0.2348 | 0.583 |
| $a+by^2z+c\sqrt{z}/y^2$ | 144.52 | 111.26 | 0.746 | 0.0818 | 0.0545 | 0.6700 | 0.2883 | 0.1935 | 0.648 |
| $a+by^2z+c/\sqrt{y}z$ | 122.30 | 90.72 | 0.818 | 0.0793 | 0.0526 | 0.6892 | 0.2697 | 0.1635 | 0.692 |
| $a+by^2z+c/\sqrt{y}z^2$ | 129.51 | 95.22 | 0.796 | 0.0830 | 0.0580 | 0.6597 | 0.2906 | 0.1993 | 0.642 |
| $a+by^2z+c/\sqrt{y}\sqrt{z}$ | 123.70 | 92.04 | 0.814 | 0.0777 | 0.0504 | 0.7018 | 0.2610 | 0.1508 | 0.711 |
| $a+by^2z+cz/\sqrt{y}$ | 143.91 | 111.01 | 0.748 | 0.0835 | 0.0617 | 0.6554 | 0.3085 | 0.2404 | 0.597 |
| $a+by^2z+cz^2/\sqrt{y}$ | 146.51 | 110.88 | 0.739 | 0.0827 | 0.0621 | 0.6624 | 0.3080 | 0.2415 | 0.598 |
| $a+by^2z+c\sqrt{z}/\sqrt{y}$ | 149.28 | 113.24 | 0.729 | 0.0864 | 0.0638 | 0.6316 | 0.3148 | 0.2392 | 0.580 |
| $a+by^2z^2+cy^2\sqrt{z}$ | 144.54 | 104.61 | 0.746 | 0.0859 | 0.0613 | 0.6360 | 0.3030 | 0.2076 | 0.611 |
| $a+by^2z^2+c\sqrt{y}/z$ | 159.73 | 121.47 | 0.690 | 0.0912 | 0.0707 | 0.5892 | 0.3356 | 0.2567 | 0.523 |
| $a+by^2z^2+c\sqrt{y}/z^2$ | 157.19 | 120.39 | 0.699 | 0.0913 | 0.0711 | 0.5882 | 0.3338 | 0.2547 | 0.528 |
| $a+by^2z^2+c\sqrt{y}/\sqrt{z}$ | 169.24 | 127.77 | 0.652 | 0.0937 | 0.0731 | 0.5668 | 0.3450 | 0.2659 | 0.496 |
| $a+by^2z^2+c\sqrt{y}z$ | 132.74 | 106.31 | 0.786 | 0.0746 | 0.0473 | 0.7254 | 0.2682 | 0.1841 | 0.695 |
| $a+by^2z^2+c\sqrt{y}z^2$ | 157.25 | 121.52 | 0.699 | 0.0823 | 0.0624 | 0.6656 | 0.3092 | 0.2444 | 0.595 |
| $a+by^2z^2+c\sqrt{y}\sqrt{z}$ | 125.80 | 99.56 | 0.807 | 0.0749 | 0.0449 | 0.7230 | 0.2600 | 0.1573 | 0.714 |
| $a+by^2z^2+c/yz$ | 124.32 | 88.98 | 0.812 | 0.0791 | 0.0551 | 0.6910 | 0.2667 | 0.1743 | 0.699 |
| $a+by^2z^2+c/yz^2$ | 126.77 | 89.27 | 0.804 | 0.0832 | 0.0606 | 0.6579 | 0.2858 | 0.1982 | 0.654 |
| $a+by^2z^2+c/y\sqrt{z}$ | 130.72 | 95.12 | 0.792 | 0.0787 | 0.0529 | 0.6940 | 0.2668 | 0.1694 | 0.698 |
| $a+by^2z^2+cz/y$ | 169.64 | 129.60 | 0.650 | 0.0936 | 0.0726 | 0.5673 | 0.3433 | 0.2627 | 0.501 |
| $a+by^2z^2+cz^2/y$ | 163.42 | 125.81 | 0.675 | 0.0897 | 0.0667 | 0.6031 | 0.3338 | 0.2532 | 0.528 |
| $a+by^2z^2+c\sqrt{z}/y$ | 161.95 | 125.48 | 0.681 | 0.0886 | 0.0652 | 0.6122 | 0.3177 | 0.2279 | 0.572 |
| $a+by^2z^2+c/y^2z$ | 136.83 | 100.75 | 0.772 | 0.0816 | 0.0574 | 0.6711 | 0.2797 | 0.1846 | 0.668 |
| $a+by^2z^2+c/y^2z^2$ | 133.08 | 94.77 | 0.785 | 0.0836 | 0.0613 | 0.6553 | 0.2865 | 0.2017 | 0.652 |
| $a+by^2z^2+c/y^2\sqrt{z}$ | 141.71 | 107.30 | 0.756 | 0.0815 | 0.0556 | 0.6723 | 0.2814 | 0.1843 | 0.664 |
| $a+by^2z^2+cz/y^2$ | 162.50 | 124.96 | 0.679 | 0.0874 | 0.0637 | 0.6230 | 0.3148 | 0.2269 | 0.580 |
| $a+by^2z^2+cz^2/y^2$ | 169.57 | 129.17 | 0.650 | 0.0931 | 0.0719 | 0.5719 | 0.3410 | 0.2578 | 0.507 |
| $a+by^2z^2+c\sqrt{z}/y^2$ | 155.72 | 120.81 | 0.705 | 0.0844 | 0.0602 | 0.6482 | 0.3000 | 0.2124 | 0.619 |
| $a+by^2z^2+c/\sqrt{y}z$ | 120.36 | 87.15 | 0.824 | 0.0792 | 0.0541 | 0.6905 | 0.2695 | 0.1705 | 0.692 |
| $a+by^2z^2+c/\sqrt{y}z^2$ | 132.70 | 98.12 | 0.786 | 0.0853 | 0.0621 | 0.6406 | 0.2991 | 0.2110 | 0.621 |
| $a+by^2z^2+c/\sqrt{y}\sqrt{z}$ | 121.11 | 88.77 | 0.822 | 0.0767 | 0.0509 | 0.7092 | 0.2583 | 0.1566 | 0.717 |
| $a+by^2z^2+cz/\sqrt{y}$ | 159.12 | 121.42 | 0.692 | 0.0888 | 0.0659 | 0.6103 | 0.3298 | 0.2492 | 0.539 |
| $a+by^2z^2+cz^2/\sqrt{y}$ | 159.47 | 123.18 | 0.691 | 0.0857 | 0.0634 | 0.6375 | 0.3207 | 0.2475 | 0.564 |
| $a+by^2z^2+c\sqrt{z}/\sqrt{y}$ | 169.60 | 129.42 | 0.650 | 0.0937 | 0.0728 | 0.5663 | 0.3442 | 0.2643 | 0.498 |
| $a+by^2\sqrt{z}+c\sqrt{y}/z$ | 138.95 | 103.62 | 0.765 | 0.0848 | 0.0597 | 0.6452 | 0.3007 | 0.2147 | 0.617 |
| $a+by^2\sqrt{z}+c\sqrt{y}/z^2$ | 140.60 | 104.84 | 0.759 | 0.0857 | 0.0605 | 0.6375 | 0.3022 | 0.2128 | 0.613 |
| $a+by^2\sqrt{z}+c\sqrt{y}/\sqrt{z}$ | 141.40 | 105.04 | 0.757 | 0.0850 | 0.0606 | 0.6431 | 0.3034 | 0.2186 | 0.610 |

(continued on next page)

**Table 4 – continued from previous page**

| Functional form | $T_{eff}$ (K) | | | Radius ($R_{\odot}$) | | | log ($L/L_{\odot}$) | | |
|---|---|---|---|---|---|---|---|---|---|
| | RMSE | MAD | $R^2_{ap}$ | RMSE | MAD | $R^2_{ap}$ | RMSE | MAD | $R^2_{ap}$ |
| $a+by^2\sqrt{z}+c\sqrt{y}z$ | 133.10 | 105.31 | 0.784 | 0.0763 | 0.0531 | 0.7124 | 0.2817 | 0.2124 | 0.664 |
| $a+by^2\sqrt{z}+c\sqrt{y}z^2$ | 141.75 | 107.06 | 0.756 | 0.0825 | 0.0608 | 0.6636 | 0.3009 | 0.2269 | 0.616 |
| $a+by^2\sqrt{z}+c\sqrt{y}\sqrt{z}$ | 125.99 | 99.52 | 0.807 | 0.0739 | 0.0435 | 0.7303 | 0.2566 | 0.1623 | 0.721 |
| $a+by^2\sqrt{z}+c/yz$ | 131.83 | 97.01 | 0.789 | 0.0824 | 0.0546 | 0.6647 | 0.2737 | 0.1644 | 0.682 |
| $a+by^2\sqrt{z}+c/yz^2$ | 130.94 | 96.49 | 0.791 | 0.0839 | 0.0563 | 0.6523 | 0.2833 | 0.1756 | 0.660 |
| $a+by^2\sqrt{z}+c/y\sqrt{z}$ | 135.90 | 100.05 | 0.775 | 0.0824 | 0.0533 | 0.6650 | 0.2747 | 0.1637 | 0.680 |
| $a+by^2\sqrt{z}+cz/y$ | 139.94 | 105.59 | 0.762 | 0.0850 | 0.0609 | 0.6430 | 0.3035 | 0.2196 | 0.610 |
| $a+by^2\sqrt{z}+cz^2/y$ | 135.65 | 103.59 | 0.776 | 0.0806 | 0.0578 | 0.6790 | 0.2945 | 0.2257 | 0.633 |
| $a+by^2\sqrt{z}+c\sqrt{z}/y$ | 144.43 | 104.56 | 0.746 | 0.0858 | 0.0596 | 0.6361 | 0.3003 | 0.1984 | 0.618 |
| $a+by^2\sqrt{z}+c/y^2z$ | 136.69 | 99.40 | 0.773 | 0.0831 | 0.0545 | 0.6587 | 0.2793 | 0.1660 | 0.669 |
| $a+by^2\sqrt{z}+c/y^2z^2$ | 133.37 | 95.77 | 0.784 | 0.0837 | 0.0562 | 0.6537 | 0.2817 | 0.1747 | 0.664 |
| $a+by^2\sqrt{z}+c/y^2\sqrt{z}$ | 139.31 | 102.31 | 0.764 | 0.0831 | 0.0536 | 0.6587 | 0.2808 | 0.1677 | 0.666 |
| $a+by^2\sqrt{z}+cz/y^2$ | 144.50 | 104.45 | 0.746 | 0.0853 | 0.0579 | 0.6404 | 0.2978 | 0.1932 | 0.624 |
| $a+by^2\sqrt{z}+cz^2/y^2$ | 139.92 | 105.55 | 0.762 | 0.0855 | 0.0612 | 0.6390 | 0.3039 | 0.2179 | 0.609 |
| $a+by^2\sqrt{z}+c\sqrt{z}/y^2$ | 144.00 | 104.87 | 0.748 | 0.0843 | 0.0552 | 0.6487 | 0.2911 | 0.1848 | 0.641 |
| $a+by^2\sqrt{z}+c/\sqrt{y}z$ | 128.27 | 95.78 | 0.800 | 0.0821 | 0.0543 | 0.6674 | 0.2742 | 0.1634 | 0.681 |
| $a+by^2\sqrt{z}+c/\sqrt{y}z^2$ | 132.78 | 99.14 | 0.786 | 0.0845 | 0.0576 | 0.6472 | 0.2899 | 0.1878 | 0.644 |
| $a+by^2\sqrt{z}+c/\sqrt{y}\sqrt{z}$ | 130.34 | 97.29 | 0.793 | 0.0810 | 0.0526 | 0.6758 | 0.2678 | 0.1571 | 0.696 |
| $a+by^2\sqrt{z}+cz/\sqrt{y}$ | 133.92 | 103.33 | 0.782 | 0.0809 | 0.0562 | 0.6771 | 0.2935 | 0.2215 | 0.635 |
| $a+by^2\sqrt{z}+cz^2/\sqrt{y}$ | 137.14 | 104.59 | 0.771 | 0.0799 | 0.0584 | 0.6845 | 0.2939 | 0.2265 | 0.634 |
| $a+by^2\sqrt{z}+c\sqrt{z}/\sqrt{y}$ | 140.22 | 105.37 | 0.761 | 0.0849 | 0.0607 | 0.6443 | 0.3033 | 0.2198 | 0.610 |
| $a+b\sqrt{y}/z + c\sqrt{y}/z^2$ | 224.09 | 157.56 | 0.389 | 0.1160 | 0.0859 | 0.3352 | 0.4115 | 0.2946 | 0.282 |
| $a+b\sqrt{y}/z + c\sqrt{y}/\sqrt{z}$ | 202.03 | 141.54 | 0.503 | 0.1126 | 0.0851 | 0.3742 | 0.3712 | 0.2629 | 0.416 |
| $a+b\sqrt{y}/z + c\sqrt{y}z$ | 134.39 | 107.07 | 0.780 | 0.0759 | 0.0535 | 0.7156 | 0.2802 | 0.2126 | 0.667 |
| $a+b\sqrt{y}/z + c\sqrt{y}z^2$ | 154.99 | 120.09 | 0.708 | 0.0852 | 0.0647 | 0.6415 | 0.3185 | 0.2450 | 0.570 |
| $a+b\sqrt{y}/z + c\sqrt{y}\sqrt{z}$ | 126.03 | 99.44 | 0.807 | 0.0745 | 0.0443 | 0.7257 | 0.2607 | 0.1710 | 0.712 |
| $a+b\sqrt{y}/z+c/yz$ | 176.74 | 119.92 | 0.620 | 0.1013 | 0.0754 | 0.4937 | 0.3234 | 0.2200 | 0.557 |
| $a+b\sqrt{y}/z + c/yz^2$ | 199.41 | 138.62 | 0.516 | 0.1127 | 0.0825 | 0.3731 | 0.3689 | 0.2584 | 0.423 |
| $a+b\sqrt{y}/z + c/y\sqrt{z}$ | 168.57 | 114.94 | 0.654 | 0.0957 | 0.0697 | 0.5481 | 0.3049 | 0.1958 | 0.606 |
| $a+b\sqrt{y}/z+cz/y$ | 225.41 | 158.39 | 0.382 | 0.1194 | 0.0895 | 0.2957 | 0.4070 | 0.2927 | 0.298 |
| $a+b\sqrt{y}/z + cz^2/y$ | 180.35 | 137.56 | 0.604 | 0.0948 | 0.0700 | 0.5564 | 0.3488 | 0.2572 | 0.485 |
| $a+b\sqrt{y}/z + c\sqrt{z}/y$ | 184.61 | 130.79 | 0.585 | 0.0994 | 0.0697 | 0.5123 | 0.3270 | 0.2120 | 0.547 |
| $a+b\sqrt{y}/z + c/y^2z$ | 180.45 | 122.55 | 0.604 | 0.1017 | 0.0748 | 0.4896 | 0.3272 | 0.2264 | 0.546 |
| $a+b\sqrt{y}/z + c/y^2z^2$ | 190.58 | 134.03 | 0.558 | 0.1086 | 0.0801 | 0.4177 | 0.3532 | 0.2528 | 0.471 |
| $a+b\sqrt{y}/z + c/y^2\sqrt{z}$ | 177.81 | 120.95 | 0.615 | 0.0984 | 0.0710 | 0.5215 | 0.3171 | 0.2105 | 0.574 |
| $a+b\sqrt{y}/z + cz/y^2$ | 191.91 | 134.91 | 0.552 | 0.0997 | 0.0699 | 0.5089 | 0.3329 | 0.2232 | 0.530 |
| $a+b\sqrt{y}/z + cz^2/y^2$ | 226.15 | 159.61 | 0.378 | 0.1188 | 0.0888 | 0.3030 | 0.4062 | 0.2934 | 0.301 |
| $a+b\sqrt{y}/z + c\sqrt{z}/y^2$ | 182.72 | 128.34 | 0.594 | 0.0965 | 0.0662 | 0.5405 | 0.3174 | 0.2078 | 0.573 |
| $a+b\sqrt{y}/z + c/\sqrt{y}z$ | 174.64 | 117.62 | 0.629 | 0.1012 | 0.0758 | 0.4947 | 0.3220 | 0.2192 | 0.561 |
| $a+b\sqrt{y}/z + c/\sqrt{y}z^2$ | 210.25 | 149.12 | 0.462 | 0.1168 | 0.0865 | 0.3262 | 0.3875 | 0.2754 | 0.364 |
| $a+b\sqrt{y}/z + c/\sqrt{y}\sqrt{z}$ | 159.69 | 108.00 | 0.690 | 0.0927 | 0.0675 | 0.5760 | 0.2934 | 0.1852 | 0.635 |
| $a+b\sqrt{y}/z + cz/\sqrt{y}$ | 179.51 | 138.13 | 0.608 | 0.0944 | 0.0682 | 0.5602 | 0.3462 | 0.2529 | 0.492 |
| $a+b\sqrt{y}/z + cz^2/\sqrt{y}$ | 162.03 | 123.47 | 0.681 | 0.0857 | 0.0636 | 0.6370 | 0.3209 | 0.2478 | 0.564 |
| $a+b\sqrt{y}/z + c\sqrt{z}/\sqrt{y}$ | 223.13 | 156.59 | 0.394 | 0.1190 | 0.0892 | 0.3010 | 0.4037 | 0.2884 | 0.310 |
| $a+b\sqrt{y}/z^2+c\sqrt{y}/\sqrt{z}$ | 248.14 | 179.76 | 0.251 | 0.1308 | 0.1004 | 0.1557 | 0.4444 | 0.3339 | 0.163 |
| $a+b\sqrt{y}/z^2+c\sqrt{y}z$ | 134.15 | 106.53 | 0.781 | 0.0761 | 0.0538 | 0.7144 | 0.2815 | 0.2132 | 0.664 |
| $a+b\sqrt{y}/z^2+c\sqrt{y}z^2$ | 151.91 | 118.13 | 0.719 | 0.0849 | 0.0645 | 0.6441 | 0.3159 | 0.2417 | 0.577 |
| $a+b\sqrt{y}/z^2+c\sqrt{y}\sqrt{z}$ | 125.95 | 99.40 | 0.807 | 0.0737 | 0.0438 | 0.7315 | 0.2601 | 0.1745 | 0.713 |
| $a+b\sqrt{y}/z^2+c/yz$ | 195.19 | 141.77 | 0.536 | 0.1087 | 0.0848 | 0.4165 | 0.3429 | 0.2491 | 0.502 |
| $a+b\sqrt{y}/z^2+c/yz^2$ | 215.55 | 157.08 | 0.435 | 0.1198 | 0.0953 | 0.2916 | 0.3853 | 0.2917 | 0.371 |
| $a+b\sqrt{y}/z^2+c/y\sqrt{z}$ | 190.85 | 138.85 | 0.557 | 0.1049 | 0.0797 | 0.4566 | 0.3312 | 0.2336 | 0.535 |
| $a+b\sqrt{y}/z^2+cz/y$ | 246.90 | 176.43 | 0.258 | 0.1304 | 0.0990 | 0.1603 | 0.4449 | 0.3333 | 0.161 |
| $a+b\sqrt{y}/z^2+cz^2/y$ | 177.67 | 137.10 | 0.616 | 0.0948 | 0.0701 | 0.5566 | 0.3470 | 0.2533 | 0.490 |
| $a+b\sqrt{y}/z^2+c\sqrt{z}/y$ | 224.41 | 166.30 | 0.387 | 0.1186 | 0.0919 | 0.3057 | 0.3885 | 0.2856 | 0.361 |
| $a+b\sqrt{y}/z^2+c/y^2z$ | 208.80 | 149.35 | 0.470 | 0.1140 | 0.0898 | 0.3584 | 0.3647 | 0.2686 | 0.436 |
| $a+b\sqrt{y}/z^2+c/y^2z^2$ | 216.31 | 157.00 | 0.431 | 0.1196 | 0.0950 | 0.2936 | 0.3859 | 0.2902 | 0.369 |
| $a+b\sqrt{y}/z^2+c/y^2\sqrt{z}$ | 207.55 | 148.82 | 0.476 | 0.1117 | 0.0865 | 0.3836 | 0.3579 | 0.2558 | 0.457 |
| $a+b\sqrt{y}/z^2+cz/y^2$ | 226.19 | 167.90 | 0.378 | 0.1172 | 0.0899 | 0.3216 | 0.3866 | 0.2854 | 0.367 |
| $a+b\sqrt{y}/z^2+cz^2/y^2$ | 247.60 | 177.75 | 0.254 | 0.1309 | 0.1015 | 0.1539 | 0.4446 | 0.3340 | 0.163 |
| $a+b\sqrt{y}/z^2+c\sqrt{z}/y^2$ | 215.40 | 160.10 | 0.436 | 0.1124 | 0.0848 | 0.3764 | 0.3662 | 0.2657 | 0.432 |
| $a+b\sqrt{y}/z^2+c/\sqrt{y}z$ | 176.49 | 126.55 | 0.621 | 0.1009 | 0.0769 | 0.4975 | 0.3135 | 0.2154 | 0.584 |
| $a+b\sqrt{y}/z^2+c/\sqrt{y}z^2$ | 215.36 | 156.93 | 0.436 | 0.1200 | 0.0955 | 0.2889 | 0.3855 | 0.2927 | 0.370 |
| $a+b\sqrt{y}/z^2+c/\sqrt{y}\sqrt{z}$ | 168.62 | 119.81 | 0.654 | 0.0953 | 0.0704 | 0.5515 | 0.2971 | 0.1957 | 0.626 |
| $a+b\sqrt{y}/z^2+cz/\sqrt{y}$ | 181.13 | 140.04 | 0.601 | 0.0962 | 0.0699 | 0.5429 | 0.3509 | 0.2548 | 0.478 |
| $a+b\sqrt{y}/z^2+cz^2/\sqrt{y}$ | 159.42 | 122.06 | 0.691 | 0.0858 | 0.0638 | 0.6368 | 0.3196 | 0.2445 | 0.567 |
| $a+b\sqrt{y}/z^2+c\sqrt{z}/\sqrt{y}$ | 247.09 | 176.75 | 0.257 | 0.1302 | 0.0985 | 0.1625 | 0.4448 | 0.3333 | 0.162 |
| $a+b\sqrt{y}/\sqrt{z}+c\sqrt{y}z$ | 132.64 | 106.17 | 0.786 | 0.0752 | 0.0512 | 0.7206 | 0.2737 | 0.2002 | 0.683 |
| $a+b\sqrt{y}/\sqrt{z}+c\sqrt{y}z^2$ | 157.69 | 123.36 | 0.697 | 0.0849 | 0.0640 | 0.6441 | 0.3163 | 0.2454 | 0.576 |
| $a+b\sqrt{y}/\sqrt{z}+c\sqrt{y}\sqrt{z}$ | 126.02 | 99.49 | 0.807 | 0.0749 | 0.0444 | 0.7232 | 0.2606 | 0.1658 | 0.712 |
| $a+b\sqrt{y}/\sqrt{z}+c/yz$ | 173.15 | 120.56 | 0.635 | 0.0992 | 0.0723 | 0.5145 | 0.3180 | 0.2189 | 0.572 |
| $a+b\sqrt{y}/\sqrt{z}+c/yz^2$ | 202.41 | 143.54 | 0.502 | 0.1141 | 0.0843 | 0.3573 | 0.3727 | 0.2690 | 0.412 |
| $a+b\sqrt{y}/\sqrt{z}+c/y\sqrt{z}$ | 161.90 | 112.60 | 0.681 | 0.0915 | 0.0650 | 0.5869 | 0.2938 | 0.1905 | 0.634 |
| $a+b\sqrt{y}/\sqrt{z}+cz/y$ | 269.05 | 191.62 | 0.119 | 0.1355 | 0.1045 | 0.0931 | 0.4717 | 0.3603 | 0.057 |
| $a+b\sqrt{y}/\sqrt{z}+cz^2/y$ | 168.13 | 136.47 | 0.656 | 0.0874 | 0.0655 | 0.6226 | 0.3206 | 0.2559 | 0.564 |
| $a+b\sqrt{y}/\sqrt{z}+c\sqrt{z}/y$ | 180.99 | 129.38 | 0.601 | 0.0919 | 0.0625 | 0.5829 | 0.3111 | 0.2087 | 0.590 |
| $a+b\sqrt{y}/\sqrt{z}+c/y^2z$ | 180.01 | 129.21 | 0.606 | 0.0998 | 0.0742 | 0.5079 | 0.3237 | 0.2361 | 0.556 |
| $a+b\sqrt{y}/\sqrt{z}+c/y^2z^2$ | 195.96 | 143.24 | 0.533 | 0.1103 | 0.0823 | 0.3990 | 0.3602 | 0.2689 | 0.450 |
| $a+b\sqrt{y}/\sqrt{z}+c/y^2\sqrt{z}$ | 175.62 | 125.98 | 0.625 | 0.0948 | 0.0691 | 0.5559 | 0.3090 | 0.2162 | 0.595 |
| $a+b\sqrt{y}/\sqrt{z}+cz/y^2$ | 200.05 | 146.20 | 0.513 | 0.0967 | 0.0692 | 0.5383 | 0.3337 | 0.2391 | 0.528 |
| $a+b\sqrt{y}/\sqrt{z}+cz^2/y^2$ | 266.91 | 189.83 | 0.133 | 0.1332 | 0.1031 | 0.1241 | 0.4641 | 0.3550 | 0.088 |
| $a+b\sqrt{y}/\sqrt{z}+c\sqrt{z}/y^2$ | 184.10 | 137.49 | 0.588 | 0.0916 | 0.0637 | 0.5856 | 0.3096 | 0.2147 | 0.594 |
| $a+b\sqrt{y}/\sqrt{z}+c/\sqrt{y}z$ | 172.40 | 116.63 | 0.638 | 0.1001 | 0.0736 | 0.5053 | 0.3206 | 0.2133 | 0.565 |
| $a+b\sqrt{y}/\sqrt{z}+c/\sqrt{y}z^2$ | 213.13 | 152.14 | 0.447 | 0.1185 | 0.0882 | 0.3063 | 0.3903 | 0.2803 | 0.354 |
| $a+b\sqrt{y}/\sqrt{z}+c/\sqrt{y}\sqrt{z}$ | 154.28 | 102.84 | 0.710 | 0.0900 | 0.0636 | 0.6002 | 0.2877 | 0.1796 | 0.649 |
| $a+b\sqrt{y}/\sqrt{z}+cz/\sqrt{y}$ | 144.08 | 114.98 | 0.747 | 0.0790 | 0.0556 | 0.6919 | 0.2838 | 0.2190 | 0.659 |
| $a+b\sqrt{y}/\sqrt{z}+cz^2/\sqrt{y}$ | 156.94 | 124.98 | 0.700 | 0.0820 | 0.0614 | 0.6681 | 0.3049 | 0.2418 | 0.606 |
| $a+b\sqrt{y}/\sqrt{z}+c\sqrt{z}/\sqrt{y}$ | 269.48 | 191.86 | 0.116 | 0.1361 | 0.1047 | 0.0852 | 0.4740 | 0.3604 | 0.048 |
| $a+b\sqrt{y}z+c\sqrt{y}z^2$ | 129.25 | 103.27 | 0.797 | 0.0749 | 0.0460 | 0.7227 | 0.2661 | 0.1690 | 0.700 |
| $a+b\sqrt{y}z+c\sqrt{y}\sqrt{z}$ | 126.02 | 99.66 | 0.807 | 0.0746 | 0.0463 | 0.7249 | 0.2611 | 0.1596 | 0.711 |
| $a+b\sqrt{y}z+c/yz$ | 122.00 | 94.27 | 0.819 | 0.0738 | 0.0461 | 0.7310 | 0.2545 | 0.1569 | 0.726 |
| $a+b\sqrt{y}z+c/yz^2$ | 122.87 | 94.23 | 0.816 | 0.0754 | 0.0487 | 0.7194 | 0.2654 | 0.1729 | 0.702 |

(continued on next page)

**Table 4 – continued from previous page**

| Functional form | $T_{eff}$ (K) | | | Radius ($R_\odot$) | | | log (L/$L_\odot$) | | |
|---|---|---|---|---|---|---|---|---|---|
| | RMSE | MAD | $R^2_{ap}$ | RMSE | MAD | $R^2_{ap}$ | RMSE | MAD | $R^2_{ap}$ |
| $a+b\sqrt{y}z+c/y\sqrt{z}$ | 124.14 | 97.08 | 0.813 | 0.0731 | 0.0446 | 0.7361 | 0.2521 | 0.1515 | 0.731 |
| $a+b\sqrt{y}z+cz/y$ | 133.38 | 107.21 | 0.784 | 0.0752 | 0.0505 | 0.7211 | 0.2730 | 0.1945 | 0.684 |
| $a+b\sqrt{y}z+cz^2/y$ | 132.88 | 106.11 | 0.785 | 0.0761 | 0.0523 | 0.7142 | 0.2770 | 0.2019 | 0.675 |
| $a+b\sqrt{y}z+c\sqrt{z}/y$ | 131.63 | 105.66 | 0.789 | 0.0740 | 0.0471 | 0.7295 | 0.2650 | 0.1805 | 0.703 |
| $a+b\sqrt{y}z+c/y^2z$ | 124.19 | 96.46 | 0.812 | 0.0733 | 0.0461 | 0.7349 | 0.2541 | 0.1580 | 0.726 |
| $a+b\sqrt{y}z+c/y^2z^2$ | 121.87 | 92.97 | 0.819 | 0.0743 | 0.0480 | 0.7274 | 0.2587 | 0.1684 | 0.716 |
| $a+b\sqrt{y}z+c/y^2\sqrt{z}$ | 126.43 | 99.26 | 0.806 | 0.0729 | 0.0450 | 0.7374 | 0.2540 | 0.1564 | 0.727 |
| $a+b\sqrt{y}z+cz/y^2$ | 132.85 | 106.81 | 0.785 | 0.0737 | 0.0466 | 0.7316 | 0.2654 | 0.1822 | 0.702 |
| $a+b\sqrt{y}z+cz^2/y^2$ | 133.97 | 107.47 | 0.782 | 0.0751 | 0.0501 | 0.7217 | 0.2735 | 0.1936 | 0.683 |
| $a+b\sqrt{y}z+c\sqrt{z}/y^2$ | 131.25 | 105.16 | 0.790 | 0.0732 | 0.0450 | 0.7357 | 0.2604 | 0.1728 | 0.713 |
| $a+b\sqrt{y}z+c/\sqrt{y}z$ | 122.99 | 94.91 | 0.816 | 0.0749 | 0.0471 | 0.7227 | 0.2618 | 0.1642 | 0.710 |
| $a+b\sqrt{y}z+c/\sqrt{y}z^2$ | 127.07 | 98.47 | 0.804 | 0.0762 | 0.0517 | 0.7132 | 0.2742 | 0.1899 | 0.681 |
| $a+b\sqrt{y}z+c/\sqrt{y}\sqrt{z}$ | 122.66 | 95.53 | 0.817 | 0.0737 | 0.0449 | 0.7317 | 0.2537 | 0.1502 | 0.727 |
| $a+b\sqrt{y}z+cz/\sqrt{y}$ | 133.92 | 107.34 | 0.782 | 0.0761 | 0.0529 | 0.7140 | 0.2788 | 0.2080 | 0.671 |
| $a+b\sqrt{y}z+cz^2/\sqrt{y}$ | 131.07 | 103.44 | 0.791 | 0.0760 | 0.0516 | 0.7144 | 0.2752 | 0.1956 | 0.679 |
| $a+b\sqrt{y}z+c\sqrt{z}/\sqrt{y}$ | 133.04 | 106.91 | 0.785 | 0.0752 | 0.0507 | 0.7209 | 0.2730 | 0.1958 | 0.684 |
| $a+b\sqrt{y}z^2+c\sqrt{y}\sqrt{z}$ | 125.95 | 99.87 | 0.807 | 0.0747 | 0.0464 | 0.7247 | 0.2613 | 0.1603 | 0.711 |
| $a+b\sqrt{y}z^2+c/yz$ | 123.25 | 91.45 | 0.815 | 0.0751 | 0.0509 | 0.7214 | 0.2580 | 0.1675 | 0.718 |
| $a+b\sqrt{y}z^2+c/yz^2$ | 125.51 | 91.45 | 0.808 | 0.0786 | 0.0552 | 0.6951 | 0.2750 | 0.1855 | 0.680 |
| $a+b\sqrt{y}z^2+c/y\sqrt{z}$ | 127.76 | 95.84 | 0.801 | 0.0743 | 0.0489 | 0.7272 | 0.2564 | 0.1624 | 0.721 |
| $a+b\sqrt{y}z^2+cz/y$ | 156.51 | 121.66 | 0.702 | 0.0836 | 0.0628 | 0.6547 | 0.3106 | 0.2337 | 0.591 |
| $a+b\sqrt{y}z^2+cz^2/y$ | 158.24 | 122.41 | 0.695 | 0.0855 | 0.0651 | 0.6391 | 0.3200 | 0.2483 | 0.566 |
| $a+b\sqrt{y}z^2+c\sqrt{z}/y$ | 149.08 | 118.92 | 0.730 | 0.0795 | 0.0555 | 0.6878 | 0.2893 | 0.2066 | 0.645 |
| $a+b\sqrt{y}z^2+c/y^2z$ | 131.63 | 98.59 | 0.789 | 0.0760 | 0.0524 | 0.7148 | 0.2649 | 0.1717 | 0.703 |
| $a+b\sqrt{y}z^2+c/y^2z^2$ | 128.42 | 93.09 | 0.799 | 0.0778 | 0.0557 | 0.7009 | 0.2714 | 0.1863 | 0.688 |
| $a+b\sqrt{y}z^2+c/y^2\sqrt{z}$ | 135.60 | 104.40 | 0.776 | 0.0757 | 0.0507 | 0.7174 | 0.2656 | 0.1699 | 0.701 |
| $a+b\sqrt{y}z^2+cz/y^2$ | 151.10 | 119.38 | 0.722 | 0.0790 | 0.0558 | 0.6916 | 0.2895 | 0.2052 | 0.645 |
| $a+b\sqrt{y}z^2+cz^2/y^2$ | 156.48 | 120.71 | 0.702 | 0.0828 | 0.0619 | 0.6611 | 0.3082 | 0.2290 | 0.598 |
| $a+b\sqrt{y}z^2+c\sqrt{z}/y^2$ | 146.31 | 115.76 | 0.740 | 0.0772 | 0.0530 | 0.7054 | 0.2790 | 0.1915 | 0.670 |
| $a+b\sqrt{y}z^2+c/\sqrt{y}z$ | 122.19 | 91.20 | 0.818 | 0.0763 | 0.0510 | 0.7127 | 0.2645 | 0.1688 | 0.704 |
| $a+b\sqrt{y}z^2+c/\sqrt{y}z^2$ | 131.89 | 100.01 | 0.788 | 0.0807 | 0.0577 | 0.6783 | 0.2885 | 0.2016 | 0.647 |
| $a+b\sqrt{y}z^2+c/\sqrt{y}\sqrt{z}$ | 121.82 | 92.45 | 0.819 | 0.0740 | 0.0479 | 0.7297 | 0.2535 | 0.1566 | 0.728 |
| $a+b\sqrt{y}z^2+cz/\sqrt{y}$ | 156.98 | 121.38 | 0.700 | 0.0852 | 0.0641 | 0.6413 | 0.3192 | 0.2456 | 0.568 |
| $a+b\sqrt{y}z^2+cz^2/\sqrt{y}$ | 158.03 | 122.49 | 0.696 | 0.0849 | 0.0632 | 0.6441 | 0.3184 | 0.2456 | 0.570 |
| $a+b\sqrt{y}z^2+c\sqrt{z}/\sqrt{y}$ | 156.79 | 122.07 | 0.701 | 0.0841 | 0.0632 | 0.6509 | 0.3124 | 0.2384 | 0.587 |
| $a+b\sqrt{y}\sqrt{z}+c/yz$ | 124.83 | 95.74 | 0.810 | 0.0749 | 0.0443 | 0.7230 | 0.2563 | 0.1476 | 0.722 |
| $a+b\sqrt{y}\sqrt{z}+c/yz^2$ | 124.50 | 95.22 | 0.811 | 0.0748 | 0.0457 | 0.7240 | 0.2604 | 0.1609 | 0.713 |
| $a+b\sqrt{y}\sqrt{z}+c/y\sqrt{z}$ | 125.55 | 97.56 | 0.808 | 0.0748 | 0.0442 | 0.7237 | 0.2552 | 0.1453 | 0.724 |
| $a+b\sqrt{y}\sqrt{z}+cz/y$ | 125.18 | 99.48 | 0.809 | 0.0749 | 0.0448 | 0.7231 | 0.2619 | 0.1676 | 0.709 |
| $a+b\sqrt{y}\sqrt{z}+cz^2/y$ | 125.37 | 100.18 | 0.809 | 0.0743 | 0.0458 | 0.7272 | 0.2627 | 0.1725 | 0.708 |
| $a+b\sqrt{y}\sqrt{z}+c\sqrt{z}/y$ | 125.71 | 99.72 | 0.808 | 0.0749 | 0.0442 | 0.7233 | 0.2598 | 0.1601 | 0.714 |
| $a+b\sqrt{y}\sqrt{z}+c/y^2z$ | 125.20 | 96.83 | 0.809 | 0.0748 | 0.0443 | 0.7240 | 0.2551 | 0.1472 | 0.724 |
| $a+b\sqrt{y}\sqrt{z}+c/y^2z^2$ | 124.03 | 94.31 | 0.813 | 0.0749 | 0.0444 | 0.7231 | 0.2568 | 0.1529 | 0.721 |
| $a+b\sqrt{y}\sqrt{z}+c/y^2\sqrt{z}$ | 125.78 | 98.36 | 0.808 | 0.0747 | 0.0440 | 0.7246 | 0.2551 | 0.1485 | 0.724 |
| $a+b\sqrt{y}\sqrt{z}+cz/y^2$ | 125.24 | 99.22 | 0.809 | 0.0748 | 0.0437 | 0.7240 | 0.2596 | 0.1612 | 0.715 |
| $a+b\sqrt{y}\sqrt{z}+cz^2/y^2$ | 124.28 | 98.56 | 0.812 | 0.0749 | 0.0448 | 0.7230 | 0.2621 | 0.1683 | 0.709 |
| $a+b\sqrt{y}\sqrt{z}+c\sqrt{z}/y^2$ | 125.81 | 99.66 | 0.807 | 0.0747 | 0.0436 | 0.7248 | 0.2577 | 0.1574 | 0.719 |
| $a+b\sqrt{y}\sqrt{z}+c/\sqrt{y}z$ | 124.85 | 95.85 | 0.810 | 0.0748 | 0.0455 | 0.7235 | 0.2596 | 0.1571 | 0.714 |
| $a+b\sqrt{y}\sqrt{z}+c/\sqrt{y}z^2$ | 125.39 | 97.47 | 0.809 | 0.0743 | 0.0460 | 0.7273 | 0.2625 | 0.1710 | 0.708 |
| $a+b\sqrt{y}\sqrt{z}+c/\sqrt{y}\sqrt{z}$ | 125.24 | 96.62 | 0.809 | 0.0749 | 0.0444 | 0.7230 | 0.2563 | 0.1469 | 0.722 |
| $a+b\sqrt{y}\sqrt{z}+cz/\sqrt{y}$ | 125.39 | 99.88 | 0.809 | 0.0747 | 0.0450 | 0.7248 | 0.2626 | 0.1717 | 0.708 |
| $a+b\sqrt{y}\sqrt{z}+cz^2/\sqrt{y}$ | 125.76 | 100.24 | 0.808 | 0.0742 | 0.0464 | 0.7280 | 0.2626 | 0.1703 | 0.708 |
| $a+b\sqrt{y}\sqrt{z}+c\sqrt{z}/\sqrt{y}$ | 125.60 | 99.72 | 0.808 | 0.0749 | 0.0448 | 0.7230 | 0.2616 | 0.1670 | 0.710 |
| $a+b/yz+c/yz^2$ | 201.38 | 145.63 | 0.507 | 0.1053 | 0.0815 | 0.4524 | 0.3315 | 0.2346 | 0.535 |
| $a+b/yz+c/y\sqrt{z}$ | 203.03 | 146.15 | 0.498 | 0.1090 | 0.0824 | 0.4134 | 0.3430 | 0.2442 | 0.502 |
| $a+b/yz+cz/y$ | 162.78 | 119.91 | 0.678 | 0.0971 | 0.0719 | 0.5343 | 0.3101 | 0.2173 | 0.593 |
| $a+b/yz+cz^2/y$ | 132.50 | 99.70 | 0.786 | 0.0791 | 0.0576 | 0.6913 | 0.2662 | 0.1815 | 0.700 |
| $a+b/yz+c\sqrt{z}/y$ | 187.30 | 135.89 | 0.573 | 0.1075 | 0.0832 | 0.4293 | 0.3379 | 0.2439 | 0.516 |
| $a+b/yz+c/y^2z$ | 173.03 | 115.15 | 0.636 | 0.1020 | 0.0776 | 0.4859 | 0.3225 | 0.2211 | 0.559 |
| $a+b/yz+c/y^2z^2$ | 171.87 | 119.76 | 0.641 | 0.0917 | 0.0658 | 0.5847 | 0.2954 | 0.1887 | 0.630 |
| $a+b/yz+c/y^2\sqrt{z}$ | 183.57 | 131.90 | 0.590 | 0.1073 | 0.0839 | 0.4311 | 0.3370 | 0.2447 | 0.519 |
| $a+b/yz+cz/y^2$ | 190.13 | 136.90 | 0.560 | 0.1092 | 0.0851 | 0.4111 | 0.3422 | 0.2500 | 0.504 |
| $a+b/yz+cz^2/y^2$ | 167.60 | 123.19 | 0.658 | 0.1007 | 0.0758 | 0.4998 | 0.3185 | 0.2220 | 0.570 |
| $a+b/yz+c\sqrt{z}/y^2$ | 192.23 | 139.43 | 0.550 | 0.1097 | 0.0856 | 0.4055 | 0.3438 | 0.2517 | 0.499 |
| $a+b/yz+c/\sqrt{y}z$ | 173.53 | 115.75 | 0.634 | 0.1012 | 0.0761 | 0.4941 | 0.3219 | 0.2187 | 0.561 |
| $a+b/yz+c/\sqrt{y}z^2$ | 201.12 | 146.70 | 0.508 | 0.1104 | 0.0849 | 0.3986 | 0.3463 | 0.2483 | 0.492 |
| $a+b/yz+c/\sqrt{y}\sqrt{z}$ | 141.40 | 101.99 | 0.757 | 0.0797 | 0.0498 | 0.6867 | 0.2656 | 0.1524 | 0.701 |
| $a+b/yz+cz/\sqrt{y}$ | 137.14 | 105.11 | 0.771 | 0.0824 | 0.0588 | 0.6648 | 0.2740 | 0.1839 | 0.682 |
| $a+b/yz+cz^2/\sqrt{y}$ | 126.73 | 92.54 | 0.805 | 0.0752 | 0.0525 | 0.7211 | 0.2578 | 0.1696 | 0.718 |
| $a+b/yz+c\sqrt{z}/\sqrt{y}$ | 163.60 | 119.31 | 0.674 | 0.0965 | 0.0711 | 0.5397 | 0.3094 | 0.2155 | 0.594 |
| $a+b/yz^2+c/y\sqrt{z}$ | 206.38 | 148.09 | 0.482 | 0.1086 | 0.0837 | 0.4180 | 0.3431 | 0.2439 | 0.501 |
| $a+b/yz^2+cz/y$ | 196.51 | 140.86 | 0.530 | 0.1134 | 0.0836 | 0.3654 | 0.3693 | 0.2669 | 0.422 |
| $a+b/yz^2+cz^2/y$ | 144.34 | 109.19 | 0.747 | 0.0861 | 0.0624 | 0.6337 | 0.2965 | 0.2030 | 0.628 |
| $a+b/yz^2+c\sqrt{z}/y$ | 218.23 | 161.03 | 0.421 | 0.1206 | 0.0969 | 0.2816 | 0.3849 | 0.2940 | 0.372 |
| $a+b/yz^2+c/y^2z$ | 218.75 | 160.53 | 0.418 | 0.1201 | 0.0958 | 0.2883 | 0.3822 | 0.2891 | 0.381 |
| $a+b/yz^2+c/y^2z^2$ | 215.24 | 156.90 | 0.436 | 0.1200 | 0.0957 | 0.2892 | 0.3853 | 0.2922 | 0.371 |
| $a+b/yz^2+c/y^2\sqrt{z}$ | 218.66 | 158.93 | 0.418 | 0.1190 | 0.0938 | 0.3010 | 0.3783 | 0.2825 | 0.394 |
| $a+b/yz^2+cz/y^2$ | 218.66 | 160.92 | 0.418 | 0.1199 | 0.0957 | 0.2900 | 0.3824 | 0.2896 | 0.380 |
| $a+b/yz^2+cz^2/y^2$ | 201.93 | 144.30 | 0.504 | 0.1165 | 0.0890 | 0.3295 | 0.3766 | 0.2778 | 0.399 |
| $a+b/yz^2+c\sqrt{z}/y^2$ | 218.65 | 158.81 | 0.418 | 0.1187 | 0.0934 | 0.3046 | 0.3779 | 0.2818 | 0.395 |
| $a+b/yz^2+c/\sqrt{y}z$ | 147.35 | 103.81 | 0.736 | 0.0811 | 0.0517 | 0.6751 | 0.2722 | 0.1586 | 0.686 |
| $a+b/yz^2+c/\sqrt{y}z^2$ | 215.42 | 156.95 | 0.435 | 0.1199 | 0.0955 | 0.2903 | 0.3853 | 0.2920 | 0.371 |
| $a+b/yz^2+c/\sqrt{y}\sqrt{z}$ | 157.04 | 104.11 | 0.700 | 0.0814 | 0.0522 | 0.6729 | 0.2653 | 0.1572 | 0.702 |
| $a+b/yz^2+cz/\sqrt{y}$ | 152.38 | 115.99 | 0.718 | 0.0903 | 0.0637 | 0.5971 | 0.3082 | 0.2061 | 0.597 |
| $a+b/yz^2+cz^2/\sqrt{y}$ | 132.40 | 96.26 | 0.787 | 0.0796 | 0.0563 | 0.6870 | 0.2789 | 0.1867 | 0.671 |
| $a+b/yz^2+c\sqrt{z}/\sqrt{y}$ | 196.25 | 140.37 | 0.531 | 0.1126 | 0.0822 | 0.3741 | 0.3678 | 0.2648 | 0.427 |
| $a+b/y\sqrt{z}+cz/y$ | 147.20 | 110.90 | 0.736 | 0.0880 | 0.0641 | 0.6172 | 0.2810 | 0.1921 | 0.665 |
| $a+b/y\sqrt{z}+cz^2/y$ | 130.58 | 98.21 | 0.793 | 0.0755 | 0.0536 | 0.7188 | 0.2547 | 0.1671 | 0.725 |
| $a+b/y\sqrt{z}+c\sqrt{z}/y$ | 168.18 | 120.61 | 0.656 | 0.0984 | 0.0739 | 0.5219 | 0.3081 | 0.2094 | 0.598 |
| $a+b/y\sqrt{z}+c/y^2z$ | 162.19 | 116.51 | 0.680 | 0.0876 | 0.0609 | 0.6212 | 0.2843 | 0.1835 | 0.657 |
| $a+b/y\sqrt{z}+c/y^2z^2$ | 196.78 | 136.14 | 0.529 | 0.0972 | 0.0708 | 0.5333 | 0.3153 | 0.2084 | 0.579 |

(continued on next page)

**Table 4 – continued from previous page**

| Functional form | $T_{eff}$ (K) | | | Radius ($R_\odot$) | | | log (L/$L_\odot$) | | |
|---|---|---|---|---|---|---|---|---|---|
| | RMSE | MAD | $R^2_{ap}$ | RMSE | MAD | $R^2_{ap}$ | RMSE | MAD | $R^2_{ap}$ |
| $a+b/y\sqrt{z}+c/y^2\sqrt{z}$ | 149.17 | 97.03 | 0.729 | 0.0919 | 0.0669 | 0.5827 | 0.2897 | 0.1850 | 0.644 |
| $a+b/y\sqrt{z}+cz/y^2$ | 172.42 | 121.26 | 0.638 | 0.1024 | 0.0783 | 0.4823 | 0.3184 | 0.2208 | 0.571 |
| $a+b/y\sqrt{z}+cz^2/y^2$ | 151.36 | 112.81 | 0.721 | 0.0920 | 0.0672 | 0.5821 | 0.2902 | 0.1969 | 0.643 |
| $a+b/y\sqrt{z}+c\sqrt{z}/y^2$ | 172.53 | 121.52 | 0.638 | 0.1029 | 0.0792 | 0.4771 | 0.3198 | 0.2238 | 0.567 |
| $a+b/y\sqrt{z}+c/\sqrt{y}z$ | 177.32 | 123.75 | 0.617 | 0.1019 | 0.0780 | 0.4870 | 0.3199 | 0.2220 | 0.566 |
| $a+b/y\sqrt{z}+c/\sqrt{y}z^2$ | 199.16 | 145.97 | 0.517 | 0.1084 | 0.0821 | 0.4203 | 0.3406 | 0.2441 | 0.508 |
| $a+b/y\sqrt{z}+c/\sqrt{y}\sqrt{z}$ | 148.16 | 95.97 | 0.733 | 0.0896 | 0.0636 | 0.6037 | 0.2859 | 0.1760 | 0.654 |
| $a+b/y\sqrt{z}+cz/\sqrt{y}$ | 131.76 | 101.27 | 0.789 | 0.0777 | 0.0543 | 0.7020 | 0.2582 | 0.1686 | 0.717 |
| $a+b/y\sqrt{z}+cz^2/\sqrt{y}$ | 128.34 | 94.59 | 0.800 | 0.0732 | 0.0499 | 0.7351 | 0.2520 | 0.1612 | 0.731 |
| $a+b/y\sqrt{z}+c\sqrt{z}/\sqrt{y}$ | 149.04 | 109.70 | 0.730 | 0.0876 | 0.0634 | 0.6207 | 0.2811 | 0.1898 | 0.665 |
| $a+bz/y+cz^2/y$ | 153.31 | 121.19 | 0.714 | 0.0775 | 0.0543 | 0.7035 | 0.2856 | 0.2103 | 0.654 |
| $a+bz/y+c\sqrt{z}/y$ | 133.29 | 103.10 | 0.784 | 0.0747 | 0.0518 | 0.7246 | 0.2509 | 0.1616 | 0.733 |
| $a+bz/y+c/y^2z$ | 172.02 | 130.14 | 0.640 | 0.0991 | 0.0761 | 0.5154 | 0.3194 | 0.2375 | 0.568 |
| $a+bz/y+c/y^2z^2$ | 195.22 | 141.40 | 0.536 | 0.1120 | 0.0841 | 0.3809 | 0.3644 | 0.2711 | 0.437 |
| $a+bz/y+c/y^2\sqrt{z}$ | 161.35 | 123.56 | 0.683 | 0.0916 | 0.0705 | 0.5858 | 0.2960 | 0.2191 | 0.629 |
| $a+bz/y+cz/y^2$ | 159.39 | 126.89 | 0.691 | 0.0781 | 0.0574 | 0.6987 | 0.2734 | 0.1966 | 0.683 |
| $a+bz/y+cz^2/y^2$ | 252.73 | 175.95 | 0.223 | 0.1220 | 0.0934 | 0.2653 | 0.4327 | 0.3208 | 0.207 |
| $a+bz/y+c\sqrt{z}/y^2$ | 153.58 | 119.19 | 0.713 | 0.0798 | 0.0602 | 0.6855 | 0.2693 | 0.1889 | 0.693 |
| $a+bz/y+c/\sqrt{y}z$ | 165.07 | 113.76 | 0.668 | 0.0984 | 0.0716 | 0.5218 | 0.3163 | 0.2087 | 0.576 |
| $a+bz/y+c/\sqrt{y}z^2$ | 208.11 | 146.22 | 0.473 | 0.1175 | 0.0857 | 0.3182 | 0.3876 | 0.2752 | 0.363 |
| $a+bz/y+c/\sqrt{y}\sqrt{z}$ | 143.28 | 102.95 | 0.750 | 0.0874 | 0.0621 | 0.6230 | 0.2796 | 0.1767 | 0.669 |
| $a+bz/y+cz/\sqrt{y}$ | 135.74 | 106.40 | 0.776 | 0.0719 | 0.0452 | 0.7446 | 0.2573 | 0.1737 | 0.720 |
| $a+bz/y+cz^2/\sqrt{y}$ | 152.15 | 121.10 | 0.718 | 0.0781 | 0.0551 | 0.6989 | 0.2902 | 0.2112 | 0.643 |
| $a+bz/y+c\sqrt{z}/\sqrt{y}$ | 263.07 | 186.42 | 0.158 | 0.1307 | 0.1010 | 0.1566 | 0.4575 | 0.3483 | 0.113 |
| $a+bz^2/y+c\sqrt{z}/y$ | 142.47 | 110.85 | 0.753 | 0.0740 | 0.0484 | 0.7297 | 0.2647 | 0.1829 | 0.703 |
| $a+bz^2/y+c/y^2z$ | 138.05 | 101.18 | 0.768 | 0.0786 | 0.0587 | 0.6948 | 0.2679 | 0.1864 | 0.696 |
| $a+bz^2/y+c/y^2z^2$ | 142.10 | 108.71 | 0.754 | 0.0836 | 0.0624 | 0.6549 | 0.2861 | 0.2023 | 0.653 |
| $a+bz^2/y+c/y^2\sqrt{z}$ | 138.54 | 101.53 | 0.766 | 0.0763 | 0.0562 | 0.7124 | 0.2619 | 0.1763 | 0.709 |
| $a+bz^2/y+cz/y^2$ | 149.73 | 114.61 | 0.727 | 0.0746 | 0.0519 | 0.7249 | 0.2707 | 0.1895 | 0.690 |
| $a+bz^2/y+cz^2/y^2$ | 155.20 | 117.19 | 0.707 | 0.0762 | 0.0545 | 0.7134 | 0.2837 | 0.2071 | 0.659 |
| $a+bz^2/y+c\sqrt{z}/y^2$ | 145.24 | 111.14 | 0.743 | 0.0743 | 0.0513 | 0.7278 | 0.2639 | 0.1769 | 0.705 |
| $a+bz^2/y+c/\sqrt{y}z$ | 136.22 | 103.68 | 0.774 | 0.0821 | 0.0578 | 0.6670 | 0.2793 | 0.1828 | 0.669 |
| $a+bz^2/y+c/\sqrt{y}z^2$ | 154.58 | 119.46 | 0.709 | 0.0897 | 0.0647 | 0.6031 | 0.3152 | 0.2173 | 0.579 |
| $a+bz^2/y+c/\sqrt{y}\sqrt{z}$ | 127.75 | 96.45 | 0.801 | 0.0766 | 0.0527 | 0.7104 | 0.2575 | 0.1643 | 0.719 |
| $a+bz^2/y+cz/\sqrt{y}$ | 179.83 | 138.07 | 0.607 | 0.0949 | 0.0701 | 0.5558 | 0.3482 | 0.2542 | 0.486 |
| $a+bz^2/y+cz^2/\sqrt{y}$ | 153.97 | 119.69 | 0.712 | 0.0806 | 0.0598 | 0.6795 | 0.3024 | 0.2291 | 0.613 |
| $a+bz^2/y+c\sqrt{z}/\sqrt{y}$ | 155.97 | 124.58 | 0.704 | 0.0800 | 0.0582 | 0.6837 | 0.2937 | 0.2266 | 0.634 |
| $a+b\sqrt{z}/y+c/y^2z$ | 220.99 | 158.33 | 0.406 | 0.1195 | 0.0918 | 0.2948 | 0.3814 | 0.2841 | 0.384 |
| $a+b\sqrt{z}/y+c/y^2z^2$ | 238.09 | 172.39 | 0.310 | 0.1278 | 0.1011 | 0.1939 | 0.4110 | 0.3070 | 0.284 |
| $a+b\sqrt{z}/y+c/y^2\sqrt{z}$ | 209.23 | 148.71 | 0.467 | 0.1125 | 0.0851 | 0.3746 | 0.3587 | 0.2668 | 0.455 |
| $a+b\sqrt{z}/y+cz/y^2$ | 282.81 | 210.04 | 0.027 | 0.1329 | 0.1030 | 0.1273 | 0.4537 | 0.3484 | 0.128 |
| $a+b\sqrt{z}/y+cz^2/y^2$ | 148.87 | 115.17 | 0.730 | 0.0877 | 0.0610 | 0.6200 | 0.2858 | 0.1968 | 0.654 |
| $a+b\sqrt{z}/y+c\sqrt{z}/y^2$ | 212.90 | 159.86 | 0.449 | 0.1014 | 0.0773 | 0.4926 | 0.3398 | 0.2568 | 0.511 |
| $a+b\sqrt{z}/y+c/\sqrt{y}z$ | 175.52 | 121.53 | 0.625 | 0.1021 | 0.0781 | 0.4855 | 0.3222 | 0.2227 | 0.560 |
| $a+b\sqrt{z}/y+c/\sqrt{y}z^2$ | 214.88 | 154.16 | 0.438 | 0.1183 | 0.0942 | 0.3088 | 0.3795 | 0.2839 | 0.390 |
| $a+b\sqrt{z}/y+c/\sqrt{y}\sqrt{z}$ | 152.86 | 102.92 | 0.716 | 0.0920 | 0.0675 | 0.5818 | 0.2900 | 0.1852 | 0.644 |
| $a+b\sqrt{z}/y+cz/\sqrt{y}$ | 132.56 | 104.74 | 0.786 | 0.0719 | 0.0454 | 0.7448 | 0.2509 | 0.1600 | 0.733 |
| $a+b\sqrt{z}/y+cz^2/\sqrt{y}$ | 143.89 | 113.78 | 0.748 | 0.0747 | 0.0497 | 0.7241 | 0.2713 | 0.1912 | 0.688 |
| $a+b\sqrt{z}/y+c\sqrt{z}/\sqrt{y}$ | 141.62 | 112.34 | 0.756 | 0.0757 | 0.0500 | 0.7173 | 0.2571 | 0.1605 | 0.720 |
| $a+b/y^2z+c/y^2z^2$ | 240.97 | 175.07 | 0.294 | 0.1229 | 0.0963 | 0.2543 | 0.3964 | 0.2928 | 0.334 |
| $a+b/y^2z+c/y^2\sqrt{z}$ | 239.97 | 173.49 | 0.299 | 0.1236 | 0.0963 | 0.2463 | 0.3978 | 0.2918 | 0.329 |
| $a+b/y^2z+cz/y^2$ | 227.51 | 164.25 | 0.370 | 0.1226 | 0.0968 | 0.2579 | 0.3910 | 0.2903 | 0.352 |
| $a+b/y^2z+cz^2/y^2$ | 184.65 | 133.88 | 0.585 | 0.1062 | 0.0791 | 0.4436 | 0.3397 | 0.2479 | 0.511 |
| $a+b/y^2z+c\sqrt{z}/y^2$ | 235.34 | 170.10 | 0.326 | 0.1240 | 0.0976 | 0.2412 | 0.3971 | 0.2937 | 0.332 |
| $a+b/y^2z+c/\sqrt{y}z$ | 173.30 | 115.50 | 0.635 | 0.1013 | 0.0764 | 0.4931 | 0.3219 | 0.2188 | 0.561 |
| $a+b/y^2z+c/\sqrt{y}z^2$ | 212.50 | 153.67 | 0.451 | 0.1171 | 0.0935 | 0.3232 | 0.3729 | 0.2808 | 0.411 |
| $a+b/y^2z+c/\sqrt{y}\sqrt{z}$ | 147.06 | 100.77 | 0.737 | 0.0872 | 0.0591 | 0.6243 | 0.2810 | 0.1665 | 0.666 |
| $a+b/y^2z+cz/\sqrt{y}$ | 137.66 | 106.18 | 0.769 | 0.0804 | 0.0594 | 0.6806 | 0.2694 | 0.1885 | 0.692 |
| $a+b/y^2z+cz^2/\sqrt{y}$ | 132.87 | 94.35 | 0.785 | 0.0751 | 0.0534 | 0.7218 | 0.2607 | 0.1741 | 0.712 |
| $a+b/y^2z+c\sqrt{z}/\sqrt{y}$ | 170.24 | 129.69 | 0.647 | 0.0973 | 0.0750 | 0.5330 | 0.3146 | 0.2343 | 0.581 |
| $a+b/y^2z^2+c/y^2\sqrt{z}$ | 241.38 | 174.88 | 0.291 | 0.1235 | 0.0965 | 0.2467 | 0.3986 | 0.2934 | 0.327 |
| $a+b/y^2z^2+cz/y^2$ | 240.69 | 175.27 | 0.295 | 0.1278 | 0.1014 | 0.1942 | 0.4111 | 0.3073 | 0.284 |
| $a+b/y^2z^2+cz^2/y^2$ | 208.57 | 147.96 | 0.471 | 0.1184 | 0.0878 | 0.3076 | 0.3831 | 0.2830 | 0.378 |
| $a+b/y^2z^2+c\sqrt{z}/y^2$ | 242.32 | 174.07 | 0.286 | 0.1262 | 0.0987 | 0.2137 | 0.4067 | 0.2993 | 0.299 |
| $a+b/y^2z^2+c/\sqrt{y}z$ | 169.04 | 110.98 | 0.652 | 0.0976 | 0.0689 | 0.5300 | 0.3151 | 0.1986 | 0.579 |
| $a+b/y^2z^2+c/\sqrt{y}z^2$ | 215.49 | 156.87 | 0.435 | 0.1198 | 0.0955 | 0.2908 | 0.3854 | 0.2916 | 0.371 |
| $a+b/y^2z^2+c/\sqrt{y}\sqrt{z}$ | 152.08 | 107.08 | 0.719 | 0.0838 | 0.0553 | 0.6529 | 0.2742 | 0.1642 | 0.682 |
| $a+b/y^2z^2+cz/\sqrt{y}$ | 144.71 | 113.84 | 0.745 | 0.0863 | 0.0637 | 0.6318 | 0.2916 | 0.2053 | 0.640 |
| $a+b/y^2z^2+cz^2/\sqrt{y}$ | 132.31 | 93.04 | 0.787 | 0.0779 | 0.0565 | 0.7003 | 0.2713 | 0.1885 | 0.688 |
| $a+b/y^2z^2+c\sqrt{z}/\sqrt{y}$ | 191.64 | 141.32 | 0.553 | 0.1098 | 0.0831 | 0.4050 | 0.3582 | 0.2679 | 0.456 |
| $a+b/y^2\sqrt{z}+cz/y^2$ | 216.71 | 155.15 | 0.429 | 0.1181 | 0.0920 | 0.3117 | 0.3745 | 0.2752 | 0.406 |
| $a+b/y^2\sqrt{z}+cz^2/y^2$ | 171.69 | 126.73 | 0.641 | 0.0985 | 0.0735 | 0.5208 | 0.3149 | 0.2277 | 0.580 |
| $a+b/y^2\sqrt{z}+c\sqrt{z}/y^2$ | 228.80 | 164.80 | 0.363 | 0.1217 | 0.0957 | 0.2686 | 0.3881 | 0.2861 | 0.362 |
| $a+b/y^2\sqrt{z}+c/\sqrt{y}z$ | 174.98 | 119.32 | 0.627 | 0.1020 | 0.0780 | 0.4859 | 0.3222 | 0.2228 | 0.560 |
| $a+b/y^2\sqrt{z}+c/\sqrt{y}z^2$ | 211.22 | 151.92 | 0.457 | 0.1155 | 0.0915 | 0.3411 | 0.3674 | 0.2729 | 0.428 |
| $a+b/y^2\sqrt{z}+c/\sqrt{y}\sqrt{z}$ | 147.75 | 95.99 | 0.734 | 0.0900 | 0.0644 | 0.5998 | 0.2863 | 0.1770 | 0.653 |
| $a+b/y^2\sqrt{z}+cz/\sqrt{y}$ | 136.22 | 104.45 | 0.774 | 0.0774 | 0.0566 | 0.7041 | 0.2606 | 0.1772 | 0.712 |
| $a+b/y^2\sqrt{z}+cz^2/\sqrt{y}$ | 135.43 | 99.52 | 0.777 | 0.0740 | 0.0514 | 0.7295 | 0.2589 | 0.1674 | 0.716 |
| $a+b/y^2\sqrt{z}+c\sqrt{z}/\sqrt{y}$ | 161.54 | 122.19 | 0.682 | 0.0904 | 0.0694 | 0.5968 | 0.2936 | 0.2142 | 0.635 |
| $a+bz/y^2+cz^2/y^2$ | 152.95 | 116.79 | 0.715 | 0.0802 | 0.0593 | 0.6828 | 0.2717 | 0.1849 | 0.687 |
| $a+bz/y^2+c\sqrt{z}/y^2$ | 185.09 | 133.18 | 0.583 | 0.1032 | 0.0760 | 0.4743 | 0.3253 | 0.2299 | 0.552 |
| $a+bz/y^2+c/\sqrt{y}z$ | 175.63 | 121.90 | 0.625 | 0.1021 | 0.0781 | 0.4854 | 0.3217 | 0.2223 | 0.562 |
| $a+bz/y^2+c/\sqrt{y}z^2$ | 214.49 | 152.78 | 0.440 | 0.1170 | 0.0923 | 0.3242 | 0.3756 | 0.2764 | 0.402 |
| $a+bz/y^2+c/\sqrt{y}\sqrt{z}$ | 152.84 | 104.72 | 0.716 | 0.0933 | 0.0695 | 0.5699 | 0.2923 | 0.1894 | 0.638 |
| $a+bz/y^2+cz/\sqrt{y}$ | 142.28 | 113.51 | 0.754 | 0.0731 | 0.0487 | 0.7362 | 0.2597 | 0.1726 | 0.714 |
| $a+bz/y^2+cz^2/\sqrt{y}$ | 148.36 | 114.73 | 0.732 | 0.0750 | 0.0516 | 0.7224 | 0.2747 | 0.1963 | 0.680 |
| $a+bz/y^2+c\sqrt{z}/\sqrt{y}$ | 169.68 | 134.09 | 0.650 | 0.0818 | 0.0601 | 0.6695 | 0.2870 | 0.2041 | 0.651 |
| $a+bz^2/y^2+c\sqrt{z}/y^2$ | 154.21 | 116.89 | 0.711 | 0.0843 | 0.0638 | 0.6487 | 0.2773 | 0.1965 | 0.674 |
| $a+bz^2/y^2+c/\sqrt{y}z$ | 165.55 | 115.58 | 0.667 | 0.0996 | 0.0741 | 0.5102 | 0.3180 | 0.2115 | 0.572 |
| $a+bz^2/y^2+c/\sqrt{y}z^2$ | 210.14 | 145.89 | 0.463 | 0.1190 | 0.0896 | 0.3002 | 0.3900 | 0.2784 | 0.355 |

(continued on next page)

**Table 4 – continued from previous page**

| Functional form | $T_{eff}$ (K) | | | Radius ($R_\odot$) | | | log (L/$L_\odot$) | | |
|---|---|---|---|---|---|---|---|---|---|
| | RMSE | MAD | $R^2_{ap}$ | RMSE | MAD | $R^2_{ap}$ | RMSE | MAD | $R^2_{ap}$ |
| $a+bz^2/y^2+c/\sqrt{y}\sqrt{z}$ | 142.96 | 104.87 | 0.751 | 0.0888 | 0.0638 | 0.6104 | 0.2816 | 0.1791 | 0.664 |
| $a+bz^2/y^2+cz/\sqrt{y}$ | 147.17 | 114.80 | 0.736 | 0.0748 | 0.0488 | 0.7240 | 0.2714 | 0.1779 | 0.688 |
| $a+bz^2/y^2+cz^2/\sqrt{y}$ | 153.15 | 118.15 | 0.715 | 0.0773 | 0.0545 | 0.7052 | 0.2887 | 0.2097 | 0.647 |
| $a+bz^2/y^2+c\sqrt{z}/\sqrt{y}$ | 257.30 | 180.59 | 0.195 | 0.1257 | 0.0967 | 0.2198 | 0.4430 | 0.3330 | 0.169 |
| $a+b\sqrt{z}/y^2+c/\sqrt{y}z$ | 176.25 | 121.94 | 0.622 | 0.1020 | 0.0780 | 0.4863 | 0.3210 | 0.2219 | 0.563 |
| $a+b\sqrt{z}/y^2+c/\sqrt{y}z^2$ | 211.96 | 152.19 | 0.453 | 0.1150 | 0.0901 | 0.3470 | 0.3675 | 0.2682 | 0.428 |
| $a+b\sqrt{z}/y^2+c/\sqrt{y}\sqrt{z}$ | 152.75 | 103.44 | 0.716 | 0.0933 | 0.0695 | 0.5701 | 0.2925 | 0.1892 | 0.637 |
| $a+b\sqrt{z}/y^2+cz/\sqrt{y}$ | 139.20 | 111.22 | 0.764 | 0.0735 | 0.0503 | 0.7330 | 0.2559 | 0.1653 | 0.723 |
| $a+b\sqrt{z}/y^2+cz^2/\sqrt{y}$ | 144.06 | 110.40 | 0.747 | 0.0740 | 0.0497 | 0.7297 | 0.2669 | 0.1846 | 0.698 |
| $a+b\sqrt{z}/y^2+c\sqrt{z}/\sqrt{y}$ | 159.77 | 126.24 | 0.689 | 0.0812 | 0.0590 | 0.6748 | 0.2756 | 0.1900 | 0.678 |
| $a+b/\sqrt{y}z+c/\sqrt{y}z^2$ | 157.08 | 107.28 | 0.700 | 0.0854 | 0.0604 | 0.6401 | 0.2663 | 0.1624 | 0.700 |
| $a+b/\sqrt{y}z+c/\sqrt{y}\sqrt{z}$ | 169.32 | 119.66 | 0.651 | 0.0933 | 0.0689 | 0.5698 | 0.2924 | 0.1908 | 0.638 |
| $a+b/\sqrt{y}z+cz/\sqrt{y}$ | 143.97 | 108.43 | 0.748 | 0.0863 | 0.0593 | 0.6325 | 0.2900 | 0.1848 | 0.644 |
| $a+b/\sqrt{y}z+cz^2/\sqrt{y}$ | 128.34 | 94.50 | 0.800 | 0.0774 | 0.0528 | 0.7045 | 0.2681 | 0.1717 | 0.695 |
| $a+b/\sqrt{y}z+c\sqrt{z}/\sqrt{y}$ | 166.52 | 113.39 | 0.663 | 0.0984 | 0.0712 | 0.5217 | 0.3168 | 0.2085 | 0.575 |
| $a+b/\sqrt{y}z^2+c/\sqrt{y}\sqrt{z}$ | 167.52 | 115.44 | 0.659 | 0.0906 | 0.0664 | 0.5944 | 0.2843 | 0.1776 | 0.657 |
| $a+b/\sqrt{y}z^2+cz/\sqrt{y}$ | 164.10 | 126.15 | 0.672 | 0.0941 | 0.0675 | 0.5629 | 0.3284 | 0.2246 | 0.543 |
| $a+b/\sqrt{y}z^2+cz^2/\sqrt{y}$ | 140.29 | 105.78 | 0.761 | 0.0822 | 0.0590 | 0.6664 | 0.2942 | 0.2048 | 0.633 |
| $a+b/\sqrt{y}z^2+c\sqrt{z}/\sqrt{y}$ | 208.66 | 147.22 | 0.470 | 0.1172 | 0.0855 | 0.3213 | 0.3875 | 0.2755 | 0.364 |
| $a+b/\sqrt{y}\sqrt{z}+cz/\sqrt{y}$ | 132.24 | 98.56 | 0.787 | 0.0797 | 0.0536 | 0.6867 | 0.2643 | 0.1646 | 0.704 |
| $a+b/\sqrt{y}\sqrt{z}+cz^2/\sqrt{y}$ | 124.56 | 93.48 | 0.811 | 0.0739 | 0.0493 | 0.7300 | 0.2530 | 0.1577 | 0.729 |
| $a+b/\sqrt{y}\sqrt{z}+c\sqrt{z}/\sqrt{y}$ | 145.57 | 101.03 | 0.742 | 0.0875 | 0.0618 | 0.6220 | 0.2807 | 0.1765 | 0.666 |
| $a+bz/\sqrt{y}+cz^2/\sqrt{y}$ | 162.34 | 123.73 | 0.679 | 0.0848 | 0.0638 | 0.6446 | 0.3187 | 0.2482 | 0.570 |
| $a+bz/\sqrt{y}+c\sqrt{z}/\sqrt{y}$ | 131.96 | 102.36 | 0.788 | 0.0717 | 0.0456 | 0.7459 | 0.2554 | 0.1737 | 0.724 |
| $a+bz^2/\sqrt{y}+c\sqrt{z}/\sqrt{y}$ | 152.85 | 122.81 | 0.716 | 0.0791 | 0.0569 | 0.6910 | 0.2936 | 0.2215 | 0.635 |
| Different EW ratio, double component functions result ( (x/y, x/z) & (x/y, y/z) | | | | | | | | | |
| a+bx/y+cx/z | 222.67 | 168.38 | 0.397 | 0.1078 | 0.0847 | 0.4260 | 0.3613 | 0.2820 | 0.447 |
| $a+bx/y+cx/z^2$ | 223.19 | 168.22 | 0.394 | 0.1110 | 0.0865 | 0.3917 | 0.3641 | 0.2814 | 0.438 |
| $a+bx/y+cx/\sqrt{z}$ | 254.34 | 191.06 | 0.213 | 0.1215 | 0.0946 | 0.2717 | 0.3992 | 0.3093 | 0.325 |
| a+bx/y+cxz | 124.53 | 92.70 | 0.811 | 0.0687 | 0.0478 | 0.7670 | 0.2421 | 0.1782 | 0.752 |
| $a+bx/y+cxz^2$ | 139.37 | 105.87 | 0.764 | 0.0728 | 0.0544 | 0.7380 | 0.2601 | 0.1987 | 0.713 |
| $a+bx/y+cx\sqrt{z}$ | 116.97 | 90.39 | 0.834 | 0.0690 | 0.0449 | 0.7649 | 0.2337 | 0.1589 | 0.769 |
| $a+bx/y+cx^2/z$ | 254.14 | 190.82 | 0.214 | 0.1211 | 0.0937 | 0.2757 | 0.3990 | 0.3083 | 0.326 |
| $a+bx/y+cx^2/z^2$ | 234.12 | 173.85 | 0.333 | 0.1138 | 0.0887 | 0.3604 | 0.3768 | 0.2898 | 0.398 |
| $a+bx/y+cx^2/\sqrt{z}$ | 194.04 | 156.89 | 0.542 | 0.1044 | 0.0822 | 0.4614 | 0.3240 | 0.2493 | 0.555 |
| $a+bx/y+cx^2z$ | 129.06 | 99.45 | 0.797 | 0.0718 | 0.0533 | 0.7455 | 0.2518 | 0.1930 | 0.731 |
| $a+bx/y+cx^2z^2$ | 142.87 | 111.71 | 0.752 | 0.0761 | 0.0590 | 0.7144 | 0.2685 | 0.2119 | 0.695 |
| $a+bx/y+cx^2\sqrt{z}$ | 121.87 | 94.90 | 0.819 | 0.0714 | 0.0511 | 0.7480 | 0.2438 | 0.1817 | 0.748 |
| $a+bx/y+c\sqrt{x}/z$ | 196.50 | 148.87 | 0.530 | 0.1001 | 0.0776 | 0.5057 | 0.3304 | 0.2507 | 0.537 |
| $a+bx/y+c\sqrt{x}/z^2$ | 214.62 | 162.98 | 0.440 | 0.1091 | 0.0842 | 0.4119 | 0.3544 | 0.2714 | 0.468 |
| $a+bx/y+c\sqrt{x}/\sqrt{z}$ | 216.90 | 162.26 | 0.428 | 0.1056 | 0.0837 | 0.4491 | 0.3544 | 0.2742 | 0.468 |
| $a+bx/y+c\sqrt{x}z$ | 126.39 | 96.06 | 0.806 | 0.0685 | 0.0462 | 0.7686 | 0.2414 | 0.1700 | 0.753 |
| $a+bx/y+c\sqrt{x}z^2$ | 139.35 | 105.44 | 0.764 | 0.0719 | 0.0527 | 0.7448 | 0.2576 | 0.1909 | 0.719 |
| $a+bx/y+c\sqrt{x}\sqrt{z}$ | 121.47 | 92.67 | 0.820 | 0.0694 | 0.0436 | 0.7621 | 0.2353 | 0.1504 | 0.765 |
| a+bx/y+c/xz | 252.36 | 189.56 | 0.225 | 0.1208 | 0.0939 | 0.2800 | 0.3942 | 0.2994 | 0.341 |
| $a+bx/y+c/xz^2$ | 240.90 | 176.73 | 0.294 | 0.1183 | 0.0898 | 0.3084 | 0.3810 | 0.2777 | 0.385 |
| $a+bx/y+c/x\sqrt{z}$ | 254.48 | 191.52 | 0.212 | 0.1218 | 0.0954 | 0.2676 | 0.3986 | 0.3069 | 0.327 |
| a+bx/y+cz/x | 232.86 | 171.40 | 0.340 | 0.1172 | 0.0916 | 0.3213 | 0.3790 | 0.2937 | 0.391 |
| $a+bx/y+cz^2/x$ | 170.52 | 131.23 | 0.646 | 0.0931 | 0.0727 | 0.5722 | 0.3036 | 0.2291 | 0.609 |
| $a+bx/y+c\sqrt{z}/x$ | 246.68 | 181.55 | 0.260 | 0.1211 | 0.0932 | 0.2764 | 0.3937 | 0.3037 | 0.343 |
| $a+bx/y+c/x^2z$ | 247.52 | 182.18 | 0.255 | 0.1214 | 0.0937 | 0.2726 | 0.3947 | 0.3050 | 0.340 |
| $a+bx/y+c/x^2z^2$ | 250.93 | 186.46 | 0.234 | 0.1218 | 0.0947 | 0.2679 | 0.3973 | 0.3090 | 0.331 |
| $a+bx/y+c/x^2\sqrt{z}$ | 246.28 | 180.49 | 0.262 | 0.1212 | 0.0933 | 0.2743 | 0.3936 | 0.3032 | 0.343 |
| $a+bx/y+cz/x^2$ | 243.54 | 176.67 | 0.278 | 0.1208 | 0.0923 | 0.2791 | 0.3912 | 0.2989 | 0.352 |
| $a+bx/y+cz^2/x^2$ | 240.76 | 174.31 | 0.295 | 0.1202 | 0.0920 | 0.2863 | 0.3884 | 0.2968 | 0.361 |
| $a+bx/y+c\sqrt{z}/x^2$ | 244.42 | 177.87 | 0.273 | 0.1210 | 0.0926 | 0.2773 | 0.3920 | 0.3003 | 0.349 |
| $a+bx/y+c/\sqrt{x}z$ | 204.07 | 145.69 | 0.493 | 0.1053 | 0.0807 | 0.4529 | 0.3328 | 0.2379 | 0.531 |
| $a+bx/y+c/\sqrt{x}z^2$ | 209.18 | 155.37 | 0.468 | 0.1101 | 0.0845 | 0.4020 | 0.3466 | 0.2534 | 0.491 |
| $a+bx/y+c/\sqrt{x}\sqrt{z}$ | 221.45 | 158.53 | 0.403 | 0.1087 | 0.0823 | 0.4161 | 0.3505 | 0.2458 | 0.479 |
| $a+bx/y+cz/\sqrt{x}$ | 162.44 | 127.30 | 0.679 | 0.0880 | 0.0679 | 0.6174 | 0.2912 | 0.2218 | 0.641 |
| $a+bx/y+cz^2/\sqrt{x}$ | 139.06 | 104.77 | 0.765 | 0.0729 | 0.0538 | 0.7378 | 0.2566 | 0.1891 | 0.721 |
| $a+bx/y+c\sqrt{z}/\sqrt{x}$ | 223.27 | 167.08 | 0.394 | 0.1125 | 0.0885 | 0.3751 | 0.3665 | 0.2827 | 0.431 |
| a+bx/y+cy/z | 220.25 | 165.42 | 0.410 | 0.1076 | 0.0836 | 0.4287 | 0.3587 | 0.2739 | 0.455 |
| $a+bx/y+cy/z^2$ | 219.16 | 164.28 | 0.416 | 0.1100 | 0.0848 | 0.4023 | 0.3596 | 0.2751 | 0.452 |
| $a+bx/y+cy/\sqrt{z}$ | 253.38 | 188.95 | 0.219 | 0.1210 | 0.0941 | 0.2777 | 0.3982 | 0.3084 | 0.328 |
| a+bx/y+cyz | 125.66 | 91.51 | 0.808 | 0.0696 | 0.0452 | 0.7606 | 0.2427 | 0.1669 | 0.750 |
| $a+bx/y+cyz^2$ | 138.46 | 102.92 | 0.767 | 0.0727 | 0.0520 | 0.7391 | 0.2585 | 0.1908 | 0.717 |
| $a+bx/y+cy\sqrt{z}$ | 126.13 | 93.32 | 0.806 | 0.0727 | 0.0469 | 0.7390 | 0.2425 | 0.1507 | 0.751 |
| $a+bx/y+cy^2/z$ | 252.63 | 187.89 | 0.224 | 0.1204 | 0.0930 | 0.2845 | 0.3973 | 0.3062 | 0.331 |
| $a+bx/y+cy^2/z^2$ | 231.17 | 169.45 | 0.350 | 0.1130 | 0.0869 | 0.3698 | 0.3733 | 0.2844 | 0.410 |
| $a+bx/y+cy^2/\sqrt{z}$ | 227.82 | 179.91 | 0.369 | 0.1146 | 0.0907 | 0.3516 | 0.3647 | 0.2827 | 0.436 |
| $a+bx/y+cy^2z$ | 129.75 | 97.00 | 0.795 | 0.0727 | 0.0499 | 0.7390 | 0.2515 | 0.1773 | 0.732 |
| $a+bx/y+cy^2z^2$ | 140.95 | 106.67 | 0.758 | 0.0755 | 0.0554 | 0.7186 | 0.2654 | 0.1991 | 0.702 |
| $a+bx/y+cy^2\sqrt{z}$ | 130.31 | 95.69 | 0.793 | 0.0752 | 0.0515 | 0.7208 | 0.2514 | 0.1665 | 0.732 |
| $a+bx/y+c\sqrt{y}/z$ | 192.88 | 146.07 | 0.547 | 0.0991 | 0.0761 | 0.5148 | 0.3261 | 0.2438 | 0.550 |
| $a+bx/y+c\sqrt{y}/z^2$ | 211.68 | 160.31 | 0.455 | 0.1085 | 0.0829 | 0.4187 | 0.3510 | 0.2662 | 0.478 |
| $a+bx/y+c\sqrt{y}/\sqrt{z}$ | 214.91 | 161.83 | 0.438 | 0.1050 | 0.0825 | 0.4560 | 0.3515 | 0.2682 | 0.476 |
| $a+bx/y+c\sqrt{y}z$ | 125.53 | 94.38 | 0.808 | 0.0687 | 0.0444 | 0.7667 | 0.2406 | 0.1646 | 0.755 |
| $a+bx/y+c\sqrt{y}z^2$ | 138.49 | 104.68 | 0.767 | 0.0718 | 0.0513 | 0.7458 | 0.2565 | 0.1863 | 0.721 |
| $a+bx/y+c\sqrt{y}\sqrt{z}$ | 123.28 | 92.78 | 0.815 | 0.0709 | 0.0449 | 0.7516 | 0.2377 | 0.1456 | 0.761 |
| a+bx/y+c/yz | 202.53 | 145.49 | 0.501 | 0.1076 | 0.0813 | 0.4289 | 0.3349 | 0.2404 | 0.525 |
| $a+bx/y+c/yz^2$ | 210.84 | 156.53 | 0.459 | 0.1117 | 0.0851 | 0.3841 | 0.3498 | 0.2568 | 0.481 |
| $a+bx/y+c/y\sqrt{z}$ | 207.71 | 150.31 | 0.475 | 0.1076 | 0.0827 | 0.4279 | 0.3377 | 0.2413 | 0.517 |
| a+bx/y+cz/y | 207.61 | 153.66 | 0.476 | 0.1024 | 0.0813 | 0.4820 | 0.3424 | 0.2651 | 0.503 |
| $a+bx/y+cz^2/y$ | 154.60 | 119.85 | 0.709 | 0.0776 | 0.0605 | 0.7024 | 0.2728 | 0.2083 | 0.685 |
| $a+bx/y+c\sqrt{z}/y$ | 253.49 | 189.57 | 0.218 | 0.1216 | 0.0949 | 0.2697 | 0.3987 | 0.3099 | 0.327 |
| $a+bx/y+c/y^2z$ | 237.25 | 172.33 | 0.315 | 0.1182 | 0.0909 | 0.3105 | 0.3775 | 0.2787 | 0.396 |
| $a+bx/y+c/y^2z^2$ | 233.49 | 172.59 | 0.337 | 0.1181 | 0.0906 | 0.3109 | 0.3757 | 0.2775 | 0.402 |
| $a+bx/y+c/y^2\sqrt{z}$ | 241.71 | 177.01 | 0.289 | 0.1187 | 0.0911 | 0.3038 | 0.3816 | 0.2798 | 0.383 |
| $a+bx/y+cz/y^2$ | 252.51 | 188.59 | 0.224 | 0.1216 | 0.0948 | 0.2694 | 0.3981 | 0.3099 | 0.328 |
| $a+bx/y+cz^2/y^2$ | 209.92 | 156.72 | 0.464 | 0.1049 | 0.0835 | 0.4569 | 0.3467 | 0.2728 | 0.491 |
| $a+bx/y+c\sqrt{z}/y^2$ | 253.75 | 191.02 | 0.217 | 0.1217 | 0.0951 | 0.2686 | 0.3971 | 0.3040 | 0.332 |

(continued on next page)

**Table 4 – continued from previous page**

| Functional form | $T_{eff}$ (K) RMSE | MAD | $R^2_{ap}$ | Radius ($R_\odot$) RMSE | MAD | $R^2_{ap}$ | log (L/$L_\odot$) RMSE | MAD | $R^2_{ap}$ |
|---|---|---|---|---|---|---|---|---|---|
| $a+bx/y+c/\sqrt{y}z$ | 176.23 | 129.51 | 0.622 | 0.0984 | 0.0752 | 0.5217 | 0.3046 | 0.2147 | 0.607 |
| $a+bx/y+c/\sqrt{y}z^2$ | 202.60 | 152.18 | 0.501 | 0.1084 | 0.0834 | 0.4202 | 0.3407 | 0.2476 | 0.508 |
| $a+bx/y+c/\sqrt{y}\sqrt{z}$ | 169.32 | 119.90 | 0.651 | 0.0944 | 0.0711 | 0.5603 | 0.2919 | 0.1984 | 0.639 |
| $a+bx/y+cz/\sqrt{y}$ | 154.18 | 121.36 | 0.711 | 0.0793 | 0.0613 | 0.6891 | 0.2740 | 0.2099 | 0.682 |
| $a+bx/y+cz^2/\sqrt{y}$ | 144.40 | 109.91 | 0.746 | 0.0729 | 0.0543 | 0.7375 | 0.2603 | 0.1955 | 0.713 |
| $a+bx/y+c\sqrt{z}/\sqrt{y}$ | 208.38 | 153.38 | 0.472 | 0.1023 | 0.0818 | 0.4836 | 0.3430 | 0.2656 | 0.501 |
| $a+bx/y^2+cx/z$ | 251.22 | 190.01 | 0.232 | 0.1353 | 0.1023 | 0.0959 | 0.4593 | 0.3447 | 0.106 |
| $a+bx/y^2+cx/z^2$ | 242.43 | 186.00 | 0.285 | 0.1323 | 0.1014 | 0.1358 | 0.4483 | 0.3404 | 0.148 |
| $a+bx/y^2+cx/\sqrt{z}$ | 244.00 | 191.17 | 0.276 | 0.1304 | 0.1047 | 0.1603 | 0.4235 | 0.3300 | 0.240 |
| $a+bx/y^2+cxz$ | 124.08 | 96.02 | 0.813 | 0.0733 | 0.0529 | 0.7347 | 0.2704 | 0.2088 | 0.690 |
| $a+bx/y^2+cxz^2$ | 148.47 | 116.75 | 0.732 | 0.0851 | 0.0658 | 0.6425 | 0.3155 | 0.2498 | 0.578 |
| $a+bx/y^2+cx\sqrt{z}$ | 114.47 | 89.71 | 0.841 | 0.0693 | 0.0454 | 0.7629 | 0.2417 | 0.1605 | 0.752 |
| $a+bx/y^2+cx^2/z$ | 250.72 | 200.36 | 0.235 | 0.1345 | 0.1073 | 0.1069 | 0.4419 | 0.3511 | 0.173 |
| $a+bx/y^2+cx^2/z^2$ | 250.13 | 190.17 | 0.239 | 0.1349 | 0.1034 | 0.1013 | 0.4574 | 0.3471 | 0.114 |
| $a+bx/y^2+cx^2/\sqrt{z}$ | 184.51 | 147.49 | 0.586 | 0.1045 | 0.0832 | 0.4607 | 0.3244 | 0.2454 | 0.554 |
| $a+bx/y^2+cx^2z$ | 133.01 | 104.72 | 0.785 | 0.0797 | 0.0611 | 0.6864 | 0.2924 | 0.2340 | 0.638 |
| $a+bx/y^2+cx^2z^2$ | 155.02 | 124.31 | 0.708 | 0.0902 | 0.0706 | 0.5987 | 0.3301 | 0.2613 | 0.538 |
| $a+bx/y^2+cx^2\sqrt{z}$ | 121.03 | 95.91 | 0.822 | 0.0749 | 0.0552 | 0.7227 | 0.2675 | 0.2036 | 0.697 |
| $a+bx/y^2+c\sqrt{x}/z$ | 231.16 | 176.03 | 0.350 | 0.1275 | 0.0936 | 0.1974 | 0.4360 | 0.3216 | 0.195 |
| $a+bx/y^2+c\sqrt{x}/z^2$ | 234.51 | 178.44 | 0.331 | 0.1295 | 0.0986 | 0.1721 | 0.4370 | 0.3282 | 0.191 |
| $a+bx/y^2+c\sqrt{x}/\sqrt{z}$ | 254.49 | 193.83 | 0.212 | 0.1367 | 0.1038 | 0.0771 | 0.4611 | 0.3520 | 0.099 |
| $a+bx/y^2+c\sqrt{x}z$ | 124.91 | 99.48 | 0.810 | 0.0724 | 0.0495 | 0.7413 | 0.2668 | 0.1989 | 0.698 |
| $a+bx/y^2+c\sqrt{x}z^2$ | 147.24 | 117.74 | 0.736 | 0.0834 | 0.0637 | 0.6562 | 0.3106 | 0.2437 | 0.591 |
| $a+bx/y^2+c\sqrt{x}\sqrt{z}$ | 118.83 | 89.95 | 0.828 | 0.0694 | 0.0432 | 0.7621 | 0.2404 | 0.1491 | 0.755 |
| $a+bx/y^2+c/xz$ | 225.67 | 166.70 | 0.380 | 0.1173 | 0.0888 | 0.3208 | 0.3808 | 0.2724 | 0.386 |
| $a+bx/y^2+c/xz^2$ | 222.68 | 160.87 | 0.397 | 0.1183 | 0.0899 | 0.3092 | 0.3798 | 0.2728 | 0.389 |
| $a+bx/y^2+c/x\sqrt{z}$ | 229.00 | 170.76 | 0.362 | 0.1183 | 0.0892 | 0.3093 | 0.3868 | 0.2789 | 0.366 |
| $a+bx/y^2+cz/x$ | 247.89 | 190.83 | 0.252 | 0.1290 | 0.0992 | 0.1780 | 0.4284 | 0.3267 | 0.222 |
| $a+bx/y^2+cz^2/x$ | 249.77 | 190.32 | 0.241 | 0.1358 | 0.1010 | 0.0900 | 0.4595 | 0.3445 | 0.105 |
| $a+bx/y^2+c\sqrt{z}/x$ | 239.71 | 180.72 | 0.301 | 0.1238 | 0.0920 | 0.2436 | 0.4093 | 0.3032 | 0.290 |
| $a+bx/y^2+c/x^2z$ | 239.02 | 179.45 | 0.305 | 0.1230 | 0.0911 | 0.2526 | 0.4077 | 0.3005 | 0.296 |
| $a+bx/y^2+c/x^2z^2$ | 237.69 | 176.90 | 0.313 | 0.1228 | 0.0913 | 0.2551 | 0.4049 | 0.2947 | 0.305 |
| $a+bx/y^2+c/x^2\sqrt{z}$ | 239.59 | 180.23 | 0.302 | 0.1232 | 0.0915 | 0.2504 | 0.4091 | 0.3023 | 0.291 |
| $a+bx/y^2+cz/x^2$ | 241.23 | 181.73 | 0.292 | 0.1240 | 0.0927 | 0.2412 | 0.4131 | 0.3061 | 0.277 |
| $a+bx/y^2+cz^2/x^2$ | 243.08 | 183.81 | 0.281 | 0.1251 | 0.0943 | 0.2269 | 0.4174 | 0.3107 | 0.262 |
| $a+bx/y^2+c\sqrt{z}/x^2$ | 240.65 | 181.31 | 0.295 | 0.1237 | 0.0924 | 0.2450 | 0.4117 | 0.3050 | 0.282 |
| $a+bx/y^2+c/\sqrt{x}z$ | 193.72 | 137.34 | 0.543 | 0.1044 | 0.0800 | 0.4618 | 0.3293 | 0.2360 | 0.541 |
| $a+bx/y^2+c/\sqrt{x}z^2$ | 205.71 | 147.23 | 0.485 | 0.1149 | 0.0917 | 0.3482 | 0.3669 | 0.2744 | 0.430 |
| $a+bx/y^2+c/\sqrt{x}\sqrt{z}$ | 201.56 | 147.78 | 0.506 | 0.1057 | 0.0796 | 0.4487 | 0.3372 | 0.2357 | 0.518 |
| $a+bx/y^2+cz/\sqrt{x}$ | 237.39 | 174.70 | 0.314 | 0.1307 | 0.0927 | 0.1561 | 0.4475 | 0.3225 | 0.151 |
| $a+bx/y^2+cz^2/\sqrt{x}$ | 168.51 | 133.38 | 0.655 | 0.0952 | 0.0682 | 0.5526 | 0.3471 | 0.2592 | 0.489 |
| $a+bx/y^2+c\sqrt{z}/\sqrt{x}$ | 252.83 | 197.31 | 0.222 | 0.1331 | 0.1042 | 0.1247 | 0.4419 | 0.3443 | 0.173 |
| $a+bx/y^2+cy/z$ | 226.57 | 171.24 | 0.375 | 0.1255 | 0.0901 | 0.2225 | 0.4303 | 0.3138 | 0.215 |
| $a+bx/y^2+cy/z^2$ | 230.74 | 175.34 | 0.352 | 0.1279 | 0.0967 | 0.1927 | 0.4324 | 0.3220 | 0.208 |
| $a+bx/y^2+cy/\sqrt{z}$ | 254.01 | 192.91 | 0.215 | 0.1366 | 0.1031 | 0.0789 | 0.4610 | 0.3504 | 0.099 |
| $a+bx/y^2+cyz$ | 136.63 | 106.62 | 0.773 | 0.0781 | 0.0573 | 0.6989 | 0.2898 | 0.2230 | 0.644 |
| $a+bx/y^2+cyz^2$ | 155.45 | 122.79 | 0.706 | 0.0879 | 0.0675 | 0.6181 | 0.3256 | 0.2536 | 0.551 |
| $a+bx/y^2+cy\sqrt{z}$ | 130.91 | 100.85 | 0.791 | 0.0748 | 0.0494 | 0.7236 | 0.2685 | 0.1838 | 0.694 |
| $a+bx/y^2+cy^2/z$ | 248.31 | 186.13 | 0.250 | 0.1342 | 0.0990 | 0.1112 | 0.4565 | 0.3403 | 0.117 |
| $a+bx/y^2+cy^2/z^2$ | 235.31 | 179.52 | 0.326 | 0.1294 | 0.0973 | 0.1738 | 0.4400 | 0.3290 | 0.180 |
| $a+bx/y^2+cy^2/\sqrt{z}$ | 243.04 | 195.68 | 0.281 | 0.1297 | 0.1043 | 0.1690 | 0.4274 | 0.3345 | 0.226 |
| $a+bx/y^2+cy^2z$ | 149.05 | 112.24 | 0.730 | 0.0857 | 0.0645 | 0.6371 | 0.3151 | 0.2425 | 0.579 |
| $a+bx/y^2+cy^2z^2$ | 164.00 | 128.23 | 0.673 | 0.0937 | 0.0723 | 0.5669 | 0.3424 | 0.2637 | 0.503 |
| $a+bx/y^2+cy^2\sqrt{z}$ | 144.24 | 104.86 | 0.747 | 0.0831 | 0.0593 | 0.6587 | 0.3001 | 0.2152 | 0.619 |
| $a+bx/y^2+c\sqrt{y}/z$ | 205.88 | 152.06 | 0.484 | 0.1167 | 0.0831 | 0.3270 | 0.3987 | 0.2787 | 0.327 |
| $a+bx/y^2+c\sqrt{y}/z^2$ | 225.58 | 169.22 | 0.381 | 0.1259 | 0.0958 | 0.2169 | 0.4233 | 0.3125 | 0.241 |
| $a+bx/y^2+c\sqrt{y}/\sqrt{z}$ | 224.78 | 168.29 | 0.385 | 0.1247 | 0.0886 | 0.2324 | 0.4290 | 0.3101 | 0.220 |
| $a+bx/y^2+c\sqrt{y}z$ | 132.85 | 106.20 | 0.785 | 0.0759 | 0.0535 | 0.7153 | 0.2817 | 0.2121 | 0.664 |
| $a+bx/y^2+c\sqrt{y}z^2$ | 151.72 | 121.82 | 0.720 | 0.0854 | 0.0649 | 0.6397 | 0.3177 | 0.2469 | 0.572 |
| $a+bx/y^2+c\sqrt{y}\sqrt{z}$ | 126.02 | 99.46 | 0.807 | 0.0724 | 0.0439 | 0.7411 | 0.2590 | 0.1708 | 0.716 |
| $a+bx/y^2+c/yz$ | 200.77 | 139.96 | 0.510 | 0.1104 | 0.0848 | 0.3987 | 0.3462 | 0.2487 | 0.492 |
| $a+bx/y^2+c/yz^2$ | 215.47 | 156.16 | 0.435 | 0.1206 | 0.0969 | 0.2821 | 0.3859 | 0.2944 | 0.369 |
| $a+bx/y^2+c/y\sqrt{z}$ | 203.31 | 146.22 | 0.497 | 0.1090 | 0.0823 | 0.4137 | 0.3434 | 0.2429 | 0.500 |
| $a+bx/y^2+cz/y$ | 235.60 | 171.94 | 0.325 | 0.1297 | 0.0918 | 0.1692 | 0.4441 | 0.3193 | 0.164 |
| $a+bx/y^2+cz^2/y$ | 164.47 | 128.74 | 0.671 | 0.0930 | 0.0662 | 0.5728 | 0.3375 | 0.2503 | 0.517 |
| $a+bx/y^2+c\sqrt{z}/y$ | 252.81 | 197.02 | 0.222 | 0.1335 | 0.1048 | 0.1198 | 0.4426 | 0.3438 | 0.170 |
| $a+bx/y^2+c/y^2z$ | 228.84 | 165.43 | 0.363 | 0.1224 | 0.0967 | 0.2597 | 0.3929 | 0.2923 | 0.346 |
| $a+bx/y^2+c/y^2z^2$ | 233.01 | 170.33 | 0.339 | 0.1267 | 0.1005 | 0.2077 | 0.4081 | 0.3069 | 0.294 |
| $a+bx/y^2+c/y^2\sqrt{z}$ | 228.96 | 167.20 | 0.362 | 0.1212 | 0.0945 | 0.2747 | 0.3901 | 0.2862 | 0.355 |
| $a+bx/y^2+cz/y^2$ | 247.65 | 189.59 | 0.254 | 0.1296 | 0.0999 | 0.1709 | 0.4283 | 0.3245 | 0.223 |
| $a+bx/y^2+cz^2/y^2$ | 247.12 | 186.16 | 0.257 | 0.1347 | 0.0984 | 0.1047 | 0.4567 | 0.3368 | 0.116 |
| $a+bx/y^2+c\sqrt{z}/y^2$ | 238.08 | 175.18 | 0.310 | 0.1242 | 0.0954 | 0.2387 | 0.4062 | 0.2937 | 0.301 |
| $a+bx/y^2+c/\sqrt{y}z$ | 177.24 | 124.54 | 0.618 | 0.1017 | 0.0771 | 0.4893 | 0.3209 | 0.2180 | 0.564 |
| $a+bx/y^2+c/\sqrt{y}z^2$ | 211.75 | 151.60 | 0.454 | 0.1200 | 0.0944 | 0.2893 | 0.3900 | 0.2844 | 0.356 |
| $a+bx/y^2+c/\sqrt{y}\sqrt{z}$ | 169.22 | 119.75 | 0.652 | 0.0943 | 0.0707 | 0.5606 | 0.2944 | 0.1961 | 0.633 |
| $a+bx/y^2+cz/\sqrt{y}$ | 165.39 | 129.45 | 0.667 | 0.0951 | 0.0659 | 0.5538 | 0.3403 | 0.2404 | 0.509 |
| $a+bx/y^2+cz^2/\sqrt{y}$ | 151.57 | 123.22 | 0.720 | 0.0852 | 0.0633 | 0.6413 | 0.3152 | 0.2460 | 0.579 |
| $a+bx/y^2+c\sqrt{z}/\sqrt{y}$ | 229.97 | 168.64 | 0.357 | 0.1271 | 0.0894 | 0.2020 | 0.4369 | 0.3126 | 0.191 |
| $a+bx/\sqrt{y}+cx/z$ | 153.43 | 121.42 | 0.714 | 0.0819 | 0.0615 | 0.6688 | 0.2618 | 0.1886 | 0.710 |
| $a+bx/\sqrt{y}+cx/z^2$ | 166.94 | 127.05 | 0.661 | 0.0890 | 0.0696 | 0.6092 | 0.2776 | 0.2009 | 0.673 |
| $a+bx/\sqrt{y}+cx/\sqrt{z}$ | 158.69 | 123.86 | 0.694 | 0.0808 | 0.0612 | 0.6776 | 0.2626 | 0.1938 | 0.708 |
| $a+bx/\sqrt{y}+cxz$ | 119.38 | 89.29 | 0.827 | 0.0681 | 0.0450 | 0.7707 | 0.2318 | 0.1582 | 0.772 |
| $a+bx/\sqrt{y}+cxz^2$ | 123.70 | 94.52 | 0.814 | 0.0691 | 0.0479 | 0.7640 | 0.2352 | 0.1646 | 0.766 |
| $a+bx/\sqrt{y}+cx\sqrt{z}$ | 117.12 | 90.67 | 0.833 | 0.0693 | 0.0442 | 0.7629 | 0.2321 | 0.1523 | 0.772 |
| $a+bx/\sqrt{y}+cx^2/z$ | 172.38 | 127.73 | 0.638 | 0.0859 | 0.0652 | 0.6353 | 0.2772 | 0.2020 | 0.674 |
| $a+bx/\sqrt{y}+cx^2/z^2$ | 170.22 | 128.63 | 0.647 | 0.0888 | 0.0691 | 0.6104 | 0.2799 | 0.2023 | 0.668 |
| $a+bx/\sqrt{y}+cx^2/\sqrt{z}$ | 183.78 | 139.58 | 0.589 | 0.0946 | 0.0748 | 0.5578 | 0.2928 | 0.2168 | 0.637 |
| $a+bx/\sqrt{y}+cx^2z$ | 121.20 | 93.50 | 0.821 | 0.0704 | 0.0494 | 0.7552 | 0.2372 | 0.1685 | 0.762 |
| $a+bx/\sqrt{y}+cx^2z^2$ | 125.41 | 96.33 | 0.809 | 0.0714 | 0.0509 | 0.7480 | 0.2402 | 0.1727 | 0.755 |
| $a+bx/\sqrt{y}+cx^2\sqrt{z}$ | 119.51 | 93.52 | 0.826 | 0.0714 | 0.0495 | 0.7481 | 0.2375 | 0.1666 | 0.761 |

(continued on next page)

**Table 4 – continued from previous page**

| Functional form | $T_{eff}$ (K) | | | Radius ($R_\odot$) | | | log ($L/L_\odot$) | | |
|---|---|---|---|---|---|---|---|---|---|
| | RMSE | MAD | $R^2_{ap}$ | RMSE | MAD | $R^2_{ap}$ | RMSE | MAD | $R^2_{ap}$ |
| $a+bx/\sqrt{y}+c\sqrt{x}/z$ | 147.16 | 115.35 | 0.737 | 0.0821 | 0.0622 | 0.6670 | 0.2579 | 0.1814 | 0.718 |
| $a+bx/\sqrt{y}+c\sqrt{x}/z^2$ | 165.38 | 125.79 | 0.667 | 0.0894 | 0.0701 | 0.6052 | 0.2769 | 0.1992 | 0.675 |
| $a+bx/\sqrt{y}+c\sqrt{x}/\sqrt{z}$ | 139.46 | 112.18 | 0.763 | 0.0777 | 0.0565 | 0.7021 | 0.2483 | 0.1762 | 0.739 |
| $a+bx/\sqrt{y}+c\sqrt{x}z$ | 121.02 | 90.81 | 0.822 | 0.0678 | 0.0429 | 0.7733 | 0.2307 | 0.1506 | 0.775 |
| $a+bx/\sqrt{y}+c\sqrt{x}z^2$ | 123.79 | 93.14 | 0.814 | 0.0683 | 0.0459 | 0.7698 | 0.2332 | 0.1603 | 0.770 |
| $a+bx/\sqrt{y}+c\sqrt{x}\sqrt{z}$ | 122.10 | 92.57 | 0.819 | 0.0695 | 0.0430 | 0.7614 | 0.2330 | 0.1460 | 0.770 |
| $a+bx/\sqrt{y}+c/xz$ | 152.15 | 123.35 | 0.718 | 0.0863 | 0.0647 | 0.6322 | 0.2636 | 0.1881 | 0.706 |
| $a+bx/\sqrt{y}+c/xz^2$ | 177.14 | 136.53 | 0.618 | 0.0895 | 0.0706 | 0.6041 | 0.2813 | 0.2159 | 0.665 |
| $a+bx/\sqrt{y}+c/x\sqrt{z}$ | 145.56 | 112.27 | 0.742 | 0.0864 | 0.0659 | 0.6317 | 0.2604 | 0.1827 | 0.713 |
| $a+bx/\sqrt{y}+cz/x$ | 131.43 | 103.63 | 0.790 | 0.0837 | 0.0643 | 0.6540 | 0.2496 | 0.1756 | 0.736 |
| $a+bx/\sqrt{y}+cz^2/x$ | 108.31 | 83.90 | 0.857 | 0.0737 | 0.0543 | 0.7316 | 0.2264 | 0.1581 | 0.783 |
| $a+bx/\sqrt{y}+c\sqrt{z}/x$ | 138.37 | 107.13 | 0.767 | 0.0858 | 0.0661 | 0.6368 | 0.2559 | 0.1810 | 0.723 |
| $a+bx/\sqrt{y}+c/x^2z$ | 141.74 | 108.70 | 0.756 | 0.0870 | 0.0672 | 0.6263 | 0.2593 | 0.1857 | 0.715 |
| $a+bx/\sqrt{y}+c/x^2z^2$ | 140.19 | 106.84 | 0.761 | 0.0855 | 0.0653 | 0.6389 | 0.2562 | 0.1792 | 0.722 |
| $a+bx/\sqrt{y}+c/x^2\sqrt{z}$ | 142.84 | 109.23 | 0.752 | 0.0875 | 0.0677 | 0.6219 | 0.2607 | 0.1875 | 0.712 |
| $a+bx/\sqrt{y}+cz/x^2$ | 144.84 | 109.58 | 0.745 | 0.0883 | 0.0683 | 0.6151 | 0.2628 | 0.1898 | 0.707 |
| $a+bx/\sqrt{y}+cz^2/x^2$ | 143.84 | 109.17 | 0.748 | 0.0880 | 0.0682 | 0.6173 | 0.2620 | 0.1893 | 0.709 |
| $a+bx/\sqrt{y}+c\sqrt{z}/x^2$ | 144.48 | 109.59 | 0.746 | 0.0882 | 0.0682 | 0.6163 | 0.2624 | 0.1895 | 0.708 |
| $a+bx/\sqrt{y}+c/\sqrt{x}z$ | 187.17 | 137.66 | 0.574 | 0.0946 | 0.0748 | 0.5581 | 0.2938 | 0.2140 | 0.634 |
| $a+bx/\sqrt{y}+c/\sqrt{x}z^2$ | 181.93 | 132.00 | 0.597 | 0.0945 | 0.0743 | 0.5595 | 0.2914 | 0.2084 | 0.640 |
| $a+bx/\sqrt{y}+c/\sqrt{x}\sqrt{z}$ | 178.33 | 136.65 | 0.613 | 0.0926 | 0.0734 | 0.5764 | 0.2861 | 0.2171 | 0.653 |
| $a+bx/\sqrt{y}+cz/\sqrt{x}$ | 110.60 | 82.01 | 0.851 | 0.0722 | 0.0528 | 0.7428 | 0.2258 | 0.1526 | 0.784 |
| $a+bx/\sqrt{y}+cz^2/\sqrt{x}$ | 115.31 | 88.36 | 0.838 | 0.0669 | 0.0438 | 0.7787 | 0.2241 | 0.1470 | 0.787 |
| $a+bx/\sqrt{y}+c\sqrt{z}/\sqrt{x}$ | 122.81 | 95.42 | 0.816 | 0.0791 | 0.0601 | 0.6914 | 0.2394 | 0.1675 | 0.757 |
| $a+bx/\sqrt{y}+cy/z$ | 157.37 | 124.65 | 0.699 | 0.0832 | 0.0626 | 0.6580 | 0.2639 | 0.1925 | 0.705 |
| $a+bx/\sqrt{y}+cy/z^2$ | 166.56 | 126.23 | 0.662 | 0.0891 | 0.0696 | 0.6083 | 0.2769 | 0.2001 | 0.675 |
| $a+bx/\sqrt{y}+cy/\sqrt{z}$ | 171.69 | 130.87 | 0.641 | 0.0861 | 0.0651 | 0.6339 | 0.2739 | 0.2038 | 0.682 |
| $a+bx/\sqrt{y}+cyz$ | 120.55 | 87.39 | 0.823 | 0.0698 | 0.0453 | 0.7592 | 0.2346 | 0.1499 | 0.767 |
| $a+bx/\sqrt{y}+cyz^2$ | 123.22 | 91.16 | 0.815 | 0.0695 | 0.0467 | 0.7616 | 0.2353 | 0.1580 | 0.765 |
| $a+bx/\sqrt{y}+cy\sqrt{z}$ | 125.52 | 93.51 | 0.808 | 0.0739 | 0.0483 | 0.7303 | 0.2419 | 0.1478 | 0.752 |
| $a+bx/\sqrt{y}+cy^2/z$ | 175.07 | 130.53 | 0.627 | 0.0872 | 0.0658 | 0.6241 | 0.2777 | 0.2054 | 0.673 |
| $a+bx/\sqrt{y}+cy^2/z^2$ | 168.93 | 128.13 | 0.653 | 0.0883 | 0.0684 | 0.6146 | 0.2774 | 0.2018 | 0.674 |
| $a+bx/\sqrt{y}+cy^2/\sqrt{z}$ | 186.95 | 138.57 | 0.575 | 0.0943 | 0.0745 | 0.5607 | 0.2936 | 0.2133 | 0.635 |
| $a+bx/\sqrt{y}+cy^2z$ | 123.48 | 91.46 | 0.814 | 0.0725 | 0.0492 | 0.7403 | 0.2411 | 0.1581 | 0.754 |
| $a+bx/\sqrt{y}+cy^2z^2$ | 124.71 | 93.55 | 0.811 | 0.0718 | 0.0499 | 0.7457 | 0.2402 | 0.1651 | 0.756 |
| $a+bx/\sqrt{y}+cy^2\sqrt{z}$ | 128.67 | 96.32 | 0.799 | 0.0762 | 0.0524 | 0.7136 | 0.2479 | 0.1587 | 0.740 |
| $a+bx/\sqrt{y}+c\sqrt{y}/z$ | 150.66 | 116.98 | 0.724 | 0.0831 | 0.0632 | 0.6590 | 0.2603 | 0.1845 | 0.713 |
| $a+bx/\sqrt{y}+c\sqrt{y}/z^2$ | 166.08 | 125.82 | 0.664 | 0.0898 | 0.0704 | 0.6018 | 0.2775 | 0.1998 | 0.674 |
| $a+bx/\sqrt{y}+c\sqrt{y}/\sqrt{z}$ | 150.60 | 121.37 | 0.724 | 0.0804 | 0.0593 | 0.6809 | 0.2560 | 0.1857 | 0.722 |
| $a+bx/\sqrt{y}+c\sqrt{y}z$ | 119.48 | 87.25 | 0.826 | 0.0685 | 0.0421 | 0.7687 | 0.2309 | 0.1444 | 0.774 |
| $a+bx/\sqrt{y}+c\sqrt{y}z^2$ | 122.98 | 91.22 | 0.816 | 0.0684 | 0.0449 | 0.7688 | 0.2329 | 0.1562 | 0.770 |
| $a+bx/\sqrt{y}+c\sqrt{y}\sqrt{z}$ | 122.11 | 90.26 | 0.819 | 0.0717 | 0.0453 | 0.7459 | 0.2360 | 0.1419 | 0.764 |
| $a+bx/\sqrt{y}+c/yz$ | 183.13 | 134.82 | 0.592 | 0.0946 | 0.0748 | 0.5583 | 0.2920 | 0.2112 | 0.639 |
| $a+bx/\sqrt{y}+c/yz^2$ | 180.12 | 133.55 | 0.605 | 0.0945 | 0.0746 | 0.5593 | 0.2906 | 0.2096 | 0.642 |
| $a+bx/\sqrt{y}+c/y\sqrt{z}$ | 186.77 | 136.44 | 0.576 | 0.0945 | 0.0746 | 0.5586 | 0.2938 | 0.2139 | 0.634 |
| $a+bx/\sqrt{y}+cz/y$ | 134.87 | 105.49 | 0.779 | 0.0757 | 0.0560 | 0.7168 | 0.2400 | 0.1699 | 0.756 |
| $a+bx/\sqrt{y}+cz^2/y$ | 124.80 | 98.26 | 0.810 | 0.0683 | 0.0468 | 0.7695 | 0.2285 | 0.1555 | 0.779 |
| $a+bx/\sqrt{y}+c\sqrt{z}/y$ | 155.80 | 123.49 | 0.705 | 0.0836 | 0.0616 | 0.6545 | 0.2609 | 0.1887 | 0.712 |
| $a+bx/\sqrt{y}+c/y^2z$ | 184.90 | 138.44 | 0.584 | 0.0917 | 0.0728 | 0.5845 | 0.2894 | 0.2183 | 0.645 |
| $a+bx/\sqrt{y}+c/y^2z^2$ | 187.23 | 137.85 | 0.573 | 0.0936 | 0.0735 | 0.5673 | 0.2934 | 0.2165 | 0.635 |
| $a+bx/\sqrt{y}+c/y^2\sqrt{z}$ | 179.05 | 135.84 | 0.610 | 0.0899 | 0.0708 | 0.6011 | 0.2834 | 0.2142 | 0.660 |
| $a+bx/\sqrt{y}+cz/y^2$ | 146.66 | 115.06 | 0.738 | 0.0837 | 0.0620 | 0.6541 | 0.2561 | 0.1760 | 0.722 |
| $a+bx/\sqrt{y}+cz^2/y^2$ | 130.39 | 98.20 | 0.793 | 0.0764 | 0.0575 | 0.7117 | 0.2379 | 0.1682 | 0.760 |
| $a+bx/\sqrt{y}+c\sqrt{z}/y^2$ | 156.61 | 124.19 | 0.702 | 0.0857 | 0.0628 | 0.6374 | 0.2646 | 0.1877 | 0.703 |
| $a+bx/\sqrt{y}+c/\sqrt{y}z$ | 165.10 | 123.08 | 0.668 | 0.0910 | 0.0710 | 0.5910 | 0.2774 | 0.1990 | 0.674 |
| $a+bx/\sqrt{y}+c/\sqrt{y}z^2$ | 172.13 | 129.09 | 0.640 | 0.0930 | 0.0727 | 0.5731 | 0.2844 | 0.2070 | 0.657 |
| $a+bx/\sqrt{y}+c/\sqrt{y}\sqrt{z}$ | 166.14 | 117.81 | 0.664 | 0.0906 | 0.0695 | 0.5946 | 0.2774 | 0.1926 | 0.674 |
| $a+bx/\sqrt{y}+cz/\sqrt{y}$ | 124.68 | 99.61 | 0.811 | 0.0700 | 0.0494 | 0.7582 | 0.2300 | 0.1566 | 0.776 |
| $a+bx/\sqrt{y}+cz^2/\sqrt{y}$ | 123.86 | 96.13 | 0.813 | 0.0674 | 0.0450 | 0.7759 | 0.2290 | 0.1561 | 0.778 |
| $a+bx/\sqrt{y}+c\sqrt{z}/\sqrt{y}$ | 138.92 | 111.29 | 0.765 | 0.0764 | 0.0557 | 0.7116 | 0.2435 | 0.1743 | 0.749 |
| $a+bxy+cx/z$ | 133.84 | 105.90 | 0.782 | 0.0831 | 0.0581 | 0.6589 | 0.2781 | 0.1944 | 0.672 |
| $a+bxy+cx/z^2$ | 135.81 | 108.86 | 0.776 | 0.0840 | 0.0582 | 0.6515 | 0.2782 | 0.1937 | 0.672 |
| $a+bxy+cx/\sqrt{z}$ | 135.75 | 105.60 | 0.776 | 0.0837 | 0.0584 | 0.6544 | 0.2786 | 0.1916 | 0.671 |
| $a+bxy+cxz$ | 120.76 | 92.01 | 0.823 | 0.0726 | 0.0504 | 0.7396 | 0.2592 | 0.1858 | 0.715 |
| $a+bxy+cxz^2$ | 125.51 | 96.72 | 0.808 | 0.0767 | 0.0555 | 0.7095 | 0.2692 | 0.1912 | 0.693 |
| $a+bxy+cx\sqrt{z}$ | 117.04 | 90.50 | 0.833 | 0.0686 | 0.0444 | 0.7676 | 0.2415 | 0.1613 | 0.753 |
| $a+bxy+cx^2/z$ | 136.12 | 106.47 | 0.775 | 0.0831 | 0.0579 | 0.6587 | 0.2786 | 0.1925 | 0.671 |
| $a+bxy+cx^2/z^2$ | 136.92 | 109.07 | 0.772 | 0.0840 | 0.0582 | 0.6518 | 0.2786 | 0.1928 | 0.671 |
| $a+bxy+cx^2/\sqrt{z}$ | 138.54 | 108.18 | 0.766 | 0.0841 | 0.0575 | 0.6511 | 0.2776 | 0.1913 | 0.673 |
| $a+bxy+cx^2z$ | 126.03 | 99.10 | 0.807 | 0.0771 | 0.0568 | 0.7061 | 0.2701 | 0.1934 | 0.691 |
| $a+bxy+cx^2z^2$ | 128.62 | 100.82 | 0.799 | 0.0793 | 0.0580 | 0.6894 | 0.2740 | 0.1932 | 0.682 |
| $a+bxy+cx^2\sqrt{z}$ | 122.86 | 96.77 | 0.816 | 0.0751 | 0.0553 | 0.7217 | 0.2640 | 0.1932 | 0.705 |
| $a+bxy+c\sqrt{x}/z$ | 130.65 | 103.65 | 0.792 | 0.0827 | 0.0576 | 0.6620 | 0.2762 | 0.1946 | 0.677 |
| $a+bxy+c\sqrt{x}/z^2$ | 134.35 | 108.11 | 0.780 | 0.0839 | 0.0581 | 0.6521 | 0.2774 | 0.1938 | 0.674 |
| $a+bxy+c\sqrt{x}/\sqrt{z}$ | 131.65 | 102.88 | 0.789 | 0.0830 | 0.0582 | 0.6602 | 0.2779 | 0.1951 | 0.673 |
| $a+bxy+c\sqrt{x}z$ | 119.50 | 91.31 | 0.826 | 0.0714 | 0.0468 | 0.7484 | 0.2546 | 0.1779 | 0.725 |
| $a+bxy+c\sqrt{x}z^2$ | 123.96 | 94.62 | 0.813 | 0.0754 | 0.0536 | 0.7194 | 0.2662 | 0.1889 | 0.700 |
| $a+bxy+c\sqrt{x}\sqrt{z}$ | 119.93 | 91.41 | 0.825 | 0.0695 | 0.0418 | 0.7613 | 0.2401 | 0.1497 | 0.756 |
| $a+bxy+c/xz$ | 137.78 | 108.04 | 0.769 | 0.0843 | 0.0575 | 0.6494 | 0.2759 | 0.1888 | 0.677 |
| $a+bxy+c/xz^2$ | 139.41 | 110.84 | 0.764 | 0.0842 | 0.0578 | 0.6497 | 0.2736 | 0.1839 | 0.683 |
| $a+bxy+c/x\sqrt{z}$ | 136.28 | 105.51 | 0.774 | 0.0843 | 0.0575 | 0.6489 | 0.2771 | 0.1906 | 0.675 |
| $a+bxy+cz/x$ | 130.11 | 96.65 | 0.794 | 0.0843 | 0.0577 | 0.6490 | 0.2786 | 0.1931 | 0.671 |
| $a+bxy+cz^2/x$ | 122.03 | 91.44 | 0.819 | 0.0823 | 0.0570 | 0.6655 | 0.2752 | 0.1950 | 0.679 |
| $a+bxy+c\sqrt{z}/x$ | 132.66 | 99.70 | 0.786 | 0.0844 | 0.0573 | 0.6481 | 0.2785 | 0.1922 | 0.671 |
| $a+bxy+c/x^2z$ | 133.21 | 100.65 | 0.784 | 0.0844 | 0.0572 | 0.6482 | 0.2784 | 0.1923 | 0.672 |
| $a+bxy+c/x^2z^2$ | 134.72 | 102.94 | 0.779 | 0.0844 | 0.0572 | 0.6483 | 0.2781 | 0.1919 | 0.672 |
| $a+bxy+c/x^2\sqrt{z}$ | 132.70 | 99.90 | 0.786 | 0.0844 | 0.0572 | 0.6482 | 0.2785 | 0.1923 | 0.671 |
| $a+bxy+cz/x^2$ | 131.66 | 98.39 | 0.789 | 0.0844 | 0.0571 | 0.6481 | 0.2786 | 0.1921 | 0.671 |
| $a+bxy+cz^2/x^2$ | 130.96 | 97.49 | 0.791 | 0.0844 | 0.0573 | 0.6481 | 0.2787 | 0.1920 | 0.671 |
| $a+bxy+c\sqrt{z}/x^2$ | 131.96 | 98.83 | 0.788 | 0.0844 | 0.0572 | 0.6482 | 0.2786 | 0.1922 | 0.671 |
| $a+bxy+c/\sqrt{x}z$ | 138.56 | 109.13 | 0.766 | 0.0833 | 0.0584 | 0.6577 | 0.2673 | 0.1758 | 0.697 |
| $a+bxy+c/\sqrt{x}z^2$ | 135.45 | 105.78 | 0.777 | 0.0838 | 0.0581 | 0.6530 | 0.2702 | 0.1773 | 0.691 |
| $a+bxy+c/\sqrt{x}\sqrt{z}$ | 139.35 | 110.76 | 0.764 | 0.0836 | 0.0582 | 0.6549 | 0.2710 | 0.1819 | 0.689 |
| $a+bxy+cz/\sqrt{x}$ | 121.39 | 92.55 | 0.821 | 0.0813 | 0.0564 | 0.6733 | 0.2736 | 0.1946 | 0.683 |

(continued on next page)

**Table 4 – continued from previous page**

| Functional form | $T_{eff}$ (K) | | | Radius ($R_\odot$) | | | log (L/$L_\odot$) | | |
|---|---|---|---|---|---|---|---|---|---|
| | RMSE | MAD | $R^2_{ap}$ | RMSE | MAD | $R^2_{ap}$ | RMSE | MAD | $R^2_{ap}$ |
| a+bxy+c$z^2/\sqrt{x}$ | 118.66 | 89.53 | 0.829 | 0.0759 | 0.0528 | 0.7155 | 0.2649 | 0.1873 | 0.703 |
| a+bxy+c$\sqrt{z}/\sqrt{x}$ | 129.56 | 96.73 | 0.796 | 0.0840 | 0.0581 | 0.6517 | 0.2784 | 0.1943 | 0.671 |
| a+bxy+cy/z | 127.62 | 100.67 | 0.802 | 0.0807 | 0.0568 | 0.6786 | 0.2720 | 0.1926 | 0.686 |
| a+bxy+cy/$z^2$ | 133.60 | 106.85 | 0.783 | 0.0835 | 0.0583 | 0.6557 | 0.2765 | 0.1936 | 0.676 |
| a+bxy+cy/$\sqrt{z}$ | 125.54 | 97.94 | 0.808 | 0.0791 | 0.0563 | 0.6912 | 0.2706 | 0.1938 | 0.690 |
| a+bxy+cyz | 126.89 | 96.31 | 0.804 | 0.0771 | 0.0530 | 0.7067 | 0.2701 | 0.1857 | 0.691 |
| a+bxy+cy$z^2$ | 127.72 | 96.86 | 0.802 | 0.0782 | 0.0554 | 0.6983 | 0.2722 | 0.1900 | 0.686 |
| a+bxy+cy$\sqrt{z}$ | 129.78 | 99.10 | 0.795 | 0.0783 | 0.0501 | 0.6972 | 0.2706 | 0.1785 | 0.690 |
| a+bxy+c$y^2$/z | 126.01 | 99.46 | 0.807 | 0.0783 | 0.0553 | 0.6973 | 0.2686 | 0.1894 | 0.694 |
| a+bxy+c$y^2/z^2$ | 133.26 | 105.70 | 0.784 | 0.0828 | 0.0584 | 0.6613 | 0.2761 | 0.1937 | 0.677 |
| a+bxy+c$y^2/\sqrt{z}$ | 121.68 | 94.48 | 0.820 | 0.0749 | 0.0533 | 0.7234 | 0.2607 | 0.1861 | 0.712 |
| a+bxy+c$y^2$z | 133.16 | 100.51 | 0.784 | 0.0815 | 0.0569 | 0.6723 | 0.2777 | 0.1908 | 0.673 |
| a+bxy+c$y^2z^2$ | 131.27 | 99.68 | 0.790 | 0.0808 | 0.0576 | 0.6773 | 0.2766 | 0.1911 | 0.676 |
| a+bxy+c$y^2\sqrt{z}$ | 137.07 | 104.64 | 0.771 | 0.0835 | 0.0571 | 0.6558 | 0.2785 | 0.1925 | 0.671 |
| a+bxy+c$\sqrt{y}$/z | 126.88 | 99.91 | 0.804 | 0.0812 | 0.0564 | 0.6745 | 0.2710 | 0.1898 | 0.689 |
| a+bxy+c$\sqrt{y}/z^2$ | 133.13 | 106.93 | 0.784 | 0.0837 | 0.0580 | 0.6544 | 0.2759 | 0.1924 | 0.677 |
| a+bxy+c$\sqrt{y}/\sqrt{z}$ | 124.26 | 97.57 | 0.812 | 0.0795 | 0.0557 | 0.6878 | 0.2698 | 0.1919 | 0.692 |
| a+bxy+c$\sqrt{y}$z | 122.37 | 93.97 | 0.818 | 0.0744 | 0.0499 | 0.7266 | 0.2627 | 0.1819 | 0.707 |
| a+bxy+c$\sqrt{y}z^2$ | 125.19 | 95.49 | 0.809 | 0.0764 | 0.0539 | 0.7119 | 0.2684 | 0.1883 | 0.695 |
| a+bxy+c$\sqrt{y}\sqrt{z}$ | 123.42 | 95.16 | 0.815 | 0.0748 | 0.0449 | 0.7234 | 0.2593 | 0.1671 | 0.715 |
| a+bxy+c/yz | 136.73 | 106.54 | 0.773 | 0.0839 | 0.0579 | 0.6526 | 0.2690 | 0.1764 | 0.693 |
| a+bxy+c/y$z^2$ | 134.23 | 104.02 | 0.781 | 0.0841 | 0.0581 | 0.6507 | 0.2714 | 0.1788 | 0.688 |
| a+bxy+c/y$\sqrt{z}$ | 138.97 | 110.36 | 0.765 | 0.0841 | 0.0578 | 0.6510 | 0.2712 | 0.1773 | 0.688 |
| a+bxy+cz/y | 117.34 | 89.22 | 0.832 | 0.0785 | 0.0544 | 0.6958 | 0.2671 | 0.1932 | 0.698 |
| a+bxy+c$z^2$/y | 114.61 | 85.53 | 0.840 | 0.0729 | 0.0497 | 0.7374 | 0.2564 | 0.1832 | 0.721 |
| a+bxy+c$\sqrt{z}$/y | 128.85 | 96.85 | 0.798 | 0.0829 | 0.0586 | 0.6610 | 0.2773 | 0.1971 | 0.674 |
| a+bxy+c/$y^2$z | 139.16 | 110.66 | 0.764 | 0.0843 | 0.0573 | 0.6490 | 0.2733 | 0.1795 | 0.683 |
| a+bxy+c/$y^2z^2$ | 137.44 | 108.01 | 0.770 | 0.0843 | 0.0574 | 0.6489 | 0.2728 | 0.1791 | 0.685 |
| a+bxy+c/$y^2\sqrt{z}$ | 139.38 | 110.70 | 0.764 | 0.0844 | 0.0571 | 0.6487 | 0.2746 | 0.1830 | 0.681 |
| a+bxy+cz/$y^2$ | 130.95 | 97.99 | 0.791 | 0.0840 | 0.0584 | 0.6519 | 0.2785 | 0.1943 | 0.671 |
| a+bxy+c$z^2/y^2$ | 116.69 | 88.76 | 0.834 | 0.0797 | 0.0553 | 0.6863 | 0.2690 | 0.1951 | 0.693 |
| a+bxy+c$\sqrt{z}/y^2$ | 135.72 | 104.15 | 0.776 | 0.0844 | 0.0578 | 0.6484 | 0.2782 | 0.1909 | 0.672 |
| a+bxy+c/$\sqrt{y}$z | 131.41 | 101.96 | 0.790 | 0.0829 | 0.0575 | 0.6608 | 0.2654 | 0.1702 | 0.702 |
| a+bxy+c/$\sqrt{y}z^2$ | 132.48 | 104.98 | 0.786 | 0.0839 | 0.0582 | 0.6522 | 0.2724 | 0.1836 | 0.686 |
| a+bxy+c/$\sqrt{y}\sqrt{z}$ | 134.71 | 103.51 | 0.779 | 0.0827 | 0.0572 | 0.6620 | 0.2641 | 0.1692 | 0.704 |
| a+bxy+cz/$\sqrt{y}$ | 114.14 | 87.12 | 0.841 | 0.0740 | 0.0492 | 0.7298 | 0.2570 | 0.1799 | 0.720 |
| a+bxy+c$z^2/\sqrt{y}$ | 118.48 | 89.60 | 0.829 | 0.0731 | 0.0502 | 0.7364 | 0.2589 | 0.1849 | 0.716 |
| a+bxy+c$\sqrt{z}/\sqrt{y}$ | 118.83 | 90.79 | 0.828 | 0.0783 | 0.0542 | 0.6969 | 0.2671 | 0.1923 | 0.698 |
| a+bx$y^2$+cx/z | 149.97 | 112.97 | 0.726 | 0.0909 | 0.0676 | 0.5924 | 0.3119 | 0.2283 | 0.588 |
| a+bx$y^2$+cx/$z^2$ | 148.94 | 113.62 | 0.730 | 0.0908 | 0.0675 | 0.5927 | 0.3117 | 0.2305 | 0.588 |
| a+bx$y^2$+cx/$\sqrt{z}$ | 151.36 | 117.25 | 0.721 | 0.0909 | 0.0657 | 0.5920 | 0.3049 | 0.2186 | 0.606 |
| a+bx$y^2$+cxz | 125.79 | 94.99 | 0.807 | 0.0733 | 0.0528 | 0.7347 | 0.2703 | 0.2077 | 0.691 |
| a+bx$y^2$+cx$z^2$ | 138.13 | 104.95 | 0.768 | 0.0820 | 0.0607 | 0.6684 | 0.2972 | 0.2246 | 0.626 |
| a+bx$y^2$+cx$\sqrt{z}$ | 117.09 | 90.50 | 0.833 | 0.0680 | 0.0433 | 0.7715 | 0.2372 | 0.1575 | 0.762 |
| a+bx$y^2$+c$x^2$/z | 151.43 | 115.91 | 0.721 | 0.0911 | 0.0670 | 0.5902 | 0.3090 | 0.2268 | 0.595 |
| a+bx$y^2$+c$x^2/z^2$ | 150.53 | 114.31 | 0.724 | 0.0910 | 0.0674 | 0.5912 | 0.3119 | 0.2286 | 0.588 |
| a+bx$y^2$+c$x^2/\sqrt{z}$ | 148.76 | 117.41 | 0.731 | 0.0898 | 0.0651 | 0.6016 | 0.2942 | 0.2142 | 0.633 |
| a+bx$y^2$+c$x^2$z | 134.69 | 103.29 | 0.779 | 0.0797 | 0.0607 | 0.6866 | 0.2906 | 0.2260 | 0.642 |
| a+bx$y^2$+c$x^2z^2$ | 142.92 | 110.88 | 0.751 | 0.0856 | 0.0643 | 0.6379 | 0.3054 | 0.2256 | 0.605 |
| a+bx$y^2$+c$x^2\sqrt{z}$ | 123.83 | 95.46 | 0.813 | 0.0730 | 0.0562 | 0.7371 | 0.2644 | 0.2034 | 0.704 |
| a+bx$y^2$+c$\sqrt{x}$/z | 145.52 | 109.28 | 0.742 | 0.0899 | 0.0673 | 0.6005 | 0.3103 | 0.2304 | 0.592 |
| a+bx$y^2$+c$\sqrt{x}/z^2$ | 146.28 | 111.90 | 0.740 | 0.0905 | 0.0673 | 0.5960 | 0.3098 | 0.2303 | 0.593 |
| a+bx$y^2$+c$\sqrt{x}/\sqrt{z}$ | 149.81 | 111.88 | 0.727 | 0.0910 | 0.0675 | 0.5913 | 0.3115 | 0.2269 | 0.589 |
| a+bx$y^2$+c$\sqrt{x}$z | 124.12 | 94.98 | 0.813 | 0.0724 | 0.0493 | 0.7413 | 0.2655 | 0.1990 | 0.701 |
| a+bx$y^2$+c$\sqrt{x}z^2$ | 135.77 | 102.64 | 0.776 | 0.0802 | 0.0593 | 0.6822 | 0.2927 | 0.2237 | 0.637 |
| a+bx$y^2$+c$\sqrt{x}\sqrt{z}$ | 119.67 | 91.71 | 0.826 | 0.0695 | 0.0424 | 0.7615 | 0.2400 | 0.1476 | 0.756 |
| a+bx$y^2$+c/xz | 150.01 | 116.44 | 0.726 | 0.0878 | 0.0626 | 0.6190 | 0.2930 | 0.2030 | 0.636 |
| a+bx$y^2$+c/x$z^2$ | 145.93 | 112.21 | 0.741 | 0.0875 | 0.0620 | 0.6223 | 0.2870 | 0.1926 | 0.651 |
| a+bx$y^2$+c/x$\sqrt{z}$ | 151.06 | 117.03 | 0.722 | 0.0884 | 0.0633 | 0.6143 | 0.2972 | 0.2077 | 0.626 |
| a+bx$y^2$+cz/x | 150.19 | 112.21 | 0.726 | 0.0906 | 0.0650 | 0.5950 | 0.3087 | 0.2182 | 0.596 |
| a+bx$y^2$+c$z^2$/x | 144.06 | 108.62 | 0.747 | 0.0906 | 0.0671 | 0.5945 | 0.3117 | 0.2298 | 0.588 |
| a+bx$y^2$+c$\sqrt{z}$/x | 151.19 | 114.88 | 0.722 | 0.0898 | 0.0639 | 0.6018 | 0.3053 | 0.2152 | 0.605 |
| a+bx$y^2$+c/$x^2$z | 151.26 | 115.23 | 0.722 | 0.0896 | 0.0640 | 0.6040 | 0.3047 | 0.2149 | 0.607 |
| a+bx$y^2$+c/$x^2z^2$ | 151.44 | 116.48 | 0.721 | 0.0892 | 0.0637 | 0.6070 | 0.3020 | 0.2118 | 0.614 |
| a+bx$y^2$+c/$x^2\sqrt{z}$ | 151.10 | 114.66 | 0.722 | 0.0897 | 0.0641 | 0.6029 | 0.3057 | 0.2157 | 0.604 |
| a+bx$y^2$+cz/$x^2$ | 150.61 | 113.45 | 0.724 | 0.0900 | 0.0641 | 0.6003 | 0.3074 | 0.2169 | 0.599 |
| a+bx$y^2$+c$z^2/x^2$ | 150.25 | 112.64 | 0.725 | 0.0902 | 0.0643 | 0.5984 | 0.3084 | 0.2173 | 0.597 |
| a+bx$y^2$+c$\sqrt{z}/x^2$ | 150.76 | 113.82 | 0.723 | 0.0899 | 0.0641 | 0.6011 | 0.3070 | 0.2166 | 0.601 |
| a+bx$y^2$+c/$\sqrt{x}$z | 140.34 | 107.78 | 0.760 | 0.0846 | 0.0603 | 0.6464 | 0.2740 | 0.1799 | 0.682 |
| a+bx$y^2$+c/$\sqrt{x}z^2$ | 136.82 | 106.90 | 0.772 | 0.0871 | 0.0631 | 0.6253 | 0.2845 | 0.1895 | 0.657 |
| a+bx$y^2$+c/$\sqrt{x}\sqrt{z}$ | 145.94 | 112.61 | 0.741 | 0.0853 | 0.0604 | 0.6403 | 0.2802 | 0.1892 | 0.667 |
| a+bx$y^2$+cz/$\sqrt{x}$ | 142.10 | 108.08 | 0.754 | 0.0898 | 0.0666 | 0.6022 | 0.3105 | 0.2297 | 0.592 |
| a+bx$y^2$+c$z^2/\sqrt{x}$ | 133.57 | 99.07 | 0.783 | 0.0826 | 0.0597 | 0.6629 | 0.2964 | 0.2201 | 0.628 |
| a+bx$y^2$+c$\sqrt{z}/\sqrt{x}$ | 150.05 | 111.47 | 0.726 | 0.0909 | 0.0658 | 0.5918 | 0.3095 | 0.2204 | 0.594 |
| a+bx$y^2$+cy/z | 143.34 | 107.80 | 0.750 | 0.0884 | 0.0660 | 0.6143 | 0.3075 | 0.2276 | 0.599 |
| a+bx$y^2$+cy/$z^2$ | 145.84 | 111.23 | 0.741 | 0.0901 | 0.0672 | 0.5994 | 0.3091 | 0.2296 | 0.595 |
| a+bx$y^2$+cy/$\sqrt{z}$ | 146.31 | 109.21 | 0.740 | 0.0891 | 0.0669 | 0.6081 | 0.3106 | 0.2303 | 0.591 |
| a+bx$y^2$+cyz | 134.24 | 101.97 | 0.781 | 0.0790 | 0.0567 | 0.6922 | 0.2880 | 0.2176 | 0.649 |
| a+bx$y^2$+cy$z^2$ | 141.12 | 106.55 | 0.758 | 0.0839 | 0.0613 | 0.6521 | 0.3020 | 0.2214 | 0.613 |
| a+bx$y^2$+cy$\sqrt{z}$ | 131.27 | 100.74 | 0.790 | 0.0772 | 0.0470 | 0.7060 | 0.2724 | 0.1822 | 0.686 |
| a+bx$y^2$+c$y^2$/z | 144.84 | 109.31 | 0.745 | 0.0879 | 0.0657 | 0.6188 | 0.3083 | 0.2279 | 0.597 |
| a+bx$y^2$+c$y^2/z^2$ | 147.07 | 111.74 | 0.737 | 0.0899 | 0.0674 | 0.6008 | 0.3101 | 0.2301 | 0.592 |
| a+bx$y^2$+c$y^2/\sqrt{z}$ | 145.94 | 109.80 | 0.741 | 0.0880 | 0.0661 | 0.6180 | 0.3094 | 0.2291 | 0.594 |
| a+bx$y^2$+c$y^2$z | 144.59 | 107.05 | 0.746 | 0.0860 | 0.0626 | 0.6349 | 0.3067 | 0.2202 | 0.601 |
| a+bx$y^2$+c$y^2z^2$ | 146.16 | 110.09 | 0.740 | 0.0877 | 0.0651 | 0.6206 | 0.3094 | 0.2254 | 0.594 |
| a+bx$y^2$+c$y^2\sqrt{z}$ | 144.48 | 104.50 | 0.746 | 0.0856 | 0.0599 | 0.6384 | 0.3040 | 0.2135 | 0.608 |
| a+bx$y^2$+c$\sqrt{y}$/z | 138.91 | 104.34 | 0.765 | 0.0875 | 0.0645 | 0.6221 | 0.3021 | 0.2215 | 0.613 |
| a+bx$y^2$+c$\sqrt{y}/z^2$ | 143.72 | 109.78 | 0.749 | 0.0898 | 0.0668 | 0.6017 | 0.3068 | 0.2272 | 0.601 |
| a+bx$y^2$+c$\sqrt{y}/\sqrt{z}$ | 141.31 | 107.40 | 0.757 | 0.0876 | 0.0652 | 0.6207 | 0.3062 | 0.2268 | 0.603 |
| a+bx$y^2$+c$\sqrt{y}$z | 128.82 | 99.05 | 0.798 | 0.0763 | 0.0532 | 0.7127 | 0.2783 | 0.2098 | 0.672 |
| a+bx$y^2$+c$\sqrt{y}z^2$ | 137.65 | 103.36 | 0.769 | 0.0816 | 0.0597 | 0.6711 | 0.2963 | 0.2231 | 0.628 |

(continued on next page)

**Table 4 – continued from previous page**

| Functional form | $T_{eff}$ (K) | | | Radius ($R_{\odot}$) | | | log (L/$L_{\odot}$) | | |
|---|---|---|---|---|---|---|---|---|---|
| | RMSE | MAD | $R^2_{ap}$ | RMSE | MAD | $R^2_{ap}$ | RMSE | MAD | $R^2_{ap}$ |
| $a+bxy^2+c\sqrt{y}\sqrt{z}$ | 125.00 | 96.47 | 0.810 | 0.0747 | 0.0440 | 0.7241 | 0.2626 | 0.1734 | 0.708 |
| $a+bxy^2+c/yz$ | 137.18 | 104.57 | 0.771 | 0.0865 | 0.0620 | 0.6306 | 0.2789 | 0.1838 | 0.670 |
| $a+bxy^2+c/yz^2$ | 135.84 | 104.25 | 0.776 | 0.0882 | 0.0644 | 0.6161 | 0.2883 | 0.1980 | 0.648 |
| $a+bxy^2+c/y\sqrt{z}$ | 142.01 | 109.69 | 0.755 | 0.0867 | 0.0606 | 0.6292 | 0.2809 | 0.1840 | 0.666 |
| $a+bxy^2+cz/y$ | 138.41 | 106.30 | 0.767 | 0.0876 | 0.0650 | 0.6212 | 0.3062 | 0.2279 | 0.603 |
| $a+bxy^2+cz^2/y$ | 127.75 | 93.75 | 0.801 | 0.0790 | 0.0561 | 0.6916 | 0.2860 | 0.2171 | 0.653 |
| $a+bxy^2+c\sqrt{z}/y$ | 150.19 | 112.17 | 0.726 | 0.0911 | 0.0669 | 0.5902 | 0.3107 | 0.2231 | 0.591 |
| $a+bxy^2+c/y^2z$ | 143.85 | 110.97 | 0.748 | 0.0881 | 0.0624 | 0.6171 | 0.2876 | 0.1888 | 0.650 |
| $a+bxy^2+c/y^2z^2$ | 140.28 | 105.41 | 0.761 | 0.0886 | 0.0641 | 0.6124 | 0.2894 | 0.1969 | 0.645 |
| $a+bxy^2+c/y^2\sqrt{z}$ | 146.55 | 113.94 | 0.739 | 0.0881 | 0.0614 | 0.6164 | 0.2894 | 0.1901 | 0.645 |
| $a+bxy^2+cz/y^2$ | 150.96 | 114.16 | 0.723 | 0.0908 | 0.0652 | 0.5931 | 0.3080 | 0.2154 | 0.598 |
| $a+bxy^2+cz^2/y^2$ | 139.40 | 107.09 | 0.764 | 0.0889 | 0.0662 | 0.6100 | 0.3085 | 0.2301 | 0.597 |
| $a+bxy^2+c\sqrt{z}/y^2$ | 151.20 | 117.22 | 0.722 | 0.0897 | 0.0628 | 0.6030 | 0.3008 | 0.2071 | 0.617 |
| $a+bxy^2+c/\sqrt{y}z$ | 130.76 | 101.49 | 0.792 | 0.0851 | 0.0606 | 0.6422 | 0.2760 | 0.1806 | 0.677 |
| $a+bxy^2+c/\sqrt{y}z^2$ | 136.22 | 106.31 | 0.774 | 0.0885 | 0.0640 | 0.6134 | 0.2935 | 0.2070 | 0.635 |
| $a+bxy^2+c/\sqrt{y}\sqrt{z}$ | 133.47 | 102.90 | 0.783 | 0.0839 | 0.0582 | 0.6523 | 0.2698 | 0.1697 | 0.692 |
| $a+bxy^2+cz/\sqrt{y}$ | 126.59 | 94.32 | 0.805 | 0.0799 | 0.0557 | 0.6852 | 0.2859 | 0.2106 | 0.654 |
| $a+bxy^2+cz^2/\sqrt{y}$ | 130.03 | 95.90 | 0.794 | 0.0782 | 0.0563 | 0.6982 | 0.2853 | 0.2191 | 0.655 |
| $a+bxy^2+c\sqrt{z}/\sqrt{y}$ | 138.70 | 106.52 | 0.766 | 0.0872 | 0.0647 | 0.6243 | 0.3055 | 0.2269 | 0.604 |
| $a+bx\sqrt{y}+cx/z$ | 127.34 | 101.21 | 0.803 | 0.0791 | 0.0528 | 0.6914 | 0.2589 | 0.1740 | 0.716 |
| $a+bx\sqrt{y}+cx/z^2$ | 132.95 | 104.92 | 0.785 | 0.0813 | 0.0563 | 0.6740 | 0.2613 | 0.1751 | 0.711 |
| $a+bx\sqrt{y}+cx/\sqrt{z}$ | 126.08 | 100.78 | 0.807 | 0.0784 | 0.0525 | 0.6962 | 0.2594 | 0.1750 | 0.715 |
| $a+bx\sqrt{y}+cxz$ | 117.81 | 90.09 | 0.831 | 0.0711 | 0.0484 | 0.7502 | 0.2469 | 0.1662 | 0.742 |
| $a+bx\sqrt{y}+cxz^2$ | 119.65 | 92.36 | 0.826 | 0.0732 | 0.0513 | 0.7355 | 0.2511 | 0.1702 | 0.733 |
| $a+bx\sqrt{y}+cx\sqrt{z}$ | 117.00 | 90.54 | 0.833 | 0.0693 | 0.0444 | 0.7628 | 0.2405 | 0.1589 | 0.755 |
| $a+bx\sqrt{y}+cx^2/z$ | 129.81 | 102.79 | 0.795 | 0.0785 | 0.0515 | 0.6959 | 0.2596 | 0.1739 | 0.714 |
| $a+bx\sqrt{y}+cx^2/z^2$ | 133.78 | 105.36 | 0.782 | 0.0810 | 0.0559 | 0.6759 | 0.2617 | 0.1754 | 0.710 |
| $a+bx\sqrt{y}+cx^2/\sqrt{z}$ | 132.30 | 102.35 | 0.787 | 0.0787 | 0.0507 | 0.6941 | 0.2606 | 0.1723 | 0.712 |
| $a+bx\sqrt{y}+cx^2z$ | 121.15 | 95.26 | 0.821 | 0.0745 | 0.0530 | 0.7262 | 0.2539 | 0.1725 | 0.727 |
| $a+bx\sqrt{y}+cx^2z^2$ | 122.05 | 95.20 | 0.819 | 0.0755 | 0.0534 | 0.7189 | 0.2552 | 0.1729 | 0.724 |
| $a+bx\sqrt{y}+cx^2\sqrt{z}$ | 120.63 | 94.87 | 0.823 | 0.0743 | 0.0530 | 0.7275 | 0.2530 | 0.1727 | 0.729 |
| $a+bx\sqrt{y}+c\sqrt{x}/z$ | 125.25 | 98.53 | 0.809 | 0.0793 | 0.0533 | 0.6898 | 0.2574 | 0.1708 | 0.719 |
| $a+bx\sqrt{y}+c\sqrt{x}/z^2$ | 132.13 | 103.97 | 0.788 | 0.0814 | 0.0566 | 0.6729 | 0.2607 | 0.1744 | 0.712 |
| $a+bx\sqrt{y}+c\sqrt{x}/\sqrt{z}$ | 122.25 | 97.36 | 0.818 | 0.0783 | 0.0524 | 0.6976 | 0.2572 | 0.1723 | 0.720 |
| $a+bx\sqrt{y}+c\sqrt{x}z$ | 117.29 | 89.28 | 0.833 | 0.0701 | 0.0450 | 0.7575 | 0.2434 | 0.1607 | 0.749 |
| $a+bx\sqrt{y}+c\sqrt{x}z^2$ | 118.58 | 90.87 | 0.829 | 0.0721 | 0.0495 | 0.7435 | 0.2487 | 0.1674 | 0.738 |
| $a+bx\sqrt{y}+c\sqrt{x}\sqrt{z}$ | 120.57 | 90.47 | 0.823 | 0.0696 | 0.0414 | 0.7609 | 0.2380 | 0.1479 | 0.760 |
| $a+bx\sqrt{y}+c/xz$ | 128.38 | 99.88 | 0.799 | 0.0816 | 0.0552 | 0.6714 | 0.2622 | 0.1747 | 0.709 |
| $a+bx\sqrt{y}+c/xz^2$ | 135.25 | 107.32 | 0.777 | 0.0816 | 0.0550 | 0.6710 | 0.2625 | 0.1749 | 0.708 |
| $a+bx\sqrt{y}+c/x\sqrt{z}$ | 125.48 | 95.85 | 0.808 | 0.0816 | 0.0553 | 0.6716 | 0.2617 | 0.1741 | 0.710 |
| $a+bx\sqrt{y}+cz/x$ | 117.70 | 86.31 | 0.831 | 0.0807 | 0.0558 | 0.6782 | 0.2587 | 0.1719 | 0.716 |
| $a+bx\sqrt{y}+cz^2/x$ | 108.92 | 80.75 | 0.856 | 0.0774 | 0.0532 | 0.7040 | 0.2521 | 0.1691 | 0.731 |
| $a+bx\sqrt{y}+c\sqrt{z}/x$ | 120.72 | 88.88 | 0.823 | 0.0813 | 0.0557 | 0.6740 | 0.2602 | 0.1714 | 0.713 |
| $a+bx\sqrt{y}+c/x^2z$ | 121.91 | 90.31 | 0.819 | 0.0815 | 0.0556 | 0.6720 | 0.2607 | 0.1718 | 0.712 |
| $a+bx\sqrt{y}+c/x^2z^2$ | 123.40 | 92.87 | 0.815 | 0.0814 | 0.0554 | 0.6729 | 0.2610 | 0.1733 | 0.711 |
| $a+bx\sqrt{y}+c/x^2\sqrt{z}$ | 121.56 | 89.57 | 0.820 | 0.0815 | 0.0557 | 0.6718 | 0.2606 | 0.1712 | 0.712 |
| $a+bx\sqrt{y}+cz/x^2$ | 120.94 | 88.23 | 0.822 | 0.0816 | 0.0558 | 0.6715 | 0.2603 | 0.1700 | 0.713 |
| $a+bx\sqrt{y}+cz^2/x^2$ | 120.23 | 87.68 | 0.824 | 0.0815 | 0.0558 | 0.6721 | 0.2599 | 0.1699 | 0.714 |
| $a+bx\sqrt{y}+c\sqrt{z}/x^2$ | 121.14 | 88.60 | 0.821 | 0.0816 | 0.0557 | 0.6715 | 0.2604 | 0.1703 | 0.713 |
| $a+bx\sqrt{y}+c/\sqrt{x}z$ | 138.18 | 109.55 | 0.768 | 0.0821 | 0.0570 | 0.6671 | 0.2612 | 0.1724 | 0.711 |
| $a+bx\sqrt{y}+c/\sqrt{x}z^2$ | 137.88 | 104.86 | 0.769 | 0.0821 | 0.0571 | 0.6671 | 0.2608 | 0.1720 | 0.712 |
| $a+bx\sqrt{y}+c/\sqrt{x}\sqrt{z}$ | 133.73 | 106.25 | 0.782 | 0.0820 | 0.0565 | 0.6676 | 0.2624 | 0.1748 | 0.708 |
| $a+bx\sqrt{y}+cz/\sqrt{x}$ | 109.64 | 82.53 | 0.854 | 0.0764 | 0.0515 | 0.7116 | 0.2507 | 0.1686 | 0.734 |
| $a+bx\sqrt{y}+cz^2/\sqrt{x}$ | 111.26 | 83.41 | 0.849 | 0.0717 | 0.0474 | 0.7460 | 0.2448 | 0.1623 | 0.746 |
| $a+bx\sqrt{y}+c\sqrt{z}/\sqrt{x}$ | 116.33 | 86.72 | 0.835 | 0.0797 | 0.0549 | 0.6863 | 0.2575 | 0.1732 | 0.719 |
| $a+bx\sqrt{y}+cy/z$ | 122.76 | 95.93 | 0.817 | 0.0770 | 0.0515 | 0.7072 | 0.2525 | 0.1665 | 0.730 |
| $a+bx\sqrt{y}+cy/z^2$ | 131.31 | 102.55 | 0.790 | 0.0809 | 0.0560 | 0.6771 | 0.2596 | 0.1741 | 0.714 |
| $a+bx\sqrt{y}+cy/\sqrt{z}$ | 118.03 | 91.60 | 0.831 | 0.0739 | 0.0498 | 0.7305 | 0.2467 | 0.1643 | 0.742 |
| $a+bx\sqrt{y}+cyz$ | 122.38 | 93.08 | 0.818 | 0.0746 | 0.0492 | 0.7251 | 0.2543 | 0.1671 | 0.726 |
| $a+bx\sqrt{y}+cyz^2$ | 121.33 | 92.98 | 0.821 | 0.0744 | 0.0510 | 0.7268 | 0.2536 | 0.1694 | 0.728 |
| $a+bx\sqrt{y}+cy\sqrt{z}$ | 127.59 | 97.38 | 0.802 | 0.0773 | 0.0485 | 0.7047 | 0.2585 | 0.1687 | 0.717 |
| $a+bx\sqrt{y}+cy^2/z$ | 121.01 | 94.83 | 0.822 | 0.0739 | 0.0490 | 0.7303 | 0.2467 | 0.1622 | 0.742 |
| $a+bx\sqrt{y}+cy^2/z^2$ | 130.24 | 100.87 | 0.794 | 0.0798 | 0.0548 | 0.6854 | 0.2583 | 0.1740 | 0.717 |
| $a+bx\sqrt{y}+cy^2/\sqrt{z}$ | 118.58 | 94.97 | 0.829 | 0.0700 | 0.0465 | 0.7577 | 0.2348 | 0.1550 | 0.766 |
| $a+bx\sqrt{y}+cy^2z$ | 127.20 | 97.49 | 0.803 | 0.0780 | 0.0522 | 0.6995 | 0.2602 | 0.1729 | 0.713 |
| $a+bx\sqrt{y}+cy^2z^2$ | 124.25 | 94.63 | 0.812 | 0.0768 | 0.0526 | 0.7090 | 0.2577 | 0.1714 | 0.719 |
| $a+bx\sqrt{y}+cy^2\sqrt{z}$ | 132.53 | 101.62 | 0.786 | 0.0806 | 0.0538 | 0.6796 | 0.2625 | 0.1746 | 0.708 |
| $a+bx\sqrt{y}+c\sqrt{y}/z$ | 123.66 | 95.63 | 0.814 | 0.0783 | 0.0524 | 0.6972 | 0.2536 | 0.1649 | 0.727 |
| $a+bx\sqrt{y}+c\sqrt{y}/z^2$ | 131.68 | 102.76 | 0.789 | 0.0813 | 0.0567 | 0.6738 | 0.2598 | 0.1737 | 0.714 |
| $a+bx\sqrt{y}+c\sqrt{y}/\sqrt{z}$ | 118.17 | 92.37 | 0.830 | 0.0754 | 0.0499 | 0.7190 | 0.2490 | 0.1642 | 0.737 |
| $a+bx\sqrt{y}+c\sqrt{y}z$ | 118.73 | 90.69 | 0.828 | 0.0723 | 0.0465 | 0.7417 | 0.2486 | 0.1608 | 0.738 |
| $a+bx\sqrt{y}+c\sqrt{y}z^2$ | 119.35 | 91.21 | 0.827 | 0.0729 | 0.0496 | 0.7379 | 0.2503 | 0.1672 | 0.735 |
| $a+bx\sqrt{y}+c\sqrt{y}\sqrt{z}$ | 122.13 | 93.72 | 0.819 | 0.0742 | 0.0448 | 0.7283 | 0.2506 | 0.1563 | 0.734 |
| $a+bx\sqrt{y}+c/yz$ | 138.69 | 107.44 | 0.766 | 0.0821 | 0.0566 | 0.6675 | 0.2611 | 0.1710 | 0.711 |
| $a+bx\sqrt{y}+c/yz^2$ | 136.91 | 103.14 | 0.772 | 0.0821 | 0.0568 | 0.6672 | 0.2609 | 0.1719 | 0.712 |
| $a+bx\sqrt{y}+c/y\sqrt{z}$ | 137.85 | 108.60 | 0.769 | 0.0818 | 0.0559 | 0.6693 | 0.2623 | 0.1732 | 0.709 |
| $a+bx\sqrt{y}+cz/y$ | 107.52 | 81.97 | 0.859 | 0.0734 | 0.0483 | 0.7336 | 0.2433 | 0.1638 | 0.749 |
| $a+bx\sqrt{y}+cz^2/y$ | 109.40 | 81.63 | 0.854 | 0.0694 | 0.0443 | 0.7623 | 0.2380 | 0.1584 | 0.760 |
| $a+bx\sqrt{y}+c\sqrt{z}/y$ | 115.90 | 87.17 | 0.837 | 0.0774 | 0.0528 | 0.7041 | 0.2534 | 0.1750 | 0.728 |
| $a+bx\sqrt{y}+c/y^2z$ | 137.59 | 108.27 | 0.770 | 0.0816 | 0.0558 | 0.6715 | 0.2625 | 0.1743 | 0.708 |
| $a+bx\sqrt{y}+c/y^2z^2$ | 138.77 | 107.99 | 0.766 | 0.0818 | 0.0559 | 0.6697 | 0.2621 | 0.1723 | 0.709 |
| $a+bx\sqrt{y}+c/y^2\sqrt{z}$ | 135.02 | 105.75 | 0.778 | 0.0814 | 0.0554 | 0.6731 | 0.2625 | 0.1752 | 0.708 |
| $a+bx\sqrt{y}+cz/y^2$ | 117.66 | 87.00 | 0.832 | 0.0794 | 0.0543 | 0.6887 | 0.2570 | 0.1753 | 0.720 |
| $a+bx\sqrt{y}+cz^2/y^2$ | 105.13 | 78.02 | 0.866 | 0.0745 | 0.0501 | 0.7256 | 0.2445 | 0.1657 | 0.747 |
| $a+bx\sqrt{y}+c\sqrt{z}/y^2$ | 124.55 | 94.09 | 0.811 | 0.0805 | 0.0545 | 0.6803 | 0.2603 | 0.1756 | 0.713 |
| $a+bx\sqrt{y}+c/\sqrt{y}z$ | 134.60 | 99.98 | 0.780 | 0.0818 | 0.0577 | 0.6698 | 0.2576 | 0.1676 | 0.719 |
| $a+bx\sqrt{y}+c/\sqrt{y}z^2$ | 134.31 | 101.99 | 0.781 | 0.0820 | 0.0575 | 0.6677 | 0.2601 | 0.1709 | 0.713 |
| $a+bx\sqrt{y}+c/\sqrt{y}\sqrt{z}$ | 137.62 | 104.16 | 0.770 | 0.0819 | 0.0577 | 0.6686 | 0.2586 | 0.1680 | 0.717 |
| $a+bx\sqrt{y}+cz/\sqrt{y}$ | 109.23 | 83.58 | 0.855 | 0.0706 | 0.0441 | 0.7538 | 0.2390 | 0.1549 | 0.758 |
| $a+bx\sqrt{y}+cz^2/\sqrt{y}$ | 113.68 | 84.70 | 0.843 | 0.0698 | 0.0456 | 0.7591 | 0.2416 | 0.1604 | 0.753 |
| $a+bx\sqrt{y}+c\sqrt{z}/\sqrt{y}$ | 110.16 | 84.90 | 0.852 | 0.0735 | 0.0483 | 0.7331 | 0.2441 | 0.1634 | 0.747 |
| $a+bx^2/y+cx/z$ | 140.99 | 115.74 | 0.758 | 0.0797 | 0.0584 | 0.6864 | 0.2532 | 0.1845 | 0.728 |

(continued on next page)

**Table 4 – continued from previous page**

| Functional form | $T_{eff}$ (K) | | | Radius ($R_\odot$) | | | log (L/$L_\odot$) | | |
|---|---|---|---|---|---|---|---|---|---|
| | RMSE | MAD | $R^2_{ap}$ | RMSE | MAD | $R^2_{ap}$ | RMSE | MAD | $R^2_{ap}$ |
| $a+bx^2/y+cx/z^2$ | 147.80 | 118.75 | 0.734 | 0.0830 | 0.0631 | 0.6598 | 0.2583 | 0.1877 | 0.717 |
| $a+bx^2/y+cx/\sqrt{z}$ | 144.00 | 116.79 | 0.748 | 0.0796 | 0.0586 | 0.6870 | 0.2548 | 0.1874 | 0.725 |
| $a+bx^2/y+cxz$ | 116.30 | 91.04 | 0.835 | 0.0683 | 0.0465 | 0.7695 | 0.2313 | 0.1669 | 0.773 |
| $a+bx^2/y+cxz^2$ | 117.60 | 93.48 | 0.832 | 0.0689 | 0.0494 | 0.7653 | 0.2327 | 0.1741 | 0.771 |
| $a+bx^2/y+cx\sqrt{z}$ | 116.50 | 91.11 | 0.835 | 0.0692 | 0.0448 | 0.7635 | 0.2308 | 0.1599 | 0.774 |
| $a+bx^2/y+cx^2/z$ | 147.80 | 119.07 | 0.734 | 0.0799 | 0.0590 | 0.6847 | 0.2559 | 0.1885 | 0.722 |
| $a+bx^2/y+cx^2/z^2$ | 149.10 | 120.43 | 0.730 | 0.0826 | 0.0626 | 0.6629 | 0.2588 | 0.1890 | 0.716 |
| $a+bx^2/y+cx^2/\sqrt{z}$ | 157.81 | 125.02 | 0.697 | 0.0839 | 0.0633 | 0.6521 | 0.2622 | 0.1899 | 0.709 |
| $a+bx^2/y+cx^2z$ | 118.59 | 95.84 | 0.829 | 0.0709 | 0.0507 | 0.7518 | 0.2372 | 0.1766 | 0.762 |
| $a+bx^2/y+cx^2z^2$ | 119.48 | 95.99 | 0.826 | 0.0712 | 0.0516 | 0.7500 | 0.2373 | 0.1789 | 0.761 |
| $a+bx^2/y+cx^2\sqrt{z}$ | 118.39 | 95.08 | 0.829 | 0.0718 | 0.0509 | 0.7451 | 0.2382 | 0.1747 | 0.760 |
| $a+bx^2/y+c\sqrt{x}/z$ | 137.36 | 111.92 | 0.770 | 0.0799 | 0.0592 | 0.6845 | 0.2512 | 0.1796 | 0.733 |
| $a+bx^2/y+c\sqrt{x}/z^2$ | 146.72 | 116.80 | 0.738 | 0.0833 | 0.0636 | 0.6576 | 0.2577 | 0.1860 | 0.719 |
| $a+bx^2/y+c\sqrt{x}/\sqrt{z}$ | 135.39 | 111.72 | 0.777 | 0.0786 | 0.0577 | 0.6952 | 0.2501 | 0.1806 | 0.735 |
| $a+bx^2/y+c\sqrt{x}z$ | 116.99 | 90.45 | 0.833 | 0.0676 | 0.0439 | 0.7742 | 0.2290 | 0.1609 | 0.778 |
| $a+bx^2/y+c\sqrt{x}z^2$ | 117.24 | 92.20 | 0.833 | 0.0680 | 0.0477 | 0.7717 | 0.2305 | 0.1704 | 0.775 |
| $a+bx^2/y+c\sqrt{x}\sqrt{z}$ | 120.87 | 92.04 | 0.822 | 0.0692 | 0.0443 | 0.7636 | 0.2296 | 0.1529 | 0.777 |
| $a+bx^2/y+c/xz$ | 148.48 | 120.91 | 0.732 | 0.0841 | 0.0616 | 0.6507 | 0.2608 | 0.1877 | 0.712 |
| $a+bx^2/y+c/xz^2$ | 155.39 | 126.12 | 0.706 | 0.0843 | 0.0623 | 0.6489 | 0.2623 | 0.1910 | 0.708 |
| $a+bx^2/y+c/x\sqrt{z}$ | 145.44 | 116.87 | 0.743 | 0.0841 | 0.0615 | 0.6511 | 0.2598 | 0.1848 | 0.714 |
| $a+bx^2/y+cz/x$ | 135.29 | 106.58 | 0.777 | 0.0827 | 0.0613 | 0.6623 | 0.2545 | 0.1788 | 0.726 |
| $a+bx^2/y+cz^2/x$ | 117.21 | 94.57 | 0.833 | 0.0768 | 0.0570 | 0.7090 | 0.2405 | 0.1747 | 0.755 |
| $a+bx^2/y+c\sqrt{z}/x$ | 139.84 | 109.00 | 0.762 | 0.0836 | 0.0618 | 0.6551 | 0.2573 | 0.1787 | 0.720 |
| $a+bx^2/y+c/x^2z$ | 141.22 | 110.22 | 0.757 | 0.0839 | 0.0620 | 0.6521 | 0.2582 | 0.1797 | 0.718 |
| $a+bx^2/y+c/x^2z^2$ | 142.59 | 113.68 | 0.753 | 0.0838 | 0.0615 | 0.6535 | 0.2585 | 0.1818 | 0.717 |
| $a+bx^2/y+c/x^2\sqrt{z}$ | 140.92 | 109.23 | 0.758 | 0.0840 | 0.0622 | 0.6515 | 0.2581 | 0.1790 | 0.718 |
| $a+bx^2/y+cz/x^2$ | 140.37 | 107.49 | 0.760 | 0.0841 | 0.0624 | 0.6509 | 0.2578 | 0.1787 | 0.718 |
| $a+bx^2/y+cz^2/x^2$ | 139.39 | 107.53 | 0.764 | 0.0840 | 0.0625 | 0.6520 | 0.2573 | 0.1791 | 0.720 |
| $a+bx^2/y+c\sqrt{z}/x^2$ | 140.57 | 107.91 | 0.760 | 0.0841 | 0.0624 | 0.6510 | 0.2580 | 0.1785 | 0.718 |
| $a+bx^2/y+c/\sqrt{x}z$ | 157.99 | 125.09 | 0.696 | 0.0851 | 0.0652 | 0.6428 | 0.2620 | 0.1864 | 0.709 |
| $a+bx^2/y+c/\sqrt{x}z^2$ | 155.28 | 116.46 | 0.707 | 0.0850 | 0.0651 | 0.6430 | 0.2608 | 0.1870 | 0.712 |
| $a+bx^2/y+c/\sqrt{x}\sqrt{z}$ | 155.38 | 125.48 | 0.706 | 0.0850 | 0.0645 | 0.6435 | 0.2627 | 0.1902 | 0.708 |
| $a+bx^2/y+cz/\sqrt{x}$ | 117.77 | 94.37 | 0.831 | 0.0756 | 0.0559 | 0.7180 | 0.2392 | 0.1737 | 0.757 |
| $a+bx^2/y+cz^2/\sqrt{x}$ | 111.59 | 85.77 | 0.848 | 0.0681 | 0.0469 | 0.7712 | 0.2270 | 0.1607 | 0.782 |
| $a+bx^2/y+c\sqrt{z}/\sqrt{x}$ | 132.01 | 104.72 | 0.788 | 0.0810 | 0.0599 | 0.6760 | 0.2515 | 0.1804 | 0.732 |
| $a+bx^2/y+cy/z$ | 145.34 | 118.73 | 0.743 | 0.0809 | 0.0591 | 0.6769 | 0.2553 | 0.1847 | 0.724 |
| $a+bx^2/y+cy/z^2$ | 148.25 | 117.53 | 0.733 | 0.0832 | 0.0633 | 0.6580 | 0.2583 | 0.1869 | 0.717 |
| $a+bx^2/y+cy/\sqrt{z}$ | 153.31 | 122.22 | 0.714 | 0.0826 | 0.0601 | 0.6632 | 0.2599 | 0.1883 | 0.714 |
| $a+bx^2/y+cyz$ | 113.84 | 86.69 | 0.842 | 0.0688 | 0.0447 | 0.7663 | 0.2297 | 0.1598 | 0.776 |
| $a+bx^2/y+cyz^2$ | 115.03 | 90.32 | 0.839 | 0.0685 | 0.0475 | 0.7682 | 0.2305 | 0.1698 | 0.775 |
| $a+bx^2/y+cy\sqrt{z}$ | 118.12 | 88.18 | 0.830 | 0.0718 | 0.0471 | 0.7455 | 0.2329 | 0.1535 | 0.770 |
| $a+bx^2/y+cy^2/z$ | 154.22 | 122.19 | 0.711 | 0.0826 | 0.0605 | 0.6632 | 0.2600 | 0.1888 | 0.713 |
| $a+bx^2/y+cy^2/z^2$ | 150.28 | 119.25 | 0.725 | 0.0830 | 0.0624 | 0.6602 | 0.2591 | 0.1883 | 0.715 |
| $a+bx^2/y+cy^2/\sqrt{z}$ | 157.32 | 124.01 | 0.699 | 0.0850 | 0.0650 | 0.6431 | 0.2625 | 0.1893 | 0.708 |
| $a+bx^2/y+cy^2z$ | 115.28 | 89.06 | 0.838 | 0.0709 | 0.0475 | 0.7515 | 0.2343 | 0.1654 | 0.767 |
| $a+bx^2/y+cy^2z^2$ | 115.47 | 91.08 | 0.838 | 0.0703 | 0.0491 | 0.7561 | 0.2338 | 0.1726 | 0.768 |
| $a+bx^2/y+cy^2\sqrt{z}$ | 119.31 | 91.16 | 0.827 | 0.0736 | 0.0497 | 0.7327 | 0.2378 | 0.1620 | 0.760 |
| $a+bx^2/y+c\sqrt{y}/z$ | 140.06 | 114.11 | 0.761 | 0.0805 | 0.0597 | 0.6804 | 0.2520 | 0.1798 | 0.731 |
| $a+bx^2/y+c\sqrt{y}/z^2$ | 147.31 | 116.05 | 0.736 | 0.0835 | 0.0639 | 0.6559 | 0.2578 | 0.1855 | 0.718 |
| $a+bx^2/y+c\sqrt{y}/\sqrt{z}$ | 142.36 | 117.07 | 0.753 | 0.0798 | 0.0584 | 0.6859 | 0.2529 | 0.1828 | 0.729 |
| $a+bx^2/y+c\sqrt{y}z$ | 113.78 | 87.01 | 0.842 | 0.0678 | 0.0431 | 0.7728 | 0.2276 | 0.1566 | 0.780 |
| $a+bx^2/y+c\sqrt{y}z^2$ | 115.42 | 89.94 | 0.838 | 0.0678 | 0.0466 | 0.7732 | 0.2291 | 0.1678 | 0.778 |
| $a+bx^2/y+c\sqrt{y}\sqrt{z}$ | 116.35 | 88.22 | 0.835 | 0.0703 | 0.0446 | 0.7563 | 0.2293 | 0.1491 | 0.777 |
| $a+bx^2/y+c/yz$ | 155.74 | 118.45 | 0.705 | 0.0850 | 0.0654 | 0.6431 | 0.2601 | 0.1865 | 0.713 |
| $a+bx^2/y+c/yz^2$ | 153.48 | 116.27 | 0.713 | 0.0850 | 0.0652 | 0.6430 | 0.2602 | 0.1873 | 0.713 |
| $a+bx^2/y+c/y\sqrt{z}$ | 157.61 | 123.16 | 0.698 | 0.0851 | 0.0653 | 0.6428 | 0.2612 | 0.1876 | 0.711 |
| $a+bx^2/y+cz/y$ | 135.38 | 106.93 | 0.777 | 0.0783 | 0.0578 | 0.6975 | 0.2484 | 0.1809 | 0.739 |
| $a+bx^2/y+cz^2/y$ | 121.14 | 93.42 | 0.821 | 0.0697 | 0.0498 | 0.7600 | 0.2319 | 0.1663 | 0.772 |
| $a+bx^2/y+c\sqrt{z}/y$ | 148.83 | 119.83 | 0.731 | 0.0830 | 0.0600 | 0.6598 | 0.2592 | 0.1862 | 0.715 |
| $a+bx^2/y+c/y^2z$ | 157.62 | 126.13 | 0.698 | 0.0846 | 0.0628 | 0.6470 | 0.2627 | 0.1901 | 0.707 |
| $a+bx^2/y+c/y^2z^2$ | 157.74 | 123.56 | 0.697 | 0.0848 | 0.0637 | 0.6452 | 0.2625 | 0.1883 | 0.708 |
| $a+bx^2/y+c/y^2\sqrt{z}$ | 156.22 | 125.74 | 0.703 | 0.0844 | 0.0622 | 0.6481 | 0.2626 | 0.1905 | 0.708 |
| $a+bx^2/y+cz/y^2$ | 145.93 | 117.05 | 0.741 | 0.0833 | 0.0606 | 0.6572 | 0.2588 | 0.1840 | 0.716 |
| $a+bx^2/y+cz^2/y^2$ | 133.56 | 103.71 | 0.783 | 0.0790 | 0.0588 | 0.6917 | 0.2485 | 0.1814 | 0.738 |
| $a+bx^2/y+c\sqrt{z}/y^2$ | 150.14 | 121.66 | 0.726 | 0.0840 | 0.0610 | 0.6520 | 0.2609 | 0.1874 | 0.712 |
| $a+bx^2/y+c/\sqrt{y}z$ | 146.31 | 110.73 | 0.740 | 0.0836 | 0.0646 | 0.6550 | 0.2537 | 0.1821 | 0.727 |
| $a+bx^2/y+c/\sqrt{y}z^2$ | 149.22 | 112.80 | 0.729 | 0.0846 | 0.0647 | 0.6468 | 0.2582 | 0.1858 | 0.717 |
| $a+bx^2/y+c/\sqrt{y}\sqrt{z}$ | 148.31 | 110.45 | 0.732 | 0.0832 | 0.0641 | 0.6582 | 0.2526 | 0.1803 | 0.730 |
| $a+bx^2/y+cz/\sqrt{y}$ | 122.76 | 96.45 | 0.817 | 0.0717 | 0.0520 | 0.7461 | 0.2351 | 0.1686 | 0.766 |
| $a+bx^2/y+cz^2/\sqrt{y}$ | 118.18 | 92.24 | 0.830 | 0.0677 | 0.0464 | 0.7736 | 0.2288 | 0.1627 | 0.778 |
| $a+bx^2/y+c\sqrt{z}/\sqrt{y}$ | 137.15 | 110.66 | 0.771 | 0.0783 | 0.0575 | 0.6969 | 0.2493 | 0.1804 | 0.737 |
| $a+bx^2/y^2+cx/z$ | 231.95 | 171.01 | 0.345 | 0.1152 | 0.0935 | 0.3447 | 0.3846 | 0.3049 | 0.373 |
| $a+bx^2/y^2+cx/z^2$ | 227.90 | 168.90 | 0.368 | 0.1155 | 0.0920 | 0.3411 | 0.3797 | 0.2974 | 0.389 |
| $a+bx^2/y^2+cx/\sqrt{z}$ | 254.58 | 191.07 | 0.211 | 0.1246 | 0.0967 | 0.2338 | 0.4053 | 0.3136 | 0.304 |
| $a+bx^2/y^2+cxz$ | 123.13 | 93.12 | 0.816 | 0.0692 | 0.0487 | 0.7634 | 0.2440 | 0.1828 | 0.748 |
| $a+bx^2/y^2+cxz^2$ | 137.85 | 106.83 | 0.769 | 0.0742 | 0.0567 | 0.7284 | 0.2646 | 0.2042 | 0.703 |
| $a+bx^2/y^2+cx\sqrt{z}$ | 117.04 | 90.79 | 0.833 | 0.0689 | 0.0450 | 0.7654 | 0.2330 | 0.1616 | 0.770 |
| $a+bx^2/y^2+cx^2/z$ | 255.02 | 190.70 | 0.209 | 0.1245 | 0.0974 | 0.2343 | 0.4073 | 0.3148 | 0.297 |
| $a+bx^2/y^2+cx^2/z^2$ | 238.08 | 175.46 | 0.310 | 0.1182 | 0.0938 | 0.3101 | 0.3912 | 0.3023 | 0.351 |
| $a+bx^2/y^2+cx^2/\sqrt{z}$ | 194.04 | 154.27 | 0.542 | 0.1041 | 0.0814 | 0.4646 | 0.3220 | 0.2473 | 0.561 |
| $a+bx^2/y^2+cx^2z$ | 127.76 | 99.71 | 0.801 | 0.0728 | 0.0552 | 0.7382 | 0.2554 | 0.1986 | 0.724 |
| $a+bx^2/y^2+cx^2z^2$ | 141.45 | 112.72 | 0.757 | 0.0776 | 0.0610 | 0.7029 | 0.2735 | 0.2172 | 0.683 |
| $a+bx^2/y^2+cx^2\sqrt{z}$ | 120.75 | 95.62 | 0.823 | 0.0719 | 0.0518 | 0.7447 | 0.2455 | 0.1855 | 0.745 |
| $a+bx^2/y^2+c\sqrt{x}/z$ | 206.27 | 155.99 | 0.482 | 0.1071 | 0.0869 | 0.4340 | 0.3547 | 0.2826 | 0.467 |
| $a+bx^2/y^2+c\sqrt{x}/z^2$ | 219.16 | 162.57 | 0.416 | 0.1134 | 0.0900 | 0.3650 | 0.3696 | 0.2899 | 0.421 |
| $a+bx^2/y^2+c\sqrt{x}/\sqrt{z}$ | 232.00 | 171.35 | 0.345 | 0.1158 | 0.0939 | 0.3376 | 0.3862 | 0.3064 | 0.368 |
| $a+bx^2/y^2+c\sqrt{x}z$ | 125.06 | 95.84 | 0.810 | 0.0689 | 0.0470 | 0.7657 | 0.2429 | 0.1740 | 0.750 |
| $a+bx^2/y^2+c\sqrt{x}z^2$ | 137.88 | 105.86 | 0.769 | 0.0732 | 0.0548 | 0.7357 | 0.2620 | 0.1973 | 0.709 |
| $a+bx^2/y^2+c\sqrt{x}\sqrt{z}$ | 122.11 | 92.32 | 0.819 | 0.0693 | 0.0442 | 0.7630 | 0.2340 | 0.1533 | 0.768 |

(continued on next page)

**Table 4 – continued from previous page**

| Functional form | $T_{eff}$ (K) | | | Radius ($R_{\odot}$) | | | log ($L/L_{\odot}$) | | |
|---|---|---|---|---|---|---|---|---|---|
| | RMSE | MAD | $R^2_{ap}$ | RMSE | MAD | $R^2_{ap}$ | RMSE | MAD | $R^2_{ap}$ |
| $a+bx^2/y^2+c/xz$ | 248.51 | 188.02 | 0.249 | 0.1198 | 0.0931 | 0.2910 | 0.3894 | 0.2969 | 0.358 |
| $a+bx^2/y^2+c/xz^2$ | 237.47 | 176.92 | 0.314 | 0.1176 | 0.0896 | 0.3173 | 0.3763 | 0.2738 | 0.400 |
| $a+bx^2/y^2+c/x\sqrt{z}$ | 252.50 | 190.89 | 0.224 | 0.1215 | 0.0953 | 0.2716 | 0.3967 | 0.3063 | 0.333 |
| $a+bx^2/y^2+cz/x$ | 249.83 | 185.88 | 0.241 | 0.1244 | 0.0983 | 0.2362 | 0.4066 | 0.3184 | 0.300 |
| $a+bx^2/y^2+cz^2/x$ | 201.39 | 153.01 | 0.507 | 0.1082 | 0.0856 | 0.4220 | 0.3563 | 0.2826 | 0.462 |
| $a+bx^2/y^2+c\sqrt{z}/x$ | 254.61 | 188.94 | 0.211 | 0.1243 | 0.0964 | 0.2368 | 0.4071 | 0.3156 | 0.298 |
| $a+bx^2/y^2+c/x^2z$ | 254.74 | 189.22 | 0.210 | 0.1242 | 0.0964 | 0.2388 | 0.4068 | 0.3156 | 0.299 |
| $a+bx^2/y^2+c/x^2z^2$ | 255.01 | 190.85 | 0.209 | 0.1238 | 0.0961 | 0.2434 | 0.4051 | 0.3142 | 0.305 |
| $a+bx^2/y^2+c/x^2\sqrt{z}$ | 254.48 | 188.52 | 0.212 | 0.1243 | 0.0965 | 0.2375 | 0.4072 | 0.3156 | 0.298 |
| $a+bx^2/y^2+cz/x^2$ | 253.64 | 186.60 | 0.217 | 0.1245 | 0.0964 | 0.2349 | 0.4077 | 0.3148 | 0.296 |
| $a+bx^2/y^2+cz^2/x^2$ | 252.64 | 185.58 | 0.223 | 0.1246 | 0.0968 | 0.2334 | 0.4078 | 0.3149 | 0.296 |
| $a+bx^2/y^2+c\sqrt{z}/x^2$ | 253.94 | 187.25 | 0.215 | 0.1244 | 0.0965 | 0.2357 | 0.4076 | 0.3151 | 0.296 |
| $a+bx^2/y^2+c/\sqrt{x}z$ | 205.05 | 143.59 | 0.488 | 0.1048 | 0.0800 | 0.4581 | 0.3299 | 0.2352 | 0.539 |
| $a+bx^2/y^2+c/\sqrt{x}z^2$ | 207.61 | 155.87 | 0.476 | 0.1104 | 0.0851 | 0.3981 | 0.3468 | 0.2535 | 0.490 |
| $a+bx^2/y^2+c/\sqrt{x}\sqrt{z}$ | 221.67 | 159.86 | 0.402 | 0.1082 | 0.0815 | 0.4221 | 0.3467 | 0.2434 | 0.491 |
| $a+bx^2/y^2+cz/\sqrt{x}$ | 188.70 | 141.53 | 0.567 | 0.1020 | 0.0805 | 0.4864 | 0.3391 | 0.2688 | 0.513 |
| $a+bx^2/y^2+cz^2/\sqrt{x}$ | 143.54 | 107.28 | 0.749 | 0.0777 | 0.0593 | 0.7019 | 0.2730 | 0.2111 | 0.684 |
| $a+bx^2/y^2+c\sqrt{z}/\sqrt{x}$ | 244.88 | 183.42 | 0.270 | 0.1229 | 0.0986 | 0.2546 | 0.4026 | 0.3184 | 0.313 |
| $a+bx^2/y^2+cy/z$ | 228.91 | 168.52 | 0.362 | 0.1142 | 0.0921 | 0.3564 | 0.3807 | 0.3000 | 0.386 |
| $a+bx^2/y^2+cy/z^2$ | 223.90 | 164.57 | 0.390 | 0.1144 | 0.0907 | 0.3539 | 0.3750 | 0.2932 | 0.404 |
| $a+bx^2/y^2+cy/\sqrt{z}$ | 255.01 | 190.86 | 0.209 | 0.1246 | 0.0975 | 0.2332 | 0.4071 | 0.3148 | 0.298 |
| $a+bx^2/y^2+cyz$ | 121.09 | 89.83 | 0.822 | 0.0693 | 0.0455 | 0.7631 | 0.2407 | 0.1734 | 0.754 |
| $a+bx^2/y^2+cyz^2$ | 135.03 | 103.17 | 0.778 | 0.0733 | 0.0536 | 0.7344 | 0.2604 | 0.1969 | 0.713 |
| $a+bx^2/y^2+cy\sqrt{z}$ | 120.64 | 87.74 | 0.823 | 0.0713 | 0.0456 | 0.7487 | 0.2360 | 0.1523 | 0.764 |
| $a+bx^2/y^2+cy^2/z$ | 254.88 | 190.07 | 0.210 | 0.1244 | 0.0977 | 0.2365 | 0.4078 | 0.3142 | 0.296 |
| $a+bx^2/y^2+cy^2/z^2$ | 236.34 | 170.27 | 0.320 | 0.1177 | 0.0933 | 0.3156 | 0.3893 | 0.3007 | 0.358 |
| $a+bx^2/y^2+cy^2/\sqrt{z}$ | 218.86 | 172.40 | 0.417 | 0.1126 | 0.0900 | 0.3735 | 0.3539 | 0.2775 | 0.469 |
| $a+bx^2/y^2+cy^2z$ | 123.10 | 91.97 | 0.816 | 0.0719 | 0.0493 | 0.7447 | 0.2479 | 0.1832 | 0.740 |
| $a+bx^2/y^2+cy^2z^2$ | 136.27 | 105.21 | 0.774 | 0.0758 | 0.0560 | 0.7162 | 0.2660 | 0.2055 | 0.700 |
| $a+bx^2/y^2+cy^2\sqrt{z}$ | 122.00 | 90.94 | 0.819 | 0.0734 | 0.0493 | 0.7339 | 0.2436 | 0.1674 | 0.749 |
| $a+bx^2/y^2+c\sqrt{y}/z$ | 199.87 | 151.66 | 0.514 | 0.1046 | 0.0837 | 0.4600 | 0.3456 | 0.2718 | 0.494 |
| $a+bx^2/y^2+c\sqrt{y}/z^2$ | 215.53 | 159.41 | 0.435 | 0.1123 | 0.0887 | 0.3768 | 0.3650 | 0.2844 | 0.436 |
| $a+bx^2/y^2+c\sqrt{y}/\sqrt{z}$ | 225.83 | 168.68 | 0.380 | 0.1128 | 0.0914 | 0.3722 | 0.3773 | 0.2998 | 0.397 |
| $a+bx^2/y^2+c\sqrt{y}z$ | 122.74 | 94.12 | 0.817 | 0.0690 | 0.0455 | 0.7648 | 0.2412 | 0.1698 | 0.754 |
| $a+bx^2/y^2+c\sqrt{y}z^2$ | 136.13 | 104.40 | 0.775 | 0.0728 | 0.0533 | 0.7385 | 0.2598 | 0.1932 | 0.714 |
| $a+bx^2/y^2+c\sqrt{y}\sqrt{z}$ | 120.01 | 88.77 | 0.825 | 0.0703 | 0.0449 | 0.7559 | 0.2344 | 0.1503 | 0.767 |
| $a+bx^2/y^2+c/yz$ | 200.85 | 146.60 | 0.509 | 0.1072 | 0.0816 | 0.4325 | 0.3324 | 0.2402 | 0.532 |
| $a+bx^2/y^2+c/yz^2$ | 209.79 | 156.42 | 0.465 | 0.1128 | 0.0879 | 0.3722 | 0.3528 | 0.2620 | 0.473 |
| $a+bx^2/y^2+c/y\sqrt{z}$ | 206.00 | 149.50 | 0.484 | 0.1067 | 0.0823 | 0.4377 | 0.3328 | 0.2385 | 0.531 |
| $a+bx^2/y^2+cz/y$ | 225.23 | 169.91 | 0.383 | 0.1134 | 0.0913 | 0.3656 | 0.3784 | 0.3021 | 0.393 |
| $a+bx^2/y^2+cz^2/y$ | 160.51 | 123.83 | 0.687 | 0.0829 | 0.0661 | 0.6606 | 0.2913 | 0.2322 | 0.641 |
| $a+bx^2/y^2+c\sqrt{z}/y$ | 254.71 | 191.49 | 0.211 | 0.1243 | 0.0959 | 0.2377 | 0.4047 | 0.3129 | 0.306 |
| $a+bx^2/y^2+c/y^2z$ | 234.09 | 173.11 | 0.333 | 0.1180 | 0.0911 | 0.3127 | 0.3747 | 0.2791 | 0.405 |
| $a+bx^2/y^2+c/y^2z^2$ | 231.50 | 172.32 | 0.348 | 0.1190 | 0.0915 | 0.3012 | 0.3769 | 0.2765 | 0.398 |
| $a+bx^2/y^2+c/y^2\sqrt{z}$ | 237.93 | 176.55 | 0.311 | 0.1181 | 0.0916 | 0.3112 | 0.3770 | 0.2804 | 0.398 |
| $a+bx^2/y^2+cz/y^2$ | 254.89 | 191.33 | 0.210 | 0.1241 | 0.0960 | 0.2401 | 0.4048 | 0.3133 | 0.306 |
| $a+bx^2/y^2+cz^2/y^2$ | 230.34 | 174.88 | 0.354 | 0.1165 | 0.0948 | 0.3295 | 0.3858 | 0.3116 | 0.369 |
| $a+bx^2/y^2+c\sqrt{z}/y^2$ | 250.50 | 189.47 | 0.237 | 0.1215 | 0.0946 | 0.2708 | 0.3942 | 0.3014 | 0.342 |
| $a+bx^2/y^2+c/\sqrt{y}z$ | 175.13 | 130.58 | 0.627 | 0.0987 | 0.0766 | 0.5188 | 0.3051 | 0.2179 | 0.606 |
| $a+bx^2/y^2+c/\sqrt{y}z^2$ | 202.83 | 150.94 | 0.499 | 0.1102 | 0.0869 | 0.4002 | 0.3471 | 0.2591 | 0.489 |
| $a+bx^2/y^2+c/\sqrt{y}\sqrt{z}$ | 168.91 | 119.79 | 0.653 | 0.0939 | 0.0711 | 0.5650 | 0.2888 | 0.2009 | 0.646 |
| $a+bx^2/y^2+cz/\sqrt{y}$ | 161.58 | 129.03 | 0.682 | 0.0853 | 0.0676 | 0.6411 | 0.2951 | 0.2348 | 0.631 |
| $a+bx^2/y^2+cz^2/\sqrt{y}$ | 145.83 | 110.08 | 0.741 | 0.0757 | 0.0586 | 0.7168 | 0.2703 | 0.2085 | 0.691 |
| $a+bx^2/y^2+c\sqrt{z}/\sqrt{y}$ | 223.97 | 167.47 | 0.390 | 0.1124 | 0.0911 | 0.3767 | 0.3762 | 0.2996 | 0.400 |
| $a+bx^2/\sqrt{y}+cx/z$ | 123.27 | 103.93 | 0.815 | 0.0753 | 0.0530 | 0.7199 | 0.2424 | 0.1728 | 0.751 |
| $a+bx^2/\sqrt{y}+cx/z^2$ | 127.83 | 106.14 | 0.801 | 0.0772 | 0.0546 | 0.7059 | 0.2440 | 0.1743 | 0.748 |
| $a+bx^2/\sqrt{y}+cx/\sqrt{z}$ | 121.83 | 102.42 | 0.819 | 0.0743 | 0.0537 | 0.7272 | 0.2419 | 0.1727 | 0.752 |
| $a+bx^2/\sqrt{y}+cxz$ | 114.79 | 90.23 | 0.840 | 0.0693 | 0.0474 | 0.7626 | 0.2352 | 0.1641 | 0.766 |
| $a+bx^2/\sqrt{y}+cxz^2$ | 114.36 | 91.12 | 0.841 | 0.0699 | 0.0496 | 0.7587 | 0.2358 | 0.1682 | 0.764 |
| $a+bx^2/\sqrt{y}+cx\sqrt{z}$ | 116.19 | 91.35 | 0.836 | 0.0695 | 0.0443 | 0.7612 | 0.2344 | 0.1584 | 0.767 |
| $a+bx^2/\sqrt{y}+cx^2/z$ | 124.14 | 105.35 | 0.813 | 0.0740 | 0.0525 | 0.7297 | 0.2416 | 0.1729 | 0.753 |
| $a+bx^2/\sqrt{y}+cx^2/z^2$ | 128.34 | 106.99 | 0.800 | 0.0769 | 0.0544 | 0.7083 | 0.2442 | 0.1746 | 0.747 |
| $a+bx^2/\sqrt{y}+cx^2/\sqrt{z}$ | 124.23 | 104.84 | 0.812 | 0.0722 | 0.0512 | 0.7424 | 0.2389 | 0.1731 | 0.758 |
| $a+bx^2/\sqrt{y}+cx^2z$ | 117.58 | 94.58 | 0.832 | 0.0720 | 0.0510 | 0.7438 | 0.2401 | 0.1698 | 0.756 |
| $a+bx^2/\sqrt{y}+cx^2z^2$ | 116.50 | 94.20 | 0.835 | 0.0719 | 0.0514 | 0.7446 | 0.2392 | 0.1701 | 0.758 |
| $a+bx^2/\sqrt{y}+cx^2\sqrt{z}$ | 118.70 | 94.34 | 0.829 | 0.0729 | 0.0512 | 0.7377 | 0.2415 | 0.1702 | 0.753 |
| $a+bx^2/\sqrt{y}+c\sqrt{x}/z$ | 121.72 | 101.97 | 0.820 | 0.0757 | 0.0530 | 0.7169 | 0.2417 | 0.1709 | 0.753 |
| $a+bx^2/\sqrt{y}+c\sqrt{x}/z^2$ | 127.06 | 105.17 | 0.804 | 0.0773 | 0.0548 | 0.7049 | 0.2437 | 0.1735 | 0.748 |
| $a+bx^2/\sqrt{y}+c\sqrt{x}/\sqrt{z}$ | 119.29 | 99.60 | 0.827 | 0.0747 | 0.0530 | 0.7242 | 0.2412 | 0.1707 | 0.753 |
| $a+bx^2/\sqrt{y}+c\sqrt{x}z$ | 114.19 | 89.60 | 0.841 | 0.0683 | 0.0448 | 0.7698 | 0.2322 | 0.1600 | 0.772 |
| $a+bx^2/\sqrt{y}+c\sqrt{x}z^2$ | 113.39 | 89.93 | 0.844 | 0.0689 | 0.0482 | 0.7658 | 0.2337 | 0.1664 | 0.769 |
| $a+bx^2/\sqrt{y}+c\sqrt{x}\sqrt{z}$ | 118.69 | 92.72 | 0.829 | 0.0693 | 0.0434 | 0.7630 | 0.2313 | 0.1525 | 0.773 |
| $a+bx^2/\sqrt{y}+c/xz$ | 125.42 | 102.41 | 0.809 | 0.0775 | 0.0536 | 0.7038 | 0.2446 | 0.1738 | 0.746 |
| $a+bx^2/\sqrt{y}+c/xz^2$ | 130.84 | 108.60 | 0.792 | 0.0775 | 0.0535 | 0.7036 | 0.2446 | 0.1727 | 0.746 |
| $a+bx^2/\sqrt{y}+c/x\sqrt{z}$ | 122.87 | 99.04 | 0.816 | 0.0774 | 0.0538 | 0.7039 | 0.2444 | 0.1734 | 0.747 |
| $a+bx^2/\sqrt{y}+cz/x$ | 115.68 | 90.49 | 0.837 | 0.0768 | 0.0545 | 0.7084 | 0.2423 | 0.1712 | 0.751 |
| $a+bx^2/\sqrt{y}+cz^2/x$ | 106.15 | 83.40 | 0.863 | 0.0739 | 0.0534 | 0.7304 | 0.2366 | 0.1682 | 0.763 |
| $a+bx^2/\sqrt{y}+c\sqrt{z}/x$ | 118.51 | 92.85 | 0.829 | 0.0772 | 0.0543 | 0.7055 | 0.2434 | 0.1711 | 0.749 |
| $a+bx^2/\sqrt{y}+c/x^2z$ | 119.59 | 94.24 | 0.826 | 0.0774 | 0.0540 | 0.7040 | 0.2437 | 0.1716 | 0.748 |
| $a+bx^2/\sqrt{y}+c/x^2z^2$ | 121.27 | 96.84 | 0.821 | 0.0774 | 0.0539 | 0.7044 | 0.2440 | 0.1727 | 0.748 |
| $a+bx^2/\sqrt{y}+c/x^2\sqrt{z}$ | 119.13 | 93.41 | 0.827 | 0.0774 | 0.0540 | 0.7038 | 0.2436 | 0.1712 | 0.749 |
| $a+bx^2/\sqrt{y}+cz/x^2$ | 118.30 | 91.97 | 0.830 | 0.0775 | 0.0541 | 0.7037 | 0.2433 | 0.1702 | 0.749 |
| $a+bx^2/\sqrt{y}+cz^2/x^2$ | 117.54 | 91.43 | 0.832 | 0.0774 | 0.0542 | 0.7042 | 0.2431 | 0.1701 | 0.750 |
| $a+bx^2/\sqrt{y}+c\sqrt{z}/x^2$ | 118.55 | 92.32 | 0.829 | 0.0775 | 0.0541 | 0.7037 | 0.2434 | 0.1705 | 0.749 |
| $a+bx^2/\sqrt{y}+c/\sqrt{x}z$ | 132.50 | 109.78 | 0.786 | 0.0778 | 0.0548 | 0.7014 | 0.2436 | 0.1691 | 0.749 |
| $a+bx^2/\sqrt{y}+c/\sqrt{x}z^2$ | 131.61 | 104.96 | 0.789 | 0.0778 | 0.0548 | 0.7014 | 0.2431 | 0.1684 | 0.750 |
| $a+bx^2/\sqrt{y}+c/\sqrt{x}\sqrt{z}$ | 129.25 | 107.11 | 0.797 | 0.0777 | 0.0544 | 0.7018 | 0.2445 | 0.1725 | 0.747 |
| $a+bx^2/\sqrt{y}+cz/\sqrt{x}$ | 107.69 | 84.81 | 0.859 | 0.0733 | 0.0523 | 0.7351 | 0.2362 | 0.1680 | 0.764 |
| $a+bx^2/\sqrt{y}+cz^2/\sqrt{x}$ | 106.62 | 82.16 | 0.862 | 0.0684 | 0.0468 | 0.7687 | 0.2300 | 0.1627 | 0.776 |

(continued on next page)

**Table 4 – continued from previous page**

| Functional form | $T_{eff}$ (K) | | | Radius ($R_\odot$) | | | log ($L/L_\odot$) | | |
|---|---|---|---|---|---|---|---|---|---|
| | RMSE | MAD | $R^2_{ap}$ | RMSE | MAD | $R^2_{ap}$ | RMSE | MAD | $R^2_{ap}$ |
| $a+bx^2/\sqrt{y}+c\sqrt{z}/\sqrt{x}$ | 114.69 | 90.10 | 0.840 | 0.0760 | 0.0542 | 0.7145 | 0.2414 | 0.1717 | 0.753 |
| $a+bx^2/\sqrt{y}+cy/z$ | 124.48 | 104.48 | 0.811 | 0.0753 | 0.0527 | 0.7199 | 0.2415 | 0.1716 | 0.753 |
| $a+bx^2/\sqrt{y}+cy/z^2$ | 127.66 | 105.62 | 0.802 | 0.0772 | 0.0546 | 0.7060 | 0.2437 | 0.1738 | 0.748 |
| $a+bx^2/\sqrt{y}+cy/\sqrt{z}$ | 126.37 | 105.74 | 0.806 | 0.0748 | 0.0533 | 0.7234 | 0.2414 | 0.1735 | 0.753 |
| $a+bx^2/\sqrt{y}+cyz$ | 114.06 | 87.09 | 0.842 | 0.0705 | 0.0469 | 0.7545 | 0.2361 | 0.1592 | 0.764 |
| $a+bx^2/\sqrt{y}+cyz^2$ | 113.19 | 88.32 | 0.844 | 0.0700 | 0.0486 | 0.7582 | 0.2354 | 0.1653 | 0.765 |
| $a+bx^2/\sqrt{y}+cy\sqrt{z}$ | 118.36 | 90.72 | 0.830 | 0.0730 | 0.0483 | 0.7367 | 0.2386 | 0.1591 | 0.759 |
| $a+bx^2/\sqrt{y}+cy^2/z$ | 127.46 | 106.45 | 0.802 | 0.0747 | 0.0527 | 0.7243 | 0.2412 | 0.1735 | 0.753 |
| $a+bx^2/\sqrt{y}+cy^2/z^2$ | 128.25 | 106.31 | 0.800 | 0.0768 | 0.0540 | 0.7091 | 0.2436 | 0.1742 | 0.748 |
| $a+bx^2/\sqrt{y}+cy^2/\sqrt{z}$ | 131.23 | 109.60 | 0.790 | 0.0756 | 0.0529 | 0.7180 | 0.2418 | 0.1749 | 0.752 |
| $a+bx^2/\sqrt{y}+cy^2z$ | 116.68 | 89.74 | 0.834 | 0.0728 | 0.0492 | 0.7382 | 0.2402 | 0.1649 | 0.756 |
| $a+bx^2/\sqrt{y}+cy^2z^2$ | 114.62 | 89.18 | 0.840 | 0.0717 | 0.0500 | 0.7458 | 0.2383 | 0.1660 | 0.759 |
| $a+bx^2/\sqrt{y}+cy^2\sqrt{z}$ | 120.75 | 92.97 | 0.823 | 0.0749 | 0.0506 | 0.7228 | 0.2425 | 0.1683 | 0.751 |
| $a+bx^2/\sqrt{y}+c\sqrt{y}/z$ | 122.74 | 102.40 | 0.817 | 0.0757 | 0.0527 | 0.7172 | 0.2409 | 0.1693 | 0.754 |
| $a+bx^2/\sqrt{y}+c\sqrt{y}/z^2$ | 127.20 | 104.84 | 0.803 | 0.0773 | 0.0549 | 0.7046 | 0.2434 | 0.1729 | 0.749 |
| $a+bx^2/\sqrt{y}+c\sqrt{y}/\sqrt{z}$ | 122.00 | 103.03 | 0.819 | 0.0745 | 0.0524 | 0.7263 | 0.2400 | 0.1700 | 0.756 |
| $a+bx^2/\sqrt{y}+c\sqrt{y}z$ | 112.43 | 87.19 | 0.846 | 0.0691 | 0.0447 | 0.7644 | 0.2329 | 0.1568 | 0.770 |
| $a+bx^2/\sqrt{y}+c\sqrt{y}z^2$ | 112.48 | 88.09 | 0.846 | 0.0690 | 0.0475 | 0.7652 | 0.2335 | 0.1645 | 0.769 |
| $a+bx^2/\sqrt{y}+c\sqrt{y}\sqrt{z}$ | 115.35 | 89.13 | 0.838 | 0.0711 | 0.0453 | 0.7504 | 0.2342 | 0.1513 | 0.768 |
| $a+bx^2/\sqrt{y}+c/yz$ | 132.14 | 106.55 | 0.788 | 0.0778 | 0.0548 | 0.7014 | 0.2425 | 0.1655 | 0.751 |
| $a+bx^2/\sqrt{y}+c/yz^2$ | 130.07 | 102.09 | 0.794 | 0.0778 | 0.0548 | 0.7014 | 0.2427 | 0.1667 | 0.751 |
| $a+bx^2/\sqrt{y}+c/y\sqrt{z}$ | 132.79 | 109.28 | 0.785 | 0.0777 | 0.0546 | 0.7016 | 0.2435 | 0.1673 | 0.749 |
| $a+bx^2/\sqrt{y}+cz/y$ | 115.37 | 94.96 | 0.838 | 0.0732 | 0.0521 | 0.7351 | 0.2370 | 0.1711 | 0.762 |
| $a+bx^2/\sqrt{y}+cz^2/y$ | 110.38 | 87.43 | 0.852 | 0.0682 | 0.0468 | 0.7704 | 0.2292 | 0.1640 | 0.777 |
| $a+bx^2/\sqrt{y}+c\sqrt{z}/y$ | 123.24 | 101.38 | 0.815 | 0.0761 | 0.0538 | 0.7140 | 0.2427 | 0.1731 | 0.750 |
| $a+bx^2/\sqrt{y}+c/y^2z$ | 132.55 | 109.38 | 0.786 | 0.0775 | 0.0539 | 0.7031 | 0.2442 | 0.1700 | 0.747 |
| $a+bx^2/\sqrt{y}+c/y^2z^2$ | 132.49 | 107.88 | 0.786 | 0.0776 | 0.0540 | 0.7026 | 0.2437 | 0.1677 | 0.748 |
| $a+bx^2/\sqrt{y}+c/y^2\sqrt{z}$ | 131.34 | 108.56 | 0.790 | 0.0775 | 0.0538 | 0.7036 | 0.2445 | 0.1719 | 0.747 |
| $a+bx^2/\sqrt{y}+cz/y^2$ | 121.82 | 99.04 | 0.819 | 0.0767 | 0.0540 | 0.7093 | 0.2433 | 0.1728 | 0.749 |
| $a+bx^2/\sqrt{y}+cz^2/y^2$ | 113.04 | 90.13 | 0.845 | 0.0738 | 0.0533 | 0.7312 | 0.2369 | 0.1713 | 0.762 |
| $a+bx^2/\sqrt{y}+c\sqrt{z}/y^2$ | 125.67 | 102.48 | 0.808 | 0.0772 | 0.0536 | 0.7060 | 0.2444 | 0.1742 | 0.747 |
| $a+bx^2/\sqrt{y}+c/\sqrt{y}z$ | 127.93 | 99.28 | 0.801 | 0.0775 | 0.0551 | 0.7036 | 0.2403 | 0.1626 | 0.755 |
| $a+bx^2/\sqrt{y}+c/\sqrt{y}z^2$ | 127.90 | 101.58 | 0.801 | 0.0777 | 0.0552 | 0.7018 | 0.2425 | 0.1681 | 0.751 |
| $a+bx^2/\sqrt{y}+c/\sqrt{y}\sqrt{z}$ | 130.36 | 102.28 | 0.793 | 0.0775 | 0.0551 | 0.7037 | 0.2403 | 0.1615 | 0.755 |
| $a+bx^2/\sqrt{y}+cz/\sqrt{y}$ | 111.47 | 90.18 | 0.849 | 0.0697 | 0.0479 | 0.7599 | 0.2313 | 0.1640 | 0.773 |
| $a+bx^2/\sqrt{y}+cz^2/\sqrt{y}$ | 111.08 | 87.76 | 0.850 | 0.0676 | 0.0463 | 0.7747 | 0.2296 | 0.1625 | 0.777 |
| $a+bx^2/\sqrt{y}+c\sqrt{z}/\sqrt{y}$ | 117.22 | 97.86 | 0.833 | 0.0733 | 0.0521 | 0.7345 | 0.2376 | 0.1709 | 0.761 |
| $a+bx^2y+cx/z$ | 139.23 | 109.62 | 0.764 | 0.0854 | 0.0640 | 0.6399 | 0.2927 | 0.2160 | 0.637 |
| $a+bx^2y+cx/z^2$ | 138.39 | 109.86 | 0.767 | 0.0854 | 0.0641 | 0.6398 | 0.2932 | 0.2192 | 0.636 |
| $a+bx^2y+cx/\sqrt{z}$ | 140.13 | 111.31 | 0.761 | 0.0854 | 0.0631 | 0.6401 | 0.2868 | 0.2073 | 0.651 |
| $a+bx^2y+cxz$ | 124.20 | 94.14 | 0.812 | 0.0733 | 0.0525 | 0.7346 | 0.2684 | 0.2049 | 0.695 |
| $a+bx^2y+cxz^2$ | 132.65 | 104.13 | 0.786 | 0.0799 | 0.0602 | 0.6848 | 0.2869 | 0.2191 | 0.651 |
| $a+bx^2y+cx\sqrt{z}$ | 116.93 | 90.54 | 0.834 | 0.0686 | 0.0418 | 0.7677 | 0.2390 | 0.1546 | 0.758 |
| $a+bx^2y+cx^2/z$ | 140.10 | 110.73 | 0.761 | 0.0855 | 0.0639 | 0.6392 | 0.2908 | 0.2143 | 0.642 |
| $a+bx^2y+cx^2/z^2$ | 139.56 | 110.11 | 0.763 | 0.0855 | 0.0640 | 0.6393 | 0.2929 | 0.2168 | 0.636 |
| $a+bx^2y+cx^2/\sqrt{z}$ | 139.53 | 111.02 | 0.763 | 0.0853 | 0.0629 | 0.6410 | 0.2831 | 0.2074 | 0.660 |
| $a+bx^2y+cx^2z$ | 132.49 | 103.39 | 0.786 | 0.0793 | 0.0600 | 0.6893 | 0.2858 | 0.2194 | 0.654 |
| $a+bx^2y+cx^2z^2$ | 136.53 | 108.36 | 0.773 | 0.0829 | 0.0632 | 0.6603 | 0.2921 | 0.2182 | 0.638 |
| $a+bx^2y+cx^2\sqrt{z}$ | 123.78 | 94.80 | 0.814 | 0.0729 | 0.0547 | 0.7376 | 0.2653 | 0.2029 | 0.702 |
| $a+bx^2y+c\sqrt{x}/z$ | 136.00 | 107.67 | 0.775 | 0.0849 | 0.0638 | 0.6440 | 0.2928 | 0.2200 | 0.637 |
| $a+bx^2y+c\sqrt{x}/z^2$ | 136.15 | 108.44 | 0.774 | 0.0852 | 0.0642 | 0.6417 | 0.2922 | 0.2199 | 0.638 |
| $a+bx^2y+c\sqrt{x}/\sqrt{z}$ | 139.07 | 108.79 | 0.765 | 0.0855 | 0.0639 | 0.6393 | 0.2922 | 0.2142 | 0.638 |
| $a+bx^2y+c\sqrt{x}z$ | 121.82 | 91.73 | 0.819 | 0.0721 | 0.0490 | 0.7435 | 0.2628 | 0.1965 | 0.707 |
| $a+bx^2y+c\sqrt{x}z^2$ | 130.39 | 100.88 | 0.793 | 0.0783 | 0.0580 | 0.6976 | 0.2831 | 0.2166 | 0.660 |
| $a+bx^2y+c\sqrt{x}\sqrt{z}$ | 118.09 | 91.93 | 0.830 | 0.0696 | 0.0417 | 0.7607 | 0.2403 | 0.1497 | 0.755 |
| $a+bx^2y+c/xz$ | 138.94 | 110.79 | 0.765 | 0.0826 | 0.0597 | 0.6635 | 0.2754 | 0.1932 | 0.679 |
| $a+bx^2y+c/xz^2$ | 134.96 | 105.44 | 0.778 | 0.0822 | 0.0588 | 0.6661 | 0.2697 | 0.1851 | 0.692 |
| $a+bx^2y+c/x\sqrt{z}$ | 139.88 | 111.48 | 0.762 | 0.0830 | 0.0604 | 0.6597 | 0.2793 | 0.1978 | 0.669 |
| $a+bx^2y+cz/x$ | 138.96 | 107.77 | 0.765 | 0.0849 | 0.0621 | 0.6439 | 0.2897 | 0.2069 | 0.644 |
| $a+bx^2y+cz^2/x$ | 134.03 | 105.74 | 0.781 | 0.0853 | 0.0636 | 0.6410 | 0.2933 | 0.2190 | 0.636 |
| $a+bx^2y+c\sqrt{z}/x$ | 139.87 | 109.90 | 0.762 | 0.0842 | 0.0612 | 0.6496 | 0.2866 | 0.2048 | 0.652 |
| $a+bx^2y+c/x^2z$ | 139.95 | 110.14 | 0.762 | 0.0840 | 0.0612 | 0.6517 | 0.2861 | 0.2046 | 0.653 |
| $a+bx^2y+c/x^2z^2$ | 140.16 | 111.17 | 0.761 | 0.0837 | 0.0609 | 0.6544 | 0.2833 | 0.2017 | 0.660 |
| $a+bx^2y+c/x^2\sqrt{z}$ | 139.77 | 109.66 | 0.762 | 0.0841 | 0.0613 | 0.6507 | 0.2870 | 0.2054 | 0.651 |
| $a+bx^2y+cz/x^2$ | 139.25 | 108.49 | 0.764 | 0.0844 | 0.0614 | 0.6484 | 0.2887 | 0.2065 | 0.647 |
| $a+bx^2y+cz^2/x^2$ | 138.89 | 107.77 | 0.765 | 0.0846 | 0.0615 | 0.6468 | 0.2896 | 0.2069 | 0.645 |
| $a+bx^2y+c\sqrt{z}/x^2$ | 139.41 | 108.84 | 0.764 | 0.0843 | 0.0614 | 0.6491 | 0.2883 | 0.2062 | 0.648 |
| $a+bx^2y+c/\sqrt{x}z$ | 130.82 | 100.19 | 0.792 | 0.0802 | 0.0575 | 0.6821 | 0.2602 | 0.1751 | 0.713 |
| $a+bx^2y+c/\sqrt{x}z^2$ | 126.85 | 98.41 | 0.804 | 0.0823 | 0.0602 | 0.6656 | 0.2691 | 0.1837 | 0.693 |
| $a+bx^2y+c/\sqrt{x}\sqrt{z}$ | 135.83 | 106.84 | 0.776 | 0.0808 | 0.0576 | 0.6780 | 0.2655 | 0.1831 | 0.701 |
| $a+bx^2y+cz/\sqrt{x}$ | 132.93 | 105.88 | 0.785 | 0.0848 | 0.0631 | 0.6453 | 0.2928 | 0.2201 | 0.637 |
| $a+bx^2y+cz^2/\sqrt{x}$ | 126.96 | 96.05 | 0.804 | 0.0795 | 0.0587 | 0.6881 | 0.2840 | 0.2169 | 0.658 |
| $a+bx^2y+c\sqrt{z}/\sqrt{x}$ | 138.97 | 107.68 | 0.765 | 0.0853 | 0.0629 | 0.6411 | 0.2903 | 0.2084 | 0.643 |
| $a+bx^2y+cy/z$ | 135.45 | 106.78 | 0.777 | 0.0840 | 0.0634 | 0.6512 | 0.2916 | 0.2193 | 0.640 |
| $a+bx^2y+cy/z^2$ | 136.29 | 108.34 | 0.774 | 0.0850 | 0.0643 | 0.6433 | 0.2920 | 0.2195 | 0.639 |
| $a+bx^2y+cy/\sqrt{z}$ | 137.79 | 107.61 | 0.769 | 0.0845 | 0.0638 | 0.6476 | 0.2931 | 0.2195 | 0.636 |
| $a+bx^2y+cyz$ | 129.81 | 98.48 | 0.795 | 0.0782 | 0.0555 | 0.6981 | 0.2814 | 0.2080 | 0.665 |
| $a+bx^2y+cyz^2$ | 133.98 | 104.57 | 0.782 | 0.0811 | 0.0606 | 0.6751 | 0.2892 | 0.2175 | 0.646 |
| $a+bx^2y+cy\sqrt{z}$ | 128.85 | 99.15 | 0.798 | 0.0783 | 0.0508 | 0.6975 | 0.2736 | 0.1861 | 0.683 |
| $a+bx^2y+cy^2/z$ | 136.93 | 107.79 | 0.772 | 0.0837 | 0.0632 | 0.6544 | 0.2921 | 0.2192 | 0.638 |
| $a+bx^2y+cy^2/z^2$ | 137.67 | 109.19 | 0.769 | 0.0850 | 0.0643 | 0.6436 | 0.2928 | 0.2196 | 0.637 |
| $a+bx^2y+cy^2/\sqrt{z}$ | 137.77 | 107.65 | 0.769 | 0.0836 | 0.0634 | 0.6548 | 0.2923 | 0.2194 | 0.638 |
| $a+bx^2y+cy^2z$ | 137.40 | 106.89 | 0.770 | 0.0835 | 0.0615 | 0.6554 | 0.2927 | 0.2173 | 0.637 |
| $a+bx^2y+cy^2z^2$ | 137.56 | 108.33 | 0.770 | 0.0839 | 0.0631 | 0.6527 | 0.2930 | 0.2183 | 0.636 |
| $a+bx^2y+cy^2\sqrt{z}$ | 138.52 | 107.53 | 0.767 | 0.0845 | 0.0612 | 0.6473 | 0.2928 | 0.2168 | 0.637 |
| $a+bx^2y+c\sqrt{y}/z$ | 131.56 | 103.69 | 0.789 | 0.0834 | 0.0625 | 0.6569 | 0.2879 | 0.2153 | 0.649 |
| $a+bx^2y+c\sqrt{y}/z^2$ | 134.19 | 106.75 | 0.781 | 0.0848 | 0.0640 | 0.6451 | 0.2901 | 0.2179 | 0.643 |
| $a+bx^2y+c\sqrt{y}/\sqrt{z}$ | 134.14 | 104.87 | 0.781 | 0.0836 | 0.0627 | 0.6551 | 0.2910 | 0.2192 | 0.641 |
| $a+bx^2y+c\sqrt{y}z$ | 124.89 | 94.19 | 0.810 | 0.0754 | 0.0519 | 0.7194 | 0.2728 | 0.2039 | 0.685 |

(continued on next page)

**Table 4 – continued from previous page**

| Functional form | $T_{eff}$ (K) | | | Radius ($R_\odot$) | | | log (L/$L_\odot$) | | |
|---|---|---|---|---|---|---|---|---|---|
| | RMSE | MAD | $R^2_{ap}$ | RMSE | MAD | $R^2_{ap}$ | RMSE | MAD | $R^2_{ap}$ |
| $a+bx^2y+c\sqrt{y}z^2$ | 131.30 | 101.36 | 0.790 | 0.0792 | 0.0585 | 0.6903 | 0.2851 | 0.2166 | 0.656 |
| $a+bx^2y+c\sqrt{y}\sqrt{z}$ | 122.04 | 95.32 | 0.819 | 0.0747 | 0.0462 | 0.7243 | 0.2614 | 0.1764 | 0.710 |
| $a+bx^2y+c/yz$ | 126.74 | 96.36 | 0.805 | 0.0816 | 0.0591 | 0.6712 | 0.2633 | 0.1756 | 0.706 |
| $a+bx^2y+c/yz^2$ | 125.06 | 95.67 | 0.810 | 0.0830 | 0.0612 | 0.6595 | 0.2716 | 0.1874 | 0.687 |
| $a+bx^2y+c/y\sqrt{z}$ | 131.26 | 101.02 | 0.790 | 0.0817 | 0.0578 | 0.6706 | 0.2648 | 0.1754 | 0.703 |
| $a+bx^2y+cz/y$ | 131.72 | 104.12 | 0.789 | 0.0835 | 0.0621 | 0.6559 | 0.2909 | 0.2201 | 0.641 |
| $a+bx^2y+cz^2/y$ | 123.24 | 91.78 | 0.815 | 0.0767 | 0.0557 | 0.7092 | 0.2765 | 0.2126 | 0.676 |
| $a+bx^2y+c\sqrt{z}/y$ | 139.65 | 109.28 | 0.763 | 0.0855 | 0.0634 | 0.6393 | 0.2908 | 0.2099 | 0.642 |
| $a+bx^2y+c/y^2z$ | 132.43 | 103.31 | 0.787 | 0.0827 | 0.0594 | 0.6626 | 0.2694 | 0.1787 | 0.692 |
| $a+bx^2y+c/y^2z^2$ | 128.70 | 97.31 | 0.798 | 0.0832 | 0.0610 | 0.6584 | 0.2711 | 0.1861 | 0.688 |
| $a+bx^2y+c/y^2\sqrt{z}$ | 135.16 | 107.03 | 0.778 | 0.0827 | 0.0584 | 0.6623 | 0.2711 | 0.1803 | 0.689 |
| $a+bx^2y+cz/y^2$ | 139.95 | 110.07 | 0.762 | 0.0850 | 0.0621 | 0.6430 | 0.2883 | 0.2039 | 0.648 |
| $a+bx^2y+cz^2/y^2$ | 131.87 | 104.36 | 0.788 | 0.0843 | 0.0628 | 0.6493 | 0.2920 | 0.2208 | 0.639 |
| $a+bx^2y+c\sqrt{z}/y^2$ | 139.79 | 111.60 | 0.762 | 0.0840 | 0.0597 | 0.6516 | 0.2815 | 0.1970 | 0.664 |
| $a+bx^2y+c/\sqrt{y}z$ | 122.00 | 94.92 | 0.819 | 0.0809 | 0.0584 | 0.6769 | 0.2630 | 0.1737 | 0.707 |
| $a+bx^2y+c/\sqrt{y}z^2$ | 126.18 | 98.22 | 0.806 | 0.0835 | 0.0616 | 0.6556 | 0.2776 | 0.1981 | 0.673 |
| $a+bx^2y+c/\sqrt{y}\sqrt{z}$ | 124.63 | 96.36 | 0.811 | 0.0799 | 0.0562 | 0.6848 | 0.2578 | 0.1643 | 0.718 |
| $a+bx^2y+cz/\sqrt{y}$ | 122.58 | 93.60 | 0.817 | 0.0776 | 0.0553 | 0.7027 | 0.2769 | 0.2097 | 0.675 |
| $a+bx^2y+cz^2/\sqrt{y}$ | 125.09 | 93.73 | 0.810 | 0.0761 | 0.0551 | 0.7142 | 0.2763 | 0.2115 | 0.677 |
| $a+bx^2y+c\sqrt{z}/\sqrt{y}$ | 132.16 | 104.27 | 0.788 | 0.0833 | 0.0620 | 0.6576 | 0.2906 | 0.2196 | 0.642 |
| $a+bx^2y^2+cx/z$ | 156.74 | 120.83 | 0.701 | 0.0933 | 0.0716 | 0.5701 | 0.3247 | 0.2407 | 0.553 |
| $a+bx^2y^2+cx/z^2$ | 154.69 | 121.17 | 0.709 | 0.0931 | 0.0721 | 0.5724 | 0.3253 | 0.2435 | 0.552 |
| $a+bx^2y^2+cx/\sqrt{z}$ | 154.84 | 123.88 | 0.708 | 0.0920 | 0.0705 | 0.5824 | 0.3101 | 0.2308 | 0.593 |
| $a+bx^2y^2+cxz$ | 127.43 | 95.39 | 0.802 | 0.0729 | 0.0518 | 0.7375 | 0.2705 | 0.2067 | 0.690 |
| $a+bx^2y^2+cxz^2$ | 144.55 | 111.08 | 0.746 | 0.0838 | 0.0644 | 0.6531 | 0.3082 | 0.2422 | 0.597 |
| $a+bx^2y^2+cx\sqrt{z}$ | 117.01 | 90.36 | 0.833 | 0.0685 | 0.0423 | 0.7683 | 0.2362 | 0.1518 | 0.764 |
| $a+bx^2y^2+cx^2/z$ | 156.37 | 123.87 | 0.703 | 0.0931 | 0.0713 | 0.5721 | 0.3181 | 0.2428 | 0.571 |
| $a+bx^2y^2+cx^2/z^2$ | 156.60 | 120.31 | 0.702 | 0.0933 | 0.0718 | 0.5702 | 0.3254 | 0.2411 | 0.551 |
| $a+bx^2y^2+cx^2/\sqrt{z}$ | 149.27 | 120.17 | 0.729 | 0.0900 | 0.0686 | 0.5997 | 0.2955 | 0.2233 | 0.630 |
| $a+bx^2y^2+cx^2z$ | 137.83 | 104.88 | 0.769 | 0.0790 | 0.0618 | 0.6917 | 0.2934 | 0.2349 | 0.635 |
| $a+bx^2y^2+cx^2z^2$ | 150.72 | 117.20 | 0.724 | 0.0883 | 0.0672 | 0.6152 | 0.3191 | 0.2438 | 0.569 |
| $a+bx^2y^2+cx^2\sqrt{z}$ | 121.60 | 94.03 | 0.820 | 0.0700 | 0.0514 | 0.7579 | 0.2520 | 0.1926 | 0.731 |
| $a+bx^2y^2+c\sqrt{x}/z$ | 152.16 | 121.13 | 0.718 | 0.0924 | 0.0713 | 0.5785 | 0.3243 | 0.2430 | 0.555 |
| $a+bx^2y^2+c\sqrt{x}/z^2$ | 151.02 | 119.67 | 0.723 | 0.0925 | 0.0719 | 0.5780 | 0.3225 | 0.2426 | 0.559 |
| $a+bx^2y^2+c\sqrt{x}/\sqrt{z}$ | 156.90 | 121.60 | 0.700 | 0.0933 | 0.0714 | 0.5701 | 0.3233 | 0.2396 | 0.557 |
| $a+bx^2y^2+c\sqrt{x}z$ | 125.61 | 95.02 | 0.808 | 0.0724 | 0.0493 | 0.7410 | 0.2670 | 0.1998 | 0.698 |
| $a+bx^2y^2+c\sqrt{x}z^2$ | 141.51 | 107.20 | 0.756 | 0.0819 | 0.0621 | 0.6691 | 0.3026 | 0.2380 | 0.612 |
| $a+bx^2y^2+c\sqrt{x}\sqrt{z}$ | 118.62 | 91.38 | 0.829 | 0.0696 | 0.0418 | 0.7607 | 0.2401 | 0.1472 | 0.756 |
| $a+bx^2y^2+c/xz$ | 150.46 | 120.00 | 0.725 | 0.0867 | 0.0640 | 0.6291 | 0.2921 | 0.2048 | 0.638 |
| $a+bx^2y^2+c/xz^2$ | 142.97 | 110.79 | 0.751 | 0.0859 | 0.0626 | 0.6353 | 0.2837 | 0.1942 | 0.659 |
| $a+bx^2y^2+c/x\sqrt{z}$ | 153.34 | 122.65 | 0.714 | 0.0876 | 0.0652 | 0.6207 | 0.2985 | 0.2096 | 0.622 |
| $a+bx^2y^2+cz/x$ | 157.07 | 122.35 | 0.700 | 0.0915 | 0.0683 | 0.5862 | 0.3172 | 0.2237 | 0.574 |
| $a+bx^2y^2+cz^2/x$ | 153.50 | 122.31 | 0.713 | 0.0933 | 0.0715 | 0.5704 | 0.3256 | 0.2421 | 0.551 |
| $a+bx^2y^2+c\sqrt{z}/x$ | 156.62 | 123.81 | 0.702 | 0.0901 | 0.0670 | 0.5990 | 0.3112 | 0.2200 | 0.590 |
| $a+bx^2y^2+c/x^2z$ | 156.53 | 123.83 | 0.702 | 0.0898 | 0.0669 | 0.6022 | 0.3106 | 0.2195 | 0.591 |
| $a+bx^2y^2+c/x^2z^2$ | 155.39 | 123.93 | 0.706 | 0.0890 | 0.0662 | 0.6086 | 0.3058 | 0.2153 | 0.604 |
| $a+bx^2y^2+c/x^2\sqrt{z}$ | 156.78 | 123.59 | 0.701 | 0.0900 | 0.0671 | 0.5997 | 0.3122 | 0.2207 | 0.587 |
| $a+bx^2y^2+cz/x^2$ | 157.05 | 122.79 | 0.700 | 0.0906 | 0.0673 | 0.5944 | 0.3154 | 0.2225 | 0.578 |
| $a+bx^2y^2+cz^2/x^2$ | 157.06 | 122.22 | 0.700 | 0.0910 | 0.0675 | 0.5909 | 0.3170 | 0.2232 | 0.574 |
| $a+bx^2y^2+c\sqrt{z}/x^2$ | 157.01 | 123.05 | 0.700 | 0.0905 | 0.0673 | 0.5959 | 0.3146 | 0.2221 | 0.581 |
| $a+bx^2y^2+c/\sqrt{x}z$ | 135.17 | 102.83 | 0.778 | 0.0824 | 0.0600 | 0.6645 | 0.2684 | 0.1800 | 0.695 |
| $a+bx^2y^2+c/\sqrt{x}z^2$ | 132.00 | 101.41 | 0.788 | 0.0860 | 0.0644 | 0.6346 | 0.2828 | 0.1936 | 0.661 |
| $a+bx^2y^2+c/\sqrt{x}\sqrt{z}$ | 143.16 | 111.37 | 0.751 | 0.0833 | 0.0605 | 0.6571 | 0.2759 | 0.1903 | 0.678 |
| $a+bx^2y^2+cz/\sqrt{x}$ | 151.45 | 120.38 | 0.721 | 0.0927 | 0.0708 | 0.5755 | 0.3253 | 0.2431 | 0.552 |
| $a+bx^2y^2+cz^2/\sqrt{x}$ | 140.63 | 108.00 | 0.759 | 0.0851 | 0.0622 | 0.6421 | 0.3094 | 0.2382 | 0.594 |
| $a+bx^2y^2+c\sqrt{z}/\sqrt{x}$ | 157.06 | 122.22 | 0.700 | 0.0922 | 0.0695 | 0.5801 | 0.3184 | 0.2273 | 0.571 |
| $a+bx^2y^2+cy/z$ | 151.97 | 119.80 | 0.719 | 0.0916 | 0.0708 | 0.5860 | 0.3232 | 0.2414 | 0.558 |
| $a+bx^2y^2+cy/z^2$ | 151.34 | 119.30 | 0.721 | 0.0922 | 0.0719 | 0.5801 | 0.3223 | 0.2418 | 0.560 |
| $a+bx^2y^2+cy/\sqrt{z}$ | 156.33 | 121.12 | 0.703 | 0.0930 | 0.0717 | 0.5732 | 0.3256 | 0.2421 | 0.551 |
| $a+bx^2y^2+cyz$ | 135.62 | 103.04 | 0.776 | 0.0789 | 0.0568 | 0.6926 | 0.2900 | 0.2230 | 0.644 |
| $a+bx^2y^2+cyz^2$ | 147.06 | 111.63 | 0.737 | 0.0858 | 0.0640 | 0.6367 | 0.3132 | 0.2401 | 0.584 |
| $a+bx^2y^2+cy\sqrt{z}$ | 130.95 | 100.19 | 0.791 | 0.0780 | 0.0478 | 0.6994 | 0.2730 | 0.1789 | 0.684 |
| $a+bx^2y^2+cy^2/z$ | 155.30 | 120.39 | 0.707 | 0.0922 | 0.0712 | 0.5805 | 0.3253 | 0.2424 | 0.552 |
| $a+bx^2y^2+cy^2/z^2$ | 154.06 | 120.48 | 0.711 | 0.0925 | 0.0721 | 0.5773 | 0.3246 | 0.2427 | 0.554 |
| $a+bx^2y^2+cy^2/\sqrt{z}$ | 156.95 | 121.91 | 0.700 | 0.0930 | 0.0718 | 0.5725 | 0.3253 | 0.2425 | 0.552 |
| $a+bx^2y^2+cy^2z$ | 147.72 | 110.70 | 0.734 | 0.0864 | 0.0635 | 0.6314 | 0.3136 | 0.2362 | 0.583 |
| $a+bx^2y^2+cy^2z^2$ | 152.97 | 117.06 | 0.715 | 0.0901 | 0.0680 | 0.5992 | 0.3227 | 0.2416 | 0.559 |
| $a+bx^2y^2+cy^2\sqrt{z}$ | 144.53 | 104.49 | 0.746 | 0.0856 | 0.0590 | 0.6380 | 0.3034 | 0.2142 | 0.610 |
| $a+bx^2y^2+c\sqrt{y}/z$ | 144.77 | 114.60 | 0.745 | 0.0897 | 0.0687 | 0.6030 | 0.3151 | 0.2331 | 0.579 |
| $a+bx^2y^2+c\sqrt{y}/z^2$ | 147.63 | 116.62 | 0.735 | 0.0916 | 0.0713 | 0.5861 | 0.3182 | 0.2384 | 0.571 |
| $a+bx^2y^2+c\sqrt{y}/\sqrt{z}$ | 150.93 | 119.30 | 0.723 | 0.0912 | 0.0700 | 0.5896 | 0.3226 | 0.2417 | 0.559 |
| $a+bx^2y^2+c\sqrt{y}z$ | 130.26 | 99.44 | 0.794 | 0.0764 | 0.0537 | 0.7118 | 0.2808 | 0.2143 | 0.666 |
| $a+bx^2y^2+c\sqrt{y}z^2$ | 143.20 | 108.46 | 0.751 | 0.0833 | 0.0628 | 0.6576 | 0.3064 | 0.2388 | 0.602 |
| $a+bx^2y^2+c\sqrt{y}\sqrt{z}$ | 124.03 | 95.84 | 0.813 | 0.0749 | 0.0446 | 0.7230 | 0.2626 | 0.1728 | 0.708 |
| $a+bx^2y^2+c/yz$ | 130.74 | 97.93 | 0.792 | 0.0847 | 0.0625 | 0.6460 | 0.2739 | 0.1843 | 0.682 |
| $a+bx^2y^2+c/yz^2$ | 130.91 | 98.55 | 0.792 | 0.0875 | 0.0663 | 0.6221 | 0.2877 | 0.2013 | 0.649 |
| $a+bx^2y^2+c/y\sqrt{z}$ | 136.53 | 104.06 | 0.773 | 0.0846 | 0.0607 | 0.6463 | 0.2752 | 0.1824 | 0.679 |
| $a+bx^2y^2+cz/y$ | 150.02 | 119.02 | 0.726 | 0.0915 | 0.0697 | 0.5864 | 0.3235 | 0.2431 | 0.557 |
| $a+bx^2y^2+cz^2/y$ | 135.48 | 103.08 | 0.777 | 0.0818 | 0.0598 | 0.6698 | 0.2996 | 0.2339 | 0.620 |
| $a+bx^2y^2+c\sqrt{z}/y$ | 156.92 | 123.39 | 0.700 | 0.0926 | 0.0697 | 0.5764 | 0.3183 | 0.2284 | 0.571 |
| $a+bx^2y^2+c/y^2z$ | 139.87 | 108.77 | 0.762 | 0.0868 | 0.0635 | 0.6281 | 0.2844 | 0.1880 | 0.657 |
| $a+bx^2y^2+c/y^2z^2$ | 135.91 | 102.14 | 0.775 | 0.0879 | 0.0662 | 0.6186 | 0.2883 | 0.2005 | 0.648 |
| $a+bx^2y^2+c/y^2\sqrt{z}$ | 143.74 | 113.72 | 0.749 | 0.0868 | 0.0621 | 0.6280 | 0.2864 | 0.1883 | 0.653 |
| $a+bx^2y^2+cz/y^2$ | 156.55 | 123.91 | 0.702 | 0.0914 | 0.0678 | 0.5871 | 0.3137 | 0.2198 | 0.583 |
| $a+bx^2y^2+cz^2/y^2$ | 151.12 | 120.03 | 0.722 | 0.0925 | 0.0707 | 0.5777 | 0.3250 | 0.2436 | 0.553 |
| $a+bx^2y^2+c\sqrt{z}/y^2$ | 153.25 | 122.97 | 0.714 | 0.0892 | 0.0649 | 0.6070 | 0.3020 | 0.2105 | 0.614 |
| $a+bx^2y^2+c/\sqrt{y}z$ | 124.83 | 94.94 | 0.810 | 0.0836 | 0.0613 | 0.6548 | 0.2729 | 0.1808 | 0.685 |
| $a+bx^2y^2+c/\sqrt{y}z^2$ | 133.54 | 101.68 | 0.783 | 0.0885 | 0.0668 | 0.6136 | 0.2965 | 0.2116 | 0.628 |
| $a+bx^2y^2+c/\sqrt{y}\sqrt{z}$ | 126.77 | 96.73 | 0.804 | 0.0818 | 0.0581 | 0.6699 | 0.2643 | 0.1684 | 0.704 |

(continued on next page)

**Table 4 – continued from previous page**

| Functional form | $T_{eff}$ (K) | | | Radius ($R_{\odot}$) | | | log (L/$L_{\odot}$) | | |
|---|---|---|---|---|---|---|---|---|---|
| | RMSE | MAD | $R^2_{ap}$ | RMSE | MAD | $R^2_{ap}$ | RMSE | MAD | $R^2_{ap}$ |
| $a+bx^2y^2+cz/\sqrt{y}$ | 133.92 | 102.28 | 0.782 | 0.0824 | 0.0587 | 0.6645 | 0.2991 | 0.2288 | 0.621 |
| $a+bx^2y^2+cz^2/\sqrt{y}$ | 136.01 | 102.04 | 0.775 | 0.0801 | 0.0594 | 0.6830 | 0.2961 | 0.2327 | 0.629 |
| $a+bx^2y^2+c\sqrt{z}/\sqrt{y}$ | 149.90 | 118.82 | 0.727 | 0.0912 | 0.0693 | 0.5897 | 0.3229 | 0.2428 | 0.558 |
| $a+bx^2\sqrt{y}+cx/z$ | 129.82 | 103.38 | 0.795 | 0.0810 | 0.0592 | 0.6763 | 0.2735 | 0.2000 | 0.683 |
| $a+bx^2\sqrt{y}+cx/z^2$ | 129.92 | 103.21 | 0.795 | 0.0812 | 0.0592 | 0.6745 | 0.2736 | 0.2015 | 0.683 |
| $a+bx^2\sqrt{y}+cx/\sqrt{z}$ | 131.13 | 103.38 | 0.791 | 0.0812 | 0.0591 | 0.6742 | 0.2715 | 0.1927 | 0.688 |
| $a+bx^2\sqrt{y}+cxz$ | 120.69 | 92.75 | 0.823 | 0.0727 | 0.0516 | 0.7387 | 0.2611 | 0.1945 | 0.711 |
| $a+bx^2\sqrt{y}+cxz^2$ | 124.82 | 98.50 | 0.810 | 0.0767 | 0.0575 | 0.7099 | 0.2699 | 0.2008 | 0.691 |
| $a+bx^2\sqrt{y}+cx\sqrt{z}$ | 116.73 | 90.75 | 0.834 | 0.0689 | 0.0419 | 0.7657 | 0.2412 | 0.1589 | 0.753 |
| $a+bx^2\sqrt{y}+cx^2/z$ | 130.71 | 104.03 | 0.792 | 0.0808 | 0.0593 | 0.6775 | 0.2731 | 0.1987 | 0.684 |
| $a+bx^2\sqrt{y}+cx^2/z^2$ | 130.82 | 103.75 | 0.792 | 0.0812 | 0.0592 | 0.6745 | 0.2734 | 0.1998 | 0.683 |
| $a+bx^2\sqrt{y}+cx^2/\sqrt{z}$ | 131.39 | 104.38 | 0.790 | 0.0811 | 0.0592 | 0.6755 | 0.2715 | 0.1951 | 0.688 |
| $a+bx^2\sqrt{y}+cx^2z$ | 126.64 | 100.98 | 0.805 | 0.0775 | 0.0581 | 0.7032 | 0.2716 | 0.2003 | 0.687 |
| $a+bx^2\sqrt{y}+cx^2z^2$ | 127.86 | 102.42 | 0.801 | 0.0791 | 0.0595 | 0.6913 | 0.2731 | 0.2011 | 0.684 |
| $a+bx^2\sqrt{y}+cx^2\sqrt{z}$ | 123.67 | 97.00 | 0.814 | 0.0748 | 0.0551 | 0.7234 | 0.2664 | 0.2000 | 0.699 |
| $a+bx^2\sqrt{y}+c\sqrt{x}/z$ | 127.19 | 101.30 | 0.803 | 0.0807 | 0.0590 | 0.6787 | 0.2732 | 0.2027 | 0.684 |
| $a+bx^2\sqrt{y}+c\sqrt{x}/z^2$ | 128.29 | 101.95 | 0.800 | 0.0811 | 0.0592 | 0.6753 | 0.2731 | 0.2025 | 0.684 |
| $a+bx^2\sqrt{y}+c\sqrt{x}/\sqrt{z}$ | 129.10 | 102.26 | 0.797 | 0.0810 | 0.0592 | 0.6760 | 0.2734 | 0.1993 | 0.683 |
| $a+bx^2\sqrt{y}+c\sqrt{x}z$ | 118.48 | 91.02 | 0.829 | 0.0713 | 0.0482 | 0.7491 | 0.2557 | 0.1864 | 0.723 |
| $a+bx^2\sqrt{y}+c\sqrt{x}z^2$ | 123.01 | 96.11 | 0.816 | 0.0753 | 0.0557 | 0.7203 | 0.2671 | 0.2004 | 0.698 |
| $a+bx^2\sqrt{y}+c\sqrt{x}\sqrt{z}$ | 117.52 | 91.62 | 0.832 | 0.0696 | 0.0418 | 0.7609 | 0.2397 | 0.1514 | 0.757 |
| $a+bx^2\sqrt{y}+c/xz$ | 131.79 | 104.41 | 0.789 | 0.0801 | 0.0568 | 0.6833 | 0.2643 | 0.1867 | 0.704 |
| $a+bx^2\sqrt{y}+c/xz^2$ | 130.34 | 101.66 | 0.793 | 0.0800 | 0.0563 | 0.6843 | 0.2604 | 0.1793 | 0.713 |
| $a+bx^2\sqrt{y}+c/x\sqrt{z}$ | 131.52 | 103.95 | 0.790 | 0.0803 | 0.0571 | 0.6816 | 0.2668 | 0.1898 | 0.698 |
| $a+bx^2\sqrt{y}+cz/x$ | 128.11 | 98.49 | 0.800 | 0.0812 | 0.0582 | 0.6746 | 0.2725 | 0.1951 | 0.685 |
| $a+bx^2\sqrt{y}+cz^2/x$ | 122.42 | 96.02 | 0.818 | 0.0807 | 0.0588 | 0.6786 | 0.2733 | 0.2026 | 0.684 |
| $a+bx^2\sqrt{y}+c\sqrt{z}/x$ | 129.70 | 100.91 | 0.795 | 0.0809 | 0.0573 | 0.6770 | 0.2709 | 0.1938 | 0.689 |
| $a+bx^2\sqrt{y}+c/x^2z$ | 129.97 | 101.31 | 0.794 | 0.0807 | 0.0575 | 0.6783 | 0.2705 | 0.1937 | 0.690 |
| $a+bx^2\sqrt{y}+c/x^2z^2$ | 130.94 | 102.87 | 0.791 | 0.0806 | 0.0573 | 0.6793 | 0.2690 | 0.1919 | 0.693 |
| $a+bx^2\sqrt{y}+c/x^2\sqrt{z}$ | 129.56 | 100.67 | 0.796 | 0.0808 | 0.0575 | 0.6779 | 0.2710 | 0.1942 | 0.689 |
| $a+bx^2\sqrt{y}+cz/x^2$ | 128.66 | 99.30 | 0.799 | 0.0809 | 0.0575 | 0.6770 | 0.2719 | 0.1947 | 0.687 |
| $a+bx^2\sqrt{y}+cz^2/x^2$ | 128.12 | 98.51 | 0.800 | 0.0810 | 0.0577 | 0.6762 | 0.2724 | 0.1948 | 0.686 |
| $a+bx^2\sqrt{y}+c\sqrt{z}/x^2$ | 128.92 | 99.70 | 0.798 | 0.0808 | 0.0575 | 0.6773 | 0.2717 | 0.1946 | 0.687 |
| $a+bx^2\sqrt{y}+c/\sqrt{x}z$ | 128.16 | 98.30 | 0.800 | 0.0788 | 0.0557 | 0.6936 | 0.2541 | 0.1718 | 0.726 |
| $a+bx^2\sqrt{y}+c/\sqrt{x}z^2$ | 124.27 | 96.21 | 0.812 | 0.0799 | 0.0571 | 0.6849 | 0.2593 | 0.1766 | 0.715 |
| $a+bx^2\sqrt{y}+c/\sqrt{x}\sqrt{z}$ | 131.01 | 102.84 | 0.791 | 0.0791 | 0.0557 | 0.6910 | 0.2581 | 0.1784 | 0.718 |
| $a+bx^2\sqrt{y}+cz/\sqrt{x}$ | 122.05 | 96.21 | 0.819 | 0.0802 | 0.0584 | 0.6828 | 0.2727 | 0.2028 | 0.685 |
| $a+bx^2\sqrt{y}+cz^2/\sqrt{x}$ | 118.39 | 89.25 | 0.829 | 0.0757 | 0.0550 | 0.7174 | 0.2661 | 0.1999 | 0.700 |
| $a+bx^2\sqrt{y}+c\sqrt{z}/\sqrt{x}$ | 128.15 | 98.70 | 0.800 | 0.0813 | 0.0587 | 0.6738 | 0.2728 | 0.1961 | 0.685 |
| $a+bx^2\sqrt{y}+cy/z$ | 126.80 | 100.29 | 0.804 | 0.0798 | 0.0589 | 0.6855 | 0.2721 | 0.2020 | 0.686 |
| $a+bx^2\sqrt{y}+cy/z^2$ | 128.41 | 101.83 | 0.799 | 0.0809 | 0.0593 | 0.6765 | 0.2729 | 0.2023 | 0.684 |
| $a+bx^2\sqrt{y}+cy/\sqrt{z}$ | 127.95 | 100.39 | 0.801 | 0.0797 | 0.0593 | 0.6867 | 0.2728 | 0.2024 | 0.685 |
| $a+bx^2\sqrt{y}+cyz$ | 124.13 | 96.11 | 0.813 | 0.0763 | 0.0541 | 0.7124 | 0.2685 | 0.1959 | 0.695 |
| $a+bx^2\sqrt{y}+cyz^2$ | 125.53 | 98.64 | 0.808 | 0.0775 | 0.0576 | 0.7036 | 0.2711 | 0.1995 | 0.689 |
| $a+bx^2\sqrt{y}+cy\sqrt{z}$ | 125.44 | 98.06 | 0.809 | 0.0774 | 0.0516 | 0.7043 | 0.2667 | 0.1873 | 0.699 |
| $a+bx^2\sqrt{y}+cy^2/z$ | 127.53 | 100.75 | 0.802 | 0.0789 | 0.0587 | 0.6923 | 0.2717 | 0.2008 | 0.687 |
| $a+bx^2\sqrt{y}+cy^2/z^2$ | 129.25 | 102.53 | 0.797 | 0.0808 | 0.0594 | 0.6779 | 0.2733 | 0.2022 | 0.684 |
| $a+bx^2\sqrt{y}+cy^2/\sqrt{z}$ | 127.60 | 99.65 | 0.802 | 0.0782 | 0.0584 | 0.6981 | 0.2705 | 0.1999 | 0.690 |
| $a+bx^2\sqrt{y}+cy^2z$ | 129.32 | 102.54 | 0.797 | 0.0800 | 0.0579 | 0.6838 | 0.2736 | 0.2013 | 0.683 |
| $a+bx^2\sqrt{y}+cy^2z^2$ | 128.33 | 102.02 | 0.800 | 0.0797 | 0.0589 | 0.6867 | 0.2735 | 0.2006 | 0.683 |
| $a+bx^2\sqrt{y}+cy^2\sqrt{z}$ | 131.09 | 103.71 | 0.791 | 0.0811 | 0.0584 | 0.6755 | 0.2731 | 0.2017 | 0.684 |
| $a+bx^2\sqrt{y}+c\sqrt{y}/z$ | 124.34 | 98.06 | 0.812 | 0.0796 | 0.0582 | 0.6868 | 0.2701 | 0.1999 | 0.691 |
| $a+bx^2\sqrt{y}+c\sqrt{y}/z^2$ | 127.05 | 100.59 | 0.804 | 0.0809 | 0.0592 | 0.6770 | 0.2719 | 0.2015 | 0.687 |
| $a+bx^2\sqrt{y}+c\sqrt{y}/\sqrt{z}$ | 125.25 | 98.37 | 0.809 | 0.0793 | 0.0584 | 0.6897 | 0.2714 | 0.2016 | 0.688 |
| $a+bx^2\sqrt{y}+c\sqrt{y}z$ | 120.15 | 92.58 | 0.824 | 0.0738 | 0.0510 | 0.7307 | 0.2622 | 0.1920 | 0.709 |
| $a+bx^2\sqrt{y}+c\sqrt{y}z^2$ | 123.46 | 96.34 | 0.815 | 0.0759 | 0.0561 | 0.7154 | 0.2683 | 0.1998 | 0.695 |
| $a+bx^2\sqrt{y}+c\sqrt{y}\sqrt{z}$ | 119.67 | 94.72 | 0.826 | 0.0741 | 0.0470 | 0.7289 | 0.2566 | 0.1743 | 0.721 |
| $a+bx^2\sqrt{y}+c/yz$ | 124.68 | 94.55 | 0.811 | 0.0796 | 0.0565 | 0.6875 | 0.2555 | 0.1689 | 0.723 |
| $a+bx^2\sqrt{y}+c/yz^2$ | 122.30 | 93.64 | 0.818 | 0.0803 | 0.0577 | 0.6819 | 0.2605 | 0.1784 | 0.712 |
| $a+bx^2\sqrt{y}+c/y\sqrt{z}$ | 128.12 | 99.37 | 0.800 | 0.0797 | 0.0556 | 0.6867 | 0.2571 | 0.1697 | 0.720 |
| $a+bx^2\sqrt{y}+cz/y$ | 121.68 | 93.78 | 0.820 | 0.0789 | 0.0578 | 0.6926 | 0.2707 | 0.2023 | 0.690 |
| $a+bx^2\sqrt{y}+cz^2/y$ | 116.04 | 86.10 | 0.836 | 0.0735 | 0.0524 | 0.7336 | 0.2604 | 0.1969 | 0.713 |
| $a+bx^2\sqrt{y}+c\sqrt{z}/y$ | 129.61 | 100.44 | 0.796 | 0.0812 | 0.0591 | 0.6743 | 0.2731 | 0.1975 | 0.684 |
| $a+bx^2\sqrt{y}+c/y^2z$ | 128.58 | 99.92 | 0.799 | 0.0802 | 0.0565 | 0.6828 | 0.2596 | 0.1732 | 0.714 |
| $a+bx^2\sqrt{y}+c/y^2z^2$ | 125.44 | 95.37 | 0.809 | 0.0804 | 0.0575 | 0.6811 | 0.2601 | 0.1772 | 0.713 |
| $a+bx^2\sqrt{y}+c/y^2\sqrt{z}$ | 130.33 | 102.46 | 0.793 | 0.0802 | 0.0559 | 0.6824 | 0.2611 | 0.1760 | 0.711 |
| $a+bx^2\sqrt{y}+cz/y^2$ | 130.06 | 101.22 | 0.794 | 0.0812 | 0.0583 | 0.6741 | 0.2719 | 0.1930 | 0.687 |
| $a+bx^2\sqrt{y}+cz^2/y^2$ | 121.10 | 93.91 | 0.822 | 0.0796 | 0.0582 | 0.6872 | 0.2715 | 0.2032 | 0.688 |
| $a+bx^2\sqrt{y}+c\sqrt{z}/y^2$ | 131.66 | 104.04 | 0.789 | 0.0809 | 0.0569 | 0.6772 | 0.2681 | 0.1885 | 0.695 |
| $a+bx^2\sqrt{y}+c/\sqrt{y}z$ | 120.45 | 93.61 | 0.823 | 0.0790 | 0.0561 | 0.6921 | 0.2551 | 0.1683 | 0.724 |
| $a+bx^2\sqrt{y}+c/\sqrt{y}z^2$ | 122.35 | 95.77 | 0.818 | 0.0804 | 0.0578 | 0.6807 | 0.2644 | 0.1878 | 0.704 |
| $a+bx^2\sqrt{y}+c/\sqrt{y}\sqrt{z}$ | 123.26 | 94.96 | 0.815 | 0.0785 | 0.0547 | 0.6961 | 0.2520 | 0.1618 | 0.731 |
| $a+bx^2\sqrt{y}+cz/\sqrt{y}$ | 115.91 | 87.44 | 0.837 | 0.0745 | 0.0522 | 0.7262 | 0.2612 | 0.1942 | 0.711 |
| $a+bx^2\sqrt{y}+cz^2/\sqrt{y}$ | 118.23 | 89.19 | 0.830 | 0.0731 | 0.0524 | 0.7358 | 0.2612 | 0.1971 | 0.711 |
| $a+bx^2\sqrt{y}+c\sqrt{z}/\sqrt{y}$ | 122.53 | 94.11 | 0.817 | 0.0788 | 0.0578 | 0.6936 | 0.2706 | 0.2018 | 0.690 |
| $a+b\sqrt{x}/y+cx/z$ | 252.50 | 192.36 | 0.224 | 0.1360 | 0.1029 | 0.0870 | 0.4624 | 0.3475 | 0.094 |
| $a+b\sqrt{x}/y+cx/z^2$ | 243.78 | 188.20 | 0.277 | 0.1329 | 0.1020 | 0.1274 | 0.4516 | 0.3432 | 0.136 |
| $a+b\sqrt{x}/y+cx/\sqrt{z}$ | 243.13 | 191.63 | 0.281 | 0.1303 | 0.1047 | 0.1613 | 0.4238 | 0.3309 | 0.239 |
| $a+b\sqrt{x}/y+cxz$ | 125.12 | 96.76 | 0.810 | 0.0732 | 0.0530 | 0.7358 | 0.2708 | 0.2086 | 0.689 |
| $a+b\sqrt{x}/y+cxz^2$ | 150.17 | 117.67 | 0.726 | 0.0853 | 0.0661 | 0.6410 | 0.3173 | 0.2515 | 0.573 |
| $a+b\sqrt{x}/y+cx\sqrt{z}$ | 114.98 | 89.93 | 0.839 | 0.0691 | 0.0457 | 0.7644 | 0.2414 | 0.1601 | 0.753 |
| $a+b\sqrt{x}/y+cx^2/z$ | 250.36 | 201.64 | 0.237 | 0.1346 | 0.1082 | 0.1051 | 0.4430 | 0.3520 | 0.169 |
| $a+b\sqrt{x}/y+cx^2/z^2$ | 251.35 | 192.60 | 0.231 | 0.1356 | 0.1040 | 0.0927 | 0.4606 | 0.3498 | 0.101 |
| $a+b\sqrt{x}/y+cx^2/\sqrt{z}$ | 184.12 | 147.19 | 0.588 | 0.1045 | 0.0831 | 0.4606 | 0.3248 | 0.2461 | 0.553 |
| $a+b\sqrt{x}/y+cx^2z$ | 134.38 | 105.28 | 0.780 | 0.0796 | 0.0615 | 0.6868 | 0.2933 | 0.2348 | 0.635 |
| $a+b\sqrt{x}/y+cx^2z^2$ | 156.93 | 125.46 | 0.700 | 0.0904 | 0.0714 | 0.5961 | 0.3322 | 0.2636 | 0.532 |
| $a+b\sqrt{x}/y+cx^2\sqrt{z}$ | 121.94 | 96.33 | 0.819 | 0.0747 | 0.0550 | 0.7244 | 0.2675 | 0.2028 | 0.697 |
| $a+b\sqrt{x}/y+c\sqrt{x}/z$ | 232.71 | 178.43 | 0.341 | 0.1282 | 0.0943 | 0.1891 | 0.4393 | 0.3241 | 0.182 |
| $a+b\sqrt{x}/y+c\sqrt{x}/z^2$ | 235.61 | 180.39 | 0.325 | 0.1300 | 0.0994 | 0.1653 | 0.4399 | 0.3304 | 0.180 |
| $a+b\sqrt{x}/y+c\sqrt{x}/\sqrt{z}$ | 255.43 | 195.98 | 0.206 | 0.1372 | 0.1044 | 0.0699 | 0.4637 | 0.3547 | 0.089 |

(continued on next page)

**Table 4 – continued from previous page**

| Functional form | $T_{eff}$ (K) | | | Radius ($R_{\odot}$) | | | log (L/$L_{\odot}$) | | |
|---|---|---|---|---|---|---|---|---|---|
| | RMSE | MAD | $R^2_{ap}$ | RMSE | MAD | $R^2_{ap}$ | RMSE | MAD | $R^2_{ap}$ |
| $a+b\sqrt{x}/y+c\sqrt{x}z$ | 125.81 | 100.18 | 0.807 | 0.0723 | 0.0495 | 0.7422 | 0.2672 | 0.1986 | 0.697 |
| $a+b\sqrt{x}/y+c\sqrt{x}z^2$ | 148.82 | 118.48 | 0.731 | 0.0836 | 0.0638 | 0.6549 | 0.3123 | 0.2452 | 0.587 |
| $a+b\sqrt{x}/y+c\sqrt{x}\sqrt{z}$ | 119.19 | 90.15 | 0.827 | 0.0693 | 0.0436 | 0.7630 | 0.2402 | 0.1493 | 0.755 |
| $a+b\sqrt{x}/y+c/xz$ | 224.38 | 165.62 | 0.387 | 0.1170 | 0.0882 | 0.3239 | 0.3806 | 0.2709 | 0.386 |
| $a+b\sqrt{x}/y+c/xz^2$ | 221.09 | 160.11 | 0.405 | 0.1180 | 0.0894 | 0.3128 | 0.3791 | 0.2726 | 0.391 |
| $a+b\sqrt{x}/y+c/x\sqrt{z}$ | 227.99 | 171.25 | 0.368 | 0.1181 | 0.0887 | 0.3113 | 0.3871 | 0.2793 | 0.365 |
| $a+b\sqrt{x}/y+cz/x$ | 247.80 | 191.51 | 0.253 | 0.1292 | 0.0993 | 0.1756 | 0.4304 | 0.3274 | 0.215 |
| $a+b\sqrt{x}/y+cz^2/x$ | 250.68 | 192.15 | 0.235 | 0.1363 | 0.1014 | 0.0834 | 0.4623 | 0.3464 | 0.094 |
| $a+b\sqrt{x}/y+c\sqrt{z}/x$ | 239.31 | 181.61 | 0.303 | 0.1238 | 0.0924 | 0.2428 | 0.4108 | 0.3043 | 0.285 |
| $a+b\sqrt{x}/y+c/x^2z$ | 238.63 | 180.29 | 0.307 | 0.1231 | 0.0915 | 0.2517 | 0.4092 | 0.3015 | 0.290 |
| $a+b\sqrt{x}/y+c/x^2z^2$ | 236.96 | 177.67 | 0.317 | 0.1227 | 0.0908 | 0.2562 | 0.4056 | 0.2956 | 0.303 |
| $a+b\sqrt{x}/y+c/x^2\sqrt{z}$ | 239.33 | 181.08 | 0.303 | 0.1233 | 0.0918 | 0.2488 | 0.4109 | 0.3034 | 0.285 |
| $a+b\sqrt{x}/y+cz/x^2$ | 241.22 | 182.57 | 0.292 | 0.1242 | 0.0930 | 0.2380 | 0.4154 | 0.3073 | 0.269 |
| $a+b\sqrt{x}/y+cz^2/x^2$ | 243.16 | 184.54 | 0.281 | 0.1254 | 0.0945 | 0.2231 | 0.4199 | 0.3117 | 0.253 |
| $a+b\sqrt{x}/y+c\sqrt{z}/x^2$ | 240.57 | 182.15 | 0.296 | 0.1239 | 0.0926 | 0.2422 | 0.4139 | 0.3061 | 0.274 |
| $a+b\sqrt{x}/y+c/\sqrt{x}z$ | 192.40 | 137.39 | 0.550 | 0.1042 | 0.0798 | 0.4636 | 0.3289 | 0.2351 | 0.542 |
| $a+b\sqrt{x}/y+c/\sqrt{x}z^2$ | 204.75 | 146.12 | 0.490 | 0.1148 | 0.0916 | 0.3493 | 0.3668 | 0.2739 | 0.430 |
| $a+b\sqrt{x}/y+c/\sqrt{x}\sqrt{z}$ | 200.18 | 146.63 | 0.512 | 0.1054 | 0.0791 | 0.4512 | 0.3368 | 0.2352 | 0.519 |
| $a+b\sqrt{x}/y+cz/\sqrt{x}$ | 238.61 | 176.46 | 0.307 | 0.1313 | 0.0936 | 0.1490 | 0.4504 | 0.3250 | 0.140 |
| $a+b\sqrt{x}/y+cz^2/\sqrt{x}$ | 169.83 | 134.72 | 0.649 | 0.0954 | 0.0685 | 0.5508 | 0.3488 | 0.2614 | 0.484 |
| $a+b\sqrt{x}/y+c\sqrt{z}/\sqrt{x}$ | 252.77 | 198.15 | 0.223 | 0.1333 | 0.1047 | 0.1224 | 0.4435 | 0.3451 | 0.166 |
| $a+b\sqrt{x}/y+cy/z$ | 228.46 | 174.00 | 0.365 | 0.1263 | 0.0912 | 0.2117 | 0.4344 | 0.3172 | 0.200 |
| $a+b\sqrt{x}/y+cy/z^2$ | 232.03 | 177.54 | 0.345 | 0.1285 | 0.0976 | 0.1850 | 0.4356 | 0.3247 | 0.196 |
| $a+b\sqrt{x}/y+cy/\sqrt{z}$ | 254.93 | 195.28 | 0.209 | 0.1371 | 0.1039 | 0.0713 | 0.4638 | 0.3535 | 0.089 |
| $a+b\sqrt{x}/y+cyz$ | 137.06 | 107.06 | 0.771 | 0.0775 | 0.0570 | 0.7035 | 0.2888 | 0.2219 | 0.647 |
| $a+b\sqrt{x}/y+cyz^2$ | 156.92 | 123.42 | 0.700 | 0.0880 | 0.0680 | 0.6179 | 0.3269 | 0.2551 | 0.547 |
| $a+b\sqrt{x}/y+cy\sqrt{z}$ | 130.53 | 100.56 | 0.793 | 0.0738 | 0.0487 | 0.7309 | 0.2654 | 0.1823 | 0.701 |
| $a+b\sqrt{x}/y+cy^2/z$ | 249.54 | 189.40 | 0.242 | 0.1349 | 0.1000 | 0.1015 | 0.4600 | 0.3432 | 0.103 |
| $a+b\sqrt{x}/y+cy^2/z^2$ | 236.89 | 182.16 | 0.317 | 0.1301 | 0.0981 | 0.1640 | 0.4437 | 0.3324 | 0.166 |
| $a+b\sqrt{x}/y+cy^2/\sqrt{z}$ | 243.24 | 196.60 | 0.280 | 0.1298 | 0.1047 | 0.1676 | 0.4279 | 0.3350 | 0.224 |
| $a+b\sqrt{x}/y+cy^2z$ | 149.52 | 112.38 | 0.728 | 0.0851 | 0.0644 | 0.6425 | 0.3142 | 0.2423 | 0.582 |
| $a+b\sqrt{x}/y+cy^2z^2$ | 165.57 | 129.06 | 0.666 | 0.0937 | 0.0730 | 0.5662 | 0.3440 | 0.2657 | 0.499 |
| $a+b\sqrt{x}/y+cy^2\sqrt{z}$ | 143.65 | 104.79 | 0.749 | 0.0819 | 0.0580 | 0.6687 | 0.2968 | 0.2120 | 0.627 |
| $a+b\sqrt{x}/y+c\sqrt{y}/z$ | 207.22 | 153.79 | 0.478 | 0.1173 | 0.0838 | 0.3206 | 0.4016 | 0.2813 | 0.317 |
| $a+b\sqrt{x}/y+c\sqrt{y}/z^2$ | 226.46 | 170.74 | 0.376 | 0.1264 | 0.0963 | 0.2114 | 0.4258 | 0.3138 | 0.232 |
| $a+b\sqrt{x}/y+c\sqrt{y}/\sqrt{z}$ | 226.72 | 171.06 | 0.375 | 0.1256 | 0.0896 | 0.2214 | 0.4331 | 0.3138 | 0.205 |
| $a+b\sqrt{x}/y+c\sqrt{y}z$ | 133.44 | 106.72 | 0.783 | 0.0755 | 0.0533 | 0.7184 | 0.2812 | 0.2113 | 0.665 |
| $a+b\sqrt{x}/y+c\sqrt{y}z^2$ | 153.17 | 122.50 | 0.715 | 0.0855 | 0.0651 | 0.6391 | 0.3190 | 0.2483 | 0.569 |
| $a+b\sqrt{x}/y+c\sqrt{y}\sqrt{z}$ | 125.97 | 99.44 | 0.807 | 0.0717 | 0.0441 | 0.7458 | 0.2569 | 0.1673 | 0.720 |
| $a+b\sqrt{x}/y+c/yz$ | 199.85 | 139.00 | 0.514 | 0.1104 | 0.0850 | 0.3986 | 0.3463 | 0.2492 | 0.492 |
| $a+b\sqrt{x}/y+c/yz^2$ | 214.59 | 155.12 | 0.440 | 0.1205 | 0.0968 | 0.2831 | 0.3858 | 0.2942 | 0.369 |
| $a+b\sqrt{x}/y+c/y\sqrt{z}$ | 202.24 | 146.07 | 0.502 | 0.1089 | 0.0820 | 0.4142 | 0.3433 | 0.2424 | 0.501 |
| $a+b\sqrt{x}/y+cz/y$ | 237.11 | 175.00 | 0.316 | 0.1304 | 0.0930 | 0.1598 | 0.4477 | 0.3226 | 0.151 |
| $a+b\sqrt{x}/y+cz^2/y$ | 166.01 | 129.97 | 0.665 | 0.0935 | 0.0666 | 0.5686 | 0.3400 | 0.2530 | 0.510 |
| $a+b\sqrt{x}/y+c\sqrt{z}/y$ | 252.66 | 197.73 | 0.223 | 0.1336 | 0.1051 | 0.1185 | 0.4437 | 0.3444 | 0.166 |
| $a+b\sqrt{x}/y+c/y^2z$ | 227.21 | 165.06 | 0.372 | 0.1221 | 0.0962 | 0.2633 | 0.3921 | 0.2915 | 0.349 |
| $a+b\sqrt{x}/y+c/y^2z^2$ | 231.50 | 169.58 | 0.348 | 0.1264 | 0.1000 | 0.2109 | 0.4074 | 0.3063 | 0.297 |
| $a+b\sqrt{x}/y+c/y^2\sqrt{z}$ | 227.39 | 166.68 | 0.371 | 0.1209 | 0.0940 | 0.2784 | 0.3893 | 0.2850 | 0.358 |
| $a+b\sqrt{x}/y+cz/y^2$ | 247.23 | 190.00 | 0.256 | 0.1296 | 0.1001 | 0.1708 | 0.4292 | 0.3246 | 0.220 |
| $a+b\sqrt{x}/y+cz^2/y^2$ | 248.17 | 188.29 | 0.251 | 0.1352 | 0.0992 | 0.0971 | 0.4598 | 0.3392 | 0.104 |
| $a+b\sqrt{x}/y+c\sqrt{z}/y^2$ | 237.09 | 175.77 | 0.316 | 0.1240 | 0.0949 | 0.2411 | 0.4062 | 0.2920 | 0.301 |
| $a+b\sqrt{x}/y+c/\sqrt{y}z$ | 176.96 | 123.67 | 0.619 | 0.1018 | 0.0773 | 0.4885 | 0.3210 | 0.2187 | 0.563 |
| $a+b\sqrt{x}/y+c/\sqrt{y}z^2$ | 211.30 | 150.65 | 0.457 | 0.1200 | 0.0942 | 0.2894 | 0.3902 | 0.2839 | 0.355 |
| $a+b\sqrt{x}/y+c/\sqrt{y}\sqrt{z}$ | 168.99 | 119.44 | 0.653 | 0.0945 | 0.0707 | 0.5590 | 0.2947 | 0.1964 | 0.632 |
| $a+b\sqrt{x}/y+cz/\sqrt{y}$ | 166.78 | 130.34 | 0.662 | 0.0955 | 0.0663 | 0.5498 | 0.3427 | 0.2428 | 0.502 |
| $a+b\sqrt{x}/y+cz^2/\sqrt{y}$ | 153.06 | 124.26 | 0.715 | 0.0855 | 0.0635 | 0.6390 | 0.3172 | 0.2478 | 0.574 |
| $a+b\sqrt{x}/y+c\sqrt{z}/\sqrt{y}$ | 231.69 | 171.76 | 0.347 | 0.1279 | 0.0906 | 0.1919 | 0.4407 | 0.3161 | 0.177 |
| $a+b\sqrt{x}/y^2+cx/z$ | 189.84 | 133.19 | 0.561 | 0.1071 | 0.0797 | 0.4334 | 0.3489 | 0.2457 | 0.484 |
| $a+b\sqrt{x}/y^2+cx/z^2$ | 199.38 | 139.06 | 0.516 | 0.1112 | 0.0863 | 0.3891 | 0.3571 | 0.2580 | 0.460 |
| $a+b\sqrt{x}/y^2+cx/\sqrt{z}$ | 219.46 | 151.28 | 0.414 | 0.1180 | 0.0899 | 0.3123 | 0.3803 | 0.2757 | 0.387 |
| $a+b\sqrt{x}/y^2+cxz$ | 117.89 | 88.20 | 0.831 | 0.0711 | 0.0466 | 0.7502 | 0.2482 | 0.1620 | 0.739 |
| $a+b\sqrt{x}/y^2+cxz^2$ | 128.60 | 96.93 | 0.799 | 0.0769 | 0.0536 | 0.7083 | 0.2683 | 0.1813 | 0.695 |
| $a+b\sqrt{x}/y^2+cx\sqrt{z}$ | 116.23 | 89.25 | 0.836 | 0.0696 | 0.0443 | 0.7609 | 0.2375 | 0.1492 | 0.761 |
| $a+b\sqrt{x}/y^2+cx^2/z$ | 221.66 | 154.03 | 0.402 | 0.1178 | 0.0886 | 0.3148 | 0.3804 | 0.2733 | 0.387 |
| $a+b\sqrt{x}/y^2+cx^2/z^2$ | 205.43 | 143.38 | 0.487 | 0.1126 | 0.0866 | 0.3744 | 0.3638 | 0.2598 | 0.439 |
| $a+b\sqrt{x}/y^2+cx^2/\sqrt{z}$ | 192.16 | 153.01 | 0.551 | 0.1048 | 0.0842 | 0.4574 | 0.3242 | 0.2518 | 0.555 |
| $a+b\sqrt{x}/y^2+cx^2z$ | 120.25 | 92.38 | 0.824 | 0.0749 | 0.0527 | 0.7230 | 0.2587 | 0.1756 | 0.716 |
| $a+b\sqrt{x}/y^2+cx^2z^2$ | 131.50 | 99.69 | 0.790 | 0.0803 | 0.0572 | 0.6820 | 0.2768 | 0.1900 | 0.675 |
| $a+b\sqrt{x}/y^2+cx^2\sqrt{z}$ | 116.54 | 91.57 | 0.835 | 0.0735 | 0.0513 | 0.7331 | 0.2496 | 0.1666 | 0.736 |
| $a+b\sqrt{x}/y^2+c\sqrt{x}/z$ | 176.87 | 124.42 | 0.619 | 0.1033 | 0.0769 | 0.4734 | 0.3333 | 0.2295 | 0.529 |
| $a+b\sqrt{x}/y^2+c\sqrt{x}/z^2$ | 197.71 | 138.62 | 0.524 | 0.1112 | 0.0869 | 0.3895 | 0.3552 | 0.2589 | 0.465 |
| $a+b\sqrt{x}/y^2+c\sqrt{x}/\sqrt{z}$ | 184.85 | 134.47 | 0.584 | 0.1069 | 0.0790 | 0.4358 | 0.3475 | 0.2460 | 0.488 |
| $a+b\sqrt{x}/y^2+c\sqrt{x}z$ | 120.31 | 92.05 | 0.824 | 0.0707 | 0.0441 | 0.7532 | 0.2473 | 0.1557 | 0.741 |
| $a+b\sqrt{x}/y^2+c\sqrt{x}z^2$ | 128.81 | 98.98 | 0.798 | 0.0758 | 0.0520 | 0.7162 | 0.2657 | 0.1774 | 0.701 |
| $a+b\sqrt{x}/y^2+c\sqrt{x}\sqrt{z}$ | 121.79 | 90.80 | 0.820 | 0.0695 | 0.0417 | 0.7614 | 0.2382 | 0.1412 | 0.760 |
| $a+b\sqrt{x}/y^2+c/xz$ | 225.43 | 165.68 | 0.382 | 0.1184 | 0.0921 | 0.3073 | 0.3796 | 0.2810 | 0.389 |
| $a+b\sqrt{x}/y^2+c/xz^2$ | 225.87 | 166.79 | 0.379 | 0.1188 | 0.0919 | 0.3028 | 0.3798 | 0.2788 | 0.389 |
| $a+b\sqrt{x}/y^2+c/x\sqrt{z}$ | 225.07 | 164.83 | 0.384 | 0.1186 | 0.0921 | 0.3056 | 0.3802 | 0.2813 | 0.387 |
| $a+b\sqrt{x}/y^2+cz/x$ | 217.42 | 161.02 | 0.425 | 0.1192 | 0.0936 | 0.2979 | 0.3810 | 0.2855 | 0.385 |
| $a+b\sqrt{x}/y^2+cz^2/x$ | 180.68 | 133.37 | 0.603 | 0.1084 | 0.0798 | 0.4203 | 0.3487 | 0.2438 | 0.485 |
| $a+b\sqrt{x}/y^2+c\sqrt{z}/x$ | 222.41 | 162.57 | 0.398 | 0.1193 | 0.0928 | 0.2967 | 0.3821 | 0.2833 | 0.382 |
| $a+b\sqrt{x}/y^2+c/x^2z$ | 222.98 | 163.24 | 0.395 | 0.1192 | 0.0924 | 0.2980 | 0.3819 | 0.2822 | 0.382 |
| $a+b\sqrt{x}/y^2+c/x^2z^2$ | 221.86 | 163.38 | 0.401 | 0.1194 | 0.0930 | 0.2963 | 0.3821 | 0.2838 | 0.381 |
| $a+b\sqrt{x}/y^2+c/x^2\sqrt{z}$ | 223.28 | 163.12 | 0.393 | 0.1192 | 0.0922 | 0.2987 | 0.3819 | 0.2816 | 0.382 |
| $a+b\sqrt{x}/y^2+cz/x^2$ | 223.57 | 162.92 | 0.392 | 0.1191 | 0.0920 | 0.2994 | 0.3818 | 0.2812 | 0.382 |
| $a+b\sqrt{x}/y^2+cz^2/x^2$ | 223.05 | 162.98 | 0.395 | 0.1192 | 0.0924 | 0.2980 | 0.3820 | 0.2823 | 0.382 |
| $a+b\sqrt{x}/y^2+c\sqrt{z}/x^2$ | 223.57 | 162.95 | 0.392 | 0.1191 | 0.0920 | 0.2994 | 0.3818 | 0.2811 | 0.382 |
| $a+b\sqrt{x}/y^2+c/\sqrt{x}z$ | 205.12 | 144.59 | 0.488 | 0.1047 | 0.0798 | 0.4583 | 0.3331 | 0.2381 | 0.530 |
| $a+b\sqrt{x}/y^2+c/\sqrt{x}z^2$ | 209.22 | 153.31 | 0.467 | 0.1139 | 0.0899 | 0.3594 | 0.3606 | 0.2672 | 0.449 |
| $a+b\sqrt{x}/y^2+c/\sqrt{x}\sqrt{z}$ | 217.73 | 156.18 | 0.423 | 0.1087 | 0.0825 | 0.4161 | 0.3492 | 0.2465 | 0.483 |
| $a+b\sqrt{x}/y^2+cz/\sqrt{x}$ | 164.84 | 120.93 | 0.669 | 0.1016 | 0.0717 | 0.4905 | 0.3291 | 0.2233 | 0.541 |
| $a+b\sqrt{x}/y^2+cz^2/\sqrt{x}$ | 132.64 | 99.98 | 0.786 | 0.0810 | 0.0556 | 0.6757 | 0.2776 | 0.1920 | 0.673 |

(continued on next page)

**Table 4 – continued from previous page**

| Functional form | $T_{eff}$ (K) RMSE | MAD | $R^2_{ap}$ | Radius ($R_\odot$) RMSE | MAD | $R^2_{ap}$ | log (L/$L_\odot$) RMSE | MAD | $R^2_{ap}$ |
|---|---|---|---|---|---|---|---|---|---|
| $a+b\sqrt{x}/y^2+c\sqrt{z}/\sqrt{x}$ | 207.26 | 153.03 | 0.477 | 0.1171 | 0.0908 | 0.3224 | 0.3744 | 0.2758 | 0.406 |
| $a+b\sqrt{x}/y^2+cy/z$ | 167.80 | 112.69 | 0.657 | 0.0977 | 0.0712 | 0.5288 | 0.3150 | 0.2095 | 0.579 |
| $a+b\sqrt{x}/y^2+cy/z^2$ | 192.47 | 136.29 | 0.549 | 0.1087 | 0.0845 | 0.4170 | 0.3470 | 0.2502 | 0.490 |
| $a+b\sqrt{x}/y^2+cy/\sqrt{z}$ | 181.94 | 126.99 | 0.597 | 0.1021 | 0.0755 | 0.4858 | 0.3293 | 0.2373 | 0.541 |
| $a+b\sqrt{x}/y^2+cyz$ | 127.68 | 96.93 | 0.802 | 0.0768 | 0.0501 | 0.7091 | 0.2676 | 0.1705 | 0.697 |
| $a+b\sqrt{x}/y^2+cyz^2$ | 133.86 | 101.74 | 0.782 | 0.0796 | 0.0544 | 0.6868 | 0.2773 | 0.1837 | 0.674 |
| $a+b\sqrt{x}/y^2+cy\sqrt{z}$ | 130.70 | 98.97 | 0.792 | 0.0783 | 0.0499 | 0.6971 | 0.2697 | 0.1611 | 0.692 |
| $a+b\sqrt{x}/y^2+cy^2/z$ | 186.44 | 130.06 | 0.577 | 0.1019 | 0.0761 | 0.4875 | 0.3300 | 0.2394 | 0.539 |
| $a+b\sqrt{x}/y^2+cy^2/z^2$ | 189.33 | 134.38 | 0.564 | 0.1063 | 0.0817 | 0.4420 | 0.3412 | 0.2406 | 0.507 |
| $a+b\sqrt{x}/y^2+cy^2/\sqrt{z}$ | 226.02 | 167.69 | 0.378 | 0.1194 | 0.0935 | 0.2964 | 0.3819 | 0.2828 | 0.382 |
| $a+b\sqrt{x}/y^2+cy^2z$ | 135.21 | 100.27 | 0.778 | 0.0823 | 0.0552 | 0.6656 | 0.2834 | 0.1789 | 0.660 |
| $a+b\sqrt{x}/y^2+cy^2z^2$ | 139.00 | 105.11 | 0.765 | 0.0839 | 0.0575 | 0.6527 | 0.2887 | 0.1902 | 0.647 |
| $a+b\sqrt{x}/y^2+cy^2\sqrt{z}$ | 139.95 | 102.83 | 0.762 | 0.0849 | 0.0565 | 0.6443 | 0.2889 | 0.1765 | 0.646 |
| $a+b\sqrt{x}/y^2+c\sqrt{y}/z$ | 166.60 | 112.27 | 0.662 | 0.0982 | 0.0727 | 0.5239 | 0.3149 | 0.2071 | 0.580 |
| $a+b\sqrt{x}/y^2+c\sqrt{y}/z^2$ | 195.01 | 138.42 | 0.537 | 0.1101 | 0.0862 | 0.4017 | 0.3506 | 0.2555 | 0.479 |
| $a+b\sqrt{x}/y^2+c\sqrt{y}/\sqrt{z}$ | 158.04 | 109.85 | 0.696 | 0.0941 | 0.0671 | 0.5626 | 0.3044 | 0.2020 | 0.608 |
| $a+b\sqrt{x}/y^2+c\sqrt{y}z$ | 124.49 | 97.26 | 0.811 | 0.0743 | 0.0474 | 0.7274 | 0.2595 | 0.1652 | 0.715 |
| $a+b\sqrt{x}/y^2+c\sqrt{y}z^2$ | 131.57 | 101.48 | 0.789 | 0.0776 | 0.0529 | 0.7030 | 0.2712 | 0.1796 | 0.688 |
| $a+b\sqrt{x}/y^2+c\sqrt{y}\sqrt{z}$ | 125.46 | 97.43 | 0.808 | 0.0749 | 0.0447 | 0.7229 | 0.2585 | 0.1550 | 0.717 |
| $a+b\sqrt{x}/y^2+c/yz$ | 199.64 | 147.07 | 0.515 | 0.1089 | 0.0840 | 0.4146 | 0.3421 | 0.2464 | 0.504 |
| $a+b\sqrt{x}/y^2+c/yz^2$ | 215.15 | 152.23 | 0.437 | 0.1176 | 0.0918 | 0.3166 | 0.3733 | 0.2766 | 0.410 |
| $a+b\sqrt{x}/y^2+c/y\sqrt{z}$ | 202.42 | 141.47 | 0.501 | 0.1030 | 0.0787 | 0.4761 | 0.3270 | 0.2298 | 0.547 |
| $a+b\sqrt{x}/y^2+cz/y$ | 155.48 | 115.22 | 0.706 | 0.0956 | 0.0663 | 0.5486 | 0.3085 | 0.2079 | 0.597 |
| $a+b\sqrt{x}/y^2+cz^2/y$ | 131.59 | 94.64 | 0.789 | 0.0783 | 0.0544 | 0.6975 | 0.2671 | 0.1840 | 0.698 |
| $a+b\sqrt{x}/y^2+c\sqrt{z}/y$ | 195.87 | 138.14 | 0.533 | 0.1133 | 0.0852 | 0.3658 | 0.3610 | 0.2548 | 0.448 |
| $a+b\sqrt{x}/y^2+c/y^2z$ | 220.95 | 166.92 | 0.406 | 0.1187 | 0.0928 | 0.3041 | 0.3810 | 0.2831 | 0.385 |
| $a+b\sqrt{x}/y^2+c/y^2z^2$ | 224.41 | 167.55 | 0.387 | 0.1173 | 0.0892 | 0.3209 | 0.3785 | 0.2769 | 0.393 |
| $a+b\sqrt{x}/y^2+c/y^2\sqrt{z}$ | 220.08 | 165.86 | 0.411 | 0.1193 | 0.0935 | 0.2970 | 0.3818 | 0.2849 | 0.382 |
| $a+b\sqrt{x}/y^2+cz/y^2$ | 209.88 | 154.96 | 0.464 | 0.1179 | 0.0922 | 0.3133 | 0.3758 | 0.2794 | 0.402 |
| $a+b\sqrt{x}/y^2+cz^2/y^2$ | 171.43 | 122.03 | 0.642 | 0.1034 | 0.0734 | 0.4718 | 0.3315 | 0.2233 | 0.534 |
| $a+b\sqrt{x}/y^2+c\sqrt{z}/y^2$ | 216.85 | 161.77 | 0.428 | 0.1192 | 0.0935 | 0.2983 | 0.3808 | 0.2852 | 0.386 |
| $a+b\sqrt{x}/y^2+c/\sqrt{y}z$ | 177.26 | 123.92 | 0.618 | 0.1020 | 0.0779 | 0.4859 | 0.3222 | 0.2231 | 0.560 |
| $a+b\sqrt{x}/y^2+c/\sqrt{y}z^2$ | 205.10 | 146.88 | 0.488 | 0.1144 | 0.0906 | 0.3537 | 0.3627 | 0.2698 | 0.443 |
| $a+b\sqrt{x}/y^2+c/\sqrt{y}\sqrt{z}$ | 158.27 | 110.17 | 0.695 | 0.0894 | 0.0625 | 0.6051 | 0.2855 | 0.1728 | 0.655 |
| $a+b\sqrt{x}/y^2+cz/\sqrt{y}$ | 129.92 | 99.94 | 0.795 | 0.0796 | 0.0540 | 0.6872 | 0.2670 | 0.1779 | 0.698 |
| $a+b\sqrt{x}/y^2+cz^2/\sqrt{y}$ | 129.34 | 95.61 | 0.796 | 0.0756 | 0.0521 | 0.7181 | 0.2630 | 0.1811 | 0.707 |
| $a+b\sqrt{x}/y^2+c\sqrt{z}/\sqrt{y}$ | 151.46 | 113.69 | 0.721 | 0.0931 | 0.0650 | 0.5725 | 0.3011 | 0.2033 | 0.616 |
| $a+b\sqrt{x}/\sqrt{y}+cx/z$ | 224.98 | 169.63 | 0.384 | 0.1070 | 0.0843 | 0.4344 | 0.3621 | 0.2816 | 0.444 |
| $a+b\sqrt{x}/\sqrt{y}+cx/z^2$ | 226.33 | 170.30 | 0.377 | 0.1112 | 0.0868 | 0.3898 | 0.3671 | 0.2806 | 0.429 |
| $a+b\sqrt{x}/\sqrt{y}+cx/\sqrt{z}$ | 259.25 | 193.83 | 0.182 | 0.1223 | 0.0945 | 0.2616 | 0.4054 | 0.3112 | 0.303 |
| $a+b\sqrt{x}/\sqrt{y}+cxz$ | 125.94 | 93.78 | 0.807 | 0.0689 | 0.0476 | 0.7654 | 0.2447 | 0.1773 | 0.746 |
| $a+b\sqrt{x}/\sqrt{y}+cxz^2$ | 142.48 | 105.88 | 0.753 | 0.0734 | 0.0544 | 0.7343 | 0.2641 | 0.1978 | 0.704 |
| $a+b\sqrt{x}/\sqrt{y}+cx\sqrt{z}$ | 116.35 | 89.73 | 0.835 | 0.0691 | 0.0447 | 0.7640 | 0.2354 | 0.1578 | 0.765 |
| $a+b\sqrt{x}/\sqrt{y}+cx^2/z$ | 259.12 | 193.64 | 0.183 | 0.1222 | 0.0935 | 0.2627 | 0.4054 | 0.3106 | 0.304 |
| $a+b\sqrt{x}/\sqrt{y}+cx^2/z^2$ | 238.30 | 176.28 | 0.309 | 0.1144 | 0.0885 | 0.3538 | 0.3815 | 0.2919 | 0.383 |
| $a+b\sqrt{x}/\sqrt{y}+cx^2/\sqrt{z}$ | 193.06 | 156.35 | 0.546 | 0.1048 | 0.0830 | 0.4580 | 0.3257 | 0.2528 | 0.550 |
| $a+b\sqrt{x}/\sqrt{y}+cx^2z$ | 131.13 | 99.46 | 0.791 | 0.0721 | 0.0532 | 0.7436 | 0.2546 | 0.1922 | 0.725 |
| $a+b\sqrt{x}/\sqrt{y}+cx^2z^2$ | 146.34 | 112.17 | 0.739 | 0.0766 | 0.0590 | 0.7099 | 0.2729 | 0.2110 | 0.685 |
| $a+b\sqrt{x}/\sqrt{y}+cx^2\sqrt{z}$ | 122.84 | 95.16 | 0.816 | 0.0716 | 0.0511 | 0.7469 | 0.2460 | 0.1806 | 0.744 |
| $a+b\sqrt{x}/\sqrt{y}+c\sqrt{x}/z$ | 196.81 | 149.11 | 0.529 | 0.0986 | 0.0756 | 0.5197 | 0.3281 | 0.2483 | 0.544 |
| $a+b\sqrt{x}/\sqrt{y}+c\sqrt{x}/z^2$ | 216.97 | 165.32 | 0.427 | 0.1091 | 0.0845 | 0.4125 | 0.3562 | 0.2697 | 0.462 |
| $a+b\sqrt{x}/\sqrt{y}+c\sqrt{x}/\sqrt{z}$ | 216.05 | 162.33 | 0.432 | 0.1029 | 0.0814 | 0.4773 | 0.3495 | 0.2729 | 0.483 |
| $a+b\sqrt{x}/\sqrt{y}+c\sqrt{x}z$ | 127.62 | 97.30 | 0.802 | 0.0687 | 0.0460 | 0.7671 | 0.2439 | 0.1688 | 0.748 |
| $a+b\sqrt{x}/\sqrt{y}+c\sqrt{x}z^2$ | 142.30 | 106.12 | 0.754 | 0.0724 | 0.0524 | 0.7415 | 0.2615 | 0.1898 | 0.710 |
| $a+b\sqrt{x}/\sqrt{y}+c\sqrt{x}\sqrt{z}$ | 120.28 | 92.44 | 0.824 | 0.0695 | 0.0430 | 0.7615 | 0.2368 | 0.1484 | 0.762 |
| $a+b\sqrt{x}/\sqrt{y}+c/xz$ | 256.77 | 190.67 | 0.198 | 0.1224 | 0.0949 | 0.2602 | 0.4020 | 0.3026 | 0.315 |
| $a+b\sqrt{x}/\sqrt{y}+c/xz^2$ | 242.75 | 178.12 | 0.283 | 0.1196 | 0.0907 | 0.2941 | 0.3866 | 0.2810 | 0.367 |
| $a+b\sqrt{x}/\sqrt{y}+c/x\sqrt{z}$ | 259.34 | 194.10 | 0.182 | 0.1233 | 0.0964 | 0.2495 | 0.4057 | 0.3108 | 0.302 |
| $a+b\sqrt{x}/\sqrt{y}+cz/x$ | 222.44 | 165.02 | 0.398 | 0.1125 | 0.0869 | 0.3745 | 0.3622 | 0.2767 | 0.444 |
| $a+b\sqrt{x}/\sqrt{y}+cz^2/x$ | 155.26 | 122.41 | 0.707 | 0.0848 | 0.0651 | 0.6449 | 0.2780 | 0.2021 | 0.673 |
| $a+b\sqrt{x}/\sqrt{y}+c\sqrt{z}/x$ | 243.81 | 178.29 | 0.277 | 0.1196 | 0.0917 | 0.2940 | 0.3885 | 0.2981 | 0.361 |
| $a+b\sqrt{x}/\sqrt{y}+c/x^2z$ | 245.26 | 179.22 | 0.268 | 0.1204 | 0.0926 | 0.2848 | 0.3906 | 0.3007 | 0.354 |
| $a+b\sqrt{x}/\sqrt{y}+c/x^2z^2$ | 251.68 | 186.09 | 0.229 | 0.1215 | 0.0947 | 0.2716 | 0.3973 | 0.3092 | 0.331 |
| $a+b\sqrt{x}/\sqrt{y}+c/x^2\sqrt{z}$ | 243.20 | 176.66 | 0.280 | 0.1200 | 0.0918 | 0.2887 | 0.3884 | 0.2973 | 0.361 |
| $a+b\sqrt{x}/\sqrt{y}+cz/x^2$ | 239.05 | 171.28 | 0.305 | 0.1192 | 0.0902 | 0.2979 | 0.3839 | 0.2902 | 0.376 |
| $a+b\sqrt{x}/\sqrt{y}+cz^2/x^2$ | 234.88 | 167.72 | 0.329 | 0.1181 | 0.0893 | 0.3115 | 0.3790 | 0.2861 | 0.392 |
| $a+b\sqrt{x}/\sqrt{y}+c\sqrt{z}/x^2$ | 240.35 | 172.93 | 0.297 | 0.1195 | 0.0907 | 0.2946 | 0.3854 | 0.2923 | 0.371 |
| $a+b\sqrt{x}/\sqrt{y}+c/\sqrt{x}z$ | 200.73 | 144.56 | 0.510 | 0.1053 | 0.0812 | 0.4523 | 0.3335 | 0.2402 | 0.529 |
| $a+b\sqrt{x}/\sqrt{y}+c/\sqrt{x}z^2$ | 210.52 | 154.67 | 0.461 | 0.1106 | 0.0847 | 0.3961 | 0.3497 | 0.2541 | 0.482 |
| $a+b\sqrt{x}/\sqrt{y}+c/\sqrt{x}\sqrt{z}$ | 215.64 | 148.85 | 0.434 | 0.1081 | 0.0819 | 0.4232 | 0.3489 | 0.2435 | 0.484 |
| $a+b\sqrt{x}/\sqrt{y}+cz/\sqrt{x}$ | 151.70 | 121.18 | 0.720 | 0.0812 | 0.0613 | 0.6741 | 0.2714 | 0.2009 | 0.688 |
| $a+b\sqrt{x}/\sqrt{y}+cz^2/\sqrt{x}$ | 140.32 | 106.11 | 0.760 | 0.0718 | 0.0520 | 0.7454 | 0.2558 | 0.1883 | 0.723 |
| $a+b\sqrt{x}/\sqrt{y}+c\sqrt{z}/\sqrt{x}$ | 211.01 | 158.49 | 0.458 | 0.1057 | 0.0820 | 0.4478 | 0.3457 | 0.2615 | 0.494 |
| $a+b\sqrt{x}/\sqrt{y}+cy/z$ | 220.31 | 165.47 | 0.409 | 0.1060 | 0.0822 | 0.4447 | 0.3563 | 0.2729 | 0.462 |
| $a+b\sqrt{x}/\sqrt{y}+cy/z^2$ | 221.21 | 165.66 | 0.405 | 0.1098 | 0.0849 | 0.4044 | 0.3610 | 0.2736 | 0.448 |
| $a+b\sqrt{x}/\sqrt{y}+cy/\sqrt{z}$ | 257.11 | 191.03 | 0.196 | 0.1210 | 0.0939 | 0.2767 | 0.4024 | 0.3094 | 0.314 |
| $a+b\sqrt{x}/\sqrt{y}+cyz$ | 129.30 | 97.01 | 0.797 | 0.0707 | 0.0464 | 0.7533 | 0.2487 | 0.1700 | 0.738 |
| $a+b\sqrt{x}/\sqrt{y}+cyz^2$ | 142.90 | 107.03 | 0.752 | 0.0738 | 0.0531 | 0.7314 | 0.2646 | 0.1909 | 0.703 |
| $a+b\sqrt{x}/\sqrt{y}+cy\sqrt{z}$ | 128.99 | 97.10 | 0.798 | 0.0739 | 0.0474 | 0.7302 | 0.2492 | 0.1540 | 0.737 |
| $a+b\sqrt{x}/\sqrt{y}+cy^2/z$ | 256.18 | 190.01 | 0.202 | 0.1204 | 0.0925 | 0.2838 | 0.4012 | 0.3080 | 0.318 |
| $a+b\sqrt{x}/\sqrt{y}+cy^2/z^2$ | 233.40 | 170.27 | 0.337 | 0.1127 | 0.0867 | 0.3723 | 0.3750 | 0.2842 | 0.404 |
| $a+b\sqrt{x}/\sqrt{y}+cy^2/\sqrt{z}$ | 234.66 | 188.04 | 0.330 | 0.1171 | 0.0940 | 0.3231 | 0.3767 | 0.2961 | 0.399 |
| $a+b\sqrt{x}/\sqrt{y}+cy^2z$ | 135.16 | 100.87 | 0.778 | 0.0743 | 0.0517 | 0.7272 | 0.2597 | 0.1828 | 0.714 |
| $a+b\sqrt{x}/\sqrt{y}+cy^2z^2$ | 146.51 | 111.72 | 0.739 | 0.0770 | 0.0575 | 0.7075 | 0.2730 | 0.2031 | 0.684 |
| $a+b\sqrt{x}/\sqrt{y}+cy^2\sqrt{z}$ | 135.61 | 99.94 | 0.776 | 0.0771 | 0.0533 | 0.7068 | 0.2606 | 0.1712 | 0.712 |
| $a+b\sqrt{x}/\sqrt{y}+c\sqrt{y}/z$ | 192.71 | 144.96 | 0.548 | 0.0978 | 0.0737 | 0.5279 | 0.3233 | 0.2411 | 0.557 |
| $a+b\sqrt{x}/\sqrt{y}+c\sqrt{y}/z^2$ | 213.58 | 162.31 | 0.445 | 0.1083 | 0.0832 | 0.4203 | 0.3523 | 0.2644 | 0.474 |
| $a+b\sqrt{x}/\sqrt{y}+c\sqrt{y}/\sqrt{z}$ | 213.55 | 162.08 | 0.445 | 0.1026 | 0.0793 | 0.4804 | 0.3464 | 0.2665 | 0.491 |
| $a+b\sqrt{x}/\sqrt{y}+c\sqrt{y}z$ | 128.11 | 97.72 | 0.800 | 0.0693 | 0.0443 | 0.7627 | 0.2448 | 0.1630 | 0.746 |
| $a+b\sqrt{x}/\sqrt{y}+c\sqrt{y}z^2$ | 142.16 | 106.25 | 0.754 | 0.0725 | 0.0509 | 0.7405 | 0.2614 | 0.1848 | 0.710 |
| $a+b\sqrt{x}/\sqrt{y}+c\sqrt{y}\sqrt{z}$ | 124.97 | 96.40 | 0.810 | 0.0717 | 0.0449 | 0.7465 | 0.2423 | 0.1476 | 0.751 |
| $a+b\sqrt{x}/\sqrt{y}+c/yz$ | 203.07 | 145.90 | 0.498 | 0.1081 | 0.0817 | 0.4226 | 0.3380 | 0.2429 | 0.516 |

(continued on next page)

**Table 4 – continued from previous page**

| Functional form | $T_{eff}$ (K) | | | Radius ($R_\odot$) | | | log (L/$L_\odot$) | | |
|---|---|---|---|---|---|---|---|---|---|
| | RMSE | MAD | $R^2_{ap}$ | RMSE | MAD | $R^2_{ap}$ | RMSE | MAD | $R^2_{ap}$ |
| $a+b\sqrt{x}/\sqrt{y}+c/yz^2$ | 212.50 | 156.35 | 0.451 | 0.1121 | 0.0853 | 0.3798 | 0.3524 | 0.2577 | 0.474 |
| $a+b\sqrt{x}/\sqrt{y}+c/y\sqrt{z}$ | 207.18 | 148.34 | 0.478 | 0.1083 | 0.0832 | 0.4206 | 0.3410 | 0.2443 | 0.507 |
| $a+b\sqrt{x}/\sqrt{y}+cz/y$ | 201.65 | 148.27 | 0.505 | 0.0975 | 0.0771 | 0.5304 | 0.3293 | 0.2502 | 0.541 |
| $a+b\sqrt{x}/\sqrt{y}+cz^2/y$ | 154.20 | 119.98 | 0.711 | 0.0759 | 0.0581 | 0.7155 | 0.2693 | 0.2055 | 0.693 |
| $a+b\sqrt{x}/\sqrt{y}+c\sqrt{z}/y$ | 256.96 | 190.95 | 0.197 | 0.1217 | 0.0954 | 0.2692 | 0.4024 | 0.3109 | 0.314 |
| $a+b\sqrt{x}/\sqrt{y}+c/y^2z$ | 239.65 | 174.56 | 0.301 | 0.1193 | 0.0914 | 0.2974 | 0.3828 | 0.2801 | 0.379 |
| $a+b\sqrt{x}/\sqrt{y}+c/y^2z^2$ | 235.93 | 172.46 | 0.323 | 0.1190 | 0.0910 | 0.3014 | 0.3799 | 0.2784 | 0.389 |
| $a+b\sqrt{x}/\sqrt{y}+c/y^2\sqrt{z}$ | 244.38 | 179.16 | 0.273 | 0.1201 | 0.0919 | 0.2882 | 0.3877 | 0.2841 | 0.363 |
| $a+b\sqrt{x}/\sqrt{y}+cz/y^2$ | 254.97 | 189.47 | 0.209 | 0.1214 | 0.0952 | 0.2719 | 0.4003 | 0.3110 | 0.321 |
| $a+b\sqrt{x}/\sqrt{y}+cz^2/y^2$ | 201.32 | 148.74 | 0.507 | 0.0989 | 0.0777 | 0.5167 | 0.3296 | 0.2533 | 0.540 |
| $a+b\sqrt{x}/\sqrt{y}+c\sqrt{z}/y^2$ | 258.85 | 192.96 | 0.185 | 0.1232 | 0.0963 | 0.2501 | 0.4050 | 0.3076 | 0.305 |
| $a+b\sqrt{x}/\sqrt{y}+c/\sqrt{y}z$ | 176.95 | 128.17 | 0.619 | 0.0987 | 0.0750 | 0.5193 | 0.3066 | 0.2129 | 0.602 |
| $a+b\sqrt{x}/\sqrt{y}+c/\sqrt{y}z^2$ | 204.23 | 152.13 | 0.493 | 0.1085 | 0.0834 | 0.4186 | 0.3425 | 0.2480 | 0.503 |
| $a+b\sqrt{x}/\sqrt{y}+c/\sqrt{y}\sqrt{z}$ | 168.52 | 118.74 | 0.654 | 0.0947 | 0.0714 | 0.5569 | 0.2942 | 0.1995 | 0.633 |
| $a+b\sqrt{x}/\sqrt{y}+cz/\sqrt{y}$ | 152.70 | 121.22 | 0.716 | 0.0771 | 0.0587 | 0.7066 | 0.2684 | 0.2029 | 0.695 |
| $a+b\sqrt{x}/\sqrt{y}+cz^2/\sqrt{y}$ | 146.00 | 109.72 | 0.741 | 0.0725 | 0.0541 | 0.7404 | 0.2611 | 0.1947 | 0.711 |
| $a+b\sqrt{x}/\sqrt{y}+c\sqrt{z}/\sqrt{y}$ | 203.92 | 151.87 | 0.494 | 0.0981 | 0.0778 | 0.5247 | 0.3324 | 0.2542 | 0.532 |
| $a+b\sqrt{x}y+cx/z$ | 140.39 | 112.36 | 0.760 | 0.0851 | 0.0572 | 0.6420 | 0.2826 | 0.1880 | 0.662 |
| $a+b\sqrt{x}y+cx/z^2$ | 145.26 | 117.11 | 0.743 | 0.0872 | 0.0603 | 0.6247 | 0.2846 | 0.1911 | 0.657 |
| $a+b\sqrt{x}y+cx/\sqrt{z}$ | 142.99 | 112.89 | 0.751 | 0.0860 | 0.0581 | 0.6352 | 0.2854 | 0.1899 | 0.655 |
| $a+b\sqrt{x}y+cxz$ | 121.14 | 91.57 | 0.821 | 0.0723 | 0.0493 | 0.7421 | 0.2564 | 0.1767 | 0.722 |
| $a+b\sqrt{x}y+cxz^2$ | 126.81 | 96.58 | 0.804 | 0.0763 | 0.0534 | 0.7126 | 0.2671 | 0.1805 | 0.698 |
| $a+b\sqrt{x}y+cx\sqrt{z}$ | 117.12 | 90.68 | 0.833 | 0.0689 | 0.0454 | 0.7659 | 0.2417 | 0.1607 | 0.752 |
| $a+b\sqrt{x}y+cx^2/z$ | 145.63 | 114.78 | 0.742 | 0.0858 | 0.0568 | 0.6361 | 0.2854 | 0.1896 | 0.655 |
| $a+b\sqrt{x}y+cx^2/z^2$ | 146.75 | 117.83 | 0.738 | 0.0871 | 0.0597 | 0.6251 | 0.2855 | 0.1917 | 0.655 |
| $a+b\sqrt{x}y+cx^2/\sqrt{z}$ | 151.48 | 119.54 | 0.721 | 0.0881 | 0.0599 | 0.6168 | 0.2858 | 0.1917 | 0.654 |
| $a+b\sqrt{x}y+cx^2z$ | 125.68 | 97.83 | 0.808 | 0.0765 | 0.0553 | 0.7114 | 0.2669 | 0.1851 | 0.698 |
| $a+b\sqrt{x}y+cx^2z^2$ | 129.81 | 100.38 | 0.795 | 0.0790 | 0.0562 | 0.6918 | 0.2728 | 0.1844 | 0.685 |
| $a+b\sqrt{x}y+cx^2\sqrt{z}$ | 122.23 | 96.20 | 0.818 | 0.0749 | 0.0545 | 0.7231 | 0.2608 | 0.1851 | 0.712 |
| $a+b\sqrt{x}y+c\sqrt{x}/z$ | 136.48 | 108.73 | 0.773 | 0.0847 | 0.0566 | 0.6457 | 0.2792 | 0.1850 | 0.670 |
| $a+b\sqrt{x}y+c\sqrt{x}/z^2$ | 143.95 | 115.71 | 0.748 | 0.0872 | 0.0608 | 0.6246 | 0.2835 | 0.1894 | 0.660 |
| $a+b\sqrt{x}y+c\sqrt{x}/\sqrt{z}$ | 135.82 | 106.84 | 0.776 | 0.0845 | 0.0570 | 0.6477 | 0.2811 | 0.1871 | 0.665 |
| $a+b\sqrt{x}y+c\sqrt{x}z$ | 120.85 | 91.67 | 0.822 | 0.0712 | 0.0455 | 0.7495 | 0.2526 | 0.1703 | 0.730 |
| $a+b\sqrt{x}y+c\sqrt{x}z^2$ | 125.63 | 95.74 | 0.808 | 0.0751 | 0.0516 | 0.7218 | 0.2641 | 0.1786 | 0.704 |
| $a+b\sqrt{x}y+c\sqrt{x}\sqrt{z}$ | 121.58 | 90.55 | 0.820 | 0.0693 | 0.0421 | 0.7627 | 0.2401 | 0.1489 | 0.756 |
| $a+b\sqrt{x}y+c/xz$ | 145.15 | 115.29 | 0.744 | 0.0882 | 0.0600 | 0.6157 | 0.2867 | 0.1909 | 0.652 |
| $a+b\sqrt{x}y+c/xz^2$ | 150.18 | 121.22 | 0.726 | 0.0883 | 0.0601 | 0.6154 | 0.2861 | 0.1896 | 0.653 |
| $a+b\sqrt{x}y+c/x\sqrt{z}$ | 142.62 | 111.51 | 0.753 | 0.0882 | 0.0599 | 0.6161 | 0.2866 | 0.1906 | 0.652 |
| $a+b\sqrt{x}y+cz/x$ | 134.01 | 100.12 | 0.781 | 0.0873 | 0.0598 | 0.6237 | 0.2840 | 0.1879 | 0.658 |
| $a+b\sqrt{x}y+cz^2/x$ | 122.65 | 88.96 | 0.817 | 0.0834 | 0.0570 | 0.6565 | 0.2754 | 0.1828 | 0.679 |
| $a+b\sqrt{x}y+c\sqrt{z}/x$ | 137.60 | 103.70 | 0.770 | 0.0879 | 0.0598 | 0.6189 | 0.2855 | 0.1879 | 0.655 |
| $a+b\sqrt{x}y+c/x^2z$ | 138.53 | 105.26 | 0.767 | 0.0880 | 0.0598 | 0.6174 | 0.2858 | 0.1884 | 0.654 |
| $a+b\sqrt{x}y+c/x^2z^2$ | 139.94 | 107.72 | 0.762 | 0.0880 | 0.0595 | 0.6178 | 0.2861 | 0.1896 | 0.653 |
| $a+b\sqrt{x}y+c/x^2\sqrt{z}$ | 138.16 | 104.54 | 0.768 | 0.0880 | 0.0599 | 0.6173 | 0.2857 | 0.1880 | 0.654 |
| $a+b\sqrt{x}y+cz/x^2$ | 137.43 | 103.12 | 0.770 | 0.0880 | 0.0600 | 0.6173 | 0.2854 | 0.1869 | 0.655 |
| $a+b\sqrt{x}y+cz^2/x^2$ | 136.64 | 102.39 | 0.773 | 0.0880 | 0.0601 | 0.6180 | 0.2851 | 0.1867 | 0.656 |
| $a+b\sqrt{x}y+c\sqrt{z}/x^2$ | 137.67 | 103.55 | 0.769 | 0.0880 | 0.0600 | 0.6172 | 0.2855 | 0.1872 | 0.655 |
| $a+b\sqrt{x}y+c/\sqrt{x}z$ | 151.85 | 120.30 | 0.719 | 0.0879 | 0.0633 | 0.6181 | 0.2809 | 0.1863 | 0.666 |
| $a+b\sqrt{x}y+c/\sqrt{x}z^2$ | 149.57 | 113.56 | 0.728 | 0.0881 | 0.0629 | 0.6165 | 0.2819 | 0.1874 | 0.663 |
| $a+b\sqrt{x}y+c/\sqrt{x}\sqrt{z}$ | 150.27 | 121.10 | 0.725 | 0.0882 | 0.0625 | 0.6158 | 0.2842 | 0.1889 | 0.658 |
| $a+b\sqrt{x}y+cz/\sqrt{x}$ | 121.60 | 90.49 | 0.820 | 0.0819 | 0.0554 | 0.6687 | 0.2726 | 0.1814 | 0.685 |
| $a+b\sqrt{x}y+cz^2/\sqrt{x}$ | 119.80 | 90.60 | 0.825 | 0.0756 | 0.0503 | 0.7177 | 0.2622 | 0.1761 | 0.709 |
| $a+b\sqrt{x}y+c\sqrt{z}/\sqrt{x}$ | 132.11 | 99.48 | 0.788 | 0.0863 | 0.0591 | 0.6325 | 0.2825 | 0.1887 | 0.662 |
| $a+b\sqrt{x}y+cy/z$ | 131.09 | 102.20 | 0.791 | 0.0814 | 0.0544 | 0.6728 | 0.2713 | 0.1784 | 0.688 |
| $a+b\sqrt{x}y+cy/z^2$ | 142.27 | 114.07 | 0.754 | 0.0864 | 0.0598 | 0.6316 | 0.2815 | 0.1882 | 0.664 |
| $a+b\sqrt{x}y+cy/\sqrt{z}$ | 124.82 | 98.12 | 0.810 | 0.0778 | 0.0524 | 0.7008 | 0.2649 | 0.1774 | 0.703 |
| $a+b\sqrt{x}y+cyz$ | 128.71 | 97.28 | 0.798 | 0.0771 | 0.0520 | 0.7066 | 0.2695 | 0.1767 | 0.692 |
| $a+b\sqrt{x}y+cyz^2$ | 130.04 | 98.91 | 0.794 | 0.0782 | 0.0536 | 0.6983 | 0.2717 | 0.1792 | 0.687 |
| $a+b\sqrt{x}y+cy\sqrt{z}$ | 131.14 | 100.15 | 0.791 | 0.0783 | 0.0504 | 0.6974 | 0.2715 | 0.1717 | 0.688 |
| $a+b\sqrt{x}y+cy^2/z$ | 127.71 | 100.61 | 0.802 | 0.0776 | 0.0514 | 0.7026 | 0.2640 | 0.1705 | 0.705 |
| $a+b\sqrt{x}y+cy^2/z^2$ | 140.63 | 112.10 | 0.759 | 0.0851 | 0.0577 | 0.6428 | 0.2796 | 0.1871 | 0.669 |
| $a+b\sqrt{x}y+cy^2/\sqrt{z}$ | 120.25 | 93.29 | 0.824 | 0.0713 | 0.0457 | 0.7489 | 0.2470 | 0.1579 | 0.742 |
| $a+b\sqrt{x}y+cy^2z$ | 135.80 | 101.05 | 0.776 | 0.0819 | 0.0559 | 0.6692 | 0.2799 | 0.1820 | 0.668 |
| $a+b\sqrt{x}y+cy^2z^2$ | 134.14 | 100.55 | 0.781 | 0.0812 | 0.0560 | 0.6743 | 0.2780 | 0.1819 | 0.673 |
| $a+b\sqrt{x}y+cy^2\sqrt{z}$ | 140.64 | 104.64 | 0.759 | 0.0845 | 0.0568 | 0.6477 | 0.2844 | 0.1872 | 0.657 |
| $a+b\sqrt{x}y+c\sqrt{y}/z$ | 132.13 | 102.78 | 0.788 | 0.0828 | 0.0551 | 0.6618 | 0.2721 | 0.1777 | 0.686 |
| $a+b\sqrt{x}y+c\sqrt{y}/z^2$ | 142.74 | 114.03 | 0.752 | 0.0869 | 0.0609 | 0.6273 | 0.2817 | 0.1871 | 0.664 |
| $a+b\sqrt{x}y+c\sqrt{y}/\sqrt{z}$ | 125.59 | 98.01 | 0.808 | 0.0795 | 0.0525 | 0.6880 | 0.2668 | 0.1766 | 0.698 |
| $a+b\sqrt{x}y+c\sqrt{y}z$ | 124.18 | 94.95 | 0.812 | 0.0744 | 0.0486 | 0.7268 | 0.2615 | 0.1729 | 0.710 |
| $a+b\sqrt{x}y+c\sqrt{y}z^2$ | 127.33 | 97.04 | 0.803 | 0.0763 | 0.0522 | 0.7129 | 0.2671 | 0.1780 | 0.698 |
| $a+b\sqrt{x}y+c\sqrt{y}\sqrt{z}$ | 125.26 | 96.02 | 0.809 | 0.0749 | 0.0447 | 0.7229 | 0.2597 | 0.1615 | 0.714 |
| $a+b\sqrt{x}y+c/yz$ | 151.06 | 117.65 | 0.722 | 0.0883 | 0.0622 | 0.6152 | 0.2823 | 0.1879 | 0.662 |
| $a+b\sqrt{x}y+c/yz^2$ | 148.82 | 113.20 | 0.731 | 0.0883 | 0.0621 | 0.6151 | 0.2830 | 0.1875 | 0.661 |
| $a+b\sqrt{x}y+c/y\sqrt{z}$ | 151.75 | 121.35 | 0.720 | 0.0883 | 0.0613 | 0.6147 | 0.2846 | 0.1870 | 0.657 |
| $a+b\sqrt{x}y+cz/y$ | 114.68 | 85.60 | 0.840 | 0.0775 | 0.0508 | 0.7031 | 0.2611 | 0.1769 | 0.711 |
| $a+b\sqrt{x}y+cz^2/y$ | 115.48 | 87.57 | 0.838 | 0.0723 | 0.0464 | 0.7418 | 0.2521 | 0.1702 | 0.731 |
| $a+b\sqrt{x}y+c\sqrt{z}/y$ | 127.30 | 95.95 | 0.803 | 0.0833 | 0.0571 | 0.6577 | 0.2766 | 0.1915 | 0.676 |
| $a+b\sqrt{x}y+c/y^2z$ | 151.39 | 121.35 | 0.721 | 0.0882 | 0.0598 | 0.6162 | 0.2860 | 0.1879 | 0.653 |
| $a+b\sqrt{x}y+c/y^2z^2$ | 151.69 | 119.71 | 0.720 | 0.0883 | 0.0603 | 0.6154 | 0.2853 | 0.1863 | 0.655 |
| $a+b\sqrt{x}y+c/y^2\sqrt{z}$ | 149.56 | 119.96 | 0.728 | 0.0880 | 0.0596 | 0.6173 | 0.2865 | 0.1897 | 0.652 |
| $a+b\sqrt{x}y+cz/y^2$ | 131.70 | 98.48 | 0.789 | 0.0858 | 0.0583 | 0.6363 | 0.2817 | 0.1916 | 0.664 |
| $a+b\sqrt{x}y+cz^2/y^2$ | 113.99 | 84.84 | 0.842 | 0.0793 | 0.0533 | 0.6895 | 0.2641 | 0.1794 | 0.704 |
| $a+b\sqrt{x}y+c\sqrt{z}/y^2$ | 139.74 | 107.41 | 0.762 | 0.0871 | 0.0589 | 0.6250 | 0.2854 | 0.1906 | 0.655 |
| $a+b\sqrt{x}y+c/\sqrt{y}z$ | 144.34 | 109.85 | 0.747 | 0.0870 | 0.0626 | 0.6263 | 0.2758 | 0.1811 | 0.678 |
| $a+b\sqrt{x}y+c/\sqrt{y}z^2$ | 145.60 | 112.18 | 0.742 | 0.0879 | 0.0627 | 0.6181 | 0.2818 | 0.1849 | 0.664 |
| $a+b\sqrt{x}y+c/\sqrt{y}\sqrt{z}$ | 147.96 | 110.42 | 0.734 | 0.0870 | 0.0629 | 0.6261 | 0.2755 | 0.1817 | 0.678 |
| $a+b\sqrt{x}y+cz/\sqrt{y}$ | 114.56 | 87.14 | 0.840 | 0.0734 | 0.0457 | 0.7342 | 0.2525 | 0.1649 | 0.730 |
| $a+b\sqrt{x}y+cz^2/\sqrt{y}$ | 120.22 | 91.27 | 0.824 | 0.0727 | 0.0479 | 0.7389 | 0.2560 | 0.1734 | 0.722 |
| $a+b\sqrt{x}y+c\sqrt{z}/\sqrt{y}$ | 116.94 | 89.10 | 0.834 | 0.0774 | 0.0507 | 0.7040 | 0.2614 | 0.1757 | 0.711 |
| $a+b\sqrt{x}y^2+cx/z$ | 151.60 | 115.21 | 0.720 | 0.0916 | 0.0666 | 0.5861 | 0.3118 | 0.2229 | 0.588 |
| $a+b\sqrt{x}y^2+cx/z^2$ | 151.45 | 118.15 | 0.721 | 0.0918 | 0.0666 | 0.5838 | 0.3113 | 0.2238 | 0.589 |
| $a+b\sqrt{x}y^2+cx/\sqrt{z}$ | 154.66 | 118.33 | 0.709 | 0.0923 | 0.0658 | 0.5795 | 0.3085 | 0.2131 | 0.597 |
| $a+b\sqrt{x}y^2+cxz$ | 125.14 | 95.34 | 0.809 | 0.0733 | 0.0527 | 0.7344 | 0.2690 | 0.2048 | 0.693 |

(continued on next page)

**Table 4 – continued from previous page**

| Functional form | $T_{eff}$ (K) | | | Radius ($R_{\odot}$) | | | log (L/$L_{\odot}$) | | |
|---|---|---|---|---|---|---|---|---|---|
| | RMSE | MAD | $R^2_{ap}$ | RMSE | MAD | $R^2_{ap}$ | RMSE | MAD | $R^2_{ap}$ |
| $a+b\sqrt{x}y^2+cxz^2$ | 136.65 | 103.84 | 0.773 | 0.0812 | 0.0594 | 0.6741 | 0.2931 | 0.2176 | 0.636 |
| $a+b\sqrt{x}y^2+cx\sqrt{z}$ | 117.12 | 90.67 | 0.833 | 0.0679 | 0.0446 | 0.7725 | 0.2384 | 0.1616 | 0.759 |
| $a+b\sqrt{x}y^2+cx^2/z$ | 154.43 | 117.14 | 0.710 | 0.0921 | 0.0664 | 0.5809 | 0.3107 | 0.2184 | 0.591 |
| $a+b\sqrt{x}y^2+cx^2/z^2$ | 153.19 | 118.27 | 0.714 | 0.0920 | 0.0666 | 0.5822 | 0.3119 | 0.2222 | 0.588 |
| $a+b\sqrt{x}y^2+cx^2/\sqrt{z}$ | 152.96 | 122.18 | 0.715 | 0.0913 | 0.0646 | 0.5883 | 0.2970 | 0.2121 | 0.626 |
| $a+b\sqrt{x}y^2+cx^2z$ | 133.02 | 102.21 | 0.785 | 0.0794 | 0.0596 | 0.6888 | 0.2873 | 0.2188 | 0.650 |
| $a+b\sqrt{x}y^2+cx^2z^2$ | 141.13 | 108.67 | 0.758 | 0.0848 | 0.0629 | 0.6451 | 0.3011 | 0.2178 | 0.616 |
| $a+b\sqrt{x}y^2+cx^2\sqrt{z}$ | 124.05 | 96.06 | 0.813 | 0.0742 | 0.0561 | 0.7281 | 0.2672 | 0.2036 | 0.697 |
| $a+b\sqrt{x}y^2+c\sqrt{x}/z$ | 146.58 | 111.73 | 0.739 | 0.0905 | 0.0658 | 0.5958 | 0.3088 | 0.2237 | 0.596 |
| $a+b\sqrt{x}y^2+c\sqrt{x}/z^2$ | 149.01 | 117.16 | 0.730 | 0.0915 | 0.0664 | 0.5868 | 0.3094 | 0.2232 | 0.594 |
| $a+b\sqrt{x}y^2+c\sqrt{x}/\sqrt{z}$ | 150.86 | 112.53 | 0.723 | 0.0917 | 0.0666 | 0.5851 | 0.3119 | 0.2225 | 0.588 |
| $a+b\sqrt{x}y^2+c\sqrt{x}z$ | 123.98 | 95.42 | 0.813 | 0.0723 | 0.0490 | 0.7416 | 0.2642 | 0.1962 | 0.704 |
| $a+b\sqrt{x}y^2+c\sqrt{x}z^2$ | 134.63 | 101.39 | 0.779 | 0.0796 | 0.0581 | 0.6868 | 0.2889 | 0.2168 | 0.646 |
| $a+b\sqrt{x}y^2+c\sqrt{x}\sqrt{z}$ | 120.69 | 91.33 | 0.823 | 0.0693 | 0.0429 | 0.7630 | 0.2399 | 0.1483 | 0.756 |
| $a+b\sqrt{x}y^2+c/xz$ | 154.72 | 120.74 | 0.709 | 0.0905 | 0.0633 | 0.5960 | 0.2998 | 0.2042 | 0.619 |
| $a+b\sqrt{x}y^2+c/xz^2$ | 152.57 | 119.47 | 0.717 | 0.0902 | 0.0631 | 0.5982 | 0.2951 | 0.1961 | 0.631 |
| $a+b\sqrt{x}y^2+c/x\sqrt{z}$ | 154.82 | 119.76 | 0.708 | 0.0908 | 0.0638 | 0.5927 | 0.3030 | 0.2082 | 0.611 |
| $a+b\sqrt{x}y^2+cz/x$ | 151.48 | 111.53 | 0.721 | 0.0922 | 0.0652 | 0.5804 | 0.3109 | 0.2157 | 0.590 |
| $a+b\sqrt{x}y^2+cz^2/x$ | 143.07 | 104.03 | 0.751 | 0.0910 | 0.0656 | 0.5910 | 0.3102 | 0.2232 | 0.592 |
| $a+b\sqrt{x}y^2+c\sqrt{z}/x$ | 153.34 | 115.25 | 0.714 | 0.0918 | 0.0640 | 0.5843 | 0.3087 | 0.2130 | 0.596 |
| $a+b\sqrt{x}y^2+c/x^2z$ | 153.53 | 115.91 | 0.713 | 0.0916 | 0.0641 | 0.5859 | 0.3083 | 0.2127 | 0.597 |
| $a+b\sqrt{x}y^2+c/x^2z^2$ | 154.31 | 117.84 | 0.710 | 0.0914 | 0.0639 | 0.5874 | 0.3066 | 0.2112 | 0.602 |
| $a+b\sqrt{x}y^2+c/x^2\sqrt{z}$ | 153.20 | 115.17 | 0.714 | 0.0916 | 0.0641 | 0.5853 | 0.3089 | 0.2133 | 0.596 |
| $a+b\sqrt{x}y^2+cz/x^2$ | 152.41 | 113.57 | 0.717 | 0.0918 | 0.0642 | 0.5839 | 0.3099 | 0.2140 | 0.593 |
| $a+b\sqrt{x}y^2+cz^2/x^2$ | 151.87 | 112.50 | 0.719 | 0.0919 | 0.0644 | 0.5827 | 0.3105 | 0.2142 | 0.592 |
| $a+b\sqrt{x}y^2+c\sqrt{z}/x^2$ | 152.65 | 114.05 | 0.716 | 0.0917 | 0.0642 | 0.5844 | 0.3096 | 0.2139 | 0.594 |
| $a+b\sqrt{x}y^2+c/\sqrt{x}z$ | 147.72 | 113.85 | 0.735 | 0.0875 | 0.0622 | 0.6224 | 0.2819 | 0.1841 | 0.663 |
| $a+b\sqrt{x}y^2+c/\sqrt{x}z^2$ | 144.24 | 113.15 | 0.747 | 0.0895 | 0.0637 | 0.6048 | 0.2907 | 0.1898 | 0.642 |
| $a+b\sqrt{x}y^2+c/\sqrt{x}\sqrt{z}$ | 152.22 | 119.32 | 0.718 | 0.0882 | 0.0620 | 0.6161 | 0.2880 | 0.1903 | 0.649 |
| $a+b\sqrt{x}y^2+cz/\sqrt{x}$ | 140.78 | 104.19 | 0.759 | 0.0898 | 0.0648 | 0.6019 | 0.3080 | 0.2220 | 0.598 |
| $a+b\sqrt{x}y^2+cz^2/\sqrt{x}$ | 132.21 | 97.50 | 0.787 | 0.0820 | 0.0582 | 0.6680 | 0.2923 | 0.2125 | 0.638 |
| $a+b\sqrt{x}y^2+c\sqrt{z}/\sqrt{x}$ | 151.01 | 110.21 | 0.723 | 0.0923 | 0.0659 | 0.5795 | 0.3114 | 0.2179 | 0.589 |
| $a+b\sqrt{x}y^2+cy/z$ | 142.62 | 107.03 | 0.753 | 0.0881 | 0.0641 | 0.6164 | 0.3039 | 0.2199 | 0.609 |
| $a+b\sqrt{x}y^2+cy/z^2$ | 147.95 | 115.73 | 0.734 | 0.0909 | 0.0659 | 0.5921 | 0.3081 | 0.2227 | 0.598 |
| $a+b\sqrt{x}y^2+cy/\sqrt{z}$ | 144.00 | 105.80 | 0.748 | 0.0882 | 0.0649 | 0.6161 | 0.3066 | 0.2228 | 0.602 |
| $a+b\sqrt{x}y^2+cyz$ | 134.19 | 102.64 | 0.781 | 0.0789 | 0.0564 | 0.6923 | 0.2867 | 0.2128 | 0.652 |
| $a+b\sqrt{x}y^2+cyz^2$ | 140.31 | 104.80 | 0.760 | 0.0834 | 0.0605 | 0.6563 | 0.2987 | 0.2145 | 0.622 |
| $a+b\sqrt{x}y^2+cy\sqrt{z}$ | 130.86 | 101.57 | 0.792 | 0.0761 | 0.0477 | 0.7144 | 0.2717 | 0.1867 | 0.687 |
| $a+b\sqrt{x}y^2+cy^2/z$ | 142.65 | 106.39 | 0.752 | 0.0868 | 0.0630 | 0.6283 | 0.3032 | 0.2184 | 0.610 |
| $a+b\sqrt{x}y^2+cy^2/z^2$ | 148.28 | 114.32 | 0.732 | 0.0904 | 0.0656 | 0.5965 | 0.3084 | 0.2231 | 0.597 |
| $a+b\sqrt{x}y^2+cy^2/\sqrt{z}$ | 141.66 | 105.64 | 0.756 | 0.0857 | 0.0627 | 0.6376 | 0.3024 | 0.2189 | 0.613 |
| $a+b\sqrt{x}y^2+cy^2z$ | 144.31 | 105.83 | 0.747 | 0.0858 | 0.0621 | 0.6365 | 0.3045 | 0.2149 | 0.607 |
| $a+b\sqrt{x}y^2+cy^2z^2$ | 145.58 | 108.48 | 0.742 | 0.0872 | 0.0637 | 0.6245 | 0.3067 | 0.2178 | 0.602 |
| $a+b\sqrt{x}y^2+cy^2\sqrt{z}$ | 144.55 | 104.67 | 0.746 | 0.0855 | 0.0607 | 0.6393 | 0.3037 | 0.2118 | 0.609 |
| $a+b\sqrt{x}y^2+c\sqrt{y}/z$ | 139.52 | 105.83 | 0.763 | 0.0877 | 0.0627 | 0.6199 | 0.2996 | 0.2144 | 0.620 |
| $a+b\sqrt{x}y^2+c\sqrt{y}/z^2$ | 146.59 | 115.53 | 0.739 | 0.0908 | 0.0656 | 0.5926 | 0.3064 | 0.2203 | 0.602 |
| $a+b\sqrt{x}y^2+c\sqrt{y}/\sqrt{z}$ | 139.56 | 103.70 | 0.763 | 0.0871 | 0.0632 | 0.6258 | 0.3018 | 0.2180 | 0.614 |
| $a+b\sqrt{x}y^2+c\sqrt{y}z$ | 128.89 | 99.66 | 0.798 | 0.0762 | 0.0528 | 0.7130 | 0.2770 | 0.2055 | 0.675 |
| $a+b\sqrt{x}y^2+c\sqrt{y}z^2$ | 136.82 | 102.55 | 0.772 | 0.0811 | 0.0588 | 0.6751 | 0.2928 | 0.2161 | 0.637 |
| $a+b\sqrt{x}y^2+c\sqrt{y}\sqrt{z}$ | 125.73 | 97.86 | 0.808 | 0.0744 | 0.0443 | 0.7266 | 0.2624 | 0.1741 | 0.708 |
| $a+b\sqrt{x}y^2+c/yz$ | 145.36 | 111.11 | 0.743 | 0.0892 | 0.0628 | 0.6072 | 0.2870 | 0.1873 | 0.651 |
| $a+b\sqrt{x}y^2+c/yz^2$ | 143.60 | 110.99 | 0.749 | 0.0904 | 0.0647 | 0.5965 | 0.2943 | 0.1985 | 0.633 |
| $a+b\sqrt{x}y^2+c/y\sqrt{z}$ | 149.62 | 116.91 | 0.728 | 0.0895 | 0.0620 | 0.6048 | 0.2893 | 0.1892 | 0.645 |
| $a+b\sqrt{x}y^2+cz/y$ | 135.02 | 101.31 | 0.778 | 0.0867 | 0.0627 | 0.6289 | 0.3010 | 0.2191 | 0.616 |
| $a+b\sqrt{x}y^2+cz^2/y$ | 125.89 | 92.73 | 0.807 | 0.0782 | 0.0545 | 0.6983 | 0.2809 | 0.2091 | 0.666 |
| $a+b\sqrt{x}y^2+c\sqrt{z}/y$ | 150.19 | 108.76 | 0.726 | 0.0919 | 0.0666 | 0.5829 | 0.3119 | 0.2218 | 0.588 |
| $a+b\sqrt{x}y^2+c/y^2z$ | 151.22 | 118.61 | 0.722 | 0.0907 | 0.0630 | 0.5939 | 0.2957 | 0.1927 | 0.629 |
| $a+b\sqrt{x}y^2+c/y^2z^2$ | 148.21 | 114.04 | 0.733 | 0.0910 | 0.0643 | 0.5914 | 0.2966 | 0.1974 | 0.627 |
| $a+b\sqrt{x}y^2+c/y^2\sqrt{z}$ | 153.11 | 120.52 | 0.715 | 0.0908 | 0.0624 | 0.5930 | 0.2975 | 0.1943 | 0.625 |
| $a+b\sqrt{x}y^2+cz/y^2$ | 152.15 | 112.13 | 0.718 | 0.0923 | 0.0658 | 0.5795 | 0.3110 | 0.2151 | 0.590 |
| $a+b\sqrt{x}y^2+cz^2/y^2$ | 136.28 | 101.21 | 0.774 | 0.0884 | 0.0641 | 0.6145 | 0.3042 | 0.2220 | 0.608 |
| $a+b\sqrt{x}y^2+c\sqrt{z}/y^2$ | 154.65 | 118.80 | 0.709 | 0.0918 | 0.0636 | 0.5836 | 0.3065 | 0.2078 | 0.602 |
| $a+b\sqrt{x}y^2+c/\sqrt{y}z$ | 137.87 | 106.44 | 0.769 | 0.0874 | 0.0617 | 0.6229 | 0.2816 | 0.1829 | 0.664 |
| $a+b\sqrt{x}y^2+c/\sqrt{y}z^2$ | 142.50 | 112.17 | 0.753 | 0.0903 | 0.0643 | 0.5972 | 0.2972 | 0.2042 | 0.626 |
| $a+b\sqrt{x}y^2+c/\sqrt{y}\sqrt{z}$ | 140.82 | 107.60 | 0.759 | 0.0864 | 0.0601 | 0.6315 | 0.2762 | 0.1767 | 0.677 |
| $a+b\sqrt{x}y^2+cz/\sqrt{y}$ | 124.70 | 93.15 | 0.811 | 0.0791 | 0.0536 | 0.6914 | 0.2809 | 0.2021 | 0.666 |
| $a+b\sqrt{x}y^2+cz^2/\sqrt{y}$ | 128.92 | 97.03 | 0.798 | 0.0776 | 0.0549 | 0.7029 | 0.2813 | 0.2117 | 0.665 |
| $a+b\sqrt{x}y^2+c\sqrt{z}/\sqrt{y}$ | 135.54 | 101.88 | 0.776 | 0.0863 | 0.0624 | 0.6324 | 0.3002 | 0.2180 | 0.618 |
| $a+b\sqrt{x}\sqrt{y}+cx/z$ | 138.65 | 107.95 | 0.766 | 0.0821 | 0.0549 | 0.6669 | 0.2679 | 0.1740 | 0.696 |
| $a+b\sqrt{x}\sqrt{y}+cx/z^2$ | 148.71 | 114.36 | 0.731 | 0.0864 | 0.0636 | 0.6317 | 0.2752 | 0.1844 | 0.679 |
| $a+b\sqrt{x}\sqrt{y}+cx/\sqrt{z}$ | 137.69 | 107.91 | 0.769 | 0.0812 | 0.0518 | 0.6743 | 0.2687 | 0.1721 | 0.694 |
| $a+b\sqrt{x}\sqrt{y}+cxz$ | 119.76 | 89.80 | 0.825 | 0.0709 | 0.0469 | 0.7520 | 0.2461 | 0.1631 | 0.743 |
| $a+b\sqrt{x}\sqrt{y}+cxz^2$ | 123.82 | 93.78 | 0.813 | 0.0733 | 0.0495 | 0.7344 | 0.2526 | 0.1673 | 0.730 |
| $a+b\sqrt{x}\sqrt{y}+cx\sqrt{z}$ | 117.11 | 90.69 | 0.833 | 0.0695 | 0.0448 | 0.7618 | 0.2398 | 0.1567 | 0.756 |
| $a+b\sqrt{x}\sqrt{y}+cx^2/z$ | 147.10 | 111.90 | 0.737 | 0.0831 | 0.0557 | 0.6589 | 0.2732 | 0.1757 | 0.684 |
| $a+b\sqrt{x}\sqrt{y}+cx^2/z^2$ | 150.35 | 115.37 | 0.725 | 0.0861 | 0.0628 | 0.6337 | 0.2763 | 0.1840 | 0.677 |
| $a+b\sqrt{x}\sqrt{y}+cx^2/\sqrt{z}$ | 158.84 | 118.49 | 0.693 | 0.0875 | 0.0626 | 0.6220 | 0.2805 | 0.1844 | 0.667 |
| $a+b\sqrt{x}\sqrt{y}+cx^2z$ | 122.72 | 95.11 | 0.817 | 0.0741 | 0.0517 | 0.7290 | 0.2538 | 0.1705 | 0.727 |
| $a+b\sqrt{x}\sqrt{y}+cx^2z^2$ | 126.14 | 96.34 | 0.806 | 0.0758 | 0.0526 | 0.7164 | 0.2578 | 0.1712 | 0.718 |
| $a+b\sqrt{x}\sqrt{y}+cx^2\sqrt{z}$ | 120.80 | 94.74 | 0.822 | 0.0739 | 0.0518 | 0.7306 | 0.2515 | 0.1696 | 0.732 |
| $a+b\sqrt{x}\sqrt{y}+c\sqrt{x}/z$ | 135.41 | 103.86 | 0.777 | 0.0823 | 0.0560 | 0.6652 | 0.2652 | 0.1705 | 0.702 |
| $a+b\sqrt{x}\sqrt{y}+c\sqrt{x}/z^2$ | 147.93 | 112.83 | 0.734 | 0.0867 | 0.0643 | 0.6292 | 0.2746 | 0.1839 | 0.681 |
| $a+b\sqrt{x}\sqrt{y}+c\sqrt{x}/\sqrt{z}$ | 129.23 | 100.63 | 0.797 | 0.0801 | 0.0518 | 0.6832 | 0.2623 | 0.1654 | 0.708 |
| $a+b\sqrt{x}\sqrt{y}+c\sqrt{x}z$ | 120.32 | 89.77 | 0.824 | 0.0701 | 0.0434 | 0.7576 | 0.2435 | 0.1560 | 0.749 |
| $a+b\sqrt{x}\sqrt{y}+c\sqrt{x}z^2$ | 123.18 | 92.94 | 0.815 | 0.0723 | 0.0474 | 0.7421 | 0.2501 | 0.1638 | 0.735 |
| $a+b\sqrt{x}\sqrt{y}+c\sqrt{x}\sqrt{z}$ | 122.06 | 91.42 | 0.819 | 0.0695 | 0.0412 | 0.7617 | 0.2386 | 0.1450 | 0.759 |
| $a+b\sqrt{x}\sqrt{y}+c/xz$ | 135.49 | 106.74 | 0.777 | 0.0857 | 0.0587 | 0.6374 | 0.2730 | 0.1757 | 0.684 |
| $a+b\sqrt{x}\sqrt{y}+c/xz^2$ | 149.04 | 120.78 | 0.730 | 0.0860 | 0.0597 | 0.6346 | 0.2769 | 0.1853 | 0.675 |
| $a+b\sqrt{x}\sqrt{y}+c/x\sqrt{z}$ | 131.84 | 100.63 | 0.789 | 0.0858 | 0.0598 | 0.6365 | 0.2718 | 0.1730 | 0.687 |
| $a+b\sqrt{x}\sqrt{y}+cz/x$ | 123.00 | 92.74 | 0.816 | 0.0843 | 0.0597 | 0.6490 | 0.2653 | 0.1713 | 0.702 |

(continued on next page)

**Table 4 – continued from previous page**

| Functional form | $T_{eff}$ (K) | | | Radius ($R_\odot$) | | | log (L/$L_\odot$) | | |
|---|---|---|---|---|---|---|---|---|---|
| | RMSE | MAD | $R^2_{ap}$ | RMSE | MAD | $R^2_{ap}$ | RMSE | MAD | $R^2_{ap}$ |
| $a+b\sqrt{x}\sqrt{y}+cz^2/x$ | 110.57 | 79.30 | 0.851 | 0.0786 | 0.0532 | 0.6947 | 0.2528 | 0.1581 | 0.729 |
| $a+b\sqrt{x}\sqrt{y}+c\sqrt{z}/x$ | 127.00 | 95.80 | 0.804 | 0.0854 | 0.0605 | 0.6401 | 0.2686 | 0.1727 | 0.694 |
| $a+b\sqrt{x}\sqrt{y}+c/x^2z$ | 128.96 | 97.89 | 0.798 | 0.0859 | 0.0609 | 0.6353 | 0.2699 | 0.1731 | 0.691 |
| $a+b\sqrt{x}\sqrt{y}+c/x^2z^2$ | 128.75 | 95.85 | 0.798 | 0.0854 | 0.0598 | 0.6402 | 0.2695 | 0.1707 | 0.692 |
| $a+b\sqrt{x}\sqrt{y}+c/x^2\sqrt{z}$ | 129.35 | 98.99 | 0.796 | 0.0861 | 0.0612 | 0.6336 | 0.2701 | 0.1737 | 0.691 |
| $a+b\sqrt{x}\sqrt{y}+cz/x^2$ | 130.11 | 100.51 | 0.794 | 0.0864 | 0.0615 | 0.6313 | 0.2703 | 0.1745 | 0.690 |
| $a+b\sqrt{x}\sqrt{y}+cz^2/x^2$ | 129.48 | 100.31 | 0.796 | 0.0863 | 0.0615 | 0.6324 | 0.2698 | 0.1744 | 0.692 |
| $a+b\sqrt{x}\sqrt{y}+c\sqrt{z}/x^2$ | 129.99 | 100.24 | 0.794 | 0.0864 | 0.0615 | 0.6316 | 0.2703 | 0.1743 | 0.690 |
| $a+b\sqrt{x}\sqrt{y}+c/\sqrt{x}z$ | 158.24 | 125.13 | 0.695 | 0.0886 | 0.0661 | 0.6126 | 0.2807 | 0.1880 | 0.666 |
| $a+b\sqrt{x}\sqrt{y}+c/\sqrt{x}z^2$ | 159.00 | 118.78 | 0.692 | 0.0888 | 0.0666 | 0.6111 | 0.2799 | 0.1909 | 0.668 |
| $a+b\sqrt{x}\sqrt{y}+c/\sqrt{x}\sqrt{z}$ | 147.98 | 120.35 | 0.734 | 0.0878 | 0.0639 | 0.6192 | 0.2792 | 0.1850 | 0.670 |
| $a+b\sqrt{x}\sqrt{y}+cz/\sqrt{x}$ | 110.99 | 79.84 | 0.850 | 0.0770 | 0.0507 | 0.7071 | 0.2503 | 0.1537 | 0.735 |
| $a+b\sqrt{x}\sqrt{y}+cz^2/\sqrt{x}$ | 115.16 | 87.56 | 0.839 | 0.0718 | 0.0455 | 0.7453 | 0.2448 | 0.1513 | 0.746 |
| $a+b\sqrt{x}\sqrt{y}+c\sqrt{z}/\sqrt{x}$ | 118.83 | 86.82 | 0.828 | 0.0820 | 0.0565 | 0.6681 | 0.2612 | 0.1662 | 0.711 |
| $a+b\sqrt{x}\sqrt{y}+cy/z$ | 131.29 | 98.30 | 0.790 | 0.0788 | 0.0521 | 0.6930 | 0.2562 | 0.1613 | 0.722 |
| $a+b\sqrt{x}\sqrt{y}+cy/z^2$ | 146.17 | 111.70 | 0.740 | 0.0856 | 0.0631 | 0.6378 | 0.2720 | 0.1824 | 0.686 |
| $a+b\sqrt{x}\sqrt{y}+cy/\sqrt{z}$ | 123.23 | 93.53 | 0.815 | 0.0734 | 0.0458 | 0.7342 | 0.2433 | 0.1478 | 0.749 |
| $a+b\sqrt{x}\sqrt{y}+cyz$ | 126.11 | 94.77 | 0.806 | 0.0750 | 0.0477 | 0.7222 | 0.2572 | 0.1616 | 0.720 |
| $a+b\sqrt{x}\sqrt{y}+cyz^2$ | 126.58 | 95.88 | 0.805 | 0.0750 | 0.0494 | 0.7222 | 0.2569 | 0.1648 | 0.720 |
| $a+b\sqrt{x}\sqrt{y}+cy\sqrt{z}$ | 130.43 | 99.11 | 0.793 | 0.0779 | 0.0482 | 0.7002 | 0.2633 | 0.1617 | 0.706 |
| $a+b\sqrt{x}\sqrt{y}+cy^2/z$ | 130.41 | 98.50 | 0.793 | 0.0748 | 0.0482 | 0.7235 | 0.2475 | 0.1530 | 0.740 |
| $a+b\sqrt{x}\sqrt{y}+cy^2/z^2$ | 143.95 | 109.48 | 0.748 | 0.0838 | 0.0601 | 0.6531 | 0.2687 | 0.1798 | 0.694 |
| $a+b\sqrt{x}\sqrt{y}+cy^2/\sqrt{z}$ | 134.84 | 99.24 | 0.779 | 0.0719 | 0.0502 | 0.7445 | 0.2354 | 0.1511 | 0.765 |
| $a+b\sqrt{x}\sqrt{y}+cy^2z$ | 131.99 | 98.87 | 0.788 | 0.0790 | 0.0520 | 0.6917 | 0.2663 | 0.1683 | 0.700 |
| $a+b\sqrt{x}\sqrt{y}+cy^2z^2$ | 130.07 | 97.47 | 0.794 | 0.0779 | 0.0525 | 0.7006 | 0.2631 | 0.1688 | 0.707 |
| $a+b\sqrt{x}\sqrt{y}+cy^2\sqrt{z}$ | 137.87 | 103.57 | 0.769 | 0.0823 | 0.0537 | 0.6654 | 0.2729 | 0.1759 | 0.685 |
| $a+b\sqrt{x}\sqrt{y}+c\sqrt{y}/z$ | 133.50 | 98.65 | 0.783 | 0.0811 | 0.0552 | 0.6753 | 0.2599 | 0.1645 | 0.714 |
| $a+b\sqrt{x}\sqrt{y}+c\sqrt{y}/z^2$ | 147.49 | 111.98 | 0.735 | 0.0865 | 0.0644 | 0.6302 | 0.2734 | 0.1831 | 0.683 |
| $a+b\sqrt{x}\sqrt{y}+c\sqrt{y}/\sqrt{z}$ | 123.78 | 93.30 | 0.814 | 0.0762 | 0.0487 | 0.7137 | 0.2491 | 0.1507 | 0.737 |
| $a+b\sqrt{x}\sqrt{y}+c\sqrt{y}z$ | 122.38 | 92.82 | 0.818 | 0.0726 | 0.0447 | 0.7398 | 0.2501 | 0.1561 | 0.735 |
| $a+b\sqrt{x}\sqrt{y}+c\sqrt{y}z^2$ | 124.42 | 94.17 | 0.812 | 0.0733 | 0.0476 | 0.7348 | 0.2526 | 0.1629 | 0.730 |
| $a+b\sqrt{x}\sqrt{y}+c\sqrt{y}\sqrt{z}$ | 124.91 | 95.07 | 0.810 | 0.0746 | 0.0442 | 0.7253 | 0.2534 | 0.1493 | 0.728 |
| $a+b\sqrt{x}\sqrt{y}+c/yz$ | 159.88 | 122.19 | 0.689 | 0.0884 | 0.0657 | 0.6140 | 0.2806 | 0.1884 | 0.666 |
| $a+b\sqrt{x}\sqrt{y}+c/yz^2$ | 158.27 | 119.67 | 0.695 | 0.0887 | 0.0665 | 0.6116 | 0.2800 | 0.1905 | 0.668 |
| $a+b\sqrt{x}\sqrt{y}+c/y\sqrt{z}$ | 156.56 | 123.64 | 0.702 | 0.0872 | 0.0631 | 0.6242 | 0.2798 | 0.1885 | 0.668 |
| $a+b\sqrt{x}\sqrt{y}+cz/y$ | 107.06 | 79.94 | 0.861 | 0.0725 | 0.0457 | 0.7406 | 0.2375 | 0.1428 | 0.761 |
| $a+b\sqrt{x}\sqrt{y}+cz^2/y$ | 113.65 | 85.05 | 0.843 | 0.0692 | 0.0419 | 0.7633 | 0.2365 | 0.1442 | 0.763 |
| $a+b\sqrt{x}\sqrt{y}+c\sqrt{z}/y$ | 112.27 | 83.72 | 0.847 | 0.0766 | 0.0502 | 0.7102 | 0.2482 | 0.1619 | 0.739 |
| $a+b\sqrt{x}\sqrt{y}+c/y^2z$ | 154.52 | 122.05 | 0.709 | 0.0861 | 0.0612 | 0.6340 | 0.2783 | 0.1862 | 0.672 |
| $a+b\sqrt{x}\sqrt{y}+c/y^2z^2$ | 159.46 | 122.86 | 0.691 | 0.0874 | 0.0636 | 0.6231 | 0.2803 | 0.1885 | 0.667 |
| $a+b\sqrt{x}\sqrt{y}+c/y^2\sqrt{z}$ | 147.66 | 117.18 | 0.735 | 0.0850 | 0.0588 | 0.6429 | 0.2754 | 0.1844 | 0.679 |
| $a+b\sqrt{x}\sqrt{y}+cz/y^2$ | 115.72 | 84.42 | 0.837 | 0.0805 | 0.0544 | 0.6801 | 0.2566 | 0.1665 | 0.721 |
| $a+b\sqrt{x}\sqrt{y}+cz^2/y^2$ | 103.88 | 74.00 | 0.869 | 0.0740 | 0.0482 | 0.7293 | 0.2391 | 0.1473 | 0.758 |
| $a+b\sqrt{x}\sqrt{y}+c\sqrt{z}/y^2$ | 125.84 | 94.55 | 0.807 | 0.0824 | 0.0551 | 0.6649 | 0.2643 | 0.1719 | 0.704 |
| $a+b\sqrt{x}\sqrt{y}+c/\sqrt{y}z$ | 152.75 | 112.65 | 0.716 | 0.0880 | 0.0658 | 0.6177 | 0.2746 | 0.1871 | 0.681 |
| $a+b\sqrt{x}\sqrt{y}+c/\sqrt{y}z^2$ | 153.83 | 115.90 | 0.712 | 0.0885 | 0.0662 | 0.6130 | 0.2776 | 0.1909 | 0.673 |
| $a+b\sqrt{x}\sqrt{y}+c/\sqrt{y}\sqrt{z}$ | 156.66 | 114.61 | 0.701 | 0.0883 | 0.0657 | 0.6151 | 0.2763 | 0.1867 | 0.677 |
| $a+b\sqrt{x}\sqrt{y}+cz/\sqrt{y}$ | 112.62 | 85.40 | 0.846 | 0.0704 | 0.0428 | 0.7554 | 0.2368 | 0.1384 | 0.762 |
| $a+b\sqrt{x}\sqrt{y}+cz^2/\sqrt{y}$ | 118.57 | 89.23 | 0.829 | 0.0700 | 0.0427 | 0.7581 | 0.2418 | 0.1534 | 0.752 |
| $a+b\sqrt{x}\sqrt{y}+c\sqrt{z}/\sqrt{y}$ | 111.06 | 83.79 | 0.850 | 0.0728 | 0.0458 | 0.7386 | 0.2393 | 0.1426 | 0.757 |
| $a+b/xy+cx/z$ | 250.53 | 177.74 | 0.236 | 0.1184 | 0.0909 | 0.3078 | 0.4111 | 0.3089 | 0.284 |
| $a+b/xy+cx/z^2$ | 247.44 | 180.25 | 0.255 | 0.1211 | 0.0953 | 0.2757 | 0.4103 | 0.3076 | 0.287 |
| $a+b/xy+cx/\sqrt{z}$ | 277.86 | 210.73 | 0.061 | 0.1343 | 0.1075 | 0.1092 | 0.4474 | 0.3524 | 0.152 |
| $a+b/xy+cxz$ | 128.38 | 96.14 | 0.799 | 0.0712 | 0.0486 | 0.7497 | 0.2590 | 0.1855 | 0.716 |
| $a+b/xy+cxz^2$ | 152.11 | 114.54 | 0.718 | 0.0786 | 0.0578 | 0.6952 | 0.2901 | 0.2099 | 0.643 |
| $a+b/xy+cx\sqrt{z}$ | 112.55 | 85.94 | 0.846 | 0.0696 | 0.0444 | 0.7610 | 0.2409 | 0.1596 | 0.754 |
| $a+b/xy+cx^2/z$ | 280.50 | 210.91 | 0.043 | 0.1344 | 0.1070 | 0.1080 | 0.4505 | 0.3516 | 0.140 |
| $a+b/xy+cx^2/z^2$ | 262.70 | 190.80 | 0.160 | 0.1261 | 0.0986 | 0.2154 | 0.4302 | 0.3266 | 0.216 |
| $a+b/xy+cx^2/\sqrt{z}$ | 186.75 | 143.04 | 0.576 | 0.1052 | 0.0823 | 0.4530 | 0.3272 | 0.2501 | 0.546 |
| $a+b/xy+cx^2z$ | 136.51 | 104.88 | 0.773 | 0.0754 | 0.0549 | 0.7195 | 0.2734 | 0.2028 | 0.683 |
| $a+b/xy+cx^2z^2$ | 157.74 | 122.12 | 0.697 | 0.0826 | 0.0628 | 0.6631 | 0.3016 | 0.2241 | 0.615 |
| $a+b/xy+cx^2\sqrt{z}$ | 124.05 | 95.79 | 0.813 | 0.0734 | 0.0523 | 0.7343 | 0.2578 | 0.1854 | 0.718 |
| $a+b/xy+c\sqrt{x}/z$ | 213.31 | 149.64 | 0.446 | 0.1055 | 0.0760 | 0.4503 | 0.3619 | 0.2569 | 0.445 |
| $a+b/xy+c\sqrt{x}/z^2$ | 234.82 | 171.78 | 0.329 | 0.1176 | 0.0919 | 0.3171 | 0.3941 | 0.2917 | 0.342 |
| $a+b/xy+c\sqrt{x}/\sqrt{z}$ | 240.64 | 167.72 | 0.295 | 0.1126 | 0.0853 | 0.3743 | 0.3957 | 0.2954 | 0.337 |
| $a+b/xy+c\sqrt{x}z$ | 129.44 | 99.88 | 0.796 | 0.0707 | 0.0457 | 0.7530 | 0.2572 | 0.1777 | 0.720 |
| $a+b/xy+c\sqrt{x}z^2$ | 151.27 | 116.21 | 0.722 | 0.0773 | 0.0556 | 0.7052 | 0.2864 | 0.2046 | 0.652 |
| $a+b/xy+c\sqrt{x}\sqrt{z}$ | 114.63 | 87.65 | 0.840 | 0.0695 | 0.0407 | 0.7614 | 0.2403 | 0.1490 | 0.755 |
| $a+b/xy+c/xz$ | 198.56 | 143.65 | 0.520 | 0.1108 | 0.0853 | 0.3942 | 0.3458 | 0.2519 | 0.493 |
| $a+b/xy+c/xz^2$ | 226.09 | 161.87 | 0.378 | 0.1203 | 0.0926 | 0.2851 | 0.3842 | 0.2818 | 0.375 |
| $a+b/xy+c/x\sqrt{z}$ | 162.36 | 117.31 | 0.679 | 0.0976 | 0.0745 | 0.5292 | 0.2962 | 0.2061 | 0.628 |
| $a+b/xy+cz/x$ | 175.91 | 121.75 | 0.624 | 0.0971 | 0.0685 | 0.5347 | 0.3143 | 0.2176 | 0.581 |
| $a+b/xy+cz^2/x$ | 144.83 | 104.50 | 0.745 | 0.0780 | 0.0544 | 0.6993 | 0.2734 | 0.1802 | 0.683 |
| $a+b/xy+c\sqrt{z}/x$ | 231.20 | 160.19 | 0.350 | 0.1191 | 0.0897 | 0.2998 | 0.3884 | 0.2792 | 0.361 |
| $a+b/xy+c/x^2z$ | 238.45 | 173.50 | 0.308 | 0.1244 | 0.0973 | 0.2363 | 0.3995 | 0.2978 | 0.324 |
| $a+b/xy+c/x^2z^2$ | 278.30 | 205.77 | 0.058 | 0.1315 | 0.1049 | 0.1458 | 0.4459 | 0.3421 | 0.157 |
| $a+b/xy+c/x^2\sqrt{z}$ | 243.19 | 175.48 | 0.280 | 0.1258 | 0.0980 | 0.2192 | 0.4056 | 0.2997 | 0.303 |
| $a+b/xy+cz/x^2$ | 244.07 | 175.16 | 0.275 | 0.1258 | 0.0979 | 0.2180 | 0.4064 | 0.2983 | 0.300 |
| $a+b/xy+cz^2/x^2$ | 235.61 | 169.61 | 0.325 | 0.1229 | 0.0962 | 0.2541 | 0.3952 | 0.2909 | 0.338 |
| $a+b/xy+c\sqrt{z}/x^2$ | 245.14 | 175.81 | 0.269 | 0.1262 | 0.0981 | 0.2131 | 0.4079 | 0.2994 | 0.295 |
| $a+b/xy+c/\sqrt{x}z$ | 175.04 | 125.80 | 0.627 | 0.1013 | 0.0774 | 0.4929 | 0.3157 | 0.2190 | 0.578 |
| $a+b/xy+c/\sqrt{x}z^2$ | 211.60 | 152.22 | 0.455 | 0.1145 | 0.0888 | 0.3531 | 0.3658 | 0.2650 | 0.433 |
| $a+b/xy+c/\sqrt{x}\sqrt{z}$ | 149.75 | 106.49 | 0.727 | 0.0923 | 0.0695 | 0.5791 | 0.2824 | 0.1895 | 0.662 |
| $a+b/xy+cz/\sqrt{x}$ | 148.80 | 116.19 | 0.731 | 0.0772 | 0.0505 | 0.7058 | 0.2749 | 0.1856 | 0.680 |
| $a+b/xy+cz^2/\sqrt{x}$ | 152.34 | 117.34 | 0.718 | 0.0766 | 0.0548 | 0.7101 | 0.2822 | 0.2041 | 0.663 |
| $a+b/xy+c\sqrt{z}/\sqrt{x}$ | 185.48 | 138.81 | 0.581 | 0.0910 | 0.0633 | 0.5915 | 0.3206 | 0.2288 | 0.565 |
| $a+b/xy+cy/z$ | 229.20 | 164.66 | 0.361 | 0.1088 | 0.0812 | 0.4160 | 0.3763 | 0.2800 | 0.400 |
| $a+b/xy+cy/z^2$ | 236.43 | 171.97 | 0.320 | 0.1170 | 0.0911 | 0.3236 | 0.3941 | 0.2914 | 0.342 |
| $a+b/xy+cy/\sqrt{z}$ | 277.24 | 204.22 | 0.065 | 0.1289 | 0.0983 | 0.1801 | 0.4418 | 0.3350 | 0.173 |
| $a+b/xy+cyz$ | 136.87 | 107.58 | 0.772 | 0.0760 | 0.0503 | 0.7146 | 0.2751 | 0.1940 | 0.679 |
| $a+b/xy+cyz^2$ | 155.98 | 120.34 | 0.704 | 0.0809 | 0.0586 | 0.6771 | 0.2973 | 0.2121 | 0.625 |
| $a+b/xy+cy\sqrt{z}$ | 129.83 | 99.38 | 0.795 | 0.0779 | 0.0481 | 0.7003 | 0.2708 | 0.1730 | 0.689 |
| $a+b/xy+cy^2/z$ | 274.86 | 201.59 | 0.081 | 0.1277 | 0.0977 | 0.1948 | 0.4383 | 0.3309 | 0.186 |

(continued on next page)

**Table 4 – continued from previous page**

| Functional form | $T_{eff}$ (K) | | | Radius ($R_{\odot}$) | | | log (L/$L_{\odot}$) | | |
|---|---|---|---|---|---|---|---|---|---|
| | RMSE | MAD | $R^2_{ap}$ | RMSE | MAD | $R^2_{ap}$ | RMSE | MAD | $R^2_{ap}$ |
| $a+b/xy+cy^2/z^2$ | 248.85 | 180.20 | 0.247 | 0.1197 | 0.0924 | 0.2925 | 0.4080 | 0.3064 | 0.295 |
| $a+b/xy+cy^2/\sqrt{z}$ | 249.41 | 203.05 | 0.243 | 0.1279 | 0.1027 | 0.1921 | 0.4214 | 0.3316 | 0.248 |
| $a+b/xy+cy^2z$ | 147.89 | 113.02 | 0.734 | 0.0820 | 0.0566 | 0.6682 | 0.2945 | 0.2064 | 0.632 |
| $a+b/xy+cy^2z^2$ | 162.97 | 124.42 | 0.677 | 0.0857 | 0.0633 | 0.6376 | 0.3113 | 0.2247 | 0.589 |
| $a+b/xy+cy^2\sqrt{z}$ | 144.54 | 104.80 | 0.746 | 0.0841 | 0.0563 | 0.6512 | 0.2935 | 0.1918 | 0.635 |
| $a+b/xy+c\sqrt{y}/z$ | 200.03 | 142.17 | 0.513 | 0.1006 | 0.0713 | 0.5002 | 0.3413 | 0.2377 | 0.506 |
| $a+b/xy+c\sqrt{y}/z^2$ | 227.81 | 166.98 | 0.369 | 0.1154 | 0.0893 | 0.3428 | 0.3842 | 0.2822 | 0.374 |
| $a+b/xy+c\sqrt{y}/\sqrt{z}$ | 218.09 | 158.70 | 0.421 | 0.1024 | 0.0778 | 0.4820 | 0.3581 | 0.2663 | 0.457 |
| $a+b/xy+c\sqrt{y}z$ | 133.84 | 107.33 | 0.782 | 0.0734 | 0.0470 | 0.7340 | 0.2663 | 0.1837 | 0.700 |
| $a+b/xy+c\sqrt{y}z^2$ | 153.30 | 119.62 | 0.714 | 0.0786 | 0.0562 | 0.6953 | 0.2904 | 0.2062 | 0.643 |
| $a+b/xy+c\sqrt{y}\sqrt{z}$ | 124.66 | 98.30 | 0.811 | 0.0745 | 0.0427 | 0.7261 | 0.2590 | 0.1625 | 0.716 |
| $a+b/xy+c/yz$ | 196.91 | 140.88 | 0.528 | 0.1104 | 0.0850 | 0.3986 | 0.3462 | 0.2508 | 0.492 |
| $a+b/xy+c/yz^2$ | 218.51 | 157.97 | 0.419 | 0.1176 | 0.0915 | 0.3169 | 0.3754 | 0.2761 | 0.403 |
| $a+b/xy+c/y\sqrt{z}$ | 187.95 | 129.81 | 0.570 | 0.1075 | 0.0812 | 0.4296 | 0.3354 | 0.2360 | 0.523 |
| $a+b/xy+cz/y$ | 192.37 | 150.13 | 0.550 | 0.0887 | 0.0715 | 0.6116 | 0.3166 | 0.2431 | 0.575 |
| $a+b/xy+cz^2/y$ | 159.02 | 120.64 | 0.692 | 0.0768 | 0.0573 | 0.7089 | 0.2821 | 0.2037 | 0.663 |
| $a+b/xy+c\sqrt{z}/y$ | 280.23 | 207.04 | 0.045 | 0.1309 | 0.1008 | 0.1538 | 0.4471 | 0.3419 | 0.153 |
| $a+b/xy+c/y^2z$ | 237.61 | 171.44 | 0.313 | 0.1240 | 0.0965 | 0.2412 | 0.3982 | 0.2919 | 0.328 |
| $a+b/xy+c/y^2z^2$ | 242.31 | 173.42 | 0.286 | 0.1255 | 0.0969 | 0.2220 | 0.4049 | 0.2938 | 0.305 |
| $a+b/xy+c/y^2\sqrt{z}$ | 235.40 | 170.03 | 0.326 | 0.1233 | 0.0963 | 0.2499 | 0.3953 | 0.2910 | 0.338 |
| $a+b/xy+cz/y^2$ | 279.32 | 205.25 | 0.051 | 0.1301 | 0.0995 | 0.1642 | 0.4449 | 0.3384 | 0.161 |
| $a+b/xy+cz^2/y^2$ | 183.66 | 144.09 | 0.590 | 0.0861 | 0.0689 | 0.6336 | 0.3044 | 0.2353 | 0.607 |
| $a+b/xy+c\sqrt{z}/y^2$ | 254.47 | 185.87 | 0.212 | 0.1294 | 0.0999 | 0.1733 | 0.4225 | 0.3161 | 0.244 |
| $a+b/xy+c/\sqrt{y}z$ | 176.61 | 123.21 | 0.621 | 0.1014 | 0.0766 | 0.4920 | 0.3196 | 0.2178 | 0.567 |
| $a+b/xy+c/\sqrt{y}z^2$ | 213.15 | 150.87 | 0.447 | 0.1144 | 0.0877 | 0.3539 | 0.3682 | 0.2632 | 0.426 |
| $a+b/xy+c/\sqrt{y}\sqrt{z}$ | 157.11 | 109.44 | 0.700 | 0.0949 | 0.0709 | 0.5552 | 0.2961 | 0.1938 | 0.628 |
| $a+b/xy+cz/\sqrt{y}$ | 154.15 | 122.30 | 0.711 | 0.0760 | 0.0556 | 0.7147 | 0.2747 | 0.1951 | 0.680 |
| $a+b/xy+cz^2/\sqrt{y}$ | 153.54 | 115.76 | 0.713 | 0.0759 | 0.0543 | 0.7159 | 0.2810 | 0.2016 | 0.665 |
| $a+b/xy+c\sqrt{z}/\sqrt{y}$ | 199.12 | 151.62 | 0.518 | 0.0919 | 0.0727 | 0.5828 | 0.3271 | 0.2469 | 0.547 |
| $a+b/xy^2+cx/z$ | 253.84 | 179.69 | 0.216 | 0.1200 | 0.0923 | 0.2892 | 0.4170 | 0.3138 | 0.263 |
| $a+b/xy^2+cx/z^2$ | 249.70 | 181.55 | 0.241 | 0.1222 | 0.0960 | 0.2624 | 0.4147 | 0.3112 | 0.271 |
| $a+b/xy^2+cx/\sqrt{z}$ | 278.68 | 211.25 | 0.055 | 0.1353 | 0.1082 | 0.0957 | 0.4500 | 0.3549 | 0.142 |
| $a+b/xy^2+cxz$ | 128.41 | 96.10 | 0.799 | 0.0713 | 0.0487 | 0.7492 | 0.2596 | 0.1862 | 0.714 |
| $a+b/xy^2+cxz^2$ | 152.64 | 114.84 | 0.717 | 0.0789 | 0.0581 | 0.6930 | 0.2917 | 0.2111 | 0.640 |
| $a+b/xy^2+cx\sqrt{z}$ | 112.37 | 85.73 | 0.846 | 0.0696 | 0.0444 | 0.7610 | 0.2409 | 0.1598 | 0.754 |
| $a+b/xy^2+cx^2/z$ | 282.27 | 212.19 | 0.031 | 0.1356 | 0.1079 | 0.0920 | 0.4544 | 0.3550 | 0.125 |
| $a+b/xy^2+cx^2/z^2$ | 265.26 | 192.07 | 0.144 | 0.1273 | 0.0994 | 0.1994 | 0.4351 | 0.3303 | 0.198 |
| $a+b/xy^2+cx^2/\sqrt{z}$ | 186.18 | 142.11 | 0.578 | 0.1052 | 0.0821 | 0.4534 | 0.3270 | 0.2494 | 0.547 |
| $a+b/xy^2+cx^2z$ | 136.74 | 104.99 | 0.773 | 0.0755 | 0.0550 | 0.7184 | 0.2743 | 0.2039 | 0.681 |
| $a+b/xy^2+cx^2z^2$ | 158.41 | 122.60 | 0.695 | 0.0830 | 0.0631 | 0.6602 | 0.3034 | 0.2254 | 0.610 |
| $a+b/xy^2+cx^2\sqrt{z}$ | 124.04 | 95.71 | 0.813 | 0.0734 | 0.0523 | 0.7340 | 0.2582 | 0.1859 | 0.717 |
| $a+b/xy^2+c\sqrt{x}/z$ | 215.59 | 150.97 | 0.434 | 0.1065 | 0.0767 | 0.4399 | 0.3660 | 0.2607 | 0.432 |
| $a+b/xy^2+c\sqrt{x}/z^2$ | 236.70 | 172.64 | 0.318 | 0.1185 | 0.0925 | 0.3063 | 0.3978 | 0.2943 | 0.329 |
| $a+b/xy^2+c\sqrt{x}/\sqrt{z}$ | 244.94 | 170.77 | 0.270 | 0.1145 | 0.0872 | 0.3523 | 0.4029 | 0.3018 | 0.312 |
| $a+b/xy^2+c\sqrt{x}z$ | 129.44 | 99.83 | 0.796 | 0.0708 | 0.0458 | 0.7526 | 0.2577 | 0.1784 | 0.719 |
| $a+b/xy^2+c\sqrt{x}z^2$ | 151.75 | 116.50 | 0.720 | 0.0775 | 0.0558 | 0.7032 | 0.2878 | 0.2058 | 0.649 |
| $a+b/xy^2+c\sqrt{x}\sqrt{z}$ | 114.38 | 87.31 | 0.841 | 0.0695 | 0.0407 | 0.7614 | 0.2403 | 0.1491 | 0.755 |
| $a+b/xy^2+c/xz$ | 190.93 | 138.76 | 0.556 | 0.1086 | 0.0836 | 0.4175 | 0.3367 | 0.2450 | 0.520 |
| $a+b/xy^2+c/xz^2$ | 223.38 | 161.35 | 0.393 | 0.1198 | 0.0929 | 0.2908 | 0.3818 | 0.2821 | 0.382 |
| $a+b/xy^2+c/x\sqrt{z}$ | 152.33 | 108.19 | 0.718 | 0.0948 | 0.0725 | 0.5566 | 0.2843 | 0.1975 | 0.657 |
| $a+b/xy^2+cz/x$ | 188.30 | 129.28 | 0.569 | 0.1011 | 0.0731 | 0.4958 | 0.3309 | 0.2339 | 0.536 |
| $a+b/xy^2+cz^2/x$ | 148.60 | 107.32 | 0.731 | 0.0791 | 0.0555 | 0.6909 | 0.2786 | 0.1841 | 0.671 |
| $a+b/xy^2+c\sqrt{z}/x$ | 257.40 | 179.53 | 0.194 | 0.1278 | 0.0958 | 0.1930 | 0.4241 | 0.3060 | 0.238 |
| $a+b/xy^2+c/x^2z$ | 261.99 | 183.56 | 0.165 | 0.1315 | 0.1004 | 0.1466 | 0.4313 | 0.3138 | 0.212 |
| $a+b/xy^2+c/x^2z^2$ | 252.78 | 172.91 | 0.223 | 0.1284 | 0.0957 | 0.1854 | 0.4192 | 0.2991 | 0.255 |
| $a+b/xy^2+c/x^2\sqrt{z}$ | 260.19 | 182.60 | 0.176 | 0.1310 | 0.1002 | 0.1527 | 0.4290 | 0.3119 | 0.220 |
| $a+b/xy^2+cz/x^2$ | 255.71 | 180.31 | 0.204 | 0.1296 | 0.0997 | 0.1703 | 0.4229 | 0.3085 | 0.242 |
| $a+b/xy^2+cz^2/x^2$ | 246.40 | 176.08 | 0.261 | 0.1265 | 0.0986 | 0.2095 | 0.4106 | 0.3034 | 0.286 |
| $a+b/xy^2+c\sqrt{z}/x^2$ | 257.68 | 181.19 | 0.192 | 0.1302 | 0.0999 | 0.1623 | 0.4256 | 0.3095 | 0.233 |
| $a+b/xy^2+c/\sqrt{x}z$ | 173.44 | 124.71 | 0.634 | 0.1010 | 0.0772 | 0.4962 | 0.3143 | 0.2179 | 0.581 |
| $a+b/xy^2+c/\sqrt{x}z^2$ | 211.30 | 152.47 | 0.457 | 0.1147 | 0.0892 | 0.3510 | 0.3664 | 0.2665 | 0.431 |
| $a+b/xy^2+c/\sqrt{x}\sqrt{z}$ | 147.66 | 104.59 | 0.735 | 0.0918 | 0.0692 | 0.5836 | 0.2802 | 0.1881 | 0.667 |
| $a+b/xy^2+cz/\sqrt{x}$ | 151.62 | 117.95 | 0.720 | 0.0780 | 0.0515 | 0.6996 | 0.2790 | 0.1889 | 0.670 |
| $a+b/xy^2+cz^2/\sqrt{x}$ | 153.49 | 118.04 | 0.713 | 0.0771 | 0.0552 | 0.7067 | 0.2844 | 0.2058 | 0.657 |
| $a+b/xy^2+c\sqrt{z}/\sqrt{x}$ | 195.70 | 146.04 | 0.534 | 0.0945 | 0.0678 | 0.5587 | 0.3348 | 0.2432 | 0.525 |
| $a+b/xy^2+cy/z$ | 231.94 | 166.02 | 0.345 | 0.1100 | 0.0823 | 0.4024 | 0.3813 | 0.2843 | 0.384 |
| $a+b/xy^2+cy/z^2$ | 238.41 | 172.86 | 0.308 | 0.1180 | 0.0917 | 0.3123 | 0.3980 | 0.2946 | 0.329 |
| $a+b/xy^2+cy/\sqrt{z}$ | 280.41 | 206.66 | 0.043 | 0.1308 | 0.1001 | 0.1557 | 0.4483 | 0.3408 | 0.148 |
| $a+b/xy^2+cyz$ | 136.98 | 107.63 | 0.772 | 0.0761 | 0.0505 | 0.7139 | 0.2758 | 0.1950 | 0.678 |
| $a+b/xy^2+cyz^2$ | 156.54 | 120.71 | 0.702 | 0.0812 | 0.0589 | 0.6747 | 0.2989 | 0.2135 | 0.621 |
| $a+b/xy^2+cy\sqrt{z}$ | 129.70 | 99.18 | 0.795 | 0.0779 | 0.0481 | 0.7002 | 0.2710 | 0.1735 | 0.689 |
| $a+b/xy^2+cy^2/z$ | 277.92 | 203.88 | 0.060 | 0.1294 | 0.0989 | 0.1728 | 0.4445 | 0.3358 | 0.163 |
| $a+b/xy^2+cy^2/z^2$ | 251.32 | 181.57 | 0.232 | 0.1209 | 0.0931 | 0.2781 | 0.4128 | 0.3103 | 0.278 |
| $a+b/xy^2+cy^2/\sqrt{z}$ | 249.35 | 203.08 | 0.244 | 0.1283 | 0.1029 | 0.1867 | 0.4228 | 0.3318 | 0.242 |
| $a+b/xy^2+cy^2z$ | 148.14 | 113.21 | 0.733 | 0.0821 | 0.0568 | 0.6668 | 0.2956 | 0.2076 | 0.630 |
| $a+b/xy^2+cy^2z^2$ | 163.66 | 124.85 | 0.674 | 0.0860 | 0.0636 | 0.6344 | 0.3131 | 0.2260 | 0.585 |
| $a+b/xy^2+cy^2\sqrt{z}$ | 144.55 | 104.69 | 0.746 | 0.0841 | 0.0563 | 0.6505 | 0.2941 | 0.1926 | 0.633 |
| $a+b/xy^2+c\sqrt{y}/z$ | 201.64 | 143.09 | 0.505 | 0.1013 | 0.0717 | 0.4931 | 0.3444 | 0.2404 | 0.497 |
| $a+b/xy^2+c\sqrt{y}/z^2$ | 229.39 | 167.50 | 0.360 | 0.1162 | 0.0898 | 0.3336 | 0.3875 | 0.2843 | 0.364 |
| $a+b/xy^2+c\sqrt{y}/\sqrt{z}$ | 221.05 | 160.28 | 0.405 | 0.1037 | 0.0789 | 0.4686 | 0.3633 | 0.2708 | 0.441 |
| $a+b/xy^2+c\sqrt{y}z$ | 133.95 | 107.39 | 0.782 | 0.0735 | 0.0471 | 0.7334 | 0.2670 | 0.1845 | 0.698 |
| $a+b/xy^2+c\sqrt{y}z^2$ | 153.84 | 119.96 | 0.712 | 0.0788 | 0.0565 | 0.6931 | 0.2919 | 0.2075 | 0.639 |
| $a+b/xy^2+c\sqrt{y}\sqrt{z}$ | 124.54 | 98.11 | 0.811 | 0.0745 | 0.0427 | 0.7260 | 0.2592 | 0.1629 | 0.715 |
| $a+b/xy^2+c/yz$ | 196.14 | 140.69 | 0.532 | 0.1104 | 0.0852 | 0.3987 | 0.3461 | 0.2513 | 0.493 |
| $a+b/xy^2+c/yz^2$ | 218.66 | 158.78 | 0.418 | 0.1180 | 0.0921 | 0.3127 | 0.3767 | 0.2783 | 0.399 |
| $a+b/xy^2+c/y\sqrt{z}$ | 186.59 | 129.12 | 0.576 | 0.1073 | 0.0813 | 0.4320 | 0.3343 | 0.2355 | 0.526 |
| $a+b/xy^2+cz/y$ | 196.26 | 152.41 | 0.531 | 0.0902 | 0.0729 | 0.5979 | 0.3228 | 0.2476 | 0.558 |
| $a+b/xy^2+cz^2/y$ | 160.21 | 121.31 | 0.688 | 0.0773 | 0.0578 | 0.7052 | 0.2844 | 0.2054 | 0.657 |
| $a+b/xy^2+c\sqrt{z}/y$ | 283.49 | 209.65 | 0.022 | 0.1334 | 0.1032 | 0.1216 | 0.4546 | 0.3490 | 0.124 |
| $a+b/xy^2+c/y^2z$ | 236.46 | 171.58 | 0.320 | 0.1240 | 0.0970 | 0.2405 | 0.3979 | 0.2933 | 0.329 |

(continued on next page)

**Table 4 – continued from previous page**

| Functional form | $T_{eff}$ (K) | | | Radius ($R_\odot$) | | | log ($L/L_\odot$) | | |
|---|---|---|---|---|---|---|---|---|---|
| | RMSE | MAD | $R^2_{ap}$ | RMSE | MAD | $R^2_{ap}$ | RMSE | MAD | $R^2_{ap}$ |
| $a+b/xy^2+c/y^2z^2$ | 242.30 | 174.34 | 0.286 | 0.1260 | 0.0976 | 0.2167 | 0.4063 | 0.2963 | 0.301 |
| $a+b/xy^2+c/y^2\sqrt{z}$ | 233.28 | 169.49 | 0.338 | 0.1230 | 0.0966 | 0.2529 | 0.3938 | 0.2914 | 0.343 |
| $a+b/xy^2+cz/y^2$ | 283.62 | 209.78 | 0.021 | 0.1336 | 0.1036 | 0.1183 | 0.4549 | 0.3493 | 0.123 |
| $a+b/xy^2+cz^2/y^2$ | 188.44 | 147.04 | 0.568 | 0.0879 | 0.0706 | 0.6181 | 0.3117 | 0.2403 | 0.588 |
| $a+b/xy^2+c\sqrt{z}/y^2$ | 249.24 | 183.66 | 0.244 | 0.1284 | 0.0995 | 0.1854 | 0.4174 | 0.3140 | 0.262 |
| $a+b/xy^2+c/\sqrt{y}z$ | 176.39 | 123.23 | 0.621 | 0.1015 | 0.0768 | 0.4910 | 0.3199 | 0.2184 | 0.566 |
| $a+b/xy^2+c/\sqrt{y}z^2$ | 213.69 | 150.57 | 0.444 | 0.1148 | 0.0883 | 0.3488 | 0.3700 | 0.2636 | 0.420 |
| $a+b/xy^2+c/\sqrt{y}\sqrt{z}$ | 156.59 | 109.21 | 0.702 | 0.0949 | 0.0709 | 0.5557 | 0.2959 | 0.1938 | 0.629 |
| $a+b/xy^2+cz/\sqrt{y}$ | 155.31 | 122.92 | 0.707 | 0.0764 | 0.0560 | 0.7116 | 0.2768 | 0.1968 | 0.675 |
| $a+b/xy^2+cz^2/\sqrt{y}$ | 154.26 | 116.13 | 0.710 | 0.0762 | 0.0546 | 0.7135 | 0.2827 | 0.2030 | 0.661 |
| $a+b/xy^2+c\sqrt{z}/\sqrt{y}$ | 202.64 | 153.59 | 0.500 | 0.0934 | 0.0740 | 0.5695 | 0.3330 | 0.2510 | 0.530 |
| $a+b/x\sqrt{y}+cx/z$ | 248.41 | 176.29 | 0.249 | 0.1173 | 0.0899 | 0.3202 | 0.4073 | 0.3054 | 0.297 |
| $a+b/x\sqrt{y}+cx/z^2$ | 245.91 | 179.20 | 0.264 | 0.1203 | 0.0947 | 0.2853 | 0.4072 | 0.3049 | 0.297 |
| $a+b/x\sqrt{y}+cx/\sqrt{z}$ | 277.08 | 210.10 | 0.066 | 0.1335 | 0.1068 | 0.1203 | 0.4451 | 0.3501 | 0.160 |
| $a+b/x\sqrt{y}+cxz$ | 128.36 | 96.14 | 0.800 | 0.0712 | 0.0486 | 0.7499 | 0.2587 | 0.1851 | 0.716 |
| $a+b/x\sqrt{y}+cxz^2$ | 151.82 | 114.31 | 0.720 | 0.0784 | 0.0577 | 0.6966 | 0.2893 | 0.2093 | 0.645 |
| $a+b/x\sqrt{y}+cx\sqrt{z}$ | 112.59 | 86.00 | 0.846 | 0.0696 | 0.0444 | 0.7610 | 0.2408 | 0.1596 | 0.754 |
| $a+b/x\sqrt{y}+cx^2/z$ | 279.14 | 209.83 | 0.052 | 0.1335 | 0.1063 | 0.1203 | 0.4475 | 0.3489 | 0.152 |
| $a+b/x\sqrt{y}+cx^2/z^2$ | 260.96 | 189.73 | 0.171 | 0.1251 | 0.0981 | 0.2269 | 0.4268 | 0.3237 | 0.228 |
| $a+b/x\sqrt{y}+cx^2/\sqrt{z}$ | 187.17 | 143.72 | 0.574 | 0.1053 | 0.0824 | 0.4528 | 0.3273 | 0.2507 | 0.546 |
| $a+b/x\sqrt{y}+cx^2z$ | 136.41 | 104.79 | 0.774 | 0.0753 | 0.0549 | 0.7201 | 0.2729 | 0.2023 | 0.685 |
| $a+b/x\sqrt{y}+cx^2z^2$ | 157.37 | 121.78 | 0.699 | 0.0824 | 0.0626 | 0.6649 | 0.3006 | 0.2234 | 0.617 |
| $a+b/x\sqrt{y}+cx^2\sqrt{z}$ | 124.05 | 95.81 | 0.813 | 0.0733 | 0.0523 | 0.7344 | 0.2576 | 0.1852 | 0.719 |
| $a+b/x\sqrt{y}+c\sqrt{x}/z$ | 211.88 | 148.70 | 0.454 | 0.1048 | 0.0755 | 0.4575 | 0.3592 | 0.2544 | 0.453 |
| $a+b/x\sqrt{y}+c\sqrt{x}/z^2$ | 233.53 | 171.08 | 0.336 | 0.1169 | 0.0914 | 0.3252 | 0.3914 | 0.2898 | 0.351 |
| $a+b/x\sqrt{y}+c\sqrt{x}/\sqrt{z}$ | 237.99 | 166.02 | 0.311 | 0.1113 | 0.0840 | 0.3883 | 0.3912 | 0.2911 | 0.352 |
| $a+b/x\sqrt{y}+c\sqrt{x}z$ | 129.43 | 99.89 | 0.796 | 0.0707 | 0.0457 | 0.7533 | 0.2569 | 0.1773 | 0.720 |
| $a+b/x\sqrt{y}+c\sqrt{x}z^2$ | 151.00 | 115.97 | 0.723 | 0.0771 | 0.0555 | 0.7065 | 0.2855 | 0.2039 | 0.655 |
| $a+b/x\sqrt{y}+c\sqrt{x}\sqrt{z}$ | 114.71 | 87.80 | 0.840 | 0.0695 | 0.0407 | 0.7614 | 0.2403 | 0.1490 | 0.755 |
| $a+b/x\sqrt{y}+c/xz$ | 207.10 | 148.14 | 0.478 | 0.1132 | 0.0869 | 0.3668 | 0.3560 | 0.2588 | 0.463 |
| $a+b/x\sqrt{y}+c/xz^2$ | 228.55 | 161.99 | 0.364 | 0.1207 | 0.0923 | 0.2803 | 0.3862 | 0.2809 | 0.368 |
| $a+b/x\sqrt{y}+c/x\sqrt{z}$ | 179.04 | 128.79 | 0.610 | 0.1030 | 0.0784 | 0.4759 | 0.3172 | 0.2220 | 0.574 |
| $a+b/x\sqrt{y}+cz/x$ | 164.40 | 114.21 | 0.671 | 0.0929 | 0.0648 | 0.5736 | 0.2987 | 0.2023 | 0.622 |
| $a+b/x\sqrt{y}+cz^2/x$ | 142.00 | 102.65 | 0.755 | 0.0770 | 0.0534 | 0.7075 | 0.2693 | 0.1782 | 0.693 |
| $a+b/x\sqrt{y}+c\sqrt{z}/x$ | 206.61 | 140.16 | 0.481 | 0.1105 | 0.0819 | 0.3972 | 0.3549 | 0.2521 | 0.466 |
| $a+b/x\sqrt{y}+c/x^2z$ | 216.16 | 159.94 | 0.431 | 0.1172 | 0.0921 | 0.3213 | 0.3693 | 0.2766 | 0.422 |
| $a+b/x\sqrt{y}+c/x^2z^2$ | 253.03 | 181.67 | 0.221 | 0.1198 | 0.0962 | 0.2910 | 0.4071 | 0.3069 | 0.298 |
| $a+b/x\sqrt{y}+c/x^2\sqrt{z}$ | 227.18 | 166.34 | 0.372 | 0.1206 | 0.0946 | 0.2817 | 0.3835 | 0.2858 | 0.377 |
| $a+b/x\sqrt{y}+cz/x^2$ | 233.34 | 169.03 | 0.338 | 0.1223 | 0.0955 | 0.2618 | 0.3912 | 0.2884 | 0.352 |
| $a+b/x\sqrt{y}+cz^2/x^2$ | 225.57 | 163.04 | 0.381 | 0.1195 | 0.0936 | 0.2954 | 0.3808 | 0.2797 | 0.385 |
| $a+b/x\sqrt{y}+c\sqrt{z}/x^2$ | 233.52 | 169.35 | 0.337 | 0.1224 | 0.0957 | 0.2600 | 0.3915 | 0.2893 | 0.350 |
| $a+b/x\sqrt{y}+c/\sqrt{x}z$ | 176.78 | 126.88 | 0.620 | 0.1017 | 0.0775 | 0.4890 | 0.3172 | 0.2202 | 0.574 |
| $a+b/x\sqrt{y}+c/\sqrt{x}z^2$ | 211.83 | 152.89 | 0.454 | 0.1143 | 0.0883 | 0.3554 | 0.3651 | 0.2651 | 0.435 |
| $a+b/x\sqrt{y}+c/\sqrt{x}\sqrt{z}$ | 152.70 | 108.73 | 0.716 | 0.0932 | 0.0701 | 0.5713 | 0.2856 | 0.1916 | 0.654 |
| $a+b/x\sqrt{y}+cz/\sqrt{x}$ | 147.03 | 115.18 | 0.737 | 0.0765 | 0.0500 | 0.7108 | 0.2722 | 0.1837 | 0.686 |
| $a+b/x\sqrt{y}+cz^2/\sqrt{x}$ | 151.66 | 116.83 | 0.720 | 0.0763 | 0.0545 | 0.7124 | 0.2808 | 0.2031 | 0.666 |
| $a+b/x\sqrt{y}+c\sqrt{z}/\sqrt{x}$ | 179.00 | 135.24 | 0.610 | 0.0884 | 0.0611 | 0.6143 | 0.3112 | 0.2188 | 0.590 |
| $a+b/x\sqrt{y}+cy/z$ | 227.60 | 163.75 | 0.370 | 0.1080 | 0.0804 | 0.4244 | 0.3734 | 0.2771 | 0.409 |
| $a+b/x\sqrt{y}+cy/z^2$ | 235.12 | 171.25 | 0.327 | 0.1163 | 0.0906 | 0.3317 | 0.3915 | 0.2894 | 0.351 |
| $a+b/x\sqrt{y}+cy/\sqrt{z}$ | 275.05 | 202.28 | 0.080 | 0.1276 | 0.0970 | 0.1965 | 0.4374 | 0.3311 | 0.189 |
| $a+b/x\sqrt{y}+cyz$ | 136.81 | 107.53 | 0.772 | 0.0759 | 0.0502 | 0.7152 | 0.2746 | 0.1935 | 0.680 |
| $a+b/x\sqrt{y}+cyz^2$ | 155.65 | 120.06 | 0.705 | 0.0807 | 0.0584 | 0.6787 | 0.2964 | 0.2113 | 0.628 |
| $a+b/x\sqrt{y}+cy\sqrt{z}$ | 129.91 | 99.49 | 0.795 | 0.0779 | 0.0481 | 0.7005 | 0.2706 | 0.1727 | 0.690 |
| $a+b/x\sqrt{y}+cy^2/z$ | 272.80 | 199.80 | 0.095 | 0.1265 | 0.0968 | 0.2095 | 0.4342 | 0.3273 | 0.201 |
| $a+b/x\sqrt{y}+cy^2/z^2$ | 247.27 | 179.10 | 0.256 | 0.1189 | 0.0918 | 0.3022 | 0.4049 | 0.3037 | 0.305 |
| $a+b/x\sqrt{y}+cy^2/\sqrt{z}$ | 249.38 | 202.90 | 0.243 | 0.1275 | 0.1026 | 0.1970 | 0.4201 | 0.3313 | 0.252 |
| $a+b/x\sqrt{y}+cy^2z$ | 147.74 | 112.89 | 0.734 | 0.0818 | 0.0565 | 0.6692 | 0.2939 | 0.2056 | 0.634 |
| $a+b/x\sqrt{y}+cy^2z^2$ | 162.56 | 124.10 | 0.678 | 0.0854 | 0.0631 | 0.6397 | 0.3101 | 0.2239 | 0.592 |
| $a+b/x\sqrt{y}+cy^2\sqrt{z}$ | 144.53 | 104.85 | 0.746 | 0.0840 | 0.0562 | 0.6518 | 0.2931 | 0.1914 | 0.636 |
| $a+b/x\sqrt{y}+c\sqrt{y}/z$ | 199.07 | 141.61 | 0.518 | 0.1001 | 0.0712 | 0.5051 | 0.3394 | 0.2359 | 0.512 |
| $a+b/x\sqrt{y}+c\sqrt{y}/z^2$ | 226.70 | 166.53 | 0.375 | 0.1147 | 0.0889 | 0.3499 | 0.3819 | 0.2808 | 0.382 |
| $a+b/x\sqrt{y}+c\sqrt{y}/\sqrt{z}$ | 216.46 | 157.67 | 0.430 | 0.1017 | 0.0772 | 0.4897 | 0.3552 | 0.2635 | 0.465 |
| $a+b/x\sqrt{y}+c\sqrt{y}z$ | 133.78 | 107.27 | 0.782 | 0.0733 | 0.0469 | 0.7345 | 0.2659 | 0.1832 | 0.700 |
| $a+b/x\sqrt{y}+c\sqrt{y}z^2$ | 153.00 | 119.34 | 0.715 | 0.0784 | 0.0561 | 0.6967 | 0.2895 | 0.2054 | 0.645 |
| $a+b/x\sqrt{y}+c\sqrt{y}\sqrt{z}$ | 124.73 | 98.41 | 0.811 | 0.0745 | 0.0428 | 0.7263 | 0.2588 | 0.1624 | 0.716 |
| $a+b/x\sqrt{y}+c/yz$ | 197.72 | 140.96 | 0.524 | 0.1104 | 0.0847 | 0.3987 | 0.3463 | 0.2501 | 0.492 |
| $a+b/x\sqrt{y}+c/yz^2$ | 218.31 | 157.12 | 0.420 | 0.1172 | 0.0908 | 0.3213 | 0.3741 | 0.2739 | 0.407 |
| $a+b/x\sqrt{y}+c/y\sqrt{z}$ | 189.59 | 130.49 | 0.563 | 0.1078 | 0.0812 | 0.4267 | 0.3366 | 0.2365 | 0.520 |
| $a+b/x\sqrt{y}+cz/y$ | 190.31 | 148.63 | 0.559 | 0.0878 | 0.0707 | 0.6192 | 0.3132 | 0.2404 | 0.584 |
| $a+b/x\sqrt{y}+cz^2/y$ | 158.36 | 120.18 | 0.695 | 0.0765 | 0.0571 | 0.7112 | 0.2808 | 0.2028 | 0.666 |
| $a+b/x\sqrt{y}+c\sqrt{z}/y$ | 277.64 | 204.43 | 0.062 | 0.1291 | 0.0988 | 0.1768 | 0.4416 | 0.3360 | 0.174 |
| $a+b/x\sqrt{y}+c/y^2z$ | 238.57 | 171.14 | 0.308 | 0.1239 | 0.0959 | 0.2426 | 0.3982 | 0.2904 | 0.328 |
| $a+b/x\sqrt{y}+c/y^2z^2$ | 242.23 | 173.44 | 0.286 | 0.1251 | 0.0965 | 0.2274 | 0.4036 | 0.2930 | 0.310 |
| $a+b/x\sqrt{y}+c/y^2\sqrt{z}$ | 237.27 | 170.23 | 0.315 | 0.1234 | 0.0959 | 0.2478 | 0.3966 | 0.2901 | 0.334 |
| $a+b/x\sqrt{y}+cz/y^2$ | 275.32 | 200.12 | 0.078 | 0.1274 | 0.0968 | 0.1985 | 0.4368 | 0.3282 | 0.192 |
| $a+b/x\sqrt{y}+cz^2/y^2$ | 180.91 | 142.29 | 0.602 | 0.0850 | 0.0680 | 0.6433 | 0.3000 | 0.2327 | 0.619 |
| $a+b/x\sqrt{y}+c\sqrt{z}/y^2$ | 258.56 | 188.77 | 0.187 | 0.1300 | 0.1009 | 0.1659 | 0.4262 | 0.3207 | 0.230 |
| $a+b/x\sqrt{y}+c/\sqrt{y}z$ | 176.81 | 123.17 | 0.620 | 0.1013 | 0.0764 | 0.4932 | 0.3191 | 0.2170 | 0.569 |
| $a+b/x\sqrt{y}+c/\sqrt{y}z^2$ | 212.64 | 151.03 | 0.450 | 0.1140 | 0.0874 | 0.3588 | 0.3666 | 0.2626 | 0.431 |
| $a+b/x\sqrt{y}+c/\sqrt{y}\sqrt{z}$ | 157.82 | 109.73 | 0.697 | 0.0950 | 0.0709 | 0.5544 | 0.2964 | 0.1937 | 0.628 |
| $a+b/x\sqrt{y}+cz/\sqrt{y}$ | 153.55 | 121.90 | 0.713 | 0.0758 | 0.0553 | 0.7166 | 0.2735 | 0.1942 | 0.683 |
| $a+b/x\sqrt{y}+cz^2/\sqrt{y}$ | 153.14 | 115.50 | 0.715 | 0.0756 | 0.0541 | 0.7175 | 0.2800 | 0.2008 | 0.668 |
| $a+b/x\sqrt{y}+c\sqrt{z}/\sqrt{y}$ | 197.27 | 150.28 | 0.527 | 0.0911 | 0.0720 | 0.5900 | 0.3240 | 0.2444 | 0.555 |
| $a+by/x+cx/z$ | 253.97 | 176.29 | 0.215 | 0.1186 | 0.0897 | 0.3058 | 0.4130 | 0.3086 | 0.277 |
| $a+by/x+cx/z^2$ | 248.62 | 178.43 | 0.248 | 0.1203 | 0.0937 | 0.2855 | 0.4090 | 0.3033 | 0.291 |
| $a+by/x+cx/\sqrt{z}$ | 277.49 | 209.80 | 0.063 | 0.1332 | 0.1065 | 0.1235 | 0.4444 | 0.3482 | 0.163 |
| $a+by/x+cxz$ | 128.44 | 95.97 | 0.799 | 0.0708 | 0.0489 | 0.7523 | 0.2584 | 0.1847 | 0.717 |
| $a+by/x+cxz^2$ | 152.68 | 113.37 | 0.716 | 0.0780 | 0.0582 | 0.7000 | 0.2891 | 0.2114 | 0.646 |
| $a+by/x+cx\sqrt{z}$ | 112.20 | 85.47 | 0.847 | 0.0695 | 0.0446 | 0.7615 | 0.2404 | 0.1595 | 0.755 |
| $a+by/x+cx^2/z$ | 280.44 | 209.32 | 0.043 | 0.1334 | 0.1059 | 0.1217 | 0.4478 | 0.3470 | 0.150 |
| $a+by/x+cx^2/z^2$ | 263.86 | 188.70 | 0.153 | 0.1253 | 0.0970 | 0.2250 | 0.4289 | 0.3218 | 0.220 |
| $a+by/x+cx^2/\sqrt{z}$ | 187.62 | 145.85 | 0.572 | 0.1053 | 0.0831 | 0.4525 | 0.3276 | 0.2526 | 0.545 |
| $a+by/x+cx^2z$ | 136.94 | 104.28 | 0.772 | 0.0749 | 0.0553 | 0.7227 | 0.2728 | 0.2036 | 0.685 |

(continued on next page)

**Table 4 – continued from previous page**

| Functional form | $T_{eff}$ (K) | | | Radius ($R_\odot$) | | | log (L/$L_\odot$) | | |
|---|---|---|---|---|---|---|---|---|---|
| | RMSE | MAD | $R^2_{ap}$ | RMSE | MAD | $R^2_{ap}$ | RMSE | MAD | $R^2_{ap}$ |
| $a+by/x+cx^2z^2$ | 158.39 | 121.12 | 0.695 | 0.0819 | 0.0634 | 0.6685 | 0.3005 | 0.2266 | 0.617 |
| $a+by/x+cx^2\sqrt{z}$ | 123.99 | 95.67 | 0.813 | 0.0730 | 0.0524 | 0.7365 | 0.2573 | 0.1861 | 0.719 |
| $a+by/x+c\sqrt{x}/z$ | 216.25 | 151.84 | 0.431 | 0.1052 | 0.0767 | 0.4538 | 0.3627 | 0.2579 | 0.443 |
| $a+by/x+c\sqrt{x}/z^2$ | 235.16 | 170.49 | 0.327 | 0.1164 | 0.0904 | 0.3313 | 0.3913 | 0.2883 | 0.351 |
| $a+by/x+c\sqrt{x}/\sqrt{z}$ | 247.00 | 168.78 | 0.258 | 0.1139 | 0.0858 | 0.3595 | 0.4012 | 0.2967 | 0.318 |
| $a+by/x+c\sqrt{x}z$ | 129.43 | 99.82 | 0.796 | 0.0703 | 0.0462 | 0.7557 | 0.2564 | 0.1763 | 0.721 |
| $a+by/x+c\sqrt{x}z^2$ | 151.80 | 115.00 | 0.720 | 0.0767 | 0.0557 | 0.7098 | 0.2854 | 0.2047 | 0.655 |
| $a+by/x+c\sqrt{x}\sqrt{z}$ | 114.54 | 87.50 | 0.840 | 0.0696 | 0.0415 | 0.7608 | 0.2402 | 0.1488 | 0.756 |
| $a+by/x+c/xz$ | 237.82 | 167.18 | 0.312 | 0.1219 | 0.0941 | 0.2660 | 0.3953 | 0.2840 | 0.338 |
| $a+by/x+c/xz^2$ | 235.68 | 167.56 | 0.324 | 0.1216 | 0.0932 | 0.2702 | 0.3918 | 0.2844 | 0.350 |
| $a+by/x+c/x\sqrt{z}$ | 248.82 | 175.61 | 0.247 | 0.1251 | 0.0958 | 0.2276 | 0.4108 | 0.2995 | 0.285 |
| $a+by/x+cz/x$ | 190.00 | 144.40 | 0.561 | 0.0922 | 0.0710 | 0.5799 | 0.3096 | 0.2336 | 0.594 |
| $a+by/x+cz^2/x$ | 145.78 | 107.93 | 0.741 | 0.0733 | 0.0531 | 0.7347 | 0.2636 | 0.1926 | 0.706 |
| $a+by/x+c\sqrt{z}/x$ | 263.36 | 187.45 | 0.156 | 0.1230 | 0.0940 | 0.2532 | 0.4156 | 0.3091 | 0.268 |
| $a+by/x+c/x^2z$ | 265.18 | 187.53 | 0.144 | 0.1255 | 0.0967 | 0.2223 | 0.4192 | 0.3154 | 0.255 |
| $a+by/x+c/x^2z^2$ | 281.71 | 208.56 | 0.034 | 0.1332 | 0.1050 | 0.1245 | 0.4498 | 0.3433 | 0.143 |
| $a+by/x+c/x^2\sqrt{z}$ | 251.37 | 183.41 | 0.231 | 0.1212 | 0.0927 | 0.2747 | 0.3981 | 0.3009 | 0.329 |
| $a+by/x+cz/x^2$ | 230.50 | 164.24 | 0.354 | 0.1158 | 0.0851 | 0.3381 | 0.3694 | 0.2679 | 0.422 |
| $a+by/x+cz^2/x^2$ | 216.10 | 152.92 | 0.432 | 0.1107 | 0.0835 | 0.3948 | 0.3496 | 0.2554 | 0.482 |
| $a+by/x+c\sqrt{z}/x^2$ | 235.50 | 170.03 | 0.325 | 0.1171 | 0.0869 | 0.3226 | 0.3760 | 0.2767 | 0.401 |
| $a+by/x+c/\sqrt{x}z$ | 186.30 | 133.84 | 0.578 | 0.1040 | 0.0789 | 0.4659 | 0.3265 | 0.2310 | 0.548 |
| $a+by/x+c/\sqrt{x}z^2$ | 212.22 | 154.65 | 0.452 | 0.1131 | 0.0876 | 0.3683 | 0.3613 | 0.2637 | 0.447 |
| $a+by/x+c/\sqrt{x}\sqrt{z}$ | 177.68 | 122.94 | 0.616 | 0.1011 | 0.0757 | 0.4957 | 0.3163 | 0.2167 | 0.576 |
| $a+by/x+cz/\sqrt{x}$ | 154.21 | 116.47 | 0.711 | 0.0757 | 0.0553 | 0.7169 | 0.2743 | 0.1950 | 0.681 |
| $a+by/x+cz^2/\sqrt{x}$ | 153.48 | 114.56 | 0.713 | 0.0755 | 0.0553 | 0.7186 | 0.2804 | 0.2030 | 0.667 |
| $a+by/x+c\sqrt{z}/\sqrt{x}$ | 213.24 | 153.90 | 0.447 | 0.0974 | 0.0748 | 0.5312 | 0.3465 | 0.2525 | 0.491 |
| $a+by/x+cy/z$ | 236.59 | 167.60 | 0.319 | 0.1113 | 0.0840 | 0.3880 | 0.3863 | 0.2865 | 0.368 |
| $a+by/x+cy/z^2$ | 238.42 | 170.47 | 0.308 | 0.1167 | 0.0896 | 0.3275 | 0.3946 | 0.2892 | 0.340 |
| $a+by/x+cy/\sqrt{z}$ | 280.16 | 204.61 | 0.045 | 0.1305 | 0.0986 | 0.1590 | 0.4459 | 0.3365 | 0.157 |
| $a+by/x+cyz$ | 136.66 | 107.19 | 0.773 | 0.0749 | 0.0505 | 0.7229 | 0.2719 | 0.1923 | 0.687 |
| $a+by/x+cyz^2$ | 156.04 | 119.06 | 0.704 | 0.0798 | 0.0588 | 0.6856 | 0.2949 | 0.2131 | 0.632 |
| $a+by/x+cy\sqrt{z}$ | 130.72 | 100.30 | 0.792 | 0.0771 | 0.0482 | 0.7068 | 0.2675 | 0.1713 | 0.697 |
| $a+by/x+cy^2/z$ | 278.25 | 202.12 | 0.058 | 0.1293 | 0.0970 | 0.1742 | 0.4430 | 0.3334 | 0.169 |
| $a+by/x+cy^2/z^2$ | 252.68 | 178.08 | 0.223 | 0.1204 | 0.0910 | 0.2839 | 0.4119 | 0.3065 | 0.281 |
| $a+by/x+cy^2/\sqrt{z}$ | 248.67 | 202.88 | 0.248 | 0.1258 | 0.1027 | 0.2182 | 0.4143 | 0.3304 | 0.273 |
| $a+by/x+cy^2z$ | 147.34 | 112.39 | 0.736 | 0.0805 | 0.0565 | 0.6797 | 0.2904 | 0.2042 | 0.643 |
| $a+by/x+cy^2z^2$ | 162.76 | 123.08 | 0.678 | 0.0844 | 0.0635 | 0.6485 | 0.3080 | 0.2252 | 0.598 |
| $a+by/x+cy^2\sqrt{z}$ | 144.29 | 105.16 | 0.747 | 0.0826 | 0.0566 | 0.6631 | 0.2886 | 0.1896 | 0.647 |
| $a+by/x+c\sqrt{y}/z$ | 203.71 | 145.60 | 0.495 | 0.1010 | 0.0740 | 0.4960 | 0.3447 | 0.2433 | 0.497 |
| $a+by/x+c\sqrt{y}/z^2$ | 228.18 | 165.98 | 0.367 | 0.1143 | 0.0880 | 0.3554 | 0.3818 | 0.2790 | 0.382 |
| $a+by/x+c\sqrt{y}/\sqrt{z}$ | 227.89 | 162.37 | 0.368 | 0.1062 | 0.0818 | 0.4429 | 0.3719 | 0.2761 | 0.414 |
| $a+by/x+c\sqrt{y}z$ | 133.76 | 106.90 | 0.782 | 0.0725 | 0.0472 | 0.7407 | 0.2638 | 0.1820 | 0.705 |
| $a+by/x+c\sqrt{y}z^2$ | 153.57 | 118.35 | 0.713 | 0.0777 | 0.0563 | 0.7021 | 0.2885 | 0.2062 | 0.647 |
| $a+by/x+c\sqrt{y}\sqrt{z}$ | 125.34 | 99.08 | 0.809 | 0.0738 | 0.0434 | 0.7314 | 0.2562 | 0.1615 | 0.722 |
| $a+by/x+c/yz$ | 201.36 | 142.42 | 0.507 | 0.1097 | 0.0837 | 0.4054 | 0.3449 | 0.2488 | 0.496 |
| $a+by/x+c/yz^2$ | 216.97 | 157.99 | 0.427 | 0.1152 | 0.0893 | 0.3448 | 0.3667 | 0.2705 | 0.430 |
| $a+by/x+c/y\sqrt{z}$ | 199.32 | 138.02 | 0.517 | 0.1090 | 0.0819 | 0.4139 | 0.3427 | 0.2409 | 0.502 |
| $a+by/x+cz/y$ | 208.87 | 152.17 | 0.469 | 0.0953 | 0.0758 | 0.5518 | 0.3394 | 0.2575 | 0.512 |
| $a+by/x+cz^2/y$ | 162.20 | 120.96 | 0.680 | 0.0771 | 0.0595 | 0.7063 | 0.2849 | 0.2113 | 0.656 |
| $a+by/x+c\sqrt{z}/y$ | 281.76 | 207.26 | 0.034 | 0.1323 | 0.1019 | 0.1356 | 0.4493 | 0.3419 | 0.145 |
| $a+by/x+c/y^2z$ | 240.84 | 174.57 | 0.294 | 0.1230 | 0.0960 | 0.2533 | 0.3963 | 0.2923 | 0.334 |
| $a+by/x+c/y^2z^2$ | 241.37 | 174.97 | 0.291 | 0.1233 | 0.0957 | 0.2493 | 0.3973 | 0.2911 | 0.331 |
| $a+by/x+c/y^2\sqrt{z}$ | 242.44 | 174.84 | 0.285 | 0.1234 | 0.0965 | 0.2480 | 0.3988 | 0.2944 | 0.326 |
| $a+by/x+cz/y^2$ | 281.75 | 207.10 | 0.034 | 0.1324 | 0.1023 | 0.1346 | 0.4491 | 0.3412 | 0.145 |
| $a+by/x+cz^2/y^2$ | 202.31 | 151.40 | 0.502 | 0.0926 | 0.0746 | 0.5766 | 0.3281 | 0.2539 | 0.544 |
| $a+by/x+c\sqrt{z}/y^2$ | 265.12 | 197.89 | 0.145 | 0.1302 | 0.1034 | 0.1625 | 0.4307 | 0.3308 | 0.214 |
| $a+by/x+c/\sqrt{y}z$ | 177.57 | 125.17 | 0.616 | 0.1001 | 0.0752 | 0.5057 | 0.3147 | 0.2150 | 0.580 |
| $a+by/x+c/\sqrt{y}z^2$ | 210.86 | 151.68 | 0.459 | 0.1119 | 0.0857 | 0.3814 | 0.3596 | 0.2581 | 0.452 |
| $a+by/x+c/\sqrt{y}\sqrt{z}$ | 163.62 | 113.60 | 0.674 | 0.0953 | 0.0707 | 0.5517 | 0.2976 | 0.1959 | 0.625 |
| $a+by/x+cz/\sqrt{y}$ | 158.48 | 122.33 | 0.694 | 0.0768 | 0.0581 | 0.7085 | 0.2792 | 0.2050 | 0.670 |
| $a+by/x+cz^2/\sqrt{y}$ | 154.85 | 115.20 | 0.708 | 0.0755 | 0.0552 | 0.7185 | 0.2812 | 0.2008 | 0.665 |
| $a+by/x+c\sqrt{z}/\sqrt{y}$ | 213.73 | 154.24 | 0.444 | 0.0979 | 0.0773 | 0.5268 | 0.3479 | 0.2605 | 0.487 |
| $a+by^2/x+cx/z$ | 256.57 | 198.19 | 0.199 | 0.1380 | 0.1041 | 0.0595 | 0.4718 | 0.3536 | 0.057 |
| $a+by^2/x+cx/z^2$ | 247.82 | 193.52 | 0.253 | 0.1348 | 0.1041 | 0.1026 | 0.4608 | 0.3490 | 0.100 |
| $a+by^2/x+cx/\sqrt{z}$ | 241.86 | 193.60 | 0.288 | 0.1306 | 0.1058 | 0.1581 | 0.4261 | 0.3356 | 0.231 |
| $a+by^2/x+cxz$ | 127.34 | 97.58 | 0.803 | 0.0720 | 0.0528 | 0.7437 | 0.2688 | 0.2016 | 0.694 |
| $a+by^2/x+cxz^2$ | 154.16 | 118.72 | 0.711 | 0.0850 | 0.0665 | 0.6436 | 0.3191 | 0.2497 | 0.569 |
| $a+by^2/x+cx\sqrt{z}$ | 116.12 | 90.00 | 0.836 | 0.0681 | 0.0459 | 0.7708 | 0.2384 | 0.1631 | 0.759 |
| $a+by^2/x+cx^2/z$ | 250.44 | 205.89 | 0.237 | 0.1354 | 0.1110 | 0.0946 | 0.4473 | 0.3593 | 0.152 |
| $a+by^2/x+cx^2/z^2$ | 255.35 | 198.66 | 0.207 | 0.1375 | 0.1054 | 0.0659 | 0.4701 | 0.3558 | 0.064 |
| $a+by^2/x+cx^2/\sqrt{z}$ | 183.33 | 148.69 | 0.591 | 0.1046 | 0.0827 | 0.4594 | 0.3259 | 0.2492 | 0.550 |
| $a+by^2/x+cx^2z$ | 137.21 | 105.36 | 0.771 | 0.0786 | 0.0612 | 0.6951 | 0.2921 | 0.2311 | 0.638 |
| $a+by^2/x+cx^2z^2$ | 161.44 | 127.50 | 0.683 | 0.0904 | 0.0725 | 0.5967 | 0.3350 | 0.2647 | 0.525 |
| $a+by^2/x+cx^2\sqrt{z}$ | 123.64 | 96.52 | 0.814 | 0.0733 | 0.0545 | 0.7344 | 0.2640 | 0.1970 | 0.705 |
| $a+by^2/x+c\sqrt{x}/z$ | 236.92 | 183.87 | 0.317 | 0.1299 | 0.0962 | 0.1670 | 0.4478 | 0.3294 | 0.150 |
| $a+by^2/x+c\sqrt{x}/z^2$ | 238.77 | 184.51 | 0.306 | 0.1315 | 0.1015 | 0.1463 | 0.4474 | 0.3346 | 0.152 |
| $a+by^2/x+c\sqrt{x}/\sqrt{z}$ | 258.77 | 202.28 | 0.185 | 0.1390 | 0.1063 | 0.0456 | 0.4722 | 0.3611 | 0.055 |
| $a+by^2/x+c\sqrt{x}z$ | 127.85 | 101.12 | 0.801 | 0.0714 | 0.0501 | 0.7485 | 0.2657 | 0.1918 | 0.701 |
| $a+by^2/x+c\sqrt{x}z^2$ | 152.59 | 119.30 | 0.717 | 0.0833 | 0.0637 | 0.6575 | 0.3140 | 0.2431 | 0.582 |
| $a+by^2/x+c\sqrt{x}\sqrt{z}$ | 120.11 | 90.50 | 0.824 | 0.0687 | 0.0448 | 0.7670 | 0.2384 | 0.1519 | 0.759 |
| $a+by^2/x+c/xz$ | 222.06 | 165.98 | 0.400 | 0.1168 | 0.0872 | 0.3266 | 0.3819 | 0.2707 | 0.382 |
| $a+by^2/x+c/xz^2$ | 217.44 | 157.04 | 0.425 | 0.1174 | 0.0884 | 0.3197 | 0.3782 | 0.2725 | 0.394 |
| $a+by^2/x+c/x\sqrt{z}$ | 226.69 | 173.05 | 0.375 | 0.1182 | 0.0878 | 0.3099 | 0.3902 | 0.2811 | 0.355 |
| $a+by^2/x+cz/x$ | 249.25 | 194.26 | 0.244 | 0.1305 | 0.1008 | 0.1594 | 0.4383 | 0.3288 | 0.186 |
| $a+by^2/x+cz^2/x$ | 253.90 | 196.81 | 0.216 | 0.1379 | 0.1034 | 0.0612 | 0.4709 | 0.3505 | 0.061 |
| $a+by^2/x+c\sqrt{z}/x$ | 239.96 | 184.97 | 0.299 | 0.1248 | 0.0940 | 0.2315 | 0.4174 | 0.3070 | 0.262 |
| $a+by^2/x+c/x^2z$ | 239.32 | 183.56 | 0.303 | 0.1241 | 0.0931 | 0.2401 | 0.4160 | 0.3041 | 0.267 |
| $a+by^2/x+c/x^2z^2$ | 236.54 | 180.33 | 0.319 | 0.1232 | 0.0919 | 0.2507 | 0.4102 | 0.2978 | 0.287 |
| $a+by^2/x+c/x^2\sqrt{z}$ | 240.42 | 184.52 | 0.297 | 0.1245 | 0.0934 | 0.2348 | 0.4184 | 0.3060 | 0.258 |
| $a+by^2/x+cz/x^2$ | 243.05 | 186.20 | 0.281 | 0.1257 | 0.0942 | 0.2193 | 0.4244 | 0.3098 | 0.237 |
| $a+by^2/x+cz^2/x^2$ | 245.24 | 187.86 | 0.268 | 0.1271 | 0.0955 | 0.2026 | 0.4294 | 0.3137 | 0.219 |
| $a+by^2/x+c\sqrt{z}/x^2$ | 242.22 | 185.75 | 0.286 | 0.1253 | 0.0940 | 0.2248 | 0.4225 | 0.3087 | 0.244 |

(continued on next page)

**Table 4 – continued from previous page**

| Functional form | $T_{eff}$ (K) | | | Radius ($R_\odot$) | | | log (L/$L_\odot$) | | |
|---|---|---|---|---|---|---|---|---|---|
| | RMSE | MAD | $R^2_{ap}$ | RMSE | MAD | $R^2_{ap}$ | RMSE | MAD | $R^2_{ap}$ |
| $a+by^2/x+c/\sqrt{x}z$ | 189.06 | 136.07 | 0.565 | 0.1038 | 0.0793 | 0.4677 | 0.3284 | 0.2334 | 0.543 |
| $a+by^2/x+c/\sqrt{x}z^2$ | 202.18 | 145.51 | 0.503 | 0.1146 | 0.0912 | 0.3518 | 0.3666 | 0.2727 | 0.431 |
| $a+by^2/x+c/\sqrt{x}\sqrt{z}$ | 197.18 | 142.99 | 0.527 | 0.1050 | 0.0788 | 0.4553 | 0.3370 | 0.2339 | 0.519 |
| $a+by^2/x+cz/\sqrt{x}$ | 242.23 | 181.23 | 0.286 | 0.1328 | 0.0951 | 0.1288 | 0.4584 | 0.3299 | 0.110 |
| $a+by^2/x+cz^2/\sqrt{x}$ | 172.99 | 137.28 | 0.636 | 0.0954 | 0.0689 | 0.5510 | 0.3513 | 0.2634 | 0.477 |
| $a+by^2/x+c\sqrt{z}/\sqrt{x}$ | 254.12 | 201.31 | 0.214 | 0.1344 | 0.1062 | 0.1075 | 0.4505 | 0.3466 | 0.140 |
| $a+by^2/x+cy/z$ | 234.05 | 181.31 | 0.334 | 0.1288 | 0.0949 | 0.1804 | 0.4458 | 0.3260 | 0.158 |
| $a+by^2/x+cy/z^2$ | 235.78 | 182.01 | 0.324 | 0.1302 | 0.1002 | 0.1629 | 0.4443 | 0.3296 | 0.164 |
| $a+by^2/x+cy/\sqrt{z}$ | 258.54 | 201.71 | 0.187 | 0.1390 | 0.1064 | 0.0455 | 0.4722 | 0.3612 | 0.055 |
| $a+by^2/x+cyz$ | 137.23 | 107.16 | 0.771 | 0.0749 | 0.0544 | 0.7230 | 0.2820 | 0.2110 | 0.663 |
| $a+by^2/x+cyz^2$ | 160.02 | 123.98 | 0.688 | 0.0871 | 0.0678 | 0.6253 | 0.3270 | 0.2526 | 0.547 |
| $a+by^2/x+cy\sqrt{z}$ | 128.99 | 98.91 | 0.798 | 0.0706 | 0.0465 | 0.7541 | 0.2538 | 0.1711 | 0.727 |
| $a+by^2/x+cy^2/z$ | 254.23 | 197.00 | 0.214 | 0.1373 | 0.1030 | 0.0687 | 0.4706 | 0.3510 | 0.061 |
| $a+by^2/x+cy^2/z^2$ | 241.73 | 189.20 | 0.289 | 0.1324 | 0.1011 | 0.1349 | 0.4544 | 0.3392 | 0.125 |
| $a+by^2/x+cy^2/\sqrt{z}$ | 243.88 | 198.36 | 0.276 | 0.1301 | 0.1055 | 0.1644 | 0.4287 | 0.3350 | 0.221 |
| $a+by^2/x+cy^2z$ | 149.21 | 112.59 | 0.729 | 0.0820 | 0.0621 | 0.6681 | 0.3065 | 0.2330 | 0.602 |
| $a+by^2/x+cy^2z^2$ | 168.77 | 130.15 | 0.653 | 0.0929 | 0.0730 | 0.5741 | 0.3443 | 0.2637 | 0.498 |
| $a+by^2/x+cy^2\sqrt{z}$ | 140.58 | 102.73 | 0.760 | 0.0773 | 0.0545 | 0.7052 | 0.2821 | 0.1984 | 0.663 |
| $a+by^2/x+c\sqrt{y}/z$ | 210.79 | 157.03 | 0.459 | 0.1187 | 0.0861 | 0.3040 | 0.4089 | 0.2887 | 0.292 |
| $a+by^2/x+c\sqrt{y}/z^2$ | 228.96 | 174.40 | 0.362 | 0.1276 | 0.0982 | 0.1961 | 0.4323 | 0.3181 | 0.208 |
| $a+by^2/x+c\sqrt{y}/\sqrt{z}$ | 232.49 | 178.44 | 0.342 | 0.1281 | 0.0927 | 0.1897 | 0.4445 | 0.3238 | 0.163 |
| $a+by^2/x+c\sqrt{y}z$ | 134.33 | 107.15 | 0.780 | 0.0737 | 0.0520 | 0.7316 | 0.2767 | 0.2035 | 0.676 |
| $a+by^2/x+c\sqrt{y}z^2$ | 156.42 | 123.33 | 0.702 | 0.0848 | 0.0649 | 0.6445 | 0.3197 | 0.2457 | 0.567 |
| $a+by^2/x+c\sqrt{y}\sqrt{z}$ | 125.53 | 98.92 | 0.808 | 0.0697 | 0.0439 | 0.7604 | 0.2491 | 0.1576 | 0.737 |
| $a+by^2/x+c/yz$ | 197.01 | 138.19 | 0.528 | 0.1102 | 0.0851 | 0.3999 | 0.3463 | 0.2496 | 0.492 |
| $a+by^2/x+c/yz^2$ | 212.06 | 155.73 | 0.453 | 0.1203 | 0.0965 | 0.2856 | 0.3855 | 0.2935 | 0.370 |
| $a+by^2/x+c/y\sqrt{z}$ | 199.25 | 144.21 | 0.517 | 0.1087 | 0.0810 | 0.4166 | 0.3429 | 0.2411 | 0.502 |
| $a+by^2/x+cz/y$ | 242.00 | 182.24 | 0.287 | 0.1327 | 0.0958 | 0.1310 | 0.4580 | 0.3308 | 0.111 |
| $a+by^2/x+cz^2/y$ | 170.30 | 132.93 | 0.647 | 0.0945 | 0.0677 | 0.5593 | 0.3458 | 0.2567 | 0.493 |
| $a+by^2/x+c\sqrt{z}/y$ | 253.27 | 200.00 | 0.220 | 0.1343 | 0.1063 | 0.1098 | 0.4479 | 0.3451 | 0.150 |
| $a+by^2/x+c/y^2z$ | 223.21 | 162.48 | 0.394 | 0.1215 | 0.0949 | 0.2712 | 0.3905 | 0.2889 | 0.354 |
| $a+by^2/x+c/y^2z^2$ | 227.66 | 167.90 | 0.369 | 0.1259 | 0.0988 | 0.2177 | 0.4061 | 0.3043 | 0.301 |
| $a+by^2/x+c/y^2\sqrt{z}$ | 223.69 | 164.37 | 0.391 | 0.1203 | 0.0927 | 0.2859 | 0.3880 | 0.2818 | 0.362 |
| $a+by^2/x+cz/y^2$ | 247.25 | 191.10 | 0.256 | 0.1301 | 0.1009 | 0.1645 | 0.4332 | 0.3242 | 0.205 |
| $a+by^2/x+cz^2/y^2$ | 252.00 | 193.83 | 0.227 | 0.1371 | 0.1014 | 0.0717 | 0.4691 | 0.3449 | 0.068 |
| $a+by^2/x+c\sqrt{z}/y^2$ | 235.40 | 177.30 | 0.326 | 0.1239 | 0.0935 | 0.2424 | 0.4076 | 0.2950 | 0.296 |
| $a+by^2/x+c/\sqrt{y}z$ | 175.82 | 121.25 | 0.624 | 0.1020 | 0.0777 | 0.4867 | 0.3212 | 0.2202 | 0.563 |
| $a+by^2/x+c/\sqrt{y}z^2$ | 210.04 | 150.16 | 0.463 | 0.1200 | 0.0939 | 0.2895 | 0.3906 | 0.2831 | 0.353 |
| $a+by^2/x+c/\sqrt{y}\sqrt{z}$ | 167.93 | 118.80 | 0.657 | 0.0949 | 0.0707 | 0.5556 | 0.2953 | 0.1967 | 0.631 |
| $a+by^2/x+cz/\sqrt{y}$ | 170.53 | 131.88 | 0.646 | 0.0964 | 0.0677 | 0.5412 | 0.3481 | 0.2468 | 0.487 |
| $a+by^2/x+cz^2/\sqrt{y}$ | 156.91 | 126.63 | 0.700 | 0.0858 | 0.0639 | 0.6365 | 0.3206 | 0.2489 | 0.564 |
| $a+by^2/x+c\sqrt{z}/\sqrt{y}$ | 237.06 | 179.09 | 0.316 | 0.1303 | 0.0934 | 0.1615 | 0.4516 | 0.3271 | 0.136 |
| $a+b\sqrt{y}/x+cx/z$ | 246.10 | 173.69 | 0.263 | 0.1156 | 0.0879 | 0.3399 | 0.4017 | 0.3002 | 0.316 |
| $a+b\sqrt{y}/x+cx/z^2$ | 243.82 | 177.02 | 0.277 | 0.1187 | 0.0935 | 0.3041 | 0.4020 | 0.2996 | 0.315 |
| $a+b\sqrt{y}/x+cx/\sqrt{z}$ | 275.41 | 208.35 | 0.077 | 0.1316 | 0.1053 | 0.1443 | 0.4402 | 0.3446 | 0.179 |
| $a+b\sqrt{y}/x+cxz$ | 128.38 | 96.07 | 0.799 | 0.0710 | 0.0486 | 0.7509 | 0.2582 | 0.1846 | 0.717 |
| $a+b\sqrt{y}/x+cxz^2$ | 151.66 | 113.66 | 0.720 | 0.0780 | 0.0577 | 0.6998 | 0.2878 | 0.2089 | 0.649 |
| $a+b\sqrt{y}/x+cx\sqrt{z}$ | 112.41 | 85.80 | 0.846 | 0.0696 | 0.0444 | 0.7610 | 0.2407 | 0.1596 | 0.754 |
| $a+b\sqrt{y}/x+cx^2/z$ | 276.81 | 207.42 | 0.068 | 0.1316 | 0.1047 | 0.1454 | 0.4417 | 0.3431 | 0.173 |
| $a+b\sqrt{y}/x+cx^2/z^2$ | 258.52 | 187.38 | 0.187 | 0.1234 | 0.0967 | 0.2485 | 0.4209 | 0.3179 | 0.249 |
| $a+b\sqrt{y}/x+cx^2/\sqrt{z}$ | 187.98 | 145.37 | 0.570 | 0.1053 | 0.0830 | 0.4525 | 0.3276 | 0.2521 | 0.545 |
| $a+b\sqrt{y}/x+cx^2z$ | 136.46 | 104.51 | 0.773 | 0.0751 | 0.0549 | 0.7217 | 0.2722 | 0.2017 | 0.686 |
| $a+b\sqrt{y}/x+cx^2z^2$ | 157.13 | 121.06 | 0.700 | 0.0819 | 0.0626 | 0.6689 | 0.2989 | 0.2233 | 0.621 |
| $a+b\sqrt{y}/x+cx^2\sqrt{z}$ | 124.05 | 95.77 | 0.813 | 0.0732 | 0.0523 | 0.7351 | 0.2574 | 0.1850 | 0.719 |
| $a+b\sqrt{y}/x+c\sqrt{x}/z$ | 210.44 | 147.28 | 0.461 | 0.1035 | 0.0749 | 0.4709 | 0.3551 | 0.2509 | 0.466 |
| $a+b\sqrt{y}/x+c\sqrt{x}/z^2$ | 231.49 | 169.74 | 0.348 | 0.1153 | 0.0903 | 0.3432 | 0.3862 | 0.2857 | 0.368 |
| $a+b\sqrt{y}/x+c\sqrt{x}/\sqrt{z}$ | 235.73 | 162.90 | 0.324 | 0.1095 | 0.0822 | 0.4075 | 0.3855 | 0.2852 | 0.370 |
| $a+b\sqrt{y}/x+c\sqrt{x}z$ | 129.44 | 99.88 | 0.796 | 0.0705 | 0.0458 | 0.7543 | 0.2564 | 0.1767 | 0.721 |
| $a+b\sqrt{y}/x+c\sqrt{x}z^2$ | 150.85 | 115.28 | 0.723 | 0.0767 | 0.0554 | 0.7095 | 0.2842 | 0.2031 | 0.658 |
| $a+b\sqrt{y}/x+c\sqrt{x}\sqrt{z}$ | 114.66 | 87.88 | 0.840 | 0.0696 | 0.0410 | 0.7611 | 0.2403 | 0.1490 | 0.755 |
| $a+b\sqrt{y}/x+c/xz$ | 231.55 | 164.42 | 0.348 | 0.1202 | 0.0922 | 0.2861 | 0.3863 | 0.2777 | 0.368 |
| $a+b\sqrt{y}/x+c/xz^2$ | 234.66 | 166.60 | 0.330 | 0.1215 | 0.0929 | 0.2711 | 0.3908 | 0.2842 | 0.353 |
| $a+b\sqrt{y}/x+c/x\sqrt{z}$ | 238.11 | 167.71 | 0.310 | 0.1221 | 0.0939 | 0.2642 | 0.3956 | 0.2834 | 0.337 |
| $a+b\sqrt{y}/x+cz/x$ | 133.44 | 99.34 | 0.783 | 0.0784 | 0.0549 | 0.6962 | 0.2497 | 0.1683 | 0.736 |
| $a+b\sqrt{y}/x+cz^2/x$ | 136.29 | 98.84 | 0.774 | 0.0731 | 0.0506 | 0.7361 | 0.2578 | 0.1787 | 0.718 |
| $a+b\sqrt{y}/x+c\sqrt{z}/x$ | 145.51 | 108.42 | 0.742 | 0.0833 | 0.0612 | 0.6573 | 0.2583 | 0.1763 | 0.717 |
| $a+b\sqrt{y}/x+c/x^2z$ | 157.45 | 114.24 | 0.698 | 0.0938 | 0.0727 | 0.5652 | 0.2776 | 0.2020 | 0.674 |
| $a+b\sqrt{y}/x+c/x^2z^2$ | 256.21 | 175.36 | 0.201 | 0.1194 | 0.0923 | 0.2961 | 0.4063 | 0.2972 | 0.301 |
| $a+b\sqrt{y}/x+c/x^2\sqrt{z}$ | 175.49 | 127.85 | 0.625 | 0.1015 | 0.0794 | 0.4916 | 0.3049 | 0.2236 | 0.606 |
| $a+b\sqrt{y}/x+cz/x^2$ | 197.72 | 143.12 | 0.524 | 0.1092 | 0.0850 | 0.4113 | 0.3365 | 0.2421 | 0.520 |
| $a+b\sqrt{y}/x+cz^2/x^2$ | 192.12 | 137.56 | 0.551 | 0.1069 | 0.0830 | 0.4360 | 0.3294 | 0.2342 | 0.540 |
| $a+b\sqrt{y}/x+c\sqrt{z}/x^2$ | 194.84 | 141.51 | 0.538 | 0.1083 | 0.0844 | 0.4209 | 0.3324 | 0.2398 | 0.532 |
| $a+b\sqrt{y}/x+c/\sqrt{x}z$ | 182.86 | 130.80 | 0.593 | 0.1032 | 0.0779 | 0.4744 | 0.3229 | 0.2252 | 0.558 |
| $a+b\sqrt{y}/x+c/\sqrt{x}z^2$ | 212.20 | 154.43 | 0.452 | 0.1135 | 0.0880 | 0.3645 | 0.3625 | 0.2648 | 0.443 |
| $a+b\sqrt{y}/x+c/\sqrt{x}\sqrt{z}$ | 166.06 | 115.82 | 0.664 | 0.0974 | 0.0731 | 0.5312 | 0.3016 | 0.2018 | 0.615 |
| $a+b\sqrt{y}/x+cz/\sqrt{x}$ | 145.09 | 114.15 | 0.744 | 0.0745 | 0.0499 | 0.7257 | 0.2665 | 0.1807 | 0.699 |
| $a+b\sqrt{y}/x+cz^2/\sqrt{x}$ | 151.03 | 115.42 | 0.722 | 0.0755 | 0.0544 | 0.7187 | 0.2783 | 0.2009 | 0.672 |
| $a+b\sqrt{y}/x+c\sqrt{z}/\sqrt{x}$ | 173.88 | 131.99 | 0.632 | 0.0838 | 0.0609 | 0.6529 | 0.2983 | 0.2088 | 0.623 |
| $a+b\sqrt{y}/x+cy/z$ | 227.37 | 163.39 | 0.371 | 0.1074 | 0.0802 | 0.4301 | 0.3717 | 0.2742 | 0.415 |
| $a+b\sqrt{y}/x+cy/z^2$ | 233.60 | 169.84 | 0.336 | 0.1151 | 0.0895 | 0.3464 | 0.3873 | 0.2855 | 0.365 |
| $a+b\sqrt{y}/x+cy/\sqrt{z}$ | 272.75 | 199.38 | 0.095 | 0.1261 | 0.0952 | 0.2143 | 0.4323 | 0.3260 | 0.208 |
| $a+b\sqrt{y}/x+cyz$ | 136.69 | 107.35 | 0.773 | 0.0756 | 0.0502 | 0.7181 | 0.2732 | 0.1925 | 0.684 |
| $a+b\sqrt{y}/x+cyz^2$ | 155.28 | 119.29 | 0.707 | 0.0801 | 0.0583 | 0.6833 | 0.2944 | 0.2110 | 0.633 |
| $a+b\sqrt{y}/x+cy\sqrt{z}$ | 130.25 | 99.87 | 0.794 | 0.0776 | 0.0482 | 0.7023 | 0.2695 | 0.1720 | 0.692 |
| $a+b\sqrt{y}/x+cy^2/z$ | 270.73 | 197.18 | 0.108 | 0.1252 | 0.0948 | 0.2260 | 0.4295 | 0.3227 | 0.219 |
| $a+b\sqrt{y}/x+cy^2/z^2$ | 245.95 | 176.78 | 0.264 | 0.1177 | 0.0906 | 0.3156 | 0.4012 | 0.2996 | 0.318 |
| $a+b\sqrt{y}/x+cy^2/\sqrt{z}$ | 248.91 | 202.65 | 0.246 | 0.1262 | 0.1023 | 0.2135 | 0.4158 | 0.3300 | 0.268 |
| $a+b\sqrt{y}/x+cy^2z$ | 147.44 | 112.54 | 0.736 | 0.0813 | 0.0564 | 0.6737 | 0.2919 | 0.2042 | 0.639 |
| $a+b\sqrt{y}/x+cy^2z^2$ | 162.01 | 123.28 | 0.681 | 0.0847 | 0.0629 | 0.6457 | 0.3077 | 0.2232 | 0.599 |
| $a+b\sqrt{y}/x+cy^2\sqrt{z}$ | 144.47 | 105.02 | 0.746 | 0.0835 | 0.0563 | 0.6558 | 0.2913 | 0.1904 | 0.641 |
| $a+b\sqrt{y}/x+c\sqrt{y}/z$ | 198.59 | 141.87 | 0.520 | 0.0994 | 0.0718 | 0.5124 | 0.3372 | 0.2337 | 0.518 |

(continued on next page)

**Table 4 – continued from previous page**

| Functional form | $T_{eff}$ (K) | | | Radius ($R_\odot$) | | | log (L/$L_\odot$) | | |
|---|---|---|---|---|---|---|---|---|---|
| | RMSE | MAD | $R^2_{ap}$ | RMSE | MAD | $R^2_{ap}$ | RMSE | MAD | $R^2_{ap}$ |
| $a+b\sqrt{y}/x+c\sqrt{y}/z^2$ | 224.97 | 165.52 | 0.384 | 0.1133 | 0.0879 | 0.3657 | 0.3773 | 0.2771 | 0.397 |
| $a+b\sqrt{y}/x+c\sqrt{y}/\sqrt{z}$ | 216.90 | 157.42 | 0.428 | 0.1015 | 0.0776 | 0.4914 | 0.3547 | 0.2623 | 0.467 |
| $a+b\sqrt{y}/x+c\sqrt{y}z$ | 133.69 | 107.08 | 0.783 | 0.0730 | 0.0469 | 0.7370 | 0.2647 | 0.1824 | 0.703 |
| $a+b\sqrt{y}/x+c\sqrt{y}z^2$ | 152.72 | 118.59 | 0.716 | 0.0779 | 0.0560 | 0.7006 | 0.2878 | 0.2044 | 0.649 |
| $a+b\sqrt{y}/x+c\sqrt{y}\sqrt{z}$ | 125.00 | 98.75 | 0.810 | 0.0743 | 0.0429 | 0.7278 | 0.2579 | 0.1620 | 0.718 |
| $a+b\sqrt{y}/x+c/yz$ | 200.25 | 140.99 | 0.512 | 0.1101 | 0.0835 | 0.4015 | 0.3459 | 0.2477 | 0.493 |
| $a+b\sqrt{y}/x+c/yz^2$ | 217.35 | 157.79 | 0.425 | 0.1158 | 0.0898 | 0.3376 | 0.3691 | 0.2720 | 0.423 |
| $a+b\sqrt{y}/x+c/y\sqrt{z}$ | 195.67 | 133.40 | 0.534 | 0.1086 | 0.0809 | 0.4173 | 0.3407 | 0.2368 | 0.508 |
| $a+b\sqrt{y}/x+cz/y$ | 191.91 | 147.44 | 0.552 | 0.0881 | 0.0709 | 0.6166 | 0.3142 | 0.2411 | 0.582 |
| $a+b\sqrt{y}/x+cz^2/y$ | 158.31 | 119.55 | 0.695 | 0.0761 | 0.0574 | 0.7144 | 0.2795 | 0.2037 | 0.669 |
| $a+b\sqrt{y}/x+c\sqrt{z}/y$ | 274.61 | 200.44 | 0.083 | 0.1272 | 0.0961 | 0.2008 | 0.4350 | 0.3275 | 0.198 |
| $a+b\sqrt{y}/x+c/y^2z$ | 240.59 | 174.31 | 0.296 | 0.1232 | 0.0961 | 0.2505 | 0.3971 | 0.2923 | 0.332 |
| $a+b\sqrt{y}/x+c/y^2z^2$ | 241.49 | 174.81 | 0.290 | 0.1236 | 0.0961 | 0.2456 | 0.3987 | 0.2919 | 0.326 |
| $a+b\sqrt{y}/x+c/y^2\sqrt{z}$ | 241.71 | 174.61 | 0.289 | 0.1235 | 0.0965 | 0.2469 | 0.3987 | 0.2939 | 0.326 |
| $a+b\sqrt{y}/x+cz/y^2$ | 271.66 | 194.36 | 0.102 | 0.1253 | 0.0942 | 0.2244 | 0.4293 | 0.3186 | 0.219 |
| $a+b\sqrt{y}/x+cz^2/y^2$ | 181.62 | 141.60 | 0.599 | 0.0845 | 0.0684 | 0.6475 | 0.2989 | 0.2350 | 0.621 |
| $a+b\sqrt{y}/x+c\sqrt{z}/y^2$ | 265.46 | 198.04 | 0.143 | 0.1302 | 0.1035 | 0.1631 | 0.4307 | 0.3307 | 0.214 |
| $a+b\sqrt{y}/x+c/\sqrt{y}z$ | 177.38 | 124.07 | 0.617 | 0.1007 | 0.0752 | 0.4995 | 0.3169 | 0.2154 | 0.575 |
| $a+b\sqrt{y}/x+c/\sqrt{y}z^2$ | 211.00 | 151.22 | 0.458 | 0.1124 | 0.0866 | 0.3757 | 0.3613 | 0.2594 | 0.447 |
| $a+b\sqrt{y}/x+c/\sqrt{y}\sqrt{z}$ | 160.97 | 110.71 | 0.685 | 0.0953 | 0.0706 | 0.5519 | 0.2974 | 0.1928 | 0.625 |
| $a+b\sqrt{y}/x+cz/\sqrt{y}$ | 153.89 | 121.43 | 0.712 | 0.0755 | 0.0558 | 0.7185 | 0.2729 | 0.1960 | 0.685 |
| $a+b\sqrt{y}/x+cz^2/\sqrt{y}$ | 153.00 | 114.99 | 0.715 | 0.0752 | 0.0540 | 0.7206 | 0.2787 | 0.1991 | 0.671 |
| $a+b\sqrt{y}/x+c\sqrt{z}/\sqrt{y}$ | 198.75 | 149.02 | 0.519 | 0.0914 | 0.0721 | 0.5871 | 0.3251 | 0.2448 | 0.552 |
| $a+b/x^2y+cx/z$ | 269.55 | 186.02 | 0.116 | 0.1273 | 0.0966 | 0.2002 | 0.4453 | 0.3278 | 0.160 |
| $a+b/x^2y+cx/z^2$ | 259.83 | 183.68 | 0.179 | 0.1266 | 0.0982 | 0.2082 | 0.4344 | 0.3214 | 0.201 |
| $a+b/x^2y+cx/\sqrt{z}$ | 279.31 | 210.22 | 0.051 | 0.1373 | 0.1093 | 0.0687 | 0.4549 | 0.3592 | 0.123 |
| $a+b/x^2y+cxz$ | 128.13 | 94.98 | 0.800 | 0.0718 | 0.0495 | 0.7452 | 0.2641 | 0.1914 | 0.704 |
| $a+b/x^2y+cxz^2$ | 155.55 | 115.12 | 0.706 | 0.0805 | 0.0596 | 0.6799 | 0.3010 | 0.2195 | 0.616 |
| $a+b/x^2y+cx\sqrt{z}$ | 109.85 | 82.82 | 0.853 | 0.0696 | 0.0443 | 0.7609 | 0.2416 | 0.1605 | 0.753 |
| $a+b/x^2y+cx^2/z$ | 286.90 | 214.28 | -0.002 | 0.1388 | 0.1102 | 0.0489 | 0.4655 | 0.3644 | 0.082 |
| $a+b/x^2y+cx^2/z^2$ | 275.86 | 194.13 | 0.074 | 0.1322 | 0.1018 | 0.1368 | 0.4557 | 0.3394 | 0.120 |
| $a+b/x^2y+cx^2/\sqrt{z}$ | 184.86 | 139.27 | 0.584 | 0.1052 | 0.0823 | 0.4533 | 0.3266 | 0.2473 | 0.548 |
| $a+b/x^2y+cx^2z$ | 138.04 | 104.48 | 0.768 | 0.0766 | 0.0561 | 0.7103 | 0.2812 | 0.2106 | 0.665 |
| $a+b/x^2y+cx^2z^2$ | 162.11 | 123.68 | 0.680 | 0.0849 | 0.0646 | 0.6439 | 0.3139 | 0.2317 | 0.583 |
| $a+b/x^2y+cx^2\sqrt{z}$ | 123.35 | 94.15 | 0.815 | 0.0738 | 0.0528 | 0.7308 | 0.2621 | 0.1899 | 0.709 |
| $a+b/x^2y+c\sqrt{x}/z$ | 228.61 | 155.31 | 0.364 | 0.1116 | 0.0801 | 0.3846 | 0.3892 | 0.2754 | 0.358 |
| $a+b/x^2y+c\sqrt{x}/z^2$ | 244.78 | 174.00 | 0.271 | 0.1219 | 0.0946 | 0.2666 | 0.4139 | 0.3029 | 0.274 |
| $a+b/x^2y+c\sqrt{x}/\sqrt{z}$ | 266.91 | 181.98 | 0.133 | 0.1247 | 0.0937 | 0.2320 | 0.4402 | 0.3222 | 0.179 |
| $a+b/x^2y+c\sqrt{x}z$ | 128.88 | 98.65 | 0.798 | 0.0712 | 0.0464 | 0.7496 | 0.2616 | 0.1831 | 0.710 |
| $a+b/x^2y+c\sqrt{x}z^2$ | 154.40 | 116.72 | 0.710 | 0.0791 | 0.0573 | 0.6912 | 0.2967 | 0.2140 | 0.627 |
| $a+b/x^2y+c\sqrt{x}\sqrt{z}$ | 111.69 | 84.08 | 0.848 | 0.0695 | 0.0409 | 0.7614 | 0.2403 | 0.1488 | 0.755 |
| $a+b/x^2y+c/xz$ | 213.11 | 153.40 | 0.447 | 0.1154 | 0.0885 | 0.3420 | 0.3636 | 0.2602 | 0.440 |
| $a+b/x^2y+c/xz^2$ | 227.24 | 161.28 | 0.372 | 0.1206 | 0.0922 | 0.2821 | 0.3850 | 0.2807 | 0.372 |
| $a+b/x^2y+c/x\sqrt{z}$ | 206.13 | 148.93 | 0.483 | 0.1130 | 0.0869 | 0.3700 | 0.3533 | 0.2540 | 0.471 |
| $a+b/x^2y+cz/x$ | 229.62 | 163.51 | 0.358 | 0.1049 | 0.0781 | 0.4563 | 0.3834 | 0.2770 | 0.377 |
| $a+b/x^2y+cz^2/x$ | 165.97 | 123.20 | 0.665 | 0.0811 | 0.0598 | 0.6756 | 0.3013 | 0.2186 | 0.615 |
| $a+b/x^2y+c\sqrt{z}/x$ | 268.06 | 197.52 | 0.126 | 0.1347 | 0.1054 | 0.1041 | 0.4407 | 0.3382 | 0.177 |
| $a+b/x^2y+c/x^2z$ | 246.98 | 177.52 | 0.258 | 0.1269 | 0.0984 | 0.2048 | 0.4104 | 0.3008 | 0.287 |
| $a+b/x^2y+c/x^2z^2$ | 253.64 | 180.09 | 0.217 | 0.1291 | 0.0993 | 0.1766 | 0.4203 | 0.3058 | 0.252 |
| $a+b/x^2y+c/x^2\sqrt{z}$ | 235.44 | 171.56 | 0.326 | 0.1231 | 0.0961 | 0.2522 | 0.3936 | 0.2906 | 0.344 |
| $a+b/x^2y+cz/x^2$ | 256.27 | 181.19 | 0.201 | 0.1292 | 0.0988 | 0.1761 | 0.4233 | 0.3097 | 0.241 |
| $a+b/x^2y+cz^2/x^2$ | 221.72 | 156.73 | 0.402 | 0.1158 | 0.0885 | 0.3379 | 0.3743 | 0.2745 | 0.407 |
| $a+b/x^2y+c\sqrt{z}/x^2$ | 273.54 | 196.90 | 0.090 | 0.1349 | 0.1038 | 0.1017 | 0.4482 | 0.3337 | 0.149 |
| $a+b/x^2y+c/\sqrt{x}z$ | 179.47 | 129.16 | 0.608 | 0.1027 | 0.0780 | 0.4793 | 0.3197 | 0.2237 | 0.567 |
| $a+b/x^2y+c/\sqrt{x}z^2$ | 211.47 | 152.57 | 0.456 | 0.1144 | 0.0884 | 0.3538 | 0.3661 | 0.2647 | 0.432 |
| $a+b/x^2y+c/\sqrt{x}\sqrt{z}$ | 165.07 | 115.49 | 0.668 | 0.0977 | 0.0735 | 0.5292 | 0.2993 | 0.2035 | 0.620 |
| $a+b/x^2y+cz/\sqrt{x}$ | 170.56 | 127.93 | 0.646 | 0.0825 | 0.0579 | 0.6642 | 0.3059 | 0.2129 | 0.603 |
| $a+b/x^2y+cz^2/\sqrt{x}$ | 160.52 | 120.99 | 0.687 | 0.0794 | 0.0578 | 0.6887 | 0.2978 | 0.2177 | 0.624 |
| $a+b/x^2y+c\sqrt{z}/\sqrt{x}$ | 256.77 | 170.37 | 0.198 | 0.1177 | 0.0868 | 0.3157 | 0.4232 | 0.3027 | 0.241 |
| $a+b/x^2y+cy/z$ | 246.56 | 168.48 | 0.260 | 0.1166 | 0.0865 | 0.3290 | 0.4086 | 0.2996 | 0.293 |
| $a+b/x^2y+cy/z^2$ | 247.37 | 174.68 | 0.255 | 0.1219 | 0.0938 | 0.2669 | 0.4159 | 0.3041 | 0.267 |
| $a+b/x^2y+cy/\sqrt{z}$ | 290.94 | 211.23 | -0.030 | 0.1374 | 0.1047 | 0.0685 | 0.4716 | 0.3552 | 0.058 |
| $a+b/x^2y+cyz$ | 137.33 | 107.11 | 0.771 | 0.0768 | 0.0516 | 0.7089 | 0.2809 | 0.2014 | 0.666 |
| $a+b/x^2y+cyz^2$ | 159.65 | 121.19 | 0.690 | 0.0829 | 0.0606 | 0.6608 | 0.3085 | 0.2223 | 0.597 |
| $a+b/x^2y+cy\sqrt{z}$ | 128.22 | 97.04 | 0.800 | 0.0780 | 0.0485 | 0.6996 | 0.2726 | 0.1767 | 0.685 |
| $a+b/x^2y+cy^2/z$ | 288.95 | 208.02 | -0.016 | 0.1357 | 0.1026 | 0.0908 | 0.4679 | 0.3494 | 0.072 |
| $a+b/x^2y+cy^2/z^2$ | 262.55 | 183.67 | 0.161 | 0.1260 | 0.0955 | 0.2159 | 0.4347 | 0.3221 | 0.199 |
| $a+b/x^2y+cy^2/\sqrt{z}$ | 248.69 | 201.74 | 0.248 | 0.1291 | 0.1036 | 0.1773 | 0.4260 | 0.3311 | 0.231 |
| $a+b/x^2y+cy^2z$ | 149.50 | 113.17 | 0.728 | 0.0832 | 0.0579 | 0.6580 | 0.3025 | 0.2152 | 0.612 |
| $a+b/x^2y+cy^2z^2$ | 167.39 | 125.69 | 0.659 | 0.0880 | 0.0652 | 0.6175 | 0.3236 | 0.2319 | 0.556 |
| $a+b/x^2y+cy^2\sqrt{z}$ | 144.13 | 103.38 | 0.747 | 0.0846 | 0.0571 | 0.6465 | 0.2980 | 0.1980 | 0.624 |
| $a+b/x^2y+c\sqrt{y}/z$ | 210.61 | 145.51 | 0.460 | 0.1048 | 0.0742 | 0.4579 | 0.3616 | 0.2506 | 0.446 |
| $a+b/x^2y+c\sqrt{y}/z^2$ | 235.85 | 168.15 | 0.323 | 0.1188 | 0.0916 | 0.3028 | 0.4009 | 0.2909 | 0.319 |
| $a+b/x^2y+c\sqrt{y}/\sqrt{z}$ | 238.02 | 164.17 | 0.311 | 0.1113 | 0.0835 | 0.3887 | 0.3942 | 0.2856 | 0.342 |
| $a+b/x^2y+c\sqrt{y}z$ | 134.40 | 106.96 | 0.780 | 0.0741 | 0.0482 | 0.7291 | 0.2719 | 0.1907 | 0.687 |
| $a+b/x^2y+c\sqrt{y}z^2$ | 156.78 | 120.42 | 0.701 | 0.0805 | 0.0581 | 0.6804 | 0.3011 | 0.2160 | 0.616 |
| $a+b/x^2y+c\sqrt{y}\sqrt{z}$ | 123.31 | 96.19 | 0.815 | 0.0745 | 0.0431 | 0.7258 | 0.2606 | 0.1652 | 0.712 |
| $a+b/x^2y+c/yz$ | 198.72 | 140.63 | 0.520 | 0.1103 | 0.0842 | 0.3995 | 0.3463 | 0.2490 | 0.492 |
| $a+b/x^2y+c/yz^2$ | 218.47 | 157.79 | 0.419 | 0.1174 | 0.0911 | 0.3196 | 0.3752 | 0.2754 | 0.403 |
| $a+b/x^2y+c/y\sqrt{z}$ | 193.00 | 133.57 | 0.547 | 0.1083 | 0.0810 | 0.4205 | 0.3388 | 0.2368 | 0.514 |
| $a+b/x^2y+cz/y$ | 220.47 | 158.51 | 0.409 | 0.1001 | 0.0788 | 0.5049 | 0.3635 | 0.2666 | 0.440 |
| $a+b/x^2y+cz^2/y$ | 167.20 | 123.56 | 0.660 | 0.0798 | 0.0601 | 0.6855 | 0.2984 | 0.2154 | 0.623 |
| $a+b/x^2y+c\sqrt{z}/y$ | 288.44 | 215.60 | -0.012 | 0.1392 | 0.1094 | 0.0429 | 0.4709 | 0.3625 | 0.061 |
| $a+b/x^2y+c/y^2z$ | 237.84 | 171.50 | 0.312 | 0.1239 | 0.0963 | 0.2415 | 0.3982 | 0.2916 | 0.328 |
| $a+b/x^2y+c/y^2z^2$ | 242.32 | 173.60 | 0.286 | 0.1256 | 0.0968 | 0.2210 | 0.4053 | 0.2939 | 0.304 |
| $a+b/x^2y+c/y^2\sqrt{z}$ | 236.15 | 170.35 | 0.322 | 0.1233 | 0.0962 | 0.2489 | 0.3958 | 0.2909 | 0.336 |
| $a+b/x^2y+cz/y^2$ | 283.66 | 212.66 | 0.021 | 0.1386 | 0.1096 | 0.0517 | 0.4649 | 0.3593 | 0.084 |
| $a+b/x^2y+cz^2/y^2$ | 215.63 | 157.70 | 0.434 | 0.0977 | 0.0785 | 0.5291 | 0.3549 | 0.2666 | 0.466 |
| $a+b/x^2y+c\sqrt{z}/y^2$ | 250.20 | 182.84 | 0.238 | 0.1286 | 0.0996 | 0.1839 | 0.4178 | 0.3130 | 0.260 |
| $a+b/x^2y+c/\sqrt{y}z$ | 176.90 | 123.51 | 0.619 | 0.1010 | 0.0756 | 0.4959 | 0.3189 | 0.2153 | 0.569 |

(continued on next page)

**Table 4 – continued from previous page**

| Functional form | $T_{eff}$ (K) | | | Radius ($R_\odot$) | | | log (L/$L_\odot$) | | |
|---|---|---|---|---|---|---|---|---|---|
| | RMSE | MAD | $R^2_{ap}$ | RMSE | MAD | $R^2_{ap}$ | RMSE | MAD | $R^2_{ap}$ |
| $a+b/x^2y+c/\sqrt{y}z^2$ | 213.99 | 150.85 | 0.443 | 0.1147 | 0.0871 | 0.3507 | 0.3710 | 0.2636 | 0.417 |
| $a+b/x^2y+c/\sqrt{y}\sqrt{z}$ | 159.91 | 110.50 | 0.689 | 0.0952 | 0.0707 | 0.5521 | 0.2971 | 0.1938 | 0.626 |
| $a+b/x^2y+cz/\sqrt{y}$ | 162.99 | 125.32 | 0.677 | 0.0790 | 0.0585 | 0.6919 | 0.2913 | 0.2067 | 0.640 |
| $a+b/x^2y+cz^2/\sqrt{y}$ | 158.44 | 117.05 | 0.695 | 0.0780 | 0.0562 | 0.6997 | 0.2931 | 0.2119 | 0.636 |
| $a+b/x^2y+c\sqrt{z}/\sqrt{y}$ | 224.66 | 159.52 | 0.386 | 0.1027 | 0.0793 | 0.4788 | 0.3709 | 0.2672 | 0.417 |
| $a+b/x^2y^2y+cx/z$ | 270.17 | 186.26 | 0.112 | 0.1276 | 0.0968 | 0.1961 | 0.4465 | 0.3284 | 0.155 |
| $a+b/x^2y^2y+cx/z^2$ | 260.25 | 183.74 | 0.176 | 0.1269 | 0.0983 | 0.2054 | 0.4353 | 0.3218 | 0.197 |
| $a+b/x^2y^2y+cx/\sqrt{z}$ | 279.28 | 210.06 | 0.051 | 0.1374 | 0.1093 | 0.0675 | 0.4551 | 0.3592 | 0.123 |
| $a+b/x^2y^2y+cxz$ | 128.09 | 94.91 | 0.800 | 0.0719 | 0.0495 | 0.7451 | 0.2643 | 0.1916 | 0.704 |
| $a+b/x^2y^2y+cxz^2$ | 155.63 | 115.10 | 0.705 | 0.0806 | 0.0596 | 0.6793 | 0.3014 | 0.2197 | 0.615 |
| $a+b/x^2y^2y+cx\sqrt{z}$ | 109.76 | 82.71 | 0.853 | 0.0696 | 0.0443 | 0.7609 | 0.2416 | 0.1604 | 0.753 |
| $a+b/x^2y^2y+cx^2/z$ | 287.08 | 214.28 | -0.003 | 0.1390 | 0.1103 | 0.0467 | 0.4660 | 0.3647 | 0.080 |
| $a+b/x^2y^2y+cx^2/z^2$ | 276.30 | 194.19 | 0.071 | 0.1325 | 0.1019 | 0.1337 | 0.4567 | 0.3397 | 0.116 |
| $a+b/x^2y^2y+cx^2/\sqrt{z}$ | 184.78 | 139.13 | 0.585 | 0.1052 | 0.0823 | 0.4534 | 0.3266 | 0.2472 | 0.548 |
| $a+b/x^2y^2y+cx^2z$ | 138.06 | 104.43 | 0.768 | 0.0766 | 0.0561 | 0.7100 | 0.2815 | 0.2108 | 0.664 |
| $a+b/x^2y^2y+cx^2z^2$ | 162.22 | 123.68 | 0.680 | 0.0850 | 0.0646 | 0.6431 | 0.3143 | 0.2319 | 0.581 |
| $a+b/x^2y^2y+cx^2\sqrt{z}$ | 123.30 | 94.07 | 0.815 | 0.0739 | 0.0528 | 0.7307 | 0.2622 | 0.1900 | 0.709 |
| $a+b/x^2y^2y+c\sqrt{x}/z$ | 229.14 | 155.47 | 0.361 | 0.1119 | 0.0802 | 0.3819 | 0.3902 | 0.2761 | 0.355 |
| $a+b/x^2y^2y+c\sqrt{x}/z^2$ | 245.13 | 174.02 | 0.269 | 0.1221 | 0.0947 | 0.2645 | 0.4147 | 0.3033 | 0.271 |
| $a+b/x^2y^2y+c\sqrt{x}/\sqrt{z}$ | 267.75 | 182.37 | 0.128 | 0.1252 | 0.0940 | 0.2266 | 0.4417 | 0.3230 | 0.173 |
| $a+b/x^2y^2y+c\sqrt{x}z$ | 128.84 | 98.57 | 0.798 | 0.0712 | 0.0464 | 0.7495 | 0.2618 | 0.1833 | 0.710 |
| $a+b/x^2y^2y+c\sqrt{x}z^2$ | 154.47 | 116.70 | 0.710 | 0.0791 | 0.0574 | 0.6907 | 0.2971 | 0.2143 | 0.626 |
| $a+b/x^2y^2y+c\sqrt{x}\sqrt{z}$ | 111.60 | 83.96 | 0.848 | 0.0695 | 0.0409 | 0.7614 | 0.2403 | 0.1488 | 0.755 |
| $a+b/x^2y^2y+c/xz$ | 212.98 | 153.38 | 0.448 | 0.1154 | 0.0885 | 0.3424 | 0.3634 | 0.2602 | 0.440 |
| $a+b/x^2y^2y+c/xz^2$ | 227.12 | 161.28 | 0.372 | 0.1206 | 0.0922 | 0.2823 | 0.3849 | 0.2807 | 0.372 |
| $a+b/x^2y^2y+c/x\sqrt{z}$ | 206.08 | 148.96 | 0.483 | 0.1130 | 0.0869 | 0.3700 | 0.3532 | 0.2541 | 0.471 |
| $a+b/x^2y^2y+cz/x$ | 235.38 | 166.19 | 0.326 | 0.1074 | 0.0799 | 0.4304 | 0.3920 | 0.2818 | 0.349 |
| $a+b/x^2y^2y+cz^2/x$ | 167.14 | 123.86 | 0.660 | 0.0814 | 0.0601 | 0.6726 | 0.3031 | 0.2197 | 0.611 |
| $a+b/x^2y^2y+c\sqrt{z}/x$ | 265.68 | 194.89 | 0.141 | 0.1341 | 0.1045 | 0.1123 | 0.4375 | 0.3343 | 0.189 |
| $a+b/x^2y^2y+c/x^2z$ | 244.55 | 176.55 | 0.272 | 0.1262 | 0.0981 | 0.2140 | 0.4070 | 0.2991 | 0.298 |
| $a+b/x^2y^2y+c/x^2z^2$ | 252.63 | 179.87 | 0.224 | 0.1289 | 0.0993 | 0.1801 | 0.4190 | 0.3054 | 0.256 |
| $a+b/x^2y^2y+c/x^2\sqrt{z}$ | 231.66 | 169.47 | 0.347 | 0.1219 | 0.0954 | 0.2663 | 0.3883 | 0.2876 | 0.361 |
| $a+b/x^2y^2y+cz/x^2$ | 262.87 | 184.09 | 0.159 | 0.1312 | 0.0993 | 0.1495 | 0.4329 | 0.3144 | 0.206 |
| $a+b/x^2y^2y+cz^2/x^2$ | 223.86 | 158.18 | 0.390 | 0.1163 | 0.0886 | 0.3323 | 0.3773 | 0.2768 | 0.397 |
| $a+b/x^2y^2y+c\sqrt{z}/x^2$ | 285.62 | 209.70 | 0.007 | 0.1383 | 0.1082 | 0.0551 | 0.4657 | 0.3546 | 0.081 |
| $a+b/x^2y^2y+c/\sqrt{x}z$ | 179.47 | 129.16 | 0.608 | 0.1027 | 0.0780 | 0.4792 | 0.3197 | 0.2237 | 0.567 |
| $a+b/x^2y^2y+c/\sqrt{x}z^2$ | 211.44 | 152.62 | 0.456 | 0.1144 | 0.0884 | 0.3536 | 0.3662 | 0.2648 | 0.432 |
| $a+b/x^2y^2y+c/\sqrt{x}\sqrt{z}$ | 165.25 | 115.53 | 0.668 | 0.0977 | 0.0735 | 0.5285 | 0.2994 | 0.2037 | 0.620 |
| $a+b/x^2y^2y+cz/\sqrt{x}$ | 171.49 | 128.29 | 0.642 | 0.0828 | 0.0582 | 0.6615 | 0.3074 | 0.2138 | 0.600 |
| $a+b/x^2y^2y+cz^2/\sqrt{x}$ | 160.79 | 121.12 | 0.685 | 0.0795 | 0.0578 | 0.6878 | 0.2984 | 0.2181 | 0.623 |
| $a+b/x^2y^2y+c\sqrt{z}/\sqrt{x}$ | 259.17 | 171.85 | 0.183 | 0.1189 | 0.0877 | 0.3019 | 0.4270 | 0.3055 | 0.227 |
| $a+b/x^2y^2y+cy/z$ | 247.12 | 168.59 | 0.257 | 0.1169 | 0.0867 | 0.3257 | 0.4097 | 0.3002 | 0.289 |
| $a+b/x^2y^2y+cy/z^2$ | 247.74 | 174.74 | 0.253 | 0.1220 | 0.0938 | 0.2645 | 0.4167 | 0.3044 | 0.264 |
| $a+b/x^2y^2y+cy/\sqrt{z}$ | 291.33 | 211.51 | -0.033 | 0.1376 | 0.1049 | 0.0646 | 0.4726 | 0.3557 | 0.054 |
| $a+b/x^2y^2y+cyz$ | 137.32 | 107.06 | 0.771 | 0.0768 | 0.0516 | 0.7087 | 0.2811 | 0.2016 | 0.665 |
| $a+b/x^2y^2y+cyz^2$ | 159.75 | 121.18 | 0.690 | 0.0830 | 0.0606 | 0.6602 | 0.3088 | 0.2226 | 0.596 |
| $a+b/x^2y^2y+cy\sqrt{z}$ | 128.16 | 96.94 | 0.800 | 0.0780 | 0.0485 | 0.6995 | 0.2727 | 0.1768 | 0.685 |
| $a+b/x^2y^2y+cy^2/z$ | 289.39 | 208.13 | -0.019 | 0.1360 | 0.1028 | 0.0869 | 0.4689 | 0.3500 | 0.068 |
| $a+b/x^2y^2y+cy^2/z^2$ | 263.00 | 183.72 | 0.158 | 0.1263 | 0.0956 | 0.2129 | 0.4357 | 0.3225 | 0.196 |
| $a+b/x^2y^2y+cy^2/\sqrt{z}$ | 248.63 | 201.62 | 0.248 | 0.1291 | 0.1036 | 0.1767 | 0.4262 | 0.3310 | 0.230 |
| $a+b/x^2y^2y+cy^2z$ | 149.53 | 113.13 | 0.728 | 0.0833 | 0.0580 | 0.6576 | 0.3027 | 0.2154 | 0.612 |
| $a+b/x^2y^2y+cy^2z^2$ | 167.51 | 125.69 | 0.659 | 0.0881 | 0.0652 | 0.6167 | 0.3240 | 0.2322 | 0.555 |
| $a+b/x^2y^2y+cy^2\sqrt{z}$ | 144.09 | 103.31 | 0.747 | 0.0846 | 0.0571 | 0.6463 | 0.2982 | 0.1981 | 0.623 |
| $a+b/x^2y^2y+c\sqrt{y}/z$ | 210.96 | 145.58 | 0.459 | 0.1050 | 0.0743 | 0.4561 | 0.3623 | 0.2511 | 0.444 |
| $a+b/x^2y^2y+c\sqrt{y}/z^2$ | 236.13 | 168.16 | 0.322 | 0.1190 | 0.0916 | 0.3011 | 0.4016 | 0.2911 | 0.317 |
| $a+b/x^2y^2y+c\sqrt{y}/\sqrt{z}$ | 238.67 | 164.33 | 0.307 | 0.1116 | 0.0836 | 0.3851 | 0.3954 | 0.2862 | 0.337 |
| $a+b/x^2y^2y+c\sqrt{y}z$ | 134.40 | 106.92 | 0.780 | 0.0741 | 0.0482 | 0.7289 | 0.2721 | 0.1909 | 0.686 |
| $a+b/x^2y^2y+c\sqrt{y}z^2$ | 156.87 | 120.41 | 0.701 | 0.0805 | 0.0581 | 0.6798 | 0.3015 | 0.2163 | 0.615 |
| $a+b/x^2y^2y+c\sqrt{y}\sqrt{z}$ | 123.26 | 96.10 | 0.815 | 0.0745 | 0.0431 | 0.7258 | 0.2606 | 0.1653 | 0.712 |
| $a+b/x^2y^2y+c/yz$ | 198.71 | 140.62 | 0.520 | 0.1103 | 0.0842 | 0.3995 | 0.3463 | 0.2490 | 0.492 |
| $a+b/x^2y^2y+c/yz^2$ | 218.48 | 157.85 | 0.419 | 0.1174 | 0.0911 | 0.3193 | 0.3753 | 0.2755 | 0.403 |
| $a+b/x^2y^2y+c/y\sqrt{z}$ | 193.01 | 133.61 | 0.547 | 0.1083 | 0.0810 | 0.4204 | 0.3388 | 0.2368 | 0.514 |
| $a+b/x^2y^2y+cz/y$ | 221.45 | 158.80 | 0.403 | 0.1006 | 0.0791 | 0.5003 | 0.3653 | 0.2672 | 0.435 |
| $a+b/x^2y^2y+cz^2/y$ | 167.47 | 123.62 | 0.659 | 0.0799 | 0.0602 | 0.6844 | 0.2990 | 0.2157 | 0.621 |
| $a+b/x^2y^2y+c\sqrt{z}/y$ | 288.46 | 215.63 | -0.012 | 0.1394 | 0.1096 | 0.0404 | 0.4713 | 0.3627 | 0.059 |
| $a+b/x^2y^2y+c/y^2z$ | 237.78 | 171.53 | 0.312 | 0.1239 | 0.0964 | 0.2415 | 0.3982 | 0.2917 | 0.328 |
| $a+b/x^2y^2y+c/y^2z^2$ | 242.32 | 173.67 | 0.286 | 0.1256 | 0.0969 | 0.2206 | 0.4054 | 0.2941 | 0.304 |
| $a+b/x^2y^2y+c/y^2\sqrt{z}$ | 236.04 | 170.35 | 0.322 | 0.1233 | 0.0962 | 0.2490 | 0.3958 | 0.2909 | 0.336 |
| $a+b/x^2y^2y+cz/y^2$ | 283.34 | 212.34 | 0.023 | 0.1386 | 0.1096 | 0.0508 | 0.4648 | 0.3593 | 0.085 |
| $a+b/x^2y^2y+cz^2/y^2$ | 216.87 | 158.10 | 0.428 | 0.0982 | 0.0788 | 0.5238 | 0.3571 | 0.2675 | 0.460 |
| $a+b/x^2y^2y+c\sqrt{z}/y^2$ | 249.87 | 182.80 | 0.240 | 0.1285 | 0.0996 | 0.1847 | 0.4174 | 0.3131 | 0.262 |
| $a+b/x^2y^2y+c/\sqrt{y}z$ | 176.89 | 123.52 | 0.619 | 0.1010 | 0.0756 | 0.4959 | 0.3189 | 0.2153 | 0.569 |
| $a+b/x^2y^2y+c/\sqrt{y}z^2$ | 214.05 | 150.82 | 0.443 | 0.1147 | 0.0872 | 0.3502 | 0.3712 | 0.2637 | 0.416 |
| $a+b/x^2y^2y+c/\sqrt{y}\sqrt{z}$ | 159.93 | 110.51 | 0.689 | 0.0952 | 0.0707 | 0.5520 | 0.2971 | 0.1938 | 0.626 |
| $a+b/x^2y^2y+cz/\sqrt{y}$ | 163.28 | 125.40 | 0.676 | 0.0791 | 0.0586 | 0.6909 | 0.2919 | 0.2070 | 0.639 |
| $a+b/x^2y^2y+cz^2/\sqrt{y}$ | 158.58 | 117.07 | 0.694 | 0.0781 | 0.0563 | 0.6990 | 0.2935 | 0.2122 | 0.635 |
| $a+b/x^2y^2y+c\sqrt{z}/\sqrt{y}$ | 225.52 | 159.74 | 0.381 | 0.1032 | 0.0796 | 0.4746 | 0.3725 | 0.2678 | 0.412 |
| $a+b/x^2\sqrt{y}+cx/z$ | 269.16 | 185.84 | 0.119 | 0.1271 | 0.0965 | 0.2028 | 0.4445 | 0.3274 | 0.163 |
| $a+b/x^2\sqrt{y}+cx/z^2$ | 259.56 | 183.62 | 0.180 | 0.1265 | 0.0982 | 0.2100 | 0.4338 | 0.3211 | 0.203 |
| $a+b/x^2\sqrt{y}+cx/\sqrt{z}$ | 279.33 | 210.34 | 0.051 | 0.1373 | 0.1093 | 0.0696 | 0.4548 | 0.3592 | 0.124 |
| $a+b/x^2\sqrt{y}+cxz$ | 128.14 | 95.02 | 0.800 | 0.0718 | 0.0495 | 0.7453 | 0.2640 | 0.1913 | 0.705 |
| $a+b/x^2\sqrt{y}+cxz^2$ | 155.50 | 115.13 | 0.706 | 0.0805 | 0.0596 | 0.6802 | 0.3008 | 0.2193 | 0.617 |
| $a+b/x^2\sqrt{y}+cx\sqrt{z}$ | 109.89 | 82.87 | 0.853 | 0.0696 | 0.0443 | 0.7609 | 0.2416 | 0.1605 | 0.753 |
| $a+b/x^2\sqrt{y}+cx^2/z$ | 286.78 | 214.26 | -0.001 | 0.1387 | 0.1102 | 0.0504 | 0.4651 | 0.3642 | 0.08 |
| $a+b/x^2\sqrt{y}+cx^2/z^2$ | 275.58 | 194.06 | 0.076 | 0.1321 | 0.1017 | 0.1389 | 0.4551 | 0.3391 | 0.122 |
| $a+b/x^2\sqrt{y}+cx^2/\sqrt{z}$ | 184.92 | 139.39 | 0.584 | 0.1052 | 0.0823 | 0.4533 | 0.3266 | 0.2474 | 0.548 |
| $a+b/x^2\sqrt{y}+cx^2z$ | 138.02 | 104.51 | 0.768 | 0.0766 | 0.0560 | 0.7105 | 0.2811 | 0.2105 | 0.665 |
| $a+b/x^2\sqrt{y}+cx^2z^2$ | 162.04 | 123.66 | 0.681 | 0.0849 | 0.0645 | 0.6443 | 0.3136 | 0.2316 | 0.583 |
| $a+b/x^2\sqrt{y}+cx^2\sqrt{z}$ | 123.37 | 94.19 | 0.815 | 0.0738 | 0.0528 | 0.7309 | 0.2620 | 0.1898 | 0.709 |

(continued on next page)

**Table 4 – continued from previous page**

| Functional form | $T_{eff}$ (K) | | | Radius ($R_\odot$) | | | log (L/$L_\odot$) | | |
|---|---|---|---|---|---|---|---|---|---|
| | RMSE | MAD | $R^2_{ap}$ | RMSE | MAD | $R^2_{ap}$ | RMSE | MAD | $R^2_{ap}$ |
| $a+b/x^2\sqrt{y}+c\sqrt{x}/z$ | 228.29 | 155.19 | 0.366 | 0.1115 | 0.0800 | 0.3863 | 0.3886 | 0.2750 | 0.360 |
| $a+b/x^2\sqrt{y}+c\sqrt{x}/z^2$ | 244.55 | 173.97 | 0.272 | 0.1218 | 0.0945 | 0.2681 | 0.4134 | 0.3026 | 0.276 |
| $a+b/x^2\sqrt{y}+c\sqrt{x}/\sqrt{z}$ | 266.39 | 181.69 | 0.137 | 0.1244 | 0.0935 | 0.2354 | 0.4393 | 0.3217 | 0.182 |
| $a+b/x^2\sqrt{y}+c\sqrt{x}z$ | 128.90 | 98.69 | 0.798 | 0.0712 | 0.0464 | 0.7497 | 0.2615 | 0.1831 | 0.710 |
| $a+b/x^2\sqrt{y}+c\sqrt{x}z^2$ | 154.36 | 116.73 | 0.710 | 0.0790 | 0.0573 | 0.6915 | 0.2965 | 0.2138 | 0.628 |
| $a+b/x^2\sqrt{y}+c\sqrt{x}\sqrt{z}$ | 111.74 | 84.15 | 0.848 | 0.0695 | 0.0408 | 0.7614 | 0.2403 | 0.1488 | 0.755 |
| $a+b/x^2\sqrt{y}+c/xz$ | 213.50 | 153.62 | 0.445 | 0.1155 | 0.0885 | 0.3409 | 0.3640 | 0.2605 | 0.439 |
| $a+b/x^2\sqrt{y}+c/xz^2$ | 227.43 | 161.32 | 0.371 | 0.1206 | 0.0922 | 0.2818 | 0.3852 | 0.2806 | 0.371 |
| $a+b/x^2\sqrt{y}+c/x\sqrt{z}$ | 206.67 | 149.30 | 0.480 | 0.1131 | 0.0870 | 0.3683 | 0.3540 | 0.2545 | 0.469 |
| $a+b/x^2\sqrt{y}+cz/x$ | 226.16 | 161.60 | 0.378 | 0.1035 | 0.0769 | 0.4715 | 0.3783 | 0.2734 | 0.394 |
| $a+b/x^2\sqrt{y}+cz^2/x$ | 165.26 | 122.76 | 0.668 | 0.0808 | 0.0596 | 0.6775 | 0.3003 | 0.2179 | 0.618 |
| $a+b/x^2\sqrt{y}+c\sqrt{z}/x$ | 270.13 | 199.63 | 0.112 | 0.1352 | 0.1061 | 0.0973 | 0.4435 | 0.3413 | 0.167 |
| $a+b/x^2\sqrt{y}+c/x^2z$ | 250.01 | 178.65 | 0.240 | 0.1278 | 0.0988 | 0.1932 | 0.4146 | 0.3029 | 0.272 |
| $a+b/x^2\sqrt{y}+c/x^2z^2$ | 254.72 | 180.31 | 0.211 | 0.1294 | 0.0993 | 0.1728 | 0.4217 | 0.3063 | 0.246 |
| $a+b/x^2\sqrt{y}+c/x^2\sqrt{z}$ | 241.91 | 174.90 | 0.288 | 0.1251 | 0.0973 | 0.2270 | 0.4027 | 0.2959 | 0.313 |
| $a+b/x^2\sqrt{y}+cz/x^2$ | 250.32 | 177.95 | 0.238 | 0.1272 | 0.0980 | 0.2007 | 0.4146 | 0.3045 | 0.272 |
| $a+b/x^2\sqrt{y}+cz^2/x^2$ | 218.52 | 154.13 | 0.419 | 0.1148 | 0.0878 | 0.3497 | 0.3696 | 0.2705 | 0.421 |
| $a+b/x^2\sqrt{y}+c\sqrt{z}/x^2$ | 263.30 | 184.66 | 0.157 | 0.1317 | 0.0999 | 0.1435 | 0.4334 | 0.3144 | 0.204 |
| $a+b/x^2\sqrt{y}+c/\sqrt{x}z$ | 179.57 | 129.21 | 0.608 | 0.1027 | 0.0780 | 0.4791 | 0.3197 | 0.2237 | 0.567 |
| $a+b/x^2\sqrt{y}+c/\sqrt{x}z^2$ | 211.49 | 152.53 | 0.456 | 0.1144 | 0.0884 | 0.3540 | 0.3660 | 0.2646 | 0.432 |
| $a+b/x^2\sqrt{y}+c/\sqrt{x}\sqrt{z}$ | 165.17 | 115.56 | 0.668 | 0.0977 | 0.0735 | 0.5290 | 0.2994 | 0.2035 | 0.620 |
| $a+b/x^2\sqrt{y}+cz/\sqrt{x}$ | 170.03 | 127.68 | 0.648 | 0.0823 | 0.0578 | 0.6658 | 0.3051 | 0.2124 | 0.606 |
| $a+b/x^2\sqrt{y}+cz^2/\sqrt{x}$ | 160.35 | 120.90 | 0.687 | 0.0793 | 0.0577 | 0.6893 | 0.2974 | 0.2175 | 0.625 |
| $a+b/x^2\sqrt{y}+c\sqrt{z}/\sqrt{x}$ | 255.31 | 169.74 | 0.207 | 0.1170 | 0.0862 | 0.3240 | 0.4209 | 0.3008 | 0.249 |
| $a+b/x^2\sqrt{y}+cy/z$ | 246.22 | 168.39 | 0.262 | 0.1164 | 0.0864 | 0.3311 | 0.4079 | 0.2992 | 0.295 |
| $a+b/x^2\sqrt{y}+cy/z^2$ | 247.14 | 174.63 | 0.257 | 0.1217 | 0.0937 | 0.2684 | 0.4154 | 0.3038 | 0.269 |
| $a+b/x^2\sqrt{y}+cy/\sqrt{z}$ | 290.67 | 211.03 | -0.028 | 0.1372 | 0.1046 | 0.0711 | 0.4710 | 0.3548 | 0.06 |
| $a+b/x^2\sqrt{y}+cyz$ | 137.33 | 107.14 | 0.771 | 0.0768 | 0.0516 | 0.7090 | 0.2808 | 0.2013 | 0.666 |
| $a+b/x^2\sqrt{y}+cyz^2$ | 159.60 | 121.19 | 0.690 | 0.0828 | 0.0605 | 0.6612 | 0.3082 | 0.2221 | 0.597 |
| $a+b/x^2\sqrt{y}+cy\sqrt{z}$ | 128.26 | 97.10 | 0.800 | 0.0780 | 0.0485 | 0.6996 | 0.2726 | 0.1767 | 0.685 |
| $a+b/x^2\sqrt{y}+cy^2/z$ | 288.66 | 207.92 | -0.014 | 0.1355 | 0.1025 | 0.0933 | 0.4672 | 0.3490 | 0.07 |
| $a+b/x^2\sqrt{y}+cy^2/z^2$ | 262.27 | 183.61 | 0.163 | 0.1259 | 0.0955 | 0.2178 | 0.4341 | 0.3217 | 0.202 |
| $a+b/x^2\sqrt{y}+cy^2/\sqrt{z}$ | 248.73 | 201.82 | 0.247 | 0.1290 | 0.1036 | 0.1777 | 0.4259 | 0.3312 | 0.231 |
| $a+b/x^2\sqrt{y}+cy^2z$ | 149.49 | 113.18 | 0.728 | 0.0832 | 0.0579 | 0.6582 | 0.3023 | 0.2150 | 0.613 |
| $a+b/x^2\sqrt{y}+cy^2z^2$ | 167.32 | 125.69 | 0.659 | 0.0880 | 0.0651 | 0.6180 | 0.3234 | 0.2318 | 0.557 |
| $a+b/x^2\sqrt{y}+cy^2\sqrt{z}$ | 144.15 | 103.42 | 0.747 | 0.0846 | 0.0571 | 0.6466 | 0.2980 | 0.1979 | 0.624 |
| $a+b/x^2\sqrt{y}+c\sqrt{y}/z$ | 210.40 | 145.46 | 0.461 | 0.1047 | 0.0742 | 0.4590 | 0.3611 | 0.2504 | 0.447 |
| $a+b/x^2\sqrt{y}+c\sqrt{y}/z^2$ | 235.66 | 168.14 | 0.324 | 0.1187 | 0.0915 | 0.3040 | 0.4005 | 0.2907 | 0.320 |
| $a+b/x^2\sqrt{y}+c\sqrt{y}/\sqrt{z}$ | 237.64 | 164.04 | 0.313 | 0.1111 | 0.0834 | 0.3908 | 0.3934 | 0.2852 | 0.344 |
| $a+b/x^2\sqrt{y}+c\sqrt{y}z$ | 134.40 | 106.99 | 0.780 | 0.0741 | 0.0482 | 0.7292 | 0.2718 | 0.1906 | 0.687 |
| $a+b/x^2\sqrt{y}+c\sqrt{y}z^2$ | 156.73 | 120.42 | 0.701 | 0.0804 | 0.0580 | 0.6807 | 0.3009 | 0.2158 | 0.616 |
| $a+b/x^2\sqrt{y}+c\sqrt{y}\sqrt{z}$ | 123.34 | 96.24 | 0.815 | 0.0745 | 0.0431 | 0.7259 | 0.2605 | 0.1652 | 0.712 |
| $a+b/x^2\sqrt{y}+c/yz$ | 198.76 | 140.63 | 0.519 | 0.1103 | 0.0842 | 0.3995 | 0.3463 | 0.2489 | 0.492 |
| $a+b/x^2\sqrt{y}+c/yz^2$ | 218.45 | 157.71 | 0.419 | 0.1174 | 0.0910 | 0.3200 | 0.3751 | 0.2752 | 0.404 |
| $a+b/x^2\sqrt{y}+c/y\sqrt{z}$ | 193.08 | 133.59 | 0.546 | 0.1083 | 0.0810 | 0.4204 | 0.3389 | 0.2368 | 0.513 |
| $a+b/x^2\sqrt{y}+cz/y$ | 219.91 | 158.29 | 0.412 | 0.0999 | 0.0787 | 0.5075 | 0.3625 | 0.2661 | 0.443 |
| $a+b/x^2\sqrt{y}+cz^2/y$ | 167.04 | 123.51 | 0.661 | 0.0797 | 0.0600 | 0.6861 | 0.2980 | 0.2152 | 0.624 |
| $a+b/x^2\sqrt{y}+c\sqrt{z}/y$ | 288.41 | 215.56 | -0.012 | 0.1391 | 0.1093 | 0.0447 | 0.4706 | 0.3624 | 0.06 |
| $a+b/x^2\sqrt{y}+c/y^2z$ | 237.93 | 171.47 | 0.311 | 0.1239 | 0.0963 | 0.2416 | 0.3982 | 0.2914 | 0.328 |
| $a+b/x^2\sqrt{y}+c/y^2z^2$ | 242.32 | 173.51 | 0.286 | 0.1256 | 0.0968 | 0.2215 | 0.4051 | 0.2937 | 0.305 |
| $a+b/x^2\sqrt{y}+c/y^2\sqrt{z}$ | 236.29 | 170.36 | 0.321 | 0.1234 | 0.0961 | 0.2487 | 0.3959 | 0.2908 | 0.336 |
| $a+b/x^2\sqrt{y}+cz/y^2$ | 283.89 | 212.92 | 0.019 | 0.1385 | 0.1096 | 0.0524 | 0.4650 | 0.3593 | 0.084 |
| $a+b/x^2\sqrt{y}+cz^2/y^2$ | 214.91 | 157.40 | 0.438 | 0.0973 | 0.0783 | 0.5322 | 0.3537 | 0.2660 | 0.470 |
| $a+b/x^2\sqrt{y}+c\sqrt{z}/y^2$ | 250.57 | 182.86 | 0.236 | 0.1286 | 0.0996 | 0.1830 | 0.4182 | 0.3129 | 0.259 |
| $a+b/x^2\sqrt{y}+c/\sqrt{y}z$ | 176.91 | 123.49 | 0.619 | 0.1010 | 0.0756 | 0.4960 | 0.3188 | 0.2152 | 0.569 |
| $a+b/x^2\sqrt{y}+c/\sqrt{y}z^2$ | 213.94 | 150.89 | 0.443 | 0.1146 | 0.0871 | 0.3513 | 0.3708 | 0.2636 | 0.417 |
| $a+b/x^2\sqrt{y}+c/\sqrt{y}\sqrt{z}$ | 159.94 | 110.50 | 0.689 | 0.0952 | 0.0707 | 0.5521 | 0.2971 | 0.1938 | 0.626 |
| $a+b/x^2\sqrt{y}+cz/\sqrt{y}$ | 162.82 | 125.26 | 0.677 | 0.0789 | 0.0584 | 0.6925 | 0.2910 | 0.2065 | 0.641 |
| $a+b/x^2\sqrt{y}+cz^2/\sqrt{y}$ | 158.35 | 117.03 | 0.695 | 0.0779 | 0.0562 | 0.7001 | 0.2929 | 0.2118 | 0.637 |
| $a+b/x^2\sqrt{y}+c\sqrt{z}/\sqrt{y}$ | 224.16 | 159.34 | 0.389 | 0.1025 | 0.0792 | 0.4812 | 0.3700 | 0.2669 | 0.420 |
| $a+by/x^2+cx/z$ | 267.59 | 184.82 | 0.129 | 0.1261 | 0.0958 | 0.2143 | 0.4413 | 0.3253 | 0.175 |
| $a+by/x^2+cx/z^2$ | 258.43 | 183.15 | 0.187 | 0.1258 | 0.0978 | 0.2186 | 0.4312 | 0.3193 | 0.212 |
| $a+by/x^2+cx/\sqrt{z}$ | 279.38 | 210.85 | 0.050 | 0.1369 | 0.1092 | 0.0752 | 0.4539 | 0.3590 | 0.127 |
| $a+by/x^2+cxz$ | 128.19 | 95.15 | 0.800 | 0.0718 | 0.0494 | 0.7458 | 0.2637 | 0.1909 | 0.705 |
| $a+by/x^2+cxz^2$ | 155.32 | 115.09 | 0.706 | 0.0803 | 0.0595 | 0.6818 | 0.2999 | 0.2186 | 0.619 |
| $a+by/x^2+cx\sqrt{z}$ | 110.01 | 83.03 | 0.853 | 0.0696 | 0.0444 | 0.7609 | 0.2415 | 0.1605 | 0.753 |
| $a+by/x^2+cx^2/z$ | 286.15 | 214.11 | 0.004 | 0.1381 | 0.1099 | 0.0588 | 0.4633 | 0.3630 | 0.091 |
| $a+by/x^2+cx^2/z^2$ | 274.34 | 193.52 | 0.084 | 0.1313 | 0.1013 | 0.1489 | 0.4524 | 0.3374 | 0.133 |
| $a+by/x^2+cx^2/\sqrt{z}$ | 185.31 | 140.13 | 0.582 | 0.1052 | 0.0824 | 0.4530 | 0.3268 | 0.2481 | 0.547 |
| $a+by/x^2+cx^2z$ | 137.98 | 104.55 | 0.768 | 0.0765 | 0.0560 | 0.7113 | 0.2805 | 0.2100 | 0.667 |
| $a+by/x^2+cx^2z^2$ | 161.80 | 123.54 | 0.681 | 0.0846 | 0.0644 | 0.6463 | 0.3126 | 0.2312 | 0.586 |
| $a+by/x^2+cx^2\sqrt{z}$ | 123.42 | 94.31 | 0.815 | 0.0738 | 0.0528 | 0.7312 | 0.2617 | 0.1896 | 0.710 |
| $a+by/x^2+c\sqrt{x}/z$ | 227.09 | 154.51 | 0.373 | 0.1108 | 0.0794 | 0.3936 | 0.3860 | 0.2731 | 0.369 |
| $a+by/x^2+c\sqrt{x}/z^2$ | 243.55 | 173.69 | 0.278 | 0.1211 | 0.0942 | 0.2755 | 0.4111 | 0.3009 | 0.284 |
| $a+by/x^2+c\sqrt{x}/\sqrt{z}$ | 264.40 | 180.19 | 0.149 | 0.1233 | 0.0926 | 0.2492 | 0.4354 | 0.3189 | 0.197 |
| $a+by/x^2+c\sqrt{x}z$ | 128.96 | 98.82 | 0.798 | 0.0711 | 0.0463 | 0.7501 | 0.2612 | 0.1827 | 0.711 |
| $a+by/x^2+c\sqrt{x}z^2$ | 154.20 | 116.69 | 0.711 | 0.0789 | 0.0572 | 0.6930 | 0.2957 | 0.2132 | 0.630 |
| $a+by/x^2+c\sqrt{x}\sqrt{z}$ | 111.92 | 84.43 | 0.848 | 0.0695 | 0.0409 | 0.7613 | 0.2403 | 0.1489 | 0.755 |
| $a+by/x^2+c/xz$ | 217.77 | 156.17 | 0.423 | 0.1167 | 0.0894 | 0.3272 | 0.3693 | 0.2640 | 0.422 |
| $a+by/x^2+c/xz^2$ | 229.10 | 161.83 | 0.361 | 0.1209 | 0.0919 | 0.2787 | 0.3866 | 0.2801 | 0.367 |
| $a+by/x^2+c/x\sqrt{z}$ | 213.37 | 153.78 | 0.446 | 0.1152 | 0.0887 | 0.3452 | 0.3629 | 0.2614 | 0.442 |
| $a+by/x^2+cz/x$ | 214.58 | 151.24 | 0.440 | 0.0982 | 0.0730 | 0.5237 | 0.3600 | 0.2535 | 0.451 |
| $a+by/x^2+cz^2/x$ | 162.59 | 120.61 | 0.678 | 0.0796 | 0.0589 | 0.6868 | 0.2958 | 0.2149 | 0.629 |
| $a+by/x^2+c\sqrt{z}/x$ | 280.81 | 209.47 | 0.041 | 0.1374 | 0.1090 | 0.0675 | 0.4580 | 0.3544 | 0.111 |
| $a+by/x^2+c/x^2z$ | 270.84 | 194.42 | 0.108 | 0.1341 | 0.1038 | 0.1127 | 0.4440 | 0.3296 | 0.165 |
| $a+by/x^2+c/x^2z^2$ | 262.32 | 183.95 | 0.163 | 0.1315 | 0.1002 | 0.1462 | 0.4318 | 0.3128 | 0.210 |
| $a+by/x^2+c/x^2\sqrt{z}$ | 283.87 | 209.71 | 0.020 | 0.1376 | 0.1084 | 0.0654 | 0.4626 | 0.3543 | 0.093 |
| $a+by/x^2+cz/x^2$ | 205.72 | 147.55 | 0.485 | 0.1113 | 0.0856 | 0.3885 | 0.3470 | 0.2484 | 0.490 |
| $a+by/x^2+cz^2/x^2$ | 189.96 | 130.55 | 0.561 | 0.1042 | 0.0784 | 0.4638 | 0.3267 | 0.2282 | 0.548 |

(continued on next page)

**Table 4 – continued from previous page**

| Functional form | $T_{eff}$ (K) | | | Radius ($R_\odot$) | | | log (L/$L_\odot$) | | |
|---|---|---|---|---|---|---|---|---|---|
| | RMSE | MAD | $R^2_{ap}$ | RMSE | MAD | $R^2_{ap}$ | RMSE | MAD | $R^2_{ap}$ |
| $a+by/x^2+c\sqrt{z}/x^2$ | 190.44 | 137.46 | 0.559 | 0.1058 | 0.0811 | 0.4476 | 0.3229 | 0.2277 | 0.558 |
| $a+by/x^2+c/\sqrt{x}z$ | 180.91 | 129.90 | 0.602 | 0.1030 | 0.0780 | 0.4763 | 0.3210 | 0.2243 | 0.564 |
| $a+by/x^2+c/\sqrt{x}z^2$ | 211.71 | 152.64 | 0.455 | 0.1142 | 0.0880 | 0.3560 | 0.3655 | 0.2642 | 0.434 |
| $a+by/x^2+c/\sqrt{x}\sqrt{z}$ | 167.51 | 116.67 | 0.659 | 0.0983 | 0.0738 | 0.5228 | 0.3021 | 0.2049 | 0.613 |
| $a+by/x^2+cz/\sqrt{x}$ | 168.30 | 126.19 | 0.655 | 0.0815 | 0.0572 | 0.6720 | 0.3020 | 0.2099 | 0.614 |
| $a+by/x^2+cz^2/\sqrt{x}$ | 159.76 | 120.36 | 0.689 | 0.0790 | 0.0575 | 0.6921 | 0.2960 | 0.2163 | 0.629 |
| $a+by/x^2+c\sqrt{z}/\sqrt{x}$ | 250.12 | 165.95 | 0.239 | 0.1144 | 0.0835 | 0.3541 | 0.4122 | 0.2926 | 0.280 |
| $a+by/x^2+cy/z$ | 245.11 | 167.94 | 0.269 | 0.1158 | 0.0858 | 0.3382 | 0.4055 | 0.2972 | 0.303 |
| $a+by/x^2+cy/z^2$ | 246.19 | 174.19 | 0.263 | 0.1211 | 0.0934 | 0.2755 | 0.4131 | 0.3021 | 0.277 |
| $a+by/x^2+cy/\sqrt{z}$ | 289.48 | 210.03 | -0.020 | 0.1363 | 0.1039 | 0.0827 | 0.4681 | 0.3528 | 0.072 |
| $a+by/x^2+cyz$ | 137.34 | 107.24 | 0.771 | 0.0767 | 0.0515 | 0.7099 | 0.2803 | 0.2008 | 0.667 |
| $a+by/x^2+cyz^2$ | 159.38 | 121.13 | 0.691 | 0.0826 | 0.0604 | 0.6631 | 0.3073 | 0.2214 | 0.600 |
| $a+by/x^2+cy\sqrt{z}$ | 128.48 | 97.41 | 0.799 | 0.0780 | 0.0485 | 0.7000 | 0.2723 | 0.1765 | 0.686 |
| $a+by/x^2+cy^2/z$ | 287.43 | 207.28 | -0.005 | 0.1347 | 0.1018 | 0.1043 | 0.4644 | 0.3470 | 0.086 |
| $a+by/x^2+cy^2/z^2$ | 261.19 | 183.09 | 0.170 | 0.1252 | 0.0951 | 0.2259 | 0.4317 | 0.3200 | 0.210 |
| $a+by/x^2+cy^2/\sqrt{z}$ | 249.00 | 202.27 | 0.246 | 0.1288 | 0.1037 | 0.1812 | 0.4251 | 0.3318 | 0.234 |
| $a+by/x^2+cy^2z$ | 149.41 | 113.23 | 0.728 | 0.0830 | 0.0578 | 0.6596 | 0.3016 | 0.2144 | 0.615 |
| $a+by/x^2+cy^2z^2$ | 167.04 | 125.59 | 0.661 | 0.0877 | 0.0650 | 0.6204 | 0.3222 | 0.2314 | 0.560 |
| $a+by/x^2+cy^2\sqrt{z}$ | 144.24 | 103.62 | 0.747 | 0.0845 | 0.0571 | 0.6476 | 0.2974 | 0.1975 | 0.625 |
| $a+by/x^2+c\sqrt{y}/z$ | 209.68 | 145.27 | 0.465 | 0.1043 | 0.0741 | 0.4634 | 0.3594 | 0.2491 | 0.453 |
| $a+by/x^2+c\sqrt{y}/z^2$ | 234.84 | 167.93 | 0.329 | 0.1182 | 0.0912 | 0.3103 | 0.3985 | 0.2895 | 0.327 |
| $a+by/x^2+c\sqrt{y}/\sqrt{z}$ | 236.49 | 163.44 | 0.320 | 0.1105 | 0.0830 | 0.3975 | 0.3910 | 0.2834 | 0.352 |
| $a+by/x^2+c\sqrt{y}z$ | 134.39 | 107.07 | 0.780 | 0.0739 | 0.0481 | 0.7300 | 0.2713 | 0.1901 | 0.688 |
| $a+by/x^2+c\sqrt{y}z^2$ | 156.54 | 120.35 | 0.702 | 0.0802 | 0.0579 | 0.6824 | 0.3000 | 0.2151 | 0.619 |
| $a+by/x^2+c\sqrt{y}\sqrt{z}$ | 123.52 | 96.52 | 0.814 | 0.0745 | 0.0431 | 0.7262 | 0.2603 | 0.1651 | 0.713 |
| $a+by/x^2+c/yz$ | 199.34 | 140.50 | 0.517 | 0.1102 | 0.0839 | 0.4002 | 0.3463 | 0.2481 | 0.492 |
| $a+by/x^2+c/yz^2$ | 218.27 | 157.12 | 0.420 | 0.1170 | 0.0904 | 0.3240 | 0.3739 | 0.2737 | 0.408 |
| $a+by/x^2+c/y\sqrt{z}$ | 194.28 | 134.08 | 0.541 | 0.1085 | 0.0809 | 0.4187 | 0.3397 | 0.2367 | 0.511 |
| $a+by/x^2+cz/y$ | 218.40 | 157.16 | 0.420 | 0.0992 | 0.0782 | 0.5145 | 0.3596 | 0.2644 | 0.452 |
| $a+by/x^2+cz^2/y$ | 166.55 | 123.20 | 0.662 | 0.0795 | 0.0599 | 0.6883 | 0.2968 | 0.2144 | 0.627 |
| $a+by/x^2+c\sqrt{z}/y$ | 288.15 | 215.18 | -0.010 | 0.1384 | 0.1087 | 0.0545 | 0.4688 | 0.3612 | 0.069 |
| $a+by/x^2+c/y^2z$ | 238.62 | 171.28 | 0.307 | 0.1238 | 0.0959 | 0.2428 | 0.3982 | 0.2905 | 0.328 |
| $a+by/x^2+c/y^2z^2$ | 242.26 | 173.21 | 0.286 | 0.1252 | 0.0964 | 0.2259 | 0.4040 | 0.2925 | 0.308 |
| $a+by/x^2+c/y^2\sqrt{z}$ | 237.58 | 170.42 | 0.313 | 0.1235 | 0.0959 | 0.2474 | 0.3968 | 0.2902 | 0.333 |
| $a+by/x^2+cz/y^2$ | 284.90 | 213.87 | 0.012 | 0.1381 | 0.1095 | 0.0577 | 0.4650 | 0.3589 | 0.084 |
| $a+by/x^2+cz^2/y^2$ | 212.84 | 155.93 | 0.449 | 0.0964 | 0.0776 | 0.5413 | 0.3500 | 0.2639 | 0.481 |
| $a+by/x^2+c\sqrt{z}/y^2$ | 253.40 | 184.12 | 0.219 | 0.1292 | 0.0998 | 0.1763 | 0.4211 | 0.3142 | 0.249 |
| $a+by/x^2+c/\sqrt{y}z$ | 177.07 | 123.33 | 0.619 | 0.1009 | 0.0754 | 0.4974 | 0.3183 | 0.2143 | 0.571 |
| $a+by/x^2+c/\sqrt{y}z^2$ | 213.53 | 151.20 | 0.445 | 0.1142 | 0.0869 | 0.3558 | 0.3693 | 0.2634 | 0.422 |
| $a+by/x^2+c/\sqrt{y}\sqrt{z}$ | 160.57 | 110.65 | 0.686 | 0.0953 | 0.0706 | 0.5518 | 0.2973 | 0.1934 | 0.626 |
| $a+by/x^2+cz/\sqrt{y}$ | 162.38 | 124.96 | 0.679 | 0.0787 | 0.0583 | 0.6943 | 0.2899 | 0.2057 | 0.644 |
| $a+by/x^2+cz^2/\sqrt{y}$ | 158.07 | 116.88 | 0.696 | 0.0777 | 0.0561 | 0.7017 | 0.2919 | 0.2109 | 0.639 |
| $a+by/x^2+c\sqrt{z}/\sqrt{y}$ | 222.82 | 158.38 | 0.396 | 0.1019 | 0.0788 | 0.4878 | 0.3674 | 0.2654 | 0.428 |
| $a+by^2/x^2+cx/z$ | 267.77 | 183.91 | 0.128 | 0.1259 | 0.0952 | 0.2174 | 0.4406 | 0.3245 | 0.178 |
| $a+by^2/x^2+cx/z^2$ | 258.33 | 182.61 | 0.188 | 0.1254 | 0.0973 | 0.2232 | 0.4302 | 0.3178 | 0.216 |
| $a+by^2/x^2+cx/\sqrt{z}$ | 279.37 | 211.01 | 0.050 | 0.1366 | 0.1091 | 0.0791 | 0.4532 | 0.3585 | 0.130 |
| $a+by^2/x^2+cxz$ | 128.19 | 95.26 | 0.800 | 0.0716 | 0.0495 | 0.7467 | 0.2633 | 0.1903 | 0.706 |
| $a+by^2/x^2+cxz^2$ | 155.31 | 114.85 | 0.707 | 0.0800 | 0.0595 | 0.6837 | 0.2992 | 0.2175 | 0.621 |
| $a+by^2/x^2+cx\sqrt{z}$ | 110.11 | 83.15 | 0.852 | 0.0696 | 0.0445 | 0.7610 | 0.2414 | 0.1605 | 0.753 |
| $a+by^2/x^2+cx^2/z$ | 286.00 | 213.77 | 0.005 | 0.1377 | 0.1096 | 0.0634 | 0.4623 | 0.3616 | 0.094 |
| $a+by^2/x^2+cx^2/z^2$ | 274.23 | 193.02 | 0.085 | 0.1309 | 0.1007 | 0.1535 | 0.4513 | 0.3359 | 0.137 |
| $a+by^2/x^2+cx^2/\sqrt{z}$ | 185.66 | 141.20 | 0.581 | 0.1053 | 0.0826 | 0.4527 | 0.3271 | 0.2491 | 0.547 |
| $a+by^2/x^2+cx^2z$ | 137.99 | 104.47 | 0.768 | 0.0763 | 0.0561 | 0.7127 | 0.2800 | 0.2094 | 0.668 |
| $a+by^2/x^2+cx^2z^2$ | 161.77 | 123.29 | 0.682 | 0.0844 | 0.0645 | 0.6485 | 0.3119 | 0.2315 | 0.588 |
| $a+by^2/x^2+cx^2\sqrt{z}$ | 123.41 | 94.42 | 0.815 | 0.0737 | 0.0528 | 0.7320 | 0.2614 | 0.1893 | 0.710 |
| $a+by^2/x^2+c\sqrt{x}/z$ | 227.33 | 153.77 | 0.371 | 0.1105 | 0.0792 | 0.3966 | 0.3854 | 0.2726 | 0.371 |
| $a+by^2/x^2+c\sqrt{x}/z^2$ | 243.34 | 173.32 | 0.280 | 0.1207 | 0.0937 | 0.2807 | 0.4098 | 0.2995 | 0.289 |
| $a+by^2/x^2+c\sqrt{x}/\sqrt{z}$ | 264.91 | 179.10 | 0.146 | 0.1232 | 0.0923 | 0.2505 | 0.4351 | 0.3180 | 0.198 |
| $a+by^2/x^2+c\sqrt{x}z$ | 128.97 | 98.91 | 0.798 | 0.0710 | 0.0464 | 0.7509 | 0.2608 | 0.1822 | 0.712 |
| $a+by^2/x^2+c\sqrt{x}z^2$ | 154.19 | 116.46 | 0.711 | 0.0786 | 0.0572 | 0.6948 | 0.2950 | 0.2122 | 0.631 |
| $a+by^2/x^2+c\sqrt{x}\sqrt{z}$ | 112.13 | 84.67 | 0.847 | 0.0696 | 0.0411 | 0.7611 | 0.2403 | 0.1490 | 0.755 |
| $a+by^2/x^2+c/xz$ | 224.26 | 160.26 | 0.388 | 0.1187 | 0.0912 | 0.3047 | 0.3784 | 0.2718 | 0.393 |
| $a+by^2/x^2+c/xz^2$ | 231.28 | 163.95 | 0.349 | 0.1212 | 0.0923 | 0.2747 | 0.3886 | 0.2820 | 0.360 |
| $a+by^2/x^2+c/x\sqrt{z}$ | 224.23 | 160.11 | 0.388 | 0.1187 | 0.0917 | 0.3044 | 0.3790 | 0.2738 | 0.391 |
| $a+by^2/x^2+cz/x$ | 228.85 | 150.71 | 0.363 | 0.1033 | 0.0756 | 0.4735 | 0.3742 | 0.2565 | 0.407 |
| $a+by^2/x^2+cz^2/x$ | 163.26 | 117.52 | 0.676 | 0.0787 | 0.0587 | 0.6940 | 0.2936 | 0.2120 | 0.635 |
| $a+by^2/x^2+c\sqrt{z}/x$ | 284.91 | 213.01 | 0.012 | 0.1378 | 0.1092 | 0.0623 | 0.4640 | 0.3578 | 0.088 |
| $a+by^2/x^2+c/x^2z$ | 281.50 | 208.79 | 0.036 | 0.1368 | 0.1081 | 0.0760 | 0.4599 | 0.3528 | 0.104 |
| $a+by^2/x^2+c/x^2z^2$ | 268.73 | 192.84 | 0.121 | 0.1332 | 0.1036 | 0.1235 | 0.4412 | 0.3285 | 0.175 |
| $a+by^2/x^2+c/x^2\sqrt{z}$ | 288.98 | 214.50 | -0.016 | 0.1380 | 0.1086 | 0.0593 | 0.4688 | 0.3591 | 0.069 |
| $a+by^2/x^2+cz/x^2$ | 237.23 | 174.81 | 0.315 | 0.1156 | 0.0877 | 0.3406 | 0.3763 | 0.2853 | 0.400 |
| $a+by^2/x^2+cz^2/x^2$ | 193.59 | 139.15 | 0.544 | 0.0995 | 0.0759 | 0.5110 | 0.3140 | 0.2297 | 0.582 |
| $a+by^2/x^2+c\sqrt{z}/x^2$ | 262.97 | 186.21 | 0.159 | 0.1248 | 0.0936 | 0.2314 | 0.4173 | 0.3058 | 0.262 |
| $a+by^2/x^2+c/\sqrt{x}z$ | 183.38 | 131.20 | 0.591 | 0.1035 | 0.0782 | 0.4706 | 0.3235 | 0.2267 | 0.557 |
| $a+by^2/x^2+c/\sqrt{x}z^2$ | 211.94 | 153.34 | 0.453 | 0.1139 | 0.0880 | 0.3598 | 0.3644 | 0.2642 | 0.437 |
| $a+by^2/x^2+c/\sqrt{x}\sqrt{z}$ | 172.78 | 119.11 | 0.637 | 0.0999 | 0.0747 | 0.5068 | 0.3090 | 0.2091 | 0.595 |
| $a+by^2/x^2+cz/\sqrt{x}$ | 169.45 | 125.00 | 0.651 | 0.0812 | 0.0573 | 0.6746 | 0.3014 | 0.2071 | 0.615 |
| $a+by^2/x^2+cz^2/\sqrt{x}$ | 159.78 | 119.35 | 0.689 | 0.0786 | 0.0575 | 0.6951 | 0.2950 | 0.2146 | 0.631 |
| $a+by^2/x^2+c\sqrt{z}/\sqrt{x}$ | 253.59 | 164.84 | 0.218 | 0.1154 | 0.0841 | 0.3422 | 0.4147 | 0.2924 | 0.271 |
| $a+by^2/x^2+cy/z$ | 246.33 | 168.25 | 0.262 | 0.1162 | 0.0858 | 0.3333 | 0.4069 | 0.2968 | 0.298 |
| $a+by^2/x^2+cy/z^2$ | 246.35 | 173.63 | 0.262 | 0.1209 | 0.0929 | 0.2780 | 0.4126 | 0.3008 | 0.279 |
| $a+by^2/x^2+cy/\sqrt{z}$ | 289.49 | 209.79 | -0.020 | 0.1363 | 0.1037 | 0.0830 | 0.4676 | 0.3522 | 0.074 |
| $a+by^2/x^2+cyz$ | 137.34 | 107.34 | 0.770 | 0.0763 | 0.0515 | 0.7122 | 0.2793 | 0.2002 | 0.670 |
| $a+by^2/x^2+cyz^2$ | 159.28 | 120.90 | 0.691 | 0.0823 | 0.0604 | 0.6659 | 0.3062 | 0.2204 | 0.603 |
| $a+by^2/x^2+cy\sqrt{z}$ | 129.01 | 98.06 | 0.798 | 0.0778 | 0.0486 | 0.7015 | 0.2716 | 0.1762 | 0.688 |
| $a+by^2/x^2+cy^2/z$ | 287.65 | 207.12 | -0.007 | 0.1348 | 0.1017 | 0.1031 | 0.4643 | 0.3465 | 0.087 |
| $a+by^2/x^2+cy^2/z^2$ | 261.69 | 182.35 | 0.167 | 0.1252 | 0.0946 | 0.2258 | 0.4318 | 0.3193 | 0.210 |
| $a+by^2/x^2+cy^2/\sqrt{z}$ | 249.28 | 202.74 | 0.244 | 0.1283 | 0.1038 | 0.1874 | 0.4235 | 0.3326 | 0.240 |
| $a+by^2/x^2+cy^2z$ | 149.31 | 113.26 | 0.729 | 0.0826 | 0.0578 | 0.6629 | 0.3003 | 0.2136 | 0.618 |

(continued on next page)

**Table 4 – continued from previous page**

| Functional form | $T_{eff}$ (K) | | | Radius ($R_{\odot}$) | | | log (L/$L_{\odot}$) | | |
|---|---|---|---|---|---|---|---|---|---|
| | RMSE | MAD | $R^2_{ap}$ | RMSE | MAD | $R^2_{ap}$ | RMSE | MAD | $R^2_{ap}$ |
| $a+by^2/x^2+cy^2z^2$ | 166.86 | 125.34 | 0.661 | 0.0873 | 0.0650 | 0.6239 | 0.3210 | 0.2313 | 0.563 |
| $a+by^2/x^2+cy^2\sqrt{z}$ | 144.39 | 103.97 | 0.746 | 0.0841 | 0.0571 | 0.6507 | 0.2962 | 0.1969 | 0.628 |
| $a+by^2/x^2+c\sqrt{y}/z$ | 210.27 | 145.77 | 0.462 | 0.1043 | 0.0744 | 0.4633 | 0.3597 | 0.2489 | 0.452 |
| $a+by^2/x^2+c\sqrt{y}/z^2$ | 234.70 | 167.60 | 0.330 | 0.1178 | 0.0908 | 0.3147 | 0.3974 | 0.2885 | 0.331 |
| $a+by^2/x^2+c\sqrt{y}/\sqrt{z}$ | 238.21 | 163.92 | 0.310 | 0.1112 | 0.0836 | 0.3898 | 0.3933 | 0.2846 | 0.345 |
| $a+by^2/x^2+c\sqrt{y}z$ | 134.39 | 107.12 | 0.780 | 0.0737 | 0.0482 | 0.7320 | 0.2704 | 0.1895 | 0.690 |
| $a+by^2/x^2+c\sqrt{y}z^2$ | 156.47 | 120.11 | 0.702 | 0.0799 | 0.0579 | 0.6848 | 0.2991 | 0.2142 | 0.621 |
| $a+by^2/x^2+c\sqrt{y}\sqrt{z}$ | 123.91 | 97.05 | 0.813 | 0.0743 | 0.0433 | 0.7275 | 0.2596 | 0.1650 | 0.714 |
| $a+by^2/x^2+c/yz$ | 200.33 | 140.78 | 0.512 | 0.1100 | 0.0836 | 0.4022 | 0.3459 | 0.2479 | 0.493 |
| $a+by^2/x^2+c/yz^2$ | 217.92 | 157.57 | 0.422 | 0.1164 | 0.0902 | 0.3313 | 0.3716 | 0.2730 | 0.415 |
| $a+by^2/x^2+c/y\sqrt{z}$ | 196.69 | 135.50 | 0.529 | 0.1088 | 0.0810 | 0.4158 | 0.3413 | 0.2378 | 0.507 |
| $a+by^2/x^2+cz/y$ | 221.62 | 157.06 | 0.402 | 0.1006 | 0.0787 | 0.5003 | 0.3640 | 0.2663 | 0.439 |
| $a+by^2/x^2+cz^2/y$ | 167.04 | 123.03 | 0.661 | 0.0794 | 0.0603 | 0.6885 | 0.2969 | 0.2143 | 0.627 |
| $a+by^2/x^2+c\sqrt{z}/y$ | 287.97 | 214.95 | -0.009 | 0.1380 | 0.1085 | 0.0592 | 0.4676 | 0.3602 | 0.074 |
| $a+by^2/x^2+c/y^2z$ | 239.46 | 172.45 | 0.302 | 0.1236 | 0.0961 | 0.2453 | 0.3979 | 0.2915 | 0.329 |
| $a+by^2/x^2+c/y^2z^2$ | 242.11 | 173.88 | 0.287 | 0.1247 | 0.0963 | 0.2327 | 0.4021 | 0.2924 | 0.315 |
| $a+by^2/x^2+c/y^2\sqrt{z}$ | 239.26 | 171.97 | 0.304 | 0.1235 | 0.0962 | 0.2463 | 0.3979 | 0.2921 | 0.329 |
| $a+by^2/x^2+cz/y^2$ | 285.31 | 214.10 | 0.010 | 0.1378 | 0.1093 | 0.0621 | 0.4645 | 0.3590 | 0.086 |
| $a+by^2/x^2+cz^2/y^2$ | 216.81 | 156.90 | 0.428 | 0.0980 | 0.0784 | 0.5256 | 0.3549 | 0.2661 | 0.466 |
| $a+by^2/x^2+c\sqrt{z}/y^2$ | 256.72 | 185.48 | 0.198 | 0.1297 | 0.0999 | 0.1690 | 0.4247 | 0.3161 | 0.236 |
| $a+by^2/x^2+c/\sqrt{y}z$ | 177.33 | 123.95 | 0.617 | 0.1005 | 0.0751 | 0.5011 | 0.3171 | 0.2143 | 0.574 |
| $a+by^2/x^2+c/\sqrt{y}z^2$ | 212.97 | 151.66 | 0.448 | 0.1136 | 0.0865 | 0.3632 | 0.3670 | 0.2629 | 0.429 |
| $a+by^2/x^2+c/\sqrt{y}\sqrt{z}$ | 162.11 | 111.34 | 0.680 | 0.0953 | 0.0703 | 0.5515 | 0.2976 | 0.1939 | 0.625 |
| $a+by^2/x^2+cz/\sqrt{y}$ | 163.16 | 124.64 | 0.676 | 0.0788 | 0.0588 | 0.6933 | 0.2904 | 0.2073 | 0.643 |
| $a+by^2/x^2+cz^2/\sqrt{y}$ | 158.18 | 116.58 | 0.696 | 0.0775 | 0.0561 | 0.7031 | 0.2915 | 0.2096 | 0.640 |
| $a+by^2/x^2+c\sqrt{z}/\sqrt{y}$ | 225.59 | 158.18 | 0.381 | 0.1031 | 0.0797 | 0.4752 | 0.3712 | 0.2680 | 0.416 |
| $a+b\sqrt{y}/x^2+cx/z$ | 268.16 | 185.26 | 0.125 | 0.1265 | 0.0961 | 0.2099 | 0.4425 | 0.3261 | 0.170 |
| $a+b\sqrt{y}/x^2+cx/z^2$ | 258.85 | 183.37 | 0.185 | 0.1261 | 0.0980 | 0.2152 | 0.4322 | 0.3200 | 0.208 |
| $a+b\sqrt{y}/x^2+cx/\sqrt{z}$ | 279.37 | 210.66 | 0.050 | 0.1370 | 0.1093 | 0.0728 | 0.4543 | 0.3591 | 0.126 |
| $a+b\sqrt{y}/x^2+cxz$ | 128.18 | 95.10 | 0.800 | 0.0718 | 0.0494 | 0.7456 | 0.2638 | 0.1911 | 0.705 |
| $a+b\sqrt{y}/x^2+cxz^2$ | 155.38 | 115.12 | 0.706 | 0.0804 | 0.0595 | 0.6811 | 0.3002 | 0.2189 | 0.618 |
| $a+b\sqrt{y}/x^2+cx\sqrt{z}$ | 109.98 | 82.98 | 0.853 | 0.0696 | 0.0443 | 0.7609 | 0.2415 | 0.1605 | 0.753 |
| $a+b\sqrt{y}/x^2+cx^2/z$ | 286.41 | 214.19 | 0.002 | 0.1383 | 0.1100 | 0.0553 | 0.4640 | 0.3635 | 0.088 |
| $a+b\sqrt{y}/x^2+cx^2/z^2$ | 274.81 | 193.77 | 0.081 | 0.1316 | 0.1015 | 0.1449 | 0.4534 | 0.3381 | 0.129 |
| $a+b\sqrt{y}/x^2+cx^2/\sqrt{z}$ | 185.14 | 139.79 | 0.583 | 0.1052 | 0.0823 | 0.4532 | 0.3267 | 0.2478 | 0.548 |
| $a+b\sqrt{y}/x^2+cx^2z$ | 138.00 | 104.55 | 0.768 | 0.0765 | 0.0560 | 0.7110 | 0.2807 | 0.2102 | 0.666 |
| $a+b\sqrt{y}/x^2+cx^2z^2$ | 161.88 | 123.60 | 0.681 | 0.0847 | 0.0645 | 0.6455 | 0.3130 | 0.2313 | 0.585 |
| $a+b\sqrt{y}/x^2+cx^2\sqrt{z}$ | 123.40 | 94.27 | 0.815 | 0.0738 | 0.0528 | 0.7310 | 0.2618 | 0.1897 | 0.710 |
| $a+b\sqrt{y}/x^2+c\sqrt{x}/z$ | 227.51 | 154.81 | 0.370 | 0.1111 | 0.0797 | 0.3908 | 0.3870 | 0.2738 | 0.365 |
| $a+b\sqrt{y}/x^2+c\sqrt{x}/z^2$ | 243.94 | 173.82 | 0.276 | 0.1214 | 0.0943 | 0.2724 | 0.4120 | 0.3017 | 0.281 |
| $a+b\sqrt{y}/x^2+c\sqrt{x}/\sqrt{z}$ | 265.10 | 180.82 | 0.145 | 0.1237 | 0.0929 | 0.2441 | 0.4368 | 0.3200 | 0.191 |
| $a+b\sqrt{y}/x^2+c\sqrt{x}z$ | 128.94 | 98.78 | 0.798 | 0.0712 | 0.0463 | 0.7499 | 0.2614 | 0.1829 | 0.711 |
| $a+b\sqrt{y}/x^2+c\sqrt{x}z^2$ | 154.25 | 116.72 | 0.710 | 0.0789 | 0.0573 | 0.6924 | 0.2960 | 0.2135 | 0.629 |
| $a+b\sqrt{y}/x^2+c\sqrt{x}\sqrt{z}$ | 111.86 | 84.32 | 0.848 | 0.0695 | 0.0408 | 0.7614 | 0.2403 | 0.1489 | 0.755 |
| $a+b\sqrt{y}/x^2+c/xz$ | 215.64 | 154.93 | 0.434 | 0.1161 | 0.0890 | 0.3342 | 0.3667 | 0.2622 | 0.430 |
| $a+b\sqrt{y}/x^2+c/xz^2$ | 228.30 | 161.60 | 0.366 | 0.1207 | 0.0920 | 0.2802 | 0.3859 | 0.2803 | 0.369 |
| $a+b\sqrt{y}/x^2+c/x\sqrt{z}$ | 209.96 | 151.56 | 0.464 | 0.1141 | 0.0878 | 0.3572 | 0.3583 | 0.2579 | 0.456 |
| $a+b\sqrt{y}/x^2+cz/x$ | 218.06 | 155.78 | 0.421 | 0.0999 | 0.0744 | 0.5069 | 0.3660 | 0.2619 | 0.432 |
| $a+b\sqrt{y}/x^2+cz^2/x$ | 163.53 | 121.55 | 0.675 | 0.0801 | 0.0591 | 0.6829 | 0.2975 | 0.2161 | 0.625 |
| $a+b\sqrt{y}/x^2+c\sqrt{z}/x$ | 276.76 | 205.90 | 0.068 | 0.1367 | 0.1081 | 0.0773 | 0.4525 | 0.3501 | 0.132 |
| $a+b\sqrt{y}/x^2+c/x^2z$ | 262.20 | 183.94 | 0.164 | 0.1315 | 0.1001 | 0.1458 | 0.4317 | 0.3127 | 0.210 |
| $a+b\sqrt{y}/x^2+c/x^2z^2$ | 258.98 | 182.22 | 0.184 | 0.1306 | 0.0998 | 0.1580 | 0.4273 | 0.3098 | 0.226 |
| $a+b\sqrt{y}/x^2+c/x^2\sqrt{z}$ | 269.79 | 192.91 | 0.114 | 0.1338 | 0.1031 | 0.1159 | 0.4426 | 0.3271 | 0.170 |
| $a+b\sqrt{y}/x^2+cz/x^2$ | 226.65 | 163.52 | 0.375 | 0.1191 | 0.0926 | 0.2997 | 0.3796 | 0.2776 | 0.390 |
| $a+b\sqrt{y}/x^2+cz^2/x^2$ | 203.73 | 142.12 | 0.495 | 0.1095 | 0.0831 | 0.4079 | 0.3479 | 0.2498 | 0.487 |
| $a+b\sqrt{y}/x^2+c\sqrt{z}/x^2$ | 222.55 | 162.01 | 0.397 | 0.1180 | 0.0918 | 0.3125 | 0.3734 | 0.2733 | 0.409 |
| $a+b\sqrt{y}/x^2+c/\sqrt{x}z$ | 180.21 | 129.55 | 0.605 | 0.1028 | 0.0780 | 0.4778 | 0.3203 | 0.2240 | 0.565 |
| $a+b\sqrt{y}/x^2+c/\sqrt{x}z^2$ | 211.61 | 152.38 | 0.455 | 0.1143 | 0.0881 | 0.3550 | 0.3657 | 0.2642 | 0.433 |
| $a+b\sqrt{y}/x^2+c/\sqrt{x}\sqrt{z}$ | 166.22 | 116.08 | 0.664 | 0.0979 | 0.0736 | 0.5263 | 0.3006 | 0.2041 | 0.617 |
| $a+b\sqrt{y}/x^2+cz/\sqrt{x}$ | 168.84 | 126.87 | 0.653 | 0.0818 | 0.0574 | 0.6696 | 0.3031 | 0.2109 | 0.611 |
| $a+b\sqrt{y}/x^2+cz^2/\sqrt{x}$ | 159.96 | 120.61 | 0.689 | 0.0791 | 0.0576 | 0.6909 | 0.2965 | 0.2168 | 0.627 |
| $a+b\sqrt{y}/x^2+c\sqrt{z}/\sqrt{x}$ | 251.80 | 167.74 | 0.229 | 0.1153 | 0.0845 | 0.3440 | 0.4152 | 0.2957 | 0.270 |
| $a+b\sqrt{y}/x^2+cy/z$ | 245.43 | 168.10 | 0.267 | 0.1160 | 0.0860 | 0.3359 | 0.4063 | 0.2979 | 0.301 |
| $a+b\sqrt{y}/x^2+cy/z^2$ | 246.53 | 174.40 | 0.261 | 0.1214 | 0.0935 | 0.2727 | 0.4140 | 0.3028 | 0.274 |
| $a+b\sqrt{y}/x^2+cy/\sqrt{z}$ | 289.93 | 210.43 | -0.023 | 0.1366 | 0.1042 | 0.0784 | 0.4692 | 0.3536 | 0.067 |
| $a+b\sqrt{y}/x^2+cyz$ | 137.34 | 107.20 | 0.771 | 0.0767 | 0.0515 | 0.7095 | 0.2805 | 0.2010 | 0.667 |
| $a+b\sqrt{y}/x^2+cyz^2$ | 159.46 | 121.17 | 0.691 | 0.0827 | 0.0605 | 0.6623 | 0.3076 | 0.2217 | 0.599 |
| $a+b\sqrt{y}/x^2+cy\sqrt{z}$ | 128.38 | 97.27 | 0.799 | 0.0780 | 0.0485 | 0.6998 | 0.2725 | 0.1766 | 0.685 |
| $a+b\sqrt{y}/x^2+cy^2/z$ | 287.88 | 207.55 | -0.008 | 0.1350 | 0.1021 | 0.1003 | 0.4654 | 0.3478 | 0.082 |
| $a+b\sqrt{y}/x^2+cy^2/z^2$ | 261.56 | 183.35 | 0.168 | 0.1255 | 0.0953 | 0.2229 | 0.4325 | 0.3207 | 0.207 |
| $a+b\sqrt{y}/x^2+cy^2/\sqrt{z}$ | 248.88 | 202.08 | 0.246 | 0.1289 | 0.1036 | 0.1795 | 0.4255 | 0.3316 | 0.233 |
| $a+b\sqrt{y}/x^2+cy^2z$ | 149.45 | 113.22 | 0.728 | 0.0831 | 0.0579 | 0.6590 | 0.3019 | 0.2147 | 0.614 |
| $a+b\sqrt{y}/x^2+cy^2z^2$ | 167.14 | 125.64 | 0.660 | 0.0878 | 0.0651 | 0.6193 | 0.3227 | 0.2315 | 0.559 |
| $a+b\sqrt{y}/x^2+cy^2\sqrt{z}$ | 144.20 | 103.53 | 0.747 | 0.0845 | 0.0571 | 0.6471 | 0.2977 | 0.1976 | 0.625 |
| $a+b\sqrt{y}/x^2+c\sqrt{y}/z$ | 209.90 | 145.32 | 0.464 | 0.1044 | 0.0741 | 0.4617 | 0.3600 | 0.2495 | 0.451 |
| $a+b\sqrt{y}/x^2+c\sqrt{y}/z^2$ | 235.15 | 168.04 | 0.327 | 0.1184 | 0.0914 | 0.3077 | 0.3993 | 0.2900 | 0.324 |
| $a+b\sqrt{y}/x^2+c\sqrt{y}/\sqrt{z}$ | 236.79 | 163.65 | 0.318 | 0.1106 | 0.0831 | 0.3956 | 0.3917 | 0.2840 | 0.350 |
| $a+b\sqrt{y}/x^2+c\sqrt{y}z$ | 134.40 | 107.04 | 0.780 | 0.0740 | 0.0481 | 0.7296 | 0.2715 | 0.1903 | 0.688 |
| $a+b\sqrt{y}/x^2+c\sqrt{y}z^2$ | 156.61 | 120.40 | 0.702 | 0.0803 | 0.0580 | 0.6817 | 0.3004 | 0.2154 | 0.618 |
| $a+b\sqrt{y}/x^2+c\sqrt{y}\sqrt{z}$ | 123.44 | 96.40 | 0.815 | 0.0745 | 0.0431 | 0.7260 | 0.2604 | 0.1651 | 0.713 |
| $a+b\sqrt{y}/x^2+c/yz$ | 199.04 | 140.58 | 0.518 | 0.1103 | 0.0841 | 0.3998 | 0.3463 | 0.2485 | 0.492 |
| $a+b\sqrt{y}/x^2+c/yz^2$ | 218.37 | 157.33 | 0.420 | 0.1172 | 0.0907 | 0.3220 | 0.3745 | 0.2741 | 0.406 |
| $a+b\sqrt{y}/x^2+c/y\sqrt{z}$ | 193.64 | 133.82 | 0.544 | 0.1084 | 0.0810 | 0.4196 | 0.3392 | 0.2368 | 0.512 |
| $a+b\sqrt{y}/x^2+cz/y$ | 218.74 | 157.60 | 0.418 | 0.0993 | 0.0783 | 0.5128 | 0.3604 | 0.2650 | 0.450 |
| $a+b\sqrt{y}/x^2+cz^2/y$ | 166.69 | 123.34 | 0.662 | 0.0796 | 0.0599 | 0.6875 | 0.2972 | 0.2147 | 0.626 |
| $a+b\sqrt{y}/x^2+c\sqrt{z}/y$ | 288.28 | 215.37 | -0.011 | 0.1387 | 0.1090 | 0.0504 | 0.4696 | 0.3617 | 0.066 |
| $a+b\sqrt{y}/x^2+c/y^2z$ | 238.30 | 171.31 | 0.309 | 0.1239 | 0.0961 | 0.2422 | 0.3982 | 0.2908 | 0.328 |
| $a+b\sqrt{y}/x^2+c/y^2z^2$ | 242.30 | 173.12 | 0.286 | 0.1254 | 0.0965 | 0.2237 | 0.4046 | 0.2926 | 0.307 |
| $a+b\sqrt{y}/x^2+c/y^2\sqrt{z}$ | 236.97 | 170.38 | 0.317 | 0.1234 | 0.0960 | 0.2480 | 0.3964 | 0.2904 | 0.334 |

(continued on next page)

**Table 4 – continued from previous page**

| Functional form | $T_{eff}$ (K) | | | Radius ($R_{\odot}$) | | | log (L/$L_{\odot}$) | | |
|---|---|---|---|---|---|---|---|---|---|
| | RMSE | MAD | $R^2_{ap}$ | RMSE | MAD | $R^2_{ap}$ | RMSE | MAD | $R^2_{ap}$ |
| $a+b\sqrt{y}/x^2+cz/y^2$ | 284.53 | 213.55 | 0.015 | 0.1383 | 0.1096 | 0.0552 | 0.4651 | 0.3590 | 0.084 |
| $a+b\sqrt{y}/x^2+cz^2/y^2$ | 213.35 | 156.50 | 0.446 | 0.0966 | 0.0779 | 0.5389 | 0.3510 | 0.2645 | 0.478 |
| $a+b\sqrt{y}/x^2+c\sqrt{z}/y^2$ | 252.09 | 183.44 | 0.227 | 0.1289 | 0.0997 | 0.1793 | 0.4197 | 0.3136 | 0.253 |
| $a+b\sqrt{y}/x^2+c/\sqrt{y}z$ | 176.99 | 123.42 | 0.619 | 0.1010 | 0.0755 | 0.4966 | 0.3186 | 0.2148 | 0.570 |
| $a+b\sqrt{y}/x^2+c/\sqrt{y}z^2$ | 213.73 | 151.05 | 0.444 | 0.1144 | 0.0870 | 0.3535 | 0.3700 | 0.2635 | 0.420 |
| $a+b\sqrt{y}/x^2+c/\sqrt{y}\sqrt{z}$ | 160.22 | 110.58 | 0.688 | 0.0953 | 0.0706 | 0.5519 | 0.2972 | 0.1936 | 0.626 |
| $a+b\sqrt{y}/x^2+cz/\sqrt{y}$ | 162.48 | 125.09 | 0.679 | 0.0788 | 0.0583 | 0.6937 | 0.2902 | 0.2059 | 0.643 |
| $a+b\sqrt{y}/x^2+cz^2/\sqrt{y}$ | 158.16 | 116.95 | 0.696 | 0.0778 | 0.0561 | 0.7011 | 0.2923 | 0.2113 | 0.638 |
| $a+b\sqrt{y}/x^2+c\sqrt{z}/\sqrt{y}$ | 223.13 | 158.77 | 0.394 | 0.1020 | 0.0789 | 0.4862 | 0.3681 | 0.2659 | 0.426 |
| $a+b/\sqrt{x}y+cx/z$ | 226.74 | 163.81 | 0.375 | 0.1093 | 0.0821 | 0.4099 | 0.3737 | 0.2761 | 0.408 |
| $a+b/\sqrt{x}y+cx/z^2$ | 231.71 | 171.10 | 0.347 | 0.1152 | 0.0899 | 0.3443 | 0.3837 | 0.2846 | 0.376 |
| $a+b/\sqrt{x}y+cx/\sqrt{z}$ | 266.73 | 198.57 | 0.134 | 0.1272 | 0.0991 | 0.2017 | 0.4253 | 0.3247 | 0.234 |
| $a+b/\sqrt{x}y+cxz$ | 127.25 | 95.58 | 0.803 | 0.0707 | 0.0473 | 0.7534 | 0.2535 | 0.1775 | 0.728 |
| $a+b/\sqrt{x}y+cxz^2$ | 146.62 | 111.14 | 0.738 | 0.0767 | 0.0553 | 0.7093 | 0.2785 | 0.1975 | 0.671 |
| $a+b/\sqrt{x}y+cx\sqrt{z}$ | 114.85 | 88.52 | 0.840 | 0.0696 | 0.0443 | 0.7610 | 0.2398 | 0.1574 | 0.756 |
| $a+b/\sqrt{x}y+cx^2/z$ | 266.74 | 198.68 | 0.134 | 0.1275 | 0.0994 | 0.1976 | 0.4255 | 0.3249 | 0.233 |
| $a+b/\sqrt{x}y+cx^2/z^2$ | 244.94 | 180.55 | 0.270 | 0.1191 | 0.0930 | 0.3001 | 0.4002 | 0.3009 | 0.321 |
| $a+b/\sqrt{x}y+cx^2/\sqrt{z}$ | 189.94 | 148.67 | 0.561 | 0.1053 | 0.0828 | 0.4525 | 0.3277 | 0.2533 | 0.545 |
| $a+b/\sqrt{x}y+cx^2z$ | 133.37 | 103.39 | 0.784 | 0.0743 | 0.0532 | 0.7273 | 0.2652 | 0.1921 | 0.702 |
| $a+b/\sqrt{x}y+cx^2z^2$ | 151.19 | 117.39 | 0.722 | 0.0804 | 0.0599 | 0.6810 | 0.2885 | 0.2124 | 0.647 |
| $a+b/\sqrt{x}y+cx^2\sqrt{z}$ | 123.59 | 96.01 | 0.814 | 0.0730 | 0.0514 | 0.7370 | 0.2533 | 0.1789 | 0.728 |
| $a+b/\sqrt{x}y+c\sqrt{x}/z$ | 197.02 | 139.38 | 0.528 | 0.1004 | 0.0708 | 0.5024 | 0.3368 | 0.2310 | 0.519 |
| $a+b/\sqrt{x}y+c\sqrt{x}/z^2$ | 222.44 | 165.21 | 0.398 | 0.1132 | 0.0873 | 0.3678 | 0.3728 | 0.2750 | 0.411 |
| $a+b/\sqrt{x}y+c\sqrt{x}/\sqrt{z}$ | 209.83 | 150.24 | 0.464 | 0.1015 | 0.0728 | 0.4917 | 0.3502 | 0.2523 | 0.480 |
| $a+b/\sqrt{x}y+c\sqrt{x}z$ | 128.73 | 99.33 | 0.798 | 0.0703 | 0.0447 | 0.7560 | 0.2523 | 0.1699 | 0.730 |
| $a+b/\sqrt{x}y+c\sqrt{x}z^2$ | 146.14 | 112.87 | 0.740 | 0.0756 | 0.0531 | 0.7180 | 0.2753 | 0.1921 | 0.679 |
| $a+b/\sqrt{x}y+c\sqrt{x}\sqrt{z}$ | 117.61 | 90.80 | 0.832 | 0.0695 | 0.0408 | 0.7614 | 0.2400 | 0.1478 | 0.756 |
| $a+b/\sqrt{x}y+c/xz$ | 227.25 | 168.26 | 0.372 | 0.1142 | 0.0849 | 0.3558 | 0.3707 | 0.2694 | 0.418 |
| $a+b/\sqrt{x}y+c/xz^2$ | 231.88 | 166.10 | 0.346 | 0.1210 | 0.0925 | 0.2766 | 0.3884 | 0.2836 | 0.361 |
| $a+b/\sqrt{x}y+c/x\sqrt{z}$ | 265.72 | 199.20 | 0.141 | 0.1281 | 0.1023 | 0.1901 | 0.4255 | 0.3256 | 0.233 |
| $a+b/\sqrt{x}y+cz/x$ | 189.00 | 131.98 | 0.565 | 0.1067 | 0.0803 | 0.4381 | 0.3366 | 0.2334 | 0.520 |
| $a+b/\sqrt{x}y+cz^2/x$ | 138.86 | 100.23 | 0.765 | 0.0818 | 0.0558 | 0.6693 | 0.2711 | 0.1734 | 0.689 |
| $a+b/\sqrt{x}y+c\sqrt{z}/x$ | 218.61 | 156.27 | 0.419 | 0.1174 | 0.0916 | 0.3191 | 0.3739 | 0.2712 | 0.408 |
| $a+b/\sqrt{x}y+c/x^2z$ | 224.01 | 165.02 | 0.389 | 0.1198 | 0.0940 | 0.2914 | 0.3808 | 0.2847 | 0.386 |
| $a+b/\sqrt{x}y+c/x^2z^2$ | 204.00 | 152.69 | 0.494 | 0.1139 | 0.0899 | 0.3598 | 0.3566 | 0.2670 | 0.461 |
| $a+b/\sqrt{x}y+c/x^2\sqrt{z}$ | 227.57 | 166.62 | 0.370 | 0.1208 | 0.0946 | 0.2799 | 0.3849 | 0.2868 | 0.372 |
| $a+b/\sqrt{x}y+cz/x^2$ | 230.49 | 167.43 | 0.354 | 0.1215 | 0.0950 | 0.2716 | 0.3880 | 0.2875 | 0.362 |
| $a+b/\sqrt{x}y+cz^2/x^2$ | 226.44 | 164.44 | 0.376 | 0.1202 | 0.0942 | 0.2872 | 0.3831 | 0.2836 | 0.378 |
| $a+b/\sqrt{x}y+c\sqrt{z}/x^2$ | 230.49 | 167.66 | 0.354 | 0.1215 | 0.0950 | 0.2711 | 0.3881 | 0.2879 | 0.362 |
| $a+b/\sqrt{x}y+c/\sqrt{x}z$ | 175.90 | 123.86 | 0.624 | 0.1006 | 0.0761 | 0.5007 | 0.3150 | 0.2140 | 0.580 |
| $a+b/\sqrt{x}y+c/\sqrt{x}z^2$ | 212.11 | 153.89 | 0.453 | 0.1141 | 0.0883 | 0.3566 | 0.3641 | 0.2658 | 0.438 |
| $a+b/\sqrt{x}y+c/\sqrt{x}\sqrt{z}$ | 147.38 | 98.53 | 0.736 | 0.0877 | 0.0637 | 0.6204 | 0.2739 | 0.1737 | 0.682 |
| $a+b/\sqrt{x}y+cz/\sqrt{x}$ | 136.80 | 101.19 | 0.772 | 0.0778 | 0.0524 | 0.7008 | 0.2635 | 0.1662 | 0.706 |
| $a+b/\sqrt{x}y+cz^2/\sqrt{x}$ | 143.60 | 111.32 | 0.749 | 0.0749 | 0.0507 | 0.7233 | 0.2690 | 0.1873 | 0.693 |
| $a+b/\sqrt{x}y+c\sqrt{z}/\sqrt{x}$ | 161.66 | 116.08 | 0.682 | 0.0916 | 0.0637 | 0.5855 | 0.2982 | 0.1978 | 0.623 |
| $a+b/\sqrt{x}y+cy/z$ | 208.31 | 153.32 | 0.472 | 0.1011 | 0.0729 | 0.4955 | 0.3427 | 0.2496 | 0.502 |
| $a+b/\sqrt{x}y+cy/z^2$ | 222.57 | 165.37 | 0.397 | 0.1120 | 0.0863 | 0.3809 | 0.3705 | 0.2720 | 0.418 |
| $a+b/\sqrt{x}y+cy/\sqrt{z}$ | 252.24 | 184.00 | 0.226 | 0.1166 | 0.0900 | 0.3292 | 0.3965 | 0.3008 | 0.334 |
| $a+b/\sqrt{x}y+cyz$ | 135.17 | 106.16 | 0.778 | 0.0754 | 0.0488 | 0.7191 | 0.2691 | 0.1840 | 0.693 |
| $a+b/\sqrt{x}y+cyz^2$ | 150.34 | 116.83 | 0.725 | 0.0790 | 0.0558 | 0.6919 | 0.2856 | 0.1996 | 0.654 |
| $a+b/\sqrt{x}y+cy\sqrt{z}$ | 130.86 | 100.68 | 0.792 | 0.0779 | 0.0477 | 0.7006 | 0.2688 | 0.1673 | 0.694 |
| $a+b/\sqrt{x}y+cy^2/z$ | 252.32 | 182.91 | 0.225 | 0.1171 | 0.0896 | 0.3227 | 0.3978 | 0.3029 | 0.329 |
| $a+b/\sqrt{x}y+cy^2/z^2$ | 230.92 | 169.96 | 0.351 | 0.1128 | 0.0867 | 0.3718 | 0.3778 | 0.2804 | 0.395 |
| $a+b/\sqrt{x}y+cy^2/\sqrt{z}$ | 247.94 | 200.91 | 0.252 | 0.1255 | 0.1000 | 0.2219 | 0.4116 | 0.3241 | 0.282 |
| $a+b/\sqrt{x}y+cy^2z$ | 144.81 | 111.18 | 0.745 | 0.0809 | 0.0547 | 0.6769 | 0.2863 | 0.1946 | 0.653 |
| $a+b/\sqrt{x}y+cy^2z^2$ | 156.45 | 120.60 | 0.702 | 0.0834 | 0.0603 | 0.6563 | 0.2981 | 0.2126 | 0.623 |
| $a+b/\sqrt{x}y+cy^2\sqrt{z}$ | 143.92 | 105.03 | 0.748 | 0.0836 | 0.0551 | 0.6549 | 0.2887 | 0.1845 | 0.647 |
| $a+b/\sqrt{x}y+c\sqrt{y}/z$ | 188.04 | 134.32 | 0.570 | 0.0969 | 0.0675 | 0.5361 | 0.3221 | 0.2181 | 0.560 |
| $a+b/\sqrt{x}y+c\sqrt{y}/z^2$ | 217.48 | 161.73 | 0.425 | 0.1117 | 0.0853 | 0.3843 | 0.3661 | 0.2680 | 0.432 |
| $a+b/\sqrt{x}y+c\sqrt{y}/\sqrt{z}$ | 195.33 | 147.01 | 0.536 | 0.0944 | 0.0695 | 0.5601 | 0.3226 | 0.2348 | 0.559 |
| $a+b/\sqrt{x}y+c\sqrt{y}z$ | 132.15 | 105.91 | 0.788 | 0.0729 | 0.0454 | 0.7376 | 0.2607 | 0.1746 | 0.712 |
| $a+b/\sqrt{x}y+c\sqrt{y}z^2$ | 147.92 | 115.93 | 0.734 | 0.0768 | 0.0536 | 0.7085 | 0.2792 | 0.1931 | 0.670 |
| $a+b/\sqrt{x}y+c\sqrt{y}\sqrt{z}$ | 125.59 | 99.50 | 0.808 | 0.0745 | 0.0430 | 0.7260 | 0.2573 | 0.1584 | 0.719 |
| $a+b/\sqrt{x}y+c/yz$ | 196.39 | 141.18 | 0.531 | 0.1103 | 0.0852 | 0.3988 | 0.3461 | 0.2513 | 0.493 |
| $a+b/\sqrt{x}y+c/yz^2$ | 218.11 | 157.09 | 0.421 | 0.1172 | 0.0907 | 0.3219 | 0.3732 | 0.2730 | 0.410 |
| $a+b/\sqrt{x}y+c/y\sqrt{z}$ | 184.23 | 128.63 | 0.587 | 0.1066 | 0.0812 | 0.4390 | 0.3324 | 0.2346 | 0.532 |
| $a+b/\sqrt{x}y+cz/y$ | 165.93 | 132.79 | 0.665 | 0.0814 | 0.0614 | 0.6727 | 0.2801 | 0.2086 | 0.668 |
| $a+b/\sqrt{x}y+cz^2/y$ | 149.61 | 114.63 | 0.728 | 0.0745 | 0.0532 | 0.7260 | 0.2673 | 0.1873 | 0.697 |
| $a+b/\sqrt{x}y+c\sqrt{z}/y$ | 237.44 | 174.05 | 0.314 | 0.1091 | 0.0863 | 0.4124 | 0.3715 | 0.2912 | 0.415 |
| $a+b/\sqrt{x}y+c/y^2z$ | 239.55 | 172.69 | 0.302 | 0.1237 | 0.0961 | 0.2448 | 0.3980 | 0.2914 | 0.329 |
| $a+b/\sqrt{x}y+c/y^2z^2$ | 241.91 | 174.33 | 0.288 | 0.1244 | 0.0966 | 0.2361 | 0.4013 | 0.2933 | 0.318 |
| $a+b/\sqrt{x}y+c/y^2\sqrt{z}$ | 239.14 | 172.12 | 0.304 | 0.1235 | 0.0961 | 0.2466 | 0.3975 | 0.2914 | 0.330 |
| $a+b/\sqrt{x}y+cz/y^2$ | 195.98 | 151.61 | 0.533 | 0.0955 | 0.0725 | 0.5501 | 0.3154 | 0.2437 | 0.579 |
| $a+b/\sqrt{x}y+cz^2/y^2$ | 159.26 | 121.78 | 0.691 | 0.0818 | 0.0634 | 0.6699 | 0.2747 | 0.2000 | 0.680 |
| $a+b/\sqrt{x}y+c\sqrt{z}/y^2$ | 266.80 | 198.83 | 0.134 | 0.1265 | 0.1002 | 0.2094 | 0.4234 | 0.3238 | 0.240 |
| $a+b/\sqrt{x}y+c/\sqrt{y}z$ | 176.72 | 122.73 | 0.620 | 0.1016 | 0.0772 | 0.4901 | 0.3196 | 0.2191 | 0.567 |
| $a+b/\sqrt{x}y+c/\sqrt{y}z^2$ | 211.20 | 151.92 | 0.457 | 0.1135 | 0.0875 | 0.3635 | 0.3633 | 0.2635 | 0.441 |
| $a+b/\sqrt{x}y+c/\sqrt{y}\sqrt{z}$ | 155.34 | 107.77 | 0.706 | 0.0944 | 0.0706 | 0.5599 | 0.2951 | 0.1925 | 0.631 |
| $a+b/\sqrt{x}y+cz/\sqrt{y}$ | 144.73 | 116.41 | 0.745 | 0.0741 | 0.0514 | 0.7289 | 0.2607 | 0.1785 | 0.712 |
| $a+b/\sqrt{x}y+cz^2/\sqrt{y}$ | 146.98 | 111.90 | 0.737 | 0.0740 | 0.0513 | 0.7293 | 0.2690 | 0.1882 | 0.693 |
| $a+b/\sqrt{x}y+c\sqrt{z}/\sqrt{y}$ | 173.23 | 137.33 | 0.635 | 0.0839 | 0.0633 | 0.6522 | 0.2897 | 0.2144 | 0.644 |
| $a+b/\sqrt{x}y^2+cx/z$ | 234.86 | 169.66 | 0.329 | 0.1129 | 0.0855 | 0.3711 | 0.3870 | 0.2896 | 0.365 |
| $a+b/\sqrt{x}y^2+cx/z^2$ | 237.58 | 175.05 | 0.313 | 0.1179 | 0.0920 | 0.3134 | 0.3942 | 0.2936 | 0.342 |
| $a+b/\sqrt{x}y^2+cx/\sqrt{z}$ | 273.18 | 205.23 | 0.092 | 0.1313 | 0.1034 | 0.1488 | 0.4377 | 0.3373 | 0.188 |
| $a+b/\sqrt{x}y^2+cxz$ | 127.51 | 95.78 | 0.802 | 0.0708 | 0.0476 | 0.7527 | 0.2545 | 0.1789 | 0.725 |
| $a+b/\sqrt{x}y^2+cxz^2$ | 148.00 | 112.32 | 0.734 | 0.0773 | 0.0559 | 0.7051 | 0.2816 | 0.2004 | 0.664 |
| $a+b/\sqrt{x}y^2+cx\sqrt{z}$ | 114.71 | 88.36 | 0.840 | 0.0696 | 0.0443 | 0.7610 | 0.2399 | 0.1576 | 0.756 |
| $a+b/\sqrt{x}y^2+cx^2/z$ | 273.47 | 204.48 | 0.090 | 0.1312 | 0.1030 | 0.1500 | 0.4379 | 0.3366 | 0.187 |
| $a+b/\sqrt{x}y^2+cx^2/z^2$ | 251.81 | 185.73 | 0.229 | 0.1222 | 0.0953 | 0.2624 | 0.4124 | 0.3125 | 0.280 |
| $a+b/\sqrt{x}y^2+cx^2/\sqrt{z}$ | 188.65 | 146.72 | 0.567 | 0.1053 | 0.0822 | 0.4530 | 0.3275 | 0.2520 | 0.546 |
| $a+b/\sqrt{x}y^2+cx^2z$ | 133.98 | 103.89 | 0.782 | 0.0745 | 0.0535 | 0.7257 | 0.2668 | 0.1943 | 0.698 |
| $a+b/\sqrt{x}y^2+cx^2z^2$ | 152.88 | 119.02 | 0.716 | 0.0811 | 0.0608 | 0.6754 | 0.2921 | 0.2158 | 0.638 |

(continued on next page)

**Table 4 – continued from previous page**

| Functional form | $T_{eff}$ (K) | | | Radius ($R_{\odot}$) | | | log (L/$L_{\odot}$) | | |
|---|---|---|---|---|---|---|---|---|---|
| | RMSE | MAD | $R^2_{ap}$ | RMSE | MAD | $R^2_{ap}$ | RMSE | MAD | $R^2_{ap}$ |
| $a+b/\sqrt{x}y^2+cx^2\sqrt{z}$ | 123.69 | 96.06 | 0.814 | 0.0730 | 0.0515 | 0.7368 | 0.2539 | 0.1798 | 0.727 |
| $a+b/\sqrt{x}y^2+c\sqrt{x}/z$ | 202.20 | 143.20 | 0.503 | 0.1025 | 0.0725 | 0.4810 | 0.3454 | 0.2405 | 0.494 |
| $a+b/\sqrt{x}y^2+c\sqrt{x}/z^2$ | 227.35 | 168.06 | 0.371 | 0.1154 | 0.0890 | 0.3419 | 0.3819 | 0.2815 | 0.382 |
| $a+b/\sqrt{x}y^2+c\sqrt{x}/\sqrt{z}$ | 219.62 | 156.04 | 0.413 | 0.1055 | 0.0775 | 0.4509 | 0.3653 | 0.2686 | 0.435 |
| $a+b/\sqrt{x}y^2+c\sqrt{x}z$ | 128.93 | 99.58 | 0.798 | 0.0704 | 0.0449 | 0.7553 | 0.2533 | 0.1713 | 0.728 |
| $a+b/\sqrt{x}y^2+c\sqrt{x}z^2$ | 147.45 | 114.09 | 0.735 | 0.0761 | 0.0536 | 0.7142 | 0.2783 | 0.1948 | 0.672 |
| $a+b/\sqrt{x}y^2+c\sqrt{x}\sqrt{z}$ | 117.32 | 90.37 | 0.833 | 0.0695 | 0.0408 | 0.7614 | 0.2401 | 0.1480 | 0.756 |
| $a+b/\sqrt{x}y^2+c/xz$ | 181.52 | 131.10 | 0.599 | 0.0993 | 0.0714 | 0.5133 | 0.3146 | 0.2092 | 0.581 |
| $a+b/\sqrt{x}y^2+c/xz^2$ | 221.69 | 161.81 | 0.402 | 0.1192 | 0.0932 | 0.2980 | 0.3799 | 0.2823 | 0.388 |
| $a+b/\sqrt{x}y^2+c/x\sqrt{z}$ | 256.45 | 179.37 | 0.200 | 0.1191 | 0.0913 | 0.2992 | 0.4050 | 0.2891 | 0.305 |
| $a+b/\sqrt{x}y^2+cz/x$ | 210.45 | 149.35 | 0.461 | 0.1141 | 0.0878 | 0.3577 | 0.3653 | 0.2672 | 0.435 |
| $a+b/\sqrt{x}y^2+cz^2/x$ | 147.05 | 106.04 | 0.737 | 0.0845 | 0.0590 | 0.6475 | 0.2819 | 0.1838 | 0.663 |
| $a+b/\sqrt{x}y^2+c\sqrt{z}/x$ | 245.71 | 174.91 | 0.265 | 0.1261 | 0.0980 | 0.2145 | 0.4095 | 0.3008 | 0.289 |
| $a+b/\sqrt{x}y^2+c/x^2z$ | 249.37 | 178.31 | 0.243 | 0.1277 | 0.0990 | 0.1948 | 0.4142 | 0.3043 | 0.273 |
| $a+b/\sqrt{x}y^2+c/x^2z^2$ | 244.71 | 177.20 | 0.271 | 0.1264 | 0.0988 | 0.2110 | 0.4084 | 0.3042 | 0.293 |
| $a+b/\sqrt{x}y^2+c/x^2\sqrt{z}$ | 250.07 | 178.38 | 0.239 | 0.1279 | 0.0990 | 0.1926 | 0.4150 | 0.3041 | 0.270 |
| $a+b/\sqrt{x}y^2+cz/x^2$ | 249.40 | 177.79 | 0.243 | 0.1277 | 0.0989 | 0.1954 | 0.4141 | 0.3031 | 0.273 |
| $a+b/\sqrt{x}y^2+cz^2/x^2$ | 244.75 | 175.65 | 0.271 | 0.1263 | 0.0987 | 0.2124 | 0.4085 | 0.3008 | 0.293 |
| $a+b/\sqrt{x}y^2+c\sqrt{z}/x^2$ | 250.12 | 178.15 | 0.239 | 0.1279 | 0.0990 | 0.1928 | 0.4150 | 0.3036 | 0.270 |
| $a+b/\sqrt{x}y^2+c/\sqrt{x}z$ | 170.10 | 119.23 | 0.648 | 0.0992 | 0.0753 | 0.5145 | 0.3099 | 0.2089 | 0.593 |
| $a+b/\sqrt{x}y^2+c/\sqrt{x}z^2$ | 211.48 | 151.79 | 0.456 | 0.1148 | 0.0897 | 0.3497 | 0.3663 | 0.2673 | 0.432 |
| $a+b/\sqrt{x}y^2+c/\sqrt{x}\sqrt{z}$ | 139.50 | 91.02 | 0.763 | 0.0856 | 0.0616 | 0.6380 | 0.2661 | 0.1649 | 0.700 |
| $a+b/\sqrt{x}y^2+cz/\sqrt{x}$ | 142.41 | 104.24 | 0.753 | 0.0795 | 0.0550 | 0.6877 | 0.2710 | 0.1739 | 0.689 |
| $a+b/\sqrt{x}y^2+cz^2/\sqrt{x}$ | 146.11 | 113.10 | 0.740 | 0.0757 | 0.0517 | 0.7171 | 0.2733 | 0.1907 | 0.684 |
| $a+b/\sqrt{x}y^2+c\sqrt{z}/\sqrt{x}$ | 179.50 | 126.97 | 0.608 | 0.0977 | 0.0705 | 0.5287 | 0.3215 | 0.2255 | 0.562 |
| $a+b/\sqrt{x}y^2+cy/z$ | 215.04 | 158.18 | 0.437 | 0.1039 | 0.0762 | 0.4665 | 0.3539 | 0.2611 | 0.469 |
| $a+b/\sqrt{x}y^2+cy/z^2$ | 227.76 | 168.34 | 0.369 | 0.1144 | 0.0881 | 0.3542 | 0.3799 | 0.2798 | 0.389 |
| $a+b/\sqrt{x}y^2+cy/\sqrt{z}$ | 262.87 | 193.49 | 0.159 | 0.1221 | 0.0935 | 0.2639 | 0.4156 | 0.3149 | 0.268 |
| $a+b/\sqrt{x}y^2+cyz$ | 135.53 | 106.59 | 0.777 | 0.0756 | 0.0490 | 0.7181 | 0.2704 | 0.1860 | 0.690 |
| $a+b/\sqrt{x}y^2+cyz^2$ | 151.77 | 117.92 | 0.720 | 0.0796 | 0.0565 | 0.6873 | 0.2888 | 0.2025 | 0.647 |
| $a+b/\sqrt{x}y^2+cy\sqrt{z}$ | 130.78 | 100.56 | 0.792 | 0.0779 | 0.0477 | 0.7005 | 0.2692 | 0.1684 | 0.693 |
| $a+b/\sqrt{x}y^2+cy^2/z$ | 261.71 | 192.21 | 0.167 | 0.1219 | 0.0933 | 0.2662 | 0.4148 | 0.3158 | 0.271 |
| $a+b/\sqrt{x}y^2+cy^2/z^2$ | 237.44 | 174.57 | 0.314 | 0.1157 | 0.0888 | 0.3385 | 0.3892 | 0.2914 | 0.358 |
| $a+b/\sqrt{x}y^2+cy^2/\sqrt{z}$ | 249.02 | 202.13 | 0.246 | 0.1271 | 0.1012 | 0.2023 | 0.4172 | 0.3282 | 0.263 |
| $a+b/\sqrt{x}y^2+cy^2z$ | 145.45 | 111.78 | 0.743 | 0.0812 | 0.0551 | 0.6746 | 0.2882 | 0.1971 | 0.648 |
| $a+b/\sqrt{x}y^2+cy^2z^2$ | 158.16 | 121.75 | 0.696 | 0.0842 | 0.0612 | 0.6502 | 0.3019 | 0.2163 | 0.614 |
| $a+b/\sqrt{x}y^2+cy^2\sqrt{z}$ | 144.06 | 105.07 | 0.747 | 0.0837 | 0.0552 | 0.6539 | 0.2898 | 0.1855 | 0.644 |
| $a+b/\sqrt{x}y^2+c\sqrt{y}/z$ | 191.96 | 137.25 | 0.552 | 0.0986 | 0.0683 | 0.5201 | 0.3289 | 0.2253 | 0.542 |
| $a+b/\sqrt{x}y^2+c\sqrt{y}/z^2$ | 221.77 | 164.08 | 0.402 | 0.1137 | 0.0868 | 0.3614 | 0.3742 | 0.2736 | 0.407 |
| $a+b/\sqrt{x}y^2+c\sqrt{y}/\sqrt{z}$ | 202.29 | 152.03 | 0.502 | 0.0972 | 0.0722 | 0.5333 | 0.3337 | 0.2470 | 0.528 |
| $a+b/\sqrt{x}y^2+c\sqrt{y}z$ | 132.51 | 106.32 | 0.786 | 0.0730 | 0.0457 | 0.7367 | 0.2619 | 0.1761 | 0.709 |
| $a+b/\sqrt{x}y^2+c\sqrt{y}z^2$ | 149.30 | 117.28 | 0.729 | 0.0774 | 0.0542 | 0.7044 | 0.2822 | 0.1958 | 0.663 |
| $a+b/\sqrt{x}y^2+c\sqrt{y}\sqrt{z}$ | 125.50 | 99.36 | 0.808 | 0.0745 | 0.0430 | 0.7259 | 0.2577 | 0.1591 | 0.719 |
| $a+b/\sqrt{x}y^2+c/yz$ | 193.41 | 140.06 | 0.545 | 0.1101 | 0.0856 | 0.4011 | 0.3451 | 0.2521 | 0.495 |
| $a+b/\sqrt{x}y^2+c/yz^2$ | 218.70 | 159.07 | 0.418 | 0.1183 | 0.0927 | 0.3086 | 0.3773 | 0.2798 | 0.397 |
| $a+b/\sqrt{x}y^2+c/y\sqrt{z}$ | 178.66 | 125.31 | 0.612 | 0.1054 | 0.0808 | 0.4513 | 0.3278 | 0.2309 | 0.545 |
| $a+b/\sqrt{x}y^2+cz/y$ | 174.48 | 139.08 | 0.630 | 0.0845 | 0.0645 | 0.6471 | 0.2925 | 0.2191 | 0.637 |
| $a+b/\sqrt{x}y^2+cz^2/y$ | 152.43 | 116.66 | 0.717 | 0.0755 | 0.0544 | 0.7185 | 0.2721 | 0.1917 | 0.686 |
| $a+b/\sqrt{x}y^2+c\sqrt{z}/y$ | 257.93 | 191.91 | 0.191 | 0.1194 | 0.0931 | 0.2967 | 0.4060 | 0.3125 | 0.302 |
| $a+b/\sqrt{x}y^2+c/y^2z$ | 235.76 | 171.38 | 0.324 | 0.1240 | 0.0973 | 0.2404 | 0.3977 | 0.2938 | 0.330 |
| $a+b/\sqrt{x}y^2+c/y^2z^2$ | 242.31 | 174.25 | 0.286 | 0.1259 | 0.0978 | 0.2169 | 0.4062 | 0.2967 | 0.301 |
| $a+b/\sqrt{x}y^2+c/y^2\sqrt{z}$ | 231.00 | 168.35 | 0.351 | 0.1227 | 0.0967 | 0.2572 | 0.3920 | 0.2909 | 0.349 |
| $a+b/\sqrt{x}y^2+cz/y^2$ | 235.41 | 175.76 | 0.326 | 0.1116 | 0.0854 | 0.3850 | 0.3735 | 0.2908 | 0.409 |
| $a+b/\sqrt{x}y^2+cz^2/y^2$ | 169.81 | 129.31 | 0.649 | 0.0855 | 0.0674 | 0.6386 | 0.2896 | 0.2105 | 0.645 |
| $a+b/\sqrt{x}y^2+c\sqrt{z}/y^2$ | 258.39 | 195.27 | 0.188 | 0.1299 | 0.1012 | 0.1666 | 0.4265 | 0.3270 | 0.229 |
| $a+b/\sqrt{x}y^2+c/\sqrt{y}z$ | 176.01 | 122.48 | 0.623 | 0.1019 | 0.0776 | 0.4877 | 0.3207 | 0.2207 | 0.564 |
| $a+b/\sqrt{x}y^2+c/\sqrt{y}z^2$ | 212.99 | 151.51 | 0.448 | 0.1149 | 0.0892 | 0.3485 | 0.3684 | 0.2654 | 0.425 |
| $a+b/\sqrt{x}y^2+c/\sqrt{y}\sqrt{z}$ | 153.47 | 106.77 | 0.713 | 0.0941 | 0.0705 | 0.5627 | 0.2942 | 0.1919 | 0.633 |
| $a+b/\sqrt{x}y^2+cz/\sqrt{y}$ | 147.37 | 118.12 | 0.736 | 0.0750 | 0.0525 | 0.7226 | 0.2650 | 0.1831 | 0.703 |
| $a+b/\sqrt{x}y^2+cz^2/\sqrt{y}$ | 148.78 | 113.27 | 0.731 | 0.0747 | 0.0521 | 0.7245 | 0.2725 | 0.1911 | 0.685 |
| $a+b/\sqrt{x}y^2+c\sqrt{z}/\sqrt{y}$ | 181.07 | 142.40 | 0.601 | 0.0869 | 0.0664 | 0.6274 | 0.3014 | 0.2251 | 0.615 |
| $a+b/\sqrt{x}\sqrt{y}+cx/z$ | 221.99 | 160.26 | 0.400 | 0.1070 | 0.0799 | 0.4344 | 0.3655 | 0.2674 | 0.434 |
| $a+b/\sqrt{x}\sqrt{y}+cx/z^2$ | 228.00 | 168.62 | 0.367 | 0.1133 | 0.0885 | 0.3657 | 0.3768 | 0.2793 | 0.398 |
| $a+b/\sqrt{x}\sqrt{y}+cx/\sqrt{z}$ | 261.57 | 194.28 | 0.168 | 0.1239 | 0.0959 | 0.2418 | 0.4157 | 0.3156 | 0.268 |
| $a+b/\sqrt{x}\sqrt{y}+cxz$ | 127.19 | 95.47 | 0.803 | 0.0706 | 0.0473 | 0.7538 | 0.2530 | 0.1770 | 0.729 |
| $a+b/\sqrt{x}\sqrt{y}+cxz^2$ | 146.00 | 110.45 | 0.741 | 0.0764 | 0.0550 | 0.7119 | 0.2769 | 0.1964 | 0.675 |
| $a+b/\sqrt{x}\sqrt{y}+cx\sqrt{z}$ | 114.78 | 88.45 | 0.840 | 0.0696 | 0.0443 | 0.7610 | 0.2398 | 0.1574 | 0.756 |
| $a+b/\sqrt{x}\sqrt{y}+cx^2/z$ | 261.94 | 194.83 | 0.165 | 0.1247 | 0.0968 | 0.2319 | 0.4165 | 0.3161 | 0.265 |
| $a+b/\sqrt{x}\sqrt{y}+cx^2/z^2$ | 240.59 | 176.85 | 0.296 | 0.1169 | 0.0913 | 0.3257 | 0.3922 | 0.2930 | 0.348 |
| $a+b/\sqrt{x}\sqrt{y}+cx^2/\sqrt{z}$ | 190.70 | 149.86 | 0.558 | 0.1053 | 0.0833 | 0.4526 | 0.3277 | 0.2541 | 0.545 |
| $a+b/\sqrt{x}\sqrt{y}+cx^2z$ | 133.20 | 103.12 | 0.784 | 0.0742 | 0.0531 | 0.7282 | 0.2644 | 0.1913 | 0.704 |
| $a+b/\sqrt{x}\sqrt{y}+cx^2z^2$ | 150.41 | 116.47 | 0.725 | 0.0799 | 0.0596 | 0.6845 | 0.2865 | 0.2109 | 0.652 |
| $a+b/\sqrt{x}\sqrt{y}+cx^2\sqrt{z}$ | 123.60 | 95.99 | 0.814 | 0.0730 | 0.0514 | 0.7371 | 0.2532 | 0.1788 | 0.728 |
| $a+b/\sqrt{x}\sqrt{y}+c\sqrt{x}/z$ | 193.94 | 137.03 | 0.542 | 0.0989 | 0.0703 | 0.5173 | 0.3313 | 0.2254 | 0.535 |
| $a+b/\sqrt{x}\sqrt{y}+c\sqrt{x}/z^2$ | 219.19 | 163.17 | 0.415 | 0.1114 | 0.0860 | 0.3868 | 0.3666 | 0.2704 | 0.431 |
| $a+b/\sqrt{x}\sqrt{y}+c\sqrt{x}/\sqrt{z}$ | 204.39 | 146.38 | 0.492 | 0.0989 | 0.0700 | 0.5167 | 0.3413 | 0.2429 | 0.506 |
| $a+b/\sqrt{x}\sqrt{y}+c\sqrt{x}z$ | 128.66 | 99.20 | 0.799 | 0.0702 | 0.0446 | 0.7564 | 0.2518 | 0.1694 | 0.731 |
| $a+b/\sqrt{x}\sqrt{y}+c\sqrt{x}z^2$ | 145.54 | 112.06 | 0.742 | 0.0752 | 0.0528 | 0.7204 | 0.2737 | 0.1911 | 0.683 |
| $a+b/\sqrt{x}\sqrt{y}+c\sqrt{x}\sqrt{z}$ | 117.61 | 90.93 | 0.832 | 0.0695 | 0.0408 | 0.7614 | 0.2400 | 0.1478 | 0.756 |
| $a+b/\sqrt{x}\sqrt{y}+c/xz$ | 254.03 | 185.98 | 0.215 | 0.1236 | 0.0942 | 0.2453 | 0.4058 | 0.2996 | 0.302 |
| $a+b/\sqrt{x}\sqrt{y}+c/xz^2$ | 237.85 | 168.49 | 0.312 | 0.1216 | 0.0933 | 0.2698 | 0.3921 | 0.2849 | 0.348 |
| $a+b/\sqrt{x}\sqrt{y}+c/x\sqrt{z}$ | 236.38 | 178.81 | 0.320 | 0.1218 | 0.0957 | 0.2671 | 0.3935 | 0.2996 | 0.344 |
| $a+b/\sqrt{x}\sqrt{y}+cz/x$ | 170.55 | 117.39 | 0.646 | 0.1001 | 0.0744 | 0.5054 | 0.3120 | 0.2037 | 0.588 |
| $a+b/\sqrt{x}\sqrt{y}+cz^2/x$ | 132.23 | 95.56 | 0.787 | 0.0791 | 0.0529 | 0.6908 | 0.2616 | 0.1670 | 0.710 |
| $a+b/\sqrt{x}\sqrt{y}+c\sqrt{z}/x$ | 194.72 | 138.41 | 0.539 | 0.1095 | 0.0841 | 0.4083 | 0.3426 | 0.2426 | 0.503 |
| $a+b/\sqrt{x}\sqrt{y}+c/x^2z$ | 201.78 | 149.66 | 0.505 | 0.1126 | 0.0883 | 0.3742 | 0.3515 | 0.2604 | 0.476 |
| $a+b/\sqrt{x}\sqrt{y}+c/x^2z^2$ | 171.52 | 131.14 | 0.642 | 0.1031 | 0.0812 | 0.4753 | 0.3151 | 0.2344 | 0.579 |
| $a+b/\sqrt{x}\sqrt{y}+c/x^2\sqrt{z}$ | 207.88 | 153.50 | 0.474 | 0.1143 | 0.0893 | 0.3547 | 0.3586 | 0.2659 | 0.455 |
| $a+b/\sqrt{x}\sqrt{y}+cz/x^2$ | 214.15 | 156.64 | 0.442 | 0.1160 | 0.0903 | 0.3359 | 0.3657 | 0.2701 | 0.433 |
| $a+b/\sqrt{x}\sqrt{y}+cz^2/x^2$ | 210.70 | 153.68 | 0.460 | 0.1148 | 0.0894 | 0.3498 | 0.3614 | 0.2658 | 0.447 |

(continued on next page)

**Table 4 – continued from previous page**

| Functional form | $T_{eff}$ (K) | | | Radius ($R_\odot$) | | | log (L/$L_\odot$) | | |
|---|---|---|---|---|---|---|---|---|---|
| | RMSE | MAD | $R^2_{ap}$ | RMSE | MAD | $R^2_{ap}$ | RMSE | MAD | $R^2_{ap}$ |
| $a+b/\sqrt{x}\sqrt{y}+c\sqrt{z}/x^2$ | 213.46 | 156.52 | 0.446 | 0.1158 | 0.0902 | 0.3375 | 0.3650 | 0.2700 | 0.436 |
| $a+b/\sqrt{x}\sqrt{y}+c/\sqrt{x}z$ | 181.01 | 129.24 | 0.601 | 0.1019 | 0.0769 | 0.4874 | 0.3196 | 0.2185 | 0.567 |
| $a+b/\sqrt{x}\sqrt{y}+c/\sqrt{x}z^2$ | 212.23 | 155.01 | 0.452 | 0.1134 | 0.0880 | 0.3646 | 0.3616 | 0.2654 | 0.446 |
| $a+b/\sqrt{x}\sqrt{y}+c/\sqrt{x}\sqrt{z}$ | 155.82 | 107.08 | 0.705 | 0.0907 | 0.0661 | 0.5938 | 0.2837 | 0.1831 | 0.659 |
| $a+b/\sqrt{x}\sqrt{y}+cz/\sqrt{x}$ | 132.87 | 99.46 | 0.785 | 0.0761 | 0.0501 | 0.7137 | 0.2575 | 0.1603 | 0.719 |
| $a+b/\sqrt{x}\sqrt{y}+cz^2/\sqrt{x}$ | 142.23 | 110.19 | 0.754 | 0.0742 | 0.0502 | 0.7282 | 0.2663 | 0.1856 | 0.699 |
| $a+b/\sqrt{x}\sqrt{y}+c\sqrt{z}/\sqrt{x}$ | 148.25 | 107.01 | 0.733 | 0.0864 | 0.0589 | 0.6317 | 0.2800 | 0.1773 | 0.668 |
| $a+b/\sqrt{x}\sqrt{y}+cy/z$ | 204.86 | 150.71 | 0.489 | 0.0994 | 0.0717 | 0.5118 | 0.3367 | 0.2431 | 0.520 |
| $a+b/\sqrt{x}\sqrt{y}+cy/z^2$ | 219.35 | 163.25 | 0.415 | 0.1103 | 0.0850 | 0.3993 | 0.3644 | 0.2674 | 0.437 |
| $a+b/\sqrt{x}\sqrt{y}+cy/\sqrt{z}$ | 245.97 | 177.77 | 0.264 | 0.1133 | 0.0875 | 0.3666 | 0.3853 | 0.2920 | 0.371 |
| $a+b/\sqrt{x}\sqrt{y}+cyz$ | 135.01 | 105.90 | 0.778 | 0.0753 | 0.0487 | 0.7202 | 0.2683 | 0.1831 | 0.695 |
| $a+b/\sqrt{x}\sqrt{y}+cyz^2$ | 149.62 | 116.13 | 0.728 | 0.0786 | 0.0555 | 0.6950 | 0.2837 | 0.1984 | 0.659 |
| $a+b/\sqrt{x}\sqrt{y}+cy\sqrt{z}$ | 130.90 | 100.73 | 0.792 | 0.0778 | 0.0477 | 0.7010 | 0.2684 | 0.1668 | 0.695 |
| $a+b/\sqrt{x}\sqrt{y}+cy^2/z$ | 246.75 | 177.39 | 0.259 | 0.1142 | 0.0874 | 0.3558 | 0.3878 | 0.2942 | 0.363 |
| $a+b/\sqrt{x}\sqrt{y}+cy^2/z^2$ | 227.15 | 166.83 | 0.372 | 0.1109 | 0.0852 | 0.3927 | 0.3709 | 0.2732 | 0.417 |
| $a+b/\sqrt{x}\sqrt{y}+cy^2/\sqrt{z}$ | 246.66 | 199.66 | 0.260 | 0.1241 | 0.0989 | 0.2401 | 0.4067 | 0.3202 | 0.299 |
| $a+b/\sqrt{x}\sqrt{y}+cy^2z$ | 144.49 | 110.80 | 0.746 | 0.0807 | 0.0547 | 0.6788 | 0.2851 | 0.1932 | 0.656 |
| $a+b/\sqrt{x}\sqrt{y}+cy^2z^2$ | 155.56 | 119.88 | 0.706 | 0.0829 | 0.0598 | 0.6605 | 0.2958 | 0.2108 | 0.629 |
| $a+b/\sqrt{x}\sqrt{y}+cy^2\sqrt{z}$ | 143.83 | 105.02 | 0.748 | 0.0834 | 0.0551 | 0.6562 | 0.2879 | 0.1841 | 0.649 |
| $a+b/\sqrt{x}\sqrt{y}+c\sqrt{y}/z$ | 185.83 | 132.76 | 0.580 | 0.0958 | 0.0672 | 0.5469 | 0.3179 | 0.2139 | 0.572 |
| $a+b/\sqrt{x}\sqrt{y}+c\sqrt{y}/z^2$ | 214.61 | 160.01 | 0.440 | 0.1101 | 0.0842 | 0.4013 | 0.3604 | 0.2640 | 0.450 |
| $a+b/\sqrt{x}\sqrt{y}+c\sqrt{y}/\sqrt{z}$ | 192.00 | 144.20 | 0.551 | 0.0928 | 0.0683 | 0.5744 | 0.3170 | 0.2285 | 0.574 |
| $a+b/\sqrt{x}\sqrt{y}+c\sqrt{y}z$ | 131.98 | 105.65 | 0.788 | 0.0728 | 0.0453 | 0.7385 | 0.2599 | 0.1739 | 0.714 |
| $a+b/\sqrt{x}\sqrt{y}+c\sqrt{y}z^2$ | 147.25 | 115.22 | 0.736 | 0.0765 | 0.0533 | 0.7113 | 0.2774 | 0.1919 | 0.674 |
| $a+b/\sqrt{x}\sqrt{y}+c\sqrt{y}\sqrt{z}$ | 125.64 | 99.56 | 0.808 | 0.0745 | 0.0430 | 0.7263 | 0.2570 | 0.1581 | 0.720 |
| $a+b/\sqrt{x}\sqrt{y}+c/yz$ | 198.80 | 141.25 | 0.519 | 0.1103 | 0.0845 | 0.3990 | 0.3463 | 0.2491 | 0.492 |
| $a+b/\sqrt{x}\sqrt{y}+c/yz^2$ | 217.19 | 157.52 | 0.426 | 0.1160 | 0.0895 | 0.3354 | 0.3692 | 0.2714 | 0.422 |
| $a+b/\sqrt{x}\sqrt{y}+c/y\sqrt{z}$ | 189.92 | 131.15 | 0.561 | 0.1077 | 0.0813 | 0.4276 | 0.3366 | 0.2368 | 0.520 |
| $a+b/\sqrt{x}\sqrt{y}+cz/y$ | 161.85 | 129.89 | 0.681 | 0.0796 | 0.0598 | 0.6869 | 0.2737 | 0.2042 | 0.683 |
| $a+b/\sqrt{x}\sqrt{y}+cz^2/y$ | 148.20 | 113.44 | 0.733 | 0.0738 | 0.0528 | 0.7308 | 0.2646 | 0.1855 | 0.703 |
| $a+b/\sqrt{x}\sqrt{y}+c\sqrt{z}/y$ | 226.34 | 165.41 | 0.377 | 0.1036 | 0.0825 | 0.4697 | 0.3534 | 0.2750 | 0.471 |
| $a+b/\sqrt{x}\sqrt{y}+c/y^2z$ | 241.17 | 175.37 | 0.292 | 0.1228 | 0.0961 | 0.2551 | 0.3963 | 0.2923 | 0.335 |
| $a+b/\sqrt{x}\sqrt{y}+c/y^2z^2$ | 240.79 | 175.07 | 0.295 | 0.1229 | 0.0959 | 0.2548 | 0.3964 | 0.2916 | 0.334 |
| $a+b/\sqrt{x}\sqrt{y}+c/y^2\sqrt{z}$ | 243.42 | 176.52 | 0.279 | 0.1233 | 0.0965 | 0.2492 | 0.3988 | 0.2944 | 0.326 |
| $a+b/\sqrt{x}\sqrt{y}+cz/y^2$ | 178.69 | 137.78 | 0.612 | 0.0880 | 0.0671 | 0.6174 | 0.2903 | 0.2251 | 0.643 |
| $a+b/\sqrt{x}\sqrt{y}+cz^2/y^2$ | 153.26 | 118.50 | 0.714 | 0.0791 | 0.0603 | 0.6907 | 0.2656 | 0.1929 | 0.701 |
| $a+b/\sqrt{x}\sqrt{y}+c\sqrt{z}/y^2$ | 256.66 | 185.92 | 0.198 | 0.1193 | 0.0921 | 0.2976 | 0.4022 | 0.2966 | 0.315 |
| $a+b/\sqrt{x}\sqrt{y}+c/\sqrt{y}z$ | 177.20 | 123.16 | 0.618 | 0.1013 | 0.0766 | 0.4935 | 0.3183 | 0.2170 | 0.571 |
| $a+b/\sqrt{x}\sqrt{y}+c/\sqrt{y}z^2$ | 209.53 | 151.78 | 0.466 | 0.1123 | 0.0869 | 0.3775 | 0.3587 | 0.2612 | 0.455 |
| $a+b/\sqrt{x}\sqrt{y}+c/\sqrt{y}\sqrt{z}$ | 157.48 | 108.84 | 0.698 | 0.0948 | 0.0708 | 0.5567 | 0.2961 | 0.1930 | 0.628 |
| $a+b/\sqrt{x}\sqrt{y}+cz/\sqrt{y}$ | 143.49 | 115.52 | 0.750 | 0.0735 | 0.0509 | 0.7331 | 0.2584 | 0.1769 | 0.717 |
| $a+b/\sqrt{x}\sqrt{y}+cz^2/\sqrt{y}$ | 146.10 | 111.09 | 0.740 | 0.0736 | 0.0509 | 0.7325 | 0.2670 | 0.1866 | 0.698 |
| $a+b/\sqrt{x}\sqrt{y}+c\sqrt{z}/\sqrt{y}$ | 169.66 | 135.03 | 0.650 | 0.0824 | 0.0619 | 0.6651 | 0.2840 | 0.2094 | 0.658 |
| $a+by/\sqrt{x}+cx/z$ | 255.20 | 196.49 | 0.208 | 0.1374 | 0.1038 | 0.0685 | 0.4688 | 0.3520 | 0.069 |
| $a+by/\sqrt{x}+cx/z^2$ | 246.51 | 191.73 | 0.261 | 0.1342 | 0.1033 | 0.1105 | 0.4580 | 0.3475 | 0.111 |
| $a+by/\sqrt{x}+cx/\sqrt{z}$ | 242.07 | 192.90 | 0.287 | 0.1304 | 0.1052 | 0.1600 | 0.4251 | 0.3332 | 0.234 |
| $a+by/\sqrt{x}+cxz$ | 126.76 | 97.52 | 0.804 | 0.0725 | 0.0528 | 0.7404 | 0.2700 | 0.2048 | 0.691 |
| $a+by/\sqrt{x}+cxz^2$ | 153.05 | 118.65 | 0.715 | 0.0852 | 0.0665 | 0.6415 | 0.3191 | 0.2514 | 0.569 |
| $a+by/\sqrt{x}+cx\sqrt{z}$ | 115.81 | 90.05 | 0.837 | 0.0685 | 0.0458 | 0.7685 | 0.2397 | 0.1625 | 0.757 |
| $a+by/\sqrt{x}+cx^2/z$ | 250.23 | 204.75 | 0.238 | 0.1351 | 0.1101 | 0.0988 | 0.4457 | 0.3560 | 0.158 |
| $a+by/\sqrt{x}+cx^2/z^2$ | 254.00 | 196.89 | 0.215 | 0.1369 | 0.1048 | 0.0747 | 0.4671 | 0.3542 | 0.076 |
| $a+by/\sqrt{x}+cx^2/\sqrt{z}$ | 183.53 | 147.99 | 0.590 | 0.1046 | 0.0828 | 0.4599 | 0.3256 | 0.2483 | 0.551 |
| $a+by/\sqrt{x}+cx^2z$ | 136.50 | 105.64 | 0.773 | 0.0791 | 0.0615 | 0.6913 | 0.2932 | 0.2333 | 0.636 |
| $a+by/\sqrt{x}+cx^2z^2$ | 160.18 | 126.97 | 0.688 | 0.0906 | 0.0724 | 0.5950 | 0.3347 | 0.2653 | 0.525 |
| $a+by/\sqrt{x}+cx^2\sqrt{z}$ | 123.25 | 96.61 | 0.815 | 0.0739 | 0.0547 | 0.7304 | 0.2657 | 0.1989 | 0.701 |
| $a+by/\sqrt{x}+c\sqrt{x}/z$ | 235.63 | 182.38 | 0.324 | 0.1294 | 0.0955 | 0.1737 | 0.4453 | 0.3280 | 0.160 |
| $a+by/\sqrt{x}+c\sqrt{x}/z^2$ | 237.78 | 183.46 | 0.312 | 0.1310 | 0.1008 | 0.1522 | 0.4452 | 0.3337 | 0.160 |
| $a+by/\sqrt{x}+c\sqrt{x}/\sqrt{z}$ | 257.60 | 200.26 | 0.193 | 0.1384 | 0.1053 | 0.0538 | 0.4694 | 0.3593 | 0.066 |
| $a+by/\sqrt{x}+c\sqrt{x}z$ | 127.29 | 100.98 | 0.803 | 0.0717 | 0.0499 | 0.7459 | 0.2666 | 0.1949 | 0.699 |
| $a+by/\sqrt{x}+c\sqrt{x}z^2$ | 151.53 | 119.24 | 0.721 | 0.0835 | 0.0640 | 0.6556 | 0.3140 | 0.2448 | 0.582 |
| $a+by/\sqrt{x}+c\sqrt{x}\sqrt{z}$ | 119.84 | 90.43 | 0.825 | 0.0689 | 0.0445 | 0.7655 | 0.2392 | 0.1510 | 0.758 |
| $a+by/\sqrt{x}+c/xz$ | 222.56 | 165.55 | 0.397 | 0.1168 | 0.0875 | 0.3268 | 0.3812 | 0.2695 | 0.384 |
| $a+by/\sqrt{x}+c/xz^2$ | 218.44 | 158.15 | 0.419 | 0.1175 | 0.0887 | 0.3181 | 0.3783 | 0.2725 | 0.394 |
| $a+by/\sqrt{x}+c/x\sqrt{z}$ | 226.84 | 172.07 | 0.374 | 0.1181 | 0.0878 | 0.3115 | 0.3888 | 0.2801 | 0.359 |
| $a+by/\sqrt{x}+cz/x$ | 248.50 | 193.24 | 0.249 | 0.1300 | 0.1003 | 0.1660 | 0.4354 | 0.3284 | 0.197 |
| $a+by/\sqrt{x}+cz^2/x$ | 252.79 | 195.43 | 0.223 | 0.1373 | 0.1025 | 0.0686 | 0.4681 | 0.3494 | 0.072 |
| $a+by/\sqrt{x}+c\sqrt{z}/x$ | 239.45 | 183.69 | 0.302 | 0.1244 | 0.0934 | 0.2365 | 0.4149 | 0.3062 | 0.271 |
| $a+by/\sqrt{x}+c/x^2z$ | 238.80 | 182.30 | 0.306 | 0.1236 | 0.0925 | 0.2453 | 0.4134 | 0.3033 | 0.276 |
| $a+by/\sqrt{x}+c/x^2z^2$ | 236.39 | 179.13 | 0.320 | 0.1229 | 0.0914 | 0.2538 | 0.4083 | 0.2971 | 0.293 |
| $a+by/\sqrt{x}+c/x^2\sqrt{z}$ | 239.77 | 183.26 | 0.301 | 0.1240 | 0.0928 | 0.2407 | 0.4156 | 0.3053 | 0.268 |
| $a+by/\sqrt{x}+cz/x^2$ | 242.17 | 184.97 | 0.286 | 0.1251 | 0.0936 | 0.2268 | 0.4212 | 0.3091 | 0.248 |
| $a+by/\sqrt{x}+cz^2/x^2$ | 244.28 | 186.74 | 0.274 | 0.1264 | 0.0949 | 0.2106 | 0.4260 | 0.3131 | 0.231 |
| $a+by/\sqrt{x}+c\sqrt{z}/x^2$ | 241.39 | 184.50 | 0.291 | 0.1247 | 0.0933 | 0.2318 | 0.4194 | 0.3080 | 0.255 |
| $a+by/\sqrt{x}+c/\sqrt{x}z$ | 190.04 | 136.76 | 0.561 | 0.1039 | 0.0794 | 0.4666 | 0.3285 | 0.2338 | 0.543 |
| $a+by/\sqrt{x}+c/\sqrt{x}z^2$ | 202.97 | 145.80 | 0.499 | 0.1146 | 0.0913 | 0.3511 | 0.3666 | 0.2731 | 0.430 |
| $a+by/\sqrt{x}+c/\sqrt{x}\sqrt{z}$ | 197.97 | 143.95 | 0.523 | 0.1051 | 0.0789 | 0.4545 | 0.3368 | 0.2343 | 0.519 |
| $a+by/\sqrt{x}+cz/\sqrt{x}$ | 241.07 | 179.81 | 0.293 | 0.1324 | 0.0948 | 0.1351 | 0.4559 | 0.3286 | 0.119 |
| $a+by/\sqrt{x}+cz^2/\sqrt{x}$ | 172.10 | 136.67 | 0.640 | 0.0955 | 0.0686 | 0.5500 | 0.3509 | 0.2635 | 0.478 |
| $a+by/\sqrt{x}+c\sqrt{z}/\sqrt{x}$ | 253.44 | 200.26 | 0.219 | 0.1340 | 0.1057 | 0.1136 | 0.4480 | 0.3463 | 0.150 |
| $a+by/\sqrt{x}+cy/z$ | 232.25 | 179.26 | 0.344 | 0.1281 | 0.0936 | 0.1903 | 0.4423 | 0.3232 | 0.171 |
| $a+by/\sqrt{x}+cy/z^2$ | 234.59 | 180.90 | 0.330 | 0.1297 | 0.0994 | 0.1698 | 0.4417 | 0.3284 | 0.173 |
| $a+by/\sqrt{x}+cy/\sqrt{z}$ | 257.25 | 199.62 | 0.195 | 0.1384 | 0.1051 | 0.0542 | 0.4695 | 0.3589 | 0.066 |
| $a+by/\sqrt{x}+cyz$ | 137.34 | 107.29 | 0.771 | 0.0759 | 0.0556 | 0.7159 | 0.2848 | 0.2157 | 0.656 |
| $a+by/\sqrt{x}+cyz^2$ | 159.22 | 123.92 | 0.692 | 0.0876 | 0.0682 | 0.6215 | 0.3276 | 0.2546 | 0.545 |
| $a+by/\sqrt{x}+cy\sqrt{z}$ | 129.52 | 99.53 | 0.796 | 0.0716 | 0.0470 | 0.7466 | 0.2579 | 0.1755 | 0.718 |
| $a+by/\sqrt{x}+cy^2/z$ | 252.57 | 194.88 | 0.224 | 0.1365 | 0.1018 | 0.0797 | 0.4672 | 0.3488 | 0.075 |
| $a+by/\sqrt{x}+cy^2/z^2$ | 240.16 | 187.21 | 0.298 | 0.1317 | 0.1001 | 0.1442 | 0.4511 | 0.3374 | 0.138 |
| $a+by/\sqrt{x}+cy^2/\sqrt{z}$ | 243.67 | 197.95 | 0.278 | 0.1300 | 0.1053 | 0.1653 | 0.4286 | 0.3352 | 0.222 |
| $a+by/\sqrt{x}+cy^2z$ | 149.57 | 112.69 | 0.728 | 0.0832 | 0.0632 | 0.6583 | 0.3098 | 0.2375 | 0.593 |
| $a+by/\sqrt{x}+cy^2z^2$ | 167.98 | 129.90 | 0.657 | 0.0933 | 0.0733 | 0.5698 | 0.3449 | 0.2658 | 0.496 |
| $a+by/\sqrt{x}+cy^2\sqrt{z}$ | 141.74 | 103.69 | 0.756 | 0.0789 | 0.0557 | 0.6926 | 0.2876 | 0.2018 | 0.650 |
| $a+by/\sqrt{x}+c\sqrt{y}/z$ | 209.71 | 156.28 | 0.465 | 0.1183 | 0.0854 | 0.3089 | 0.4068 | 0.2867 | 0.299 |
| $a+by/\sqrt{x}+c\sqrt{y}/z^2$ | 228.18 | 173.47 | 0.367 | 0.1272 | 0.0976 | 0.2008 | 0.4303 | 0.3158 | 0.215 |

(continued on next page)

**Table 4 – continued from previous page**

| Functional form | $T_{eff}$ (K) | | | Radius ($R_\odot$) | | | log (L/$L_\odot$) | | |
|---|---|---|---|---|---|---|---|---|---|
| | RMSE | MAD | $R^2_{ap}$ | RMSE | MAD | $R^2_{ap}$ | RMSE | MAD | $R^2_{ap}$ |
| $a+by/\sqrt{x}+c\sqrt{y}/\sqrt{z}$ | 230.63 | 176.38 | 0.353 | 0.1273 | 0.0916 | 0.1997 | 0.4410 | 0.3205 | 0.176 |
| $a+by/\sqrt{x}+c\sqrt{y}z$ | 134.17 | 107.16 | 0.781 | 0.0744 | 0.0526 | 0.7267 | 0.2786 | 0.2069 | 0.671 |
| $a+by/\sqrt{x}+c\sqrt{y}z^2$ | 155.54 | 123.14 | 0.706 | 0.0852 | 0.0652 | 0.6416 | 0.3201 | 0.2476 | 0.566 |
| $a+by/\sqrt{x}+c\sqrt{y}\sqrt{z}$ | 125.69 | 99.13 | 0.808 | 0.0703 | 0.0441 | 0.7557 | 0.2518 | 0.1609 | 0.731 |
| $a+by/\sqrt{x}+c/yz$ | 197.93 | 138.48 | 0.523 | 0.1103 | 0.0851 | 0.3994 | 0.3463 | 0.2496 | 0.492 |
| $a+by/\sqrt{x}+c/yz^2$ | 212.86 | 155.62 | 0.449 | 0.1203 | 0.0966 | 0.2848 | 0.3856 | 0.2937 | 0.370 |
| $a+by/\sqrt{x}+c/y\sqrt{z}$ | 200.17 | 145.02 | 0.512 | 0.1088 | 0.0813 | 0.4158 | 0.3430 | 0.2414 | 0.501 |
| $a+by/\sqrt{x}+cz/y$ | 240.37 | 180.20 | 0.297 | 0.1319 | 0.0950 | 0.1404 | 0.4547 | 0.3280 | 0.124 |
| $a+by/\sqrt{x}+cz^2/y$ | 168.97 | 132.07 | 0.653 | 0.0942 | 0.0673 | 0.5618 | 0.3443 | 0.2562 | 0.498 |
| $a+by/\sqrt{x}+c\sqrt{z}/y$ | 252.91 | 199.19 | 0.222 | 0.1340 | 0.1059 | 0.1133 | 0.4464 | 0.3450 | 0.156 |
| $a+by/\sqrt{x}+c/y^2z$ | 224.36 | 163.53 | 0.388 | 0.1217 | 0.0953 | 0.2691 | 0.3909 | 0.2897 | 0.353 |
| $a+by/\sqrt{x}+c/y^2z^2$ | 228.78 | 168.48 | 0.363 | 0.1260 | 0.0992 | 0.2160 | 0.4064 | 0.3049 | 0.300 |
| $a+by/\sqrt{x}+c/y^2\sqrt{z}$ | 224.72 | 165.23 | 0.386 | 0.1204 | 0.0930 | 0.2841 | 0.3882 | 0.2828 | 0.361 |
| $a+by/\sqrt{x}+cz/y^2$ | 247.04 | 190.47 | 0.257 | 0.1298 | 0.1006 | 0.1675 | 0.4317 | 0.3245 | 0.211 |
| $a+by/\sqrt{x}+cz^2/y^2$ | 250.66 | 192.17 | 0.236 | 0.1365 | 0.1007 | 0.0803 | 0.4660 | 0.3433 | 0.080 |
| $a+by/\sqrt{x}+c\sqrt{z}/y^2$ | 235.74 | 176.56 | 0.324 | 0.1238 | 0.0939 | 0.2428 | 0.4069 | 0.2934 | 0.298 |
| $a+by/\sqrt{x}+c/\sqrt{y}z$ | 176.23 | 121.80 | 0.622 | 0.1019 | 0.0776 | 0.4871 | 0.3211 | 0.2198 | 0.563 |
| $a+by/\sqrt{x}+c/\sqrt{y}z^2$ | 210.44 | 150.22 | 0.461 | 0.1200 | 0.0940 | 0.2895 | 0.3905 | 0.2833 | 0.354 |
| $a+by/\sqrt{x}+c/\sqrt{y}\sqrt{z}$ | 168.32 | 118.94 | 0.655 | 0.0948 | 0.0707 | 0.5565 | 0.2951 | 0.1966 | 0.631 |
| $a+by/\sqrt{x}+cz/\sqrt{y}$ | 169.39 | 131.52 | 0.651 | 0.0962 | 0.0671 | 0.5434 | 0.3466 | 0.2459 | 0.491 |
| $a+by/\sqrt{x}+cz^2/\sqrt{y}$ | 155.76 | 126.00 | 0.705 | 0.0858 | 0.0636 | 0.6365 | 0.3200 | 0.2493 | 0.566 |
| $a+by/\sqrt{x}+c\sqrt{z}/\sqrt{y}$ | 235.30 | 177.03 | 0.326 | 0.1296 | 0.0927 | 0.1713 | 0.4482 | 0.3235 | 0.149 |
| $a+by^2/\sqrt{x}+cx/z$ | 182.45 | 139.47 | 0.595 | 0.1048 | 0.0775 | 0.4578 | 0.3549 | 0.2492 | 0.466 |
| $a+by^2/\sqrt{x}+cx/z^2$ | 182.99 | 144.37 | 0.593 | 0.1054 | 0.0783 | 0.4517 | 0.3535 | 0.2519 | 0.470 |
| $a+by^2/\sqrt{x}+cx/\sqrt{z}$ | 190.87 | 149.86 | 0.557 | 0.1073 | 0.0773 | 0.4310 | 0.3552 | 0.2489 | 0.465 |
| $a+by^2/\sqrt{x}+cxz$ | 126.04 | 97.48 | 0.807 | 0.0733 | 0.0527 | 0.7344 | 0.2692 | 0.2051 | 0.693 |
| $a+by^2/\sqrt{x}+cxz^2$ | 142.44 | 109.56 | 0.753 | 0.0827 | 0.0617 | 0.6622 | 0.3010 | 0.2285 | 0.616 |
| $a+by^2/\sqrt{x}+cx\sqrt{z}$ | 117.06 | 90.81 | 0.833 | 0.0680 | 0.0462 | 0.7718 | 0.2397 | 0.1640 | 0.757 |
| $a+by^2/\sqrt{x}+cx^2/z$ | 190.78 | 148.99 | 0.557 | 0.1073 | 0.0777 | 0.4320 | 0.3569 | 0.2513 | 0.460 |
| $a+by^2/\sqrt{x}+cx^2/z^2$ | 186.50 | 146.46 | 0.577 | 0.1061 | 0.0784 | 0.4443 | 0.3566 | 0.2510 | 0.461 |
| $a+by^2/\sqrt{x}+cx^2/\sqrt{z}$ | 176.91 | 145.64 | 0.619 | 0.1005 | 0.0772 | 0.5013 | 0.3172 | 0.2386 | 0.574 |
| $a+by^2/\sqrt{x}+cx^2z$ | 133.57 | 102.92 | 0.783 | 0.0794 | 0.0594 | 0.6888 | 0.2882 | 0.2223 | 0.648 |
| $a+by^2/\sqrt{x}+cx^2z^2$ | 147.38 | 113.30 | 0.736 | 0.0868 | 0.0643 | 0.6282 | 0.3116 | 0.2307 | 0.589 |
| $a+by^2/\sqrt{x}+cx^2\sqrt{z}$ | 123.77 | 96.74 | 0.814 | 0.0748 | 0.0553 | 0.7236 | 0.2675 | 0.2029 | 0.697 |
| $a+by^2/\sqrt{x}+c\sqrt{x}/z$ | 172.62 | 132.59 | 0.637 | 0.1019 | 0.0751 | 0.4871 | 0.3451 | 0.2426 | 0.495 |
| $a+by^2/\sqrt{x}+c\sqrt{x}/z^2$ | 179.65 | 141.46 | 0.607 | 0.1047 | 0.0776 | 0.4588 | 0.3498 | 0.2503 | 0.482 |
| $a+by^2/\sqrt{x}+c\sqrt{x}/\sqrt{z}$ | 181.25 | 137.57 | 0.600 | 0.1050 | 0.0776 | 0.4554 | 0.3554 | 0.2491 | 0.465 |
| $a+by^2/\sqrt{x}+c\sqrt{x}z$ | 126.28 | 99.54 | 0.806 | 0.0724 | 0.0492 | 0.7410 | 0.2654 | 0.1958 | 0.702 |
| $a+by^2/\sqrt{x}+c\sqrt{x}z^2$ | 140.98 | 108.13 | 0.758 | 0.0812 | 0.0602 | 0.6746 | 0.2966 | 0.2249 | 0.627 |
| $a+by^2/\sqrt{x}+c\sqrt{x}\sqrt{z}$ | 122.05 | 91.60 | 0.819 | 0.0685 | 0.0442 | 0.7683 | 0.2391 | 0.1501 | 0.758 |
| $a+by^2/\sqrt{x}+c/xz$ | 190.97 | 152.31 | 0.556 | 0.1052 | 0.0757 | 0.4539 | 0.3457 | 0.2377 | 0.494 |
| $a+by^2/\sqrt{x}+c/xz^2$ | 189.15 | 148.90 | 0.565 | 0.1050 | 0.0761 | 0.4556 | 0.3415 | 0.2318 | 0.506 |
| $a+by^2/\sqrt{x}+c/x\sqrt{z}$ | 191.13 | 152.00 | 0.556 | 0.1056 | 0.0757 | 0.4494 | 0.3490 | 0.2420 | 0.484 |
| $a+by^2/\sqrt{x}+cz/x$ | 186.96 | 144.05 | 0.575 | 0.1073 | 0.0771 | 0.4312 | 0.3577 | 0.2466 | 0.458 |
| $a+by^2/\sqrt{x}+cz^2/x$ | 170.22 | 125.33 | 0.647 | 0.1036 | 0.0745 | 0.4706 | 0.3497 | 0.2407 | 0.482 |
| $a+by^2/\sqrt{x}+c\sqrt{z}/x$ | 189.63 | 147.25 | 0.562 | 0.1068 | 0.0758 | 0.4363 | 0.3554 | 0.2437 | 0.465 |
| $a+by^2/\sqrt{x}+c/x^2z$ | 189.84 | 148.01 | 0.562 | 0.1067 | 0.0759 | 0.4381 | 0.3550 | 0.2436 | 0.466 |
| $a+by^2/\sqrt{x}+c/x^2z^2$ | 190.40 | 149.59 | 0.559 | 0.1066 | 0.0756 | 0.4390 | 0.3539 | 0.2430 | 0.469 |
| $a+by^2/\sqrt{x}+c/x^2\sqrt{z}$ | 189.62 | 147.41 | 0.563 | 0.1067 | 0.0760 | 0.4377 | 0.3554 | 0.2437 | 0.465 |
| $a+by^2/\sqrt{x}+cz/x^2$ | 189.06 | 145.99 | 0.565 | 0.1068 | 0.0759 | 0.4363 | 0.3563 | 0.2434 | 0.462 |
| $a+by^2/\sqrt{x}+cz^2/x^2$ | 188.50 | 145.24 | 0.568 | 0.1070 | 0.0762 | 0.4346 | 0.3569 | 0.2437 | 0.460 |
| $a+by^2/\sqrt{x}+c\sqrt{z}/x^2$ | 189.24 | 146.45 | 0.564 | 0.1068 | 0.0760 | 0.4368 | 0.3560 | 0.2436 | 0.463 |
| $a+by^2/\sqrt{x}+c/\sqrt{x}z$ | 179.15 | 132.66 | 0.610 | 0.0991 | 0.0741 | 0.5155 | 0.3159 | 0.2183 | 0.577 |
| $a+by^2/\sqrt{x}+c/\sqrt{x}z^2$ | 177.66 | 135.71 | 0.616 | 0.1028 | 0.0769 | 0.4780 | 0.3308 | 0.2271 | 0.536 |
| $a+by^2/\sqrt{x}+c/\sqrt{x}\sqrt{z}$ | 185.57 | 144.72 | 0.581 | 0.1004 | 0.0743 | 0.5022 | 0.3246 | 0.2199 | 0.553 |
| $a+by^2/\sqrt{x}+cz/\sqrt{x}$ | 163.93 | 120.43 | 0.673 | 0.1006 | 0.0714 | 0.5002 | 0.3426 | 0.2324 | 0.503 |
| $a+by^2/\sqrt{x}+cz^2/\sqrt{x}$ | 143.39 | 111.49 | 0.750 | 0.0862 | 0.0593 | 0.6332 | 0.3079 | 0.2193 | 0.598 |
| $a+by^2/\sqrt{x}+c\sqrt{z}/\sqrt{x}$ | 184.84 | 141.04 | 0.584 | 0.1072 | 0.0779 | 0.4327 | 0.3580 | 0.2491 | 0.457 |
| $a+by^2/\sqrt{x}+cy/z$ | 162.97 | 121.23 | 0.677 | 0.0972 | 0.0693 | 0.5336 | 0.3326 | 0.2263 | 0.531 |
| $a+by^2/\sqrt{x}+cy/z^2$ | 176.21 | 138.73 | 0.622 | 0.1032 | 0.0763 | 0.4746 | 0.3456 | 0.2465 | 0.494 |
| $a+by^2/\sqrt{x}+cy/\sqrt{z}$ | 165.51 | 122.10 | 0.667 | 0.0980 | 0.0695 | 0.5259 | 0.3390 | 0.2287 | 0.513 |
| $a+by^2/\sqrt{x}+cyz$ | 136.61 | 106.30 | 0.773 | 0.0788 | 0.0576 | 0.6932 | 0.2894 | 0.2188 | 0.645 |
| $a+by^2/\sqrt{x}+cyz^2$ | 148.27 | 113.20 | 0.733 | 0.0856 | 0.0629 | 0.6379 | 0.3101 | 0.2291 | 0.593 |
| $a+by^2/\sqrt{x}+cy\sqrt{z}$ | 126.58 | 99.27 | 0.805 | 0.0727 | 0.0490 | 0.7392 | 0.2656 | 0.1923 | 0.701 |
| $a+by^2/\sqrt{x}+cy^2/z$ | 163.15 | 118.89 | 0.676 | 0.0956 | 0.0659 | 0.5484 | 0.3324 | 0.2206 | 0.532 |
| $a+by^2/\sqrt{x}+cy^2/z^2$ | 174.89 | 136.75 | 0.628 | 0.1019 | 0.0750 | 0.4870 | 0.3444 | 0.2429 | 0.497 |
| $a+by^2/\sqrt{x}+cy^2/\sqrt{z}$ | 169.61 | 125.39 | 0.650 | 0.0979 | 0.0671 | 0.5270 | 0.3412 | 0.2270 | 0.507 |
| $a+by^2/\sqrt{x}+cy^2z$ | 148.27 | 110.56 | 0.733 | 0.0864 | 0.0634 | 0.6314 | 0.3122 | 0.2301 | 0.587 |
| $a+by^2/\sqrt{x}+cy^2z^2$ | 155.29 | 116.61 | 0.707 | 0.0905 | 0.0663 | 0.5958 | 0.3229 | 0.2328 | 0.558 |
| $a+by^2/\sqrt{x}+cy^2\sqrt{z}$ | 142.44 | 105.95 | 0.753 | 0.0835 | 0.0601 | 0.6560 | 0.3025 | 0.2228 | 0.612 |
| $a+by^2/\sqrt{x}+c\sqrt{y}/z$ | 159.77 | 118.95 | 0.689 | 0.0966 | 0.0685 | 0.5393 | 0.3265 | 0.2217 | 0.548 |
| $a+by^2/\sqrt{x}+c\sqrt{y}/z^2$ | 175.69 | 137.90 | 0.624 | 0.1034 | 0.0762 | 0.4724 | 0.3442 | 0.2455 | 0.498 |
| $a+by^2/\sqrt{x}+c\sqrt{y}/\sqrt{z}$ | 157.31 | 115.95 | 0.699 | 0.0951 | 0.0665 | 0.5530 | 0.3276 | 0.2203 | 0.545 |
| $a+by^2/\sqrt{x}+c\sqrt{y}z$ | 132.22 | 105.68 | 0.787 | 0.0765 | 0.0535 | 0.7114 | 0.2800 | 0.2079 | 0.668 |
| $a+by^2/\sqrt{x}+c\sqrt{y}z^2$ | 144.38 | 110.40 | 0.746 | 0.0831 | 0.0611 | 0.6591 | 0.3026 | 0.2262 | 0.612 |
| $a+by^2/\sqrt{x}+c\sqrt{y}\sqrt{z}$ | 125.18 | 99.57 | 0.809 | 0.0723 | 0.0457 | 0.7416 | 0.2594 | 0.1756 | 0.715 |
| $a+by^2/\sqrt{x}+c/yz$ | 179.19 | 135.09 | 0.609 | 0.1025 | 0.0756 | 0.4815 | 0.3264 | 0.2214 | 0.549 |
| $a+by^2/\sqrt{x}+c/yz^2$ | 179.64 | 137.17 | 0.607 | 0.1048 | 0.0782 | 0.4575 | 0.3387 | 0.2384 | 0.514 |
| $a+by^2/\sqrt{x}+c/y\sqrt{z}$ | 183.81 | 140.12 | 0.589 | 0.1026 | 0.0749 | 0.4801 | 0.3280 | 0.2234 | 0.544 |
| $a+by^2/\sqrt{x}+cz/y$ | 152.77 | 113.59 | 0.716 | 0.0953 | 0.0659 | 0.5517 | 0.3281 | 0.2217 | 0.544 |
| $a+by^2/\sqrt{x}+cz^2/y$ | 135.88 | 106.16 | 0.775 | 0.0818 | 0.0552 | 0.6700 | 0.2932 | 0.2119 | 0.636 |
| $a+by^2/\sqrt{x}+c\sqrt{z}/y$ | 180.83 | 138.96 | 0.602 | 0.1060 | 0.0782 | 0.4453 | 0.3567 | 0.2505 | 0.461 |
| $a+by^2/\sqrt{x}+c/y^2z$ | 188.91 | 148.18 | 0.566 | 0.1060 | 0.0764 | 0.4455 | 0.3445 | 0.2312 | 0.497 |
| $a+by^2/\sqrt{x}+c/y^2z^2$ | 187.00 | 144.07 | 0.575 | 0.1064 | 0.0772 | 0.4410 | 0.3463 | 0.2379 | 0.492 |
| $a+by^2/\sqrt{x}+c/y^2\sqrt{z}$ | 190.22 | 150.92 | 0.560 | 0.1060 | 0.0759 | 0.4452 | 0.3458 | 0.2335 | 0.493 |
| $a+by^2/\sqrt{x}+cz/y^2$ | 186.01 | 142.97 | 0.579 | 0.1073 | 0.0779 | 0.4318 | 0.3580 | 0.2479 | 0.457 |
| $a+by^2/\sqrt{x}+cz^2/y^2$ | 158.78 | 115.79 | 0.693 | 0.0990 | 0.0701 | 0.5157 | 0.3373 | 0.2298 | 0.518 |
| $a+by^2/\sqrt{x}+c\sqrt{z}/y^2$ | 190.38 | 149.72 | 0.559 | 0.1071 | 0.0761 | 0.4339 | 0.3545 | 0.2421 | 0.467 |
| $a+by^2/\sqrt{x}+c/\sqrt{y}z$ | 164.17 | 123.43 | 0.672 | 0.0977 | 0.0727 | 0.5287 | 0.3106 | 0.2082 | 0.591 |
| $a+by^2/\sqrt{x}+c/\sqrt{y}z^2$ | 175.44 | 133.54 | 0.626 | 0.1038 | 0.0776 | 0.4678 | 0.3378 | 0.2351 | 0.516 |

(continued on next page)

**Table 4 – continued from previous page**

| Functional form | $T_{eff}$ (K) | | | Radius ($R_{\odot}$) | | | log (L/$L_{\odot}$) | | |
|---|---|---|---|---|---|---|---|---|---|
| | RMSE | MAD | $R^2_{ap}$ | RMSE | MAD | $R^2_{ap}$ | RMSE | MAD | $R^2_{ap}$ |
| $a+by^2/\sqrt{x}+c/\sqrt{y}\sqrt{z}$ | 164.21 | 120.93 | 0.672 | 0.0945 | 0.0692 | 0.5591 | 0.2966 | 0.1927 | 0.627 |
| $a+by^2/\sqrt{x}+cz/\sqrt{y}$ | 134.02 | 105.64 | 0.781 | 0.0827 | 0.0531 | 0.6623 | 0.2927 | 0.2029 | 0.637 |
| $a+by^2/\sqrt{x}+cz^2/\sqrt{y}$ | 137.31 | 107.83 | 0.771 | 0.0800 | 0.0560 | 0.6837 | 0.2909 | 0.2148 | 0.641 |
| $a+by^2/\sqrt{x}+c\sqrt{z}/\sqrt{y}$ | 151.96 | 113.58 | 0.719 | 0.0942 | 0.0650 | 0.5621 | 0.3253 | 0.2198 | 0.552 |
| $a+b\sqrt{y}/\sqrt{x}+cx/z$ | 243.54 | 172.22 | 0.278 | 0.1136 | 0.0867 | 0.3625 | 0.3932 | 0.2960 | 0.345 |
| $a+b\sqrt{y}/\sqrt{x}+cx/z^2$ | 241.12 | 174.87 | 0.293 | 0.1167 | 0.0901 | 0.3271 | 0.3937 | 0.2906 | 0.343 |
| $a+b\sqrt{y}/\sqrt{x}+cx/\sqrt{z}$ | 273.62 | 204.87 | 0.089 | 0.1298 | 0.1022 | 0.1679 | 0.4339 | 0.3335 | 0.202 |
| $a+b\sqrt{y}/\sqrt{x}+cxz$ | 128.13 | 95.47 | 0.800 | 0.0702 | 0.0482 | 0.7567 | 0.2542 | 0.1810 | 0.726 |
| $a+b\sqrt{y}/\sqrt{x}+cxz^2$ | 150.02 | 110.74 | 0.726 | 0.0764 | 0.0569 | 0.7120 | 0.2811 | 0.2059 | 0.665 |
| $a+b\sqrt{y}/\sqrt{x}+cx\sqrt{z}$ | 113.67 | 87.02 | 0.843 | 0.0694 | 0.0446 | 0.7620 | 0.2393 | 0.1584 | 0.757 |
| $a+b\sqrt{y}/\sqrt{x}+cx^2/z$ | 274.66 | 203.68 | 0.082 | 0.1297 | 0.1016 | 0.1697 | 0.4347 | 0.3331 | 0.199 |
| $a+b\sqrt{y}/\sqrt{x}+cx^2/z^2$ | 255.55 | 183.50 | 0.205 | 0.1212 | 0.0932 | 0.2744 | 0.4122 | 0.3078 | 0.280 |
| $a+b\sqrt{y}/\sqrt{x}+cx^2/\sqrt{z}$ | 189.30 | 149.58 | 0.564 | 0.1052 | 0.0833 | 0.4531 | 0.3277 | 0.2544 | 0.545 |
| $a+b\sqrt{y}/\sqrt{x}+cx^2z$ | 135.59 | 103.13 | 0.776 | 0.0739 | 0.0545 | 0.7301 | 0.2670 | 0.1990 | 0.698 |
| $a+b\sqrt{y}/\sqrt{x}+cx^2z^2$ | 155.13 | 118.32 | 0.707 | 0.0801 | 0.0621 | 0.6832 | 0.2915 | 0.2215 | 0.640 |
| $a+b\sqrt{y}/\sqrt{x}+cx^2\sqrt{z}$ | 124.03 | 95.87 | 0.813 | 0.0726 | 0.0519 | 0.7400 | 0.2538 | 0.1837 | 0.727 |
| $a+b\sqrt{y}/\sqrt{x}+c\sqrt{x}/z$ | 208.63 | 151.03 | 0.470 | 0.1019 | 0.0761 | 0.4871 | 0.3479 | 0.2520 | 0.487 |
| $a+b\sqrt{y}/\sqrt{x}+c\sqrt{x}/z^2$ | 228.95 | 168.96 | 0.362 | 0.1135 | 0.0874 | 0.3645 | 0.3782 | 0.2775 | 0.394 |
| $a+b\sqrt{y}/\sqrt{x}+c\sqrt{x}/\sqrt{z}$ | 234.22 | 166.72 | 0.333 | 0.1081 | 0.0837 | 0.4233 | 0.3781 | 0.2848 | 0.394 |
| $a+b\sqrt{y}/\sqrt{x}+c\sqrt{x}z$ | 129.32 | 99.74 | 0.797 | 0.0698 | 0.0458 | 0.7594 | 0.2527 | 0.1712 | 0.730 |
| $a+b\sqrt{y}/\sqrt{x}+c\sqrt{x}z^2$ | 149.35 | 112.38 | 0.729 | 0.0752 | 0.0543 | 0.7210 | 0.2777 | 0.1984 | 0.673 |
| $a+b\sqrt{y}/\sqrt{x}+c\sqrt{x}\sqrt{z}$ | 116.39 | 89.36 | 0.835 | 0.0696 | 0.0418 | 0.7607 | 0.2396 | 0.1476 | 0.757 |
| $a+b\sqrt{y}/\sqrt{x}+c/xz$ | 250.93 | 180.02 | 0.234 | 0.1242 | 0.0965 | 0.2383 | 0.4078 | 0.3010 | 0.295 |
| $a+b\sqrt{y}/\sqrt{x}+c/xz^2$ | 239.26 | 170.53 | 0.304 | 0.1215 | 0.0935 | 0.2706 | 0.3929 | 0.2833 | 0.346 |
| $a+b\sqrt{y}/\sqrt{x}+c/x\sqrt{z}$ | 266.30 | 198.46 | 0.137 | 0.1281 | 0.1023 | 0.1902 | 0.4267 | 0.3256 | 0.229 |
| $a+b\sqrt{y}/\sqrt{x}+cz/x$ | 197.44 | 148.62 | 0.526 | 0.0991 | 0.0761 | 0.5146 | 0.3217 | 0.2422 | 0.562 |
| $a+b\sqrt{y}/\sqrt{x}+cz^2/x$ | 141.14 | 108.47 | 0.758 | 0.0736 | 0.0525 | 0.7323 | 0.2552 | 0.1834 | 0.724 |
| $a+b\sqrt{y}/\sqrt{x}+c\sqrt{z}/x$ | 247.15 | 182.48 | 0.257 | 0.1185 | 0.0911 | 0.3070 | 0.3906 | 0.2960 | 0.354 |
| $a+b\sqrt{y}/\sqrt{x}+c/x^2z$ | 249.92 | 182.54 | 0.240 | 0.1208 | 0.0932 | 0.2796 | 0.3955 | 0.3030 | 0.337 |
| $a+b\sqrt{y}/\sqrt{x}+c/x^2z^2$ | 269.91 | 194.84 | 0.114 | 0.1269 | 0.0985 | 0.2052 | 0.4249 | 0.3198 | 0.235 |
| $a+b\sqrt{y}/\sqrt{x}+c/x^2\sqrt{z}$ | 242.98 | 177.34 | 0.282 | 0.1192 | 0.0907 | 0.2989 | 0.3863 | 0.2929 | 0.368 |
| $a+b\sqrt{y}/\sqrt{x}+cz/x^2$ | 232.35 | 164.64 | 0.343 | 0.1168 | 0.0865 | 0.3269 | 0.3729 | 0.2739 | 0.411 |
| $a+b\sqrt{y}/\sqrt{x}+cz^2/x^2$ | 223.07 | 157.19 | 0.395 | 0.1136 | 0.0858 | 0.3625 | 0.3604 | 0.2642 | 0.450 |
| $a+b\sqrt{y}/\sqrt{x}+c\sqrt{z}/x^2$ | 235.27 | 168.25 | 0.327 | 0.1175 | 0.0875 | 0.3182 | 0.3767 | 0.2792 | 0.399 |
| $a+b\sqrt{y}/\sqrt{x}+c/\sqrt{x}z$ | 189.93 | 136.92 | 0.561 | 0.1045 | 0.0798 | 0.4611 | 0.3292 | 0.2350 | 0.541 |
| $a+b\sqrt{y}/\sqrt{x}+c/\sqrt{x}z^2$ | 212.14 | 155.34 | 0.452 | 0.1124 | 0.0870 | 0.3762 | 0.3582 | 0.2618 | 0.456 |
| $a+b\sqrt{y}/\sqrt{x}+c/\sqrt{x}\sqrt{z}$ | 186.96 | 130.00 | 0.575 | 0.1029 | 0.0775 | 0.4768 | 0.3261 | 0.2263 | 0.549 |
| $a+b\sqrt{y}/\sqrt{x}+cz/\sqrt{x}$ | 147.78 | 116.74 | 0.734 | 0.0746 | 0.0544 | 0.7253 | 0.2631 | 0.1920 | 0.707 |
| $a+b\sqrt{y}/\sqrt{x}+cz^2/\sqrt{x}$ | 148.84 | 110.39 | 0.730 | 0.0736 | 0.0535 | 0.7324 | 0.2704 | 0.1941 | 0.690 |
| $a+b\sqrt{y}/\sqrt{x}+c\sqrt{z}/\sqrt{x}$ | 199.78 | 151.54 | 0.514 | 0.0945 | 0.0745 | 0.5586 | 0.3248 | 0.2469 | 0.553 |
| $a+b\sqrt{y}/\sqrt{x}+cy/z$ | 230.06 | 166.55 | 0.356 | 0.1085 | 0.0829 | 0.4186 | 0.3731 | 0.2804 | 0.410 |
| $a+b\sqrt{y}/\sqrt{x}+cy/z^2$ | 232.47 | 169.35 | 0.342 | 0.1139 | 0.0870 | 0.3595 | 0.3819 | 0.2810 | 0.382 |
| $a+b\sqrt{y}/\sqrt{x}+cy/\sqrt{z}$ | 272.48 | 198.52 | 0.097 | 0.1266 | 0.0958 | 0.2089 | 0.4299 | 0.3238 | 0.217 |
| $a+b\sqrt{y}/\sqrt{x}+cyz$ | 135.29 | 105.62 | 0.777 | 0.0737 | 0.0494 | 0.7319 | 0.2653 | 0.1844 | 0.702 |
| $a+b\sqrt{y}/\sqrt{x}+cyz^2$ | 152.71 | 115.96 | 0.716 | 0.0779 | 0.0572 | 0.7007 | 0.2855 | 0.2066 | 0.655 |
| $a+b\sqrt{y}/\sqrt{x}+cy\sqrt{z}$ | 131.25 | 100.79 | 0.790 | 0.0763 | 0.0481 | 0.7124 | 0.2631 | 0.1653 | 0.707 |
| $a+b\sqrt{y}/\sqrt{x}+cy^2/z$ | 270.86 | 197.02 | 0.107 | 0.1257 | 0.0947 | 0.2201 | 0.4276 | 0.3215 | 0.225 |
| $a+b\sqrt{y}/\sqrt{x}+cy^2/z^2$ | 245.95 | 175.34 | 0.264 | 0.1173 | 0.0885 | 0.3212 | 0.3979 | 0.2958 | 0.329 |
| $a+b\sqrt{y}/\sqrt{x}+cy^2/\sqrt{z}$ | 246.22 | 201.00 | 0.262 | 0.1234 | 0.1008 | 0.2478 | 0.4045 | 0.3234 | 0.307 |
| $a+b\sqrt{y}/\sqrt{x}+cy^2z$ | 144.74 | 110.39 | 0.745 | 0.0787 | 0.0552 | 0.6939 | 0.2816 | 0.1977 | 0.664 |
| $a+b\sqrt{y}/\sqrt{x}+cy^2z^2$ | 158.63 | 119.85 | 0.694 | 0.0820 | 0.0618 | 0.6677 | 0.2973 | 0.2189 | 0.625 |
| $a+b\sqrt{y}/\sqrt{x}+cy^2\sqrt{z}$ | 143.02 | 104.83 | 0.751 | 0.0812 | 0.0559 | 0.6748 | 0.2813 | 0.1829 | 0.665 |
| $a+b\sqrt{y}/\sqrt{x}+c\sqrt{y}/z$ | 199.29 | 145.23 | 0.517 | 0.0992 | 0.0737 | 0.5142 | 0.3351 | 0.2414 | 0.524 |
| $a+b\sqrt{y}/\sqrt{x}+c\sqrt{y}/z^2$ | 223.22 | 165.30 | 0.394 | 0.1119 | 0.0854 | 0.3821 | 0.3707 | 0.2704 | 0.418 |
| $a+b\sqrt{y}/\sqrt{x}+c\sqrt{y}/\sqrt{z}$ | 221.45 | 161.24 | 0.403 | 0.1037 | 0.0806 | 0.4695 | 0.3592 | 0.2708 | 0.453 |
| $a+b\sqrt{y}/\sqrt{x}+c\sqrt{y}z$ | 132.66 | 105.45 | 0.786 | 0.0715 | 0.0465 | 0.7477 | 0.2581 | 0.1745 | 0.718 |
| $a+b\sqrt{y}/\sqrt{x}+c\sqrt{y}z^2$ | 150.63 | 115.40 | 0.724 | 0.0759 | 0.0548 | 0.7152 | 0.2799 | 0.1997 | 0.668 |
| $a+b\sqrt{y}/\sqrt{x}+c\sqrt{y}\sqrt{z}$ | 125.93 | 99.61 | 0.807 | 0.0732 | 0.0438 | 0.7352 | 0.2527 | 0.1570 | 0.729 |
| $a+b\sqrt{y}/\sqrt{x}+c/yz$ | 202.17 | 143.81 | 0.503 | 0.1094 | 0.0835 | 0.4092 | 0.3436 | 0.2486 | 0.500 |
| $a+b\sqrt{y}/\sqrt{x}+c/yz^2$ | 215.93 | 157.81 | 0.433 | 0.1142 | 0.0882 | 0.3561 | 0.3624 | 0.2669 | 0.444 |
| $a+b\sqrt{y}/\sqrt{x}+c/y\sqrt{z}$ | 201.90 | 140.97 | 0.504 | 0.1090 | 0.0827 | 0.4134 | 0.3434 | 0.2431 | 0.500 |
| $a+b\sqrt{y}/\sqrt{x}+cz/y$ | 202.81 | 150.88 | 0.500 | 0.0937 | 0.0742 | 0.5664 | 0.3284 | 0.2515 | 0.543 |
| $a+b\sqrt{y}/\sqrt{x}+cz^2/y$ | 158.93 | 119.94 | 0.693 | 0.0760 | 0.0589 | 0.7151 | 0.2774 | 0.2092 | 0.674 |
| $a+b\sqrt{y}/\sqrt{x}+c\sqrt{z}/y$ | 273.79 | 199.56 | 0.088 | 0.1277 | 0.0974 | 0.1948 | 0.4318 | 0.3247 | 0.210 |
| $a+b\sqrt{y}/\sqrt{x}+c/y^2z$ | 241.46 | 175.83 | 0.291 | 0.1221 | 0.0954 | 0.2633 | 0.3938 | 0.2910 | 0.343 |
| $a+b\sqrt{y}/\sqrt{x}+c/y^2z^2$ | 240.31 | 175.27 | 0.297 | 0.1220 | 0.0947 | 0.2646 | 0.3926 | 0.2884 | 0.347 |
| $a+b\sqrt{y}/\sqrt{x}+c/y^2\sqrt{z}$ | 244.52 | 176.61 | 0.273 | 0.1229 | 0.0961 | 0.2545 | 0.3979 | 0.2938 | 0.329 |
| $a+b\sqrt{y}/\sqrt{x}+cz/y^2$ | 272.56 | 198.24 | 0.096 | 0.1272 | 0.0977 | 0.2015 | 0.4293 | 0.3241 | 0.219 |
| $a+b\sqrt{y}/\sqrt{x}+cz^2/y^2$ | 197.03 | 149.65 | 0.528 | 0.0920 | 0.0723 | 0.5822 | 0.3190 | 0.2465 | 0.569 |
| $a+b\sqrt{y}/\sqrt{x}+c\sqrt{z}/y^2$ | 267.84 | 201.56 | 0.127 | 0.1290 | 0.1030 | 0.1789 | 0.4282 | 0.3298 | 0.223 |
| $a+b\sqrt{y}/\sqrt{x}+c/\sqrt{y}z$ | 177.62 | 126.15 | 0.616 | 0.0996 | 0.0751 | 0.5097 | 0.3124 | 0.2147 | 0.586 |
| $a+b\sqrt{y}/\sqrt{x}+c/\sqrt{y}z^2$ | 208.97 | 150.87 | 0.469 | 0.1107 | 0.0847 | 0.3949 | 0.3538 | 0.2529 | 0.470 |
| $a+b\sqrt{y}/\sqrt{x}+c/\sqrt{y}\sqrt{z}$ | 165.10 | 115.59 | 0.668 | 0.0952 | 0.0710 | 0.5524 | 0.2972 | 0.1975 | 0.626 |
| $a+b\sqrt{y}/\sqrt{x}+cz/\sqrt{y}$ | 155.63 | 121.54 | 0.705 | 0.0760 | 0.0577 | 0.7146 | 0.2728 | 0.2038 | 0.685 |
| $a+b\sqrt{y}/\sqrt{x}+cz^2/\sqrt{y}$ | 152.09 | 113.38 | 0.719 | 0.0742 | 0.0547 | 0.7283 | 0.2737 | 0.1973 | 0.682 |
| $a+b\sqrt{y}/\sqrt{x}+c\sqrt{z}/\sqrt{y}$ | 207.50 | 153.99 | 0.476 | 0.0960 | 0.0761 | 0.5454 | 0.3362 | 0.2564 | 0.521 |
| Different EW ratio, double component functions result (y/z, x/z) | | | | | | | | | |
| $a+by/z+cx/z$ | 229.74 | 171.63 | 0.358 | 0.1161 | 0.0930 | 0.3350 | 0.3850 | 0.2992 | 0.372 |
| $a+by/z+cx/z^2$ | 271.39 | 193.67 | 0.104 | 0.1369 | 0.1053 | 0.0740 | 0.4770 | 0.3615 | 0.036 |
| $a+by/z+cx/\sqrt{z}$ | 165.60 | 130.23 | 0.666 | 0.0916 | 0.0677 | 0.5854 | 0.2843 | 0.1984 | 0.658 |
| $a+by/z+cxz$ | 127.64 | 96.27 | 0.802 | 0.0726 | 0.0509 | 0.7399 | 0.2654 | 0.1998 | 0.702 |
| $a+by/z+cxz^2$ | 156.75 | 117.29 | 0.701 | 0.0851 | 0.0658 | 0.6421 | 0.3176 | 0.2498 | 0.573 |
| $a+by/z+cx\sqrt{z}$ | 117.08 | 90.85 | 0.833 | 0.0696 | 0.0444 | 0.7611 | 0.2399 | 0.1606 | 0.756 |
| $a+by/z+cx^2/z$ | 167.66 | 124.48 | 0.658 | 0.0971 | 0.0771 | 0.5345 | 0.3016 | 0.2292 | 0.615 |
| $a+by/z+cx^2/z^2$ | 256.40 | 184.66 | 0.200 | 0.1289 | 0.0969 | 0.1795 | 0.4473 | 0.3252 | 0.152 |
| $a+by/z+cx^2/\sqrt{z}$ | 138.57 | 109.72 | 0.766 | 0.0852 | 0.0617 | 0.6414 | 0.2668 | 0.1878 | 0.698 |
| $a+by/z+cx^2z$ | 138.10 | 105.11 | 0.768 | 0.0796 | 0.0606 | 0.6874 | 0.2918 | 0.2309 | 0.639 |
| $a+by/z+cx^2z^2$ | 164.04 | 125.48 | 0.673 | 0.0906 | 0.0722 | 0.5948 | 0.3349 | 0.2643 | 0.525 |
| $a+by/z+cx^2\sqrt{z}$ | 124.04 | 95.80 | 0.813 | 0.0751 | 0.0552 | 0.7218 | 0.2663 | 0.2005 | 0.700 |
| $a+by/z+c\sqrt{x}/z$ | 248.39 | 185.88 | 0.249 | 0.1323 | 0.0992 | 0.1356 | 0.4556 | 0.3373 | 0.120 |
| $a+by/z+c\sqrt{x}/z^2$ | 259.89 | 188.54 | 0.178 | 0.1353 | 0.1039 | 0.0967 | 0.4628 | 0.3506 | 0.092 |
| $a+by/z+c\sqrt{x}/\sqrt{z}$ | 233.79 | 169.34 | 0.335 | 0.1159 | 0.0869 | 0.3369 | 0.3864 | 0.2767 | 0.367 |

(continued on next page)

**Table 4 – continued from previous page**

| Functional form | $T_{eff}$ (K) | | | Radius ($R_\odot$) | | | log (L/$L_\odot$) | | |
|---|---|---|---|---|---|---|---|---|---|
| | RMSE | MAD | $R^2_{ap}$ | RMSE | MAD | $R^2_{ap}$ | RMSE | MAD | $R^2_{ap}$ |
| $a+by/z+c\sqrt{x}z$ | 127.66 | 98.69 | 0.802 | 0.0710 | 0.0466 | 0.7512 | 0.2586 | 0.1867 | 0.717 |
| $a+by/z+c\sqrt{x}z^2$ | 155.12 | 119.11 | 0.707 | 0.0832 | 0.0630 | 0.6586 | 0.3111 | 0.2431 | 0.590 |
| $a+by/z+c\sqrt{x}\sqrt{z}$ | 122.11 | 92.34 | 0.819 | 0.0695 | 0.0422 | 0.7614 | 0.2376 | 0.1477 | 0.761 |
| $a+by/z+c/xz$ | 209.36 | 154.26 | 0.467 | 0.1024 | 0.0736 | 0.4822 | 0.3449 | 0.2514 | 0.496 |
| $a+by/z+c/xz^2$ | 202.50 | 146.86 | 0.501 | 0.1051 | 0.0737 | 0.4543 | 0.3452 | 0.2364 | 0.495 |
| $a+by/z+c/x\sqrt{z}$ | 217.15 | 158.85 | 0.426 | 0.1040 | 0.0765 | 0.4655 | 0.3556 | 0.2621 | 0.464 |
| $a+by/z+cz/x$ | 250.29 | 170.48 | 0.238 | 0.1194 | 0.0876 | 0.2955 | 0.4165 | 0.3035 | 0.265 |
| $a+by/z+cz^2/x$ | 268.91 | 191.90 | 0.120 | 0.1372 | 0.1053 | 0.0704 | 0.4771 | 0.3619 | 0.035 |
| $a+by/z+c\sqrt{z}/x$ | 237.10 | 166.87 | 0.316 | 0.1122 | 0.0833 | 0.3786 | 0.3904 | 0.2880 | 0.354 |
| $a+by/z+c/x^2z$ | 239.96 | 167.79 | 0.299 | 0.1135 | 0.0846 | 0.3644 | 0.3958 | 0.2932 | 0.336 |
| $a+by/z+c/x^2z^2$ | 230.56 | 165.76 | 0.353 | 0.1097 | 0.0820 | 0.4053 | 0.3792 | 0.2832 | 0.391 |
| $a+by/z+c/x^2\sqrt{z}$ | 243.25 | 168.09 | 0.280 | 0.1150 | 0.0856 | 0.3475 | 0.4020 | 0.2963 | 0.315 |
| $a+by/z+cz/x^2$ | 249.62 | 168.63 | 0.242 | 0.1182 | 0.0872 | 0.3106 | 0.4148 | 0.3019 | 0.271 |
| $a+by/z+cz^2/x^2$ | 252.97 | 169.25 | 0.221 | 0.1201 | 0.0882 | 0.2875 | 0.4218 | 0.3049 | 0.246 |
| $a+by/z+c\sqrt{z}/x^2$ | 247.89 | 168.47 | 0.252 | 0.1172 | 0.0868 | 0.3214 | 0.4113 | 0.3004 | 0.283 |
| $a+by/z+c/\sqrt{x}z$ | 184.18 | 132.43 | 0.587 | 0.0975 | 0.0678 | 0.5309 | 0.3149 | 0.2065 | 0.580 |
| $a+by/z+c/\sqrt{x}z^2$ | 204.76 | 143.03 | 0.490 | 0.1124 | 0.0847 | 0.3766 | 0.3645 | 0.2598 | 0.437 |
| $a+by/z+c/\sqrt{x}\sqrt{z}$ | 186.85 | 137.10 | 0.575 | 0.0942 | 0.0666 | 0.5614 | 0.3106 | 0.2132 | 0.591 |
| $a+by/z+cz/\sqrt{x}$ | 259.15 | 181.27 | 0.183 | 0.1350 | 0.1014 | 0.1006 | 0.4706 | 0.3464 | 0.061 |
| $a+by/z+cz^2/\sqrt{x}$ | 171.91 | 142.38 | 0.640 | 0.0931 | 0.0691 | 0.5719 | 0.3418 | 0.2681 | 0.505 |
| $a+by/z+c\sqrt{z}/\sqrt{x}$ | 247.50 | 171.26 | 0.255 | 0.1190 | 0.0868 | 0.3010 | 0.4112 | 0.3001 | 0.283 |
| $a+by/z^2+cx/z$ | 239.90 | 179.15 | 0.300 | 0.1274 | 0.1018 | 0.1987 | 0.4140 | 0.3206 | 0.274 |
| $a+by/z^2+cx/z^2$ | 213.41 | 159.88 | 0.446 | 0.1140 | 0.0863 | 0.3583 | 0.3665 | 0.2714 | 0.431 |
| $a+by/z^2+cx/\sqrt{z}$ | 201.13 | 153.27 | 0.508 | 0.1102 | 0.0847 | 0.4005 | 0.3453 | 0.2548 | 0.495 |
| $a+by/z^2+cxz$ | 128.40 | 96.04 | 0.799 | 0.0730 | 0.0520 | 0.7371 | 0.2698 | 0.2079 | 0.691 |
| $a+by/z^2+cxz^2$ | 153.99 | 114.61 | 0.711 | 0.0851 | 0.0664 | 0.6420 | 0.3182 | 0.2499 | 0.571 |
| $a+by/z^2+cx\sqrt{z}$ | 117.08 | 90.97 | 0.833 | 0.0692 | 0.0441 | 0.7637 | 0.2399 | 0.1609 | 0.756 |
| $a+by/z^2+cx^2/z$ | 196.55 | 145.05 | 0.530 | 0.1119 | 0.0885 | 0.3820 | 0.3475 | 0.2680 | 0.488 |
| $a+by/z^2+cx^2/z^2$ | 193.92 | 141.61 | 0.542 | 0.1117 | 0.0847 | 0.3838 | 0.3427 | 0.2494 | 0.502 |
| $a+by/z^2+cx^2/\sqrt{z}$ | 156.72 | 120.40 | 0.701 | 0.0940 | 0.0698 | 0.5641 | 0.2895 | 0.2102 | 0.645 |
| $a+by/z^2+cx^2z$ | 136.99 | 103.40 | 0.772 | 0.0797 | 0.0612 | 0.6864 | 0.2936 | 0.2346 | 0.635 |
| $a+by/z^2+cx^2z^2$ | 159.10 | 120.99 | 0.692 | 0.0898 | 0.0721 | 0.6015 | 0.3319 | 0.2630 | 0.533 |
| $a+by/z^2+cx^2\sqrt{z}$ | 123.55 | 96.08 | 0.814 | 0.0750 | 0.0550 | 0.7221 | 0.2674 | 0.2030 | 0.697 |
| $a+by/z^2+c\sqrt{x}/z$ | 257.06 | 181.89 | 0.196 | 0.1334 | 0.1003 | 0.1215 | 0.4626 | 0.3468 | 0.093 |
| $a+by/z^2+c\sqrt{x}/z^2$ | 258.95 | 188.25 | 0.184 | 0.1355 | 0.1057 | 0.0936 | 0.4627 | 0.3500 | 0.093 |
| $a+by/z^2+c\sqrt{x}/\sqrt{z}$ | 248.14 | 183.14 | 0.251 | 0.1290 | 0.1034 | 0.1785 | 0.4262 | 0.3282 | 0.230 |
| $a+by/z^2+c\sqrt{x}z$ | 129.38 | 99.67 | 0.796 | 0.0715 | 0.0484 | 0.7478 | 0.2646 | 0.1971 | 0.703 |
| $a+by/z^2+c\sqrt{x}z^2$ | 153.55 | 116.92 | 0.713 | 0.0836 | 0.0640 | 0.6549 | 0.3137 | 0.2437 | 0.583 |
| $a+by/z^2+c\sqrt{x}\sqrt{z}$ | 122.08 | 91.99 | 0.819 | 0.0687 | 0.0411 | 0.7667 | 0.2367 | 0.1499 | 0.763 |
| $a+by/z^2+c/xz$ | 222.35 | 165.27 | 0.398 | 0.1120 | 0.0859 | 0.3810 | 0.3694 | 0.2711 | 0.422 |
| $a+by/z^2+c/xz^2$ | 217.84 | 160.40 | 0.423 | 0.1138 | 0.0859 | 0.3608 | 0.3691 | 0.2618 | 0.423 |
| $a+by/z^2+c/x\sqrt{z}$ | 227.48 | 167.80 | 0.370 | 0.1131 | 0.0877 | 0.3681 | 0.3771 | 0.2785 | 0.397 |
| $a+by/z^2+cz/x$ | 251.22 | 176.26 | 0.232 | 0.1252 | 0.0967 | 0.2261 | 0.4253 | 0.3080 | 0.234 |
| $a+by/z^2+cz^2/x$ | 257.40 | 184.24 | 0.194 | 0.1350 | 0.1025 | 0.1002 | 0.4642 | 0.3509 | 0.087 |
| $a+by/z^2+c\sqrt{z}/x$ | 241.60 | 173.87 | 0.290 | 0.1194 | 0.0928 | 0.2959 | 0.4042 | 0.2973 | 0.308 |
| $a+by/z^2+c/x^2z$ | 243.30 | 174.15 | 0.280 | 0.1200 | 0.0929 | 0.2894 | 0.4073 | 0.3002 | 0.297 |
| $a+by/z^2+c/x^2z^2$ | 237.71 | 172.87 | 0.312 | 0.1179 | 0.0916 | 0.3136 | 0.3969 | 0.2941 | 0.333 |
| $a+by/z^2+c/x^2\sqrt{z}$ | 245.28 | 174.41 | 0.268 | 0.1208 | 0.0933 | 0.2791 | 0.4114 | 0.3021 | 0.283 |
| $a+by/z^2+cz/x^2$ | 249.26 | 174.64 | 0.244 | 0.1228 | 0.0941 | 0.2551 | 0.4201 | 0.3053 | 0.252 |
| $a+by/z^2+cz^2/x^2$ | 251.62 | 174.82 | 0.230 | 0.1243 | 0.0947 | 0.2369 | 0.4255 | 0.3072 | 0.233 |
| $a+by/z^2+c\sqrt{z}/x^2$ | 248.14 | 174.59 | 0.251 | 0.1222 | 0.0939 | 0.2625 | 0.4175 | 0.3044 | 0.261 |
| $a+by/z^2+c/\sqrt{x}z$ | 196.19 | 143.44 | 0.532 | 0.1035 | 0.0782 | 0.4715 | 0.3295 | 0.2324 | 0.540 |
| $a+by/z^2+c/\sqrt{x}z^2$ | 211.40 | 151.44 | 0.456 | 0.1153 | 0.0910 | 0.3439 | 0.3684 | 0.2743 | 0.425 |
| $a+by/z^2+c/\sqrt{x}\sqrt{z}$ | 200.47 | 148.00 | 0.511 | 0.1025 | 0.0766 | 0.4813 | 0.3317 | 0.2335 | 0.534 |
| $a+by/z^2+cz/\sqrt{x}$ | 250.73 | 177.79 | 0.235 | 0.1324 | 0.0995 | 0.1341 | 0.4586 | 0.3413 | 0.109 |
| $a+by/z^2+cz^2/\sqrt{x}$ | 175.74 | 135.37 | 0.624 | 0.0955 | 0.0687 | 0.5501 | 0.3513 | 0.2630 | 0.477 |
| $a+by/z^2+c\sqrt{z}/\sqrt{x}$ | 251.09 | 178.38 | 0.233 | 0.1265 | 0.0991 | 0.2103 | 0.4263 | 0.3132 | 0.230 |
| $a+by/\sqrt{z}+cx/z$ | 256.67 | 197.25 | 0.198 | 0.1343 | 0.1061 | 0.1089 | 0.4574 | 0.3562 | 0.113 |
| $a+by/\sqrt{z}+cx/z^2$ | 251.71 | 191.92 | 0.229 | 0.1329 | 0.1074 | 0.1283 | 0.4439 | 0.3516 | 0.165 |
| $a+by/\sqrt{z}+cx/\sqrt{z}$ | 247.92 | 180.96 | 0.252 | 0.1217 | 0.0940 | 0.2684 | 0.3940 | 0.2968 | 0.342 |
| $a+by/\sqrt{z}+cxz$ | 124.85 | 95.79 | 0.810 | 0.0723 | 0.0493 | 0.7421 | 0.2596 | 0.1861 | 0.714 |
| $a+by/\sqrt{z}+cxz^2$ | 148.30 | 116.66 | 0.732 | 0.0823 | 0.0619 | 0.6653 | 0.2999 | 0.2316 | 0.619 |
| $a+by/\sqrt{z}+cx\sqrt{z}$ | 117.09 | 90.74 | 0.833 | 0.0695 | 0.0446 | 0.7614 | 0.2405 | 0.1597 | 0.755 |
| $a+by/\sqrt{z}+cx^2/z$ | 280.44 | 203.12 | 0.043 | 0.1404 | 0.1123 | 0.0273 | 0.4642 | 0.3660 | 0.087 |
| $a+by/\sqrt{z}+cx^2/z^2$ | 271.37 | 200.09 | 0.104 | 0.1392 | 0.1121 | 0.0438 | 0.4707 | 0.3681 | 0.061 |
| $a+by/\sqrt{z}+cx^2/\sqrt{z}$ | 151.63 | 120.95 | 0.720 | 0.0881 | 0.0652 | 0.6166 | 0.2770 | 0.1988 | 0.675 |
| $a+by/\sqrt{z}+cx^2z$ | 134.60 | 107.80 | 0.780 | 0.0786 | 0.0583 | 0.6946 | 0.2829 | 0.2141 | 0.661 |
| $a+by/\sqrt{z}+cx^2z^2$ | 157.42 | 125.86 | 0.698 | 0.0883 | 0.0691 | 0.6151 | 0.3190 | 0.2504 | 0.569 |
| $a+by/\sqrt{z}+cx^2\sqrt{z}$ | 123.73 | 96.80 | 0.814 | 0.0750 | 0.0550 | 0.7221 | 0.2640 | 0.1945 | 0.705 |
| $a+by/\sqrt{z}+c\sqrt{x}/z$ | 204.69 | 159.07 | 0.490 | 0.1159 | 0.0882 | 0.3369 | 0.3850 | 0.2881 | 0.372 |
| $a+by/\sqrt{z}+c\sqrt{x}/z^2$ | 237.39 | 180.75 | 0.314 | 0.1282 | 0.1027 | 0.1879 | 0.4234 | 0.3331 | 0.240 |
| $a+by/\sqrt{z}+c\sqrt{x}/\sqrt{z}$ | 264.69 | 203.73 | 0.148 | 0.1395 | 0.1078 | 0.0385 | 0.4746 | 0.3642 | 0.046 |
| $a+by/\sqrt{z}+c\sqrt{x}z$ | 124.77 | 95.91 | 0.811 | 0.0710 | 0.0453 | 0.7514 | 0.2538 | 0.1752 | 0.727 |
| $a+by/\sqrt{z}+c\sqrt{x}z^2$ | 145.63 | 116.30 | 0.742 | 0.0801 | 0.0589 | 0.6833 | 0.2923 | 0.2225 | 0.638 |
| $a+by/\sqrt{z}+c\sqrt{x}\sqrt{z}$ | 122.11 | 92.48 | 0.819 | 0.0696 | 0.0414 | 0.7610 | 0.2389 | 0.1469 | 0.758 |
| $a+by/\sqrt{z}+c/xz$ | 245.94 | 178.00 | 0.264 | 0.1149 | 0.0881 | 0.3486 | 0.3873 | 0.2942 | 0.364 |
| $a+by/\sqrt{z}+c/xz^2$ | 228.15 | 165.82 | 0.367 | 0.1136 | 0.0832 | 0.3632 | 0.3720 | 0.2679 | 0.414 |
| $a+by/\sqrt{z}+c/x\sqrt{z}$ | 259.34 | 188.63 | 0.182 | 0.1198 | 0.0917 | 0.2919 | 0.4084 | 0.3087 | 0.293 |
| $a+by/\sqrt{z}+cz/x$ | 297.30 | 219.43 | -0.075 | 0.1432 | 0.1102 | -0.0126 | 0.4888 | 0.3732 | -0.012 |
| $a+by/\sqrt{z}+cz^2/x$ | 248.28 | 191.70 | 0.250 | 0.1359 | 0.1055 | 0.0887 | 0.4579 | 0.3472 | 0.112 |
| $a+by/\sqrt{z}+c\sqrt{z}/x$ | 286.18 | 208.97 | 0.004 | 0.1342 | 0.1025 | 0.1107 | 0.4603 | 0.3484 | 0.102 |
| $a+by/\sqrt{z}+c/x^2z$ | 286.19 | 209.20 | 0.003 | 0.1342 | 0.1027 | 0.1110 | 0.4606 | 0.3491 | 0.101 |
| $a+by/\sqrt{z}+c/x^2z^2$ | 278.16 | 205.37 | 0.059 | 0.1297 | 0.0989 | 0.1689 | 0.4441 | 0.3371 | 0.164 |
| $a+by/\sqrt{z}+c/x^2\sqrt{z}$ | 288.59 | 209.90 | -0.013 | 0.1357 | 0.1037 | 0.0906 | 0.4660 | 0.3522 | 0.080 |
| $a+by/\sqrt{z}+cz/x^2$ | 292.81 | 212.44 | -0.043 | 0.1388 | 0.1054 | 0.0491 | 0.4764 | 0.3581 | 0.038 |
| $a+by/\sqrt{z}+cz^2/x^2$ | 295.12 | 213.90 | -0.060 | 0.1408 | 0.1065 | 0.0216 | 0.4826 | 0.3622 | 0.013 |
| $a+by/\sqrt{z}+c\sqrt{z}/x^2$ | 291.69 | 211.72 | -0.035 | 0.1379 | 0.1049 | 0.0611 | 0.4735 | 0.3561 | 0.050 |
| $a+by/\sqrt{z}+c/\sqrt{x}z$ | 193.66 | 141.65 | 0.544 | 0.0994 | 0.0709 | 0.5120 | 0.3205 | 0.2215 | 0.565 |
| $a+by/\sqrt{z}+c/\sqrt{x}z^2$ | 211.06 | 150.38 | 0.458 | 0.1149 | 0.0899 | 0.3487 | 0.3685 | 0.2721 | 0.425 |
| $a+by/\sqrt{z}+c/\sqrt{x}\sqrt{z}$ | 204.87 | 149.38 | 0.489 | 0.0982 | 0.0719 | 0.5243 | 0.3247 | 0.2381 | 0.553 |
| $a+by/\sqrt{z}+cz/\sqrt{x}$ | 204.87 | 152.26 | 0.489 | 0.1195 | 0.0862 | 0.2952 | 0.4023 | 0.2875 | 0.314 |
| $a+by/\sqrt{z}+cz^2/\sqrt{x}$ | 145.97 | 119.18 | 0.741 | 0.0844 | 0.0588 | 0.6486 | 0.3005 | 0.2245 | 0.617 |

(continued on next page)

**Table 4 – continued from previous page**

| Functional form | $T_{eff}$ (K) | | | Radius ($R_{\odot}$) | | | log (L/$L_{\odot}$) | | |
|---|---|---|---|---|---|---|---|---|---|
| | RMSE | MAD | $R^2_{ap}$ | RMSE | MAD | $R^2_{ap}$ | RMSE | MAD | $R^2_{ap}$ |
| $a+by/\sqrt{z}+c\sqrt{z}/\sqrt{x}$ | 299.13 | 226.61 | -0.089 | 0.1467 | 0.1158 | -0.0622 | 0.4982 | 0.3904 | -0.052 |
| $a+byz+cx/z$ | 133.69 | 106.17 | 0.783 | 0.0766 | 0.0514 | 0.7104 | 0.2743 | 0.2009 | 0.681 |
| $a+byz+cx/z^2$ | 137.24 | 106.82 | 0.771 | 0.0782 | 0.0556 | 0.6977 | 0.2872 | 0.2190 | 0.651 |
| $a+byz+cx/\sqrt{z}$ | 126.64 | 98.26 | 0.805 | 0.0743 | 0.0476 | 0.7276 | 0.2560 | 0.1701 | 0.722 |
| $a+byz+cxz$ | 127.62 | 96.41 | 0.802 | 0.0715 | 0.0541 | 0.7475 | 0.2626 | 0.2067 | 0.708 |
| $a+byz+cxz^2$ | 135.84 | 106.50 | 0.775 | 0.0788 | 0.0549 | 0.6934 | 0.2852 | 0.2014 | 0.655 |
| $a+byz+cx\sqrt{z}$ | 117.10 | 91.04 | 0.833 | 0.0694 | 0.0444 | 0.7619 | 0.2340 | 0.1582 | 0.768 |
| $a+byz+cx^2/z$ | 124.80 | 97.76 | 0.810 | 0.0747 | 0.0500 | 0.7244 | 0.2581 | 0.1776 | 0.718 |
| $a+byz+cx^2/z^2$ | 135.20 | 107.18 | 0.778 | 0.0773 | 0.0538 | 0.7050 | 0.2807 | 0.2150 | 0.666 |
| $a+byz+cx^2/\sqrt{z}$ | 118.92 | 92.39 | 0.828 | 0.0736 | 0.0494 | 0.7326 | 0.2490 | 0.1641 | 0.737 |
| $a+byz+cx^2z$ | 135.24 | 102.16 | 0.777 | 0.0783 | 0.0577 | 0.6971 | 0.2887 | 0.2263 | 0.647 |
| $a+byz+cx^2z^2$ | 136.39 | 108.40 | 0.774 | 0.0783 | 0.0526 | 0.6970 | 0.2833 | 0.1971 | 0.660 |
| $a+byz+cx^2\sqrt{z}$ | 123.94 | 95.23 | 0.813 | 0.0749 | 0.0547 | 0.7232 | 0.2673 | 0.2031 | 0.697 |
| $a+byz+c\sqrt{x}/z$ | 137.26 | 106.99 | 0.771 | 0.0782 | 0.0552 | 0.6980 | 0.2863 | 0.2162 | 0.653 |
| $a+byz+c\sqrt{x}/z^2$ | 136.91 | 107.34 | 0.772 | 0.0788 | 0.0567 | 0.6936 | 0.2899 | 0.2230 | 0.644 |
| $a+byz+c\sqrt{x}/\sqrt{z}$ | 134.04 | 105.50 | 0.781 | 0.0762 | 0.0502 | 0.7130 | 0.2721 | 0.1926 | 0.686 |
| $a+byz+c\sqrt{x}z$ | 129.33 | 100.13 | 0.796 | 0.0707 | 0.0498 | 0.7529 | 0.2590 | 0.1883 | 0.716 |
| $a+byz+c\sqrt{x}z^2$ | 135.72 | 105.62 | 0.776 | 0.0789 | 0.0564 | 0.6922 | 0.2870 | 0.2089 | 0.651 |
| $a+byz+c\sqrt{x}\sqrt{z}$ | 121.38 | 91.52 | 0.821 | 0.0696 | 0.0418 | 0.7607 | 0.2363 | 0.1456 | 0.763 |
| $a+byz+c/xz$ | 134.28 | 105.43 | 0.781 | 0.0750 | 0.0482 | 0.7224 | 0.2661 | 0.1789 | 0.700 |
| $a+byz+c/xz^2$ | 129.59 | 100.53 | 0.796 | 0.0750 | 0.0469 | 0.7221 | 0.2613 | 0.1651 | 0.711 |
| $a+byz+c/x\sqrt{z}$ | 135.83 | 106.83 | 0.776 | 0.0754 | 0.0493 | 0.7197 | 0.2702 | 0.1867 | 0.691 |
| $a+byz+cz/x$ | 137.32 | 107.43 | 0.771 | 0.0767 | 0.0514 | 0.7093 | 0.2798 | 0.2006 | 0.668 |
| $a+byz+cz^2/x$ | 137.34 | 107.34 | 0.771 | 0.0774 | 0.0523 | 0.7041 | 0.2822 | 0.2021 | 0.663 |
| $a+byz+c\sqrt{z}/x$ | 137.18 | 107.56 | 0.771 | 0.0763 | 0.0509 | 0.7126 | 0.2773 | 0.1976 | 0.674 |
| $a+byz+c/x^2z$ | 137.29 | 107.55 | 0.771 | 0.0764 | 0.0511 | 0.7115 | 0.2785 | 0.1986 | 0.671 |
| $a+byz+c/x^2z^2$ | 136.80 | 107.59 | 0.772 | 0.0760 | 0.0503 | 0.7147 | 0.2749 | 0.1935 | 0.680 |
| $a+byz+c/x^2\sqrt{z}$ | 137.34 | 107.36 | 0.771 | 0.0766 | 0.0513 | 0.7102 | 0.2797 | 0.2001 | 0.668 |
| $a+byz+cz/x^2$ | 137.26 | 106.81 | 0.771 | 0.0769 | 0.0518 | 0.7077 | 0.2820 | 0.2025 | 0.663 |
| $a+byz+cz^2/x^2$ | 137.20 | 106.59 | 0.771 | 0.0771 | 0.0520 | 0.7067 | 0.2827 | 0.2032 | 0.661 |
| $a+byz+c\sqrt{z}/x^2$ | 137.30 | 106.98 | 0.771 | 0.0769 | 0.0517 | 0.7084 | 0.2814 | 0.2019 | 0.664 |
| $a+byz+c/\sqrt{x}z$ | 126.90 | 97.92 | 0.804 | 0.0742 | 0.0450 | 0.7285 | 0.2552 | 0.1544 | 0.724 |
| $a+byz+c/\sqrt{x}z^2$ | 124.68 | 95.60 | 0.811 | 0.0766 | 0.0496 | 0.7106 | 0.2669 | 0.1695 | 0.698 |
| $a+byz+c/\sqrt{x}\sqrt{z}$ | 131.07 | 101.82 | 0.791 | 0.0739 | 0.0460 | 0.7301 | 0.2579 | 0.1646 | 0.718 |
| $a+byz+cz/\sqrt{x}$ | 137.31 | 107.31 | 0.771 | 0.0777 | 0.0531 | 0.7021 | 0.2828 | 0.2035 | 0.661 |
| $a+byz+cz^2/\sqrt{x}$ | 136.77 | 106.82 | 0.772 | 0.0786 | 0.0549 | 0.6950 | 0.2852 | 0.2077 | 0.655 |
| $a+byz+c\sqrt{z}/\sqrt{x}$ | 136.87 | 107.17 | 0.772 | 0.0764 | 0.0510 | 0.7116 | 0.2766 | 0.1970 | 0.676 |
| $a+byz^2+cx/z$ | 157.68 | 122.83 | 0.697 | 0.0856 | 0.0672 | 0.6384 | 0.3136 | 0.2488 | 0.583 |
| $a+byz^2+cx/z^2$ | 160.53 | 122.30 | 0.686 | 0.0880 | 0.0678 | 0.6179 | 0.3276 | 0.2548 | 0.545 |
| $a+byz^2+cx/\sqrt{z}$ | 138.16 | 108.95 | 0.768 | 0.0779 | 0.0558 | 0.7004 | 0.2718 | 0.2014 | 0.687 |
| $a+byz^2+cxz$ | 122.76 | 98.16 | 0.817 | 0.0702 | 0.0467 | 0.7567 | 0.2470 | 0.1702 | 0.742 |
| $a+byz^2+cxz^2$ | 155.33 | 113.09 | 0.706 | 0.0836 | 0.0667 | 0.6551 | 0.3124 | 0.2490 | 0.587 |
| $a+byz^2+cx\sqrt{z}$ | 117.06 | 89.91 | 0.833 | 0.0696 | 0.0445 | 0.7609 | 0.2376 | 0.1513 | 0.761 |
| $a+byz^2+cx^2/z$ | 139.12 | 108.64 | 0.765 | 0.0798 | 0.0601 | 0.6854 | 0.2802 | 0.2133 | 0.667 |
| $a+byz^2+cx^2/z^2$ | 160.62 | 124.65 | 0.686 | 0.0872 | 0.0680 | 0.6242 | 0.3232 | 0.2576 | 0.557 |
| $a+byz^2+cx^2/\sqrt{z}$ | 120.64 | 94.59 | 0.823 | 0.0744 | 0.0545 | 0.7263 | 0.2522 | 0.1826 | 0.730 |
| $a+byz^2+cx^2z$ | 135.70 | 102.55 | 0.776 | 0.0791 | 0.0601 | 0.6908 | 0.2864 | 0.2204 | 0.652 |
| $a+byz^2+cx^2z^2$ | 161.05 | 122.31 | 0.684 | 0.0879 | 0.0673 | 0.6183 | 0.3275 | 0.2537 | 0.545 |
| $a+byz^2+cx^2\sqrt{z}$ | 123.91 | 96.71 | 0.813 | 0.0751 | 0.0553 | 0.7217 | 0.2642 | 0.1939 | 0.704 |
| $a+byz^2+c\sqrt{x}/z$ | 160.68 | 122.48 | 0.686 | 0.0879 | 0.0677 | 0.6181 | 0.3274 | 0.2542 | 0.546 |
| $a+byz^2+c\sqrt{x}/z^2$ | 156.62 | 121.11 | 0.702 | 0.0876 | 0.0678 | 0.6207 | 0.3256 | 0.2534 | 0.551 |
| $a+byz^2+c\sqrt{x}/\sqrt{z}$ | 155.87 | 122.51 | 0.704 | 0.0840 | 0.0649 | 0.6515 | 0.3063 | 0.2357 | 0.603 |
| $a+byz^2+c\sqrt{x}z$ | 126.98 | 101.07 | 0.804 | 0.0703 | 0.0442 | 0.7559 | 0.2493 | 0.1630 | 0.737 |
| $a+byz^2+c\sqrt{x}z^2$ | 153.68 | 113.61 | 0.713 | 0.0799 | 0.0610 | 0.6851 | 0.3002 | 0.2357 | 0.618 |
| $a+byz^2+c\sqrt{x}\sqrt{z}$ | 120.98 | 91.28 | 0.822 | 0.0694 | 0.0415 | 0.7619 | 0.2386 | 0.1422 | 0.759 |
| $a+byz^2+c/xz$ | 147.58 | 113.52 | 0.735 | 0.0778 | 0.0548 | 0.7011 | 0.2797 | 0.1955 | 0.669 |
| $a+byz^2+c/xz^2$ | 137.25 | 102.16 | 0.771 | 0.0769 | 0.0522 | 0.7081 | 0.2694 | 0.1794 | 0.692 |
| $a+byz^2+c/x\sqrt{z}$ | 152.01 | 117.23 | 0.719 | 0.0790 | 0.0567 | 0.6915 | 0.2876 | 0.2034 | 0.650 |
| $a+byz^2+cz/x$ | 159.21 | 121.17 | 0.692 | 0.0829 | 0.0607 | 0.6603 | 0.3078 | 0.2223 | 0.599 |
| $a+byz^2+cz^2/x$ | 160.43 | 120.32 | 0.687 | 0.0848 | 0.0632 | 0.6447 | 0.3154 | 0.2314 | 0.579 |
| $a+byz^2+c\sqrt{z}/x$ | 157.70 | 120.91 | 0.697 | 0.0817 | 0.0597 | 0.6701 | 0.3021 | 0.2172 | 0.613 |
| $a+byz^2+c/x^2z$ | 158.31 | 121.14 | 0.695 | 0.0820 | 0.0598 | 0.6681 | 0.3038 | 0.2183 | 0.609 |
| $a+byz^2+c/x^2z^2$ | 155.76 | 120.18 | 0.705 | 0.0808 | 0.0586 | 0.6773 | 0.2970 | 0.2117 | 0.626 |
| $a+byz^2+c/x^2\sqrt{z}$ | 159.03 | 121.22 | 0.692 | 0.0824 | 0.0602 | 0.6646 | 0.3061 | 0.2204 | 0.603 |
| $a+byz^2+cz/x^2$ | 160.13 | 121.00 | 0.688 | 0.0833 | 0.0609 | 0.6575 | 0.3105 | 0.2239 | 0.591 |
| $a+byz^2+cz^2/x^2$ | 160.43 | 120.79 | 0.687 | 0.0836 | 0.0611 | 0.6547 | 0.3121 | 0.2250 | 0.587 |
| $a+byz^2+c\sqrt{z}/x^2$ | 159.88 | 121.11 | 0.689 | 0.0831 | 0.0607 | 0.6594 | 0.3094 | 0.2230 | 0.594 |
| $a+byz^2+c/\sqrt{x}z$ | 129.62 | 97.05 | 0.796 | 0.0743 | 0.0487 | 0.7274 | 0.2564 | 0.1644 | 0.721 |
| $a+byz^2+c/\sqrt{x}z^2$ | 126.78 | 93.94 | 0.804 | 0.0785 | 0.0545 | 0.6961 | 0.2731 | 0.1802 | 0.684 |
| $a+byz^2+c/\sqrt{x}\sqrt{z}$ | 138.57 | 104.16 | 0.766 | 0.0749 | 0.0505 | 0.7234 | 0.2633 | 0.1770 | 0.706 |
| $a+byz^2+cz/\sqrt{x}$ | 160.96 | 121.78 | 0.685 | 0.0862 | 0.0654 | 0.6335 | 0.3200 | 0.2407 | 0.566 |
| $a+byz^2+cz^2/\sqrt{x}$ | 161.18 | 124.04 | 0.684 | 0.0880 | 0.0680 | 0.6180 | 0.3274 | 0.2550 | 0.546 |
| $a+byz^2+c\sqrt{z}/\sqrt{x}$ | 157.67 | 121.13 | 0.698 | 0.0826 | 0.0608 | 0.6634 | 0.3042 | 0.2225 | 0.608 |
| $a+by\sqrt{z}+cx/z$ | 131.02 | 99.37 | 0.791 | 0.0780 | 0.0485 | 0.7000 | 0.2683 | 0.1672 | 0.695 |
| $a+by\sqrt{z}+cx/z^2$ | 131.24 | 100.47 | 0.790 | 0.0778 | 0.0488 | 0.7008 | 0.2717 | 0.1796 | 0.687 |
| $a+by\sqrt{z}+cx/\sqrt{z}$ | 130.05 | 97.98 | 0.794 | 0.0776 | 0.0477 | 0.7025 | 0.2622 | 0.1597 | 0.709 |
| $a+by\sqrt{z}+cxz$ | 125.63 | 97.78 | 0.808 | 0.0733 | 0.0519 | 0.7349 | 0.2676 | 0.2000 | 0.697 |
| $a+by\sqrt{z}+cxz^2$ | 130.06 | 101.08 | 0.794 | 0.0772 | 0.0528 | 0.7060 | 0.2744 | 0.1864 | 0.681 |
| $a+by\sqrt{z}+cx\sqrt{z}$ | 116.96 | 91.42 | 0.834 | 0.0684 | 0.0462 | 0.7691 | 0.2352 | 0.1673 | 0.766 |
| $a+by\sqrt{z}+cx^2/z$ | 128.67 | 97.03 | 0.799 | 0.0776 | 0.0482 | 0.7029 | 0.2617 | 0.1612 | 0.710 |
| $a+by\sqrt{z}+cx^2/z^2$ | 130.53 | 97.95 | 0.793 | 0.0776 | 0.0481 | 0.7028 | 0.2681 | 0.1703 | 0.695 |
| $a+by\sqrt{z}+cx^2/\sqrt{z}$ | 126.05 | 95.88 | 0.807 | 0.0771 | 0.0486 | 0.7069 | 0.2563 | 0.1655 | 0.722 |
| $a+by\sqrt{z}+cx^2z$ | 127.67 | 98.77 | 0.802 | 0.0765 | 0.0536 | 0.7111 | 0.2734 | 0.1948 | 0.683 |
| $a+by\sqrt{z}+cx^2z^2$ | 130.10 | 100.71 | 0.794 | 0.0778 | 0.0525 | 0.7010 | 0.2743 | 0.1805 | 0.681 |
| $a+by\sqrt{z}+cx^2\sqrt{z}$ | 122.36 | 94.71 | 0.818 | 0.0746 | 0.0535 | 0.7250 | 0.2650 | 0.1952 | 0.702 |
| $a+by\sqrt{z}+c\sqrt{x}/z$ | 131.06 | 101.25 | 0.791 | 0.0782 | 0.0495 | 0.6979 | 0.2728 | 0.1789 | 0.685 |
| $a+by\sqrt{z}+c\sqrt{x}/z^2$ | 131.08 | 101.05 | 0.791 | 0.0780 | 0.0495 | 0.6993 | 0.2736 | 0.1844 | 0.683 |
| $a+by\sqrt{z}+c\sqrt{x}/\sqrt{z}$ | 131.26 | 100.68 | 0.790 | 0.0781 | 0.0487 | 0.6990 | 0.2691 | 0.1682 | 0.693 |
| $a+by\sqrt{z}+c\sqrt{x}z$ | 126.13 | 99.44 | 0.806 | 0.0724 | 0.0492 | 0.7410 | 0.2651 | 0.1950 | 0.702 |
| $a+by\sqrt{z}+c\sqrt{x}z^2$ | 130.08 | 101.09 | 0.794 | 0.0768 | 0.0527 | 0.7091 | 0.2743 | 0.1892 | 0.681 |
| $a+by\sqrt{z}+c\sqrt{x}\sqrt{z}$ | 121.72 | 91.06 | 0.820 | 0.0690 | 0.0445 | 0.7647 | 0.2361 | 0.1527 | 0.764 |
| $a+by\sqrt{z}+c/xz$ | 131.13 | 100.81 | 0.791 | 0.0777 | 0.0474 | 0.7019 | 0.2672 | 0.1643 | 0.697 |

(continued on next page)

**Table 4 – continued from previous page**

| Functional form | $T_{eff}$ (K) | | | Radius ($R_\odot$) | | | log ($L/L_\odot$) | | |
|---|---|---|---|---|---|---|---|---|---|
| | RMSE | MAD | $R^2_{ap}$ | RMSE | MAD | $R^2_{ap}$ | RMSE | MAD | $R^2_{ap}$ |
| $a+by\sqrt{z}+c/xz^2$ | 130.96 | 99.91 | 0.791 | 0.0779 | 0.0475 | 0.7006 | 0.2654 | 0.1558 | 0.702 |
| $a+by\sqrt{z}+c/x\sqrt{z}$ | 130.66 | 100.38 | 0.792 | 0.0777 | 0.0478 | 0.7016 | 0.2688 | 0.1688 | 0.694 |
| $a+by\sqrt{z}+cz/x$ | 128.74 | 98.08 | 0.798 | 0.0781 | 0.0486 | 0.6989 | 0.2725 | 0.1760 | 0.685 |
| $a+by\sqrt{z}+cz^2/x$ | 128.09 | 97.66 | 0.800 | 0.0783 | 0.0501 | 0.6971 | 0.2738 | 0.1781 | 0.682 |
| $a+by\sqrt{z}+c\sqrt{z}/x$ | 129.35 | 98.81 | 0.796 | 0.0779 | 0.0484 | 0.7000 | 0.2715 | 0.1748 | 0.688 |
| $a+by\sqrt{z}+c/x^2z$ | 128.98 | 98.15 | 0.798 | 0.0780 | 0.0483 | 0.6999 | 0.2719 | 0.1754 | 0.687 |
| $a+by\sqrt{z}+c/x^2z^2$ | 129.93 | 99.46 | 0.795 | 0.0779 | 0.0481 | 0.7003 | 0.2707 | 0.1727 | 0.689 |
| $a+by\sqrt{z}+c/x^2\sqrt{z}$ | 128.61 | 97.61 | 0.799 | 0.0780 | 0.0484 | 0.6998 | 0.2723 | 0.1761 | 0.686 |
| $a+by\sqrt{z}+cz/x^2$ | 127.88 | 96.53 | 0.801 | 0.0780 | 0.0485 | 0.6994 | 0.2729 | 0.1772 | 0.684 |
| $a+by\sqrt{z}+cz^2/x^2$ | 127.60 | 96.14 | 0.802 | 0.0781 | 0.0486 | 0.6991 | 0.2732 | 0.1774 | 0.684 |
| $a+by\sqrt{z}+c\sqrt{z}/x^2$ | 128.07 | 96.82 | 0.800 | 0.0780 | 0.0485 | 0.6995 | 0.2728 | 0.1770 | 0.685 |
| $a+by\sqrt{z}+c/\sqrt{x}z$ | 130.19 | 98.76 | 0.794 | 0.0774 | 0.0469 | 0.7040 | 0.2613 | 0.1508 | 0.711 |
| $a+by\sqrt{z}+c/\sqrt{x}z^2$ | 128.62 | 97.20 | 0.799 | 0.0782 | 0.0488 | 0.6981 | 0.2675 | 0.1574 | 0.697 |
| $a+by\sqrt{z}+c/\sqrt{x}\sqrt{z}$ | 131.17 | 100.39 | 0.791 | 0.0773 | 0.0471 | 0.7053 | 0.2627 | 0.1555 | 0.708 |
| $a+by\sqrt{z}+cz/\sqrt{x}$ | 128.74 | 98.95 | 0.798 | 0.0783 | 0.0502 | 0.6971 | 0.2739 | 0.1788 | 0.682 |
| $a+by\sqrt{z}+cz^2/\sqrt{x}$ | 129.25 | 101.31 | 0.797 | 0.0775 | 0.0513 | 0.7034 | 0.2744 | 0.1862 | 0.681 |
| $a+by\sqrt{z}+c\sqrt{z}/\sqrt{x}$ | 129.86 | 99.85 | 0.795 | 0.0781 | 0.0487 | 0.6987 | 0.2716 | 0.1738 | 0.687 |
| $a+by^2/z+cx/z$ | 274.62 | 207.70 | 0.082 | 0.1422 | 0.1100 | 0.0014 | 0.4872 | 0.3719 | -0.006 |
| $a+by^2/z+cx/z^2$ | 258.27 | 198.08 | 0.188 | 0.1364 | 0.1100 | 0.0810 | 0.4588 | 0.3631 | 0.108 |
| $a+by^2/z+cx/\sqrt{z}$ | 240.13 | 178.62 | 0.298 | 0.1165 | 0.0860 | 0.3301 | 0.3781 | 0.2782 | 0.394 |
| $a+by^2/z+cxz$ | 124.79 | 96.02 | 0.811 | 0.0726 | 0.0500 | 0.7400 | 0.2618 | 0.1920 | 0.709 |
| $a+by^2/z+cxz^2$ | 150.29 | 117.14 | 0.725 | 0.0835 | 0.0636 | 0.6555 | 0.3062 | 0.2420 | 0.603 |
| $a+by^2/z+cx\sqrt{z}$ | 117.11 | 90.57 | 0.833 | 0.0695 | 0.0445 | 0.7614 | 0.2406 | 0.1600 | 0.755 |
| $a+by^2/z+cx^2/z$ | 263.30 | 190.69 | 0.156 | 0.1309 | 0.1027 | 0.1543 | 0.4303 | 0.3336 | 0.215 |
| $a+by^2/z+cx^2/z^2$ | 279.53 | 205.35 | 0.049 | 0.1431 | 0.1141 | -0.0112 | 0.4873 | 0.3775 | -0.006 |
| $a+by^2/z+cx^2/\sqrt{z}$ | 150.27 | 121.29 | 0.725 | 0.0857 | 0.0637 | 0.6370 | 0.2700 | 0.1896 | 0.691 |
| $a+by^2/z+cx^2z$ | 135.43 | 108.01 | 0.777 | 0.0792 | 0.0593 | 0.6903 | 0.2867 | 0.2214 | 0.652 |
| $a+by^2/z+cx^2z^2$ | 159.76 | 126.39 | 0.689 | 0.0895 | 0.0707 | 0.6044 | 0.3256 | 0.2605 | 0.551 |
| $a+by^2/z+cx^2\sqrt{z}$ | 123.80 | 96.70 | 0.814 | 0.0751 | 0.0553 | 0.7217 | 0.2655 | 0.1984 | 0.701 |
| $a+by^2/z+c\sqrt{x}/z$ | 214.18 | 170.74 | 0.442 | 0.1213 | 0.0940 | 0.2737 | 0.4064 | 0.3111 | 0.300 |
| $a+by^2/z+c\sqrt{x}/z^2$ | 241.63 | 186.00 | 0.290 | 0.1309 | 0.1051 | 0.1534 | 0.4348 | 0.3429 | 0.199 |
| $a+by^2/z+c\sqrt{x}/\sqrt{z}$ | 288.17 | 218.32 | -0.010 | 0.1474 | 0.1138 | -0.0721 | 0.5041 | 0.3883 | -0.077 |
| $a+by^2/z+c\sqrt{x}z$ | 124.22 | 96.30 | 0.812 | 0.0712 | 0.0460 | 0.7500 | 0.2553 | 0.1796 | 0.724 |
| $a+by^2/z+c\sqrt{x}z^2$ | 147.44 | 117.15 | 0.736 | 0.0813 | 0.0607 | 0.6738 | 0.2984 | 0.2332 | 0.623 |
| $a+by^2/z+c\sqrt{x}\sqrt{z}$ | 121.98 | 91.16 | 0.819 | 0.0696 | 0.0415 | 0.7608 | 0.2385 | 0.1467 | 0.759 |
| $a+by^2/z+c/xz$ | 246.82 | 177.73 | 0.259 | 0.1156 | 0.0878 | 0.3397 | 0.3896 | 0.2959 | 0.357 |
| $a+by^2/z+c/xz^2$ | 230.60 | 167.14 | 0.353 | 0.1143 | 0.0833 | 0.3551 | 0.3750 | 0.2712 | 0.404 |
| $a+by^2/z+c/x\sqrt{z}$ | 258.55 | 187.98 | 0.187 | 0.1198 | 0.0916 | 0.2919 | 0.4081 | 0.3100 | 0.294 |
| $a+by^2/z+cz/x$ | 295.88 | 213.33 | -0.065 | 0.1412 | 0.1073 | 0.0157 | 0.4847 | 0.3631 | 0.005 |
| $a+by^2/z+cz^2/x$ | 267.64 | 206.88 | 0.128 | 0.1420 | 0.1090 | 0.0043 | 0.4843 | 0.3680 | 0.006 |
| $a+by^2/z+c\sqrt{z}/x$ | 283.49 | 206.15 | 0.022 | 0.1325 | 0.1002 | 0.1336 | 0.4556 | 0.3421 | 0.120 |
| $a+by^2/z+c/x^2z$ | 283.84 | 206.50 | 0.020 | 0.1326 | 0.1006 | 0.1314 | 0.4566 | 0.3431 | 0.117 |
| $a+by^2/z+c/x^2z^2$ | 275.85 | 202.72 | 0.074 | 0.1286 | 0.0985 | 0.1836 | 0.4407 | 0.3325 | 0.177 |
| $a+by^2/z+c/x^2\sqrt{z}$ | 286.38 | 207.31 | 0.002 | 0.1341 | 0.1016 | 0.1121 | 0.4621 | 0.3463 | 0.095 |
| $a+by^2/z+cz/x^2$ | 291.11 | 208.22 | -0.031 | 0.1371 | 0.1033 | 0.0715 | 0.4730 | 0.3515 | 0.052 |
| $a+by^2/z+cz^2/x^2$ | 293.79 | 208.57 | -0.050 | 0.1391 | 0.1043 | 0.0440 | 0.4796 | 0.3541 | 0.025 |
| $a+by^2/z+c\sqrt{z}/x^2$ | 289.82 | 208.04 | -0.022 | 0.1363 | 0.1028 | 0.0834 | 0.4699 | 0.3501 | 0.064 |
| $a+by^2/z+c/\sqrt{x}z$ | 197.27 | 143.70 | 0.527 | 0.1006 | 0.0724 | 0.4999 | 0.3244 | 0.2242 | 0.554 |
| $a+by^2/z+c/\sqrt{x}z^2$ | 211.51 | 151.90 | 0.456 | 0.1148 | 0.0895 | 0.3496 | 0.3685 | 0.2720 | 0.425 |
| $a+by^2/z+c/\sqrt{x}\sqrt{z}$ | 209.15 | 151.85 | 0.468 | 0.1002 | 0.0726 | 0.5040 | 0.3311 | 0.2401 | 0.536 |
| $a+by^2/z+cz/\sqrt{x}$ | 231.33 | 173.44 | 0.349 | 0.1291 | 0.0935 | 0.1768 | 0.4405 | 0.3205 | 0.178 |
| $a+by^2/z+cz^2/\sqrt{x}$ | 152.71 | 126.90 | 0.716 | 0.0879 | 0.0626 | 0.6184 | 0.3152 | 0.2422 | 0.579 |
| $a+by^2/z+c\sqrt{z}/\sqrt{x}$ | 298.99 | 220.65 | -0.088 | 0.1445 | 0.1120 | -0.0304 | 0.4940 | 0.3785 | -0.034 |
| $a+by^2/z^2+cx/z$ | 267.50 | 192.10 | 0.129 | 0.1354 | 0.1057 | 0.0953 | 0.4533 | 0.3400 | 0.130 |
| $a+by^2/z^2+cx/z^2$ | 275.51 | 199.32 | 0.076 | 0.1407 | 0.1092 | 0.0222 | 0.4843 | 0.3698 | 0.006 |
| $a+by^2/z^2+cx/\sqrt{z}$ | 205.02 | 153.02 | 0.489 | 0.1089 | 0.0826 | 0.4142 | 0.3445 | 0.2502 | 0.497 |
| $a+by^2/z^2+cxz$ | 127.93 | 95.86 | 0.801 | 0.0726 | 0.0510 | 0.7397 | 0.2668 | 0.2032 | 0.698 |
| $a+by^2/z^2+cxz^2$ | 156.76 | 115.79 | 0.701 | 0.0853 | 0.0661 | 0.6409 | 0.3187 | 0.2498 | 0.570 |
| $a+by^2/z^2+cx\sqrt{z}$ | 117.08 | 90.34 | 0.833 | 0.0693 | 0.0441 | 0.7626 | 0.2390 | 0.1595 | 0.758 |
| $a+by^2/z^2+cx^2/z$ | 201.93 | 148.19 | 0.504 | 0.1114 | 0.0859 | 0.3868 | 0.3498 | 0.2624 | 0.481 |
| $a+by^2/z^2+cx^2/z^2$ | 259.32 | 183.76 | 0.182 | 0.1312 | 0.1002 | 0.1503 | 0.4433 | 0.3279 | 0.168 |
| $a+by^2/z^2+cx^2/\sqrt{z}$ | 155.57 | 117.74 | 0.706 | 0.0920 | 0.0674 | 0.5821 | 0.2861 | 0.2071 | 0.653 |
| $a+by^2/z^2+cx^2z$ | 138.16 | 104.02 | 0.768 | 0.0796 | 0.0606 | 0.6873 | 0.2925 | 0.2325 | 0.637 |
| $a+by^2/z^2+cx^2z^2$ | 163.63 | 123.40 | 0.674 | 0.0905 | 0.0724 | 0.5952 | 0.3350 | 0.2649 | 0.525 |
| $a+by^2/z^2+cx^2\sqrt{z}$ | 124.06 | 95.88 | 0.813 | 0.0750 | 0.0549 | 0.7224 | 0.2662 | 0.2008 | 0.700 |
| $a+by^2/z^2+c\sqrt{x}/z$ | 234.79 | 169.35 | 0.329 | 0.1269 | 0.0915 | 0.2047 | 0.4401 | 0.3165 | 0.179 |
| $a+by^2/z^2+c\sqrt{x}/z^2$ | 245.59 | 180.62 | 0.266 | 0.1328 | 0.1056 | 0.1286 | 0.4431 | 0.3393 | 0.168 |
| $a+by^2/z^2+c\sqrt{x}/\sqrt{z}$ | 269.41 | 193.34 | 0.117 | 0.1352 | 0.1066 | 0.0975 | 0.4555 | 0.3437 | 0.121 |
| $a+by^2/z^2+c\sqrt{x}z$ | 128.09 | 98.92 | 0.800 | 0.0710 | 0.0471 | 0.7509 | 0.2604 | 0.1911 | 0.713 |
| $a+by^2/z^2+c\sqrt{x}z^2$ | 155.45 | 118.15 | 0.706 | 0.0834 | 0.0633 | 0.6562 | 0.3129 | 0.2426 | 0.585 |
| $a+by^2/z^2+c\sqrt{x}\sqrt{z}$ | 121.87 | 91.07 | 0.819 | 0.0691 | 0.0418 | 0.7645 | 0.2358 | 0.1471 | 0.764 |
| $a+by^2/z^2+c/xz$ | 229.72 | 169.44 | 0.358 | 0.1126 | 0.0862 | 0.3734 | 0.3754 | 0.2784 | 0.403 |
| $a+by^2/z^2+c/xz^2$ | 221.39 | 162.76 | 0.404 | 0.1136 | 0.0845 | 0.3628 | 0.3706 | 0.2639 | 0.418 |
| $a+by^2/z^2+c/x\sqrt{z}$ | 237.19 | 173.27 | 0.315 | 0.1147 | 0.0885 | 0.3510 | 0.3867 | 0.2889 | 0.366 |
| $a+by^2/z^2+cz/x$ | 267.40 | 185.39 | 0.130 | 0.1298 | 0.0985 | 0.1678 | 0.4460 | 0.3259 | 0.157 |
| $a+by^2/z^2+cz^2/x$ | 271.21 | 194.54 | 0.105 | 0.1398 | 0.1064 | 0.0352 | 0.4838 | 0.3679 | 0.008 |
| $a+by^2/z^2+c\sqrt{z}/x$ | 255.77 | 182.37 | 0.204 | 0.1229 | 0.0944 | 0.2538 | 0.4212 | 0.3137 | 0.248 |
| $a+by^2/z^2+c/x^2z$ | 257.43 | 183.15 | 0.194 | 0.1235 | 0.0946 | 0.2464 | 0.4242 | 0.3172 | 0.237 |
| $a+by^2/z^2+c/x^2z^2$ | 250.11 | 181.44 | 0.239 | 0.1206 | 0.0930 | 0.2819 | 0.4107 | 0.3092 | 0.285 |
| $a+by^2/z^2+c/x^2\sqrt{z}$ | 259.96 | 183.41 | 0.178 | 0.1247 | 0.0951 | 0.2321 | 0.4293 | 0.3196 | 0.219 |
| $a+by^2/z^2+cz/x^2$ | 264.88 | 183.55 | 0.146 | 0.1273 | 0.0959 | 0.2003 | 0.4397 | 0.3236 | 0.181 |
| $a+by^2/z^2+cz^2/x^2$ | 267.65 | 183.69 | 0.128 | 0.1290 | 0.0965 | 0.1782 | 0.4460 | 0.3258 | 0.157 |
| $a+by^2/z^2+c\sqrt{z}/x^2$ | 263.52 | 183.54 | 0.155 | 0.1265 | 0.0956 | 0.2098 | 0.4368 | 0.3226 | 0.192 |
| $a+by^2/z^2+c/\sqrt{x}z$ | 196.78 | 143.65 | 0.529 | 0.1028 | 0.0767 | 0.4786 | 0.3287 | 0.2293 | 0.542 |
| $a+by^2/z^2+c/\sqrt{x}z^2$ | 211.50 | 151.83 | 0.456 | 0.1151 | 0.0906 | 0.3454 | 0.3686 | 0.2741 | 0.424 |
| $a+by^2/z^2+c/\sqrt{x}\sqrt{z}$ | 203.34 | 149.08 | 0.497 | 0.1019 | 0.0750 | 0.4876 | 0.3323 | 0.2335 | 0.532 |
| $a+by^2/z^2+cz/\sqrt{x}$ | 259.00 | 181.94 | 0.184 | 0.1354 | 0.1010 | 0.0944 | 0.4715 | 0.3474 | 0.058 |
| $a+by^2/z^2+cz^2/\sqrt{x}$ | 175.13 | 139.66 | 0.627 | 0.0945 | 0.0683 | 0.5586 | 0.3477 | 0.2650 | 0.488 |
| $a+by^2/z^2+c\sqrt{z}/\sqrt{x}$ | 267.84 | 187.27 | 0.127 | 0.1312 | 0.1011 | 0.1497 | 0.4480 | 0.3299 | 0.149 |
| $a+by^2/\sqrt{z}+cx/z$ | 207.79 | 169.15 | 0.475 | 0.1164 | 0.0919 | 0.3316 | 0.3909 | 0.2996 | 0.352 |

(continued on next page)

**Table 4 – continued from previous page**

| Functional form | $T_{eff}$ (K) | | | Radius ($R_\odot$) | | | log (L/$L_\odot$) | | |
|---|---|---|---|---|---|---|---|---|---|
| | RMSE | MAD | $R^2_{ap}$ | RMSE | MAD | $R^2_{ap}$ | RMSE | MAD | $R^2_{ap}$ |
| $a+by^2/\sqrt{z}+cx/z^2$ | 212.66 | 171.93 | 0.450 | 0.1185 | 0.0939 | 0.3068 | 0.3910 | 0.3020 | 0.352 |
| $a+by^2/\sqrt{z}+cx/\sqrt{z}$ | 247.57 | 202.41 | 0.254 | 0.1302 | 0.1058 | 0.1632 | 0.4283 | 0.3366 | 0.223 |
| $a+by^2/\sqrt{z}+cxz$ | 123.75 | 93.86 | 0.814 | 0.0729 | 0.0506 | 0.7375 | 0.2630 | 0.1922 | 0.707 |
| $a+by^2/\sqrt{z}+cxz^2$ | 141.10 | 110.69 | 0.758 | 0.0817 | 0.0595 | 0.6707 | 0.2946 | 0.2185 | 0.632 |
| $a+by^2/\sqrt{z}+cx\sqrt{z}$ | 117.12 | 90.67 | 0.833 | 0.0690 | 0.0450 | 0.7650 | 0.2417 | 0.1606 | 0.752 |
| $a+by^2/\sqrt{z}+cx^2/z$ | 243.74 | 196.34 | 0.277 | 0.1286 | 0.1006 | 0.1835 | 0.4273 | 0.3305 | 0.226 |
| $a+by^2/\sqrt{z}+cx^2/z^2$ | 221.25 | 179.69 | 0.404 | 0.1208 | 0.0950 | 0.2794 | 0.4019 | 0.3071 | 0.316 |
| $a+by^2/\sqrt{z}+cx^2/\sqrt{z}$ | 188.82 | 143.82 | 0.566 | 0.1012 | 0.0764 | 0.4946 | 0.3133 | 0.2367 | 0.584 |
| $a+by^2/\sqrt{z}+cx^2z$ | 132.67 | 104.59 | 0.786 | 0.0790 | 0.0587 | 0.6921 | 0.2837 | 0.2134 | 0.659 |
| $a+by^2/\sqrt{z}+cx^2z^2$ | 149.02 | 119.08 | 0.730 | 0.0869 | 0.0647 | 0.6274 | 0.3102 | 0.2321 | 0.592 |
| $a+by^2/\sqrt{z}+cx^2\sqrt{z}$ | 123.64 | 96.67 | 0.814 | 0.0750 | 0.0553 | 0.7221 | 0.2661 | 0.1991 | 0.700 |
| $a+by^2/\sqrt{z}+c\sqrt{x}/z$ | 185.21 | 149.89 | 0.583 | 0.1087 | 0.0837 | 0.4163 | 0.3613 | 0.2743 | 0.447 |
| $a+by^2/\sqrt{z}+c\sqrt{x}/z^2$ | 205.70 | 162.98 | 0.485 | 0.1165 | 0.0921 | 0.3293 | 0.3813 | 0.2925 | 0.384 |
| $a+by^2/\sqrt{z}+c\sqrt{x}/\sqrt{z}$ | 207.37 | 170.77 | 0.477 | 0.1179 | 0.0930 | 0.3140 | 0.3955 | 0.3024 | 0.337 |
| $a+by^2/\sqrt{z}+c\sqrt{x}z$ | 123.29 | 94.45 | 0.815 | 0.0717 | 0.0470 | 0.7458 | 0.2577 | 0.1820 | 0.719 |
| $a+by^2/\sqrt{z}+c\sqrt{x}z^2$ | 138.48 | 108.97 | 0.767 | 0.0797 | 0.0574 | 0.6866 | 0.2882 | 0.2122 | 0.648 |
| $a+by^2/\sqrt{z}+c\sqrt{x}\sqrt{z}$ | 121.96 | 90.97 | 0.819 | 0.0693 | 0.0420 | 0.7630 | 0.2401 | 0.1487 | 0.756 |
| $a+by^2/\sqrt{z}+c/xz$ | 244.20 | 196.61 | 0.274 | 0.1226 | 0.0967 | 0.2575 | 0.4005 | 0.3123 | 0.320 |
| $a+by^2/\sqrt{z}+c/xz^2$ | 234.79 | 181.78 | 0.329 | 0.1203 | 0.0938 | 0.2854 | 0.3867 | 0.2887 | 0.366 |
| $a+by^2/\sqrt{z}+c/x\sqrt{z}$ | 247.47 | 200.82 | 0.255 | 0.1247 | 0.0999 | 0.2321 | 0.4096 | 0.3236 | 0.289 |
| $a+by^2/\sqrt{z}+cz/x$ | 243.66 | 202.83 | 0.278 | 0.1302 | 0.1061 | 0.1625 | 0.4287 | 0.3357 | 0.221 |
| $a+by^2/\sqrt{z}+cz^2/x$ | 194.16 | 157.18 | 0.541 | 0.1163 | 0.0895 | 0.3324 | 0.3856 | 0.2916 | 0.370 |
| $a+by^2/\sqrt{z}+c\sqrt{z}/x$ | 248.83 | 202.26 | 0.247 | 0.1291 | 0.1035 | 0.1773 | 0.4254 | 0.3319 | 0.233 |
| $a+by^2/\sqrt{z}+c/x^2z$ | 249.16 | 202.72 | 0.245 | 0.1286 | 0.1034 | 0.1830 | 0.4243 | 0.3320 | 0.237 |
| $a+by^2/\sqrt{z}+c/x^2z^2$ | 249.41 | 203.05 | 0.243 | 0.1280 | 0.1026 | 0.1904 | 0.4216 | 0.3315 | 0.247 |
| $a+by^2/\sqrt{z}+c/x^2\sqrt{z}$ | 248.98 | 202.34 | 0.246 | 0.1288 | 0.1035 | 0.1805 | 0.4251 | 0.3317 | 0.234 |
| $a+by^2/\sqrt{z}+cz/x^2$ | 248.38 | 201.06 | 0.249 | 0.1293 | 0.1036 | 0.1748 | 0.4267 | 0.3305 | 0.229 |
| $a+by^2/\sqrt{z}+cz^2/x^2$ | 247.56 | 201.02 | 0.254 | 0.1297 | 0.1042 | 0.1697 | 0.4277 | 0.3308 | 0.225 |
| $a+by^2/\sqrt{z}+c\sqrt{z}/x^2$ | 248.60 | 201.52 | 0.248 | 0.1291 | 0.1036 | 0.1766 | 0.4262 | 0.3310 | 0.230 |
| $a+by^2/\sqrt{z}+c/\sqrt{x}z$ | 203.88 | 143.14 | 0.494 | 0.1053 | 0.0811 | 0.4521 | 0.3332 | 0.2408 | 0.530 |
| $a+by^2/\sqrt{z}+c/\sqrt{x}z^2$ | 204.60 | 153.92 | 0.491 | 0.1131 | 0.0888 | 0.3688 | 0.3573 | 0.2654 | 0.459 |
| $a+by^2/\sqrt{z}+c/\sqrt{x}\sqrt{z}$ | 219.96 | 162.01 | 0.411 | 0.1087 | 0.0822 | 0.4161 | 0.3504 | 0.2469 | 0.480 |
| $a+by^2/\sqrt{z}+cz/\sqrt{x}$ | 173.12 | 131.78 | 0.635 | 0.1075 | 0.0776 | 0.4294 | 0.3593 | 0.2539 | 0.453 |
| $a+by^2/\sqrt{z}+cz^2/\sqrt{x}$ | 136.73 | 105.87 | 0.773 | 0.0837 | 0.0561 | 0.6543 | 0.2955 | 0.2057 | 0.630 |
| $a+by^2/\sqrt{z}+c\sqrt{z}/\sqrt{x}$ | 235.24 | 199.57 | 0.327 | 0.1291 | 0.1051 | 0.1777 | 0.4252 | 0.3374 | 0.234 |
| $a+by^2z+cx/z$ | 148.16 | 115.77 | 0.733 | 0.0853 | 0.0613 | 0.6407 | 0.3061 | 0.2297 | 0.603 |
| $a+by^2z+cx/z^2$ | 149.36 | 112.84 | 0.729 | 0.0864 | 0.0633 | 0.6316 | 0.3149 | 0.2411 | 0.580 |
| $a+by^2z+cx/\sqrt{z}$ | 138.66 | 106.69 | 0.766 | 0.0815 | 0.0573 | 0.6721 | 0.2808 | 0.1924 | 0.666 |
| $a+by^2z+cxz$ | 127.29 | 97.10 | 0.803 | 0.0702 | 0.0510 | 0.7569 | 0.2564 | 0.1919 | 0.721 |
| $a+by^2z+cxz^2$ | 149.24 | 112.56 | 0.729 | 0.0846 | 0.0652 | 0.6463 | 0.3135 | 0.2466 | 0.584 |
| $a+by^2z+cx\sqrt{z}$ | 117.12 | 90.77 | 0.833 | 0.0691 | 0.0442 | 0.7642 | 0.2323 | 0.1531 | 0.771 |
| $a+by^2z+cx^2/z$ | 139.30 | 108.70 | 0.764 | 0.0828 | 0.0602 | 0.6611 | 0.2875 | 0.2051 | 0.650 |
| $a+by^2z+cx^2/z^2$ | 149.24 | 114.94 | 0.729 | 0.0859 | 0.0621 | 0.6358 | 0.3112 | 0.2387 | 0.590 |
| $a+by^2z+cx^2/\sqrt{z}$ | 128.53 | 99.28 | 0.799 | 0.0794 | 0.0562 | 0.6885 | 0.2667 | 0.1848 | 0.699 |
| $a+by^2z+cx^2z$ | 138.01 | 103.08 | 0.768 | 0.0790 | 0.0612 | 0.6922 | 0.2905 | 0.2319 | 0.642 |
| $a+by^2z+cx^2z^2$ | 149.59 | 111.66 | 0.728 | 0.0864 | 0.0638 | 0.6315 | 0.3146 | 0.2377 | 0.581 |
| $a+by^2z+cx^2\sqrt{z}$ | 123.28 | 98.15 | 0.815 | 0.0743 | 0.0545 | 0.7275 | 0.2582 | 0.1971 | 0.717 |
| $a+by^2z+c\sqrt{x}/z$ | 149.13 | 113.34 | 0.729 | 0.0864 | 0.0634 | 0.6314 | 0.3149 | 0.2407 | 0.580 |
| $a+by^2z+c\sqrt{x}/z^2$ | 146.91 | 112.33 | 0.737 | 0.0863 | 0.0635 | 0.6322 | 0.3144 | 0.2413 | 0.581 |
| $a+by^2z+c\sqrt{x}/\sqrt{z}$ | 147.76 | 115.37 | 0.734 | 0.0847 | 0.0601 | 0.6459 | 0.3025 | 0.2191 | 0.612 |
| $a+by^2z+c\sqrt{x}z$ | 129.44 | 99.97 | 0.796 | 0.0711 | 0.0488 | 0.7506 | 0.2600 | 0.1889 | 0.714 |
| $a+by^2z+c\sqrt{x}z^2$ | 148.45 | 111.44 | 0.732 | 0.0833 | 0.0639 | 0.6577 | 0.3105 | 0.2451 | 0.591 |
| $a+by^2z+c\sqrt{x}\sqrt{z}$ | 120.80 | 90.70 | 0.822 | 0.0696 | 0.0419 | 0.7608 | 0.2372 | 0.1457 | 0.762 |
| $a+by^2z+c/xz$ | 142.79 | 108.67 | 0.752 | 0.0799 | 0.0540 | 0.6849 | 0.2811 | 0.1893 | 0.665 |
| $a+by^2z+c/xz^2$ | 135.40 | 100.94 | 0.777 | 0.0794 | 0.0523 | 0.6889 | 0.2733 | 0.1744 | 0.684 |
| $a+by^2z+c/x\sqrt{z}$ | 145.62 | 111.38 | 0.742 | 0.0807 | 0.0553 | 0.6784 | 0.2871 | 0.1973 | 0.651 |
| $a+by^2z+cz/x$ | 149.44 | 113.38 | 0.728 | 0.0836 | 0.0580 | 0.6549 | 0.3028 | 0.2147 | 0.611 |
| $a+by^2z+cz^2/x$ | 149.67 | 112.50 | 0.727 | 0.0854 | 0.0610 | 0.6396 | 0.3099 | 0.2252 | 0.593 |
| $a+by^2z+c\sqrt{z}/x$ | 148.80 | 113.46 | 0.731 | 0.0826 | 0.0574 | 0.6629 | 0.2983 | 0.2107 | 0.623 |
| $a+by^2z+c/x^2z$ | 149.00 | 113.37 | 0.730 | 0.0827 | 0.0575 | 0.6627 | 0.2991 | 0.2118 | 0.621 |
| $a+by^2z+c/x^2z^2$ | 147.71 | 112.88 | 0.735 | 0.0819 | 0.0566 | 0.6686 | 0.2941 | 0.2059 | 0.633 |
| $a+by^2z+c/x^2\sqrt{z}$ | 149.29 | 113.32 | 0.729 | 0.0829 | 0.0577 | 0.6604 | 0.3008 | 0.2136 | 0.617 |
| $a+by^2z+cz/x^2$ | 149.63 | 112.91 | 0.728 | 0.0835 | 0.0581 | 0.6557 | 0.3040 | 0.2165 | 0.608 |
| $a+by^2z+cz^2/x^2$ | 149.68 | 112.65 | 0.727 | 0.0838 | 0.0582 | 0.6535 | 0.3052 | 0.2174 | 0.605 |
| $a+by^2z+c\sqrt{z}/x^2$ | 149.57 | 113.05 | 0.728 | 0.0833 | 0.0580 | 0.6570 | 0.3032 | 0.2158 | 0.611 |
| $a+by^2z+c/\sqrt{x}z$ | 129.75 | 96.70 | 0.795 | 0.0772 | 0.0503 | 0.7059 | 0.2619 | 0.1591 | 0.709 |
| $a+by^2z+c/\sqrt{x}z^2$ | 126.84 | 94.07 | 0.804 | 0.0805 | 0.0546 | 0.6800 | 0.2761 | 0.1746 | 0.677 |
| $a+by^2z+c/\sqrt{x}\sqrt{z}$ | 136.65 | 102.01 | 0.773 | 0.0776 | 0.0512 | 0.7030 | 0.2676 | 0.1716 | 0.697 |
| $a+by^2z+cz/\sqrt{x}$ | 149.54 | 113.08 | 0.728 | 0.0860 | 0.0623 | 0.6346 | 0.3122 | 0.2314 | 0.587 |
| $a+by^2z+cz^2/\sqrt{x}$ | 148.74 | 113.01 | 0.731 | 0.0858 | 0.0640 | 0.6366 | 0.3149 | 0.2440 | 0.580 |
| $a+by^2z+c\sqrt{z}/\sqrt{x}$ | 148.92 | 113.95 | 0.730 | 0.0836 | 0.0577 | 0.6545 | 0.3010 | 0.2115 | 0.616 |
| $a+by^2z^2+cx/z$ | 167.94 | 129.58 | 0.657 | 0.0925 | 0.0735 | 0.5774 | 0.3363 | 0.2657 | 0.521 |
| $a+by^2z^2+cx/z^2$ | 167.70 | 126.61 | 0.658 | 0.0936 | 0.0732 | 0.5674 | 0.3447 | 0.2669 | 0.497 |
| $a+by^2z^2+cx/\sqrt{z}$ | 147.78 | 115.94 | 0.734 | 0.0842 | 0.0630 | 0.6500 | 0.2917 | 0.2157 | 0.639 |
| $a+by^2z^2+cxz$ | 124.76 | 98.36 | 0.811 | 0.0697 | 0.0455 | 0.7598 | 0.2479 | 0.1705 | 0.740 |
| $a+by^2z^2+cxz^2$ | 153.69 | 113.63 | 0.713 | 0.0800 | 0.0615 | 0.6837 | 0.3009 | 0.2369 | 0.616 |
| $a+by^2z^2+cx\sqrt{z}$ | 116.99 | 89.45 | 0.833 | 0.0696 | 0.0438 | 0.7611 | 0.2365 | 0.1500 | 0.763 |
| $a+by^2z^2+cx^2/z$ | 150.65 | 116.49 | 0.724 | 0.0868 | 0.0675 | 0.6280 | 0.3031 | 0.2330 | 0.611 |
| $a+by^2z^2+cx^2/z^2$ | 169.58 | 130.25 | 0.650 | 0.0935 | 0.0734 | 0.5681 | 0.3430 | 0.2700 | 0.502 |
| $a+by^2z^2+cx^2/\sqrt{z}$ | 127.80 | 102.52 | 0.801 | 0.0791 | 0.0598 | 0.6909 | 0.2653 | 0.1944 | 0.702 |
| $a+by^2z^2+cx^2z$ | 132.46 | 104.09 | 0.787 | 0.0763 | 0.0573 | 0.7127 | 0.2727 | 0.2127 | 0.685 |
| $a+by^2z^2+cx^2z^2$ | 163.96 | 127.38 | 0.673 | 0.0900 | 0.0726 | 0.5997 | 0.3326 | 0.2660 | 0.531 |
| $a+by^2z^2+cx^2\sqrt{z}$ | 123.34 | 98.03 | 0.815 | 0.0746 | 0.0536 | 0.7252 | 0.2586 | 0.1903 | 0.717 |
| $a+by^2z^2+c\sqrt{x}/z$ | 167.48 | 126.97 | 0.659 | 0.0936 | 0.0730 | 0.5676 | 0.3447 | 0.2669 | 0.497 |
| $a+by^2z^2+c\sqrt{x}/z^2$ | 162.10 | 124.34 | 0.680 | 0.0926 | 0.0725 | 0.5763 | 0.3400 | 0.2629 | 0.510 |
| $a+by^2z^2+c\sqrt{x}/\sqrt{z}$ | 166.25 | 128.18 | 0.664 | 0.0911 | 0.0718 | 0.5900 | 0.3294 | 0.2559 | 0.540 |
| $a+by^2z^2+c\sqrt{x}z$ | 128.63 | 101.08 | 0.799 | 0.0706 | 0.0451 | 0.7536 | 0.2536 | 0.1734 | 0.727 |
| $a+by^2z^2+c\sqrt{x}z^2$ | 154.34 | 115.26 | 0.710 | 0.0801 | 0.0607 | 0.6835 | 0.3014 | 0.2357 | 0.615 |
| $a+by^2z^2+c\sqrt{x}\sqrt{z}$ | 120.35 | 89.94 | 0.824 | 0.0695 | 0.0417 | 0.7614 | 0.2387 | 0.1433 | 0.759 |

(continued on next page)

**Table 4 – continued from previous page**

| Functional form | $T_{eff}$ (K) | | | Radius ($R_{\odot}$) | | | log (L/$L_{\odot}$) | | |
|---|---|---|---|---|---|---|---|---|---|
| | RMSE | MAD | $R^2_{ap}$ | RMSE | MAD | $R^2_{ap}$ | RMSE | MAD | $R^2_{ap}$ |
| $a+by^2z^2+c/xz$ | 152.78 | 116.55 | 0.716 | 0.0818 | 0.0584 | 0.6697 | 0.2906 | 0.2049 | 0.642 |
| $a+by^2z^2+c/xz^2$ | 140.91 | 103.73 | 0.758 | 0.0805 | 0.0556 | 0.6804 | 0.2786 | 0.1878 | 0.671 |
| $a+by^2z^2+c/x\sqrt{z}$ | 158.05 | 120.93 | 0.696 | 0.0834 | 0.0606 | 0.6569 | 0.2998 | 0.2142 | 0.619 |
| $a+by^2z^2+cz/x$ | 167.34 | 126.11 | 0.659 | 0.0886 | 0.0659 | 0.6125 | 0.3246 | 0.2350 | 0.553 |
| $a+by^2z^2+cz^2/x$ | 169.40 | 128.19 | 0.651 | 0.0918 | 0.0703 | 0.5838 | 0.3370 | 0.2502 | 0.519 |
| $a+by^2z^2+c\sqrt{z}/x$ | 165.22 | 125.36 | 0.668 | 0.0869 | 0.0647 | 0.6275 | 0.3172 | 0.2299 | 0.574 |
| $a+by^2z^2+c/x^2z$ | 165.73 | 125.47 | 0.666 | 0.0870 | 0.0645 | 0.6265 | 0.3184 | 0.2289 | 0.571 |
| $a+by^2z^2+c/x^2z^2$ | 162.71 | 124.20 | 0.678 | 0.0856 | 0.0631 | 0.6380 | 0.3109 | 0.2239 | 0.590 |
| $a+by^2z^2+c/x^2\sqrt{z}$ | 166.62 | 125.64 | 0.662 | 0.0875 | 0.0648 | 0.6221 | 0.3210 | 0.2305 | 0.563 |
| $a+by^2z^2+cz/x^2$ | 168.01 | 125.60 | 0.657 | 0.0885 | 0.0654 | 0.6133 | 0.3260 | 0.2331 | 0.550 |
| $a+by^2z^2+cz^2/x^2$ | 168.45 | 125.54 | 0.655 | 0.0890 | 0.0657 | 0.6092 | 0.3279 | 0.2340 | 0.544 |
| $a+by^2z^2+c\sqrt{z}/x^2$ | 167.69 | 125.63 | 0.658 | 0.0882 | 0.0653 | 0.6157 | 0.3247 | 0.2325 | 0.553 |
| $a+by^2z^2+c/\sqrt{x}z$ | 130.71 | 95.60 | 0.792 | 0.0766 | 0.0515 | 0.7100 | 0.2613 | 0.1683 | 0.711 |
| $a+by^2z^2+c/\sqrt{x}z^2$ | 127.70 | 93.21 | 0.802 | 0.0813 | 0.0575 | 0.6737 | 0.2793 | 0.1861 | 0.669 |
| $a+by^2z^2+c/\sqrt{x}\sqrt{z}$ | 141.43 | 105.47 | 0.757 | 0.0777 | 0.0530 | 0.7019 | 0.2701 | 0.1830 | 0.691 |
| $a+by^2z^2+cz/\sqrt{x}$ | 169.62 | 129.74 | 0.650 | 0.0931 | 0.0725 | 0.5716 | 0.3419 | 0.2605 | 0.505 |
| $a+by^2z^2+cz^2/\sqrt{x}$ | 165.94 | 128.90 | 0.665 | 0.0919 | 0.0695 | 0.5830 | 0.3404 | 0.2609 | 0.509 |
| $a+by^2z^2+c\sqrt{z}/\sqrt{x}$ | 166.24 | 126.67 | 0.664 | 0.0887 | 0.0663 | 0.6118 | 0.3227 | 0.2372 | 0.559 |
| $a+by^2\sqrt{z}+cx/z$ | 144.49 | 104.28 | 0.746 | 0.0858 | 0.0597 | 0.6363 | 0.3002 | 0.2026 | 0.618 |
| $a+by^2\sqrt{z}+cx/z^2$ | 144.16 | 105.73 | 0.747 | 0.0860 | 0.0604 | 0.6350 | 0.3038 | 0.2138 | 0.609 |
| $a+by^2\sqrt{z}+cx/\sqrt{z}$ | 141.75 | 105.20 | 0.756 | 0.0845 | 0.0565 | 0.6476 | 0.2871 | 0.1888 | 0.651 |
| $a+by^2\sqrt{z}+cxz$ | 128.08 | 97.40 | 0.800 | 0.0727 | 0.0534 | 0.7392 | 0.2701 | 0.2061 | 0.691 |
| $a+by^2\sqrt{z}+cxz^2$ | 141.24 | 106.72 | 0.757 | 0.0824 | 0.0613 | 0.6645 | 0.3006 | 0.2283 | 0.617 |
| $a+by^2\sqrt{z}+cx\sqrt{z}$ | 117.05 | 91.19 | 0.833 | 0.0680 | 0.0449 | 0.7714 | 0.2317 | 0.1574 | 0.772 |
| $a+by^2\sqrt{z}+cx^2/z$ | 141.70 | 105.22 | 0.756 | 0.0851 | 0.0582 | 0.6426 | 0.2908 | 0.1982 | 0.642 |
| $a+by^2\sqrt{z}+cx^2/z^2$ | 144.48 | 104.40 | 0.746 | 0.0858 | 0.0597 | 0.6365 | 0.3014 | 0.2070 | 0.615 |
| $a+by^2\sqrt{z}+cx^2/\sqrt{z}$ | 135.59 | 103.21 | 0.776 | 0.0830 | 0.0565 | 0.6600 | 0.2754 | 0.1887 | 0.679 |
| $a+by^2\sqrt{z}+cx^2z$ | 135.75 | 103.60 | 0.776 | 0.0796 | 0.0606 | 0.6868 | 0.2919 | 0.2289 | 0.639 |
| $a+by^2\sqrt{z}+cx^2z^2$ | 143.01 | 107.28 | 0.751 | 0.0846 | 0.0612 | 0.6463 | 0.3037 | 0.2200 | 0.609 |
| $a+by^2\sqrt{z}+cx^2\sqrt{z}$ | 123.95 | 96.12 | 0.813 | 0.0742 | 0.0557 | 0.7278 | 0.2642 | 0.2039 | 0.704 |
| $a+by^2\sqrt{z}+c\sqrt{x}/z$ | 143.18 | 105.57 | 0.751 | 0.0859 | 0.0608 | 0.6353 | 0.3041 | 0.2148 | 0.608 |
| $a+by^2\sqrt{z}+c\sqrt{x}/z^2$ | 142.50 | 105.69 | 0.753 | 0.0859 | 0.0607 | 0.6352 | 0.3038 | 0.2153 | 0.609 |
| $a+by^2\sqrt{z}+c\sqrt{x}/\sqrt{z}$ | 144.54 | 104.58 | 0.746 | 0.0857 | 0.0594 | 0.6370 | 0.2992 | 0.1988 | 0.621 |
| $a+by^2\sqrt{z}+c\sqrt{x}z$ | 127.99 | 100.08 | 0.801 | 0.0722 | 0.0492 | 0.7427 | 0.2671 | 0.1965 | 0.698 |
| $a+by^2\sqrt{z}+c\sqrt{x}z^2$ | 140.24 | 106.57 | 0.761 | 0.0812 | 0.0607 | 0.6742 | 0.2981 | 0.2292 | 0.623 |
| $a+by^2\sqrt{z}+c\sqrt{x}\sqrt{z}$ | 121.11 | 91.00 | 0.822 | 0.0693 | 0.0437 | 0.7627 | 0.2370 | 0.1494 | 0.762 |
| $a+by^2\sqrt{z}+c/xz$ | 143.04 | 104.86 | 0.751 | 0.0829 | 0.0547 | 0.6609 | 0.2847 | 0.1807 | 0.657 |
| $a+by^2\sqrt{z}+c/xz^2$ | 139.19 | 102.80 | 0.764 | 0.0827 | 0.0538 | 0.6622 | 0.2795 | 0.1702 | 0.669 |
| $a+by^2\sqrt{z}+c/x\sqrt{z}$ | 144.08 | 105.20 | 0.747 | 0.0833 | 0.0555 | 0.6574 | 0.2886 | 0.1859 | 0.647 |
| $a+by^2\sqrt{z}+cz/x$ | 144.08 | 103.56 | 0.747 | 0.0850 | 0.0575 | 0.6430 | 0.2989 | 0.1975 | 0.622 |
| $a+by^2\sqrt{z}+cz^2/x$ | 142.37 | 104.67 | 0.753 | 0.0860 | 0.0604 | 0.6350 | 0.3033 | 0.2085 | 0.610 |
| $a+by^2\sqrt{z}+c\sqrt{z}/x$ | 144.48 | 104.28 | 0.746 | 0.0844 | 0.0568 | 0.6481 | 0.2959 | 0.1950 | 0.629 |
| $a+by^2\sqrt{z}+c/x^2z$ | 144.45 | 104.14 | 0.746 | 0.0843 | 0.0568 | 0.6487 | 0.2961 | 0.1956 | 0.628 |
| $a+by^2\sqrt{z}+c/x^2z^2$ | 144.53 | 104.89 | 0.746 | 0.0840 | 0.0562 | 0.6515 | 0.2932 | 0.1914 | 0.636 |
| $a+by^2\sqrt{z}+c/x^2\sqrt{z}$ | 144.31 | 103.80 | 0.747 | 0.0845 | 0.0570 | 0.6477 | 0.2971 | 0.1969 | 0.626 |
| $a+by^2\sqrt{z}+cz/x^2$ | 143.90 | 102.93 | 0.748 | 0.0847 | 0.0573 | 0.6454 | 0.2989 | 0.1989 | 0.621 |
| $a+by^2\sqrt{z}+cz^2/x^2$ | 143.67 | 102.52 | 0.749 | 0.0849 | 0.0574 | 0.6441 | 0.2997 | 0.1994 | 0.619 |
| $a+by^2\sqrt{z}+c\sqrt{z}/x^2$ | 144.03 | 103.19 | 0.748 | 0.0847 | 0.0572 | 0.6461 | 0.2984 | 0.1984 | 0.623 |
| $a+by^2\sqrt{z}+c/\sqrt{x}z$ | 135.14 | 100.63 | 0.778 | 0.0808 | 0.0530 | 0.6774 | 0.2694 | 0.1606 | 0.693 |
| $a+by^2\sqrt{z}+c/\sqrt{x}z^2$ | 132.35 | 99.19 | 0.787 | 0.0832 | 0.0555 | 0.6586 | 0.2803 | 0.1705 | 0.667 |
| $a+by^2\sqrt{z}+c/\sqrt{x}\sqrt{z}$ | 139.71 | 103.07 | 0.763 | 0.0811 | 0.0531 | 0.6752 | 0.2740 | 0.1694 | 0.682 |
| $a+by^2\sqrt{z}+cz/\sqrt{x}$ | 141.91 | 105.44 | 0.755 | 0.0859 | 0.0609 | 0.6353 | 0.3039 | 0.2124 | 0.609 |
| $a+by^2\sqrt{z}+cz^2/\sqrt{x}$ | 139.62 | 105.41 | 0.763 | 0.0834 | 0.0597 | 0.6568 | 0.3013 | 0.2248 | 0.615 |
| $a+by^2\sqrt{z}+c\sqrt{z}/\sqrt{x}$ | 144.36 | 104.27 | 0.746 | 0.0852 | 0.0580 | 0.6412 | 0.2984 | 0.1965 | 0.623 |
| $a+b\sqrt{y}/z+cx/z$ | 157.12 | 114.54 | 0.700 | 0.0926 | 0.0706 | 0.5766 | 0.2800 | 0.1960 | 0.668 |
| $a+b\sqrt{y}/z+cx/z^2$ | 165.81 | 132.77 | 0.665 | 0.0902 | 0.0659 | 0.5986 | 0.3086 | 0.2238 | 0.597 |
| $a+b\sqrt{y}/z+cx/\sqrt{z}$ | 155.30 | 111.80 | 0.707 | 0.0912 | 0.0681 | 0.5893 | 0.2794 | 0.1896 | 0.669 |
| $a+b\sqrt{y}/z+cxz$ | 128.31 | 95.80 | 0.800 | 0.0731 | 0.0524 | 0.7361 | 0.2701 | 0.2082 | 0.691 |
| $a+b\sqrt{y}/z+cxz^2$ | 152.57 | 113.76 | 0.717 | 0.0848 | 0.0658 | 0.6449 | 0.3167 | 0.2474 | 0.575 |
| $a+b\sqrt{y}/z+cx\sqrt{z}$ | 116.77 | 91.09 | 0.834 | 0.0695 | 0.0446 | 0.7616 | 0.2408 | 0.1619 | 0.754 |
| $a+b\sqrt{y}/z+cx^2/z$ | 147.68 | 104.29 | 0.735 | 0.0921 | 0.0693 | 0.5808 | 0.2789 | 0.1966 | 0.670 |
| $a+b\sqrt{y}/z+cx^2/z^2$ | 144.53 | 108.23 | 0.746 | 0.0877 | 0.0618 | 0.6206 | 0.2763 | 0.1865 | 0.677 |
| $a+b\sqrt{y}/z+cx^2/\sqrt{z}$ | 135.61 | 102.27 | 0.776 | 0.0857 | 0.0615 | 0.6375 | 0.2650 | 0.1844 | 0.702 |
| $a+b\sqrt{y}/z+cx^2z$ | 136.11 | 102.80 | 0.775 | 0.0796 | 0.0611 | 0.6874 | 0.2931 | 0.2339 | 0.636 |
| $a+b\sqrt{y}/z+cx^2z^2$ | 156.14 | 116.73 | 0.703 | 0.0888 | 0.0706 | 0.6108 | 0.3281 | 0.2580 | 0.544 |
| $a+b\sqrt{y}/z+cx^2\sqrt{z}$ | 122.82 | 94.77 | 0.816 | 0.0750 | 0.0553 | 0.7219 | 0.2675 | 0.2033 | 0.697 |
| $a+b\sqrt{y}/z+c\sqrt{x}/z$ | 185.24 | 142.61 | 0.582 | 0.0978 | 0.0731 | 0.5276 | 0.3151 | 0.2292 | 0.579 |
| $a+b\sqrt{y}/z+c\sqrt{x}/z^2$ | 206.37 | 152.80 | 0.482 | 0.1055 | 0.0793 | 0.4507 | 0.3777 | 0.2685 | 0.396 |
| $a+b\sqrt{y}/z+c\sqrt{x}/\sqrt{z}$ | 182.19 | 133.48 | 0.596 | 0.0997 | 0.0724 | 0.5097 | 0.3162 | 0.2159 | 0.576 |
| $a+b\sqrt{y}/z+c\sqrt{x}z$ | 129.41 | 99.77 | 0.796 | 0.0716 | 0.0487 | 0.7468 | 0.2647 | 0.1972 | 0.703 |
| $a+b\sqrt{y}/z+c\sqrt{x}z^2$ | 152.63 | 116.03 | 0.717 | 0.0835 | 0.0637 | 0.6560 | 0.3130 | 0.2421 | 0.585 |
| $a+b\sqrt{y}/z+c\sqrt{x}\sqrt{z}$ | 122.02 | 92.81 | 0.819 | 0.0693 | 0.0421 | 0.7630 | 0.2381 | 0.1507 | 0.760 |
| $a+b\sqrt{y}/z+c/xz$ | 190.44 | 136.35 | 0.559 | 0.0984 | 0.0683 | 0.5220 | 0.3261 | 0.2220 | 0.549 |
| $a+b\sqrt{y}/z+c/xz^2$ | 189.70 | 132.49 | 0.562 | 0.1023 | 0.0727 | 0.4828 | 0.3336 | 0.2186 | 0.529 |
| $a+b\sqrt{y}/z+c/x\sqrt{z}$ | 193.77 | 138.78 | 0.543 | 0.0984 | 0.0697 | 0.5219 | 0.3300 | 0.2276 | 0.538 |
| $a+b\sqrt{y}/z+cz/x$ | 211.52 | 146.13 | 0.456 | 0.1063 | 0.0753 | 0.4421 | 0.3642 | 0.2505 | 0.438 |
| $a+b\sqrt{y}/z+cz^2/x$ | 229.58 | 161.41 | 0.359 | 0.1207 | 0.0897 | 0.2805 | 0.4154 | 0.3036 | 0.269 |
| $a+b\sqrt{y}/z+c\sqrt{z}/x$ | 203.94 | 143.69 | 0.494 | 0.1021 | 0.0730 | 0.4857 | 0.3484 | 0.2416 | 0.486 |
| $a+b\sqrt{y}/z+c/x^2z$ | 206.63 | 144.79 | 0.481 | 0.1031 | 0.0732 | 0.4748 | 0.3536 | 0.2465 | 0.470 |
| $a+b\sqrt{y}/z+c/x^2z^2$ | 201.28 | 143.00 | 0.507 | 0.1015 | 0.0716 | 0.4915 | 0.3440 | 0.2402 | 0.498 |
| $a+b\sqrt{y}/z+c/x^2\sqrt{z}$ | 208.59 | 145.18 | 0.471 | 0.1039 | 0.0738 | 0.4671 | 0.3574 | 0.2485 | 0.459 |
| $a+b\sqrt{y}/z+cz/x^2$ | 212.50 | 145.59 | 0.451 | 0.1057 | 0.0747 | 0.4487 | 0.3656 | 0.2521 | 0.434 |
| $a+b\sqrt{y}/z+cz^2/x^2$ | 214.61 | 145.85 | 0.440 | 0.1069 | 0.0753 | 0.4357 | 0.3703 | 0.2540 | 0.419 |
| $a+b\sqrt{y}/z+c\sqrt{z}/x^2$ | 211.43 | 145.51 | 0.456 | 0.1051 | 0.0744 | 0.4542 | 0.3633 | 0.2511 | 0.441 |
| $a+b\sqrt{y}/z+c/\sqrt{x}z$ | 178.48 | 126.28 | 0.612 | 0.0970 | 0.0686 | 0.5353 | 0.3121 | 0.2004 | 0.587 |
| $a+b\sqrt{y}/z+c/\sqrt{x}z^2$ | 198.27 | 138.02 | 0.522 | 0.1102 | 0.0810 | 0.4004 | 0.3593 | 0.2486 | 0.453 |
| $a+b\sqrt{y}/z+c/\sqrt{x}\sqrt{z}$ | 177.22 | 126.89 | 0.618 | 0.0934 | 0.0649 | 0.5695 | 0.3042 | 0.1986 | 0.608 |
| $a+b\sqrt{y}/z+cz/\sqrt{x}$ | 229.41 | 161.40 | 0.360 | 0.1214 | 0.0904 | 0.2726 | 0.4184 | 0.3065 | 0.258 |
| $a+b\sqrt{y}/z+cz^2/\sqrt{x}$ | 175.17 | 133.52 | 0.627 | 0.0955 | 0.0684 | 0.5501 | 0.3507 | 0.2604 | 0.479 |
| $a+b\sqrt{y}/z+c\sqrt{z}/\sqrt{x}$ | 207.31 | 145.07 | 0.477 | 0.1055 | 0.0751 | 0.4500 | 0.3566 | 0.2437 | 0.461 |
| $a+b\sqrt{y}/z^2+cx/z$ | 228.32 | 171.34 | 0.366 | 0.1241 | 0.0985 | 0.2395 | 0.3991 | 0.3077 | 0.325 |

(continued on next page)

**Table 4 – continued from previous page**

| Functional form | $T_{eff}$ (K) | | | Radius ($R_\odot$) | | | log (L/$L_\odot$) | | |
|---|---|---|---|---|---|---|---|---|---|
| | RMSE | MAD | $R^2_{ap}$ | RMSE | MAD | $R^2_{ap}$ | RMSE | MAD | $R^2_{ap}$ |
| $a+b\sqrt{y}/z^2+cx/z^2$ | 193.18 | 140.61 | 0.546 | 0.1110 | 0.0881 | 0.3920 | 0.3402 | 0.2556 | 0.509 |
| $a+b\sqrt{y}/z^2+cx/\sqrt{z}$ | 200.10 | 151.91 | 0.513 | 0.1110 | 0.0870 | 0.3913 | 0.3465 | 0.2523 | 0.491 |
| $a+b\sqrt{y}/z^2+cxz$ | 127.44 | 95.53 | 0.802 | 0.0732 | 0.0526 | 0.7352 | 0.2708 | 0.2083 | 0.689 |
| $a+b\sqrt{y}/z^2+cxz^2$ | 149.17 | 111.66 | 0.729 | 0.0844 | 0.0657 | 0.6480 | 0.3138 | 0.2440 | 0.583 |
| $a+b\sqrt{y}/z^2+cx\sqrt{z}$ | 116.84 | 91.32 | 0.834 | 0.0692 | 0.0443 | 0.7638 | 0.2409 | 0.1616 | 0.754 |
| $a+b\sqrt{y}/z^2+cx^2/z$ | 194.85 | 144.42 | 0.538 | 0.1121 | 0.0893 | 0.3796 | 0.3464 | 0.2636 | 0.492 |
| $a+b\sqrt{y}/z^2+cx^2/z^2$ | 190.31 | 139.70 | 0.559 | 0.1119 | 0.0899 | 0.3816 | 0.3402 | 0.2610 | 0.510 |
| $a+b\sqrt{y}/z^2+cx^2/\sqrt{z}$ | 157.26 | 120.60 | 0.699 | 0.0949 | 0.0719 | 0.5556 | 0.2903 | 0.2091 | 0.643 |
| $a+b\sqrt{y}/z^2+cx^2z$ | 134.18 | 102.08 | 0.781 | 0.0795 | 0.0610 | 0.6878 | 0.2919 | 0.2318 | 0.639 |
| $a+b\sqrt{y}/z^2+cx^2z^2$ | 152.81 | 116.07 | 0.716 | 0.0886 | 0.0708 | 0.6125 | 0.3253 | 0.2553 | 0.552 |
| $a+b\sqrt{y}/z^2+cx^2\sqrt{z}$ | 122.23 | 95.52 | 0.818 | 0.0751 | 0.0553 | 0.7217 | 0.2674 | 0.2030 | 0.697 |
| $a+b\sqrt{y}/z^2+c\sqrt{x}/z$ | 248.13 | 179.87 | 0.251 | 0.1309 | 0.1017 | 0.1537 | 0.4427 | 0.3356 | 0.169 |
| $a+b\sqrt{y}/z^2+c\sqrt{x}/z^2$ | 198.42 | 139.88 | 0.521 | 0.1082 | 0.0801 | 0.4216 | 0.3384 | 0.2291 | 0.515 |
| $a+b\sqrt{y}/z^2+c\sqrt{x}/\sqrt{z}$ | 235.92 | 174.80 | 0.323 | 0.1255 | 0.1001 | 0.2219 | 0.4102 | 0.3157 | 0.287 |
| $a+b\sqrt{y}/z^2+c\sqrt{x}z$ | 129.20 | 99.78 | 0.797 | 0.0719 | 0.0492 | 0.7447 | 0.2667 | 0.1991 | 0.699 |
| $a+b\sqrt{y}/z^2+c\sqrt{x}z^2$ | 149.44 | 114.05 | 0.728 | 0.0831 | 0.0635 | 0.6586 | 0.3104 | 0.2388 | 0.592 |
| $a+b\sqrt{y}/z^2+c\sqrt{x}\sqrt{z}$ | 122.11 | 92.40 | 0.819 | 0.0686 | 0.0407 | 0.7678 | 0.2378 | 0.1520 | 0.760 |
| $a+b\sqrt{y}/z^2+c/xz$ | 217.72 | 161.85 | 0.423 | 0.1117 | 0.0851 | 0.3840 | 0.3656 | 0.2672 | 0.434 |
| $a+b\sqrt{y}/z^2+c/xz^2$ | 215.89 | 158.06 | 0.433 | 0.1140 | 0.0872 | 0.3579 | 0.3685 | 0.2619 | 0.425 |
| $a+b\sqrt{y}/z^2+c/x\sqrt{z}$ | 221.02 | 163.85 | 0.406 | 0.1123 | 0.0866 | 0.3776 | 0.3707 | 0.2724 | 0.418 |
| $a+b\sqrt{y}/z^2+cz/x$ | 239.05 | 169.84 | 0.305 | 0.1219 | 0.0945 | 0.2667 | 0.4092 | 0.2971 | 0.290 |
| $a+b\sqrt{y}/z^2+cz^2/x$ | 243.97 | 174.48 | 0.276 | 0.1305 | 0.0997 | 0.1592 | 0.4447 | 0.3327 | 0.162 |
| $a+b\sqrt{y}/z^2+c\sqrt{z}/x$ | 231.38 | 168.20 | 0.349 | 0.1170 | 0.0907 | 0.3237 | 0.3915 | 0.2872 | 0.350 |
| $a+b\sqrt{y}/z^2+c/x^2z$ | 232.91 | 168.07 | 0.340 | 0.1175 | 0.0909 | 0.3183 | 0.3945 | 0.2883 | 0.341 |
| $a+b\sqrt{y}/z^2+c/x^2z^2$ | 229.09 | 167.51 | 0.361 | 0.1162 | 0.0897 | 0.3330 | 0.3871 | 0.2841 | 0.365 |
| $a+b\sqrt{y}/z^2+c/x^2\sqrt{z}$ | 234.31 | 168.11 | 0.332 | 0.1181 | 0.0912 | 0.3116 | 0.3974 | 0.2895 | 0.331 |
| $a+b\sqrt{y}/z^2+cz/x^2$ | 237.21 | 168.04 | 0.315 | 0.1195 | 0.0919 | 0.2947 | 0.4041 | 0.2917 | 0.308 |
| $a+b\sqrt{y}/z^2+cz^2/x^2$ | 239.10 | 168.10 | 0.304 | 0.1208 | 0.0925 | 0.2800 | 0.4087 | 0.2933 | 0.292 |
| $a+b\sqrt{y}/z^2+c\sqrt{z}/x^2$ | 236.37 | 168.07 | 0.320 | 0.1191 | 0.0917 | 0.3001 | 0.4021 | 0.2911 | 0.315 |
| $a+b\sqrt{y}/z^2+c/\sqrt{x}z$ | 196.21 | 143.19 | 0.532 | 0.1040 | 0.0791 | 0.4662 | 0.3303 | 0.2346 | 0.538 |
| $a+b\sqrt{y}/z^2+c/\sqrt{x}z^2$ | 211.38 | 151.36 | 0.456 | 0.1153 | 0.0912 | 0.3432 | 0.3683 | 0.2742 | 0.425 |
| $a+b\sqrt{y}/z^2+c/\sqrt{x}\sqrt{z}$ | 199.07 | 147.12 | 0.518 | 0.1031 | 0.0779 | 0.4755 | 0.3317 | 0.2336 | 0.534 |
| $a+b\sqrt{y}/z^2+cz/\sqrt{x}$ | 239.62 | 169.17 | 0.301 | 0.1287 | 0.0960 | 0.1822 | 0.4416 | 0.3278 | 0.174 |
| $a+b\sqrt{y}/z^2+cz^2/\sqrt{x}$ | 172.29 | 131.88 | 0.639 | 0.0952 | 0.0680 | 0.5525 | 0.3484 | 0.2563 | 0.486 |
| $a+b\sqrt{y}/z^2+c\sqrt{z}/\sqrt{x}$ | 239.06 | 172.13 | 0.305 | 0.1232 | 0.0968 | 0.2501 | 0.4106 | 0.3041 | 0.286 |
| $a+b\sqrt{y}/\sqrt{z}+cx/z$ | 228.88 | 179.00 | 0.363 | 0.1156 | 0.0949 | 0.3400 | 0.3905 | 0.3184 | 0.354 |
| $a+b\sqrt{y}/\sqrt{z}+cx/z^2$ | 269.26 | 192.12 | 0.118 | 0.1363 | 0.1044 | 0.0828 | 0.4754 | 0.3578 | 0.042 |
| $a+b\sqrt{y}/\sqrt{z}+cx/\sqrt{z}$ | 146.19 | 117.83 | 0.740 | 0.0838 | 0.0638 | 0.6531 | 0.2570 | 0.1755 | 0.720 |
| $a+b\sqrt{y}/\sqrt{z}+cxz$ | 127.57 | 96.16 | 0.802 | 0.0726 | 0.0508 | 0.7401 | 0.2647 | 0.1974 | 0.703 |
| $a+b\sqrt{y}/\sqrt{z}+cxz^2$ | 156.54 | 117.54 | 0.702 | 0.0850 | 0.0656 | 0.6436 | 0.3164 | 0.2493 | 0.576 |
| $a+b\sqrt{y}/\sqrt{z}+cx\sqrt{z}$ | 116.89 | 90.83 | 0.834 | 0.0696 | 0.0444 | 0.7609 | 0.2404 | 0.1608 | 0.755 |
| $a+b\sqrt{y}/\sqrt{z}+cx^2/z$ | 159.47 | 124.69 | 0.691 | 0.0939 | 0.0726 | 0.5648 | 0.2932 | 0.2211 | 0.636 |
| $a+b\sqrt{y}/\sqrt{z}+cx^2/z^2$ | 261.28 | 184.32 | 0.169 | 0.1316 | 0.0984 | 0.1453 | 0.4587 | 0.3357 | 0.108 |
| $a+b\sqrt{y}/\sqrt{z}+cx^2/\sqrt{z}$ | 130.37 | 103.52 | 0.793 | 0.0823 | 0.0589 | 0.6654 | 0.2585 | 0.1829 | 0.717 |
| $a+b\sqrt{y}/\sqrt{z}+cx^2z$ | 138.04 | 105.56 | 0.768 | 0.0795 | 0.0605 | 0.6877 | 0.2912 | 0.2294 | 0.641 |
| $a+b\sqrt{y}/\sqrt{z}+cx^2z^2$ | 164.20 | 126.60 | 0.672 | 0.0906 | 0.0721 | 0.5948 | 0.3345 | 0.2642 | 0.526 |
| $a+b\sqrt{y}/\sqrt{z}+cx^2\sqrt{z}$ | 124.00 | 95.55 | 0.813 | 0.0751 | 0.0552 | 0.7217 | 0.2663 | 0.2002 | 0.699 |
| $a+b\sqrt{y}/\sqrt{z}+c\sqrt{x}/z$ | 254.41 | 184.47 | 0.213 | 0.1333 | 0.1001 | 0.1223 | 0.4607 | 0.3412 | 0.101 |
| $a+b\sqrt{y}/\sqrt{z}+c\sqrt{x}/z^2$ | 259.32 | 186.33 | 0.182 | 0.1345 | 0.1022 | 0.1073 | 0.4627 | 0.3495 | 0.093 |
| $a+b\sqrt{y}/\sqrt{z}+c\sqrt{x}/\sqrt{z}$ | 212.68 | 160.39 | 0.450 | 0.1046 | 0.0835 | 0.4602 | 0.3476 | 0.2643 | 0.488 |
| $a+b\sqrt{y}/\sqrt{z}+c\sqrt{x}z$ | 127.64 | 98.45 | 0.802 | 0.0710 | 0.0465 | 0.7511 | 0.2578 | 0.1839 | 0.718 |
| $a+b\sqrt{y}/\sqrt{z}+c\sqrt{x}z^2$ | 154.67 | 118.70 | 0.709 | 0.0828 | 0.0628 | 0.6611 | 0.3094 | 0.2418 | 0.595 |
| $a+b\sqrt{y}/\sqrt{z}+c\sqrt{x}\sqrt{z}$ | 121.98 | 93.10 | 0.819 | 0.0696 | 0.0419 | 0.7608 | 0.2385 | 0.1480 | 0.759 |
| $a+b\sqrt{y}/\sqrt{z}+c/xz$ | 197.43 | 148.24 | 0.526 | 0.0964 | 0.0703 | 0.5409 | 0.3269 | 0.2387 | 0.547 |
| $a+b\sqrt{y}/\sqrt{z}+c/xz^2$ | 191.42 | 138.14 | 0.554 | 0.1003 | 0.0708 | 0.5028 | 0.3303 | 0.2250 | 0.538 |
| $a+b\sqrt{y}/\sqrt{z}+c/x\sqrt{z}$ | 205.59 | 152.66 | 0.486 | 0.0979 | 0.0735 | 0.5271 | 0.3374 | 0.2494 | 0.518 |
| $a+b\sqrt{y}/\sqrt{z}+cz/x$ | 240.83 | 166.25 | 0.294 | 0.1134 | 0.0848 | 0.3646 | 0.3996 | 0.2902 | 0.323 |
| $a+b\sqrt{y}/\sqrt{z}+cz^2/x$ | 268.67 | 190.94 | 0.122 | 0.1362 | 0.1048 | 0.0845 | 0.4748 | 0.3591 | 0.045 |
| $a+b\sqrt{y}/\sqrt{z}+c\sqrt{z}/x$ | 226.69 | 161.38 | 0.375 | 0.1060 | 0.0806 | 0.4453 | 0.3729 | 0.2744 | 0.411 |
| $a+b\sqrt{y}/\sqrt{z}+c/x^2z$ | 230.33 | 162.72 | 0.355 | 0.1077 | 0.0816 | 0.4273 | 0.3797 | 0.2796 | 0.389 |
| $a+b\sqrt{y}/\sqrt{z}+c/x^2z^2$ | 219.47 | 160.03 | 0.414 | 0.1035 | 0.0784 | 0.4715 | 0.3610 | 0.2698 | 0.448 |
| $a+b\sqrt{y}/\sqrt{z}+c/x^2\sqrt{z}$ | 234.19 | 163.39 | 0.333 | 0.1094 | 0.0825 | 0.4088 | 0.3868 | 0.2825 | 0.366 |
| $a+b\sqrt{y}/\sqrt{z}+cz/x^2$ | 241.62 | 164.42 | 0.290 | 0.1131 | 0.0842 | 0.3683 | 0.4012 | 0.2876 | 0.318 |
| $a+b\sqrt{y}/\sqrt{z}+cz^2/x^2$ | 245.36 | 165.09 | 0.268 | 0.1152 | 0.0851 | 0.3443 | 0.4088 | 0.2909 | 0.292 |
| $a+b\sqrt{y}/\sqrt{z}+c\sqrt{z}/x^2$ | 239.62 | 164.18 | 0.301 | 0.1121 | 0.0838 | 0.3799 | 0.3973 | 0.2863 | 0.331 |
| $a+b\sqrt{y}/\sqrt{z}+c/\sqrt{x}z$ | 175.94 | 126.39 | 0.623 | 0.0941 | 0.0656 | 0.5629 | 0.3053 | 0.1972 | 0.605 |
| $a+b\sqrt{y}/\sqrt{z}+c/\sqrt{x}z^2$ | 199.39 | 139.62 | 0.516 | 0.1103 | 0.0809 | 0.3995 | 0.3595 | 0.2513 | 0.452 |
| $a+b\sqrt{y}/\sqrt{z}+c/\sqrt{x}\sqrt{z}$ | 176.81 | 132.37 | 0.620 | 0.0897 | 0.0625 | 0.6028 | 0.2972 | 0.2041 | 0.626 |
| $a+b\sqrt{y}/\sqrt{z}+cz/\sqrt{x}$ | 259.54 | 180.88 | 0.180 | 0.1351 | 0.1014 | 0.0994 | 0.4712 | 0.3453 | 0.059 |
| $a+b\sqrt{y}/\sqrt{z}+cz^2/\sqrt{x}$ | 168.51 | 141.89 | 0.655 | 0.0916 | 0.0687 | 0.5861 | 0.3355 | 0.2659 | 0.523 |
| $a+b\sqrt{y}/\sqrt{z}+c\sqrt{z}/\sqrt{x}$ | 235.39 | 166.99 | 0.326 | 0.1115 | 0.0841 | 0.3867 | 0.3889 | 0.2874 | 0.359 |
| $a+b\sqrt{y}z+cx/z$ | 127.62 | 103.55 | 0.802 | 0.0724 | 0.0463 | 0.7415 | 0.2581 | 0.1834 | 0.718 |
| $a+b\sqrt{y}z+cx/z^2$ | 133.42 | 105.63 | 0.783 | 0.0747 | 0.0514 | 0.7247 | 0.2752 | 0.2058 | 0.679 |
| $a+b\sqrt{y}z+cx/\sqrt{z}$ | 120.92 | 92.68 | 0.822 | 0.0706 | 0.0437 | 0.7536 | 0.2422 | 0.1540 | 0.752 |
| $a+b\sqrt{y}z+cxz$ | 128.19 | 95.46 | 0.800 | 0.0730 | 0.0533 | 0.7372 | 0.2687 | 0.2075 | 0.694 |
| $a+b\sqrt{y}z+cxz^2$ | 132.82 | 106.91 | 0.785 | 0.0759 | 0.0495 | 0.7154 | 0.2741 | 0.1887 | 0.682 |
| $a+b\sqrt{y}z+cx\sqrt{z}$ | 117.12 | 90.58 | 0.833 | 0.0696 | 0.0444 | 0.7609 | 0.2374 | 0.1580 | 0.761 |
| $a+b\sqrt{y}z+cx^2/z$ | 117.46 | 90.65 | 0.832 | 0.0706 | 0.0444 | 0.7538 | 0.2419 | 0.1614 | 0.752 |
| $a+b\sqrt{y}z+cx^2/z^2$ | 129.89 | 105.74 | 0.795 | 0.0734 | 0.0495 | 0.7341 | 0.2665 | 0.2013 | 0.699 |
| $a+b\sqrt{y}z+cx^2/\sqrt{z}$ | 113.40 | 87.22 | 0.844 | 0.0705 | 0.0456 | 0.7547 | 0.2382 | 0.1535 | 0.760 |
| $a+b\sqrt{y}z+cx^2z$ | 132.47 | 100.84 | 0.786 | 0.0762 | 0.0547 | 0.7132 | 0.2814 | 0.2153 | 0.664 |
| $a+b\sqrt{y}z+cx^2z^2$ | 134.10 | 107.38 | 0.781 | 0.0760 | 0.0501 | 0.7151 | 0.2760 | 0.1986 | 0.677 |
| $a+b\sqrt{y}z+cx^2\sqrt{z}$ | 122.85 | 92.75 | 0.816 | 0.0738 | 0.0523 | 0.7313 | 0.2666 | 0.2024 | 0.699 |
| $a+b\sqrt{y}z+c\sqrt{x}/z$ | 133.22 | 105.94 | 0.784 | 0.0743 | 0.0505 | 0.7275 | 0.2726 | 0.2007 | 0.685 |
| $a+b\sqrt{y}z+c\sqrt{x}/z^2$ | 134.40 | 107.00 | 0.780 | 0.0755 | 0.0531 | 0.7183 | 0.2799 | 0.2123 | 0.668 |
| $a+b\sqrt{y}z+c\sqrt{x}/\sqrt{z}$ | 128.56 | 102.47 | 0.799 | 0.0722 | 0.0452 | 0.7429 | 0.2565 | 0.1774 | 0.721 |
| $a+b\sqrt{y}z+c\sqrt{x}z$ | 128.56 | 99.00 | 0.799 | 0.0696 | 0.0502 | 0.7610 | 0.2534 | 0.1880 | 0.728 |
| $a+b\sqrt{y}z+c\sqrt{x}z^2$ | 131.12 | 105.48 | 0.791 | 0.0759 | 0.0493 | 0.7157 | 0.2726 | 0.1812 | 0.685 |
| $a+b\sqrt{y}z+c\sqrt{x}\sqrt{z}$ | 121.58 | 92.66 | 0.820 | 0.0696 | 0.0413 | 0.7608 | 0.2365 | 0.1451 | 0.763 |
| $a+b\sqrt{y}z+c/xz$ | 131.62 | 105.25 | 0.789 | 0.0727 | 0.0449 | 0.7388 | 0.2589 | 0.1710 | 0.716 |
| $a+b\sqrt{y}z+c/xz^2$ | 127.81 | 101.03 | 0.801 | 0.0731 | 0.0449 | 0.7359 | 0.2557 | 0.1592 | 0.723 |
| $a+b\sqrt{y}z+c/x\sqrt{z}$ | 132.93 | 106.57 | 0.785 | 0.0729 | 0.0460 | 0.7375 | 0.2622 | 0.1772 | 0.709 |

(continued on next page)

**Table 4 – continued from previous page**

| Functional form | $T_{eff}$ (K) | | | Radius ($R_{\odot}$) | | | log (L/$L_{\odot}$) | | |
|---|---|---|---|---|---|---|---|---|---|
| | RMSE | MAD | $R^2_{ap}$ | RMSE | MAD | $R^2_{ap}$ | RMSE | MAD | $R^2_{ap}$ |
| $a+b\sqrt{y}z+cz/x$ | 134.28 | 107.32 | 0.781 | 0.0738 | 0.0481 | 0.7312 | 0.2698 | 0.1897 | 0.691 |
| $a+b\sqrt{y}z+cz^2/x$ | 134.17 | 107.25 | 0.781 | 0.0740 | 0.0480 | 0.7296 | 0.2702 | 0.1901 | 0.691 |
| $a+b\sqrt{y}z+c\sqrt{z}/x$ | 134.12 | 107.36 | 0.781 | 0.0735 | 0.0476 | 0.7331 | 0.2680 | 0.1870 | 0.696 |
| $a+b\sqrt{y}z+c/x^2z$ | 134.30 | 107.33 | 0.781 | 0.0738 | 0.0477 | 0.7313 | 0.2696 | 0.1880 | 0.692 |
| $a+b\sqrt{y}z+c/x^2z^2$ | 133.79 | 107.32 | 0.782 | 0.0734 | 0.0469 | 0.7339 | 0.2662 | 0.1831 | 0.700 |
| $a+b\sqrt{y}z+c/x^2\sqrt{z}$ | 134.38 | 107.18 | 0.780 | 0.0739 | 0.0480 | 0.7303 | 0.2707 | 0.1894 | 0.689 |
| $a+b\sqrt{y}z+cz/x^2$ | 134.37 | 106.71 | 0.780 | 0.0742 | 0.0484 | 0.7281 | 0.2729 | 0.1917 | 0.684 |
| $a+b\sqrt{y}z+cz^2/x^2$ | 134.34 | 106.54 | 0.780 | 0.0743 | 0.0486 | 0.7274 | 0.2735 | 0.1924 | 0.683 |
| $a+b\sqrt{y}z+c\sqrt{z}/x^2$ | 134.39 | 106.85 | 0.780 | 0.0741 | 0.0483 | 0.7287 | 0.2724 | 0.1912 | 0.686 |
| $a+b\sqrt{y}z+c/\sqrt{x}z$ | 126.17 | 99.26 | 0.806 | 0.0728 | 0.0440 | 0.7385 | 0.2519 | 0.1515 | 0.731 |
| $a+b\sqrt{y}z+c/\sqrt{x}z^2$ | 125.05 | 97.31 | 0.810 | 0.0751 | 0.0479 | 0.7217 | 0.2640 | 0.1685 | 0.705 |
| $a+b\sqrt{y}z+c/\sqrt{x}\sqrt{z}$ | 129.15 | 102.24 | 0.797 | 0.0722 | 0.0435 | 0.7429 | 0.2528 | 0.1602 | 0.729 |
| $a+b\sqrt{y}z+cz/\sqrt{x}$ | 133.78 | 107.11 | 0.782 | 0.0739 | 0.0484 | 0.7305 | 0.2691 | 0.1912 | 0.693 |
| $a+b\sqrt{y}z+cz^2/\sqrt{x}$ | 131.34 | 103.69 | 0.790 | 0.0744 | 0.0474 | 0.7269 | 0.2667 | 0.1793 | 0.699 |
| $a+b\sqrt{y}z+c\sqrt{z}/\sqrt{x}$ | 133.44 | 106.89 | 0.783 | 0.0732 | 0.0475 | 0.7353 | 0.2654 | 0.1858 | 0.701 |
| $a+b\sqrt{y}z^2+cx/z$ | 153.20 | 122.50 | 0.714 | 0.0821 | 0.0637 | 0.6671 | 0.3019 | 0.2386 | 0.614 |
| $a+b\sqrt{y}z^2+cx/z^2$ | 158.00 | 121.94 | 0.696 | 0.0854 | 0.0648 | 0.6401 | 0.3197 | 0.2468 | 0.567 |
| $a+b\sqrt{y}z^2+cx/\sqrt{z}$ | 133.60 | 104.59 | 0.783 | 0.0747 | 0.0525 | 0.7247 | 0.2610 | 0.1926 | 0.711 |
| $a+b\sqrt{y}z^2+cxz$ | 122.17 | 97.14 | 0.818 | 0.0710 | 0.0477 | 0.7514 | 0.2499 | 0.1728 | 0.735 |
| $a+b\sqrt{y}z^2+cxz^2$ | 156.81 | 116.72 | 0.701 | 0.0852 | 0.0660 | 0.6413 | 0.3190 | 0.2502 | 0.569 |
| $a+b\sqrt{y}z^2+cx\sqrt{z}$ | 117.06 | 89.99 | 0.833 | 0.0695 | 0.0449 | 0.7613 | 0.2386 | 0.1520 | 0.759 |
| $a+b\sqrt{y}z^2+cx^2/z$ | 133.46 | 103.89 | 0.783 | 0.0762 | 0.0563 | 0.7131 | 0.2677 | 0.2020 | 0.696 |
| $a+b\sqrt{y}z^2+cx^2/z^2$ | 157.04 | 124.28 | 0.700 | 0.0843 | 0.0650 | 0.6494 | 0.3135 | 0.2495 | 0.583 |
| $a+b\sqrt{y}z^2+cx^2/\sqrt{z}$ | 116.78 | 91.13 | 0.834 | 0.0719 | 0.0513 | 0.7447 | 0.2445 | 0.1744 | 0.747 |
| $a+b\sqrt{y}z^2+cx^2z$ | 137.39 | 104.05 | 0.770 | 0.0797 | 0.0612 | 0.6864 | 0.2919 | 0.2308 | 0.639 |
| $a+b\sqrt{y}z^2+cx^2z^2$ | 158.16 | 121.66 | 0.696 | 0.0852 | 0.0637 | 0.6417 | 0.3190 | 0.2480 | 0.569 |
| $a+b\sqrt{y}z^2+cx^2\sqrt{z}$ | 124.06 | 95.95 | 0.813 | 0.0749 | 0.0552 | 0.7231 | 0.2665 | 0.1996 | 0.699 |
| $a+b\sqrt{y}z^2+c\sqrt{x}/z$ | 158.16 | 121.69 | 0.696 | 0.0852 | 0.0647 | 0.6416 | 0.3189 | 0.2454 | 0.569 |
| $a+b\sqrt{y}z^2+c\sqrt{x}/z^2$ | 155.03 | 121.28 | 0.708 | 0.0854 | 0.0651 | 0.6399 | 0.3191 | 0.2469 | 0.568 |
| $a+b\sqrt{y}z^2+c\sqrt{x}/\sqrt{z}$ | 151.31 | 121.40 | 0.721 | 0.0804 | 0.0610 | 0.6806 | 0.2942 | 0.2238 | 0.633 |
| $a+b\sqrt{y}z^2+c\sqrt{x}z$ | 125.40 | 99.81 | 0.809 | 0.0702 | 0.0431 | 0.7568 | 0.2470 | 0.1564 | 0.742 |
| $a+b\sqrt{y}z^2+c\sqrt{x}z^2$ | 152.83 | 111.64 | 0.716 | 0.0804 | 0.0642 | 0.6807 | 0.3016 | 0.2407 | 0.615 |
| $a+b\sqrt{y}z^2+c\sqrt{x}\sqrt{z}$ | 121.26 | 92.18 | 0.821 | 0.0694 | 0.0414 | 0.7623 | 0.2387 | 0.1415 | 0.759 |
| $a+b\sqrt{y}z^2+c/xz$ | 145.63 | 112.69 | 0.742 | 0.0759 | 0.0526 | 0.7155 | 0.2742 | 0.1891 | 0.681 |
| $a+b\sqrt{y}z^2+c/xz^2$ | 136.11 | 102.68 | 0.775 | 0.0753 | 0.0502 | 0.7203 | 0.2650 | 0.1749 | 0.702 |
| $a+b\sqrt{y}z^2+c/x\sqrt{z}$ | 149.69 | 116.53 | 0.727 | 0.0770 | 0.0544 | 0.7075 | 0.2815 | 0.1969 | 0.664 |
| $a+b\sqrt{y}z^2+cz/x$ | 156.14 | 120.54 | 0.703 | 0.0803 | 0.0582 | 0.6819 | 0.2995 | 0.2159 | 0.620 |
| $a+b\sqrt{y}z^2+cz^2/x$ | 156.96 | 120.04 | 0.700 | 0.0814 | 0.0596 | 0.6725 | 0.3047 | 0.2216 | 0.607 |
| $a+b\sqrt{y}z^2+c\sqrt{z}/x$ | 154.83 | 120.19 | 0.708 | 0.0793 | 0.0572 | 0.6897 | 0.2947 | 0.2111 | 0.632 |
| $a+b\sqrt{y}z^2+c/x^2z$ | 155.52 | 120.37 | 0.706 | 0.0796 | 0.0574 | 0.6870 | 0.2966 | 0.2122 | 0.627 |
| $a+b\sqrt{y}z^2+c/x^2z^2$ | 153.13 | 119.45 | 0.715 | 0.0786 | 0.0562 | 0.6953 | 0.2902 | 0.2055 | 0.643 |
| $a+b\sqrt{y}z^2+c/x^2\sqrt{z}$ | 156.20 | 120.45 | 0.703 | 0.0800 | 0.0577 | 0.6838 | 0.2989 | 0.2142 | 0.621 |
| $a+b\sqrt{y}z^2+cz/x^2$ | 157.23 | 120.24 | 0.699 | 0.0808 | 0.0584 | 0.6774 | 0.3031 | 0.2175 | 0.611 |
| $a+b\sqrt{y}z^2+cz^2/x^2$ | 157.49 | 120.06 | 0.698 | 0.0811 | 0.0586 | 0.6751 | 0.3045 | 0.2186 | 0.607 |
| $a+b\sqrt{y}z^2+c\sqrt{z}/x^2$ | 157.00 | 120.34 | 0.700 | 0.0806 | 0.0582 | 0.6791 | 0.3020 | 0.2167 | 0.614 |
| $a+b\sqrt{y}z^2+c/\sqrt{x}z$ | 129.64 | 98.33 | 0.796 | 0.0732 | 0.0475 | 0.7351 | 0.2541 | 0.1625 | 0.726 |
| $a+b\sqrt{y}z^2+c/\sqrt{x}z^2$ | 127.31 | 95.32 | 0.803 | 0.0773 | 0.0529 | 0.7050 | 0.2706 | 0.1788 | 0.690 |
| $a+b\sqrt{y}z^2+c/\sqrt{x}\sqrt{z}$ | 137.62 | 104.29 | 0.770 | 0.0735 | 0.0487 | 0.7335 | 0.2597 | 0.1741 | 0.714 |
| $a+b\sqrt{y}z^2+cz/\sqrt{x}$ | 157.46 | 120.65 | 0.698 | 0.0826 | 0.0616 | 0.6631 | 0.3087 | 0.2279 | 0.596 |
| $a+b\sqrt{y}z^2+cz^2/\sqrt{x}$ | 157.51 | 119.11 | 0.698 | 0.0842 | 0.0648 | 0.6499 | 0.3147 | 0.2426 | 0.580 |
| $a+b\sqrt{y}z^2+c\sqrt{z}/\sqrt{x}$ | 154.30 | 120.58 | 0.710 | 0.0796 | 0.0576 | 0.6870 | 0.2949 | 0.2135 | 0.631 |
| $a+b\sqrt{y}\sqrt{z}+cx/z$ | 124.16 | 94.55 | 0.812 | 0.0735 | 0.0432 | 0.7332 | 0.2498 | 0.1497 | 0.736 |
| $a+b\sqrt{y}\sqrt{z}+cx/z^2$ | 124.82 | 97.15 | 0.810 | 0.0731 | 0.0428 | 0.7362 | 0.2544 | 0.1634 | 0.726 |
| $a+b\sqrt{y}\sqrt{z}+cx/\sqrt{z}$ | 123.42 | 92.19 | 0.815 | 0.0736 | 0.0441 | 0.7324 | 0.2462 | 0.1420 | 0.743 |
| $a+b\sqrt{y}\sqrt{z}+cxz$ | 123.67 | 97.03 | 0.814 | 0.0727 | 0.0488 | 0.7392 | 0.2616 | 0.1832 | 0.710 |
| $a+b\sqrt{y}\sqrt{z}+cxz^2$ | 125.45 | 99.59 | 0.809 | 0.0744 | 0.0475 | 0.7266 | 0.2623 | 0.1669 | 0.709 |
| $a+b\sqrt{y}\sqrt{z}+cx\sqrt{z}$ | 117.11 | 90.76 | 0.833 | 0.0693 | 0.0460 | 0.7632 | 0.2392 | 0.1668 | 0.758 |
| $a+b\sqrt{y}\sqrt{z}+cx^2/z$ | 120.47 | 88.62 | 0.823 | 0.0732 | 0.0439 | 0.7355 | 0.2432 | 0.1423 | 0.749 |
| $a+b\sqrt{y}\sqrt{z}+cx^2/z^2$ | 122.88 | 93.58 | 0.816 | 0.0727 | 0.0424 | 0.7387 | 0.2492 | 0.1535 | 0.737 |
| $a+b\sqrt{y}\sqrt{z}+cx^2/\sqrt{z}$ | 118.89 | 90.42 | 0.828 | 0.0733 | 0.0450 | 0.7351 | 0.2425 | 0.1505 | 0.751 |
| $a+b\sqrt{y}\sqrt{z}+cx^2z$ | 123.31 | 95.81 | 0.815 | 0.0739 | 0.0484 | 0.7300 | 0.2626 | 0.1775 | 0.708 |
| $a+b\sqrt{y}\sqrt{z}+cx^2z^2$ | 124.85 | 98.33 | 0.810 | 0.0746 | 0.0471 | 0.7254 | 0.2623 | 0.1676 | 0.709 |
| $a+b\sqrt{y}\sqrt{z}+cx^2\sqrt{z}$ | 119.43 | 92.16 | 0.826 | 0.0729 | 0.0492 | 0.7373 | 0.2583 | 0.1832 | 0.717 |
| $a+b\sqrt{y}\sqrt{z}+c\sqrt{x}/z$ | 125.67 | 98.42 | 0.808 | 0.0738 | 0.0432 | 0.7313 | 0.2556 | 0.1626 | 0.723 |
| $a+b\sqrt{y}\sqrt{z}+c\sqrt{x}/z^2$ | 125.69 | 98.94 | 0.808 | 0.0733 | 0.0430 | 0.7345 | 0.2579 | 0.1709 | 0.718 |
| $a+b\sqrt{y}\sqrt{z}+c\sqrt{x}/\sqrt{z}$ | 125.43 | 97.30 | 0.809 | 0.0739 | 0.0435 | 0.7301 | 0.2521 | 0.1518 | 0.731 |
| $a+b\sqrt{y}\sqrt{z}+c\sqrt{x}z$ | 124.90 | 99.34 | 0.810 | 0.0723 | 0.0480 | 0.7420 | 0.2614 | 0.1821 | 0.710 |
| $a+b\sqrt{y}\sqrt{z}+c\sqrt{x}z^2$ | 125.75 | 99.97 | 0.808 | 0.0743 | 0.0474 | 0.7271 | 0.2623 | 0.1666 | 0.709 |
| $a+b\sqrt{y}\sqrt{z}+c\sqrt{x}\sqrt{z}$ | 121.81 | 91.89 | 0.819 | 0.0689 | 0.0449 | 0.7655 | 0.2347 | 0.1551 | 0.767 |
| $a+b\sqrt{y}\sqrt{z}+c/xz$ | 125.71 | 99.61 | 0.808 | 0.0745 | 0.0430 | 0.7261 | 0.2567 | 0.1566 | 0.721 |
| $a+b\sqrt{y}\sqrt{z}+c/xz^2$ | 126.00 | 99.20 | 0.807 | 0.0748 | 0.0439 | 0.7240 | 0.2564 | 0.1509 | 0.721 |
| $a+b\sqrt{y}\sqrt{z}+c/x\sqrt{z}$ | 125.28 | 99.16 | 0.809 | 0.0744 | 0.0428 | 0.7266 | 0.2576 | 0.1598 | 0.719 |
| $a+b\sqrt{y}\sqrt{z}+cz/x$ | 124.19 | 97.74 | 0.812 | 0.0745 | 0.0431 | 0.7259 | 0.2599 | 0.1643 | 0.714 |
| $a+b\sqrt{y}\sqrt{z}+cz^2/x$ | 124.32 | 98.55 | 0.812 | 0.0748 | 0.0438 | 0.7239 | 0.2605 | 0.1625 | 0.712 |
| $a+b\sqrt{y}\sqrt{z}+c\sqrt{z}/x$ | 124.44 | 98.01 | 0.812 | 0.0744 | 0.0430 | 0.7264 | 0.2593 | 0.1637 | 0.715 |
| $a+b\sqrt{y}\sqrt{z}+c/x^2z$ | 123.91 | 97.16 | 0.813 | 0.0745 | 0.0429 | 0.7260 | 0.2599 | 0.1643 | 0.714 |
| $a+b\sqrt{y}\sqrt{z}+c/x^2z^2$ | 124.69 | 98.34 | 0.811 | 0.0745 | 0.0428 | 0.7259 | 0.2590 | 0.1623 | 0.716 |
| $a+b\sqrt{y}\sqrt{z}+c/x^2\sqrt{z}$ | 123.62 | 96.69 | 0.814 | 0.0745 | 0.0430 | 0.7260 | 0.2602 | 0.1648 | 0.713 |
| $a+b\sqrt{y}\sqrt{z}+cz/x^2$ | 123.06 | 95.78 | 0.816 | 0.0745 | 0.0432 | 0.7258 | 0.2608 | 0.1656 | 0.712 |
| $a+b\sqrt{y}\sqrt{z}+cz^2/x^2$ | 122.90 | 95.56 | 0.816 | 0.0745 | 0.0432 | 0.7257 | 0.2610 | 0.1657 | 0.711 |
| $a+b\sqrt{y}\sqrt{z}+c\sqrt{z}/x^2$ | 123.20 | 96.01 | 0.815 | 0.0745 | 0.0431 | 0.7259 | 0.2607 | 0.1654 | 0.712 |
| $a+b\sqrt{y}\sqrt{z}+c/\sqrt{x}z$ | 125.91 | 98.70 | 0.807 | 0.0747 | 0.0438 | 0.7244 | 0.2548 | 0.1471 | 0.725 |
| $a+b\sqrt{y}\sqrt{z}+c/\sqrt{x}z^2$ | 125.47 | 97.42 | 0.808 | 0.0748 | 0.0455 | 0.7236 | 0.2603 | 0.1592 | 0.713 |
| $a+b\sqrt{y}\sqrt{z}+c/\sqrt{x}\sqrt{z}$ | 126.01 | 99.59 | 0.807 | 0.0744 | 0.0431 | 0.7268 | 0.2543 | 0.1512 | 0.726 |
| $a+b\sqrt{y}\sqrt{z}+cz/\sqrt{x}$ | 125.20 | 99.47 | 0.809 | 0.0747 | 0.0437 | 0.7242 | 0.2597 | 0.1621 | 0.714 |
| $a+b\sqrt{y}\sqrt{z}+cz^2/\sqrt{x}$ | 125.69 | 100.27 | 0.808 | 0.0748 | 0.0453 | 0.7235 | 0.2612 | 0.1608 | 0.711 |
| $a+b\sqrt{y}\sqrt{z}+c\sqrt{z}/\sqrt{x}$ | 125.34 | 99.33 | 0.809 | 0.0744 | 0.0430 | 0.7264 | 0.2582 | 0.1617 | 0.717 |
| $a+b/yz+cx/z$ | 189.50 | 130.93 | 0.563 | 0.1061 | 0.0808 | 0.4445 | 0.3386 | 0.2396 | 0.514 |
| $a+b/yz+cx/z^2$ | 196.62 | 142.40 | 0.530 | 0.1089 | 0.0847 | 0.4146 | 0.3440 | 0.2489 | 0.499 |
| $a+b/yz+cx/\sqrt{z}$ | 200.46 | 142.91 | 0.511 | 0.1099 | 0.0852 | 0.4034 | 0.3463 | 0.2496 | 0.492 |
| $a+b/yz+cxz$ | 115.33 | 86.13 | 0.838 | 0.0707 | 0.0461 | 0.7535 | 0.2434 | 0.1518 | 0.749 |
| $a+b/yz+cxz^2$ | 119.73 | 86.03 | 0.826 | 0.0743 | 0.0521 | 0.7278 | 0.2545 | 0.1672 | 0.726 |

(continued on next page)

**Table 4 – continued from previous page**

| Functional form | $T_{eff}$ (K) | | | Radius ($R_{\odot}$) | | | log (L/$L_{\odot}$) | | |
|---|---|---|---|---|---|---|---|---|---|
| | RMSE | MAD | $R^2_{ap}$ | RMSE | MAD | $R^2_{ap}$ | RMSE | MAD | $R^2_{ap}$ |
| $a+b/yz+cx\sqrt{z}$ | 115.75 | 89.39 | 0.837 | 0.0696 | 0.0442 | 0.7609 | 0.2362 | 0.1427 | 0.764 |
| $a+b/yz+cx^2/z$ | 202.63 | 145.77 | 0.500 | 0.1102 | 0.0851 | 0.4005 | 0.3461 | 0.2491 | 0.492 |
| $a+b/yz+cx^2/z^2$ | 199.01 | 144.25 | 0.518 | 0.1093 | 0.0848 | 0.4105 | 0.3454 | 0.2492 | 0.495 |
| $a+b/yz+cx^2/\sqrt{z}$ | 180.42 | 142.24 | 0.604 | 0.1008 | 0.0797 | 0.4985 | 0.3060 | 0.2316 | 0.603 |
| $a+b/yz+cx^2z$ | 113.67 | 84.89 | 0.843 | 0.0731 | 0.0516 | 0.7362 | 0.2480 | 0.1633 | 0.739 |
| $a+b/yz+cx^2z^2$ | 119.27 | 85.43 | 0.827 | 0.0764 | 0.0553 | 0.7117 | 0.2585 | 0.1768 | 0.717 |
| $a+b/yz+cx^2\sqrt{z}$ | 112.72 | 88.00 | 0.845 | 0.0726 | 0.0507 | 0.7397 | 0.2427 | 0.1550 | 0.750 |
| $a+b/yz+c\sqrt{x}/z$ | 182.01 | 123.81 | 0.597 | 0.1040 | 0.0787 | 0.4656 | 0.3319 | 0.2317 | 0.533 |
| $a+b/yz+c\sqrt{x}/z^2$ | 196.09 | 142.12 | 0.532 | 0.1090 | 0.0850 | 0.4132 | 0.3439 | 0.2496 | 0.499 |
| $a+b/yz+c\sqrt{x}/\sqrt{z}$ | 183.73 | 126.92 | 0.589 | 0.1050 | 0.0796 | 0.4557 | 0.3350 | 0.2358 | 0.525 |
| $a+b/yz+c\sqrt{x}z$ | 119.37 | 90.72 | 0.827 | 0.0707 | 0.0443 | 0.7531 | 0.2451 | 0.1474 | 0.745 |
| $a+b/yz+c\sqrt{x}z^2$ | 121.62 | 89.32 | 0.820 | 0.0738 | 0.0503 | 0.7310 | 0.2542 | 0.1643 | 0.726 |
| $a+b/yz+c\sqrt{x}\sqrt{z}$ | 121.88 | 91.31 | 0.819 | 0.0693 | 0.0417 | 0.7627 | 0.2384 | 0.1396 | 0.759 |
| $a+b/yz+c/xz$ | 196.98 | 140.48 | 0.528 | 0.1104 | 0.0850 | 0.3986 | 0.3463 | 0.2505 | 0.492 |
| $a+b/yz+c/xz^2$ | 182.61 | 128.91 | 0.594 | 0.1081 | 0.0839 | 0.4231 | 0.3380 | 0.2440 | 0.516 |
| $a+b/yz+c/x\sqrt{z}$ | 198.60 | 140.85 | 0.520 | 0.1103 | 0.0844 | 0.3992 | 0.3463 | 0.2490 | 0.492 |
| $a+b/yz+cz/x$ | 194.19 | 139.13 | 0.541 | 0.1102 | 0.0855 | 0.4008 | 0.3454 | 0.2516 | 0.495 |
| $a+b/yz+cz^2/x$ | 166.23 | 118.04 | 0.664 | 0.1022 | 0.0776 | 0.4844 | 0.3233 | 0.2260 | 0.557 |
| $a+b/yz+c\sqrt{z}/x$ | 197.79 | 140.71 | 0.524 | 0.1104 | 0.0848 | 0.3987 | 0.3463 | 0.2501 | 0.492 |
| $a+b/yz+c/x^2z$ | 197.81 | 140.72 | 0.524 | 0.1103 | 0.0846 | 0.3988 | 0.3463 | 0.2500 | 0.492 |
| $a+b/yz+c/x^2z^2$ | 195.45 | 140.33 | 0.535 | 0.1103 | 0.0853 | 0.3990 | 0.3459 | 0.2516 | 0.493 |
| $a+b/yz+c/x^2\sqrt{z}$ | 198.44 | 140.68 | 0.521 | 0.1103 | 0.0844 | 0.3992 | 0.3463 | 0.2493 | 0.492 |
| $a+b/yz+cz/x^2$ | 199.25 | 140.48 | 0.517 | 0.1102 | 0.0840 | 0.4000 | 0.3463 | 0.2483 | 0.492 |
| $a+b/yz+cz^2/x^2$ | 198.88 | 140.39 | 0.519 | 0.1103 | 0.0842 | 0.3995 | 0.3463 | 0.2489 | 0.492 |
| $a+b/yz+c\sqrt{z}/x^2$ | 199.13 | 140.54 | 0.518 | 0.1102 | 0.0840 | 0.3999 | 0.3463 | 0.2485 | 0.492 |
| $a+b/yz+c/\sqrt{x}z$ | 201.93 | 145.87 | 0.504 | 0.1051 | 0.0807 | 0.4542 | 0.3335 | 0.2405 | 0.529 |
| $a+b/yz+c/\sqrt{x}z^2$ | 203.08 | 145.34 | 0.498 | 0.1101 | 0.0832 | 0.4017 | 0.3449 | 0.2425 | 0.496 |
| $a+b/yz+c/\sqrt{x}\sqrt{z}$ | 203.06 | 145.85 | 0.498 | 0.1071 | 0.0820 | 0.4332 | 0.3384 | 0.2443 | 0.515 |
| $a+b/yz+cz/\sqrt{x}$ | 159.59 | 114.84 | 0.690 | 0.0986 | 0.0726 | 0.5202 | 0.3147 | 0.2151 | 0.580 |
| $a+b/yz+cz^2/\sqrt{x}$ | 128.03 | 93.82 | 0.801 | 0.0797 | 0.0551 | 0.6864 | 0.2687 | 0.1773 | 0.694 |
| $a+b/yz+c\sqrt{z}/\sqrt{x}$ | 188.16 | 134.88 | 0.569 | 0.1089 | 0.0848 | 0.4150 | 0.3419 | 0.2489 | 0.505 |
| $a+b/yz^2+cx/z$ | 215.40 | 156.39 | 0.436 | 0.1197 | 0.0948 | 0.2923 | 0.3858 | 0.2923 | 0.369 |
| $a+b/yz^2+cx/z^2$ | 217.61 | 159.20 | 0.424 | 0.1205 | 0.0965 | 0.2834 | 0.3862 | 0.2949 | 0.368 |
| $a+b/yz^2+cx/\sqrt{z}$ | 217.55 | 156.93 | 0.424 | 0.1195 | 0.0953 | 0.2955 | 0.3757 | 0.2856 | 0.402 |
| $a+b/yz^2+cxz$ | 114.64 | 85.61 | 0.840 | 0.0719 | 0.0487 | 0.7445 | 0.2524 | 0.1689 | 0.730 |
| $a+b/yz^2+cxz^2$ | 121.42 | 85.56 | 0.821 | 0.0777 | 0.0565 | 0.7021 | 0.2711 | 0.1872 | 0.688 |
| $a+b/yz^2+cx\sqrt{z}$ | 114.19 | 88.61 | 0.841 | 0.0696 | 0.0446 | 0.7611 | 0.2384 | 0.1486 | 0.759 |
| $a+b/yz^2+cx^2/z$ | 216.52 | 156.42 | 0.430 | 0.1197 | 0.0959 | 0.2925 | 0.3754 | 0.2882 | 0.403 |
| $a+b/yz^2+cx^2/z^2$ | 218.64 | 160.11 | 0.418 | 0.1207 | 0.0969 | 0.2806 | 0.3853 | 0.2958 | 0.371 |
| $a+b/yz^2+cx^2/\sqrt{z}$ | 177.24 | 139.74 | 0.618 | 0.1017 | 0.0797 | 0.4890 | 0.3081 | 0.2314 | 0.598 |
| $a+b/yz^2+cx^2z$ | 113.70 | 84.10 | 0.843 | 0.0754 | 0.0544 | 0.7190 | 0.2607 | 0.1803 | 0.712 |
| $a+b/yz^2+cx^2z^2$ | 121.61 | 85.52 | 0.820 | 0.0805 | 0.0605 | 0.6804 | 0.2772 | 0.1994 | 0.674 |
| $a+b/yz^2+cx^2\sqrt{z}$ | 111.23 | 87.32 | 0.849 | 0.0737 | 0.0524 | 0.7317 | 0.2504 | 0.1703 | 0.734 |
| $a+b/yz^2+c\sqrt{x}/z$ | 207.68 | 147.06 | 0.475 | 0.1170 | 0.0898 | 0.3243 | 0.3802 | 0.2783 | 0.387 |
| $a+b/yz^2+c\sqrt{x}/z^2$ | 216.84 | 158.52 | 0.428 | 0.1203 | 0.0962 | 0.2853 | 0.3861 | 0.2941 | 0.368 |
| $a+b/yz^2+c\sqrt{x}/\sqrt{z}$ | 213.81 | 155.40 | 0.444 | 0.1197 | 0.0948 | 0.2927 | 0.3856 | 0.2917 | 0.370 |
| $a+b/yz^2+c\sqrt{x}z$ | 119.14 | 90.39 | 0.827 | 0.0718 | 0.0467 | 0.7458 | 0.2536 | 0.1636 | 0.728 |
| $a+b/yz^2+c\sqrt{x}z^2$ | 123.42 | 89.15 | 0.815 | 0.0771 | 0.0544 | 0.7068 | 0.2704 | 0.1817 | 0.690 |
| $a+b/yz^2+c\sqrt{x}\sqrt{z}$ | 121.05 | 90.18 | 0.822 | 0.0691 | 0.0418 | 0.7642 | 0.2396 | 0.1428 | 0.757 |
| $a+b/yz^2+c/xz$ | 217.87 | 157.40 | 0.422 | 0.1166 | 0.0899 | 0.3292 | 0.3714 | 0.2725 | 0.416 |
| $a+b/yz^2+c/xz^2$ | 218.75 | 159.55 | 0.418 | 0.1186 | 0.0932 | 0.3058 | 0.3779 | 0.2812 | 0.395 |
| $a+b/yz^2+c/x\sqrt{z}$ | 217.71 | 157.52 | 0.423 | 0.1163 | 0.0899 | 0.3321 | 0.3708 | 0.2723 | 0.418 |
| $a+b/yz^2+cz/x$ | 218.68 | 160.98 | 0.418 | 0.1195 | 0.0949 | 0.2949 | 0.3813 | 0.2869 | 0.384 |
| $a+b/yz^2+cz^2/x$ | 199.38 | 141.91 | 0.516 | 0.1169 | 0.0904 | 0.3253 | 0.3777 | 0.2797 | 0.396 |
| $a+b/yz^2+c\sqrt{z}/x$ | 218.50 | 158.01 | 0.419 | 0.1177 | 0.0917 | 0.3157 | 0.3755 | 0.2767 | 0.403 |
| $a+b/yz^2+c/x^2z$ | 218.54 | 158.12 | 0.419 | 0.1176 | 0.0914 | 0.3174 | 0.3756 | 0.2762 | 0.402 |
| $a+b/yz^2+c/x^2z^2$ | 218.71 | 159.13 | 0.418 | 0.1182 | 0.0924 | 0.3107 | 0.3773 | 0.2793 | 0.397 |
| $a+b/yz^2+c/x^2\sqrt{z}$ | 218.47 | 157.79 | 0.419 | 0.1174 | 0.0911 | 0.3194 | 0.3752 | 0.2753 | 0.404 |
| $a+b/yz^2+cz/x^2$ | 218.40 | 157.50 | 0.420 | 0.1173 | 0.0908 | 0.3212 | 0.3749 | 0.2747 | 0.405 |
| $a+b/yz^2+cz^2/x^2$ | 218.56 | 158.25 | 0.419 | 0.1176 | 0.0915 | 0.3166 | 0.3761 | 0.2768 | 0.401 |
| $a+b/yz^2+c\sqrt{z}/x^2$ | 218.40 | 157.46 | 0.420 | 0.1172 | 0.0908 | 0.3214 | 0.3748 | 0.2745 | 0.405 |
| $a+b/yz^2+c/\sqrt{x}z$ | 203.88 | 148.14 | 0.494 | 0.1044 | 0.0790 | 0.4621 | 0.3327 | 0.2362 | 0.531 |
| $a+b/yz^2+c/\sqrt{x}z^2$ | 211.67 | 154.32 | 0.455 | 0.1120 | 0.0841 | 0.3811 | 0.3621 | 0.2552 | 0.445 |
| $a+b/yz^2+c/\sqrt{x}\sqrt{z}$ | 208.49 | 152.09 | 0.471 | 0.1080 | 0.0828 | 0.4241 | 0.3436 | 0.2490 | 0.500 |
| $a+b/yz^2+cz/\sqrt{x}$ | 191.63 | 134.67 | 0.553 | 0.1133 | 0.0843 | 0.3664 | 0.3692 | 0.2662 | 0.422 |
| $a+b/yz^2+cz^2/\sqrt{x}$ | 139.49 | 102.27 | 0.763 | 0.0866 | 0.0599 | 0.6297 | 0.2983 | 0.1969 | 0.623 |
| $a+b/yz^2+c\sqrt{z}/\sqrt{x}$ | 217.46 | 161.14 | 0.425 | 0.1206 | 0.0968 | 0.2819 | 0.3849 | 0.2935 | 0.372 |
| $a+b/y\sqrt{z}+cx/z$ | 182.24 | 124.70 | 0.596 | 0.1001 | 0.0728 | 0.5048 | 0.3222 | 0.2119 | 0.560 |
| $a+b/y\sqrt{z}+cx/z^2$ | 193.02 | 138.85 | 0.547 | 0.1050 | 0.0791 | 0.4555 | 0.3332 | 0.2344 | 0.530 |
| $a+b/y\sqrt{z}+cx/\sqrt{z}$ | 197.97 | 138.91 | 0.523 | 0.1057 | 0.0785 | 0.4482 | 0.3380 | 0.2336 | 0.516 |
| $a+b/y\sqrt{z}+cxz$ | 118.47 | 88.67 | 0.829 | 0.0702 | 0.0450 | 0.7564 | 0.2425 | 0.1504 | 0.751 |
| $a+b/y\sqrt{z}+cxz^2$ | 124.92 | 90.63 | 0.810 | 0.0736 | 0.0500 | 0.7323 | 0.2536 | 0.1634 | 0.728 |
| $a+b/y\sqrt{z}+cx\sqrt{z}$ | 116.86 | 90.34 | 0.834 | 0.0696 | 0.0441 | 0.7609 | 0.2364 | 0.1456 | 0.763 |
| $a+b/y\sqrt{z}+cx^2/z$ | 204.37 | 143.08 | 0.492 | 0.1073 | 0.0802 | 0.4310 | 0.3421 | 0.2407 | 0.504 |
| $a+b/y\sqrt{z}+cx^2/z^2$ | 197.06 | 140.91 | 0.528 | 0.1056 | 0.0794 | 0.4490 | 0.3367 | 0.2371 | 0.520 |
| $a+b/y\sqrt{z}+cx^2/\sqrt{z}$ | 186.90 | 146.94 | 0.575 | 0.1017 | 0.0818 | 0.4896 | 0.3116 | 0.2399 | 0.589 |
| $a+b/y\sqrt{z}+cx^2z$ | 118.27 | 88.12 | 0.830 | 0.0726 | 0.0501 | 0.7395 | 0.2474 | 0.1603 | 0.741 |
| $a+b/y\sqrt{z}+cx^2z^2$ | 125.42 | 91.51 | 0.809 | 0.0759 | 0.0530 | 0.7156 | 0.2581 | 0.1717 | 0.718 |
| $a+b/y\sqrt{z}+cx^2\sqrt{z}$ | 116.20 | 90.28 | 0.836 | 0.0724 | 0.0497 | 0.7413 | 0.2427 | 0.1544 | 0.750 |
| $a+b/y\sqrt{z}+c\sqrt{x}/z$ | 173.22 | 116.62 | 0.635 | 0.0982 | 0.0722 | 0.5243 | 0.3136 | 0.2052 | 0.583 |
| $a+b/y\sqrt{z}+c\sqrt{x}/z^2$ | 191.95 | 138.92 | 0.552 | 0.1053 | 0.0798 | 0.4530 | 0.3328 | 0.2347 | 0.531 |
| $a+b/y\sqrt{z}+c\sqrt{x}/\sqrt{z}$ | 172.02 | 117.11 | 0.640 | 0.0976 | 0.0708 | 0.5293 | 0.3138 | 0.2067 | 0.583 |
| $a+b/y\sqrt{z}+c\sqrt{x}z$ | 121.69 | 92.60 | 0.820 | 0.0702 | 0.0431 | 0.7565 | 0.2435 | 0.1459 | 0.749 |
| $a+b/y\sqrt{z}+c\sqrt{x}z^2$ | 126.17 | 93.61 | 0.806 | 0.0731 | 0.0483 | 0.7364 | 0.2527 | 0.1601 | 0.729 |
| $a+b/y\sqrt{z}+c\sqrt{x}\sqrt{z}$ | 122.09 | 92.55 | 0.819 | 0.0694 | 0.0414 | 0.7621 | 0.2384 | 0.1410 | 0.759 |
| $a+b/y\sqrt{z}+c/xz$ | 187.04 | 128.15 | 0.574 | 0.1073 | 0.0809 | 0.4319 | 0.3350 | 0.2338 | 0.525 |
| $a+b/y\sqrt{z}+c/xz^2$ | 162.74 | 119.86 | 0.678 | 0.0983 | 0.0715 | 0.5231 | 0.3068 | 0.2069 | 0.601 |
| $a+b/y\sqrt{z}+c/x\sqrt{z}$ | 191.20 | 131.13 | 0.555 | 0.1080 | 0.0811 | 0.4237 | 0.3379 | 0.2363 | 0.516 |
| $a+b/y\sqrt{z}+cz/x$ | 184.25 | 126.97 | 0.587 | 0.1064 | 0.0808 | 0.4412 | 0.3321 | 0.2330 | 0.533 |
| $a+b/y\sqrt{z}+cz^2/x$ | 151.50 | 107.92 | 0.721 | 0.0949 | 0.0696 | 0.5551 | 0.2997 | 0.1976 | 0.619 |
| $a+b/y\sqrt{z}+c\sqrt{z}/x$ | 190.28 | 130.54 | 0.559 | 0.1078 | 0.0812 | 0.4264 | 0.3369 | 0.2364 | 0.519 |
| $a+b/y\sqrt{z}+c/x^2z$ | 190.76 | 131.88 | 0.557 | 0.1080 | 0.0811 | 0.4241 | 0.3374 | 0.2365 | 0.518 |

(continued on next page)

**Table 4 – continued from previous page**

| Functional form | $T_{eff}$ (K) | | | Radius ($R_\odot$) | | | log ($L/L_\odot$) | | |
|---|---|---|---|---|---|---|---|---|---|
| | RMSE | MAD | $R^2_{ap}$ | RMSE | MAD | $R^2_{ap}$ | RMSE | MAD | $R^2_{ap}$ |
| $a+b/y\sqrt{z}+c/x^2z^2$ | 185.28 | 127.95 | 0.582 | 0.1070 | 0.0811 | 0.4348 | 0.3333 | 0.2344 | 0.529 |
| $a+b/y\sqrt{z}+c/x^2\sqrt{z}$ | 192.26 | 132.98 | 0.550 | 0.1082 | 0.0811 | 0.4216 | 0.3383 | 0.2367 | 0.515 |
| $a+b/y\sqrt{z}+cz/x^2$ | 194.25 | 134.31 | 0.541 | 0.1085 | 0.0809 | 0.4188 | 0.3396 | 0.2367 | 0.511 |
| $a+b/y\sqrt{z}+cz^2/x^2$ | 193.66 | 133.99 | 0.544 | 0.1084 | 0.0810 | 0.4199 | 0.3392 | 0.2367 | 0.513 |
| $a+b/y\sqrt{z}+c\sqrt{z}/x^2$ | 193.93 | 134.09 | 0.542 | 0.1085 | 0.0810 | 0.4192 | 0.3394 | 0.2368 | 0.512 |
| $a+b/y\sqrt{z}+c/\sqrt{x}z$ | 204.83 | 144.35 | 0.490 | 0.1051 | 0.0807 | 0.4544 | 0.3335 | 0.2400 | 0.529 |
| $a+b/y\sqrt{z}+c/\sqrt{x}z^2$ | 204.85 | 148.59 | 0.489 | 0.1089 | 0.0824 | 0.4139 | 0.3430 | 0.2457 | 0.501 |
| $a+b/y\sqrt{z}+c/\sqrt{x}\sqrt{z}$ | 207.07 | 149.53 | 0.478 | 0.1077 | 0.0824 | 0.4269 | 0.3416 | 0.2430 | 0.505 |
| $a+b/y\sqrt{z}+cz/\sqrt{x}$ | 144.84 | 107.18 | 0.745 | 0.0909 | 0.0646 | 0.5923 | 0.2899 | 0.1901 | 0.644 |
| $a+b/y\sqrt{z}+cz^2/\sqrt{x}$ | 126.81 | 93.51 | 0.804 | 0.0765 | 0.0522 | 0.7113 | 0.2586 | 0.1697 | 0.717 |
| $a+b/y\sqrt{z}+c\sqrt{z}/\sqrt{x}$ | 173.74 | 121.24 | 0.633 | 0.1029 | 0.0782 | 0.4775 | 0.3223 | 0.2225 | 0.560 |
| $a+bz/y+cx/z$ | 273.11 | 201.09 | 0.093 | 0.1388 | 0.1062 | 0.0488 | 0.4788 | 0.3619 | 0.029 |
| $a+bz/y+cx/z^2$ | 270.87 | 193.39 | 0.107 | 0.1387 | 0.1053 | 0.0496 | 0.4807 | 0.3620 | 0.021 |
| $a+bz/y+cx/\sqrt{z}$ | 143.53 | 109.20 | 0.749 | 0.0871 | 0.0689 | 0.6250 | 0.2674 | 0.2050 | 0.697 |
| $a+bz/y+cxz$ | 128.04 | 96.57 | 0.801 | 0.0725 | 0.0506 | 0.7405 | 0.2640 | 0.1925 | 0.705 |
| $a+bz/y+cxz^2$ | 155.57 | 117.03 | 0.706 | 0.0839 | 0.0643 | 0.6528 | 0.3112 | 0.2392 | 0.590 |
| $a+bz/y+cx\sqrt{z}$ | 115.20 | 89.03 | 0.839 | 0.0695 | 0.0446 | 0.7618 | 0.2415 | 0.1607 | 0.753 |
| $a+bz/y+cx^2/z$ | 196.42 | 145.71 | 0.531 | 0.1107 | 0.0843 | 0.3952 | 0.3584 | 0.2760 | 0.456 |
| $a+bz/y+cx^2/z^2$ | 277.32 | 196.55 | 0.064 | 0.1406 | 0.1050 | 0.0235 | 0.4883 | 0.3595 | -0.010 |
| $a+bz/y+cx^2/\sqrt{z}$ | 122.37 | 101.07 | 0.818 | 0.0821 | 0.0567 | 0.6673 | 0.2567 | 0.1841 | 0.721 |
| $a+bz/y+cx^2z$ | 138.00 | 105.48 | 0.768 | 0.0792 | 0.0600 | 0.6900 | 0.2893 | 0.2241 | 0.645 |
| $a+bz/y+cx^2z^2$ | 163.99 | 127.22 | 0.673 | 0.0901 | 0.0715 | 0.5993 | 0.3312 | 0.2598 | 0.535 |
| $a+bz/y+cx^2\sqrt{z}$ | 123.59 | 94.06 | 0.814 | 0.0751 | 0.0553 | 0.7217 | 0.2664 | 0.1991 | 0.699 |
| $a+bz/y+c\sqrt{x}/z$ | 256.64 | 183.18 | 0.199 | 0.1333 | 0.1003 | 0.1227 | 0.4610 | 0.3442 | 0.100 |
| $a+bz/y+c\sqrt{x}/z^2$ | 257.85 | 184.63 | 0.191 | 0.1346 | 0.1019 | 0.1057 | 0.4624 | 0.3485 | 0.094 |
| $a+bz/y+c\sqrt{x}/\sqrt{z}$ | 246.04 | 189.05 | 0.263 | 0.1251 | 0.1021 | 0.2277 | 0.4240 | 0.3432 | 0.238 |
| $a+bz/y+c\sqrt{x}z$ | 128.66 | 99.63 | 0.799 | 0.0712 | 0.0465 | 0.7499 | 0.2583 | 0.1836 | 0.717 |
| $a+bz/y+c\sqrt{x}z^2$ | 153.39 | 118.39 | 0.714 | 0.0815 | 0.0613 | 0.6724 | 0.3032 | 0.2289 | 0.610 |
| $a+bz/y+c\sqrt{x}\sqrt{z}$ | 119.93 | 93.91 | 0.825 | 0.0694 | 0.0409 | 0.7619 | 0.2402 | 0.1490 | 0.756 |
| $a+bz/y+c/xz$ | 169.05 | 133.82 | 0.652 | 0.0843 | 0.0630 | 0.6494 | 0.2863 | 0.2122 | 0.653 |
| $a+bz/y+c/xz^2$ | 169.44 | 124.89 | 0.651 | 0.0933 | 0.0717 | 0.5704 | 0.3044 | 0.2237 | 0.607 |
| $a+bz/y+c/x\sqrt{z}$ | 177.57 | 141.10 | 0.616 | 0.0844 | 0.0663 | 0.6481 | 0.2948 | 0.2254 | 0.632 |
| $a+bz/y+cz/x$ | 220.74 | 158.63 | 0.407 | 0.1004 | 0.0795 | 0.5019 | 0.3626 | 0.2690 | 0.443 |
| $a+bz/y+cz^2/x$ | 276.73 | 198.49 | 0.068 | 0.1401 | 0.1056 | 0.0311 | 0.4873 | 0.3592 | -0.006 |
| $a+bz/y+c\sqrt{z}/x$ | 202.93 | 152.70 | 0.499 | 0.0923 | 0.0744 | 0.5795 | 0.3327 | 0.2524 | 0.531 |
| $a+bz/y+c/x^2z$ | 208.95 | 156.01 | 0.469 | 0.0951 | 0.0764 | 0.5533 | 0.3435 | 0.2590 | 0.500 |
| $a+bz/y+c/x^2z^2$ | 193.85 | 151.62 | 0.543 | 0.0899 | 0.0723 | 0.6009 | 0.3196 | 0.2457 | 0.567 |
| $a+bz/y+c/x^2\sqrt{z}$ | 214.71 | 157.09 | 0.439 | 0.0975 | 0.0776 | 0.5304 | 0.3533 | 0.2629 | 0.471 |
| $a+bz/y+cz/x^2$ | 226.01 | 158.98 | 0.379 | 0.1028 | 0.0797 | 0.4781 | 0.3735 | 0.2691 | 0.409 |
| $a+bz/y+cz^2/x^2$ | 231.27 | 160.08 | 0.349 | 0.1055 | 0.0807 | 0.4502 | 0.3831 | 0.2719 | 0.378 |
| $a+bz/y+c\sqrt{z}/x^2$ | 222.99 | 158.57 | 0.395 | 0.1013 | 0.0792 | 0.4930 | 0.3681 | 0.2675 | 0.426 |
| $a+bz/y+c/\sqrt{x}z$ | 156.02 | 113.54 | 0.704 | 0.0878 | 0.0639 | 0.6194 | 0.2839 | 0.1919 | 0.659 |
| $a+bz/y+c/\sqrt{x}z^2$ | 188.51 | 131.94 | 0.568 | 0.1076 | 0.0793 | 0.4287 | 0.3504 | 0.2456 | 0.480 |
| $a+bz/y+c/\sqrt{x}\sqrt{z}$ | 151.75 | 120.01 | 0.720 | 0.0804 | 0.0577 | 0.6807 | 0.2661 | 0.1835 | 0.700 |
| $a+bz/y+cz/\sqrt{x}$ | 246.30 | 182.56 | 0.262 | 0.1338 | 0.0949 | 0.1158 | 0.4624 | 0.3328 | 0.094 |
| $a+bz/y+cz^2/\sqrt{x}$ | 156.80 | 127.53 | 0.701 | 0.0845 | 0.0611 | 0.6477 | 0.3100 | 0.2330 | 0.593 |
| $a+bz/y+c\sqrt{z}/\sqrt{x}$ | 208.21 | 154.30 | 0.473 | 0.0951 | 0.0769 | 0.5538 | 0.3382 | 0.2612 | 0.515 |
| $a+bz^2/y+cx/z$ | 161.34 | 127.16 | 0.683 | 0.0837 | 0.0646 | 0.6543 | 0.3013 | 0.2404 | 0.615 |
| $a+bz^2/y+cx/z^2$ | 180.56 | 136.42 | 0.603 | 0.0937 | 0.0686 | 0.5664 | 0.3454 | 0.2555 | 0.494 |
| $a+bz^2/y+cx/\sqrt{z}$ | 123.01 | 95.18 | 0.816 | 0.0695 | 0.0486 | 0.7614 | 0.2333 | 0.1635 | 0.769 |
| $a+bz^2/y+cxz$ | 127.43 | 96.65 | 0.802 | 0.0730 | 0.0519 | 0.7367 | 0.2663 | 0.1984 | 0.700 |
| $a+bz^2/y+cxz^2$ | 156.75 | 116.92 | 0.701 | 0.0852 | 0.0659 | 0.6412 | 0.3191 | 0.2504 | 0.569 |
| $a+bz^2/y+cx\sqrt{z}$ | 116.20 | 89.10 | 0.836 | 0.0691 | 0.0442 | 0.7643 | 0.2416 | 0.1602 | 0.753 |
| $a+bz^2/y+cx^2/z$ | 125.69 | 89.81 | 0.808 | 0.0732 | 0.0516 | 0.7352 | 0.2473 | 0.1830 | 0.741 |
| $a+bz^2/y+cx^2/z^2$ | 175.30 | 137.41 | 0.626 | 0.0909 | 0.0684 | 0.5916 | 0.3326 | 0.2583 | 0.531 |
| $a+bz^2/y+cx^2/\sqrt{z}$ | 104.90 | 82.53 | 0.866 | 0.0681 | 0.0452 | 0.7707 | 0.2254 | 0.1545 | 0.785 |
| $a+bz^2/y+cx^2z$ | 137.95 | 102.10 | 0.768 | 0.0794 | 0.0610 | 0.6890 | 0.2936 | 0.2348 | 0.635 |
| $a+bz^2/y+cx^2z^2$ | 160.86 | 119.14 | 0.685 | 0.0883 | 0.0676 | 0.6152 | 0.3291 | 0.2549 | 0.541 |
| $a+bz^2/y+cx^2\sqrt{z}$ | 122.82 | 91.91 | 0.816 | 0.0741 | 0.0540 | 0.7290 | 0.2673 | 0.2037 | 0.697 |
| $a+bz^2/y+c\sqrt{x}/z$ | 179.41 | 137.81 | 0.608 | 0.0921 | 0.0699 | 0.5807 | 0.3403 | 0.2599 | 0.509 |
| $a+bz^2/y+c\sqrt{x}/z^2$ | 180.04 | 138.01 | 0.606 | 0.0948 | 0.0699 | 0.5565 | 0.3488 | 0.2573 | 0.485 |
| $a+bz^2/y+c\sqrt{x}/\sqrt{z}$ | 152.46 | 118.77 | 0.717 | 0.0778 | 0.0593 | 0.7014 | 0.2781 | 0.2167 | 0.672 |
| $a+bz^2/y+c\sqrt{x}z$ | 127.19 | 96.99 | 0.803 | 0.0714 | 0.0468 | 0.7483 | 0.2578 | 0.1798 | 0.718 |
| $a+bz^2/y+c\sqrt{x}z^2$ | 155.16 | 116.74 | 0.707 | 0.0835 | 0.0644 | 0.6559 | 0.3131 | 0.2453 | 0.585 |
| $a+bz^2/y+c\sqrt{x}\sqrt{z}$ | 120.93 | 94.29 | 0.822 | 0.0692 | 0.0410 | 0.7638 | 0.2401 | 0.1476 | 0.756 |
| $a+bz^2/y+c/xz$ | 148.45 | 114.68 | 0.732 | 0.0746 | 0.0536 | 0.7254 | 0.2655 | 0.1869 | 0.701 |
| $a+bz^2/y+c/xz^2$ | 140.95 | 107.33 | 0.758 | 0.0766 | 0.0566 | 0.7106 | 0.2640 | 0.1782 | 0.705 |
| $a+bz^2/y+c/x\sqrt{z}$ | 153.38 | 117.58 | 0.714 | 0.0751 | 0.0554 | 0.7214 | 0.2720 | 0.1954 | 0.687 |
| $a+bz^2/y+cz/x$ | 164.61 | 121.90 | 0.670 | 0.0786 | 0.0594 | 0.6952 | 0.2928 | 0.2118 | 0.637 |
| $a+bz^2/y+cz^2/x$ | 168.82 | 124.95 | 0.653 | 0.0804 | 0.0617 | 0.6808 | 0.3005 | 0.2200 | 0.617 |
| $a+bz^2/y+c\sqrt{z}/x$ | 161.63 | 121.02 | 0.682 | 0.0774 | 0.0583 | 0.7042 | 0.2867 | 0.2077 | 0.652 |
| $a+bz^2/y+c/x^2z$ | 163.93 | 122.81 | 0.673 | 0.0785 | 0.0592 | 0.6959 | 0.2914 | 0.2111 | 0.640 |
| $a+bz^2/y+c/x^2z^2$ | 159.13 | 120.96 | 0.692 | 0.0770 | 0.0575 | 0.7069 | 0.2826 | 0.2041 | 0.662 |
| $a+bz^2/y+c/x^2\sqrt{z}$ | 165.59 | 123.21 | 0.666 | 0.0791 | 0.0596 | 0.6910 | 0.2949 | 0.2134 | 0.632 |
| $a+bz^2/y+cz/x^2$ | 168.59 | 123.61 | 0.654 | 0.0804 | 0.0604 | 0.6805 | 0.3015 | 0.2169 | 0.615 |
| $a+bz^2/y+cz^2/x^2$ | 169.54 | 123.70 | 0.650 | 0.0809 | 0.0607 | 0.6767 | 0.3038 | 0.2178 | 0.609 |
| $a+bz^2/y+c\sqrt{z}/x^2$ | 167.85 | 123.55 | 0.657 | 0.0801 | 0.0602 | 0.6833 | 0.2998 | 0.2161 | 0.619 |
| $a+bz^2/y+c/\sqrt{x}z$ | 135.25 | 105.05 | 0.777 | 0.0751 | 0.0538 | 0.7216 | 0.2557 | 0.1666 | 0.723 |
| $a+bz^2/y+c/\sqrt{x}z^2$ | 143.23 | 108.31 | 0.750 | 0.0838 | 0.0607 | 0.6533 | 0.2882 | 0.1955 | 0.648 |
| $a+bz^2/y+c/\sqrt{x}\sqrt{z}$ | 139.45 | 108.36 | 0.763 | 0.0728 | 0.0509 | 0.7386 | 0.2530 | 0.1723 | 0.729 |
| $a+bz^2/y+cz/\sqrt{x}$ | 169.25 | 124.85 | 0.651 | 0.0811 | 0.0620 | 0.6751 | 0.3025 | 0.2208 | 0.612 |
| $a+bz^2/y+cz^2/\sqrt{x}$ | 176.21 | 136.31 | 0.622 | 0.0947 | 0.0682 | 0.5576 | 0.3484 | 0.2566 | 0.486 |
| $a+bz^2/y+c\sqrt{z}/\sqrt{x}$ | 158.87 | 120.24 | 0.693 | 0.0764 | 0.0573 | 0.7121 | 0.2815 | 0.2047 | 0.664 |
| $a+b\sqrt{z}/y+cx/z$ | 239.02 | 174.70 | 0.305 | 0.1194 | 0.0889 | 0.2962 | 0.4078 | 0.2957 | 0.295 |
| $a+b\sqrt{z}/y+cx/z^2$ | 243.67 | 181.34 | 0.278 | 0.1247 | 0.0975 | 0.2328 | 0.4156 | 0.3141 | 0.268 |
| $a+b\sqrt{z}/y+cx/\sqrt{z}$ | 276.88 | 204.11 | 0.067 | 0.1389 | 0.1132 | 0.0470 | 0.4546 | 0.3630 | 0.124 |
| $a+b\sqrt{z}/y+cxz$ | 126.69 | 95.80 | 0.805 | 0.0715 | 0.0478 | 0.7475 | 0.2568 | 0.1824 | 0.721 |
| $a+b\sqrt{z}/y+cxz^2$ | 148.03 | 115.17 | 0.733 | 0.0796 | 0.0574 | 0.6874 | 0.2893 | 0.2119 | 0.645 |
| $a+b\sqrt{z}/y+cx\sqrt{z}$ | 115.88 | 89.82 | 0.837 | 0.0696 | 0.0446 | 0.7610 | 0.2405 | 0.1593 | 0.755 |
| $a+b\sqrt{z}/y+cx^2/z$ | 287.31 | 215.11 | -0.004 | 0.1418 | 0.1145 | 0.0072 | 0.4725 | 0.3766 | 0.054 |
| $a+b\sqrt{z}/y+cx^2/z^2$ | 260.42 | 191.46 | 0.175 | 0.1299 | 0.1009 | 0.1667 | 0.4381 | 0.3291 | 0.187 |

(continued on next page)

**Table 4 – continued from previous page**

| Functional form | $T_{eff}$ (K) | | | Radius ($R_\odot$) | | | log (L/$L_\odot$) | | |
|---|---|---|---|---|---|---|---|---|---|
| | RMSE | MAD | $R^2_{ap}$ | RMSE | MAD | $R^2_{ap}$ | RMSE | MAD | $R^2_{ap}$ |
| $a+b\sqrt{z}/y+cx^2/\sqrt{z}$ | 169.04 | 127.44 | 0.652 | 0.0997 | 0.0754 | 0.5095 | 0.3100 | 0.2352 | 0.593 |
| $a+b\sqrt{z}/y+cx^2z$ | 134.50 | 106.36 | 0.780 | 0.0767 | 0.0552 | 0.7092 | 0.2747 | 0.1998 | 0.680 |
| $a+b\sqrt{z}/y+cx^2z^2$ | 155.07 | 123.57 | 0.707 | 0.0847 | 0.0639 | 0.6456 | 0.3047 | 0.2260 | 0.607 |
| $a+b\sqrt{z}/y+cx^2\sqrt{z}$ | 123.86 | 96.35 | 0.813 | 0.0744 | 0.0534 | 0.7269 | 0.2596 | 0.1851 | 0.714 |
| $a+b\sqrt{z}/y+c\sqrt{x}/z$ | 199.76 | 141.77 | 0.514 | 0.1064 | 0.0760 | 0.4408 | 0.3550 | 0.2380 | 0.466 |
| $a+b\sqrt{z}/y+c\sqrt{x}/z^2$ | 231.90 | 171.53 | 0.346 | 0.1214 | 0.0948 | 0.2722 | 0.4002 | 0.2981 | 0.321 |
| $a+b\sqrt{z}/y+c\sqrt{x}/\sqrt{z}$ | 220.79 | 164.36 | 0.407 | 0.1127 | 0.0807 | 0.3732 | 0.3868 | 0.2743 | 0.366 |
| $a+b\sqrt{z}/y+c\sqrt{x}z$ | 127.70 | 98.71 | 0.802 | 0.0706 | 0.0447 | 0.7537 | 0.2532 | 0.1745 | 0.728 |
| $a+b\sqrt{z}/y+c\sqrt{x}z^2$ | 146.45 | 115.41 | 0.739 | 0.0777 | 0.0545 | 0.7017 | 0.2835 | 0.2048 | 0.659 |
| $a+b\sqrt{z}/y+c\sqrt{x}\sqrt{z}$ | 120.21 | 93.48 | 0.824 | 0.0695 | 0.0410 | 0.7615 | 0.2399 | 0.1480 | 0.756 |
| $a+b\sqrt{z}/y+c/xz$ | 230.62 | 170.16 | 0.353 | 0.1086 | 0.0842 | 0.4181 | 0.3643 | 0.2847 | 0.438 |
| $a+b\sqrt{z}/y+c/xz^2$ | 216.77 | 155.09 | 0.428 | 0.1132 | 0.0864 | 0.3676 | 0.3644 | 0.2665 | 0.437 |
| $a+b\sqrt{z}/y+c/x\sqrt{z}$ | 253.69 | 183.99 | 0.217 | 0.1164 | 0.0904 | 0.3312 | 0.3978 | 0.3037 | 0.329 |
| $a+b\sqrt{z}/y+cz/x$ | 281.55 | 216.02 | 0.036 | 0.1417 | 0.1147 | 0.0082 | 0.4724 | 0.3750 | 0.054 |
| $a+b\sqrt{z}/y+cz^2/x$ | 175.90 | 134.83 | 0.624 | 0.1045 | 0.0788 | 0.4604 | 0.3446 | 0.2445 | 0.497 |
| $a+b\sqrt{z}/y+c\sqrt{z}/x$ | 287.51 | 214.30 | -0.006 | 0.1374 | 0.1077 | 0.0680 | 0.4658 | 0.3585 | 0.081 |
| $a+b\sqrt{z}/y+c/x^2z$ | 287.16 | 214.00 | -0.003 | 0.1369 | 0.1070 | 0.0752 | 0.4648 | 0.3576 | 0.085 |
| $a+b\sqrt{z}/y+c/x^2z^2$ | 281.10 | 208.31 | 0.039 | 0.1319 | 0.1016 | 0.1415 | 0.4494 | 0.3443 | 0.144 |
| $a+b\sqrt{z}/y+c/x^2\sqrt{z}$ | 288.02 | 214.89 | -0.009 | 0.1381 | 0.1084 | 0.0584 | 0.4681 | 0.3606 | 0.072 |
| $a+b\sqrt{z}/y+cz/x^2$ | 288.41 | 215.52 | -0.012 | 0.1400 | 0.1101 | 0.0321 | 0.4725 | 0.3632 | 0.054 |
| $a+b\sqrt{z}/y+cz^2/x^2$ | 287.66 | 215.53 | -0.007 | 0.1410 | 0.1112 | 0.0181 | 0.4742 | 0.3669 | 0.047 |
| $a+b\sqrt{z}/y+c\sqrt{z}/x^2$ | 288.46 | 215.64 | -0.012 | 0.1395 | 0.1097 | 0.0389 | 0.4715 | 0.3628 | 0.058 |
| $a+b\sqrt{z}/y+c/\sqrt{x}z$ | 178.70 | 126.47 | 0.611 | 0.0973 | 0.0715 | 0.5326 | 0.3095 | 0.2064 | 0.594 |
| $a+b\sqrt{z}/y+c/\sqrt{x}z^2$ | 210.40 | 150.12 | 0.461 | 0.1153 | 0.0913 | 0.3430 | 0.3686 | 0.2734 | 0.424 |
| $a+b\sqrt{z}/y+c/\sqrt{x}\sqrt{z}$ | 177.96 | 136.41 | 0.615 | 0.0900 | 0.0650 | 0.6000 | 0.2939 | 0.2108 | 0.634 |
| $a+b\sqrt{z}/y+cz/\sqrt{x}$ | 144.37 | 110.59 | 0.746 | 0.0894 | 0.0596 | 0.6055 | 0.2976 | 0.1897 | 0.625 |
| $a+b\sqrt{z}/y+cz^2/\sqrt{x}$ | 142.52 | 115.26 | 0.753 | 0.0778 | 0.0516 | 0.7015 | 0.2784 | 0.1915 | 0.672 |
| $a+b\sqrt{z}/y+c\sqrt{z}/\sqrt{x}$ | 255.51 | 194.71 | 0.206 | 0.1355 | 0.1079 | 0.0939 | 0.4477 | 0.3472 | 0.151 |
| $a+b/y^2z+cx/z$ | 205.50 | 141.97 | 0.486 | 0.1110 | 0.0847 | 0.3917 | 0.3618 | 0.2646 | 0.445 |
| $a+b/y^2z+cx/z^2$ | 214.66 | 152.59 | 0.439 | 0.1155 | 0.0906 | 0.3418 | 0.3718 | 0.2713 | 0.414 |
| $a+b/y^2z+cx/\sqrt{z}$ | 238.23 | 169.21 | 0.309 | 0.1232 | 0.0951 | 0.2505 | 0.3973 | 0.2888 | 0.331 |
| $a+b/y^2z+cxz$ | 118.48 | 87.44 | 0.829 | 0.0704 | 0.0463 | 0.7556 | 0.2440 | 0.1554 | 0.748 |
| $a+b/y^2z+cxz^2$ | 129.06 | 93.81 | 0.797 | 0.0754 | 0.0535 | 0.7190 | 0.2624 | 0.1739 | 0.708 |
| $a+b/y^2z+cx\sqrt{z}$ | 116.59 | 89.88 | 0.835 | 0.0696 | 0.0439 | 0.7611 | 0.2358 | 0.1452 | 0.764 |
| $a+b/y^2z+cx^2/z$ | 239.89 | 172.05 | 0.300 | 0.1232 | 0.0943 | 0.2500 | 0.3978 | 0.2879 | 0.330 |
| $a+b/y^2z+cx^2/z^2$ | 222.45 | 157.33 | 0.398 | 0.1174 | 0.0913 | 0.3195 | 0.3804 | 0.2761 | 0.387 |
| $a+b/y^2z+cx^2/\sqrt{z}$ | 193.73 | 154.75 | 0.543 | 0.1051 | 0.0840 | 0.4550 | 0.3248 | 0.2520 | 0.553 |
| $a+b/y^2z+cx^2z$ | 119.63 | 89.37 | 0.826 | 0.0735 | 0.0520 | 0.7335 | 0.2520 | 0.1680 | 0.731 |
| $a+b/y^2z+cx^2z^2$ | 131.31 | 96.61 | 0.790 | 0.0786 | 0.0573 | 0.6950 | 0.2701 | 0.1856 | 0.691 |
| $a+b/y^2z+cx^2\sqrt{z}$ | 116.09 | 89.08 | 0.836 | 0.0726 | 0.0507 | 0.7397 | 0.2442 | 0.1593 | 0.747 |
| $a+b/y^2z+c\sqrt{x}/z$ | 188.57 | 128.72 | 0.567 | 0.1059 | 0.0797 | 0.4462 | 0.3421 | 0.2419 | 0.504 |
| $a+b/y^2z+c\sqrt{x}/z^2$ | 211.51 | 150.78 | 0.456 | 0.1150 | 0.0908 | 0.3465 | 0.3688 | 0.2717 | 0.424 |
| $a+b/y^2z+c\sqrt{x}/\sqrt{z}$ | 197.65 | 139.25 | 0.525 | 0.1096 | 0.0837 | 0.4071 | 0.3560 | 0.2628 | 0.463 |
| $a+b/y^2z+c\sqrt{x}z$ | 121.64 | 92.04 | 0.820 | 0.0702 | 0.0443 | 0.7564 | 0.2445 | 0.1489 | 0.747 |
| $a+b/y^2z+c\sqrt{x}z^2$ | 129.84 | 96.04 | 0.795 | 0.0746 | 0.0516 | 0.7252 | 0.2606 | 0.1685 | 0.712 |
| $a+b/y^2z+c\sqrt{x}\sqrt{z}$ | 122.11 | 92.14 | 0.819 | 0.0695 | 0.0414 | 0.7613 | 0.2378 | 0.1399 | 0.760 |
| $a+b/y^2z+c/xz$ | 241.28 | 175.62 | 0.292 | 0.1226 | 0.0956 | 0.2580 | 0.3957 | 0.2913 | 0.336 |
| $a+b/y^2z+c/xz^2$ | 241.04 | 175.41 | 0.293 | 0.1216 | 0.0931 | 0.2701 | 0.3926 | 0.2847 | 0.347 |
| $a+b/y^2z+c/x\sqrt{z}$ | 240.76 | 174.71 | 0.295 | 0.1231 | 0.0960 | 0.2519 | 0.3969 | 0.2920 | 0.332 |
| $a+b/y^2z+cz/x$ | 230.34 | 168.18 | 0.354 | 0.1235 | 0.0979 | 0.2474 | 0.3948 | 0.2940 | 0.340 |
| $a+b/y^2z+cz^2/x$ | 183.66 | 128.89 | 0.590 | 0.1085 | 0.0799 | 0.4184 | 0.3479 | 0.2482 | 0.487 |
| $a+b/y^2z+c\sqrt{z}/x$ | 237.07 | 171.14 | 0.316 | 0.1240 | 0.0969 | 0.2406 | 0.3981 | 0.2925 | 0.329 |
| $a+b/y^2z+c/x^2z$ | 237.57 | 171.52 | 0.313 | 0.1240 | 0.0965 | 0.2413 | 0.3982 | 0.2920 | 0.328 |
| $a+b/y^2z+c/x^2z^2$ | 236.34 | 171.58 | 0.320 | 0.1240 | 0.0970 | 0.2405 | 0.3979 | 0.2934 | 0.329 |
| $a+b/y^2z+c/x^2\sqrt{z}$ | 237.88 | 171.46 | 0.312 | 0.1239 | 0.0963 | 0.2416 | 0.3982 | 0.2915 | 0.328 |
| $a+b/y^2z+cz/x^2$ | 238.10 | 171.39 | 0.310 | 0.1239 | 0.0962 | 0.2418 | 0.3982 | 0.2912 | 0.328 |
| $a+b/y^2z+cz^2/x^2$ | 237.34 | 171.50 | 0.315 | 0.1240 | 0.0967 | 0.2409 | 0.3981 | 0.2923 | 0.328 |
| $a+b/y^2z+c\sqrt{z}/x^2$ | 238.15 | 171.39 | 0.310 | 0.1239 | 0.0962 | 0.2419 | 0.3982 | 0.2911 | 0.328 |
| $a+b/y^2z+c/\sqrt{x}z$ | 195.44 | 142.57 | 0.535 | 0.0982 | 0.0743 | 0.5240 | 0.3185 | 0.2212 | 0.570 |
| $a+b/y^2z+c/\sqrt{x}z^2$ | 211.97 | 153.38 | 0.453 | 0.1153 | 0.0914 | 0.3430 | 0.3677 | 0.2737 | 0.427 |
| $a+b/y^2z+c/\sqrt{x}\sqrt{z}$ | 222.06 | 160.00 | 0.400 | 0.1063 | 0.0807 | 0.4421 | 0.3482 | 0.2452 | 0.486 |
| $a+b/y^2z+cz/\sqrt{x}$ | 167.07 | 119.58 | 0.660 | 0.1010 | 0.0731 | 0.4961 | 0.3259 | 0.2295 | 0.550 |
| $a+b/y^2z+cz^2/\sqrt{x}$ | 133.40 | 94.67 | 0.783 | 0.0795 | 0.0568 | 0.6879 | 0.2715 | 0.1858 | 0.688 |
| $a+b/y^2z+c\sqrt{z}/\sqrt{x}$ | 218.13 | 156.45 | 0.421 | 0.1204 | 0.0943 | 0.2842 | 0.3845 | 0.2836 | 0.374 |
| $a+b/y^2z^2+cx/z$ | 218.95 | 158.81 | 0.417 | 0.1202 | 0.0938 | 0.2863 | 0.3923 | 0.2983 | 0.348 |
| $a+b/y^2z^2+cx/z^2$ | 222.81 | 161.10 | 0.396 | 0.1219 | 0.0971 | 0.2667 | 0.3945 | 0.2972 | 0.341 |
| $a+b/y^2z^2+cx/\sqrt{z}$ | 242.25 | 173.65 | 0.286 | 0.1278 | 0.1021 | 0.1936 | 0.4095 | 0.3113 | 0.290 |
| $a+b/y^2z^2+cxz$ | 114.89 | 83.86 | 0.839 | 0.0711 | 0.0481 | 0.7507 | 0.2468 | 0.1644 | 0.742 |
| $a+b/y^2z^2+cxz^2$ | 125.24 | 87.17 | 0.809 | 0.0772 | 0.0569 | 0.7061 | 0.2684 | 0.1890 | 0.695 |
| $a+b/y^2z^2+cx\sqrt{z}$ | 114.73 | 87.82 | 0.840 | 0.0696 | 0.0440 | 0.7610 | 0.2359 | 0.1432 | 0.764 |
| $a+b/y^2z^2+cx^2/z$ | 242.27 | 173.33 | 0.286 | 0.1279 | 0.1016 | 0.1920 | 0.4105 | 0.3125 | 0.286 |
| $a+b/y^2z^2+cx^2/z^2$ | 229.54 | 164.90 | 0.359 | 0.1237 | 0.0982 | 0.2439 | 0.4018 | 0.3042 | 0.316 |
| $a+b/y^2z^2+cx^2/\sqrt{z}$ | 191.26 | 151.89 | 0.555 | 0.1049 | 0.0838 | 0.4562 | 0.3231 | 0.2510 | 0.558 |
| $a+b/y^2z^2+cx^2z$ | 115.53 | 83.62 | 0.838 | 0.0747 | 0.0544 | 0.7248 | 0.2563 | 0.1812 | 0.722 |
| $a+b/y^2z^2+cx^2z^2$ | 127.44 | 90.53 | 0.802 | 0.0805 | 0.0611 | 0.6797 | 0.2768 | 0.2021 | 0.675 |
| $a+b/y^2z^2+cx^2\sqrt{z}$ | 112.36 | 85.51 | 0.846 | 0.0732 | 0.0522 | 0.7357 | 0.2463 | 0.1672 | 0.743 |
| $a+b/y^2z^2+c\sqrt{x}/z$ | 201.80 | 143.74 | 0.505 | 0.1143 | 0.0871 | 0.3550 | 0.3721 | 0.2735 | 0.413 |
| $a+b/y^2z^2+c\sqrt{x}/z^2$ | 219.63 | 159.59 | 0.413 | 0.1211 | 0.0965 | 0.2763 | 0.3909 | 0.2951 | 0.352 |
| $a+b/y^2z^2+c\sqrt{x}/\sqrt{z}$ | 217.53 | 158.25 | 0.424 | 0.1209 | 0.0941 | 0.2781 | 0.3935 | 0.2995 | 0.344 |
| $a+b/y^2z^2+c\sqrt{x}z$ | 118.65 | 88.67 | 0.829 | 0.0709 | 0.0456 | 0.7519 | 0.2474 | 0.1570 | 0.741 |
| $a+b/y^2z^2+c\sqrt{x}z^2$ | 126.30 | 90.12 | 0.806 | 0.0763 | 0.0547 | 0.7127 | 0.2666 | 0.1831 | 0.699 |
| $a+b/y^2z^2+c\sqrt{x}\sqrt{z}$ | 121.23 | 89.84 | 0.821 | 0.0695 | 0.0416 | 0.7614 | 0.2377 | 0.1381 | 0.761 |
| $a+b/y^2z^2+c/xz$ | 240.75 | 174.88 | 0.295 | 0.1226 | 0.0953 | 0.2579 | 0.3958 | 0.2895 | 0.336 |
| $a+b/y^2z^2+c/xz^2$ | 239.40 | 173.98 | 0.303 | 0.1216 | 0.0933 | 0.2704 | 0.3926 | 0.2834 | 0.347 |
| $a+b/y^2z^2+c/x\sqrt{z}$ | 241.34 | 174.80 | 0.291 | 0.1234 | 0.0958 | 0.2487 | 0.3982 | 0.2912 | 0.328 |
| $a+b/y^2z^2+cz/x$ | 240.84 | 175.91 | 0.294 | 0.1276 | 0.1009 | 0.1962 | 0.4106 | 0.3057 | 0.286 |
| $a+b/y^2z^2+cz^2/x$ | 207.39 | 145.34 | 0.477 | 0.1196 | 0.0896 | 0.2934 | 0.3874 | 0.2863 | 0.364 |
| $a+b/y^2z^2+c\sqrt{z}/x$ | 242.32 | 174.03 | 0.286 | 0.1259 | 0.0977 | 0.2168 | 0.4059 | 0.2962 | 0.302 |
| $a+b/y^2z^2+c/x^2z$ | 242.32 | 173.71 | 0.286 | 0.1256 | 0.0970 | 0.2205 | 0.4054 | 0.2943 | 0.304 |
| $a+b/y^2z^2+c/x^2z^2$ | 242.30 | 174.39 | 0.286 | 0.1260 | 0.0976 | 0.2164 | 0.4064 | 0.2964 | 0.300 |

(continued on next page)

**Table 4 – continued from previous page**

| Functional form | $T_{eff}$ (K) | | | Radius ($R_\odot$) | | | log (L/$L_\odot$) | | |
|---|---|---|---|---|---|---|---|---|---|
| | RMSE | MAD | $R^2_{ap}$ | RMSE | MAD | $R^2_{ap}$ | RMSE | MAD | $R^2_{ap}$ |
| $a+b/y^2z^2+c/x^2\sqrt{z}$ | 242.32 | 173.49 | 0.286 | 0.1256 | 0.0968 | 0.2217 | 0.4051 | 0.2936 | 0.305 |
| $a+b/y^2z^2+cz/x^2$ | 242.31 | 173.41 | 0.286 | 0.1255 | 0.0967 | 0.2219 | 0.4050 | 0.2934 | 0.305 |
| $a+b/y^2z^2+cz^2/x^2$ | 242.31 | 174.18 | 0.286 | 0.1259 | 0.0975 | 0.2168 | 0.4061 | 0.2957 | 0.301 |
| $a+b/y^2z^2+c\sqrt{z}/x^2$ | 242.31 | 173.32 | 0.286 | 0.1255 | 0.0966 | 0.2225 | 0.4049 | 0.2932 | 0.305 |
| $a+b/y^2z^2+c/\sqrt{x}z$ | 203.18 | 144.85 | 0.498 | 0.1005 | 0.0768 | 0.5014 | 0.3253 | 0.2294 | 0.552 |
| $a+b/y^2z^2+c/\sqrt{x}z^2$ | 210.68 | 151.94 | 0.460 | 0.1142 | 0.0880 | 0.3560 | 0.3676 | 0.2675 | 0.428 |
| $a+b/y^2z^2+c/\sqrt{x}\sqrt{z}$ | 221.05 | 158.40 | 0.405 | 0.1083 | 0.0816 | 0.4213 | 0.3506 | 0.2454 | 0.479 |
| $a+b/y^2z^2+cz/\sqrt{x}$ | 190.81 | 133.12 | 0.557 | 0.1127 | 0.0825 | 0.3727 | 0.3675 | 0.2666 | 0.428 |
| $a+b/y^2z^2+cz^2/\sqrt{x}$ | 137.83 | 102.31 | 0.769 | 0.0845 | 0.0603 | 0.6474 | 0.2897 | 0.2007 | 0.644 |
| $a+b/y^2z^2+c\sqrt{z}/\sqrt{x}$ | 235.81 | 171.48 | 0.323 | 0.1277 | 0.1012 | 0.1945 | 0.4109 | 0.3071 | 0.284 |
| $a+b/y^2\sqrt{z}+cx/z$ | 203.26 | 140.07 | 0.497 | 0.1071 | 0.0791 | 0.4333 | 0.3517 | 0.2450 | 0.476 |
| $a+b/y^2\sqrt{z}+cx/z^2$ | 214.35 | 153.60 | 0.441 | 0.1132 | 0.0867 | 0.3674 | 0.3658 | 0.2603 | 0.433 |
| $a+b/y^2\sqrt{z}+cx/\sqrt{z}$ | 240.31 | 169.64 | 0.297 | 0.1213 | 0.0904 | 0.2733 | 0.3952 | 0.2856 | 0.338 |
| $a+b/y^2\sqrt{z}+cxz$ | 121.25 | 90.23 | 0.821 | 0.0702 | 0.0454 | 0.7565 | 0.2449 | 0.1584 | 0.746 |
| $a+b/y^2\sqrt{z}+cxz^2$ | 133.45 | 99.63 | 0.783 | 0.0752 | 0.0518 | 0.7208 | 0.2636 | 0.1733 | 0.705 |
| $a+b/y^2\sqrt{z}+cx\sqrt{z}$ | 117.10 | 90.60 | 0.833 | 0.0696 | 0.0440 | 0.7611 | 0.2366 | 0.1483 | 0.763 |
| $a+b/y^2\sqrt{z}+cx^2/z$ | 243.22 | 173.20 | 0.280 | 0.1220 | 0.0911 | 0.2647 | 0.3973 | 0.2888 | 0.331 |
| $a+b/y^2\sqrt{z}+cx^2/z^2$ | 223.35 | 158.94 | 0.393 | 0.1154 | 0.0872 | 0.3426 | 0.3760 | 0.2684 | 0.401 |
| $a+b/y^2\sqrt{z}+cx^2/\sqrt{z}$ | 194.22 | 156.05 | 0.541 | 0.1052 | 0.0838 | 0.4537 | 0.3263 | 0.2516 | 0.549 |
| $a+b/y^2\sqrt{z}+cx^2z$ | 123.46 | 94.40 | 0.815 | 0.0733 | 0.0507 | 0.7346 | 0.2532 | 0.1688 | 0.728 |
| $a+b/y^2\sqrt{z}+cx^2z^2$ | 136.17 | 103.23 | 0.774 | 0.0784 | 0.0554 | 0.6965 | 0.2716 | 0.1847 | 0.687 |
| $a+b/y^2\sqrt{z}+cx^2\sqrt{z}$ | 118.73 | 92.29 | 0.828 | 0.0725 | 0.0499 | 0.7401 | 0.2454 | 0.1620 | 0.745 |
| $a+b/y^2\sqrt{z}+c\sqrt{x}/z$ | 184.89 | 123.87 | 0.584 | 0.1021 | 0.0749 | 0.4855 | 0.3306 | 0.2232 | 0.537 |
| $a+b/y^2\sqrt{z}+c\sqrt{x}/z^2$ | 210.36 | 150.26 | 0.462 | 0.1127 | 0.0873 | 0.3727 | 0.3620 | 0.2583 | 0.445 |
| $a+b/y^2\sqrt{z}+c\sqrt{x}/\sqrt{z}$ | 190.47 | 128.57 | 0.559 | 0.1036 | 0.0768 | 0.4696 | 0.3393 | 0.2394 | 0.512 |
| $a+b/y^2\sqrt{z}+c\sqrt{x}z$ | 123.90 | 94.42 | 0.813 | 0.0701 | 0.0433 | 0.7576 | 0.2451 | 0.1518 | 0.745 |
| $a+b/y^2\sqrt{z}+c\sqrt{x}z^2$ | 133.88 | 101.58 | 0.782 | 0.0743 | 0.0500 | 0.7274 | 0.2615 | 0.1679 | 0.710 |
| $a+b/y^2\sqrt{z}+c\sqrt{x}\sqrt{z}$ | 121.86 | 92.96 | 0.819 | 0.0695 | 0.0413 | 0.7613 | 0.2383 | 0.1423 | 0.759 |
| $a+b/y^2\sqrt{z}+c/xz$ | 244.15 | 177.02 | 0.275 | 0.1231 | 0.0961 | 0.2520 | 0.3986 | 0.2941 | 0.327 |
| $a+b/y^2\sqrt{z}+c/xz^2$ | 242.94 | 177.42 | 0.282 | 0.1215 | 0.0929 | 0.2715 | 0.3929 | 0.2835 | 0.346 |
| $a+b/y^2\sqrt{z}+c/x\sqrt{z}$ | 242.27 | 175.44 | 0.286 | 0.1234 | 0.0965 | 0.2476 | 0.3988 | 0.2942 | 0.326 |
| $a+b/y^2\sqrt{z}+cz/x$ | 223.82 | 162.38 | 0.391 | 0.1209 | 0.0957 | 0.2786 | 0.3855 | 0.2856 | 0.370 |
| $a+b/y^2\sqrt{z}+cz^2/x$ | 170.23 | 120.19 | 0.647 | 0.1017 | 0.0734 | 0.4890 | 0.3257 | 0.2237 | 0.550 |
| $a+b/y^2\sqrt{z}+c\sqrt{z}/x$ | 234.54 | 169.19 | 0.331 | 0.1231 | 0.0964 | 0.2520 | 0.3947 | 0.2905 | 0.340 |
| $a+b/y^2\sqrt{z}+c/x^2z$ | 235.57 | 170.16 | 0.325 | 0.1233 | 0.0963 | 0.2496 | 0.3955 | 0.2910 | 0.337 |
| $a+b/y^2\sqrt{z}+c/x^2z^2$ | 233.07 | 169.31 | 0.339 | 0.1230 | 0.0966 | 0.2534 | 0.3936 | 0.2915 | 0.343 |
| $a+b/y^2\sqrt{z}+c/x^2\sqrt{z}$ | 236.18 | 170.30 | 0.321 | 0.1233 | 0.0962 | 0.2488 | 0.3959 | 0.2908 | 0.336 |
| $a+b/y^2\sqrt{z}+cz/x^2$ | 236.65 | 170.38 | 0.319 | 0.1234 | 0.0961 | 0.2484 | 0.3962 | 0.2906 | 0.335 |
| $a+b/y^2\sqrt{z}+cz^2/x^2$ | 235.34 | 170.01 | 0.326 | 0.1232 | 0.0964 | 0.2503 | 0.3953 | 0.2910 | 0.338 |
| $a+b/y^2\sqrt{z}+c\sqrt{z}/x^2$ | 236.71 | 170.40 | 0.318 | 0.1234 | 0.0961 | 0.2483 | 0.3962 | 0.2906 | 0.335 |
| $a+b/y^2\sqrt{z}+c/\sqrt{x}z$ | 187.07 | 138.06 | 0.574 | 0.0975 | 0.0710 | 0.5302 | 0.3141 | 0.2112 | 0.582 |
| $a+b/y^2\sqrt{z}+c/\sqrt{x}z^2$ | 212.15 | 154.09 | 0.452 | 0.1150 | 0.0907 | 0.3470 | 0.3658 | 0.2702 | 0.433 |
| $a+b/y^2\sqrt{z}+c/\sqrt{x}\sqrt{z}$ | 216.60 | 151.77 | 0.429 | 0.1024 | 0.0787 | 0.4827 | 0.3387 | 0.2374 | 0.514 |
| $a+b/y^2\sqrt{z}+cz/\sqrt{x}$ | 154.62 | 113.67 | 0.709 | 0.0941 | 0.0669 | 0.5631 | 0.3036 | 0.2058 | 0.609 |
| $a+b/y^2\sqrt{z}+cz^2/\sqrt{x}$ | 133.81 | 96.07 | 0.782 | 0.0773 | 0.0546 | 0.7053 | 0.2656 | 0.1786 | 0.701 |
| $a+b/y^2\sqrt{z}+c\sqrt{z}/\sqrt{x}$ | 206.04 | 144.70 | 0.483 | 0.1152 | 0.0886 | 0.3452 | 0.3668 | 0.2656 | 0.430 |
| $a+bz/y^2+cx/z$ | 244.43 | 176.58 | 0.273 | 0.1186 | 0.0905 | 0.3060 | 0.4084 | 0.3032 | 0.293 |
| $a+bz/y^2+cx/z^2$ | 245.50 | 181.52 | 0.267 | 0.1230 | 0.0965 | 0.2526 | 0.4130 | 0.3096 | 0.277 |
| $a+bz/y^2+cx/\sqrt{z}$ | 279.33 | 210.19 | 0.051 | 0.1382 | 0.1101 | 0.0573 | 0.4561 | 0.3592 | 0.119 |
| $a+bz/y^2+cxz$ | 127.72 | 96.27 | 0.802 | 0.0714 | 0.0482 | 0.7486 | 0.2576 | 0.1839 | 0.719 |
| $a+bz/y^2+cxz^2$ | 149.96 | 115.11 | 0.726 | 0.0790 | 0.0574 | 0.6915 | 0.2893 | 0.2103 | 0.645 |
| $a+bz/y^2+cx\sqrt{z}$ | 114.55 | 88.40 | 0.840 | 0.0696 | 0.0444 | 0.7609 | 0.2407 | 0.1595 | 0.755 |
| $a+bz/y^2+cx^2/z$ | 284.74 | 214.68 | 0.014 | 0.1388 | 0.1092 | 0.0488 | 0.4637 | 0.3632 | 0.089 |
| $a+bz/y^2+cx^2/z^2$ | 261.74 | 191.82 | 0.167 | 0.1282 | 0.1003 | 0.1882 | 0.4346 | 0.3274 | 0.200 |
| $a+bz/y^2+cx^2/\sqrt{z}$ | 177.47 | 131.15 | 0.617 | 0.1032 | 0.0797 | 0.4739 | 0.3204 | 0.2447 | 0.565 |
| $a+bz/y^2+cx^2z$ | 135.48 | 105.81 | 0.777 | 0.0761 | 0.0547 | 0.7140 | 0.2738 | 0.2014 | 0.682 |
| $a+bz/y^2+cx^2z^2$ | 156.30 | 123.19 | 0.703 | 0.0837 | 0.0631 | 0.6537 | 0.3030 | 0.2256 | 0.611 |
| $a+bz/y^2+cx^2\sqrt{z}$ | 124.01 | 96.13 | 0.813 | 0.0740 | 0.0525 | 0.7299 | 0.2587 | 0.1853 | 0.716 |
| $a+bz/y^2+c\sqrt{x}/z$ | 205.57 | 145.19 | 0.486 | 0.1055 | 0.0758 | 0.4503 | 0.3564 | 0.2428 | 0.462 |
| $a+bz/y^2+c\sqrt{x}/z^2$ | 233.34 | 172.97 | 0.338 | 0.1197 | 0.0927 | 0.2923 | 0.3972 | 0.2956 | 0.331 |
| $a+bz/y^2+c\sqrt{x}/\sqrt{z}$ | 228.76 | 166.24 | 0.363 | 0.1111 | 0.0818 | 0.3909 | 0.3867 | 0.2792 | 0.366 |
| $a+bz/y^2+c\sqrt{x}z$ | 128.88 | 99.63 | 0.798 | 0.0706 | 0.0452 | 0.7536 | 0.2549 | 0.1762 | 0.725 |
| $a+bz/y^2+c\sqrt{x}z^2$ | 148.77 | 116.05 | 0.731 | 0.0774 | 0.0552 | 0.7040 | 0.2844 | 0.2037 | 0.657 |
| $a+bz/y^2+c\sqrt{x}\sqrt{z}$ | 118.02 | 91.79 | 0.831 | 0.0695 | 0.0407 | 0.7616 | 0.2402 | 0.1487 | 0.756 |
| $a+bz/y^2+c/xz$ | 203.06 | 152.93 | 0.498 | 0.1014 | 0.0745 | 0.4927 | 0.3310 | 0.2490 | 0.536 |
| $a+bz/y^2+c/xz^2$ | 214.05 | 154.85 | 0.443 | 0.1154 | 0.0900 | 0.3428 | 0.3675 | 0.2711 | 0.428 |
| $a+bz/y^2+c/x\sqrt{z}$ | 232.44 | 169.93 | 0.343 | 0.1073 | 0.0853 | 0.4320 | 0.3654 | 0.2853 | 0.434 |
| $a+bz/y^2+cz/x$ | 257.37 | 193.05 | 0.194 | 0.1338 | 0.1063 | 0.1161 | 0.4396 | 0.3360 | 0.181 |
| $a+bz/y^2+cz^2/x$ | 152.74 | 117.20 | 0.716 | 0.0901 | 0.0610 | 0.5987 | 0.3013 | 0.2008 | 0.615 |
| $a+bz/y^2+c\sqrt{z}/x$ | 285.37 | 214.21 | 0.009 | 0.1378 | 0.1092 | 0.0623 | 0.4644 | 0.3588 | 0.086 |
| $a+bz/y^2+c/x^2z$ | 285.60 | 214.21 | 0.008 | 0.1372 | 0.1084 | 0.0700 | 0.4637 | 0.3583 | 0.089 |
| $a+bz/y^2+c/x^2z^2$ | 280.55 | 207.36 | 0.042 | 0.1315 | 0.1008 | 0.1468 | 0.4480 | 0.3422 | 0.150 |
| $a+bz/y^2+c/x^2\sqrt{z}$ | 285.00 | 214.10 | 0.012 | 0.1381 | 0.1093 | 0.0589 | 0.4649 | 0.3589 | 0.084 |
| $a+bz/y^2+cz/x^2$ | 282.32 | 210.91 | 0.030 | 0.1388 | 0.1095 | 0.0491 | 0.4643 | 0.3585 | 0.087 |
| $a+bz/y^2+cz^2/x^2$ | 278.82 | 208.30 | 0.054 | 0.1387 | 0.1095 | 0.0504 | 0.4616 | 0.3570 | 0.097 |
| $a+bz/y^2+c\sqrt{z}/x^2$ | 283.31 | 212.09 | 0.023 | 0.1387 | 0.1097 | 0.0506 | 0.4648 | 0.3592 | 0.085 |
| $a+bz/y^2+c/\sqrt{x}z$ | 172.35 | 120.98 | 0.639 | 0.0980 | 0.0737 | 0.5260 | 0.3079 | 0.2062 | 0.598 |
| $a+bz/y^2+c/\sqrt{x}z^2$ | 210.53 | 151.42 | 0.461 | 0.1153 | 0.0911 | 0.3435 | 0.3681 | 0.2721 | 0.426 |
| $a+bz/y^2+c/\sqrt{x}\sqrt{z}$ | 156.23 | 113.94 | 0.703 | 0.0870 | 0.0640 | 0.6261 | 0.2757 | 0.1854 | 0.678 |
| $a+bz/y^2+cz/\sqrt{x}$ | 138.50 | 104.17 | 0.767 | 0.0807 | 0.0519 | 0.6785 | 0.2756 | 0.1763 | 0.678 |
| $a+bz/y^2+cz^2/\sqrt{x}$ | 146.48 | 116.92 | 0.739 | 0.0768 | 0.0514 | 0.7091 | 0.2783 | 0.1968 | 0.672 |
| $a+bz/y^2+c\sqrt{z}/\sqrt{x}$ | 206.03 | 148.20 | 0.484 | 0.1137 | 0.0832 | 0.3616 | 0.3756 | 0.2627 | 0.402 |
| $a+bz^2/y^2+cx/z$ | 287.65 | 210.06 | -0.007 | 0.1454 | 0.1094 | -0.0445 | 0.5014 | 0.3817 | -0.065 |
| $a+bz^2/y^2+cx/z^2$ | 274.11 | 197.91 | 0.086 | 0.1405 | 0.1081 | 0.0248 | 0.4841 | 0.3683 | 0.007 |
| $a+bz^2/y^2+cx/\sqrt{z}$ | 179.36 | 126.78 | 0.609 | 0.1047 | 0.0845 | 0.4592 | 0.3266 | 0.2592 | 0.548 |
| $a+bz^2/y^2+cxz$ | 128.39 | 96.36 | 0.799 | 0.0725 | 0.0506 | 0.7407 | 0.2646 | 0.1926 | 0.703 |
| $a+bz^2/y^2+cxz^2$ | 155.49 | 116.42 | 0.706 | 0.0831 | 0.0635 | 0.6590 | 0.3088 | 0.2332 | 0.596 |
| $a+bz^2/y^2+cx\sqrt{z}$ | 113.52 | 87.32 | 0.843 | 0.0694 | 0.0446 | 0.7620 | 0.2417 | 0.1604 | 0.753 |
| $a+bz^2/y^2+cx^2/z$ | 233.78 | 167.67 | 0.335 | 0.1270 | 0.0989 | 0.2030 | 0.4154 | 0.3202 | 0.269 |

(continued on next page)

**Table 4 – continued from previous page**

| Functional form | $T_{eff}$ (K) | | | Radius ($R_\odot$) | | | log (L/$L_\odot$) | | |
|---|---|---|---|---|---|---|---|---|---|
| | RMSE | MAD | $R^2_{ap}$ | RMSE | MAD | $R^2_{ap}$ | RMSE | MAD | $R^2_{ap}$ |
| $a+bz^2/y^2+cx^2/z^2$ | 285.29 | 202.90 | 0.010 | 0.1445 | 0.1097 | -0.0309 | 0.4991 | 0.3758 | -0.055 |
| $a+bz^2/y^2+cx^2/\sqrt{z}$ | 130.62 | 104.64 | 0.792 | 0.0874 | 0.0649 | 0.6226 | 0.2707 | 0.1976 | 0.689 |
| $a+bz^2/y^2+cx^2z$ | 138.09 | 104.77 | 0.768 | 0.0790 | 0.0596 | 0.6922 | 0.2884 | 0.2214 | 0.648 |
| $a+bz^2/y^2+cx^2z^2$ | 163.75 | 126.16 | 0.674 | 0.0894 | 0.0705 | 0.6057 | 0.3285 | 0.2534 | 0.543 |
| $a+bz^2/y^2+cx^2\sqrt{z}$ | 123.15 | 93.02 | 0.815 | 0.0751 | 0.0552 | 0.7218 | 0.2663 | 0.1982 | 0.700 |
| $a+bz^2/y^2+c\sqrt{x}/z$ | 255.46 | 182.60 | 0.206 | 0.1321 | 0.1006 | 0.1382 | 0.4561 | 0.3405 | 0.119 |
| $a+bz^2/y^2+c\sqrt{x}/z^2$ | 259.22 | 186.60 | 0.182 | 0.1355 | 0.1051 | 0.0940 | 0.4629 | 0.3507 | 0.092 |
| $a+bz^2/y^2+c\sqrt{x}/\sqrt{z}$ | 282.46 | 210.86 | 0.029 | 0.1437 | 0.1107 | -0.0189 | 0.4896 | 0.3780 | -0.016 |
| $a+bz^2/y^2+c\sqrt{x}z$ | 129.28 | 99.91 | 0.797 | 0.0713 | 0.0466 | 0.7490 | 0.2598 | 0.1842 | 0.714 |
| $a+bz^2/y^2+c\sqrt{x}z^2$ | 153.52 | 117.30 | 0.713 | 0.0808 | 0.0605 | 0.6780 | 0.3013 | 0.2243 | 0.615 |
| $a+bz^2/y^2+c\sqrt{x}\sqrt{z}$ | 117.81 | 92.87 | 0.831 | 0.0693 | 0.0409 | 0.7626 | 0.2404 | 0.1491 | 0.755 |
| $a+bz^2/y^2+c/xz$ | 161.29 | 124.45 | 0.683 | 0.0839 | 0.0658 | 0.6527 | 0.2789 | 0.2052 | 0.670 |
| $a+bz^2/y^2+c/xz^2$ | 170.74 | 128.38 | 0.645 | 0.0967 | 0.0745 | 0.5385 | 0.3107 | 0.2338 | 0.591 |
| $a+bz^2/y^2+c/x\sqrt{z}$ | 167.53 | 133.04 | 0.659 | 0.0822 | 0.0634 | 0.6664 | 0.2822 | 0.2157 | 0.662 |
| $a+bz^2/y^2+cz/x$ | 216.11 | 161.37 | 0.432 | 0.0982 | 0.0792 | 0.5236 | 0.3537 | 0.2697 | 0.470 |
| $a+bz^2/y^2+cz^2/x$ | 271.49 | 208.45 | 0.103 | 0.1429 | 0.1084 | -0.0084 | 0.4910 | 0.3768 | -0.022 |
| $a+bz^2/y^2+c\sqrt{z}/x$ | 194.37 | 149.55 | 0.540 | 0.0889 | 0.0724 | 0.6094 | 0.3193 | 0.2480 | 0.568 |
| $a+bz^2/y^2+c/x^2z$ | 201.74 | 153.53 | 0.505 | 0.0921 | 0.0752 | 0.5811 | 0.3319 | 0.2557 | 0.533 |
| $a+bz^2/y^2+c/x^2z^2$ | 185.84 | 145.94 | 0.580 | 0.0878 | 0.0699 | 0.6194 | 0.3087 | 0.2380 | 0.596 |
| $a+bz^2/y^2+c/x^2\sqrt{z}$ | 208.51 | 155.66 | 0.471 | 0.0947 | 0.0769 | 0.5576 | 0.3429 | 0.2613 | 0.502 |
| $a+bz^2/y^2+cz/x^2$ | 222.48 | 159.37 | 0.398 | 0.1008 | 0.0798 | 0.4988 | 0.3668 | 0.2703 | 0.430 |
| $a+bz^2/y^2+cz^2/x^2$ | 229.09 | 161.81 | 0.361 | 0.1040 | 0.0811 | 0.4661 | 0.3783 | 0.2742 | 0.394 |
| $a+bz^2/y^2+c\sqrt{z}/x^2$ | 218.70 | 158.05 | 0.418 | 0.0990 | 0.0790 | 0.5160 | 0.3602 | 0.2681 | 0.450 |
| $a+bz^2/y^2+c/\sqrt{x}z$ | 152.24 | 112.61 | 0.718 | 0.0887 | 0.0661 | 0.6116 | 0.2827 | 0.1976 | 0.661 |
| $a+bz^2/y^2+c/\sqrt{x}z^2$ | 190.28 | 135.03 | 0.559 | 0.1096 | 0.0829 | 0.4064 | 0.3544 | 0.2524 | 0.468 |
| $a+bz^2/y^2+c/\sqrt{x}\sqrt{z}$ | 143.81 | 110.01 | 0.748 | 0.0800 | 0.0597 | 0.6839 | 0.2595 | 0.1819 | 0.715 |
| $a+bz^2/y^2+cz/\sqrt{x}$ | 207.32 | 155.94 | 0.477 | 0.1163 | 0.0807 | 0.3319 | 0.4034 | 0.2825 | 0.311 |
| $a+bz^2/y^2+cz^2/\sqrt{x}$ | 155.52 | 123.33 | 0.706 | 0.0816 | 0.0579 | 0.6711 | 0.3022 | 0.2190 | 0.613 |
| $a+bz^2/y^2+c\sqrt{z}/\sqrt{x}$ | 206.66 | 162.67 | 0.480 | 0.0964 | 0.0794 | 0.5411 | 0.3360 | 0.2709 | 0.522 |
| $a+b\sqrt{z}/y^2+cx/z$ | 220.64 | 159.38 | 0.408 | 0.1088 | 0.0801 | 0.4152 | 0.3695 | 0.2671 | 0.421 |
| $a+b\sqrt{z}/y^2+cx/z^2$ | 228.70 | 169.31 | 0.364 | 0.1157 | 0.0893 | 0.3385 | 0.3830 | 0.2824 | 0.378 |
| $a+b\sqrt{z}/y^2+cx/\sqrt{z}$ | 267.46 | 199.72 | 0.130 | 0.1291 | 0.0997 | 0.1770 | 0.4304 | 0.3282 | 0.215 |
| $a+b\sqrt{z}/y^2+cxz$ | 126.37 | 95.14 | 0.806 | 0.0708 | 0.0469 | 0.7527 | 0.2526 | 0.1758 | 0.730 |
| $a+b\sqrt{z}/y^2+cxz^2$ | 144.92 | 111.18 | 0.744 | 0.0771 | 0.0546 | 0.7065 | 0.2782 | 0.1961 | 0.672 |
| $a+b\sqrt{z}/y^2+cx\sqrt{z}$ | 115.84 | 89.67 | 0.837 | 0.0696 | 0.0443 | 0.7609 | 0.2395 | 0.1568 | 0.757 |
| $a+b\sqrt{z}/y^2+cx^2/z$ | 267.42 | 199.85 | 0.130 | 0.1292 | 0.0998 | 0.1755 | 0.4304 | 0.3281 | 0.215 |
| $a+b\sqrt{z}/y^2+cx^2/z^2$ | 242.13 | 178.39 | 0.287 | 0.1196 | 0.0925 | 0.2940 | 0.3999 | 0.2962 | 0.322 |
| $a+b\sqrt{z}/y^2+cx^2/\sqrt{z}$ | 188.19 | 145.50 | 0.569 | 0.1050 | 0.0814 | 0.4553 | 0.3269 | 0.2501 | 0.547 |
| $a+b\sqrt{z}/y^2+cx^2z$ | 132.21 | 103.56 | 0.787 | 0.0747 | 0.0528 | 0.7245 | 0.2651 | 0.1903 | 0.702 |
| $a+b\sqrt{z}/y^2+cx^2z^2$ | 149.80 | 117.59 | 0.727 | 0.0810 | 0.0598 | 0.6758 | 0.2891 | 0.2118 | 0.646 |
| $a+b\sqrt{z}/y^2+cx^2\sqrt{z}$ | 123.18 | 96.00 | 0.815 | 0.0733 | 0.0512 | 0.7350 | 0.2534 | 0.1779 | 0.728 |
| $a+b\sqrt{z}/y^2+c\sqrt{x}/z$ | 191.83 | 134.41 | 0.552 | 0.1004 | 0.0693 | 0.5022 | 0.3337 | 0.2207 | 0.528 |
| $a+b\sqrt{z}/y^2+c\sqrt{x}/z^2$ | 220.23 | 163.42 | 0.410 | 0.1139 | 0.0867 | 0.3589 | 0.3732 | 0.2728 | 0.410 |
| $a+b\sqrt{z}/y^2+c\sqrt{x}/\sqrt{z}$ | 201.31 | 146.21 | 0.507 | 0.1009 | 0.0693 | 0.4976 | 0.3447 | 0.2374 | 0.497 |
| $a+b\sqrt{z}/y^2+c\sqrt{x}z$ | 127.90 | 98.56 | 0.801 | 0.0703 | 0.0441 | 0.7560 | 0.2511 | 0.1684 | 0.733 |
| $a+b\sqrt{z}/y^2+c\sqrt{x}z^2$ | 144.30 | 112.47 | 0.747 | 0.0758 | 0.0525 | 0.7162 | 0.2746 | 0.1903 | 0.681 |
| $a+b\sqrt{z}/y^2+c\sqrt{x}\sqrt{z}$ | 119.35 | 92.39 | 0.827 | 0.0695 | 0.0409 | 0.7614 | 0.2397 | 0.1471 | 0.756 |
| $a+b\sqrt{z}/y^2+c/xz$ | 250.07 | 180.71 | 0.239 | 0.1182 | 0.0910 | 0.3102 | 0.3937 | 0.2947 | 0.343 |
| $a+b\sqrt{z}/y^2+c/xz^2$ | 227.38 | 162.41 | 0.371 | 0.1192 | 0.0921 | 0.2989 | 0.3817 | 0.2768 | 0.383 |
| $a+b\sqrt{z}/y^2+c/x\sqrt{z}$ | 267.65 | 200.91 | 0.128 | 0.1279 | 0.1020 | 0.1929 | 0.4268 | 0.3263 | 0.228 |
| $a+b\sqrt{z}/y^2+cz/x$ | 221.62 | 164.30 | 0.402 | 0.1202 | 0.0953 | 0.2868 | 0.3856 | 0.2901 | 0.370 |
| $a+b\sqrt{z}/y^2+cz^2/x$ | 151.01 | 112.65 | 0.723 | 0.0903 | 0.0615 | 0.5970 | 0.2955 | 0.1941 | 0.630 |
| $a+b\sqrt{z}/y^2+c\sqrt{z}/x$ | 247.94 | 180.91 | 0.252 | 0.1279 | 0.0996 | 0.1924 | 0.4157 | 0.3109 | 0.268 |
| $a+b\sqrt{z}/y^2+c/x^2z$ | 251.18 | 183.48 | 0.232 | 0.1288 | 0.0995 | 0.1812 | 0.4190 | 0.3138 | 0.256 |
| $a+b\sqrt{z}/y^2+c/x^2z^2$ | 251.14 | 184.26 | 0.233 | 0.1287 | 0.0995 | 0.1816 | 0.4192 | 0.3149 | 0.255 |
| $a+b\sqrt{z}/y^2+c/x^2\sqrt{z}$ | 251.24 | 183.21 | 0.232 | 0.1288 | 0.0996 | 0.1812 | 0.4190 | 0.3134 | 0.256 |
| $a+b\sqrt{z}/y^2+cz/x^2$ | 250.31 | 182.44 | 0.238 | 0.1285 | 0.0996 | 0.1841 | 0.4178 | 0.3126 | 0.260 |
| $a+b\sqrt{z}/y^2+cz^2/x^2$ | 246.88 | 181.49 | 0.258 | 0.1277 | 0.0999 | 0.1944 | 0.4141 | 0.3122 | 0.273 |
| $a+b\sqrt{z}/y^2+c\sqrt{z}/x^2$ | 250.90 | 182.67 | 0.234 | 0.1287 | 0.0995 | 0.1824 | 0.4184 | 0.3127 | 0.258 |
| $a+b\sqrt{z}/y^2+c/\sqrt{x}z$ | 176.74 | 124.10 | 0.620 | 0.0989 | 0.0734 | 0.5168 | 0.3119 | 0.2034 | 0.588 |
| $a+b\sqrt{z}/y^2+c/\sqrt{x}z^2$ | 211.92 | 153.01 | 0.454 | 0.1148 | 0.0901 | 0.3492 | 0.3659 | 0.2682 | 0.433 |
| $a+b\sqrt{z}/y^2+c/\sqrt{x}\sqrt{z}$ | 167.53 | 124.10 | 0.659 | 0.0885 | 0.0641 | 0.6134 | 0.2853 | 0.1976 | 0.655 |
| $a+b\sqrt{z}/y^2+cz/\sqrt{x}$ | 138.53 | 104.06 | 0.767 | 0.0825 | 0.0552 | 0.6642 | 0.2743 | 0.1753 | 0.681 |
| $a+b\sqrt{z}/y^2+cz^2/\sqrt{x}$ | 141.15 | 110.72 | 0.758 | 0.0757 | 0.0509 | 0.7171 | 0.2694 | 0.1826 | 0.693 |
| $a+b\sqrt{z}/y^2+c\sqrt{z}/\sqrt{x}$ | 185.36 | 130.09 | 0.582 | 0.1055 | 0.0768 | 0.4507 | 0.3401 | 0.2332 | 0.510 |
| $a+b/\sqrt{y}z+cx/z$ | 177.43 | 124.09 | 0.617 | 0.1021 | 0.0781 | 0.4852 | 0.3205 | 0.2255 | 0.565 |
| $a+b/\sqrt{y}z+cx/z^2$ | 176.57 | 127.07 | 0.621 | 0.1012 | 0.0776 | 0.4944 | 0.3135 | 0.2182 | 0.584 |
| $a+b/\sqrt{y}z+cx/\sqrt{z}$ | 177.28 | 127.68 | 0.618 | 0.1017 | 0.0785 | 0.4898 | 0.3152 | 0.2212 | 0.579 |
| $a+b/\sqrt{y}z+cxz$ | 115.54 | 87.62 | 0.838 | 0.0716 | 0.0472 | 0.7469 | 0.2502 | 0.1613 | 0.735 |
| $a+b/\sqrt{y}z+cxz^2$ | 118.20 | 86.74 | 0.830 | 0.0753 | 0.0517 | 0.7203 | 0.2607 | 0.1677 | 0.712 |
| $a+b/\sqrt{y}z+cx\sqrt{z}$ | 115.08 | 89.60 | 0.839 | 0.0696 | 0.0447 | 0.7611 | 0.2387 | 0.1478 | 0.759 |
| $a+b/\sqrt{y}z+cx^2/z$ | 175.36 | 127.85 | 0.626 | 0.1013 | 0.0788 | 0.4936 | 0.3111 | 0.2221 | 0.590 |
| $a+b/\sqrt{y}z+cx^2/z^2$ | 175.91 | 126.96 | 0.623 | 0.1012 | 0.0780 | 0.4943 | 0.3119 | 0.2189 | 0.588 |
| $a+b/\sqrt{y}z+cx^2/\sqrt{z}$ | 158.19 | 119.10 | 0.696 | 0.0939 | 0.0715 | 0.5650 | 0.2824 | 0.2036 | 0.662 |
| $a+b/\sqrt{y}z+cx^2z$ | 113.00 | 85.84 | 0.845 | 0.0740 | 0.0514 | 0.7294 | 0.2544 | 0.1674 | 0.726 |
| $a+b/\sqrt{y}z+cx^2z^2$ | 116.24 | 84.84 | 0.836 | 0.0769 | 0.0545 | 0.7082 | 0.2629 | 0.1740 | 0.707 |
| $a+b/\sqrt{y}z+cx^2\sqrt{z}$ | 111.75 | 88.94 | 0.848 | 0.0731 | 0.0507 | 0.7361 | 0.2476 | 0.1625 | 0.740 |
| $a+b/\sqrt{y}z+c\sqrt{x}/z$ | 176.33 | 120.00 | 0.622 | 0.1020 | 0.0775 | 0.4868 | 0.3220 | 0.2241 | 0.561 |
| $a+b/\sqrt{y}z+c\sqrt{x}/z^2$ | 176.36 | 126.83 | 0.622 | 0.1007 | 0.0768 | 0.4989 | 0.3123 | 0.2149 | 0.587 |
| $a+b/\sqrt{y}z+c\sqrt{x}/\sqrt{z}$ | 176.04 | 119.61 | 0.623 | 0.1020 | 0.0776 | 0.4867 | 0.3219 | 0.2241 | 0.561 |
| $a+b/\sqrt{y}z+c\sqrt{x}z$ | 119.97 | 92.11 | 0.825 | 0.0716 | 0.0459 | 0.7468 | 0.2521 | 0.1586 | 0.731 |
| $a+b/\sqrt{y}z+c\sqrt{x}z^2$ | 120.67 | 89.40 | 0.823 | 0.0750 | 0.0503 | 0.7219 | 0.2611 | 0.1671 | 0.711 |
| $a+b/\sqrt{y}z+c\sqrt{x}\sqrt{z}$ | 121.55 | 91.16 | 0.820 | 0.0690 | 0.0421 | 0.7652 | 0.2399 | 0.1439 | 0.756 |
| $a+b/\sqrt{y}z+c/xz$ | 176.30 | 122.69 | 0.622 | 0.1017 | 0.0773 | 0.4892 | 0.3201 | 0.2197 | 0.566 |
| $a+b/\sqrt{y}z+c/xz^2$ | 171.49 | 117.33 | 0.642 | 0.1018 | 0.0777 | 0.4882 | 0.3222 | 0.2208 | 0.560 |
| $a+b/\sqrt{y}z+c/x\sqrt{z}$ | 176.92 | 123.00 | 0.619 | 0.1013 | 0.0764 | 0.4935 | 0.3188 | 0.2169 | 0.569 |
| $a+b/\sqrt{y}z+cz/x$ | 175.94 | 123.11 | 0.623 | 0.1018 | 0.0774 | 0.4884 | 0.3207 | 0.2197 | 0.564 |
| $a+b/\sqrt{y}z+cz^2/x$ | 162.91 | 112.47 | 0.677 | 0.1000 | 0.0753 | 0.5066 | 0.3187 | 0.2133 | 0.570 |
| $a+b/\sqrt{y}z+c\sqrt{z}/x$ | 176.91 | 123.18 | 0.619 | 0.1013 | 0.0763 | 0.4938 | 0.3189 | 0.2165 | 0.569 |
| $a+b/\sqrt{y}z+c/x^2z$ | 176.69 | 123.45 | 0.620 | 0.1013 | 0.0762 | 0.4937 | 0.3193 | 0.2167 | 0.568 |

(continued on next page)

**Table 4 – continued from previous page**

| Functional form | $T_{eff}$ (K) | | | Radius ($R_\odot$) | | | log ($L/L_\odot$) | | |
|---|---|---|---|---|---|---|---|---|---|
| | RMSE | MAD | $R^2_{ap}$ | RMSE | MAD | $R^2_{ap}$ | RMSE | MAD | $R^2_{ap}$ |
| $a+b/\sqrt{y}z+c/x^2z^2$ | 176.12 | 123.10 | 0.623 | 0.1017 | 0.0771 | 0.4897 | 0.3204 | 0.2193 | 0.565 |
| $a+b/\sqrt{y}z+c/x^2\sqrt{z}$ | 176.84 | 123.47 | 0.620 | 0.1011 | 0.0758 | 0.4951 | 0.3190 | 0.2158 | 0.569 |
| $a+b/\sqrt{y}z+cz/x^2$ | 177.03 | 123.45 | 0.619 | 0.1009 | 0.0753 | 0.4972 | 0.3186 | 0.2144 | 0.570 |
| $a+b/\sqrt{y}z+cz^2/x^2$ | 176.91 | 123.56 | 0.619 | 0.1010 | 0.0756 | 0.4960 | 0.3189 | 0.2150 | 0.569 |
| $a+b/\sqrt{y}z+c\sqrt{z}/x^2$ | 177.00 | 123.45 | 0.619 | 0.1009 | 0.0754 | 0.4969 | 0.3186 | 0.2146 | 0.570 |
| $a+b/\sqrt{y}z+c/\sqrt{x}z$ | 177.03 | 122.50 | 0.619 | 0.1013 | 0.0767 | 0.4930 | 0.3183 | 0.2173 | 0.571 |
| $a+b/\sqrt{y}z+c/\sqrt{x}z^2$ | 136.05 | 92.62 | 0.775 | 0.0858 | 0.0570 | 0.6363 | 0.2794 | 0.1685 | 0.669 |
| $a+b/\sqrt{y}z+c/\sqrt{x}\sqrt{z}$ | 177.62 | 126.10 | 0.616 | 0.1000 | 0.0753 | 0.5067 | 0.3137 | 0.2157 | 0.583 |
| $a+b/\sqrt{y}z+cz/\sqrt{x}$ | 161.80 | 110.61 | 0.681 | 0.0988 | 0.0728 | 0.5182 | 0.3171 | 0.2094 | 0.574 |
| $a+b/\sqrt{y}z+cz^2/\sqrt{x}$ | 131.73 | 96.74 | 0.789 | 0.0824 | 0.0550 | 0.6649 | 0.2803 | 0.1784 | 0.667 |
| $a+b/\sqrt{y}z+c\sqrt{z}/\sqrt{x}$ | 174.99 | 121.88 | 0.627 | 0.1021 | 0.0782 | 0.4852 | 0.3217 | 0.2222 | 0.562 |
| $a+b/\sqrt{y}z^2+cx/z$ | 215.87 | 156.65 | 0.433 | 0.1202 | 0.0954 | 0.2871 | 0.3851 | 0.2948 | 0.372 |
| $a+b/\sqrt{y}z^2+cx/z^2$ | 212.81 | 156.63 | 0.449 | 0.1190 | 0.0955 | 0.3011 | 0.3780 | 0.2910 | 0.395 |
| $a+b/\sqrt{y}z^2+cx/\sqrt{z}$ | 206.54 | 153.62 | 0.481 | 0.1152 | 0.0917 | 0.3443 | 0.3596 | 0.2722 | 0.452 |
| $a+b/\sqrt{y}z^2+cxz$ | 118.63 | 89.26 | 0.829 | 0.0728 | 0.0509 | 0.7382 | 0.2612 | 0.1854 | 0.711 |
| $a+b/\sqrt{y}z^2+cxz^2$ | 127.81 | 93.51 | 0.801 | 0.0798 | 0.0588 | 0.6854 | 0.2848 | 0.2024 | 0.656 |
| $a+b/\sqrt{y}z^2+cx\sqrt{z}$ | 114.90 | 90.15 | 0.839 | 0.0694 | 0.0448 | 0.7620 | 0.2409 | 0.1568 | 0.754 |
| $a+b/\sqrt{y}z^2+cx^2/z$ | 203.39 | 151.68 | 0.497 | 0.1155 | 0.0931 | 0.3412 | 0.3580 | 0.2760 | 0.457 |
| $a+b/\sqrt{y}z^2+cx^2/z^2$ | 209.95 | 155.16 | 0.464 | 0.1182 | 0.0952 | 0.3101 | 0.3719 | 0.2889 | 0.414 |
| $a+b/\sqrt{y}z^2+cx^2/\sqrt{z}$ | 166.14 | 127.96 | 0.664 | 0.0986 | 0.0762 | 0.5198 | 0.2977 | 0.2205 | 0.624 |
| $a+b/\sqrt{y}z^2+cx^2z$ | 119.05 | 88.55 | 0.828 | 0.0770 | 0.0568 | 0.7072 | 0.2722 | 0.1988 | 0.686 |
| $a+b/\sqrt{y}z^2+cx^2z^2$ | 128.06 | 94.47 | 0.800 | 0.0827 | 0.0624 | 0.6626 | 0.2911 | 0.2129 | 0.641 |
| $a+b/\sqrt{y}z^2+cx^2\sqrt{z}$ | 114.19 | 90.38 | 0.841 | 0.0744 | 0.0540 | 0.7266 | 0.2579 | 0.1845 | 0.718 |
| $a+b/\sqrt{y}z^2+c\sqrt{x}/z$ | 215.54 | 155.01 | 0.435 | 0.1200 | 0.0915 | 0.2891 | 0.3914 | 0.2869 | 0.351 |
| $a+b/\sqrt{y}z^2+c\sqrt{x}/z^2$ | 213.90 | 156.82 | 0.443 | 0.1193 | 0.0956 | 0.2978 | 0.3804 | 0.2914 | 0.387 |
| $a+b/\sqrt{y}z^2+c\sqrt{x}/\sqrt{z}$ | 216.43 | 155.38 | 0.430 | 0.1203 | 0.0951 | 0.2860 | 0.3870 | 0.2929 | 0.365 |
| $a+b/\sqrt{y}z^2+c\sqrt{x}z$ | 122.77 | 94.15 | 0.817 | 0.0723 | 0.0485 | 0.7416 | 0.2614 | 0.1802 | 0.711 |
| $a+b/\sqrt{y}z^2+c\sqrt{x}z^2$ | 129.74 | 96.72 | 0.795 | 0.0792 | 0.0570 | 0.6906 | 0.2838 | 0.1982 | 0.659 |
| $a+b/\sqrt{y}z^2+c\sqrt{x}\sqrt{z}$ | 121.42 | 91.44 | 0.821 | 0.0687 | 0.0415 | 0.7670 | 0.2404 | 0.1494 | 0.755 |
| $a+b/\sqrt{y}z^2+c/xz$ | 211.31 | 151.87 | 0.457 | 0.1133 | 0.0873 | 0.3663 | 0.3626 | 0.2628 | 0.443 |
| $a+b/\sqrt{y}z^2+c/xz^2$ | 213.41 | 152.06 | 0.446 | 0.1160 | 0.0914 | 0.3361 | 0.3706 | 0.2728 | 0.418 |
| $a+b/\sqrt{y}z^2+c/x\sqrt{z}$ | 211.23 | 151.49 | 0.457 | 0.1129 | 0.0871 | 0.3704 | 0.3622 | 0.2614 | 0.444 |
| $a+b/\sqrt{y}z^2+cz/x$ | 215.59 | 153.49 | 0.434 | 0.1171 | 0.0911 | 0.3231 | 0.3777 | 0.2727 | 0.396 |
| $a+b/\sqrt{y}z^2+cz^2/x$ | 206.69 | 141.84 | 0.480 | 0.1188 | 0.0900 | 0.3026 | 0.3895 | 0.2770 | 0.357 |
| $a+b/\sqrt{y}z^2+c\sqrt{z}/x$ | 213.41 | 150.92 | 0.446 | 0.1146 | 0.0877 | 0.3512 | 0.3692 | 0.2629 | 0.423 |
| $a+b/\sqrt{y}z^2+c/x^2z$ | 213.81 | 150.70 | 0.444 | 0.1147 | 0.0875 | 0.3508 | 0.3702 | 0.2627 | 0.419 |
| $a+b/\sqrt{y}z^2+c/x^2z^2$ | 213.89 | 150.52 | 0.443 | 0.1151 | 0.0887 | 0.3461 | 0.3707 | 0.2643 | 0.418 |
| $a+b/\sqrt{y}z^2+c/x^2\sqrt{z}$ | 213.82 | 150.86 | 0.444 | 0.1146 | 0.0872 | 0.3518 | 0.3703 | 0.2632 | 0.419 |
| $a+b/\sqrt{y}z^2+cz/x^2$ | 214.03 | 150.98 | 0.443 | 0.1147 | 0.0869 | 0.3509 | 0.3712 | 0.2641 | 0.416 |
| $a+b/\sqrt{y}z^2+cz^2/x^2$ | 214.53 | 151.65 | 0.440 | 0.1152 | 0.0876 | 0.3447 | 0.3731 | 0.2663 | 0.410 |
| $a+b/\sqrt{y}z^2+c\sqrt{z}/x^2$ | 213.92 | 151.00 | 0.443 | 0.1146 | 0.0869 | 0.3519 | 0.3708 | 0.2638 | 0.418 |
| $a+b/\sqrt{y}z^2+c/\sqrt{x}z$ | 199.38 | 146.80 | 0.516 | 0.1053 | 0.0812 | 0.4522 | 0.3332 | 0.2404 | 0.530 |
| $a+b/\sqrt{y}z^2+c/\sqrt{x}z^2$ | 211.85 | 152.68 | 0.454 | 0.1148 | 0.0901 | 0.3492 | 0.3654 | 0.2677 | 0.434 |
| $a+b/\sqrt{y}z^2+c/\sqrt{x}\sqrt{z}$ | 200.71 | 147.33 | 0.510 | 0.1059 | 0.0819 | 0.4461 | 0.3364 | 0.2430 | 0.520 |
| $a+b/\sqrt{y}z^2+cz/\sqrt{x}$ | 202.60 | 139.66 | 0.501 | 0.1168 | 0.0852 | 0.3270 | 0.3858 | 0.2709 | 0.369 |
| $a+b/\sqrt{y}z^2+cz^2/\sqrt{x}$ | 149.35 | 111.31 | 0.729 | 0.0899 | 0.0617 | 0.6011 | 0.3160 | 0.2104 | 0.577 |
| $a+b/\sqrt{y}z^2+c\sqrt{z}/\sqrt{x}$ | 216.22 | 154.71 | 0.431 | 0.1187 | 0.0937 | 0.3044 | 0.3820 | 0.2818 | 0.382 |
| $a+b/\sqrt{y}\sqrt{z}+cx/z$ | 164.22 | 112.92 | 0.672 | 0.0940 | 0.0685 | 0.5640 | 0.2970 | 0.1894 | 0.626 |
| $a+b/\sqrt{y}\sqrt{z}+cx/z^2$ | 168.59 | 119.52 | 0.654 | 0.0953 | 0.0703 | 0.5515 | 0.2971 | 0.1964 | 0.626 |
| $a+b/\sqrt{y}\sqrt{z}+cx/\sqrt{z}$ | 166.81 | 115.60 | 0.661 | 0.0948 | 0.0694 | 0.5567 | 0.2976 | 0.1948 | 0.625 |
| $a+b/\sqrt{y}\sqrt{z}+cxz$ | 116.43 | 88.05 | 0.835 | 0.0707 | 0.0449 | 0.7532 | 0.2440 | 0.1477 | 0.748 |
| $a+b/\sqrt{y}\sqrt{z}+cxz^2$ | 118.44 | 88.21 | 0.829 | 0.0731 | 0.0487 | 0.7363 | 0.2502 | 0.1551 | 0.735 |
| $a+b/\sqrt{y}\sqrt{z}+cx\sqrt{z}$ | 116.28 | 90.03 | 0.836 | 0.0696 | 0.0445 | 0.7609 | 0.2374 | 0.1445 | 0.761 |
| $a+b/\sqrt{y}\sqrt{z}+cx^2/z$ | 169.26 | 119.63 | 0.651 | 0.0952 | 0.0699 | 0.5522 | 0.2966 | 0.1999 | 0.627 |
| $a+b/\sqrt{y}\sqrt{z}+cx^2/z^2$ | 169.06 | 119.84 | 0.652 | 0.0953 | 0.0702 | 0.5515 | 0.2966 | 0.1973 | 0.627 |
| $a+b/\sqrt{y}\sqrt{z}+cx^2/\sqrt{z}$ | 161.17 | 119.50 | 0.684 | 0.0924 | 0.0703 | 0.5788 | 0.2803 | 0.1987 | 0.667 |
| $a+b/\sqrt{y}\sqrt{z}+cx^2z$ | 114.06 | 87.14 | 0.842 | 0.0725 | 0.0495 | 0.7406 | 0.2462 | 0.1537 | 0.743 |
| $a+b/\sqrt{y}\sqrt{z}+cx^2z^2$ | 116.76 | 86.45 | 0.834 | 0.0744 | 0.0510 | 0.7265 | 0.2518 | 0.1607 | 0.731 |
| $a+b/\sqrt{y}\sqrt{z}+cx^2\sqrt{z}$ | 113.46 | 89.56 | 0.843 | 0.0723 | 0.0493 | 0.7417 | 0.2426 | 0.1504 | 0.751 |
| $a+b/\sqrt{y}\sqrt{z}+c\sqrt{x}/z$ | 161.64 | 109.91 | 0.682 | 0.0937 | 0.0686 | 0.5668 | 0.2959 | 0.1885 | 0.629 |
| $a+b/\sqrt{y}\sqrt{z}+c\sqrt{x}/z^2$ | 168.67 | 119.73 | 0.654 | 0.0953 | 0.0704 | 0.5516 | 0.2969 | 0.1961 | 0.626 |
| $a+b/\sqrt{y}\sqrt{z}+c\sqrt{x}/\sqrt{z}$ | 159.15 | 107.29 | 0.692 | 0.0929 | 0.0674 | 0.5737 | 0.2949 | 0.1860 | 0.632 |
| $a+b/\sqrt{y}\sqrt{z}+c\sqrt{x}z$ | 120.23 | 92.06 | 0.824 | 0.0708 | 0.0435 | 0.7523 | 0.2458 | 0.1460 | 0.744 |
| $a+b/\sqrt{y}\sqrt{z}+c\sqrt{x}z^2$ | 120.48 | 90.75 | 0.823 | 0.0729 | 0.0473 | 0.7378 | 0.2505 | 0.1547 | 0.734 |
| $a+b/\sqrt{y}\sqrt{z}+c\sqrt{x}\sqrt{z}$ | 122.05 | 91.89 | 0.819 | 0.0691 | 0.0419 | 0.7641 | 0.2392 | 0.1418 | 0.757 |
| $a+b/\sqrt{y}\sqrt{z}+c/xz$ | 153.86 | 108.12 | 0.712 | 0.0943 | 0.0705 | 0.5612 | 0.2947 | 0.1921 | 0.632 |
| $a+b/\sqrt{y}\sqrt{z}+c/xz^2$ | 139.18 | 95.31 | 0.764 | 0.0888 | 0.0629 | 0.6102 | 0.2817 | 0.1775 | 0.664 |
| $a+b/\sqrt{y}\sqrt{z}+c/x\sqrt{z}$ | 157.39 | 109.75 | 0.699 | 0.0949 | 0.0709 | 0.5552 | 0.2963 | 0.1934 | 0.628 |
| $a+b/\sqrt{y}\sqrt{z}+cz/x$ | 157.04 | 109.15 | 0.700 | 0.0948 | 0.0708 | 0.5562 | 0.2960 | 0.1934 | 0.629 |
| $a+b/\sqrt{y}\sqrt{z}+cz^2/x$ | 141.51 | 102.15 | 0.756 | 0.0902 | 0.0658 | 0.5982 | 0.2854 | 0.1815 | 0.655 |
| $a+b/\sqrt{y}\sqrt{z}+c\sqrt{z}/x$ | 159.08 | 110.04 | 0.692 | 0.0951 | 0.0708 | 0.5534 | 0.2968 | 0.1936 | 0.627 |
| $a+b/\sqrt{y}\sqrt{z}+c/x^2z$ | 158.51 | 110.06 | 0.694 | 0.0951 | 0.0709 | 0.5532 | 0.2967 | 0.1940 | 0.627 |
| $a+b/\sqrt{y}\sqrt{z}+c/x^2z^2$ | 155.60 | 108.84 | 0.705 | 0.0947 | 0.0709 | 0.5570 | 0.2955 | 0.1936 | 0.630 |
| $a+b/\sqrt{y}\sqrt{z}+c/x^2\sqrt{z}$ | 159.40 | 110.26 | 0.691 | 0.0952 | 0.0708 | 0.5524 | 0.2969 | 0.1939 | 0.626 |
| $a+b/\sqrt{y}\sqrt{z}+cz/x^2$ | 160.72 | 110.79 | 0.686 | 0.0953 | 0.0705 | 0.5517 | 0.2973 | 0.1935 | 0.626 |
| $a+b/\sqrt{y}\sqrt{z}+cz^2/x^2$ | 160.57 | 110.71 | 0.686 | 0.0953 | 0.0706 | 0.5518 | 0.2972 | 0.1936 | 0.626 |
| $a+b/\sqrt{y}\sqrt{z}+c\sqrt{z}/x^2$ | 160.46 | 110.70 | 0.687 | 0.0953 | 0.0706 | 0.5518 | 0.2972 | 0.1936 | 0.626 |
| $a+b/\sqrt{y}\sqrt{z}+c/\sqrt{x}z$ | 150.43 | 107.35 | 0.725 | 0.0932 | 0.0685 | 0.5715 | 0.2925 | 0.1889 | 0.638 |
| $a+b/\sqrt{y}\sqrt{z}+c/\sqrt{x}z^2$ | 152.42 | 108.64 | 0.717 | 0.0833 | 0.0563 | 0.6573 | 0.2667 | 0.1593 | 0.699 |
| $a+b/\sqrt{y}\sqrt{z}+c/\sqrt{x}\sqrt{z}$ | 160.42 | 110.95 | 0.687 | 0.0952 | 0.0706 | 0.5525 | 0.2974 | 0.1926 | 0.625 |
| $a+b/\sqrt{y}\sqrt{z}+cz/\sqrt{x}$ | 141.22 | 101.45 | 0.757 | 0.0889 | 0.0634 | 0.6097 | 0.2836 | 0.1790 | 0.659 |
| $a+b/\sqrt{y}\sqrt{z}+cz^2/\sqrt{x}$ | 124.38 | 90.79 | 0.812 | 0.0773 | 0.0508 | 0.7053 | 0.2599 | 0.1622 | 0.714 |
| $a+b/\sqrt{y}\sqrt{z}+c\sqrt{z}/\sqrt{x}$ | 154.51 | 106.84 | 0.710 | 0.0939 | 0.0699 | 0.5647 | 0.2944 | 0.1907 | 0.633 |
| $a+bz/\sqrt{y}+cx/z$ | 140.78 | 108.12 | 0.759 | 0.0766 | 0.0570 | 0.7101 | 0.2672 | 0.2044 | 0.698 |
| $a+bz/\sqrt{y}+cx/z^2$ | 175.40 | 134.71 | 0.626 | 0.0918 | 0.0663 | 0.5838 | 0.3357 | 0.2457 | 0.523 |
| *** $a+bz/\sqrt{y}+cx/\sqrt{z}$** | 111.48 | 85.13 | 0.849 | 0.0677 | 0.0449 | 0.7734 | **0.2184** | **0.1369** | **0.798** |
| $a+bz/\sqrt{y}+cxz$ | 128.30 | 96.33 | 0.800 | 0.0731 | 0.0524 | 0.7359 | 0.2684 | 0.2038 | 0.695 |
| $a+bz/\sqrt{y}+cxz^2$ | 154.87 | 115.71 | 0.708 | 0.0848 | 0.0648 | 0.6451 | 0.3175 | 0.2469 | 0.573 |
| $a+bz/\sqrt{y}+cx\sqrt{z}$ | 116.05 | 89.49 | 0.836 | 0.0693 | 0.0442 | 0.7626 | 0.2415 | 0.1609 | 0.753 |
| $a+bz/\sqrt{y}+cx^2/z$ | 111.84 | 84.44 | 0.848 | 0.0710 | 0.0476 | 0.7509 | 0.2302 | 0.1563 | 0.775 |
| $a+bz/\sqrt{y}+cx^2/z^2$ | 164.18 | 128.36 | 0.672 | 0.0875 | 0.0633 | 0.6222 | 0.3148 | 0.2369 | 0.580 |

(continued on next page)

**Table 4 – continued from previous page**

| Functional form | $T_{eff}$ (K) | | | Radius ($R_\odot$) | | | log (L/$L_\odot$) | | |
|---|---|---|---|---|---|---|---|---|---|
| | RMSE | MAD | $R^2_{ap}$ | RMSE | MAD | $R^2_{ap}$ | RMSE | MAD | $R^2_{ap}$ |
| $a+bz/\sqrt{y}+cx^2/\sqrt{z}$ | 104.04 | 78.63 | 0.868 | 0.0698 | 0.0461 | 0.7592 | 0.2266 | 0.1492 | 0.783 |
| $a+bz/\sqrt{y}+cx^2z$ | 136.97 | 101.51 | 0.772 | 0.0792 | 0.0606 | 0.6903 | 0.2930 | 0.2341 | 0.636 |
| $a+bz/\sqrt{y}+cx^2z^2$ | 157.06 | 114.87 | 0.700 | 0.0874 | 0.0668 | 0.6224 | 0.3254 | 0.2511 | 0.551 |
| $a+bz/\sqrt{y}+cx^2\sqrt{z}$ | 122.26 | 91.37 | 0.818 | 0.0743 | 0.0538 | 0.7276 | 0.2672 | 0.2033 | 0.698 |
| $a+bz/\sqrt{y}+c\sqrt{x}/z$ | 169.53 | 132.56 | 0.650 | 0.0873 | 0.0668 | 0.6237 | 0.3202 | 0.2459 | 0.566 |
| $a+bz/\sqrt{y}+c\sqrt{x}/z^2$ | 180.48 | 138.77 | 0.604 | 0.0948 | 0.0685 | 0.5559 | 0.3474 | 0.2528 | 0.489 |
| $a+bz/\sqrt{y}+c\sqrt{x}/\sqrt{z}$ | 132.10 | 103.60 | 0.788 | 0.0706 | 0.0516 | 0.7542 | 0.2427 | 0.1746 | 0.750 |
| $a+bz/\sqrt{y}+c\sqrt{x}z$ | 128.51 | 99.20 | 0.799 | 0.0715 | 0.0478 | 0.7478 | 0.2606 | 0.1874 | 0.712 |
| $a+bz/\sqrt{y}+c\sqrt{x}z^2$ | 154.82 | 117.20 | 0.708 | 0.0836 | 0.0636 | 0.6550 | 0.3139 | 0.2432 | 0.583 |
| $a+bz/\sqrt{y}+c\sqrt{x}\sqrt{z}$ | 120.98 | 94.27 | 0.822 | 0.0695 | 0.0407 | 0.7618 | 0.2398 | 0.1484 | 0.756 |
| $a+bz/\sqrt{y}+c/xz$ | 145.66 | 116.83 | 0.742 | 0.0752 | 0.0522 | 0.7205 | 0.2627 | 0.1815 | 0.708 |
| $a+bz/\sqrt{y}+c/xz^2$ | 141.91 | 110.19 | 0.755 | 0.0789 | 0.0574 | 0.6923 | 0.2676 | 0.1802 | 0.697 |
| $a+bz/\sqrt{y}+c/x\sqrt{z}$ | 149.41 | 119.57 | 0.728 | 0.0750 | 0.0538 | 0.7220 | 0.2668 | 0.1879 | 0.698 |
| $a+bz/\sqrt{y}+cz/x$ | 159.45 | 123.97 | 0.691 | 0.0774 | 0.0576 | 0.7044 | 0.2840 | 0.2031 | 0.658 |
| $a+bz/\sqrt{y}+cz^2/x$ | 166.09 | 127.57 | 0.664 | 0.0812 | 0.0608 | 0.6746 | 0.2963 | 0.2127 | 0.628 |
| $a+bz/\sqrt{y}+c\sqrt{z}/x$ | 156.55 | 122.87 | 0.702 | 0.0764 | 0.0565 | 0.7121 | 0.2785 | 0.1989 | 0.671 |
| $a+bz/\sqrt{y}+c/x^2z$ | 159.47 | 124.48 | 0.691 | 0.0777 | 0.0575 | 0.7019 | 0.2843 | 0.2024 | 0.658 |
| $a+bz/\sqrt{y}+c/x^2z^2$ | 154.51 | 122.55 | 0.710 | 0.0764 | 0.0558 | 0.7114 | 0.2757 | 0.1957 | 0.678 |
| $a+bz/\sqrt{y}+c/x^2\sqrt{z}$ | 161.25 | 124.93 | 0.684 | 0.0783 | 0.0580 | 0.6972 | 0.2877 | 0.2045 | 0.649 |
| $a+bz/\sqrt{y}+cz/x^2$ | 164.55 | 125.51 | 0.671 | 0.0796 | 0.0589 | 0.6868 | 0.2947 | 0.2083 | 0.632 |
| $a+bz/\sqrt{y}+cz^2/x^2$ | 165.66 | 125.69 | 0.666 | 0.0802 | 0.0591 | 0.6826 | 0.2971 | 0.2095 | 0.626 |
| $a+bz/\sqrt{y}+c\sqrt{z}/x^2$ | 163.72 | 125.36 | 0.674 | 0.0793 | 0.0587 | 0.6896 | 0.2929 | 0.2074 | 0.637 |
| $a+bz/\sqrt{y}+c/\sqrt{x}z$ | 138.84 | 108.09 | 0.765 | 0.0783 | 0.0548 | 0.6976 | 0.2626 | 0.1690 | 0.708 |
| $a+bz/\sqrt{y}+c/\sqrt{x}z^2$ | 151.68 | 115.67 | 0.720 | 0.0884 | 0.0622 | 0.6144 | 0.3009 | 0.2015 | 0.616 |
| $a+bz/\sqrt{y}+c/\sqrt{x}\sqrt{z}$ | 139.08 | 111.53 | 0.765 | 0.0744 | 0.0508 | 0.7264 | 0.2543 | 0.1692 | 0.726 |
| $a+bz/\sqrt{y}+cz/\sqrt{x}$ | 161.48 | 124.99 | 0.683 | 0.0782 | 0.0601 | 0.6977 | 0.2853 | 0.2129 | 0.655 |
| $a+bz/\sqrt{y}+cz^2/\sqrt{x}$ | 175.29 | 131.76 | 0.626 | 0.0949 | 0.0673 | 0.5556 | 0.3478 | 0.2515 | 0.487 |
| $a+bz/\sqrt{y}+c\sqrt{z}/\sqrt{x}$ | 151.33 | 119.56 | 0.721 | 0.0742 | 0.0550 | 0.7283 | 0.2683 | 0.1941 | 0.695 |
| $a+bz^2/\sqrt{y}+cx/z$ | 150.82 | 118.72 | 0.723 | 0.0785 | 0.0590 | 0.6959 | 0.2874 | 0.2265 | 0.650 |
| $a+bz^2/\sqrt{y}+cx/z^2$ | 162.54 | 123.36 | 0.679 | 0.0850 | 0.0623 | 0.6437 | 0.3182 | 0.2449 | 0.571 |
| $a+bz^2/\sqrt{y}+cx/\sqrt{z}$ | 125.90 | 97.45 | 0.807 | 0.0696 | 0.0447 | 0.7611 | 0.2400 | 0.1655 | 0.756 |
| $a+bz^2/\sqrt{y}+cxz$ | 125.61 | 95.43 | 0.808 | 0.0728 | 0.0514 | 0.7381 | 0.2634 | 0.1935 | 0.706 |
| $a+bz^2/\sqrt{y}+cxz^2$ | 156.28 | 117.77 | 0.703 | 0.0844 | 0.0635 | 0.6481 | 0.3168 | 0.2436 | 0.575 |
| $a+bz^2/\sqrt{y}+cx\sqrt{z}$ | 116.83 | 89.43 | 0.834 | 0.0692 | 0.0446 | 0.7636 | 0.2410 | 0.1589 | 0.754 |
| $a+bz^2/\sqrt{y}+cx^2/z$ | 124.68 | 94.20 | 0.811 | 0.0711 | 0.0475 | 0.7504 | 0.2461 | 0.1753 | 0.743 |
| $a+bz^2/\sqrt{y}+cx^2/z^2$ | 158.83 | 125.25 | 0.693 | 0.0828 | 0.0623 | 0.6613 | 0.3078 | 0.2463 | 0.599 |
| $a+bz^2/\sqrt{y}+cx^2/\sqrt{z}$ | 108.68 | 83.40 | 0.856 | 0.0678 | 0.0442 | 0.7731 | 0.2290 | 0.1559 | 0.778 |
| $a+bz^2/\sqrt{y}+cx^2z$ | 138.05 | 102.52 | 0.768 | 0.0790 | 0.0606 | 0.6915 | 0.2933 | 0.2345 | 0.635 |
| $a+bz^2/\sqrt{y}+cx^2z^2$ | 157.80 | 118.63 | 0.697 | 0.0853 | 0.0627 | 0.6411 | 0.3195 | 0.2434 | 0.568 |
| $a+bz^2/\sqrt{y}+cx^2\sqrt{z}$ | 123.40 | 92.90 | 0.815 | 0.0739 | 0.0541 | 0.7301 | 0.2674 | 0.2036 | 0.697 |
| $a+bz^2/\sqrt{y}+c\sqrt{x}/z$ | 162.03 | 124.43 | 0.681 | 0.0839 | 0.0630 | 0.6522 | 0.3146 | 0.2460 | 0.581 |
| $a+bz^2/\sqrt{y}+c\sqrt{x}/z^2$ | 161.53 | 123.83 | 0.683 | 0.0858 | 0.0635 | 0.6369 | 0.3209 | 0.2477 | 0.564 |
| $a+bz^2/\sqrt{y}+c\sqrt{x}/\sqrt{z}$ | 147.31 | 117.36 | 0.736 | 0.0756 | 0.0547 | 0.7175 | 0.2754 | 0.2065 | 0.679 |
| $a+bz^2/\sqrt{y}+c\sqrt{x}z$ | 124.78 | 95.65 | 0.811 | 0.0709 | 0.0450 | 0.7515 | 0.2525 | 0.1676 | 0.730 |
| $a+bz^2/\sqrt{y}+c\sqrt{x}z^2$ | 155.40 | 117.47 | 0.706 | 0.0836 | 0.0636 | 0.6548 | 0.3140 | 0.2439 | 0.582 |
| $a+bz^2/\sqrt{y}+c\sqrt{x}\sqrt{z}$ | 121.42 | 93.64 | 0.821 | 0.0692 | 0.0408 | 0.7636 | 0.2396 | 0.1444 | 0.757 |
| $a+bz^2/\sqrt{y}+c/xz$ | 145.43 | 109.52 | 0.743 | 0.0737 | 0.0512 | 0.7319 | 0.2660 | 0.1842 | 0.700 |
| $a+bz^2/\sqrt{y}+c/xz^2$ | 137.12 | 101.59 | 0.771 | 0.0741 | 0.0513 | 0.7289 | 0.2602 | 0.1691 | 0.713 |
| $a+bz^2/\sqrt{y}+c/x\sqrt{z}$ | 149.53 | 112.80 | 0.728 | 0.0744 | 0.0527 | 0.7265 | 0.2724 | 0.1925 | 0.686 |
| $a+bz^2/\sqrt{y}+cz/x$ | 156.92 | 116.95 | 0.700 | 0.0772 | 0.0554 | 0.7058 | 0.2893 | 0.2091 | 0.645 |
| $a+bz^2/\sqrt{y}+cz^2/x$ | 157.83 | 116.70 | 0.697 | 0.0776 | 0.0552 | 0.7028 | 0.2920 | 0.2091 | 0.639 |
| $a+bz^2/\sqrt{y}+c\sqrt{z}/x$ | 155.28 | 116.46 | 0.707 | 0.0764 | 0.0548 | 0.7119 | 0.2849 | 0.2055 | 0.656 |
| $a+bz^2/\sqrt{y}+c/x^2z$ | 156.57 | 116.63 | 0.702 | 0.0771 | 0.0556 | 0.7068 | 0.2880 | 0.2080 | 0.649 |
| $a+bz^2/\sqrt{y}+c/x^2z^2$ | 153.47 | 115.54 | 0.713 | 0.0759 | 0.0544 | 0.7152 | 0.2811 | 0.2011 | 0.665 |
| $a+bz^2/\sqrt{y}+c/x^2\sqrt{z}$ | 157.55 | 116.88 | 0.698 | 0.0775 | 0.0559 | 0.7034 | 0.2906 | 0.2101 | 0.642 |
| $a+bz^2/\sqrt{y}+cz/x^2$ | 159.16 | 117.07 | 0.692 | 0.0784 | 0.0564 | 0.6964 | 0.2953 | 0.2134 | 0.630 |
| $a+bz^2/\sqrt{y}+cz^2/x^2$ | 159.61 | 117.08 | 0.690 | 0.0787 | 0.0565 | 0.6942 | 0.2969 | 0.2142 | 0.627 |
| $a+bz^2/\sqrt{y}+c\sqrt{z}/x^2$ | 158.78 | 117.04 | 0.693 | 0.0782 | 0.0563 | 0.6982 | 0.2941 | 0.2126 | 0.633 |
| $a+bz^2/\sqrt{y}+c/\sqrt{x}z$ | 131.99 | 100.26 | 0.788 | 0.0728 | 0.0490 | 0.7381 | 0.2523 | 0.1596 | 0.730 |
| $a+bz^2/\sqrt{y}+c/\sqrt{x}z^2$ | 133.46 | 97.37 | 0.783 | 0.0782 | 0.0546 | 0.6978 | 0.2739 | 0.1814 | 0.682 |
| $a+bz^2/\sqrt{y}+c/\sqrt{x}\sqrt{z}$ | 137.89 | 103.53 | 0.769 | 0.0719 | 0.0480 | 0.7446 | 0.2539 | 0.1690 | 0.727 |
| $a+bz^2/\sqrt{y}+cz/\sqrt{x}$ | 157.94 | 118.94 | 0.696 | 0.0782 | 0.0553 | 0.6980 | 0.2938 | 0.2111 | 0.634 |
| $a+bz^2/\sqrt{y}+cz^2/\sqrt{x}$ | 157.85 | 116.51 | 0.697 | 0.0772 | 0.0579 | 0.7057 | 0.2893 | 0.2118 | 0.645 |
| $a+bz^2/\sqrt{y}+c\sqrt{z}/\sqrt{x}$ | 153.46 | 116.85 | 0.713 | 0.0758 | 0.0536 | 0.7166 | 0.2815 | 0.2021 | 0.664 |
| $a+b\sqrt{z}/\sqrt{y}+cx/z$ | 260.39 | 194.27 | 0.175 | 0.1323 | 0.1035 | 0.1362 | 0.4559 | 0.3500 | 0.119 |
| $a+b\sqrt{z}/\sqrt{y}+cx/z^2$ | 269.43 | 192.24 | 0.117 | 0.1376 | 0.1047 | 0.0653 | 0.4782 | 0.3591 | 0.031 |
| $a+b\sqrt{z}/\sqrt{y}+cx/\sqrt{z}$ | 133.53 | 105.40 | 0.783 | 0.0813 | 0.0628 | 0.6738 | 0.2477 | 0.1827 | 0.740 |
| $a+b\sqrt{z}/\sqrt{y}+cxz$ | 127.81 | 96.40 | 0.801 | 0.0725 | 0.0507 | 0.7404 | 0.2640 | 0.1935 | 0.705 |
| $a+b\sqrt{z}/\sqrt{y}+cxz^2$ | 155.82 | 117.05 | 0.705 | 0.0843 | 0.0649 | 0.6493 | 0.3129 | 0.2434 | 0.585 |
| $a+b\sqrt{z}/\sqrt{y}+cx\sqrt{z}$ | 115.93 | 89.80 | 0.836 | 0.0695 | 0.0445 | 0.7615 | 0.2412 | 0.1609 | 0.753 |
| $a+b\sqrt{z}/\sqrt{y}+cx^2/z$ | 177.57 | 137.79 | 0.616 | 0.1022 | 0.0784 | 0.4840 | 0.3279 | 0.2531 | 0.544 |
| $a+b\sqrt{z}/\sqrt{y}+cx^2/z^2$ | 272.29 | 192.87 | 0.098 | 0.1379 | 0.1031 | 0.0617 | 0.4800 | 0.3512 | 0.024 |
| $a+b\sqrt{z}/\sqrt{y}+cx^2/\sqrt{z}$ | 121.78 | 98.66 | 0.820 | 0.0807 | 0.0555 | 0.6786 | 0.2533 | 0.1804 | 0.728 |
| $a+b\sqrt{z}/\sqrt{y}+cx^2z$ | 137.98 | 105.73 | 0.768 | 0.0794 | 0.0602 | 0.6890 | 0.2899 | 0.2258 | 0.644 |
| $a+b\sqrt{z}/\sqrt{y}+cx^2z^2$ | 164.14 | 127.51 | 0.672 | 0.0904 | 0.0718 | 0.5968 | 0.3326 | 0.2624 | 0.531 |
| $a+b\sqrt{z}/\sqrt{y}+cx^2\sqrt{z}$ | 123.78 | 94.54 | 0.814 | 0.0751 | 0.0553 | 0.7217 | 0.2664 | 0.1995 | 0.699 |
| $a+b\sqrt{z}/\sqrt{y}+c\sqrt{x}/z$ | 256.72 | 183.22 | 0.198 | 0.1334 | 0.1003 | 0.1209 | 0.4619 | 0.3445 | 0.096 |
| $a+b\sqrt{z}/\sqrt{y}+c\sqrt{x}/z^2$ | 257.66 | 184.17 | 0.192 | 0.1341 | 0.1016 | 0.1117 | 0.4619 | 0.3482 | 0.096 |
| $a+b\sqrt{z}/\sqrt{y}+c\sqrt{x}/\sqrt{z}$ | 221.78 | 173.84 | 0.402 | 0.1114 | 0.0924 | 0.3871 | 0.3756 | 0.3098 | 0.402 |
| $a+b\sqrt{z}/\sqrt{y}+c\sqrt{x}z$ | 128.23 | 99.28 | 0.800 | 0.0711 | 0.0464 | 0.7504 | 0.2578 | 0.1834 | 0.718 |
| $a+b\sqrt{z}/\sqrt{y}+c\sqrt{x}z^2$ | 153.65 | 118.93 | 0.713 | 0.0819 | 0.0618 | 0.6686 | 0.3050 | 0.2339 | 0.606 |
| $a+b\sqrt{z}/\sqrt{y}+c\sqrt{x}\sqrt{z}$ | 120.85 | 93.98 | 0.822 | 0.0695 | 0.0411 | 0.7613 | 0.2398 | 0.1487 | 0.756 |
| $a+b\sqrt{z}/\sqrt{y}+c/xz$ | 176.43 | 138.59 | 0.621 | 0.0868 | 0.0643 | 0.6279 | 0.2961 | 0.2179 | 0.628 |
| $a+b\sqrt{z}/\sqrt{y}+c/xz^2$ | 173.71 | 126.28 | 0.633 | 0.0939 | 0.0708 | 0.5648 | 0.3082 | 0.2203 | 0.598 |
| $a+b\sqrt{z}/\sqrt{y}+c/x\sqrt{z}$ | 185.15 | 143.71 | 0.583 | 0.0876 | 0.0679 | 0.6215 | 0.3058 | 0.2305 | 0.604 |
| $a+b\sqrt{z}/\sqrt{y}+cz/x$ | 225.53 | 159.68 | 0.381 | 0.1035 | 0.0808 | 0.4715 | 0.3716 | 0.2719 | 0.415 |
| $a+b\sqrt{z}/\sqrt{y}+cz^2/x$ | 272.75 | 191.32 | 0.095 | 0.1373 | 0.1050 | 0.0698 | 0.4792 | 0.3571 | 0.027 |
| $a+b\sqrt{z}/\sqrt{y}+c\sqrt{z}/x$ | 209.15 | 153.85 | 0.468 | 0.0956 | 0.0752 | 0.5485 | 0.3431 | 0.2552 | 0.501 |
| $a+b\sqrt{z}/\sqrt{y}+c/x^2z$ | 214.42 | 157.35 | 0.441 | 0.0981 | 0.0770 | 0.5244 | 0.3527 | 0.2608 | 0.473 |
| $a+b\sqrt{z}/\sqrt{y}+c/x^2z^2$ | 200.50 | 152.89 | 0.511 | 0.0930 | 0.0734 | 0.5726 | 0.3300 | 0.2497 | 0.538 |
| $a+b\sqrt{z}/\sqrt{y}+c/x^2\sqrt{z}$ | 219.56 | 158.44 | 0.413 | 0.1004 | 0.0780 | 0.5026 | 0.3617 | 0.2641 | 0.446 |
| $a+b\sqrt{z}/\sqrt{y}+cz/x^2$ | 229.53 | 159.75 | 0.359 | 0.1051 | 0.0804 | 0.4541 | 0.3800 | 0.2703 | 0.388 |

(continued on next page)

**Table 4 – continued from previous page**

| Functional form | $T_{eff}$ (K) | | | Radius ($R_{\odot}$) | | | log (L/$L_{\odot}$) | | |
|---|---|---|---|---|---|---|---|---|---|
| | RMSE | MAD | $R^2_{ap}$ | RMSE | MAD | $R^2_{ap}$ | RMSE | MAD | $R^2_{ap}$ |
| a+b$\sqrt{z}/\sqrt{y}$+c$z^2/x^2$ | 234.24 | 160.26 | 0.332 | 0.1076 | 0.0817 | 0.4278 | 0.3888 | 0.2744 | 0.359 |
| a+b$\sqrt{z}/\sqrt{y}$+c$\sqrt{z}/x^2$ | 226.88 | 159.49 | 0.374 | 0.1038 | 0.0798 | 0.4679 | 0.3750 | 0.2683 | 0.404 |
| a+b$\sqrt{z}/\sqrt{y}$+c/$\sqrt{x}$z | 160.97 | 118.12 | 0.685 | 0.0888 | 0.0635 | 0.6103 | 0.2885 | 0.1906 | 0.647 |
| a+b$\sqrt{z}/\sqrt{y}$+c/$\sqrt{x}z^2$ | 190.36 | 133.82 | 0.559 | 0.1076 | 0.0784 | 0.4288 | 0.3513 | 0.2450 | 0.477 |
| a+b$\sqrt{z}/\sqrt{y}$+c/$\sqrt{x}\sqrt{z}$ | 158.50 | 124.31 | 0.694 | 0.0823 | 0.0577 | 0.6652 | 0.2737 | 0.1889 | 0.683 |
| a+b$\sqrt{z}/\sqrt{y}$+cz/$\sqrt{x}$ | 256.77 | 186.99 | 0.198 | 0.1360 | 0.0989 | 0.0866 | 0.4725 | 0.3405 | 0.054 |
| a+b$\sqrt{z}/\sqrt{y}$+c$z^2/\sqrt{x}$ | 159.78 | 133.41 | 0.689 | 0.0868 | 0.0644 | 0.6282 | 0.3177 | 0.2463 | 0.572 |
| a+b$\sqrt{z}/\sqrt{y}$+c$\sqrt{z}/\sqrt{x}$ | 214.51 | 156.44 | 0.440 | 0.0985 | 0.0788 | 0.5208 | 0.3498 | 0.2656 | 0.481 |
